# Supplementary material for: Dispersionless integrable systems in 3D and Einstein-Weyl geometry
Source: arXiv:1208.2728 ancillary file (2013-05-09)
Supplement: Supplementary file 1 [file BKEF-2012-I-divergense_quasilinear_integrability.pdf]

This is the worksheet accompanying the paper E.Ferapontov & B.Kruglikov "Dispersionless integrable systems in 3D and Einstein-Weyl geometry".

The file ran on **Maple** version 16, the package **DifferentialGeometry** was used.

We are going to attack the general 2nd order PDE  $a(u)_{xx}+b(u)_{yy}+c(u)_{zz}+2p(u)_{xy}+2q(u)_{xt}+2r(u)_{yt}=0$  and check if the corresponding conformal metric is EW

>

> with(DifferentialGeometry) : with(Tensor) : with(Tools) : with(JetCalculus) :  
with(LinearAlgebra) : with(PDEtools, D\_Dx, declare, ToJet, FromJet) :

> DGsetup([t, x, y], [u], J2) :

> F := TotalDiff(a(u[]), [2, 2]) + TotalDiff(b(u[]), [3, 3]) + TotalDiff(c(u[]), [1, 1]) + 2  
· TotalDiff(p(u[]), [2, 3]) + 2· TotalDiff(q(u[]), [1, 2]) + 2· TotalDiff(r(u[]), [1, 3])

$$F := \left( \frac{d^2}{du^2} a(u) \right) u_2^2 + \left( \frac{d}{du} a(u) \right) u_{2,2} + \left( \frac{d^2}{du^2} b(u) \right) u_3^2 \quad (1)$$

$$+ \left( \frac{d}{du} b(u) \right) u_{3,3} + \left( \frac{d^2}{du^2} c(u) \right) u_1^2 + \left( \frac{d}{du} c(u) \right) u_{1,1}$$

$$+ 2 \left( \frac{d^2}{du^2} p(u) \right) u_2 u_3 + 2 \left( \frac{d}{du} p(u) \right) u_{2,3} + 2 \left( \frac{d^2}{du^2} q(u) \right) u_1 u_2$$

$$+ 2 \left( \frac{d}{du} q(u) \right) u_{1,2} + 2 \left( \frac{d^2}{du^2} r(u) \right) u_1 u_3 + 2 \left( \frac{d}{du} r(u) \right) u_{1,3}$$

Let us for simplicity assume that  $c(u)$  is not constant, and change the variables  $u \rightarrow c(u)$ .

This is only a local in  $J^0$  transformation, but for our purposes this does not reduce the generality.

> F := TotalDiff(a(u[]), [2, 2]) + TotalDiff(b(u[]), [3, 3]) + TotalDiff(u[], [1, 1]) + 2  
· TotalDiff(p(u[]), [2, 3]) + 2· TotalDiff(q(u[]), [1, 2]) + 2· TotalDiff(r(u[]), [1, 3])

$$F := \left( \frac{d^2}{du^2} a(u) \right) u_2^2 + \left( \frac{d}{du} a(u) \right) u_{2,2} + \left( \frac{d^2}{du^2} b(u) \right) u_3^2 \quad (2)$$

$$+ \left( \frac{d}{du} b(u) \right) u_{3,3} + u_{1,1} + 2 \left( \frac{d^2}{du^2} p(u) \right) u_2 u_3 + 2 \left( \frac{d}{du} p(u) \right) u_{2,3}$$

$$+ 2 \left( \frac{d^2}{du^2} q(u) \right) u_1 u_2 + 2 \left( \frac{d}{du} q(u) \right) u_{1,2} + 2 \left( \frac{d^2}{du^2} r(u) \right) u_1 u_3$$

$$+ 2 \left( \frac{d}{du} r(u) \right) u_{1,3}$$

> A := Matrix( [[diff(F, u[1, 1]), 1/2 diff(F, u[1, 2]), 1/2 diff(F, u[1, 3])], [1/2 diff(F, u[1, 2]), diff(F, u[2, 2]), 1/2 diff(F, u[2, 3])], [1/2 diff(F, u[1, 3]), 1/2 diff(F, u[2, 3]), diff(F, u[3, 3])]] ); AA := expand(MatrixInverse(A)) : AM := simplify(Determinant(A) · AA) :

$$A := \begin{bmatrix} 1 & \frac{d}{du_{[]}} q(u_{[]}) & \frac{d}{du_{[]}} r(u_{[]}) \\ \frac{d}{du_{[]}} q(u_{[]}) & \frac{d}{du_{[]}} a(u_{[]}) & \frac{d}{du_{[]}} p(u_{[]}) \\ \frac{d}{du_{[]}} r(u_{[]}) & \frac{d}{du_{[]}} p(u_{[]}) & \frac{d}{du_{[]}} b(u_{[]}) \end{bmatrix} \quad (3)$$

**J2** >  $DDA := Matrix\left(\left[\left[0, \frac{d^2}{du_{[]}^2} q(u_{[]}), \frac{d^2}{du_{[]}^2} r(u_{[]})\right], \left[\frac{d^2}{du_{[]}^2} q(u_{[]}), \frac{d^2}{du_{[]}^2} a(u_{[]}), \frac{d^2}{du_{[]}^2} p(u_{[]})\right], \left[\frac{d^2}{du_{[]}^2} r(u_{[]}), \frac{d^2}{du_{[]}^2} p(u_{[]}), \frac{d^2}{du_{[]}^2} b(u_{[]})\right]\right):$

**J2** >  $VA := simplify(-2 \cdot AA.DDA):$

>  $DepVars := [u(t, x, y)]: AJ := FromJet(AM, DepVars); VJ := FromJet(VA, DepVars):$   
 $AJ := [[D(a)(u(t, x, y)) D(b)(u(t, x, y)) - D(p)(u(t, x, y))^2, -D(q)(u(t, x, y)) D(b)(u(t, x, y)) + D(r)(u(t, x, y)) D(p)(u(t, x, y)), D(q)(u(t, x, y)) D(p)(u(t, x, y)) - D(r)(u(t, x, y)) D(a)(u(t, x, y))],$   
 $[-D(q)(u(t, x, y)) D(b)(u(t, x, y)) + D(r)(u(t, x, y)) D(p)(u(t, x, y)), D(b)(u(t, x, y)) - D(r)(u(t, x, y))^2, -D(p)(u(t, x, y)) + D(r)(u(t, x, y)) D(q)(u(t, x, y))],$   
 $[D(q)(u(t, x, y)) D(p)(u(t, x, y)) - D(r)(u(t, x, y)) D(a)(u(t, x, y)), -D(p)(u(t, x, y)) + D(r)(u(t, x, y)) D(q)(u(t, x, y)), D(a)(u(t, x, y)) - D(q)(u(t, x, y))^2]]$  (4)

Here A is the matrix of the linearized operator (bivector=metric with upper indices),  
AA - the inverse (metric, which we remember is defined only up to conformal rescaling)  
and AM=AJ the adjoint matrix (which we use as a representative for the conformal class).

>  
>  $DGsetup([t, x, y], M):$   
>  $g := evalDG(AJ[1, 1] \cdot dt \& t \& t dt + AJ[1, 2] \cdot dt \& t dx + AJ[1, 3] \cdot dt \& t dy + AJ[2, 1] \cdot dx \& t dt + AJ[2, 2] \cdot dx \& t dx + AJ[2, 3] \cdot dx \& t dy + AJ[3, 1] \cdot dy \& t dt + AJ[3, 2] \cdot dy \& t dx + AJ[3, 3] \cdot dy \& t dy):$   
>  $C := Connection(a000 \cdot dt \& t D\_t \& t dt + a111 \cdot dx \& t D\_x \& t dx + a222 \cdot dy \& t D\_y \& t dy + a001 \cdot (dt \& t D\_t \& t dx + dx \& t D\_t \& t dt) + a002 \cdot (dt \& t D\_t \& t dy + dy \& t D\_t \& t dt) + a102 \cdot (dx \& t D\_t \& t dy + dy \& t D\_t \& t dx) + a011 \cdot (dt \& t D\_x \& t dx + dx \& t D\_x \& t dt) + a012 \cdot (dt \& t D\_x \& t dy + dy \& t D\_x \& t dt) + a112 \cdot (dx \& t D\_x \& t dy + dy \& t D\_x \& t dx) + a021 \cdot (dt \& t D\_y \& t dx + dx \& t D\_y \& t dt) + a022 \cdot (dt \& t D\_y \& t dy + dy \& t D\_y \& t dt) + a122 \cdot (dx \& t D\_y \& t dy + dy \& t D\_y \& t dx) + a010 \cdot dt \& t D\_x \& t dt + a121 \cdot dx \& t D\_y \& t dx + a202 \cdot dy \& t D\_t \& t dy + a020 \cdot dt \& t D\_y \& t dt + a101 \cdot dx \& t D\_t \& t dx + a212 \cdot dy \& t D\_x \& t dy):$   
>  $TorsionTensor(C);$

$$0 \ dt \ D\_t \ dt \quad (5)$$

VA=VJ is the set from which we compose the coefficients of the covector  $-\omega = U1 \cdot dt + U2 \cdot dx + U3 \cdot dy$ .

The source of minus is historical. We started with the negative sign of the covector and then changed to the standard convention.

We also omit in this version search for the coefficients  $U[i]$  in general form, we already

use the established formula, which in this version is

```
> U1 := x11(u(t, x, y)) · diff(u(t, x, y), t) + x12(u(t, x, y)) · diff(u(t, x, y), x) + x13(u(t, x, y))
    · diff(u(t, x, y), y) :
U2 := x21(u(t, x, y)) · diff(u(t, x, y), t) + x22(u(t, x, y)) · diff(u(t, x, y), x) + x23(u(t, x, y))
    · diff(u(t, x, y), y) :
U3 := x31(u(t, x, y)) · diff(u(t, x, y), t) + x32(u(t, x, y)) · diff(u(t, x, y), x) + x33(u(t, x, y))
    · diff(u(t, x, y), y) :
```

We however do not use our *universal formula* at once, as we want to be persuaded that it is uniquely determined. So we start with the natural for this equation ansatz, claiming that every coefficient of the covector is a quasilinear expression of the first order in  $u(t, x, y)$  and the unknown coefficients of this expression are functions of  $u(t, x, y)$  to be determined below. It is possible to demonstrate that any other (finite-jet) ansatz leads to the same output - our universal formula.

```
> Et := evalDG(DirectionalCovariantDerivative(D_t, g, C) + U1·g) :
Ex := evalDG(DirectionalCovariantDerivative(D_x, g, C) + U2·g) :
Ey := evalDG(DirectionalCovariantDerivative(D_y, g, C) + U3·g) :
```

```
>
> Eq000 := TensorInnerProduct(g, Et, dt &t dt) :
Eq001 := TensorInnerProduct(g, Et, dt &t dx) :
Eq002 := TensorInnerProduct(g, Et, dt &t dy) :
Eq011 := TensorInnerProduct(g, Et, dx &t dx) :
Eq012 := TensorInnerProduct(g, Et, dx &t dy) :
Eq022 := TensorInnerProduct(g, Et, dy &t dy) :
Eq100 := TensorInnerProduct(g, Ex, dt &t dt) :
Eq101 := TensorInnerProduct(g, Ex, dt &t dx) :
Eq102 := TensorInnerProduct(g, Ex, dt &t dy) :
Eq111 := TensorInnerProduct(g, Ex, dx &t dx) :
Eq112 := TensorInnerProduct(g, Ex, dx &t dy) :
Eq122 := TensorInnerProduct(g, Ex, dy &t dy) :
Eq200 := TensorInnerProduct(g, Ey, dt &t dt) :
Eq201 := TensorInnerProduct(g, Ey, dt &t dx) :
Eq202 := TensorInnerProduct(g, Ey, dt &t dy) :
Eq211 := TensorInnerProduct(g, Ey, dx &t dx) :
Eq212 := TensorInnerProduct(g, Ey, dx &t dy) :
Eq222 := TensorInnerProduct(g, Ey, dy &t dy) :
> sA := solve( {Eq000=0, Eq001=0, Eq002=0, Eq011=0, Eq012=0, Eq022=0, Eq100=0,
    Eq101=0, Eq102=0, Eq111=0, Eq112=0, Eq122=0, Eq200=0, Eq201=0, Eq202=0,
    Eq211=0, Eq212=0, Eq222=0}, [a000, a001, a002, a010, a011, a012, a020, a021, a022,
    a101, a102, a111, a112, a121, a122, a202, a212, a222]) :
```

```
> C1 := evalDG( subs( {op(op(sA))}, C) ) :
```

```
> evalDG( CovariantDerivative(g, C1) + g &t (U1·dt + U2·dx + U3·dy) );
0 dt dt dt
```

(6)

```
> R1 := CurvatureTensor(C1) : Ric1 := RicciTensor(R1) : T1 := SymmetrizeIndices(Ric1, [1, 2],
    "Symmetric") : Res := evalDG(T1 - V·g) :
```

```
> NEQt1 := ContractIndices(Res, D_t &t D_t, [[1, 1], [2, 2]]) : NEQt1x := ContractIndices(Res,
    D_t &t D_x, [[1, 1], [2, 2]]) :
NEQt1y := ContractIndices(Res, D_t &t D_y, [[1, 1], [2, 2]]) : NEQxx := ContractIndices(Res,
    D_x &t D_x, [[1, 1], [2, 2]]) :
NEQxy := ContractIndices(Res, D_x &t D_y, [[1, 1], [2, 2]]) : NEQyy := ContractIndices(Res,
    D_y &t D_y, [[1, 1], [2, 2]]) :
```

```

>
> DGsetup([t, x, y], [u], J2, 4) :
> de := DifferentialEquationData([F], [u1,1])
de := [ {u1,1}, [ ( (d2/du[]2 a(u[])) u22 + (d/du[] a(u[])) u2,2 + (d2/du[]2 b(u[])) u32
+ (d/du[] b(u[])) u3,3 + u1,1 + 2 (d2/du[]2 p(u[])) u2 u3 + 2 (d/du[] p(u[])) u2,3
+ 2 (d2/du[]2 q(u[])) u1 u2 + 2 (d/du[] q(u[])) u1,2 + 2 (d2/du[]2 r(u[])) u1 u3
+ 2 (d/du[] r(u[])) u1,3 ] ]

```

```

> de2 := Prolong(de, 2) : deTRA := Transformation(de2) :
>
> Eq0 := Pullback(deTRA, ToJet(NEQtt, DepVars, notation = jetnumbers)) :
> VS := solve(Eq0, V) :
> Eq1 := numer(subs(V = VS, Pullback(deTRA, ToJet(NEQtx, DepVars, notation
= jetnumbers)))) :
Eq2 := numer(subs(V = VS, Pullback(deTRA, ToJet(NEQty, DepVars, notation
= jetnumbers)))) :
Eq3 := numer(subs(V = VS, Pullback(deTRA, ToJet(NEQxx, DepVars, notation
= jetnumbers)))) :
Eq4 := numer(subs(V = VS, Pullback(deTRA, ToJet(NEQxy, DepVars, notation
= jetnumbers)))) :
Eq5 := numer(subs(V = VS, Pullback(deTRA, ToJet(NEQyy, DepVars, notation
= jetnumbers)))) :

```

We have to determine the coefficients  $\kappa[i,j]$  from this formula. The key observation is that the symbol of these contain the coefficients  $\kappa$  linearly (non-differentially!).

Thus we take the symbols and resolve the system. We do not provide output, as every of 25 equations on these 9 unknowns is pretty big.

```

> SUS := solve([diff(Eq1, u1,2), diff(Eq1, u1,3), diff(Eq1, u2,2), diff(Eq1, u2,3), diff(Eq1,
u3,3), diff(Eq2, u1,2), diff(Eq2, u1,3), diff(Eq2, u2,2), diff(Eq2, u2,3), diff(Eq2, u3,3),
diff(Eq3, u1,2), diff(Eq3, u1,3), diff(Eq3, u2,2), diff(Eq3, u2,3), diff(Eq3, u3,3),
diff(Eq4, u1,2), diff(Eq4, u1,3), diff(Eq4, u2,2), diff(Eq4, u2,3), diff(Eq4, u3,3),
diff(Eq5, u1,2), diff(Eq5, u1,3), diff(Eq5, u2,2), diff(Eq5, u2,3), diff(Eq5, u3,3),
[ $\kappa11(u_{[]} )$ ,  $\kappa12(u_{[]} )$ ,  $\kappa13(u_{[]} )$ ,  $\kappa21(u_{[]} )$ ,  $\kappa22(u_{[]} )$ ,  $\kappa23(u_{[]} )$ ,  $\kappa31(u_{[]} )$ ,  $\kappa32(u_{[]} )$ ,
 $\kappa33(u_{[]} )$ ]) :
> nops(SUS)

```

1

(8)

The system has a unique solution (indeed, this is a linear nondegenerate overdetermined but compatible system), and we check that it is given by the prescribed formulae.

```

> [simplify(subs(SUS[1],  $\kappa11(u_{[]} )$ ) - ToJet(VJ[1, 1], DepVars, notation = jetnumbers)),
simplify(subs(SUS[1],  $\kappa12(u_{[]} )$ ) - ToJet(VJ[1, 2], DepVars, notation = jetnumbers)),

```

$$\begin{aligned}
& \text{simplify}(\text{subs}(SUS[1], \kappa13(u_{[\ ]})) - \text{ToJet}(VJ[1, 3], \text{DepVars}, \text{notation} = \text{jetnumbers})) , \\
& \text{simplify}(\text{subs}(SUS[1], \kappa21(u_{[\ ]})) - \text{ToJet}(VJ[2, 1], \text{DepVars}, \text{notation} = \text{jetnumbers})) , \\
& \text{simplify}(\text{subs}(SUS[1], \kappa22(u_{[\ ]})) - \text{ToJet}(VJ[2, 2], \text{DepVars}, \text{notation} = \text{jetnumbers})) , \\
& \text{simplify}(\text{subs}(SUS[1], \kappa23(u_{[\ ]})) - \text{ToJet}(VJ[2, 3], \text{DepVars}, \text{notation} = \text{jetnumbers})) , \\
& \text{simplify}(\text{subs}(SUS[1], \kappa31(u_{[\ ]})) - \text{ToJet}(VJ[3, 1], \text{DepVars}, \text{notation} = \text{jetnumbers})) , \\
& \text{simplify}(\text{subs}(SUS[1], \kappa32(u_{[\ ]})) - \text{ToJet}(VJ[3, 2], \text{DepVars}, \text{notation} = \text{jetnumbers})) , \\
& \text{simplify}(\text{subs}(SUS[1], \kappa33(u_{[\ ]})) - \text{ToJet}(VJ[3, 3], \text{DepVars}, \text{notation} = \text{jetnumbers})) ] \\
& \quad [0, 0, 0, 0, 0, 0, 0, 0, 0]
\end{aligned} \tag{9}$$

Lovely. Thus we can use our universal formula for the covector. Now we set it in, restart the calculation and check the EW property.

$$\begin{aligned}
& > \\
& > U1 := VJ[1, 1] \cdot \text{diff}(u(t, x, y), t) + VJ[1, 2] \cdot \text{diff}(u(t, x, y), x) + VJ[1, 3] \cdot \text{diff}(u(t, x, y), y) : \\
& \quad U2 := VJ[2, 1] \cdot \text{diff}(u(t, x, y), t) + VJ[2, 2] \cdot \text{diff}(u(t, x, y), x) + VJ[2, 3] \cdot \text{diff}(u(t, x, y), y) : \\
& \quad U3 := VJ[3, 1] \cdot \text{diff}(u(t, x, y), t) + VJ[3, 2] \cdot \text{diff}(u(t, x, y), x) + VJ[3, 3] \cdot \text{diff}(u(t, x, y), y) : \\
& > \text{ChangeFrame}(M)
\end{aligned} \tag{10}$$

$$\begin{aligned}
& \mathbf{M} > \\
& > Et := \text{evalDG}(\text{DirectionalCovariantDerivative}(D\_t, g, C) + U1 \cdot g) : \\
& \quad Ex := \text{evalDG}(\text{DirectionalCovariantDerivative}(D\_x, g, C) + U2 \cdot g) : \\
& \quad Ey := \text{evalDG}(\text{DirectionalCovariantDerivative}(D\_y, g, C) + U3 \cdot g) : \\
& > Eq000 := \text{TensorInnerProduct}(g, Et, dt \& t dt) : \\
& \quad Eq001 := \text{TensorInnerProduct}(g, Et, dt \& t dx) : \\
& \quad Eq002 := \text{TensorInnerProduct}(g, Et, dt \& t dy) : \\
& \quad Eq011 := \text{TensorInnerProduct}(g, Et, dx \& t dx) : \\
& \quad Eq012 := \text{TensorInnerProduct}(g, Et, dx \& t dy) : \\
& \quad Eq022 := \text{TensorInnerProduct}(g, Et, dy \& t dy) : \\
& \quad Eq100 := \text{TensorInnerProduct}(g, Ex, dt \& t dt) : \\
& \quad Eq101 := \text{TensorInnerProduct}(g, Ex, dt \& t dx) : \\
& \quad Eq102 := \text{TensorInnerProduct}(g, Ex, dt \& t dy) : \\
& \quad Eq111 := \text{TensorInnerProduct}(g, Ex, dx \& t dx) : \\
& \quad Eq112 := \text{TensorInnerProduct}(g, Ex, dx \& t dy) : \\
& \quad Eq122 := \text{TensorInnerProduct}(g, Ex, dy \& t dy) : \\
& \quad Eq200 := \text{TensorInnerProduct}(g, Ey, dt \& t dt) : \\
& \quad Eq201 := \text{TensorInnerProduct}(g, Ey, dt \& t dx) : \\
& \quad Eq202 := \text{TensorInnerProduct}(g, Ey, dt \& t dy) : \\
& \quad Eq211 := \text{TensorInnerProduct}(g, Ey, dx \& t dx) : \\
& \quad Eq212 := \text{TensorInnerProduct}(g, Ey, dx \& t dy) : \\
& \quad Eq222 := \text{TensorInnerProduct}(g, Ey, dy \& t dy) : \\
& > sA := \text{solve}(\{Eq000=0, Eq001=0, Eq002=0, Eq011=0, Eq012=0, Eq022=0, Eq100=0, \\
& \quad Eq101=0, Eq102=0, Eq111=0, Eq112=0, Eq122=0, Eq200=0, Eq201=0, Eq202=0, \\
& \quad Eq211=0, Eq212=0, Eq222=0\}, [a000, a001, a002, a010, a011, a012, a020, a021, a022, \\
& \quad a101, a102, a111, a112, a121, a122, a202, a212, a222]) : \\
& > C1 := \text{evalDG}(\text{subs}(\{op(op(sA))\}, C)) : \\
& > \text{evalDG}(\text{CovariantDerivative}(g, C1) + g \& t (U1 \cdot dt + U2 \cdot dx + U3 \cdot dy)); \\
& \quad 0 \text{ dt dt dt}
\end{aligned} \tag{11}$$

$$> R1 := \text{CurvatureTensor}(C1) : Ric1 := \text{RicciTensor}(R1) : T1 := \text{SymmetrizeIndices}(Ric1, [1, 2],$$

```

"Symmetric") : Res := evalDG(TI - V·g) :
> NEQt := ContractIndices(Res, D_t &t D_t, [[1, 1], [2, 2]]) : NEQt_x := ContractIndices(Res,
D_t &t D_x, [[1, 1], [2, 2]]) :
NEQty := ContractIndices(Res, D_t &t D_y, [[1, 1], [2, 2]]) : NEQxx := ContractIndices(Res,
D_x &t D_x, [[1, 1], [2, 2]]) :
NEQxy := ContractIndices(Res, D_x &t D_y, [[1, 1], [2, 2]]) : NEQyy := ContractIndices(Res,
D_y &t D_y, [[1, 1], [2, 2]]) :
>
> DGsetup([t, x, y], [u], J2, 4) :
> de := DifferentialEquationData([F], [u1,1])
de := [ {u1,1}, [ (  $\frac{d^2}{du^2} a(u_{[]})$  ) u22 + (  $\frac{d}{du} a(u_{[]})$  ) u2,2 + (  $\frac{d^2}{du^2} b(u_{[]})$  ) u32
+ (  $\frac{d}{du} b(u_{[]})$  ) u3,3 + u1,1 + 2 (  $\frac{d^2}{du^2} p(u_{[]})$  ) u2 u3 + 2 (  $\frac{d}{du} p(u_{[]})$  ) u2,3
+ 2 (  $\frac{d^2}{du^2} q(u_{[]})$  ) u1 u2 + 2 (  $\frac{d}{du} q(u_{[]})$  ) u1,2 + 2 (  $\frac{d^2}{du^2} r(u_{[]})$  ) u1 u3
+ 2 (  $\frac{d}{du} r(u_{[]})$  ) u1,3 ] ]
> de2 := Prolong(de, 2) : deTRA := Transformation(de2) :
>
> Eq0 := Pullback(deTRA, ToJet(NEQt, DepVars, notation = jetnumbers)) :
> VS := solve(Eq0, V) :
> Eq1 := numer(subs(V = VS, Pullback(deTRA, ToJet(NEQt_x, DepVars, notation
= jetnumbers)))) :
Eq2 := numer(subs(V = VS, Pullback(deTRA, ToJet(NEQty, DepVars, notation
= jetnumbers)))) :
Eq3 := numer(subs(V = VS, Pullback(deTRA, ToJet(NEQxx, DepVars, notation
= jetnumbers)))) :
Eq4 := numer(subs(V = VS, Pullback(deTRA, ToJet(NEQxy, DepVars, notation
= jetnumbers)))) :
Eq5 := numer(subs(V = VS, Pullback(deTRA, ToJet(NEQyy, DepVars, notation
= jetnumbers)))) :

```

These equations have a unique solution for the 3rd derivatives of (a,b,p,q,r), so it is the same to find the solution or to check if the given set is a solution.

VST below is the set IC of Integrability conditions (from the work of Ferapontov, Huard and Zhang).

```

J2 > VST := [  $\frac{d^3}{du^3} a(u_{[]}) = \text{simplify}(\text{diff}(\ln(\text{Determinant}(A)), u_{[]}) \cdot \text{DDA}[2, 2]),$ 
 $\frac{d^3}{du^3} b(u_{[]}) = \text{simplify}(\text{diff}(\ln(\text{Determinant}(A)), u_{[]}) \cdot \text{DDA}[3, 3]),$ 
 $\frac{d^3}{du^3} p(u_{[]}) = \text{simplify}(\text{diff}(\ln(\text{Determinant}(A)), u_{[]}) \cdot \text{DDA}[2, 3]),$ 

```

$$\left. \begin{aligned} \frac{d^3}{du_{[]}^3} q(u_{[]}) &= \text{simplify}(\text{diff}(\ln(\text{Determinant}(A)), u_{[]} \cdot DDA[1, 2]), \\ \frac{d^3}{du_{[]}^3} r(u_{[]}) &= \text{simplify}(\text{diff}(\ln(\text{Determinant}(A)), u_{[]} \cdot DDA[1, 3]) \end{aligned} \right):$$

**J2** > DDA[2, 3]

$$\frac{d^2}{du_{[]}^2} p(u_{[]}) \quad (13)$$

**J2** > simplify(subs(VST, [Eq1, Eq2, Eq3, Eq4, Eq5]))  
[0, 0, 0, 0, 0]

(14)

Perfect! We have proved that EW  $\Leftrightarrow$  Integrability in this case!

> In fact, it won't hurt actually to check that the solution is unique. Substitution above shows that IC  $\Rightarrow$  EW. To show the opposite EW  $\Rightarrow$  IC we have to resolve the set of equations

[Eq1, Eq2, Eq3, Eq4, Eq5] with respect to the third order derivatives of (a, b, c, p, q, r)

. Again the system is involved, but the key observation is that its symbol

= 0 consists of 30 equations linear in the 6 functions - third derivatives

. These equations we resolve below and compare to the set VST of integrability conditions IC .

>

$$\begin{aligned} > \text{SOU} := \text{solve} \left( \left[ \text{diff}(Eq1, u_1, u_1), \text{diff}(Eq1, u_1, u_2), \text{diff}(Eq1, u_1, u_3), \text{diff}(Eq1, u_2, u_2), \right. \right. \\ &\quad \text{diff}(Eq1, u_2, u_3), \text{diff}(Eq1, u_3, u_3), \text{diff}(Eq2, u_1, u_1), \text{diff}(Eq2, u_1, u_2), \text{diff}(Eq2, u_1, u_3), \\ &\quad \text{diff}(Eq2, u_2, u_2), \text{diff}(Eq2, u_2, u_3), \text{diff}(Eq2, u_3, u_3), \text{diff}(Eq3, u_1, u_1), \text{diff}(Eq3, u_1, u_2), \\ &\quad \text{diff}(Eq3, u_1, u_3), \text{diff}(Eq3, u_2, u_2), \text{diff}(Eq3, u_2, u_3), \text{diff}(Eq3, u_3, u_3), \text{diff}(Eq4, u_1, u_1), \\ &\quad \text{diff}(Eq4, u_1, u_2), \text{diff}(Eq4, u_1, u_3), \text{diff}(Eq4, u_2, u_2), \text{diff}(Eq4, u_2, u_3), \text{diff}(Eq4, u_3, u_3), \\ &\quad \text{diff}(Eq5, u_1, u_1), \text{diff}(Eq5, u_1, u_2), \text{diff}(Eq5, u_1, u_3), \text{diff}(Eq5, u_2, u_2), \text{diff}(Eq5, u_2, u_3), \\ &\quad \left. \left. \text{diff}(Eq5, u_3, u_3) \right], \left[ \frac{d^3}{du_{[]}^3} a(u_{[]}), \frac{d^3}{du_{[]}^3} b(u_{[]}), \frac{d^3}{du_{[]}^3} c(u_{[]}), \frac{d^3}{du_{[]}^3} p(u_{[]}), \right. \right. \\ &\quad \left. \left. \frac{d^3}{du_{[]}^3} q(u_{[]}), \frac{d^3}{du_{[]}^3} r(u_{[]}) \right] \right) : \end{aligned}$$

> nops(SOU)

(15)

$$> \text{simplify} \left( \text{subs} \left( \text{SOU}[1], \left[ \frac{d^3}{du_{[]}^3} a(u_{[]}), \frac{d^3}{du_{[]}^3} b(u_{[]}), \frac{d^3}{du_{[]}^3} c(u_{[]}), \frac{d^3}{du_{[]}^3} p(u_{[]}), \right. \right. \right.$$

$$\left. \left. \left. \left. \frac{d^3}{du_{[]}^3} q(u_{[]}), \frac{d^3}{du_{[]}^3} r(u_{[]} \right) \right] \right) - subs \left( VST, \left[ \frac{d^3}{du_{[]}^3} a(u_{[]}), \frac{d^3}{du_{[]}^3} b(u_{[]}), \frac{d^3}{du_{[]}^3} c(u_{[]}), \right. \right. \right. \\ \left. \left. \left. \frac{d^3}{du_{[]}^3} p(u_{[]}), \frac{d^3}{du_{[]}^3} q(u_{[]}), \frac{d^3}{du_{[]}^3} r(u_{[]} \right) \right] \right) \right) \\ [0, 0, 0, 0, 0, 0, 0]$$
(16)

So well done!

In the other files concerning equations of types II, III, IV we will not be so detailed as here (the computations there are already sufficiently large), and some of the simple steps done here for pedantic reasons will be omitted in those files.

>

>

Below we check what happens if  $V=0$ . It turns out that in this case the symbol matrix  $A$  (in the text of the paper denoted by  $V$  - do not be confused) is constant, so indeed we have both linearization and integration.

>

**J2** > *simplify(diff(VS, u<sub>1,2</sub>))*

$$- \left( 2 \left( \frac{d^2}{du_{[]}^2} q(u_{[]}) \right) \right) / \left( -2 \left( \frac{d}{du_{[]}} r(u_{[]}) \right) \left( \frac{d}{du_{[]}} q(u_{[]}) \right) \left( \frac{d}{du_{[]}} p(u_{[]}) \right) \right. \\ \left. + \left( \frac{d}{du_{[]}} r(u_{[]}) \right)^2 \left( \frac{d}{du_{[]}} a(u_{[]}) \right) + \left( \frac{d}{du_{[]}} q(u_{[]}) \right)^2 \left( \frac{d}{du_{[]}} b(u_{[]}) \right) \right. \\ \left. - \left( \frac{d}{du_{[]}} a(u_{[]}) \right) \left( \frac{d}{du_{[]}} b(u_{[]}) \right) + \left( \frac{d}{du_{[]}} p(u_{[]}) \right)^2 \right)$$
(17)

**J2** > *simplify(diff(VS, u<sub>1,3</sub>))*

$$- \left( 2 \left( \frac{d^2}{du_{[]}^2} r(u_{[]}) \right) \right) / \left( -2 \left( \frac{d}{du_{[]}} r(u_{[]}) \right) \left( \frac{d}{du_{[]}} q(u_{[]}) \right) \left( \frac{d}{du_{[]}} p(u_{[]}) \right) \right. \\ \left. + \left( \frac{d}{du_{[]}} r(u_{[]}) \right)^2 \left( \frac{d}{du_{[]}} a(u_{[]}) \right) + \left( \frac{d}{du_{[]}} q(u_{[]}) \right)^2 \left( \frac{d}{du_{[]}} b(u_{[]}) \right) \right. \\ \left. - \left( \frac{d}{du_{[]}} a(u_{[]}) \right) \left( \frac{d}{du_{[]}} b(u_{[]}) \right) + \left( \frac{d}{du_{[]}} p(u_{[]}) \right)^2 \right)$$
(18)

**J2** > *simplify(diff(VS, u<sub>2,2</sub>))*

$$- \left( \frac{d^2}{du_{[]}^2} a(u_{[]}) \right) / \left( -2 \left( \frac{d}{du_{[]}} r(u_{[]}) \right) \left( \frac{d}{du_{[]}} q(u_{[]}) \right) \left( \frac{d}{du_{[]}} p(u_{[]}) \right) \right. \\ \left. + \left( \frac{d}{du_{[]}} r(u_{[]}) \right)^2 \left( \frac{d}{du_{[]}} a(u_{[]}) \right) + \left( \frac{d}{du_{[]}} q(u_{[]}) \right)^2 \left( \frac{d}{du_{[]}} b(u_{[]}) \right) \right. \\ \left. - \left( \frac{d}{du_{[]}} a(u_{[]}) \right) \left( \frac{d}{du_{[]}} b(u_{[]}) \right) + \left( \frac{d}{du_{[]}} p(u_{[]}) \right)^2 \right)$$
(19)

**J2** > *simplify(diff(VS, u<sub>2,3</sub>))*

(20)



$$\left[ - \left( 2 \left( \frac{d^2}{du_{[]}^2} p(u_{[]}) \right) \right) / \left( -2 \left( \frac{d}{du_{[]}} r(u_{[]}) \right) \left( \frac{d}{du_{[]}} q(u_{[]}) \right) \left( \frac{d}{du_{[]}} p(u_{[]}) \right) \right. \right. \\ \left. \left. + \left( \frac{d}{du_{[]}} r(u_{[]}) \right)^2 \left( \frac{d}{du_{[]}} a(u_{[]}) \right) + \left( \frac{d}{du_{[]}} q(u_{[]}) \right)^2 \left( \frac{d}{du_{[]}} b(u_{[]}) \right) \right. \\ \left. \left. - \left( \frac{d}{du_{[]}} a(u_{[]}) \right) \left( \frac{d}{du_{[]}} b(u_{[]}) \right) + \left( \frac{d}{du_{[]}} p(u_{[]}) \right)^2 \right) \right] \quad (20)$$

**J2** > *simplify(diff(VS, u<sub>3,3</sub>))*

$$\left[ - \left( \frac{d^2}{du_{[]}^2} b(u_{[]}) \right) / \left( -2 \left( \frac{d}{du_{[]}} r(u_{[]}) \right) \left( \frac{d}{du_{[]}} q(u_{[]}) \right) \left( \frac{d}{du_{[]}} p(u_{[]}) \right) \right. \right. \\ \left. \left. + \left( \frac{d}{du_{[]}} r(u_{[]}) \right)^2 \left( \frac{d}{du_{[]}} a(u_{[]}) \right) + \left( \frac{d}{du_{[]}} q(u_{[]}) \right)^2 \left( \frac{d}{du_{[]}} b(u_{[]}) \right) \right. \\ \left. \left. - \left( \frac{d}{du_{[]}} a(u_{[]}) \right) \left( \frac{d}{du_{[]}} b(u_{[]}) \right) + \left( \frac{d}{du_{[]}} p(u_{[]}) \right)^2 \right) \right] \quad (21)$$

Finished.
