# Supplementary material for: Dispersionless integrable systems in 3D and Einstein-Weyl geometry
Source: arXiv:1208.2728 ancillary file (2013-05-09)
Supplement: Supplementary file 2 [file BKEF-2012-I-divergense_quasilinear_linearization.pdf]

This is the worksheet accompanying the paper E.Ferapontov & B.Kruglikov "Dispersionless integrable systems in 3D and Einstein-Weyl geometry".

The file ran on **Maple** version 16, the package **DifferentialGeometry** was used.

We are going to attack the general 2nd order PDE  $a(u)_{xx}+b(u)_{yy}+c(u)_{zz}+2p(u)_{xy}+2q(u)_{xt}+2r(u)_{yt}=0$

studying its linearization and check if the corresponding conformal metric is flat

>

> with(DifferentialGeometry) : with(Tensor) : with(Tools) : with(JetCalculus) :  
with(LinearAlgebra) : with(PDEtools, D\_Dx, declare, ToJet, FromJet) :

> DGsetup([t, x, y], [u], J2, 3) :

> EQ := TotalDiff(a(u[1]), [2, 2]) + TotalDiff(b(u[1]), [3, 3]) + TotalDiff(c(u[1]), [1, 1])  
+ 2·TotalDiff(p(u[1]), [2, 3]) + 2·TotalDiff(q(u[1]), [1, 2]) + 2·TotalDiff(r(u[1]), [1, 3])

$$\begin{aligned} EQ := & \left( \frac{d^2}{du_{[1]}^2} a(u_{[1]}) \right) u_2^2 + \left( \frac{d}{du_{[1]}} a(u_{[1]}) \right) u_{2,2} + \left( \frac{d^2}{du_{[1]}^2} b(u_{[1]}) \right) u_3^2 \\ & + \left( \frac{d}{du_{[1]}} b(u_{[1]}) \right) u_{3,3} + \left( \frac{d^2}{du_{[1]}^2} c(u_{[1]}) \right) u_1^2 + \left( \frac{d}{du_{[1]}} c(u_{[1]}) \right) u_{1,1} \\ & + 2 \left( \frac{d^2}{du_{[1]}^2} p(u_{[1]}) \right) u_2 u_3 + 2 \left( \frac{d}{du_{[1]}} p(u_{[1]}) \right) u_{2,3} + 2 \left( \frac{d^2}{du_{[1]}^2} q(u_{[1]}) \right) u_1 u_2 \\ & + 2 \left( \frac{d}{du_{[1]}} q(u_{[1]}) \right) u_{1,2} + 2 \left( \frac{d^2}{du_{[1]}^2} r(u_{[1]}) \right) u_1 u_3 + 2 \left( \frac{d}{du_{[1]}} r(u_{[1]}) \right) u_{1,3} \end{aligned} \quad (1)$$

Let us for simplicity assume that c(u) is not constant, and change the variables  $u \rightarrow c(u)$ .

This is only a local in  $J^0$  transformation, but we hope this does not reduce the generality.

> EQ := TotalDiff(a(u[1]), [2, 2]) + TotalDiff(b(u[1]), [3, 3]) + TotalDiff(u[1], [1, 1]) + 2  
·TotalDiff(p(u[1]), [2, 3]) + 2·TotalDiff(q(u[1]), [1, 2]) + 2·TotalDiff(r(u[1]), [1, 3])

$$\begin{aligned} EQ := & \left( \frac{d^2}{du_{[1]}^2} a(u_{[1]}) \right) u_2^2 + \left( \frac{d}{du_{[1]}} a(u_{[1]}) \right) u_{2,2} + \left( \frac{d^2}{du_{[1]}^2} b(u_{[1]}) \right) u_3^2 \\ & + \left( \frac{d}{du_{[1]}} b(u_{[1]}) \right) u_{3,3} + u_{1,1} + 2 \left( \frac{d^2}{du_{[1]}^2} p(u_{[1]}) \right) u_2 u_3 + 2 \left( \frac{d}{du_{[1]}} p(u_{[1]}) \right) u_{2,3} \\ & + 2 \left( \frac{d^2}{du_{[1]}^2} q(u_{[1]}) \right) u_1 u_2 + 2 \left( \frac{d}{du_{[1]}} q(u_{[1]}) \right) u_{1,2} + 2 \left( \frac{d^2}{du_{[1]}^2} r(u_{[1]}) \right) u_1 u_3 \\ & + 2 \left( \frac{d}{du_{[1]}} r(u_{[1]}) \right) u_{1,3} \end{aligned} \quad (2)$$

> A := Matrix( [[diff(EQ, u[1, 1]), 1/2 diff(EQ, u[1, 2]), 1/2 diff(EQ, u[1, 3])], [1/2 diff(EQ, u[1, 2]), diff(EQ, u[2, 2]), 1/2 diff(EQ, u[2, 3])], [1/2 diff(EQ, u[1, 3]), 1/2 diff(EQ, u[2, 3]), diff(EQ, u[3, 3])] ] ); AA := expand(MatrixInverse(A)) : AM

$:= \text{simplify}(\text{Determinant}(A) \cdot AA) :$

$$A := \begin{bmatrix} 1 & \frac{d}{du_{[]}} q(u_{[]}) & \frac{d}{du_{[]}} r(u_{[]}) \\ \frac{d}{du_{[]}} q(u_{[]}) & \frac{d}{du_{[]}} a(u_{[]}) & \frac{d}{du_{[]}} p(u_{[]}) \\ \frac{d}{du_{[]}} r(u_{[]}) & \frac{d}{du_{[]}} p(u_{[]}) & \frac{d}{du_{[]}} b(u_{[]}) \end{bmatrix} \quad (3)$$

>  $\text{simplify}(\text{Determinant}(A))$

$$2 r_u q_u p_u - r_u^2 a_u - q_u^2 b_u + a_u b_u - p_u^2 \quad (4)$$

>  $\text{smb13} := Z \rightarrow \text{add}(\text{add}(\text{add}(\text{diff}(Z, u[p, q, r]) \cdot u[p, q, r], r = q \dots 3), q = p \dots 3), p = 1 \dots 3) :$

>  $G2 := (i, j, k, l) \rightarrow \text{diff}(AA[i, j], u_{[]}) \cdot \text{TotalDiff}(u_{[]}, [k, l]) :$

>  $G3 := (i, j, k, l, m) \rightarrow \text{diff}(AA[i, j], u_{[]}) \cdot \text{TotalDiff}(u_{[]}, [k, l, m]) :$

>  $\text{Ric} := (i, j) \rightarrow \frac{1}{2} \cdot \text{add}(\text{add}(A[k, l] \cdot (G2(i, j, k, l) + G2(k, l, i, j) - G2(i, k, j, l) - G2(j, l, i, k)), l = 1 \dots 3), k = 1 \dots 3) :$

>  $\text{Ric2} := (i, j, m) \rightarrow \frac{1}{2} \cdot \text{add}(\text{add}(A[k, l] \cdot (G3(i, j, k, l, m) + G3(k, l, i, j, m) - G3(i, k, j, l, m) - G3(j, l, i, k, m)), l = 1 \dots 3), k = 1 \dots 3) :$

>  $\text{Sc} := \text{add}(\text{add}(A[i, j] \cdot \text{Ric}(i, j), j = 1 \dots 3), i = 1 \dots 3) :$

>  $\text{Sc2} := k \rightarrow \text{add}(\text{add}(A[i, j] \cdot \text{Ric2}(i, j, k), j = 1 \dots 3), i = 1 \dots 3) :$

>  $\text{Cot} := (i, j, t) \rightarrow \text{smb13} \left( \text{Ric2}(i, j, t) - \text{Ric2}(i, t, j) - \frac{1}{4} AA[i, j] \cdot \text{Sc2}(t) + \frac{1}{4} AA[i, t] \cdot \text{Sc2}(j) \right) :$

>

Here I define the symbol of the Cotton tensor - it has order 3 in the entries of the metric, so order 4 in the functions  $a(u)$ ,  $b(u)$ ,  $p(u)$ ,  $q(u)$ ,  $r(u)$ .

The highest order of derivatives of  $u$  involved here is 3.

>

**M** >  $\text{DE} := \text{DifferentialEquationData}([EQ], [u_{1, 1}])$

$$\begin{aligned} \text{DE} := & \left[ \{u_{1, 1}\}, \left[ \left( \frac{d^2}{du_{[]}^2} a(u_{[]}) \right) u_{2, 2}^2 + \left( \frac{d}{du_{[]}} a(u_{[]}) \right) u_{2, 2} + \left( \frac{d^2}{du_{[]}^2} b(u_{[]}) \right) u_3^2 \right. \right. \\ & + \left( \frac{d}{du_{[]}} b(u_{[]}) \right) u_{3, 3} + u_{1, 1} + 2 \left( \frac{d^2}{du_{[]}^2} p(u_{[]}) \right) u_2 u_3 + 2 \left( \frac{d}{du_{[]}} p(u_{[]}) \right) u_{2, 3} \\ & + 2 \left( \frac{d^2}{du_{[]}^2} q(u_{[]}) \right) u_1 u_2 + 2 \left( \frac{d}{du_{[]}} q(u_{[]}) \right) u_{1, 2} + 2 \left( \frac{d^2}{du_{[]}^2} r(u_{[]}) \right) u_1 u_3 \\ & \left. \left. + 2 \left( \frac{d}{du_{[]}} r(u_{[]}) \right) u_{1, 3} \right] \right] \end{aligned} \quad (5)$$

**M** >  $\text{DE1} := \text{Prolong}(\text{DE}, 1) :$

**M** >  $\text{alpha} := \text{Transformation}(\text{DE1}) :$

**E** >

**E** > with(PDEtools) : declare( $a(u_{[]})$ ) :  
 $a(u_{[]})$  will now be displayed as  $a$  (6)

**E** > simplify(Pullback(alpha, u[1, 1, 3]))  

$$\begin{aligned} & -u_3 a_{u_{[]}, u_{[]}, u_{[]}} u_2^2 - u_3 a_{u_{[]}, u_{[]}} u_{2,2} - b_{u_{[]}, u_{[]}, u_{[]}} u_3^3 - 3 u_3 b_{u_{[]}, u_{[]}} u_{3,3} - 2 p_{u_{[]}, u_{[]}, u_{[]}} u_2 u_3^2 \\ & - 4 u_3 p_{u_{[]}, u_{[]}} u_{2,3} - 2 u_3 q_{u_{[]}, u_{[]}, u_{[]}} u_1 u_2 - 2 u_3 q_{u_{[]}, u_{[]}} u_{1,2} - 2 r_{u_{[]}, u_{[]}, u_{[]}} u_1 u_3^2 \\ & - 4 u_3 r_{u_{[]}, u_{[]}} u_{1,3} - 2 u_{1,3} q_{u_{[]}, u_{[]}} u_2 - 2 u_{2,3} a_{u_{[]}, u_{[]}} u_2 - 2 u_{2,3} q_{u_{[]}, u_{[]}} u_1 \\ & - 2 u_{3,3} p_{u_{[]}, u_{[]}} u_2 - 2 u_{3,3} r_{u_{[]}, u_{[]}} u_1 - 2 p_{u_{[]}} u_{2,3,3} - 2 q_{u_{[]}} u_{1,2,3} - 2 r_{u_{[]}} u_{1,3,3} \\ & - a_{u_{[]}} u_{2,2,3} - b_{u_{[]}} u_{3,3,3} \end{aligned}$$
 (7)

>  
 > Res112 := simplify(smb13(Determinant(A) · Pullback(alpha, Cot(1, 1, 2)))) :  
 > Res112a := simplify(subs([ ], factor([numer(diff(Res112, u[1, 2, 2])), numer(diff(Res112, u[1, 2, 3])), numer(diff(Res112, u[1, 3, 3])), numer(diff(Res112, u[2, 2, 2])), numer(diff(Res112, u[2, 2, 3])), numer(diff(Res112, u[2, 3, 3])), numer(diff(Res112, u[3, 3, 3])))])) :  
 > Res113 := simplify(smb13(Determinant(A) · Pullback(alpha, Cot(1, 1, 3)))) :  
 > Res113a := simplify(subs([ ], factor([numer(diff(Res113, u[1, 2, 2])), numer(diff(Res113, u[1, 2, 3])), numer(diff(Res113, u[1, 3, 3])), numer(diff(Res113, u[2, 2, 2])), numer(diff(Res113, u[2, 2, 3])), numer(diff(Res113, u[2, 3, 3])), numer(diff(Res113, u[3, 3, 3])))])) :  
 > Res123 := simplify(smb13(Determinant(A) · Pullback(alpha, Cot(1, 2, 3)))) :  
 > Res123a := simplify(subs([ ], factor([numer(diff(Res123, u[1, 2, 2])), numer(diff(Res123, u[1, 2, 3])), numer(diff(Res123, u[1, 3, 3])), numer(diff(Res123, u[2, 2, 2])), numer(diff(Res123, u[2, 2, 3])), numer(diff(Res123, u[2, 3, 3])), numer(diff(Res123, u[3, 3, 3])))])) :  
 > Res212 := simplify(smb13(Determinant(A) · Pullback(alpha, Cot(2, 1, 2)))) :  
 > Res212a := simplify(subs([ ], factor([numer(diff(Res212, u[1, 2, 2])), numer(diff(Res212, u[1, 2, 3])), numer(diff(Res212, u[1, 3, 3])), numer(diff(Res212, u[2, 2, 2])), numer(diff(Res212, u[2, 2, 3])), numer(diff(Res212, u[2, 3, 3])), numer(diff(Res212, u[3, 3, 3])))])) :  
 > Res213 := simplify(smb13(Determinant(A) · Pullback(alpha, Cot(2, 1, 3)))) :  
 > Res213a := simplify(subs([ ], factor([numer(diff(Res213, u[1, 2, 2])), numer(diff(Res213, u[1, 2, 3])), numer(diff(Res213, u[1, 3, 3])), numer(diff(Res213, u[2, 2, 2])), numer(diff(Res213, u[2, 2, 3])), numer(diff(Res213, u[2, 3, 3])), numer(diff(Res213, u[3, 3, 3])))])) :  
 > Res223 := simplify(smb13(Determinant(A) · Pullback(alpha, Cot(2, 2, 3)))) :  
 > Res223a := simplify(subs([ ], factor([numer(diff(Res223, u[1, 2, 2])), numer(diff(Res223, u[1, 2, 3])), numer(diff(Res223, u[1, 3, 3])), numer(diff(Res223, u[2, 2, 2])), numer(diff(Res223, u[2, 2, 3])), numer(diff(Res223, u[2, 3, 3])), numer(diff(Res223, u[3, 3, 3])))])) :  
 > Res312 := simplify(smb13(Determinant(A) · Pullback(alpha, Cot(3, 1, 2)))) :  
 > Res312a := simplify(subs([ ], factor([numer(diff(Res312, u[1, 2, 2])), numer(diff(Res312, u[1, 2, 3])), numer(diff(Res312, u[1, 3, 3])), numer(diff(Res312, u[2, 2, 2])), numer(diff(Res312, u[2, 2, 3])), numer(diff(Res312, u[2, 3, 3])), numer(diff(Res312, u[3, 3, 3])))])) :

$u[3, 3, 3])))) :$

>  $Res313 := simplify(smb13(Determinant(A) \cdot Pullback(alpha, Cot(3, 1, 3)))) :$

>  $Res313a := simplify(subs([ ], factor([numer(diff(Res313, u[1, 2, 2])), numer(diff(Res313, u[1, 2, 3])), numer(diff(Res313, u[1, 3, 3])), numer(diff(Res313, u[2, 2, 2])), numer(diff(Res313, u[2, 2, 3])), numer(diff(Res313, u[2, 3, 3])), numer(diff(Res313, u[3, 3, 3]))])))) :$

>  $Res323 := simplify(smb13(Determinant(A) \cdot Pullback(alpha, Cot(3, 2, 3)))) :$

>  $Res323a := simplify(subs([ ], factor([numer(diff(Res323, u[1, 2, 2])), numer(diff(Res323, u[1, 2, 3])), numer(diff(Res323, u[1, 3, 3])), numer(diff(Res323, u[2, 2, 2])), numer(diff(Res323, u[2, 2, 3])), numer(diff(Res323, u[2, 3, 3])), numer(diff(Res323, u[3, 3, 3]))])))) :$

>

Consider some of the output

>

>  $Res223a[1]$

$$r_{u_{[]}, u_{[]}} \left( -a_{u_{[]}} + q_{u_{[]}}^2 \right) \quad (8)$$

>  $Res223a[2]$

$$r_{u_{[]}, u_{[]}} \left( -p_{u_{[]}} + r_{u_{[]}} q_{u_{[]}} \right) \quad (9)$$

>  $Res223a[3]$

$$r_{u_{[]}, u_{[]}} \left( r_{u_{[]}}^2 - b_{u_{[]}} \right) \quad (10)$$

>  $Res323a[1]$

$$-q_{u_{[]}, u_{[]}} \left( -a_{u_{[]}} + q_{u_{[]}}^2 \right) \quad (11)$$

>  $Res323a[2]$

$$-q_{u_{[]}, u_{[]}} \left( -p_{u_{[]}} + r_{u_{[]}} q_{u_{[]}} \right) \quad (12)$$

>  $Res323a[3]$

$$-q_{u_{[]}, u_{[]}} \left( r_{u_{[]}}^2 - b_{u_{[]}} \right) \quad (13)$$

>  $Res323a[4]$

$$-a_{u_{[]}, u_{[]}} \left( -a_{u_{[]}} + q_{u_{[]}}^2 \right) \quad (14)$$

>  $Res223a[7]$

$$b_{u_{[]}, u_{[]}} \left( r_{u_{[]}}^2 - b_{u_{[]}} \right) \quad (15)$$

>

We see 3 types of factors (of first order)

. All three cannot vanish since otherwise the determinant of A will be zero as well.

>  $factor\left(subs\left(\left[b_{u_{[]}} = r_{u_{[]}}^2, a_{u_{[]}} = q_{u_{[]}}^2, p_{u_{[]}} = r_{u_{[]}} q_{u_{[]}}\right], 2 r_{u_{[]}} q_{u_{[]}} p_{u_{[]}} - r_{u_{[]}}^2 a_{u_{[]}} - q_{u_{[]}}^2 b_{u_{[]}} + a_{u_{[]}} b_{u_{[]}} - p_{u_{[]}}^2\right)\right)$

0

(16)

So then the above implies that  $r_{u, u} = 0$ ,  $q_{u, u} = 0$ , and thereafter  $a_{u, u} = 0$ ,  $b_{u, u} = 0$  (even

if we assume the first order factor in the last two expression vanishes this implies the claim).

>

> Res123a[1]

$$-a_{u[]} p_{u[],u[]} - 2 q_{u[]} p_{u[]} q_{u[],u[]} + 2 r_{u[]} q_{u[]}^2 q_{u[],u[]} - r_{u[]} q_{u[]} a_{u[],u[]} + p_{u[]} a_{u[],u[]} - 2 q_{u[]}^3 r_{u[],u[]} + q_{u[]}^2 p_{u[],u[]} + 2 q_{u[]} a_{u[]} r_{u[],u[]} \quad (17)$$

$$\begin{aligned} &> \text{factor}\left(\text{subs}\left(\left[a_{u[],u[]} = 0, b_{u[],u[]} = 0, r_{u[],u[]} = 0, q_{u[],u[]} = 0\right], -a_{u[]} p_{u[],u[]} \right. \\ &\quad \left. - 2 q_{u[]} p_{u[]} q_{u[],u[]} + 2 r_{u[]} q_{u[]}^2 q_{u[],u[]} - r_{u[]} q_{u[]} a_{u[],u[]} + p_{u[]} a_{u[],u[]} - 2 \right. \\ &\quad \left. q_{u[]}^3 r_{u[],u[]} + q_{u[]}^2 p_{u[],u[]} + 2 q_{u[]} a_{u[]} r_{u[],u[]} \right) \\ &\quad \left. - p_{u[],u[]} \left(a_{u[]} - q_{u[]}^2\right) \right) \quad (18) \end{aligned}$$

> Res323a[7]

$$b_{u[],u[]} q_{u[]} r_{u[]} + 2 r_{u[],u[]} p_{u[]} r_{u[]} - 2 q_{u[]} b_{u[]} r_{u[],u[]} - 2 p_{u[],u[]} r_{u[]}^2 - b_{u[],u[]} p_{u[]} + 2 p_{u[],u[]} b_{u[]} \quad (19)$$

$$\begin{aligned} &> \text{factor}\left(\text{subs}\left(\left[a_{u[],u[]} = 0, b_{u[],u[]} = 0, r_{u[],u[]} = 0, q_{u[],u[]} = 0\right], b_{u[],u[]} q_{u[]} r_{u[]} \right. \right. \\ &\quad \left. \left. + 2 r_{u[],u[]} p_{u[]} r_{u[]} - 2 q_{u[]} b_{u[]} r_{u[],u[]} - 2 p_{u[],u[]} r_{u[]}^2 - b_{u[],u[]} p_{u[]} + 2 p_{u[],u[]} b_{u[]} \right) \right. \\ &\quad \left. 2 p_{u[],u[]} \left(-r_{u[]}^2 + b_{u[]}\right) \right) \quad (20) \end{aligned}$$

> Res112a[5]

$$\begin{aligned} &-p_{u[],u[]} p_{u[]}^2 - 2 q_{u[],u[]} r_{u[]} a_{u[]} b_{u[]} + 4 r_{u[],u[]} p_{u[]} r_{u[]} a_{u[]} + 4 q_{u[],u[]} p_{u[]} q_{u[]} r_{u[]}^2 \\ &\quad - 4 r_{u[],u[]} p_{u[]} q_{u[]}^2 r_{u[]} - 2 r_{u[],u[]} q_{u[]} r_{u[]}^2 a_{u[]} + b_{u[],u[]} q_{u[]} r_{u[]} a_{u[]} \\ &\quad + 2 p_{u[],u[]} p_{u[]} q_{u[]} r_{u[]} - 2 q_{u[],u[]} p_{u[]} q_{u[]} b_{u[]} + 2 r_{u[],u[]} p_{u[]}^2 q_{u[]} - 2 p_{u[]} r_{u[]}^2 a_{u[],u[]} \\ &\quad - b_{u[],u[]} p_{u[]} a_{u[]} + 2 p_{u[]} b_{u[]} a_{u[],u[]} + 2 q_{u[],u[]} r_{u[]}^3 a_{u[]} - p_{u[],u[]} r_{u[]}^2 a_{u[]} - 2 q_{u[],u[]} p_{u[]}^2 r_{u[]} \quad (21) \end{aligned}$$

$$\begin{aligned} &> \text{factor}\left(\text{subs}\left(\left[a_{u[],u[]} = 0, b_{u[],u[]} = 0, r_{u[],u[]} = 0, q_{u[],u[]} = 0\right], -p_{u[],u[]} p_{u[]}^2 \right. \right. \\ &\quad \left. \left. - 2 q_{u[],u[]} r_{u[]} a_{u[]} b_{u[]} + 4 r_{u[],u[]} p_{u[]} r_{u[]} a_{u[]} + 4 q_{u[],u[]} p_{u[]} q_{u[]} r_{u[]}^2 \right. \right. \\ &\quad \left. \left. - 4 r_{u[],u[]} p_{u[]} q_{u[]}^2 r_{u[]} - 2 r_{u[],u[]} q_{u[]} r_{u[]}^2 a_{u[]} + b_{u[],u[]} q_{u[]} r_{u[]} a_{u[]} \right. \right. \\ &\quad \left. \left. + 2 p_{u[],u[]} p_{u[]} q_{u[]} r_{u[]} - 2 q_{u[],u[]} p_{u[]} q_{u[]} b_{u[]} + 2 r_{u[],u[]} p_{u[]}^2 q_{u[]} - 2 p_{u[]} r_{u[]}^2 a_{u[]} \right) \right) \end{aligned}$$

$$\left[ \begin{aligned} & r_{u[]}^2 a_{u[],u[]} - b_{u[],u[]} p_{u[]} a_{u[]} + 2 p_{u[]} b_{u[]} a_{u[],u[]} + 2 q_{u[],u[]} r_{u[]}^3 a_{u[]} - p_{u[],u[]} \\ & r_{u[]}^2 a_{u[]} - 2 q_{u[],u[]} p_{u[]}^2 r_{u[]} \Big) \Big) \\ & \quad - p_{u[],u[]} \left( p_{u[]}^2 - 2 r_{u[]} q_{u[]} p_{u[]} + r_{u[]}^2 a_{u[]} \right) \end{aligned} \right] \quad (22)$$

$$\begin{aligned} & \text{factor} \left( \text{subs} \left( \left[ b_{u[]} = r_{u[]}^2, a_{u[]} = q_{u[]}^2 \right], p_{u[]}^2 - 2 r_{u[]} q_{u[]} p_{u[]} + r_{u[]}^2 a_{u[]} \right) \right) \\ & \quad \left( p_{u[]} - r_{u[]} q_{u[]} \right)^2 \end{aligned} \quad (23)$$

So we see, since not all the coefficients of  $p_{u,u}$  can vanish simultaneuosly, that  $p_{u,u} = 0$ . This proves our claim!

This finishes the proof of Theorem 2. Done!

>

>
