# Supplementary material for: Dispersionless integrable systems in 3D and Einstein-Weyl geometry
Source: arXiv:1208.2728 ancillary file (2013-05-09)
Supplement: Supplementary file 3 [file BKEF-2012-II-quasilinear_wave_integrability-Lax.pdf]

This is the worksheet accompanying the paper E.Ferapontov & B.Kruglikov "Dispersionless integrable systems in 3D and Einstein-Weyl geometry".

The file ran on **Maple** version 16, the package **DifferentialGeometry** was used.

We consider type II quasilinear wave system and study it's integrability in Lax/pseudopotential sense via EW property of the linearization conformal structure

>

We first check that the fields X,Y form a Lax pair in 4D (t,x,y,w=λ), as well as the similar property for their 3D analogs (when we let λ=λ(t,x,y)).

We start by deriving the compatibility condition for the system {w\_t=D\_x[f(u\_1,u\_2,u\_3,w)], w\_y=D\_x[g(u\_1,u\_2,u\_3,w)]}.

>

> restart : with(DifferentialGeometry) : with(Tensor) : with(Tools) : with(JetCalculus) :  
with(LinearAlgebra) : with(PDEtools, D\_Dx, declare, ToJet, FromJet) :

> DGsetup([t, x, y], [u, w], L2, 2) :

> declare(Ctt(u\_1, u\_2, u\_3)) : declare(Ctx(u\_1, u\_2, u\_3)) : declare(Cty(u\_1, u\_2, u\_3)) :  
declare(Cxx(u\_1, u\_2, u\_3)) : declare(Cxy(u\_1, u\_2, u\_3)) : declare(Cyy(u\_1, u\_2, u\_3)) :

*Ctt(u\_1, u\_2, u\_3) will now be displayed as Ctt*

*Ctx(u\_1, u\_2, u\_3) will now be displayed as Ctx*

*Cty(u\_1, u\_2, u\_3) will now be displayed as Cty*

*Cxx(u\_1, u\_2, u\_3) will now be displayed as Cxx*

*Cxy(u\_1, u\_2, u\_3) will now be displayed as Cxy*

*Cyy(u\_1, u\_2, u\_3) will now be displayed as Cyy*

(1)

>

> SI := { w\_1 =  $\frac{\partial}{\partial u_1} f(u_1, u_2, u_3, w_{[]}) \cdot u_{1,2} + \frac{\partial}{\partial u_2} f(u_1, u_2, u_3, w_{[]}) \cdot u_{2,2} + \frac{\partial}{\partial u_3} f(u_1, u_2, u_3, w_{[]}) \cdot u_{2,3} + \frac{\partial}{\partial w_{[]}} f(u_1, u_2, u_3, w_{[]}) \cdot w_2$ ,  
w\_3 =  $\frac{\partial}{\partial u_1} g(u_1, u_2, u_3, w_{[]}) \cdot u_{1,2} + \frac{\partial}{\partial u_2} g(u_1, u_2, u_3, w_{[]}) \cdot u_{2,2} + \frac{\partial}{\partial u_3} g(u_1, u_2, u_3, w_{[]}) \cdot u_{2,3} + \frac{\partial}{\partial w_{[]}} g(u_1, u_2, u_3, w_{[]}) \cdot w_2$  } :

>

> F := Ctt(u\_1, u\_2, u\_3) · u\_{1,1} + 2 Ctx(u\_1, u\_2, u\_3) · u\_{1,2} + 2 Cty(u\_1, u\_2, u\_3) · u\_{1,3} + Cxx(u\_1, u\_2, u\_3) · u\_{2,2} + 2 Cxy(u\_1, u\_2, u\_3) · u\_{2,3} + Cyy(u\_1, u\_2, u\_3) · u\_{3,3} :

> de := DifferentialEquationData([F, SI[1]], [u\_{1,1}, w\_1])

de := [ {u\_{1,1}, w\_1}, [ Ctt u\_{1,1} + 2 Ctx u\_{1,2} + 2 Cty u\_{1,3} + Cxx u\_{2,2} + 2 Cxy u\_{2,3} + Cyy u\_{3,3}, w\_1  
- f\_{u\_1} u\_{1,2} - f\_{u\_2} u\_{2,2} - f\_{u\_3} u\_{2,3} - f\_{w\_{[]}} w\_2 ] ] (2)

> de1 := Prolong(de, 1) : deTR := Transformation(de1) :

>

$$\begin{aligned}
& \text{> } S2a := \{w_{2,3} = \text{TotalDiff}(\text{subs}(SI, w_3), 2)\} : \\
& \text{> } S2 := \text{simplify}(\{\text{subs}(SI, \text{subs}(S2a, w_{3,3} = \text{Pullback}(\text{deTR}, \text{TotalDiff}(\text{subs}(SI, w_3), 3)))\}, \\
& \quad S2a[1], SI[2])\}
\end{aligned}$$

$$\begin{aligned}
S2 := \{ & w_3 = g_{u_1} u_{1,2} + g_{u_2} u_{2,2} + g_{u_3} u_{2,3} + g_{w_{[]}} w_{2,3} = g_{u_1, u_1} u_{1,2}^2 + 2 u_{1,2} g_{u_1, u_2} u_{2,2} \\
& + 2 u_{1,2} g_{u_1, u_3} u_{2,3} + 2 u_{1,2} g_{u_1, w_{[]}} w_2 + g_{u_2, u_2} u_{2,2}^2 + 2 u_{2,2} g_{u_2, u_3} u_{2,3} + 2 u_{2,2} g_{u_2, w_{[]}} w_2 \\
& + g_{u_3, u_3} u_{2,3}^2 + 2 u_{2,3} g_{u_3, w_{[]}} w_2 + g_{u_1} u_{1,2,2} + g_{u_2} u_{2,2,2} + g_{u_3} u_{2,2,3} + g_{w_{[]}, w_{[]}} w_2^2 \\
& + g_{w_{[]}} w_{2,2} w_{3,3} = g_{u_1, w_{[]}} u_{1,2} g_{u_3} u_{2,3} + 3 g_{u_1, w_{[]}} u_{1,2} g_{w_{[]}} w_2 + g_{u_2, w_{[]}} u_{2,2} g_{u_1} u_{1,2} \\
& + g_{u_2, w_{[]}} u_{2,2} g_{u_3} u_{2,3} + 3 g_{u_2, w_{[]}} u_{2,2} g_{w_{[]}} w_2 + g_{u_3, w_{[]}} u_{2,3} g_{u_1} u_{1,2} + g_{u_3, w_{[]}} u_{2,3} g_{u_2} u_{2,2} \\
& + 3 g_{u_3, w_{[]}} u_{2,3} g_{w_{[]}} w_2 + g_{w_{[]}, w_{[]}} w_2 g_{u_1} u_{1,2} + g_{w_{[]}, w_{[]}} w_2 g_{u_2} u_{2,2} + g_{w_{[]}, w_{[]}} w_2 g_{u_3} u_{2,3} \\
& + 2 g_{w_{[]}} u_{1,2} g_{u_1, u_2} u_{2,2} + 2 g_{w_{[]}} u_{1,2} g_{u_1, u_3} u_{2,3} + 2 g_{w_{[]}} u_{2,2} g_{u_2, u_3} u_{2,3} \\
& + g_{u_1, w_{[]}} u_{1,2} g_{u_2} u_{2,2} + g_{w_{[]}} g_{u_3} u_{2,2,3} + u_{1,3} g_{u_1, u_1} u_{1,2} + u_{1,3} g_{u_1, u_2} u_{2,2} \\
& + u_{1,3} g_{u_1, u_3} u_{2,3} + u_{1,3} g_{u_1, w_{[]}} w_2 + u_{2,3} g_{u_1, u_2} u_{1,2} + u_{2,3} g_{u_2, u_2} u_{2,2} + u_{2,3} g_{u_2, w_{[]}} w_2 \\
& + u_{3,3} g_{u_1, u_3} u_{1,2} + u_{3,3} g_{u_2, u_3} u_{2,2} + u_{3,3} g_{u_3, u_3} u_{2,3} + u_{3,3} g_{u_3, w_{[]}} w_2 + g_{u_1, w_{[]}} u_{1,2}^2 g_{u_1} \\
& + g_{u_2, w_{[]}} u_{2,2}^2 g_{u_2} + g_{u_3, w_{[]}} u_{2,3}^2 g_{u_3} + 2 g_{w_{[]}, w_{[]}} w_2^2 g_{w_{[]}} + g_{w_{[]}} g_{u_1, u_1} u_{1,2}^2 + g_{w_{[]}} g_{u_2, u_2} \\
& u_{2,2}^2 + g_{w_{[]}} g_{u_3, u_3} u_{2,3}^2 + g_{w_{[]}} g_{u_1} u_{1,2,2} + g_{w_{[]}} g_{u_2} u_{2,2,2} + g_{u_2, u_3} u_{2,3}^2 + g_{w_{[]}}^2 w_{2,2} \\
& + g_{u_1} u_{1,2,3} + g_{u_2} u_{2,2,3} + g_{u_3} u_{2,3,3} \}
\end{aligned}$$

$$\begin{aligned}
& \text{> } \\
& \text{> } DeS := \text{numer}(\text{simplify}(\text{subs}(S2, \text{Pullback}(\text{deTR}, w_{1,3} - \text{TotalDiff}(\text{subs}(SI, w_3), 1)))) \\
DeS := & Ctt g_{u_1, u_2} u_{2,2}^2 Cxx + 2 Ctt g_{u_1, u_3} u_{2,3}^2 Cxy - Ctt^2 g_{u_1, w_{[]}} u_{1,2}^2 f_{u_1} - Ctt^2 g_{u_2, w_{[]}} u_{2,2}^2 f_{u_2} \\
& - Ctt^2 g_{u_3, w_{[]}} u_{2,3}^2 f_{u_3} - u_{1,2} Ctt^2 g_{u_2, u_2} u_{2,2} - u_{1,2} Ctt^2 g_{u_2, u_3} u_{2,3} - u_{1,2} Ctt^2 g_{u_2, w_{[]}} w_2 \\
& - u_{1,3} Ctt^2 g_{u_1, u_3} u_{1,2} - u_{1,3} Ctt^2 g_{u_2, u_3} u_{2,2} - u_{1,3} Ctt^2 g_{u_3, u_3} u_{2,3} - u_{1,3} Ctt^2 g_{u_3, w_{[]}} w_2 \\
& - g_{w_{[]}} Ctt^2 f_{u_1, u_1} u_{1,2}^2 - g_{w_{[]}} Ctt^2 f_{u_2, u_2} u_{2,2}^2 - g_{w_{[]}} Ctt^2 f_{u_3, u_3} u_{2,3}^2 - g_{w_{[]}} Ctt^2 f_{u_1} u_{1,2,2} \\
& - g_{w_{[]}} Ctt^2 f_{u_2} u_{2,2,2} - g_{w_{[]}} Ctt^2 f_{u_3} u_{2,2,3} + g_{u_1} Cxx u_{2,2}^2 Ctt + g_{u_1} Cxx u_{2,2,2} Ctt \\
& + g_{u_1} Cyy u_{2,3,3} Ctt + 2 g_{u_1} Ctx_{u_1} u_{1,2}^2 Ctt + 2 g_{u_1} Cxy_{u_3} u_{2,3}^2 Ctt + 2 g_{u_1} Ctx u_{1,2,2} Ctt \\
& + 2 g_{u_1} Cty u_{1,2,3} Ctt + 2 g_{u_1} Cxy u_{2,2,3} Ctt - 2 g_{u_1} u_{1,2}^2 Ctt_{u_1} Ctx - g_{u_1} u_{2,2}^2 Ctt_{u_2} Cxx
\end{aligned}$$

$$\begin{aligned}
& -2 g_{u_1} u_{2,3}^2 Ctt_{u_3} Cxy + f_{u_3, w} u_{2,3}^2 Ctt^2 g_{u_3} + f_{u_1, w} u_{1,2}^2 Ctt^2 g_{u_1} + f_{u_2, w} u_{2,2}^2 Ctt^2 g_{u_2} \\
& + u_{1,3} f_{u_1, u_2} u_{2,2} Ctt^2 + u_{1,3} f_{u_1, u_3} u_{2,3} Ctt^2 + u_{1,3} f_{u_1, w} w_2 Ctt^2 + u_{2,3} f_{u_1, u_2} u_{1,2} Ctt^2 \\
& + u_{2,3} f_{u_2, u_2} u_{2,2} Ctt^2 + u_{2,3} f_{u_2, w} w_2 Ctt^2 + u_{3,3} f_{u_1, u_3} u_{1,2} Ctt^2 + u_{3,3} f_{u_2, u_3} u_{2,2} Ctt^2 \\
& + u_{3,3} f_{u_3, u_3} u_{2,3} Ctt^2 + u_{3,3} f_{u_3, w} w_2 Ctt^2 + u_{1,3} f_{u_1, u_1} u_{1,2} Ctt^2 + f_{w} Ctt^2 g_{u_1, u_1} u_{1,2}^2 \\
& + f_{w} Ctt^2 g_{u_2, u_2} u_{2,2}^2 + f_{w} Ctt^2 g_{u_3, u_3} u_{2,3}^2 + f_{w} Ctt^2 g_{u_1} u_{1,2,2} + f_{w} Ctt^2 g_{u_2} u_{2,2,2} \\
& + f_{w} Ctt^2 g_{u_3} u_{2,2,3} + 2 Ctt g_{u_1, u_1} u_{1,2}^2 Ctx + g_{u_1} u_{1,2} Cyy_{u_1} u_{3,3} Ctt \\
& + g_{u_1} u_{2,2} Cyy_{u_2} u_{3,3} Ctt + g_{u_1} u_{2,3} Cxx_{u_3} u_{2,2} Ctt + g_{u_1} u_{2,3} Cyy_{u_3} u_{3,3} Ctt \\
& + 2 g_{u_1} u_{1,2} Cty_{u_1} u_{1,3} Ctt + 2 g_{u_1} u_{1,2} Cxy_{u_1} u_{2,3} Ctt + 2 g_{u_1} u_{2,2} Ctx_{u_2} u_{1,2} Ctt \\
& + 2 g_{u_1} u_{2,2} Cty_{u_2} u_{1,3} Ctt + 2 g_{u_1} u_{2,2} Cxy_{u_2} u_{2,3} Ctt + 2 g_{u_1} u_{2,3} Ctx_{u_3} u_{1,2} Ctt \\
& + 2 g_{u_1} u_{2,3} Cty_{u_3} u_{1,3} Ctt - 2 g_{u_1} u_{1,2} Ctt_{u_1} Cty u_{1,3} - g_{u_1} u_{1,2} Ctt_{u_1} Cxx u_{2,2} \\
& - 2 g_{u_1} u_{1,2} Ctt_{u_1} Cxy u_{2,3} - g_{u_1} u_{1,2} Ctt_{u_1} Cyy u_{3,3} - 2 g_{u_1} u_{2,2} Ctt_{u_2} Ctx u_{1,2} \\
& - 2 g_{u_1} u_{2,2} Ctt_{u_2} Cty u_{1,3} - 2 g_{u_1} u_{2,2} Ctt_{u_2} Cxy u_{2,3} - g_{u_1} u_{2,2} Ctt_{u_2} Cyy u_{3,3} \\
& + f_{w, w} w_2 Ctt^2 g_{u_3} u_{2,3} + f_{u_3, w} u_{2,3} Ctt^2 g_{u_1} u_{1,2} + f_{u_3, w} u_{2,3} Ctt^2 g_{u_2} u_{2,2} \\
& + f_{u_1, w} u_{1,2} Ctt^2 g_{u_2} u_{2,2} + f_{u_1, w} u_{1,2} Ctt^2 g_{u_3} u_{2,3} + f_{u_2, w} u_{2,2} Ctt^2 g_{u_1} u_{1,2} \\
& + f_{u_2, w} u_{2,2} Ctt^2 g_{u_3} u_{2,3} + 2 Ctt g_{u_1, u_1} u_{1,2} Cxy u_{2,3} + 2 Ctt g_{u_1, u_1} u_{1,2} Cty u_{1,3} \\
& + Ctt g_{u_1, u_1} u_{1,2} Cxx u_{2,2} + Ctt g_{u_1, u_1} u_{1,2} Cyy u_{3,3} + 2 Ctt g_{u_1, u_2} u_{2,2} Cxy u_{2,3} \\
& + 2 Ctt g_{u_1, u_2} u_{2,2} Ctx u_{1,2} + 2 f_{w} Ctt^2 u_{1,2} g_{u_1, u_2} u_{2,2} + 2 f_{w} Ctt^2 u_{1,2} g_{u_1, u_3} u_{2,3} \\
& + f_{w} Ctt^2 u_{1,2} g_{u_1, w} w_2 + 2 f_{w} Ctt^2 u_{2,2} g_{u_2, u_3} u_{2,3} + f_{w} Ctt^2 u_{2,2} g_{u_2, w} w_2 \\
& + f_{w} Ctt^2 u_{2,3} g_{u_3, w} w_2 - Ctt^2 g_{u_1, w} u_{1,2} f_{u_2} u_{2,2} - Ctt^2 g_{u_1, w} u_{1,2} f_{u_3} u_{2,3} \\
& - Ctt^2 g_{u_2, w} u_{2,2} f_{u_1} u_{1,2} - Ctt^2 g_{u_2, w} u_{2,2} f_{u_3} u_{2,3} - Ctt^2 g_{u_3, w} u_{2,3} f_{u_1} u_{1,2} \\
& - Ctt^2 g_{u_3, w} u_{2,3} f_{u_2} u_{2,2} - Ctt^2 g_{w, w} w_2 f_{u_1} u_{1,2} - Ctt^2 g_{w, w} w_2 f_{u_2} u_{2,2} \\
& - Ctt^2 g_{w, w} w_2 f_{u_3} u_{2,3} - 2 g_{w} Ctt^2 u_{1,2} f_{u_1, u_2} u_{2,2} - 2 g_{w} Ctt^2 u_{1,2} f_{u_1, u_3} u_{2,3} \\
& + 2 Ctt g_{u_1, u_2} u_{2,2} Cty u_{1,3} + Ctt g_{u_1, u_2} u_{2,2} Cyy u_{3,3} + 2 Ctt g_{u_1, u_3} u_{2,3} Ctx u_{1,2}
\end{aligned}$$

$$\begin{aligned}
& + 2 \text{Ctt} g_{u_1, u_3} u_{2,3} \text{Cty} u_{1,3} + \text{Ctt} g_{u_1, u_3} u_{2,3} \text{Cxx} u_{2,2} + \text{Ctt} g_{u_1, u_3} u_{2,3} \text{Cyy} u_{3,3} \\
& + 2 \text{Ctt} g_{u_1, w_{[]}} w_2 \text{Cxy} u_{2,3} + 2 \text{Ctt} g_{u_1, w_{[]}} w_2 \text{Ctx} u_{1,2} + 2 \text{Ctt} g_{u_1, w_{[]}} w_2 \text{Cty} u_{1,3} \\
& + \text{Ctt} g_{u_1, w_{[]}} w_2 \text{Cxx} u_{2,2} + \text{Ctt} g_{u_1, w_{[]}} w_2 \text{Cyy} u_{3,3} - g_{w_{[]}} \text{Ctt}^2 u_{1,2} f_{u_1, w_{[]}} w_2 \\
& - 2 g_{w_{[]}} \text{Ctt}^2 u_{2,2} f_{u_2, u_3} u_{2,3} - g_{w_{[]}} \text{Ctt}^2 u_{2,2} f_{u_2, w_{[]}} w_2 - g_{w_{[]}} \text{Ctt}^2 u_{2,3} f_{u_3, w_{[]}} w_2 \\
& + g_{u_1} u_{1,2} \text{Cxx} u_{1,2} \text{Ctt} - 2 g_{u_1} u_{2,3} \text{Ctt}_{u_3} \text{Ctx} u_{1,2} - 2 g_{u_1} u_{2,3} \text{Ctt}_{u_3} \text{Cty} u_{1,3} \\
& - g_{u_1} u_{2,3} \text{Ctt}_{u_3} \text{Cxx} u_{2,2} - g_{u_1} u_{2,3} \text{Ctt}_{u_3} \text{Cyy} u_{3,3} + f_{w_{[]}, w_{[]}} w_2 \text{Ctt}^2 g_{u_1} u_{1,2} \\
& + f_{w_{[]}, w_{[]}} w_2 \text{Ctt}^2 g_{u_2} u_{2,2} + f_{u_2, u_3} u_{2,3}^2 \text{Ctt}^2 + f_{u_1} u_{1,2,3} \text{Ctt}^2 + f_{u_2} u_{2,2,3} \text{Ctt}^2 + f_{u_3} u_{2,3,3} \text{Ctt}^2 \\
& - g_{u_2} u_{1,2,2} \text{Ctt}^2 - g_{u_3} u_{1,2,3} \text{Ctt}^2 - u_{1,2}^2 \text{Ctt}^2 g_{u_1, u_2}
\end{aligned}$$

This is the compatibility constraint, but it contains many conditions: all the coefficients of jets of u and w

>

$$Qn1 := \text{diff}(DeS, u_{1,2,2})$$

$$Qn1 := -g_{u_2} \text{Ctt}^2 + f_{w_{[]}} \text{Ctt}^2 g_{u_1} - g_{w_{[]}} \text{Ctt}^2 f_{u_1} + 2 g_{u_1} \text{Ctx} \text{Ctt} \quad (5)$$

$$Qn2 := \text{diff}(DeS, u_{1,2,3})$$

$$Qn2 := f_{u_1} \text{Ctt}^2 - g_{u_3} \text{Ctt}^2 + 2 g_{u_1} \text{Cty} \text{Ctt} \quad (6)$$

$$\text{diff}(DeS, u_{1,3,3})$$

$$0 \quad (7)$$

$$Qn3 := \text{diff}(DeS, u_{2,2,2})$$

$$Qn3 := f_{w_{[]}} \text{Ctt}^2 g_{u_2} - g_{w_{[]}} \text{Ctt}^2 f_{u_2} + g_{u_1} \text{Cxx} \text{Ctt} \quad (8)$$

$$Qn4 := \text{diff}(DeS, u_{2,2,3})$$

$$Qn4 := f_{u_2} \text{Ctt}^2 + f_{w_{[]}} \text{Ctt}^2 g_{u_3} - g_{w_{[]}} \text{Ctt}^2 f_{u_3} + 2 g_{u_1} \text{Cxy} \text{Ctt} \quad (9)$$

$$Qn5 := \text{diff}(DeS, u_{2,3,3})$$

$$Qn5 := f_{u_3} \text{Ctt}^2 + g_{u_1} \text{Cyy} \text{Ctt} \quad (10)$$

$$\text{diff}(DeS, u_{3,3,3})$$

$$0 \quad (11)$$

$$\text{diff}(DeS, w_{2,2})$$

$$0 \quad (12)$$

$$Qn6 := \text{diff}(DeS, u_{1,2}, u_{1,2})$$

$$Qn6 := -2 \text{Ctt}^2 g_{u_1, u_2} - 2 g_{w_{[]}} \text{Ctt}^2 f_{u_1, u_1} + 4 g_{u_1} \text{Ctx}_{u_1} \text{Ctt} - 4 g_{u_1} \text{Ctt}_{u_1} \text{Ctx} + 2 f_{u_1, w_{[]}} \text{Ctt}^2 g_{u_1} \quad (13)$$

$$+ 2 f_w \text{[]} C t t^2 g_{u_1, u_1} + 4 C t t g_{u_1, u_1} C t x - 2 C t t^2 g_{u_1, w} \text{[]} f_{u_1}$$

$$> Qn7 := \text{diff} (DeS, u_{1,2}, u_{1,3})$$

$$Qn7 := 2 g_{u_1} C t y_{u_1} C t t - 2 g_{u_1} C t t_{u_1} C t y + 2 C t t g_{u_1, u_1} C t y - C t t^2 g_{u_1, u_3} + f_{u_1, u_1} C t t^2 \quad (14)$$

$$> Qn8 := \text{diff} (DeS, u_{1,2}, u_{2,2})$$

$$Qn8 := -C t t^2 g_{u_2, w} \text{[]} f_{u_1} - 2 g_w \text{[]} C t t^2 f_{u_1, u_2} + g_{u_1} C x x_{u_1} C t t + 2 g_{u_1} C t x_{u_2} C t t - g_{u_1} C t t_{u_1} C x x \quad (15)$$

$$- 2 g_{u_1} C t t_{u_2} C t x + f_{u_1, w} \text{[]} C t t^2 g_{u_2} + f_{u_2, w} \text{[]} C t t^2 g_{u_1} + C t t g_{u_1, u_1} C x x + 2 C t t g_{u_1, u_2} C t x$$

$$+ 2 f_w \text{[]} C t t^2 g_{u_1, u_2} - C t t^2 g_{u_1, w} \text{[]} f_{u_2} - C t t^2 g_{u_2, u_2}$$

$$> Qn9 := \text{diff} (DeS, u_{1,2}, u_{2,3})$$

$$Qn9 := -C t t^2 g_{u_1, w} \text{[]} f_{u_3} - C t t^2 g_{u_3, w} \text{[]} f_{u_1} - 2 g_w \text{[]} C t t^2 f_{u_1, u_3} + 2 C t t g_{u_1, u_3} C t x + 2 g_{u_1} C x y_{u_1} C t t \quad (16)$$

$$+ 2 g_{u_1} C t x_{u_3} C t t - 2 g_{u_1} C t t_{u_1} C x y - 2 g_{u_1} C t t_{u_3} C t x + f_{u_3, w} \text{[]} C t t^2 g_{u_1} + f_{u_1, w} \text{[]} C t t^2 g_{u_3}$$

$$+ 2 C t t g_{u_1, u_1} C x y + 2 f_w \text{[]} C t t^2 g_{u_1, u_3} - C t t^2 g_{u_2, u_3} + f_{u_1, u_2} C t t^2$$

$$> Qn10 := \text{diff} (DeS, u_{1,2}, u_{3,3})$$

$$Qn10 := g_{u_1} C y y_{u_1} C t t - g_{u_1} C t t_{u_1} C y y + C t t g_{u_1, u_1} C y y + f_{u_1, u_3} C t t^2 \quad (17)$$

$$> \text{diff} (DeS, u_{1,3}, u_{1,3})$$

$$0 \quad (18)$$

$$> Qn11 := \text{diff} (DeS, u_{1,3}, u_{2,2})$$

$$Qn11 := -C t t^2 g_{u_2, u_3} + f_{u_1, u_2} C t t^2 + 2 C t t g_{u_1, u_2} C t y + 2 g_{u_1} C t y_{u_2} C t t - 2 g_{u_1} C t t_{u_2} C t y \quad (19)$$

$$> Qn12 := \text{diff} (DeS, u_{1,3}, u_{2,3})$$

$$Qn12 := -C t t^2 g_{u_3, u_3} + f_{u_1, u_3} C t t^2 - 2 g_{u_1} C t t_{u_3} C t y + 2 C t t g_{u_1, u_3} C t y + 2 g_{u_1} C t y_{u_3} C t t \quad (20)$$

$$> \text{diff} (DeS, u_{1,3}, u_{3,3})$$

$$0 \quad (21)$$

$$> Qn13 := \text{diff} (DeS, u_{2,2}, u_{2,2})$$

$$Qn13 := 2 f_{u_2, w} \text{[]} C t t^2 g_{u_2} + 2 f_w \text{[]} C t t^2 g_{u_2, u_2} + 2 C t t g_{u_1, u_2} C x x - 2 C t t^2 g_{u_2, w} \text{[]} f_{u_2} \quad (22)$$

$$- 2 g_w \text{[]} C t t^2 f_{u_2, u_2} + 2 g_{u_1} C x x_{u_2} C t t - 2 g_{u_1} C t t_{u_2} C x x$$

$$> Qn14 := \text{diff} (DeS, u_{2,2}, u_{2,3})$$

$$Qn14 := f_{u_2, u_2} C t t^2 - g_{u_1} C t t_{u_3} C x x + f_{u_3, w} \text{[]} C t t^2 g_{u_2} + f_{u_2, w} \text{[]} C t t^2 g_{u_3} + 2 C t t g_{u_1, u_2} C x y \quad (23)$$

$$+ 2 f_w \text{[]} C t t^2 g_{u_2, u_3} - C t t^2 g_{u_2, w} \text{[]} f_{u_3} - C t t^2 g_{u_3, w} \text{[]} f_{u_2} + C t t g_{u_1, u_3} C x x - 2 g_w \text{[]} C t t^2 f_{u_2, u_3}$$

$$+ g_{u_1} Cxx_{u_3} Ctt + 2 g_{u_1} Cxy_{u_2} Ctt - 2 g_{u_1} Ctt_{u_2} Cxy$$

$$> Qn15 := \text{diff}(DeS, u_{2,2}, u_{3,3})$$

$$Qn15 := f_{u_2, u_3} Ctt^2 + Ctt g_{u_1, u_2} Cyy + g_{u_1} Cyy_{u_2} Ctt - g_{u_1} Ctt_{u_2} Cyy \quad (24)$$

$$> Qn16 := \text{diff}(DeS, u_{2,3}, u_{2,3})$$

$$Qn16 := 2 f_{u_2, u_3} Ctt^2 + 2 f_{w[]} Ctt^2 g_{u_3, u_3} + 4 Ctt g_{u_1, u_3} Cxy - 2 Ctt^2 g_{u_3, w[]} f_{u_3} - 2 g_{w[]} Ctt^2 f_{u_3, u_3} \\ + 4 g_{u_1} Cxy_{u_3} Ctt - 4 g_{u_1} Ctt_{u_3} Cxy + 2 f_{u_3, w[]} Ctt^2 g_{u_3} \quad (25)$$

$$> Qn17 := \text{diff}(DeS, u_{2,3}, u_{3,3})$$

$$Qn17 := f_{u_3, u_3} Ctt^2 + Ctt g_{u_1, u_3} Cyy + g_{u_1} Cyy_{u_3} Ctt - g_{u_1} Ctt_{u_3} Cyy \quad (26)$$

$$> \text{diff}(DeS, u_{3,3}, u_{3,3})$$

$$0 \quad (27)$$

$$> Qn18 := \text{diff}(DeS, u_{1,2}, w_2)$$

$$Qn18 := -Ctt^2 g_{w[], w[]} f_{u_1} + 2 Ctt g_{u_1, w[]} Ctx - g_{w[]} Ctt^2 f_{u_1, w[]} + f_{w[], w[]} Ctt^2 g_{u_1} \\ + f_{w[]} Ctt^2 g_{u_1, w[]} - Ctt^2 g_{u_2, w[]} \quad (28)$$

$$> Qn19 := \text{diff}(DeS, u_{1,3}, w_2)$$

$$Qn19 := f_{u_1, w[]} Ctt^2 - Ctt^2 g_{u_3, w[]} + 2 Ctt g_{u_1, w[]} Cty \quad (29)$$

$$> Qn20 := \text{diff}(DeS, u_{2,2}, w_2)$$

$$Qn20 := f_{w[], w[]} Ctt^2 g_{u_2} + f_{w[]} Ctt^2 g_{u_2, w[]} - Ctt^2 g_{w[], w[]} f_{u_2} + Ctt g_{u_1, w[]} Cxx \\ - g_{w[]} Ctt^2 f_{u_2, w[]} \quad (30)$$

$$> Qn21 := \text{diff}(DeS, u_{2,3}, w_2)$$

$$Qn21 := f_{u_2, w[]} Ctt^2 + f_{w[]} Ctt^2 g_{u_3, w[]} - Ctt^2 g_{w[], w[]} f_{u_3} + 2 Ctt g_{u_1, w[]} Cxy - g_{w[]} Ctt^2 f_{u_3, w[]} \\ + f_{w[], w[]} Ctt^2 g_{u_3} \quad (31)$$

$$> Qn22 := \text{diff}(DeS, u_{3,3}, w_2)$$

$$Qn22 := f_{u_3, w[]} Ctt^2 + Ctt g_{u_1, w[]} Cyy \quad (32)$$

$$> \text{diff}(DeS, w_2, w_2)$$

$$0 \quad (33)$$

$$> DpVar := [f(u_1, u_2, u_3, w[]), g(u_1, u_2, u_3, w[])]:$$

$$> Qn := \text{ToJet}([Qn1, Qn2, Qn3, Qn4, Qn5, Qn6, Qn7, Qn8, Qn9, Qn10, Qn11, Qn12, Qn13, Qn14, \\ Qn15, Qn16, Qn17, Qn18, Qn19, Qn20, Qn21, Qn22], DpVar, \text{notation} = \text{jetnumbers})$$

$$(34)$$

$$\begin{aligned}
Qn := & \left[ -g_2 Ctt^2 + f_4 Ctt^2 g_1 - g_4 Ctt^2 f_1 + 2 g_1 Ctx Ctt, f_1 Ctt^2 - g_3 Ctt^2 + 2 g_1 Cty Ctt, f_4 Ctt^2 g_2 \right. \\
& - g_4 Ctt^2 f_2 + g_1 Cxx Ctt, f_2 Ctt^2 + f_4 Ctt^2 g_3 - g_4 Ctt^2 f_3 + 2 g_1 Cxy Ctt, f_3 Ctt^2 + g_1 Cyy Ctt, \\
& - 2 Ctt^2 g_{1,2} - 2 g_4 Ctt^2 f_{1,1} + 4 g_1 Ctx_{u_1} Ctt - 4 g_1 Ctt_{u_1} Ctx + 2 f_{1,4} Ctt^2 g_1 + 2 f_4 Ctt^2 g_{1,1} \\
& + 4 Ctt g_{1,1} Ctx - 2 Ctt^2 g_{1,4} f_{1,2} g_1 Cty_{u_1} Ctt - 2 g_1 Ctt_{u_1} Cty + 2 Ctt g_{1,1} Cty - Ctt^2 g_{1,3} \\
& + f_{1,1} Ctt^2, - Ctt^2 g_{2,4} f_1 - 2 g_4 Ctt^2 f_{1,2} + g_1 Cxx_{u_1} Ctt + 2 g_1 Ctx_{u_2} Ctt - g_1 Ctt_{u_1} Cxx \\
& - 2 g_1 Ctt_{u_2} Ctx + f_{1,4} Ctt^2 g_2 + f_{2,4} Ctt^2 g_1 + Ctt g_{1,1} Cxx + 2 Ctt g_{1,2} Ctx + 2 f_4 Ctt^2 g_{1,2} \\
& - Ctt^2 g_{1,4} f_2 - Ctt^2 g_{2,2}, - Ctt^2 g_{1,4} f_3 - Ctt^2 g_{3,4} f_1 - 2 g_4 Ctt^2 f_{1,3} + 2 Ctt g_{1,3} Ctx \\
& + 2 g_1 Cxy_{u_1} Ctt + 2 g_1 Ctx_{u_3} Ctt - 2 g_1 Ctt_{u_1} Cxy - 2 g_1 Ctt_{u_3} Ctx + f_{3,4} Ctt^2 g_1 + f_{1,4} Ctt^2 g_3 \\
& + 2 Ctt g_{1,1} Cxy + 2 f_4 Ctt^2 g_{1,3} - Ctt^2 g_{2,3} + f_{1,2} Ctt^2, g_1 Cyy_{u_1} Ctt - g_1 Ctt_{u_1} Cyy \\
& + Ctt g_{1,1} Cyy + f_{1,3} Ctt^2, - Ctt^2 g_{2,3} + f_{1,2} Ctt^2 + 2 Ctt g_{1,2} Cty + 2 g_1 Cty_{u_2} Ctt \\
& - 2 g_1 Ctt_{u_2} Cty, - Ctt^2 g_{3,3} + f_{1,3} Ctt^2 - 2 g_1 Ctt_{u_3} Cty + 2 Ctt g_{1,3} Cty + 2 g_1 Cty_{u_3} Ctt, \\
& 2 f_{2,4} Ctt^2 g_2 + 2 f_4 Ctt^2 g_{2,2} + 2 Ctt g_{1,2} Cxx - 2 Ctt^2 g_{2,4} f_2 - 2 g_4 Ctt^2 f_{2,2} + 2 g_1 Cxx_{u_2} Ctt \\
& - 2 g_1 Ctt_{u_2} Cxx, f_{2,2} Ctt^2 - g_1 Ctt_{u_3} Cxx + f_{3,4} Ctt^2 g_2 + f_{2,4} Ctt^2 g_3 + 2 Ctt g_{1,2} Cxy \\
& + 2 f_4 Ctt^2 g_{2,3} - Ctt^2 g_{2,4} f_3 - Ctt^2 g_{3,4} f_2 + Ctt g_{1,3} Cxx - 2 g_4 Ctt^2 f_{2,3} + g_1 Cxx_{u_3} Ctt \\
& + 2 g_1 Cxy_{u_2} Ctt - 2 g_1 Ctt_{u_2} Cxy, f_{2,3} Ctt^2 + Ctt g_{1,2} Cyy + g_1 Cyy_{u_2} Ctt - g_1 Ctt_{u_2} Cyy, \\
& 2 f_{2,3} Ctt^2 + 2 f_4 Ctt^2 g_{3,3} + 4 Ctt g_{1,3} Cxy - 2 Ctt^2 g_{3,4} f_3 - 2 g_4 Ctt^2 f_{3,3} + 4 g_1 Cxy_{u_3} Ctt \\
& - 4 g_1 Ctt_{u_3} Cxy + 2 f_{3,4} Ctt^2 g_{3,3} f_{3,3} Ctt^2 + Ctt g_{1,3} Cyy + g_1 Cyy_{u_3} Ctt - g_1 Ctt_{u_3} Cyy, \\
& - Ctt^2 g_{4,4} f_1 + 2 Ctt g_{1,4} Ctx - g_4 Ctt^2 f_{1,4} + f_{4,4} Ctt^2 g_1 + f_4 Ctt^2 g_{1,4} - Ctt^2 g_{2,4} f_{1,4} Ctt^2 \\
& - Ctt^2 g_{3,4} + 2 Ctt g_{1,4} Cty, f_{4,4} Ctt^2 g_2 + f_4 Ctt^2 g_{2,4} - Ctt^2 g_{4,4} f_2 + Ctt g_{1,4} Cxx \\
& - g_4 Ctt^2 f_{2,4} f_{2,4} Ctt^2 + f_4 Ctt^2 g_{3,4} - Ctt^2 g_{4,4} f_3 + 2 Ctt g_{1,4} Cxy - g_4 Ctt^2 f_{3,4} \\
& + f_{4,4} Ctt^2 g_{3,4} f_{3,4} Ctt^2 + Ctt g_{1,4} Cyy]
\end{aligned}$$

We got the required eqns and hereafter we shall resolve them, making the compatibility into a substitution

$$Svl0 := solve([Qn[1], Qn[2], Qn[3], Qn[4], Qn[5]], [f_1, f_2, f_3, g_1, g_2, g_3])$$

$$Svl0 := [ [f_1 = g_3, f_2 = -f_4 g_3, f_3 = 0, g_1 = 0, g_2 = -g_4 g_3, g_3 = g_3] ] \quad (35)$$

$$> Svl0 := solve([Qn[1], Qn[2], Qn[3], Qn[4], Qn[5]], [f_1, f_2, f_3, f_4, g_1, g_2, g_3, g_4])$$

$$Svl0 := \left[ [f_1 = g_3, f_2 = -f_4 g_3, f_3 = 0, f_4 = f_4, g_1 = 0, g_2 = -g_4 g_3, g_3 = g_3, g_4 = g_4], \left[ f_1 \right. \right. \quad (36)$$

$$\begin{aligned} &= \frac{g_3 Ctt - 2 g_1 Cty}{Ctt}, f_2 = -\frac{1}{Ctt} \left( RootOf(-Z^2 Ctt + (2 Ctx + 2 g_4 Cty) -Z + g_4^2 Cyy \right. \\ &+ 2 g_4 Cxy + Cxx) Ctt g_3 + g_4 g_1 Cyy + 2 g_1 Cxy \Big), f_3 = -\frac{g_1 Cyy}{Ctt}, f_4 = RootOf(-Z^2 Ctt \\ &+ (2 Ctx + 2 g_4 Cty) -Z + g_4^2 Cyy + 2 g_4 Cxy + Cxx), g_1 = g_1, g_2 = \frac{1}{Ctt} \left( -g_4 g_3 Ctt \right. \\ &+ 2 g_4 g_1 Cty + RootOf(-Z^2 Ctt + (2 Ctx + 2 g_4 Cty) -Z + g_4^2 Cyy + 2 g_4 Cxy \\ &+ Cxx) Ctt g_1 + 2 g_1 Ctx \Big), g_3 = g_3, g_4 = g_4 \Big] \end{aligned}$$

$$> expand(subs([g_1 = -k \cdot Ctt, g_3 = p - k \cdot Cty], Svl0[2])[1]);$$

$$simplify\left(subs\left([g_1 = -k \cdot Ctt, g_3 = p - k \cdot Cty], f_2 = -\frac{f_4 Ctt g_3 + g_4 g_1 Cyy + 2 g_1 Cxy}{Ctt}\right)\right);$$

$$expand(subs([g_1 = -k \cdot Ctt, g_3 = p - k \cdot Cty], Svl0[2])[3]);$$

$$simplify\left(subs\left([g_1 = -k \cdot Ctt, g_3 = p - k \cdot Cty], g_2 = \frac{-g_4 g_3 Ctt + 2 g_4 g_1 Cty + f_4 Ctt g_1 + 2 g_1 Ctx}{Ctt}\right)\right)$$

$$f_1 = p + k Cty$$

$$f_2 = -f_4 p + f_4 k Cty + g_4 k Cyy + 2 k Cxy$$

$$f_3 = k Cyy$$

$$g_2 = -g_4 p - g_4 k Cty - f_4 Ctt k - 2 k Ctx$$

(37)

>

>

$$> DGsetup([u_1, u_2, u_3, w[]], [f, g, k, p], TEQ, 2) :$$

$$> SB0 := \{f_1 = p[] + k[] \cdot Cty(u_1, u_2, u_3), f_2 = -f_4 p[] + f_4 k[] \cdot Cty(u_1, u_2, u_3) + g_4 k[] \cdot Cyy(u_1, u_2, u_3) + 2 k[] \cdot Cxy(u_1, u_2, u_3), f_3 = k[] \cdot Cyy(u_1, u_2, u_3), g_1 = -k[] \cdot Ctt(u_1, u_2, u_3), g_2 = -g_4 p[] - g_4 k[] \cdot Cty(u_1, u_2, u_3) - f_4 k[] \cdot Ctt(u_1, u_2, u_3) - 2 k[] \cdot Ctx(u_1, u_2, u_3), g_3 = p[] - k[] \cdot Cty(u_1, u_2, u_3)\}$$

$$SB0 := \{f_1 = p[] + k[] Cty, f_2 = -f_4 p[] + f_4 k[] Cty + g_4 k[] Cyy + 2 k[] Cxy, f_3 = k[] Cyy, g_1 = -k[] Ctt, g_2 = -g_4 p[] - g_4 k[] Cty - f_4 k[] Ctt - 2 k[] Ctx, g_3 = p[] - k[] Cty\} \quad (38)$$

$$> simplify\left(subs\left(SB0, \left[Qn[1], Qn[2], -\frac{Qn[3]}{k[] \cdot Ctt(u_1, u_2, u_3)^2}, Qn[4], Qn[5]\right]\right)\right)$$

$$\left[0, 0, 2 f_4 g_4 Cty + f_4^2 Ctt + 2 f_4 Ctx + g_4^2 Cyy + 2 g_4 Cxy + Cxx, 0, 0\right] \quad (39)$$

$$> SB0a := \{Cxx(u_1, u_2, u_3) = -(2 f_4 g_4 Cty(u_1, u_2, u_3) + f_4^2 Ctt(u_1, u_2, u_3) + 2 f_4 Ctx(u_1, u_2, u_3))$$



$$+ g_4^2 Cyy(u_1, u_2, u_3) + 2 g_4 Cxy(u_1, u_2, u_3) \} \\ SB0a := \{ Cxx = -2 f_4 g_4 Cty - f_4^2 Ctt - 2 f_4 Ctx - g_4^2 Cyy - 2 g_4 Cxy \} \quad (40)$$

```
> dE1 := DifferentialEquationData([SB0[1], SB0[4]], [f1, g1]) : dE1a := Prolong(dE1, 1) :
dETR1 := Transformation(dE1a) :
> dE2 := DifferentialEquationData([SB0[2], SB0[5]], [f2, g2]) : dE2a := Prolong(dE2, 1) :
dETR2 := Transformation(dE2a) :
> dE3 := DifferentialEquationData([SB0[3], SB0[6]], [f3, g3]) : dE3a := Prolong(dE3, 1) :
dETR3 := Transformation(dE3a) :
```

```
> DC1 := simplify(Pullback(dETR3, Pullback(dETR2, Pullback(dETR1, Pullback(dETR1, f1, 2)
- Pullback(dETR2, f1, 2))))))
DC1 := k1 Cty2 + Cty k2 + p2 - f4 k1 Ctyu1 - g4 k1 Cyyu1 - 2 k1 Cxyu1 - k1 f4 Cty + p1 k4 Cty
+ p1 p4 - k1 Cty2 k4 - k1 Cty p4 + k1 Cyy k4 Ctt - k1 g4 Cyy - 2 k1 Cxy + f4 p1 \quad (41)
```

```
> DC2 := simplify(Pullback(dETR3, Pullback(dETR2, Pullback(dETR1, Pullback(dETR1, g1, 2)
- Pullback(dETR2, g1, 2))))))
DC2 := -k1 Cttu2 - Ctt k2 + g4 k1 Ctyu1 + f4 k1 Cttu1 + 2 k1 Ctxu1 + k1 Ctt p4 + k1 f4 Ctt
- p1 k4 Ctt + k1 g4 Cty + 2 k1 Ctx + g4 p1 \quad (42)
```

```
> DC3 := simplify(Pullback(dETR3, Pullback(dETR2, Pullback(dETR1, Pullback(dETR1, f1, 3)
- Pullback(dETR3, f1, 3))))))
DC3 := k1 Ctyu3 + Cty k3 + p3 - k1 Cyyu1 - k1 Cyy \quad (43)
```

```
> DC4 := simplify(Pullback(dETR3, Pullback(dETR2, Pullback(dETR1, Pullback(dETR1, g1, 3)
- Pullback(dETR3, g1, 3))))))
DC4 := -k1 Cttu3 - Ctt k3 + k1 Ctyu1 + Cty k1 - p1 \quad (44)
```

```
> DC5 := simplify(Pullback(dETR3, Pullback(dETR2, Pullback(dETR1, Pullback(dETR2, f2, 3)
- Pullback(dETR3, f2, 3))))))
DC5 := f4 k1 Ctyu3 + g4 k1 Cyyu3 + 2 k1 Cxyu3 + k3 f4 Cty - p1 k4 Cyy + k1 Cyy p4 + k3 g4 Cyy
+ 2 k3 Cxy - f4 p3 - k1 Cyyu2 - k2 Cyy \quad (45)
```

```
> DC6 := simplify(Pullback(dETR3, Pullback(dETR2, Pullback(dETR1, Pullback(dETR2, g2, 3)
- Pullback(dETR3, g2, 3))))))
DC6 := -g4 k1 Ctyu3 - f4 k1 Cttu3 - 2 k1 Ctxu3 - k1 Cyy k4 Ctt - k3 f4 Ctt + p1 k4 Cty - p1 p4
+ k1 Cty2 k4 - k1 Cty p4 - k3 g4 Cty - 2 k3 Ctx - g4 p3 + k1 Ctyu2 + Cty k2 - p2 \quad (46)
```

$$\begin{aligned}
& \text{KP} := \text{solve}([DC1=0, DC2=0, DC3=0, DC4=0, DC5=0, DC6=0], [k_1, k_2, k_3, k_4, p_1, p_2, p_3, \\
& \quad p_4]) : \\
& \text{SB0b} := \{ \text{diff}(Cxx(u_1, u_2, u_3), u_1) = \text{simplify}(\text{Pullback}(dETR1, \text{TotalDiff}(\text{subs}(SB0a, \\
& \quad Cxx(u_1, u_2, u_3)), 1))), \text{diff}(Cxx(u_1, u_2, u_3), u_2) = \text{simplify}(\text{Pullback}(dETR2, \\
& \quad \text{TotalDiff}(\text{subs}(SB0a, Cxx(u_1, u_2, u_3)), 2))), \text{diff}(Cxx(u_1, u_2, u_3), u_3) \\
& \quad = \text{simplify}(\text{Pullback}(dETR3, \text{TotalDiff}(\text{subs}(SB0a, Cxx(u_1, u_2, u_3)), 3))) \} : \\
& \text{SB0c} := \{ f_{4,4} = \text{solve}(\text{TotalDiff}(\text{subs}(SB0a, Cxx(u_1, u_2, u_3)), 4) = 0, f_{4,4}) \} \\
& \quad \text{SB0c} := \left\{ f_{4,4} = - \frac{g_{4,4} (f_4 C_{ty} + g_4 C_{yy} + C_{xy})}{g_4 C_{ty} + f_4 C_{tt} + C_{tx}} \right\} \tag{47}
\end{aligned}$$

$$\begin{aligned}
& \text{SB0p} := \{ \text{op}(SB0), \text{op}(SB0a), \text{op}(SB0b), \text{op}(SB0c) \} \\
& \text{SB0p} := \left\{ Cxx = -2 f_4 g_4 C_{ty} - f_4^2 C_{tt} - 2 f_4 C_{tx} - g_4^2 C_{yy} - 2 g_4 C_{xy}, Cxx_{u_1} = -2 f_4 g_4 C_{ty_{u_1}} - \right. \tag{48} \\
& \quad f_4^2 C_{tt_{u_1}} - 2 f_4 C_{tx_{u_1}} - g_4^2 C_{yy_{u_1}} - 2 g_4 C_{xy_{u_1}} - 2 C_{ty}^2 k_4 g_4 - 2 C_{ty} g_4 p_4 - 2 C_{tt} f_4 p_4 \\
& \quad - 2 C_{ty} k_4 C_{tx} - 2 C_{tx} p_4 + 2 C_{tt} k_4 g_4 C_{yy} + 2 C_{tt} k_4 C_{xy}, Cxx_{u_2} = 2 C_{xy} g_4 p_4 + 2 f_4^2 C_{tt} p_4 \\
& \quad + 2 C_{tx} f_{4,4} p_{[]} + 2 C_{tx} f_4 p_4 + 2 g_4^2 C_{yy} p_4 + 2 C_{xy} g_{4,4} p_{[]} - 2 f_4 g_4 C_{ty_{u_2}} - f_4^2 C_{tt_{u_2}} \\
& \quad - 2 f_4 C_{tx_{u_2}} - g_4^2 C_{yy_{u_2}} - 2 g_4 C_{xy_{u_2}} - 2 f_4 C_{tt} k_{[]} C_{yy} g_{4,4} + 2 g_4 C_{yy} k_{[]} C_{tt} f_{4,4} \\
& \quad + 2 C_{xy} g_{4,4} k_{[]} C_{ty} + 2 g_4 C_{ty} f_{4,4} p_{[]} - 2 g_4 C_{ty}^2 f_{4,4} k_{[]} - 2 g_4 C_{ty} k_4 C_{xy} + 4 g_4 C_{ty} f_4 p_4 \\
& \quad + 2 f_4 C_{tt} f_{4,4} p_{[]} - 2 f_4 C_{tt} k_4 C_{xy} + 2 C_{tx} k_4 f_4 C_{ty} - 2 C_{tx} f_{4,4} k_{[]} C_{ty} - 2 C_{tx} k_{[]} C_{yy} g_{4,4} \\
& \quad + 2 C_{tx} k_4 g_4 C_{yy} + 2 f_4 C_{ty} g_{4,4} p_{[]} + 2 f_4 C_{ty}^2 g_{4,4} k_{[]} + 2 g_4 C_{yy} g_{4,4} p_{[]} \\
& \quad + 2 C_{xy} k_{[]} C_{tt} f_{4,4}, Cxx_{u_3} = -2 f_4 g_4 C_{ty_{u_3}} - f_4^2 C_{tt_{u_3}} - 2 f_4 C_{tx_{u_3}} - g_4^2 C_{yy_{u_3}} - 2 g_4 C_{xy_{u_3}} \\
& \quad - 2 C_{yy} k_4 f_4 C_{tt} - 2 C_{yy} k_4 C_{tx} + 2 C_{ty}^2 k_4 f_4 - 2 C_{ty} f_4 p_4 - 2 C_{yy} g_4 p_4 + 2 C_{ty} k_4 C_{xy} \\
& \quad - 2 C_{xy} p_4, f_1 = p_{[]} + k_{[]} C_{ty}, f_2 = -f_4 p_{[]} + f_4 k_{[]} C_{ty} + g_4 k_{[]} C_{yy} + 2 k_{[]} C_{xy}, f_3 = k_{[]} C_{yy}, \\
& \quad f_{4,4} = - \frac{g_{4,4} (f_4 C_{ty} + g_4 C_{yy} + C_{xy})}{g_4 C_{ty} + f_4 C_{tt} + C_{tx}}, g_1 = -k_{[]} C_{tt}, g_2 = -g_4 p_{[]} - g_4 k_{[]} C_{ty} - f_4 k_{[]} C_{tt}
\end{aligned}$$

$$\left. -2 k_{[]} Ctx, g_3 = p_{[]} - k_{[]} Cty \right\}$$

$$\begin{aligned} &> \text{subs}(SB0p, \text{diff}(Cxx(u_1, u_2, u_3), u_1)) \\ &-2 f_4 g_4 Cty_{u_1} - f_4^2 Ctt_{u_1} - 2 f_4 Ctx_{u_1} - g_4^2 Cyy_{u_1} - 2 g_4 Cxy_{u_1} - 2 Cty^2 k_4 g_4 - 2 Cty g_4 p_4 \\ &- 2 Ctt f_4 p_4 - 2 Cty k_4 Ctx - 2 Ctx p_4 + 2 Ctt k_4 g_4 Cyy + 2 Ctt k_4 Cxy \end{aligned} \quad (49)$$

$$\begin{aligned} &> KPI := \text{solve}([DC1=0, DC2=0, DC3=0, DC4=0, DC5=0, DC6=0, \\ &\text{simplify}(\text{Pullback}(dETR1, \text{TotalDiff}(\text{subs}(SB0a, Cxx(u_1, u_2, u_3)), 1)) = \text{diff}(Cxx(u_1, \\ &u_2, u_3), u_1), \text{simplify}(\text{Pullback}(dETR2, \text{TotalDiff}(\text{subs}(SB0a, Cxx(u_1, u_2, u_3)), 2)) = \\ &\text{diff}(Cxx(u_1, u_2, u_3), u_2), \text{simplify}(\text{Pullback}(dETR3, \text{TotalDiff}(\text{subs}(SB0a, Cxx(u_1, u_2, \\ &u_3)), 3)) = \text{diff}(Cxx(u_1, u_2, u_3), u_3)], [k_1, k_2, k_3, k_4, p_1, p_2, p_3, p_4, f_4, g_4, 4]) : \end{aligned}$$

$$\begin{aligned} &> KPI[1] \\ &> \text{simplify}(\text{subs}(SB0p, \text{subs}(KP[1], \text{Pullback}(dETR3, \text{Pullback}(dETR2, \text{Pullback}(dETR1, \\ &\text{subs}(SB0p, [Qn[1], Qn[2], Qn[3], Qn[4], Qn[5], Qn[6], Qn[7], Qn[8], Qn[9], Qn[10], \\ &Qn[11], Qn[12], Qn[13], Qn[14], Qn[15], Qn[16], Qn[17], Qn[18], Qn[19], Qn[20], \\ &Qn[21], Qn[22]])))))) \end{aligned} \quad (50)$$

Done: here I was not elegant, and we have several substitutions instead of one, but anyway all of them encode compatibility condition for the pseudopotential and else.

Let us now check that X,Y form a Lax pair in 4D:

$$\begin{aligned} &> DGsetup([t, x, y], [u], LI, 2) : \\ &> SeD0 := \text{simplify}\left(\text{subs}\left(S2, \text{Pullback}\left(\text{deTR}, -\text{TotalDiff}\left(\frac{\partial}{\partial w_{[]}} g(u_1, u_2, u_3, w_{[]}), 1\right) \right. \right. \\ &\quad + \frac{\partial}{\partial w_{[]}} f(u_1, u_2, u_3, w_{[]}) \cdot \text{TotalDiff}\left(\frac{\partial}{\partial w_{[]}} g(u_1, u_2, u_3, w_{[]}), 2\right) - \left(\left(\frac{\partial}{\partial u_1} f(u_1, u_2, u_3, \right. \right. \\ &\quad w_{[]})\right) u_{1,2} + \left(\frac{\partial}{\partial u_2} f(u_1, u_2, u_3, w_{[]})\right) u_{2,2} + \left(\frac{\partial}{\partial u_3} f(u_1, u_2, u_3, w_{[]})\right) u_{2,3} \\ &\quad \cdot \frac{\partial^2}{\partial w_{[]}^2} g(u_1, u_2, u_3, w_{[]}) + \text{TotalDiff}\left(\frac{\partial}{\partial w_{[]}} f(u_1, u_2, u_3, w_{[]}), 3\right) - \frac{\partial}{\partial w_{[]}} g(u_1, u_2, u_3, \\ &\quad w_{[]}) \cdot \text{TotalDiff}\left(\frac{\partial}{\partial w_{[]}} f(u_1, u_2, u_3, w_{[]}), 2\right) + \left(\left(\frac{\partial}{\partial u_1} g(u_1, u_2, u_3, w_{[]})\right) u_{1,2} \right. \\ &\quad + \left(\frac{\partial}{\partial u_2} g(u_1, u_2, u_3, w_{[]})\right) u_{2,2} + \left(\frac{\partial}{\partial u_3} g(u_1, u_2, u_3, w_{[]})\right) u_{2,3} \cdot \frac{\partial^2}{\partial w_{[]}^2} f(u_1, u_2, u_3, \\ &\quad w_{[]}) \left. \left. \left. \right) \right) \right) \end{aligned}$$

$$\begin{aligned}
SeD0 := & \frac{1}{Ctt} \left( 2 g_{u_1, w[]} Cxy u_{2,3} + 2 g_{u_1, w[]} Ctx u_{1,2} + 2 g_{u_1, w[]} Cty u_{1,3} + g_{u_1, w[]} Cxx u_{2,2} \right. \\
& + g_{u_1, w[]} Cyy u_{3,3} - g_{u_2, w[]} u_{1,2} Ctt - g_{u_3, w[]} u_{1,3} Ctt + f_{w[]} Ctt g_{u_1, w[]} u_{1,2} \\
& + f_{w[]} Ctt g_{u_2, w[]} u_{2,2} + f_{w[]} Ctt g_{u_3, w[]} u_{2,3} - g_{w[], w[]} Ctt f_{u_1} u_{1,2} - g_{w[], w[]} Ctt f_{u_2} u_{2,2} \\
& - g_{w[], w[]} Ctt f_{u_3} u_{2,3} + u_{1,3} f_{u_1, w[]} Ctt + u_{2,3} f_{u_2, w[]} Ctt + u_{3,3} f_{u_3, w[]} Ctt \\
& - g_{w[]} Ctt f_{u_1, w[]} u_{1,2} - g_{w[]} Ctt f_{u_2, w[]} u_{2,2} - g_{w[]} Ctt f_{u_3, w[]} u_{2,3} + f_{w[], w[]} Ctt g_{u_1} u_{1,2} \\
& \left. + f_{w[], w[]} Ctt g_{u_2} u_{2,2} + f_{w[], w[]} Ctt g_{u_3} u_{2,3} \right)
\end{aligned} \tag{51}$$

> SeD0a := ToJet(SeD0, DpVar, notation = jetnumbers)

$$\begin{aligned}
SeD0a := & \frac{1}{Ctt} \left( 2 g_{1,4} Cxy u_{2,3} + 2 g_{1,4} Ctx u_{1,2} + 2 g_{1,4} Cty u_{1,3} + g_{1,4} Cxx u_{2,2} \right. \\
& + g_{1,4} Cyy u_{3,3} - g_{2,4} u_{1,2} Ctt - g_{3,4} u_{1,3} Ctt + f_4 Ctt g_{1,4} u_{1,2} + f_4 Ctt g_{2,4} u_{2,2} \\
& + f_4 Ctt g_{3,4} u_{2,3} - g_{4,4} Ctt f_1 u_{1,2} - g_{4,4} Ctt f_2 u_{2,2} - g_{4,4} Ctt f_3 u_{2,3} + u_{1,3} f_{1,4} Ctt \\
& + u_{2,3} f_{2,4} Ctt + u_{3,3} f_{3,4} Ctt - g_4 Ctt f_{1,4} u_{1,2} - g_4 Ctt f_{2,4} u_{2,2} - g_4 Ctt f_{3,4} u_{2,3} \\
& \left. + f_{4,4} Ctt g_1 u_{1,2} + f_{4,4} Ctt g_2 u_{2,2} + f_{4,4} Ctt g_3 u_{2,3} \right)
\end{aligned} \tag{52}$$

> simplify(subs(SB0p, subs(KP[1], Pullback(dETR3, Pullback(dETR2, Pullback(dETR1, subs(SB0p, SeD0a))))))

$$0 \tag{53}$$

>

> ChangeFrame(L1)

$$L1 \tag{54}$$

$$\begin{aligned}
> SeD1 := & simplify \left( subs \left( S2, Pullback \left( deTR, TotalDiff \left( \left( \left( \frac{\partial}{\partial u_1} g(u_1, u_2, u_3, w[]) \right) u_{1,2} \right. \right. \right. \right. \right. \\
& + \left( \frac{\partial}{\partial u_2} g(u_1, u_2, u_3, w[]) \right) u_{2,2} + \left( \frac{\partial}{\partial u_3} g(u_1, u_2, u_3, w[]) \right) u_{2,3}, 1 \right) - \frac{\partial}{\partial w[]} f(u_1, u_2, \\
& u_3, w[]) \cdot TotalDiff \left( \left( \left( \frac{\partial}{\partial u_1} g(u_1, u_2, u_3, w[]) \right) u_{1,2} + \left( \frac{\partial}{\partial u_2} g(u_1, u_2, u_3, w[]) \right) u_{2,2} \right. \right. \\
& + \left( \frac{\partial}{\partial u_3} g(u_1, u_2, u_3, w[]) \right) u_{2,3}, 2 \right) + \left( \left( \frac{\partial}{\partial u_1} f(u_1, u_2, u_3, w[]) \right) u_{1,2} + \left( \frac{\partial}{\partial u_2} f(u_1, \right. \right. \\
& u_2, u_3, w[]) \right) u_{2,2} + \left( \frac{\partial}{\partial u_3} f(u_1, u_2, u_3, w[]) \right) u_{2,3} \cdot diff \left( \left( \left( \frac{\partial}{\partial u_1} g(u_1, u_2, u_3, w[]) \right) u_{1,2} \right. \right. \\
& + \left( \frac{\partial}{\partial u_2} g(u_1, u_2, u_3, w[]) \right) u_{2,2} + \left( \frac{\partial}{\partial u_3} g(u_1, u_2, u_3, w[]) \right) u_{2,3}, w[]) \\
& - TotalDiff \left( \left( \left( \frac{\partial}{\partial u_1} f(u_1, u_2, u_3, w[]) \right) u_{1,2} + \left( \frac{\partial}{\partial u_2} f(u_1, u_2, u_3, w[]) \right) u_{2,2} \right. \right. \\
& + \left( \frac{\partial}{\partial u_3} f(u_1, u_2, u_3, w[]) \right) u_{2,3}, 3 \right) + \frac{\partial}{\partial w[]} g(u_1, u_2, u_3, w[]) \cdot TotalDiff \left( \left( \left( \frac{\partial}{\partial u_1} f(u_1, \right. \right. \right. \\
& u_2, u_3, w[]) \right) u_{1,2} + \left( \frac{\partial}{\partial u_2} f(u_1, u_2, u_3, w[]) \right) u_{2,2} + \left( \frac{\partial}{\partial u_3} f(u_1, u_2, u_3, w[]) \right) u_{2,3}, 2 \right)
\end{aligned}$$

$$\begin{aligned}
& - \left( \left( \frac{\partial}{\partial u_1} g(u_1, u_2, u_3, w_{[\ ]}) \right) u_{1,2} + \left( \frac{\partial}{\partial u_2} g(u_1, u_2, u_3, w_{[\ ]}) \right) u_{2,2} + \left( \frac{\partial}{\partial u_3} g(u_1, u_2, u_3, w_{[\ ]}) \right) u_{2,3} \right) \cdot \text{diff} \left( \left( \left( \frac{\partial}{\partial u_1} f(u_1, u_2, u_3, w_{[\ ]}) \right) u_{1,2} + \left( \frac{\partial}{\partial u_2} f(u_1, u_2, u_3, w_{[\ ]}) \right) u_{2,2} + \left( \frac{\partial}{\partial u_3} f(u_1, u_2, u_3, w_{[\ ]}) \right) u_{2,3} \right), w_{[\ ]} \right) :
\end{aligned}$$

> *SeD1a* := *ToJet*(*SeD1*, *DpVar*, *notation* = *jetnumbers*)

$$\begin{aligned}
\text{\textit{SeD1a}} := & -\frac{1}{Ct^2} \left( 2 Ct g_{1,2} u_{2,2} Cxy u_{2,3} + 2 Ct g_{1,2} u_{2,2} Ctx u_{1,2} + 2 f_4 Ct^2 u_{1,2} g_{1,2} u_{2,2} \right. & (55) \\
& + 2 f_4 Ct^2 u_{1,2} g_{1,3} u_{2,3} - Ct^2 g_{2,4} u_{2,2} f_3 u_{2,3} - Ct^2 g_{3,4} u_{2,3} f_1 u_{1,2} - Ct^2 g_{3,4} u_{2,3} f_2 u_{2,2} \\
& - 2 g_4 Ct^2 u_{1,2} f_{1,2} u_{2,2} - 2 g_4 Ct^2 u_{1,2} f_{1,3} u_{2,3} + 2 Ct g_{1,2} u_{2,2} Cty u_{1,3} \\
& + Ct g_{1,2} u_{2,2} Cyy u_{3,3} + 2 Ct g_{1,3} u_{2,3} Ctx u_{1,2} + 2 Ct g_{1,3} u_{2,3} Cty u_{1,3} \\
& + Ct g_{1,3} u_{2,3} Cxx u_{2,2} + Ct g_{1,3} u_{2,3} Cyy u_{3,3} - 2 g_4 Ct^2 u_{2,2} f_{2,3} u_{2,3} \\
& + f_{3,4} u_{2,3} Ct^2 g_1 u_{1,2} + f_{3,4} u_{2,3} Ct^2 g_2 u_{2,2} + g_1 u_{2,2} Cyy_{u_2} u_{3,3} Ct \\
& + g_1 u_{2,3} Cxx_{u_3} u_{2,2} Ct + g_1 u_{2,3} Cyy_{u_3} u_{3,3} Ct + 2 g_1 u_{1,2} Cty_{u_1} u_{1,3} Ct \\
& + 2 g_1 u_{1,2} Cxy_{u_1} u_{2,3} Ct + 2 g_1 u_{2,2} Ctx_{u_2} u_{1,2} Ct + 2 g_1 u_{2,2} Cty_{u_2} u_{1,3} Ct \\
& + 2 g_1 u_{2,2} Cxy_{u_2} u_{2,3} Ct + 2 g_1 u_{2,3} Ctx_{u_3} u_{1,2} Ct + 2 g_1 u_{2,3} Cty_{u_3} u_{1,3} Ct \\
& - 2 g_1 u_{1,2} Ct_{u_1} Cty u_{1,3} - g_1 u_{1,2} Ct_{u_1} Cxx u_{2,2} - 2 g_1 u_{1,2} Ct_{u_1} Cxy u_{2,3} \\
& - g_1 u_{1,2} Ct_{u_1} Cyy u_{3,3} - 2 g_1 u_{2,2} Ct_{u_2} Ctx u_{1,2} - 2 g_1 u_{2,2} Ct_{u_2} Cty u_{1,3} \\
& - 2 g_1 u_{2,2} Ct_{u_2} Cxy u_{2,3} - g_1 u_{2,2} Ct_{u_2} Cyy u_{3,3} - 2 g_1 u_{2,3} Ct_{u_3} Ctx u_{1,2} \\
& - 2 g_1 u_{2,3} Ct_{u_3} Cty u_{1,3} - g_1 u_{2,3} Ct_{u_3} Cxx u_{2,2} - g_1 u_{2,3} Ct_{u_3} Cyy u_{3,3} \\
& + g_1 u_{1,2} Cxx_{u_1} u_{2,2} Ct + g_1 u_{1,2} Cyy_{u_1} u_{3,3} Ct + f_{1,4} u_{1,2} Ct^2 g_2 u_{2,2} \\
& + f_{1,4} u_{1,2} Ct^2 g_3 u_{2,3} + f_{2,4} u_{2,2} Ct^2 g_1 u_{1,2} + f_{2,4} u_{2,2} Ct^2 g_3 u_{2,3} \\
& + 2 Ct g_{1,1} u_{1,2} Cxy u_{2,3} + 2 Ct g_{1,1} u_{1,2} Cty u_{1,3} + Ct g_{1,1} u_{1,2} Cxx u_{2,2} \\
& + Ct g_{1,1} u_{1,2} Cyy u_{3,3} + 2 f_4 Ct^2 u_{2,2} g_{2,3} u_{2,3} - Ct^2 g_{1,4} u_{1,2} f_2 u_{2,2} \\
& - Ct^2 g_{1,4} u_{1,2} f_3 u_{2,3} - Ct^2 g_{2,4} u_{2,2} f_1 u_{1,2} + f_3 u_{2,3,3} Ct^2 + f_2 u_{2,2,3} Ct^2 - g_2 u_{1,2,2} Ct^2 \\
& + f_{2,3} u_{2,3}^2 Ct^2 - g_3 u_{1,2,3} Ct^2 + f_1 u_{1,2,3} Ct^2 - u_{1,2}^2 Ct^2 g_{1,2} - u_{1,3} Ct^2 g_{1,3} u_{1,2}
\end{aligned}$$

$$\begin{aligned}
& -u_{1,3} Ctt^2 g_{2,3} u_{2,2} - u_{1,3} Ctt^2 g_{3,3} u_{2,3} - g_4 Ctt^2 f_{1,1} u_{1,2}^2 - g_4 Ctt^2 f_{2,2} u_{2,2}^2 - g_4 Ctt^2 f_{3,3} \\
& u_{2,3}^2 + f_{3,4} u_{2,3}^2 Ctt^2 g_3 + g_1 Cxx u_{2,2,2} Ctt + g_1 Cyy u_{2,3,3} Ctt + 2 g_1 Ctx u_{1,2,2} Ctt \\
& + 2 g_1 Cty u_{1,2,3} Ctt + 2 g_1 Cxy u_{2,2,3} Ctt + u_{2,3} f_{2,2} u_{2,2} Ctt^2 + u_{3,3} f_{1,3} u_{1,2} Ctt^2 \\
& + u_{3,3} f_{2,3} u_{2,2} Ctt^2 + u_{3,3} f_{3,3} u_{2,3} Ctt^2 + 2 g_1 Cxy u_{2,3}^2 Ctt - 2 g_1 u_{1,2}^2 Ctt u_1 Ctx - g_1 \\
& u_{2,2}^2 Ctt u_2 Cxx - 2 g_1 u_{2,3}^2 Ctt u_3 Cxy + u_{1,3} f_{1,1} u_{1,2} Ctt^2 + f_4 Ctt^2 g_{1,1} u_{1,2}^2 + f_4 Ctt^2 g_{2,2} u_{2,2}^2 \\
& + f_4 Ctt^2 g_{3,3} u_{2,3}^2 + 2 Ctt g_{1,1} u_{1,2}^2 Ctx + Ctt g_{1,2} u_{2,2}^2 Cxx + 2 Ctt g_{1,3} u_{2,3}^2 Cxy - Ctt^2 g_{1,4} \\
& u_{1,2}^2 f_1 - Ctt^2 g_{2,4} u_{2,2}^2 f_2 - Ctt^2 g_{3,4} u_{2,3}^2 f_3 - u_{1,2} Ctt^2 g_{2,2} u_{2,2} - u_{1,2} Ctt^2 g_{2,3} u_{2,3} \\
& + g_1 Cxx u_2^2 Ctt + 2 g_1 Ctx u_1^2 Ctt + f_{1,4} u_{1,2}^2 Ctt^2 g_1 + f_{2,4} u_{2,2}^2 Ctt^2 g_2 \\
& + u_{1,3} f_{1,2} u_{2,2} Ctt^2 + u_{1,3} f_{1,3} u_{2,3} Ctt^2 + u_{2,3} f_{1,2} u_{1,2} Ctt^2 + f_4 Ctt^2 g_1 u_{1,2,2} \\
& + f_4 Ctt^2 g_2 u_{2,2,2} + f_4 Ctt^2 g_3 u_{2,2,3} - g_4 Ctt^2 f_1 u_{1,2,2} - g_4 Ctt^2 f_2 u_{2,2,2} - g_4 Ctt^2 f_3 u_{2,2,3}
\end{aligned}$$

> simplify(subs(SB0p, subs(KP[1], Pullback(dETR3, Pullback(dETR2, Pullback(dETR1, subs(SB0p, SeD0a))))))

0

(56)

Checking Lax pair condition in 3D follows from that one in 4D, but we can easily do it:

> ChangeFrame(L2)

TEQ

(57)

> SeD0 := simplify( subs( S2, Pullback( deTR, -TotalDiff( ( \frac{\partial}{\partial w\_{[]}} g(u\_1, u\_2, u\_3, w\_{[]}), 1 ) + \frac{\partial}{\partial w\_{[]}} f(u\_1, u\_2, u\_3, w\_{[]}) \cdot TotalDiff( ( \frac{\partial}{\partial w\_{[]}} g(u\_1, u\_2, u\_3, w\_{[]}), 2 ) + TotalDiff( ( \frac{\partial}{\partial w\_{[]}} f(u\_1, u\_2, u\_3, w\_{[]}), 3 ) - \frac{\partial}{\partial w\_{[]}} g(u\_1, u\_2, u\_3, w\_{[]}) \cdot TotalDiff( ( \frac{\partial}{\partial w\_{[]}} f(u\_1, u\_2, u\_3, w\_{[]}), 2 ) ) ) ) ) ) ) :

> SeD0a := ToJet(SeD0, DpVar, notation = jetnumbers)

SeD0a := \frac{1}{Ctt} ( 2 g\_{1,4} Cxy u\_{2,3} + 2 g\_{1,4} Ctx u\_{1,2} + 2 g\_{1,4} Cty u\_{1,3} + g\_{1,4} Cxx u\_{2,2}

(58)

$$\begin{aligned}
& + g_{1,4} C_{yy} u_{3,3} - g_{2,4} u_{1,2} C_{tt} - g_{3,4} u_{1,3} C_{tt} + f_{4,4} C_{tt} g_{1,4} u_{1,2} + f_{4,4} C_{tt} g_{2,4} u_{2,2} \\
& + f_{4,4} C_{tt} g_{3,4} u_{2,3} - g_{4,4} C_{tt} f_{1,4} u_{1,2} - g_{4,4} C_{tt} f_{2,4} u_{2,2} - g_{4,4} C_{tt} f_{3,4} u_{2,3} + u_{1,3} f_{1,4} C_{tt} \\
& + u_{2,3} f_{2,4} C_{tt} + u_{3,3} f_{3,4} C_{tt} - g_{4,4} C_{tt} f_{1,4} u_{1,2} - g_{4,4} C_{tt} f_{2,4} u_{2,2} - g_{4,4} C_{tt} f_{3,4} u_{2,3} \\
& + f_{4,4} C_{tt} g_{1,4} u_{1,2} + f_{4,4} C_{tt} g_{2,4} u_{2,2} + f_{4,4} C_{tt} g_{3,4} u_{2,3}
\end{aligned}$$

> simplify(subs(SB0p, subs(KP[1], Pullback(dETR3, Pullback(dETR2, Pullback(dETR1, subs(SB0p, SeD0a))))))

0

(59)

Yes, we got commutativity modulo the equation. Now we are ready to check that the surfaces wiped by X,Y in 3D are totally geodesic.

(there's no need to check that the covector  $\theta = f_{\lambda} dt + dx + g_{\lambda} dy$  is null, this condition was obtained above)

Now let us specify the equation and calculate the connection

> DGsetup([t, x, y], [u], J2, 3) :

> F := Ctt(u<sub>1</sub>, u<sub>2</sub>, u<sub>3</sub>) · u<sub>1,1</sub> + 2 Ctx(u<sub>1</sub>, u<sub>2</sub>, u<sub>3</sub>) · u<sub>1,2</sub> + 2 Cty(u<sub>1</sub>, u<sub>2</sub>, u<sub>3</sub>) · u<sub>1,3</sub> + Cxx(u<sub>1</sub>, u<sub>2</sub>, u<sub>3</sub>) · u<sub>2,2</sub> + 2 Cxy(u<sub>1</sub>, u<sub>2</sub>, u<sub>3</sub>) · u<sub>2,3</sub> + Cyy(u<sub>1</sub>, u<sub>2</sub>, u<sub>3</sub>) · u<sub>3,3</sub> :

> A := Matrix( [[ diff(F, u[1, 1]), 1/2 diff(F, u[1, 2]), 1/2 diff(F, u[1, 3]) ], [ 1/2 diff(F, u[1, 2]), diff(F, u[2, 2]), 1/2 diff(F, u[2, 3]) ], [ 1/2 diff(F, u[1, 3]), 1/2 diff(F, u[2, 3]), diff(F, u[3, 3]) ] ] ); AA := expand(MatrixInverse(A)) : AM := simplify(Determinant(A) · AA) :

$$A := \begin{bmatrix} C_{tt} & C_{tx} & C_{ty} \\ C_{tx} & C_{xx} & C_{xy} \\ C_{ty} & C_{xy} & C_{yy} \end{bmatrix}$$

(60)

Here A is the matrix of the linearized operator, AA - the inverse (metric) and AJ=AM the adjoint matrix (which we use as a representative for the conformal class)

> aA := [TotalDiff(A[1, 1], 1) + TotalDiff(A[1, 2], 2) + TotalDiff(A[1, 3], 3), TotalDiff(A[2, 1], 1) + TotalDiff(A[2, 2], 2) + TotalDiff(A[2, 3], 3), TotalDiff(A[3, 1], 1) + TotalDiff(A[3, 2], 2) + TotalDiff(A[3, 3], 3)] :

> ω := 2 · [AA[1, 1] · aA[1] + AA[1, 2] · aA[2] + AA[1, 3] · aA[3], AA[2, 1] · aA[1] + AA[2, 2] · aA[2] + AA[2, 3] · aA[3], AA[3, 1] · aA[1] + AA[3, 2] · aA[2] + AA[3, 3] · aA[3]] :

This is our form connection Omega, but we will use the general form U below

> DepVars := [u(t, x, y)] : AJ := simplify(FromJet(AM, DepVars)) :

> DGsetup([t, x, y], M) :

```
> gg := evalDG(AJ[1, 1]·dt &t dt + AJ[1, 2]·dt &t dx + AJ[1, 3]·dt &t dy + AJ[2, 1]·dx &t dt
+ AJ[2, 2]·dx &t dx + AJ[2, 3]·dx &t dy + AJ[3, 1]·dy &t dt + AJ[3, 2]·dy &t dx
+ AJ[3, 3]·dy &t dy) :
```

```
>
```

```
> C := Connection(a000*dt &t D_t &t dt + a111*dx &t D_x &t dx + a222*dy &t D_y &t dy
+ a001*(dt &t D_t &t dx + dx &t D_t &t dt) + a002*(dt &t D_t &t dy + dy &t D_t
&t dt) + a102*(dx &t D_t &t dy + dy &t D_t &t dx) + a011*(dt &t D_x &t dx + dx
&t D_x &t dt) + a012*(dt &t D_x &t dy + dy &t D_x &t dt) + a112*(dx &t D_x &t dy
+ dy &t D_x &t dx) + a021*(dt &t D_y &t dx + dx &t D_y &t dt) + a022*(dt &t D_y
&t dy + dy &t D_y &t dt) + a122*(dx &t D_y &t dy + dy &t D_y &t dx) + a010*dt
&t D_x &t dt + a121*dx &t D_y &t dx + a202*dy &t D_t &t dy + a020*dt &t D_y &t dt
+ a101*dx &t D_t &t dx + a212*dy &t D_x &t dy) :
```

```
> TorsionTensor(C);
```

$0 \, dt \, D_t \, dt$

(61)

```
> Ω1 := simplify(FromJet(ω[1], DepVars)) :
```

```
Ω2 := simplify(FromJet(ω[2], DepVars)) :
```

```
Ω3 := simplify(FromJet(ω[3], DepVars)) :
```

Here we determine the connection C and define the covector Ω. However we wait to let U=Ω, we want to obtain this from the total geodesicity condition.

```
> Et := evalDG(DirectionalCovariantDerivative(D_t, gg, C) - U1·gg) :
```

```
Ex := evalDG(DirectionalCovariantDerivative(D_x, gg, C) - U2·gg) :
```

```
Ey := evalDG(DirectionalCovariantDerivative(D_y, gg, C) - U3·gg) :
```

```
> Eq000 := TensorInnerProduct(gg, Et, dt &t dt) :
```

```
Eq001 := TensorInnerProduct(gg, Et, dt &t dx) :
```

```
Eq002 := TensorInnerProduct(gg, Et, dt &t dy) :
```

```
Eq011 := TensorInnerProduct(gg, Et, dx &t dx) :
```

```
Eq012 := TensorInnerProduct(gg, Et, dx &t dy) :
```

```
Eq022 := TensorInnerProduct(gg, Et, dy &t dy) :
```

```
Eq100 := TensorInnerProduct(gg, Ex, dt &t dt) :
```

```
Eq101 := TensorInnerProduct(gg, Ex, dt &t dx) :
```

```
Eq102 := TensorInnerProduct(gg, Ex, dt &t dy) :
```

```
Eq111 := TensorInnerProduct(gg, Ex, dx &t dx) :
```

```
Eq112 := TensorInnerProduct(gg, Ex, dx &t dy) :
```

```
Eq122 := TensorInnerProduct(gg, Ex, dy &t dy) :
```

```
Eq200 := TensorInnerProduct(gg, Ey, dt &t dt) :
```

```
Eq201 := TensorInnerProduct(gg, Ey, dt &t dx) :
```

```
Eq202 := TensorInnerProduct(gg, Ey, dt &t dy) :
```

```
Eq211 := TensorInnerProduct(gg, Ey, dx &t dx) :
```

```
Eq212 := TensorInnerProduct(gg, Ey, dx &t dy) :
```

```
Eq222 := TensorInnerProduct(gg, Ey, dy &t dy) :
```

```
> sA := solve( {Eq000=0, Eq001=0, Eq002=0, Eq011=0, Eq012=0, Eq022=0, Eq100=0,
Eq101=0, Eq102=0, Eq111=0, Eq112=0, Eq122=0, Eq200=0, Eq201=0, Eq202=0,
Eq211=0, Eq212=0, Eq222=0}, [a000, a001, a002, a010, a011, a012, a020, a021, a022,
a101, a102, a111, a112, a121, a122, a202, a212, a222]) :
```

```
> C1 := evalDG( subs( {op(op(sA))}, C) ) :
```

```
> evalDG( CovariantDerivative(gg, C1) - gg &t (U1·dt + U2·dx + U3·dy) );
```

$0 \, dt \, dt \, dt$

(62)



>

We want to check that the connection preserves the conformal class of the form  $\theta$  in the direction of  $\text{Ann}(\theta)$

$$\begin{aligned} > \theta := \text{evalDG}(dx + D_4(f) (\text{diff}(u(t, x, y), t), \text{diff}(u(t, x, y), x), \text{diff}(u(t, x, y), y), w(t, x, y)) \cdot dt \\ &\quad + D_4(g) (\text{diff}(u(t, x, y), t), \text{diff}(u(t, x, y), x), \text{diff}(u(t, x, y), y), w(t, x, y)) \cdot dy) \\ \theta &:= D_4(f) (D_1(u)(t, x, y), D_2(u)(t, x, y), D_3(u)(t, x, y), w(t, x, y)) dt + dx \\ &\quad + D_4(g) (D_1(u)(t, x, y), D_2(u)(t, x, y), D_3(u)(t, x, y), w(t, x, y)) dy \end{aligned} \quad (63)$$

$$\begin{aligned} > X &:= \text{evalDG}(D_x - D_4(f) (\text{diff}(u(t, x, y), t), \text{diff}(u(t, x, y), x), \text{diff}(u(t, x, y), y), w(t, x, y)) \\ &\quad \cdot D_x) : \\ Y &:= \text{evalDG}(D_y - D_4(g) (\text{diff}(u(t, x, y), t), \text{diff}(u(t, x, y), x), \text{diff}(u(t, x, y), y), w(t, x, y)) \\ &\quad \cdot D_x) : \end{aligned}$$

$$\begin{aligned} > [\text{Hook}(X, \theta), \text{Hook}(Y, \theta)] \\ &\quad [0, 0] \end{aligned} \quad (64)$$

$$\begin{aligned} > X\theta X &:= \text{ContractIndices}(\text{evalDG}(\text{DirectionalCovariantDerivative}(X, \theta, C1)), X, [[1, 1]]) : \\ X\theta Y &:= \text{ContractIndices}(\text{evalDG}(\text{DirectionalCovariantDerivative}(X, \theta, C1)), Y, [[1, 1]]) : \\ Y\theta X &:= \text{ContractIndices}(\text{evalDG}(\text{DirectionalCovariantDerivative}(Y, \theta, C1)), X, [[1, 1]]) : \\ Y\theta Y &:= \text{ContractIndices}(\text{evalDG}(\text{DirectionalCovariantDerivative}(Y, \theta, C1)), Y, [[1, 1]]) : \end{aligned}$$

>

These are the 4 condtions to check and determine the connection for U (=Omega).  
Let us restrict them to the equations of the Lax pair and their compatibility conditions

$$\begin{aligned} > \text{ChangeFrame}(L2); \\ &\quad \text{TEQ} \end{aligned} \quad (65)$$

$$\begin{aligned} > \text{Tools:-DGinfo}(\text{"CurrentFrame"}); \\ &\quad L2 \end{aligned} \quad (66)$$

>

$$\begin{aligned} > de &:= \text{DifferentialEquationData}([F, w_1 = w_1], [u_1, w_1]) \\ de &:= [\{u_1, w_1\}, [Ctt u_{1,1} + 2 Ctx u_{1,2} + 2 Cty u_{1,3} + Cxx u_{2,2} + 2 Cxy u_{2,3} + Cyy u_{3,3}, 0]] \end{aligned} \quad (67)$$

$$> de1 := \text{Prolong}(de, 1) : deTRA := \text{Transformation}(de1) :$$

>

$$\begin{aligned} > \text{DepVarsP} &:= [\text{op}(\text{DepVars}), w(t, x, y)] \\ &\quad \text{DepVarsP} := [u(t, x, y), w(t, x, y)] \end{aligned} \quad (68)$$

>

$$\begin{aligned} > XX1 &:= \text{Pullback}(deTRA, \text{subs}(S1, \text{ToJet}(X\theta X, \text{DepVarsP}, \text{notation} = \text{jetnumbers}))) : \\ XX2 &:= \text{ToJet}(XX1, [f(u_1, u_2, u_3, w), g(u_1, u_2, u_3, w)], \text{notation} = \text{jetnumbers}) : \\ XX3 &:= \text{simplify}(\text{subs}(SB0p, \text{subs}(KP[1], \text{Pullback}(dETR3, \text{Pullback}(dETR2, \text{Pullback}(dETR1, \\ &\quad \text{subs}(SB0p, XX2)))))) : \\ > XY1 &:= \text{Pullback}(deTRA, \text{subs}(S1, \text{ToJet}(X\theta Y, \text{DepVarsP}, \text{notation} = \text{jetnumbers}))) : \\ XY2 &:= \text{ToJet}(XY1, [f(u_1, u_2, u_3, w), g(u_1, u_2, u_3, w)], \text{notation} = \text{jetnumbers}) : \\ XY3 &:= \text{simplify}(\text{subs}(SB0p, \text{subs}(KP[1], \text{Pullback}(dETR3, \text{Pullback}(dETR2, \text{Pullback}(dETR1, \\ &\quad \text{subs}(SB0p, XY2)))))) : \\ > YX1 &:= \text{Pullback}(deTRA, \text{subs}(S1, \text{ToJet}(Y\theta X, \text{DepVarsP}, \text{notation} = \text{jetnumbers}))) : \end{aligned}$$

```

YX2 := ToJet(YX1, [f(u1, u2, u3, w[]), g(u1, u2, u3, w[])], notation = jetnumbers) :
YX3 := simplify(subs(SB0p, subs(KP[1], Pullback(dETR3, Pullback(dETR2, Pullback(dETR1,
subs(SB0p, YX2)))))) :

```

```

> YY1 := Pullback(deTRA, subs(S1, ToJet(Y0Y, DepVarsP, notation = jetnumbers))) :

```

```

YY2 := ToJet(YY1, [f(u1, u2, u3, w[]), g(u1, u2, u3, w[])], notation = jetnumbers) :

```

```

YY3 := simplify(subs(SB0p, subs(KP[1], Pullback(dETR3, Pullback(dETR2, Pullback(dETR1,
subs(SB0p, YY2)))))) :

```

These are the final 4 equations (to this end all our information was used) that allow to determined the connection form.

Let us first check that our  $\omega$  is a solution.

```

>
> simplify(subs(SB0p, subs(KP[1], Pullback(dETR3, Pullback(dETR2, Pullback(dETR1,
Pullback(deTRA, subs(SB0p, subs([U1 = ω[1], U2 = ω[2], U3 = ω[3]], XX3))))))
0 (69)

```

```

> simplify(subs(SB0p, subs(KP[1], Pullback(dETR3, Pullback(dETR2, Pullback(dETR1,
Pullback(deTRA, subs(SB0p, subs([U1 = ω[1], U2 = ω[2], U3 = ω[3]], XY3))))))
0 (70)

```

```

> simplify(subs(SB0p, subs(KP[1], Pullback(dETR3, Pullback(dETR2, Pullback(dETR1,
Pullback(deTRA, subs(SB0p, subs([U1 = ω[1], U2 = ω[2], U3 = ω[3]], YX3))))))
0 (71)

```

```

> simplify(subs(SB0p, subs(KP[1], Pullback(dETR3, Pullback(dETR2, Pullback(dETR1,
Pullback(deTRA, subs(SB0p, subs([U1 = ω[1], U2 = ω[2], U3 = ω[3]], YY3))))))
0 (72)

```

Great - as expected!

```

>
>

```

This how one of the components looks like, and we want to prove that any solution U coincide with this  $\Omega$ .

But direct approach does not work - no unique solution:

```

>
> solve([XX3, XY3, YX3, YY3], [U1, U2, U3]) :
> MAT := Matrix([ [diff(numer(XX3), U1), diff(numer(XX3), U2), diff(numer(XX3), U3)],
[diff(numer(XY3), U1), diff(numer(XY3), U2), diff(numer(XY3), U3)],
[diff(numer(YX3), U1), diff(numer(YX3), U2), diff(numer(YX3), U3)],
[diff(numer(YY3), U1), diff(numer(YY3), U2), diff(numer(YY3), U3)]]) :
> sDelta := (i, k, j, l) → simplify(MAT[i, j]·MAT[k, l] - MAT[i, l]·MAT[k, j]) :
> [sDelta(1, 2, 1, 2), sDelta(1, 2, 1, 3), sDelta(1, 2, 2, 3), sDelta(1, 3, 1, 2), sDelta(1, 3, 1, 3),
sDelta(1, 3, 2, 3), sDelta(1, 4, 1, 2), sDelta(1, 4, 1, 3), sDelta(1, 4, 2, 3), sDelta(2, 3, 2, 1,
2), sDelta(2, 3, 1, 3), sDelta(2, 3, 2, 3), sDelta(2, 4, 1, 2), sDelta(2, 4, 1, 3), sDelta(2, 4,
2, 3), sDelta(3, 4, 1, 2), sDelta(3, 4, 1, 3), sDelta(3, 4, 2, 3)]
[0, 0, 0, 0, 0, 0, 0, 0, 0, 0, 0, 0, 0, 0, 0, 0] (73)

```

and even worse: the system shows to have a 2D family of solutions (up to addition of  $\theta \perp$ ).

However this happens at any fixed (t,x,y,λ=w) (i.e. a point in the mini-twistor space) and in our 3D manifold a curve of possible λ hangs over a point (t,x,y) of M.

Thus we can decompose by λ and get more equations; it is enough to work only with the coefficients of

the equation XX3, as the others are proportional.

**TEQ** >

**TEQ** >  $Mat := Matrix(5, 3, symbol = m) :$

**TEQ** >  $m[1, 1] := diff(numer(XX3), U1, f_4\$4) : m[1, 2] := diff(numer(XX3), U2, f_4\$4) :$   
 $m[1, 3] := diff(numer(XX3), U3, f_4\$4) :$

**TEQ** >  $m[2, 1] := diff(numer(XX3), U1, f_4\$3, g_4) : m[2, 2] := diff(numer(XX3), U2, f_4$   
 $\$3, g_4) : m[2, 3] := diff(numer(XX3), U3, f_4\$3, g_4) :$

**TEQ** >  $m[3, 1] := diff(numer(XX3), U1, f_4\$2, g_4\$2) : m[3, 2] := diff(numer(XX3), U2, f_4$   
 $\$2, g_4\$2) : m[3, 3] := diff(numer(XX3), U3, f_4\$2, g_4\$2) :$

**TEQ** >  $m[4, 1] := diff(numer(XX3), U1, f_4, g_4\$3) : m[4, 2] := diff(numer(XX3), U2, f_4,$   
 $g_4\$3) : m[4, 3] := diff(numer(XX3), U3, f_4, g_4\$3) :$

**TEQ** >  $m[5, 1] := diff(numer(XX3), U1, g_4\$4) : m[5, 2] := diff(numer(XX3), U2, g_4$   
 $\$4) : m[5, 3] := diff(numer(XX3), U3, g_4\$4) :$

**TEQ** >  $Mat$

$$\begin{aligned} & \left[ \begin{aligned} & -24 C_{ty}^2 C_{tt}^3, 120 f_4 C_{ty}^2 C_{tt}^3 + 48 C_{yy} C_{tt}^3 g_4 C_{ty} + 72 C_{ty}^3 C_{tt}^2 g_4 + 48 C_{ty}^2 C_{tt}^2 C_{tx} \\ & + 48 C_{ty} C_{xy} C_{tt}^3, -24 C_{ty}^3 C_{tt}^2 \end{aligned} \right], \\ & \left[ \begin{aligned} & -12 C_{yy} C_{tt}^3 C_{ty} - 12 C_{ty}^3 C_{tt}^2, 24 C_{yy} C_{tt}^2 C_{ty} C_{tx} + 48 f_4 C_{yy} C_{tt}^3 C_{ty} \\ & + 84 C_{ty}^2 C_{yy} C_{tt}^2 g_4 + 12 C_{yy} C_{tt}^3 C_{xy} + 42 C_{ty}^2 C_{xy} C_{tt}^2 + 18 C_{ty}^3 C_{tt} C_{tx} \\ & + 12 C_{yy}^2 C_{tt}^3 g_4 + 72 f_4 C_{ty}^3 C_{tt}^2 + 24 C_{ty}^4 C_{tt} g_4, -6 C_{ty}^4 C_{tt} - 18 C_{ty}^2 C_{yy} C_{tt}^2 \end{aligned} \right], \\ & \left[ \begin{aligned} & -16 C_{ty}^2 C_{yy} C_{tt}^2 - 4 C_{yy}^2 C_{tt}^3 - 4 C_{ty}^4 C_{tt}, 40 C_{xy} C_{yy} C_{tt}^2 C_{ty} + 28 C_{ty}^2 C_{tx} C_{yy} C_{tt} \\ & + 20 C_{ty}^3 C_{xy} C_{tt} + 60 C_{ty}^3 C_{yy} C_{tt} g_4 + 84 f_4 C_{ty}^2 C_{yy} C_{tt}^2 + 60 C_{ty} C_{yy}^2 C_{tt}^2 g_4 \\ & + 8 C_{yy}^2 C_{tt}^2 C_{tx} + 12 f_4 C_{yy}^2 C_{tt}^3 + 24 f_4 C_{ty}^4 C_{tt}, -12 C_{ty} C_{yy}^2 C_{tt}^2 - 12 C_{ty}^3 C_{yy} C_{tt} \end{aligned} \right], \\ & \left[ \begin{aligned} & -12 C_{ty} C_{yy}^2 C_{tt}^2 - 12 C_{ty}^3 C_{yy} C_{tt}, 48 C_{xy} C_{yy} C_{tt} C_{ty}^2 + 30 C_{ty} C_{yy}^2 C_{tt} C_{tx} \\ & + 24 g_4 C_{yy}^3 C_{tt}^2 + 96 C_{ty}^2 C_{yy}^2 C_{tt} g_4 + 60 f_4 C_{ty} C_{yy}^2 C_{tt}^2 + 60 f_4 C_{ty}^3 C_{yy} C_{tt} \\ & + 18 C_{xy} C_{yy}^2 C_{tt}^2, -6 C_{yy}^3 C_{tt}^2 - 18 C_{ty}^2 C_{yy}^2 C_{tt} \end{aligned} \right], \\ & \left[ \begin{aligned} & -24 C_{ty}^2 C_{yy}^2 C_{tt}, 24 C_{yy}^3 C_{tt} C_{tx} + 120 g_4 C_{yy}^3 C_{tt} C_{ty} + 24 C_{yy}^3 C_{tt}^2 f_4 \\ & + 96 f_4 C_{ty}^2 C_{yy}^2 C_{tt} + 72 C_{xy} C_{yy}^2 C_{tt} C_{ty}, -24 C_{yy}^3 C_{tt} C_{ty} \end{aligned} \right] \end{aligned} \quad (74)$$

**>**  $mMat := SubMatrix(Mat, [1..3], [1..3])$

$$\begin{aligned} mMat := & \left[ \begin{aligned} & -24 C_{ty}^2 C_{tt}^3, 120 f_4 C_{ty}^2 C_{tt}^3 + 48 C_{yy} C_{tt}^3 g_4 C_{ty} + 72 C_{ty}^3 C_{tt}^2 g_4 \\ & + 48 C_{ty}^2 C_{tt}^2 C_{tx} + 48 C_{ty} C_{xy} C_{tt}^3, -24 C_{ty}^3 C_{tt}^2 \end{aligned} \right], \\ & \left[ \begin{aligned} & -12 C_{yy} C_{tt}^3 C_{ty} - 12 C_{ty}^3 C_{tt}^2, 24 C_{yy} C_{tt}^2 C_{ty} C_{tx} + 48 f_4 C_{yy} C_{tt}^3 C_{ty} \\ & + 84 C_{ty}^2 C_{yy} C_{tt}^2 g_4 + 12 C_{yy} C_{tt}^3 C_{xy} + 42 C_{ty}^2 C_{xy} C_{tt}^2 + 18 C_{ty}^3 C_{tt} C_{tx} \\ & + 12 C_{yy}^2 C_{tt}^3 g_4 + 72 f_4 C_{ty}^3 C_{tt}^2 + 24 C_{ty}^4 C_{tt} g_4, -6 C_{ty}^4 C_{tt} - 18 C_{ty}^2 C_{yy} C_{tt}^2 \end{aligned} \right], \end{aligned} \quad (75)$$

$$\begin{aligned} & \left[ -16 C_{ty}^2 C_{yy} C_{tt}^2 - 4 C_{yy}^2 C_{tt}^3 - 4 C_{ty}^4 C_{tt}, 40 C_{xy} C_{yy} C_{tt}^2 C_{ty} + 28 C_{ty}^2 C_{tx} C_{yy} C_{tt} \right. \\ & + 20 C_{ty}^3 C_{xy} C_{tt} + 60 C_{ty}^3 C_{yy} C_{tt} g_4 + 84 f_4 C_{ty}^2 C_{yy} C_{tt}^2 + 60 C_{ty} C_{yy}^2 C_{tt}^2 g_4 \\ & \left. + 8 C_{yy}^2 C_{tt}^2 C_{tx} + 12 f_4 C_{yy}^2 C_{tt}^3 + 24 f_4 C_{ty}^4 C_{tt}, -12 C_{ty} C_{yy}^2 C_{tt}^2 - 12 C_{ty}^3 C_{yy} C_{tt} \right] \end{aligned}$$

> factor(Determinant(mMat))

$$\begin{aligned} & -576 C_{ty}^3 C_{tt}^4 (C_{ty}^2 - C_{tt} C_{yy})^2 (g_4 C_{ty}^4 + C_{ty}^3 C_{tt} f_4 + C_{ty}^3 C_{tx} + 2 C_{tt}^2 C_{yy} f_4 C_{ty} \\ & + 2 C_{tt}^2 C_{xy} C_{yy} + 2 C_{tt}^2 C_{yy}^2 g_4) \end{aligned} \quad (76)$$

Thus the system has highest rank =3, and so the solution (U1,U2,U3) is unique (and hence coincides with the prescribed  $\omega$ ).

Done!

>

>
