# Supplementary material for: Dispersionless integrable systems in 3D and Einstein-Weyl geometry
Source: arXiv:1208.2728 ancillary file (2013-05-09)
Supplement: Supplementary file 4 [file BKEF-2012-II-quasilinear_wave_integrability.pdf]

This is the worksheet accompanying the paper E.Ferapontov & B.Kruglikov "Dispersionless integrable systems in 3D and Einstein-Weyl geometry".

The file ran on **Maple** version 16, the package **DifferentialGeometry** was used.

We consider type II quasilinear wave equation and prove that it's integrability is equivalent to the EW property of the linearization conformal structure

```
>
> with(DifferentialGeometry) : with(Tensor) : with(Tools) : with(JetCalculus) :
  with(LinearAlgebra) : with(PDEtools, D_Dx, declare, ToJet, FromJet) :
> DGsetup([t, x, y], [u], J2, 3) :
> declare(Ctt(u1, u2, u3)) : declare(Ctx(u1, u2, u3)) : declare(Cty(u1, u2, u3)) :
  declare(Cxx(u1, u2, u3)) : declare(Cxy(u1, u2, u3)) : declare(Cyy(u1, u2, u3)) :

      Ctt(u1, u2, u3) will now be displayed as Ctt
      Ctx(u1, u2, u3) will now be displayed as Ctx
      Cty(u1, u2, u3) will now be displayed as Cty
      Cxx(u1, u2, u3) will now be displayed as Cxx
      Cxy(u1, u2, u3) will now be displayed as Cxy
      Cyy(u1, u2, u3) will now be displayed as Cyy
```

(1)

```
>
> F := Ctt(u1, u2, u3) · u1,1 + 2 Ctx(u1, u2, u3) · u1,2 + 2 Cty(u1, u2, u3) · u1,3 + Cxx(u1, u2, u3)
  · u2,2 + 2 Cxy(u1, u2, u3) · u2,3 + Cyy(u1, u2, u3) · u3,3 :
```

For simplicity (and since this is not restrictive) we normalize the coefficient Cyy=1 (in Burowski particular form of the integrability conditions one assumes that Cyy≠0)

```
> F := Ctt(u1, u2, u3) · u1,1 + 2 Ctx(u1, u2, u3) · u1,2 + 2 Cty(u1, u2, u3) · u1,3 + Cxx(u1, u2, u3)
  · u2,2 + 2 Cxy(u1, u2, u3) · u2,3 + u3,3 :
```

```
>
> A := Matrix(⌈⌈⌈diff(F, u[1, 1]), 1/2 diff(F, u[1, 2]), 1/2 diff(F, u[1, 3])⌋, ⌈1/2 diff(F, u[1,
  2]), diff(F, u[2, 2]), 1/2 diff(F, u[2, 3])⌋, ⌈1/2 diff(F, u[1, 3]), 1/2 diff(F, u[2, 3]),
  diff(F, u[3, 3])⌋⌋⌋); AA := expand(MatrixInverse(A)) : AM := simplify(Determinant(A)
  · AA) :
```

$$A := \begin{bmatrix} Ctt & Ctx & Cty \\ Ctx & Cxx & Cxy \\ Cty & Cxy & 1 \end{bmatrix}$$

(2)

Here A is the matrix of the linearized operator, AA - the inverse (metric) and AJ=AM the adjoint matrix (which we use as a representative for the conformal class)

```
>
> aA := [TotalDiff(A[1, 1], 1) + TotalDiff(A[1, 2], 2) + TotalDiff(A[1, 3], 3), TotalDiff(A[2,
```

```
1], 1) + TotalDiff(A[2, 2], 2) + TotalDiff(A[2, 3], 3), TotalDiff(A[3, 1], 1)
+ TotalDiff(A[3, 2], 2) + TotalDiff(A[3, 3], 3) ] :
```

```
> ω := 2·[AA[1, 1]· aA[1] + AA[1, 2]· aA[2] + AA[1, 3]· aA[3], AA[2, 1]· aA[1] + AA[2, 2]
· aA[2] + AA[2, 3]· aA[3], AA[3, 1]· aA[1] + AA[3, 2]· aA[2] + AA[3, 3]· aA[3]] :
```

```
>
```

```
> DepVars := [u(t, x, y)] : AJ := simplify(FromJet(AM, DepVars)) :
```

```
>
```

```
> DGsetup([t, x, y], M) :
```

```
> g := evalDG(AJ[1, 1]·dt &t dt + AJ[1, 2]·dt &t dx + AJ[1, 3]·dt &t dy + AJ[2, 1]·dx &t dt
+ AJ[2, 2]·dx &t dx + AJ[2, 3]·dx &t dy + AJ[3, 1]·dy &t dt + AJ[3, 2]·dy &t dx
+ AJ[3, 3]·dy &t dy) :
```

```
>
```

```
> C := Connection(a000*dt &t D_t &t dt + a111*dx &t D_x &t dx + a222*dy &t D_y &t dy
+ a001*(dt &t D_t &t dx + dx &t D_t &t dt) + a002*(dt &t D_t &t dy + dy &t D_t
&t dt) + a102*(dx &t D_t &t dy + dy &t D_t &t dx) + a011*(dt &t D_x &t dx + dx
&t D_x &t dt) + a012*(dt &t D_x &t dy + dy &t D_x &t dt) + a112*(dx &t D_x &t dy
+ dy &t D_x &t dx) + a021*(dt &t D_y &t dx + dx &t D_y &t dt) + a022*(dt &t D_y
&t dy + dy &t D_y &t dt) + a122*(dx &t D_y &t dy + dy &t D_y &t dx) + a010*dt
&t D_x &t dt + a121*dx &t D_y &t dx + a202*dy &t D_t &t dy + a020*dt &t D_y &t dt
+ a101*dx &t D_t &t dx + a212*dy &t D_x &t dy) :
```

```
> TorsionTensor(C);
```

$0 \, dt \, D_t \, dt$

(3)

```
>
```

```
> U1 := simplify(FromJet(ω[1], DepVars)) :
```

```
U2 := simplify(FromJet(ω[2], DepVars)) :
```

```
U3 := simplify(FromJet(ω[3], DepVars)) :
```

```
>
```

Here we determine the connection C and define the covector U=ω.

```
> Et := evalDG(DirectionalCovariantDerivative(D_t, g, C) - U1·g) :
```

```
Ex := evalDG(DirectionalCovariantDerivative(D_x, g, C) - U2·g) :
```

```
Ey := evalDG(DirectionalCovariantDerivative(D_y, g, C) - U3·g) :
```

```
> Eq000 := TensorInnerProduct(g, Et, dt &t dt) :
```

```
Eq001 := TensorInnerProduct(g, Et, dt &t dx) :
```

```
Eq002 := TensorInnerProduct(g, Et, dt &t dy) :
```

```
Eq011 := TensorInnerProduct(g, Et, dx &t dx) :
```

```
Eq012 := TensorInnerProduct(g, Et, dx &t dy) :
```

```
Eq022 := TensorInnerProduct(g, Et, dy &t dy) :
```

```
Eq100 := TensorInnerProduct(g, Ex, dt &t dt) :
```

```
Eq101 := TensorInnerProduct(g, Ex, dt &t dx) :
```

```
Eq102 := TensorInnerProduct(g, Ex, dt &t dy) :
```

```
Eq111 := TensorInnerProduct(g, Ex, dx &t dx) :
```

```
Eq112 := TensorInnerProduct(g, Ex, dx &t dy) :
```

```
Eq122 := TensorInnerProduct(g, Ex, dy &t dy) :
```

```
Eq200 := TensorInnerProduct(g, Ey, dt &t dt) :
```

```
Eq201 := TensorInnerProduct(g, Ey, dt &t dx) :
```

```
Eq202 := TensorInnerProduct(g, Ey, dt &t dy) :
```

```
Eq211 := TensorInnerProduct(g, Ey, dx &t dx) :
```

$Eq212 := TensorInnerProduct(g, Ey, dx \& t dy) :$

$Eq222 := TensorInnerProduct(g, Ey, dy \& t dy) :$

>  $sA := solve(\{Eq000=0, Eq001=0, Eq002=0, Eq011=0, Eq012=0, Eq022=0, Eq100=0, Eq101=0, Eq102=0, Eq111=0, Eq112=0, Eq122=0, Eq200=0, Eq201=0, Eq202=0, Eq211=0, Eq212=0, Eq222=0\}, [a000, a001, a002, a010, a011, a012, a020, a021, a022, a101, a102, a111, a112, a121, a122, a202, a212, a222]) :$

>  $C1 := evalDG(subs(\{op(op(sA))\}, C)) :$

>  $evalDG(CovariantDerivative(g, C1) - g \& t (U1 \cdot dt + U2 \cdot dx + U3 \cdot dy)) ;$   
 $0 \ dt \ dt \ dt$

(4)

The connection  $C=C1$  is uniquely determined by the 1st equation of EW property:  $D_C(g)=\omega \cdot g$ .  
 Let us consider the main defining relation:  $Ricci(C)=V \cdot g$  ( $V$  is some scalar function).

>  $R1 := CurvatureTensor(C1) : Ric1 := RicciTensor(R1) : T1 := SymmetrizeIndices(Ric1, [1, 2], "Symmetric") : Res := evalDG(T1 - V \cdot g) :$

>  $NEQtt := ContractIndices(Res, D_t \& t D_t, [[1, 1], [2, 2]]) : NEQtx := ContractIndices(Res, D_t \& t D_x, [[1, 1], [2, 2]]) :$

$NEQty := ContractIndices(Res, D_t \& t D_y, [[1, 1], [2, 2]]) : NEQxx := ContractIndices(Res, D_x \& t D_x, [[1, 1], [2, 2]]) :$

$NEQxy := ContractIndices(Res, D_x \& t D_y, [[1, 1], [2, 2]]) : NEQyy := ContractIndices(Res, D_y \& t D_y, [[1, 1], [2, 2]]) :$

>

>  $DGsetup([t, x, y], [u], J2, 4) :$

>  $de := DifferentialEquationData([F], [u_{3,3}])$

$de := [\{u_{3,3}\}, [Ctt u_{1,1} + 2 Ctx u_{1,2} + 2 Cty u_{1,3} + Cxx u_{2,2} + 2 Cxy u_{2,3} + u_{3,3}]]$

(5)

>  $de2 := Prolong(de, 2) : deTRA := Transformation(de2) :$

>

>  $Eq0 := Pullback(deTRA, ToJet(NEQtt, DepVars, notation = jetnumbers)) :$

>  $VS := solve(Eq0, V) :$

>  $Eq1 := numer(subs(V=VS, Pullback(deTRA, ToJet(NEQtx, DepVars, notation = jetnumbers)))) :$

$Eq2 := numer(subs(V=VS, Pullback(deTRA, ToJet(NEQty, DepVars, notation = jetnumbers)))) :$

$Eq3 := numer(subs(V=VS, Pullback(deTRA, ToJet(NEQxx, DepVars, notation = jetnumbers)))) :$

$Eq4 := numer(subs(V=VS, Pullback(deTRA, ToJet(NEQxy, DepVars, notation = jetnumbers)))) :$

$Eq5 := numer(subs(V=VS, Pullback(deTRA, ToJet(NEQyy, DepVars, notation = jetnumbers)))) :$

We first check that the highest (3rd order) derivatives have zero coefficients:  
 this condition uniquely specifies the covector  $\omega$ , so the universal formula for covector holds here

J2 >  $simplify([diff(Eq1, u_{1,1,1}), diff(Eq1, u_{1,1,2}), diff(Eq1, u_{1,1,3}), diff(Eq1, u_{1,2,2}), diff(Eq1, u_{1,2,3}), diff(Eq1, u_{2,2,2}), diff(Eq1, u_{2,2,3})])$   
 $[0, 0, 0, 0, 0, 0, 0]$

(6)

J2 >  $simplify([diff(Eq2, u_{1,1,1}), diff(Eq2, u_{1,1,2}), diff(Eq2, u_{1,1,3}), diff(Eq2, u_{1,2,2}), diff(Eq2, u_{1,2,3}), diff(Eq2, u_{2,2,2}), diff(Eq2, u_{2,2,3})])$   
 $[0, 0, 0, 0, 0, 0, 0]$

(7)

J2 >  $simplify([diff(Eq3, u_{1,1,1}), diff(Eq3, u_{1,1,2}), diff(Eq3, u_{1,1,3}), diff(Eq3, u_{1,2,2}),$

$$\text{diff}(Eq3, u_{1,2,3}), \text{diff}(Eq3, u_{2,2,2}), \text{diff}(Eq3, u_{2,2,3}) ] ] \\ [0, 0, 0, 0, 0, 0, 0] \quad (8)$$

$$\mathbf{J2} > \text{simplify}([ \text{diff}(Eq4, u_{1,1,1}), \text{diff}(Eq4, u_{1,1,2}), \text{diff}(Eq4, u_{1,1,3}), \text{diff}(Eq4, u_{1,2,2}), \\ \text{diff}(Eq4, u_{1,2,3}), \text{diff}(Eq4, u_{2,2,2}), \text{diff}(Eq4, u_{2,2,3}) ] ] \\ [0, 0, 0, 0, 0, 0, 0] \quad (9)$$

$$\mathbf{J2} > \text{simplify}([ \text{diff}(Eq5, u_{1,1,1}), \text{diff}(Eq5, u_{1,1,2}), \text{diff}(Eq5, u_{1,1,3}), \text{diff}(Eq5, u_{1,2,2}), \\ \text{diff}(Eq5, u_{1,2,3}), \text{diff}(Eq5, u_{2,2,2}), \text{diff}(Eq5, u_{2,2,3}) ] ] \\ [0, 0, 0, 0, 0, 0, 0] \quad (10)$$

$$> \text{declare}(Ctt(r, p, q)) : \text{declare}(Ctx(r, p, q)) : \text{declare}(Cty(r, p, q)) : \text{declare}(Cxx(r, p, q)) : \\ \text{declare}(Cxy(r, p, q)) : \\ Ctt(r, p, q) \text{ will now be displayed as } Ctt \\ Ctx(r, p, q) \text{ will now be displayed as } Ctx \\ Cty(r, p, q) \text{ will now be displayed as } Cty \\ Cxx(r, p, q) \text{ will now be displayed as } Cxx \\ Cxy(r, p, q) \text{ will now be displayed as } Cxy \quad (11)$$

Now we have to consider the second order terms in u. They depend quadratically on  $u_{ij}$ . The corresponding coefficients  $K_{ij}^{\wedge}$  (where  $ij=11..23$  numerates the second derivatives mod  $F=0$  and  $k=1..5$  numerates the equations  $Eq||i$ ) are complicated, but they depend linearly on the 2-jet of  $f_{ij}$  (like  $Cxx$  etc) with coeffs. before being 0-order in  $f_{ij}$ .

$$> \text{cnd}[1] := \text{simplify}(\text{subs}([u_1=r, u_2=p, u_3=q], \text{diff}(Eq1, u_{1,1}, u_{1,1}))) \\ > \text{factor}(\text{coeff}(\text{cnd}[1], \text{diff}(Cxx(r, p, q), r, r))) \\ -4 Ctt (Cxy Cty - Ctx) (Ctt Cxy^2 - 2 Ctx Cty Cxy - Cxx Ctt + Cxx Cty^2 + Ctx^2)^3 \quad (12)$$

This was an example. Now we want to show that  $Eq||i=0$  is equivalent to the integrability conditions from [Burovski, Ferapontov, Tsarev 2009]. We first write down theirs condition (it is translated here from another file). These are 30 conditions on 2-jets of  $f_{ij}$  (=Ctt etc); since there are exactly 30 second ord derivatives of these latter, we get expressions of  $Ctt_{ij}$  etc (derivatives are with respect to  $r=u_t=u_1=a, p=u_x=u_2=b, q=u_y=u_3=c$ ):

$$> \text{HessUniv} := -Ctt(r, p, q) Cxy(r, p, q)^2 + 2 Cxy(r, p, q) Ctx(r, p, q) Cty(r, p, q) - Ctx(r, p, q)^2 \\ - Cxx(r, p, q) Cty(r, p, q)^2 + Cxx(r, p, q) Ctt(r, p, q) : \\ > \text{ICsubs} := \left[ D_{1,1}(Ctt)(r, p, q) = -\frac{1}{2} \frac{1}{\text{HessUniv}} \left( 4 Ctt(r, p, q)^2 D_2(Cxy)(r, p, q) D_1(Cty)(r, p, \right. \right. \\ & q) + 4 Ctx(r, p, q) D_1(Ctt)(r, p, q) D_1(Ctx)(r, p, q) + 2 Ctt(r, p, q)^2 D_3(Ctt)(r, p, \\ & q) D_2(Cxy)(r, p, q) - 2 Ctt(r, p, q) D_1(Ctt)(r, p, q) D_2(Ctx)(r, p, q) + 8 Cty(r, p, \\ & q)^2 D_1(Ctt)(r, p, q) D_2(Ctx)(r, p, q) - 4 Cty(r, p, q)^2 D_2(Ctt)(r, p, q) D_1(Ctx)(r, p, q) \end{aligned}$$

$$\begin{aligned}
& + 8 \text{Ctx}(r, p, q)^2 D_1(\text{Ctt})(r, p, q) D_3(\text{Cty})(r, p, q) - 4 \text{Ctx}(r, p, q)^2 D_3(\text{Ctt})(r, p, \\
& q) D_1(\text{Cty})(r, p, q) - 4 \text{Ctt}(r, p, q)^2 D_2(\text{Cty})(r, p, q) D_1(\text{Cxy})(r, p, q) - 4 \text{Ctt}(r, p, \\
& q)^2 D_2(\text{Cty})(r, p, q) D_3(\text{Ctx})(r, p, q) + 4 \text{Ctt}(r, p, q)^2 D_2(\text{Ctx})(r, p, q) D_3(\text{Cty})(r, p, q) \\
& + 2 \text{Ctt}(r, p, q)^2 D_1(\text{Cxx})(r, p, q) D_3(\text{Cty})(r, p, q) - 2 \text{Ctt}(r, p, q)^2 D_3(\text{Cxx})(r, p, \\
& q) D_1(\text{Cty})(r, p, q) - \text{Ctt}(r, p, q)^2 D_3(\text{Cxx})(r, p, q) D_3(\text{Ctt})(r, p, q) + \text{Cxx}(r, p, q) \text{Ctt}(r, \\
& p, q) D_3(\text{Ctt})(r, p, q)^2 - \text{Ctt}(r, p, q) D_1(\text{Cxx})(r, p, q) D_1(\text{Ctt})(r, p, q) - 2 \text{Cty}(r, p, \\
& q)^2 D_2(\text{Ctt})(r, p, q)^2 - 2 \text{Ctx}(r, p, q)^2 D_3(\text{Ctt})(r, p, q)^2 + 2 \text{Cxy}(r, p, q)^2 D_1(\text{Ctt})(r, p, q)^2 \\
& - 2 \text{Cxx}(r, p, q) D_1(\text{Ctt})(r, p, q)^2 + \text{Ctt}(r, p, q) D_2(\text{Ctt})(r, p, q)^2 + 2 \text{Ctt}(r, p, q) \text{Cty}(r, p, \\
& q) D_2(\text{Ctt})(r, p, q) D_2(\text{Cty})(r, p, q) - 2 \text{Ctt}(r, p, q) \text{Ctx}(r, p, q) D_3(\text{Ctt})(r, p, \\
& q) D_1(\text{Cxy})(r, p, q) + 2 \text{Ctt}(r, p, q) \text{Ctx}(r, p, q) D_3(\text{Ctt})(r, p, q) D_3(\text{Ctx})(r, p, q) \\
& + 2 \text{Ctt}(r, p, q) \text{Ctx}(r, p, q) D_3(\text{Ctt})(r, p, q) D_2(\text{Cty})(r, p, q) + 2 \text{Ctt}(r, p, q) \text{Cxy}(r, p, \\
& q) D_1(\text{Ctt})(r, p, q) D_1(\text{Cxy})(r, p, q) + 2 \text{Ctt}(r, p, q) \text{Cxy}(r, p, q) D_1(\text{Ctt})(r, p, \\
& q) D_3(\text{Ctx})(r, p, q) + 2 \text{Ctt}(r, p, q) \text{Cxy}(r, p, q) D_1(\text{Ctt})(r, p, q) D_2(\text{Cty})(r, p, q) \\
& - 2 \text{Ctt}(r, p, q) \text{Cxy}(r, p, q) D_2(\text{Ctt})(r, p, q) D_3(\text{Ctt})(r, p, q) - 2 \text{Cxx}(r, p, q) \text{Ctt}(r, p, \\
& q) D_1(\text{Ctt})(r, p, q) D_3(\text{Cty})(r, p, q) - 8 \text{Ctx}(r, p, q) \text{Cty}(r, p, q) D_1(\text{Ctt})(r, p, \\
& q) D_3(\text{Ctx})(r, p, q) - 8 \text{Ctx}(r, p, q) \text{Cty}(r, p, q) D_1(\text{Ctt})(r, p, q) D_2(\text{Cty})(r, p, q) \\
& + 4 \text{Ctx}(r, p, q) \text{Cty}(r, p, q) D_3(\text{Ctt})(r, p, q) D_1(\text{Ctx})(r, p, q) + 4 \text{Ctx}(r, p, q) \text{Cty}(r, p, \\
& q) D_2(\text{Ctt})(r, p, q) D_1(\text{Cty})(r, p, q) + 4 \text{Ctx}(r, p, q) \text{Cty}(r, p, q) D_2(\text{Ctt})(r, p, \\
& q) D_3(\text{Ctt})(r, p, q) - 4 \text{Ctt}(r, p, q) \text{Cty}(r, p, q) D_1(\text{Ctt})(r, p, q) D_2(\text{Cxy})(r, p, q) - 4 \text{Ctt}(r, \\
& p, q) \text{Cty}(r, p, q) D_3(\text{Ctt})(r, p, q) D_2(\text{Ctx})(r, p, q) + 8 \text{Ctt}(r, p, q) \text{Cty}(r, p, q) D_2(\text{Cty})(r, \\
& p, q) D_1(\text{Ctx})(r, p, q) - 8 \text{Ctt}(r, p, q) \text{Cty}(r, p, q) D_2(\text{Ctx})(r, p, q) D_1(\text{Cty})(r, p, q) \\
& - 8 \text{Ctt}(r, p, q) \text{Ctx}(r, p, q) D_3(\text{Cty})(r, p, q) D_1(\text{Ctx})(r, p, q) + 8 \text{Ctt}(r, p, q) \text{Ctx}(r, p, \\
& q) D_3(\text{Ctx})(r, p, q) D_1(\text{Cty})(r, p, q) - 4 \text{Ctt}(r, p, q) \text{Ctx}(r, p, q) D_2(\text{Ctt})(r, p, \\
& q) D_3(\text{Cty})(r, p, q) - 4 \text{Cxy}(r, p, q) \text{Cty}(r, p, q) D_1(\text{Ctt})(r, p, q) D_1(\text{Ctx})(r, p, q) \\
& - 4 \text{Cxy}(r, p, q) \text{Ctx}(r, p, q) D_1(\text{Ctt})(r, p, q) D_1(\text{Cty})(r, p, q) + 4 \text{Cxx}(r, p, q) \text{Cty}(r, p, \\
& q) D_1(\text{Ctt})(r, p, q) D_1(\text{Cty})(r, p, q) + 2 \text{Ctt}(r, p, q) \text{Cty}(r, p, q) D_3(\text{Cxx})(r, p, \\
& q) D_1(\text{Ctt})(r, p, q) + 2 \text{Ctt}(r, p, q) \text{Cty}(r, p, q) D_2(\text{Ctt})(r, p, q) D_1(\text{Cxy})(r, p, q) + 2 \text{Ctt}(r, \\
& p, q) \text{Cty}(r, p, q) D_2(\text{Ctt})(r, p, q) D_3(\text{Ctx})(r, p, q) \Big),
\end{aligned}$$

$$\begin{aligned}
D_{1,2}(\text{Ctt})(r, p, q) &= \frac{1}{2} \frac{1}{\text{HessUniv}} \Big( -2 \text{Cty}(r, p, q)^2 D_2(\text{Cxx})(r, p, q) D_1(\text{Ctt})(r, p, q) + \text{Cxx}(r, \\
& p, q) \text{Ctx}(r, p, q) D_3(\text{Ctt})(r, p, q)^2 + 2 \text{Cxx}(r, p, q) D_2(\text{Ctt})(r, p, q) D_1(\text{Ctt})(r, p, q) \\
& + 2 \text{Ctt}(r, p, q)^2 D_3(\text{Cxx})(r, p, q) D_2(\text{Cty})(r, p, q) - 2 \text{Ctt}(r, p, q)^2 D_2(\text{Cxx})(r, p, \\
& q) D_3(\text{Cty})(r, p, q) + 2 \text{Cxy}(r, p, q) \text{Cty}(r, p, q) D_2(\text{Ctt})(r, p, q)^2 - 2 \text{Cxy}(r, p, \\
& q)^2 D_2(\text{Ctt})(r, p, q) D_1(\text{Ctt})(r, p, q) - 2 \text{Ctx}(r, p, q) D_2(\text{Ctt})(r, p, q) D_1(\text{Ctx})(r, p, q) \\
& - \text{Ctx}(r, p, q) D_2(\text{Ctt})(r, p, q)^2 + \text{Ctt}(r, p, q) D_2(\text{Cxx})(r, p, q) D_1(\text{Ctt})(r, p, q) - \text{Ctx}(r, p, \\
& q) D_1(\text{Cxx})(r, p, q) D_1(\text{Ctt})(r, p, q) + \text{Ctt}(r, p, q) D_2(\text{Ctt})(r, p, q) D_1(\text{Cxx})(r, p, q) \\
& - 4 \text{Cxx}(r, p, q) \text{Ctt}(r, p, q) D_3(\text{Ctx})(r, p, q) D_1(\text{Cty})(r, p, q) + 2 \text{Ctt}(r, p, q) \text{Cxy}(r, p, \\
& q) D_3(\text{Ctt})(r, p, q) D_2(\text{Ctx})(r, p, q) - 2 \text{Ctt}(r, p, q) \text{Cxy}(r, p, q) D_2(\text{Ctt})(r, p,
\end{aligned}$$

$$\begin{aligned}
& q) D_1(Cxy)(r, p, q) - 2 Ctt(r, p, q) Cxy(r, p, q) D_2(Ctt)(r, p, q) D_2(Cty)(r, p, q) \\
& + 2 Cxy(r, p, q) Cty(r, p, q) D_1(Cxx)(r, p, q) D_1(Ctt)(r, p, q) - 2 Cxx(r, p, q) Cty(r, p, q) D_1(Ctt)(r, p, q) D_1(Cxy)(r, p, q) - 2 Cxx(r, p, q) Cty(r, p, q) D_3(Ctt)(r, p, q) \\
& q) D_1(Ctx)(r, p, q) - 2 Cxx(r, p, q) Cty(r, p, q) D_2(Ctt)(r, p, q) D_1(Cty)(r, p, q) \\
& - 2 Cxx(r, p, q) Cty(r, p, q) D_2(Ctt)(r, p, q) D_3(Ctt)(r, p, q) + 2 Cxx(r, p, q) Ctx(r, p, q) D_3(Ctt)(r, p, q) D_1(Cty)(r, p, q) + 2 Cxx(r, p, q) Ctt(r, p, q) D_3(Ctt)(r, p, q) \\
& q) D_1(Cxy)(r, p, q) - 2 Cxx(r, p, q) Ctt(r, p, q) D_3(Ctt)(r, p, q) D_3(Ctx)(r, p, q) \\
& + 2 Cxx(r, p, q) Ctt(r, p, q) D_2(Ctt)(r, p, q) D_3(Cty)(r, p, q) - 2 Ctt(r, p, q) Cty(r, p, q) D_1(Cxx)(r, p, q) D_2(Cty)(r, p, q) + 2 Ctt(r, p, q) Cty(r, p, q) D_2(Cxx)(r, p, q) \\
& q) D_1(Cty)(r, p, q) - 2 Ctt(r, p, q) Ctx(r, p, q) D_3(Ctt)(r, p, q) D_2(Cxy)(r, p, q) \\
& + 4 Ctx(r, p, q) Cty(r, p, q) D_1(Ctt)(r, p, q) D_2(Cxy)(r, p, q) + 4 Ctt(r, p, q) Ctx(r, p, q) D_2(Cty)(r, p, q) D_1(Cxy)(r, p, q) - 4 Ctt(r, p, q) Ctx(r, p, q) D_2(Cxy)(r, p, q) \\
& q) D_1(Cty)(r, p, q) - 4 Ctt(r, p, q) Cxy(r, p, q) D_2(Cty)(r, p, q) D_1(Ctx)(r, p, q) \\
& + 4 Ctt(r, p, q) Cxy(r, p, q) D_2(Ctx)(r, p, q) D_1(Cty)(r, p, q) - 4 Cxy(r, p, q) Cty(r, p, q) D_1(Ctt)(r, p, q) D_2(Ctx)(r, p, q) + 4 Cxy(r, p, q) Cty(r, p, q) D_2(Ctt)(r, p, q) \\
& q) D_1(Ctx)(r, p, q) + 4 Cxy(r, p, q) Ctx(r, p, q) D_1(Ctt)(r, p, q) D_2(Cty)(r, p, q) \\
& + 4 Cxx(r, p, q) Cty(r, p, q) D_1(Ctt)(r, p, q) D_3(Ctx)(r, p, q) - 4 Cxx(r, p, q) Ctx(r, p, q) D_1(Ctt)(r, p, q) D_3(Cty)(r, p, q) + 4 Cxx(r, p, q) Ctt(r, p, q) D_3(Cty)(r, p, q) \\
& q) D_1(Ctx)(r, p, q) - Ctt(r, p, q) Cxy(r, p, q) D_3(Ctt)(r, p, q) D_1(Cxx)(r, p, q) - Ctt(r, p, q) Cxy(r, p, q) D_3(Cxx)(r, p, q) D_1(Ctt)(r, p, q) - Ctt(r, p, q) Cty(r, p, q) D_2(Ctt)(r, p, q) \\
& q) D_3(Cxx)(r, p, q) + Ctt(r, p, q) Cty(r, p, q) D_2(Cxx)(r, p, q) D_3(Ctt)(r, p, q) + Ctt(r, p, q) Ctx(r, p, q) D_3(Cxx)(r, p, q) D_3(Ctt)(r, p, q) \Big),
\end{aligned}$$

$$\begin{aligned}
D_{1,3}(Ctt)(r, p, q) = & \frac{1}{2} \frac{1}{HessUniv} \Big( 2 Ctt(r, p, q) Cxy(r, p, q) D_2(Ctt)(r, p, q) D_3(Cty)(r, p, q) \\
& - 2 Ctt(r, p, q) Cty(r, p, q) D_1(Cxx)(r, p, q) D_3(Cty)(r, p, q) + 4 Cxy(r, p, q) Ctx(r, p, q) D_3(Ctt)(r, p, q) D_1(Cty)(r, p, q) - 4 Cxy(r, p, q) Ctx(r, p, q) D_1(Ctt)(r, p, q) \\
& q) D_3(Cty)(r, p, q) - 4 Ctt(r, p, q) Cxy(r, p, q) D_3(Ctx)(r, p, q) D_1(Cty)(r, p, q) \\
& + 4 Ctt(r, p, q) Ctx(r, p, q) D_3(Cty)(r, p, q) D_1(Cxy)(r, p, q) + 2 Cxx(r, p, q) D_3(Ctt)(r, p, q) D_1(Ctt)(r, p, q) + 4 Ctt(r, p, q)^2 D_2(Cty)(r, p, q) D_3(Cxy)(r, p, q) + 4 Ctx(r, p, q) \\
& q) D_1(Ctt)(r, p, q) D_2(Cty)(r, p, q) - 4 Ctt(r, p, q) D_2(Cty)(r, p, q) D_1(Ctx)(r, p, q) \\
& - 2 Cty(r, p, q)^2 D_3(Cxx)(r, p, q) D_1(Ctt)(r, p, q) + 2 Cxy(r, p, q) Ctx(r, p, q) D_3(Ctt)(r, p, q)^2 - 2 Cxy(r, p, q)^2 D_3(Ctt)(r, p, q) D_1(Ctt)(r, p, q) - 2 Ctx(r, p, q) \\
& q) D_1(Ctt)(r, p, q) D_1(Cxy)(r, p, q) - 2 Ctx(r, p, q) D_2(Ctt)(r, p, q) D_1(Cty)(r, p, q) \\
& - 2 Ctx(r, p, q) D_2(Ctt)(r, p, q) D_3(Ctt)(r, p, q) + Cty(r, p, q) D_1(Cxx)(r, p, q) D_1(Ctt)(r, p, q) - Cxx(r, p, q) Cty(r, p, q) D_3(Ctt)(r, p, q)^2 + Cty(r, p, q) \\
& q) D_2(Ctt)(r, p, q)^2 - 2 Ctt(r, p, q) Cxy(r, p, q) D_1(Ctt)(r, p, q) D_3(Cxy)(r, p, q) \\
& - 2 Ctt(r, p, q) Cxy(r, p, q) D_3(Ctt)(r, p, q) D_3(Ctx)(r, p, q) - 2 Cxx(r, p, q) Cty(r, p, q) D_3(Ctt)(r, p, q) D_1(Cty)(r, p, q) + 4 Ctx(r, p, q) Cty(r, p, q) D_1(Ctt)(r, p, q) \Big),
\end{aligned}$$

$$\begin{aligned}
& q) D_3(Cxy)(r, p, q) - 4 Ctt(r, p, q) Ctx(r, p, q) D_3(Cxy)(r, p, q) D_1(Cty)(r, p, q) \\
& + 4 Ctt(r, p, q) Cxy(r, p, q) D_3(Cty)(r, p, q) D_1(Ctx)(r, p, q) + 4 Cxy(r, p, q) Cty(r, p, \\
& q) D_1(Ctt)(r, p, q) D_3(Ctx)(r, p, q) + 2 Ctt(r, p, q) Cty(r, p, q) D_3(Cxx)(r, p, \\
& q) D_1(Cty)(r, p, q) - 2 Ctt(r, p, q) Cty(r, p, q) D_2(Ctt)(r, p, q) D_3(Cxy)(r, p, q) \\
& - 4 Ctt(r, p, q)^2 D_2(Cxy)(r, p, q) D_3(Cty)(r, p, q) - 2 Ctx(r, p, q) D_3(Ctt)(r, p, \\
& q) D_1(Ctx)(r, p, q) - 2 Ctt(r, p, q) D_2(Ctt)(r, p, q) D_2(Cty)(r, p, q) - 4 Cty(r, p, \\
& q) D_1(Ctt)(r, p, q) D_2(Ctx)(r, p, q) + 4 Ctt(r, p, q) D_2(Ctx)(r, p, q) D_1(Cty)(r, p, q) \\
& + 2 Ctt(r, p, q) D_1(Ctt)(r, p, q) D_2(Cxy)(r, p, q) + 2 Ctt(r, p, q) D_3(Ctt)(r, p, \\
& q) D_2(Ctx)(r, p, q) + 2 Cty(r, p, q) D_2(Ctt)(r, p, q) D_1(Ctx)(r, p, q) + Ctt(r, p, q) Cty(r, \\
& p, q) D_3(Cxx)(r, p, q) D_3(Ctt)(r, p, q) \big),
\end{aligned}$$

$$\begin{aligned}
D_{2,2}(Ctt)(r, p, q) = & -\frac{1}{2} \frac{1}{HessUniv} \big( 2 Cty(r, p, q)^2 D_2(Cxx)(r, p, q) D_2(Ctt)(r, p, q) \\
& - 2 Ctx(r, p, q)^2 D_3(Cxx)(r, p, q) D_3(Ctt)(r, p, q) - 2 Cxx(r, p, q) D_1(Ctt)(r, p, \\
& q) D_2(Ctx)(r, p, q) + 2 Cxx(r, p, q)^2 D_1(Ctt)(r, p, q) D_3(Cty)(r, p, q) + 4 Ctx(r, p, \\
& q)^2 D_3(Ctt)(r, p, q) D_2(Cxy)(r, p, q) + 4 Cxy(r, p, q)^2 D_1(Ctt)(r, p, q) D_2(Ctx)(r, p, q) \\
& + 4 Ctx(r, p, q) D_2(Ctt)(r, p, q) D_2(Ctx)(r, p, q) - 2 Cxy(r, p, q)^2 D_1(Cxx)(r, p, \\
& q) D_1(Ctt)(r, p, q) - 2 Ctt(r, p, q) D_2(Cxx)(r, p, q) D_2(Ctt)(r, p, q) + Cxx(r, p, \\
& q) D_1(Cxx)(r, p, q) D_1(Ctt)(r, p, q) - Cxx(r, p, q) D_2(Ctt)(r, p, q)^2 - Cxx(r, p, \\
& q)^2 D_3(Ctt)(r, p, q)^2 - 4 Cxx(r, p, q) Ctt(r, p, q) D_2(Cty)(r, p, q) D_1(Cxy)(r, p, q) \\
& + 4 Cxx(r, p, q) Ctt(r, p, q) D_2(Cty)(r, p, q) D_3(Ctx)(r, p, q) - 2 Cxx(r, p, q) Cty(r, p, \\
& q) D_3(Cxx)(r, p, q) D_1(Ctt)(r, p, q) + 2 Cxx(r, p, q) Cty(r, p, q) D_2(Ctt)(r, p, \\
& q) D_1(Cxy)(r, p, q) - 2 Cxx(r, p, q) Cty(r, p, q) D_2(Ctt)(r, p, q) D_3(Ctx)(r, p, q) \\
& + 2 Cxx(r, p, q) Cty(r, p, q) D_2(Ctt)(r, p, q) D_2(Cty)(r, p, q) - 2 Cxx(r, p, q) Ctx(r, p, \\
& q) D_3(Ctt)(r, p, q) D_1(Cxy)(r, p, q) + 2 Cxx(r, p, q) Ctx(r, p, q) D_3(Ctt)(r, p, \\
& q) D_3(Ctx)(r, p, q) - 2 Cxx(r, p, q) Ctx(r, p, q) D_3(Ctt)(r, p, q) D_2(Cty)(r, p, q) \\
& - 2 Cxx(r, p, q) Ctt(r, p, q) D_1(Cxx)(r, p, q) D_3(Cty)(r, p, q) - 2 Cxx(r, p, q) Ctt(r, p, \\
& q) D_3(Ctt)(r, p, q) D_2(Cxy)(r, p, q) + 2 Cxx(r, p, q) Ctt(r, p, q) D_3(Cxx)(r, p, \\
& q) D_1(Cty)(r, p, q) + 2 Cxx(r, p, q) Cxy(r, p, q) D_1(Ctt)(r, p, q) D_1(Cxy)(r, p, q) \\
& - 2 Cxx(r, p, q) Cxy(r, p, q) D_1(Ctt)(r, p, q) D_3(Ctx)(r, p, q) - 2 Cxx(r, p, q) Cxy(r, p, \\
& q) D_1(Ctt)(r, p, q) D_2(Cty)(r, p, q) + 2 Cxx(r, p, q) Cxy(r, p, q) D_2(Ctt)(r, p, \\
& q) D_3(Ctt)(r, p, q) + 2 Ctx(r, p, q) Cty(r, p, q) D_2(Ctt)(r, p, q) D_3(Cxx)(r, p, q) \\
& - 2 Ctx(r, p, q) Cty(r, p, q) D_2(Cxx)(r, p, q) D_3(Ctt)(r, p, q) - 2 Cxy(r, p, q) Cty(r, p, \\
& q) D_2(Ctt)(r, p, q) D_1(Cxx)(r, p, q) + 2 Cxy(r, p, q) Cty(r, p, q) D_2(Cxx)(r, p, \\
& q) D_1(Ctt)(r, p, q) + 2 Cxy(r, p, q) Ctx(r, p, q) D_3(Ctt)(r, p, q) D_1(Cxx)(r, p, q) \\
& + 2 Cxy(r, p, q) Ctx(r, p, q) D_3(Cxx)(r, p, q) D_1(Ctt)(r, p, q) - 4 Cxx(r, p, q) Ctt(r, p, \\
& q) D_2(Ctx)(r, p, q) D_3(Cty)(r, p, q) + 4 Cxx(r, p, q) Ctt(r, p, q) D_2(Cxy)(r, p, \\
& q) D_1(Cty)(r, p, q) - 4 Ctx(r, p, q) Cty(r, p, q) D_2(Ctt)(r, p, q) D_2(Cxy)(r, p, q) \\
& - 4 Ctt(r, p, q) Ctx(r, p, q) D_3(Cxx)(r, p, q) D_2(Cty)(r, p, q) + 4 Ctt(r, p, q) Ctx(r, p,
\end{aligned}$$

$$\begin{aligned}
& q) D_2(Cxx)(r, p, q) D_3(Cty)(r, p, q) + 4 Ctt(r, p, q) Cxy(r, p, q) D_1(Cxx)(r, p, \\
& q) D_2(Cty)(r, p, q) + 4 Ctt(r, p, q) Cxy(r, p, q) D_2(Ctt)(r, p, q) D_2(Cxy)(r, p, q) \\
& - 4 Ctt(r, p, q) Cxy(r, p, q) D_2(Cxx)(r, p, q) D_1(Cty)(r, p, q) - 4 Cxy(r, p, q) Cty(r, p, \\
& q) D_2(Ctt)(r, p, q) D_2(Ctx)(r, p, q) - 4 Cxy(r, p, q) Ctx(r, p, q) D_1(Ctt)(r, p, \\
& q) D_2(Cxy)(r, p, q) - 4 Cxy(r, p, q) Ctx(r, p, q) D_3(Ctt)(r, p, q) D_2(Ctx)(r, p, q) \\
& + 4 Cxx(r, p, q) Cty(r, p, q) D_3(Ctt)(r, p, q) D_2(Ctx)(r, p, q) + Cxx(r, p, q) Ctt(r, p, \\
& q) D_3(Cxx)(r, p, q) D_3(Ctt)(r, p, q) ),
\end{aligned}$$

$$\begin{aligned}
D_{2,3}(Ctt)(r, p, q) = & \frac{1}{2} \frac{1}{HessUniv} \left( -2 Cxx(r, p, q) D_1(Ctt)(r, p, q) D_1(Cxy)(r, p, q) \right. \\
& + 4 Ctt(r, p, q) Ctx(r, p, q) D_2(Cty)(r, p, q) D_3(Cxy)(r, p, q) + 4 Ctt(r, p, q) Cxy(r, p, \\
& q) D_2(Ctx)(r, p, q) D_3(Cty)(r, p, q) - 4 Ctt(r, p, q) Ctx(r, p, q) D_2(Cxy)(r, p, \\
& q) D_3(Cty)(r, p, q) - 2 Cxx(r, p, q) Cxy(r, p, q) D_1(Ctt)(r, p, q) D_3(Cty)(r, p, q) \\
& + 2 Cxx(r, p, q) Cty(r, p, q) D_1(Ctt)(r, p, q) D_3(Cxy)(r, p, q) - 2 Cxx(r, p, q) Cty(r, p, \\
& q) D_3(Ctt)(r, p, q) D_3(Ctx)(r, p, q) + 4 Cxx(r, p, q) Ctt(r, p, q) D_3(Cty)(r, p, \\
& q) D_1(Cxy)(r, p, q) - 2 Ctt(r, p, q) Cty(r, p, q) D_2(Cxx)(r, p, q) D_3(Cty)(r, p, q) \\
& + 2 Ctt(r, p, q) Cty(r, p, q) D_3(Cxx)(r, p, q) D_2(Cty)(r, p, q) - 2 Cxx(r, p, q) Cty(r, p, \\
& q) D_3(Ctt)(r, p, q) D_2(Cty)(r, p, q) - 2 Ctt(r, p, q) Cxy(r, p, q) D_2(Ctt)(r, p, \\
& q) D_3(Cxy)(r, p, q) - 2 Ctx(r, p, q) D_2(Ctt)(r, p, q) D_2(Cty)(r, p, q) - 2 Cxy(r, p, \\
& q)^2 D_2(Ctt)(r, p, q) D_3(Ctt)(r, p, q) - 2 Cty(r, p, q)^2 D_2(Ctt)(r, p, q) D_3(Cxx)(r, p, q) \\
& + Cxy(r, p, q) D_1(Cxx)(r, p, q) D_1(Ctt)(r, p, q) + Cxx(r, p, q) Cxy(r, p, q) D_3(Ctt)(r, \\
& p, q)^2 + 2 Ctx(r, p, q) D_1(Ctt)(r, p, q) D_2(Cxy)(r, p, q) + Cxy(r, p, q) D_2(Ctt)(r, p, q)^2 \\
& + 2 Ctx(r, p, q) Cty(r, p, q) D_3(Cxx)(r, p, q) D_3(Ctt)(r, p, q) - 4 Ctt(r, p, q) Cxy(r, p, \\
& q) D_2(Cty)(r, p, q) D_3(Ctx)(r, p, q) + 4 Cxy(r, p, q) Cty(r, p, q) D_2(Ctt)(r, p, \\
& q) D_3(Ctx)(r, p, q) + 4 Cxy(r, p, q) Ctx(r, p, q) D_3(Ctt)(r, p, q) D_2(Cty)(r, p, q) - Ctx(r, \\
& p, q) D_3(Cxx)(r, p, q) D_1(Ctt)(r, p, q) - Ctx(r, p, q) D_3(Ctt)(r, p, q) D_1(Cxx)(r, p, q) \\
& - Cty(r, p, q) D_2(Cxx)(r, p, q) D_1(Ctt)(r, p, q) + Cty(r, p, q) D_2(Ctt)(r, p, q) D_1(Cxx)(r, \\
& p, q) - 2 Ctt(r, p, q) D_1(Cxx)(r, p, q) D_2(Cty)(r, p, q) + Ctt(r, p, q) D_2(Cxx)(r, p, \\
& q) D_3(Ctt)(r, p, q) + Ctt(r, p, q) D_2(Ctt)(r, p, q) D_3(Cxx)(r, p, q) + 2 Ctt(r, p, \\
& q) D_2(Cxx)(r, p, q) D_1(Cty)(r, p, q) + 2 Cxx(r, p, q) D_1(Ctt)(r, p, q) D_2(Cty)(r, p, q) \\
& - 2 Cxy(r, p, q) D_1(Ctt)(r, p, q) D_2(Ctx)(r, p, q) + 2 Cxx(r, p, q) D_1(Ctt)(r, p, \\
& q) D_3(Ctx)(r, p, q) - 2 Ctx(r, p, q) D_2(Ctt)(r, p, q) D_3(Ctx)(r, p, q) - Ctt(r, p, q) Cxy(r, \\
& p, q) D_3(Cxx)(r, p, q) D_3(Ctt)(r, p, q) - 4 Cxx(r, p, q) Ctt(r, p, q) D_3(Cxy)(r, p, \\
& q) D_1(Cty)(r, p, q) ),
\end{aligned}$$

$$\begin{aligned}
D_{3,3}(Ctt)(r, p, q) = & \frac{1}{2} \frac{1}{HessUniv} \left( -8 Ctt(r, p, q) Cxy(r, p, q) D_3(Cxy)(r, p, q) D_1(Cty)(r, p, \right. \\
& q) - 8 Ctt(r, p, q) Cty(r, p, q) D_2(Cxy)(r, p, q) D_3(Cty)(r, p, q) + 8 Ctt(r, p, q) Cty(r, p, \\
& q) D_2(Cty)(r, p, q) D_3(Cxy)(r, p, q) - 4 Cxx(r, p, q) Cty(r, p, q) D_3(Ctt)(r, p, \\
& q) D_3(Cty)(r, p, q) + 4 Cxy(r, p, q) Ctx(r, p, q) D_3(Ctt)(r, p, q) D_3(Cty)(r, p, q)
\end{aligned}$$



$$\begin{aligned}
& + 4 Ctt(r, p, q) D_2(Cxy)(r, p, q) D_1(Cty)(r, p, q) + 2 Ctt(r, p, q) D_3(Ctt)(r, p, \\
& q) D_2(Cxy)(r, p, q) - 2 D_1(Ctt)(r, p, q) D_2(Ctx)(r, p, q) + 4 Ctt(r, p, q) D_2(Ctx)(r, p, \\
& q) D_3(Cty)(r, p, q) - 4 Ctx(r, p, q) D_2(Ctt)(r, p, q) D_3(Cty)(r, p, q) + 2 Ctx(r, p, \\
& q) D_3(Ctt)(r, p, q) D_2(Cty)(r, p, q) - 4 Cxy(r, p, q)^2 D_1(Ctt)(r, p, q) D_3(Cty)(r, p, q) \\
& - 2 Ctx(r, p, q) D_3(Ctt)(r, p, q) D_1(Cxy)(r, p, q) - 2 Cty(r, p, q) D_2(Ctt)(r, p, \\
& q) D_2(Cty)(r, p, q) - 2 Cty(r, p, q) D_3(Cxx)(r, p, q) D_1(Ctt)(r, p, q) + 2 Cxx(r, p, \\
& q) D_1(Ctt)(r, p, q) D_3(Cty)(r, p, q) + 2 Cxy(r, p, q) D_1(Ctt)(r, p, q) D_3(Ctx)(r, p, q) \\
& + 2 Cxy(r, p, q) D_1(Ctt)(r, p, q) D_2(Cty)(r, p, q) + 4 Ctx(r, p, q) Cty(r, p, q) D_3(Ctt)(r, \\
& p, q) D_3(Cxy)(r, p, q) + 8 Ctt(r, p, q) Cxy(r, p, q) D_3(Cty)(r, p, q) D_1(Cxy)(r, p, q) \\
& - 4 Ctt(r, p, q) Cxy(r, p, q) D_3(Ctt)(r, p, q) D_3(Cxy)(r, p, q) - 2 Cxy(r, p, q) D_1(Ctt)(r, \\
& p, q) D_1(Cxy)(r, p, q) - 2 Cxy(r, p, q) D_2(Ctt)(r, p, q) D_3(Ctt)(r, p, q) + 2 Cty(r, p, \\
& q) D_2(Ctt)(r, p, q) D_1(Cxy)(r, p, q) + 2 Cty(r, p, q) D_2(Ctt)(r, p, q) D_3(Ctx)(r, p, q) \\
& - 2 Ctx(r, p, q) D_3(Ctt)(r, p, q) D_3(Ctx)(r, p, q) - 4 Cty(r, p, q)^2 D_2(Ctt)(r, p, \\
& q) D_3(Cxy)(r, p, q) - 4 Ctt(r, p, q) D_2(Cty)(r, p, q) D_1(Cxy)(r, p, q) - 4 Ctt(r, p, \\
& q) D_2(Cty)(r, p, q) D_3(Ctx)(r, p, q) - 2 Ctt(r, p, q) D_1(Cxx)(r, p, q) D_3(Cty)(r, p, q) \\
& + 2 Ctt(r, p, q) D_3(Cxx)(r, p, q) D_1(Cty)(r, p, q) + Ctt(r, p, q) D_3(Cxx)(r, p, \\
& q) D_3(Ctt)(r, p, q) + D_1(Cxx)(r, p, q) D_1(Ctt)(r, p, q) + Cxx(r, p, q) D_3(Ctt)(r, p, q)^2 \\
& + D_2(Ctt)(r, p, q)^2 + 4 Cxy(r, p, q) Cty(r, p, q) D_1(Ctt)(r, p, q) D_3(Cxy)(r, p, q) \\
& + 4 Cxy(r, p, q) Cty(r, p, q) D_2(Ctt)(r, p, q) D_3(Cty)(r, p, q) \Big), \\
D_{1,1}(Cxx)(r, p, q) = & -\frac{1}{2} \frac{1}{HessUniv} \Big( -4 Cxx(r, p, q) Cty(r, p, q) D_1(Ctt)(r, p, q) D_2(Cxy)(r, \\
& p, q) + 4 Cxx(r, p, q) Cty(r, p, q) D_1(Cxx)(r, p, q) D_1(Cty)(r, p, q) + 4 Cxx(r, p, q) Ctx(r, \\
& p, q) D_1(Ctt)(r, p, q) D_3(Cxy)(r, p, q) + 4 Cxx(r, p, q) Ctt(r, p, q) D_3(Ctx)(r, p, \\
& q) D_1(Cxy)(r, p, q) - 4 Cxx(r, p, q) Ctt(r, p, q) D_3(Cxy)(r, p, q) D_1(Ctx)(r, p, q) \\
& - 4 Ctx(r, p, q) Cty(r, p, q) D_3(Cxx)(r, p, q) D_1(Ctx)(r, p, q) - 4 Ctx(r, p, q) Cty(r, p, \\
& q) D_2(Cxx)(r, p, q) D_1(Cty)(r, p, q) + 4 Ctt(r, p, q) Cxy(r, p, q) D_3(Cxx)(r, p, \\
& q) D_1(Ctx)(r, p, q) - 4 Cxy(r, p, q) Cty(r, p, q) D_1(Cxx)(r, p, q) D_1(Ctx)(r, p, q) \\
& - 4 Cxy(r, p, q) Ctx(r, p, q) D_1(Cxx)(r, p, q) D_1(Cty)(r, p, q) - 2 Cxx(r, p, q) Ctt(r, p, \\
& q) D_2(Ctt)(r, p, q) D_3(Cxy)(r, p, q) + 2 Ctt(r, p, q) Cty(r, p, q) D_3(Cxx)(r, p, \\
& q) D_1(Cxx)(r, p, q) - 2 Ctt(r, p, q) Cty(r, p, q) D_2(Cxx)(r, p, q) D_1(Cxy)(r, p, q) \\
& - 2 Ctt(r, p, q) Cty(r, p, q) D_2(Cxx)(r, p, q) D_3(Ctx)(r, p, q) + 2 Ctt(r, p, q) Cty(r, p, \\
& q) D_2(Cxx)(r, p, q) D_2(Cty)(r, p, q) - 2 Ctt(r, p, q) Ctx(r, p, q) D_3(Cxx)(r, p, \\
& q) D_1(Cxy)(r, p, q) + 2 Ctt(r, p, q) Ctx(r, p, q) D_3(Cxx)(r, p, q) D_3(Ctx)(r, p, q) \\
& + 2 Ctt(r, p, q) Cxy(r, p, q) D_1(Cxx)(r, p, q) D_1(Cxy)(r, p, q) - 2 Ctt(r, p, q) Cxy(r, p,
\end{aligned}$$

$$\begin{aligned}
& q) D_1(Cxx)(r, p, q) D_3(Ctx)(r, p, q) - 2 Ctt(r, p, q) Cxy(r, p, q) D_2(Cxx)(r, p, \\
& q) D_3(Ctt)(r, p, q) + 4 Cty(r, p, q)^2 D_2(Cxx)(r, p, q) D_1(Ctx)(r, p, q) + 4 Ctx(r, p, \\
& q)^2 D_3(Cxx)(r, p, q) D_1(Cty)(r, p, q) + 4 Ctx(r, p, q) D_1(Cxx)(r, p, q) D_1(Ctx)(r, p, q) \\
& - 2 Ctt(r, p, q) D_2(Cxx)(r, p, q) D_1(Ctx)(r, p, q) + 2 Ctt(r, p, q)^2 D_2(Cxx)(r, p, \\
& q) D_3(Cxy)(r, p, q) - 2 Cty(r, p, q)^2 D_2(Cxx)(r, p, q) D_2(Ctt)(r, p, q) - 2 Ctx(r, p, \\
& q)^2 D_3(Cxx)(r, p, q) D_3(Ctt)(r, p, q) + 2 Cxy(r, p, q)^2 D_1(Cxx)(r, p, q) D_1(Ctt)(r, p, q) \\
& + Ctt(r, p, q) D_2(Cxx)(r, p, q) D_2(Ctt)(r, p, q) - 2 Cxx(r, p, q) D_1(Cxx)(r, p, \\
& q) D_1(Ctt)(r, p, q) - Ctt(r, p, q)^2 D_3(Cxx)(r, p, q)^2 - Ctt(r, p, q) D_1(Cxx)(r, p, q)^2 \\
& - 4 Cxx(r, p, q) Ctt(r, p, q) D_2(Cty)(r, p, q) D_1(Cxy)(r, p, q) + 4 Cxx(r, p, q) Cty(r, p, \\
& q) D_2(Ctt)(r, p, q) D_1(Cxy)(r, p, q) - 4 Cxx(r, p, q) Ctx(r, p, q) D_3(Ctt)(r, p, \\
& q) D_1(Cxy)(r, p, q) + 2 Cxx(r, p, q) Ctt(r, p, q) D_3(Ctt)(r, p, q) D_2(Cxy)(r, p, q) \\
& - 2 Cxx(r, p, q) Ctt(r, p, q) D_3(Cxx)(r, p, q) D_1(Cty)(r, p, q) + 2 Ctx(r, p, q) Cty(r, p, \\
& q) D_2(Ctt)(r, p, q) D_3(Cxx)(r, p, q) + 2 Ctx(r, p, q) Cty(r, p, q) D_2(Cxx)(r, p, \\
& q) D_3(Ctt)(r, p, q) - 2 Cxy(r, p, q) Cty(r, p, q) D_2(Ctt)(r, p, q) D_1(Cxx)(r, p, q) \\
& + 2 Cxy(r, p, q) Cty(r, p, q) D_2(Cxx)(r, p, q) D_1(Ctt)(r, p, q) + 2 Cxy(r, p, q) Ctx(r, p, \\
& q) D_3(Ctt)(r, p, q) D_1(Cxx)(r, p, q) - 2 Cxy(r, p, q) Ctx(r, p, q) D_3(Cxx)(r, p, \\
& q) D_1(Ctt)(r, p, q) + 4 Cxx(r, p, q) Ctt(r, p, q) D_2(Cxy)(r, p, q) D_1(Cty)(r, p, q) \\
& - 2 Ctt(r, p, q) Ctx(r, p, q) D_3(Cxx)(r, p, q) D_2(Cty)(r, p, q) + 2 Ctt(r, p, q) Cxy(r, p, \\
& q) D_1(Cxx)(r, p, q) D_2(Cty)(r, p, q) + Cxx(r, p, q) Ctt(r, p, q) D_3(Cxx)(r, p, \\
& q) D_3(Ctt)(r, p, q) ), \\
D_{1,2}(Cxx)(r, p, q) = & -\frac{1}{2} \frac{1}{HessUniv} \left( 2 Cxx(r, p, q) Ctt(r, p, q) D_3(Cxx)(r, p, q) D_3(Ctx)(r, p, \right. \\
& q) - 2 Cxx(r, p, q) Ctt(r, p, q) D_3(Cxx)(r, p, q) D_2(Cty)(r, p, q) + Cxx(r, p, q) Cxy(r, p, \\
& q) D_3(Ctt)(r, p, q) D_1(Cxx)(r, p, q) - Cxx(r, p, q) Cxy(r, p, q) D_3(Cxx)(r, p, \\
& q) D_1(Ctt)(r, p, q) - 2 Ctt(r, p, q) Ctx(r, p, q) D_3(Cxx)(r, p, q) D_2(Cxy)(r, p, q) \\
& + 4 Ctt(r, p, q) Ctx(r, p, q) D_2(Cxx)(r, p, q) D_3(Cxy)(r, p, q) + 4 Cxy(r, p, q) Cty(r, p, \\
& q) D_2(Cxx)(r, p, q) D_1(Ctx)(r, p, q) - 4 Cxy(r, p, q) Cty(r, p, q) D_1(Cxx)(r, p, \\
& q) D_2(Ctx)(r, p, q) + 2 Ctt(r, p, q) Cxy(r, p, q) D_1(Cxx)(r, p, q) D_2(Cxy)(r, p, q) \\
& - 4 Cxx(r, p, q) Ctx(r, p, q) D_2(Cty)(r, p, q) D_1(Cxy)(r, p, q) + 2 Cxx(r, p, q) Ctx(r, p, \\
& q) D_3(Cxx)(r, p, q) D_1(Cty)(r, p, q) + 4 Cxx(r, p, q) Cty(r, p, q) D_2(Ctx)(r, p, \\
& q) D_1(Cxy)(r, p, q) - 2 Cxx(r, p, q) Cty(r, p, q) D_3(Cxx)(r, p, q) D_1(Ctx)(r, p, q) \\
& - 4 Cxy(r, p, q) Ctx(r, p, q) D_2(Cxx)(r, p, q) D_1(Cty)(r, p, q) + 4 Cxx(r, p, q) Ctx(r, p, \\
& q) D_2(Cxy)(r, p, q) D_1(Cty)(r, p, q) - 4 Cxx(r, p, q) Ctt(r, p, q) D_2(Ctx)(r, p, \\
& q) D_3(Cxy)(r, p, q) - 2 Cxx(r, p, q) Cxy(r, p, q) D_1(Ctt)(r, p, q) D_2(Cxy)(r, p, q) \\
& + 2 Cxx(r, p, q) Cxy(r, p, q) D_2(Ctt)(r, p, q) D_1(Cxy)(r, p, q) + Cxx(r, p, q) Cty(r, p, \\
& q) D_2(Ctt)(r, p, q) D_3(Cxx)(r, p, q) - 2 Cxx(r, p, q) Ctt(r, p, q) D_1(Cxx)(r, p,
\end{aligned}$$

$$\begin{aligned}
& q) D_3(Cxy)(r, p, q) + Cxx(r, p, q) Cty(r, p, q) D_2(Cxx)(r, p, q) D_3(Ctt)(r, p, q) \\
& + 2 Cxx(r, p, q) Cty(r, p, q) D_1(Cxx)(r, p, q) D_1(Cxy)(r, p, q) + 2 Cxx(r, p, q) Cty(r, p, \\
& q) D_1(Cxx)(r, p, q) D_2(Cty)(r, p, q) + 2 Ctt(r, p, q) Cxy(r, p, q) D_3(Cxx)(r, p, \\
& q) D_1(Cxx)(r, p, q) + 2 Ctt(r, p, q) Cxy(r, p, q) D_3(Cxx)(r, p, q) D_2(Ctx)(r, p, q) \\
& + 2 Ctt(r, p, q) Cxy(r, p, q) D_2(Cxx)(r, p, q) D_2(Cty)(r, p, q) - 2 Cxy(r, p, q) Cty(r, p, \\
& q) D_2(Cxx)(r, p, q) D_2(Ctt)(r, p, q) - 4 Ctx(r, p, q) Cty(r, p, q) D_2(Cxx)(r, p, \\
& q) D_1(Cxy)(r, p, q) - 4 Ctt(r, p, q) Cxy(r, p, q) D_2(Cxx)(r, p, q) D_3(Ctx)(r, p, q) \\
& - 4 Cxx(r, p, q) Cty(r, p, q) D_2(Cxy)(r, p, q) D_1(Ctx)(r, p, q) + 4 Cxx(r, p, q) Ctt(r, p, \\
& q) D_2(Cxy)(r, p, q) D_3(Ctx)(r, p, q) - 2 Cxy(r, p, q) Cty(r, p, q) D_1(Cxx)(r, p, q)^2 \\
& + 2 Ctx(r, p, q) D_1(Cxx)(r, p, q) D_2(Ctx)(r, p, q) - 2 Ctt(r, p, q) D_2(Cxx)(r, p, \\
& q) D_1(Cxx)(r, p, q) + 2 Cty(r, p, q)^2 D_2(Cxx)(r, p, q) D_1(Cxx)(r, p, q) - Ctt(r, p, \\
& q) Ctx(r, p, q) D_3(Cxx)(r, p, q)^2 + Ctx(r, p, q) D_2(Cxx)(r, p, q) D_2(Ctt)(r, p, q) + Ctx(r, \\
& p, q) D_1(Cxx)(r, p, q)^2 - Cxx(r, p, q) Ctx(r, p, q) D_3(Cxx)(r, p, q) D_3(Ctt)(r, p, q) \\
& + 2 Cxx(r, p, q)^2 D_1(Ctt)(r, p, q) D_3(Cxy)(r, p, q) - Cxx(r, p, q) D_2(Cxx)(r, p, \\
& q) D_1(Ctt)(r, p, q) - 2 Cxx(r, p, q)^2 D_3(Ctt)(r, p, q) D_1(Cxy)(r, p, q) - Cxx(r, p, \\
& q) D_2(Ctt)(r, p, q) D_1(Cxx)(r, p, q) + 2 Cxy(r, p, q)^2 D_2(Cxx)(r, p, q) D_1(Ctt)(r, p, q) \Big), \\
D_{1,3}(Cxx)(r, p, q) = & -\frac{1}{2} \frac{1}{HessUniv} \Big( -4 Cxx(r, p, q) Ctx(r, p, q) D_3(Cty)(r, p, q) D_1(Cxy)(r, \\
& p, q) - 2 Ctt(r, p, q) Cxy(r, p, q) D_2(Cxx)(r, p, q) D_3(Cty)(r, p, q) + 2 Ctt(r, p, q) Cxy(r, \\
& p, q) D_3(Cxx)(r, p, q) D_3(Ctx)(r, p, q) + 2 Ctt(r, p, q) Cty(r, p, q) D_2(Cxx)(r, p, \\
& q) D_3(Cxy)(r, p, q) + 4 Cxx(r, p, q) Ctx(r, p, q) D_3(Cxy)(r, p, q) D_1(Cty)(r, p, q) \\
& - 4 Cxx(r, p, q) Cty(r, p, q) D_3(Cxy)(r, p, q) D_1(Ctx)(r, p, q) + Cxy(r, p, q) D_2(Cxx)(r, \\
& p, q) D_1(Ctt)(r, p, q) - 2 Cxx(r, p, q) D_1(Ctt)(r, p, q) D_2(Cxy)(r, p, q) + 2 Ctx(r, p, \\
& q) D_1(Cxx)(r, p, q) D_1(Cxy)(r, p, q) + 4 Cxx(r, p, q) Ctt(r, p, q) D_2(Cxy)(r, p, \\
& q) D_3(Cty)(r, p, q) + 2 Cxx(r, p, q) Cty(r, p, q) D_1(Cxx)(r, p, q) D_3(Cty)(r, p, q) \\
& + 2 Cxx(r, p, q) Cxy(r, p, q) D_1(Ctt)(r, p, q) D_3(Cxy)(r, p, q) - 2 Cxx(r, p, q) Cxy(r, p, \\
& q) D_3(Ctt)(r, p, q) D_1(Cxy)(r, p, q) - 4 Cxx(r, p, q) Ctt(r, p, q) D_2(Cty)(r, p, \\
& q) D_3(Cxy)(r, p, q) + 2 Ctt(r, p, q) D_2(Cxx)(r, p, q) D_2(Cty)(r, p, q) - 4 Ctx(r, p, \\
& q) Cty(r, p, q) D_3(Cxx)(r, p, q) D_1(Cxy)(r, p, q) - 4 Cxy(r, p, q) Cty(r, p, q) D_1(Cxx)(r, \\
& p, q) D_3(Ctx)(r, p, q) + 4 Cxx(r, p, q) Cty(r, p, q) D_3(Ctx)(r, p, q) D_1(Cxy)(r, p, q) \\
& - 2 Cxy(r, p, q) Ctx(r, p, q) D_3(Cxx)(r, p, q) D_3(Ctt)(r, p, q) + 2 Cty(r, p, q) D_2(Cxx)(r, \\
& p, q) D_1(Ctx)(r, p, q) - 2 Ctt(r, p, q) D_2(Cxx)(r, p, q) D_1(Cxy)(r, p, q) + 2 Cty(r, p, \\
& q)^2 D_3(Cxx)(r, p, q) D_1(Cxx)(r, p, q) + 2 Cxy(r, p, q)^2 D_3(Ctt)(r, p, q) D_1(Cxx)(r, p, q) \\
& - Ctt(r, p, q) Cty(r, p, q) D_3(Cxx)(r, p, q)^2 - Cty(r, p, q) D_2(Cxx)(r, p, q) D_2(Ctt)(r, p,
\end{aligned}$$

$$\begin{aligned}
& q) + 2 Cxx(r, p, q) D_2(Ctt)(r, p, q) D_1(Cxy)(r, p, q) - Cty(r, p, q) D_1(Cxx)(r, p, q)^2 \\
& + Cxx(r, p, q) Cty(r, p, q) D_3(Cxx)(r, p, q) D_3(Ctt)(r, p, q) + 2 Ctx(r, p, q) D_1(Cxx)(r, \\
& p, q) D_3(Ctx)(r, p, q) + 2 Ctt(r, p, q) Cxy(r, p, q) D_3(Cxx)(r, p, q) D_1(Cxy)(r, p, q) \\
& - 2 Ctt(r, p, q) D_2(Cxx)(r, p, q) D_3(Ctx)(r, p, q) - Cxx(r, p, q) D_3(Ctt)(r, p, \\
& q) D_1(Cxx)(r, p, q) - Cxy(r, p, q) D_2(Ctt)(r, p, q) D_1(Cxx)(r, p, q) + Ctx(r, p, \\
& q) D_2(Ctt)(r, p, q) D_3(Cxx)(r, p, q) - Cxx(r, p, q) D_3(Cxx)(r, p, q) D_1(Ctt)(r, p, q) \\
& + Ctx(r, p, q) D_2(Cxx)(r, p, q) D_3(Ctt)(r, p, q) - 2 Ctx(r, p, q) D_2(Cxx)(r, p, \\
& q) D_1(Cty)(r, p, q) ),
\end{aligned}$$

$$\begin{aligned}
D_{2,2}(Cxx)(r, p, q) = & -\frac{1}{2} \frac{1}{HessUniv} \Big( -4 Cxx(r, p, q) Cxy(r, p, q) D_2(Cxx)(r, p, q) D_1(Cty)(r, \\
& p, q) - 2 Cxx(r, p, q) Cty(r, p, q) D_3(Cxx)(r, p, q) D_1(Cxx)(r, p, q) + 2 Cxx(r, p, \\
& q) Cty(r, p, q) D_2(Cxx)(r, p, q) D_1(Cxy)(r, p, q) + 2 Cxx(r, p, q) Cty(r, p, q) D_2(Cxx)(r, \\
& p, q) D_3(Ctx)(r, p, q) + 2 Cxx(r, p, q) Cty(r, p, q) D_2(Cxx)(r, p, q) D_2(Cty)(r, p, q) \\
& + 2 Cxx(r, p, q) Ctx(r, p, q) D_3(Cxx)(r, p, q) D_1(Cxy)(r, p, q) + 2 Cxx(r, p, q) Ctx(r, p, \\
& q) D_3(Cxx)(r, p, q) D_3(Ctx)(r, p, q) - 2 Cxx(r, p, q) Ctx(r, p, q) D_3(Cxx)(r, p, \\
& q) D_2(Cty)(r, p, q) - 2 Cxx(r, p, q) Ctt(r, p, q) D_2(Cxx)(r, p, q) D_3(Cxy)(r, p, q) \\
& + 2 Cxx(r, p, q) Cxy(r, p, q) D_1(Cxx)(r, p, q) D_1(Cxy)(r, p, q) + 2 Cxx(r, p, q) Cxy(r, p, \\
& q) D_1(Cxx)(r, p, q) D_3(Ctx)(r, p, q) + 2 Cxx(r, p, q) Cxy(r, p, q) D_1(Cxx)(r, p, \\
& q) D_2(Cty)(r, p, q) + 2 Cxx(r, p, q) Cxy(r, p, q) D_2(Cxx)(r, p, q) D_3(Ctt)(r, p, q) \\
& - 4 Ctx(r, p, q) Cty(r, p, q) D_2(Cxx)(r, p, q) D_2(Cxy)(r, p, q) + 4 Ctt(r, p, q) Cxy(r, p, \\
& q) D_2(Cxx)(r, p, q) D_2(Cxy)(r, p, q) - 4 Cxy(r, p, q) Cty(r, p, q) D_2(Cxx)(r, p, \\
& q) D_2(Ctx)(r, p, q) + 4 Cxy(r, p, q) Ctx(r, p, q) D_1(Cxx)(r, p, q) D_2(Cxy)(r, p, q) \\
& + 4 Cxy(r, p, q) Ctx(r, p, q) D_3(Cxx)(r, p, q) D_1(Cxx)(r, p, q) + 4 Cxy(r, p, q) Ctx(r, p, \\
& q) D_3(Cxx)(r, p, q) D_2(Ctx)(r, p, q) - 8 Cxy(r, p, q) Ctx(r, p, q) D_2(Cxx)(r, p, \\
& q) D_1(Cxy)(r, p, q) - 8 Cxy(r, p, q) Ctx(r, p, q) D_2(Cxx)(r, p, q) D_3(Ctx)(r, p, q) \\
& - 4 Cxx(r, p, q) Ctx(r, p, q) D_1(Cxx)(r, p, q) D_3(Cxy)(r, p, q) - 8 Cxx(r, p, q) Ctx(r, p, \\
& q) D_2(Ctx)(r, p, q) D_3(Cxy)(r, p, q) + 8 Cxx(r, p, q) Ctx(r, p, q) D_2(Cxy)(r, p, \\
& q) D_3(Ctx)(r, p, q) - 4 Cxx(r, p, q) Cxy(r, p, q) D_3(Cxx)(r, p, q) D_1(Ctx)(r, p, q) \\
& + 8 Cxx(r, p, q) Cxy(r, p, q) D_2(Ctx)(r, p, q) D_1(Cxy)(r, p, q) - 8 Cxx(r, p, q) Cxy(r, p, \\
& q) D_2(Cxy)(r, p, q) D_1(Ctx)(r, p, q) - 2 Cxx(r, p, q)^2 D_3(Ctt)(r, p, q) D_2(Cxy)(r, p, q) \\
& + 2 Cxx(r, p, q)^2 D_3(Cxx)(r, p, q) D_1(Cty)(r, p, q) + 2 Cxx(r, p, q)^2 D_2(Ctt)(r, p, \\
& q) D_3(Cxy)(r, p, q) - 4 Ctx(r, p, q)^2 D_3(Cxx)(r, p, q) D_2(Cxy)(r, p, q) + 8 Ctx(r, p, \\
& q)^2 D_2(Cxx)(r, p, q) D_3(Cxy)(r, p, q) - 4 Cxy(r, p, q)^2 D_1(Cxx)(r, p, q) D_2(Ctx)(r, p, q) \\
& + 8 Cxy(r, p, q)^2 D_2(Cxx)(r, p, q) D_1(Ctx)(r, p, q) + 4 Ctx(r, p, q) D_2(Cxx)(r, p, \\
& q) D_2(Ctx)(r, p, q) - 4 Cxx(r, p, q)^2 D_3(Ctx)(r, p, q) D_1(Cxy)(r, p, q) + 4 Cxx(r, p,
\end{aligned}$$

$$\begin{aligned}
& q)^2 D_3(Cxy)(r, p, q) D_1(Ctx)(r, p, q) - 4 Cxx(r, p, q)^2 D_2(Cty)(r, p, q) D_1(Cxy)(r, p, q) \\
& + 4 Cxx(r, p, q)^2 D_2(Cxy)(r, p, q) D_1(Cty)(r, p, q) - 2 Cxx(r, p, q) D_2(Cxx)(r, p, \\
& q) D_1(Ctx)(r, p, q) + Cxx(r, p, q) Ctt(r, p, q) D_3(Cxx)(r, p, q)^2 - Cxx(r, p, q) D_2(Cxx)(r, \\
& p, q) D_2(Ctt)(r, p, q) - Cxx(r, p, q)^2 D_3(Cxx)(r, p, q) D_3(Ctt)(r, p, q) + 2 Cty(r, p, \\
& q)^2 D_2(Cxx)(r, p, q)^2 - 2 Ctx(r, p, q)^2 D_3(Cxx)(r, p, q)^2 - 2 Cxy(r, p, q)^2 D_1(Cxx)(r, \\
& p, q)^2 - 2 Ctt(r, p, q) D_2(Cxx)(r, p, q)^2 + Cxx(r, p, q) D_1(Cxx)(r, p, q)^2), \\
D_{2,3}(Cxx)(r, p, q) = & \frac{1}{2} \frac{1}{HessUniv} \left( -2 Ctx(r, p, q) D_3(Cxx)(r, p, q) D_2(Ctx)(r, p, q) \right. \\
& + 2 Cxy(r, p, q) D_1(Cxx)(r, p, q) D_2(Ctx)(r, p, q) - 2 Cxx(r, p, q) Cxy(r, p, \\
& q) D_1(Cxx)(r, p, q) D_3(Cty)(r, p, q) + 2 Cxx(r, p, q) Cxy(r, p, q) D_3(Ctt)(r, p, \\
& q) D_2(Cxy)(r, p, q) - 2 Ctt(r, p, q) Cxy(r, p, q) D_3(Cxx)(r, p, q) D_2(Cxy)(r, p, q) \\
& - 2 Cxx(r, p, q) Cty(r, p, q) D_3(Cxx)(r, p, q) D_3(Ctx)(r, p, q) - 2 Cxx(r, p, q) Cty(r, p, \\
& q) D_2(Cxx)(r, p, q) D_3(Cty)(r, p, q) + 4 Cxx(r, p, q) Cty(r, p, q) D_2(Ctx)(r, p, \\
& q) D_3(Cxy)(r, p, q) - 4 Cxx(r, p, q) Ctx(r, p, q) D_2(Cxy)(r, p, q) D_3(Cty)(r, p, q) \\
& + 4 Cxy(r, p, q) Cty(r, p, q) D_2(Cxx)(r, p, q) D_3(Ctx)(r, p, q) + 4 Cxy(r, p, q) Ctx(r, p, \\
& q) D_2(Cxx)(r, p, q) D_3(Cty)(r, p, q) - 4 Cxy(r, p, q) D_2(Cxx)(r, p, q) D_1(Ctx)(r, p, q) \\
& + 4 Cxx(r, p, q)^2 D_3(Cty)(r, p, q) D_1(Cxy)(r, p, q) - 2 Cxy(r, p, q)^2 D_2(Cxx)(r, p, \\
& q) D_3(Ctt)(r, p, q) - 2 Ctx(r, p, q) D_1(Cxx)(r, p, q) D_2(Cxy)(r, p, q) - 2 Ctx(r, p, \\
& q) D_3(Cxx)(r, p, q) D_1(Cxx)(r, p, q) - 2 Ctx(r, p, q) D_2(Cxx)(r, p, q) D_2(Cty)(r, p, q) \\
& + 2 Ctt(r, p, q) D_2(Cxx)(r, p, q) D_3(Cxx)(r, p, q) - 2 Cty(r, p, q)^2 D_2(Cxx)(r, p, \\
& q) D_3(Cxx)(r, p, q) + 2 Ctx(r, p, q) Cty(r, p, q) D_3(Cxx)(r, p, q)^2 + 4 Ctx(r, p, \\
& q) D_2(Cxx)(r, p, q) D_1(Cxy)(r, p, q) - 4 Cxx(r, p, q) D_2(Ctx)(r, p, q) D_1(Cxy)(r, p, q) \\
& - Ctt(r, p, q) Cxy(r, p, q) D_3(Cxx)(r, p, q)^2 + Cxy(r, p, q) D_2(Cxx)(r, p, q) D_2(Ctt)(r, p, \\
& q) + 4 Cxx(r, p, q) D_2(Cxy)(r, p, q) D_1(Ctx)(r, p, q) - 2 Cxx(r, p, q) D_1(Cxx)(r, p, \\
& q) D_1(Cxy)(r, p, q) - 4 Cxx(r, p, q)^2 D_3(Cxy)(r, p, q) D_1(Cty)(r, p, q) + 2 Cxx(r, p, \\
& q) D_3(Cxx)(r, p, q) D_1(Ctx)(r, p, q) + 2 Cxx(r, p, q) D_2(Cxx)(r, p, q) D_1(Cty)(r, p, q) \\
& + Cxy(r, p, q) D_1(Cxx)(r, p, q)^2 + 2 Cxx(r, p, q) Cty(r, p, q) D_1(Cxx)(r, p, q) D_3(Cxy)(r, \\
& p, q) - 4 Cxx(r, p, q) Cty(r, p, q) D_2(Cxy)(r, p, q) D_3(Ctx)(r, p, q) + 4 Cxx(r, p, q) Ctx(r, \\
& p, q) D_2(Cty)(r, p, q) D_3(Cxy)(r, p, q) - 2 Cxx(r, p, q) Cxy(r, p, q) D_2(Ctt)(r, p, \\
& q) D_3(Cxy)(r, p, q) + 4 Ctx(r, p, q) Cty(r, p, q) D_3(Cxx)(r, p, q) D_2(Cxy)(r, p, q) \\
& - 4 Ctx(r, p, q) Cty(r, p, q) D_2(Cxx)(r, p, q) D_3(Cxy)(r, p, q) + Cxx(r, p, q) Cxy(r, p, \\
& q) D_3(Cxx)(r, p, q) D_3(Ctt)(r, p, q) \Big), \\
D_{3,3}(Cxx)(r, p, q) = & \frac{1}{2} \frac{1}{HessUniv} \left( 4 Cxy(r, p, q) Cty(r, p, q) D_1(Cxx)(r, p, q) D_3(Cxy)(r, p, \\
& q) + 4 Cxy(r, p, q) Cty(r, p, q) D_2(Cxx)(r, p, q) D_3(Cty)(r, p, q) + 4 Cxy(r, p, q) Ctx(r, p, \\
& q) D_3(Cxx)(r, p, q) D_3(Cty)(r, p, q) - 4 Cxx(r, p, q) Cty(r, p, q) D_3(Cxx)(r, p,
\end{aligned}$$

$$\begin{aligned}
& q) D_3(Cty)(r, p, q) + 8 Cxx(r, p, q) Cty(r, p, q) D_2(Cty)(r, p, q) D_3(Cxy)(r, p, q) \\
& - 4 Cty(r, p, q)^2 D_2(Cxx)(r, p, q) D_3(Cxy)(r, p, q) + 2 Cty(r, p, q) D_2(Cxx)(r, p, \\
& q) D_3(Ctx)(r, p, q) + 2 Cty(r, p, q) D_2(Cxx)(r, p, q) D_1(Cxy)(r, p, q) + 2 Ctx(r, p, \\
& q) D_3(Cxx)(r, p, q) D_1(Cxy)(r, p, q) - 4 Ctx(r, p, q) D_1(Cxx)(r, p, q) D_3(Cxy)(r, p, q) \\
& - 2 Ctx(r, p, q) D_3(Cxx)(r, p, q) D_2(Cty)(r, p, q) + 2 Cxx(r, p, q) D_3(Cxx)(r, p, \\
& q) D_1(Cty)(r, p, q) + D_1(Cxx)(r, p, q)^2 + 4 Cxx(r, p, q) D_2(Cxy)(r, p, q) D_1(Cty)(r, p, q) \\
& + 4 Cxx(r, p, q) D_3(Cxy)(r, p, q) D_1(Ctx)(r, p, q) - 2 Cxy(r, p, q) D_2(Cxx)(r, p, \\
& q) D_3(Ctt)(r, p, q) - 2 Cty(r, p, q) D_3(Cxx)(r, p, q) D_1(Cxx)(r, p, q) - 2 Cty(r, p, \\
& q) D_2(Cxx)(r, p, q) D_2(Cty)(r, p, q) - 2 Ctx(r, p, q) D_3(Cxx)(r, p, q) D_3(Ctx)(r, p, q) \\
& + 2 Cxy(r, p, q) D_1(Cxx)(r, p, q) D_3(Ctx)(r, p, q) + 2 Cxy(r, p, q) D_1(Cxx)(r, p, \\
& q) D_2(Cty)(r, p, q) - 2 Cxx(r, p, q) D_2(Ctt)(r, p, q) D_3(Cxy)(r, p, q) - 4 Cxy(r, p, \\
& q)^2 D_1(Cxx)(r, p, q) D_3(Cty)(r, p, q) - 4 Cxx(r, p, q) D_3(Ctx)(r, p, q) D_1(Cxy)(r, p, q) \\
& - 4 Cxx(r, p, q) D_2(Cty)(r, p, q) D_1(Cxy)(r, p, q) + 2 Cxx(r, p, q) D_3(Ctt)(r, p, \\
& q) D_2(Cxy)(r, p, q) + Cxx(r, p, q) D_3(Cxx)(r, p, q) D_3(Ctt)(r, p, q) + 2 Ctt(r, p, \\
& q) D_2(Cxx)(r, p, q) D_3(Cxy)(r, p, q) - 2 Cxy(r, p, q) D_1(Cxx)(r, p, q) D_1(Cxy)(r, p, q) \\
& + Ctt(r, p, q) D_3(Cxx)(r, p, q)^2 + D_2(Cxx)(r, p, q) D_2(Ctt)(r, p, q) - 2 D_2(Cxx)(r, p, \\
& q) D_1(Ctx)(r, p, q) - 4 Ctt(r, p, q) Cxy(r, p, q) D_3(Cxx)(r, p, q) D_3(Cxy)(r, p, q) \\
& - 8 Cxx(r, p, q) Cty(r, p, q) D_2(Cxy)(r, p, q) D_3(Cty)(r, p, q) + 8 Cxx(r, p, q) Cxy(r, p, \\
& q) D_3(Cty)(r, p, q) D_1(Cxy)(r, p, q) - 8 Cxx(r, p, q) Cxy(r, p, q) D_3(Cxy)(r, p, \\
& q) D_1(Cty)(r, p, q) + 4 Ctx(r, p, q) Cty(r, p, q) D_3(Cxx)(r, p, q) D_3(Cxy)(r, p, q) ), \\
D_{1,1}(Ctx)(r, p, q) = & \frac{1}{4} \frac{1}{HessUniv} \left( -8 Cty(r, p, q)^2 D_2(Ctx)(r, p, q) D_1(Ctx)(r, p, q) \right. \\
& + 4 Cty(r, p, q)^2 D_2(Ctt)(r, p, q) D_1(Cxx)(r, p, q) + 4 Cty(r, p, q)^2 D_2(Ctt)(r, p, \\
& q) D_2(Ctx)(r, p, q) - 8 Ctx(r, p, q)^2 D_1(Ctt)(r, p, q) D_3(Cxy)(r, p, q) - 8 Ctx(r, p, \\
& q)^2 D_3(Ctx)(r, p, q) D_1(Cty)(r, p, q) + 8 Ctx(r, p, q)^2 D_3(Ctt)(r, p, q) D_1(Cxy)(r, p, q) \\
& + 4 Ctx(r, p, q)^2 D_3(Ctt)(r, p, q) D_3(Ctx)(r, p, q) - 4 Ctt(r, p, q) Ctx(r, p, \\
& q) D_3(Ctx)(r, p, q)^2 - 4 Ctt(r, p, q)^2 D_2(Ctx)(r, p, q) D_3(Cxy)(r, p, q) + 8 Cxy(r, p, \\
& q) Cty(r, p, q) D_1(Ctx)(r, p, q)^2 - 4 Cxy(r, p, q)^2 D_1(Ctt)(r, p, q) D_1(Ctx)(r, p, q) \\
& + 4 Ctt(r, p, q) D_2(Ctx)(r, p, q) D_1(Ctx)(r, p, q) + 4 Cxx(r, p, q) D_1(Ctt)(r, p, \\
& q) D_1(Ctx)(r, p, q) + 2 Ctt(r, p, q) D_1(Cxx)(r, p, q) D_1(Ctx)(r, p, q) - 2 Ctt(r, p, \\
& q) D_2(Ctt)(r, p, q) D_2(Ctx)(r, p, q) - 2 Ctt(r, p, q)^2 D_1(Cxx)(r, p, q) D_3(Cxy)(r, p, q) \\
& + 2 Ctt(r, p, q)^2 D_3(Cxx)(r, p, q) D_1(Cxy)(r, p, q) + 2 Ctt(r, p, q)^2 D_3(Cxx)(r, p, \\
& q) D_3(Ctx)(r, p, q) + 4 Cxx(r, p, q) Ctt(r, p, q) D_3(Cty)(r, p, q) D_1(Ctx)(r, p, q) \\
& - 4 Cxx(r, p, q) Cty(r, p, q) D_2(Ctt)(r, p, q) D_1(Cty)(r, p, q) + 4 Cxx(r, p, q) Ctx(r, p, \\
& q) D_3(Ctt)(r, p, q) D_1(Cty)(r, p, q) - 2 Cxx(r, p, q) Ctt(r, p, q) D_3(Ctt)(r, p,
\end{aligned}$$

$$\begin{aligned}
& q) D_1(Cxy)(r, p, q) - 2 Cxx(r, p, q) Ctt(r, p, q) D_3(Ctt)(r, p, q) D_3(Ctx)(r, p, q) \\
& + 2 Cxx(r, p, q) Ctt(r, p, q) D_2(Ctt)(r, p, q) D_3(Cty)(r, p, q) - 4 Cxx(r, p, q) Ctx(r, p, \\
& q) D_1(Ctt)(r, p, q) D_3(Cty)(r, p, q) - 4 Ctt(r, p, q) Cty(r, p, q) D_1(Cxx)(r, p, \\
& q) D_2(Cty)(r, p, q) + 4 Ctt(r, p, q) Cty(r, p, q) D_2(Cxx)(r, p, q) D_1(Cty)(r, p, q) \\
& - 4 Ctt(r, p, q) Ctx(r, p, q) D_3(Ctt)(r, p, q) D_2(Cxy)(r, p, q) + 4 Ctt(r, p, q) Cxy(r, p, \\
& q) D_3(Ctt)(r, p, q) D_2(Ctx)(r, p, q) + 8 Ctx(r, p, q) Cty(r, p, q) D_1(Ctt)(r, p, \\
& q) D_2(Cxy)(r, p, q) - 2 Ctt(r, p, q) Cty(r, p, q) D_2(Ctt)(r, p, q) D_3(Cxx)(r, p, q) \\
& + 2 Ctt(r, p, q) Cty(r, p, q) D_2(Cxx)(r, p, q) D_3(Ctt)(r, p, q) + 8 Ctt(r, p, q) Ctx(r, p, \\
& q) D_2(Cty)(r, p, q) D_1(Cxy)(r, p, q) - 8 Ctt(r, p, q) Ctx(r, p, q) D_2(Cxy)(r, p, \\
& q) D_1(Cty)(r, p, q) + 2 Ctt(r, p, q) Cxy(r, p, q) D_3(Ctt)(r, p, q) D_1(Cxx)(r, p, q) \\
& - 2 Ctt(r, p, q) Cxy(r, p, q) D_3(Cxx)(r, p, q) D_1(Ctt)(r, p, q) - 4 Ctt(r, p, q) Cxy(r, p, \\
& q) D_2(Cty)(r, p, q) D_1(Ctx)(r, p, q) - 4 Cxy(r, p, q) Cty(r, p, q) D_1(Ctt)(r, p, \\
& q) D_2(Ctx)(r, p, q) + 4 Cxy(r, p, q) Cty(r, p, q) D_2(Ctt)(r, p, q) D_1(Ctx)(r, p, q) \\
& - 4 Cty(r, p, q)^2 D_2(Cxx)(r, p, q) D_1(Ctt)(r, p, q) + 2 Ctt(r, p, q)^2 D_3(Cxx)(r, p, \\
& q) D_2(Cty)(r, p, q) - 2 Ctt(r, p, q)^2 D_2(Cxx)(r, p, q) D_3(Cty)(r, p, q) - Ctt(r, p, \\
& q) D_2(Ctt)(r, p, q) D_1(Cxx)(r, p, q) + Ctt(r, p, q) D_2(Cxx)(r, p, q) D_1(Ctt)(r, p, q) \\
& - 8 Ctx(r, p, q) D_1(Ctx)(r, p, q)^2 + 2 Cxx(r, p, q) Ctt(r, p, q) D_1(Ctt)(r, p, q) D_3(Cxy)(r, \\
& p, q) - 2 Cxx(r, p, q) Ctt(r, p, q) D_3(Ctt)(r, p, q) D_2(Cty)(r, p, q) - 8 Cxx(r, p, q) Cty(r, \\
& p, q) D_1(Ctx)(r, p, q) D_1(Cty)(r, p, q) + 4 Cxx(r, p, q) Cty(r, p, q) D_1(Ctt)(r, p, \\
& q) D_2(Cty)(r, p, q) + 8 Ctx(r, p, q) Cty(r, p, q) D_3(Ctx)(r, p, q) D_1(Ctx)(r, p, q) \\
& - 4 Ctx(r, p, q) Cty(r, p, q) D_3(Ctt)(r, p, q) D_1(Cxx)(r, p, q) - 4 Ctx(r, p, q) Cty(r, p, \\
& q) D_3(Ctt)(r, p, q) D_2(Ctx)(r, p, q) + 4 Ctx(r, p, q) Cty(r, p, q) D_3(Cxx)(r, p, \\
& q) D_1(Ctt)(r, p, q) + 8 Ctx(r, p, q) Cty(r, p, q) D_2(Ctx)(r, p, q) D_1(Cty)(r, p, q) \\
& - 8 Ctx(r, p, q) Cty(r, p, q) D_2(Ctt)(r, p, q) D_1(Cxy)(r, p, q) - 4 Ctx(r, p, q) Cty(r, p, \\
& q) D_2(Ctt)(r, p, q) D_3(Ctx)(r, p, q) - 4 Ctt(r, p, q) Cty(r, p, q) D_3(Cxx)(r, p, \\
& q) D_1(Ctx)(r, p, q) + 4 Ctt(r, p, q) Cty(r, p, q) D_2(Ctx)(r, p, q) D_1(Cxy)(r, p, q) \\
& + 4 Ctt(r, p, q) Cty(r, p, q) D_2(Ctx)(r, p, q) D_3(Ctx)(r, p, q) - 4 Ctt(r, p, q) Cty(r, p, \\
& q) D_2(Ctx)(r, p, q) D_2(Cty)(r, p, q) - 4 Ctt(r, p, q) Ctx(r, p, q) D_3(Ctx)(r, p, \\
& q) D_1(Cxy)(r, p, q) + 8 Ctt(r, p, q) Ctx(r, p, q) D_3(Cxy)(r, p, q) D_1(Ctx)(r, p, q) \\
& + 4 Ctt(r, p, q) Ctx(r, p, q) D_2(Cty)(r, p, q) D_3(Ctx)(r, p, q) + 4 Ctt(r, p, q) Ctx(r, p, \\
& q) D_2(Ctt)(r, p, q) D_3(Cxy)(r, p, q) - 4 Ctt(r, p, q) Cxy(r, p, q) D_1(Cxy)(r, p, \\
& q) D_1(Ctx)(r, p, q) - 4 Ctt(r, p, q) Cxy(r, p, q) D_3(Ctx)(r, p, q) D_1(Ctx)(r, p, q) \\
& + 8 Cxy(r, p, q) Ctx(r, p, q) D_1(Ctx)(r, p, q) D_1(Cty)(r, p, q) + 4 Cxy(r, p, q) Ctx(r, p, \\
& q) D_1(Ctt)(r, p, q) D_3(Ctx)(r, p, q) - 4 Cxy(r, p, q) Ctx(r, p, q) D_3(Ctt)(r, p, \\
& q) D_1(Ctx)(r, p, q) \big), \\
D_{1,2}(Ctx)(r, p, q) = & -\frac{1}{4} \frac{1}{HessUniv} \big( 4 Cty(r, p, q)^2 D_2(Cxx)(r, p, q) D_1(Ctx)(r, p, q)
\end{aligned}$$

$$\begin{aligned}
& + 2 \text{Ctx}(r, p, q) D_1(\text{Cxx})(r, p, q) D_1(\text{Ctx})(r, p, q) - 2 \text{Ctt}(r, p, q) D_2(\text{Cxx})(r, p, \\
& q) D_1(\text{Ctx})(r, p, q) + 2 \text{Ctt}(r, p, q)^2 D_2(\text{Cxx})(r, p, q) D_3(\text{Cxy})(r, p, q) - 8 \text{Ctx}(r, p, \\
& q)^2 D_2(\text{Cty})(r, p, q) D_1(\text{Cxy})(r, p, q) + 8 \text{Ctx}(r, p, q)^2 D_2(\text{Cxy})(r, p, q) D_1(\text{Cty})(r, p, q) \\
& + 4 \text{Ctx}(r, p, q) D_2(\text{Ctx})(r, p, q) D_1(\text{Ctx})(r, p, q) + \text{Ctx}(r, p, q) D_2(\text{Ctt})(r, p, \\
& q) D_1(\text{Cxx})(r, p, q) - \text{Ctx}(r, p, q) D_2(\text{Cxx})(r, p, q) D_1(\text{Ctt})(r, p, q) + 4 \text{Cxx}(r, p, q) \text{Ctt}(r, \\
& p, q) D_3(\text{Ctx})(r, p, q)^2 - 2 \text{Cxx}(r, p, q) D_2(\text{Ctt})(r, p, q) D_1(\text{Ctx})(r, p, q) - 2 \text{Cxx}(r, p, \\
& q)^2 D_3(\text{Ctt})(r, p, q) D_1(\text{Cty})(r, p, q) - 2 \text{Ctt}(r, p, q) D_1(\text{Cxx})(r, p, q) D_2(\text{Ctx})(r, p, q) \\
& - 2 \text{Ctt}(r, p, q)^2 D_3(\text{Cxx})(r, p, q) D_2(\text{Cxy})(r, p, q) - 2 \text{Cxx}(r, p, q) D_1(\text{Ctt})(r, p, \\
& q) D_2(\text{Ctx})(r, p, q) + 2 \text{Cxx}(r, p, q)^2 D_1(\text{Ctt})(r, p, q) D_3(\text{Cty})(r, p, q) + 4 \text{Cxy}(r, p, \\
& q)^2 D_1(\text{Ctt})(r, p, q) D_2(\text{Ctx})(r, p, q) + 2 \text{Ctx}(r, p, q) D_2(\text{Ctt})(r, p, q) D_2(\text{Ctx})(r, p, q) \\
& + 2 \text{Cxx}(r, p, q) \text{Cxy}(r, p, q) D_3(\text{Ctt})(r, p, q) D_1(\text{Ctx})(r, p, q) + 2 \text{Cxx}(r, p, q) \text{Cxy}(r, p, \\
& q) D_2(\text{Ctt})(r, p, q) D_1(\text{Cty})(r, p, q) + 4 \text{Cxx}(r, p, q) \text{Cty}(r, p, q) D_1(\text{Cxy})(r, p, \\
& q) D_1(\text{Ctx})(r, p, q) - 4 \text{Cxx}(r, p, q) \text{Cty}(r, p, q) D_3(\text{Ctx})(r, p, q) D_1(\text{Ctx})(r, p, q) \\
& + 4 \text{Cxx}(r, p, q) \text{Cty}(r, p, q) D_2(\text{Ctx})(r, p, q) D_1(\text{Cty})(r, p, q) + 4 \text{Cxx}(r, p, q) \text{Ctx}(r, p, \\
& q) D_3(\text{Ctx})(r, p, q) D_1(\text{Cty})(r, p, q) + 4 \text{Ctx}(r, p, q) \text{Cty}(r, p, q) D_1(\text{Cxx})(r, p, \\
& q) D_2(\text{Cty})(r, p, q) - 8 \text{Ctx}(r, p, q) \text{Cty}(r, p, q) D_2(\text{Cxy})(r, p, q) D_1(\text{Ctx})(r, p, q) \\
& + 4 \text{Ctt}(r, p, q) \text{Ctx}(r, p, q) D_2(\text{Cxy})(r, p, q) D_3(\text{Ctx})(r, p, q) - 4 \text{Ctt}(r, p, q) \text{Cxy}(r, p, \\
& q) D_2(\text{Ctx})(r, p, q) D_3(\text{Ctx})(r, p, q) + 4 \text{Ctt}(r, p, q) \text{Cxy}(r, p, q) D_2(\text{Ctx})(r, p, \\
& q) D_2(\text{Cty})(r, p, q) + 4 \text{Ctt}(r, p, q) \text{Cxy}(r, p, q) D_2(\text{Cxy})(r, p, q) D_1(\text{Ctx})(r, p, q) \\
& - 8 \text{Cxy}(r, p, q) \text{Ctx}(r, p, q) D_2(\text{Ctx})(r, p, q) D_1(\text{Cty})(r, p, q) + 4 \text{Cxy}(r, p, q) \text{Ctx}(r, p, \\
& q) D_2(\text{Ctt})(r, p, q) D_1(\text{Cxy})(r, p, q) + 2 \text{Cxx}(r, p, q) \text{Cty}(r, p, q) D_3(\text{Ctt})(r, p, \\
& q) D_1(\text{Cxx})(r, p, q) + 2 \text{Ctt}(r, p, q) \text{Cty}(r, p, q) D_1(\text{Cxx})(r, p, q) D_2(\text{Cxy})(r, p, q) \\
& + 2 \text{Ctt}(r, p, q) \text{Cty}(r, p, q) D_3(\text{Cxx})(r, p, q) D_2(\text{Ctx})(r, p, q) + 2 \text{Ctt}(r, p, q) \text{Cxy}(r, p, \\
& q) D_2(\text{Ctt})(r, p, q) D_3(\text{Cxx})(r, p, q) - 2 \text{Cxx}(r, p, q) \text{Ctt}(r, p, q) D_2(\text{Ctt})(r, p, \\
& q) D_3(\text{Cxy})(r, p, q) - 2 \text{Ctt}(r, p, q) \text{Cty}(r, p, q) D_2(\text{Cxx})(r, p, q) D_1(\text{Cxy})(r, p, q) \\
& - 2 \text{Ctt}(r, p, q) \text{Cty}(r, p, q) D_2(\text{Cxx})(r, p, q) D_3(\text{Ctx})(r, p, q) - 2 \text{Ctt}(r, p, q) \text{Ctx}(r, p, \\
& q) D_3(\text{Cxx})(r, p, q) D_3(\text{Ctx})(r, p, q) + 2 \text{Ctt}(r, p, q) \text{Cxy}(r, p, q) D_1(\text{Cxx})(r, p, \\
& q) D_3(\text{Ctx})(r, p, q) - 2 \text{Ctt}(r, p, q) \text{Cxy}(r, p, q) D_2(\text{Cxx})(r, p, q) D_3(\text{Ctt})(r, p, q) \\
& - 4 \text{Cxy}(r, p, q) \text{Cty}(r, p, q) D_1(\text{Cxx})(r, p, q) D_1(\text{Ctx})(r, p, q) - 2 \text{Cxx}(r, p, q) \text{Cty}(r, p, \\
& q) D_1(\text{Ctt})(r, p, q) D_2(\text{Cxy})(r, p, q) + 4 \text{Cxx}(r, p, q) \text{Ctx}(r, p, q) D_1(\text{Ctt})(r, p, \\
& q) D_3(\text{Cxy})(r, p, q) - 4 \text{Cxx}(r, p, q) \text{Ctt}(r, p, q) D_3(\text{Cxy})(r, p, q) D_1(\text{Ctx})(r, p, q) \\
& - 4 \text{Ctx}(r, p, q) \text{Cty}(r, p, q) D_2(\text{Cxx})(r, p, q) D_1(\text{Cty})(r, p, q) + 2 \text{Ctt}(r, p, q) \text{Cxy}(r, p, \\
& q) D_3(\text{Cxx})(r, p, q) D_1(\text{Ctx})(r, p, q) - 4 \text{Cxy}(r, p, q) \text{Cty}(r, p, q) D_2(\text{Ctt})(r, p, \\
& q) D_1(\text{Cxx})(r, p, q) + 4 \text{Cxy}(r, p, q) \text{Cty}(r, p, q) D_2(\text{Cxx})(r, p, q) D_1(\text{Ctt})(r, p, q) \\
& - 2 \text{Cxx}(r, p, q) \text{Cty}(r, p, q) D_3(\text{Cxx})(r, p, q) D_1(\text{Ctt})(r, p, q) + 2 \text{Cxx}(r, p, q) \text{Cty}(r, p, \\
& q) D_2(\text{Ctt})(r, p, q) D_1(\text{Cxy})(r, p, q) + 2 \text{Cxx}(r, p, q) \text{Cty}(r, p, q) D_2(\text{Ctt})(r, p, \\
& q) D_3(\text{Ctx})(r, p, q) - 4 \text{Cxx}(r, p, q) \text{Ctx}(r, p, q) D_3(\text{Ctt})(r, p, q) D_1(\text{Cxy})(r, p, q) \\
& - 2 \text{Cxx}(r, p, q) \text{Ctx}(r, p, q) D_3(\text{Ctt})(r, p, q) D_3(\text{Ctx})(r, p, q) - 2 \text{Cxx}(r, p, q) \text{Ctt}(r, p,
\end{aligned}$$



$$\begin{aligned}
& q) D_1(Cxx)(r, p, q) D_3(Cty)(r, p, q) + 2 Cxx(r, p, q) Ctt(r, p, q) D_3(Ctt)(r, p, \\
& q) D_2(Cxy)(r, p, q) + 2 Cxx(r, p, q) Ctt(r, p, q) D_3(Cxx)(r, p, q) D_1(Cty)(r, p, q) \\
& - 2 Cxx(r, p, q) Cxy(r, p, q) D_1(Ctt)(r, p, q) D_3(Ctx)(r, p, q) - 2 Cxx(r, p, q) Cxy(r, p, \\
& q) D_1(Ctt)(r, p, q) D_2(Cty)(r, p, q) - 4 Ctt(r, p, q) Ctx(r, p, q) D_3(Cxx)(r, p, \\
& q) D_2(Cty)(r, p, q) + 4 Ctt(r, p, q) Ctx(r, p, q) D_2(Cxx)(r, p, q) D_3(Cty)(r, p, q) \\
& + 2 Ctt(r, p, q) Cxy(r, p, q) D_1(Cxx)(r, p, q) D_2(Cty)(r, p, q) - 2 Ctt(r, p, q) Cxy(r, p, \\
& q) D_2(Cxx)(r, p, q) D_1(Cty)(r, p, q) - 4 Cxy(r, p, q) Cty(r, p, q) D_2(Ctt)(r, p, \\
& q) D_2(Ctx)(r, p, q) - 4 Cxy(r, p, q) Ctx(r, p, q) D_1(Ctt)(r, p, q) D_2(Cxy)(r, p, q) \\
& + 2 Cxx(r, p, q) Cty(r, p, q) D_3(Ctt)(r, p, q) D_2(Ctx)(r, p, q) - 4 Cxx(r, p, q) Ctt(r, p, \\
& q) D_2(Ctx)(r, p, q) D_3(Cty)(r, p, q) ), \\
D_{1,3}(Ctx)(r, p, q) = & -\frac{1}{4} \frac{1}{HessUniv} \left( -2 Cxx(r, p, q) D_3(Ctt)(r, p, q) D_1(Ctx)(r, p, q) \right. \\
& + 2 Cxx(r, p, q) D_2(Ctt)(r, p, q) D_1(Cty)(r, p, q) + 4 Ctx(r, p, q) D_2(Ctt)(r, p, \\
& q) D_1(Cxy)(r, p, q) - 2 Cxy(r, p, q) D_2(Ctt)(r, p, q) D_1(Ctx)(r, p, q) + 4 Cty(r, p, \\
& q)^2 D_3(Cxx)(r, p, q) D_1(Ctx)(r, p, q) - 8 Ctx(r, p, q)^2 D_3(Cty)(r, p, q) D_1(Cxy)(r, p, q) \\
& + 4 Ctt(r, p, q) Cxy(r, p, q) D_3(Ctx)(r, p, q)^2 + 4 Cxy(r, p, q)^2 D_3(Ctt)(r, p, \\
& q) D_1(Ctx)(r, p, q) + 4 Cty(r, p, q) D_2(Ctx)(r, p, q) D_1(Ctx)(r, p, q) + 4 Ctx(r, p, \\
& q) D_3(Ctx)(r, p, q) D_1(Ctx)(r, p, q) - 4 Ctx(r, p, q) D_2(Ctx)(r, p, q) D_1(Cty)(r, p, q) \\
& - 4 Ctt(r, p, q) D_2(Ctx)(r, p, q) D_1(Cxy)(r, p, q) - 4 Ctt(r, p, q) D_2(Ctx)(r, p, \\
& q) D_3(Ctx)(r, p, q) + 4 Ctt(r, p, q) D_2(Ctx)(r, p, q) D_2(Cty)(r, p, q) - 2 Cty(r, p, \\
& q) D_1(Cxx)(r, p, q) D_1(Ctx)(r, p, q) - 2 Cty(r, p, q) D_2(Ctt)(r, p, q) D_2(Ctx)(r, p, q) \\
& + 2 Ctx(r, p, q) D_3(Ctt)(r, p, q) D_2(Ctx)(r, p, q) - 2 Cxx(r, p, q) D_1(Ctt)(r, p, \\
& q) D_3(Ctx)(r, p, q) - 2 Cxx(r, p, q) D_1(Ctt)(r, p, q) D_2(Cty)(r, p, q) - 4 Ctx(r, p, \\
& q) D_1(Ctt)(r, p, q) D_2(Cxy)(r, p, q) + 2 Ctx(r, p, q) D_2(Ctt)(r, p, q) D_3(Ctx)(r, p, q) \\
& + 2 Cxy(r, p, q) D_1(Ctt)(r, p, q) D_2(Ctx)(r, p, q) + 8 Ctx(r, p, q)^2 D_3(Cxy)(r, p, \\
& q) D_1(Cty)(r, p, q) + 4 Ctx(r, p, q) D_1(Cxy)(r, p, q) D_1(Ctx)(r, p, q) + Ctt(r, p, \\
& q) D_2(Ctt)(r, p, q) D_3(Cxx)(r, p, q) - Ctt(r, p, q) D_2(Cxx)(r, p, q) D_3(Ctt)(r, p, q) \\
& - 2 Cty(r, p, q) D_2(Ctt)(r, p, q) D_1(Cxx)(r, p, q) + 2 Cty(r, p, q) D_2(Cxx)(r, p, \\
& q) D_1(Ctt)(r, p, q) + Ctx(r, p, q) D_3(Ctt)(r, p, q) D_1(Cxx)(r, p, q) - Ctx(r, p, \\
& q) D_3(Cxx)(r, p, q) D_1(Ctt)(r, p, q) + 2 Ctt(r, p, q) D_1(Cxx)(r, p, q) D_2(Cty)(r, p, q) \\
& - 2 Ctt(r, p, q) D_2(Cxx)(r, p, q) D_1(Cty)(r, p, q) - 8 Ctx(r, p, q) Cty(r, p, q) D_3(Cxy)(r, \\
& p, q) D_1(Ctx)(r, p, q) + 2 Ctt(r, p, q) Cty(r, p, q) D_1(Cxx)(r, p, q) D_3(Cxy)(r, p, q) \\
& + 4 Ctx(r, p, q) Cty(r, p, q) D_1(Cxx)(r, p, q) D_3(Cty)(r, p, q) - 4 Ctx(r, p, q) Cty(r, p, \\
& q) D_3(Cxx)(r, p, q) D_1(Cty)(r, p, q) + 2 Cxx(r, p, q) Cty(r, p, q) D_3(Ctt)(r, p, \\
& q) D_1(Cxy)(r, p, q) - 2 Ctt(r, p, q) Cty(r, p, q) D_3(Cxx)(r, p, q) D_1(Cxy)(r, p, q) \\
& - 2 Ctt(r, p, q) Cty(r, p, q) D_3(Cxx)(r, p, q) D_3(Ctx)(r, p, q) - 2 Cxx(r, p, q) Cxy(r, p, \\
& q) D_3(Ctt)(r, p, q) D_1(Cty)(r, p, q) - 2 Ctt(r, p, q) Cxy(r, p, q) D_1(Cxx)(r, p,
\end{aligned}$$

$$\begin{aligned}
& q) D_3(Cty)(r, p, q) + 2 Ctt(r, p, q) Cxy(r, p, q) D_3(Cxx)(r, p, q) D_1(Cty)(r, p, q) \\
& + 4 Ctt(r, p, q) Cty(r, p, q) D_2(Ctx)(r, p, q) D_3(Cxy)(r, p, q) - 8 Cxy(r, p, q) Cty(r, p, \\
& q) D_3(Ctx)(r, p, q) D_1(Ctx)(r, p, q) - 4 Cxy(r, p, q) Ctx(r, p, q) D_3(Ctt)(r, p, \\
& q) D_3(Ctx)(r, p, q) + 4 Cxx(r, p, q) Cty(r, p, q) D_3(Ctx)(r, p, q) D_1(Cty)(r, p, q) \\
& - 2 Cxx(r, p, q) Cty(r, p, q) D_1(Ctt)(r, p, q) D_3(Cxy)(r, p, q) + 2 Cxx(r, p, q) Cty(r, p, \\
& q) D_3(Ctt)(r, p, q) D_3(Ctx)(r, p, q) + 2 Cxx(r, p, q) Cxy(r, p, q) D_1(Ctt)(r, p, \\
& q) D_3(Cty)(r, p, q) + 8 Ctt(r, p, q) Ctx(r, p, q) D_2(Cxy)(r, p, q) D_3(Cty)(r, p, q) \\
& - 4 Ctt(r, p, q) Cxy(r, p, q) D_2(Ctx)(r, p, q) D_3(Cty)(r, p, q) - 8 Ctt(r, p, q) Ctx(r, p, \\
& q) D_2(Cty)(r, p, q) D_3(Cxy)(r, p, q) + 4 Ctt(r, p, q) Cxy(r, p, q) D_3(Ctx)(r, p, \\
& q) D_1(Cxy)(r, p, q) + 4 Cxy(r, p, q) Ctx(r, p, q) D_1(Ctt)(r, p, q) D_3(Cxy)(r, p, q) \\
& - 4 Cxy(r, p, q) Ctx(r, p, q) D_3(Ctt)(r, p, q) D_1(Cxy)(r, p, q) \Big),
\end{aligned}$$

$$\begin{aligned}
D_{2,2}(Ctx)(r, p, q) = & \frac{1}{4} \frac{1}{HessUniv} \Big( 4 Cxx(r, p, q) Ctt(r, p, q) D_2(Ctx)(r, p, q) D_3(Cxy)(r, p, \\
& q) + 4 Cxx(r, p, q) Cxy(r, p, q) D_1(Ctt)(r, p, q) D_2(Cxy)(r, p, q) - 4 Cxx(r, p, q) Cxy(r, \\
& p, q) D_1(Cxy)(r, p, q) D_1(Ctx)(r, p, q) + 4 Cxx(r, p, q) Cxy(r, p, q) D_3(Ctx)(r, p, \\
& q) D_1(Ctx)(r, p, q) - 4 Cxx(r, p, q) Cxy(r, p, q) D_3(Ctt)(r, p, q) D_2(Ctx)(r, p, q) \\
& + 4 Cxx(r, p, q) Cxy(r, p, q) D_2(Cty)(r, p, q) D_1(Ctx)(r, p, q) - 4 Cxx(r, p, q) Cxy(r, p, \\
& q) D_2(Ctt)(r, p, q) D_1(Cxy)(r, p, q) + 2 Cxx(r, p, q) Cty(r, p, q) D_2(Ctt)(r, p, \\
& q) D_3(Cxx)(r, p, q) - 2 Cxx(r, p, q) Cty(r, p, q) D_2(Cxx)(r, p, q) D_3(Ctt)(r, p, q) \\
& + 2 Cxx(r, p, q) Ctt(r, p, q) D_1(Cxx)(r, p, q) D_3(Cxy)(r, p, q) - 2 Cxx(r, p, q) Ctt(r, p, \\
& q) D_3(Cxx)(r, p, q) D_1(Cxy)(r, p, q) - 2 Cxx(r, p, q) Ctt(r, p, q) D_3(Cxx)(r, p, \\
& q) D_3(Ctx)(r, p, q) - 2 Cxx(r, p, q) Ctt(r, p, q) D_3(Cxx)(r, p, q) D_2(Cty)(r, p, q) \\
& + 2 Cxx(r, p, q) Ctt(r, p, q) D_2(Cxx)(r, p, q) D_3(Cty)(r, p, q) - 2 Cxx(r, p, q) Cxy(r, p, \\
& q) D_3(Ctt)(r, p, q) D_1(Cxx)(r, p, q) + 2 Cxx(r, p, q) Cxy(r, p, q) D_3(Cxx)(r, p, \\
& q) D_1(Ctt)(r, p, q) - 4 Ctx(r, p, q) Cty(r, p, q) D_3(Cxx)(r, p, q) D_2(Ctx)(r, p, q) \\
& + 8 Ctx(r, p, q) Cty(r, p, q) D_2(Cxy)(r, p, q) D_2(Ctx)(r, p, q) + 4 Ctx(r, p, q) Cty(r, p, \\
& q) D_2(Cxx)(r, p, q) D_3(Ctx)(r, p, q) + 4 Ctt(r, p, q) Ctx(r, p, q) D_3(Cxx)(r, p, \\
& q) D_2(Cxy)(r, p, q) - 4 Ctt(r, p, q) Ctx(r, p, q) D_2(Cxx)(r, p, q) D_3(Cxy)(r, p, q) \\
& - 4 Ctt(r, p, q) Cxy(r, p, q) D_1(Cxx)(r, p, q) D_2(Cxy)(r, p, q) - 8 Ctt(r, p, q) Cxy(r, p, \\
& q) D_2(Cxy)(r, p, q) D_2(Ctx)(r, p, q) + 4 Ctt(r, p, q) Cxy(r, p, q) D_2(Cxx)(r, p, \\
& q) D_1(Cxy)(r, p, q) + 4 Cxy(r, p, q) Cty(r, p, q) D_1(Cxx)(r, p, q) D_2(Ctx)(r, p, q) \\
& - 4 Cxy(r, p, q) Cty(r, p, q) D_2(Cxx)(r, p, q) D_1(Ctx)(r, p, q) - 4 Cxy(r, p, q) Ctx(r, p, \\
& q) D_1(Cxx)(r, p, q) D_3(Ctx)(r, p, q) - 8 Cxy(r, p, q) Ctx(r, p, q) D_1(Cxx)(r, p, \\
& q) D_2(Cty)(r, p, q) - 4 Cxy(r, p, q) Ctx(r, p, q) D_3(Cxx)(r, p, q) D_1(Ctx)(r, p, q) \\
& + 8 Cxy(r, p, q) Ctx(r, p, q) D_2(Ctx)(r, p, q) D_3(Ctx)(r, p, q) - 4 Cxy(r, p, q) Ctx(r, p, \\
& q) D_2(Ctt)(r, p, q) D_3(Cxx)(r, p, q) + 8 Cxy(r, p, q) Ctx(r, p, q) D_2(Cxy)(r, p,
\end{aligned}$$

$$\begin{aligned}
& q) D_1(Ctx)(r, p, q) + 8 Cxy(r, p, q) Ctx(r, p, q) D_2(Cxx)(r, p, q) D_1(Cty)(r, p, q) \\
& + 4 Cxy(r, p, q) Ctx(r, p, q) D_2(Cxx)(r, p, q) D_3(Ctt)(r, p, q) + 4 Cxx(r, p, q) Cty(r, p, \\
& q) D_3(Cxx)(r, p, q) D_1(Ctx)(r, p, q) - 4 Cxx(r, p, q) Cty(r, p, q) D_2(Ctx)(r, p, \\
& q) D_1(Cxy)(r, p, q) - 4 Cxx(r, p, q) Cty(r, p, q) D_2(Ctx)(r, p, q) D_3(Ctx)(r, p, q) \\
& - 4 Cxx(r, p, q) Cty(r, p, q) D_2(Ctx)(r, p, q) D_2(Cty)(r, p, q) + 4 Cxx(r, p, q) Ctx(r, p, \\
& q) D_1(Cxx)(r, p, q) D_3(Cty)(r, p, q) + 4 Cxx(r, p, q) Ctx(r, p, q) D_3(Ctx)(r, p, \\
& q) D_1(Cxy)(r, p, q) - 4 Cxx(r, p, q) Ctx(r, p, q) D_3(Cxx)(r, p, q) D_1(Cty)(r, p, q) \\
& + 8 Cxx(r, p, q) Ctx(r, p, q) D_2(Cty)(r, p, q) D_1(Cxy)(r, p, q) - 4 Cxx(r, p, q) Ctx(r, p, \\
& q) D_2(Cty)(r, p, q) D_3(Ctx)(r, p, q) + 8 Cxx(r, p, q) Ctx(r, p, q) D_2(Ctx)(r, p, \\
& q) D_3(Cty)(r, p, q) - 8 Cxx(r, p, q) Ctx(r, p, q) D_2(Cxy)(r, p, q) D_1(Cty)(r, p, q) \\
& + 2 Cxx(r, p, q) D_2(Ctt)(r, p, q) D_2(Ctx)(r, p, q) - 2 Cxx(r, p, q)^2 D_1(Ctt)(r, p, \\
& q) D_3(Cxy)(r, p, q) + 2 Cxx(r, p, q)^2 D_3(Ctt)(r, p, q) D_1(Cxy)(r, p, q) + 2 Cxx(r, p, \\
& q)^2 D_3(Ctt)(r, p, q) D_3(Ctx)(r, p, q) + 2 Cxx(r, p, q)^2 D_3(Ctt)(r, p, q) D_2(Cty)(r, p, q) \\
& - 2 Cxx(r, p, q)^2 D_2(Ctt)(r, p, q) D_3(Cty)(r, p, q) - 4 Cty(r, p, q)^2 D_2(Cxx)(r, p, \\
& q) D_2(Ctx)(r, p, q) + 4 Ctx(r, p, q)^2 D_3(Cxx)(r, p, q) D_3(Ctx)(r, p, q) + 8 Ctx(r, p, \\
& q)^2 D_3(Cxx)(r, p, q) D_2(Cty)(r, p, q) - 8 Ctx(r, p, q)^2 D_2(Cxy)(r, p, q) D_3(Ctx)(r, p, q) \\
& - 8 Ctx(r, p, q)^2 D_2(Cxx)(r, p, q) D_3(Cty)(r, p, q) + 8 Cxy(r, p, q) Cty(r, p, \\
& q) D_2(Ctx)(r, p, q)^2 + 4 Cxy(r, p, q)^2 D_1(Cxx)(r, p, q) D_1(Ctx)(r, p, q) - 8 Cxy(r, p, \\
& q)^2 D_2(Ctx)(r, p, q) D_1(Ctx)(r, p, q) + 4 Cxy(r, p, q)^2 D_2(Ctt)(r, p, q) D_1(Cxx)(r, p, q) \\
& - 4 Cxy(r, p, q)^2 D_2(Cxx)(r, p, q) D_1(Ctt)(r, p, q) + 4 Ctt(r, p, q) D_2(Cxx)(r, p, \\
& q) D_2(Ctx)(r, p, q) - 4 Cxx(r, p, q) Ctx(r, p, q) D_3(Ctx)(r, p, q)^2 + 4 Cxx(r, p, \\
& q) D_2(Ctx)(r, p, q) D_1(Ctx)(r, p, q) - Cxx(r, p, q) D_2(Ctt)(r, p, q) D_1(Cxx)(r, p, q) \\
& + Cxx(r, p, q) D_2(Cxx)(r, p, q) D_1(Ctt)(r, p, q) - 4 Cxx(r, p, q)^2 D_3(Cty)(r, p, \\
& q) D_1(Ctx)(r, p, q) - 2 Cxx(r, p, q) D_1(Cxx)(r, p, q) D_1(Ctx)(r, p, q) - 8 Ctx(r, p, \\
& q) D_2(Ctx)(r, p, q)^2), \\
D_{2,3}(Ctx)(r, p, q) = & -\frac{1}{4} \frac{1}{HessUniv} \left( -4 Ctx(r, p, q) Cty(r, p, q) D_3(Cxx)(r, p, q) D_2(Cty)(r, \right. \\
& p, q) + 4 Ctx(r, p, q) Cty(r, p, q) D_2(Cxx)(r, p, q) D_3(Cty)(r, p, q) - 8 Cxy(r, p, q) Ctx(r, \\
& p, q) D_2(Ctx)(r, p, q) D_3(Cty)(r, p, q) + 4 Cxx(r, p, q) Cty(r, p, q) D_2(Cty)(r, p, \\
& q) D_3(Ctx)(r, p, q) - 8 Cxx(r, p, q) Ctx(r, p, q) D_3(Cty)(r, p, q) D_1(Cxy)(r, p, q) \\
& + 2 Cxx(r, p, q) Cxy(r, p, q) D_2(Ctt)(r, p, q) D_3(Cty)(r, p, q) - 4 Cxx(r, p, q) Cty(r, p, \\
& q) D_3(Cxy)(r, p, q) D_1(Ctx)(r, p, q) + 8 Cxx(r, p, q) Ctx(r, p, q) D_3(Cxy)(r, p, \\
& q) D_1(Cty)(r, p, q) + 4 Cxx(r, p, q) Cxy(r, p, q) D_3(Cty)(r, p, q) D_1(Ctx)(r, p, q) \\
& \left. - 2 Ctt(r, p, q) Cty(r, p, q) D_3(Cxx)(r, p, q) D_2(Cxy)(r, p, q) + 2 Ctt(r, p, q) Cty(r, p, \right.
\end{aligned}$$

$$\begin{aligned}
& q) D_2(Cxx)(r, p, q) D_3(Cxy)(r, p, q) + 2 Ctt(r, p, q) Cxy(r, p, q) D_3(Cxx)(r, p, \\
& q) D_3(Ctx)(r, p, q) + 2 Ctt(r, p, q) Cxy(r, p, q) D_3(Cxx)(r, p, q) D_2(Cty)(r, p, q) \\
& - 2 Ctt(r, p, q) Cxy(r, p, q) D_2(Cxx)(r, p, q) D_3(Cty)(r, p, q) + 2 Cxx(r, p, q) Cty(r, p, \\
& q) D_3(Ctt)(r, p, q) D_2(Cxy)(r, p, q) - 2 Cxx(r, p, q) Cty(r, p, q) D_2(Ctt)(r, p, \\
& q) D_3(Cxy)(r, p, q) - 2 Cxx(r, p, q) Cxy(r, p, q) D_3(Ctt)(r, p, q) D_3(Ctx)(r, p, q) \\
& - 2 Cxx(r, p, q) Cxy(r, p, q) D_3(Ctt)(r, p, q) D_2(Cty)(r, p, q) - 4 Ctx(r, p, q) Cty(r, p, \\
& q) D_3(Cxx)(r, p, q) D_3(Ctx)(r, p, q) + 4 Ctt(r, p, q) Cxy(r, p, q) D_2(Cxy)(r, p, \\
& q) D_3(Ctx)(r, p, q) - 8 Cxy(r, p, q) Cty(r, p, q) D_2(Ctx)(r, p, q) D_3(Ctx)(r, p, q) \\
& - 4 Cxy(r, p, q) Ctx(r, p, q) D_3(Ctt)(r, p, q) D_2(Cxy)(r, p, q) + 4 Cxy(r, p, q) Ctx(r, p, \\
& q) D_2(Ctt)(r, p, q) D_3(Cxy)(r, p, q) + 4 Cty(r, p, q)^2 D_3(Cxx)(r, p, q) D_2(Ctx)(r, p, q) \\
& - 8 Ctx(r, p, q)^2 D_2(Cty)(r, p, q) D_3(Cxy)(r, p, q) + 4 Cxy(r, p, q)^2 D_3(Ctt)(r, p, \\
& q) D_2(Ctx)(r, p, q) + 4 Ctx(r, p, q) D_1(Cxx)(r, p, q) D_2(Cty)(r, p, q) + 4 Ctx(r, p, \\
& q) D_2(Ctx)(r, p, q) D_3(Ctx)(r, p, q) - 4 Ctx(r, p, q) D_2(Cxy)(r, p, q) D_1(Ctx)(r, p, q) \\
& - 4 Ctx(r, p, q) D_2(Cxx)(r, p, q) D_1(Cty)(r, p, q) + 4 Cxy(r, p, q) D_2(Ctx)(r, p, \\
& q) D_1(Ctx)(r, p, q) + 4 Cxx(r, p, q) Cty(r, p, q) D_3(Ctx)(r, p, q)^2 + 4 Cxx(r, p, \\
& q) D_1(Cxy)(r, p, q) D_1(Ctx)(r, p, q) - 4 Cxx(r, p, q) D_3(Ctx)(r, p, q) D_1(Ctx)(r, p, q) \\
& - 4 Cxx(r, p, q) D_2(Cty)(r, p, q) D_1(Ctx)(r, p, q) - 2 Cty(r, p, q) D_1(Cxx)(r, p, \\
& q) D_2(Ctx)(r, p, q) + 2 Cty(r, p, q) D_2(Cxx)(r, p, q) D_1(Ctx)(r, p, q) + 2 Ctx(r, p, \\
& q) D_1(Cxx)(r, p, q) D_3(Ctx)(r, p, q) + 2 Ctx(r, p, q) D_3(Cxx)(r, p, q) D_1(Ctx)(r, p, q) \\
& + 2 Ctt(r, p, q) D_1(Cxx)(r, p, q) D_2(Cxy)(r, p, q) - 2 Ctt(r, p, q) D_3(Cxx)(r, p, \\
& q) D_2(Ctx)(r, p, q) - 2 Ctt(r, p, q) D_2(Cxx)(r, p, q) D_1(Cxy)(r, p, q) - 2 Ctt(r, p, \\
& q) D_2(Cxx)(r, p, q) D_3(Ctx)(r, p, q) - 2 Cxy(r, p, q) D_1(Cxx)(r, p, q) D_1(Ctx)(r, p, q) \\
& - 2 Cxy(r, p, q) D_2(Ctt)(r, p, q) D_2(Ctx)(r, p, q) + 4 Ctx(r, p, q) D_2(Ctx)(r, p, \\
& q) D_2(Cty)(r, p, q) + Cxx(r, p, q) D_3(Ctt)(r, p, q) D_1(Cxx)(r, p, q) - Cxx(r, p, \\
& q) D_3(Cxx)(r, p, q) D_1(Ctt)(r, p, q) + Ctx(r, p, q) D_2(Ctt)(r, p, q) D_3(Cxx)(r, p, q) \\
& - Ctx(r, p, q) D_2(Cxx)(r, p, q) D_3(Ctt)(r, p, q) - 2 Cxy(r, p, q) D_2(Ctt)(r, p, \\
& q) D_1(Cxx)(r, p, q) + 2 Cxy(r, p, q) D_2(Cxx)(r, p, q) D_1(Ctt)(r, p, q) - 2 Cxx(r, p, \\
& q) D_1(Ctt)(r, p, q) D_2(Cxy)(r, p, q) + 2 Cxx(r, p, q) D_2(Ctt)(r, p, q) D_1(Cxy)(r, p, q) \\
& + 8 Ctx(r, p, q)^2 D_2(Cxy)(r, p, q) D_3(Cty)(r, p, q) \Big), \\
D_{3,3}(Ctx)(r, p, q) = & -\frac{1}{4} \frac{1}{HessUniv} \Big( -4 Ctt(r, p, q) D_2(Ctx)(r, p, q) D_3(Cxy)(r, p, q) \\
& + 4 Cxy(r, p, q) D_1(Cxy)(r, p, q) D_1(Ctx)(r, p, q) - 4 Cxy(r, p, q) D_3(Ctx)(r, p, \\
& q) D_1(Ctx)(r, p, q) - 4 Cxy(r, p, q) D_2(Cty)(r, p, q) D_1(Ctx)(r, p, q) - 4 Cxx(r, p, \\
& q) D_3(Cty)(r, p, q) D_1(Ctx)(r, p, q) - 2 Cxx(r, p, q) D_3(Ctt)(r, p, q) D_3(Ctx)(r, p, q)
\end{aligned}$$

$$\begin{aligned}
& -2 Cxx(r, p, q) D_3(Ctt)(r, p, q) D_2(Cty)(r, p, q) + 2 Cxx(r, p, q) D_2(Ctt)(r, p, \\
& q) D_3(Cty)(r, p, q) + 8 Cty(r, p, q)^2 D_2(Ctx)(r, p, q) D_3(Cxy)(r, p, q) + 8 Cxy(r, p, \\
& q)^2 D_3(Cty)(r, p, q) D_1(Ctx)(r, p, q) - 4 Cty(r, p, q) D_2(Ctx)(r, p, q) D_1(Cxy)(r, p, q) \\
& - 4 Cty(r, p, q) D_2(Ctx)(r, p, q) D_3(Ctx)(r, p, q) + 4 Cty(r, p, q) D_2(Ctx)(r, p, \\
& q) D_2(Cty)(r, p, q) + 8 Ctx(r, p, q) D_2(Cty)(r, p, q) D_1(Cxy)(r, p, q) + 2 Ctt(r, p, \\
& q) D_1(Cxx)(r, p, q) D_3(Cxy)(r, p, q) - 2 Ctt(r, p, q) D_3(Cxx)(r, p, q) D_1(Cxy)(r, p, q) \\
& - 2 Ctt(r, p, q) D_3(Cxx)(r, p, q) D_3(Ctx)(r, p, q) + 8 Cxx(r, p, q) Cty(r, p, q) D_3(Ctx)(r, \\
& p, q) D_3(Cty)(r, p, q) - 16 Ctx(r, p, q) Cty(r, p, q) D_2(Cty)(r, p, q) D_3(Cxy)(r, p, q) \\
& + 16 Ctx(r, p, q) Cty(r, p, q) D_2(Cxy)(r, p, q) D_3(Cty)(r, p, q) - 8 Cxy(r, p, q) Cty(r, p, \\
& q) D_2(Ctx)(r, p, q) D_3(Cty)(r, p, q) + 4 Cty(r, p, q) D_3(Cxx)(r, p, q) D_1(Ctx)(r, p, q) \\
& + 4 Ctx(r, p, q) D_3(Ctx)(r, p, q) D_1(Cxy)(r, p, q) + 4 Ctx(r, p, q) D_1(Cxx)(r, p, \\
& q) D_3(Cty)(r, p, q) - 4 Ctx(r, p, q) D_3(Ctt)(r, p, q) D_2(Cxy)(r, p, q) - 4 Ctx(r, p, \\
& q) D_3(Cxx)(r, p, q) D_1(Cty)(r, p, q) + 4 Ctx(r, p, q) D_2(Ctt)(r, p, q) D_3(Cxy)(r, p, q) \\
& + 2 Ctt(r, p, q) D_3(Cxx)(r, p, q) D_2(Cty)(r, p, q) - 2 Ctt(r, p, q) D_2(Cxx)(r, p, \\
& q) D_3(Cty)(r, p, q) + 4 Cxy(r, p, q) D_3(Ctt)(r, p, q) D_2(Ctx)(r, p, q) - 2 Cxx(r, p, \\
& q) D_1(Ctt)(r, p, q) D_3(Cxy)(r, p, q) + 2 Cxx(r, p, q) D_3(Ctt)(r, p, q) D_1(Cxy)(r, p, q) \\
& + 4 Ctx(r, p, q) D_2(Cty)(r, p, q) D_3(Ctx)(r, p, q) - 8 Ctx(r, p, q) D_2(Cxy)(r, p, \\
& q) D_1(Cty)(r, p, q) + 8 Ctt(r, p, q) Cxy(r, p, q) D_3(Cxy)(r, p, q) D_3(Ctx)(r, p, q) \\
& - 8 Cxy(r, p, q) Cty(r, p, q) D_3(Cxy)(r, p, q) D_1(Ctx)(r, p, q) - 16 Cxy(r, p, q) Ctx(r, p, \\
& q) D_3(Cty)(r, p, q) D_1(Cxy)(r, p, q) + 16 Cxy(r, p, q) Ctx(r, p, q) D_3(Cxy)(r, p, \\
& q) D_1(Cty)(r, p, q) + 4 Ctx(r, p, q) D_3(Ctx)(r, p, q)^2 + 4 D_2(Ctx)(r, p, q) D_1(Ctx)(r, p, q) \\
& - 2 D_1(Cxx)(r, p, q) D_1(Ctx)(r, p, q) - 2 D_2(Ctt)(r, p, q) D_2(Ctx)(r, p, q) - D_2(Ctt)(r, \\
& p, q) D_1(Cxx)(r, p, q) + D_2(Cxx)(r, p, q) D_1(Ctt)(r, p, q) - 8 Ctx(r, p, q) Cty(r, p, \\
& q) D_3(Cxy)(r, p, q) D_3(Ctx)(r, p, q) - 8 Cxy(r, p, q) Ctx(r, p, q) D_3(Ctx)(r, p, \\
& q) D_3(Cty)(r, p, q) ),
\end{aligned}$$

$$\begin{aligned}
D_{1,1}(Cty)(r, p, q) &= \frac{1}{4} \frac{1}{HessUniv} \left( -Ctt(r, p, q) D_3(Cxx)(r, p, q) D_1(Ctt)(r, p, q) - 8 Cxx(r, \right. \\
& p, q) Cty(r, p, q) D_1(Cty)(r, p, q)^2 + 4 Cxx(r, p, q) D_1(Ctt)(r, p, q) D_1(Cty)(r, p, q) \\
& - 8 Cty(r, p, q)^2 D_2(Cty)(r, p, q) D_1(Ctx)(r, p, q) + 4 Cty(r, p, q)^2 D_2(Ctt)(r, p, \\
& q) D_2(Cty)(r, p, q) - 8 Ctx(r, p, q)^2 D_3(Cty)(r, p, q) D_1(Cty)(r, p, q) + 4 Ctx(r, p, \\
& q)^2 D_3(Ctt)(r, p, q) D_3(Cty)(r, p, q) - 4 Ctt(r, p, q) Cty(r, p, q) D_2(Cty)(r, p, q)^2 \\
& + 8 Cxy(r, p, q) Ctx(r, p, q) D_1(Cty)(r, p, q)^2 - 4 Cxy(r, p, q)^2 D_1(Ctt)(r, p, \\
& q) D_1(Cty)(r, p, q) - 8 Ctx(r, p, q) D_1(Ctx)(r, p, q) D_1(Cty)(r, p, q) + 4 Ctx(r, p, \\
& q) D_1(Ctt)(r, p, q) D_3(Ctx)(r, p, q) + Ctt(r, p, q) D_3(Ctt)(r, p, q) D_1(Cxx)(r, p, q) \\
& \left. + 2 Ctt(r, p, q) D_1(Cxx)(r, p, q) D_1(Cty)(r, p, q) - 2 Ctt(r, p, q) D_2(Ctt)(r, p, \right.
\end{aligned}$$

$$\begin{aligned}
& q) D_1(Cxy)(r, p, q) - 2 Ctt(r, p, q) D_2(Ctt)(r, p, q) D_3(Ctx)(r, p, q) + 2 Ctt(r, p, \\
& q)^2 D_3(Cxx)(r, p, q) D_3(Cty)(r, p, q) + 4 Ctt(r, p, q) Ctx(r, p, q) D_3(Cty)(r, p, \\
& q) D_1(Cxy)(r, p, q) - 4 Ctt(r, p, q) Cxy(r, p, q) D_3(Ctx)(r, p, q) D_1(Cty)(r, p, q) \\
& - 4 Cxy(r, p, q) Ctx(r, p, q) D_1(Ctt)(r, p, q) D_3(Cty)(r, p, q) + 4 Cxy(r, p, q) Ctx(r, p, \\
& q) D_3(Ctt)(r, p, q) D_1(Cty)(r, p, q) - 4 Ctt(r, p, q) Cty(r, p, q) D_1(Cxx)(r, p, \\
& q) D_3(Cty)(r, p, q) + 4 Ctt(r, p, q) Cxy(r, p, q) D_2(Ctt)(r, p, q) D_3(Cty)(r, p, q) \\
& + 4 Cty(r, p, q) D_2(Ctt)(r, p, q) D_1(Ctx)(r, p, q) - 4 Ctx(r, p, q) D_3(Ctt)(r, p, \\
& q) D_1(Ctx)(r, p, q) + 2 Ctt(r, p, q) D_1(Ctt)(r, p, q) D_2(Cxy)(r, p, q) + 2 Ctt(r, p, \\
& q) D_3(Ctt)(r, p, q) D_2(Ctx)(r, p, q) - 2 Ctt(r, p, q) D_2(Ctt)(r, p, q) D_2(Cty)(r, p, q) \\
& - 4 Ctt(r, p, q)^2 D_2(Cxy)(r, p, q) D_3(Cty)(r, p, q) - 4 Cty(r, p, q) D_1(Ctt)(r, p, \\
& q) D_2(Ctx)(r, p, q) + 4 Ctt(r, p, q) D_2(Ctx)(r, p, q) D_1(Cty)(r, p, q) + 8 Ctx(r, p, \\
& q) Cty(r, p, q) D_3(Cty)(r, p, q) D_1(Ctx)(r, p, q) - 4 Ctx(r, p, q) Cty(r, p, q) D_3(Ctt)(r, p, \\
& q) D_2(Cty)(r, p, q) + 8 Ctx(r, p, q) Cty(r, p, q) D_2(Cty)(r, p, q) D_1(Cty)(r, p, q) \\
& - 4 Ctx(r, p, q) Cty(r, p, q) D_2(Ctt)(r, p, q) D_3(Cty)(r, p, q) + 4 Ctt(r, p, q) Cty(r, p, \\
& q) D_2(Cty)(r, p, q) D_1(Cxy)(r, p, q) + 4 Ctt(r, p, q) Cty(r, p, q) D_2(Cty)(r, p, \\
& q) D_3(Ctx)(r, p, q) - 4 Ctt(r, p, q) Ctx(r, p, q) D_3(Ctx)(r, p, q) D_3(Cty)(r, p, q) \\
& + 4 Ctt(r, p, q) Ctx(r, p, q) D_2(Cty)(r, p, q) D_3(Cty)(r, p, q) - 4 Ctt(r, p, q) Cxy(r, p, \\
& q) D_1(Cxy)(r, p, q) D_1(Cty)(r, p, q) - 4 Ctt(r, p, q) Cxy(r, p, q) D_2(Cty)(r, p, \\
& q) D_1(Cty)(r, p, q) + 8 Cxy(r, p, q) Cty(r, p, q) D_1(Ctx)(r, p, q) D_1(Cty)(r, p, q) \\
& + 4 Cxy(r, p, q) Cty(r, p, q) D_1(Ctt)(r, p, q) D_2(Cty)(r, p, q) - 4 Cxy(r, p, q) Cty(r, p, \\
& q) D_2(Ctt)(r, p, q) D_1(Cty)(r, p, q) + 4 Cxx(r, p, q) Ctt(r, p, q) D_3(Cty)(r, p, \\
& q) D_1(Cty)(r, p, q) - 2 Cxx(r, p, q) Ctt(r, p, q) D_3(Ctt)(r, p, q) D_3(Cty)(r, p, q) \Big), \\
D_{1,2}(Cty)(r, p, q) = & \frac{1}{4} \frac{1}{HessUniv} \Big( -4 Cty(r, p, q)^2 D_1(Cxx)(r, p, q) D_2(Cty)(r, p, q) \\
& - 4 Ctt(r, p, q) Cxy(r, p, q) D_2(Cty)(r, p, q)^2 - 4 Cxy(r, p, q)^2 D_2(Ctt)(r, p, \\
& q) D_1(Cty)(r, p, q) - 4 Ctx(r, p, q) D_2(Cty)(r, p, q) D_1(Ctx)(r, p, q) - 2 Cxx(r, p, \\
& q) D_3(Ctt)(r, p, q) D_1(Ctx)(r, p, q) + 2 Cxx(r, p, q) D_2(Ctt)(r, p, q) D_1(Cty)(r, p, q) \\
& - 2 Ctx(r, p, q) D_1(Cxx)(r, p, q) D_1(Cty)(r, p, q) - 2 Ctx(r, p, q) D_2(Ctt)(r, p, \\
& q) D_1(Cxy)(r, p, q) + 2 Cxy(r, p, q) D_2(Ctt)(r, p, q) D_1(Ctx)(r, p, q) + 2 Cxx(r, p, \\
& q) D_1(Ctt)(r, p, q) D_3(Ctx)(r, p, q) + 2 Cxx(r, p, q) D_1(Ctt)(r, p, q) D_2(Cty)(r, p, q) \\
& + 2 Ctx(r, p, q) D_1(Ctt)(r, p, q) D_2(Cxy)(r, p, q) - 2 Ctx(r, p, q) D_2(Ctt)(r, p, \\
& q) D_2(Cty)(r, p, q) - 2 Cxy(r, p, q) D_1(Ctt)(r, p, q) D_2(Ctx)(r, p, q) - Ctt(r, p, \\
& q) D_2(Ctt)(r, p, q) D_3(Cxx)(r, p, q) + Ctt(r, p, q) D_2(Cxx)(r, p, q) D_3(Ctt)(r, p, q) \\
& + Cty(r, p, q) D_2(Ctt)(r, p, q) D_1(Cxx)(r, p, q) - Cty(r, p, q) D_2(Cxx)(r, p, q) D_1(Ctt)(r, \\
& p, q) + 2 Ctt(r, p, q) D_1(Cxx)(r, p, q) D_2(Cty)(r, p, q) + 2 Ctt(r, p, q) D_2(Cxx)(r, p, \\
& q) D_1(Cty)(r, p, q) + 8 Ctx(r, p, q) Cty(r, p, q) D_2(Cty)(r, p, q) D_1(Cxy)(r, p, q) \\
& + 4 Cxy(r, p, q) Cty(r, p, q) D_1(Cxx)(r, p, q) D_1(Cty)(r, p, q) + 4 Cxy(r, p, q) Cty(r, p, \\
& q) D_2(Ctt)(r, p, q) D_2(Cty)(r, p, q) + 8 Cxy(r, p, q) Ctx(r, p, q) D_2(Cty)(r, p,
\end{aligned}$$

$$\begin{aligned}
& q) D_1(Cty)(r, p, q) + 4 Cxx(r, p, q) Cty(r, p, q) D_3(Cty)(r, p, q) D_1(Ctx)(r, p, q) \\
& - 4 Cxx(r, p, q) Cty(r, p, q) D_2(Cty)(r, p, q) D_1(Cty)(r, p, q) - 4 Cxx(r, p, q) Ctx(r, p, \\
& q) D_3(Cty)(r, p, q) D_1(Cty)(r, p, q) - 4 Cxx(r, p, q) Ctt(r, p, q) D_3(Ctx)(r, p, \\
& q) D_3(Cty)(r, p, q) + 4 Cxx(r, p, q) Ctt(r, p, q) D_2(Cty)(r, p, q) D_3(Cty)(r, p, q) \\
& - 2 Cxx(r, p, q) Cty(r, p, q) D_2(Ctt)(r, p, q) D_3(Cty)(r, p, q) + 2 Cxx(r, p, q) Ctx(r, p, \\
& q) D_3(Ctt)(r, p, q) D_3(Cty)(r, p, q) + 2 Cxx(r, p, q) Cxy(r, p, q) D_3(Ctt)(r, p, \\
& q) D_1(Cty)(r, p, q) + 2 Ctt(r, p, q) Ctx(r, p, q) D_3(Cxx)(r, p, q) D_3(Cty)(r, p, q) \\
& - 2 Ctt(r, p, q) Cxy(r, p, q) D_1(Cxx)(r, p, q) D_3(Cty)(r, p, q) - 2 Ctt(r, p, q) Cxy(r, p, \\
& q) D_3(Cxx)(r, p, q) D_1(Cty)(r, p, q) + 4 Cxx(r, p, q) Ctt(r, p, q) D_3(Cty)(r, p, \\
& q) D_1(Cxy)(r, p, q) + 2 Ctt(r, p, q) Cty(r, p, q) D_3(Cxx)(r, p, q) D_2(Cty)(r, p, q) \\
& - 2 Ctt(r, p, q) Cty(r, p, q) D_2(Cxx)(r, p, q) D_3(Cty)(r, p, q) - 2 Cxx(r, p, q) Cty(r, p, \\
& q) D_3(Ctt)(r, p, q) D_2(Cty)(r, p, q) - 2 Cxx(r, p, q) Cxy(r, p, q) D_1(Ctt)(r, p, \\
& q) D_3(Cty)(r, p, q) - 4 Ctt(r, p, q) Ctx(r, p, q) D_2(Cxy)(r, p, q) D_3(Cty)(r, p, q) \\
& + 4 Ctt(r, p, q) Cxy(r, p, q) D_2(Ctx)(r, p, q) D_3(Cty)(r, p, q) - 4 Ctt(r, p, q) Cxy(r, p, \\
& q) D_2(Cty)(r, p, q) D_1(Cxy)(r, p, q) - 4 Cxx(r, p, q) Cty(r, p, q) D_1(Cxy)(r, p, \\
& q) D_1(Cty)(r, p, q) ),
\end{aligned}$$

$$\begin{aligned}
D_{1,3}(Cty)(r, p, q) &= \frac{1}{4} \frac{1}{HessUniv} \left( 2 Cxx(r, p, q) D_3(Ctt)(r, p, q) D_1(Cty)(r, p, q) - 4 Cty(r, \right. \\
& p, q)^2 D_1(Cxx)(r, p, q) D_3(Cty)(r, p, q) + Cty(r, p, q) D_3(Ctt)(r, p, q) D_1(Cxx)(r, p, q) \\
& - 4 Cty(r, p, q) D_2(Cty)(r, p, q) D_1(Ctx)(r, p, q) - 4 Ctx(r, p, q) D_1(Cxy)(r, p, \\
& q) D_1(Cty)(r, p, q) - 4 Ctx(r, p, q) D_3(Cty)(r, p, q) D_1(Ctx)(r, p, q) + 4 Ctx(r, p, \\
& q) D_2(Cty)(r, p, q) D_1(Cty)(r, p, q) + 2 Ctx(r, p, q) D_1(Ctt)(r, p, q) D_3(Cxy)(r, p, q) \\
& - 2 Ctt(r, p, q) D_2(Ctt)(r, p, q) D_3(Cxy)(r, p, q) - 2 Cxy(r, p, q) D_3(Ctt)(r, p, \\
& q) D_1(Ctx)(r, p, q) - 2 Cxy(r, p, q) D_2(Ctt)(r, p, q) D_1(Cty)(r, p, q) + 2 Cty(r, p, \\
& q) D_1(Cxx)(r, p, q) D_1(Cty)(r, p, q) - Cty(r, p, q) D_3(Cxx)(r, p, q) D_1(Ctt)(r, p, q) \\
& + 2 Cty(r, p, q) D_2(Ctt)(r, p, q) D_2(Cty)(r, p, q) - 2 Ctx(r, p, q) D_3(Ctt)(r, p, \\
& q) D_1(Cxy)(r, p, q) - 2 Ctx(r, p, q) D_3(Ctt)(r, p, q) D_2(Cty)(r, p, q) + 2 Ctt(r, p, \\
& q) D_3(Ctt)(r, p, q) D_2(Cxy)(r, p, q) + 4 Ctt(r, p, q) D_2(Ctx)(r, p, q) D_3(Cty)(r, p, q) \\
& + 4 Ctt(r, p, q) D_2(Cxy)(r, p, q) D_1(Cty)(r, p, q) + 2 Cxy(r, p, q) D_1(Ctt)(r, p, \\
& q) D_3(Ctx)(r, p, q) + 2 Cxy(r, p, q) D_1(Ctt)(r, p, q) D_2(Cty)(r, p, q) + 2 Cxx(r, p, \\
& q) D_1(Ctt)(r, p, q) D_3(Cty)(r, p, q) - 4 Cxy(r, p, q)^2 D_1(Ctt)(r, p, q) D_3(Cty)(r, p, q) \\
& - 2 Ctx(r, p, q) D_2(Ctt)(r, p, q) D_3(Cty)(r, p, q) - 2 D_1(Ctt)(r, p, q) D_2(Ctx)(r, p, q) \\
& - 4 Ctt(r, p, q) D_2(Cty)(r, p, q)^2 + 2 D_2(Ctt)(r, p, q) D_1(Ctx)(r, p, q) - 4 Cxx(r, p, \\
& q) Cty(r, p, q) D_3(Cty)(r, p, q) D_1(Cty)(r, p, q) + 8 Ctx(r, p, q) Cty(r, p, q) D_3(Cty)(r, p, \\
& q) D_1(Cxy)(r, p, q) - 4 Ctt(r, p, q) Cxy(r, p, q) D_3(Ctx)(r, p, q) D_3(Cty)(r, p, q) \\
& + 4 Ctt(r, p, q) Cxy(r, p, q) D_2(Cty)(r, p, q) D_3(Cty)(r, p, q) + 8 Cxy(r, p, q) Cty(r, p, \\
& q) D_3(Cty)(r, p, q) D_1(Ctx)(r, p, q) + 2 Ctt(r, p, q) Cty(r, p, q) D_3(Cxx)(r, p,
\end{aligned}$$

$$\begin{aligned}
& q) D_3(Cty)(r, p, q) + 4 Ctt(r, p, q) Cty(r, p, q) D_2(Cty)(r, p, q) D_3(Cxy)(r, p, q) \\
& - 8 Ctt(r, p, q) Cty(r, p, q) D_2(Cxy)(r, p, q) D_3(Cty)(r, p, q) - 4 Ctt(r, p, q) Cxy(r, p, \\
& q) D_3(Cxy)(r, p, q) D_1(Cty)(r, p, q) + 4 Cxy(r, p, q) Ctx(r, p, q) D_3(Ctt)(r, p, \\
& q) D_3(Cty)(r, p, q) - 2 Cxx(r, p, q) Cty(r, p, q) D_3(Ctt)(r, p, q) D_3(Cty)(r, p, q) \Big), \\
D_{2,2}(Cty)(r, p, q) = & -\frac{1}{4} \frac{1}{HessUniv} \Big( -4 Ctx(r, p, q) Cty(r, p, q) D_3(Cxx)(r, p, q) D_2(Cty)(r, \\
& p, q) - 8 Ctx(r, p, q) Cty(r, p, q) D_2(Cxy)(r, p, q) D_2(Cty)(r, p, q) + 4 Ctx(r, p, q) Cty(r, \\
& p, q) D_2(Cxx)(r, p, q) D_3(Cty)(r, p, q) + 8 Ctt(r, p, q) Cxy(r, p, q) D_2(Cxy)(r, p, \\
& q) D_2(Cty)(r, p, q) + 4 Cxy(r, p, q) Cty(r, p, q) D_1(Cxx)(r, p, q) D_2(Cty)(r, p, q) \\
& - 8 Cxy(r, p, q) Cty(r, p, q) D_2(Ctx)(r, p, q) D_2(Cty)(r, p, q) - 4 Cxy(r, p, q) Cty(r, p, \\
& q) D_2(Cxx)(r, p, q) D_1(Cty)(r, p, q) + 4 Cxy(r, p, q) Ctx(r, p, q) D_1(Cxx)(r, p, \\
& q) D_3(Cty)(r, p, q) + 4 Cxy(r, p, q) Ctx(r, p, q) D_3(Cxx)(r, p, q) D_1(Cty)(r, p, q) \\
& - 8 Cxy(r, p, q) Ctx(r, p, q) D_2(Ctx)(r, p, q) D_3(Cty)(r, p, q) - 8 Cxy(r, p, q) Ctx(r, p, \\
& q) D_2(Cxy)(r, p, q) D_1(Cty)(r, p, q) - 4 Cxx(r, p, q) Cty(r, p, q) D_1(Cxx)(r, p, \\
& q) D_3(Cty)(r, p, q) - 4 Cxx(r, p, q) Cty(r, p, q) D_2(Cty)(r, p, q) D_1(Cxy)(r, p, q) \\
& + 4 Cxx(r, p, q) Cty(r, p, q) D_2(Cty)(r, p, q) D_3(Ctx)(r, p, q) + 8 Cxx(r, p, q) Cty(r, p, \\
& q) D_2(Cxy)(r, p, q) D_1(Cty)(r, p, q) - 4 Cxx(r, p, q) Ctx(r, p, q) D_3(Cty)(r, p, \\
& q) D_1(Cxy)(r, p, q) + 4 Cxx(r, p, q) Ctx(r, p, q) D_3(Ctx)(r, p, q) D_3(Cty)(r, p, q) \\
& - 4 Cxx(r, p, q) Ctx(r, p, q) D_2(Cty)(r, p, q) D_3(Cty)(r, p, q) - 4 Cxx(r, p, q) Ctt(r, p, \\
& q) D_2(Cxy)(r, p, q) D_3(Cty)(r, p, q) + 4 Cxx(r, p, q) Cxy(r, p, q) D_1(Cxy)(r, p, \\
& q) D_1(Cty)(r, p, q) - 4 Cxx(r, p, q) Cxy(r, p, q) D_3(Ctx)(r, p, q) D_1(Cty)(r, p, q) \\
& - 4 Cxx(r, p, q) Cxy(r, p, q) D_2(Cty)(r, p, q) D_1(Cty)(r, p, q) + 4 Cxx(r, p, q) Cxy(r, p, \\
& q) D_2(Ctt)(r, p, q) D_3(Cty)(r, p, q) + 2 Cxx(r, p, q) Ctt(r, p, q) D_3(Cxx)(r, p, \\
& q) D_3(Cty)(r, p, q) + 8 Ctx(r, p, q) D_2(Ctx)(r, p, q) D_2(Cty)(r, p, q) - 4 Ctt(r, p, \\
& q) D_2(Cxx)(r, p, q) D_2(Cty)(r, p, q) + 4 Cxx(r, p, q) Cty(r, p, q) D_2(Cty)(r, p, q)^2 \\
& + Cxx(r, p, q) D_3(Ctt)(r, p, q) D_1(Cxx)(r, p, q) - Cxx(r, p, q) D_3(Cxx)(r, p, \\
& q) D_1(Ctt)(r, p, q) - 4 Cxx(r, p, q) D_2(Ctx)(r, p, q) D_1(Cty)(r, p, q) + 4 Cxx(r, p, \\
& q)^2 D_3(Cty)(r, p, q) D_1(Cty)(r, p, q) + 2 Ctx(r, p, q) D_2(Ctt)(r, p, q) D_3(Cxx)(r, p, q) \\
& - 2 Ctx(r, p, q) D_2(Cxx)(r, p, q) D_3(Ctt)(r, p, q) - 2 Cxy(r, p, q) D_2(Ctt)(r, p, \\
& q) D_1(Cxx)(r, p, q) + 2 Cxy(r, p, q) D_2(Cxx)(r, p, q) D_1(Ctt)(r, p, q) - 2 Cxx(r, p, \\
& q) D_1(Ctt)(r, p, q) D_2(Cxy)(r, p, q) + 2 Cxx(r, p, q) D_1(Cxx)(r, p, q) D_1(Cty)(r, p, q) \\
& + 2 Cxx(r, p, q) D_3(Ctt)(r, p, q) D_2(Ctx)(r, p, q) + 2 Cxx(r, p, q) D_2(Ctt)(r, p, \\
& q) D_1(Cxy)(r, p, q) - 2 Cxx(r, p, q) D_2(Ctt)(r, p, q) D_3(Ctx)(r, p, q) - 2 Cxx(r, p, \\
& q) D_2(Ctt)(r, p, q) D_2(Cty)(r, p, q) - 2 Cxx(r, p, q)^2 D_3(Ctt)(r, p, q) D_3(Cty)(r, p, q) \\
& + 4 Cty(r, p, q)^2 D_2(Cxx)(r, p, q) D_2(Cty)(r, p, q) - 4 Ctx(r, p, q)^2 D_3(Cxx)(r, p,
\end{aligned}$$



$$\begin{aligned}
& q) D_3(Cty)(r, p, q) + 8 Ctx(r, p, q)^2 D_2(Cxy)(r, p, q) D_3(Cty)(r, p, q) - 4 Cxy(r, p, \\
& q)^2 D_1(Cxx)(r, p, q) D_1(Cty)(r, p, q) + 8 Cxy(r, p, q)^2 D_2(Ctx)(r, p, q) D_1(Cty)(r, p, q) \Big), \\
D_{2,3}(Cty)(r, p, q) = & \frac{1}{4} \frac{1}{HessUniv} \Big( 8 Cxx(r, p, q) Cty(r, p, q) D_3(Cty)(r, p, q) D_1(Cxy)(r, p, \\
& q) - 4 Cxx(r, p, q) Cty(r, p, q) D_3(Ctx)(r, p, q) D_3(Cty)(r, p, q) - 4 Cxx(r, p, q) Cty(r, p, \\
& q) D_3(Cxy)(r, p, q) D_1(Cty)(r, p, q) - 4 Cxx(r, p, q) Cty(r, p, q) D_2(Cty)(r, p, \\
& q) D_3(Cty)(r, p, q) - 4 Cxx(r, p, q) Cxy(r, p, q) D_3(Cty)(r, p, q) D_1(Cty)(r, p, q) \\
& - 2 Ctt(r, p, q) Cxy(r, p, q) D_3(Cxx)(r, p, q) D_3(Cty)(r, p, q) + 4 Ctx(r, p, q) Cty(r, p, \\
& q) D_3(Cxx)(r, p, q) D_3(Cty)(r, p, q) + 8 Ctx(r, p, q) Cty(r, p, q) D_2(Cty)(r, p, \\
& q) D_3(Cxy)(r, p, q) - 8 Ctx(r, p, q) Cty(r, p, q) D_2(Cxy)(r, p, q) D_3(Cty)(r, p, q) \\
& - 4 Ctt(r, p, q) Cxy(r, p, q) D_2(Cty)(r, p, q) D_3(Cxy)(r, p, q) + 8 Cxy(r, p, q) Cty(r, p, \\
& q) D_2(Ctx)(r, p, q) D_3(Cty)(r, p, q) + 8 Cxy(r, p, q) Ctx(r, p, q) D_2(Cty)(r, p, \\
& q) D_3(Cty)(r, p, q) - 4 Cxx(r, p, q) D_1(Cxy)(r, p, q) D_1(Cty)(r, p, q) + 4 Cxx(r, p, \\
& q) D_3(Ctx)(r, p, q) D_1(Cty)(r, p, q) + 4 Cxx(r, p, q) D_2(Cty)(r, p, q) D_1(Cty)(r, p, q) \\
& - 2 Cty(r, p, q) D_1(Cxx)(r, p, q) D_2(Cty)(r, p, q) + 2 Cty(r, p, q) D_2(Cxx)(r, p, \\
& q) D_1(Cty)(r, p, q) - 2 Ctx(r, p, q) D_1(Cxx)(r, p, q) D_3(Cty)(r, p, q) + 2 Ctx(r, p, \\
& q) D_3(Ctt)(r, p, q) D_2(Cxy)(r, p, q) - 2 Ctx(r, p, q) D_3(Cxx)(r, p, q) D_1(Cty)(r, p, q) \\
& - 2 Ctx(r, p, q) D_2(Ctt)(r, p, q) D_3(Cxy)(r, p, q) + 2 Ctt(r, p, q) D_3(Cxx)(r, p, \\
& q) D_2(Cty)(r, p, q) + 2 Ctt(r, p, q) D_2(Cxx)(r, p, q) D_3(Cty)(r, p, q) + 2 Cxy(r, p, \\
& q) D_1(Cxx)(r, p, q) D_1(Cty)(r, p, q) - 2 Cxy(r, p, q) D_3(Ctt)(r, p, q) D_2(Ctx)(r, p, q) \\
& + 2 Cxy(r, p, q) D_2(Ctt)(r, p, q) D_3(Ctx)(r, p, q) + 2 Cxy(r, p, q) D_2(Ctt)(r, p, \\
& q) D_2(Cty)(r, p, q) + 2 Cxx(r, p, q) D_1(Ctt)(r, p, q) D_3(Cxy)(r, p, q) - 2 Cxx(r, p, \\
& q) D_3(Ctt)(r, p, q) D_1(Cxy)(r, p, q) - 4 Cty(r, p, q)^2 D_2(Cxx)(r, p, q) D_3(Cty)(r, p, q) \\
& - 4 Cxy(r, p, q)^2 D_2(Ctt)(r, p, q) D_3(Cty)(r, p, q) - Cty(r, p, q) D_2(Ctt)(r, p, \\
& q) D_3(Cxx)(r, p, q) + Cty(r, p, q) D_2(Cxx)(r, p, q) D_3(Ctt)(r, p, q) - 4 Ctx(r, p, \\
& q) D_2(Cty)(r, p, q) D_3(Ctx)(r, p, q) + 4 Ctx(r, p, q) D_2(Cxy)(r, p, q) D_1(Cty)(r, p, q) \\
& - 4 Cxy(r, p, q) D_2(Ctx)(r, p, q) D_1(Cty)(r, p, q) + 2 Cxx(r, p, q) Cxy(r, p, q) D_3(Ctt)(r, \\
& p, q) D_3(Cty)(r, p, q) + D_2(Ctt)(r, p, q) D_1(Cxx)(r, p, q) - 4 Ctx(r, p, q) D_2(Cty)(r, \\
& p, q)^2 - D_2(Cxx)(r, p, q) D_1(Ctt)(r, p, q) \Big), \\
D_{3,3}(Cty)(r, p, q) = & \frac{1}{4} \frac{1}{HessUniv} \Big( 8 Ctx(r, p, q) Cty(r, p, q) D_3(Cxy)(r, p, q) D_3(Cty)(r, p, \\
& q) - 8 Ctt(r, p, q) Cxy(r, p, q) D_3(Cxy)(r, p, q) D_3(Cty)(r, p, q) + 16 Cxy(r, p, q) Cty(r, \\
& p, q) D_3(Cty)(r, p, q) D_1(Cxy)(r, p, q) - 8 Cxy(r, p, q) Cty(r, p, q) D_3(Cxy)(r, p, \\
& q) D_1(Cty)(r, p, q) + 8 Cxy(r, p, q) Cty(r, p, q) D_2(Cty)(r, p, q) D_3(Cty)(r, p, q) \\
& + 8 Cxy(r, p, q) Ctx(r, p, q) D_3(Cty)(r, p, q)^2 - 8 Cxy(r, p, q)^2 D_3(Cty)(r, p,
\end{aligned}$$

$$\begin{aligned}
& q) D_1(Cty)(r, p, q) - 4 Cty(r, p, q) D_1(Cxx)(r, p, q) D_3(Cty)(r, p, q) + 4 Cty(r, p, \\
& q) D_3(Ctt)(r, p, q) D_2(Cxy)(r, p, q) - 4 Cty(r, p, q) D_2(Cty)(r, p, q) D_1(Cxy)(r, p, q) \\
& - 4 Cty(r, p, q) D_2(Cty)(r, p, q) D_3(Ctx)(r, p, q) + 8 Cty(r, p, q) D_2(Ctx)(r, p, \\
& q) D_3(Cty)(r, p, q) - 4 Cty(r, p, q) D_2(Ctt)(r, p, q) D_3(Cxy)(r, p, q) + 8 Cty(r, p, \\
& q) D_2(Cxy)(r, p, q) D_1(Cty)(r, p, q) - 4 Ctx(r, p, q) D_3(Cty)(r, p, q) D_1(Cxy)(r, p, q) \\
& - 4 Ctx(r, p, q) D_3(Ctx)(r, p, q) D_3(Cty)(r, p, q) - 4 Ctx(r, p, q) D_2(Cty)(r, p, \\
& q) D_3(Cty)(r, p, q) + 4 Ctt(r, p, q) D_2(Cxy)(r, p, q) D_3(Cty)(r, p, q) + 4 Cxy(r, p, \\
& q) D_1(Ctt)(r, p, q) D_3(Cxy)(r, p, q) - 4 Cxy(r, p, q) D_1(Cxy)(r, p, q) D_1(Cty)(r, p, q) \\
& + 4 Cxy(r, p, q) D_3(Ctx)(r, p, q) D_1(Cty)(r, p, q) - 4 Cxy(r, p, q) D_3(Ctt)(r, p, \\
& q) D_1(Cxy)(r, p, q) + 4 Cxy(r, p, q) D_2(Cty)(r, p, q) D_1(Cty)(r, p, q) - 4 Cxy(r, p, \\
& q) D_2(Ctt)(r, p, q) D_3(Cty)(r, p, q) - 8 Cxx(r, p, q) Cty(r, p, q) D_3(Cty)(r, p, q)^2 \\
& + 4 Cxx(r, p, q) D_3(Cty)(r, p, q) D_1(Cty)(r, p, q) + 2 Ctt(r, p, q) D_3(Cxx)(r, p, \\
& q) D_3(Cty)(r, p, q) + 2 Cxx(r, p, q) D_3(Ctt)(r, p, q) D_3(Cty)(r, p, q) + 8 Cty(r, p, \\
& q)^2 D_2(Cty)(r, p, q) D_3(Cxy)(r, p, q) - 16 Cty(r, p, q)^2 D_2(Cxy)(r, p, q) D_3(Cty)(r, p, q) \\
& + 2 D_2(Ctt)(r, p, q) D_1(Cxy)(r, p, q) + 2 D_2(Ctt)(r, p, q) D_3(Ctx)(r, p, q) + 2 D_2(Ctt)(r, \\
& p, q) D_2(Cty)(r, p, q) - 2 D_3(Ctt)(r, p, q) D_2(Ctx)(r, p, q) - D_3(Cxx)(r, p, q) D_1(Ctt)(r, \\
& p, q) - 4 D_2(Ctx)(r, p, q) D_1(Cty)(r, p, q) + 2 D_1(Cxx)(r, p, q) D_1(Cty)(r, p, q) \\
& - 4 Cty(r, p, q) D_2(Cty)(r, p, q)^2 - 2 D_1(Ctt)(r, p, q) D_2(Cxy)(r, p, q) + D_3(Ctt)(r, p, \\
& q) D_1(Cxx)(r, p, q) \Big),
\end{aligned}$$

$$\begin{aligned}
D_{1,1}(Cxy)(r, p, q) = & -\frac{1}{4} \frac{1}{HessUniv} \Big( -4 Cty(r, p, q)^2 D_2(Ctt)(r, p, q) D_2(Cxy)(r, p, q) \\
& + 8 Cty(r, p, q)^2 D_2(Cxy)(r, p, q) D_1(Ctx)(r, p, q) - 4 Ctx(r, p, q)^2 D_3(Ctt)(r, p, \\
& q) D_3(Cxy)(r, p, q) + 8 Ctx(r, p, q)^2 D_3(Cxy)(r, p, q) D_1(Cty)(r, p, q) + 4 Ctt(r, p, \\
& q)^2 D_2(Cxy)(r, p, q) D_3(Cxy)(r, p, q) + 4 Ctt(r, p, q) Cxy(r, p, q) D_1(Cxy)(r, p, q)^2 \\
& + 4 Cxy(r, p, q)^2 D_1(Ctt)(r, p, q) D_1(Cxy)(r, p, q) + 8 Ctx(r, p, q) D_1(Cxy)(r, p, \\
& q) D_1(Ctx)(r, p, q) + Ctt(r, p, q) D_2(Ctt)(r, p, q) D_3(Cxx)(r, p, q) - 4 Ctt(r, p, \\
& q) D_2(Cxy)(r, p, q) D_1(Ctx)(r, p, q) - Ctt(r, p, q) D_2(Cxx)(r, p, q) D_3(Ctt)(r, p, q) \\
& - 4 Cxx(r, p, q) D_1(Ctt)(r, p, q) D_1(Cxy)(r, p, q) - 2 Ctt(r, p, q)^2 D_3(Cxx)(r, p, \\
& q) D_3(Cxy)(r, p, q) - 2 Cty(r, p, q) D_2(Ctt)(r, p, q) D_1(Cxx)(r, p, q) + 2 Cty(r, p, \\
& q) D_2(Cxx)(r, p, q) D_1(Ctt)(r, p, q) + 2 Ctx(r, p, q) D_3(Ctt)(r, p, q) D_1(Cxx)(r, p, q) \\
& - 2 Ctx(r, p, q) D_3(Cxx)(r, p, q) D_1(Ctt)(r, p, q) - 2 Ctt(r, p, q) D_1(Cxx)(r, p, \\
& q) D_1(Cxy)(r, p, q) - 2 Ctt(r, p, q) D_1(Cxx)(r, p, q) D_3(Ctx)(r, p, q) + 2 Ctt(r, p, \\
& q) D_1(Cxx)(r, p, q) D_2(Cty)(r, p, q) + 2 Ctt(r, p, q) D_3(Cxx)(r, p, q) D_1(Ctx)(r, p, q) \\
& + 2 Ctt(r, p, q) D_2(Ctt)(r, p, q) D_2(Cxy)(r, p, q) - 2 Ctt(r, p, q) D_2(Cxx)(r, p, \\
& q) D_1(Cty)(r, p, q) - 8 Ctx(r, p, q) Cty(r, p, q) D_3(Cxy)(r, p, q) D_1(Ctx)(r, p, q)
\end{aligned}$$

$$\begin{aligned}
& + 4 Ctx(r, p, q) Cty(r, p, q) D_2(Ctt)(r, p, q) D_3(Cxy)(r, p, q) - 8 Ctx(r, p, q) Cty(r, p, q) D_2(Cxy)(r, p, q) D_1(Cty)(r, p, q) + 4 Ctt(r, p, q) Cty(r, p, q) D_1(Cxx)(r, p, q) D_3(Cxy)(r, p, q) - 4 Ctt(r, p, q) Cty(r, p, q) D_2(Cxy)(r, p, q) D_1(Cxy)(r, p, q) \\
& - 4 Ctt(r, p, q) Cty(r, p, q) D_2(Cxy)(r, p, q) D_3(Ctx)(r, p, q) + 4 Ctt(r, p, q) Cty(r, p, q) D_2(Cxy)(r, p, q) D_2(Cty)(r, p, q) + 4 Ctx(r, p, q) Cty(r, p, q) D_3(Ctt)(r, p, q) D_2(Cxy)(r, p, q) - 4 Ctt(r, p, q) Ctx(r, p, q) D_3(Cxy)(r, p, q) D_1(Cxy)(r, p, q) \\
& + 4 Ctt(r, p, q) Ctx(r, p, q) D_3(Cxy)(r, p, q) D_3(Ctx)(r, p, q) - 4 Ctt(r, p, q) Ctx(r, p, q) D_2(Cty)(r, p, q) D_3(Cxy)(r, p, q) + 4 Ctt(r, p, q) Cxy(r, p, q) D_3(Ctx)(r, p, q) D_1(Cxy)(r, p, q) - 4 Ctt(r, p, q) Cxy(r, p, q) D_2(Cty)(r, p, q) D_1(Cxy)(r, p, q) \\
& - 4 Ctt(r, p, q) Cxy(r, p, q) D_2(Ctt)(r, p, q) D_3(Cxy)(r, p, q) + 8 Ctt(r, p, q) Cxy(r, p, q) D_2(Cxy)(r, p, q) D_1(Cty)(r, p, q) - 4 Cxy(r, p, q) Cty(r, p, q) D_1(Ctt)(r, p, q) D_2(Cxy)(r, p, q) - 8 Cxy(r, p, q) Cty(r, p, q) D_1(Cxy)(r, p, q) D_1(Ctx)(r, p, q) \\
& + 4 Cxy(r, p, q) Cty(r, p, q) D_2(Ctt)(r, p, q) D_1(Cxy)(r, p, q) + 4 Cxy(r, p, q) Ctx(r, p, q) D_1(Ctt)(r, p, q) D_3(Cxy)(r, p, q) - 8 Cxy(r, p, q) Ctx(r, p, q) D_1(Cxy)(r, p, q) D_1(Cty)(r, p, q) - 4 Cxy(r, p, q) Ctx(r, p, q) D_3(Ctt)(r, p, q) D_1(Cxy)(r, p, q) \\
& + 8 Cxx(r, p, q) Cty(r, p, q) D_1(Cxy)(r, p, q) D_1(Cty)(r, p, q) - 4 Cxx(r, p, q) Ctt(r, p, q) D_3(Cxy)(r, p, q) D_1(Cty)(r, p, q) + 2 Cxx(r, p, q) Ctt(r, p, q) D_3(Ctt)(r, p, q) D_3(Cxy)(r, p, q) ),
\end{aligned}$$

$$\begin{aligned}
D_{1,2}(Cxy)(r, p, q) = & -\frac{1}{4} \frac{1}{HessUniv} \left( 4 Ctt(r, p, q) Cxy(r, p, q) D_2(Cxy)(r, p, q) D_2(Cty)(r, p, q) + 4 Cxx(r, p, q) Cty(r, p, q) D_2(Cty)(r, p, q) D_1(Cxy)(r, p, q) - 4 Cxx(r, p, q) Cty(r, p, q) D_3(Cxy)(r, p, q) D_1(Ctx)(r, p, q) + 4 Cxx(r, p, q) Ctx(r, p, q) D_3(Cxy)(r, p, q) D_1(Cty)(r, p, q) - 2 Ctt(r, p, q) Cty(r, p, q) D_3(Cxx)(r, p, q) D_2(Cxy)(r, p, q) + 2 Ctt(r, p, q) Cty(r, p, q) D_2(Cxx)(r, p, q) D_3(Cxy)(r, p, q) + 2 Cxx(r, p, q) Cty(r, p, q) D_3(Ctt)(r, p, q) D_2(Cxy)(r, p, q) + 2 Cxx(r, p, q) Cty(r, p, q) D_2(Ctt)(r, p, q) D_3(Cxy)(r, p, q) + 2 Ctx(r, p, q) D_1(Cxx)(r, p, q) D_1(Cxy)(r, p, q) + 2 Ctx(r, p, q) D_2(Ctt)(r, p, q) D_2(Cxy)(r, p, q) + 4 Cty(r, p, q)^2 D_1(Cxx)(r, p, q) D_2(Cxy)(r, p, q) + 4 Cxy(r, p, q)^2 D_2(Ctt)(r, p, q) D_1(Cxy)(r, p, q) + 4 Ctx(r, p, q) D_2(Ctx)(r, p, q) D_1(Cxy)(r, p, q) + 4 Cxx(r, p, q) Cty(r, p, q) D_1(Cxy)(r, p, q)^2 + 2 Ctx(r, p, q) D_1(Cxx)(r, p, q) D_2(Cty)(r, p, q) - 2 Ctx(r, p, q) D_2(Cxx)(r, p, q) D_1(Cty)(r, p, q) - 2 Cty(r, p, q) D_1(Cxx)(r, p, q) D_2(Ctx)(r, p, q) + 2 Cty(r, p, q) D_2(Cxx)(r, p, q) D_1(Ctx)(r, p, q) - 2 Ctt(r, p, q) D_1(Cxx)(r, p, q) D_2(Cxy)(r, p, q) + 2 Ctt(r, p, q) D_3(Cxx)(r, p, q) D_2(Ctx)(r, p, q) - 2 Ctt(r, p, q) D_2(Cxx)(r, p, q) D_1(Cxy)(r, p, q) - 2 Ctt(r, p, q) D_2(Cxx)(r, p, q) D_3(Ctx)(r, p, q) + Cxx(r, p, q) D_3(Ctt)(r, p, q) D_1(Cxx)(r, p, q) - Cxx(r, p, q) D_3(Cxx)(r, p, q) D_1(Ctt)(r, p, q) - Cxy(r, p, q) D_2(Ctt)(r, p, q) D_1(Cxx)(r, p, q) + Cxy(r, p, q) D_2(Cxx)(r, p, q) D_1(Ctt)(r, p, q) - 2 Cxx(r, p, q) D_1(Ctt)(r, p, q) D_2(Cxy)(r, p, q) - 2 Cxx(r, p, q) D_2(Ctt)(r, p, q) D_1(Cxy)(r, p, q) - 8 Ctx(r, p, q) Cty(r, p, q) D_2(Cxy)(r, p, q) D_1(Cxy)(r, p, q) \right)
\end{aligned}$$

$$\begin{aligned}
& + 4 Ctt(r, p, q) Ctx(r, p, q) D_2(Cxy)(r, p, q) D_3(Cxy)(r, p, q) - 4 Ctt(r, p, q) Cxy(r, p, q) D_2(Ctx)(r, p, q) D_3(Cxy)(r, p, q) + 4 Ctt(r, p, q) Cxy(r, p, q) D_2(Cxy)(r, p, q) \\
& D_1(Cxy)(r, p, q) - 4 Cxy(r, p, q) Cty(r, p, q) D_1(Cxx)(r, p, q) D_1(Cxy)(r, p, q) - 4 Cxy(r, p, q) Cty(r, p, q) D_2(Ctt)(r, p, q) D_2(Cxy)(r, p, q) - 8 Cxy(r, p, q) Ctx(r, p, q) D_2(Cty)(r, p, q) D_1(Cxy)(r, p, q) \\
& - 4 Cxx(r, p, q) Ctt(r, p, q) D_3(Cxy)(r, p, q) D_3(Ctx)(r, p, q) - 4 Cxx(r, p, q) Ctt(r, p, q) D_2(Cty)(r, p, q) D_3(Cxy)(r, p, q) - 2 Ctt(r, p, q) Ctx(r, p, q) D_3(Cxx)(r, p, q) D_3(Cxy)(r, p, q) + 2 Ctt(r, p, q) Cxy(r, p, q) D_1(Cxx)(r, p, q) D_3(Cxy)(r, p, q) + 2 Ctt(r, p, q) Cxy(r, p, q) D_3(Cxx)(r, p, q) D_1(Cxy)(r, p, q) \\
& - 2 Cxx(r, p, q) Ctx(r, p, q) D_3(Ctt)(r, p, q) D_3(Cxy)(r, p, q) + 2 Cxx(r, p, q) Cxy(r, p, q) D_1(Ctt)(r, p, q) D_3(Cxy)(r, p, q) - 2 Cxx(r, p, q) Cxy(r, p, q) D_3(Ctt)(r, p, q) D_1(Cxy)(r, p, q) \Big), \\
D_{1,3}(Cxy)(r, p, q) = & -\frac{1}{4} \frac{1}{HessUniv} \Big( 4 Cxx(r, p, q) Cty(r, p, q) D_3(Cty)(r, p, q) D_1(Cxy)(r, p, q) - 8 Ctt(r, p, q) Cxy(r, p, q) D_2(Cty)(r, p, q) D_3(Cxy)(r, p, q) - 2 Cty(r, p, q) D_1(Cxx)(r, p, q) D_1(Cxy)(r, p, q) - 2 Cty(r, p, q) D_1(Cxx)(r, p, q) D_3(Ctx)(r, p, q) + 2 Cty(r, p, q) D_3(Cxx)(r, p, q) D_1(Ctx)(r, p, q) - 2 Cty(r, p, q) D_2(Ctt)(r, p, q) D_2(Cxy)(r, p, q) + 2 Cxy(r, p, q) D_2(Ctt)(r, p, q) D_1(Cxy)(r, p, q) + 4 Cty(r, p, q)^2 D_1(Cxx)(r, p, q) D_3(Cxy)(r, p, q) + 4 Cxy(r, p, q)^2 D_1(Ctt)(r, p, q) D_3(Cxy)(r, p, q) + 4 Cty(r, p, q) D_2(Cxy)(r, p, q) D_1(Ctx)(r, p, q) + 4 Ctx(r, p, q) D_3(Ctx)(r, p, q) D_1(Cxy)(r, p, q) - 4 Ctt(r, p, q) D_2(Cxy)(r, p, q) D_1(Cxy)(r, p, q) - 4 Ctt(r, p, q) D_2(Cxy)(r, p, q) D_3(Ctx)(r, p, q) + 4 Ctt(r, p, q) D_2(Cxy)(r, p, q) D_2(Cty)(r, p, q) + Cxy(r, p, q) D_3(Ctt)(r, p, q) D_1(Cxx)(r, p, q) - Cxy(r, p, q) D_3(Cxx)(r, p, q) D_1(Ctt)(r, p, q) + 2 Ctx(r, p, q) D_1(Cxx)(r, p, q) D_3(Cty)(r, p, q) + 2 Ctx(r, p, q) D_3(Ctt)(r, p, q) D_2(Cxy)(r, p, q) - 2 Ctx(r, p, q) D_3(Cxx)(r, p, q) D_1(Cty)(r, p, q) + 2 Ctx(r, p, q) D_2(Ctt)(r, p, q) D_3(Cxy)(r, p, q) + 2 Ctt(r, p, q) D_3(Cxx)(r, p, q) D_2(Cty)(r, p, q) - 2 Ctt(r, p, q) D_2(Cxx)(r, p, q) D_3(Cty)(r, p, q) - 2 Cxx(r, p, q) D_1(Ctt)(r, p, q) D_3(Cxy)(r, p, q) - 2 Cxx(r, p, q) D_3(Ctt)(r, p, q) D_1(Cxy)(r, p, q) - 4 Ctx(r, p, q) D_2(Cxy)(r, p, q) D_1(Cty)(r, p, q) - 2 Ctt(r, p, q) Cty(r, p, q) D_3(Cxx)(r, p, q) D_3(Cxy)(r, p, q) + 2 Cxx(r, p, q) Cty(r, p, q) D_3(Ctt)(r, p, q) D_3(Cxy)(r, p, q) - 8 Ctx(r, p, q) Cty(r, p, q) D_3(Cxy)(r, p, q) D_1(Cxy)(r, p, q) + 4 Ctt(r, p, q) Cty(r, p, q) D_2(Cxy)(r, p, q) D_3(Cxy)(r, p, q) + 4 Ctt(r, p, q) Cxy(r, p, q) D_3(Cxy)(r, p, q) D_3(Ctx)(r, p, q) + 4 Ctt(r, p, q) Cxy(r, p, q) D_2(Cxy)(r, p, q) D_3(Cty)(r, p, q) - 8 Cxy(r, p, q) Cty(r, p, q) D_3(Cxy)(r, p, q) D_1(Ctx)(r, p, q) - 8 Cxy(r, p, q) Ctx(r, p, q) D_3(Cty)(r, p, q) D_1(Cxy)(r, p, q) \Big)
\end{aligned}$$

$$\begin{aligned}
& -4 Cxy(r, p, q) Ctx(r, p, q) D_3(Ctt)(r, p, q) D_3(Cxy)(r, p, q) + 8 Cxy(r, p, q) Ctx(r, p, \\
& q) D_3(Cxy)(r, p, q) D_1(Cty)(r, p, q) - D_2(Ctt)(r, p, q) D_1(Cxx)(r, p, q) + 4 Ctx(r, p, \\
& q) D_1(Cxy)(r, p, q)^2 + D_2(Cxx)(r, p, q) D_1(Ctt)(r, p, q) \Big), \\
D_{2,2}(Cxy)(r, p, q) = & \frac{1}{4} \frac{1}{HessUniv} \Big( -8 Ctx(r, p, q) D_2(Cxy)(r, p, q) D_2(Ctx)(r, p, q) \\
& + 4 Ctx(r, p, q) D_2(Cxx)(r, p, q) D_3(Ctx)(r, p, q) + 4 Ctt(r, p, q) D_2(Cxx)(r, p, \\
& q) D_2(Cxy)(r, p, q) + 4 Cxy(r, p, q) D_1(Cxx)(r, p, q) D_2(Ctx)(r, p, q) - 4 Cxy(r, p, \\
& q) D_2(Cxx)(r, p, q) D_1(Ctx)(r, p, q) - 4 Cxx(r, p, q) Cxy(r, p, q) D_1(Cxy)(r, p, q)^2 \\
& + Cxx(r, p, q) D_2(Ctt)(r, p, q) D_3(Cxx)(r, p, q) + 4 Cxx(r, p, q) D_2(Cxy)(r, p, \\
& q) D_1(Ctx)(r, p, q) - Cxx(r, p, q) D_2(Cxx)(r, p, q) D_3(Ctt)(r, p, q) - 4 Cxx(r, p, \\
& q)^2 D_3(Cxy)(r, p, q) D_1(Cty)(r, p, q) + 2 Cxx(r, p, q) D_2(Cxx)(r, p, q) D_1(Cty)(r, p, q) \\
& + 2 Cxx(r, p, q)^2 D_3(Ctt)(r, p, q) D_3(Cxy)(r, p, q) - 4 Cty(r, p, q)^2 D_2(Cxx)(r, p, \\
& q) D_2(Cxy)(r, p, q) + 8 Ctx(r, p, q) Cty(r, p, q) D_2(Cxy)(r, p, q)^2 + 4 Ctx(r, p, \\
& q)^2 D_3(Cxx)(r, p, q) D_3(Cxy)(r, p, q) - 8 Ctx(r, p, q)^2 D_2(Cxy)(r, p, q) D_3(Cxy)(r, p, q) \\
& - 8 Ctt(r, p, q) Cxy(r, p, q) D_2(Cxy)(r, p, q)^2 + 4 Cxy(r, p, q)^2 D_1(Cxx)(r, p, \\
& q) D_1(Cxy)(r, p, q) - 8 Cxy(r, p, q)^2 D_2(Ctx)(r, p, q) D_1(Cxy)(r, p, q) - 4 Ctx(r, p, \\
& q) D_3(Cxx)(r, p, q) D_2(Ctx)(r, p, q) - 2 Cxx(r, p, q) D_1(Cxx)(r, p, q) D_1(Cxy)(r, p, q) \\
& - 2 Cxx(r, p, q) D_1(Cxx)(r, p, q) D_3(Ctx)(r, p, q) - 2 Cxx(r, p, q) D_1(Cxx)(r, p, \\
& q) D_2(Cty)(r, p, q) + 2 Cxx(r, p, q) D_3(Cxx)(r, p, q) D_1(Ctx)(r, p, q) + 2 Cxx(r, p, \\
& q) D_2(Ctt)(r, p, q) D_2(Cxy)(r, p, q) + 4 Cxx(r, p, q) Ctx(r, p, q) D_2(Cty)(r, p, \\
& q) D_3(Cxy)(r, p, q) + 4 Cxx(r, p, q) Ctt(r, p, q) D_2(Cxy)(r, p, q) D_3(Cxy)(r, p, q) \\
& + 4 Cxx(r, p, q) Cxy(r, p, q) D_3(Ctx)(r, p, q) D_1(Cxy)(r, p, q) + 4 Cxx(r, p, q) Cxy(r, p, \\
& q) D_2(Cty)(r, p, q) D_1(Cxy)(r, p, q) - 4 Cxx(r, p, q) Cxy(r, p, q) D_2(Ctt)(r, p, \\
& q) D_3(Cxy)(r, p, q) + 4 Ctx(r, p, q) Cty(r, p, q) D_3(Cxx)(r, p, q) D_2(Cxy)(r, p, q) \\
& - 4 Ctx(r, p, q) Cty(r, p, q) D_2(Cxx)(r, p, q) D_3(Cxy)(r, p, q) - 4 Cxy(r, p, q) Cty(r, p, \\
& q) D_1(Cxx)(r, p, q) D_2(Cxy)(r, p, q) + 8 Cxy(r, p, q) Cty(r, p, q) D_2(Cxy)(r, p, \\
& q) D_2(Ctx)(r, p, q) + 4 Cxy(r, p, q) Cty(r, p, q) D_2(Cxx)(r, p, q) D_1(Cxy)(r, p, q) \\
& - 4 Cxy(r, p, q) Ctx(r, p, q) D_1(Cxx)(r, p, q) D_3(Cxy)(r, p, q) - 4 Cxy(r, p, q) Ctx(r, p, \\
& q) D_3(Cxx)(r, p, q) D_1(Cxy)(r, p, q) + 8 Cxy(r, p, q) Ctx(r, p, q) D_2(Ctx)(r, p, \\
& q) D_3(Cxy)(r, p, q) + 8 Cxy(r, p, q) Ctx(r, p, q) D_2(Cxy)(r, p, q) D_1(Cxy)(r, p, q) \\
& - 2 Cxx(r, p, q) Ctt(r, p, q) D_3(Cxx)(r, p, q) D_3(Cxy)(r, p, q) + 4 Cxx(r, p, q) Cty(r, p, \\
& q) D_1(Cxx)(r, p, q) D_3(Cxy)(r, p, q) - 4 Cxx(r, p, q) Cty(r, p, q) D_2(Cxy)(r, p, \\
& q) D_1(Cxy)(r, p, q) - 4 Cxx(r, p, q) Cty(r, p, q) D_2(Cxy)(r, p, q) D_3(Ctx)(r, p, q) \\
& - 4 Cxx(r, p, q) Cty(r, p, q) D_2(Cxy)(r, p, q) D_2(Cty)(r, p, q) + 4 Cxx(r, p, q) Ctx(r, p, \\
& q) D_3(Cxy)(r, p, q) D_1(Cxy)(r, p, q) - 4 Cxx(r, p, q) Ctx(r, p, q) D_3(Cxy)(r, p, \\
& q) D_3(Ctx)(r, p, q) \Big), \\
D_{2,3}(Cxy)(r, p, q) = & -\frac{1}{4} \frac{1}{HessUniv} \Big( 2 Cxx(r, p, q) D_1(Cxx)(r, p, q) D_3(Cty)(r, p, q)
\end{aligned}$$

$$\begin{aligned}
& -2 Cxx(r, p, q) D_3(Cxx)(r, p, q) D_1(Cty)(r, p, q) + 4 Cty(r, p, q)^2 D_2(Cxx)(r, p, q) D_3(Cxy)(r, p, q) + 4 Cxy(r, p, q)^2 D_2(Ctt)(r, p, q) D_3(Cxy)(r, p, q) + 4 Ctx(r, p, q) D_2(Ctx)(r, p, q) D_3(Cxy)(r, p, q) - 4 Ctx(r, p, q) D_2(Cxy)(r, p, q) D_1(Cxy)(r, p, q) \\
& + 4 Ctx(r, p, q) D_2(Cxy)(r, p, q) D_2(Cty)(r, p, q) + 4 Cxy(r, p, q) D_2(Ctx)(r, p, q) D_1(Cxy)(r, p, q) - Cxy(r, p, q) D_2(Ctt)(r, p, q) D_3(Cxx)(r, p, q) + Cxy(r, p, q) D_2(Cxx)(r, p, q) D_3(Ctt)(r, p, q) - 4 Cxx(r, p, q) D_3(Cxy)(r, p, q) D_1(Ctx)(r, p, q) \\
& - 4 Cxx(r, p, q) D_2(Cxy)(r, p, q) D_1(Cty)(r, p, q) + 2 Cty(r, p, q) D_1(Cxx)(r, p, q) D_2(Cxy)(r, p, q) + 2 Cty(r, p, q) D_3(Cxx)(r, p, q) D_2(Ctx)(r, p, q) - 2 Cty(r, p, q) D_2(Cxx)(r, p, q) D_1(Cxy)(r, p, q) - 2 Cty(r, p, q) D_2(Cxx)(r, p, q) D_3(Ctx)(r, p, q) \\
& + 2 Ctx(r, p, q) D_1(Cxx)(r, p, q) D_3(Cxy)(r, p, q) + 2 Ctx(r, p, q) D_3(Cxx)(r, p, q) D_1(Cxy)(r, p, q) + 2 Ctx(r, p, q) D_3(Cxx)(r, p, q) D_2(Cty)(r, p, q) - 2 Ctx(r, p, q) D_2(Cxx)(r, p, q) D_3(Cty)(r, p, q) - 2 Ctt(r, p, q) D_3(Cxx)(r, p, q) D_2(Cxy)(r, p, q) \\
& - 2 Ctt(r, p, q) D_2(Cxx)(r, p, q) D_3(Cxy)(r, p, q) - 2 Cxy(r, p, q) D_1(Cxx)(r, p, q) D_1(Cxy)(r, p, q) - 2 Cxy(r, p, q) D_2(Ctt)(r, p, q) D_2(Cxy)(r, p, q) - 2 D_1(Cxx)(r, p, q) D_2(Ctx)(r, p, q) + 2 D_2(Cxx)(r, p, q) D_1(Ctx)(r, p, q) + 4 Cxx(r, p, q) D_1(Cxy)(r, p, q)^2 + 4 Cxx(r, p, q) Cty(r, p, q) D_3(Cxy)(r, p, q) D_3(Ctx)(r, p, q) + 4 Cxx(r, p, q) Cty(r, p, q) D_2(Cxy)(r, p, q) D_3(Cty)(r, p, q) - 4 Cxx(r, p, q) Cxy(r, p, q) D_3(Cty)(r, p, q) D_1(Cxy)(r, p, q) + 8 Cxx(r, p, q) Cxy(r, p, q) D_3(Cxy)(r, p, q) D_1(Cty)(r, p, q) - 4 Ctx(r, p, q) Cty(r, p, q) D_3(Cxx)(r, p, q) D_3(Cxy)(r, p, q) + 4 Ctt(r, p, q) Cxy(r, p, q) D_2(Cxy)(r, p, q) D_3(Cxy)(r, p, q) - 2 Cxx(r, p, q) Cxy(r, p, q) D_3(Ctt)(r, p, q) D_3(Cxy)(r, p, q) + 2 Ctt(r, p, q) Cxy(r, p, q) D_3(Cxx)(r, p, q) D_3(Cxy)(r, p, q) - 8 Cxy(r, p, q) Cty(r, p, q) D_2(Ctx)(r, p, q) D_3(Cxy)(r, p, q) - 8 Cxy(r, p, q) Ctx(r, p, q) D_2(Cty)(r, p, q) D_3(Cxy)(r, p, q) - 4 Cxx(r, p, q) Cty(r, p, q) D_3(Cxy)(r, p, q) D_1(Cxy)(r, p, q) \Big), \\
D_{3,3}(Cxy)(r, p, q) = & -\frac{1}{4} \frac{1}{HessUniv} \Big( -4 Cxx(r, p, q) D_3(Cxy)(r, p, q) D_1(Cty)(r, p, q) + 8 Cty(r, p, q)^2 D_2(Cxy)(r, p, q) D_3(Cxy)(r, p, q) - 8 Ctx(r, p, q) Cty(r, p, q) D_3(Cxy)(r, p, q)^2 + 8 Ctt(r, p, q) Cxy(r, p, q) D_3(Cxy)(r, p, q)^2 - 8 Cxy(r, p, q)^2 D_3(Cty)(r, p, q) D_1(Cxy)(r, p, q) + 16 Cxy(r, p, q)^2 D_3(Cxy)(r, p, q) D_1(Cty)(r, p, q) + 4 Cty(r, p, q) D_1(Cxx)(r, p, q) D_3(Cxy)(r, p, q) + 4 Cty(r, p, q) D_3(Cxx)(r, p, q) D_2(Cty)(r, p, q) - 4 Cty(r, p, q) D_2(Cxy)(r, p, q) D_1(Cxy)(r, p, q) - 4 Cty(r, p, q) D_2(Cxy)(r, p, q) D_3(Ctx)(r, p, q) + 4 Cty(r, p, q) D_2(Cxy)(r, p, q) D_2(Cty)(r, p, q) - 4 Cty(r, p, q) D_2(Cxx)(r, p, q) D_3(Cty)(r, p, q) + 4 Ctx(r, p, q) D_3(Cxy)(r, p, q) D_1(Cxy)(r, p, q) + 4 Ctx(r, p, q) D_3(Cxy)(r, p, q) D_3(Ctx)(r, p, q) + 4 Ctx(r, p, q) D_2(Cty)(r, p, q) D_3(Cxy)(r, p, q) - 4 Ctt(r, p, q) D_2(Cxy)(r, p, q) D_3(Cxy)(r, p, q) + 4 Cxy(r, p, q) D_1(Cxx)(r, p, q) D_3(Cty)(r, p, q) + 4 Cxy(r, p, q) D_3(Ctx)(r, p, q)
\end{aligned}$$

$$\begin{aligned}
& q) D_1(Cxy)(r, p, q) - 8 Cxy(r, p, q) D_3(Cxy)(r, p, q) D_1(Ctx)(r, p, q) - 4 Cxy(r, p, \\
& q) D_3(Cxx)(r, p, q) D_1(Cty)(r, p, q) + 4 Cxy(r, p, q) D_2(Cty)(r, p, q) D_1(Cxy)(r, p, q) \\
& + 4 Cxy(r, p, q) D_2(Ctt)(r, p, q) D_3(Cxy)(r, p, q) - 8 Cxy(r, p, q) D_2(Cxy)(r, p, \\
& q) D_1(Cty)(r, p, q) - 2 Cxx(r, p, q) D_3(Ctt)(r, p, q) D_3(Cxy)(r, p, q) - 2 Ctt(r, p, \\
& q) D_3(Cxx)(r, p, q) D_3(Cxy)(r, p, q) + 4 Cxy(r, p, q) D_1(Cxy)(r, p, q)^2 - D_2(Ctt)(r, p, \\
& q) D_3(Cxx)(r, p, q) + 4 D_2(Cxy)(r, p, q) D_1(Ctx)(r, p, q) + D_2(Cxx)(r, p, q) D_3(Ctt)(r, \\
& p, q) - 2 D_1(Cxx)(r, p, q) D_1(Cxy)(r, p, q) - 2 D_1(Cxx)(r, p, q) D_3(Ctx)(r, p, q) \\
& - 2 D_1(Cxx)(r, p, q) D_2(Cty)(r, p, q) + 2 D_3(Cxx)(r, p, q) D_1(Ctx)(r, p, q) \\
& - 2 D_2(Ctt)(r, p, q) D_2(Cxy)(r, p, q) + 2 D_2(Cxx)(r, p, q) D_1(Cty)(r, p, q) - 8 Cxy(r, p, \\
& q) Cty(r, p, q) D_3(Cxy)(r, p, q) D_1(Cxy)(r, p, q) - 16 Cxy(r, p, q) Cty(r, p, q) D_2(Cty)(r, \\
& p, q) D_3(Cxy)(r, p, q) + 8 Cxy(r, p, q) Cty(r, p, q) D_2(Cxy)(r, p, q) D_3(Cty)(r, p, q) \\
& - 8 Cxy(r, p, q) Ctx(r, p, q) D_3(Cxy)(r, p, q) D_3(Cty)(r, p, q) + 8 Cxx(r, p, q) Cty(r, p, \\
& q) D_3(Cxy)(r, p, q) D_3(Cty)(r, p, q) \Big] :
\end{aligned}$$

Now we want to resolve the highest parts of Eq||i with respect to the second derivatives of  $f_{ij}$  and compare to these expressions but this is a bit tricky. So instead we substitute these 30 conditions to Eq||i (not only to their top degree parts) and check that they vanish.

```

> ICsubs[1]
> ICsd := convert(ICsubs, diff) :
> simplify(subs(ICsd, cnd[1]))
0
(13)

> EQQ1 := simplify(subs([u1=r, u2=p, u3=q], Eq1)) :
> EQQ2 := simplify(subs([u1=r, u2=p, u3=q], Eq2)) :
> EQQ3 := simplify(subs([u1=r, u2=p, u3=q], Eq3)) :
> EQQ4 := simplify(subs([u1=r, u2=p, u3=q], Eq4)) :
> EQQ5 := simplify(subs([u1=r, u2=p, u3=q], Eq5)) :
>
>
> [simplify(subs(ICsd, EQQ1)), simplify(subs(ICsd, EQQ2)), simplify(subs(ICsd, EQQ3)),
simplify(subs(ICsd, EQQ4)), simplify(subs(ICsd, EQQ5))]
[0, 0, 0, 0, 0]
(14)

```

Wow! The machine strained itself, but managed. So IC (integrability conditions) imply EW. Now to show the equivalence (to get the converse) we have to prove the solution to Eq||i=0 is unique. And for this it is enough to see to the top degree (quadratic in  $u_{ij}$ ) terms. There are  $5 \cdot \text{binom}(6,2)=75$  such (=cnd[i]). Every such a term is a 2nd order differential expression of  $f_{ij}$ . We consider the coefficients of the higher jets (symbol), and there are 30 of them (=SecJets). These coefficients are functions of  $f_{ij}$  alone (no derivatives). Since the equivalence group is GL(3), we can arrange any nondegenerate value for the matrix of the symbol of F at the given point. Since working over C does not restrict generality in this

respect, we assume the matrix is identity (substitution Sval below).

>

>  $SecJets := [D_{1,1}(Ctt)(r, p, q), D_{1,2}(Ctt)(r, p, q), D_{1,3}(Ctt)(r, p, q), D_{2,2}(Ctt)(r, p, q),$   
 $D_{2,3}(Ctt)(r, p, q), D_{3,3}(Ctt)(r, p, q), D_{1,1}(Cxx)(r, p, q), D_{1,2}(Cxx)(r, p, q), D_{1,3}(Cxx)(r,$   
 $p, q), D_{2,2}(Cxx)(r, p, q), D_{2,3}(Cxx)(r, p, q), D_{3,3}(Cxx)(r, p, q), D_{1,1}(Ctx)(r, p, q),$   
 $D_{1,2}(Ctx)(r, p, q), D_{1,3}(Ctx)(r, p, q), D_{2,2}(Ctx)(r, p, q), D_{2,3}(Ctx)(r, p, q), D_{3,3}(Ctx)(r,$   
 $p, q), D_{1,1}(Cty)(r, p, q), D_{1,2}(Cty)(r, p, q), D_{1,3}(Cty)(r, p, q), D_{2,2}(Cty)(r, p, q),$   
 $D_{2,3}(Cty)(r, p, q), D_{3,3}(Cty)(r, p, q), D_{1,1}(Cxy)(r, p, q), D_{1,2}(Cxy)(r, p, q),$   
 $D_{1,3}(Cxy)(r, p, q), D_{2,2}(Cxy)(r, p, q), D_{2,3}(Cxy)(r, p, q), D_{3,3}(Cxy)(r, p, q)] :$

>  $nops(SecJets)$

30

(15)

>

>  $cnd[1] := simplify(subs([u_1 = r, u_2 = p, u_3 = q], diff(Eq1, u_{1,1}, u_{1,1}))) :$   
 $cnd[2] := simplify(subs([u_1 = r, u_2 = p, u_3 = q], diff(Eq1, u_{1,1}, u_{1,2}))) :$   
 $cnd[3] := simplify(subs([u_1 = r, u_2 = p, u_3 = q], diff(Eq1, u_{1,1}, u_{1,3}))) :$   
 $cnd[4] := simplify(subs([u_1 = r, u_2 = p, u_3 = q], diff(Eq1, u_{1,1}, u_{2,2}))) :$   
 $cnd[5] := simplify(subs([u_1 = r, u_2 = p, u_3 = q], diff(Eq1, u_{1,1}, u_{2,3}))) :$   
 $cnd[6] := simplify(subs([u_1 = r, u_2 = p, u_3 = q], diff(Eq1, u_{1,2}, u_{1,2}))) :$   
 $cnd[7] := simplify(subs([u_1 = r, u_2 = p, u_3 = q], diff(Eq1, u_{1,2}, u_{1,3}))) :$   
 $cnd[8] := simplify(subs([u_1 = r, u_2 = p, u_3 = q], diff(Eq1, u_{1,2}, u_{2,2}))) :$   
 $cnd[9] := simplify(subs([u_1 = r, u_2 = p, u_3 = q], diff(Eq1, u_{1,2}, u_{2,3}))) :$   
 $cnd[10] := simplify(subs([u_1 = r, u_2 = p, u_3 = q], diff(Eq1, u_{1,3}, u_{1,3}))) :$   
 $cnd[11] := simplify(subs([u_1 = r, u_2 = p, u_3 = q], diff(Eq1, u_{1,3}, u_{2,2}))) :$   
 $cnd[12] := simplify(subs([u_1 = r, u_2 = p, u_3 = q], diff(Eq1, u_{1,3}, u_{2,3}))) :$   
 $cnd[13] := simplify(subs([u_1 = r, u_2 = p, u_3 = q], diff(Eq1, u_{2,2}, u_{2,2}))) :$   
 $cnd[14] := simplify(subs([u_1 = r, u_2 = p, u_3 = q], diff(Eq1, u_{2,2}, u_{2,3}))) :$   
 $cnd[15] := simplify(subs([u_1 = r, u_2 = p, u_3 = q], diff(Eq1, u_{2,3}, u_{2,3}))) :$   

>  $cnd[16] := simplify(subs([u_1 = r, u_2 = p, u_3 = q], diff(Eq2, u_{1,1}, u_{1,1}))) :$   
 $cnd[17] := simplify(subs([u_1 = r, u_2 = p, u_3 = q], diff(Eq2, u_{1,1}, u_{1,2}))) :$   
 $cnd[18] := simplify(subs([u_1 = r, u_2 = p, u_3 = q], diff(Eq2, u_{1,1}, u_{1,3}))) :$   
 $cnd[19] := simplify(subs([u_1 = r, u_2 = p, u_3 = q], diff(Eq2, u_{1,1}, u_{2,2}))) :$   
 $cnd[20] := simplify(subs([u_1 = r, u_2 = p, u_3 = q], diff(Eq2, u_{1,1}, u_{2,3}))) :$   
 $cnd[21] := simplify(subs([u_1 = r, u_2 = p, u_3 = q], diff(Eq2, u_{1,2}, u_{1,2}))) :$   
 $cnd[22] := simplify(subs([u_1 = r, u_2 = p, u_3 = q], diff(Eq2, u_{1,2}, u_{1,3}))) :$   
 $cnd[23] := simplify(subs([u_1 = r, u_2 = p, u_3 = q], diff(Eq2, u_{1,2}, u_{2,2}))) :$   
 $cnd[24] := simplify(subs([u_1 = r, u_2 = p, u_3 = q], diff(Eq2, u_{1,2}, u_{2,3}))) :$   
 $cnd[25] := simplify(subs([u_1 = r, u_2 = p, u_3 = q], diff(Eq2, u_{1,3}, u_{1,3}))) :$   
 $cnd[26] := simplify(subs([u_1 = r, u_2 = p, u_3 = q], diff(Eq2, u_{1,3}, u_{2,2}))) :$   
 $cnd[27] := simplify(subs([u_1 = r, u_2 = p, u_3 = q], diff(Eq2, u_{1,3}, u_{2,3}))) :$   
 $cnd[28] := simplify(subs([u_1 = r, u_2 = p, u_3 = q], diff(Eq2, u_{2,2}, u_{2,2}))) :$



[illegible]

```
> factor(coeff(cnd[1], diff(Cxy(r, p, q), r, r)))
```

$$> \text{factor}(\text{coeff}(\text{convert}(\text{cnd}[1], D), D_{1,1}(Cxy)(r, p, q)))$$

**>**

```
> seq( [seq(Mjau(i,j),j=1..30) ], i=1..7);
```

```
> MEQ := Matrix(75, 30, Mjau) :
```

>

>

>
