# Supplementary material for: Dispersionless integrable systems in 3D and Einstein-Weyl geometry
Source: arXiv:1208.2728 ancillary file (2013-05-09)
Supplement: Supplementary file 6 [file BKEF-2012-III-Hirota_form_integrability.pdf]

This is the worksheet accompanying the paper E.Ferapontov & B.Kruglikov "Dispersionless integrable systems in 3D and Einstein-Weyl geometry".  
The file ran on **Maple** version 16, the package **DifferentialGeometry** was used.

We consider the general 2nd order PDE in Hirota form:  $u_{tt}=F(u_{tx},u_{ty},u_{xx},u_{xy},u_{yy})$   
and prove that it's integrability is equivalent to EW property of the linearization conformal structure

> alias( $f=f(u_{2,2}, u_{2,3}, u_{3,3}, u_{1,2}, u_{1,3})$ );  
$$f$$
 (1)

> with(DifferentialGeometry) : with(Tensor) : with(Tools) : with(JetCalculus) :  
with(LinearAlgebra) : with(PDEtools, D\_Dx, declare, ToJet, FromJet) :

> declare( $h(u_{2,2}, u_{2,3}, u_{3,3})$ ) : subs( $[h_r(r, s, t) = haha]$ , subs( $[u_{2,2}=r, u_{2,3}=s, u_{3,3}=t, u_{1,2}$   
 $=a, u_{1,3}=b]$ ,  $\frac{d^3}{du_{1,3}^3} f(u_{2,2}, u_{2,3}, u_{3,3}, u_{1,2}, u_{1,3})$ ))  
$$h(u_{2,2}, u_{2,3}, u_{3,3})$$
 will now be displayed as 
$$f_{b,b,b}$$
 (2)

> DGsetup([t, x, y], [u], J2) :

>  $F := u_{1,1} - f(u_{2,2}, u_{2,3}, u_{3,3}, u_{1,2}, u_{1,3})$   
$$F := u_{1,1} - f(u_{2,2}, u_{2,3}, u_{3,3}, u_{1,2}, u_{1,3})$$
 (3)

>  $A := \text{Matrix}\left(\left[\left[\text{diff}(F, u[1,1]), \frac{1}{2} \text{diff}(F, u[1,2]), \frac{1}{2} \text{diff}(F, u[1,3])\right], \left[\frac{1}{2} \text{diff}(F, u[1,2]), \text{diff}(F, u[2,2]), \frac{1}{2} \text{diff}(F, u[2,3])\right], \left[\frac{1}{2} \text{diff}(F, u[1,3]), \frac{1}{2} \text{diff}(F, u[2,3]), \text{diff}(F, u[3,3])\right]\right]\right)$   
 $AA := \text{expand}(\text{MatrixInverse}(A)) : AM := \text{simplify}(\text{Determinant}(A) \cdot AA) : AdA := \text{Adjoint}(A) :$

> [A, AM - AdA]  
$$\left[ \begin{bmatrix} 1 & -\frac{1}{2} f_{u_{1,2}} & -\frac{1}{2} f_{u_{1,3}} \\ -\frac{1}{2} f_{u_{1,2}} & -f_{u_{2,2}} & -\frac{1}{2} f_{u_{2,3}} \\ -\frac{1}{2} f_{u_{1,3}} & -\frac{1}{2} f_{u_{2,3}} & -f_{u_{3,3}} \end{bmatrix}, \begin{bmatrix} 0 & 0 & 0 \\ 0 & 0 & 0 \\ 0 & 0 & 0 \end{bmatrix} \right]$$
 (4)

Here A is the matrix of the linearized operator (bivector=metric with upper indices),  
AA - the inverse (metric, which we remember is defined only up to conformal rescaling)  
and AJ=AM=AdA the adjoint matrix (which we use as a representative for the conformal class)

>  $aA := [\text{TotalDiff}(A[1,1], 1) + \text{TotalDiff}(A[1,2], 2) + \text{TotalDiff}(A[1,3], 3), \text{TotalDiff}(A[2,1], 1) + \text{TotalDiff}(A[2,2], 2) + \text{TotalDiff}(A[2,3], 3), \text{TotalDiff}(A[3,1], 1) + \text{TotalDiff}(A[3,2], 2) + \text{TotalDiff}(A[3,3], 3)] :$

>  $\omega := [AA[1,1] \cdot aA[1] + AA[1,2] \cdot aA[2] + AA[1,3] \cdot aA[3], AA[2,1] \cdot aA[1] + AA[2,2] \cdot aA[2] + AA[2,3] \cdot aA[3], AA[3,1] \cdot aA[1] + AA[3,2] \cdot aA[2] + AA[3,3] \cdot aA[3]]$

```

    · aA[2] + AA[2, 3] · aA[3], AA[3, 1] · aA[1] + AA[3, 2] · aA[2] + AA[3, 3] · aA[3]] :
  > DepVars := [u(t, x, y)] : AJ := simplify(FromJet(AM, DepVars)) :

```

```

  > DGsetup([t, x, y], M) :
  > g := evalDG(AJ[1, 1]·dt &t dt + AJ[1, 2]·dt &t dx + AJ[1, 3]·dt &t dy + AJ[2, 1]·dx &t dt
    + AJ[2, 2]·dx &t dx + AJ[2, 3]·dx &t dy + AJ[3, 1]·dy &t dt + AJ[3, 2]·dy &t dx
    + AJ[3, 3]·dy &t dy) :
  > C := Connection(a000*dt &t D_t &t dt + a111*dx &t D_x &t dx + a222*dy &t D_y &t dy
    + a001*(dt &t D_t &t dx + dx &t D_t &t dt) + a002*(dt &t D_t &t dy + dy &t D_t
    &t dt) + a102*(dx &t D_t &t dy + dy &t D_t &t dx) + a011*(dt &t D_x &t dx + dx
    &t D_x &t dt) + a012*(dt &t D_x &t dy + dy &t D_x &t dt) + a112*(dx &t D_x &t dy
    + dy &t D_x &t dx) + a021*(dt &t D_y &t dx + dx &t D_y &t dt) + a022*(dt &t D_y
    &t dy + dy &t D_y &t dt) + a122*(dx &t D_y &t dy + dy &t D_y &t dx) + a010*dt
    &t D_x &t dt + a121*dx &t D_y &t dx + a202*dy &t D_t &t dy + a020*dt &t D_y &t dt
    + a101*dx &t D_t &t dx + a212*dy &t D_x &t dy) :
  > TorsionTensor(C);

```

$0 \, dt \, D_t \, dt$

(5)

```

  > U1 := simplify(2·FromJet(ω[1], DepVars)) :
  U2 := simplify(2·FromJet(ω[2], DepVars)) :
  U3 := simplify(2·FromJet(ω[3], DepVars)) :

```

Here we determine the connection C and define the covector U=omega. Later we will demonstrate that this choice of omega is the only natural

```

  > Et := evalDG(DirectionalCovariantDerivative(D_t, g, C) - U1·g) :
  Ex := evalDG(DirectionalCovariantDerivative(D_x, g, C) - U2·g) :
  Ey := evalDG(DirectionalCovariantDerivative(D_y, g, C) - U3·g) :
  > Eq000 := TensorInnerProduct(g, Et, dt &t dt) :
  Eq001 := TensorInnerProduct(g, Et, dt &t dx) :
  Eq002 := TensorInnerProduct(g, Et, dt &t dy) :
  Eq011 := TensorInnerProduct(g, Et, dx &t dx) :
  Eq012 := TensorInnerProduct(g, Et, dx &t dy) :
  Eq022 := TensorInnerProduct(g, Et, dy &t dy) :
  Eq100 := TensorInnerProduct(g, Ex, dt &t dt) :
  Eq101 := TensorInnerProduct(g, Ex, dt &t dx) :
  Eq102 := TensorInnerProduct(g, Ex, dt &t dy) :
  Eq111 := TensorInnerProduct(g, Ex, dx &t dx) :
  Eq112 := TensorInnerProduct(g, Ex, dx &t dy) :
  Eq122 := TensorInnerProduct(g, Ex, dy &t dy) :
  Eq200 := TensorInnerProduct(g, Ey, dt &t dt) :
  Eq201 := TensorInnerProduct(g, Ey, dt &t dx) :
  Eq202 := TensorInnerProduct(g, Ey, dt &t dy) :
  Eq211 := TensorInnerProduct(g, Ey, dx &t dx) :
  Eq212 := TensorInnerProduct(g, Ey, dx &t dy) :
  Eq222 := TensorInnerProduct(g, Ey, dy &t dy) :
  > sA := solve({Eq000=0, Eq001=0, Eq002=0, Eq011=0, Eq012=0, Eq022=0, Eq100=0,
    Eq101=0, Eq102=0, Eq111=0, Eq112=0, Eq122=0, Eq200=0, Eq201=0, Eq202=0,
    Eq211=0, Eq212=0, Eq222=0}, [a000, a001, a002, a010, a011, a012, a020, a021, a022,
    a101, a102, a111, a112, a121, a122, a202, a212, a222]) :
  > C1 := evalDG(subs({op(op(sA))}, C)) :

```

```
> evalDG(CovariantDerivative(g, C1) - g &t (U1*dt + U2*dx + U3*dy));
0 dt dt dt
```

(6)

The connection  $C=C1$  is uniquely determined by the 1st equation of EW property:  $D_C(g)=\omega g$ .  
Let us consider the main defining relation:  $Ricci(C)=V*g$  ( $V$  is some scalar function).

```
> R1 := CurvatureTensor(C1) : Ric1 := RicciTensor(R1) : T1 := SymmetrizeIndices(Ric1, [1, 2],
"Symmetric") : Res := evalDG(T1 - V*g) :
> NEQt1 := ContractIndices(Res, D_t &t D_t, [[1, 1], [2, 2]]) : NEQt2 := ContractIndices(Res,
D_t &t D_x, [[1, 1], [2, 2]]) :
NEQt3 := ContractIndices(Res, D_t &t D_y, [[1, 1], [2, 2]]) : NEQt4 := ContractIndices(Res,
D_x &t D_x, [[1, 1], [2, 2]]) :
NEQt5 := ContractIndices(Res, D_x &t D_y, [[1, 1], [2, 2]]) : NEQt6 := ContractIndices(Res,
D_y &t D_y, [[1, 1], [2, 2]]) :
```

```
> DGsetup([t, x, y], [u], J2, 4) :
```

```
> de := DifferentialEquationData([F], [u1, 1])
```

```
de := [ {u1, 1}, [u1, 1 - f(u2, 2, u2, 3, u3, 3, u1, 2, u1, 3) ] ]
```

(7)

```
> de2 := Prolong(de, 2) : deTRA := Transformation(de2) :
```

```
> Eq0 := Pullback(deTRA, ToJet(NEQt1, DepVars, notation = jetnumbers)) :
```

```
> VS := solve(Eq0, V) :
```

```
> Eq1 := numer(subs(V=VS, Pullback(deTRA, ToJet(NEQt2, DepVars, notation
= jetnumbers)))) :
```

```
Eq2 := numer(subs(V=VS, Pullback(deTRA, ToJet(NEQt3, DepVars, notation
= jetnumbers)))) :
```

```
Eq3 := numer(subs(V=VS, Pullback(deTRA, ToJet(NEQt4, DepVars, notation
= jetnumbers)))) :
```

```
Eq4 := numer(subs(V=VS, Pullback(deTRA, ToJet(NEQt5, DepVars, notation
= jetnumbers)))) :
```

```
Eq5 := numer(subs(V=VS, Pullback(deTRA, ToJet(NEQt6, DepVars, notation
= jetnumbers)))) :
```

We first check that the highest (4th order) derivatives have zero coefficients:  
this condition uniquely specifies the covector  $\omega$ , so the universal formula for covector holds here

```
J2 > simplify(subs([u2, 2=r, u2, 3=s, u3, 3=t, u1, 2=a, u1, 3=b], [diff(Eq1, u1, 2, 2, 2),
diff(Eq1, u1, 2, 2, 3), diff(Eq1, u1, 2, 3, 3), diff(Eq1, u1, 3, 3, 3), diff(Eq1, u2, 2, 2, 2),
diff(Eq1, u2, 2, 2, 3), diff(Eq1, u2, 2, 3, 3), diff(Eq1, u2, 3, 3, 3), diff(Eq1, u3, 3, 3, 3) ]))
[0, 0, 0, 0, 0, 0, 0, 0, 0]
```

(8)

```
J2 > simplify(subs([u2, 2=r, u2, 3=s, u3, 3=t, u1, 2=a, u1, 3=b], [diff(Eq2, u1, 2, 2, 2),
diff(Eq2, u1, 2, 2, 3), diff(Eq2, u1, 2, 3, 3), diff(Eq2, u1, 3, 3, 3), diff(Eq2, u2, 2, 2, 2),
diff(Eq2, u2, 2, 2, 3), diff(Eq2, u2, 2, 3, 3), diff(Eq2, u2, 3, 3, 3), diff(Eq2, u3, 3, 3, 3) ]))
[0, 0, 0, 0, 0, 0, 0, 0, 0]
```

(9)

```
J2 > simplify(subs([u2, 2=r, u2, 3=s, u3, 3=t, u1, 2=a, u1, 3=b], [diff(Eq3, u1, 2, 2, 2),
diff(Eq3, u1, 2, 2, 3), diff(Eq3, u1, 2, 3, 3), diff(Eq3, u1, 3, 3, 3), diff(Eq3, u2, 2, 2, 2),
diff(Eq3, u2, 2, 2, 3), diff(Eq3, u2, 2, 3, 3), diff(Eq3, u2, 3, 3, 3), diff(Eq3, u3, 3, 3, 3) ]))
```

$$) \quad [0, 0, 0, 0, 0, 0, 0, 0, 0] \quad (10)$$

$$\begin{aligned} \mathbf{J2} > \text{simplify}(\text{subs}([u_{2,2}=r, u_{2,3}=s, u_{3,3}=t, u_{1,2}=a, u_{1,3}=b], [\text{diff}(Eq4, u_{1,2,2,2}), \\ &\text{diff}(Eq4, u_{1,2,2,3}), \text{diff}(Eq4, u_{1,2,3,3}), \text{diff}(Eq4, u_{1,3,3,3}), \text{diff}(Eq4, u_{2,2,2,2}), \\ &\text{diff}(Eq4, u_{2,2,2,3}), \text{diff}(Eq4, u_{2,2,3,3}), \text{diff}(Eq4, u_{2,3,3,3}), \text{diff}(Eq4, u_{3,3,3,3})]) \\ &)) \quad [0, 0, 0, 0, 0, 0, 0, 0, 0] \quad (11) \end{aligned}$$

$$\begin{aligned} \mathbf{J2} > \text{simplify}(\text{subs}([u_{2,2}=r, u_{2,3}=s, u_{3,3}=t, u_{1,2}=a, u_{1,3}=b], [\text{diff}(Eq5, u_{1,2,2,2}), \\ &\text{diff}(Eq5, u_{1,2,2,3}), \text{diff}(Eq5, u_{1,2,3,3}), \text{diff}(Eq5, u_{1,3,3,3}), \text{diff}(Eq5, u_{2,2,2,2}), \\ &\text{diff}(Eq5, u_{2,2,2,3}), \text{diff}(Eq5, u_{2,2,3,3}), \text{diff}(Eq5, u_{2,3,3,3}), \text{diff}(Eq5, u_{3,3,3,3})]) \\ &)) \quad [0, 0, 0, 0, 0, 0, 0, 0, 0] \quad (12) \end{aligned}$$

Thus the expressions Eq\_i (which are 5 components of Ricci-V\*g for suitably chosen V) are of the 3rd order in u.

Let us look to one of the coefficient of the quadratic part in the third derivatives to estimate the size of the whole data set

(in fact it is easy to check the expressions Eq\_i are purely quadratic in the 3-jet of u).

$$\mathbf{J2} > \text{Rest1} := \text{simplify}(\text{subs}([u_{2,2}=r, u_{2,3}=s, u_{3,3}=t, u_{1,2}=a, u_{1,3}=b], \text{diff}(Eq1, u_{2,2,2}, u_{2,2,2})))$$

$$\begin{aligned} \text{Rest1} := & 2f_r \left( -72f_s^4 f_t^3 f_{a,a} f_r^2 f_a^2 + 8f_a^3 f_t^3 f_b^4 f_r^2 f_{a,r} + 128f_b f_s f_a^2 s f_r^4 f_t^3 + 8f_b f_r f_s^5 f_r^2 s f_t - 12 \right. \\ & f_{a,t}^2 f_a^2 f_r^2 f_s^5 f_b + 32f_{a,t}^2 f_a^3 f_r^2 f_s^4 f_t + 4f_b^7 f_r s f_r^3 f_r f_t + 5f_b^4 f_s^4 f_a f_r^2 f_{b,r} - 24f_{a,t}^2 f_a^5 f_r^2 f_s^2 f_t^2 + 4 \\ & f_{a,t}^2 f_a^3 f_r^2 f_s^4 f_b^2 + f_b^7 f_r s f_r^2 f_r f_s^2 + 4f_b^3 f_s^5 f_r^2 f_a a f_{r,t} - 3f_{a,a} b f_s^7 f_r f_a^2 f_t + 36f_{a,a} b f_s^5 f_r^2 f_t^2 f_a^2 \\ & - 32f_b^4 f_a f_r^2 s f_r^3 f_t^2 - 4f_b^6 f_a f_r^2 s f_r^3 f_t - 64f_b^2 f_a f_r^2 s f_r^3 f_t^3 - 144f_{a,a} b f_s^3 f_r^3 f_t^3 f_a^2 - 24f_{a,a} b f_s^3 \\ & f_r^3 f_t^3 f_a^4 + 3f_{a,a} b f_s^5 f_r f_a^4 f_t^2 + 3f_{a,a} b f_s^7 f_r f_b^2 f_a^2 + 3f_{a,a} b f_s^8 f_r f_b f_a + 16f_a^3 f_t^2 f_s^4 f_r f_{b,r} - 32f_a^3 \\ & f_t^3 f_s^2 f_r^2 f_{b,r} - 896f_a^4 f_r^3 f_{a,a} f_s^2 - 72f_a^5 f_t^4 f_{a,a} f_r^2 f_s f_r + 8f_t^4 f_{a,t} f_a^6 f_{a,a} f_r^2 - 12f_a^3 f_t^2 \\ & f_s^5 f_{a,a} s f_r - 480f_a^3 f_t^4 f_s^2 f_{a,a} f_r^2 - 96f_a^4 f_s^4 f_{a,a} f_r^3 f_t^2 + 14f_a^4 f_r^6 f_{a,a} f_t^2 + 96f_b^3 f_r^4 f_{a,a} s f_t^3 \\ & f_a^2 - 48f_b^3 f_r^4 f_{a,a} s f_t^2 f_s^2 + 12f_b^3 f_r^3 f_{a,a} s f_t^3 f_a^4 - 12f_b^3 f_r^3 f_{a,a} s f_t f_s^4 - 8f_b^6 f_s f_r^4 f_{b,r} f_{r,t} - 192f_s \\ & f_a^4 f_t^4 f_{a,b} f_r^3 - 48f_s f_a^5 f_t^4 f_{a,b} f_r^2 - 4f_s f_a^7 f_t^4 f_{a,b} f_r f_r - 6f_a^5 f_s^4 f_{a,a} f_r f_t^2 - 6f_a^3 f_s^6 f_{a,a} f_r f_b^2 \\ & - 6f_a^2 f_s^7 f_{a,a} f_r f_b + 6f_a^3 f_s^6 f_{a,a} f_r f_t - 48f_a^3 f_s^4 f_{a,a} f_r^2 f_t^2 + 128f_a f_s^2 f_{a,a} f_r^4 f_t^3 + 96f_a^3 \\ & f_s^2 f_{a,a} f_t^3 f_t^3 + 384f_s^2 f_a f_t^4 f_{r,r} f_r^2 + 30f_b^4 f_s^4 f_a f_r^2 f_{r,t} - 16f_t^4 f_{a,t} f_a^7 f_r f_{a,r} + 4f_t^4 f_a^6 f_{a,a} b f_s \\ & f_r^2 - f_t^3 f_a^6 f_{a,a} b f_s^3 f_r + 12f_b^3 f_s^5 f_r^2 f_a f_{r,t} - 24f_b^3 f_s^4 f_r^2 f_{r,s} f_{r,t} + 3f_{a,t}^2 f_a^2 f_{b,s}^7 f_r + 8f_b^4 f_s^4 \\ & f_r^3 f_{a,a} f_{a,t} - 14f_b^4 f_s^4 f_r^2 f_{a,t} f_{r,r} + 64f_b^3 f_s f_r^3 f_t^2 f_{a,r} + 8f_b^5 f_s f_r^3 f_t^2 f_{a,r} - 192f_s^3 f_{b,r} f_{r,r} f_r^2 f_t^3 \\ & + 128f_a f_r^3 f_{r,t} f_t^2 f_s^2 - 6f_s^4 f_t^3 f_{a,a} a f_r f_a^4 - 12f_b f_s^6 f_{a,a} s f_{a,t} f_r^2 - 12f_b^3 f_s^5 f_{a,a} f_r^2 f_t \\ & - 144f_{a,a} b f_s^3 f_r^4 f_b^2 f_t^2 + 4f_{a,a} b f_s^5 f_r^6 f_t + 36f_{a,a} b f_s^5 f_r^3 f_b^2 f_t + 96f_b f_s^3 f_t^3 f_{a,a} f_r^3 + 32f_a^3 f_t^4 \\ & f_{a,r}^2 f_r^2 f_b^2 + 6f_b^4 f_s^4 f_r^2 f_{a,r} f_{r,t} - 2f_b^4 f_s^5 f_r^2 f_{a,s} f_{a,a} - 4f_b^7 f_r s f_r^4 f_{a,a} f_t - 128 \end{aligned} \quad (13)$$

$$\begin{aligned}
& f_b^3 f_s f_r^4 f_t^2 f_{r,t} + 6 f_s^6 f_t^2 f_{a,a} f_r f_a^2 - 8 f_a^7 f_t^4 f_{a,s} f_r f_b + 40 f_a f_r^3 f_r^2 f_t^2 f_b^4 + 24 f_a^5 f_r f_r^2 f_s^2 f_t^2 - 4 \\
& f_a^3 f_r f_r^2 f_s^4 f_b^2 + 12 f_a^2 f_r f_r^2 f_t^5 f_b + 192 f_b f_s^3 f_r^3 f_t^3 f_{a,a,r} - 12 f_b^3 f_a^5 f_r^2 f_{a,r,s} f_t^3 - 12 f_b^5 f_a^3 f_r^3 f_{a,r,s} \\
& f_t^2 + 192 f_b f_s^3 f_r^4 f_t^2 f_{a,a,t} - 4 f_b^7 f_a f_r^4 f_{a,r,s} f_t + 48 f_a^5 f_t^4 f_s f_r f_{r,s} + f_b^2 f_s^7 f_{a,s} f_a f_r + 256 f_b f_r, s \\
& f_r^3 f_t^4 f_{r,r} + 48 f_a^2 f_t^2 f_r f_s^5 f_{a,r,s} - 3 f_b^2 f_s^7 f_{a,a,s} f_r f_a - 192 f_b^3 f_s f_r^2 f_r^2 f_t^3 - 128 f_b f_s^2 f_{a,a,s} f_r^4 f_t^3 \\
& + 8 f_b f_s^6 f_{a,a,s} f_r^2 f_t - 3 f_b^3 f_s^6 f_{a,a,s} f_r f_a^2 + 24 f_a^5 f_s^2 f_{a,a,t} f_r^2 f_t^3 - 48 f_b^5 f_s f_s^5 f_t f_{a,a,t} + 256 \\
& f_t^3 f_{a,t} f_a f_r^5 f_b^2 + 384 f_t^4 f_{a,t} f_a f_r^4 f_a^2 - 384 f_t^3 f_{a,t} f_a f_r^4 f_s^2 + 32 f_t^2 f_{a,t} f_a f_r^5 f_b^4 + 96 f_b^3 f_s^3 \\
& f_r^4 f_t f_{a,a,t} - 32 f_b^3 f_s^3 f_r^3 f_t f_b^2 r - 8 f_t f_{a,t} f_a f_r^2 f_s^6 + 96 f_t^4 f_{a,t} f_a f_r^3 f_a^4 - f_b f_s^8 f_{a,b} f_a f_r - f_b^5 \\
& f_s^4 f_{a,b} f_a f_r^3 + 480 f_a^4 f_t^4 f_r^2 f_{a,t} f_{r,r} + 104 f_a^6 f_t^4 f_r f_{a,t} f_{r,r} + 896 f_a^2 f_t^4 f_r^3 f_{a,t} f_{r,r} + 2 f_b^3 \\
& f_s^6 f_{a,b} f_a f_r^2 + 32 f_a^2 f_b f_s^3 f_r^4 f_b^3 f_t + 192 f_t^4 f_{a,a,b} f_s f_r^4 f_a^2 + 48 f_t^4 f_{a,a,b} f_s f_r^3 f_a^4 + 4 f_{a,t} f_a f_{a,s} f_s^7 f_r \\
& + 24 f_a f_s^6 f_{a,a,t} f_r^2 f_t + 3 f_b^5 f_r^2 f_{a,a,s} f_s^4 f_a^2 + 6 f_b^4 f_r^2 f_{a,a,s} f_s^5 f_a - 3 f_b^6 f_r^3 f_{a,a,s} f_s^3 f_a + 12 f_b^5 \\
& f_r^4 f_{a,a,s} f_t^2 f_a^2 + 4 f_b f_r f_{a,t} f_a^5 f_s^5 f_t + 4 f_b f_s^7 f_a f_r, s f_b, r - 30 f_a f_r^3 f_b f_{a,a,t} f_s^4 + 10 f_a^3 f_r^2 f_b^4 f_{a,a,t} f_s^4 \\
& + 24 f_a^2 f_r^2 f_b^3 f_{a,a,t} f_s^5 - 18 f_a^2 f_r^3 f_b^5 f_{a,a,t} f_s^3 + 18 f_a f_r^2 f_b^2 f_{a,a,t} f_s^6 - 64 f_a^2 f_b f_s f_r^5 f_b^3 f_t^2 + 96 f_a^2 f_b \\
& f_s^3 f_r^4 f_b f_t^2 - 8 f_a^2 f_b f_s f_r^5 f_b^5 f_t - 24 f_a^2 f_b f_s^3 f_r^3 f_b f_t - 128 f_a^2 f_b f_s f_r^5 f_b f_t^3 + 256 f_a^2 f_t^4 f_r^3 f_{a,r,s} f_s \\
& - 768 f_t^4 f_{a,t} f_a^3 f_r^3 f_{a,r} - 192 f_t^4 f_{a,t} f_a^5 f_r^2 f_{a,r} + 24 f_a^2 f_{a,t} f_r^3 f_s^3 f_b^3 - 24 f_b^3 f_s^5 f_a^2 f_r f_{r,r,t} - 96 f_a^2 f_{a,t} \\
& f_a^3 f_r^3 f_t^2 f_s^2 - 24 f_b f_s^5 f_t^2 f_a^2 f_r^2 + 2 f_b f_s^7 f_t f_a^2 f_r - 128 f_b f_s f_t^4 f_a^2 f_r^4 - 3 f_{a,a,b} f_s^5 f_r^2 f_b^4 f_a^2 \\
& - 6 f_{a,a,b} f_s^6 f_r^2 f_b^3 f_a - 24 f_{a,a,b} f_s^3 f_r^4 f_b^4 f_t + 3 f_{a,a,b} f_s^4 f_r^3 f_b^5 f_a + 6 f_a f_t^3 f_{a,a,r} f_s^3 f_b - 4 \\
& f_s^7 f_{a,a} f_b f_r, r f_t - f_b^4 f_s^5 f_a f_{a,r} f_b, r + 2 f_a f_r, t f_b^2 f_r, r f_s^6 + 15 f_a^6 f_t^2 f_b^2 f_s^3 f_{a,r,s} - 4 f_s^7 f_a f_{a,b} f_r, r f_t \\
& + 24 f_a^3 f_t^2 f_b f_s^5 f_{a,r,r} + 8 f_a^6 f_t^3 f_s^2 f_r, t f_{a,r} - 2 f_b^3 f_s^6 f_{a,s} f_a^2 f_{a,r} + 15 f_a^5 f_t^2 f_b^2 f_s^3 f_{r,r,s} + 63 f_a^5 f_t^3 \\
& f_b^2 f_s^2 f_{a,r} - 24 f_t^3 f_a^3 f_{a,s} f_r, r - 13 f_a^6 f_t^3 f_s^2 f_b f_{r,r,s} + 12 f_b f_s^6 f_r, s f_r, r f_t - 8 f_a^3 f_t^2 f_s^5 f_{a,s} f_{a,r} + 7 \\
& f_a^6 f_t^2 f_s^3 f_r, s f_{a,t} + 2 f_b f_s^7 f_a f_{a,r} f_t + 4 f_s^6 f_t^2 f_{a,a} f_a^2 f_{a,r} - 2 f_a^4 f_t f_s^5 f_r, s f_{a,t} + 20 f_a^5 f_t^2 f_b^3 f_s^3 f_{a,r,r} \\
& + 16 f_b^3 f_s^5 f_{a,r} f_t^2 f_a^2 - 2 f_b^3 f_s^6 f_a f_{a,r} f_b, r - 52 f_a^6 f_t^4 f_a^2 f_r f_s f_b - 2 f_b f_s^7 f_a f_r, s f_{a,s} - 36 f_a^6 f_t^3 f_b^2 \\
& f_s^2 f_{a,r,r} + 27 f_a^5 f_t^2 f_b f_s^4 f_{a,r,s} + 2 f_a^4 f_r, t f_b^4 f_{a,r} f_s^4 + 48 f_b^2 f_s^4 f_t^2 f_{r,r} f_a^3 - 4 f_b^3 f_s^5 f_a f_r, s f_{a,s} - 6 \\
& f_a^6 f_s^4 f_b^2 f_{a,r,t} f_t + 6 f_a^7 f_s^3 f_b f_{a,r,t} f_t^2 + 2 f_s^5 f_a^4 f_b f_r f_t^2 f_{a,a} + f_b^5 f_s^4 f_a^3 f_r, s f_{a,r} - 5 f_b^2 f_s^6 f_a^2 f_r, s f_{a,s} \\
& + 4 f_a^6 f_t^4 f_{a,a} f_s^2 f_{a,r} + 2 f_b^4 f_s^5 f_r, s f_r, r f_a + 6 f_a^6 f_b f_s^3 f_r, r f_t^2 - 6 f_a^5 f_b^2 f_s^4 f_r, r, t f_t - 14 f_a^4 f_t^2 \\
& f_s^4 f_r, t f_{a,r} + 2 f_{a,t} f_a^8 f_r, t f_s^2 f_t^2 + 2 f_{a,t} f_a^6 f_r, t f_s^4 f_b^2 + 4 f_{a,t} f_a^5 f_r, t f_s^5 f_b - 4 f_{a,t} f_a^6 f_r, t f_s^4 f_t + 4 f_t^3 \\
& f_a^5 f_{a,b} f_s^3 f_r, r - f_s^3 f_a^6 f_b f_r f_t^3 f_{a,a} + 96 f_t^2 f_{a,t} f_a f_r^3 f_s^4 + 10 f_b^2 f_s^6 f_{a,t} f_r, r f_r - 4 f_b^2 f_s^6 f_{a,a} f_{a,t} f_r^2 \\
& - 192 f_b f_s^3 f_r^3 f_t^2 f_{r,r,t} + 12 f_a^5 f_t^3 f_{a,a,s} f_s^3 f_r - 8 f_b^6 f_s f_r^4 f_{a,t} f_{r,s} + 192 f_s^2 f_a^3 f_t^4 f_{r,r} f_r - 96 f_s^4 f_a \\
& f_t^3 f_{r,r} f_r - 128 f_b^3 f_b f_r f_t^4 f_{a,r} - 16 f_b^5 f_b f_r^4 f_t^2 f_{a,r} - 256 f_b f_b f_r^4 f_t^4 f_{a,r} + 32 f_t^3 f_a^3 f_{a,s} f_r^3 f_b^2 \\
& + 6 f_b^2 f_s^6 f_a^3 f_{a,r} f_t + f_b^3 f_s^4 f_a^5 f_r, s f_{a,t} + 8 f_b^2 f_s^6 f_a^2 f_r, t f_{a,r} - 2 f_b f_r f_{a,t} f_a^5 f_s^5 f_b^2 - 4 f_b f_r f_{a,t} f_a^4
\end{aligned}$$

$$\begin{aligned}
& f_s^6 f_b + 64 f_a^3 f_t^3 f_s^3 f_r, s f_r, r + 18 f_a, t f_a^2 f_b^3 f_a, r f_r f_s^5 + 7 f_a, t f_a f_b^2 f_a, r f_r f_s^6 - 448 f_a, t f_a f_b^2 f_a, r f_r^4 f_t^3 \\
& - 32 f_a, t f_a f_b^4 f_a, r f_r^4 f_t^2 - 224 f_a, t f_a^3 f_b^2 f_a, r f_r^3 f_t^3 + 5 f_a, t f_a f_b^6 f_a, r f_r^3 f_s^2 - 11 f_a, t f_a f_b^4 f_a, r f_r^2 f_s^4 \\
& - 128 f_b^2 f_s^3 f_r^3 f_t f_a, s f_r, t - 80 f_b f_s^4 f_r^2 f_t f_r, s f_r, t + 48 f_s^5 f_a, a f_b f_r, r f_r f_t^2 - 12 f_s^3 f_a, a f_b^5 f_r, r f_r^2 f_t \\
& + 80 f_b^3 f_s^2 f_r^3 f_t^2 f_r, s f_a, a + 12 f_s^5 f_a, a f_b^3 f_r, r f_r f_t - 256 f_b f_s^2 f_a, s f_r^3 f_t^3 f_a, r + 24 f_a^5 f_t f_b^3 f_s^3 f_r f_a, r, t \\
& - 16 f_b^5 f_s^3 f_r^2 f_a f_a, t f_r, r + 48 f_a, a, b f_s^4 f_r^2 f_t^2 f_b f_a^3 - 39 f_a^5 f_t^2 f_b^3 f_s^2 f_r f_a, r, s + 16 f_a^2 f_t^2 f_b^3 f_s f_r^3 f_b^2, r \\
& + 12 f_a^2 f_t f_b^3 f_s^3 f_r^2 f_b^2, r - 16 f_b^5 f_s f_r^4 f_a f_a, t f_r, t - 4 f_b^5 f_s f_r^3 f_a^3 f_a, t f_r, t - 32 f_b^3 f_s^3 f_r^3 f_t f_a, a f_r, t - 480 \\
& f_a^2 f_t^3 f_b^3 f_s f_r^3 f_a, a, r + 8 f_a^4 f_t f_b^3 f_s f_r^3 f_a^2, t + 12 f_a^2 f_t f_b^5 f_s f_r^3 f_r, r, t - 32 f_a^5 f_t^4 f_a, s f_s f_r f_a, r - 20 f_a f_t f_b^4 \\
& f_r^3 f_s^2 f_b^2, r + 16 f_b^4 f_s f_r^4 f_t^2 f_a, s f_a, a - 24 f_t^3 f_a^3 f_a, a f_r, r f_r^2 f_b^4 + 12 f_a, t f_a f_s^6 f_r f_t f_a, r + 48 f_b^4 f_s \\
& f_r^5 f_t f_a, t f_a, b - 80 f_b^4 f_s f_r^4 f_t f_a, t f_r, s + 256 f_b^3 f_s f_r^4 f_t^2 f_a, t f_a, r + 216 f_a^5 f_t^4 f_b f_s f_a, r, r f_r - 8 f_a^2 f_t^2 f_b^5 \\
& f_r^3 f_r, s f_a, a + 12 f_b^3 f_s^4 f_r^2 f_t f_a f_a, r, s + 48 f_s^5 f_a f_a, b f_r, r f_r f_t^2 - 192 f_s^3 f_a f_a, b f_r, r f_r^2 f_t^3 - 108 f_a^2 f_t^2 f_b \\
& f_s^5 f_a, a, r f_r - 16 f_a^5 f_t^4 f_s f_r f_b, r f_a, r - 32 f_a^3 f_t^3 f_b^3 f_r^3 f_a, s f_a, a - 32 f_a^4 f_t^3 f_b^2 f_r^2 f_r, s f_a, s + 9 f_b^3 f_s^4 \\
& f_a^4 f_a, t f_b, r f_r - 10 f_b^5 f_s^2 f_a^3 f_r^2 f_a, s f_r, t - 13 f_a, t f_a^2 f_b^5 f_a, r f_r^2 f_s^3 - 8 f_a, t f_a f_b^4 f_a, r f_r^3 f_t^2 + 11 f_a, t f_a^3 \\
& f_b^4 f_a, r f_r f_s^4 + 192 f_a^3 f_t^3 f_r^3 f_b f_a, t f_r, s + 9 f_b^5 f_s^2 f_r^3 f_a^2 f_a, s f_a, t + 8 f_a^4 f_t^2 f_b^3 f_r^3 f_a, b f_r, t + 24 f_a^4 f_t^3 f_b^3 \\
& f_r^2 f_a, b f_r, r - 8 f_a^4 f_t^2 f_b^3 f_r^3 f_a, s f_a, t - 8 f_a^4 f_t^2 f_b^3 f_r^3 f_a, t f_b, r + 4 f_a^5 f_t^3 f_b^2 f_r^2 f_r, s f_a, b + 16 f_a f_t f_b^5 \\
& f_r^4 f_a, t f_r, s + 64 f_a^3 f_t^2 f_b^3 f_r^3 f_a, t f_r, s - 36 f_a, a, b f_s^6 f_r^2 f_t f_b f_a - 192 f_r f_t^3 f_a, r, r f_s^3 f_b f_a^3 + 8 f_b^2 f_s^5 \\
& f_a^3 f_r f_a, b f_r, t - 16 f_s^3 f_a^4 f_b, r f_t^3 f_a, a f_r - 9 f_b^2 f_s^3 f_a^5 f_r f_a, b, r f_t^2 + 48 f_b^3 f_r^3 f_t^3 f_a, a, a f_a^3 f_s + 96 f_r^2 \\
& f_t^3 f_a, r, r f_b f_a^3 f_s^3 + 384 f_r^2 f_t^4 f_a, r, r f_b f_a^3 f_s - 5 f_b^4 f_s^4 f_a^3 f_a, a f_r f_r, t - 12 f_t^3 f_a^5 f_a, a, b f_s^2 f_r^2 f_b + 3 f_t^2 \\
& f_a^5 f_a, a, b f_s^4 f_r f_b - 3 f_t f_a^4 f_a, a, b f_s^5 f_r f_b^2 + 16 f_a^2 f_t^2 f_b^4 f_r^3 f_b, r f_r, s + 64 f_b^3 f_s^2 f_r^3 f_t f_r, s f_r, t + 24 f_a^6 \\
& f_t^4 f_a, r f_a, s f_b f_r - 16 f_b f_s^6 f_a, s f_r f_t f_a, r - 128 f_b^3 f_s^2 f_a, s f_r^3 f_t^2 f_a, r + 10 f_b^6 f_s^2 f_a^2 f_r^2 f_a, r f_r, t - 11 f_b^4 f_s^3 \\
& f_a^3 f_r^2 f_a, b f_r, t - 33 f_b^4 f_s^3 f_a^2 f_r^2 f_r, s f_a, t + 256 f_b f_a^3 f_r, s f_r^2 f_t^4 f_a, r + 32 f_b f_a^5 f_r, s f_r f_t^4 f_a, r \\
& + 512 f_b f_a f_r, s f_r^3 f_t^4 f_a, r - 2 f_a, b f_s^5 f_r f_b^4 f_a^2 f_a, r + 144 f_a, a, b f_s^4 f_r^3 f_t^2 f_b f_a - 6 f_a, a, b f_s^6 f_r f_b f_a^3 f_t \\
& + 10 f_a f_r^2 f_r, t f_b^6 f_r, r f_s^2 - 12 f_a f_r f_r, t f_b^4 f_r, r f_s^4 - 4 f_b^5 f_s^3 f_r^2 f_a f_r, s f_b, r - 8 f_b^5 f_a, s f_r^2 f_a^3 f_t^2 f_r, r \\
& - 80 f_b f_s^4 f_r, s f_r, r f_r f_t^2 + 12 f_b^5 f_s^2 f_r, s f_r, r f_r^2 f_t - 12 f_a^4 f_t^3 f_s^3 f_a, s f_a, a f_r + 24 f_b^2 f_s^4 f_r^2 f_t f_r, s f_b, r \\
& + 16 f_a^4 f_t^2 f_s^4 f_a, b f_b, r f_r + 64 f_a f_t^3 f_b^2 f_r^4 f_a, s f_b, r + 4 f_a^6 f_t^3 f_b f_r f_r, s f_r, t - 6 f_b^5 f_r^3 f_t f_a, a, a f_s^3 f_a \\
& + 24 f_b^5 f_r^4 f_t^2 f_a, a, a f_a f_s + 128 f_b f_s^4 f_a, s f_r^2 f_t^2 f_a, r - 12 f_b^2 f_s^5 f_a, s f_a, a f_r^2 f_t - 32 f_a f_t^2 f_b^4 f_r^4 f_a, a f_r, t \\
& + 4 f_s^3 f_a^5 f_a, b f_t^3 f_a, a f_r - 8 f_s^5 f_a^3 f_a, b f_t^2 f_a, a f_r + 512 f_a f_t^4 f_r^3 f_a, s f_s f_a, r - 512 f_a f_t^4 f_r^2 f_r, s f_s f_r, r \\
& + 192 f_b^3 f_s f_r^4 f_t^2 f_a f_a, r, t + 192 f_b f_s f_r^3 f_t^3 f_a^3 f_a, r, t - 56 f_b^2 f_s^4 f_r^2 f_t f_a, t f_r, r - 288 f_b f_s^3 f_r f_t^3 f_r, r, r f_a^2 \\
& - 112 f_a, t f_a f_s^4 f_r^2 f_t^2 f_a, r + 576 f_a, t f_a f_s^2 f_r^3 f_t^3 f_a, r - 8 f_b^2 f_a, b f_a, s f_r^3 f_t^3 f_a^4 + 8 f_a^6 f_t^4 f_a, s f_a, a f_s f_r \\
& - 96 f_a f_t^2 f_b^2 f_r^3 f_s^2 f_b^2, r - 64 f_b^2 f_a, b f_a, s f_r^4 f_t^3 f_a^2 + 192 f_b^3 f_r^4 f_t^3 f_a, a, a f_a f_s - 4 f_b^3 f_r^2 f_t^2 f_a, a, a f_s^3 f_a^3
\end{aligned}$$

$$\begin{aligned}
& -18f_b^2f_r^2f_t^3f_{a,a}f_s^2f_a^4 + 6f_b^4f_r^2f_tf_{a,a}af_s^4f_a^2 + 12f_b^3f_r^2f_tf_{a,a}af_s^5f_a + 36f_b^2f_r^2f_t^2f_{a,a}af_s^4f_a^2 \\
& -16f_b^4f_s^3f_a^3f_r^2f_{a,t}f_{b,r} - 32f_bf_s^5f_rf_tf_r{}_tf_r{}_r + 48f_b^3f_s^2f_r{}_sf_r{}_rf_r^2f_t^2 + 24f_b^4f_s^4f_rf_tf_r{}_rf_a \\
& + 288f_b^3f_s^2f_r^2f_t^3f_r{}_rf_a^2 + 32f_bf_s^5f_a{}_tf_r^2f_tf_a{}_r + 256f_af_t^3f_rf_s^3f_r{}_sf_r{}_r - 18f_a^5f_t^2f_b^2f_s^2f_rf_r{}_rf_t \\
& -16f_a^2f_t^3f_{a,a}f_b^4f_r^3f_a{}_r - 16f_b^4f_sf_b{}_rf_r^3f_r{}_rf_t^2 - 4f_b^6f_sf_b{}_rf_r^3f_r{}_rf_t + 64f_b^2f_sf_b{}_rf_r^3f_r{}_rf_t^3 \\
& -2f_b^5f_s^3f_a^2f_r^2f_b{}_rf_a{}_s - f_b^5f_s^4f_a^2f_rf_r{}_sf_a{}_a - 8f_b^4f_s^4f_a^2f_r^2f_{a,t}f_a{}_a + 24f_b^5f_s^2f_r^3f_af_b{}_rf_r{}_t - 9f_b^5 \\
& f_s^2f_r^2f_a^2f_r{}_sf_r{}_t - 16f_a^4f_t^2f_b^3f_s^3f_rf_a{}_a{}_r + 12f_a^5f_t^3f_s^2f_rf_r{}_sf_a{}_b + 12f_a^5f_t^3f_a{}_sf_b{}_rf_s^2f_r - 2 \\
& f_b^4f_a{}_bf_a{}_sf_r^2f_s^4f_a^2 + 8f_b^4f_a{}_bf_a{}_sf_r^4f_t^2f_s^2 + 64f_s^3f_a{}_bf_t^3f_a{}_af_r^2 - 128f_sf_a^3f_a{}_bf_t^4f_a{}_af_r^3 + 66 \\
& f_a^3f_t^2f_b^4f_s^2f_r^2f_{a,a}{}_r + 22f_a^4f_tf_b^4f_s^3f_rf_a{}_r{}_s - 18f_b^4f_r^3f_t^2f_{a,a}{}_af_a^2f_s^2 - 96f_b^3f_r^3f_t^2f_{a,a}{}_af_a^3f_s - 2 \\
& f_b^5f_s^4f_af_r^2f_{a,a}{}_f_b{}_r + 4f_a^2f_tf_b^5f_r^3f_r{}_sf_r{}_t - 4f_a^2f_tf_b^5f_r^4f_{a,t}f_b{}_r - 8f_bf_s^6f_rf_af_a{}_sf_r{}_t - 12f_b \\
& f_s^6f_a{}_bf_r{}_rf_r{}_f_t + 20f_bf_s^6f_af_r{}_sf_a{}_tf_r - 128f_r^3f_t^4f_a{}_r{}_rf_b{}_faf_s + 36f_rf_t^2f_a{}_r{}_rf_s^4f_b^2f_a^2 - 24f_r \\
& f_t^2f_a{}_r{}_rf_s^5f_b{}_f_a - 18f_b^4f_s^4f_a^2f_rf_a{}_rf_r{}_t + 6f_b^2f_s^5f_a^2f_rf_a{}_sf_r{}_t + 18f_b^4f_s^4f_a^2f_a{}_r{}_rf_r{}_f_t - 56f_a^4 \\
& f_t^4f_a{}_af_b^2f_r^2f_a{}_r + 64f_bf_s^2f_r{}_sf_r{}_rf_r^2f_t^3 - 28f_b^3f_s^4f_r{}_sf_r{}_rf_r{}_f_t - 64f_af_t^3f_b^3f_sf_r{}_f_a{}_r - 30f_b^3f_s^4f_a^2 \\
& f_r^2f_a{}_sf_a{}_t + 128f_a^3f_t^4f_r^2f_a{}_rf_a{}_sf_s - 512f_a^2f_t^4f_r^2f_a{}_sf_s{}_f_r + 30f_b^2f_s^5f_a^2f_r{}_sf_a{}_tf_r + 8f_b^4f_s^3 \\
& f_a^4f_rf_a{}_sf_r{}_t - 4f_a^6f_t^3f_bf_r^2f_a{}_sf_a{}_t + 96f_b^2f_a{}_bf_a{}_sf_r^4f_t^2f_s^2 - 256f_af_t^4f_r^4f_a{}_sf_a{}_af_b - 192f_a^3f_t^3 \\
& f_r^2f_sf_r{}_sf_r{}_t - 48f_s^5f_af_a{}_bf_t^2f_a{}_af_r^2 + 4f_s^7f_af_a{}_bf_tf_a{}_af_r - 256f_sf_af_a{}_bf_t^4f_a{}_af_r^4 + 192f_a^3f_t^3 \\
& f_r^3f_a{}_sf_a{}_tf_s - 48f_b^3f_s^4f_a^2f_r^2f_{a,b}{}_rf_t + 96f_b^3f_s^2f_a^2f_r^3f_{a,b}{}_rf_t^2 - 2f_b^3f_s^4f_a^4f_rf_a{}_b{}_rf_t + 64f_s \\
& f_a^2f_b{}_rf_t^4f_a{}_af_r^3 - 16f_a^3f_t^2f_r^2f_s^3f_{a,b}{}_f_r{}_t - 144f_a^2f_t^2f_r^2f_s^3f_a{}_sf_r{}_t + 208f_a^2f_t^2f_r^2f_s^3f_r{}_sf_a{}_t - 16 \\
& f_b^4f_a{}_bf_a{}_sf_r^4f_t^2f_a^2 - 32f_a^3f_a{}_af_s^2f_r{}_tf_r^2f_t^3 + 48f_af_a{}_af_s^4f_r{}_tf_r^2f_t^2 - 4f_a^5f_a{}_af_s^2f_r{}_tf_r^3f_t - 2f_b^5 \\
& f_s^4f_af_r^2f_a{}_sf_a{}_a + 192f_s^3f_af_a{}_bf_t^3f_a{}_af_r^3 - 16f_sf_a^5f_a{}_bf_t^4f_a{}_af_r^2 - 30f_a^3f_tf_b^4f_s^2f_r^2f_r{}_rf_t - 12 \\
& f_b^4f_sf_a^3f_r^3f_{a,b}{}_rf_t^2 + 12f_b^5f_s^2f_a^2f_r^3f_{a,b}{}_rf_t + 24f_b^3f_s^2f_a^4f_r^2f_{a,b}{}_rf_t^2 - 9f_b^4f_s^3f_a^3f_r^2f_{a,b}{}_rf_t \\
& + 256f_af_t^4f_r^3f_r{}_sf_a{}_af_s + 4f_b^5f_a{}_bf_a{}_sf_r^3f_s^3f_a - 48f_s^3f_b{}_rf_r{}_rf_r^2f_t^2f_b^2 - 4f_s^3f_b{}_rf_r{}_rf_r^2f_tf_b^4 \\
& + 12f_s^5f_b{}_rf_r{}_rf_r{}_f_t^2f_b^2 - 64f_a^2f_r^3f_r{}_tf_t^3f_b^3f_s - 48f_a^4f_r^2f_r{}_tf_t^2f_b^2f_s + 96f_a^3f_r^2f_r{}_tf_t^2f_b^2f_s^2 - 192f_a^2 \\
& f_r^3f_r{}_tf_t^2f_b^2f_s - 16f_t^4f_a^5f_a{}_bf_sf_rf_r{}_r + 144f_t^4f_a^4f_a{}_bf_sf_r^2f_a{}_r + 18f_b^2f_s^5f_a^3f_rf_a{}_b{}_rf_t + 24f_b^4 \\
& f_s^3f_af_r^3f_{a,b}{}_rf_t + 144f_b^2f_s^3f_af_r^3f_{a,b}{}_rf_t^2 - 4f_b^6f_sf_af_r^4f_{a,b}{}_rf_t - 12f_b^2f_sf_a^5f_r^2f_{a,b}{}_rf_t - 36f_b^2 \\
& f_s^5f_af_r^2f_{a,b}{}_rf_t - 64f_a^5f_t^4f_rf_a{}_sf_r{}_rf_b + 192f_a^4f_t^4f_r^2f_a{}_rf_a{}_sf_b - 24f_b^2f_a{}_bf_a{}_sf_r^3f_tf_s^4 + 64f_t^4 \\
& f_a^3f_a{}_bf_sf_r^2f_r{}_r + 36f_t^2f_a^2f_a{}_bf_sf_r{}_f_a{}_r + 32f_a^3f_t^3f_b^2f_r^3f_r{}_sf_a{}_b - 144f_t^3f_a^2f_a{}_bf_sf_r^3f_r{}_f_a{}_r - 12f_b^6 \\
& f_s^2f_r^2f_a^2f_a{}_r{}_rf_t - 36f_b^4f_s^3f_r^2f_af_r{}_sf_r{}_t - 64f_af_a{}_af_s^2f_r{}_tf_r^3f_t^3 - 6f_a^6f_t^3f_s^2f_a{}_tf_a{}_af_r + f_b^7f_s^2 \\
& f_r^2f_af_r{}_sf_a{}_r - 128f_a^2f_t^4f_r^3f_bf_r{}_sf_a{}_a - 12f_b^2f_s^5f_r^2f_tf_b{}_rf_a{}_a + 36f_a^3f_t^2f_b^5f_sf_r^2f_a{}_r{}_r - 27f_a^3f_t \\
& f_b^5f_s^2f_r^2f_a{}_r{}_s + 32f_af_t^2f_b^4f_r^4f_a{}_sf_b{}_r + 8f_a^3f_t^2f_b^4f_r^3f_r{}_sf_a{}_b - 8f_b^5f_s^3f_a^3f_rf_a{}_rf_r{}_t - 8f_a^3f_t^2f_b^4
\end{aligned}$$

$$\begin{aligned}
& f_r^3 f_a a f_{r,t} - 192 f_b^2 f_s f_a f_r^4 f_{a,b} r f_t^3 - 48 f_b^4 f_s f_a f_r^4 f_{a,b} r f_t^2 - 96 f_b^2 f_s f_a^3 f_r^3 f_{a,b} r f_t^3 + 4 f_s f_a^6 f_{b,r} \\
& f_t^4 f_a a f_r + 12 f_s^5 f_a^2 f_{b,r} f_t^2 f_a a f_r + 4 f_b^5 f_a^3 f_{r,s} f_a t f_r^3 f_t - 4 f_b^2 f_s^5 f_r f_t f_a s f_{r,r} + 15 f_b^4 f_s^4 f_a \\
& f_r^2 f_a a f_{r,t} + 6 f_b^2 f_s^6 f_a f_{a,a} r f_t f_r - f_b^2 f_s^6 f_a f_r f_{r,s} f_{a,b} - 27 f_b^5 f_r^2 f_{r,r} s f_t f_a^2 f_s^2 + 144 f_b^4 f_r^3 f_{r,r} s \\
& f_t^2 f_a f_s - f_b^2 f_s^6 f_a f_{a,s} f_{b,r} f_r - 96 f_a^5 f_t^3 f_b f_s^2 f_{a,r} s f_r - 48 f_a^4 f_t^3 f_r^3 f_b f_{a,s} f_{a,t} + 4 f_b f_a^7 f_{r,s} f_{a,t} f_r f_t^3 \\
& + 8 f_b^3 f_a^5 f_{r,s} f_{a,t} f_r^2 f_t^2 - 8 f_b^4 f_a^4 f_{a,s} f_{r,s} f_r^2 f_t^2 - 48 f_s^3 f_a^2 f_{b,r} f_t^3 f_a a f_r^2 + 32 f_s f_a^4 f_{b,r} f_t^4 f_a a f_r^2 \\
& - 64 f_a^2 f_t^2 f_r f_s^4 f_{r,s} f_{a,s} + 20 f_t^4 f_a^6 f_{a,b} f_s f_r f_{a,r} - 48 f_b f_{b,r} f_{a,t} f_r^3 f_t f_s^4 + 24 f_a^4 f_t^2 f_b^2 f_s^3 f_{a,r} s f_r \\
& - 6 f_a^2 f_t f_b^5 f_s^3 f_r^2 f_{a,a} r + 60 f_a^5 f_t^3 f_b^3 f_s f_r f_{a,r} r - 60 f_a^2 f_t^2 f_b^5 f_s^3 f_{a,a} r + 96 f_a^3 f_t^2 f_b^3 f_s f_r^3 f_{a,r} t \\
& - 108 f_a^4 f_t^3 f_b^3 f_s f_r^2 f_{a,a} r - 64 f_a^2 f_t^2 f_b^3 f_r^4 f_{a,t} f_{b,r} - 16 f_b^5 f_s^2 f_{a,s} f_r^3 f_t f_{a,r} + 320 f_b^3 f_a f_{r,s} f_{a,r} f_r^3 \\
& f_t^3 + 64 f_b^5 f_a f_{r,s} f_{a,r} f_r^3 f_t^2 + 384 f_a^2 f_t^3 f_b^2 f_r^3 f_{a,r} s f_s - 128 f_a^3 f_t^4 f_r^2 f_{a,s} f_{r,r} f_b - 192 f_a f_t^3 \\
& f_r^2 f_{r,s} f_{a,a} f_s^3 + 48 f_b^3 f_r^2 f_s f_{r,s} f_t^2 f_a^2 + 144 f_b^2 f_r^2 f_s^2 f_{r,s} f_t^2 f_a + 16 f_a^3 f_{a,a} f_s^4 f_{r,t} f_r f_t^2 + 36 f_b^3 f_s^3 f_{a,s} \\
& f_r^2 f_t f_a^2 + f_b^4 f_s^4 f_a f_r f_{a,b} f_{r,s} - 2 f_b^2 f_s^7 f_a f_{a,b} f_{a,a} f_r + 192 f_a f_r^3 f_{r,t} f_t f_b^2 f_s^2 - 12 f_b^4 f_s^3 f_r^2 f_t f_a^2 f_{a,r} s \\
& + 96 f_b^3 f_a^3 f_{r,s} f_{a,r} r f_t^2 f_t^3 + 4 f_b^7 f_a f_{r,s} f_{a,r} f_r^3 f_t + 4 f_b^3 f_a^5 f_{r,s} f_{a,r} f_r f_t^3 + 4 f_b f_s^6 f_{r,s} f_{a,a} f_r f_t - f_b^6 f_s^3 \\
& f_r^2 f_a f_{a,r} f_{b,r} + 32 f_b^3 f_s^4 f_{a,s} f_r^2 f_t f_{a,r} + 4 f_a^7 f_t^3 f_{a,t} f_{b,r} f_s f_r + 2 f_b^5 f_a^4 f_{a,b} f_{r,r} f_r + 12 f_{a,a} b f_s f_r^4 \\
& f_b^4 f_t^2 f_a^2 - 12 f_{a,b} f_s^3 f_r^3 f_b^4 f_t f_{a,r} - 60 f_t^3 f_a^4 f_{a,b} f_s^3 f_r f_{a,r} + 32 f_b^5 f_s f_r^4 f_{a,t} f_t f_{a,r} + 16 f_b^6 \\
& f_r^3 f_{r,r} s f_t f_a f_s + 36 f_b^4 f_r^2 f_{r,r} s f_t^2 f_a f_s - 39 f_b^3 f_r f_{r,r} s f_s^2 f_a f_t^2 + 22 f_b^4 f_r f_{r,r} s f_s^3 f_a f_t + 192 f_t^4 \\
& f_a^2 f_{a,b} f_s f_r^3 f_{a,r} + 84 f_t^3 f_{a,t} f_s^5 f_r^2 f_{a,r} + 4 f_b^4 f_s^3 f_r^3 f_t f_{a,s} f_{a,a} + 30 f_a^3 f_t f_b^3 f_s^4 f_{a,r} s f_r + 64 \\
& f_b^3 f_{b,r} f_{a,t} f_r^4 f_t f_s^2 + 9 f_{a,a} b f_s^3 f_r^3 f_b^4 f_t f_a^2 + 48 f_{a,a} b f_s^4 f_r^3 f_b^3 f_t f_a - 96 f_{a,a} b f_s^2 f_r^4 f_b^3 f_t^2 f_a \\
& + 2 f_{a,a} b f_s^4 f_r^2 f_b^3 f_a^3 f_t - 208 f_a^4 f_t^4 f_r f_{a,s} f_s f_{r,r} - 16 f_b f_s^5 f_r^2 f_a f_{a,t} f_{r,t} + 48 f_b f_s^5 f_r^2 f_a f_t f_{a,r} t \\
& + 12 f_b f_s^5 f_r f_a^3 f_{a,t} f_{r,t} - 48 f_a^5 f_t^3 f_s f_r f_{r,s} f_{r,t} - 24 f_b f_s f_a^2 s f_r^2 f_t^3 f_a^4 + 16 f_t^3 f_{a,t} f_a^6 f_{r,r} f_r f_b^2 - 4 \\
& f_a^6 f_t^3 f_b f_r^2 f_{a,t} f_{b,r} - 12 f_{a,a} b f_s^2 f_r^4 f_b^5 f_t f_a - 24 f_{a,a} b f_s^2 f_r^3 f_b^3 f_t^2 f_a^3 + 14 f_b^5 f_s^3 f_r^2 f_a f_{a,r} f_{r,t} - 6 f_b^5 \\
& f_s^3 f_r^2 f_a f_{a,r} r f_t + 4 f_b^6 f_s f_r^3 f_a^2 f_{a,s} f_{r,t} - 40 f_t f_{a,t} f_{a,a} f_r^4 f_s^2 f_b^4 + 48 f_t f_{a,t} f_{a,a} f_r^3 f_s^4 f_b^2 + 48 f_a^4 f_t^3 \\
& f_r^2 f_{r,r} t f_b f_s - 144 f_a^3 f_t^2 f_r^2 f_{r,r} t f_b^2 f_s^2 - 12 f_b^3 f_a^4 f_{r,s} f_t^3 f_{r,r} f_r - 960 f_b f_s f_r^3 f_t^4 f_a^2 f_{a,a} r - 40 f_a^4 f_t^3 \\
& f_r^2 f_b^2 f_{a,r} f_{r,t} - 256 f_a^3 f_t^4 f_r^3 f_{a,b} f_{a,r} f_b + 48 f_a^4 f_t^3 f_r^2 f_s f_{a,s} f_{r,t} - 20 f_a^3 f_t^2 f_b^3 f_s^3 f_{a,r} r f_r - 24 f_a^4 f_r \\
& f_{r,t} f_s^3 f_b f_t + 9 f_{a,a} b f_s^3 f_r^2 f_b^2 f_a^2 f_t^2 - 18 f_{a,a} b f_s^5 f_r^2 f_b^2 f_a^2 f_t + 24 f_b^3 f_s^4 f_a f_r^3 f_{a,t} f_{a,b} + 240 f_a^3 f_t^3 \\
& f_b^3 f_s f_r^2 f_{a,r} r - 4 f_b^6 f_s f_r^4 f_a f_{a,s} f_{a,t} - 24 f_b^5 f_s^2 f_r^4 f_a f_{a,b} f_{a,t} + 192 f_b f_{b,r} f_{a,t} f_r^4 f_t^2 f_s^2 - 120 f_a f_t \\
& f_r^3 f_{r,r} t f_s^2 f_b^4 + 12 f_a^3 f_t f_r f_{r,r} t f_s^4 f_b^2 - 36 f_a^2 f_t f_r f_{r,r} t f_s^5 f_b + 144 f_a f_t f_r^2 f_{r,r} t f_s^4 f_b^2 - 288 f_a f_t^2 \\
& f_r^3 f_{r,r} t f_b^2 f_s^2 + 96 f_a^2 f_t^2 f_r^3 f_{r,r} t f_b^3 f_s + 72 f_a^2 f_t f_r^2 f_{r,r} t f_s^3 f_b^3 + 36 f_a^4 f_t^2 f_r f_{r,r} t f_s^3 f_b + 8 f_t^2 f_{a,t} \\
& f_a^4 f_{r,r} f_r^2 f_b^4 - 64 f_b f_s^2 f_r^4 f_t^2 f_{a,s} f_{a,t} + 48 f_b f_s^4 f_r^2 f_t^2 f_{a,b} f_{r,r} + 96 f_{a,a} b f_s f_r^4 f_b^2 f_t^3 f_a^2 + 12 f_{a,a} b f_s \\
& f_r^3 f_b^2 f_t^3 f_a^4 + 48 f_a^2 f_t^2 f_r^2 f_s^4 f_{a,b} f_{b,r} - 48 f_b f_s^4 f_r^2 f_t^2 f_{r,s} f_{a,a} + 24 f_b f_r f_s f_{r,s} f_t^3 f_a^4 - 96 f_b f_r f_s^3 f_{r,s}^2
\end{aligned}$$



$$\begin{aligned}
& f_t^2 f_a^2 + 24 f_b^4 f_r^2 f_s^2 f_{r,s} f_t f_a - 36 f_b^3 f_r f_s^3 f_{r,s}^2 f_t f_a^2 - 12 f_b^2 f_r f_s^4 f_{r,s}^2 f_t f_a - 64 f_b^2 f_s f_r^4 f_t^3 f_{b,r} f_{a,a} \\
& - 64 f_a f_t^3 f_r^4 f_b^2 f_{a,a} f_{r,t} - 16 f_a f_t^2 f_b^5 f_r^4 f_{a,s} f_{a,a} + 8 f_a^3 f_t^2 f_b^4 f_r^3 f_{a,s} f_{b,r} - 48 f_b f_a^4 f_{r,s} f_t^4 f_{r,r} f_r \\
& + 26 f_b f_s^3 f_{a,s}^2 f_r f_a^4 f_t^2 + 384 f_a^2 f_t^4 f_r^3 f_{a,r} f_{a,s} f_b - 48 f_a^4 f_t^3 f_r^3 f_{b,a} f_{t,b,r} + 96 f_b f_s^2 f_{a,a} s f_r^2 f_t^3 f_a^4 \\
& + 48 f_b^2 f_s^3 f_r^3 f_t^2 f_{a,a} f_{b,r} - 16 f_b^3 f_{a,s} f_r f_a^5 f_t^3 f_{r,r} - 64 f_b^3 f_{a,s} f_r^2 f_a^3 f_t^3 f_{r,r} + 64 f_s f_a^3 f_{b,r} f_r^2 f_t^4 f_{a,r} \\
& + 12 f_b^2 f_s^4 f_{a,s}^2 f_r^2 f_t f_a - 144 f_b^2 f_s^2 f_{a,s}^2 f_r^3 f_t^2 f_a - 22 f_b^2 f_s^4 f_{a,s}^2 f_r f_a^3 f_t - 12 f_a f_{a,a} f_s^6 f_{r,t} f_r f_t - 24 \\
& f_b^4 f_s^2 f_{a,s}^2 f_r^3 f_t f_a + 8 f_b^5 f_a^3 f_{r,s} f_{a,r} f_r^2 f_t^2 - 10 f_b^3 f_s^5 f_a^2 f_{a,a} f_r f_{r,t} - 64 f_b^2 f_s f_r^4 f_t^3 f_{a,s} f_{a,a} - 192 \\
& f_s^3 f_a f_{b,r} f_r^2 f_t^3 f_{a,r} - 256 f_a f_t^3 f_r^2 f_{a,s} f_s^3 f_{a,r} - 12 f_a^2 f_t f_s^6 f_{a,b} f_{b,r} f_r - 64 f_a f_t^3 f_r^3 f_s^2 f_{r,s} f_{a,b} \\
& - 64 f_a f_t^3 f_r^3 f_{a,s} f_{b,r} f_s^2 + 144 f_b f_s^2 f_{a,a} s f_r^3 f_t^3 f_a^2 + 32 f_b^3 f_s^3 f_r^3 f_{a,a} f_{t,r,t} - 24 f_b^3 f_s^3 f_r^2 f_a^3 f_{a,t} f_{r,t} \\
& - 48 f_a^2 f_t^3 f_{a,r}^2 f_b^3 f_s - 216 f_a^4 f_t^4 f_{a,r} f_r f_b f_s + 144 f_a^3 f_t^3 f_{a,r} f_r^2 f_b^2 f_s - 54 f_b^4 f_s^2 f_r^2 f_t^2 f_{a,r,r} \\
& + 32 f_b^5 f_s^4 f_t f_{a,a} f_{r,t} + 32 f_b^4 f_s^2 f_r^3 f_t f_{a,t} f_{r,r} + 24 f_b^3 f_s^5 f_{a,a} f_{t,r} f_r - 6 f_b^2 f_s^6 f_a^2 f_{a,b} f_{b,r} f_r - 18 \\
& f_b^3 f_s^4 f_a^2 f_r^2 f_{a,b} f_{r,t} - 24 f_b f_s^5 f_{a,s}^2 f_r f_a^2 f_t + 96 f_b f_s^3 f_{a,s}^2 f_r^2 f_t^2 f_a^2 - 48 f_b^3 f_s f_{a,s}^3 f_t^2 f_a^2 + 48 f_a^5 \\
& f_t^3 f_{a,s} f_{a,t} f_s f_r^2 - 32 f_t^2 f_a f_r f_{r,t} f_{r,r} f_s^4 - 12 f_a^2 f_t f_b f_s^5 f_r f_b^2 f_r + 576 f_a^2 f_t^3 f_b f_s^3 f_{a,a} f_r^2 f_r + 6 \\
& f_s^4 f_{a,b} f_{a,s} f_r f_a^4 f_t^2 - 2 f_s^6 f_{a,b} f_{a,s} f_r f_b^2 f_a^2 - 4 f_s^7 f_{a,b} f_{a,s} f_r f_b f_a - 24 f_s^2 f_{a,b} f_{a,s} f_r^2 f_t^3 f_a^4 + 192 f_a^3 \\
& f_t^3 f_b^2 f_r^2 f_s f_{r,s} - 8 f_a^5 f_t^2 f_s^3 f_r f_{a,b} f_{r,t} + 2 f_b^5 f_{a,s} f_{a,r} f_r f_s^4 f_a^2 - f_b^6 f_{a,s} f_{a,r} f_r^2 f_s^3 f_a - 64 f_t^3 \\
& f_a^3 f_r f_{r,t} f_r f_s^2 - 12 f_t^4 f_a^5 f_{a,a} f_{r,r} f_r f_b^2 + 48 f_b^3 f_{a,s} f_{a,r} f_r^2 f_t^3 f_a^4 + 96 f_s^2 f_a^2 f_{b,r} f_r^4 f_t^2 f_b^2 + 192 f_a^2 f_t^3 \\
& f_r^3 f_{r,r} f_t f_b f_s + 192 f_a^2 f_t^3 f_r^3 f_{b,r} f_{s,r,t} + 72 f_s^2 f_t^2 f_{a,r} f_r f_r^2 f_b^4 - 72 f_s^4 f_t^2 f_{a,r} f_r f_r f_b^2 - 12 f_b^5 f_a^2 \\
& f_{a,s} f_r^3 f_t f_s + 20 f_s^2 f_a^2 f_{b,r} f_t f_b^4 - 48 f_s^4 f_a^2 f_{b,r} f_t f_b^2 + 24 f_a^5 f_t^3 f_s f_b^2 f_r f_{r,s} + 256 f_a^2 f_t^3 f_r \\
& f_s^3 f_{a,s} f_{r,r} + 24 f_b^5 f_{a,s} f_{a,r} f_r^3 f_t^2 f_a^2 + 192 f_b^3 f_{a,s} f_{a,r} f_r^3 f_t^3 f_a^2 + 128 f_t^3 f_a^3 f_r^2 f_{r,t} f_r f_b^2 - 144 f_b f_s^2 \\
& f_r^2 f_t^3 f_a^3 f_{a,r,s} - 32 f_b^2 f_s^2 f_r^3 f_t^2 f_{a,t} f_{r,r} - 12 f_a f_t f_s^6 f_r f_{r,s} f_{a,b} - 12 f_a f_t f_s^6 f_{a,s} f_{b,r} f_r - 24 f_a^5 \\
& f_t^3 f_{a,a} s f_s f_r^2 f_b^2 + 48 f_s^5 f_a f_{b,r} f_r f_t^2 f_{a,r} - 32 f_s^3 f_a^3 f_{b,r} f_r f_t^3 f_{a,r} - 256 f_s^2 f_t^4 f_{a,r} f_r f_r f_a^2 - 12 \\
& f_s^4 f_t f_{a,r} f_r f_r f_b^4 f_r + 96 f_a^4 f_t^4 f_r^2 f_{a,b} f_{r,r} f_b + 32 f_a^3 f_t^3 f_s^3 f_r f_{r,s} f_{r,t} + 128 f_a^3 f_t^4 f_r^2 f_{r,s} f_{a,a} f_s + 12 \\
& f_b^5 f_s f_r^2 f_a^2 f_t f_{r,s} + 16 f_a f_t f_s^5 f_r f_{r,s} f_{r,t} - 16 f_a f_t f_s^5 f_{a,s} f_{a,t} f_r^2 - 12 f_b^5 f_s f_r^2 f_a^2 f_{a,r} f_t^2 + 15 f_b \\
& f_s^6 f_{a,a} s f_r f_a^2 f_t - 18 f_b^4 f_s^4 f_{a,r} f_r f_t f_a - 96 f_a^4 f_t^3 f_r f_{a,t} f_{r,r} f_s^2 + 152 f_a^4 f_t^3 f_r^2 f_{a,t} f_{r,r} f_b^2 + 192 f_a^3 f_t^3 \\
& f_r^3 f_{a,t} f_{b,r} f_s + 256 f_a f_t^3 f_r^4 f_b f_{a,t} f_{r,s} - 6 f_a^2 f_t f_s^6 f_{a,t} f_{a,a} f_r - 6 f_b^3 f_s^4 f_a^2 f_r^2 f_{a,t} f_{b,r} + 4 f_b^6 f_s \\
& f_r^4 f_{a,s} f_{a,a} f_t - 2 f_b^4 f_s^5 f_a f_{r,s} f_{a,a} f_r + 28 f_a^3 f_t f_s^5 f_{a,t} f_{b,r} f_r - 192 f_a^2 f_t^3 f_r^2 f_r f_b^3 f_s + 96 f_b^3 f_s^2 f_a \\
& f_r^3 f_{b,r} f_r f_t^2 + 80 f_b^4 f_s f_r^4 f_t f_{a,s} f_{r,t} - 64 f_b^3 f_s^2 f_r^4 f_t f_{a,s} f_{a,t} + 16 f_b^3 f_s^4 f_r^2 f_t f_{a,b} f_{r,r} + 64 f_a^2 f_t^3 f_b^2 \\
& f_r^3 f_{b,r} f_{r,s} + 2 f_b^6 f_s^3 f_r^2 f_{r,s} f_{a,a} f_a + f_{a,b} f_s^4 f_r^2 f_b^5 f_a f_{a,r} - 384 f_a^2 f_t^4 f_{r,r} f_r f_b f_s + 48 f_a^2 f_r^2 f_s^2 f_b^4 f_r \\
& - 120 f_a^2 f_s^2 f_{a,r} f_t f_r^3 f_t f_b^4 + 32 f_t^2 f_a^3 f_r^3 f_{r,t} f_r f_b^4 + 4 f_b^4 f_s^3 f_r^2 f_t f_{a,s} f_{r,r} + 14 f_{a,t} f_s^2 f_s^4 f_{r,r} f_b^4 f_r \\
& - 32 f_a^3 f_t^2 f_s^3 f_{a,s} f_{a,t} f_r^2 - 36 f_a^4 f_s^3 f_{a,a} f_{t,r}^2 f_t^2 f_b + 36 f_a^2 f_s^5 f_{a,a} f_{t,r}^2 f_t f_b + 128 f_a f_t^2 f_b^3 f_r^4 f_{a,t} f_{r,s}
\end{aligned}$$

$$\begin{aligned}
& -64f_a^2f_t^3f_b^3f_r^3f_{r,s}f_{a,a} + 288f_s^2f_t^3f_a,r f_r,r f_r^2f_b^2 - 192f_a f_r^3f_a,t f_s^3f_b,r f_t^2 + 48f_a f_r^2f_a,t f_s^5f_b,r f_t \\
& + 256f_a f_r^4f_a,t f_s f_b,r f_t^3 - 64f_b^3f_s^3f_r^3f_t f_a,r f_{a,t} - 384f_a f_t^3f_b^2f_r^4f_{a,a} f_s - 8f_b^3f_s^3f_a^5f_r f_{a,t} f_r,t \\
& + 68f_a^4f_t^2f_s^3f_r,s f_{a,t} f_r - 36f_a^4f_t^2f_s^3f_r f_{a,s} f_{r,t} + 96f_a^4f_t^2f_s^2f_r^2f_{a,t} f_{r,t} + 24f_a^6f_t^2f_s^2f_r f_{a,t} f_{r,t} \\
& + 36f_a^4f_t^2f_b^4f_r^2f_{a,r} f_s f_s - 64f_a^2f_t f_s^4f_r^2f_{a,t} f_{r,t} - 32f_a^4f_t f_s^4f_r f_{a,t} f_{r,t} + 256f_s f_a f_b,r f_r^3f_t^4f_{a,r} \\
& + 8f_a^3f_r^2f_r,t f_b^4f_r,r f_t^2 + 80f_b^2f_s^3f_r^2f_t^2f_{a,s} f_{r,r} - 288f_a^2f_s^2f_{a,r} f_r^3f_t^2f_b^2 + 32f_a^3f_t^3f_b^2f_r^3f_{a,s} f_{b,r} \\
& - 128f_a^3f_t^4f_r^3f_{a,s} f_{a,a} f_b + 48f_a^4f_t^3f_r^3f_b f_{a,b} f_{r,t} - f_b^3f_s^6f_a^2f_{a,b} f_{a,a} f_r + 16f_b f_b,r f_r^2f_t^4f_{a,r} f_a^4 \\
& - 48f_b f_b,r f_r^2f_t^2f_{a,r} f_s^4 + 64f_b^3f_b,r f_r^3f_t^2f_{a,r} f_s^2 + 4f_b f_b,r f_r f_t f_{a,r} f_s^6 - 16f_b^3f_s^5f_a f_r f_{a,r} f_{r,t} + 6 \\
& f_b^4f_s^4f_r f_r,s f_a^2f_{a,s} + 8f_{a,b} f_s f_r^4f_b^6f_t f_{a,r} - 16f_b^3f_a^4f_{a,s} f_r^2f_t^2f_s + 14f_b^4f_a^3f_{a,s} f_r^2f_t f_s^2 - 320f_b^3f_s \\
& f_r^3f_t^2f_r,t f_{r,r} - 6f_b^3f_a^4f_{a,s} f_r f_s^3f_t + 4f_a^7f_t^3f_s f_b f_r f_{a,r} f_{a,t} + 6f_b^2f_s^5f_a^3f_{a,s} f_{a,t} f_r + 256f_t^4 \\
& f_r^3f_s f_{a,a} f_b f_{r,r} + 16f_a^5f_t^4f_r,s f_{a,a} f_s f_r + 9f_b^2f_a^5f_{a,s} f_r f_s^2f_t^2 - 48f_s^4f_a^4f_{a,b} f_r f_t^2f_b + 36f_s^6 \\
& f_a^2f_{a,b} f_r f_r f_t f_b - 144f_s^4f_a^2f_{a,b} f_r f_t^2f_b + 448f_a^2f_t^3f_r^3f_{a,t} f_{r,r} f_b^2 + 2f_b^5f_s^4f_a f_{a,s} f_{r,r} f_r - 4f_b^3f_s^4 \\
& f_r^2f_t f_{r,s} f_{a,a} - 2f_b^5f_s^3f_r^2f_a^2f_{a,b} f_{r,s} + 384f_t^3f_{a,t} f_a^3f_s^2f_r^2f_{a,r} + 10f_b^6f_s^2f_r^3f_a f_{a,a} f_{r,t} - 6f_b^6f_s^2 \\
& f_r^3f_{a,r} f_{a,a} f_t + 10f_b^5f_s^3f_r^3f_{a,t} f_a f_{a,a} + 13f_b^5f_s^2f_r^3f_a^2f_{a,t} f_{b,r} - 108f_b f_s^4f_{a,a} f_r^2f_t^2f_a^2 - 27f_b \\
& f_s^4f_{a,a} f_s f_r f_a^4f_t^2 + 12f_a^4f_s^5f_{a,a} f_r f_b f_t - 24f_b^2f_s^3f_{a,a} f_s f_r^2f_t^2f_a^3 + 144f_b^2f_s^3f_{a,a} f_s f_r^3f_t^2f_a + 18 \\
& f_b^2f_s^5f_{a,a} f_s f_r f_a^3f_t - 11f_b^6f_s^2f_r^3f_{a,a} f_a f_{r,t} - 576f_r^3f_t^4f_{a,a} f_b^2f_a f_{r,r} - 144f_r^3f_t^3f_{a,a} f_b^4f_a f_{r,r} + 18 \\
& f_b^2f_s^5f_a^2f_r f_b,r f_t + 192f_s f_{r,t} f_a^2f_b,r f_r^3f_t^3 + 48f_s f_{r,t} f_a^4f_b,r f_r^2f_t^3 + 72f_t^2f_{a,t} f_{a,a} f_r^2f_s^4f_a^2 - 192 \\
& f_t^2f_{a,t} f_{a,a} f_r^4f_b^2f_s^2 - 288f_t^3f_{a,t} f_{a,a} f_r^3f_a^2f_s^2 + 128f_t^3f_{a,t} f_{a,a} f_r^4f_b^2f_a^2 - 96f_b^2f_s^2f_r^3f_t^2f_{r,s} f_{b,r} \\
& - 144f_t^3f_a f_{a,a} f_s^4f_r,r f_r - 48f_b f_s^4f_a^3f_r f_b,r r f_t^2 + f_b^6f_s^2f_r^3f_b,r f_a f_{a,s} + f_b^6f_s^2f_r^3f_a f_{a,b} f_{r,s} + 96 \\
& f_b^3f_s^3f_r^2f_t f_r,r f_{r,t} - 80f_t^2f_{a,t} f_a^3f_s^4f_r f_{a,r} - 48f_b^4f_s f_r^4f_t f_b,r f_{r,t} - 96f_b^3f_s^3f_r^3f_t f_a f_{a,r} f_{a,t} - 3f_b^4f_s^3 \\
& f_r^2f_a^2f_{a,s} f_{r,t} + 12f_b^5f_s^2f_a f_r^3f_b,r r f_t + 12f_b f_s^2f_a^5f_r f_b,r r f_t^3 + 36f_b f_s^6f_a f_r f_b,r r f_t - 48f_b^3f_s^4f_a \\
& f_r^2f_b,r r f_t + 4f_a^2f_t f_b^5f_r^4f_{a,b} f_{r,t} + 192f_b f_s^2f_r^3f_t^3f_{r,s} f_{a,a} - 288f_a^2f_t^3f_r^2f_{a,t} f_{r,r} f_s^2 + 56f_a^2f_t^2 \\
& f_r^3f_{a,t} f_{r,r} f_b^4 - 24f_a^2f_t^2f_r f_{a,t} f_{r,r} f_s^4 + 12f_b^4f_s^2f_{a,a} f_r^3f_t^2f_a + 2f_b^3f_s^5f_{a,a} f_r f_a^2f_t + 4f_b^3f_s^3f_{a,a} f_r^2 \\
& f_t^2f_a^2 - 64f_b f_b,r f_r^3f_t^4f_{a,r} f_a^2 - 9f_b^2f_s^3f_a^4f_r f_b,r r f_t^2 - 2f_b^3f_s^4f_a^3f_r f_b,r r f_t - 32f_a^4f_t^3f_s^2f_r^2f_b,r f_{a,b} \\
& + 64f_a^4f_t^3f_s^2f_{r,s} f_{a,s} f_r - 12f_b^3f_s^5f_a f_{a,a} f_{a,t} f_r^2 + 96f_b f_s^2f_a^3f_r^2f_b,r r f_t^3 - 144f_b f_s^4f_a f_r^2f_b,r r f_t^2 \\
& + 192f_b f_b,r f_r^3f_t^3f_{a,r} f_s^2 + 4f_b^5f_b,r f_r^3f_t f_{a,r} f_s^2 - 8f_b^3f_b,r f_r^2f_t f_{a,r} f_s^4 - 24f_a^4f_r^2f_b^3f_{a,a} f_t f_s^3f_t \\
& - 192f_b f_s f_r^4f_t^3f_a^2f_{a,t} + 72f_t^2f_{a,a} f_a f_{r,r} f_s^4f_b^2 - 2f_b^4f_s^3f_a^4f_r f_{r,s} f_{a,t} + 108f_a^3f_t^2f_b f_s^4f_{a,r} f_s f_r \\
& + 48f_b^5f_s f_r^4f_t f_a f_{a,r} f_{a,t} + 18f_a^5f_r^2f_b^2f_{a,a} f_t f_s^2f_t^2 - 12f_a^3f_r^2f_b^2f_{a,a} f_t f_s^4f_t - 24f_b^5f_s f_r^2f_r f_r f_t^2f_a^2 \\
& + 256f_b^2f_s f_{r,s} f_r^3f_{a,r} f_t^3 + 48f_a f_t^2f_r f_s^5f_{r,s} f_{a,a} + 7f_b^6f_s^2f_r^2f_a f_{a,r} f_t^2 + 8f_b^6f_s^2f_r^2f_r f_r f_t f_a + 4f_a^7 \\
& f_t^3f_{a,s} f_{a,t} f_s f_r + 12f_s^5f_b f_a^2f_{a,b} f_r^2f_t - 4f_a^4f_t^3f_b^3f_r^2f_{r,s} f_{a,a} + 4f_b^3f_s^5f_r f_a f_{r,s} f_{a,s} - 4f_a^6
\end{aligned}$$

$$\begin{aligned}
& f_t^3 f_a b f_a s f_s^2 f_r + 13 f_a^6 f_t^3 f_a a s f_s^2 f_b f_r + 64 f_b^3 f_s f_r^4 f_t^2 f_a a f_r t - 48 f_b^3 f_s f_a^2 a f_r^3 f_t^2 f_a^2 + 36 f_b^4 f_s^3 \\
& f_r^3 f_a f_a s f_a t + 32 f_a f_t^2 f_b^4 f_r^4 f_r s f_a b - 240 f_a^4 f_t^3 f_r^2 f_r s f_a t f_s - f_b^6 f_s^2 f_r^2 f_r s f_a^2 f_a s + 16 f_b^2 \\
& f_s^5 f_r s f_r f_a r f_t - 8 f_b^4 f_s^3 f_r s f_r^2 f_a r f_t + 384 f_a f_t^3 f_b^2 f_r^3 f_s f_r r s + 8 f_b f_a b f_r^2 f_t f_a a f_s^6 - 32 f_b^3 f_a b \\
& f_r^4 f_t^2 f_a a f_s^2 - 128 f_b f_a b f_r^4 f_t^3 f_a a f_s^2 - 8 f_b^3 f_a b f_r^3 f_t f_a a f_s^4 - 72 f_t^3 f_a t f_a a f_r^2 f_s^2 f_a^4 + 16 f_b^4 f_s^3 \\
& f_r^3 f_t f_a a f_b r - 192 f_a^2 f_t^3 f_r^4 f_b f_a t f_b r + 4 f_s f_r t f_a^6 f_b r f_r f_t^3 + 36 f_s^5 f_r t f_a^2 f_b r f_r f_t - 36 f_s^3 f_r t \\
& f_a^4 f_b r f_r f_t^2 + 14 f_s^4 f_r t f_a^3 f_b r f_r f_b^3 - 20 f_a^2 f_t f_s^5 f_r s f_a t f_r - 2 f_s^4 f_b^2 f_a^3 f_a b f_r^2 f_t + 24 f_s^2 f_b^2 f_a^3 f_a b \\
& f_r^3 f_t^2 + 36 f_a^2 f_t f_s^5 f_r f_a s f_r t + 4 f_a f_t f_s^6 f_a^2 a f_b^2 f_r + 576 f_t^4 f_a f_a a f_s^2 f_r r f_r^2 + 192 f_t^4 f_a^3 f_a a f_s^2 f_r r f_r \\
& - 8 f_s f_b f_a^4 f_a b f_r^3 f_t^3 - 64 f_s f_b f_a^2 f_a b f_r^4 f_t^3 + 192 f_r^3 f_t^4 f_a a a f_b f_a^3 f_s + 384 f_r^4 f_t^4 f_a a a f_b f_a f_s \\
& - 72 f_t^2 f_a a f_a r f_r^3 f_s^2 f_b^4 - 60 f_a f_t^2 f_a^2 r f_r f_s^4 f_b^2 + 96 f_a^2 f_t^3 f_a^2 r f_r f_b f_s^3 - 2 f_a b f_s^5 f_r f_b^4 f_a f_r r - 16 \\
& f_a^4 f_t^2 f_r^2 f_b f_r s f_a a - 8 f_a^3 f_t^2 f_a^2 a f_r f_s^4 f_b^2 + 24 f_b^3 f_s^2 f_a^3 f_r^2 f_b r r f_t^2 + 192 f_b f_s^2 f_a f_r^3 f_b r r f_t^3 \\
& + 192 f_b f_s^2 f_a^2 a b r f_r^3 f_t^3 + 6 f_b^6 f_s^2 f_a r f_r r f_r^2 f_t - 9 f_b^4 f_s^3 f_a^2 f_r^2 f_b r r f_t - 4 f_b^4 f_a^4 a f_r^2 f_t f_a \\
& - 128 f_b^2 f_s^3 f_r s f_r^2 f_a r f_t^2 - 288 f_t^3 f_a a f_a r f_r^3 f_b^2 f_s^2 + 192 f_t^4 f_a a f_a r f_r^2 f_a^2 f_s^2 - 128 f_t^4 f_a a f_a r \\
& f_r^3 f_b^2 f_a^2 + 128 f_a^2 f_t^2 f_r^3 f_s^2 f_a t f_r t + 64 f_a f_t^2 f_r^3 f_s^2 f_r s f_r t - 64 f_a f_t^2 f_r^3 f_s^3 f_a s f_a t - 16 f_s f_b^3 f_a^2 f_a b \\
& f_r^4 f_t^2 + 12 f_a^4 f_t^2 f_b^3 f_s f_r^2 f_r r t - 144 f_s^3 f_r t f_a^2 f_b r f_r^2 f_t^2 - 27 f_s^3 f_r t f_a^2 f_b r f_r^2 f_b^4 + 18 f_s^5 f_r t \\
& f_a^2 f_b r f_r f_b^2 - 8 f_b f_s^6 f_a f_a r s f_r f_t + 12 f_b^2 f_s^5 f_r^2 f_a f_a t f_b r + 88 f_t^4 f_a a f_a r f_r f_s^2 f_a^4 - 48 \\
& f_t^3 f_a a f_a r f_r f_s^4 f_a^2 + 16 f_a^5 f_r f_r t f_b^2 f_r r f_t^3 + 4 f_a^6 f_t^3 f_s f_b f_r f_r r t - 32 f_a^5 f_t^4 f_a b f_a r f_r^2 f_b - 256 f_b \\
& f_s^3 f_r^3 f_t^2 f_a r f_a t + 256 f_b^2 f_s f_r^4 f_t^2 f_a s f_r t + 256 f_b f_s f_r^4 f_t^3 f_a f_a r t + 192 f_a^2 f_t^3 f_r^4 f_b f_a b f_r t \\
& + 120 f_a f_r^4 f_b f_a a t f_t f_s^2 + 144 f_a^3 f_r^3 f_b^2 f_a a t f_t^2 f_s^2 + 36 f_a^2 f_t^2 f_b^5 f_s f_r^2 f_r r r + 256 f_t^3 f_a f_r^3 f_r t f_r r \\
& f_b^2 - 128 f_t^3 f_a f_r^2 f_r t f_r r f_s^2 - 12 f_a^2 f_r^4 f_b^5 f_a a t f_t f_s - 2 f_b^5 f_a^4 f_a f_r s f_a r f_r - 128 f_a^3 f_t^2 f_r^2 f_s^3 f_a t f_b r \\
& + 2 f_b^5 f_s^3 f_a^3 f_r f_r s f_a s - 14 f_b^5 f_s^3 f_a^2 f_r f_a r f_t + 2 f_a^3 f_t f_b^2 f_s^4 f_r f_b^2 r + 32 f_b^4 f_s f_r s f_r^3 f_a r f_t^2 - 12 f_a^4 \\
& f_r^3 f_b^3 f_a a t f_t^2 f_s + 30 f_a^3 f_r^3 f_b^4 f_a a t f_t f_s^2 - 72 f_a^2 f_r^3 f_b^3 f_a a t f_t f_s^3 - 96 f_a^2 f_r^4 f_b^3 f_a a t f_t^2 f_s + 8 f_a^3 f_t \\
& f_s^5 f_r f_a b f_r t - 192 f_r^2 f_t^4 f_a a f_b^2 f_a^3 f_r r - 2 f_a b f_s^6 f_r f_b^3 f_a f_a r - 4 f_t^3 f_a^6 f_a a t f_r^2 f_b f_s - 48 f_t^3 \\
& f_a^4 f_a a t f_r^3 f_b f_s - 6 f_t^2 f_a^6 f_a a t f_r f_s^3 f_b + 6 f_t f_a^5 f_a a t f_r f_s^4 f_b^2 + 64 f_b f_s^2 f_r^2 f_t^3 f_r s f_r t - 6 f_s^3 f_b f_a^4 \\
& f_a b f_r^2 f_t^2 - 16 f_a^5 f_t^4 f_a s f_a a f_r^2 f_b + 2 f_s^5 f_b f_a^4 f_a^2 b f_r f_t - 12 f_s^3 f_b^3 f_a^2 f_a b f_r^3 f_t + 48 f_a^5 f_t^3 f_b f_s \\
& f_r^2 f_a r t + 50 f_a^3 f_t^2 f_b^4 f_s^2 f_r f_a^2 r + 12 f_a^3 f_t f_b^5 f_s f_r^3 f_a r t - 2 f_b^3 f_s^5 f_a^3 f_t f_a a f_r + 4 f_b^6 f_a f_b r f_a s f_r^4 f_t \\
& - 256 f_a^3 f_t^4 f_r f_r s f_s f_r r + 240 f_b f_s f_r f_t^4 f_r r r f_a^4 + 144 f_a^2 f_t^2 f_b^4 f_r^3 f_a r s f_s - 32 f_a^2 f_t^2 f_b^4 f_r^3 f_a r f_r t \\
& - 256 f_a f_t^3 f_b^3 f_r^4 f_a b f_a r - 64 f_a^2 f_t^2 f_b^3 f_r^4 f_a s f_a t - 64 f_a^3 f_t^3 f_s f_r s f_a a f_r + 48 f_b^2 f_s^3 f_r^3 f_t^2 f_a s f_a a \\
& - 24 f_a f_t^2 f_a^2 a f_r^2 f_s^4 f_b^2 + 144 f_a f_t^3 f_a^2 r f_r^2 f_b^2 f_s^2 - 12 f_a^2 f_t^2 f_a^2 r f_r f_s^3 f_b^3 + 12 f_a^5 f_t^2 f_b^3 f_s f_r^2 f_a r t \\
& + 288 f_a f_r^4 f_b^2 f_a a t f_t^2 f_s^2 - 144 f_a f_r^3 f_b^2 f_a a t f_t f_s^4 + 48 f_a f_t^2 f_a^2 r f_r^2 f_s^2 f_b^4 - 4 f_a^6 f_t^3 f_s f_b f_a^2 s f_r
\end{aligned}$$

$$\begin{aligned}
& -4f_a^5 f_t^2 f_s^3 f_a s f_a t f_r - 48f_a t f_a^4 f_a b f_s f_r^3 f_t^3 + 144f_a t f_a^2 f_a b f_s^3 f_r^3 f_t^2 + 27f_a t f_a^2 f_a b f_s^3 f_r^3 f_b^4 \\
& - 18f_a t f_a^2 f_a b f_s^5 f_r^2 f_b^2 - 4f_a t f_a^6 f_a b f_s f_r^2 f_t^3 - 36f_a t f_a^2 f_a b f_s^5 f_r^2 f_t - 96f_t^3 f_a a b f_s^2 f_r^3 f_b f_a \\
& - 192f_t^3 f_a a b f_s^2 f_r^4 f_b f_a + 96f_a^2 f_t^3 f_a a f_r^2 f_b f_s^3 - 192f_a^2 f_t^4 f_a a f_r^3 f_b f_s + 10f_a^4 f_t^3 f_a a f_r f_s^3 f_b \\
& - 144f_b^2 f_s^3 f_r^2 f_t^2 f_a f_a r s - 192f_b f_s^3 f_r^3 f_t^2 f_a f_a r t - 512f_b f_s f_r^3 f_t^3 f_r t f_r r - 72f_b^4 f_s^2 f_r^2 \\
& f_t^2 f_r r r f_a - 144f_b^2 f_s^2 f_r f_t^3 f_r r r f_a^3 - 24f_b^3 f_s^3 f_r f_t^2 f_r r r f_a^2 + 72f_b^2 f_s^4 f_r f_t^2 f_r r r f_a + 576f_b f_s f_s^2 \\
& f_t^4 f_r r r f_a^2 - 2f_b f_s^7 f_a f_a b f_b r f_r - 12f_b^2 f_s^5 f_r^2 f_a f_a b f_r t - 192f_a b f_r^4 f_r t f_b f_t^2 f_s^2 + f_b^4 f_s^4 \\
& f_a^3 f_r f_b r f_a s + 256f_b f_s^3 f_r^2 f_t^2 f_r r f_r t - 4f_a f_t f_b^6 f_r^4 f_a a f_r t + 12f_a^2 f_t^2 f_b^5 f_r^3 f_a b f_r r - 2f_b^5 f_s^3 \\
& f_r^3 f_a f_a b f_b r - 4f_b^6 f_s f_r^4 f_a f_a b f_r t + 3f_a t f_a^6 f_a b f_s^3 f_r f_t^2 + 3f_a t f_a^4 f_a b f_s^5 f_r f_b^2 + 6f_a t f_a^3 f_a b \\
& f_s^6 f_r f_b - 6f_a t f_a^4 f_a b f_s^5 f_r f_t + 36f_a t f_a^4 f_a b f_s^3 f_r^2 f_t^2 - 14f_a t f_a^3 f_a b f_s^4 f_r^2 f_b^3 + 4f_r^3 f_s f_a a f_b^7 f_r r f_t \\
& + 48f_r^3 f_s f_a a f_b^5 f_r r f_t^2 + 32f_a^2 f_t^3 f_b^3 f_r^4 f_a b f_a a - 96f_s f_a^2 f_r^3 f_t^3 f_b r r f_b^2 - 12f_s f_a^2 f_r^3 f_t^2 f_b r r f_b^4 \\
& - 12f_s f_a^4 f_r^2 f_t^3 f_b r r f_b^2 + 4f_b^6 f_a f_a b f_r s f_r^4 f_t + 2f_b^3 f_s^5 f_a^3 f_a t f_a a f_r + 96f_a^2 f_t^3 f_a r f_r r f_r^2 f_b^4 \\
& + 12f_b^3 f_s^4 f_r f_a^3 f_r s f_a t - 4f_b^4 f_s^3 f_r^3 f_a f_a t f_b r - 12f_b^6 f_s^2 f_a f_r r r f_r^2 f_t - 8f_b^4 f_s^2 f_r^3 f_t f_r s f_b r + 10 \\
& f_b^2 f_s^5 f_a^3 f_a t f_b r f_r - 48f_b^4 f_s^2 f_a^3 f_r r r f_r f_t^2 + 12f_b^5 f_s^3 f_a^2 f_r r r f_r f_t + 24f_b^4 f_s^2 f_r^3 f_t^2 f_a f_a a r + f_b^3 f_s^4 \\
& f_a^4 f_a s f_a t f_r + 256f_a f_t^3 f_r^4 f_a s f_a t f_s - 256f_a f_t^3 f_r^3 f_s f_r s f_r t + 512f_b f_s f_r^4 f_t^3 f_a t f_a r - 2 \\
& f_b^6 f_r s f_r f_r r f_s^3 f_a + 144f_a^3 f_t^3 f_b^2 f_s^2 f_a a r f_r^2 + 9f_b f_s^6 f_a^2 f_a s f_a t f_r - 40f_a^4 f_t^4 f_a a f_r^2 f_b f_s + 24f_a^3 \\
& f_t^3 f_a a f_r^2 f_b^2 f_s^2 + 24f_a^2 f_t^4 f_r^2 f_s^3 f_b f_t + 2f_b f_s^7 f_a t f_a f_a a f_r - 4f_b^6 f_a^2 f_a s f_r s f_r^3 f_t + 192f_a^2 f_t^4 \\
& f_r^3 f_a b f_r r f_b + 128f_a^2 f_t^4 f_r^4 f_b f_a b f_a a - 64f_a^2 f_t^3 f_r^3 f_a b f_b r f_s^2 - 48f_s f_a^4 f_b r f_t^4 f_r r f_r - 18f_a^6 f_t^2 \\
& f_b^2 f_s^2 f_r f_a r t - 96f_s f_a^4 f_r s f_t^4 f_a r f_r - 8f_a^2 f_s^3 f_r t f_b^5 f_r r f_r + 64f_a^2 f_t^2 f_b^3 f_r^4 f_a b f_r t - 192f_a^2 f_a \\
& f_r^4 f_t f_b^2 f_s^2 + 4f_b^2 f_s^6 f_a^2 f_a t f_a a f_r + 2f_b^3 f_s^6 f_a f_a a f_b r f_r + 24f_b^5 f_s f_r^3 f_t^2 f_a f_a r r - 32f_b^3 f_s^2 f_r^3 \\
& f_t^2 f_a b f_r r + 152f_a^4 f_t^4 f_a r f_r r f_r f_b^2 + 24f_a^5 f_t^4 f_a a a f_r^2 f_b f_s - 6f_a^5 f_t^3 f_a a a f_r f_s^3 f_b + 6f_a^4 \\
& f_t^2 f_a a a f_r f_s^4 f_b^2 + 4f_a^6 f_t^3 f_s f_r f_a s f_r t + 24f_a^6 f_t^3 f_a r s f_s f_r f_b^2 - 52f_a^6 f_t^3 f_r s f_a t f_s f_r - 4f_a^5 f_t^3 f_b^2 \\
& f_r^2 f_a a f_r t + 48f_a b f_s f_r^4 f_b^4 f_t^2 f_a r + f_b^4 f_s^5 f_a^2 f_a a f_b r f_r + 30f_b^3 f_s^4 f_a^2 f_r f_r s f_r t - 64f_b^5 f_s \\
& f_r^3 f_t f_r t f_r r - 192f_a t f_a^2 f_a b f_s f_r^4 f_t^3 - 32f_b^4 f_s f_r^4 f_t^2 f_b r f_a a + 384f_a^2 f_t^4 f_a r f_r r f_r^2 f_b^2 - 2f_b^6 f_s^3 \\
& f_a^2 f_r f_r s f_a r + 18f_b^3 f_s^4 f_a^3 f_r f_a s f_r t - 432f_a^4 f_t^4 f_b f_s f_a a r f_r^2 + 192f_r^3 f_s f_a a f_b^3 f_r r f_t^3 - 8f_a^4 f_r^2 \\
& f_r t f_t f_b^3 f_s - 4f_a^6 f_r f_r^2 f_t^2 f_b f_s + 12f_a^5 f_r f_r t f_t f_b^2 f_s^2 + 2f_b^4 f_s^5 f_r^2 f_a f_a b f_a a + 16f_b^4 f_s^3 f_r^3 f_a f_a b f_r t \\
& + 32f_a f_t^2 f_r f_s^5 f_a s f_a r - 144f_a^3 f_t^2 f_b^3 f_s^2 f_r^2 f_a r s - 4f_a^3 f_t f_s^5 f_a s f_a t f_r - 6f_s^6 f_t f_a a f_b^2 f_r f_a r \\
& + 48f_a b f_r^3 f_r t f_b f_t f_s^4 - 64f_a b f_r^4 f_r t f_b^3 f_t f_s^2 - 48f_b^3 f_s^4 f_a f_r^2 f_a t f_r s + 48f_b^2 f_s^4 f_a f_r^2 f_t f_b^2 r - 6 \\
& f_s^7 f_t f_a a a f_r f_b f_a - 96f_s^3 f_t^3 f_a a a f_r^2 f_b f_a^3 + 72f_s^5 f_t^2 f_a a a f_r^2 f_b f_a - 288f_s^3 f_t^3 f_a a a f_r^3 f_b f_a + 12 \\
& f_s^5 f_t^2 f_a a a f_r f_b f_a^3 + 36f_b^2 f_s^5 f_a f_r f_r s f_r t + 144f_a^2 f_s^4 f_a r t f_r^2 f_t f_b^2 - 144f_a^4 f_s^2 f_a r t f_r^2 f_t^2 f_b^2 - 6
\end{aligned}$$

$$\begin{aligned}
& f_s^6 f_t f_{a,a} a f_r f_b^2 f_a^2 + 64 f_{a,t}^2 f_a^2 f_r^4 f_t f_b^3 f_s + 48 f_{a,t}^2 f_a^4 f_r^3 f_t^2 f_b f_s - 96 f_{a,t}^2 f_a^3 f_r^3 f_t f_b^2 f_s^2 + 192 f_{a,t}^2 f_a^2 \\
& f_r^4 f_t^2 f_b f_s - 4 f_b^6 f_s f_a s f_r r f_r^3 f_t + 120 f_a^2 f_t^2 f_b^3 f_s^3 f_{a,a} r f_r^2 + 128 f_b^2 f_s^3 f_r^3 f_t f_a t f_r s + 6 f_a^4 f_t^2 f_b \\
& f_s^3 f_r f_b^2 r + 8 f_a^4 f_t^3 f_b f_s f_r^2 f_b^2 r - 84 f_b^2 f_s^4 f_a^3 f_{a,a} r f_t^2 f_r - 32 f_t^3 f_a^3 f_{a,b} f_s^3 f_r f_r r - 48 f_s f_a s f_t^2 f_r r \\
& f_r^3 f_b^4 - 192 f_s f_a s f_t^3 f_r r f_r^3 f_b^2 - 18 f_b^4 f_s^4 f_a f_{a,a} r f_r^2 f_t - 32 f_a^2 f_t^2 f_b^4 f_r^3 f_r s f_a s + 4 f_b^6 f_s \\
& f_r^3 f_a f_r s f_r t - 2 f_b^5 f_s^3 f_r^2 f_a f_r s f_a s - 4 f_b^6 f_s f_r^4 f_t f_b r f_a a - 4 f_b^2 f_a^6 f_{a,s} f_r s f_r f_t^3 - 256 f_b^2 f_s^4 f_r \\
& f_t^2 f_a t f_r s - 64 f_a^2 f_t^3 f_b^2 f_r^3 f_r s f_a s + f_b^5 f_s^2 f_r^2 f_a^3 f_r s f_a t - 4 f_b^6 f_s f_r^4 f_a f_{a,t} f_b r + 2 f_b^3 \\
& f_s^6 f_a f_a s f_a a f_r + 40 f_b^4 f_s^2 f_a^2 f_r^3 f_{a,t} f_r t + 10 f_b^4 f_s^2 f_a^4 f_r^2 f_{a,t} f_r t + 12 f_s^2 f_a^6 f_t^3 f_{a,b} r f_r f_b + 96 f_a^2 f_t^3 \\
& f_b^3 f_r^3 f_{a,b} f_r r + 192 f_a^4 f_t^3 f_b^2 f_r^2 f_{a,r} s f_s + 156 f_a^4 f_t^3 f_b f_s^3 f_{a,a} r f_r - 12 f_a^2 f_t^2 f_a^2 a f_r f_s^5 f_b - 48 f_b^2 f_s^4 \\
& f_a^2 f_r^2 f_{a,t} f_r t + 24 f_b^3 f_s^4 f_a f_r^2 f_{a,s} f_r t - 4 f_b^2 f_s^4 f_a^4 f_r f_{a,t} f_r t - 36 f_b^2 f_s^5 f_a f_{a,s} f_{a,t} f_r^2 - 16 f_b^5 f_s^2 \\
& f_r^3 f_a f_{a,s} f_r t + 4 f_b^7 f_s f_r^3 f_a f_{a,r} r f_t - 4 f_b^5 f_s^2 f_r^3 f_{a,b} f_r r f_t + 28 f_b^5 f_s^2 f_r^3 f_a f_r s f_{a,t} - 4 f_b^7 f_s \\
& f_r^3 f_a f_{a,r} f_r t - 32 f_a^3 f_t^3 f_r^3 f_b^2 f_{a,a} f_r t + 24 f_b^2 f_r^3 f_s^3 f_r r s f_t^2 f_a^3 + 30 f_b^3 f_r f_s^4 f_r r s f_t f_a^2 - 144 f_b^2 f_r^2 \\
& f_s^3 f_r r s f_t^2 f_a - 144 f_b f_r^2 f_s^2 f_r r s f_t^3 f_a^2 - 96 f_b f_r f_s^2 f_r r s f_t^3 f_a^4 + 108 f_b f_r f_s^4 f_r r s f_t^2 f_a^2 - 144 f_b^3 \\
& f_r^2 f_s^2 f_r r s f_t^2 f_a^2 + 8 f_t f_r^3 f_{a,r} f_r t f_s^2 f_b^4 + 104 f_t^3 f_r f_{a,r} f_r t f_s^2 f_a^4 + 64 f_a^2 f_t^2 f_b^3 f_r^3 f_r s f_r t + 2 f_b^4 \\
& f_s^5 f_a s f_a f_r f_{a,r} + 72 f_a^3 f_s^3 f_{a,r} t f_r^2 f_t f_b^3 + 36 f_a^5 f_s^3 f_{a,r} t f_r f_t f_b^2 + 12 f_a^4 f_s^4 f_{a,r} t f_r f_t f_b^2 - 36 f_a^3 \\
& f_s^5 f_{a,r} t f_r f_t f_b - 288 f_b^2 f_s^2 f_r^3 f_t^3 f_a f_{a,a} r + 3 f_b f_s^6 f_r f_a^2 f_{a,b} f_r t + 16 f_a^4 f_r^2 s f_t^2 f_r f_b^3 f_s + 4 f_b^3 f_s^5 \\
& f_r^2 f_a f_{a,b} f_b r + 8 f_a^4 f_t^2 f_b^3 f_r^2 f_r s f_r t - 48 f_a^4 f_t^2 f_b^4 f_s^2 f_r f_{a,r} r - f_b^4 f_s^4 f_r^2 f_b r f_a f_{a,s} - f_b^4 f_s^4 \\
& f_r^2 f_a f_{a,b} f_r s - 192 f_s^3 f_{a,a} f_b f_r r f_r^2 f_t^3 - 30 f_a^4 f_t f_b^4 f_s^2 f_r^2 f_{a,r} t - 24 f_a^3 f_t^2 f_b^2 f_s^2 f_r^2 f_b^2 r + 12 \\
& f_s^4 f_t f_{a,a} f_b^4 f_r^2 f_{a,r} + 12 f_a^4 f_t^2 f_s^4 f_{a,t} f_{a,a} f_r + 8 f_t^2 f_{a,t} f_a^2 f_{a,a} f_r^4 f_b^4 + 16 f_t^3 f_{a,t} f_a^4 f_{a,a} f_r^3 f_b^2 + 54 f_a^5 \\
& f_t^3 f_{a,a} r f_s^2 f_r f_b^2 - 192 f_a^3 f_t^3 f_b^2 f_r^3 f_{a,a} s f_s - 2 f_a^3 f_t f_b^4 f_s^4 f_r f_{a,a} r - 128 f_a f_t^3 f_b^3 f_r^4 f_{a,s} f_{a,a} + 11 f_b^5 \\
& f_s^2 f_r^3 f_a^2 f_{a,b} f_r t + 5 f_b^4 f_s^4 f_a^2 f_r^2 f_{a,b} f_b r + 2 f_b^4 f_s^4 f_a^2 f_r f_r s f_b r + 6 f_b^4 f_s^3 f_a^3 f_r f_r s f_r t + 11 f_b^5 f_s^3 f_a^2 \\
& f_r^2 f_{a,a} f_r t + 2 f_b^5 f_s^4 f_a^2 f_r f_{a,r} f_b r - 6 f_b^4 f_s^3 f_a^3 f_r^2 f_{a,s} f_{a,t} - 5 f_b^2 f_s^6 f_{a,a} f_r f_a f_r t + 12 f_b^5 f_s^3 \\
& f_a^3 f_r f_{a,r} r f_t - 64 f_b f_s^2 f_r^3 f_t^3 f_{a,b} f_r r + 48 f_b^3 f_s^2 f_r^3 f_t^2 f_a f_{a,r} s + 8 f_t f_r^2 f_{a,r} f_r t f_s^4 f_b^2 - 80 \\
& f_t^2 f_r f_{a,r} f_r t f_s^4 f_a^2 + 224 f_t^2 f_r^3 f_{a,r} f_r t f_b^2 f_s^2 + 448 f_t^3 f_r^2 f_{a,r} f_r t f_a^2 f_s^2 - 320 f_t^3 f_r^3 f_{a,r} f_r t f_b^2 f_a^2 \\
& - 12 f_b^4 f_r^2 f_s^3 f_r r s f_t f_a + 24 f_a^4 f_t f_b^3 f_s^3 f_r f_r r t - 15 f_a^5 f_t^2 f_b^2 f_s^3 f_{a,a} s f_r - 14 f_a^3 f_r^2 s f_t f_s^2 f_b^4 f_r + 4 \\
& f_a^2 f_t^2 f_b^5 f_r^3 f_{a,r} f_b r + 8 f_a^2 f_t^2 f_b^6 f_r^2 f_{a,r} f_r r + 16 f_a^4 f_t^4 f_r^3 f_b f_{a,b} f_{a,a} + 5 f_b^3 f_s^4 f_a^4 f_r f_{a,b} f_r t + 4 f_a^6 \\
& f_t^3 f_b f_r^2 f_{a,b} f_r t - 192 f_a^2 f_t^3 f_r^4 f_b f_{a,s} f_{a,t} + 128 f_b f_s^2 f_r^3 f_t^3 f_a f_{a,r} s - 20 f_a^6 f_s f_r t f_b f_r r f_t^3 + 12 f_a^2 \\
& f_s^5 f_r t f_b f_r r f_t + 2 f_b r f_t f_a^5 f_{a,s} f_s^4 f_b^2 + 2 f_b r f_t f_a^4 f_{a,s} f_s^5 f_b - 96 f_b f_a^2 f_r s f_t^2 f_r r f_s^4 + 96 f_s^2 f_a^4 \\
& f_t^3 f_{a,b} r f_r^2 f_b + 32 f_b^3 f_a^3 f_b r f_r^2 f_t^3 f_r r + 256 f_b f_a f_b r f_r^3 f_t^4 f_r r - 12 f_b^6 f_r^3 f_t^2 f_{a,a} f_a f_r r + f_b^4 f_s^5 \\
& f_a^2 f_{a,s} f_a a f_r + 2 f_b^4 f_s^5 f_r f_a f_{a,r} f_b r + 48 f_a^2 f_t^2 f_r^2 f_s^4 f_r s f_{a,b} + 16 f_a^2 f_t f_b^6 f_r^3 f_{a,r} s f_s - 32 f_a f_t^2 f_b^5
\end{aligned}$$

$$\begin{aligned}
& f_r^4 f_a b f_{a,r} - 4 f_a^2 f_t f_b^5 f_r^4 f_{a,s} f_{a,t} + 48 f_a^4 f_t^4 f_r^2 f_{a,s} f_{a,a} f_s + 48 f_a^4 f_t^3 f_r^2 f_b f_{r,s} f_{r,t} + 60 f_a^4 \\
& f_t^3 f_{r,r} r f_r f_b^3 f_s + 128 f_a^2 f_t^3 f_r^2 f_{r,s} f_{a,s} f_s^2 - 3 f_b f_s^6 f_a^2 f_{a,t} f_b r f_r - 64 f_a^3 f_t^3 f_b^3 f_r f_{a,b} f_{a,r} - 52 f_a^6 \\
& f_t^4 f_{a,a} r f_s f_r f_b + 4 f_a^6 f_t^4 f_b f_r f_{a,r} f_b r - 126 f_a^4 f_t^3 f_b^2 f_s^2 f_{a,r} r f_r + 64 f_a f_t^3 f_b^2 f_r^4 f_{r,s} f_{a,b} + 24 f_a^4 f_t^3 \\
& f_s^2 f_r f_b r f_{r,s} - 4 f_b^3 f_s^5 f_a^3 f_{a,b} f_b r f_r + 12 f_a^6 f_t^4 f_{a,b} f_r r f_r f_b - 96 f_s^3 f_{a,a} f_b^3 f_{r,r} f_r^2 f_t^2 - 24 f_b^3 f_s^4 f_a \\
& f_r^2 f_b r f_{r,t} - 30 f_b^3 f_r^2 f_{a,a} s f_s^4 f_a^2 f_t + 144 f_b^3 f_r^3 f_{a,a} s f_t^2 f_a^2 f_s^2 + 39 f_b^3 f_r^2 f_{a,a} s f_s^2 f_a^4 f_t^2 + 48 f_a^5 f_t^3 \\
& f_r^2 f_{a,t} f_b r f_s + 48 f_a^5 f_t^3 f_b f_r^2 f_{a,t} f_{r,s} + 8 f_a^4 f_t^3 f_b^2 f_r^2 f_b r f_{r,s} - 2 f_s^8 f_{a,t} f_{r,r} - 8 f_a^8 f_t^5 f_{a,r,r} + 16 f_a^7 \\
& f_t^5 f_{a,r}^2 + 2 f_s^8 f_b r f_{r,s} - 8 f_a^7 f_t^5 f_{r,r,r} + 32 f_a^5 f_t^5 f_{r,r}^2 + 2 f_a f_s^8 f_{r,r,t} + 2 f_a^2 f_s^8 f_{a,r,t} + 2 f_s^8 f_{r,t} f_{a,r} \\
& + 2 f_a^3 f_r^2 f_s^6 + 2 f_s^8 f_t f_{a,r,r} - f_s^9 f_a f_{a,b,r} + f_b f_s^8 f_{r,r,s} - 512 f_r^5 f_t^5 f_{a,a,a} + f_{a,a,b} f_s^9 f_r + 512 f_r^4 \\
& f_t^5 f_{a,r,r} + f_s^8 f_a f_b^2 r - 2 f_b f_s^7 f_{r,s}^2 - 5 f_t f_a^4 f_{a,b} f_s^5 f_b^2 f_{a,r} + 102 f_a^4 f_t^3 f_{a,r} f_{r,r} f_b^2 f_s^2 - 5 f_a^2 f_t f_b \\
& f_s^6 f_b r f_{a,r} + 80 f_b f_s^2 f_a^5 f_{a,s} f_r r f_t^3 + 9 f_t^3 f_a^6 f_{a,b} f_s^2 f_b f_{r,r} - 6 f_t^2 f_a^5 f_{a,b} f_s^3 f_b^2 f_{r,r} + 7 f_t^2 f_a^5 f_{a,b} \\
& f_s^4 f_b f_{a,r} + 8 f_a^3 f_t f_b f_s^5 f_{r,t} f_{a,r} - 9 f_s^6 f_a^2 f_{a,b} f_r r f_t f_b - 81 f_b^2 f_s^3 f_a^4 f_{a,s} f_{r,r} f_t^2 + 192 f_a^2 f_t^3 \\
& f_r^3 f_s f_{a,s} f_{r,t} + 16 f_a^4 f_t^3 f_b^4 f_r f_{a,r} f_{r,r} + 4 f_a^5 f_t^3 f_b^2 f_r^2 f_{a,s} f_b r + 4 f_b^5 f_s^2 f_r^3 f_t f_{r,s} f_{a,a} + 8 f_a^4 f_t^3 f_b^3 \\
& f_r^2 f_{a,r} f_b r + 4 f_{a,t} f_a f_b^6 f_{a,r} f_r^4 f_t - 28 f_{a,t} f_a^5 f_b^2 f_{a,r} f_r^2 f_t^3 + 64 f_a^2 f_t^3 f_b f_s f_r^3 f_b^2 r + 80 f_b f_s^4 \\
& f_r^3 f_t f_{a,s} f_{a,t} - 12 f_{a,t}^2 f_a^5 f_r^2 f_t f_b^2 f_s^2 + 4 f_{a,t}^2 f_a^6 f_r f_s^3 f_b f_t + 4 f_{a,t}^2 f_a^6 f_r^2 f_t^2 f_b f_s + 256 f_a f_t^4 f_r^3 f_{a,b} f_{r,r} f_s \\
& - 16 f_b^6 f_r^4 f_{a,a} s f_t f_a f_s - 36 f_b^4 f_r^3 f_{a,a} s f_t^2 f_a^3 f_s + 27 f_b^5 f_r^3 f_{a,a} s f_t f_a^2 f_s^2 + 12 f_b^4 f_r^3 f_{a,a} s f_t f_a f_s^3 \\
& - 144 f_b^4 f_r^4 f_{a,a} s f_t^2 f_a f_s - 22 f_b^4 f_r^2 f_{a,a} s f_s^3 f_a^3 f_t + 48 f_a f_t^2 f_r^2 f_s^4 f_{a,s} f_b r + 128 f_b^3 f_a f_b r f_r^3 \\
& f_t^3 f_{r,r} + 128 f_b f_a^3 f_b r f_r^2 f_t^4 f_{r,r} + 16 f_b^5 f_a f_b r f_r^3 f_t^2 f_{r,r} + 16 f_b f_a^5 f_b r f_r f_t^4 f_{r,r} + 7 f_a^4 f_t f_b^3 \\
& f_s^4 f_{a,a} s f_r - 28 f_a^5 f_t^2 f_s^3 f_{a,t} f_b r f_r - 448 f_a^2 f_t^3 f_r^3 f_{r,s} f_{a,t} f_s - 512 f_a f_t^4 f_r^4 f_{a,b} f_{a,r} f_b - 4 f_a^6 \\
& f_t^3 f_{a,b} f_b r f_s^2 f_r + 4 f_a^4 f_t f_b^2 f_s^4 f_{r,s} f_b r - 2 f_a^5 f_t f_b^2 f_s^3 f_{r,s} f_{r,t} - 4 f_s^6 f_t f_{a,a} f_b^2 f_a^2 f_{a,r} - 16 f_s^4 f_a^3 f_{r,s} \\
& f_t^2 f_{a,r} f_b - 12 f_s^5 f_a^2 f_{r,s} f_t f_{a,r} f_b^2 + 8 f_a^4 f_t f_b^3 f_s^4 f_{a,s} f_{a,r} + 16 f_{a,t} f_a^6 f_s^2 f_b^2 f_{r,r} f_t^2 - 4 f_{a,t} f_a^5 f_s^3 \\
& f_b^3 f_{r,r} f_t + 12 f_t f_{a,t} f_a^5 f_b^2 f_s^4 f_{a,r} - 10 f_a^5 f_t^3 f_{a,a} f_b f_s^3 f_{a,r} + 32 f_s^2 f_a^5 f_{r,s} f_t^3 f_{a,r} f_b + 92 f_b f_a^4 f_{r,s} \\
& f_t^3 f_{r,r} f_s^2 - 2 f_b^4 f_a^3 f_{r,s} f_t f_{r,r} f_s^3 - 4 f_b f_s^6 f_a f_b r f_r r f_t + 4 f_a^5 f_t^2 f_b^2 f_s^3 f_{r,s} f_{a,a} + 8 f_a^4 f_s^3 f_{r,t} f_b f_r r f_t^2 \\
& + 24 f_b^2 f_s^5 f_{r,s} f_{r,r} f_t f_a + 18 f_a^5 f_s^2 f_{r,t} f_b^2 f_{r,r} f_t^2 - 8 f_a^4 f_s^3 f_{r,t} f_b^3 f_{r,r} f_t - 4 f_a^3 f_s^4 f_{r,t} f_b^2 f_{r,r} f_t - 128 \\
& f_a^5 f_t^4 f_{a,r} f_{r,r} f_b f_s - 4 f_b r f_t^2 f_a^6 f_{a,s} f_s^3 f_b + 144 f_s^3 f_t^3 f_{a,r} f_{r,r} f_b f_a^3 - 60 f_s^4 f_t^2 f_{a,r} f_{r,r} f_b^2 f_a^2 - 16 f_s^5 \\
& f_t^2 f_{a,r} f_{r,r} f_b f_a + 8 f_s^5 f_t f_{a,r} f_{r,r} f_b^3 f_a + 16 f_a^4 f_t^2 f_b^2 f_s^2 f_{a,r} f_{r,r} - 2 f_s^5 f_a^5 f_{a,b} f_b r f_b f_t + 12 f_s^5 \\
& f_t^2 f_{a,a} f_b f_a^3 f_{a,r} - 6 f_a^6 f_t f_b^2 f_s^3 f_{r,s} f_{a,t} + 9 f_a^5 f_t^2 f_b^3 f_s^2 f_{r,s} f_{a,r} + 4 f_b r f_{a,t} f_a^6 f_s^4 f_b f_t + 9 f_a^7 f_t^2 f_b \\
& f_s^2 f_{r,s} f_{a,t} + 2 f_s^4 f_{r,t} f_a^6 f_{a,b} f_b f_t - 2 f_a^4 f_t f_b^3 f_s^4 f_{r,s} f_{a,a} - 4 f_b^5 f_s^3 f_a^3 f_{a,r} f_t f_{r,r} - 21 f_a^5 f_t^2 f_b^2 \\
& f_s^3 f_{a,r} f_{a,s} - 11 f_a^5 f_t^2 f_b^2 f_s^3 f_{a,r} f_b r - 2 f_a^3 f_t f_b^3 f_s^5 f_{a,r} f_{a,a} + 4 f_t^4 f_a^6 f_{a,a} f_r r f_b f_s - 9 f_t^3 f_a^5 f_{a,a} f_{r,r} \\
& f_b^2 f_s^2 + 11 f_a^6 f_t^3 f_{a,r} f_b r f_s^2 f_b - 2 f_b^2 f_s^4 f_{r,t} f_a^5 f_{a,a} f_t - 10 f_a^2 f_t f_b f_s^6 f_{r,s} f_{a,a} - 2 f_s^7 f_t f_{a,a} f_b f_a f_{a,r}
\end{aligned}$$

$$\begin{aligned}
& + 20f_a^6 f_t^3 f_b^2 f_s f_{a,s} f_{r,r} - 20f_a^3 f_t^2 f_{a,r} f_{r,r} f_s^3 f_b^3 + 22f_a^4 f_t f_b^2 f_s^4 f_{r,s} f_{a,s} + 5f_a^4 f_t f_b^3 f_s^4 f_{a,r} f_{b,r} \\
& + 10f_b^3 f_a^2 f_{r,s} f_t f_{r,r} f_s^4 + 2f_a^4 f_t f_b f_s^4 f_{r,s} f_{r,t} + 4f_a^3 f_t f_b f_s^5 f_{r,s} f_{b,r} - 8f_a^3 f_t f_b^2 f_s^5 f_{r,s} f_{a,a} - 6f_a^4 \\
& f_t^2 f_b f_s^4 f_{a,r} f_{b,r} + 26f_b^3 f_s^4 f_a^3 f_{a,s} f_{r,r} f_t + 42f_b^2 f_s^5 f_a^2 f_{a,s} f_{r,r} f_t + 2f_a^6 f_{r,t} f_b^2 f_{a,r} f_s^2 f_t^2 - 4f_a^5 f_{r,t} \\
& f_b^3 f_{a,r} f_s^3 f_t + 2f_s^4 f_a^5 f_{b,r} f_t^2 f_{a,a} f_b - f_s^5 f_a^4 f_{b,r} f_t f_{a,a} f_b^2 - 2f_s^6 f_a^3 f_{b,r} f_t f_{a,a} f_b + 7f_a^6 f_t^2 f_b f_s^2 f_{r,s} f_{r,t} \\
& - 15f_t^2 f_{a,t} f_a^6 f_b f_s^3 f_{a,r} + 20f_t f_{a,t} f_a^4 f_b f_s^5 f_{a,r} + 24f_b f_s^6 f_a f_{a,s} f_{r,r} f_t - 96f_b f_s^4 f_a^3 f_{a,s} f_{r,r} f_t^2 - 9 \\
& f_a^6 f_t^2 f_b^2 f_s^2 f_{r,s} f_{a,s} + 12f_a^4 f_t^2 f_s^4 f_{r,s} f_{a,a} f_b + 6f_s^4 f_{r,t} f_a^5 f_{b,r} f_b f_t + 6f_t^2 f_a^4 f_{a,r} f_s^3 f_b^3 - 8f_t \\
& f_a^3 f_{a,b} f_s^6 f_b f_{a,r} - 4f_t f_a^3 f_{a,b} f_s^5 f_b^2 f_{r,r} - 20f_{a,t} f_a^7 f_s f_b f_{r,r} f_t^3 + 4f_a^7 f_t^3 f_{r,s} f_s f_b f_{a,s} - 4f_{a,t} f_a^7 f_{r,t} \\
& f_s^3 f_b f_t - f_a^3 f_t f_b^4 f_s^4 f_{a,a} f_{r,r} + f_t f_a^4 f_{a,b} f_s^4 f_b^3 f_{r,r} + 4f_b^4 f_{a,s} f_s^3 f_a^4 f_t f_{r,r} - 4f_a^6 f_t^2 f_b f_s^3 f_{a,b} f_{r,s} \\
& - 28f_b f_s^4 f_{a,s} f_a^4 f_t^2 f_{a,r} - 26f_a^5 f_t^2 f_s^3 f_{r,s} f_b f_{a,s} - 20f_a^5 f_t^3 f_b^3 f_s f_{a,r} f_{r,r} + 6f_s^4 f_a^3 f_{b,r} f_t f_{r,r} f_b^3 \\
& - 9f_t f_a f_{a,a} f_s^6 f_{r,r} f_b^2 - 6f_t f_a^2 f_{a,a} f_s^5 f_{r,r} f_b^3 - 4f_a^4 f_{a,a} f_s^5 f_{r,t} f_b f_t - 14f_a^5 f_t^2 f_b f_s^3 f_{r,t} f_{a,r} + 16 \\
& f_b^2 f_a^5 f_{r,s} f_t^3 f_{r,r} f_s - 7f_b^3 f_a^4 f_{r,s} f_t^2 f_{r,r} f_s^2 - 72f_b^2 f_a^3 f_{r,s} f_t^2 f_{r,r} f_s^3 - 36f_t^3 f_a^4 f_{a,a} f_s^3 f_{r,r} f_b + 30f_t^2 \\
& f_a^3 f_{a,a} f_s^4 f_{r,r} f_b^2 + 36f_t^2 f_a^2 f_{a,a} f_s^5 f_{r,r} f_b - 6f_a^4 f_t f_b^4 f_s^3 f_{r,s} f_{a,r} - 2f_b^4 f_s^4 f_a^2 f_{a,r} f_t f_{r,r} + 2f_a^5 f_t f_b^2 \\
& f_s^4 f_{a,b} f_{r,s} - 8f_s^3 f_a^4 f_{r,s} f_t^2 f_{a,r} f_b^2 + 6f_s^5 f_a^2 f_{b,r} f_t f_{r,r} f_b^2 + 20f_s^2 f_a^5 f_{b,r} f_t^3 f_{r,r} f_b - 17f_s^3 f_a^4 f_{b,r} \\
& f_t^2 f_{r,r} f_b^2 - 16f_s^4 f_a^3 f_{b,r} f_t^2 f_{r,r} f_b + 2f_a^4 f_t f_b f_s^5 f_{a,b} f_{r,s} - 2f_a^6 f_t^3 f_{r,s} f_{a,a} f_s^2 f_b - 16f_b^3 f_{a,s} f_s^2 f_a^5 \\
& f_t^2 f_{r,r} + 22f_a^6 f_t^3 f_{a,s} f_s^2 f_b f_{a,r} + 6f_a^5 f_t f_b^3 f_s^3 f_{r,s} f_{a,s} - 8f_a^5 f_t^2 f_b f_s^3 f_{r,s} f_{b,r} - 4f_a^6 f_t^3 f_{r,s} f_{a,a} f_s f_b^2 \\
& + 8f_a^5 f_t^2 f_{a,t} f_{r,s} f_s^3 f_b + 6f_a^4 f_t f_{a,t} f_{r,r} f_s^4 f_b^2 - 10f_s^4 f_a^3 f_{r,s} f_t f_{a,r} f_b^3 + f_b f_s^3 f_{r,t} f_a^6 f_{a,a} f_t^2 + 8f_a^4 \\
& f_t^2 f_{a,a} f_b^2 f_s^4 f_{a,r} + 20f_a^3 f_t f_{a,t} f_{r,r} f_s^5 f_b + 4f_a^6 f_{a,s} f_{r,t} f_b^2 f_s^3 f_t - 2f_a^7 f_{a,s} f_{r,t} f_b f_s^2 f_t^2 + 10 \\
& f_a^5 f_{a,s} f_{r,t} f_b f_s^4 f_t - 8f_a^5 f_t f_b f_s^4 f_{r,s} f_{a,t} - 16f_b f_s^6 f_a f_{r,s} f_{a,r} f_t + 24f_a^3 f_t f_b f_s^5 f_{r,s} f_{a,s} + 4f_b^2 f_s^5 \\
& f_a^3 f_{a,r} f_b f_t - f_t^2 f_a^4 f_{a,b} f_s^4 f_b f_{r,r} + 14f_b^2 f_s^5 f_{a,s} f_a^3 f_t f_{a,r} + 6f_b f_s^6 f_{a,s} f_a^2 f_t f_{a,r} - 9f_b f_s^6 f_a^2 f_{r,s} f_{r,t} \\
& - 3f_t^3 f_a^6 f_{a,b} f_s^3 f_{a,r} - 7f_a^4 f_t f_b^3 f_s^4 f_{r,r} f_s + 6f_t^2 f_a^4 f_{a,b} f_s^5 f_{a,r} - 4f_t^4 f_a^7 f_{a,b} f_s f_{r,r} - 3f_t f_a^2 f_{a,b} \\
& f_s^7 f_{a,r} - f_b^2 f_s^7 f_a f_b f_{r,a} r + 28f_a^7 f_t^4 f_{a,r} f_s f_b - 12f_a^4 f_s^5 f_{r,r} f_t f_b f_t + 52f_a^4 f_t^3 f_s^3 f_{a,s} f_{r,r} - 8f_b \\
& f_a^6 f_{r,s} f_t^4 f_{r,r} - 58f_a^3 f_t^2 f_{a,r} f_s^4 f_b^2 + 2f_{a,b} f_s^7 f_b^2 f_a f_{r,r} - 13f_t^2 f_{a,t} f_a^5 f_s^4 f_{a,r} - f_b^2 f_s^7 f_{a,s} f_a f_{a,r} \\
& + 22f_b^2 f_s^4 f_{r,s} f_a^3 f_t - 2f_b^3 f_s^6 f_a f_b f_{r,r} - f_b^4 f_s^5 f_a^2 f_b f_{r,r} - 4f_a^8 f_t^3 f_{r,s} f_{a,t} f_s + f_s^8 f_{a,b} f_{a,r} f_b f_a \\
& + 8f_a^2 f_t f_s^6 f_{r,s} f_{a,s} + 8f_t f_a f_{r,t} f_{r,r} f_s^6 - 26f_b f_s^3 f_{r,s} f_a^4 f_t^2 + 24f_b f_s^5 f_{r,s} f_a^2 f_t - 4f_a^7 f_t^3 f_s f_{r,s} f_{r,t} \\
& - 4f_s^7 f_a f_b f_{r,t} f_{a,r} + f_b^3 f_s^6 f_a^3 f_{a,b} f_{a,r} + 2f_s^7 f_{a,b} f_{a,r} f_b^2 f_a^2 + f_a^5 f_{a,a} f_s^4 f_{r,t} f_t^2 + 3f_a^3 f_{a,a} f_s^6 f_{r,t} f_b^2 \\
& + 3f_a^2 f_{a,a} f_s^7 f_{r,t} f_b - 2f_a^3 f_{a,a} f_s^6 f_{r,t} f_t - 18f_b^2 f_s^5 f_a^4 f_{a,r} f_s f_t + 11f_b^2 f_s^6 f_a^2 f_t f_a - 80f_a^4 f_t^4 \\
& f_{r,r} f_b f_s + 48f_a^3 f_t^3 f_{r,r} f_b^2 f_s^2 + 96f_a^2 f_t^3 f_{r,r} f_b f_s^3 - 4f_a^5 f_t^3 f_{r,s} f_{a,a} f_s^3 - 2f_{b,r} f_{a,t} f_a^7 f_s^3 f_t^2 - 32f_a \\
& f_t^2 f_s^5 f_{r,s} f_{r,r} + 4f_s^5 f_a^3 f_{b,r} f_t^2 f_{a,r} + 32f_s^4 f_t^3 f_{a,r} f_{r,r} f_a^2 + 10f_a^2 f_t f_{a,t} f_{r,r} f_s^6 + f_b^2 f_s^5 f_a^4 f_{r,s} f_{a,t} + 8 \\
& f_a^2 f_t^2 f_{r,r} f_s^3 f_b^3 - 24f_a f_t^2 f_{r,r} f_s^4 f_b^2 - 8f_t^3 f_a^5 f_{r,t} f_{r,r} f_s^2 - 8f_t^2 f_a^3 f_{r,t} f_{r,r} f_s^4 - 10f_{a,t} f_a^2 f_s^6 f_{r,r} f_b^2
\end{aligned}$$

$$\begin{aligned}
& -4f_a f_t f_s^7 f_r, s f_{a,a} - 16f_a^4 f_t^2 f_s^4 f_r, s f_{a,s} - f_s^7 f_a^2 f_b, r f_t f_{a,a} + 6f_t^3 f_a, t f_a^7 f_s^2 f_{a,r} + 6f_s^6 f_t f_{a,r} f_r, r f_b^2 \\
& - 88f_s^2 f_t^4 f_{a,r} f_r, r f_a^4 + 6f_s^6 f_a^4 f_{a,b}, r f_b f_t - f_b^4 f_s^5 f_a^2 f_{a,s} f_r, r - 2f_b^3 f_s^6 f_a f_{a,s} f_r, r + 4f_a^6 f_t^3 \\
& f_s^2 f_r, s f_b, r + 2f_b f_s^7 f_a^2 f_{a,b} f_r, s + 6f_a^2 f_t f_b f_s^7 f_{a,a}, r - 7f_{a,t} f_a^3 f_s^6 f_b^2 f_{a,r} + 8f_t f_{a,t} f_a^3 f_s^6 f_{a,r} + 6f_b \\
& f_s^6 f_a^3 f_b, r, r f_t - 10f_a^6 f_t^3 f_{a,t} f_r, r f_s^2 - 6f_a^4 f_t^2 f_{a,t} f_r, r f_s^4 - 4f_a^7 f_t^4 f_{a,r} f_b, r f_s - 3f_b f_s^4 f_a^5 f_b, r, r f_t^2 \\
& + 2f_b^2 f_s^6 f_a^2 f_r, s f_b, r - 13f_a^7 f_t^3 f_{a,r}, s f_s^2 f_b - 32f_a^5 f_t^4 f_r, s f_s f_r, r - 8f_s^4 f_t^3 f_{a,a} f_a^4 f_{a,r} - f_b f_s^6 \\
& f_a^3 f_r, s f_{a,t} + 12f_t^4 f_a^5 f_{a,a} f_s^2 f_r, r + 3f_b^2 f_s^5 f_a^4 f_b, r, r f_t + 7f_b^4 f_s^4 f_a^3 f_{a,r} f_t - f_b^4 f_s^4 f_a^4 f_r, s f_{a,s} - 8f_a^7 \\
& f_t^4 f_{a,r} f_{a,s} f_s - 3f_s^3 f_r, t f_a^6 f_b, r f_t^2 - 3f_s^5 f_r, t f_a^4 f_b, r f_b^2 - 6f_s^6 f_r, t f_a^3 f_b, r f_b + 6f_s^5 f_r, t f_a^4 f_b, r f_t + 6 \\
& f_b^3 f_s^5 f_a^3 f_r, t f_{a,r} + 16f_b^4 f_s^2 f_r, r f_t^2 f_a^3 - 4f_b^5 f_s^3 f_r, r f_t f_a^2 - 8f_b^4 f_s^4 f_r, r f_t f_a - 20f_b^3 f_s^2 f_r, r f_t^3 f_a^4 \\
& - 5f_{a,t} f_a^2 f_s^7 f_b f_{a,r} - 96f_b f_s^3 f_r^3 f_t^2 f_b, r - 4f_a^5 f_t^3 f_s^2 f_r f_b, r + 2f_a^4 f_t f_b^3 f_s^5 f_{a,a}, r + 8f_a^3 f_t^2 \\
& f_s^5 f_r, s f_{a,a} + 74f_a^4 f_t^3 f_{a,r} f_s^3 f_b + 12f_t^2 f_{a,a} f_a^6 f_r, r + 8f_a^6 f_t^3 f_r, s f_{a,s} f_s^2 - 6f_b^2 f_s^5 f_a^3 f_r, s f_r, t \\
& - 60f_b f_s^3 f_t^3 f_r, r, r f_a^4 + f_s^6 f_a^3 f_b, r f_{a,s} f_b^2 + 2f_s^7 f_a^2 f_b, r f_{a,s} f_b + f_b^3 f_s^6 f_a f_r, s f_{a,r} + 2f_b^4 f_s^5 f_a^2 f_r, s f_{a,r} \\
& + 2f_a^3 f_s^4 f_r, t f_b^4 f_r, r - 12f_b^3 f_s^5 f_t f_r, r, r f_a^2 - 12f_b^2 f_s^6 f_t f_r, r, r f_a + 36f_b f_s^5 f_t^2 f_r, r, r f_a^2 - 6f_a^4 f_t^2 \\
& f_s^4 f_r, s f_b, r + 4f_a^5 f_t^2 f_s^3 f_r, s f_r, t - 24f_a^2 f_t^2 f_{a,r} f_s^5 f_b + 4f_a^2 f_s^5 f_r, t f_b^3 f_r, r - 4f_a^6 f_r, t f_s^3 f_b f_t - 3f_a^5 f_t^2 \\
& f_s^4 f_{a,b} f_r, s - 4f_b^4 f_s^4 f_a^4 f_{a,r}, r f_t - 15f_a^3 f_t f_b f_s^6 f_{a,r}, s + 12f_s^3 f_a^4 f_b, r f_t^3 f_r, r + f_b^3 f_s^5 f_r, t f_a^4 f_{a,a} - 10 \\
& f_b^3 f_s^5 f_a^3 f_{a,r}, r f_t + 24f_s^3 f_a^4 f_r, s f_t^3 f_{a,r} - 36f_b^2 f_s^2 f_a^5 f_r, r, r f_t^3 - 24f_a^6 f_t^4 f_{a,s} f_s f_r, r + 20f_b^3 f_s^3 \\
& f_a^4 f_r, r, r f_t^2 - 4f_b^4 f_s^4 f_a^3 f_r, r, r f_t + 4f_a^3 f_t f_s^5 f_r, s f_r, t - 32f_a^2 f_t^2 f_s^5 f_{a,s} f_r, r + 2f_b, r f_t^3 f_a^7 f_{a,s} f_s^2 \\
& - 3f_b, r f_t^2 f_a^5 f_{a,s} f_s^4 - 8f_s f_a^6 f_b, r f_t^4 f_r, r - 16f_s f_a^6 f_r, s f_t^4 f_{a,r} + 4f_a^5 f_t^3 f_s^3 f_b, r f_{a,r} + 42f_b^2 f_s^4 \\
& f_a^4 f_{a,r}, r f_t^2 - 6f_b^2 f_s^6 f_a^2 f_{a,r}, r f_t + f_{a,b} f_s^6 f_b^3 f_a^2 f_r, r - 2f_s^5 f_a^4 f_b^2 f_r f_b f_t - 34f_a^4 f_t^2 f_b^3 f_s^3 f_{a,r}^2 + 96f_r^2 \\
& f_t^4 f_{a,r}, r f_a^2 f_s^2 - 192f_r^3 f_t^4 f_{a,r}, r f_b^2 f_a^2 - 48f_r^3 f_t^2 f_{a,r}, r f_s^2 f_b^4 + 144f_r f_t^4 f_{a,r}, r f_s^2 f_a^4 + 72f_r^2 \\
& f_t^2 f_{a,r}, r f_s^4 f_b^2 + 4f_t^2 f_a^3 f_{a,b} f_s^5 f_r, r - f_b^3 f_s^4 f_a^4 f_r, s f_r, t - 54f_a^5 f_t^3 f_b f_s^3 f_{a,r}, r + 27f_b f_s^4 f_r, r, s f_a^4 f_t^2 \\
& - 15f_b f_s^6 f_r, r, s f_a^2 f_t - 18f_b^2 f_s^5 f_r, r, s f_a^3 f_t + 4f_a^2 f_t f_s^6 f_r, t f_{a,r} + 8f_a^6 f_t^4 f_{a,r} f_b^2 f_r, r - 12f_a^5 \\
& f_s^5 f_{a,r}, t f_b f_t + 28f_a^6 f_t^4 f_r, r, r f_b f_s + f_b^2 f_s^6 f_a^3 f_{a,b} f_r, s + 16f_a^5 f_t^3 f_{a,s} f_s^3 f_{a,r} + 4f_a^6 f_r^2 f_s f_t^3 f_b f_s - 9 \\
& f_a^5 f_r, s f_t^2 f_b^2 f_s^2 - 3f_s^4 f_a^6 f_t^2 f_{a,b}, r f_b + f_s^4 f_a^6 f_{a,b} f_b, r f_t^2 + f_s^6 f_a^4 f_{a,b} f_b, r f_b^2 - 12f_a^4 f_t^2 f_b f_s^5 f_{a,a}, r \\
& - 3f_s^3 f_r, t f_a^6 f_{a,s} f_t^2 + 6f_s^5 f_r, t f_a^4 f_{a,s} f_t + 6f_a^4 f_r, s f_t f_s^3 f_b^3 - 3f_b^3 f_s^5 f_a^4 f_{a,r} f_{a,t} + 2f_a^7 f_t^3 f_{a,b} f_r, s f_s^2 \\
& + 2f_s^7 f_a^3 f_{a,b} f_b, r f_b - 2f_s^6 f_a^4 f_{a,b} f_b, r f_t - 4f_{a,t} f_a^3 f_s^5 f_b^3 f_r, r - 6f_a^5 f_t^2 f_b^2 f_s^4 f_{a,a}, r - 7f_a^5 f_t f_b^3 \\
& f_s^4 f_{a,r}, s - 2f_a^5 f_{a,s} f_r, t f_b^3 f_s^4 - 7f_a^4 f_{a,s} f_r, t f_b^2 f_s^5 - 8f_a^3 f_{a,s} f_r, t f_b f_s^6 + 6f_b f_s^7 f_a f_r, t f_{a,r} - 8f_b \\
& f_s^7 f_a f_{a,t} f_r, r + f_b^5 f_r, s f_r, r f_s^4 f_a^2 - f_s^3 f_r, t f_a^7 f_{a,b} f_t^2 - f_s^5 f_r, t f_a^5 f_{a,b} f_b^2 - 2f_s^6 f_r, t f_a^4 f_{a,b} f_b + 2f_s^5 f_r, t \\
& f_a^5 f_{a,b} f_t + 3f_s^5 f_a^5 f_t f_{a,b}, r f_b^2 - f_b^4 f_s^5 f_a^3 f_{a,s} f_{a,r} - 36f_s^5 f_a^2 f_r f_t^2 f_b, r, r + 24f_s^3 f_a^4 f_r f_t^3 f_b, r, r + 192 \\
& f_s^3 f_{a,s} f_t^3 f_{a,a} f_r^3 - 48f_s^5 f_{a,s} f_t^2 f_{a,a} f_r^2 + 4f_s^7 f_{a,s} f_t f_{a,a} f_r - 256f_s f_{a,s} f_t^4 f_{a,a} f_r^4 - 288f_r^3 f_t^3 f_{a,r}, r
\end{aligned}$$



$$\begin{aligned}
& f_b^2 f_s^2 + 96 f_s^5 f_r s f_r f_t^2 f_{a,r} + 3 f_b^5 f_s^4 f_r^2 f_{a,a,r,s} + 2 f_b^5 f_s^3 f_a^2 f_r^2 f_t - 4 f_b^3 f_s^5 f_a^2 f_r f_t - 32 f_b f_s^3 f_a^2 r \\
& f_r^2 f_t^3 + 8 f_a^2 f_r f_{a,t} f_r f_s^6 - 4 f_b^6 f_s^2 f_r^4 f_{a,a,t} + 6 f_b^6 f_s^2 f_r^3 f_{a,t} f_{r,r} + 4 f_b^7 f_s f_r^4 f_{a,a,t} + 24 f_b^3 f_s^4 \\
& f_r^3 f_{a,s} f_{a,t} + 48 f_s^5 f_r f_{t,b} f_r^2 f_t + 256 f_s f_r f_{t,b} f_r^4 f_t^3 + 12 f_b^5 f_s^3 f_r^3 f_t f_{a,a,r} + 48 f_a^5 f_t^4 f_{a,a,r} f_r^2 f_b^2 \\
& - 48 f_a^5 f_t^4 f_{a,a,s} f_s f_r^2 + 48 f_a^3 f_t^3 f_b^4 f_r^3 f_{a,a,r} - 24 f_a^4 f_t^3 f_b^4 f_r^2 f_{a,r,r} + 16 f_a f_t^2 f_b^6 f_r^4 f_{a,a,r} + 8 f_{a,b} \\
& f_r^3 f_r f_t^3 f_s^4 + 16 f_{a,b} f_r^5 f_r f_t^5 f_t + f_b^3 f_s^6 f_a^3 f_{a,b} f_r - 8 f_a^4 f_r f_r^2 f_s^3 f_b^3 + 96 f_t^3 f_{a,a} f_{a,r} f_b^4 - 224 \\
& f_t^5 f_{a,a} f_{a,r} f_r^2 f_a^4 + 96 f_t^3 f_{a,a} f_{a,r} f_r^2 f_s^4 - 4 f_b f_s^7 f_r f_{a,r,t} + 48 f_b f_s^5 f_r^2 f_t f_{r,r,t} + 384 f_a f_t^4 f_r^2 f_r^2 f_b^2 \\
& - 256 f_a f_t^4 f_r^2 f_r f_s^2 + 96 f_a f_t^3 f_r^2 f_r^2 f_b^4 + 128 f_a^3 f_t^4 f_r^2 f_r f_b^2 + 384 f_t^4 f_{a,a} f_{a,r} f_r^4 f_b^2 - 256 \\
& f_t^5 f_{a,a} f_{a,r} f_r^3 f_a^2 - 384 f_t^4 f_{a,a} f_{a,r} f_r^3 f_s^2 - 16 f_s^4 f_a^3 f_{a,b} f_r^2 f_t^2 + 8 f_b^5 f_s f_r^4 f_t f_b^2 r - f_s^4 f_a^5 f_{a,b} f_r f_t^2 \\
& - 8 f_b^5 f_r^3 f_s f_r^2 s f_t + 5 f_b^2 f_s^6 f_a^2 s f_r f_a + 192 f_s^3 f_{a,b} f_{a,r} f_r^3 f_t^3 + 12 f_b^4 f_s^3 f_r^3 f_b f_{r,t} + 192 f_s^3 f_{a,s} \\
& f_t^3 f_r f_r^2 - 48 f_s^5 f_{a,s} f_t^2 f_r f_r - 4 f_b f_s^7 f_t^4 f_{a,r,s} f_r + 6 f_b^4 f_r f_s^4 f_r^2 s f_a + 192 f_a f_t^3 f_r^3 f_{a,a,s} f_s^3 \\
& + 288 f_a f_t^3 f_r^2 f_{a,a,r} f_s^4 - 6 f_b^2 f_s^6 f_r f_{a,r} f_r t - 4 f_a^7 f_t^4 f_{a,a,s} f_s f_r - 2 f_b^2 f_s^6 f_r f_r s f_b r - 2 f_b^3 \\
& f_s^6 f_r f_{a,b} f_r r + 96 f_b^3 f_s^3 f_r^3 f_t^2 f_{a,a,r} - 192 f_b^3 f_s f_r^4 f_r^3 f_{a,a,r} + 2 f_t^3 f_a^7 f_{a,a,t} f_r f_s^2 - 16 f_a^6 \\
& f_t^4 f_r f_{a,r} f_r t + 10 f_a^3 f_r^2 f_r^2 f_s^4 f_b^4 - 192 f_s^3 f_r f_{t,b} f_r^3 f_t^2 + 128 f_b f_s f_r^3 f_t^4 f_{a,r} - 8 f_a f_t^2 f_b^6 f_r^3 f_{r,r,r} \\
& + 384 f_t^4 f_a^3 f_r^2 f_r f_{r,r} + 96 f_t^4 f_a^5 f_r f_r f_{t,r,r} + 28 f_a^5 f_t^4 f_b^2 f_r f_{a,r} + 2 f_b^4 f_s^5 f_r f_{a,s} f_r r + 512 f_t^4 f_a \\
& f_r^3 f_r f_{r,r} - 2 f_b^4 f_s^5 f_r^2 f_{a,a} f_b r + 2 f_a^6 f_t^4 f_{a,a,a} f_r f_s^2 + 48 f_b^5 f_s f_r^3 f_t^2 f_{r,r,r} + 48 f_b f_s^5 f_r f_t^2 f_{r,r,r} \\
& - 96 f_b^3 f_s^3 f_r^2 f_t^2 f_{r,r,r} + 256 f_b f_s f_r^3 f_t^4 f_{r,r,r} - 48 f_s f_a^4 f_r^2 f_t^4 f_{b,r,r} + 144 f_s^3 f_a^2 f_r^2 f_t^3 f_{b,r,r} - 4 f_s \\
& f_a^6 f_r f_t^4 f_{b,r,r} - 192 f_s^3 f_r f_{t,a} f_s f_r^3 f_t^2 - 8 f_b^6 f_r f_{t,r}^4 f_{a,r} f_t + 48 f_b^5 f_r s f_r^3 f_r f_t^2 - 2 f_b^6 f_r^3 f_t f_{a,r} f_s^2 \\
& + 2 f_s^6 f_a^3 f_{a,b} f_r f_t + 192 f_b^3 f_s f_r^3 f_t^3 f_{r,r,r} - 192 f_b f_s^3 f_r^2 f_t^3 f_{r,r,r} - 12 f_b^5 f_s^3 f_r^2 f_t f_{r,r,r} + 12 f_b^3 \\
& f_s^5 f_r f_t f_{r,r,r} - 192 f_s f_a^2 f_r^3 f_t^4 f_{b,r,r} - 96 f_b^3 f_a^3 f_r^3 f_t^3 f_{a,r,s} - 256 f_b f_a f_r^4 f_t^4 f_{a,r,s} - 192 f_b^3 f_a f_r^4 \\
& f_t^3 f_{a,r,s} - 192 f_b f_a^3 f_r^3 f_t^4 f_{a,r,s} - 48 f_b^5 f_a f_r^4 f_t^2 f_{a,r,s} + 384 f_a^3 f_t^4 f_b^2 f_r^3 f_{a,a,r} - 8 f_b^6 f_{a,b} f_{a,s} f_r^5 f_t \\
& + 2 f_b^2 f_{a,b} f_{a,s} f_r^2 f_s^6 - 128 f_b^2 f_{a,b} f_{a,s} f_r^5 f_t^3 + 288 f_s^2 f_t^4 f_{a,a,a} f_r^3 f_a^2 + 32 f_s^2 f_a^3 f_{a,b} f_r^3 f_t^3 \\
& - 128 f_b f_r^3 f_s f_r^2 s f_t^3 + 4 f_b^5 f_s f_r^4 f_a^2 f_{a,t} + 64 f_s^2 f_a f_{a,b} f_r^4 f_t^3 - 2 f_b^6 f_s^2 f_r^3 f_{a,r} f_{r,t} - 14 f_b^6 f_s^2 \\
& f_r^3 f_a f_{r,t} + 3 f_b^6 f_s^3 f_r^2 f_a^2 f_{a,r,s} + f_b^6 f_s^3 f_r^3 f_{a,s} f_{a,a} - 4 f_b^7 f_s f_r^2 f_r^2 f_t + 8 f_b^5 f_s^3 f_r^2 f_r f_t + 48 f_a f_t^2 f_r^2 \\
& f_s^4 f_b r - 64 f_a f_t^2 f_r f_s^4 f_r^2 s + 48 f_a f_t^2 f_r f_s^5 f_{r,r,s} + 12 f_b^5 f_s^2 f_r^3 f_{r,s} f_{r,t} - f_b^7 f_s^2 f_r^3 f_a f_{a,r,s} - 64 f_a^3 f_t^4 \\
& f_{a,r} f_r^2 f_s^2 + 48 f_s^2 f_t^4 f_{a,a,a} f_r^2 f_a^4 + 4 f_b^7 f_s f_r^4 f_a f_{a,r,t} - 320 f_a f_t^4 f_{a,r}^2 f_r^3 f_b^2 + 256 f_a f_t^4 f_{a,r}^2 f_r^2 f_s^2 \\
& - 64 f_a f_t^3 f_{a,r}^2 f_r^3 f_b^4 - 32 f_a f_t^3 f_{a,r} f_r f_s^4 - 96 f_s^4 f_t^3 f_{a,r} f_r f_r + 384 f_s^2 f_t^4 f_{a,r} f_r f_r^2 + 96 f_a^3 f_t^3 \\
& f_s^3 f_{a,a,s} f_r^2 - 48 f_s^5 f_{a,b} f_{a,r} f_r^2 f_t^2 + 4 f_s^7 f_{a,b} f_{a,r} f_r f_t - 192 f_b^3 f_s f_r^5 f_t^2 f_{a,a,t} - 18 f_b^2 f_s^6 f_a f_r f_{r,t} \\
& - 6 f_b^2 f_s^6 f_a f_r f_b r - 48 f_b^5 f_s f_r^2 f_r^2 f_t^2 + 64 f_b^3 f_s^3 f_r^2 f_r f_t^2 + 8 f_b^5 f_s f_{a,s} f_r^4 f_t - 8 f_b f_s^5 f_{a,s} f_r^2 f_t + 4 \\
& f_b^3 f_s^5 f_{a,s} f_r f_a^2 - 12 f_b^5 f_r^3 f_{r,r,s} f_t^2 f_a^2 + 48 f_s^5 f_b f_r f_r f_r f_t^2 + 2 f_s^5 f_b f_r f_r f_b f_r + 2 f_b^6 f_r^4 f_t f_{a,a,a} f_s^2
\end{aligned}$$

$$\begin{aligned}
& -6f_b^4 f_r^3 f_t f_{a,a} f_s^4 - 24f_b^2 f_r^3 f_t^4 f_{a,a} f_a^4 - 72f_b^2 f_r^3 f_t^2 f_{a,a} f_s^4 - 48f_r f_t^5 f_{a,a} f_s^5 f_{r,r} \\
& - 256f_b f_s f_r^4 f_t^2 f_{r,t}^2 + 64f_b^3 f_s f_a^2 f_r^4 f_t^2 - 32f_b f_s^3 f_a^2 f_r^3 f_t^2 + 192f_b f_a^2 f_t^4 f_{a,a} f_s^4 + 4f_a f_t \\
& f_s^7 f_{a,a} f_r + 128f_b^3 f_{a,b} f_r^5 f_t^3 f_{a,a} + 16f_b^5 f_{a,b} f_r^5 f_t^2 f_{a,a} + 256f_b f_{a,b} f_r^5 f_t^4 f_{a,a} - 12f_a f_t f_s^6 f_r f_b^2 r \\
& - 48f_b f_a^5 f_r^2 f_t^4 f_{a,r,s} + 2f_b^5 f_s^3 f_a^2 f_r^3 f_t - 64f_b^3 f_s f_a^2 f_r^4 f_t^3 - 8f_b^5 f_s f_a^2 f_r^4 f_t^2 + 32f_b^3 f_s^3 f_a^2 f_r^3 \\
& f_t^2 - 3f_b^5 f_a^4 f_r^2 f_b^2 r_{r,r} + 6f_b^3 f_s^6 f_a f_r f_b^2 r_{r,r} + 3f_b^4 f_s^5 f_a^2 f_r f_b^2 r_{r,r} + 16f_{a,t} f_t f_r f_r f_s^6 - 256f_{a,t} f_t^3 \\
& f_r^3 f_r f_s^2 - 192f_a^2 f_t^3 f_r^2 f_{a,r} f_s^3 - 256f_a f_t^4 f_r^4 f_{a,a} f_s f_s - 3f_b^3 f_s^6 f_a f_{a,r} f_s f_r - 10f_b^4 f_s^4 f_a^4 f_r f_{a,r,t} \\
& + 512f_a^2 f_t^5 f_{a,r} f_r f_r^2 + 2f_b^6 f_s^2 f_r^3 f_r f_s f_b^2 r + 128f_s^2 f_{a,b} f_a f_r^4 f_t^3 + 352f_a^4 f_t^5 f_{a,r} f_r f_r + 48f_a^4 \\
& f_s^4 f_{a,r} f_t f_r^2 - 24f_a^3 f_s^5 f_{a,r} f_r f_b^3 - 6f_b^4 f_s^5 f_a^2 f_{a,r} f_s f_r + 48f_s^5 f_r f_{a,s} f_r^2 f_t - 128f_a^2 f_s^2 f_{a,r} f_r^3 f_t^3 \\
& - 96f_a^4 f_s^2 f_{a,r} f_r^2 f_t^3 + 96f_a^2 f_s^4 f_{a,r} f_r^2 f_t^2 + 30f_a^2 f_s^4 f_{a,r} f_r^2 f_b^4 - 18f_a^2 f_s^6 f_{a,r} f_r f_b^2 - 24f_a^6 \\
& f_s^2 f_{a,r} f_t f_r^3 + 48f_{a,a} b f_s f_r^5 f_b^4 f_t^2 + f_b^2 f_s^7 f_{a,a} f_b^2 r_{r,r} - 3f_b^5 f_s^4 f_r^3 f_{a,r} f_s + 18f_b^5 f_s^3 f_a^2 f_r^2 f_{r,t} \\
& + 6f_s^4 f_r^2 f_t f_{a,r} f_b^4 - 6f_s^6 f_r f_t f_{a,r} f_b^2 + f_b^4 f_a^3 f_a^2 f_r f_s^4 - 2f_b^5 f_a^2 f_a^2 f_r^2 f_s^3 + 8f_b^4 f_a^3 f_a^2 f_r^3 f_t^2 \\
& - 64f_b^4 f_{a,b} f_a f_s f_r^5 f_t^2 - 2f_b^6 f_{a,b} f_a f_s f_r^4 f_s^2 - 4f_b^3 f_s^5 f_a^2 f_r^2 f_t + 48f_b f_a^4 f_t^4 f_{a,a} f_s^3 + 4f_b f_a^6 \\
& f_t^4 f_{a,a} f_s f_r^2 + 192f_{a,t} f_a b f_s^3 f_r^4 f_t^2 - 48f_a f_r^2 f_r^2 f_t^4 f_b^2 - 32f_a^3 f_r f_r^2 f_s^4 f_t - 64f_a f_r^2 f_r^2 f_t^4 f_s^4 + 96 \\
& f_a^3 f_r^2 f_r^2 f_t^2 f_s^2 - 24f_a^2 f_r^2 f_r^2 f_t^3 f_b^3 + 4f_b f_b^2 r_{a,t} f_r^2 f_s^6 - 128f_b f_s^3 f_r^4 f_t^2 f_{a,t} - 256f_b f_b^2 r_{a,t} f_r^5 f_t^3 \\
& - 128f_b^3 f_b^2 r_{a,t} f_r^5 f_t^2 + 4f_b^5 f_b^2 r_{a,t} f_r^4 f_s^2 - 8f_b^3 f_b^2 r_{a,t} f_r^3 f_s^4 - 48f_b^5 f_s f_r^4 f_t^2 f_{a,a} r + 16f_b^2 f_s^5 \\
& f_r^2 f_{a,s} f_r t + 12f_b f_s^6 f_r f_r f_s f_{r,t} + 128f_b f_s^3 f_r^3 f_t^2 f_{r,t} + 64f_b^3 f_s f_r^4 f_t^2 f_b^2 r - 192f_t^4 f_b f_r^3 f_{r,r} f_a^2 \\
& - 48f_t^4 f_b f_r^2 f_{r,r} f_a^4 - 16f_b^5 f_b^2 r_{a,t} f_r^5 f_t - 96f_a^3 f_t^3 f_s^3 f_r f_{r,r} f_s - 256f_b f_s f_t^4 f_r^2 f_r^2 + 192f_b^3 f_s \\
& f_r^4 f_t^2 f_{r,r} t + 48f_b^5 f_s f_r^4 f_t f_{r,r} t + 256f_a f_t^4 f_r^3 f_s f_{r,r} f_s - 384f_r^2 f_t^5 f_{a,a} f_a^3 f_{r,r} - 768f_r^3 f_t^5 f_{a,a} f_a f_{r,r} \\
& - 96f_b^3 f_r^3 f_{r,r} f_t^3 f_a^2 - 3f_b^5 f_r f_{r,r} f_s^4 f_a^2 - 12f_b^3 f_r^2 f_{r,r} f_t^3 f_a^4 + 3f_b^6 f_r^2 f_{r,r} f_s^3 f_a - 4f_b^6 f_s \\
& f_r^4 f_b^2 r_{r,r} f_t - 2f_a^4 f_s^5 f_b^3 f_{a,a} f_r + 384f_b^2 f_r^4 f_{a,t} f_r f_r^3 + 96f_b^4 f_r^4 f_{a,t} f_r f_r^2 + 8f_b^6 f_r^4 f_{a,t} f_r f_t \\
& + 256f_b^2 r_{r,t}^4 f_s f_r^3 f_{r,r} - 6f_b^4 f_s^4 f_a^2 f_r^2 f_a + 2f_b^5 f_s^3 f_r f_r^2 f_a^2 - 256f_t^4 f_{a,b} f_s f_r^4 f_{a,r} + 8f_b^6 f_a^2 f_t^2 \\
& f_r^2 f_r^2 + 16f_b^4 f_a^3 f_t^3 f_r^2 f_r f_r - 4f_b^7 f_s f_r^3 f_r f_{r,r} - 14f_b^6 f_s^2 f_r^3 f_a^2 f_{a,r} t - 96f_s^4 f_{a,b} f_a f_s f_r^3 f_t^2 + 24 \\
& f_s^6 f_{a,b} f_a f_s f_r^2 f_t - f_b^6 f_s^3 f_r^2 f_r f_b^2 r - 8f_b^5 f_s^2 f_a^2 f_r f_t^2 - 192f_a f_t^2 f_a^2 f_r^3 f_s^2 + 16f_a f_t^3 f_a^2 f_r^4 f_b^4 \\
& + 48f_a f_t^3 f_a^2 f_r^2 f_s^4 - 4f_a f_r f_{a,t} f_s^7 f_b^2 r - 192f_a^3 f_t^4 f_r^3 f_{a,a} f_s f_s + 8f_b^6 f_b^2 r_{r,r} f_s^4 f_t + 128 \\
& f_b^2 f_b^2 r_{r,r} f_s f_r^3 f_t^3 + 64f_b^4 f_b^2 r_{r,r} f_s f_r^4 f_t^2 - 40f_a f_t^2 f_r f_s^6 f_{a,a} r - 96f_b^3 f_s^3 f_r^3 f_t f_{r,t} - 2f_s^7 f_b f_a^2 f_{a,b} f_r \\
& + 4f_s^5 f_b^3 f_a^2 f_{a,b} f_r^2 - f_s^6 f_b^2 f_a^2 f_{a,b} f_r - 8f_b^5 f_s^3 f_r^3 f_{a,a} f_{r,t} - 168f_a^4 f_t^4 f_b^2 f_r^2 f_{a,r} r + 192f_a f_t^3 f_b^4 \\
& f_r^4 f_{a,a} r - 96f_a f_t^3 f_b^4 f_r^3 f_{r,r} r + 48f_b^4 f_r^4 f_t^2 f_{a,a} f_s^2 - 24f_b^4 f_r^4 f_t^3 f_{a,a} f_a^2 - 2f_b^5 f_s^4 f_r f_s f_r f_r \\
& - 48f_{a,t} f_a b f_s^5 f_r^3 f_t - 256f_{a,t} f_a b f_s f_r^5 f_t^3 - 72f_a^2 f_t^3 f_b^4 f_r^3 f_{a,r} r + 2f_b^4 f_{a,b} f_a f_s f_r^3 f_s^4 + 4f_b \\
& f_s^7 f_{a,a} r f_t f_r + 192f_b^3 f_r f_s f_r^3 f_r f_t^3 + 8f_b^6 f_r^4 f_t^2 f_{a,a} f_r - 256f_s f_a f_r^4 f_t^4 f_{a,b} r - 384f_r^3
\end{aligned}$$

$$\begin{aligned}
& f_t^4 f_a r f_r r f_b^2 - 192 f_s f_r^4 f_t^3 f_{b,r} r f_b^2 + 24 f_s^3 f_r^3 f_t f_{b,r} r f_b^4 - 36 f_s^5 f_r^2 f_t f_{b,r} r f_b^2 - 48 f_s f_r^4 f_t^2 f_{b,r} r \\
& f_b^4 - 8 f_t^2 f_a a f_a r f_r f_s^6 - 4 f_b^3 f_s^5 f_r f_r t f_r r + f_b^6 f_a f_a s f_r^3 f_s^2 + 4 f_b^6 f_a f_a s f_r^4 f_t + 4 f_b^2 f_a^5 f_a s f_r^2 f_t^3 \\
& - 48 f_s^4 f_a f_a^2 b f_r^3 f_t^2 - 5 f_s^4 f_a f_a^2 b f_r^3 f_b^4 + 6 f_s^6 f_a f_a^2 b f_r^2 f_b^2 + 4 f_s^2 f_a^5 f_a^2 b f_r^2 f_t^3 + 12 f_s^6 f_a f_a^2 b f_r^2 f_t \\
& - 256 f_r^4 f_a t f_s f_r s f_t^3 + 192 f_r^3 f_a t f_s^3 f_r s f_t^2 - 48 f_r^2 f_a t f_s^5 f_r s f_t - 128 f_a^2 t f_a f_r^4 f_t^2 f_s^2 - 40 \\
& f_a^2 t f_a f_r^4 f_s^2 f_b^4 + 48 f_a^2 t f_a f_r^3 f_s^4 f_b^2 + 64 f_a^2 t f_a f_r^3 f_t f_s^4 + 18 f_b^5 f_s^3 f_a f_r^2 f_a r s t - 256 f_b f_r s f_r^4 f_t^4 f_a a \\
& - 192 f_b^3 f_r s f_r^4 f_t^3 f_a a - 48 f_b^5 f_r s f_r^4 f_t^2 f_a a - 4 f_b^5 f_s f_r^3 f_a^2 f_r^2 t - 4 f_a^5 f_t^4 f_a^2 a f_r f_s^2 + 8 f_a^3 f_t^3 \\
& f_a^2 a f_r f_s^4 - 64 f_a^3 f_t^4 f_a^2 a f_r^2 f_s^2 + 32 f_a^3 f_t^4 f_a^2 a f_r^3 f_b^2 - 4 f_a f_t^2 f_a^2 a f_r f_s^6 + 128 f_a f_t^4 f_a^2 a f_r^4 f_b^2 + 6 f_b^2 \\
& f_r^2 f_t f_a a a f_s^6 - 192 f_b^2 f_r^4 f_t^4 f_a a a f_a^2 + 288 f_b^2 f_r^4 f_t^3 f_a a a f_s^2 + 192 f_a a b f_s f_r^5 f_b^2 f_t^3 + 8 f_b^5 f_s^3 \\
& f_r^2 f_r t f_r r + 3 f_b^2 f_s^7 f_a f_r f_a b r + f_b^6 f_s^3 f_a f_r^3 f_a b r - 3 f_b^4 f_s^5 f_a f_r^2 f_a b r + 3 f_b^4 f_s^5 f_a^3 f_r f_a b r + 6 f_b^3 \\
& f_s^6 f_a^2 f_r f_a b r - 3 f_b^5 f_s^4 f_a^2 f_r^2 f_a b r - 24 f_a f_t f_r f_r r t f_s^6 - 96 f_a^4 f_t^3 f_s^3 f_a r s f_r - 48 f_b f_s^5 f_r^3 f_t f_a a t \\
& - 48 f_b f_s^5 f_a a r f_r^2 f_t^2 - 8 f_a^2 f_t^2 f_b^6 f_r^3 f_a r r + 48 f_a^6 f_t^4 f_a r s f_s f_r - 20 f_b^4 f_s^3 f_r^3 f_a s f_r t - 12 f_b^4 f_s^3 \\
& f_r^4 f_a t f_a b + 20 f_b^4 f_s^3 f_r^3 f_a t f_r s - 256 f_b f_s f_r^5 f_t^3 f_a a t - 256 f_b f_s f_r^4 f_t^4 f_a a r - 1024 f_a f_t^4 \\
& f_r^4 f_a t f_a r - 24 f_a^2 f_s^6 f_a r t f_r f_t - 192 f_a f_t^3 f_r^2 f_s^3 f_r r s + 128 f_a f_t^3 f_r^2 f_s^2 f_r^2 s - f_b^4 f_s^5 f_a^3 f_a a s f_r - 4 \\
& f_a^6 f_t^4 f_b f_r f_r r s - 64 f_a f_t^3 f_r^3 f_s^2 f_b^2 r - 10 f_b^4 f_s^4 f_a^3 f_r f_r r t - 256 f_s f_a s f_t^4 f_r r f_r^3 + 144 f_s^3 f_r^3 \\
& f_t^2 f_{b,r} r f_b^2 - f_b^3 f_s^6 f_r s f_a a f_r - 64 f_b^3 f_r^3 f_s^2 f_r^2 s f_t^2 + 32 f_b f_r^2 f_s^3 f_r^2 s f_t^2 - 96 f_t^2 f_r^2 f_a r f_r t f_s^4 + 48 f_b^3 \\
& f_r^3 f_s^2 f_r r s f_t^2 - 8 f_b f_r f_s^6 f_r r s f_t + 12 f_b^3 f_r^2 f_s^4 f_r r s f_t - 6 f_b^4 f_r f_s^5 f_r r s f_a + 128 f_b f_r^3 f_s^2 f_r r s f_t^3 \\
& + 256 f_b f_s f_r^5 f_t^2 f_a t - 384 f_a f_t^4 f_b^2 f_r^3 f_r r r - 8 f_t f_r f_a r f_r t f_s^6 - 640 f_t^3 f_r^4 f_a r f_r t f_b^2 - 768 f_t^4 \\
& f_r^3 f_a r f_r t f_a^2 + 640 f_t^3 f_r^3 f_a r f_r t f_s^2 - 128 f_t^2 f_r^4 f_a r f_r t f_b^4 - 192 f_t^4 f_r^2 f_a r f_r t f_a^4 + 768 f_a f_t^4 f_b^2 \\
& f_r^4 f_a a r + 256 f_b f_r^4 f_r s f_r t f_t^3 - 96 f_r^3 f_t^3 f_a r f_r r f_b^4 - 48 f_a f_t^2 f_r^2 f_s^5 f_a a s - 128 f_b^3 f_a s f_a t f_r^5 f_t^2 \\
& - 16 f_b^5 f_a s f_a t f_r^5 f_t - 256 f_b f_a s f_a t f_r^5 f_t^3 - 128 f_a f_t^3 f_r^3 f_r r t f_s^2 - 24 f_a^5 f_t^3 f_r f_r r t f_s^2 + 48 f_a^3 \\
& f_t^2 f_r f_r r t f_s^4 + 96 f_a f_t^2 f_r^2 f_r r t f_s^4 - 96 f_a^3 f_t^3 f_r^2 f_r r t f_s^2 + 96 f_s^4 f_b r f_r s f_r^2 f_t^2 - 24 f_s^6 f_b r f_r s f_r f_t \\
& - 128 f_s^2 f_b r f_r s f_r^3 f_t^3 + 256 f_s f_r t f_a s f_r^4 f_t^3 - 24 f_r f_t^3 f_a r r f_s^4 f_a^2 - f_b^7 f_s^2 f_r^3 f_r s f_a a - 8 f_t^3 f_a^5 \\
& f_a^2 s f_r f_s^2 + 16 f_t^2 f_a^3 f_a^2 s f_r f_s^4 - 64 f_t^3 f_a^3 f_a^2 s f_r^2 f_s^2 + 256 f_s^3 f_a f_a b r f_r^3 f_t^3 + 144 f_s^3 f_a^3 f_a b r f_r^2 f_t^3 \\
& - 36 f_s^5 f_a^3 f_a b r f_r f_t^2 - 24 f_a^3 f_t^3 f_r r r f_r^2 f_b^4 + f_b^6 f_s^3 f_r^3 f_a a f_b r - 24 f_a^5 f_t^4 f_r r r f_r f_b^2 - 8 f_b^6 f_r^3 \\
& f_t^2 f_a r f_r r + 32 f_t^2 f_a f_a^2 s f_r^4 f_b^4 + 64 f_t^2 f_a f_a^2 s f_r^2 f_s^4 + 64 f_t^3 f_a f_a^2 s f_r^4 f_b^2 - 128 f_t^3 f_a f_a^2 s f_r^3 f_s^2 + 96 \\
& f_a^3 f_t^3 f_s^4 f_a a r f_r + 4 f_b^7 f_s f_r^3 f_t f_r r r - 96 f_s^5 f_a f_a b r f_r^2 f_t^2 + 24 f_s^3 f_a^5 f_a b r f_r f_t^3 + 16 \\
& f_s^7 f_a f_a b r f_r f_t + 128 f_b^3 f_r^4 f_r s f_r t f_t^2 + 16 f_b^5 f_r^4 f_r s f_r t f_t - 192 f_a^3 f_t^4 f_r r r f_r^2 f_b^2 - 16 f_b^2 f_s^5 \\
& f_r^2 f_a t f_r s - 8 f_t f_a f_a^2 s f_r f_s^6 - f_b^6 f_s^2 f_r^2 f_r^2 s f_a - f_b^6 f_s^3 f_r^2 f_a s f_r r + 8 f_b^6 f_s f_r^5 f_a t f_a b - 4 f_t^2 f_a f_b^6 f_a^2 r \\
& f_r^3 + 24 f_b f_s^5 f_r^2 f_t f_b^2 r + 128 f_b^3 f_s f_r^5 f_t f_a t - 4 f_b^3 f_s^5 f_a^2 f_r f_b^2 r - 4 f_a^5 f_r^2 s f_t^3 f_r f_b^2 + 256 f_b f_s f_r^4
\end{aligned}$$

$$\begin{aligned}
& f_t^3 f_{r,r,t} + 192 f_a^3 f_t^4 f_r^2 f_s f_{r,r,s} - 24 f_a^6 f_t^4 f_{a,r,r} f_r f_b^2 - 12 f_b^5 f_s^2 f_r^4 f_{a,s} f_{a,t} + f_b^5 f_s^4 f_r^2 f_{a,b} f_{r,r} - 32 \\
& f_a^3 f_r^2 f_s^3 f_r^2 f_b^2 + 64 f_a^3 f_r^2 f_s^3 f_r f_s^2 - 8 f_a^3 f_r^2 f_s^3 f_r^2 f_b^4 + 256 f_{a,b} f_r^5 f_{r,t} f_b f_t^3 + 128 f_{a,b} f_r^5 f_{r,t} f_b^3 f_t^2 \\
& - 4 f_{a,b} f_r^4 f_{r,t} f_b^5 f_s^2 + 192 f_a^4 f_t^4 f_r^2 f_{a,r,s} f_s + 128 f_b f_s f_r^4 f_t^3 f_b^2 f_{r,r} + 512 f_s f_{r,s} f_r^3 f_t^4 f_{a,r} + 128 f_b \\
& f_s^3 f_r^3 f_t^2 f_{r,r} - 384 f_s^3 f_{r,s} f_r^2 f_t^3 f_{a,r} - 2 f_{a,t}^2 f_a^7 f_r f_s^2 f_t^2 - 2 f_{a,t}^2 f_a^5 f_r f_s^4 f_b^2 - 4 f_{a,t}^2 f_a^4 f_r f_s^5 f_b + 4 f_{a,t}^2 \\
& f_a^5 f_r^4 f_s f_t + 8 f_{a,t}^2 f_a^4 f_r^2 f_s^3 f_b^3 - 10 f_{a,t}^2 f_a^3 f_r^3 f_s^2 f_b^4 - 12 f_b^5 f_s^3 f_r^3 f_{a,r,t} + 2 f_b^5 f_s^4 f_r^2 f_{r,s} f_{a,a} - 4 \\
& f_b^7 f_s f_r^4 f_{a,a,r} f_t + 8 f_b^6 f_s f_r^4 f_{a,s} f_{r,t} - 4 f_{a,b} f_r^2 f_{r,t} f_b f_s^6 - 32 f_a^6 f_t^5 f_{a,a} f_r f_{a,r} + 96 f_b^2 f_s^3 f_r^3 \\
& f_t^2 f_a f_{a,b} f_{a,a} + 96 f_a^2 f_s^3 f_{r,t} f_b f_{r,r} f_t^2 - 12 f_a^2 f_s f_{r,t} f_b^5 f_{r,r} f_r^2 f_t - 80 f_t^2 f_r f_{a,r} f_{r,t} f_s^3 f_b f_a^3 + 64 f_t^2 \\
& f_r^3 f_{a,r} f_{r,t} f_b^3 f_a f_s + 192 f_t^3 f_r^2 f_{a,r} f_{r,t} f_b f_a^3 f_s + 144 f_t^2 f_r^2 f_{a,r} f_{r,t} f_b^2 f_a^2 f_s^2 + 576 f_r^2 f_t^4 f_{a,a} f_b f_s \\
& f_a^2 f_{r,r} + 120 f_b^3 f_a^2 f_{r,s} f_t^2 f_{r,r} f_r f_s^2 - 24 f_a^4 f_t^2 f_b^2 f_s^2 f_r^2 f_b, r f_{a,b} - 4 f_a^3 f_t f_b^4 f_s f_r^2 f_{r,s} f_{r,t} - 96 f_a^2 f_t^2 \\
& f_b^2 f_r^3 f_{a,b} f_b, r f_s^2 - 64 f_t^3 f_{a,t} f_{a,a} f_r^3 f_b f_a^3 f_s + 192 f_a^2 f_t^3 f_b^2 f_r^3 f_{a,s} f_{a,a} f_s - 48 f_b f_s^5 f_r f_{a,t} f_b, r f_{r,s} \\
& - 4 f_b^4 f_s^2 f_r^3 f_t f_a f_{a,b} f_{r,s} - 28 f_b^4 f_s^3 f_r^2 f_t f_{r,s} f_{a,a} f_a - 20 f_a^5 f_t^3 f_{a,s} f_{a,a} f_s^2 f_b f_r - 128 f_a^3 f_t^3 f_b f_s \\
& f_r^2 f_b, r f_{r,s} + 16 f_a^4 f_t^2 f_s^3 f_{a,a} f_r f_b f_{r,t} - 192 f_b f_s^2 f_a f_b, r f_{r,r} f_r^2 f_t^3 + 64 f_a^2 f_t^2 f_b^3 f_r^3 f_{a,a} f_s f_{r,t} + 30 f_t^2 \\
& f_a^4 f_{a,b} f_s^2 f_b^3 f_r f_{r,r} + 12 f_t f_{a,t} f_{a,a} f_r^2 f_s^4 f_b^2 f_a^2 - 48 f_a^2 f_s^3 f_{r,t} f_b^3 f_{r,r} f_r f_t - 28 f_a^4 f_s f_{r,t} f_b^3 f_{r,r} f_r f_t^2 \\
& + 8 f_a^5 f_t^2 f_b f_s^3 f_{a,b} f_{a,s} f_r - 16 f_a^4 f_t^2 f_b^4 f_r f_{r,s} f_{a,r} f_s - 32 f_b^2 f_a^3 f_{r,s} f_t^3 f_{r,r} f_r f_s + 384 f_b f_a^2 f_{r,s} \\
& f_t^3 f_{r,r} f_r f_s^2 + 240 f_b f_s^2 f_r^2 f_t^2 f_a f_{r,s} f_{a,t} + 192 f_b^2 f_s f_r^4 f_t^2 f_a f_{a,t} f_b, r + 192 f_b f_s^2 f_r^3 f_t^3 f_a f_{a,s} f_{a,a} \\
& + 9 f_{a,b} f_s^2 f_r^2 f_b^5 f_a^2 f_{r,r} - 20 f_{a,b} f_s^2 f_r^3 f_b^5 f_a f_t f_{a,r} - 6 f_t f_a^3 f_{a,b} f_s^3 f_b^4 f_r f_{r,r} - 28 f_a^3 f_t f_b^3 \\
& f_s^3 f_r f_{r,s} f_b, r + 60 f_a^2 f_t f_b^4 f_s^2 f_r^2 f_{a,r} f_{r,t} + 2 f_a^4 f_t f_b^3 f_s^2 f_r f_{r,s} f_{r,t} - 128 f_t^3 f_{a,t} f_{a,a} f_r^4 f_b f_a f_s + 80 \\
& f_t^2 f_{a,t} f_{a,a} f_r^2 f_s^3 f_b f_a^3 + 24 f_b^4 f_s^2 f_r^2 f_t f_{r,s} f_a^2 f_{a,s} - 576 f_a^2 f_s f_{r,t} f_b f_{r,r} f_r^2 f_t^3 - 192 f_a^2 f_s f_{r,t} f_b^3 f_{r,r} f_r^2 \\
& f_t^2 - 192 f_a^4 f_s f_{r,t} f_b f_{r,r} f_r f_t^3 + 48 f_a^2 f_t f_b^4 f_s^2 f_r^2 f_{r,s} f_b, r - 4 f_{a,b} f_s f_r^3 f_b^6 f_a f_t f_{r,r} - 4 \\
& f_s^6 f_{a,b} f_{a,r} f_r f_t f_b f_a - 48 f_s^4 f_{a,b} f_{a,r} f_r^2 f_t^2 f_b f_a - 12 f_a^4 f_t f_b^4 f_r^2 f_{r,s} f_{a,t} f_s + 20 f_a^3 f_s^2 f_{r,t} f_b^4 f_{r,r} f_r f_t \\
& + 144 f_a^3 f_s^2 f_{r,t} f_b^2 f_{r,r} f_r f_t^2 - 48 f_b f_s^4 f_r^2 f_t^2 f_a f_{a,s} f_{a,a} - 48 f_b^5 f_s f_r^2 f_t^2 f_{a,r} f_a f_{r,r} - 52 f_b^4 f_s^2 \\
& f_r^3 f_t f_{a,a} f_a f_{r,t} - 96 f_t^2 f_a^3 f_{a,b} f_s^2 f_b^3 f_r^2 f_{a,r} + 48 f_b f_s^4 f_a f_b, r f_{r,r} f_r f_t^2 + 64 f_a^3 f_t^3 f_b f_s f_r^3 f_b, r f_{a,b} \\
& + 192 f_b^2 f_s f_r^4 f_t^2 f_a f_{a,s} f_{a,t} - 6 f_b^2 f_s^5 f_a^2 f_{a,s} f_{a,a} f_t f_r - 26 f_b^4 f_{a,s} f_{a,r} f_r f_s^3 f_a f_t - 64 f_b^4 f_{a,s} f_{a,r} f_r^3 \\
& f_t^2 f_a f_s + 76 f_b^3 f_{a,s} f_{a,r} f_r f_s^2 f_a f_t^2 - 12 f_b^6 f_{a,s} f_{a,r} f_r^3 f_t f_a f_s - 80 f_b^4 f_{a,s} f_{a,r} f_r^2 f_t^2 f_a f_s + 30 \\
& f_b^5 f_{a,s} f_{a,r} f_r^2 f_t f_a^2 f_s^2 - 4 f_b^4 f_s^2 f_r^3 f_t f_b, r f_a f_{a,s} + 128 f_s^3 f_t^3 f_{a,r} f_{r,r} f_r f_b f_a + 144 f_s^2 f_t^3 f_{a,r} f_{r,r} f_r f_b^2 f_a^2 \\
& + 10 f_a^2 f_t f_s^6 f_b f_{a,b} f_{a,a} f_r - 144 f_t^2 f_{a,t} f_{a,a} f_r^3 f_b^2 f_a^2 f_s^2 + 96 f_t^2 f_{a,t} f_{a,a} f_r^3 f_b f_a f_s^3 + 12 f_b^5 \\
& f_s^2 f_a f_b, r f_{r,r} f_r f_t^2 - 240 f_b f_s^2 f_r^2 f_t^2 f_a^2 f_{a,b} f_{r,r} + 96 f_b^3 f_s^2 f_r^3 f_t f_a f_b, r f_{r,t} + 48 f_b^3 f_s^3 f_r^2 f_t f_a f_{r,s} f_b, r \\
& - 12 f_b^2 f_s^4 f_a^2 f_{r,s} f_{a,s} f_r f_t - 12 f_a^6 f_t^3 f_{a,r,s} f_s^3 - 3 f_s^5 f_a^5 f_{a,b,r} f_t^2 - 3 f_s^7 f_a^3 f_{a,b,r} f_b^2 - 3 f_s^8 \\
& f_a^2 f_{a,b,r} f_b + 3 f_s^7 f_a^3 f_{a,b,r} f_t - 18 f_a^4 f_t^3 f_s^4 f_{a,r,r} + 8 f_t^4 f_a^7 f_{r,t} f_{r,r} + 4 f_a^7 f_t^4 f_s f_{r,r,s} - 12 f_a^5 f_t^3
\end{aligned}$$

$$\begin{aligned}
& f_s^3 f_{r,r,s} - 2 f_t^3 f_a^8 f_{a,r,t} f_s^2 + 8 f_a^5 f_r^2 f_t^3 f_s^2 - 16 f_a^3 f_r^2 f_t^2 f_s^4 - f_{a,t} f_a f_s^8 f_{a,r} - 8 f_s^7 f_{r,s} f_t f_{a,r} \\
& - 2 f_{b,r} f_{a,t} f_a^3 f_s^7 + 3 f_b^5 f_r^2 f_s^4 f_{r,r,s} - 3 f_b^3 f_r f_s^6 f_{r,r,s} + 48 f_b^5 f_r^5 f_{a,a,s} f_t^2 - 12 f_b^5 f_s^3 f_r^3 f_{r,r,t} \\
& + 16 f_a^7 f_t^5 f_{a,a,r} f_r + 32 f_b^3 f_s^3 f_r^3 f_{r,t}^2 - 32 f_b^3 f_s^3 f_r^4 f_{a,t}^2 + 512 f_{a,t} f_t^4 f_r^4 f_{r,r} - 1024 f_t^4 f_r^4 f_{a,r} f_{r,t} \\
& + 22 f_a^6 f_t^4 f_{a,r,r} f_s^2 + 4 f_a^8 f_t^4 f_{a,r,s} f_s - 6 f_a^3 f_t^2 f_s^6 f_{a,a,r} + 6 f_a^5 f_t^3 f_{a,a,r} f_s^4 + 12 f_a^3 f_t^2 f_s^5 f_{r,r,s} \\
& - f_{r,s} f_{a,t} f_a^2 f_s^7 + 8 f_t^4 f_{a,t} f_a^8 f_{r,r} + f_s^3 f_a^7 f_t^3 f_{a,b,r} + 24 f_s^2 f_a^5 f_t^4 f_{r,r,r} + 8 f_s^6 f_a f_t^2 f_{r,r,r} - 24 f_s^4 f_a^3 \\
& f_t^3 f_{r,r,r} - f_b^2 f_s^7 f_{a,s} f_{r,r} + 2 f_{a,b}^2 f_s^7 f_r^2 f_b + 256 f_t^4 f_{a,a,b} f_s^5 f_r + 8 f_{a,r} f_r^2 f_s^6 - 48 f_b^5 f_r^4 f_{r,r,s} f_t^2 - \\
& f_b^7 f_r^3 f_{r,r,s} f_s^2 - 4 f_b^7 f_r^4 f_{r,r,s} f_t - 192 f_b^3 f_r^4 f_{r,r,s} f_t^3 - 512 f_r^3 f_t^4 f_{a,r,r} f_s^2 - 16 f_b^5 f_s^4 f_r^4 f_{r,t}^2 + 4 f_b^7 f_s \\
& f_r^4 f_{r,r,t} - 4 f_b^7 f_s f_r^5 f_{a,a,t} + 16 f_b f_s^5 f_r^3 f_{a,t}^2 - 256 f_t^4 f_b f_r^4 f_{r,r,s} - 8 f_b^6 f_r^5 f_t^2 f_{a,a,a} + f_b^6 f_s^3 f_r^3 f_{b,r,r} \\
& - 3 f_s^5 f_r^2 f_{b,r,r} f_b^4 + 3 f_s^7 f_r f_{b,r,r} f_b^2 - 384 f_b^2 f_r^5 f_t^4 f_{a,a,a} + f_b^4 f_s^5 f_a^4 f_{a,r,s} + 4 f_s^7 f_{a,s} f_t f_{r,r} - 96 \\
& f_b^4 f_s^5 f_t^3 f_{a,a,a} + 2 f_b^5 f_s^3 f_{a,s} f_r^2 - 4 f_b^3 f_s^5 f_{a,s} f_r^2 - f_s^8 f_{a,a,b} f_r - 2 f_b^5 f_r^2 f_s^3 f_{r,s}^2 + 4 f_b^3 f_r f_s^5 f_{r,s}^2 + 8 \\
& f_b^6 f_r^4 f_t^2 f_{a,r,r} + 2 f_b f_s^7 f_{a,s} f_r - 88 f_a^6 f_t^5 f_{a,r,r} f_r + 4 f_{a,t} f_{a,b} f_s^7 f_r^2 - 4 f_s^7 f_{r,t} f_{a,s} f_r - 4 f_{a,b}^2 f_s^5 f_r^3 \\
& f_b^3 + f_a f_{a,a} f_s^8 f_{r,t} + 6 f_a^3 f_s^6 f_{r,r,t} f_b^2 + 6 f_a^2 f_s^7 f_{r,r,t} f_b - 6 f_a^3 f_s^6 f_{r,r,t} f_t + 48 f_a^6 f_t^5 f_{a,r} f_{r,r} + 3 f_b^3 \\
& f_s^6 f_{r,r,s} f_a^2 + 3 f_b^2 f_s^7 f_{r,r,s} f_a - 2 f_a^7 f_t^3 f_{r,r,t} f_s^2 + f_s^8 f_a f_{a,b} f_{r,s} - 3 f_s^7 f_{r,t} f_a^2 f_{a,s} + f_s^4 f_a^5 f_{b,r}^2 f_t^2 + \\
& f_s^6 f_a^3 f_{b,r}^2 f_b^2 + 2 f_s^7 f_a^2 f_{b,r}^2 f_b + f_b^3 f_s^6 f_{r,s} f_{r,r} - 4 f_{a,t} f_s^7 f_{r,r,s} + 2 f_a^5 f_s^5 f_b^3 f_{a,r,t} + f_b f_s^8 f_{a,b} f_{r,r} \\
& + 12 f_a^4 f_t^2 f_s^5 f_{a,r,s} - f_b^4 f_s^4 f_a^3 f_{r,s}^2 - 256 f_{a,a,b} f_s^3 f_r^4 f_t^3 + 96 f_{a,a,b} f_s^5 f_r^3 f_t^2 - 16 f_{a,a,b} f_s^7 f_r^2 f_t \\
& - 2 f_s^8 f_t f_{a,a,a} f_r + 512 f_s^2 f_t^4 f_{a,a,a} f_r^4 - 192 f_s^4 f_t^3 f_{a,a,a} f_r^3 + 32 f_s^6 f_t^2 f_{a,a,a} f_r^2 - 16 f_b f_s^5 f_r^2 f_{r,t}^2 \\
& - 96 f_s^5 f_r^2 f_t^2 f_{b,r,r} - 256 f_s f_r^4 f_t^4 f_{b,r,r} + 192 f_a^5 f_t^5 f_{a,a,r} f_r^2 + 256 f_b f_r^5 f_t^4 f_{a,a,s} - 512 f_r^3 \\
& f_t^5 f_{a,r} f_{r,r} + 2 f_{a,b}^2 f_s^3 f_r^4 f_b^5 - 96 f_a^5 f_t^5 f_{r,r,r} f_r - 384 f_a^3 f_t^5 f_{r,r,r} f_r^2 + 256 f_a^3 f_t^5 f_{r,r} f_r + 512 f_a f_t^5 \\
& f_{r,r}^2 f_r^2 - 2 f_b^5 f_s^3 f_r^3 f_{b,r}^2 - 32 f_a^5 f_t^4 f_{a,r} f_s^2 + 8 f_{a,t} f_s^6 f_{r,s}^2 + 2 f_{a,t} f_s^8 f_{a,a,r} - 3 f_b f_s^8 f_a f_{b,r,r} - f_b^3 f_s^6 \\
& f_a^3 f_{b,r,r} - 3 f_b^2 f_s^7 f_a^2 f_{b,r,r} + f_s^8 f_a^2 f_{a,b} f_{b,r} + 6 f_a^6 f_s^4 f_{a,r,t} f_t^2 + 6 f_a^4 f_s^6 f_{a,r,t} f_b^2 + 6 f_a^3 f_s^7 f_{a,r,t} f_b \\
& - 6 f_a^4 f_s^6 f_{a,r,t} f_t + 3 f_b^2 f_s^7 f_a^2 f_{a,r,s} - f_s^7 f_{b,r} f_{r,r} f_b^2 - 4 f_s^7 f_{b,r} f_{r,r} f_t + 6 f_a^5 f_s^4 f_{r,r,t} f_t^2 + 3 f_s^7 \\
& f_a^2 f_t f_{b,r,r} + f_s^3 f_a^6 f_t^3 f_{b,r,r} - 3 f_s^5 f_a^4 f_t^2 f_{b,r,r} - f_s^7 f_{r,t} f_a^3 f_{a,b} + f_b f_s^8 f_a f_{a,r,s} - 3 f_s^7 f_{r,t} f_a^2 f_{b,r} \\
& - 4 f_b f_s^7 f_t f_{r,r,r} + 3 f_b^3 f_s^6 f_a^3 f_{a,r,s} - 4 f_b^3 f_s^5 f_{r,r} f_t + 2 f_{a,t} f_a^4 f_{r,t} f_s^6 + 16 f_a^3 f_t^3 f_{a,r} f_s^4 + 8 f_s^6 \\
& f_t^2 f_{a,r} f_{r,r} + 96 f_a^5 f_t^5 f_{a,r} f_r + f_s^8 f_a f_{b,r} f_{a,s} + 32 f_a f_t^3 f_{r,r} f_s^4 - 64 f_a^3 f_t^4 f_{r,r} f_s^2 + 2 f_a^2 f_t^2 f_s^6 f_{a,r,r} \\
& - 4 f_b^3 f_s^5 f_{r,s} f_a^2 - 5 f_b^2 f_s^6 f_{r,s} f_a - f_b^3 f_s^6 f_a^4 f_{a,b,r} + 2 f_a^7 f_{r,t} f_s^2 f_t^2 + f_b^4 f_s^5 f_a^3 f_{r,r,s} - 2 f_a^7 f_t^4 f_{a,a,r} \\
& f_s^2 + 16 f_b^5 f_s f_r^5 f_{a,t}^2 + 96 f_r^4 f_t^3 f_{a,r,r} f_b^4 - 288 f_r^2 f_t^5 f_{a,r,r} f_a^4 + 192 f_r^2 f_t^3 f_{a,r,r} f_s^4 - 32 f_r f_t^2 f_{a,r,r} \\
& f_s^6 + 384 f_r^4 f_t^4 f_{a,r,r} f_b^2 - 128 f_r^3 f_t^5 f_{a,r,r} f_a^2 + f_b^7 f_r^4 f_{a,a,s} f_s^2 - 3 f_b^5 f_r^3 f_{a,a,s} f_s^4 + 4 f_b^7 f_r^5 f_{a,a,s} f_t \\
& - 2 f_a f_s^8 f_{a,a,t} f_r + 12 f_b^3 f_s^5 f_r^2 f_{r,r,t} + 512 f_t^4 f_{a,t} f_{a,a} f_r^5 + 16 f_s^7 f_r f_t f_{b,r,r} + 256 f_s^3 f_r^3 f_t^3 f_{b,r,r} \\
& - 384 f_r^4 f_t^5 f_{a,a,a} f_a^2 - 96 f_r^3 f_t^5 f_{a,a,a} f_a^4 + 512 f_t^5 f_{a,a} f_{a,r} f_r^4 + 768 f_a^3 f_t^5 f_r^3 f_{a,a,r} + 3 f_b^3
\end{aligned}$$

$$\begin{aligned}
& f_r^2 f_{a,a,s} f_s^6 + 192 f_b^3 f_r^5 f_{a,a,s} f_t^3 - 2 f_{a,t}^2 f_s^3 f_r f_s^6 + 4 f_b f_s^7 f_r^2 f_{a,a,t} - 12 f_b^3 f_s^5 f_r^3 f_{a,a,t} - 8 f_{a,t}^2 f_a \\
& f_r^2 f_s^6 - 4 f_b f_s^7 f_r f_{r,r,t} - f_b f_s^8 f_{a,a,s} f_r - 2 f_b f_s^7 f_r f_b^2 r - 3 f_{a,a,b} f_s^7 f_r^2 f_b^2 - f_{a,a,b} f_s^3 f_r^4 f_b^6 \\
& + 3 f_{a,a,b} f_s^5 f_r^3 f_b^4 + 128 f_a^3 f_t^5 f_{a,a}^2 f_r^3 + 16 f_a^5 f_t^5 f_{a,a}^2 f_r^2 + 256 f_a f_t^5 f_{a,a}^2 f_r^4 + 4 f_b^3 f_s^5 f_r^2 f_b^2 r + 12 \\
& f_b^5 f_s^3 f_r^4 f_{a,a,t} + 4 f_r f_{a,t} f_s^7 f_{r,s} - 4 f_s^7 f_{r,t} f_b r f_r - 2 f_s^8 f_{a,b} f_{a,s} f_r - 8 f_a^6 f_t^5 f_{a,a} f_r^2 - 512 f_a f_t^5 \\
& f_r^3 f_{r,r,r} + 1024 f_a f_t^5 f_r^4 f_{a,a,r} - 512 f_a f_t^5 f_{a,r}^2 f_r^3 - 16 f_b f_s^5 f_t^2 f_{r,r}^2 - 2 f_s^6 f_a^3 f_b^2 r f_t + 8 f_b^2 f_a^5 f_t^4 f_{r,r}^2 \\
& - 4 f_s^7 f_{r,t} f_a f_{r,s} + 2 f_a^4 f_b^3 f_s^5 f_{r,r,t} + 2 f_b f_s^7 f_{a,r}^2 f_t - 4 f_a^2 f_t f_s^7 f_{a,r,s} + 2 f_a^5 f_{r,t}^2 f_b^4 f_r^2 + 4 f_a^4 f_{r,t}^2 \\
& f_s^5 f_b - 4 f_a^5 f_{r,t}^2 f_s^4 f_t + 16 f_b f_s^5 f_{r,r} f_{a,t} f_r f_a f_t - 24 f_a^2 f_t f_b^3 f_s^2 f_r^3 f_{a,s} f_{a,t} + 8 f_a^4 f_t f_b^3 f_s^3 f_{a,a} f_r f_{r,t} \\
& + 60 f_a^4 f_t^2 f_s^2 f_b f_r f_{r,s} f_{r,t} - 24 f_a^4 f_t^2 f_b^2 f_s^2 f_{a,a} f_{a,t} f_r^2 + 32 f_a^3 f_t f_b^2 f_s^3 f_r^2 f_{a,s} f_{a,t} + 12 f_b^2 f_s^4 f_a \\
& f_r^2 f_{r,s} f_{a,b} + 96 f_a^2 f_t^2 f_b f_s^3 f_{a,s} f_b r f_r^2 - 8 f_a^3 f_t f_b^5 f_s f_r^2 f_{a,r} f_{r,t} + 30 f_a^4 f_t^2 f_s^2 f_b^2 f_r f_{a,r} f_{r,t} - 240 \\
& f_a^3 f_t^3 f_{a,r} f_{r,r} f_r f_b^3 f_s + 256 f_b f_s^3 f_r^2 f_t^2 f_{a,a} f_{t,r,r} - 10 f_b^3 f_s^4 f_a^2 f_r^2 f_t f_{a,b} f_{a,a} - 48 f_b^2 f_s^2 f_r^3 \\
& f_t^2 f_{a,a} f_a f_{r,t} + 320 f_b f_s^2 f_r^3 f_t^3 f_a f_{a,b} f_{a,r} + 16 f_s^3 f_t^2 f_{a,r} f_{r,r} f_r f_b^3 f_a + 4 f_a^6 f_t^2 f_b^2 f_s f_r f_{a,s} f_{r,t} - 9 f_a^4 \\
& f_t^2 f_s^4 f_b f_{a,b} f_{a,a} f_r - 96 f_a^3 f_t^2 f_b^2 f_r^3 f_s f_{a,b} f_{r,t} - 24 f_a^5 f_t^2 f_s^2 f_b f_r f_{a,s} f_{r,t} - 12 f_a^2 f_t f_b^6 f_r^2 f_{r,s} f_{a,r} f_s \\
& + 12 f_a^5 f_t^2 f_b^2 f_s f_r^2 f_{a,t} f_b r - 24 f_t f_{a,t} f_{a,a} f_r^2 f_s^5 f_b f_a + 48 f_t f_{a,t} f_{a,a} f_r^3 f_s^3 f_b^3 f_a + 10 f_b^5 f_s^3 \\
& f_r^2 f_a f_{a,r} f_{a,a} f_t - 256 f_b f_s f_r^4 f_t^2 f_a f_{a,t} f_{r,t} - 192 f_b f_s f_r^3 f_t^2 f_a^3 f_{a,t} f_{r,t} + 14 f_b^3 f_b r f_r f_t f_{a,r} f_s^4 f_a^2 \\
& + 24 f_b^2 f_b r f_r f_t f_{a,r} f_s^5 f_a + 36 f_b f_b r f_r f_t^2 f_{a,r} f_s^4 f_a^2 - 48 f_b f_b r f_r^2 f_t^3 f_{a,r} f_a^2 f_s^2 - 192 f_b \\
& f_s^4 f_a f_{a,s} f_{r,r} f_r f_t^2 + 24 f_b^5 f_s^2 f_a f_{a,s} f_{r,r} f_r^2 f_t - 18 f_s^3 f_{r,t} f_b^4 f_b r f_r f_t f_b^2 - 44 f_t^3 f_a^5 f_{a,b} f_s^2 f_b f_r f_{a,r} \\
& + 22 f_t^2 f_a^4 f_{a,b} f_s^3 f_b^2 f_r f_{a,r} + 128 f_a^3 f_t^3 f_b^2 f_s f_r^2 f_{r,s} f_{a,a} + 16 f_a^5 f_t^3 f_{a,b} f_{a,s} f_s^2 f_r^2 f_b - 48 f_a^2 f_t^2 f_{a,a} \\
& f_b^4 f_s^2 f_r^2 f_{a,r} - 46 f_b^4 f_s^3 f_a^2 f_{a,s} f_{r,r} f_r f_t - 4 f_a^2 f_t^2 f_b^4 f_s f_r^3 f_b r f_{a,a} - 48 f_b^2 f_s^4 f_a^2 f_r f_t f_b r f_{r,s} - 64 f_a^3 f_t \\
& f_b^3 f_s f_r^3 f_{a,t} f_{r,t} + 52 f_a^2 f_t f_b^4 f_s f_r^3 f_{a,s} f_{r,t} - 8 f_a^5 f_t f_b^3 f_s f_r^2 f_{a,t} f_{r,t} + 24 f_a^2 f_t f_b^3 f_s^2 f_r^2 f_{r,s} f_{r,t} - 96 f_a^2 \\
& f_t^2 f_b^3 f_s f_r^3 f_{r,s} f_{a,b} + 14 f_a^3 f_t f_b^4 f_s^3 f_r f_{r,s} f_{a,a} + 24 f_a^3 f_t f_b^4 f_s^2 f_r^2 f_{a,b} f_{r,s} - 20 f_b^4 f_b r f_r^2 f_t f_{a,r} f_s^3 f_a \\
& - 16 f_b^2 f_b r f_r f_t^2 f_{a,r} f_s^3 f_a^3 + 12 f_a^4 f_t f_b^4 f_s^2 f_r f_{a,r} f_{r,t} - 8 f_a^5 f_t f_b^2 f_s^3 f_r f_{a,b} f_{r,t} - 38 f_a^4 f_t f_b^2 \\
& f_s^3 f_{r,s} f_{a,t} f_r + 24 f_a^3 f_t f_b^4 f_s^2 f_r^2 f_b r f_{a,s} - 7 f_a^6 f_t^2 f_b f_s^2 f_{a,s} f_{a,t} f_r + 34 f_b^3 f_s^4 f_a^2 f_r f_t f_{r,s} f_{a,a} - 30 \\
& f_a^2 f_t f_b^4 f_s^2 f_r^3 f_{a,a} f_{a,t} + 12 f_b f_s^4 f_r^2 f_t f_a^2 f_{a,t} f_b r - 192 f_b^2 f_s f_r^3 f_t^2 f_a f_{r,s} f_{r,t} - 16 f_{a,b} f_s f_r^3 f_b^4 f_a f_t^2 f_{r,r} \\
& - 120 f_a^2 f_t^2 f_b^2 f_s^2 f_r^2 f_{r,s} f_{a,a} - 24 f_a^4 f_t^2 f_b^3 f_s f_r^2 f_{a,s} f_b r + 72 f_a^3 f_t^2 f_b^2 f_s^2 f_{a,s} f_b r f_r^2 + 72 f_b^3 f_s^2 \\
& f_a^3 f_{a,s} f_{r,r} f_r f_t^2 + 22 f_a^4 f_t f_b f_s^4 f_{a,t} f_b r f_r - 14 f_a^4 f_t f_b^3 f_s^3 f_r f_{a,b} f_{r,s} + 16 f_a^5 f_t^2 f_b^3 f_r f_{r,s} f_s f_{a,s} + 40 \\
& f_b^3 f_s^2 f_r^3 f_t f_a^2 f_{a,t} f_b r + 6 f_a^5 f_t^2 f_b f_s^3 f_{a,b} f_b r f_r - 12 f_a^5 f_t^2 f_b^2 f_s f_r^2 f_{a,b} f_{r,t} + 8 f_a^5 f_t^3 f_b f_s f_r^2 f_b r f_{a,b} \\
& + 24 f_a^5 f_t^3 f_b f_s f_{r,s} f_{a,s} f_r - 44 f_a^4 f_t^3 f_s^2 f_b f_r f_{r,s} f_{a,a} - 36 f_t^2 f_a^3 f_{a,b} f_s f_b^4 f_r^2 f_{r,r} - 12 f_a^5 f_t^2 \\
& f_b^2 f_s f_r f_{r,s} f_{r,t} - 576 f_a^3 f_t^4 f_{a,r} f_{r,r} f_r f_b f_s - 24 f_a^2 f_t^2 f_b^2 f_s^3 f_{a,s} f_{a,a} f_r^2 + 48 f_b^4 f_b r f_r^3 f_t^2 f_{a,r} f_a f_s \\
& - 24 f_b^3 f_b r f_r^2 f_t^2 f_{a,r} f_a^2 f_s^2 - 144 f_b^2 f_b r f_r^2 f_t^2 f_{a,r} f_a f_s^3 + 256 f_b^2 f_b r f_r^3 f_t^3 f_{a,r} f_a f_s + 20 f_b f_b r f_r
\end{aligned}$$

$$\begin{aligned}
& f_t^3 f_a r f_s^2 f_a^4 - 24 f_{a,b} f_s^2 f_r^2 f_b^3 f_a^2 f_t^2 f_r - 4 f_{a,b} f_s^4 f_r f_b^3 f_a^2 f_t f_r + 24 f_{a,b} f_s^4 f_r^2 f_b^3 f_a f_t f_a r \\
& + 12 f_{a,b} f_s^3 f_r^2 f_b^4 f_a f_t f_r - 24 f_a^2 f_t f_b^5 f_s^2 f_r^2 f_r s f_a - 64 f_a^4 f_t^3 f_b f_s f_r^2 f_r s f_a b + 384 f_b \\
& f_s^2 f_a f_a s f_r r f_r^2 f_t^3 + 192 f_b^3 f_s^2 f_a f_a s f_r r f_r^2 f_t^2 + 416 f_b f_s^2 f_a^3 f_a s f_r r f_r f_t^3 + 24 f_a^2 f_t f_b^3 f_s^3 f_r^2 f_r s f_a b \\
& + 96 f_a^3 f_t^2 f_b^2 f_r^3 f_a s f_a t f_s - 32 f_a^3 f_t f_b^2 f_s^3 f_r f_r s f_r t + 16 f_b^6 f_s f_r^3 f_a f_t f_r s f_a a - 14 f_a^4 f_t f_b^4 \\
& f_s^2 f_r f_r s f_a s + 12 f_b^2 f_s^4 f_a f_a s f_b r f_r^2 f_t - 24 f_b^5 f_s f_r^3 f_t f_a f_a r f_r t - 96 f_b^3 f_s^2 f_r^3 f_t f_a f_a s f_r t + 56 f_b^3 \\
& f_s^2 f_r^3 f_t f_a^2 f_a b f_r t + 160 f_b^3 f_s^2 f_r^3 f_t f_a f_r s f_a t - 24 f_b^4 f_s^3 f_r s f_r r f_r f_t f_a + 84 f_s^4 f_a^2 f_a b f_r r f_r f_t^2 f_b \\
& - 120 f_b^2 f_s^3 f_a^2 f_a s f_r r f_r f_t^2 + 24 f_a^2 f_t f_b^3 f_s^3 f_r^2 f_a a f_r t - 64 f_b^3 f_s f_r^3 f_t^2 f_a f_r s f_a s - 32 f_b^3 f_s^3 \\
& f_r^3 f_t f_a f_a b f_b r - 64 f_b^4 f_s f_r^4 f_t f_a f_a b f_r t + 64 f_b^3 f_s f_r^4 f_t^2 f_a f_b r f_a b - 4 f_a^3 f_t f_b^2 f_s^4 f_a a f_r f_r t - 96 \\
& f_a^2 f_t^3 f_b f_s^2 f_r^2 f_r s f_a a + 24 f_s^2 f_r t f_a^3 f_b r f_r^2 f_t f_b^3 - 12 f_a^4 f_t^2 f_s^2 f_b f_r^2 f_a t f_b r + 52 f_a^4 f_t^3 f_b^2 f_s f_a s f_a a \\
& f_r^2 - 3 f_a^6 f_t^2 f_b f_s^2 f_a t f_b r f_r + 28 f_t^3 f_a t f_a^6 f_b f_s f_r f_a r + 96 f_a^3 f_t^3 f_a a f_b^3 f_s f_r^2 f_a r + 4 f_b^4 f_s^3 \\
& f_r^3 f_t f_a f_a b f_a a + 8 f_a f_t f_b^5 f_r^4 f_a a f_a t f_s - 20 f_a^2 f_t f_b^4 f_r^3 f_a b f_b r f_s^2 - 40 f_b^3 f_s^4 f_a f_a s f_r r f_r f_t \\
& + 96 f_a f_t f_b^2 f_r^3 f_s^3 f_a s f_a t + 192 f_a^2 f_t f_b^2 f_r^3 f_s^2 f_a t f_r t - 96 f_a f_t f_b^2 f_r^2 f_s^3 f_r s f_r t + 96 f_a^2 f_t^3 f_r^3 \\
& f_s^2 f_b f_a b f_a a + 704 f_b f_s f_r^3 f_t^3 f_a^2 f_a t f_a r + 120 f_t f_a f_r^2 f_r t f_r r f_s^2 f_b^4 - 96 f_t f_a f_r f_r t f_r r f_s^4 f_b^2 \\
& + 288 f_t^2 f_a f_r^2 f_r t f_r r f_b^2 f_s^2 - 36 f_t^3 f_a^5 f_a b f_s f_b^2 f_r f_r + 112 f_t^3 f_a^4 f_a b f_s f_b^2 f_r^2 f_a r + 4 f_b^6 f_a s f_r^2 f_s \\
& f_a^2 f_t f_r - 4 f_b^7 f_s f_r^2 f_a r f_t f_a f_r - 24 f_b^2 f_s^4 f_a^3 f_r f_t f_r s f_a b - 24 f_a^4 f_t^2 f_b^3 f_s f_r^2 f_r s f_a b + 48 f_b^4 \\
& f_s^3 f_a s f_a f_r^2 f_t f_a r + 21 f_a^5 f_t^2 f_b^2 f_s^2 f_a s f_b r f_r + 2 f_a^5 f_t f_b^2 f_s^3 f_a s f_a t f_r + 8 f_a t f_a^4 f_s^2 f_b^4 f_r r f_r f_t + 24 \\
& f_s^4 f_r t f_a^3 f_b r f_r f_t f_b - 12 f_s f_r t f_a^2 f_b r f_r^3 f_t f_b^4 - 72 f_s^3 f_r t f_a^2 f_b r f_r^2 f_t f_b^2 + 14 f_a^2 f_t f_b^4 f_s^3 f_r^2 f_a s f_a a \\
& + 8 f_b^5 f_s f_r^4 f_a f_t f_b r f_a b - 8 f_b^5 f_s f_r^3 f_a f_r s f_a s f_t + 96 f_b^2 f_s^3 f_r^3 f_t f_a f_a b f_r t - 16 f_b^5 f_s f_r^3 \\
& f_a^2 f_a s f_b r f_t - 192 f_r^2 f_t^3 f_a r f_r r f_b^3 f_a f_s - 256 f_r^2 f_t^4 f_a r f_r r f_b f_a f_s + 4 f_t f_a^3 f_a b f_s^4 f_b^3 f_r f_a r - 128 \\
& f_t^3 f_a^3 f_a b f_s f_b^2 f_r^2 f_r - 120 f_t^2 f_a^2 f_a b f_s^3 f_b^2 f_r^2 f_a r + 24 f_a^2 f_t f_b^3 f_s^3 f_r^2 f_a s f_b r - 32 f_a^3 f_t^3 f_s^2 \\
& f_r^2 f_b f_b r f_a a - 12 f_{a,b} f_s^5 f_r f_b^2 f_a f_t f_r - 16 f_b^3 f_s^4 f_a f_r^2 f_t f_b r f_a a - 8 f_s^5 f_t f_a a f_b^3 f_a f_r f_a r + 192 f_b \\
& f_s^2 f_r^3 f_t^2 f_a f_r s f_a t - 48 f_b f_s^2 f_r^3 f_t^2 f_a^2 f_a b f_r t - 42 f_b^2 f_a b f_a s f_r^2 f_s^2 f_a f_t^2 + 48 f_b^2 f_a b f_a s f_r^2 f_s^4 f_a^2 f_t \\
& - 144 f_b^2 f_a b f_a s f_r^3 f_t^2 f_a^2 f_s^2 - 128 f_b f_s^2 f_r^3 f_t^2 f_a f_a s f_r t + 288 f_r^2 f_t^3 f_a a f_b^3 f_s f_a^2 f_r - 24 f_a t \\
& f_a^5 f_s f_b^3 f_r r f_r f_t^2 + 12 f_a^3 f_t f_b^5 f_r^2 f_r s f_s f_a s - 4 f_a t f_a^3 f_s f_b^5 f_r r f_r^2 f_t + 36 f_b^5 f_s f_r^2 f_a^2 f_a a f_t^2 f_r - 48 \\
& f_b^5 f_s f_r^3 f_r r f_a t f_a f_t - 16 f_b^5 f_s f_r^3 f_a^2 f_t f_r s f_a b + 8 f_b^5 f_s f_r^3 f_a f_a r f_a a f_t^2 - 16 f_b f_s^2 f_a s f_a^4 f_r f_t^3 f_a r \\
& + 36 f_b^2 f_s^4 f_r^2 f_t f_a a f_a f_r t + 6 f_a^2 f_t f_b^5 f_s^3 f_r f_a a f_r r + 6 f_a^4 f_t f_b^3 f_s^2 f_r^2 f_a t f_b r + 144 f_r f_t^4 f_a a f_b f_s \\
& f_a^4 f_r r + 8 f_a^5 f_t^3 f_r s f_a a f_s f_r f_b^2 + 36 f_a t f_a^2 f_s^5 f_b f_r f_t f_a r - 240 f_a t f_a^2 f_s^3 f_b f_r^2 f_t^2 f_a r - 12 f_b^5 f_s^2 \\
& f_r^3 f_a f_a s f_a a f_t - 16 f_a^6 f_t^2 f_b^2 f_r f_r s f_a t f_s - 68 f_a^2 f_t f_b^4 f_s f_r^3 f_a t f_r s + 14 f_a^5 f_t^2 f_b f_s^3 f_a t f_a a f_r + 3 \\
& f_a^4 f_t^2 f_b^2 f_s^3 f_a a f_b r f_r - 256 f_b f_s f_r^3 f_t^3 f_a f_b r f_r s - 96 f_b^2 f_s^3 f_r^3 f_t f_a f_a t f_b r - 4 f_s^5 f_a b f_a s f_r f_b f_a^3 f_t
\end{aligned}$$

$$\begin{aligned}
& -10f_a^4 f_t f_b^2 f_s^4 f_{a,t} f_{a,a} f_r + 128f_a^3 f_t^3 f_b f_s f_r^3 f_{a,b} f_{a,s} + 16f_b^4 f_s f_r^4 f_t f_a f_{a,s} f_{a,t} - 96f_b^3 f_s^2 \\
& f_r^4 f_t f_a f_{a,b} f_{a,t} - 24f_a^3 f_t f_b^3 f_s^3 f_r f_{a,r} f_{r,t} - 32f_a^3 f_t^2 f_s^2 f_{a,s} f_{a,a} f_r^2 f_b + 42f_a^4 f_t^2 f_b^2 f_s^2 f_r f_b, r f_{r,s} \\
& + 32f_b f_s^3 f_r^2 f_t^2 f_a f_{r,s} f_{a,s} + 192f_b^3 f_{a,b} f_{a,s} f_r^4 f_t^2 f_a f_s + 28f_b^3 f_{a,b} f_{a,s} f_r^2 f_s^3 f_a f_t - 24f_b^2 f_s^4 \\
& f_a^3 f_{a,s} f_b, r f_r f_t + 32f_b^5 f_{a,b} f_{a,s} f_r^4 f_t f_a f_s + 48f_b^3 f_{a,b} f_{a,s} f_r^3 f_t^2 f_a^3 f_s - 48f_b^4 f_{a,b} f_{a,s} f_r^3 f_t f_a^2 f_s^2 \\
& - 48f_b^3 f_{a,b} f_{a,s} f_r^3 f_t f_a f_s^3 - 384f_s f_a^2 f_{r,s} f_t^3 f_{a,r} f_r^2 f_b^2 + 8f_s^3 f_a^2 f_{r,s} f_t f_a, r f_b^4 f_r - 144f_s f_a^2 f_{r,s} \\
& f_t^2 f_{a,r} f_r^2 f_b^4 + 144f_s^3 f_a^2 f_{r,s} f_t^2 f_{a,r} f_r f_b^2 - 4f_b^5 f_s^3 f_r f_{a,r} f_t f_a f_{r,r} - 8f_a^6 f_t^3 f_s f_r f_b f_b, r f_{a,s} - 8f_a^6 \\
& f_t^3 f_{a,b} f_{r,s} f_s f_r f_b - 32f_b^5 f_s f_r^3 f_a f_t f_b, r f_{r,s} + 14f_a^3 f_t f_b^5 f_s^2 f_r f_{r,s} f_{a,r} + 48f_a^2 f_t^2 f_r^2 f_s^3 f_{a,a} f_b f_{r,t} \\
& - 24f_a^2 f_t f_b^2 f_s^3 f_r^2 f_{a,t} f_{r,s} + 96f_a^4 f_t f_b^2 f_s^2 f_r^2 f_{a,t} f_{r,t} + 12f_a^6 f_t f_b^2 f_s^2 f_r f_{a,t} f_{r,t} + 72f_a^3 f_t^2 f_b^2 f_s^2 \\
& f_r^2 f_{r,s} f_{a,b} - 48f_a^3 f_t^2 f_b^3 f_s f_r^2 f_b, r f_{r,s} + 96f_a^2 f_t^2 f_b f_s^3 f_r^2 f_{r,s} f_{a,b} + 384f_b^2 f_s f_r^3 f_t^3 f_a f_{r,s} f_{a,a} - 78 \\
& f_a^4 f_t^3 f_{a,a} f_b^2 f_s^2 f_r f_{a,r} - 12f_a^3 f_t f_b f_s^5 f_{a,b} f_b, r f_r - 8f_a^3 f_t f_b^2 f_s^3 f_r^2 f_{a,b} f_{r,t} - 96f_a^3 f_t^2 f_b f_s^3 f_{r,s} f_{a,s} f_r \\
& - 96f_a^3 f_t^2 f_b^2 f_r^2 f_s f_{r,s} f_{r,t} + 16f_a^3 f_t^2 f_s^4 f_{a,a} f_b, r f_r f_b - 56f_a^3 f_t f_r f_{a,t} f_{r,r} f_s^3 f_b^3 + 90f_a^2 f_t f_r^2 f_{a,t} f_{r,r} \\
& f_s^2 f_b^4 + 21f_a^5 f_t^2 f_b^2 f_s^2 f_r f_{r,s} f_{a,b} - 48f_a^3 f_t^2 f_b^3 f_s^2 f_r^2 f_{a,s} f_{a,a} - 48f_b^4 f_s f_r^4 f_t^2 f_a f_{a,b} f_{a,a} - 192f_s \\
& f_a^2 f_b, r f_t^3 f_{r,r} f_r^2 f_b^2 - 14f_s^3 f_a^2 f_b, r f_t f_{r,r} f_b^4 f_r - 48f_s f_a^2 f_b, r f_t^2 f_{r,r} f_r^2 f_b^4 + 48f_s^2 f_a^3 f_b, r f_t^2 f_{r,r} f_r f_b^3 \\
& + 32f_s^2 f_a^3 f_b, r f_t^3 f_{r,r} f_r f_b - 16f_s^3 f_{a,b} f_{a,s} f_r^2 f_t^2 f_b f_a^3 + 48f_s^5 f_{a,b} f_{a,s} f_r^2 f_t f_b f_a - 192f_s^3 f_{a,b} f_{a,s} \\
& f_r^3 f_t^2 f_b f_a - 144f_t^3 f_{a,a} f_{a,r} f_r f_s^3 f_b f_a^3 - 60f_a^2 f_t f_r f_{a,t} f_{r,r} f_s^4 f_b^2 + 288f_a^2 f_t^2 f_r^2 f_{a,t} f_{r,r} f_b^2 f_s^2 + 16 \\
& f_a^3 f_t^2 f_b f_s^4 f_{a,s} f_{a,a} f_r - 60f_a^4 f_t^2 f_s^2 f_b f_r^2 f_{a,s} f_{a,t} - 96f_b f_s^3 f_r^3 f_t^2 f_a f_{a,b} f_b, r + 64f_t^3 f_{a,a} f_{a,r} f_r^3 \\
& f_b^3 f_a f_s + 384f_t^4 f_{a,a} f_{a,r} f_r^2 f_b f_a^3 f_s - 144f_t^3 f_{a,a} f_{a,r} f_r^2 f_b^2 f_a^2 f_s^2 - 96f_t^3 f_{a,a} f_{a,r} f_r^2 f_b f_a f_s^3 \\
& - 128f_s f_a^4 f_{r,s} f_t^3 f_{a,r} f_r f_b^2 + 24f_b^2 f_s^5 f_a f_{r,s} f_{a,a} f_r f_t + 96f_s^2 f_a^3 f_{r,s} f_t^2 f_{a,r} f_r f_b^3 + 12f_a^5 f_t^2 f_b^2 f_s \\
& f_r^2 f_{a,s} f_{a,t} + 64f_b f_s^4 f_r^2 f_t f_a f_{a,s} f_{r,t} - 144f_b f_s^4 f_r^2 f_t f_a f_{r,s} f_{a,t} - 12f_b f_s^4 f_r^2 f_t f_a^2 f_{a,b} f_{r,t} + 3f_b^5 f_s^2 \\
& f_r^2 f_a^2 f_{r,b} f_r f_t - 8f_a^3 f_t^2 f_b^2 f_s^3 f_r^2 f_{a,b} f_{a,a} + 24f_a^3 f_t^2 f_{a,a} f_b^3 f_s^3 f_r f_{a,r} + 16f_a^3 f_t^2 f_b^3 f_s f_r^3 f_b, r f_{a,b} \\
& - 8f_b^6 f_{r,s} f_r^2 f_{r,r} f_t f_a f_s + 4f_b f_s^6 f_a f_{a,s} f_{a,a} f_t f_r - 9f_b^6 f_s^2 f_r^2 f_a f_{a,a} f_t f_{r,r} - 2f_a^2 f_t f_b^4 f_s^4 f_r f_{a,r} f_{a,a} \\
& + 144f_b^2 f_s^2 f_r^2 f_t^2 f_{r,s} f_a^2 f_{a,s} + 56f_a^3 f_t f_b f_s^4 f_r f_{a,s} f_{r,t} - 18f_a^3 f_t f_b^4 f_s^2 f_r^2 f_{a,a} f_{r,t} - 288f_a^3 f_t^3 f_b^2 \\
& f_r^2 f_{a,r} f_{a,s} f_s + 48f_a^2 f_t^2 f_b^3 f_r^3 f_s^2 f_{a,b} f_{a,a} - 8f_a^3 f_t f_b^4 f_s^3 f_r f_{a,r} f_b, r - 24f_a^2 f_t f_b f_s^5 f_r f_{r,s} f_{a,b} \\
& - 24f_{a,t} f_a^2 f_b^3 f_{a,r} f_r^2 f_t f_s^3 - 8f_b^5 f_{a,s} f_r f_s^2 f_a f_t f_{r,r} + 48f_a^3 f_t^2 f_b^3 f_s f_r^2 f_{r,s} f_{a,s} - 24f_a^3 f_t^2 \\
& f_b^5 f_s f_r f_{a,r} f_{r,r} - 12f_a^3 f_t^2 f_b^4 f_s f_r^2 f_{a,r} f_b, r + 18f_a^4 f_t f_b^3 f_s^2 f_r^2 f_{a,b} f_{r,t} - 192f_b^3 f_s f_r^3 f_t^2 f_a f_b, r f_{r,s} \\
& + 60f_t^2 f_{a,a} f_{a,r} f_r f_s^4 f_b^2 f_a^2 + 24f_t^2 f_{a,a} f_{a,r} f_r f_s^5 f_b f_a + 16f_t^2 f_{a,a} f_{a,r} f_r^2 f_s^3 f_b^3 f_a + 12f_a^2 f_t f_b \\
& f_s^4 f_{a,s} f_{a,t} f_r^2 + 32f_a^2 f_t^2 f_b^3 f_r^3 f_{a,a} f_b, r f_s^2 - 14f_a^4 f_t f_b^3 f_s^3 f_r f_b, r f_{a,s} - 480f_b f_s^2 f_{a,s} f_a^2 f_r^2 f_t^3 f_{a,r} \\
& - 12f_a^2 f_t f_b f_s^4 f_r f_{r,s} f_{r,t} - 72f_a^2 f_t f_b^2 f_s^3 f_r^2 f_{a,s} f_{r,t} - 24f_a^5 f_t f_b f_s^3 f_r f_{a,t} f_{r,t} - 68f_a^3 f_t f_b \\
& f_s^4 f_{r,s} f_{a,t} f_r + 12f_a^3 f_t f_b^3 f_s^3 f_r^2 f_{a,b} f_b, r - 16f_a^3 f_t f_b^4 f_s f_r^3 f_{a,b} f_{r,t} + 192f_b^2 f_s f_r^3 f_t^2 f_a^2 f_{a,s} f_{r,t} + 12
\end{aligned}$$



$$\begin{aligned}
& f_a^4 f_t^2 f_b^3 f_s f_r^2 f_{a,a} f_{r,t} - 384 f_b^3 f_s f_r^3 f_t^2 f_{r,r} f_{a,t} f_a + 6 f_a^4 f_t f_b^2 f_s^3 f_r f_{a,s} f_{r,t} - 8 f_a^5 f_t^3 f_{a,a} f_{a,t} f_s f_r^2 f_b \\
& - 24 f_a^2 f_t f_b f_s^5 f_{a,s} f_{b,r} f_r + 128 f_{a,t} f_a^2 f_b^3 f_{a,r} f_r^3 f_t^2 f_s - 32 f_{a,t} f_a^4 f_b^3 f_{a,r} f_r f_s^3 f_t - 48 f_a^5 f_t^2 f_b f_s \\
& f_r^2 f_{a,t} f_{r,t} + 48 f_a^4 f_t^2 f_b^2 f_s f_r^2 f_{a,s} f_{r,t} - 4 f_a^7 f_t^2 f_b f_s f_r f_{a,t} f_{r,t} + 128 f_t^4 f_{a,a} f_{a,r} f_r^3 f_b f_a f_s + 160 f_b \\
& f_s^4 f_a f_r s f_{a,r} f_r f_t^2 + 72 f_{a,t} f_a^2 f_{a,b} f_s^3 f_r^3 f_t f_b^2 + 16 f_a^2 f_t f_b^5 f_s f_r^3 f_{a,a} f_{r,t} + 72 f_t^2 f_a^3 f_{a,b} f_s^4 f_b f_r f_{a,r} \\
& + 12 f_a^4 f_t^2 f_s^2 f_b f_r^2 f_{a,b} f_{r,t} - 16 f_a^3 f_t f_b f_s^5 f_{a,t} f_{a,a} f_r - 64 f_a^4 f_t^3 f_b f_s f_{a,s} f_{b,r} f_r^2 - 30 f_t^2 f_a^3 f_{a,a} f_{r,r} \\
& f_s^2 f_b^4 f_r + 16 f_b^4 f_s f_r^4 f_t f_a f_{a,t} f_{b,r} - 24 f_a^2 f_t f_s^5 f_{a,a} f_r f_b f_{r,t} - 16 f_a^5 f_t^3 f_s f_b f_r f_{r,s} f_{b,r} + 24 f_a^5 \\
& f_t^3 f_s f_b f_r f_{a,r} f_{r,t} - 384 f_a f_t^3 f_b^2 f_r^2 f_{r,s} f_s f_{r,r} + 48 f_a^2 f_t^2 f_b^4 f_s f_r^3 f_{a,s} f_{a,a} - 2 f_a^4 f_t f_b^3 f_s^2 f_{a,s} f_{a,t} \\
& + 36 f_t^3 f_a^4 f_{a,a} f_{r,r} f_r f_b^3 f_s + 32 f_a^3 f_t f_b^3 f_s^2 f_{a,t} f_{a,a} - 3 f_a^2 f_t f_b^4 f_s^3 f_{a,a} f_{b,r} - 36 f_a^3 f_t f_b^3 \\
& f_s^3 f_r f_{r,s} f_{a,s} + 4 f_a^3 f_t f_b^4 f_s f_r^3 f_{a,s} f_{a,t} + 16 f_a^3 f_t^2 f_b f_s^3 f_r f_{b,r} f_{r,s} + 84 f_a^2 f_t^2 f_{a,r} f_{r,r} f_s^2 f_b^4 f_r + 14 \\
& f_a^5 f_t f_b^3 f_s^2 f_r f_{r,s} f_{a,t} + 24 f_b^4 f_{a,s} f_r f_s f_a^4 f_t^2 f_{r,r} - 36 f_b^2 f_s^5 f_{a,s} f_a f_r f_t f_{a,r} + 144 f_b^2 f_s^3 f_{a,s} f_a f_r^2 f_t^2 f_{a,r} \\
& - 24 f_a^3 f_t^2 f_s^2 f_b^2 f_r^2 f_{a,a} f_{r,t} - 48 f_{a,t} f_a f_b^2 f_{a,r} f_r^3 f_t^2 f_s^2 + 12 f_{a,t} f_a f_b^2 f_{a,r} f_r^2 f_t f_s^4 + 8 f_a f_t f_b^5 \\
& f_r^3 f_{a,a} f_{b,r} f_s^2 - 12 f_{a,t} f_a^2 f_b^5 f_{a,r} f_r^3 f_t f_s + 16 f_{a,t} f_a^4 f_b^3 f_{a,r} f_r^2 f_t^2 f_s + 28 f_{a,t} f_a^3 f_b^4 f_{a,r} f_r^2 f_t f_s^2 \\
& - 28 f_{a,t} f_a f_b^4 f_{a,r} f_r^3 f_t f_s^2 + 48 f_t f_r^2 f_{a,r} f_{r,t} f_s^3 f_b^3 f_a - 288 f_t^3 f_a^2 f_{a,a} f_s^3 f_{r,r} f_r f_b + 448 f_t^3 f_a^2 f_{a,b} f_s \\
& f_b^2 f_r^3 f_{a,r} - 6 f_t f_a^2 f_{a,b} f_s^5 f_b^2 f_r f_{a,r} + 13 f_t f_a^2 f_{a,b} f_s^3 f_b^4 f_r^2 f_{a,r} + 100 f_t^2 f_a^2 f_{a,b} f_s f_b^4 f_r^3 f_{a,r} - 16 \\
& f_b^4 f_s f_r^3 f_t f_a f_{r,s} f_{r,t} + 72 f_a^2 f_t^2 f_b f_s^4 f_{r,s} f_{a,a} f_r + 8 f_a^4 f_t^2 f_b f_s^3 f_{a,s} f_{b,r} f_r - 76 f_a^5 f_t^3 f_b^2 f_s f_{a,r} f_{a,s} f_r \\
& + 24 f_b f_s^5 f_r^2 f_a f_t f_b, r f_{a,b} + 96 f_a^3 f_t f_b^3 f_s^2 f_r^2 f_{r,s} f_{a,t} + 12 f_{a,t} f_a^2 f_{a,b} f_s f_r^4 f_t f_b^4 + 2 f_a^4 f_t f_b \\
& f_s^4 f_r f_{a,b} f_{r,t} - 2 f_a^4 f_t f_b f_s^4 f_{a,s} f_{a,t} f_r - 24 f_{a,t} f_a^3 f_{a,b} f_s^2 f_r^3 f_t f_b^3 + 18 f_{a,t} f_a^4 f_{a,b} f_s^3 f_r^2 f_t f_b^2 - 144 f_a^4 \\
& f_t^2 f_b^2 f_s f_r^2 f_{a,t} f_{r,s} - 64 f_a^3 f_t f_b^2 f_s^3 f_r^2 f_{a,t} f_{b,r} - 192 f_b^2 f_s f_r^2 f_t^3 f_a^2 f_{a,s} f_{r,r} + 64 f_b^2 f_s f_r^3 f_t^3 f_a f_{a,r} f_{a,s} \\
& + 3 f_a^6 f_t^2 f_b f_s^2 f_r f_{a,b} f_{r,t} + 84 f_a^5 f_t^2 f_b f_s^2 f_{r,s} f_{a,t} f_r - 4 f_a^5 f_t^2 f_b^3 f_s f_r f_{a,r} f_{r,t} + 4 f_a^4 f_t^3 f_b^2 f_s \\
& f_r^2 f_b, r f_{a,a} - 192 f_b^2 f_s f_r^4 f_t^2 f_a f_{a,b} f_{r,t} + 128 f_b f_s f_r^4 f_t^3 f_a f_{b,r} f_{a,b} - 128 f_b f_s f_r^3 f_t^3 f_a f_{r,s} f_{a,s} \\
& + 128 f_b f_s^3 f_r^3 f_t f_a f_{a,t} f_{r,t} - 384 f_a^2 f_t^2 f_b^2 f_r^3 f_{r,s} f_{a,t} f_s - 144 f_b^3 f_s^2 f_a f_{r,s} f_{a,s} f_r^2 f_t^2 + 256 f_t^3 f_{a,t} \\
& f_a^4 f_b f_s f_r^2 f_{a,r} + 17 f_a^4 f_t^2 f_b^2 f_s^3 f_{a,s} f_{a,a} f_r - 64 f_a^3 f_t^3 f_b^2 f_s f_r^3 f_{a,b} f_{a,a} - 3 f_a^5 f_t^2 f_b^2 f_s^2 f_{a,a} f_r f_{r,t} - 16 \\
& f_a^5 f_t^3 f_b^2 f_s f_r f_{a,r} f_{b,r} - 48 f_b^2 f_s^2 f_r^3 f_t^2 f_{b,r} f_a f_{a,s} - 48 f_b^2 f_s^2 f_r^3 f_t^2 f_a f_{a,b} f_{r,s} - 192 f_b^2 f_s^3 f_r^2 \\
& f_t^2 f_{r,s} f_{a,a} f_a - 768 f_b f_s f_r^3 f_t^3 f_{r,r} f_{a,t} f_a - 128 f_b f_s f_r^3 f_t^3 f_a^2 f_{r,s} f_{a,b} - 10 f_a^5 f_t f_b^2 f_s^3 f_{a,t} f_{b,r} f_r + 6 \\
& f_b^5 f_a^2 f_{r,s} f_t f_r, r f_s^2 f_r - 21 f_a^4 f_t^2 f_b^3 f_s^2 f_r f_{r,s} f_{a,a} + 48 f_t^2 f_a^3 f_{a,b} f_s^3 f_b^2 f_r f_{r,r} - 20 f_t^3 f_a^4 f_{a,b} f_s^2 f_b f_r f_{r,r} \\
& - 96 f_t^3 f_a^3 f_{a,b} f_s^2 f_b f_r^2 f_{a,r} + 96 f_a^3 f_t^2 f_b^2 f_r^3 f_{a,t} f_{b,r} f_s - 96 f_a^2 f_t^2 f_b^3 f_s f_r^3 f_{a,s} f_{b,r} - 256 f_b^2 f_s f_r^4 \\
& f_t^3 f_a f_{a,b} f_{a,a} - 44 f_b^3 f_s^4 f_{a,s} f_a^2 f_r f_t f_{a,r} + 72 f_b f_s^4 f_{a,s} f_a^2 f_r f_t^2 f_{a,r} + 96 f_b^2 f_s^3 f_{a,s} f_a^3 f_r f_t^2 f_{a,r} \\
& + 48 f_b f_s^2 f_r^3 f_t^2 f_a^2 f_{a,t} f_{b,r} + 32 f_a^4 f_t^3 f_s^2 f_r^2 f_b f_{a,b} f_{a,a} - 24 f_{a,t} f_a^3 f_{a,b} f_s^4 f_r^2 f_t f_b - 6 f_{a,t} f_a^5 f_{a,b} \\
& f_s^4 f_r f_b f_t + 88 f_a^5 f_t^4 f_{a,a} f_b f_s f_r f_{a,r} + 9 f_{a,t} f_a^5 f_b^2 f_{a,r} f_r f_s^2 f_t^2 - 4 f_{a,t} f_a^3 f_b^2 f_{a,r} f_r f_s^4 f_t - 8 f_a^5
\end{aligned}$$

$$\begin{aligned}
& f_t^3 f_a a f_b r f_s^2 f_r f_b - 128 f_b^3 f_s f_r^4 f_t f_a f_a t f_r t + 8 f_a^4 f_t f_b^4 f_s f_r^2 f_a s f_r t - 48 f_t^2 f_a^2 f_a a f_s^3 f_r r f_r f_b^3 \\
& + 192 f_b f_s^3 f_r^2 f_t^2 f_a f_r s f_b r + 24 f_s^3 f_a^2 f_b r f_t^2 f_r r f_r f_b^2 - 52 f_s f_a^4 f_b r f_t^3 f_r r f_r f_b^2 + 64 f_a b f_s f_r^3 \\
& f_b^2 f_a f_t^3 f_r r + 144 f_t^3 f_a f_a a f_s^2 f_r r f_r^2 f_b^2 + 18 f_t f_a f_a a f_s^4 f_r r f_b^4 f_r - 36 f_t^2 f_a f_a a f_s^2 f_r r f_r^2 f_b^4 + 36 \\
& f_t^2 f_a f_a a f_s^4 f_r r f_r f_b^2 + 8 f_b f_s^5 f_a f_r s f_a s f_r f_t + 256 f_b f_s f_r^4 f_t^3 f_a f_a b f_a s - 72 f_a^3 f_t f_b^3 f_s^2 f_r^2 f_a s f_r t \\
& + 24 f_a t f_a^3 f_b^2 f_a r f_r^2 f_t^2 f_s^2 - 72 f_t^3 f_a^3 f_a a f_s^2 f_r r f_r f_b^2 - 96 f_b^4 f_r s f_r^2 f_r r f_t^2 f_a f_s + 8 f_b^6 f_s^2 \\
& f_a^2 f_r f_a r f_t f_r r + 8 f_b^4 f_a^3 f_r s f_t^2 f_r r f_r f_s + 12 f_b^3 f_s^4 f_a f_r s f_a r f_r f_t - 512 f_b f_s^2 f_a f_r s f_a r f_r^2 f_t^3 + 144 \\
& f_a^2 f_t^2 f_b^2 f_r^2 f_s^2 f_r s f_b r + 44 f_a^4 f_t^3 f_b^2 f_s f_r f_a s f_r r + 4 f_a^3 f_t f_b^4 f_s f_r^3 f_a t f_b r + 144 f_b^4 f_s f_r^3 f_t^2 f_a f_r s f_a a \\
& + 24 f_a^3 f_t^2 f_b^4 f_s f_r^2 f_r s f_a a + 18 f_a^4 f_t^2 f_b^3 f_s^2 f_r f_a r f_b r + 2 f_a^4 f_t f_b^2 f_s^4 f_a b f_b r f_r + 8 f_a^4 f_t^2 f_b \\
& f_s^3 f_r f_r s f_a b - 104 f_t^2 f_a t f_a^4 f_b f_s^3 f_r f_a r - 128 f_b f_s f_r^3 f_t^3 f_a^2 f_a s f_b r - 72 f_a^2 f_t^2 f_r^2 f_s^4 f_b f_a b f_a a \\
& - 96 f_t^2 f_r^2 f_a r f_r t f_b f_a f_s^3 + 384 f_t^3 f_r^3 f_a r f_r t f_b f_a f_s - 48 f_t f_r f_a r f_r t f_s^4 f_b^2 f_a^2 - 24 f_t f_r f_a r f_r t \\
& f_s^5 f_b f_a - 4 f_a^4 f_t f_b^2 f_s^4 f_a b f_a s f_r - 144 f_b f_s^2 f_r^3 f_t^2 f_a^2 f_a s f_a t + 144 f_b f_s^2 f_r^2 f_t^2 f_a^2 f_r s f_r t - 192 f_a^3 \\
& f_t^2 f_r^2 f_a t f_r r f_b^3 f_s - 208 f_a^5 f_t^3 f_r f_a t f_r r f_b f_s + 138 f_a^4 f_t^2 f_r f_a t f_r r f_b^2 f_s^2 + 96 f_a^3 f_t^2 f_r f_a t f_r r f_b f_s^3 \\
& - 704 f_a^3 f_t^3 f_r^2 f_a t f_r r f_b f_s - 12 f_a^5 f_t f_b^3 f_s^2 f_r f_a s f_r t + 6 f_a^3 f_t f_b^2 f_s^5 f_a b f_a a f_r + 48 f_b^2 f_s^4 f_a^2 \\
& f_r^2 f_t f_b r f_a b - 6 f_a^3 f_t f_b^3 f_s^4 f_a s f_a a f_r - 96 f_a^3 f_t^2 f_s^2 f_b f_r^2 f_a s f_r t - f_s^9 f_b r r r)
\end{aligned}$$

This is impressive. Seems hopeless to resolve all these equations (in totality 140) with respect to the highest (3rd order) derivatives of the function  $f$  defining PDE. However here is the working strategy: copy the integrability conditions of Ferapontov, Hadjikos, Khusnutdinova, IMRN (2009) - we brought it to the Maple form (from the original Mathematica output) by several accurate replacement options (we preferred this over an old un-tested convertor since we also compactified the set of integrability conditions - see below, still huge even after reduction by at least factor 3 in height in comparison to the original 'sparse' version). Then insert them into the equations Eq\_i and check vanishing, so these integrability conditions are solutions. Then prove uniqueness of the solution.

$$\begin{aligned}
> IC := \{ D[1, 1, 1](f)(r, s, t, a, b) = \\
& ((-2 * D[2, 4](f)(r, s, t, a, b)^2 * D[1](f)(r, s, t, a, b)^2 - 2 * D[4, 5](f)(r, s, t, a, b)^2 \\
& * D[1](f)(r, s, t, a, b)^3 - 2 * D[1](f)(r, s, t, a, b)^2 * \\
& D[1, 5](f)(r, s, t, a, b)^2 - 4 * D[4](f)(r, s, t, a, b) * D[2, 2](f)(r, s, t, a, b) \\
& * D[1](f)(r, s, t, a, b) * D[1, 4](f)(r, s, t, a, b) - \\
& 4 * D[3, 4](f)(r, s, t, a, b) * D[1](f)(r, s, t, a, b)^2 * D[1, 4](f)(r, s, t, a, b) + 8 * D[2, \\
& 5](f)(r, s, t, a, b) * D[1](f)(r, s, t, a, b)^2 * \\
& D[1, 4](f)(r, s, t, a, b) - 2 * D[2](f)(r, s, t, a, b) * D[1](f)(r, s, t, a, b) * D[1, 5](f)(r, \\
& s, t, a, b) * D[1, 4](f)(r, s, t, a, b) - \\
& 2 * D[2](f)(r, s, t, a, b)^2 * D[1, 4](f)(r, s, t, a, b)^2 + 2 * D[3](f)(r, s, t, a, b) \\
& * D[1](f)(r, s, t, a, b) * D[1, 4](f)(r, s, t, a, b)^2 - \\
& 2 * D[4](f)(r, s, t, a, b) * D[1](f)(r, s, t, a, b) * D[1, 4](f)(r, s, t, a, b) * D[1, 3](f)(r, \\
& s, t, a, b) - 4 * D[4, 5](f)(r, s, t, a, b) * \\
& D[1](f)(r, s, t, a, b)^2 * D[1, 2](f)(r, s, t, a, b) + 4 * D[4](f)(r, s, t, a, b) * D[1](f)(r,
\end{aligned}$$

$$\begin{aligned}
& s, t, a, b) * D[1, 5](f)(r, s, t, a, b) * D[1, 2](f)(r, s, t, a, b) + \\
& 4 * D[4](f)(r, s, t, a, b) * D[2](f)(r, s, t, a, b) * D[1, 4](f)(r, s, t, a, b) * D[1, 2](f)(r, \\
& s, t, a, b) - 2 * D[5](f)(r, s, t, a, b) * D[1](f)(r, s, t, a, b) * \\
& D[1, 4](f)(r, s, t, a, b) * D[1, 2](f)(r, s, t, a, b) - 2 * D[4](f)(r, s, t, a, b)^2 * D[1, \\
& 2](f)(r, s, t, a, b)^2 - 2 * D[1](f)(r, s, t, a, b) * D[1, 2](f)(r, s, t, a, b)^2 + \\
& 2 * D[4](f)(r, s, t, a, b)^2 * D[2, 2](f)(r, s, t, a, b) * D[1, 1](f)(r, s, t, a, b) + 2 \\
& * D[4](f)(r, s, t, a, b) * D[3, 4](f)(r, s, t, a, b) * \\
& D[1](f)(r, s, t, a, b) * D[1, 1](f)(r, s, t, a, b) + 2 * D[4, 5](f)(r, s, t, a, b) * D[2](f)(r, \\
& s, t, a, b) * D[1](f)(r, s, t, a, b) * D[1, 1](f)(r, s, t, a, b) - \\
& 4 * D[4](f)(r, s, t, a, b) * D[2, 5](f)(r, s, t, a, b) * D[1](f)(r, s, t, a, b) * D[1, 1](f)(r, \\
& s, t, a, b) + 2 * D[2, 2](f)(r, s, t, a, b) * \\
& D[1](f)(r, s, t, a, b) * D[1, 1](f)(r, s, t, a, b) + 2 * D[5, 5](f)(r, s, t, a, b) * D[1](f)(r, \\
& s, t, a, b)^2 * D[1, 1](f)(r, s, t, a, b) - \\
& D[4](f)(r, s, t, a, b) * D[2](f)(r, s, t, a, b) * D[1, 5](f)(r, s, t, a, b) * D[1, 1](f)(r, s, t, \\
& a, b) + 2 * D[5](f)(r, s, t, a, b) * D[1](f)(r, s, t, a, b) * D[1, 5](f)(r, s, t, a, b) * \\
& D[1, 1](f)(r, s, t, a, b) + 2 * D[4](f)(r, s, t, a, b) * D[3](f)(r, s, t, a, b) * D[1, 4](f)(r, \\
& s, t, a, b) * D[1, 1](f)(r, s, t, a, b) - \\
& D[5](f)(r, s, t, a, b) * D[2](f)(r, s, t, a, b) * D[1, 4](f)(r, s, t, a, b) * D[1, 1](f)(r, s, t, \\
& a, b) + D[4](f)(r, s, t, a, b)^2 * D[1, 3](f)(r, s, t, a, b) * \\
& D[1, 1](f)(r, s, t, a, b) + 4 * D[1](f)(r, s, t, a, b) * D[1, 3](f)(r, s, t, a, b) * D[1, \\
& 1](f)(r, s, t, a, b) - \\
& D[5](f)(r, s, t, a, b) * D[4](f)(r, s, t, a, b) * D[1, 2](f)(r, s, t, a, b) * D[1, 1](f)(r, s, t, \\
& a, b) - 2 * D[2](f)(r, s, t, a, b) * D[1, 2](f)(r, s, t, a, b) * \\
& D[1, 1](f)(r, s, t, a, b) + D[5](f)(r, s, t, a, b)^2 * D[1, 1](f)(r, s, t, a, b)^2 + 4 \\
& * D[3](f)(r, s, t, a, b) * D[1, 1](f)(r, s, t, a, b)^2 + \\
& 2 * D[4, 4](f)(r, s, t, a, b) * (D[2, 2](f)(r, s, t, a, b) * D[1](f)(r, s, t, a, b)^2 + D[5, \\
& 5](f)(r, s, t, a, b) * D[1](f)(r, s, t, a, b)^3 + \\
& 2 * D[1](f)(r, s, t, a, b)^2 * D[1, 3](f)(r, s, t, a, b) - 2 * D[2](f)(r, s, t, a, b) \\
& * D[1](f)(r, s, t, a, b) * D[1, 2](f)(r, s, t, a, b) + \\
& D[2](f)(r, s, t, a, b)^2 * D[1, 1](f)(r, s, t, a, b) - D[3](f)(r, s, t, a, b) * D[1](f)(r, s, t, \\
& a, b) * D[1, 1](f)(r, s, t, a, b)) + \\
& D[2, 4](f)(r, s, t, a, b) * (-4 * D[1](f)(r, s, t, a, b)^2 * D[1, 5](f)(r, s, t, a, b) - 4 \\
& * D[4](f)(r, s, t, a, b) * D[2](f)(r, s, t, a, b) * \\
& D[1, 1](f)(r, s, t, a, b) + 2 * D[1](f)(r, s, t, a, b) * (2 * D[2](f)(r, s, t, a, b) * D[1, \\
& 4](f)(r, s, t, a, b) + \\
& 2 * D[4](f)(r, s, t, a, b) * D[1, 2](f)(r, s, t, a, b) + D[5](f)(r, s, t, a, b) * D[1, 1](f)(r, \\
& s, t, a, b))) / \\
& (D[4](f)(r, s, t, a, b)^2 * D[3](f)(r, s, t, a, b) - D[5](f)(r, s, t, a, b) * D[4](f)(r, s, t, \\
& a, b) * D[2](f)(r, s, t, a, b) - \\
& D[2](f)(r, s, t, a, b)^2 + (D[5](f)(r, s, t, a, b)^2 + 4 * D[3](f)(r, s, t, a, b)) \\
& * D[1](f)(r, s, t, a, b)), \\
& D[1, 1, 2](f)(r, s, t, a, b) = \\
& ((-2 * D[4, 5](f)(r, s, t, a, b)^2 * D[2](f)(r, s, t, a, b) * D[1](f)(r, s, t, a, b)^2 - 4 \\
& * D[3, 4](f)(r, s, t, a, b) * D[2, 4](f)(r, s, t, a, b) * \\
& D[1](f)(r, s, t, a, b)^2 + 4 * D[4, 4](f)(r, s, t, a, b) * D[2, 3](f)(r, s, t, a, b) \\
& * D[1](f)(r, s, t, a, b)^2 - 2 * D[2](f)(r, s, t, a, b) * \\
& D[2, 4](f)(r, s, t, a, b) * D[1](f)(r, s, t, a, b) * D[1, 5](f)(r, s, t, a, b) - 4 * D[3, \\
& 4](f)(r, s, t, a, b) * D[1](f)(r, s, t, a, b)^2 *
\end{aligned}$$

$$\begin{aligned}
& D[1, 5](f)(r, s, t, a, b) - 2 * D[2](f)(r, s, t, a, b) * D[1](f)(r, s, t, a, b) * D[1, 5](f)(r, \\
& \quad s, t, a, b)^2 + 6 * D[2](f)(r, s, t, a, b) * \\
& D[2, 5](f)(r, s, t, a, b) * D[1](f)(r, s, t, a, b) * D[1, 4](f)(r, s, t, a, b) + 4 * D[3](f)(r, \\
& \quad s, t, a, b) * D[2, 4](f)(r, s, t, a, b) * \\
& D[1](f)(r, s, t, a, b) * D[1, 4](f)(r, s, t, a, b) - 6 * D[4](f)(r, s, t, a, b) * D[2, 3](f)(r, \\
& \quad s, t, a, b) * D[1](f)(r, s, t, a, b) * D[1, 4](f)(r, s, t, a, b) - \\
& 2 * D[5](f)(r, s, t, a, b) * D[2, 2](f)(r, s, t, a, b) * D[1](f)(r, s, t, a, b) * D[1, 4](f)(r, \\
& \quad s, t, a, b) + 4 * D[3, 5](f)(r, s, t, a, b) * D[1](f)(r, s, t, a, b)^2 * \\
& D[1, 4](f)(r, s, t, a, b) - 2 * D[2](f)(r, s, t, a, b)^2 * D[1, 5](f)(r, s, t, a, b) * D[1, \\
& \quad 4](f)(r, s, t, a, b) - 2 * D[3](f)(r, s, t, a, b) * \\
& D[2](f)(r, s, t, a, b) * D[1, 4](f)(r, s, t, a, b)^2 + 2 * D[4](f)(r, s, t, a, b) * D[2, \\
& \quad 4](f)(r, s, t, a, b) * D[1](f)(r, s, t, a, b) * \\
& D[1, 3](f)(r, s, t, a, b) + 2 * D[4](f)(r, s, t, a, b) * D[1](f)(r, s, t, a, b) * D[1, 5](f)(r, \\
& \quad s, t, a, b) * D[1, 3](f)(r, s, t, a, b) + 2 * D[4](f)(r, s, t, a, b) * \\
& D[2](f)(r, s, t, a, b) * D[1, 4](f)(r, s, t, a, b) * D[1, 3](f)(r, s, t, a, b) - 2 * D[5](f)(r, \\
& \quad s, t, a, b) * D[1](f)(r, s, t, a, b) * \\
& D[1, 4](f)(r, s, t, a, b) * D[1, 3](f)(r, s, t, a, b) - 4 * D[4, 4](f)(r, s, t, a, b) \\
& \quad * D[3](f)(r, s, t, a, b) * D[1](f)(r, s, t, a, b) * D[1, 2](f)(r, s, t, a, b) + \\
& 4 * D[4](f)(r, s, t, a, b) * D[3, 4](f)(r, s, t, a, b) * D[1](f)(r, s, t, a, b) * D[1, 2](f)(r, \\
& \quad s, t, a, b) + 2 * D[5](f)(r, s, t, a, b) * D[2, 4](f)(r, s, t, a, b) * \\
& D[1](f)(r, s, t, a, b) * D[1, 2](f)(r, s, t, a, b) + 2 * D[4](f)(r, s, t, a, b) * D[2](f)(r, s, \\
& \quad t, a, b) * D[1, 5](f)(r, s, t, a, b) * \\
& D[1, 2](f)(r, s, t, a, b) + 2 * D[5](f)(r, s, t, a, b) * D[1](f)(r, s, t, a, b) * D[1, 5](f)(r, \\
& \quad s, t, a, b) * D[1, 2](f)(r, s, t, a, b) + \\
& 4 * D[4](f)(r, s, t, a, b) * D[3](f)(r, s, t, a, b) * D[1, 4](f)(r, s, t, a, b) * D[1, 2](f)(r, \\
& \quad s, t, a, b) - 2 * D[4](f)(r, s, t, a, b)^2 * \\
& D[1, 3](f)(r, s, t, a, b) * D[1, 2](f)(r, s, t, a, b) - 2 * D[5](f)(r, s, t, a, b) * D[4](f)(r, \\
& \quad s, t, a, b) * D[1, 2](f)(r, s, t, a, b)^2 - 2 * D[2](f)(r, s, t, a, b) * \\
& D[1, 2](f)(r, s, t, a, b)^2 + 2 * D[4, 4](f)(r, s, t, a, b) * D[3](f)(r, s, t, a, b) \\
& \quad * D[2](f)(r, s, t, a, b) * D[1, 1](f)(r, s, t, a, b) - 2 * D[4](f)(r, s, t, a, b) * \\
& D[3, 4](f)(r, s, t, a, b) * D[2](f)(r, s, t, a, b) * D[1, 1](f)(r, s, t, a, b) - 3 * D[4](f)(r, \\
& \quad s, t, a, b) * D[2](f)(r, s, t, a, b) * \\
& D[2, 5](f)(r, s, t, a, b) * D[1, 1](f)(r, s, t, a, b) - 2 * D[4](f)(r, s, t, a, b) * D[3](f)(r, \\
& \quad s, t, a, b) * D[2, 4](f)(r, s, t, a, b) * D[1, 1](f)(r, s, t, a, b) - \\
& D[5](f)(r, s, t, a, b) * D[2](f)(r, s, t, a, b) * D[2, 4](f)(r, s, t, a, b) * D[1, 1](f)(r, s, t, \\
& \quad a, b) + 3 * D[4](f)(r, s, t, a, b)^2 * \\
& D[2, 3](f)(r, s, t, a, b) * D[1, 1](f)(r, s, t, a, b) + D[5](f)(r, s, t, a, b) * D[4](f)(r, s, \\
& \quad t, a, b) * D[2, 2](f)(r, s, t, a, b) * D[1, 1](f)(r, s, t, a, b) - \\
& 2 * D[4](f)(r, s, t, a, b) * D[3, 5](f)(r, s, t, a, b) * D[1](f)(r, s, t, a, b) * D[1, 1](f)(r, \\
& \quad s, t, a, b) + 2 * D[5](f)(r, s, t, a, b) * D[3, 4](f)(r, s, t, a, b) * \\
& D[1](f)(r, s, t, a, b) * D[1, 1](f)(r, s, t, a, b) + 4 * D[2, 3](f)(r, s, t, a, b) * D[1](f)(r, \\
& \quad s, t, a, b) * D[1, 1](f)(r, s, t, a, b) + D[5](f)(r, s, t, a, b)^2 * \\
& D[1, 2](f)(r, s, t, a, b) * D[1, 1](f)(r, s, t, a, b) + 4 * D[3](f)(r, s, t, a, b) * D[1, \\
& \quad 2](f)(r, s, t, a, b) * D[1, 1](f)(r, s, t, a, b) + 2 * D[5, 5](f)(r, s, t, a, b) * \\
& D[2](f)(r, s, t, a, b) * D[1](f)(r, s, t, a, b) * (D[4, 4](f)(r, s, t, a, b) * D[1](f)(r, s, t, \\
& \quad a, b) + D[1, 1](f)(r, s, t, a, b)) + 2 * D[4, 5](f)(r, s, t, a, b) * \\
& D[2](f)(r, s, t, a, b) * (-2 * D[1](f)(r, s, t, a, b) * D[1, 2](f)(r, s, t, a, b) \\
& \quad + D[2](f)(r, s, t, a, b) * D[1, 1](f)(r, s, t, a, b)) /
\end{aligned}$$

$$\begin{aligned}
& (D[4](f)(r, s, t, a, b)^2 * D[3](f)(r, s, t, a, b) - D[5](f)(r, s, t, a, b) * D[4](f)(r, s, t, \\
& a, b) * D[2](f)(r, s, t, a, b) - \\
& D[2](f)(r, s, t, a, b)^2 + (D[5](f)(r, s, t, a, b)^2 + 4 * D[3](f)(r, s, t, a, b)) \\
& * D[1](f)(r, s, t, a, b))), \\
D[1, 1, 3](f)(r, s, t, a, b) = & \\
& ((-2 * D[4, 5](f)(r, s, t, a, b)^2 * D[3](f)(r, s, t, a, b) * D[1](f)(r, s, t, a, b)^2 - 2 \\
& * D[3, 4](f)(r, s, t, a, b)^2 * D[1](f)(r, s, t, a, b)^2 + \\
& 2 * D[4, 4](f)(r, s, t, a, b) * D[3, 3](f)(r, s, t, a, b) * D[1](f)(r, s, t, a, b)^2 - 2 * D[3, \\
& 4](f)(r, s, t, a, b) * D[2](f)(r, s, t, a, b) * \\
& D[1](f)(r, s, t, a, b) * D[1, 5](f)(r, s, t, a, b) - 2 * D[3](f)(r, s, t, a, b) * D[1](f)(r, s, \\
& t, a, b) * D[1, 5](f)(r, s, t, a, b)^2 - \\
& 2 * D[4](f)(r, s, t, a, b) * D[3, 3](f)(r, s, t, a, b) * D[1](f)(r, s, t, a, b) * D[1, 4](f)(r, \\
& s, t, a, b) + 2 * D[3, 5](f)(r, s, t, a, b) * D[2](f)(r, s, t, a, b) * \\
& D[1](f)(r, s, t, a, b) * D[1, 4](f)(r, s, t, a, b) + 4 * D[3](f)(r, s, t, a, b) * D[2, 5](f)(r, \\
& s, t, a, b) * D[1](f)(r, s, t, a, b) * D[1, 4](f)(r, s, t, a, b) - \\
& 2 * D[5](f)(r, s, t, a, b) * D[2, 3](f)(r, s, t, a, b) * D[1](f)(r, s, t, a, b) * D[1, 4](f)(r, \\
& s, t, a, b) - 2 * D[3](f)(r, s, t, a, b) * \\
& D[2](f)(r, s, t, a, b) * D[1, 5](f)(r, s, t, a, b) * D[1, 4](f)(r, s, t, a, b) + 2 * D[4](f)(r, \\
& s, t, a, b) * D[3, 4](f)(r, s, t, a, b) * D[1](f)(r, s, t, a, b) * \\
& D[1, 3](f)(r, s, t, a, b) + 2 * D[5](f)(r, s, t, a, b) * D[1](f)(r, s, t, a, b) * D[1, 5](f)(r, \\
& s, t, a, b) * D[1, 3](f)(r, s, t, a, b) + 2 * D[4](f)(r, s, t, a, b) * \\
& D[3](f)(r, s, t, a, b) * D[1, 4](f)(r, s, t, a, b) * D[1, 3](f)(r, s, t, a, b) + 2 * D[1](f)(r, \\
& s, t, a, b) * D[1, 3](f)(r, s, t, a, b)^2 + \\
& 2 * D[5](f)(r, s, t, a, b) * D[3, 4](f)(r, s, t, a, b) * D[1](f)(r, s, t, a, b) * D[1, 2](f)(r, \\
& s, t, a, b) + 2 * D[4](f)(r, s, t, a, b) * D[3](f)(r, s, t, a, b) * \\
& D[1, 5](f)(r, s, t, a, b) * D[1, 2](f)(r, s, t, a, b) - 2 * D[5](f)(r, s, t, a, b) * D[4](f)(r, \\
& s, t, a, b) * D[1, 3](f)(r, s, t, a, b) * D[1, 2](f)(r, s, t, a, b) - \\
& 2 * D[2](f)(r, s, t, a, b) * D[1, 3](f)(r, s, t, a, b) * D[1, 2](f)(r, s, t, a, b) + D[4](f)(r, \\
& s, t, a, b)^2 * D[3, 3](f)(r, s, t, a, b) * D[1, 1](f)(r, s, t, a, b) - \\
& D[4](f)(r, s, t, a, b) * D[3, 5](f)(r, s, t, a, b) * D[2](f)(r, s, t, a, b) * D[1, 1](f)(r, s, t, \\
& a, b) - \\
& D[5](f)(r, s, t, a, b) * D[3, 4](f)(r, s, t, a, b) * D[2](f)(r, s, t, a, b) * D[1, 1](f)(r, s, t, \\
& a, b) - \\
& 2 * D[4](f)(r, s, t, a, b) * D[3](f)(r, s, t, a, b) * D[2, 5](f)(r, s, t, a, b) * D[1, 1](f)(r, \\
& s, t, a, b) + \\
& D[5](f)(r, s, t, a, b) * D[4](f)(r, s, t, a, b) * D[2, 3](f)(r, s, t, a, b) * D[1, 1](f)(r, s, t, \\
& a, b) + 2 * D[3, 3](f)(r, s, t, a, b) * D[1](f)(r, s, t, a, b) * \\
& D[1, 1](f)(r, s, t, a, b) + D[5](f)(r, s, t, a, b)^2 * D[1, 3](f)(r, s, t, a, b) * D[1, \\
& 1](f)(r, s, t, a, b) + 4 * D[3](f)(r, s, t, a, b) * D[1, 3](f)(r, s, t, a, b) * \\
& D[1, 1](f)(r, s, t, a, b) + 2 * D[5, 5](f)(r, s, t, a, b) * D[3](f)(r, s, t, a, b) * D[1](f)(r, \\
& s, t, a, b) * (D[4, 4](f)(r, s, t, a, b) * D[1](f)(r, s, t, a, b) + \\
& D[1, 1](f)(r, s, t, a, b)) + 2 * D[4, 5](f)(r, s, t, a, b) * D[3](f)(r, s, t, a, b) * (-2 \\
& * D[1](f)(r, s, t, a, b) * D[1, 2](f)(r, s, t, a, b) + \\
& D[2](f)(r, s, t, a, b) * D[1, 1](f)(r, s, t, a, b))) / \\
& (D[4](f)(r, s, t, a, b)^2 * D[3](f)(r, s, t, a, b) - D[5](f)(r, s, t, a, b) * D[4](f)(r, s, t, \\
& a, b) * D[2](f)(r, s, t, a, b) - \\
& D[2](f)(r, s, t, a, b)^2 + (D[5](f)(r, s, t, a, b)^2 + 4 * D[3](f)(r, s, t, a, b)) \\
& * D[1](f)(r, s, t, a, b))),
\end{aligned}$$

$$\begin{aligned}
& D[1, 1, 4](f)(r, s, t, a, b) = \\
& ((-4 * D[4, 5](f)(r, s, t, a, b) * D[2, 4](f)(r, s, t, a, b) * D[1](f)(r, s, t, a, b)^2 - 4 \\
& \quad * D[4, 5](f)(r, s, t, a, b) * D[1](f)(r, s, t, a, b)^2 * \\
& D[1, 5](f)(r, s, t, a, b) + 2 * D[4, 5](f)(r, s, t, a, b) * D[2](f)(r, s, t, a, b) * D[1](f)(r, \\
& \quad s, t, a, b) * D[1, 4](f)(r, s, t, a, b) + \\
& 2 * D[5](f)(r, s, t, a, b) * D[2, 4](f)(r, s, t, a, b) * D[1](f)(r, s, t, a, b) * D[1, 4](f)(r, \\
& \quad s, t, a, b) + 4 * D[2, 2](f)(r, s, t, a, b) * \\
& D[1](f)(r, s, t, a, b) * D[1, 4](f)(r, s, t, a, b) + 4 * D[5, 5](f)(r, s, t, a, b) * D[1](f)(r, \\
& \quad s, t, a, b)^2 * D[1, 4](f)(r, s, t, a, b) - 2 * D[5](f)(r, s, t, a, b) * \\
& D[2](f)(r, s, t, a, b) * D[1, 4](f)(r, s, t, a, b)^2 + 4 * D[1](f)(r, s, t, a, b) * D[1, \\
& \quad 4](f)(r, s, t, a, b) * D[1, 3](f)(r, s, t, a, b) - \\
& 4 * D[2, 4](f)(r, s, t, a, b) * D[1](f)(r, s, t, a, b) * D[1, 2](f)(r, s, t, a, b) - 4 \\
& \quad * D[1](f)(r, s, t, a, b) * D[1, 5](f)(r, s, t, a, b) * D[1, 2](f)(r, s, t, a, b) - \\
& 4 * D[2](f)(r, s, t, a, b) * D[1, 4](f)(r, s, t, a, b) * D[1, 2](f)(r, s, t, a, b) + D[4](f)(r, \\
& \quad s, t, a, b)^2 * D[3, 4](f)(r, s, t, a, b) * D[1, 1](f)(r, s, t, a, b) + \\
& 2 * D[2](f)(r, s, t, a, b) * D[2, 4](f)(r, s, t, a, b) * D[1, 1](f)(r, s, t, a, b) + 2 \\
& \quad * D[5](f)(r, s, t, a, b) * D[4, 5](f)(r, s, t, a, b) * D[1](f)(r, s, t, a, b) * \\
& D[1, 1](f)(r, s, t, a, b) + 4 * D[2, 5](f)(r, s, t, a, b) * D[1](f)(r, s, t, a, b) * D[1, \\
& \quad 1](f)(r, s, t, a, b) + D[5](f)(r, s, t, a, b)^2 * \\
& D[1, 4](f)(r, s, t, a, b) * D[1, 1](f)(r, s, t, a, b) + 4 * D[3](f)(r, s, t, a, b) * D[1, \\
& \quad 4](f)(r, s, t, a, b) * D[1, 1](f)(r, s, t, a, b) - \\
& D[4](f)(r, s, t, a, b) * (2 * D[4, 5](f)(r, s, t, a, b)^2 * D[1](f)(r, s, t, a, b)^2 - 2 * D[5, \\
& \quad 5](f)(r, s, t, a, b) * D[4, 4](f)(r, s, t, a, b) * \\
& D[1](f)(r, s, t, a, b)^2 + 2 * D[3, 4](f)(r, s, t, a, b) * D[1](f)(r, s, t, a, b) * D[1, \\
& \quad 4](f)(r, s, t, a, b) - 2 * D[3](f)(r, s, t, a, b) * \\
& D[1, 4](f)(r, s, t, a, b)^2 - 2 * D[4, 4](f)(r, s, t, a, b) * D[1](f)(r, s, t, a, b) * D[1, \\
& \quad 3](f)(r, s, t, a, b) - 2 * D[1, 2](f)(r, s, t, a, b)^2 + \\
& D[4, 5](f)(r, s, t, a, b) * D[2](f)(r, s, t, a, b) * D[1, 1](f)(r, s, t, a, b) + D[5](f)(r, s, \\
& \quad t, a, b) * D[2, 4](f)(r, s, t, a, b) * D[1, 1](f)(r, s, t, a, b) + \\
& 2 * D[2, 2](f)(r, s, t, a, b) * D[1, 1](f)(r, s, t, a, b)) + D[4, 4](f)(r, s, t, a, b) * (4 \\
& \quad * D[2, 5](f)(r, s, t, a, b) * D[1](f)(r, s, t, a, b)^2 - 2 * D[5](f)(r, s, t, a, b) * \\
& D[1](f)(r, s, t, a, b) * D[1, 2](f)(r, s, t, a, b) + D[2](f)(r, s, t, a, b) * (-2 \\
& \quad * D[1](f)(r, s, t, a, b) * D[1, 5](f)(r, s, t, a, b) + \\
& D[5](f)(r, s, t, a, b) * D[1, 1](f)(r, s, t, a, b))) / \\
& (D[4](f)(r, s, t, a, b)^2 * D[3](f)(r, s, t, a, b) - D[5](f)(r, s, t, a, b) * D[4](f)(r, s, t, \\
& \quad a, b) * D[2](f)(r, s, t, a, b) - \\
& D[2](f)(r, s, t, a, b)^2 + (D[5](f)(r, s, t, a, b)^2 + 4 * D[3](f)(r, s, t, a, b)) \\
& \quad * D[1](f)(r, s, t, a, b))), \\
& D[1, 1, 5](f)(r, s, t, a, b) = \\
& ((4 * D[4, 4](f)(r, s, t, a, b) * D[3, 5](f)(r, s, t, a, b) * D[1](f)(r, s, t, a, b)^2 - 4 * D[4, \\
& \quad 5](f)(r, s, t, a, b) * D[3, 4](f)(r, s, t, a, b) * \\
& D[1](f)(r, s, t, a, b)^2 - 2 * D[4, 5](f)(r, s, t, a, b) * D[2](f)(r, s, t, a, b) * D[1](f)(r, \\
& \quad s, t, a, b) * D[1, 5](f)(r, s, t, a, b) - \\
& 2 * D[4](f)(r, s, t, a, b) * D[3, 5](f)(r, s, t, a, b) * D[1](f)(r, s, t, a, b) * D[1, 4](f)(r, \\
& \quad s, t, a, b) + 2 * D[5, 5](f)(r, s, t, a, b) * \\
& D[2](f)(r, s, t, a, b) * D[1](f)(r, s, t, a, b) * D[1, 4](f)(r, s, t, a, b) + 4 * D[2, 3](f)(r, \\
& \quad s, t, a, b) * D[1](f)(r, s, t, a, b) * \\
& D[1, 4](f)(r, s, t, a, b) + 2 * D[4](f)(r, s, t, a, b) * D[3](f)(r, s, t, a, b) * D[1, 5](f)(r,
\end{aligned}$$

$$\begin{aligned}
& s, t, a, b) * D[1, 4](f)(r, s, t, a, b) + 2 * D[4](f)(r, s, t, a, b) * \\
& D[4, 5](f)(r, s, t, a, b) * D[1](f)(r, s, t, a, b) * D[1, 3](f)(r, s, t, a, b) - 2 * D[2](f)(r, \\
& s, t, a, b) * D[1, 4](f)(r, s, t, a, b) * \\
& D[1, 3](f)(r, s, t, a, b) - 4 * D[3, 4](f)(r, s, t, a, b) * D[1](f)(r, s, t, a, b) * D[1, \\
& 2](f)(r, s, t, a, b) - 2 * D[2](f)(r, s, t, a, b) * \\
& D[1, 5](f)(r, s, t, a, b) * D[1, 2](f)(r, s, t, a, b) + 2 * D[4](f)(r, s, t, a, b) * D[1, \\
& 3](f)(r, s, t, a, b) * D[1, 2](f)(r, s, t, a, b) + \\
& D[4](f)(r, s, t, a, b)^2 * D[3, 5](f)(r, s, t, a, b) * D[1, 1](f)(r, s, t, a, b) - D[5, \\
& 5](f)(r, s, t, a, b) * D[4](f)(r, s, t, a, b) * D[2](f)(r, s, t, a, b) * \\
& D[1, 1](f)(r, s, t, a, b) + 2 * D[3, 4](f)(r, s, t, a, b) * D[2](f)(r, s, t, a, b) * D[1, \\
& 1](f)(r, s, t, a, b) - 2 * D[4](f)(r, s, t, a, b) * \\
& D[2, 3](f)(r, s, t, a, b) * D[1, 1](f)(r, s, t, a, b) + 4 * D[3, 5](f)(r, s, t, a, b) \\
& * D[1](f)(r, s, t, a, b) * D[1, 1](f)(r, s, t, a, b) + \\
& D[5](f)(r, s, t, a, b)^2 * D[1, 5](f)(r, s, t, a, b) * D[1, 1](f)(r, s, t, a, b) + 4 \\
& * D[3](f)(r, s, t, a, b) * D[1, 5](f)(r, s, t, a, b) * D[1, 1](f)(r, s, t, a, b) + \\
& D[5](f)(r, s, t, a, b) * (-2 * D[4, 5](f)(r, s, t, a, b)^2 * D[1](f)(r, s, t, a, b)^2 + 2 \\
& * D[2, 5](f)(r, s, t, a, b) * D[1](f)(r, s, t, a, b) * \\
& D[1, 4](f)(r, s, t, a, b) - 2 * D[2](f)(r, s, t, a, b) * D[1, 5](f)(r, s, t, a, b) * D[1, \\
& 4](f)(r, s, t, a, b) - D[4](f)(r, s, t, a, b) * D[2, 5](f)(r, s, t, a, b) * \\
& D[1, 1](f)(r, s, t, a, b) + 2 * D[5, 5](f)(r, s, t, a, b) * D[1](f)(r, s, t, a, b) * (D[4, \\
& 4](f)(r, s, t, a, b) * D[1](f)(r, s, t, a, b) + \\
& D[1, 1](f)(r, s, t, a, b)) + D[4, 5](f)(r, s, t, a, b) * (-2 * D[1](f)(r, s, t, a, b) * D[1, \\
& 2](f)(r, s, t, a, b) + D[2](f)(r, s, t, a, b) * D[1, 1](f)(r, s, t, a, b))) / \\
& (D[4](f)(r, s, t, a, b)^2 * D[3](f)(r, s, t, a, b) - D[5](f)(r, s, t, a, b) * D[4](f)(r, s, t, \\
& a, b) * D[2](f)(r, s, t, a, b) - \\
& D[2](f)(r, s, t, a, b)^2 + (D[5](f)(r, s, t, a, b)^2 + 4 * D[3](f)(r, s, t, a, b)) \\
& * D[1](f)(r, s, t, a, b))), \\
& D[1, 2, 2](f)(r, s, t, a, b) = \\
& (-2 * D[4, 5](f)(r, s, t, a, b)^2 * D[2](f)(r, s, t, a, b)^2 * D[1](f)(r, s, t, a, b) - 4 \\
& * D[3, 4](f)(r, s, t, a, b) * \\
& D[2](f)(r, s, t, a, b) * D[2, 4](f)(r, s, t, a, b) * D[1](f)(r, s, t, a, b) + 2 * D[2](f)(r, s, \\
& t, a, b) * \\
& D[2, 5](f)(r, s, t, a, b) * D[2, 4](f)(r, s, t, a, b) * D[1](f)(r, s, t, a, b) + 2 * D[3](f)(r, \\
& s, t, a, b) * D[2, 4](f)(r, s, t, a, b)^2 * \\
& D[1](f)(r, s, t, a, b) + 4 * D[4, 4](f)(r, s, t, a, b) * D[2](f)(r, s, t, a, b) * D[2, 3](f)(r, \\
& s, t, a, b) * D[1](f)(r, s, t, a, b) - \\
& 2 * D[4](f)(r, s, t, a, b) * D[2, 4](f)(r, s, t, a, b) * D[2, 3](f)(r, s, t, a, b) * D[1](f)(r, s, \\
& t, a, b) - \\
& 2 * D[4, 4](f)(r, s, t, a, b) * D[3](f)(r, s, t, a, b) * D[2, 2](f)(r, s, t, a, b) * D[1](f)(r, s, \\
& t, a, b) + \\
& 2 * D[4](f)(r, s, t, a, b) * D[3, 4](f)(r, s, t, a, b) * D[2, 2](f)(r, s, t, a, b) * D[1](f)(r, s, \\
& t, a, b) - \\
& 2 * D[3, 4](f)(r, s, t, a, b)^2 * D[1](f)(r, s, t, a, b)^2 + 2 * D[4, 4](f)(r, s, t, a, b) \\
& * D[3, 3](f)(r, s, t, a, b) * D[1](f)(r, s, t, a, b)^2 - \\
& 4 * D[3, 4](f)(r, s, t, a, b) * D[2, 5](f)(r, s, t, a, b) * D[1](f)(r, s, t, a, b)^2 - 2 \\
& * D[2](f)(r, s, t, a, b)^2 * \\
& D[2, 4](f)(r, s, t, a, b) * D[1, 5](f)(r, s, t, a, b) + D[4](f)(r, s, t, a, b) * D[2](f)(r, s, t, \\
& a, b) * D[2, 2](f)(r, s, t, a, b) * D[1, 5](f)(r, s, t, a, b) -
\end{aligned}$$

$$\begin{aligned}
& 4 * D[3, 4](f)(r, s, t, a, b) * D[2](f)(r, s, t, a, b) * D[1](f)(r, s, t, a, b) * D[1, 5](f)(r, s, \\
& \quad t, a, b) - \\
& 2 * D[4](f)(r, s, t, a, b) * D[2, 3](f)(r, s, t, a, b) * D[1](f)(r, s, t, a, b) * D[1, 5](f)(r, s, \\
& \quad t, a, b) - \\
& 2 * D[2](f)(r, s, t, a, b)^2 * D[1, 5](f)(r, s, t, a, b)^2 + \\
& 2 * D[2](f)(r, s, t, a, b)^2 * D[2, 5](f)(r, s, t, a, b) * D[1, 4](f)(r, s, t, a, b) - 2 \\
& \quad * D[4](f)(r, s, t, a, b) * \\
& D[2](f)(r, s, t, a, b) * D[2, 3](f)(r, s, t, a, b) * D[1, 4](f)(r, s, t, a, b) + 2 * D[4](f)(r, \\
& \quad s, t, a, b) * \\
& D[3](f)(r, s, t, a, b) * D[2, 2](f)(r, s, t, a, b) * D[1, 4](f)(r, s, t, a, b) - D[5](f)(r, s, t, \\
& \quad a, b) * D[2](f)(r, s, t, a, b) * D[2, 2](f)(r, s, t, a, b) * \\
& D[1, 4](f)(r, s, t, a, b) + 4 * D[3](f)(r, s, t, a, b) * D[3, 4](f)(r, s, t, a, b) * D[1](f)(r, \\
& \quad s, t, a, b) * D[1, 4](f)(r, s, t, a, b) - \\
& 4 * D[4](f)(r, s, t, a, b) * D[3, 3](f)(r, s, t, a, b) * D[1](f)(r, s, t, a, b) * D[1, 4](f)(r, s, \\
& \quad t, a, b) + \\
& 8 * D[3, 5](f)(r, s, t, a, b) * D[2](f)(r, s, t, a, b) * D[1](f)(r, s, t, a, b) * D[1, 4](f)(r, s, \\
& \quad t, a, b) + \\
& 4 * D[3](f)(r, s, t, a, b) * D[2, 5](f)(r, s, t, a, b) * D[1](f)(r, s, t, a, b) * D[1, 4](f)(r, s, \\
& \quad t, a, b) - \\
& 6 * D[5](f)(r, s, t, a, b) * D[2, 3](f)(r, s, t, a, b) * D[1](f)(r, s, t, a, b) * D[1, 4](f)(r, s, \\
& \quad t, a, b) - \\
& 4 * D[3](f)(r, s, t, a, b) * D[2](f)(r, s, t, a, b) * D[1, 5](f)(r, s, t, a, b) * D[1, 4](f)(r, s, \\
& \quad t, a, b) - \\
& 2 * D[3](f)(r, s, t, a, b)^2 * D[1, 4](f)(r, s, t, a, b)^2 + \\
& 2 * D[4](f)(r, s, t, a, b) * D[2](f)(r, s, t, a, b) * D[2, 4](f)(r, s, t, a, b) * D[1, 3](f)(r, s, \\
& \quad t, a, b) - \\
& D[4](f)(r, s, t, a, b)^2 * D[2, 2](f)(r, s, t, a, b) * D[1, 3](f)(r, s, t, a, b) - 4 * D[4, \\
& \quad 4](f)(r, s, t, a, b) * \\
& D[3](f)(r, s, t, a, b) * D[1](f)(r, s, t, a, b) * D[1, 3](f)(r, s, t, a, b) + 4 * D[4](f)(r, s, \\
& \quad t, a, b) * \\
& D[3, 4](f)(r, s, t, a, b) * D[1](f)(r, s, t, a, b) * D[1, 3](f)(r, s, t, a, b) + 2 * D[4](f)(r, \\
& \quad s, t, a, b) * \\
& D[2, 5](f)(r, s, t, a, b) * D[1](f)(r, s, t, a, b) * D[1, 3](f)(r, s, t, a, b) + 2 * D[5](f)(r, \\
& \quad s, t, a, b) * \\
& D[2, 4](f)(r, s, t, a, b) * D[1](f)(r, s, t, a, b) * D[1, 3](f)(r, s, t, a, b) + 4 * D[4](f)(r, \\
& \quad s, t, a, b) * \\
& D[2](f)(r, s, t, a, b) * D[1, 5](f)(r, s, t, a, b) * D[1, 3](f)(r, s, t, a, b) + 4 * D[4](f)(r, \\
& \quad s, t, a, b) * \\
& D[3](f)(r, s, t, a, b) * D[1, 4](f)(r, s, t, a, b) * D[1, 3](f)(r, s, t, a, b) - 2 * D[4](f)(r, \\
& \quad s, t, a, b)^2 * D[1, 3](f)(r, s, t, a, b)^2 - \\
& 2 * D[1](f)(r, s, t, a, b) * D[1, 3](f)(r, s, t, a, b)^2 - \\
& 2 * D[4](f)(r, s, t, a, b) * D[2](f)(r, s, t, a, b) * D[2, 5](f)(r, s, t, a, b) * D[1, 2](f)(r, s, \\
& \quad t, a, b) + \\
& 2 * D[4](f)(r, s, t, a, b)^2 * D[2, 3](f)(r, s, t, a, b) * D[1, 2](f)(r, s, t, a, b) \\
& \quad - D[5](f)(r, s, t, a, b) * \\
& D[4](f)(r, s, t, a, b) * D[2, 2](f)(r, s, t, a, b) * D[1, 2](f)(r, s, t, a, b) - 2 * D[2](f)(r, \\
& \quad s, t, a, b) * \\
& D[2, 2](f)(r, s, t, a, b) * D[1, 2](f)(r, s, t, a, b) + 4 * D[5](f)(r, s, t, a, b) * D[3,
\end{aligned}$$



$$\begin{aligned}
& 4](f)(r, s, t, a, b) * D[1](f)(r, s, t, a, b) * D[1, 2](f)(r, s, t, a, b) + \\
& 2 * D[5](f)(r, s, t, a, b) * D[2, 5](f)(r, s, t, a, b) * D[1](f)(r, s, t, a, b) * D[1, 2](f)(r, s, \\
& t, a, b) + \\
& 4 * D[2, 3](f)(r, s, t, a, b) * D[1](f)(r, s, t, a, b) * D[1, 2](f)(r, s, t, a, b) + 2 \\
& * D[4](f)(r, s, t, a, b) * \\
& D[3](f)(r, s, t, a, b) * D[1, 5](f)(r, s, t, a, b) * D[1, 2](f)(r, s, t, a, b) + 2 * D[5](f)(r, \\
& s, t, a, b) * \\
& D[2](f)(r, s, t, a, b) * D[1, 5](f)(r, s, t, a, b) * D[1, 2](f)(r, s, t, a, b) + 2 * D[5](f)(r, \\
& s, t, a, b) * \\
& D[3](f)(r, s, t, a, b) * D[1, 4](f)(r, s, t, a, b) * D[1, 2](f)(r, s, t, a, b) - 4 * D[5](f)(r, \\
& s, t, a, b) * \\
& D[4](f)(r, s, t, a, b) * D[1, 3](f)(r, s, t, a, b) * D[1, 2](f)(r, s, t, a, b) - 2 * D[2](f)(r, \\
& s, t, a, b) * \\
& D[1, 3](f)(r, s, t, a, b) * D[1, 2](f)(r, s, t, a, b) + 2 * D[3](f)(r, s, t, a, b) * D[1, \\
& 2](f)(r, s, t, a, b)^2 + \\
& 2 * D[4, 4](f)(r, s, t, a, b) * D[3](f)(r, s, t, a, b)^2 * D[1, 1](f)(r, s, t, a, b) - 4 \\
& * D[4](f)(r, s, t, a, b) * \\
& D[3](f)(r, s, t, a, b) * D[3, 4](f)(r, s, t, a, b) * D[1, 1](f)(r, s, t, a, b) + 2 * D[4](f)(r, \\
& s, t, a, b)^2 * \\
& D[3, 3](f)(r, s, t, a, b) * D[1, 1](f)(r, s, t, a, b) - 4 * D[4](f)(r, s, t, a, b) * D[3, \\
& 5](f)(r, s, t, a, b) * D[2](f)(r, s, t, a, b) * D[1, 1](f)(r, s, t, a, b) - \\
& 2 * D[4](f)(r, s, t, a, b) * D[3](f)(r, s, t, a, b) * D[2, 5](f)(r, s, t, a, b) * D[1, 1](f)(r, s, \\
& t, a, b) - \\
& 2 * D[5](f)(r, s, t, a, b) * D[2](f)(r, s, t, a, b) * D[2, 5](f)(r, s, t, a, b) * D[1, 1](f)(r, s, \\
& t, a, b) - \\
& 2 * D[5](f)(r, s, t, a, b) * D[3](f)(r, s, t, a, b) * D[2, 4](f)(r, s, t, a, b) * D[1, 1](f)(r, s, \\
& t, a, b) + \\
& 4 * D[5](f)(r, s, t, a, b) * D[4](f)(r, s, t, a, b) * D[2, 3](f)(r, s, t, a, b) * D[1, 1](f)(r, s, \\
& t, a, b) + \\
& 2 * D[2](f)(r, s, t, a, b) * D[2, 3](f)(r, s, t, a, b) * D[1, 1](f)(r, s, t, a, b) + D[5](f)(r, \\
& s, t, a, b)^2 * \\
& D[2, 2](f)(r, s, t, a, b) * D[1, 1](f)(r, s, t, a, b) + 2 * D[3](f)(r, s, t, a, b) * D[2, \\
& 2](f)(r, s, t, a, b) * D[1, 1](f)(r, s, t, a, b) + 2 * D[3, 3](f)(r, s, t, a, b) * \\
& D[1](f)(r, s, t, a, b) * D[1, 1](f)(r, s, t, a, b) + 2 * D[5, 5](f)(r, s, t, a, b) * D[2](f)(r, \\
& s, t, a, b)^2 * (D[4, 4](f)(r, s, t, a, b) * D[1](f)(r, s, t, a, b) + \\
& D[1, 1](f)(r, s, t, a, b)) - 2 * D[4, 5](f)(r, s, t, a, b) * (2 * D[1](f)(r, s, t, a, b) * ( \\
& - (D[2, 3](f)(r, s, t, a, b) * D[1](f)(r, s, t, a, b)) + \\
& D[3](f)(r, s, t, a, b) * D[1, 2](f)(r, s, t, a, b)) + D[2](f)(r, s, t, a, b) * (D[2, 2](f)(r, \\
& s, t, a, b) * D[1](f)(r, s, t, a, b) + \\
& 2 * D[1](f)(r, s, t, a, b) * D[1, 3](f)(r, s, t, a, b) - 2 * D[3](f)(r, s, t, a, b) * D[1, \\
& 1](f)(r, s, t, a, b))) / \\
& (D[4](f)(r, s, t, a, b)^2 * D[3](f)(r, s, t, a, b) - D[5](f)(r, s, t, a, b) * D[4](f)(r, s, t, a, \\
& b) * D[2](f)(r, s, t, a, b) - \\
& D[2](f)(r, s, t, a, b)^2 + (D[5](f)(r, s, t, a, b)^2 + 4 * D[3](f)(r, s, t, a, b)) \\
& * D[1](f)(r, s, t, a, b)), \\
& D[1, 2, 3](f)(r, s, t, a, b) = \\
& (-2 * D[4, 5](f)(r, s, t, a, b)^2 * D[3](f)(r, s, t, a, b) * D[2](f)(r, s, t, a, b) \\
& * D[1](f)(r, s, t, a, b) - 2 * D[3, 4](f)(r, s, t, a, b)^2 *
\end{aligned}$$

$$\begin{aligned}
& D[2](f)(r, s, t, a, b) * D[1](f)(r, s, t, a, b) + 2 * D[4, 4](f)(r, s, t, a, b) * D[3, 3](f)(r, s, t, a, b) * D[2](f)(r, s, t, a, b) * D[1](f)(r, s, t, a, b) - \\
& D[3, 4](f)(r, s, t, a, b) * D[2](f)(r, s, t, a, b) * D[2, 5](f)(r, s, t, a, b) * D[1](f)(r, s, t, a, b) - \\
& D[4](f)(r, s, t, a, b) * D[3, 3](f)(r, s, t, a, b) * D[2, 4](f)(r, s, t, a, b) * D[1](f)(r, s, t, a, b) + \\
& D[3, 5](f)(r, s, t, a, b) * D[2](f)(r, s, t, a, b) * D[2, 4](f)(r, s, t, a, b) * D[1](f)(r, s, t, a, b) + 2 * D[3](f)(r, s, t, a, b) * \\
& D[2, 5](f)(r, s, t, a, b) * D[2, 4](f)(r, s, t, a, b) * D[1](f)(r, s, t, a, b) + D[4](f)(r, s, t, a, b) * D[3, 4](f)(r, s, t, a, b) * D[2, 3](f)(r, s, t, a, b) * \\
& D[1](f)(r, s, t, a, b) - D[5](f)(r, s, t, a, b) * D[2, 4](f)(r, s, t, a, b) * D[2, 3](f)(r, s, t, a, b) * D[1](f)(r, s, t, a, b) + \\
& D[5](f)(r, s, t, a, b) * D[3, 4](f)(r, s, t, a, b) * D[2, 2](f)(r, s, t, a, b) * D[1](f)(r, s, t, a, b) - 2 * D[3, 5](f)(r, s, t, a, b) * \\
& D[3, 4](f)(r, s, t, a, b) * D[1](f)(r, s, t, a, b)^2 - D[3, 4](f)(r, s, t, a, b) * D[2](f)(r, s, t, a, b)^2 * D[1, 5](f)(r, s, t, a, b) - \\
& D[3](f)(r, s, t, a, b) * D[2](f)(r, s, t, a, b) * D[2, 4](f)(r, s, t, a, b) * D[1, 5](f)(r, s, t, a, b) + \\
& D[4](f)(r, s, t, a, b) * D[3](f)(r, s, t, a, b) * D[2, 2](f)(r, s, t, a, b) * D[1, 5](f)(r, s, t, a, b) - 2 * D[3](f)(r, s, t, a, b) * \\
& D[3, 4](f)(r, s, t, a, b) * D[1](f)(r, s, t, a, b) * D[1, 5](f)(r, s, t, a, b) - D[4](f)(r, s, t, a, b) * D[3, 3](f)(r, s, t, a, b) * D[1](f)(r, s, t, a, b) * \\
& D[1, 5](f)(r, s, t, a, b) - 2 * D[3](f)(r, s, t, a, b) * D[2](f)(r, s, t, a, b) * D[1, 5](f)(r, s, t, a, b)^2 - \\
& D[4](f)(r, s, t, a, b) * D[3, 3](f)(r, s, t, a, b) * D[2](f)(r, s, t, a, b) * D[1, 4](f)(r, s, t, a, b) + D[3, 5](f)(r, s, t, a, b) * D[2](f)(r, s, t, a, b)^2 * \\
& D[1, 4](f)(r, s, t, a, b) + D[3](f)(r, s, t, a, b) * D[2](f)(r, s, t, a, b) * D[2, 5](f)(r, s, t, a, b) * D[1, 4](f)(r, s, t, a, b) + \\
& D[4](f)(r, s, t, a, b) * D[3](f)(r, s, t, a, b) * D[2, 3](f)(r, s, t, a, b) * D[1, 4](f)(r, s, t, a, b) - \\
& D[5](f)(r, s, t, a, b) * D[2](f)(r, s, t, a, b) * D[2, 3](f)(r, s, t, a, b) * D[1, 4](f)(r, s, t, a, b) + 6 * D[3](f)(r, s, t, a, b) * \\
& D[3, 5](f)(r, s, t, a, b) * D[1](f)(r, s, t, a, b) * D[1, 4](f)(r, s, t, a, b) - 3 * D[5](f)(r, s, t, a, b) * \\
& D[3, 3](f)(r, s, t, a, b) * D[1](f)(r, s, t, a, b) * D[1, 4](f)(r, s, t, a, b) - 2 * D[3](f)(r, s, t, a, b)^2 * \\
& D[1, 5](f)(r, s, t, a, b) * D[1, 4](f)(r, s, t, a, b) + D[4](f)(r, s, t, a, b) * D[3, 4](f)(r, s, t, a, b) * D[2](f)(r, s, t, a, b) * D[1, 3](f)(r, s, t, a, b) + \\
& D[4](f)(r, s, t, a, b) * D[3](f)(r, s, t, a, b) * D[2, 4](f)(r, s, t, a, b) * D[1, 3](f)(r, s, t, a, b) - \\
& D[5](f)(r, s, t, a, b) * D[4](f)(r, s, t, a, b) * D[2, 2](f)(r, s, t, a, b) * D[1, 3](f)(r, s, t, a, b) - \\
& D[2](f)(r, s, t, a, b) * D[2, 2](f)(r, s, t, a, b) * D[1, 3](f)(r, s, t, a, b) + D[4](f)(r, s, t, a, b) * D[3, 5](f)(r, s, t, a, b) * D[1](f)(r, s, t, a, b) * \\
& D[1, 3](f)(r, s, t, a, b) + 3 * D[5](f)(r, s, t, a, b) * D[3, 4](f)(r, s, t, a, b) * D[1](f)(r, s, t, a, b) * D[1, 3](f)(r, s, t, a, b) + \\
& D[5](f)(r, s, t, a, b) * D[2, 5](f)(r, s, t, a, b) * D[1](f)(r, s, t, a, b) * D[1, 3](f)(r, s, t, a, b) + 2 * D[2, 3](f)(r, s, t, a, b) *
\end{aligned}$$

$$\begin{aligned}
& D[1](f)(r, s, t, a, b) * D[1, 3](f)(r, s, t, a, b) + 3 * D[4](f)(r, s, t, a, b) * D[3](f)(r, s, \\
& t, a, b) * D[1, 5](f)(r, s, t, a, b) * D[1, 3](f)(r, s, t, a, b) + \\
& D[5](f)(r, s, t, a, b) * D[2](f)(r, s, t, a, b) * D[1, 5](f)(r, s, t, a, b) * D[1, 3](f)(r, s, t, \\
& a, b) + \\
& D[5](f)(r, s, t, a, b) * D[3](f)(r, s, t, a, b) * D[1, 4](f)(r, s, t, a, b) * D[1, 3](f)(r, s, t, \\
& a, b) - 2 * D[5](f)(r, s, t, a, b) * D[4](f)(r, s, t, a, b) * \\
& D[1, 3](f)(r, s, t, a, b)^2 - D[2](f)(r, s, t, a, b) * D[1, 3](f)(r, s, t, a, b)^2 \\
& + D[4](f)(r, s, t, a, b)^2 * \\
& D[3, 3](f)(r, s, t, a, b) * D[1, 2](f)(r, s, t, a, b) - D[4](f)(r, s, t, a, b) * D[3, 5](f)(r, s, \\
& t, a, b) * D[2](f)(r, s, t, a, b) * D[1, 2](f)(r, s, t, a, b) - \\
& D[4](f)(r, s, t, a, b) * D[3](f)(r, s, t, a, b) * D[2, 5](f)(r, s, t, a, b) * D[1, 2](f)(r, s, t, \\
& a, b) - \\
& D[2](f)(r, s, t, a, b) * D[2, 3](f)(r, s, t, a, b) * D[1, 2](f)(r, s, t, a, b) + D[5](f)(r, s, t, \\
& a, b) * D[3, 5](f)(r, s, t, a, b) * D[1](f)(r, s, t, a, b) * \\
& D[1, 2](f)(r, s, t, a, b) + 2 * D[3, 3](f)(r, s, t, a, b) * D[1](f)(r, s, t, a, b) * D[1, \\
& 2](f)(r, s, t, a, b) + D[5](f)(r, s, t, a, b) * \\
& D[3](f)(r, s, t, a, b) * D[1, 5](f)(r, s, t, a, b) * D[1, 2](f)(r, s, t, a, b) + 2 * D[3](f)(r, \\
& s, t, a, b) * \\
& D[1, 3](f)(r, s, t, a, b) * D[1, 2](f)(r, s, t, a, b) - 3 * D[4](f)(r, s, t, a, b) * D[3](f)(r, \\
& s, t, a, b) * D[3, 5](f)(r, s, t, a, b) * D[1, 1](f)(r, s, t, a, b) - \\
& D[5](f)(r, s, t, a, b) * D[3](f)(r, s, t, a, b) * D[3, 4](f)(r, s, t, a, b) * D[1, 1](f)(r, s, t, \\
& a, b) + \\
& 2 * D[5](f)(r, s, t, a, b) * D[4](f)(r, s, t, a, b) * D[3, 3](f)(r, s, t, a, b) * D[1, 1](f)(r, s, \\
& t, a, b) - \\
& D[5](f)(r, s, t, a, b) * D[3, 5](f)(r, s, t, a, b) * D[2](f)(r, s, t, a, b) * D[1, 1](f)(r, s, t, \\
& a, b) + \\
& D[3, 3](f)(r, s, t, a, b) * D[2](f)(r, s, t, a, b) * D[1, 1](f)(r, s, t, a, b) - D[5](f)(r, s, t, \\
& a, b) * D[3](f)(r, s, t, a, b) * D[2, 5](f)(r, s, t, a, b) * \\
& D[1, 1](f)(r, s, t, a, b) + D[5](f)(r, s, t, a, b)^2 * D[2, 3](f)(r, s, t, a, b) * D[1, \\
& 1](f)(r, s, t, a, b) + 2 * D[3](f)(r, s, t, a, b) * \\
& D[2, 3](f)(r, s, t, a, b) * D[1, 1](f)(r, s, t, a, b) + 2 * D[5, 5](f)(r, s, t, a, b) \\
& * D[3](f)(r, s, t, a, b) * D[2](f)(r, s, t, a, b) * (D[4, 4](f)(r, s, t, a, b) * \\
& D[1](f)(r, s, t, a, b) + D[1, 1](f)(r, s, t, a, b)) + 2 * D[4, 5](f)(r, s, t, a, b) * (D[3, \\
& 3](f)(r, s, t, a, b) * D[1](f)(r, s, t, a, b)^2 - D[3](f)(r, s, t, a, b) * \\
& D[1](f)(r, s, t, a, b) * (D[2, 2](f)(r, s, t, a, b) + 2 * D[1, 3](f)(r, s, t, a, b)) \\
& + D[3](f)(r, s, t, a, b)^2 * D[1, 1](f)(r, s, t, a, b))) / \\
& (D[4](f)(r, s, t, a, b)^2 * D[3](f)(r, s, t, a, b) - D[5](f)(r, s, t, a, b) * D[4](f)(r, s, t, a, \\
& b) * D[2](f)(r, s, t, a, b) - \\
& D[2](f)(r, s, t, a, b)^2 + (D[5](f)(r, s, t, a, b)^2 + 4 * D[3](f)(r, s, t, a, b)) \\
& * D[1](f)(r, s, t, a, b)), \\
& D[1, 2, 4](f)(r, s, t, a, b) = \\
& (-3 * D[4, 5](f)(r, s, t, a, b) * D[2](f)(r, s, t, a, b) * D[2, 4](f)(r, s, t, a, b) \\
& * D[1](f)(r, s, t, a, b) + D[5](f)(r, s, t, a, b) * D[2, 4](f)(r, s, t, a, b)^2 * \\
& D[1](f)(r, s, t, a, b) - 2 * D[4, 5](f)(r, s, t, a, b) * D[3, 4](f)(r, s, t, a, b) * D[1](f)(r, \\
& s, t, a, b)^2 - 4 * D[4, 5](f)(r, s, t, a, b) * \\
& D[2](f)(r, s, t, a, b) * D[1](f)(r, s, t, a, b) * D[1, 5](f)(r, s, t, a, b) + D[5](f)(r, s, t, a, \\
& b) * D[2, 4](f)(r, s, t, a, b) * D[1](f)(r, s, t, a, b) * \\
& D[1, 5](f)(r, s, t, a, b) + D[4, 5](f)(r, s, t, a, b) * D[2](f)(r, s, t, a, b)^2 * D[1,
\end{aligned}$$

$$\begin{aligned}
& 4](f)(r, s, t, a, b) - \\
& D[5](f)(r, s, t, a, b) * D[2](f)(r, s, t, a, b) * D[2, 4](f)(r, s, t, a, b) * D[1, 4](f)(r, s, t, a, b) + 2 * D[4, 5](f)(r, s, t, a, b) * \\
& D[3](f)(r, s, t, a, b) * D[1](f)(r, s, t, a, b) * D[1, 4](f)(r, s, t, a, b) + D[5](f)(r, s, t, a, b) * D[3, 4](f)(r, s, t, a, b) * D[1](f)(r, s, t, a, b) * \\
& D[1, 4](f)(r, s, t, a, b) + 4 * D[5, 5](f)(r, s, t, a, b) * D[2](f)(r, s, t, a, b) * D[1](f)(r, s, t, a, b) * D[1, 4](f)(r, s, t, a, b) + \\
& 8 * D[2, 3](f)(r, s, t, a, b) * D[1](f)(r, s, t, a, b) * D[1, 4](f)(r, s, t, a, b) - D[5](f)(r, s, t, a, b) * D[2](f)(r, s, t, a, b) * D[1, 5](f)(r, s, t, a, b) * D[1, 4](f)(r, s, t, a, b) - \\
& D[5](f)(r, s, t, a, b) * D[3](f)(r, s, t, a, b) * D[1, 4](f)(r, s, t, a, b)^2 - 2 * D[2, 4](f)(r, s, t, a, b) * \\
& D[1](f)(r, s, t, a, b) * D[1, 3](f)(r, s, t, a, b) - 2 * D[1](f)(r, s, t, a, b) * D[1, 5](f)(r, s, t, a, b) * \\
& D[1, 3](f)(r, s, t, a, b) - D[2](f)(r, s, t, a, b) * \\
& D[1, 4](f)(r, s, t, a, b) * D[1, 3](f)(r, s, t, a, b) + D[4](f)(r, s, t, a, b)^2 * D[3, 4](f)(r, s, t, a, b) * D[1, 2](f)(r, s, t, a, b) - 2 * D[2](f)(r, s, t, a, b) * \\
& D[2, 4](f)(r, s, t, a, b) * D[1, 2](f)(r, s, t, a, b) + D[5](f)(r, s, t, a, b) * D[4, 5](f)(r, s, t, a, b) * D[1](f)(r, s, t, a, b) * D[1, 2](f)(r, s, t, a, b) - \\
& 2 * D[3, 4](f)(r, s, t, a, b) * D[1](f)(r, s, t, a, b) * D[1, 2](f)(r, s, t, a, b) - 3 \\
& * D[2](f)(r, s, t, a, b) * \\
& D[1, 5](f)(r, s, t, a, b) * D[1, 2](f)(r, s, t, a, b) + D[5](f)(r, s, t, a, b)^2 * D[1, 4](f)(r, s, t, a, b) * D[1, 2](f)(r, s, t, a, b) + D[5](f)(r, s, t, a, b) * \\
& D[1, 2](f)(r, s, t, a, b)^2 + D[5](f)(r, s, t, a, b) * D[4, 5](f)(r, s, t, a, b) * D[2](f)(r, s, t, a, b) * D[1, 1](f)(r, s, t, a, b) + \\
& D[3, 4](f)(r, s, t, a, b) * D[2](f)(r, s, t, a, b) * D[1, 1](f)(r, s, t, a, b) + \\
& 3 * D[2](f)(r, s, t, a, b) * D[2, 5](f)(r, s, t, a, b) * D[1, 1](f)(r, s, t, a, b) + 4 \\
& * D[3](f)(r, s, t, a, b) * D[2, 4](f)(r, s, t, a, b) * D[1, 1](f)(r, s, t, a, b) - D[5](f)(r, s, t, a, b) * \\
& D[2, 2](f)(r, s, t, a, b) * D[1, 1](f)(r, s, t, a, b) + 2 * D[3, 5](f)(r, s, t, a, b) * \\
& * D[1](f)(r, s, t, a, b) * D[1, 1](f)(r, s, t, a, b) - D[4, 4](f)(r, s, t, a, b) * \\
& (-3 * D[2](f)(r, s, t, a, b) * D[2, 5](f)(r, s, t, a, b) * D[1](f)(r, s, t, a, b) + D[2](f)(r, s, t, a, b)^2 * D[1, 5](f)(r, s, t, a, b) + 2 * D[1](f)(r, s, t, a, b) * \\
& (- (D[3, 5](f)(r, s, t, a, b) * D[1](f)(r, s, t, a, b)) + D[3](f)(r, s, t, a, b) * D[1, 5](f)(r, s, t, a, b)) + D[5](f)(r, s, t, a, b) * (D[2, 2](f)(r, s, t, a, b) * \\
& D[1](f)(r, s, t, a, b) + D[1](f)(r, s, t, a, b) * D[1, 3](f)(r, s, t, a, b) - D[3](f)(r, s, t, a, b) * D[1, 1](f)(r, s, t, a, b))) - D[4](f)(r, s, t, a, b) * \\
& (2 * D[4, 5](f)(r, s, t, a, b)^2 * D[2](f)(r, s, t, a, b) * D[1](f)(r, s, t, a, b) - 2 * D[5, 5](f)(r, s, t, a, b) * D[4, 4](f)(r, s, t, a, b) * \\
& D[2](f)(r, s, t, a, b) * D[1](f)(r, s, t, a, b) + D[3, 4](f)(r, s, t, a, b) * D[2, 4](f)(r, s, t, a, b) * D[1](f)(r, s, t, a, b) - D[4, 4](f)(r, s, t, a, b) * \\
& D[2, 3](f)(r, s, t, a, b) * D[1](f)(r, s, t, a, b) + D[3, 4](f)(r, s, t, a, b) * D[1](f)(r, s, t, a, b) * D[1, 5](f)(r, s, t, a, b) + D[3, 4](f)(r, s, t, a, b) * \\
& D[2](f)(r, s, t, a, b) * D[1, 4](f)(r, s, t, a, b) - 2 * D[3](f)(r, s, t, a, b) * D[2, 4](f)(r, s, t, a, b) * D[1, 4](f)(r, s, t, a, b) - D[3](f)(r, s, t, a, b) * \\
& D[1, 5](f)(r, s, t, a, b) * D[1, 4](f)(r, s, t, a, b) - D[4, 4](f)(r, s, t, a, b) * D[2](f)(r, s, t, a, b) * D[1, 3](f)(r, s, t, a, b) + D[5](f)(r, s, t, a, b) * \\
& D[2, 4](f)(r, s, t, a, b) * D[1, 2](f)(r, s, t, a, b) - 3 * D[1, 3](f)(r, s, t, a, b) * D[1, 2](f)(r, s, t, a, b) + 3 * D[2, 3](f)(r, s, t, a, b) * \\
& D[1, 1](f)(r, s, t, a, b) + D[4, 5](f)(r, s, t, a, b) * (- (D[1](f)(r, s, t, a, b) * D[1, 3](f)(r, s, t, a, b)) + D[2](f)(r, s, t, a, b) *
\end{aligned}$$

$$\begin{aligned}
& D[1, 2](f)(r, s, t, a, b) + D[3](f)(r, s, t, a, b) * D[1, 1](f)(r, s, t, a, b))) / \\
& (D[4](f)(r, s, t, a, b)^2 * D[3](f)(r, s, t, a, b) - D[5](f)(r, s, t, a, b) * D[4](f)(r, s, t, a, b) * D[2](f)(r, s, t, a, b) - \\
& D[2](f)(r, s, t, a, b)^2 + (D[5](f)(r, s, t, a, b)^2 + 4 * D[3](f)(r, s, t, a, b)) \\
& * D[1](f)(r, s, t, a, b)), \\
D[1, 2, 5](f)(r, s, t, a, b) = & \\
& (4 * D[4, 4](f)(r, s, t, a, b) * D[3, 5](f)(r, s, t, a, b) * D[2](f)(r, s, t, a, b) * D[1](f)(r, s, t, a, b) - 4 * D[4, 5](f)(r, s, t, a, b) * \\
& D[3, 4](f)(r, s, t, a, b) * D[2](f)(r, s, t, a, b) * D[1](f)(r, s, t, a, b) - D[4, 5](f)(r, s, t, a, b) * D[2](f)(r, s, t, a, b) * D[2, 5](f)(r, s, t, a, b) * \\
& D[1](f)(r, s, t, a, b) - D[4](f)(r, s, t, a, b) * D[3, 5](f)(r, s, t, a, b) * D[2, 4](f)(r, s, t, a, b) * D[1](f)(r, s, t, a, b) + \\
& D[5, 5](f)(r, s, t, a, b) * D[2](f)(r, s, t, a, b) * D[2, 4](f)(r, s, t, a, b) * D[1](f)(r, s, t, a, b) + \\
& D[4](f)(r, s, t, a, b) * D[4, 5](f)(r, s, t, a, b) * D[2, 3](f)(r, s, t, a, b) * D[1](f)(r, s, t, a, b) + 2 * D[2, 4](f)(r, s, t, a, b) * \\
& D[2, 3](f)(r, s, t, a, b) * D[1](f)(r, s, t, a, b) - 2 * D[3, 4](f)(r, s, t, a, b) * D[2, 2](f)(r, s, t, a, b) * D[1](f)(r, s, t, a, b) + 2 * D[4, 5](f)(r, s, t, a, b) * \\
& D[3, 5](f)(r, s, t, a, b) * D[1](f)(r, s, t, a, b)^2 - 2 * D[5, 5](f)(r, s, t, a, b) * D[3, 4](f)(r, s, t, a, b) * D[1](f)(r, s, t, a, b)^2 - D[4, 5](f)(r, s, t, a, b) * \\
& D[2](f)(r, s, t, a, b)^2 * D[1, 5](f)(r, s, t, a, b) + D[4](f)(r, s, t, a, b) * D[3](f)(r, s, t, a, b) * D[2, 4](f)(r, s, t, a, b) * D[1, 5](f)(r, s, t, a, b) - \\
& D[2](f)(r, s, t, a, b) * D[2, 2](f)(r, s, t, a, b) * D[1, 5](f)(r, s, t, a, b) - 2 * D[4, 5](f)(r, s, t, a, b) * \\
& D[3](f)(r, s, t, a, b) * D[1](f)(r, s, t, a, b) * D[1, 5](f)(r, s, t, a, b) - D[4](f)(r, s, t, a, b) * D[3, 5](f)(r, s, t, a, b) * D[1](f)(r, s, t, a, b) * \\
& D[1, 5](f)(r, s, t, a, b) + 2 * D[2, 3](f)(r, s, t, a, b) * D[1](f)(r, s, t, a, b) * D[1, 5](f)(r, s, t, a, b) + D[4](f)(r, s, t, a, b) * \\
& D[3](f)(r, s, t, a, b) * D[1, 5](f)(r, s, t, a, b)^2 - D[4](f)(r, s, t, a, b) * D[3, 5](f)(r, s, t, a, b) * D[2](f)(r, s, t, a, b) * D[1, 4](f)(r, s, t, a, b) + \\
& D[5, 5](f)(r, s, t, a, b) * D[2](f)(r, s, t, a, b)^2 * D[1, 4](f)(r, s, t, a, b) + D[4](f)(r, s, t, a, b) * D[3](f)(r, s, t, a, b) * D[2, 5](f)(r, s, t, a, b) * \\
& D[1, 4](f)(r, s, t, a, b) + D[2](f)(r, s, t, a, b) * D[2, 3](f)(r, s, t, a, b) * D[1, 4](f)(r, s, t, a, b) + 2 * D[5, 5](f)(r, s, t, a, b) * \\
& D[3](f)(r, s, t, a, b) * D[1](f)(r, s, t, a, b) * D[1, 4](f)(r, s, t, a, b) + 4 * D[3, 3](f)(r, s, t, a, b) * \\
& D[1](f)(r, s, t, a, b) * D[1, 4](f)(r, s, t, a, b) + D[4](f)(r, s, t, a, b) * D[4, 5](f)(r, s, t, a, b) * D[2](f)(r, s, t, a, b) * D[1, 3](f)(r, s, t, a, b) - \\
& D[2](f)(r, s, t, a, b) * D[2, 4](f)(r, s, t, a, b) * D[1, 3](f)(r, s, t, a, b) + D[4](f)(r, s, t, a, b) * D[2, 2](f)(r, s, t, a, b) * D[1, 3](f)(r, s, t, a, b) + \\
& D[5, 5](f)(r, s, t, a, b) * D[4](f)(r, s, t, a, b) * D[1](f)(r, s, t, a, b) * D[1, 3](f)(r, s, t, a, b) - 4 * D[3, 4](f)(r, s, t, a, b) * \\
& D[1](f)(r, s, t, a, b) * D[1, 3](f)(r, s, t, a, b) - 3 * D[2](f)(r, s, t, a, b) * D[1, 5](f)(r, s, t, a, b) * D[1, 3](f)(r, s, t, a, b) - 2 * D[3](f)(r, s, t, a, b) * \\
& D[1, 4](f)(r, s, t, a, b) * D[1, 3](f)(r, s, t, a, b) + 2 * D[4](f)(r, s, t, a, b) * D[1, 3](f)(r, s, t, a, b)^2 + D[4](f)(r, s, t, a, b)^2 * \\
& D[3, 5](f)(r, s, t, a, b) * D[1, 2](f)(r, s, t, a, b) - D[5, 5](f)(r, s, t, a, b) * D[4](f)(r, s, t, a, b) * D[2](f)(r, s, t, a, b) * D[1, 2](f)(r, s, t, a, b) -
\end{aligned}$$

$$\begin{aligned}
& D[2](f)(r, s, t, a, b) * D[2, 5](f)(r, s, t, a, b) * D[1, 2](f)(r, s, t, a, b) - D[4](f)(r, s, t, a, b) * D[2, 3](f)(r, s, t, a, b) * D[1, 2](f)(r, s, t, a, b) + \\
& 2 * D[3, 5](f)(r, s, t, a, b) * D[1](f)(r, s, t, a, b) * D[1, 2](f)(r, s, t, a, b) + D[5](f)(r, s, t, a, b)^2 * \\
& D[1, 5](f)(r, s, t, a, b) * D[1, 2](f)(r, s, t, a, b) + 2 * D[3](f)(r, s, t, a, b) * D[1, 5](f)(r, s, t, a, b) * D[1, 2](f)(r, s, t, a, b) - D[5, 5](f)(r, s, t, a, b) * \\
& D[4](f)(r, s, t, a, b) * D[3](f)(r, s, t, a, b) * D[1, 1](f)(r, s, t, a, b) + 2 * D[3](f)(r, s, t, a, b) * \\
& D[3, 4](f)(r, s, t, a, b) * D[1, 1](f)(r, s, t, a, b) - 2 * D[4](f)(r, s, t, a, b) * D[3, 3](f)(r, s, t, a, b) * D[1, 1](f)(r, s, t, a, b) + 3 * D[3, 5](f)(r, s, t, a, b) * \\
& D[2](f)(r, s, t, a, b) * D[1, 1](f)(r, s, t, a, b) + 2 * D[3](f)(r, s, t, a, b) * D[2, 5](f)(r, s, t, a, b) * D[1, 1](f)(r, s, t, a, b) + D[5](f)(r, s, t, a, b) * \\
& (-2 * D[4, 5](f)(r, s, t, a, b)^2 * D[2](f)(r, s, t, a, b) * D[1](f)(r, s, t, a, b) + D[2, 5](f)(r, s, t, a, b) * D[2, 4](f)(r, s, t, a, b) * \\
& D[1](f)(r, s, t, a, b) - D[2](f)(r, s, t, a, b) * D[2, 4](f)(r, s, t, a, b) * D[1, 5](f)(r, s, t, a, b) + D[2, 5](f)(r, s, t, a, b) * D[1](f)(r, s, t, a, b) * \\
& D[1, 5](f)(r, s, t, a, b) - D[2](f)(r, s, t, a, b) * D[1, 5](f)(r, s, t, a, b)^2 + D[3, 5](f)(r, s, t, a, b) * D[1](f)(r, s, t, a, b) * D[1, 4](f)(r, s, t, a, b) - \\
& D[3](f)(r, s, t, a, b) * D[1, 5](f)(r, s, t, a, b) * D[1, 4](f)(r, s, t, a, b) - D[4](f)(r, s, t, a, b) * D[2, 5](f)(r, s, t, a, b) * D[1, 2](f)(r, s, t, a, b) + \\
& D[1, 3](f)(r, s, t, a, b) * D[1, 2](f)(r, s, t, a, b) - D[2, 3](f)(r, s, t, a, b) * D[1, 1](f)(r, s, t, a, b) - D[4, 5](f)(r, s, t, a, b) * (D[2, 2](f)(r, s, t, a, b) * \\
& D[1](f)(r, s, t, a, b) + D[1](f)(r, s, t, a, b) * D[1, 3](f)(r, s, t, a, b) - D[3](f)(r, s, t, a, b) * D[1, 1](f)(r, s, t, a, b)) + D[5, 5](f)(r, s, t, a, b) * \\
& (2 * D[4, 4](f)(r, s, t, a, b) * D[2](f)(r, s, t, a, b) * D[1](f)(r, s, t, a, b) + D[1](f)(r, s, t, a, b) * D[1, 2](f)(r, s, t, a, b) + \\
& D[2](f)(r, s, t, a, b) * D[1, 1](f)(r, s, t, a, b))) / \\
& (D[4](f)(r, s, t, a, b)^2 * D[3](f)(r, s, t, a, b) - D[5](f)(r, s, t, a, b) * D[4](f)(r, s, t, a, b) * D[2](f)(r, s, t, a, b) - \\
& D[2](f)(r, s, t, a, b)^2 + (D[5](f)(r, s, t, a, b)^2 + 4 * D[3](f)(r, s, t, a, b)) * D[1](f)(r, s, t, a, b)), \\
& D[1, 3, 3](f)(r, s, t, a, b) = \\
& (-2 * D[4, 5](f)(r, s, t, a, b)^2 * D[3](f)(r, s, t, a, b)^2 * D[1](f)(r, s, t, a, b) - 2 * D[3](f)(r, s, t, a, b) * D[3, 4](f)(r, s, t, a, b)^2 * \\
& D[1](f)(r, s, t, a, b) + 2 * D[4, 4](f)(r, s, t, a, b) * D[3](f)(r, s, t, a, b) * D[3, 3](f)(r, s, t, a, b) * D[1](f)(r, s, t, a, b) - 2 * D[3, 5](f)(r, s, t, a, b) * \\
& D[3, 4](f)(r, s, t, a, b) * D[2](f)(r, s, t, a, b) * D[1](f)(r, s, t, a, b) + 4 * D[3](f)(r, s, t, a, b) * D[3, 5](f)(r, s, t, a, b) * D[2, 4](f)(r, s, t, a, b) * D[1](f)(r, s, t, a, b) - \\
& 2 * D[5](f)(r, s, t, a, b) * D[3, 3](f)(r, s, t, a, b) * D[2, 4](f)(r, s, t, a, b) * D[1](f)(r, s, t, a, b) + 2 * D[5](f)(r, s, t, a, b) * D[3, 4](f)(r, s, t, a, b) * D[2, 3](f)(r, s, t, a, b) * \\
& D[1](f)(r, s, t, a, b) + \\
& 2 * D[4, 5](f)(r, s, t, a, b) * (D[3, 3](f)(r, s, t, a, b) * D[2](f)(r, s, t, a, b) - 2 * D[3](f)(r, s, t, a, b) * D[2, 3](f)(r, s, t, a, b)) * \\
& D[1](f)(r, s, t, a, b) - 2 * D[3](f)(r, s, t, a, b) * D[3, 4](f)(r, s, t, a, b) * D[2](f)(r, s, t, a, b) * D[1, 5](f)(r, s, t, a, b) - \\
& D[4](f)(r, s, t, a, b) * D[3, 3](f)(r, s, t, a, b) * D[2](f)(r, s, t, a, b) * D[1, 5](f)(r, s, t, a, b) + 2 * D[4](f)(r, s, t, a, b) * \\
& D[3](f)(r, s, t, a, b) * D[2, 3](f)(r, s, t, a, b) * D[1, 5](f)(r, s, t, a, b) - 2 * D[3](f)(r, s, t, a, b) *
\end{aligned}$$

$$\begin{aligned}
& s, t, a, b)^2 * D[1, 5](f)(r, s, t, a, b)^2 + \\
& 2 * D[3](f)(r, s, t, a, b) * D[3, 5](f)(r, s, t, a, b) * D[2](f)(r, s, t, a, b) * D[1, 4](f)(r, s, \\
& t, a, b) - \\
& D[5](f)(r, s, t, a, b) * D[3, 3](f)(r, s, t, a, b) * D[2](f)(r, s, t, a, b) * D[1, 4](f)(r, s, t, \\
& a, b) + 2 * D[4](f)(r, s, t, a, b) * \\
& D[3](f)(r, s, t, a, b) * D[3, 4](f)(r, s, t, a, b) * D[1, 3](f)(r, s, t, a, b) + D[4](f)(r, s, t, \\
& a, b)^2 * \\
& D[3, 3](f)(r, s, t, a, b) * D[1, 3](f)(r, s, t, a, b) - 2 * D[5](f)(r, s, t, a, b) * D[4](f)(r, \\
& s, t, a, b) * D[2, 3](f)(r, s, t, a, b) * D[1, 3](f)(r, s, t, a, b) - \\
& 2 * D[2](f)(r, s, t, a, b) * D[2, 3](f)(r, s, t, a, b) * D[1, 3](f)(r, s, t, a, b) + 2 \\
& * D[5](f)(r, s, t, a, b) * \\
& D[3, 5](f)(r, s, t, a, b) * D[1](f)(r, s, t, a, b) * D[1, 3](f)(r, s, t, a, b) + 4 * D[3, \\
& 3](f)(r, s, t, a, b) * \\
& D[1](f)(r, s, t, a, b) * D[1, 3](f)(r, s, t, a, b) + 2 * D[5](f)(r, s, t, a, b) * D[3](f)(r, s, \\
& t, a, b) * D[1, 5](f)(r, s, t, a, b) * D[1, 3](f)(r, s, t, a, b) + \\
& 2 * D[3](f)(r, s, t, a, b) * D[1, 3](f)(r, s, t, a, b)^2 - 2 * D[4](f)(r, s, t, a, b) \\
& * D[3](f)(r, s, t, a, b) * D[3, 5](f)(r, s, t, a, b) * D[1, 2](f)(r, s, t, a, b) + \\
& D[5](f)(r, s, t, a, b) * D[4](f)(r, s, t, a, b) * D[3, 3](f)(r, s, t, a, b) * D[1, 2](f)(r, s, t, \\
& a, b) - 2 * D[5](f)(r, s, t, a, b) * \\
& D[3](f)(r, s, t, a, b) * D[3, 5](f)(r, s, t, a, b) * D[1, 1](f)(r, s, t, a, b) + D[5](f)(r, s, t, \\
& a, b)^2 * \\
& D[3, 3](f)(r, s, t, a, b) * D[1, 1](f)(r, s, t, a, b) + 2 * D[3](f)(r, s, t, a, b) * D[3, \\
& 3](f)(r, s, t, a, b) * D[1, 1](f)(r, s, t, a, b) + 2 * D[5, 5](f)(r, s, t, a, b) * \\
& D[3](f)(r, s, t, a, b)^2 * (D[4, 4](f)(r, s, t, a, b) * D[1](f)(r, s, t, a, b) + D[1, 1](f)(r, \\
& s, t, a, b))) / \\
& (D[4](f)(r, s, t, a, b)^2 * D[3](f)(r, s, t, a, b) - D[5](f)(r, s, t, a, b) * D[4](f)(r, s, t, a, \\
& b) * D[2](f)(r, s, t, a, b) - \\
& D[2](f)(r, s, t, a, b)^2 + (D[5](f)(r, s, t, a, b)^2 + 4 * D[3](f)(r, s, t, a, b)) \\
& * D[1](f)(r, s, t, a, b)), \\
& D[1, 3, 4](f)(r, s, t, a, b) = \\
& (- (D[4, 5](f)(r, s, t, a, b) * D[3, 4](f)(r, s, t, a, b) * D[2](f)(r, s, t, a, b) * D[1](f)(r, \\
& s, t, a, b)) - 2 * D[4, 5](f)(r, s, t, a, b) * \\
& D[3](f)(r, s, t, a, b) * D[2, 4](f)(r, s, t, a, b) * D[1](f)(r, s, t, a, b) + D[5](f)(r, s, t, a, \\
& b) * D[3, 4](f)(r, s, t, a, b) * D[2, 4](f)(r, s, t, a, b) * \\
& D[1](f)(r, s, t, a, b) - 4 * D[4, 5](f)(r, s, t, a, b) * D[3](f)(r, s, t, a, b) * D[1](f)(r, s, t, \\
& a, b) * D[1, 5](f)(r, s, t, a, b) + \\
& D[5](f)(r, s, t, a, b) * D[3, 4](f)(r, s, t, a, b) * D[1](f)(r, s, t, a, b) * D[1, 5](f)(r, s, t, \\
& a, b) + D[4, 4](f)(r, s, t, a, b) * \\
& (D[3, 5](f)(r, s, t, a, b) * D[2](f)(r, s, t, a, b) * D[1](f)(r, s, t, a, b) - D[5](f)(r, s, t, \\
& a, b) * D[2, 3](f)(r, s, t, a, b) * D[1](f)(r, s, t, a, b) + \\
& D[3](f)(r, s, t, a, b) * (2 * D[2, 5](f)(r, s, t, a, b) * D[1](f)(r, s, t, a, b) - D[2](f)(r, s, \\
& t, a, b) * D[1, 5](f)(r, s, t, a, b))) + \\
& D[4, 5](f)(r, s, t, a, b) * D[3](f)(r, s, t, a, b) * D[2](f)(r, s, t, a, b) * D[1, 4](f)(r, s, t, \\
& a, b) - D[5](f)(r, s, t, a, b) * D[3, 4](f)(r, s, t, a, b) * D[2](f)(r, s, t, a, b) * \\
& D[1, 4](f)(r, s, t, a, b) + 4 * D[5, 5](f)(r, s, t, a, b) * D[3](f)(r, s, t, a, b) * D[1](f)(r, \\
& s, t, a, b) * D[1, 4](f)(r, s, t, a, b) + \\
& 4 * D[3, 3](f)(r, s, t, a, b) * D[1](f)(r, s, t, a, b) * D[1, 4](f)(r, s, t, a, b) - D[5](f)(r, \\
& s, t, a, b) *
\end{aligned}$$

$$\begin{aligned}
& D[3](f)(r, s, t, a, b) * D[1, 5](f)(r, s, t, a, b) * D[1, 4](f)(r, s, t, a, b) + D[4](f)(r, s, t, a, b)^2 * \\
& D[3, 4](f)(r, s, t, a, b) * D[1, 3](f)(r, s, t, a, b) - D[2](f)(r, s, t, a, b) * D[2, 4](f)(r, s, t, a, b) * D[1, 3](f)(r, s, t, a, b) + D[5](f)(r, s, t, a, b) * \\
& D[4, 5](f)(r, s, t, a, b) * D[1](f)(r, s, t, a, b) * D[1, 3](f)(r, s, t, a, b) - D[2](f)(r, s, t, a, b) * D[1, 5](f)(r, s, t, a, b) * D[1, 3](f)(r, s, t, a, b) + \\
& D[5](f)(r, s, t, a, b)^2 * D[1, 4](f)(r, s, t, a, b) * D[1, 3](f)(r, s, t, a, b) + 2 \\
& * D[3](f)(r, s, t, a, b) * \\
& D[1, 4](f)(r, s, t, a, b) * D[1, 3](f)(r, s, t, a, b) - D[3, 4](f)(r, s, t, a, b) * D[2](f)(r, s, t, a, b) * D[1, 2](f)(r, s, t, a, b) - 2 * D[3](f)(r, s, t, a, b) * \\
& D[1, 5](f)(r, s, t, a, b) * D[1, 2](f)(r, s, t, a, b) + D[5](f)(r, s, t, a, b) * D[1, 3](f)(r, s, t, a, b) * D[1, 2](f)(r, s, t, a, b) + D[5](f)(r, s, t, a, b) * \\
& D[4, 5](f)(r, s, t, a, b) * D[3](f)(r, s, t, a, b) * D[1, 1](f)(r, s, t, a, b) + 2 * D[3](f)(r, s, t, a, b) * \\
& D[3, 4](f)(r, s, t, a, b) * D[1, 1](f)(r, s, t, a, b) + D[3, 5](f)(r, s, t, a, b) * D[2](f)(r, s, t, a, b) * D[1, 1](f)(r, s, t, a, b) + 2 * D[3](f)(r, s, t, a, b) * \\
& D[2, 5](f)(r, s, t, a, b) * D[1, 1](f)(r, s, t, a, b) - D[5](f)(r, s, t, a, b) * D[2, 3](f)(r, s, t, a, b) * D[1, 1](f)(r, s, t, a, b) + D[4](f)(r, s, t, a, b) * \\
& (-2 * D[4, 5](f)(r, s, t, a, b)^2 * D[3](f)(r, s, t, a, b) * D[1](f)(r, s, t, a, b) + 2 * D[5, \\
& 5](f)(r, s, t, a, b) * D[4, 4](f)(r, s, t, a, b) * \\
& D[3](f)(r, s, t, a, b) * D[1](f)(r, s, t, a, b) - D[3, 4](f)(r, s, t, a, b)^2 * D[1](f)(r, s, t, a, b) + D[4, 4](f)(r, s, t, a, b) * D[3, 3](f)(r, s, t, a, b) * \\
& D[1](f)(r, s, t, a, b) - D[3, 4](f)(r, s, t, a, b) * D[2](f)(r, s, t, a, b) * D[1, 5](f)(r, s, t, a, b) + D[3](f)(r, s, t, a, b) * D[2, 4](f)(r, s, t, a, b) * \\
& D[1, 5](f)(r, s, t, a, b) + D[3](f)(r, s, t, a, b) * D[3, 4](f)(r, s, t, a, b) * D[1, 4](f)(r, s, t, a, b) + D[4, 4](f)(r, s, t, a, b) * D[3](f)(r, s, t, a, b) * \\
& D[1, 3](f)(r, s, t, a, b) - D[5](f)(r, s, t, a, b) * D[2, 4](f)(r, s, t, a, b) * D[1, 3](f)(r, s, t, a, b) + D[1, 3](f)(r, s, t, a, b)^2 - \\
& D[4, 5](f)(r, s, t, a, b) * D[3](f)(r, s, t, a, b) * D[1, 2](f)(r, s, t, a, b) - D[3, 3](f)(r, s, t, a, b) * D[1, 1](f)(r, s, t, a, b)) / \\
& (D[4](f)(r, s, t, a, b)^2 * D[3](f)(r, s, t, a, b) - D[5](f)(r, s, t, a, b) * D[4](f)(r, s, t, a, b) * D[2](f)(r, s, t, a, b) - \\
& D[2](f)(r, s, t, a, b)^2 + (D[5](f)(r, s, t, a, b)^2 + 4 * D[3](f)(r, s, t, a, b)) \\
& * D[1](f)(r, s, t, a, b)), \\
& D[1, 3, 5](f)(r, s, t, a, b) = \\
& (4 * D[4, 4](f)(r, s, t, a, b) * D[3](f)(r, s, t, a, b) * D[3, 5](f)(r, s, t, a, b) * D[1](f)(r, s, t, a, b) - 4 * D[4, 5](f)(r, s, t, a, b) * \\
& D[3](f)(r, s, t, a, b) * D[3, 4](f)(r, s, t, a, b) * D[1](f)(r, s, t, a, b) - D[4](f)(r, s, t, a, b) * D[3, 5](f)(r, s, t, a, b) * D[3, 4](f)(r, s, t, a, b) * \\
& D[1](f)(r, s, t, a, b) + D[4](f)(r, s, t, a, b) * D[4, 5](f)(r, s, t, a, b) * D[3, 3](f)(r, s, t, a, b) * D[1](f)(r, s, t, a, b) + \\
& D[4, 5](f)(r, s, t, a, b) * D[3, 5](f)(r, s, t, a, b) * D[2](f)(r, s, t, a, b) * D[1](f)(r, s, t, a, b) - \\
& D[5, 5](f)(r, s, t, a, b) * D[3, 4](f)(r, s, t, a, b) * D[2](f)(r, s, t, a, b) * D[1](f)(r, s, t, a, b) - 2 * D[4, 5](f)(r, s, t, a, b) * \\
& D[3](f)(r, s, t, a, b) * D[2, 5](f)(r, s, t, a, b) * D[1](f)(r, s, t, a, b) + 2 * D[5, 5](f)(r, s, t, a, b) * \\
& D[3](f)(r, s, t, a, b) * D[2, 4](f)(r, s, t, a, b) * D[1](f)(r, s, t, a, b) + 2 * D[3, 3](f)(r, s, t, a, b) *
\end{aligned}$$



$$\begin{aligned}
& s, t, a, b) * \\
& D[2, 4](f)(r, s, t, a, b) * D[1](f)(r, s, t, a, b) - 2 * D[3, 4](f)(r, s, t, a, b) * D[2, \\
& 3](f)(r, s, t, a, b) * D[1](f)(r, s, t, a, b) + D[4](f)(r, s, t, a, b) * \\
& D[3](f)(r, s, t, a, b) * D[3, 4](f)(r, s, t, a, b) * D[1, 5](f)(r, s, t, a, b) - D[4, 5](f)(r, s, \\
& t, a, b) * D[3](f)(r, s, t, a, b) * D[2](f)(r, s, t, a, b) * \\
& D[1, 5](f)(r, s, t, a, b) - D[4](f)(r, s, t, a, b) * D[3, 5](f)(r, s, t, a, b) * D[2](f)(r, s, t, \\
& a, b) * \\
& D[1, 5](f)(r, s, t, a, b) + D[4](f)(r, s, t, a, b) * D[3](f)(r, s, t, a, b) * D[2, 5](f)(r, s, t, \\
& a, b) * D[1, 5](f)(r, s, t, a, b) - \\
& D[2](f)(r, s, t, a, b) * D[2, 3](f)(r, s, t, a, b) * D[1, 5](f)(r, s, t, a, b) + 2 * D[3, \\
& 3](f)(r, s, t, a, b) * \\
& D[1](f)(r, s, t, a, b) * D[1, 5](f)(r, s, t, a, b) + D[5, 5](f)(r, s, t, a, b) * D[3](f)(r, s, t, \\
& a, b) * D[2](f)(r, s, t, a, b) * D[1, 4](f)(r, s, t, a, b) + \\
& D[3, 3](f)(r, s, t, a, b) * D[2](f)(r, s, t, a, b) * D[1, 4](f)(r, s, t, a, b) + D[4](f)(r, s, t, \\
& a, b) * D[4, 5](f)(r, s, t, a, b) * D[3](f)(r, s, t, a, b) * \\
& D[1, 3](f)(r, s, t, a, b) + D[4](f)(r, s, t, a, b)^2 * D[3, 5](f)(r, s, t, a, b) * D[1, \\
& 3](f)(r, s, t, a, b) - D[3, 4](f)(r, s, t, a, b) * \\
& D[2](f)(r, s, t, a, b) * D[1, 3](f)(r, s, t, a, b) - D[2](f)(r, s, t, a, b) * D[2, 5](f)(r, s, t, \\
& a, b) * D[1, 3](f)(r, s, t, a, b) + D[4](f)(r, s, t, a, b) * \\
& D[2, 3](f)(r, s, t, a, b) * D[1, 3](f)(r, s, t, a, b) + 2 * D[3, 5](f)(r, s, t, a, b) \\
& * D[1](f)(r, s, t, a, b) * D[1, 3](f)(r, s, t, a, b) + D[5](f)(r, s, t, a, b)^2 * \\
& D[1, 5](f)(r, s, t, a, b) * D[1, 3](f)(r, s, t, a, b) - D[5, 5](f)(r, s, t, a, b) * D[4](f)(r, s, \\
& t, a, b) * D[3](f)(r, s, t, a, b) * D[1, 2](f)(r, s, t, a, b) - \\
& D[4](f)(r, s, t, a, b) * D[3, 3](f)(r, s, t, a, b) * D[1, 2](f)(r, s, t, a, b) + 4 * D[3](f)(r, \\
& s, t, a, b) * \\
& D[3, 5](f)(r, s, t, a, b) * D[1, 1](f)(r, s, t, a, b) + D[5](f)(r, s, t, a, b) * (-2 * D[4, \\
& 5](f)(r, s, t, a, b)^2 * D[3](f)(r, s, t, a, b) * D[1](f)(r, s, t, a, b) + \\
& D[3, 4](f)(r, s, t, a, b) * D[2, 5](f)(r, s, t, a, b) * D[1](f)(r, s, t, a, b) - D[4, 5](f)(r, s, \\
& t, a, b) * D[2, 3](f)(r, s, t, a, b) * D[1](f)(r, s, t, a, b) - \\
& D[3, 4](f)(r, s, t, a, b) * D[2](f)(r, s, t, a, b) * D[1, 5](f)(r, s, t, a, b) + D[3, 5](f)(r, \\
& s, t, a, b) * D[1](f)(r, s, t, a, b) * D[1, 5](f)(r, s, t, a, b) - \\
& D[3](f)(r, s, t, a, b) * D[1, 5](f)(r, s, t, a, b)^2 - D[4](f)(r, s, t, a, b) * D[2, 5](f)(r, s, \\
& t, a, b) * D[1, 3](f)(r, s, t, a, b) + \\
& D[1, 3](f)(r, s, t, a, b)^2 - D[3, 3](f)(r, s, t, a, b) * D[1, 1](f)(r, s, t, a, b) + D[5, \\
& 5](f)(r, s, t, a, b) * (2 * D[4, 4](f)(r, s, t, a, b) * \\
& D[3](f)(r, s, t, a, b) * D[1](f)(r, s, t, a, b) + D[1](f)(r, s, t, a, b) * D[1, 3](f)(r, s, t, a, \\
& b) + D[3](f)(r, s, t, a, b) * D[1, 1](f)(r, s, t, a, b))) / \\
& (D[4](f)(r, s, t, a, b)^2 * D[3](f)(r, s, t, a, b) - D[5](f)(r, s, t, a, b) * D[4](f)(r, s, t, a, \\
& b) * D[2](f)(r, s, t, a, b) - \\
& D[2](f)(r, s, t, a, b)^2 + (D[5](f)(r, s, t, a, b)^2 + 4 * D[3](f)(r, s, t, a, b)) \\
& * D[1](f)(r, s, t, a, b)), \\
& D[1, 4, 4](f)(r, s, t, a, b) = \\
& (-2 * D[2, 4](f)(r, s, t, a, b)^2 * D[1](f)(r, s, t, a, b) + 2 * D[4, 4](f)(r, s, t, a, b) \\
& * D[2, 2](f)(r, s, t, a, b) * D[1](f)(r, s, t, a, b) - 2 * D[4, 5](f)(r, s, t, a, b)^2 * \\
& D[1](f)(r, s, t, a, b)^2 + 2 * D[5, 5](f)(r, s, t, a, b) * D[4, 4](f)(r, s, t, a, b) \\
& * D[1](f)(r, s, t, a, b)^2 - 2 * D[5](f)(r, s, t, a, b) * \\
& D[4, 4](f)(r, s, t, a, b) * D[1](f)(r, s, t, a, b) * D[1, 5](f)(r, s, t, a, b) - 2 * D[1](f)(r, \\
& s, t, a, b) * D[1, 5](f)(r, s, t, a, b)^2 -
\end{aligned}$$

$$\begin{aligned}
& D[5](f)(r, s, t, a, b) * D[4, 4](f)(r, s, t, a, b) * D[2](f)(r, s, t, a, b) * D[1, 4](f)(r, s, t, a, b) + 4 * D[5](f)(r, s, t, a, b) * \\
& D[4, 5](f)(r, s, t, a, b) * D[1](f)(r, s, t, a, b) * D[1, 4](f)(r, s, t, a, b) + 4 * D[3, \\
& 4](f)(r, s, t, a, b) * D[1](f)(r, s, t, a, b) * D[1, 4](f)(r, s, t, a, b) + 8 * D[2, 5](f)(r, s, \\
& t, a, b) * \\
& D[1](f)(r, s, t, a, b) * D[1, 4](f)(r, s, t, a, b) - 2 * D[2](f)(r, s, t, a, b) * D[1, 5](f)(r, \\
& s, t, a, b) * D[1, 4](f)(r, s, t, a, b) + 2 * D[3](f)(r, s, t, a, b) * \\
& D[1, 4](f)(r, s, t, a, b)^2 + D[4](f)(r, s, t, a, b)^2 * (-2 * D[4, 5](f)(r, s, t, a, b)^2 \\
& * D[1](f)(r, s, t, a, b) + D[4, 4](f)(r, s, t, a, b) * \\
& (2 * D[5, 5](f)(r, s, t, a, b) * D[1](f)(r, s, t, a, b) + D[1, 3](f)(r, s, t, a, b))) - 2 * D[4, \\
& 4](f)(r, s, t, a, b) * \\
& D[2](f)(r, s, t, a, b) * D[1, 2](f)(r, s, t, a, b) - 4 * D[4, 5](f)(r, s, t, a, b) * D[1](f)(r, \\
& s, t, a, b) * D[1, 2](f)(r, s, t, a, b) - 2 * D[5](f)(r, s, t, a, b) * \\
& D[1, 4](f)(r, s, t, a, b) * D[1, 2](f)(r, s, t, a, b) - 2 * D[1, 2](f)(r, s, t, a, b)^2 \\
& + D[5](f)(r, s, t, a, b)^2 * \\
& D[4, 4](f)(r, s, t, a, b) * D[1, 1](f)(r, s, t, a, b) + 2 * D[4, 4](f)(r, s, t, a, b) \\
& * D[3](f)(r, s, t, a, b) * D[1, 1](f)(r, s, t, a, b) + 2 * D[4, 5](f)(r, s, t, a, b) * \\
& D[2](f)(r, s, t, a, b) * D[1, 1](f)(r, s, t, a, b) + 2 * D[2, 2](f)(r, s, t, a, b) * D[1, \\
& 1](f)(r, s, t, a, b) + 2 * D[5, 5](f)(r, s, t, a, b) * \\
& D[1](f)(r, s, t, a, b) * D[1, 1](f)(r, s, t, a, b) + D[2, 4](f)(r, s, t, a, b) * (-4 \\
& * D[1](f)(r, s, t, a, b) * D[1, 5](f)(r, s, t, a, b) + \\
& 2 * D[5](f)(r, s, t, a, b) * D[1, 1](f)(r, s, t, a, b)) + D[4](f)(r, s, t, a, b) * (-4 * D[4, \\
& 5](f)(r, s, t, a, b) * D[1](f)(r, s, t, a, b) * \\
& (D[2, 4](f)(r, s, t, a, b) + D[1, 5](f)(r, s, t, a, b)) + 4 * D[5, 5](f)(r, s, t, a, b) \\
& * D[1](f)(r, s, t, a, b) * D[1, 4](f)(r, s, t, a, b) + \\
& 2 * D[1, 4](f)(r, s, t, a, b) * D[1, 3](f)(r, s, t, a, b) + D[4, 4](f)(r, s, t, a, b) * (4 * D[2, \\
& 5](f)(r, s, t, a, b) * D[1](f)(r, s, t, a, b) - \\
& D[2](f)(r, s, t, a, b) * D[1, 5](f)(r, s, t, a, b) + 2 * D[3](f)(r, s, t, a, b) * D[1, 4](f)(r, \\
& s, t, a, b) - D[5](f)(r, s, t, a, b) * \\
& D[1, 2](f)(r, s, t, a, b)) - 2 * D[3, 4](f)(r, s, t, a, b) * D[1, 1](f)(r, s, t, a, b))) / \\
& (D[4](f)(r, s, t, a, b)^2 * D[3](f)(r, s, t, a, b) - D[5](f)(r, s, t, a, b) * D[4](f)(r, s, t, a, \\
& b) * D[2](f)(r, s, t, a, b) - \\
& D[2](f)(r, s, t, a, b)^2 + (D[5](f)(r, s, t, a, b)^2 + 4 * D[3](f)(r, s, t, a, b)) \\
& * D[1](f)(r, s, t, a, b)), \\
& D[1, 4, 5](f)(r, s, t, a, b) = \\
& (- (D[4, 5](f)(r, s, t, a, b)^2 * D[2](f)(r, s, t, a, b) * D[1](f)(r, s, t, a, b)) + D[5, \\
& 5](f)(r, s, t, a, b) * D[4, 4](f)(r, s, t, a, b) * D[2](f)(r, s, t, a, b) * \\
& D[1](f)(r, s, t, a, b) - 2 * D[3, 4](f)(r, s, t, a, b) * D[2, 4](f)(r, s, t, a, b) * D[1](f)(r, \\
& s, t, a, b) + 2 * D[4, 4](f)(r, s, t, a, b) * \\
& D[2, 3](f)(r, s, t, a, b) * D[1](f)(r, s, t, a, b) - D[2](f)(r, s, t, a, b) * D[2, 4](f)(r, s, t, \\
& a, b) * D[1, 5](f)(r, s, t, a, b) - 2 * D[3, 4](f)(r, s, t, a, b) * \\
& D[1](f)(r, s, t, a, b) * D[1, 5](f)(r, s, t, a, b) - D[2](f)(r, s, t, a, b) * D[1, 5](f)(r, s, t, \\
& a, b)^2 + \\
& D[3, 4](f)(r, s, t, a, b) * D[2](f)(r, s, t, a, b) * D[1, 4](f)(r, s, t, a, b) + 8 * D[3, \\
& 5](f)(r, s, t, a, b) * \\
& D[1](f)(r, s, t, a, b) * D[1, 4](f)(r, s, t, a, b) + 2 * D[3](f)(r, s, t, a, b) * D[1, 5](f)(r, \\
& s, t, a, b) * D[1, 4](f)(r, s, t, a, b) + D[4](f)(r, s, t, a, b)^2 * \\
& D[4, 5](f)(r, s, t, a, b) * D[1, 3](f)(r, s, t, a, b) - D[4, 4](f)(r, s, t, a, b) * D[2](f)(r, s, \\
& t, a, b) * D[1, 3](f)(r, s, t, a, b) - 2 * D[4, 5](f)(r, s, t, a, b) *
\end{aligned}$$

$$\begin{aligned}
& D[1](f)(r, s, t, a, b) * D[1, 3](f)(r, s, t, a, b) - D[4, 5](f)(r, s, t, a, b) * D[2](f)(r, s, t, a, b) * D[1, 2](f)(r, s, t, a, b) - 2 * D[1, 3](f)(r, s, t, a, b) * \\
& D[1, 2](f)(r, s, t, a, b) + D[5](f)(r, s, t, a, b)^2 * D[4, 5](f)(r, s, t, a, b) * D[1, 1](f)(r, s, t, a, b) + 2 * D[4, 5](f)(r, s, t, a, b) * \\
& D[3](f)(r, s, t, a, b) * D[1, 1](f)(r, s, t, a, b) + D[5, 5](f)(r, s, t, a, b) * D[2](f)(r, s, t, a, b) * D[1, 1](f)(r, s, t, a, b) + 2 * D[2, 3](f)(r, s, t, a, b) * \\
& D[1, 1](f)(r, s, t, a, b) + D[4](f)(r, s, t, a, b) * (D[4, 4](f)(r, s, t, a, b) * (3 * D[3, 5](f)(r, s, t, a, b) * D[1](f)(r, s, t, a, b) + \\
& D[3](f)(r, s, t, a, b) * D[1, 5](f)(r, s, t, a, b)) + D[4, 5](f)(r, s, t, a, b) * (-3 * D[3, 4](f)(r, s, t, a, b) * D[1](f)(r, s, t, a, b) - \\
& D[2](f)(r, s, t, a, b) * D[1, 5](f)(r, s, t, a, b) + D[3](f)(r, s, t, a, b) * D[1, 4](f)(r, s, t, a, b)) + D[2, 4](f)(r, s, t, a, b) * D[1, 3](f)(r, s, t, a, b) + \\
& D[1, 5](f)(r, s, t, a, b) * D[1, 3](f)(r, s, t, a, b) - D[3, 4](f)(r, s, t, a, b) * D[1, 2](f)(r, s, t, a, b) - D[3, 5](f)(r, s, t, a, b) * D[1, 1](f)(r, s, t, a, b)) - \\
& D[5](f)(r, s, t, a, b) * (D[4, 5](f)(r, s, t, a, b) * D[2, 4](f)(r, s, t, a, b) * D[1](f)(r, s, t, a, b) + 2 * D[4, 5](f)(r, s, t, a, b) * D[1](f)(r, s, t, a, b) * \\
& D[1, 5](f)(r, s, t, a, b) + D[4, 4](f)(r, s, t, a, b) * (- (D[2, 5](f)(r, s, t, a, b) * D[1](f)(r, s, t, a, b)) + D[2](f)(r, s, t, a, b) * \\
& D[1, 5](f)(r, s, t, a, b)) - 4 * D[5, 5](f)(r, s, t, a, b) * D[1](f)(r, s, t, a, b) * D[1, 4](f)(r, s, t, a, b) + D[1, 4](f)(r, s, t, a, b) * \\
& D[1, 3](f)(r, s, t, a, b) + D[1, 5](f)(r, s, t, a, b) * D[1, 2](f)(r, s, t, a, b) + D[4](f)(r, s, t, a, b) * (2 * D[4, 5](f)(r, s, t, a, b)^2 * \\
& D[1](f)(r, s, t, a, b) - 2 * D[5, 5](f)(r, s, t, a, b) * D[4, 4](f)(r, s, t, a, b) * D[1](f)(r, s, t, a, b) + D[4, 5](f)(r, s, t, a, b) * \\
& D[1, 2](f)(r, s, t, a, b)) - D[3, 4](f)(r, s, t, a, b) * D[1, 1](f)(r, s, t, a, b) - D[2, 5](f)(r, s, t, a, b) * D[1, 1](f)(r, s, t, a, b)) / \\
& (D[4](f)(r, s, t, a, b)^2 * D[3](f)(r, s, t, a, b) - D[5](f)(r, s, t, a, b) * D[4](f)(r, s, t, a, b) * D[2](f)(r, s, t, a, b) - \\
& D[2](f)(r, s, t, a, b)^2 + (D[5](f)(r, s, t, a, b)^2 + 4 * D[3](f)(r, s, t, a, b)) * D[1](f)(r, s, t, a, b)), \\
& D[1, 5, 5](f)(r, s, t, a, b) = \\
& (-2 * D[4, 5](f)(r, s, t, a, b)^2 * D[3](f)(r, s, t, a, b) * D[1](f)(r, s, t, a, b) + 2 * D[5, 5](f)(r, s, t, a, b) * \\
& D[4, 4](f)(r, s, t, a, b) * D[3](f)(r, s, t, a, b) * D[1](f)(r, s, t, a, b) - 2 * D[5, 5](f)(r, s, t, a, b) * \\
& D[4](f)(r, s, t, a, b) * D[3, 4](f)(r, s, t, a, b) * D[1](f)(r, s, t, a, b) - 2 * D[3, 4](f)(r, s, t, a, b) * D[1](f)(r, s, t, a, b)^2 * D[1](f)(r, s, t, a, b) + \\
& 2 * D[4, 4](f)(r, s, t, a, b) * D[3, 3](f)(r, s, t, a, b) * D[1](f)(r, s, t, a, b) - 4 * D[3, 4](f)(r, s, t, a, b) * \\
& D[2, 5](f)(r, s, t, a, b) * D[1](f)(r, s, t, a, b) + 4 * D[3, 5](f)(r, s, t, a, b) * D[2, 4](f)(r, s, t, a, b) * D[1](f)(r, s, t, a, b) - D[5, 5](f)(r, s, t, a, b) * \\
& D[4](f)(r, s, t, a, b) * D[2](f)(r, s, t, a, b) * D[1, 5](f)(r, s, t, a, b) - 2 * D[2](f)(r, s, t, a, b) * \\
& D[2, 5](f)(r, s, t, a, b) * D[1, 5](f)(r, s, t, a, b) + 4 * D[3, 5](f)(r, s, t, a, b) * D[1](f)(r, s, t, a, b) * D[1, 5](f)(r, s, t, a, b) + 2 * D[3](f)(r, s, t, a, b) * \\
& D[1, 5](f)(r, s, t, a, b)^2 + 2 * D[3, 5](f)(r, s, t, a, b) * D[2](f)(r, s, t, a, b) * D[1, 4](f)(r, s, t, a, b) + D[5, 5](f)(r, s, t, a, b) * \\
& D[4](f)(r, s, t, a, b)^2 * D[1, 3](f)(r, s, t, a, b) + 2 * D[4](f)(r, s, t, a, b) * D[2,
\end{aligned}$$

$$\begin{aligned}
& 5](f)(r, s, t, a, b) * D[1, 3](f)(r, s, t, a, b) - 2 * D[1, 3](f)(r, s, t, a, b)^2 + \\
& 2 * D[4, 5](f)(r, s, t, a, b) * (D[4](f)(r, s, t, a, b) * (D[3, 5](f)(r, s, t, a, b) \\
& * D[1](f)(r, s, t, a, b) + D[3](f)(r, s, t, a, b) * D[1, 5](f)(r, s, t, a, b)) - \\
& D[2](f)(r, s, t, a, b) * D[1, 3](f)(r, s, t, a, b)) - 2 * D[4](f)(r, s, t, a, b) * D[3, 5](f)(r, \\
& s, t, a, b) * D[1, 2](f)(r, s, t, a, b) + 2 * D[5, 5](f)(r, s, t, a, b) * \\
& D[3](f)(r, s, t, a, b) * D[1, 1](f)(r, s, t, a, b) + 2 * D[3, 3](f)(r, s, t, a, b) * D[1, \\
& 1](f)(r, s, t, a, b) + D[5](f)(r, s, t, a, b) * \\
& (4 * D[4, 4](f)(r, s, t, a, b) * D[3, 5](f)(r, s, t, a, b) * D[1](f)(r, s, t, a, b) + 2 * D[5, \\
& 5](f)(r, s, t, a, b) * D[2, 4](f)(r, s, t, a, b) * D[1](f)(r, s, t, a, b) + \\
& 2 * D[5, 5](f)(r, s, t, a, b) * D[1](f)(r, s, t, a, b) * D[1, 5](f)(r, s, t, a, b) - 2 * D[4, \\
& 5](f)(r, s, t, a, b) * (2 * D[3, 4](f)(r, s, t, a, b) * D[1](f)(r, s, t, a, b) + \\
& D[2, 5](f)(r, s, t, a, b) * D[1](f)(r, s, t, a, b) + D[2](f)(r, s, t, a, b) * D[1, 5](f)(r, s, t, \\
& a, b)) + D[5, 5](f)(r, s, t, a, b) * D[2](f)(r, s, t, a, b) * \\
& D[1, 4](f)(r, s, t, a, b) - 2 * D[1, 5](f)(r, s, t, a, b) * D[1, 3](f)(r, s, t, a, b) - D[5, \\
& 5](f)(r, s, t, a, b) * D[4](f)(r, s, t, a, b) * D[1, 2](f)(r, s, t, a, b) + \\
& 2 * D[3, 5](f)(r, s, t, a, b) * D[1, 1](f)(r, s, t, a, b)) + D[5](f)(r, s, t, a, b)^2 * (-2 \\
& * D[4, 5](f)(r, s, t, a, b)^2 * D[1](f)(r, s, t, a, b) + \\
& D[5, 5](f)(r, s, t, a, b) * (2 * D[4, 4](f)(r, s, t, a, b) * D[1](f)(r, s, t, a, b) + D[1, \\
& 1](f)(r, s, t, a, b)))) / \\
& (D[4](f)(r, s, t, a, b)^2 * D[3](f)(r, s, t, a, b) - D[5](f)(r, s, t, a, b) * D[4](f)(r, s, t, a, \\
& b) * D[2](f)(r, s, t, a, b) - \\
& D[2](f)(r, s, t, a, b)^2 + (D[5](f)(r, s, t, a, b)^2 + 4 * D[3](f)(r, s, t, a, b)) \\
& * D[1](f)(r, s, t, a, b)), \\
& D[2, 2, 2](f)(r, s, t, a, b) = \\
& (-2 * D[4, 5](f)(r, s, t, a, b)^2 * D[2](f)(r, s, t, a, b)^3 - 4 * D[3, 4](f)(r, s, t, a, b) \\
& * D[2](f)(r, s, t, a, b)^2 * D[2, 4](f)(r, s, t, a, b) + \\
& 2 * D[2](f)(r, s, t, a, b)^2 * D[2, 5](f)(r, s, t, a, b) * D[2, 4](f)(r, s, t, a, b) + 2 \\
& * D[3](f)(r, s, t, a, b) * D[2](f)(r, s, t, a, b) * D[2, 4](f)(r, s, t, a, b)^2 + \\
& 4 * D[4, 4](f)(r, s, t, a, b) * D[2](f)(r, s, t, a, b)^2 * D[2, 3](f)(r, s, t, a, b) - 2 \\
& * D[4](f)(r, s, t, a, b) * \\
& D[2](f)(r, s, t, a, b) * D[2, 4](f)(r, s, t, a, b) * D[2, 3](f)(r, s, t, a, b) - 2 * D[4, \\
& 4](f)(r, s, t, a, b) * \\
& D[3](f)(r, s, t, a, b) * D[2](f)(r, s, t, a, b) * D[2, 2](f)(r, s, t, a, b) + 2 * D[4](f)(r, s, \\
& t, a, b) * \\
& D[3, 4](f)(r, s, t, a, b) * D[2](f)(r, s, t, a, b) * D[2, 2](f)(r, s, t, a, b) - D[4](f)(r, s, t, \\
& a, b) * D[2](f)(r, s, t, a, b) * D[2, 5](f)(r, s, t, a, b) * \\
& D[2, 2](f)(r, s, t, a, b) + 2 * D[4](f)(r, s, t, a, b) * D[3](f)(r, s, t, a, b) * D[2, 4](f)(r, \\
& s, t, a, b) * D[2, 2](f)(r, s, t, a, b) - \\
& D[5](f)(r, s, t, a, b) * D[2](f)(r, s, t, a, b) * D[2, 4](f)(r, s, t, a, b) * D[2, 2](f)(r, s, t, \\
& a, b) + \\
& D[4](f)(r, s, t, a, b)^2 * D[2, 3](f)(r, s, t, a, b) * D[2, 2](f)(r, s, t, a, b) - D[5](f)(r, s, \\
& t, a, b) * D[4](f)(r, s, t, a, b) * D[2, 2](f)(r, s, t, a, b)^2 - \\
& 2 * D[2](f)(r, s, t, a, b) * D[2, 2](f)(r, s, t, a, b)^2 - 4 * D[3, 4](f)(r, s, t, a, b)^2 \\
& * D[2](f)(r, s, t, a, b) * D[1](f)(r, s, t, a, b) + 4 * D[4, 4](f)(r, s, t, a, b) * \\
& D[3, 3](f)(r, s, t, a, b) * D[2](f)(r, s, t, a, b) * D[1](f)(r, s, t, a, b) - 8 * D[3, 4](f)(r, \\
& s, t, a, b) * \\
& D[2](f)(r, s, t, a, b) * D[2, 5](f)(r, s, t, a, b) * D[1](f)(r, s, t, a, b) + 2 * D[2](f)(r, s, \\
& t, a, b) * D[2, 5](f)(r, s, t, a, b)^2 *
\end{aligned}$$

$$\begin{aligned}
& D[1](f)(r, s, t, a, b) + 4 * D[3](f)(r, s, t, a, b) * D[3, 4](f)(r, s, t, a, b) * D[2, 4](f)(r, \\
& \quad s, t, a, b) * D[1](f)(r, s, t, a, b) - 4 * D[4](f)(r, s, t, a, b) * \\
& D[3, 3](f)(r, s, t, a, b) * D[2, 4](f)(r, s, t, a, b) * D[1](f)(r, s, t, a, b) + 4 * D[3, \\
& \quad 5](f)(r, s, t, a, b) * \\
& D[2](f)(r, s, t, a, b) * D[2, 4](f)(r, s, t, a, b) * D[1](f)(r, s, t, a, b) + 4 * D[3](f)(r, s, \\
& \quad t, a, b) * \\
& D[2, 5](f)(r, s, t, a, b) * D[2, 4](f)(r, s, t, a, b) * D[1](f)(r, s, t, a, b) - 4 * D[4, \\
& \quad 4](f)(r, s, t, a, b) * \\
& D[3](f)(r, s, t, a, b) * D[2, 3](f)(r, s, t, a, b) * D[1](f)(r, s, t, a, b) + 4 * D[4](f)(r, s, \\
& \quad t, a, b) * \\
& D[3, 4](f)(r, s, t, a, b) * D[2, 3](f)(r, s, t, a, b) * D[1](f)(r, s, t, a, b) - 2 * D[4](f)(r, \\
& \quad s, t, a, b) * D[2, 5](f)(r, s, t, a, b) * D[2, 3](f)(r, s, t, a, b) * D[1](f)(r, s, t, a, b) - \\
& 2 * D[5](f)(r, s, t, a, b) * D[2, 4](f)(r, s, t, a, b) * D[2, 3](f)(r, s, t, a, b) * D[1](f)(r, s, \\
& \quad t, a, b) + \\
& 2 * D[4](f)(r, s, t, a, b) * D[3, 5](f)(r, s, t, a, b) * D[2, 2](f)(r, s, t, a, b) * D[1](f)(r, s, \\
& \quad t, a, b) + \\
& 2 * D[5](f)(r, s, t, a, b) * D[3, 4](f)(r, s, t, a, b) * D[2, 2](f)(r, s, t, a, b) * D[1](f)(r, s, \\
& \quad t, a, b) + \\
& 2 * D[5](f)(r, s, t, a, b) * D[2, 5](f)(r, s, t, a, b) * D[2, 2](f)(r, s, t, a, b) * D[1](f)(r, s, \\
& \quad t, a, b) + \\
& 4 * D[2, 3](f)(r, s, t, a, b) * D[2, 2](f)(r, s, t, a, b) * D[1](f)(r, s, t, a, b) - 4 * D[3, \\
& \quad 5](f)(r, s, t, a, b) * \\
& D[3, 4](f)(r, s, t, a, b) * D[1](f)(r, s, t, a, b)^2 - 4 * D[3, 5](f)(r, s, t, a, b) * D[2, \\
& \quad 5](f)(r, s, t, a, b) * D[1](f)(r, s, t, a, b)^2 - \\
& 4 * D[3, 4](f)(r, s, t, a, b) * D[2](f)(r, s, t, a, b)^2 * D[1, 5](f)(r, s, t, a, b) - 4 \\
& \quad * D[2](f)(r, s, t, a, b)^2 * \\
& D[2, 5](f)(r, s, t, a, b) * D[1, 5](f)(r, s, t, a, b) - 8 * D[3](f)(r, s, t, a, b) * D[2](f)(r, \\
& \quad s, t, a, b) * D[2, 4](f)(r, s, t, a, b) * D[1, 5](f)(r, s, t, a, b) + \\
& 4 * D[4](f)(r, s, t, a, b) * D[2](f)(r, s, t, a, b) * D[2, 3](f)(r, s, t, a, b) * D[1, 5](f)(r, s, \\
& \quad t, a, b) + \\
& 2 * D[4](f)(r, s, t, a, b) * D[3](f)(r, s, t, a, b) * D[2, 2](f)(r, s, t, a, b) * D[1, 5](f)(r, s, \\
& \quad t, a, b) + \\
& 2 * D[5](f)(r, s, t, a, b) * D[2](f)(r, s, t, a, b) * D[2, 2](f)(r, s, t, a, b) * D[1, 5](f)(r, s, \\
& \quad t, a, b) + \\
& 4 * D[3](f)(r, s, t, a, b) * D[3, 4](f)(r, s, t, a, b) * D[1](f)(r, s, t, a, b) * D[1, 5](f)(r, s, \\
& \quad t, a, b) - \\
& 4 * D[4](f)(r, s, t, a, b) * D[3, 3](f)(r, s, t, a, b) * D[1](f)(r, s, t, a, b) * D[1, 5](f)(r, s, \\
& \quad t, a, b) + \\
& 4 * D[3, 5](f)(r, s, t, a, b) * D[2](f)(r, s, t, a, b) * D[1](f)(r, s, t, a, b) * D[1, 5](f)(r, s, \\
& \quad t, a, b) + \\
& 4 * D[3](f)(r, s, t, a, b) * D[2, 5](f)(r, s, t, a, b) * D[1](f)(r, s, t, a, b) * D[1, 5](f)(r, s, \\
& \quad t, a, b) - \\
& 8 * D[5](f)(r, s, t, a, b) * D[2, 3](f)(r, s, t, a, b) * D[1](f)(r, s, t, a, b) * D[1, 5](f)(r, s, \\
& \quad t, a, b) - \\
& 4 * D[3](f)(r, s, t, a, b) * D[2](f)(r, s, t, a, b) * D[1, 5](f)(r, s, t, a, b)^2 + 4 \\
& \quad * D[3](f)(r, s, t, a, b) * \\
& D[3, 4](f)(r, s, t, a, b) * D[2](f)(r, s, t, a, b) * D[1, 4](f)(r, s, t, a, b) - 4 * D[4](f)(r, \\
& \quad s, t, a, b) *
\end{aligned}$$

$$\begin{aligned}
& D[3, 3](f)(r, s, t, a, b) * D[2](f)(r, s, t, a, b) * D[1, 4](f)(r, s, t, a, b) + 8 * D[3, \\
& 5](f)(r, s, t, a, b) * D[2](f)(r, s, t, a, b)^2 * D[1, 4](f)(r, s, t, a, b) + \\
& 4 * D[3](f)(r, s, t, a, b) * D[2](f)(r, s, t, a, b) * D[2, 5](f)(r, s, t, a, b) * D[1, 4](f)(r, s, \\
& t, a, b) - \\
& 4 * D[3](f)(r, s, t, a, b)^2 * D[2, 4](f)(r, s, t, a, b) * D[1, 4](f)(r, s, t, a, b) + 4 \\
& * D[4](f)(r, s, t, a, b) * \\
& D[3](f)(r, s, t, a, b) * D[2, 3](f)(r, s, t, a, b) * D[1, 4](f)(r, s, t, a, b) - 8 * D[5](f)(r, \\
& s, t, a, b) * \\
& D[2](f)(r, s, t, a, b) * D[2, 3](f)(r, s, t, a, b) * D[1, 4](f)(r, s, t, a, b) + 2 * D[5](f)(r, \\
& s, t, a, b) * \\
& D[3](f)(r, s, t, a, b) * D[2, 2](f)(r, s, t, a, b) * D[1, 4](f)(r, s, t, a, b) + 4 * D[3](f)(r, \\
& s, t, a, b) * \\
& D[3, 5](f)(r, s, t, a, b) * D[1](f)(r, s, t, a, b) * D[1, 4](f)(r, s, t, a, b) - 4 * D[5](f)(r, \\
& s, t, a, b) * \\
& D[3, 3](f)(r, s, t, a, b) * D[1](f)(r, s, t, a, b) * D[1, 4](f)(r, s, t, a, b) - 4 * D[3](f)(r, \\
& s, t, a, b)^2 * \\
& D[1, 5](f)(r, s, t, a, b) * D[1, 4](f)(r, s, t, a, b) - 4 * D[4, 4](f)(r, s, t, a, b) \\
& * D[3](f)(r, s, t, a, b) * D[2](f)(r, s, t, a, b) * D[1, 3](f)(r, s, t, a, b) + \\
& 4 * D[4](f)(r, s, t, a, b) * D[3, 4](f)(r, s, t, a, b) * D[2](f)(r, s, t, a, b) * D[1, 3](f)(r, s, \\
& t, a, b) + \\
& 4 * D[4](f)(r, s, t, a, b) * D[2](f)(r, s, t, a, b) * D[2, 5](f)(r, s, t, a, b) * D[1, 3](f)(r, s, \\
& t, a, b) + \\
& 4 * D[4](f)(r, s, t, a, b) * D[3](f)(r, s, t, a, b) * D[2, 4](f)(r, s, t, a, b) * D[1, 3](f)(r, s, \\
& t, a, b) + \\
& 4 * D[5](f)(r, s, t, a, b) * D[2](f)(r, s, t, a, b) * D[2, 4](f)(r, s, t, a, b) * D[1, 3](f)(r, s, \\
& t, a, b) - \\
& 4 * D[4](f)(r, s, t, a, b)^2 * D[2, 3](f)(r, s, t, a, b) * D[1, 3](f)(r, s, t, a, b) - 4 \\
& * D[5](f)(r, s, t, a, b) * D[4](f)(r, s, t, a, b) * D[2, 2](f)(r, s, t, a, b) * D[1, 3](f)(r, \\
& s, t, a, b) - \\
& 2 * D[2](f)(r, s, t, a, b) * D[2, 2](f)(r, s, t, a, b) * D[1, 3](f)(r, s, t, a, b) + 4 \\
& * D[4](f)(r, s, t, a, b) * \\
& D[3, 5](f)(r, s, t, a, b) * D[1](f)(r, s, t, a, b) * D[1, 3](f)(r, s, t, a, b) + 4 * D[5](f)(r, \\
& s, t, a, b) * \\
& D[3, 4](f)(r, s, t, a, b) * D[1](f)(r, s, t, a, b) * D[1, 3](f)(r, s, t, a, b) + 4 * D[5](f)(r, \\
& s, t, a, b) * \\
& D[2, 5](f)(r, s, t, a, b) * D[1](f)(r, s, t, a, b) * D[1, 3](f)(r, s, t, a, b) - 4 * D[2, \\
& 3](f)(r, s, t, a, b) * \\
& D[1](f)(r, s, t, a, b) * D[1, 3](f)(r, s, t, a, b) + 4 * D[4](f)(r, s, t, a, b) * D[3](f)(r, s, \\
& t, a, b) * D[1, 5](f)(r, s, t, a, b) * D[1, 3](f)(r, s, t, a, b) + \\
& 4 * D[5](f)(r, s, t, a, b) * D[2](f)(r, s, t, a, b) * D[1, 5](f)(r, s, t, a, b) * D[1, 3](f)(r, s, \\
& t, a, b) + \\
& 4 * D[5](f)(r, s, t, a, b) * D[3](f)(r, s, t, a, b) * D[1, 4](f)(r, s, t, a, b) * D[1, 3](f)(r, s, \\
& t, a, b) - \\
& 4 * D[5](f)(r, s, t, a, b) * D[4](f)(r, s, t, a, b) * D[1, 3](f)(r, s, t, a, b)^2 - 2 \\
& * D[2](f)(r, s, t, a, b) * D[1, 3](f)(r, s, t, a, b)^2 + \\
& 4 * D[4, 4](f)(r, s, t, a, b) * D[3](f)(r, s, t, a, b)^2 * D[1, 2](f)(r, s, t, a, b) - 8 \\
& * D[4](f)(r, s, t, a, b) * \\
& D[3](f)(r, s, t, a, b) * D[3, 4](f)(r, s, t, a, b) * D[1, 2](f)(r, s, t, a, b) + 4 * D[4](f)(r, \\
& s, t, a, b)^2 *
\end{aligned}$$

$$\begin{aligned}
& D[3, 3](f)(r, s, t, a, b) * D[1, 2](f)(r, s, t, a, b) - 8 * D[4](f)(r, s, t, a, b) * D[3, \\
& 5](f)(r, s, t, a, b) * D[2](f)(r, s, t, a, b) * D[1, 2](f)(r, s, t, a, b) + \\
& 4 * D[5](f)(r, s, t, a, b) * D[3, 4](f)(r, s, t, a, b) * D[2](f)(r, s, t, a, b) * D[1, 2](f)(r, s, \\
& t, a, b) - \\
& 2 * D[4](f)(r, s, t, a, b) * D[3](f)(r, s, t, a, b) * D[2, 5](f)(r, s, t, a, b) * D[1, 2](f)(r, s, \\
& t, a, b) - \\
& 2 * D[5](f)(r, s, t, a, b) * D[2](f)(r, s, t, a, b) * D[2, 5](f)(r, s, t, a, b) * D[1, 2](f)(r, s, \\
& t, a, b) - \\
& 2 * D[5](f)(r, s, t, a, b) * D[3](f)(r, s, t, a, b) * D[2, 4](f)(r, s, t, a, b) * D[1, 2](f)(r, s, \\
& t, a, b) + \\
& 4 * D[5](f)(r, s, t, a, b) * D[4](f)(r, s, t, a, b) * D[2, 3](f)(r, s, t, a, b) * D[1, 2](f)(r, s, \\
& t, a, b) + \\
& 2 * D[2](f)(r, s, t, a, b) * D[2, 3](f)(r, s, t, a, b) * D[1, 2](f)(r, s, t, a, b) + D[5](f)(r, \\
& s, t, a, b)^2 * \\
& D[2, 2](f)(r, s, t, a, b) * D[1, 2](f)(r, s, t, a, b) + 4 * D[3](f)(r, s, t, a, b) * D[2, \\
& 2](f)(r, s, t, a, b) * D[1, 2](f)(r, s, t, a, b) + 4 * D[5](f)(r, s, t, a, b) * \\
& D[3, 5](f)(r, s, t, a, b) * D[1](f)(r, s, t, a, b) * D[1, 2](f)(r, s, t, a, b) + 4 * D[3, \\
& 3](f)(r, s, t, a, b) * \\
& D[1](f)(r, s, t, a, b) * D[1, 2](f)(r, s, t, a, b) + 4 * D[5](f)(r, s, t, a, b) * D[3](f)(r, s, \\
& t, a, b) * D[1, 5](f)(r, s, t, a, b) * D[1, 2](f)(r, s, t, a, b) - \\
& 4 * D[5](f)(r, s, t, a, b)^2 * D[1, 3](f)(r, s, t, a, b) * D[1, 2](f)(r, s, t, a, b) - 4 \\
& * D[3](f)(r, s, t, a, b) * \\
& D[1, 3](f)(r, s, t, a, b) * D[1, 2](f)(r, s, t, a, b) - 4 * D[4](f)(r, s, t, a, b) * D[3](f)(r, \\
& s, t, a, b) * D[3, 5](f)(r, s, t, a, b) * D[1, 1](f)(r, s, t, a, b) - \\
& 4 * D[5](f)(r, s, t, a, b) * D[3](f)(r, s, t, a, b) * D[3, 4](f)(r, s, t, a, b) * D[1, 1](f)(r, s, \\
& t, a, b) + \\
& 4 * D[5](f)(r, s, t, a, b) * D[4](f)(r, s, t, a, b) * D[3, 3](f)(r, s, t, a, b) * D[1, 1](f)(r, s, \\
& t, a, b) - \\
& 4 * D[5](f)(r, s, t, a, b) * D[3, 5](f)(r, s, t, a, b) * D[2](f)(r, s, t, a, b) * D[1, 1](f)(r, s, \\
& t, a, b) + \\
& 2 * D[3, 3](f)(r, s, t, a, b) * D[2](f)(r, s, t, a, b) * D[1, 1](f)(r, s, t, a, b) - 4 \\
& * D[5](f)(r, s, t, a, b) * D[3](f)(r, s, t, a, b) * D[2, 5](f)(r, s, t, a, b) * D[1, 1](f)(r, \\
& s, t, a, b) + \\
& 4 * D[5](f)(r, s, t, a, b)^2 * D[2, 3](f)(r, s, t, a, b) * D[1, 1](f)(r, s, t, a, b) + 4 \\
& * D[3](f)(r, s, t, a, b) * \\
& D[2, 3](f)(r, s, t, a, b) * D[1, 1](f)(r, s, t, a, b) + 2 * D[5, 5](f)(r, s, t, a, b) * (D[4, \\
& 4](f)(r, s, t, a, b) * D[2](f)(r, s, t, a, b)^3 + \\
& 2 * D[2](f)(r, s, t, a, b)^2 * D[1, 2](f)(r, s, t, a, b) + 2 * D[1](f)(r, s, t, a, b) * (D[2, \\
& 3](f)(r, s, t, a, b) * D[1](f)(r, s, t, a, b) - \\
& D[3](f)(r, s, t, a, b) * D[1, 2](f)(r, s, t, a, b)) - D[2](f)(r, s, t, a, b) * (D[2, 2](f)(r, s, \\
& t, a, b) * D[1](f)(r, s, t, a, b) + 2 * D[1](f)(r, s, t, a, b) * \\
& D[1, 3](f)(r, s, t, a, b) - 2 * D[3](f)(r, s, t, a, b) * D[1, 1](f)(r, s, t, a, b))) + D[4, \\
& 5](f)(r, s, t, a, b) * (-2 * D[2](f)(r, s, t, a, b)^2 * \\
& (D[2, 2](f)(r, s, t, a, b) + 2 * D[1, 3](f)(r, s, t, a, b)) + 4 * D[2](f)(r, s, t, a, b) \\
& * (D[2, 3](f)(r, s, t, a, b) * D[1](f)(r, s, t, a, b) + \\
& D[3](f)(r, s, t, a, b) * D[1, 2](f)(r, s, t, a, b)) + 4 * (D[3, 3](f)(r, s, t, a, b) \\
& * D[1](f)(r, s, t, a, b)^2 - D[3](f)(r, s, t, a, b) * D[1](f)(r, s, t, a, b) * \\
& (D[2, 2](f)(r, s, t, a, b) + 2 * D[1, 3](f)(r, s, t, a, b)) + D[3](f)(r, s, t, a, b)^2 * D[1, \\
& 1](f)(r, s, t, a, b))) /
\end{aligned}$$

$$\begin{aligned}
& (D[4](f)(r, s, t, a, b)^2 * D[3](f)(r, s, t, a, b) - D[5](f)(r, s, t, a, b) * D[4](f)(r, s, t, a, b) \\
& \quad * D[2](f)(r, s, t, a, b) - \\
& \quad D[2](f)(r, s, t, a, b)^2 + (D[5](f)(r, s, t, a, b)^2 + 4 * D[3](f)(r, s, t, a, b)) \\
& \quad * D[1](f)(r, s, t, a, b)), \\
D[2, 2, 3](f)(r, s, t, a, b) = & \\
& (-2 * D[4, 5](f)(r, s, t, a, b)^2 * D[3](f)(r, s, t, a, b) * D[2](f)(r, s, t, a, b)^2 - 2 \\
& \quad * D[3, 4](f)(r, s, t, a, b)^2 * \\
& \quad D[2](f)(r, s, t, a, b)^2 + 2 * D[4, 4](f)(r, s, t, a, b) * D[3, 3](f)(r, s, t, a, b) \\
& \quad * D[2](f)(r, s, t, a, b)^2 - 2 * D[3, 4](f)(r, s, t, a, b) * \\
& \quad D[2](f)(r, s, t, a, b)^2 * D[2, 5](f)(r, s, t, a, b) - 2 * D[4](f)(r, s, t, a, b) * D[3, \\
& \quad 3](f)(r, s, t, a, b) * D[2](f)(r, s, t, a, b) * D[2, 4](f)(r, s, t, a, b) + \\
& \quad 2 * D[3, 5](f)(r, s, t, a, b) * D[2](f)(r, s, t, a, b)^2 * D[2, 4](f)(r, s, t, a, b) + 2 \\
& \quad * D[3](f)(r, s, t, a, b) * \\
& \quad D[2](f)(r, s, t, a, b) * D[2, 5](f)(r, s, t, a, b) * D[2, 4](f)(r, s, t, a, b) + 2 * D[4](f)(r, \\
& \quad s, t, a, b) * \\
& \quad D[3, 4](f)(r, s, t, a, b) * D[2](f)(r, s, t, a, b) * D[2, 3](f)(r, s, t, a, b) + 2 * D[4](f)(r, \\
& \quad s, t, a, b) * \\
& \quad D[3](f)(r, s, t, a, b) * D[2, 4](f)(r, s, t, a, b) * D[2, 3](f)(r, s, t, a, b) - 2 * D[5](f)(r, \\
& \quad s, t, a, b) * \\
& \quad D[2](f)(r, s, t, a, b) * D[2, 4](f)(r, s, t, a, b) * D[2, 3](f)(r, s, t, a, b) + D[4](f)(r, s, t, \\
& \quad a, b)^2 * \\
& \quad D[3, 3](f)(r, s, t, a, b) * D[2, 2](f)(r, s, t, a, b) - D[4](f)(r, s, t, a, b) * D[3, 5](f)(r, s, \\
& \quad t, a, b) * D[2](f)(r, s, t, a, b) * D[2, 2](f)(r, s, t, a, b) + \\
& \quad D[5](f)(r, s, t, a, b) * D[3, 4](f)(r, s, t, a, b) * D[2](f)(r, s, t, a, b) * D[2, 2](f)(r, s, t, \\
& \quad a, b) - \\
& \quad D[5](f)(r, s, t, a, b) * D[4](f)(r, s, t, a, b) * D[2, 3](f)(r, s, t, a, b) * D[2, 2](f)(r, s, t, \\
& \quad a, b) - 2 * D[2](f)(r, s, t, a, b) * \\
& \quad D[2, 3](f)(r, s, t, a, b) * D[2, 2](f)(r, s, t, a, b) - 4 * D[3, 5](f)(r, s, t, a, b) * D[3, \\
& \quad 4](f)(r, s, t, a, b) * D[2](f)(r, s, t, a, b) * D[1](f)(r, s, t, a, b) - \\
& \quad 2 * D[4](f)(r, s, t, a, b) * D[3, 3](f)(r, s, t, a, b) * D[2, 5](f)(r, s, t, a, b) * D[1](f)(r, s, \\
& \quad t, a, b) + \\
& \quad 2 * D[3](f)(r, s, t, a, b) * D[2, 5](f)(r, s, t, a, b)^2 * D[1](f)(r, s, t, a, b) + 4 \\
& \quad * D[3](f)(r, s, t, a, b) * \\
& \quad D[3, 5](f)(r, s, t, a, b) * D[2, 4](f)(r, s, t, a, b) * D[1](f)(r, s, t, a, b) - 2 * D[5](f)(r, \\
& \quad s, t, a, b) * \\
& \quad D[3, 3](f)(r, s, t, a, b) * D[2, 4](f)(r, s, t, a, b) * D[1](f)(r, s, t, a, b) + 2 * D[4](f)(r, \\
& \quad s, t, a, b) * \\
& \quad D[3, 5](f)(r, s, t, a, b) * D[2, 3](f)(r, s, t, a, b) * D[1](f)(r, s, t, a, b) + 2 * D[5](f)(r, \\
& \quad s, t, a, b) * \\
& \quad D[3, 4](f)(r, s, t, a, b) * D[2, 3](f)(r, s, t, a, b) * D[1](f)(r, s, t, a, b) + 2 * D[2, \\
& \quad 3](f)(r, s, t, a, b)^2 * D[1](f)(r, s, t, a, b) + \\
& \quad 2 * D[5](f)(r, s, t, a, b) * D[3, 5](f)(r, s, t, a, b) * D[2, 2](f)(r, s, t, a, b) * D[1](f)(r, s, \\
& \quad t, a, b) + 2 * D[3, 3](f)(r, s, t, a, b) * \\
& \quad D[2, 2](f)(r, s, t, a, b) * D[1](f)(r, s, t, a, b) - 2 * D[3, 5](f)(r, s, t, a, b)^2 \\
& \quad * D[1](f)(r, s, t, a, b)^2 - 4 * D[3](f)(r, s, t, a, b) * \\
& \quad D[3, 4](f)(r, s, t, a, b) * D[2](f)(r, s, t, a, b) * D[1, 5](f)(r, s, t, a, b) - 4 * D[3](f)(r, \\
& \quad s, t, a, b) * D[2](f)(r, s, t, a, b) * D[2, 5](f)(r, s, t, a, b) * D[1, 5](f)(r, s, t, a, b) - \\
& \quad 4 * D[3](f)(r, s, t, a, b)^2 * D[2, 4](f)(r, s, t, a, b) * D[1, 5](f)(r, s, t, a, b) + 4
\end{aligned}$$



$$\begin{aligned}
& *D[4](f)(r, s, t, a, b) * \\
& D[3](f)(r, s, t, a, b) * D[2, 3](f)(r, s, t, a, b) * D[1, 5](f)(r, s, t, a, b) + 2 * D[5](f)(r, \\
& s, t, a, b) * \\
& D[3](f)(r, s, t, a, b) * D[2, 2](f)(r, s, t, a, b) * D[1, 5](f)(r, s, t, a, b) + 4 * D[3](f)(r, \\
& s, t, a, b) * \\
& D[3, 5](f)(r, s, t, a, b) * D[1](f)(r, s, t, a, b) * D[1, 5](f)(r, s, t, a, b) - 4 * D[5](f)(r, \\
& s, t, a, b) * \\
& D[3, 3](f)(r, s, t, a, b) * D[1](f)(r, s, t, a, b) * D[1, 5](f)(r, s, t, a, b) - 2 * D[3](f)(r, \\
& s, t, a, b)^2 * D[1, 5](f)(r, s, t, a, b)^2 + \\
& 8 * D[3](f)(r, s, t, a, b) * D[3, 5](f)(r, s, t, a, b) * D[2](f)(r, s, t, a, b) * D[1, 4](f)(r, s, \\
& t, a, b) - 4 * D[5](f)(r, s, t, a, b) * \\
& D[3, 3](f)(r, s, t, a, b) * D[2](f)(r, s, t, a, b) * D[1, 4](f)(r, s, t, a, b) + 4 * D[5](f)(r, \\
& s, t, a, b) * D[3, 4](f)(r, s, t, a, b) * D[2](f)(r, s, t, a, b) * D[1, 3](f)(r, s, t, a, b) + \\
& 2 * D[4](f)(r, s, t, a, b) * D[3](f)(r, s, t, a, b) * D[2, 5](f)(r, s, t, a, b) * D[1, 3](f)(r, s, \\
& t, a, b) + 2 * D[5](f)(r, s, t, a, b) * \\
& D[2](f)(r, s, t, a, b) * D[2, 5](f)(r, s, t, a, b) * D[1, 3](f)(r, s, t, a, b) + 2 * D[5](f)(r, \\
& s, t, a, b) * \\
& D[3](f)(r, s, t, a, b) * D[2, 4](f)(r, s, t, a, b) * D[1, 3](f)(r, s, t, a, b) - 4 * D[5](f)(r, \\
& s, t, a, b) * \\
& D[4](f)(r, s, t, a, b) * D[2, 3](f)(r, s, t, a, b) * D[1, 3](f)(r, s, t, a, b) - 2 * D[2](f)(r, \\
& s, t, a, b) * \\
& D[2, 3](f)(r, s, t, a, b) * D[1, 3](f)(r, s, t, a, b) - D[5](f)(r, s, t, a, b)^2 * \\
& D[2, 2](f)(r, s, t, a, b) * D[1, 3](f)(r, s, t, a, b) + 4 * D[5](f)(r, s, t, a, b) * \\
& D[3, 5](f)(r, s, t, a, b) * D[1](f)(r, s, t, a, b) * D[1, 3](f)(r, s, t, a, b) + 4 * D[5](f)(r, \\
& s, t, a, b) * \\
& D[3](f)(r, s, t, a, b) * D[1, 5](f)(r, s, t, a, b) * D[1, 3](f)(r, s, t, a, b) - 2 * D[5](f)(r, \\
& s, t, a, b)^2 * D[1, 3](f)(r, s, t, a, b)^2 - \\
& 2 * D[3](f)(r, s, t, a, b) * D[1, 3](f)(r, s, t, a, b)^2 - 6 * D[4](f)(r, s, t, a, b) * \\
& D[3](f)(r, s, t, a, b) * D[3, 5](f)(r, s, t, a, b) * D[1, 2](f)(r, s, t, a, b) - 2 * D[5](f)(r, \\
& s, t, a, b) * \\
& D[3](f)(r, s, t, a, b) * D[3, 4](f)(r, s, t, a, b) * D[1, 2](f)(r, s, t, a, b) + 4 * D[5](f)(r, \\
& s, t, a, b) * \\
& D[4](f)(r, s, t, a, b) * D[3, 3](f)(r, s, t, a, b) * D[1, 2](f)(r, s, t, a, b) - 2 * D[5](f)(r, \\
& s, t, a, b) * \\
& D[3, 5](f)(r, s, t, a, b) * D[2](f)(r, s, t, a, b) * D[1, 2](f)(r, s, t, a, b) + 2 * D[3, \\
& 3](f)(r, s, t, a, b) * \\
& D[2](f)(r, s, t, a, b) * D[1, 2](f)(r, s, t, a, b) - 2 * D[5](f)(r, s, t, a, b) * D[3](f)(r, s, t, \\
& a, b) * D[2, 5](f)(r, s, t, a, b) * D[1, 2](f)(r, s, t, a, b) + \\
& 2 * D[5](f)(r, s, t, a, b)^2 * D[2, 3](f)(r, s, t, a, b) * D[1, 2](f)(r, s, t, a, b) + 4 \\
& * D[3](f)(r, s, t, a, b) * \\
& D[2, 3](f)(r, s, t, a, b) * D[1, 2](f)(r, s, t, a, b) + D[4, 5](f)(r, s, t, a, b) * (4 * D[3, \\
& 3](f)(r, s, t, a, b) * D[2](f)(r, s, t, a, b) * \\
& D[1](f)(r, s, t, a, b) - 2 * D[3](f)(r, s, t, a, b) * (2 * D[2, 3](f)(r, s, t, a, b) \\
& * D[1](f)(r, s, t, a, b) + D[2](f)(r, s, t, a, b) * (D[2, 2](f)(r, s, t, a, b) + \\
& 2 * D[1, 3](f)(r, s, t, a, b))) + 4 * D[3](f)(r, s, t, a, b)^2 * D[1, 2](f)(r, s, t, a, b)) - 4 \\
& * D[5](f)(r, s, t, a, b) * \\
& D[3](f)(r, s, t, a, b) * D[3, 5](f)(r, s, t, a, b) * D[1, 1](f)(r, s, t, a, b) + 2 * D[5](f)(r, \\
& s, t, a, b)^2 *
\end{aligned}$$

$$\begin{aligned}
& D[3, 3](f)(r, s, t, a, b) * D[1, 1](f)(r, s, t, a, b) + 2 * D[3](f)(r, s, t, a, b) * D[3, \\
& 3](f)(r, s, t, a, b) * D[1, 1](f)(r, s, t, a, b) + 2 * D[5, 5](f)(r, s, t, a, b) * \\
& (D[4, 4](f)(r, s, t, a, b) * D[3](f)(r, s, t, a, b) * D[2](f)(r, s, t, a, b)^2 + D[3, 3](f)(r, \\
& s, t, a, b) * D[1](f)(r, s, t, a, b)^2 - \\
& D[3](f)(r, s, t, a, b) * (D[2, 2](f)(r, s, t, a, b) * D[1](f)(r, s, t, a, b) + 2 * D[1](f)(r, s, \\
& t, a, b) * D[1, 3](f)(r, s, t, a, b) - \\
& 2 * D[2](f)(r, s, t, a, b) * D[1, 2](f)(r, s, t, a, b)) + D[3](f)(r, s, t, a, b)^2 * D[1, \\
& 1](f)(r, s, t, a, b))) / \\
& (D[4](f)(r, s, t, a, b)^2 * D[3](f)(r, s, t, a, b) - D[5](f)(r, s, t, a, b) * D[4](f)(r, s, t, a, \\
& b) * D[2](f)(r, s, t, a, b) - \\
& D[2](f)(r, s, t, a, b)^2 + (D[5](f)(r, s, t, a, b)^2 + 4 * D[3](f)(r, s, t, a, b)) \\
& * D[1](f)(r, s, t, a, b)), \\
D[2, 2, 4](f)(r, s, t, a, b) = & \\
& (-2 * D[4, 5](f)(r, s, t, a, b) * D[2](f)(r, s, t, a, b)^2 * D[2, 4](f)(r, s, t, a, b) \\
& + D[4](f)(r, s, t, a, b)^2 * \\
& D[3, 4](f)(r, s, t, a, b) * D[2, 2](f)(r, s, t, a, b) - 2 * D[2](f)(r, s, t, a, b) * D[2, \\
& 4](f)(r, s, t, a, b) * D[2, 2](f)(r, s, t, a, b) - 4 * D[4, 5](f)(r, s, t, a, b) * \\
& D[3, 4](f)(r, s, t, a, b) * D[2](f)(r, s, t, a, b) * D[1](f)(r, s, t, a, b) + 2 * D[5](f)(r, s, \\
& t, a, b) * \\
& D[3, 4](f)(r, s, t, a, b) * D[2, 4](f)(r, s, t, a, b) * D[1](f)(r, s, t, a, b) + 2 * D[5](f)(r, \\
& s, t, a, b) * \\
& D[2, 5](f)(r, s, t, a, b) * D[2, 4](f)(r, s, t, a, b) * D[1](f)(r, s, t, a, b) + 4 * D[2, \\
& 4](f)(r, s, t, a, b) * \\
& D[2, 3](f)(r, s, t, a, b) * D[1](f)(r, s, t, a, b) - 4 * D[4, 5](f)(r, s, t, a, b) * D[2](f)(r, \\
& s, t, a, b)^2 * D[1, 5](f)(r, s, t, a, b) - \\
& 2 * D[2](f)(r, s, t, a, b) * D[2, 2](f)(r, s, t, a, b) * D[1, 5](f)(r, s, t, a, b) + 4 * D[2, \\
& 3](f)(r, s, t, a, b) * \\
& D[1](f)(r, s, t, a, b) * D[1, 5](f)(r, s, t, a, b) + 4 * D[4, 5](f)(r, s, t, a, b) * D[3](f)(r, \\
& s, t, a, b) * D[2](f)(r, s, t, a, b) * D[1, 4](f)(r, s, t, a, b) + \\
& 4 * D[5, 5](f)(r, s, t, a, b) * D[2](f)(r, s, t, a, b)^2 * D[1, 4](f)(r, s, t, a, b) - 2 \\
& * D[5](f)(r, s, t, a, b) * \\
& D[2](f)(r, s, t, a, b) * D[2, 5](f)(r, s, t, a, b) * D[1, 4](f)(r, s, t, a, b) - 2 * D[5](f)(r, \\
& s, t, a, b) * \\
& D[3](f)(r, s, t, a, b) * D[2, 4](f)(r, s, t, a, b) * D[1, 4](f)(r, s, t, a, b) + 6 * D[2](f)(r, \\
& s, t, a, b) * \\
& D[2, 3](f)(r, s, t, a, b) * D[1, 4](f)(r, s, t, a, b) + D[5](f)(r, s, t, a, b)^2 * D[2, \\
& 2](f)(r, s, t, a, b) * D[1, 4](f)(r, s, t, a, b) + 4 * D[3, 3](f)(r, s, t, a, b) * \\
& D[1](f)(r, s, t, a, b) * D[1, 4](f)(r, s, t, a, b) - 4 * D[2](f)(r, s, t, a, b) * D[2, 4](f)(r, \\
& s, t, a, b) * D[1, 3](f)(r, s, t, a, b) - 4 * D[3, 4](f)(r, s, t, a, b) * \\
& D[1](f)(r, s, t, a, b) * D[1, 3](f)(r, s, t, a, b) - 4 * D[2, 5](f)(r, s, t, a, b) * D[1](f)(r, \\
& s, t, a, b) * D[1, 3](f)(r, s, t, a, b) - 4 * D[2](f)(r, s, t, a, b) * \\
& D[1, 5](f)(r, s, t, a, b) * D[1, 3](f)(r, s, t, a, b) - 4 * D[3](f)(r, s, t, a, b) * D[1, \\
& 4](f)(r, s, t, a, b) * D[1, 3](f)(r, s, t, a, b) + 2 * D[5](f)(r, s, t, a, b) * \\
& D[4, 5](f)(r, s, t, a, b) * D[2](f)(r, s, t, a, b) * D[1, 2](f)(r, s, t, a, b) - 2 * D[3, \\
& 4](f)(r, s, t, a, b) * \\
& D[2](f)(r, s, t, a, b) * D[1, 2](f)(r, s, t, a, b) + 2 * D[2](f)(r, s, t, a, b) * D[2, 5](f)(r, \\
& s, t, a, b) * D[1, 2](f)(r, s, t, a, b) + 4 * D[3](f)(r, s, t, a, b) * \\
& D[2, 4](f)(r, s, t, a, b) * D[1, 2](f)(r, s, t, a, b) - 4 * D[3](f)(r, s, t, a, b) * D[1,
\end{aligned}$$

$$\begin{aligned}
& 5](f)(r, s, t, a, b) * D[1, 2](f)(r, s, t, a, b) + 4 * D[5](f)(r, s, t, a, b) * \\
& D[1, 3](f)(r, s, t, a, b) * D[1, 2](f)(r, s, t, a, b) + D[4, 4](f)(r, s, t, a, b) * (2 \\
& * D[2](f)(r, s, t, a, b)^2 * D[2, 5](f)(r, s, t, a, b) - \\
& D[2](f)(r, s, t, a, b) * (D[5](f)(r, s, t, a, b) * D[2, 2](f)(r, s, t, a, b) - 4 * D[3, 5](f)(r, \\
& s, t, a, b) * D[1](f)(r, s, t, a, b) + 4 * D[3](f)(r, s, t, a, b) * \\
& D[1, 5](f)(r, s, t, a, b)) + 2 * D[5](f)(r, s, t, a, b) * (- (D[2, 3](f)(r, s, t, a, b) \\
& * D[1](f)(r, s, t, a, b)) + D[3](f)(r, s, t, a, b) * D[1, 2](f)(r, s, t, a, b))) + \\
& 4 * D[3](f)(r, s, t, a, b) * D[3, 4](f)(r, s, t, a, b) * D[1, 1](f)(r, s, t, a, b) + 4 * D[3, \\
& 5](f)(r, s, t, a, b) * D[2](f)(r, s, t, a, b) * D[1, 1](f)(r, s, t, a, b) + 4 * D[3](f)(r, s, t, \\
& a, b) * \\
& D[2, 5](f)(r, s, t, a, b) * D[1, 1](f)(r, s, t, a, b) - 4 * D[5](f)(r, s, t, a, b) * D[2, \\
& 3](f)(r, s, t, a, b) * D[1, 1](f)(r, s, t, a, b) - D[4](f)(r, s, t, a, b) * \\
& (2 * D[4, 5](f)(r, s, t, a, b)^2 * D[2](f)(r, s, t, a, b)^2 - 2 * D[5, 5](f)(r, s, t, a, b) \\
& * D[4, 4](f)(r, s, t, a, b) * D[2](f)(r, s, t, a, b)^2 + \\
& 2 * D[3, 4](f)(r, s, t, a, b) * D[2](f)(r, s, t, a, b) * D[2, 4](f)(r, s, t, a, b) - 2 \\
& * D[3](f)(r, s, t, a, b) * D[2, 4](f)(r, s, t, a, b)^2 - \\
& 2 * D[4, 4](f)(r, s, t, a, b) * D[2](f)(r, s, t, a, b) * D[2, 3](f)(r, s, t, a, b) + D[5](f)(r, \\
& s, t, a, b) * D[2, 4](f)(r, s, t, a, b) * D[2, 2](f)(r, s, t, a, b) + \\
& 2 * D[3, 4](f)(r, s, t, a, b) * D[2, 5](f)(r, s, t, a, b) * D[1](f)(r, s, t, a, b) - 2 \\
& * D[3](f)(r, s, t, a, b) * D[2, 5](f)(r, s, t, a, b) * D[1, 4](f)(r, s, t, a, b) - \\
& 2 * D[2, 2](f)(r, s, t, a, b) * D[1, 3](f)(r, s, t, a, b) - 2 * D[1, 3](f)(r, s, t, a, b)^2 + 2 \\
& * D[2, 3](f)(r, s, t, a, b) * D[1, 2](f)(r, s, t, a, b) + D[4, 5](f)(r, s, t, a, b) * \\
& (D[2](f)(r, s, t, a, b) * D[2, 2](f)(r, s, t, a, b) - 2 * D[2, 3](f)(r, s, t, a, b) * D[1](f)(r, \\
& s, t, a, b) + 2 * D[3](f)(r, s, t, a, b) * \\
& D[1, 2](f)(r, s, t, a, b)) + 2 * D[3, 3](f)(r, s, t, a, b) * D[1, 1](f)(r, s, t, a, b))) / \\
& (D[4](f)(r, s, t, a, b)^2 * D[3](f)(r, s, t, a, b) - D[5](f)(r, s, t, a, b) * D[4](f)(r, s, t, a, \\
& b) * D[2](f)(r, s, t, a, b) - \\
& D[2](f)(r, s, t, a, b)^2 + (D[5](f)(r, s, t, a, b)^2 + 4 * D[3](f)(r, s, t, a, b)) \\
& * D[1](f)(r, s, t, a, b)), \\
& D[2, 2, 5](f)(r, s, t, a, b) = \\
& (4 * D[4, 4](f)(r, s, t, a, b) * D[3, 5](f)(r, s, t, a, b) * D[2](f)(r, s, t, a, b)^2 - 4 * D[4, \\
& 5](f)(r, s, t, a, b) * D[3, 4](f)(r, s, t, a, b) * \\
& D[2](f)(r, s, t, a, b)^2 - 2 * D[4, 5](f)(r, s, t, a, b) * D[2](f)(r, s, t, a, b)^2 * D[2, \\
& 5](f)(r, s, t, a, b) - 2 * D[4](f)(r, s, t, a, b) * \\
& D[3, 5](f)(r, s, t, a, b) * D[2](f)(r, s, t, a, b) * D[2, 4](f)(r, s, t, a, b) + 2 * D[5, \\
& 5](f)(r, s, t, a, b) * D[2](f)(r, s, t, a, b)^2 * D[2, 4](f)(r, s, t, a, b) + \\
& 2 * D[4](f)(r, s, t, a, b) * D[3](f)(r, s, t, a, b) * D[2, 5](f)(r, s, t, a, b) * D[2, 4](f)(r, s, \\
& t, a, b) + 2 * D[4](f)(r, s, t, a, b) * \\
& D[4, 5](f)(r, s, t, a, b) * D[2](f)(r, s, t, a, b) * D[2, 3](f)(r, s, t, a, b) + 2 * D[2](f)(r, \\
& s, t, a, b) * D[2, 4](f)(r, s, t, a, b) * D[2, 3](f)(r, s, t, a, b) + D[4](f)(r, s, t, a, b)^2 * \\
& D[3, 5](f)(r, s, t, a, b) * D[2, 2](f)(r, s, t, a, b) - D[5, 5](f)(r, s, t, a, b) * D[4](f)(r, s, \\
& t, a, b) * D[2](f)(r, s, t, a, b) * D[2, 2](f)(r, s, t, a, b) - \\
& 2 * D[3, 4](f)(r, s, t, a, b) * D[2](f)(r, s, t, a, b) * D[2, 2](f)(r, s, t, a, b) - 2 \\
& * D[2](f)(r, s, t, a, b) * \\
& D[2, 5](f)(r, s, t, a, b) * D[2, 2](f)(r, s, t, a, b) + 4 * D[4, 5](f)(r, s, t, a, b) * D[3, \\
& 5](f)(r, s, t, a, b) * D[2](f)(r, s, t, a, b) * D[1](f)(r, s, t, a, b) - \\
& 4 * D[5, 5](f)(r, s, t, a, b) * D[3, 4](f)(r, s, t, a, b) * D[2](f)(r, s, t, a, b) * D[1](f)(r, s, \\
& t, a, b) - 2 * D[4](f)(r, s, t, a, b) * \\
& D[3, 5](f)(r, s, t, a, b) * D[2, 5](f)(r, s, t, a, b) * D[1](f)(r, s, t, a, b) + 4 * D[3,
\end{aligned}$$

$$\begin{aligned}
& 3](f)(r, s, t, a, b) * \\
& D[2, 4](f)(r, s, t, a, b) * D[1](f)(r, s, t, a, b) + 2 * D[5, 5](f)(r, s, t, a, b) * D[4](f)(r, \\
& s, t, a, b) * D[2, 3](f)(r, s, t, a, b) * D[1](f)(r, s, t, a, b) - \\
& 4 * D[3, 4](f)(r, s, t, a, b) * D[2, 3](f)(r, s, t, a, b) * D[1](f)(r, s, t, a, b) + 4 * D[2, \\
& 5](f)(r, s, t, a, b) * \\
& D[2, 3](f)(r, s, t, a, b) * D[1](f)(r, s, t, a, b) - 4 * D[4, 5](f)(r, s, t, a, b) * D[3](f)(r, \\
& s, t, a, b) * D[2](f)(r, s, t, a, b) * D[1, 5](f)(r, s, t, a, b) + \\
& 2 * D[4](f)(r, s, t, a, b) * D[3](f)(r, s, t, a, b) * D[2, 5](f)(r, s, t, a, b) * D[1, 5](f)(r, s, \\
& t, a, b) - 2 * D[2](f)(r, s, t, a, b) * \\
& D[2, 3](f)(r, s, t, a, b) * D[1, 5](f)(r, s, t, a, b) + D[5](f)(r, s, t, a, b)^2 * D[2, \\
& 2](f)(r, s, t, a, b) * D[1, 5](f)(r, s, t, a, b) + 4 * D[3, 3](f)(r, s, t, a, b) * \\
& D[1](f)(r, s, t, a, b) * D[1, 5](f)(r, s, t, a, b) + 4 * D[5, 5](f)(r, s, t, a, b) * D[3](f)(r, \\
& s, t, a, b) * D[2](f)(r, s, t, a, b) * D[1, 4](f)(r, s, t, a, b) + \\
& 4 * D[3, 3](f)(r, s, t, a, b) * D[2](f)(r, s, t, a, b) * D[1, 4](f)(r, s, t, a, b) - 4 * D[3, \\
& 4](f)(r, s, t, a, b) * \\
& D[2](f)(r, s, t, a, b) * D[1, 3](f)(r, s, t, a, b) - 4 * D[2](f)(r, s, t, a, b) * D[2, 5](f)(r, \\
& s, t, a, b) * D[1, 3](f)(r, s, t, a, b) - 4 * D[3](f)(r, s, t, a, b) * \\
& D[2, 4](f)(r, s, t, a, b) * D[1, 3](f)(r, s, t, a, b) + 4 * D[4](f)(r, s, t, a, b) * D[2, \\
& 3](f)(r, s, t, a, b) * D[1, 3](f)(r, s, t, a, b) - 4 * D[3, 5](f)(r, s, t, a, b) * \\
& D[1](f)(r, s, t, a, b) * D[1, 3](f)(r, s, t, a, b) - 4 * D[3](f)(r, s, t, a, b) * D[1, 5](f)(r, \\
& s, t, a, b) * D[1, 3](f)(r, s, t, a, b) - 2 * D[5, 5](f)(r, s, t, a, b) * \\
& D[4](f)(r, s, t, a, b) * D[3](f)(r, s, t, a, b) * D[1, 2](f)(r, s, t, a, b) + 4 * D[3](f)(r, s, \\
& t, a, b) * \\
& D[3, 4](f)(r, s, t, a, b) * D[1, 2](f)(r, s, t, a, b) - 4 * D[4](f)(r, s, t, a, b) * D[3, \\
& 3](f)(r, s, t, a, b) * D[1, 2](f)(r, s, t, a, b) + 6 * D[3, 5](f)(r, s, t, a, b) * \\
& D[2](f)(r, s, t, a, b) * D[1, 2](f)(r, s, t, a, b) + 4 * D[3](f)(r, s, t, a, b) * D[2, 5](f)(r, \\
& s, t, a, b) * D[1, 2](f)(r, s, t, a, b) + 4 * D[3](f)(r, s, t, a, b) * \\
& D[3, 5](f)(r, s, t, a, b) * D[1, 1](f)(r, s, t, a, b) - D[5](f)(r, s, t, a, b) * (2 * D[4, \\
& 5](f)(r, s, t, a, b)^2 * D[2](f)(r, s, t, a, b)^2 + \\
& D[4](f)(r, s, t, a, b) * D[2, 5](f)(r, s, t, a, b) * D[2, 2](f)(r, s, t, a, b) - 2 * D[2, \\
& 5](f)(r, s, t, a, b)^2 * D[1](f)(r, s, t, a, b) - 2 * D[3, 5](f)(r, s, t, a, b) * \\
& D[2, 4](f)(r, s, t, a, b) * D[1](f)(r, s, t, a, b) + 2 * D[2](f)(r, s, t, a, b) * D[2, 5](f)(r, \\
& s, t, a, b) * D[1, 5](f)(r, s, t, a, b) + 2 * D[3](f)(r, s, t, a, b) * \\
& D[2, 4](f)(r, s, t, a, b) * D[1, 5](f)(r, s, t, a, b) - 2 * D[2, 2](f)(r, s, t, a, b) * D[1, \\
& 3](f)(r, s, t, a, b) - 2 * D[1, 3](f)(r, s, t, a, b)^2 + \\
& 2 * D[2, 3](f)(r, s, t, a, b) * D[1, 2](f)(r, s, t, a, b) - 2 * D[5, 5](f)(r, s, t, a, b) \\
& * D[2](f)(r, s, t, a, b) * (D[4, 4](f)(r, s, t, a, b) * \\
& D[2](f)(r, s, t, a, b) + D[1, 2](f)(r, s, t, a, b)) + D[4, 5](f)(r, s, t, a, b) * (D[2](f)(r, \\
& s, t, a, b) * D[2, 2](f)(r, s, t, a, b) + \\
& 2 * D[2, 3](f)(r, s, t, a, b) * D[1](f)(r, s, t, a, b) - 2 * D[3](f)(r, s, t, a, b) * D[1, \\
& 2](f)(r, s, t, a, b)) + 2 * D[3, 3](f)(r, s, t, a, b) * D[1, 1](f)(r, s, t, a, b)) / \\
& (D[4](f)(r, s, t, a, b)^2 * D[3](f)(r, s, t, a, b) - D[5](f)(r, s, t, a, b) * D[4](f)(r, s, t, a, \\
& b) * D[2](f)(r, s, t, a, b) - \\
& D[2](f)(r, s, t, a, b)^2 + (D[5](f)(r, s, t, a, b)^2 + 4 * D[3](f)(r, s, t, a, b)) \\
& * D[1](f)(r, s, t, a, b)), \\
& D[2, 3, 3](f)(r, s, t, a, b) = \\
& (-2 * D[4, 5](f)(r, s, t, a, b)^2 * D[3](f)(r, s, t, a, b)^2 * D[2](f)(r, s, t, a, b) - 2 \\
& * D[3](f)(r, s, t, a, b) * D[3, 4](f)(r, s, t, a, b)^2 *
\end{aligned}$$

$$\begin{aligned}
& D[2](f)(r, s, t, a, b) + 2 * D[4, 4](f)(r, s, t, a, b) * D[3](f)(r, s, t, a, b) * D[3, 3](f)(r, \\
& s, t, a, b) * D[2](f)(r, s, t, a, b) - \\
& 2 * D[3, 5](f)(r, s, t, a, b) * D[3, 4](f)(r, s, t, a, b) * D[2](f)(r, s, t, a, b)^2 - 2 \\
& * D[3](f)(r, s, t, a, b) * D[3, 4](f)(r, s, t, a, b) * D[2](f)(r, s, t, a, b) * D[2, 5](f)(r, \\
& s, t, a, b) - \\
& D[4](f)(r, s, t, a, b) * D[3, 3](f)(r, s, t, a, b) * D[2](f)(r, s, t, a, b) * D[2, 5](f)(r, s, t, \\
& a, b) + 6 * D[3](f)(r, s, t, a, b) * \\
& D[3, 5](f)(r, s, t, a, b) * D[2](f)(r, s, t, a, b) * D[2, 4](f)(r, s, t, a, b) - 3 * D[5](f)(r, \\
& s, t, a, b) * D[3, 3](f)(r, s, t, a, b) * D[2](f)(r, s, t, a, b) * D[2, 4](f)(r, s, t, a, b) + \\
& 2 * D[4](f)(r, s, t, a, b) * D[3](f)(r, s, t, a, b) * D[3, 4](f)(r, s, t, a, b) * D[2, 3](f)(r, s, \\
& t, a, b) + \\
& D[4](f)(r, s, t, a, b)^2 * D[3, 3](f)(r, s, t, a, b) * D[2, 3](f)(r, s, t, a, b) + 2 \\
& * D[5](f)(r, s, t, a, b) * \\
& D[3, 4](f)(r, s, t, a, b) * D[2](f)(r, s, t, a, b) * D[2, 3](f)(r, s, t, a, b) + 2 * D[4](f)(r, \\
& s, t, a, b) * D[3](f)(r, s, t, a, b) * D[2, 5](f)(r, s, t, a, b) * D[2, 3](f)(r, s, t, a, b) - \\
& 2 * D[5](f)(r, s, t, a, b) * D[4](f)(r, s, t, a, b) * D[2, 3](f)(r, s, t, a, b)^2 - 2 \\
& * D[2](f)(r, s, t, a, b) * D[2, 3](f)(r, s, t, a, b)^2 + \\
& 2 * D[4, 5](f)(r, s, t, a, b) * D[2](f)(r, s, t, a, b) * (D[3, 3](f)(r, s, t, a, b) * D[2](f)(r, \\
& s, t, a, b) - 2 * D[3](f)(r, s, t, a, b) * \\
& D[2, 3](f)(r, s, t, a, b)) - 2 * D[4](f)(r, s, t, a, b) * D[3](f)(r, s, t, a, b) * D[3, 5](f)(r, \\
& s, t, a, b) * D[2, 2](f)(r, s, t, a, b) + \\
& D[5](f)(r, s, t, a, b) * D[4](f)(r, s, t, a, b) * D[3, 3](f)(r, s, t, a, b) * D[2, 2](f)(r, s, t, \\
& a, b) - 2 * D[3, 5](f)(r, s, t, a, b)^2 * \\
& D[2](f)(r, s, t, a, b) * D[1](f)(r, s, t, a, b) + 4 * D[3](f)(r, s, t, a, b) * D[3, 5](f)(r, s, \\
& t, a, b) * D[2, 5](f)(r, s, t, a, b) * D[1](f)(r, s, t, a, b) - \\
& 2 * D[5](f)(r, s, t, a, b) * D[3, 3](f)(r, s, t, a, b) * D[2, 5](f)(r, s, t, a, b) * D[1](f)(r, s, \\
& t, a, b) + 4 * D[5](f)(r, s, t, a, b) * \\
& D[3, 5](f)(r, s, t, a, b) * D[2, 3](f)(r, s, t, a, b) * D[1](f)(r, s, t, a, b) + 4 * D[3, \\
& 3](f)(r, s, t, a, b) * \\
& D[2, 3](f)(r, s, t, a, b) * D[1](f)(r, s, t, a, b) - 4 * D[3](f)(r, s, t, a, b)^2 * D[3, \\
& 4](f)(r, s, t, a, b) * D[1, 5](f)(r, s, t, a, b) + 2 * D[4](f)(r, s, t, a, b) * \\
& D[3](f)(r, s, t, a, b) * D[3, 3](f)(r, s, t, a, b) * D[1, 5](f)(r, s, t, a, b) - 2 * D[5](f)(r, \\
& s, t, a, b) * \\
& D[3, 3](f)(r, s, t, a, b) * D[2](f)(r, s, t, a, b) * D[1, 5](f)(r, s, t, a, b) - 4 * D[3](f)(r, \\
& s, t, a, b)^2 * \\
& D[2, 5](f)(r, s, t, a, b) * D[1, 5](f)(r, s, t, a, b) + 4 * D[5](f)(r, s, t, a, b) * D[3](f)(r, \\
& s, t, a, b) * D[2, 3](f)(r, s, t, a, b) * D[1, 5](f)(r, s, t, a, b) + \\
& 4 * D[3](f)(r, s, t, a, b)^2 * D[3, 5](f)(r, s, t, a, b) * D[1, 4](f)(r, s, t, a, b) - 2 \\
& * D[5](f)(r, s, t, a, b) * D[3](f)(r, s, t, a, b) * D[3, 3](f)(r, s, t, a, b) * D[1, 4](f)(r, \\
& s, t, a, b) - \\
& 2 * D[4](f)(r, s, t, a, b) * D[3](f)(r, s, t, a, b) * D[3, 5](f)(r, s, t, a, b) * D[1, 3](f)(r, s, \\
& t, a, b) + \\
& 2 * D[5](f)(r, s, t, a, b) * D[3](f)(r, s, t, a, b) * D[3, 4](f)(r, s, t, a, b) * D[1, 3](f)(r, s, \\
& t, a, b) + \\
& 2 * D[5](f)(r, s, t, a, b) * D[3, 5](f)(r, s, t, a, b) * D[2](f)(r, s, t, a, b) * D[1, 3](f)(r, s, \\
& t, a, b) + \\
& 2 * D[5](f)(r, s, t, a, b) * D[3](f)(r, s, t, a, b) * D[2, 5](f)(r, s, t, a, b) * D[1, 3](f)(r, s, \\
& t, a, b) - \\
& 2 * D[5](f)(r, s, t, a, b)^2 * D[2, 3](f)(r, s, t, a, b) * D[1, 3](f)(r, s, t, a, b) - 6
\end{aligned}$$

$$\begin{aligned}
& *D[5](f)(r, s, t, a, b) * \\
& D[3](f)(r, s, t, a, b) * D[3, 5](f)(r, s, t, a, b) * D[1, 2](f)(r, s, t, a, b) + 3 * D[5](f)(r, \\
& s, t, a, b)^2 * \\
& D[3, 3](f)(r, s, t, a, b) * D[1, 2](f)(r, s, t, a, b) + 4 * D[3](f)(r, s, t, a, b) * D[3, \\
& 3](f)(r, s, t, a, b) * D[1, 2](f)(r, s, t, a, b) + 2 * D[5, 5](f)(r, s, t, a, b) * \\
& (D[4, 4](f)(r, s, t, a, b) * D[3](f)(r, s, t, a, b)^2 * D[2](f)(r, s, t, a, b) + D[3, 3](f)(r, \\
& s, t, a, b) * D[2](f)(r, s, t, a, b) * D[1](f)(r, s, t, a, b) - \\
& 2 * D[3](f)(r, s, t, a, b) * D[2, 3](f)(r, s, t, a, b) * D[1](f)(r, s, t, a, b) + 2 * D[3](f)(r, \\
& s, t, a, b)^2 * D[1, 2](f)(r, s, t, a, b)) / \\
& (D[4](f)(r, s, t, a, b)^2 * D[3](f)(r, s, t, a, b) - D[5](f)(r, s, t, a, b) * D[4](f)(r, s, t, a, \\
& b) * D[2](f)(r, s, t, a, b) - \\
& D[2](f)(r, s, t, a, b)^2 + (D[5](f)(r, s, t, a, b)^2 + 4 * D[3](f)(r, s, t, a, b)) \\
& * D[1](f)(r, s, t, a, b)), \\
& D[2, 3, 4](f)(r, s, t, a, b) = \\
& (- (D[4, 5](f)(r, s, t, a, b) * D[3, 4](f)(r, s, t, a, b) * D[2](f)(r, s, t, a, b)^2) - D[4, \\
& 5](f)(r, s, t, a, b) * D[3](f)(r, s, t, a, b) * D[2](f)(r, s, t, a, b) * \\
& D[2, 4](f)(r, s, t, a, b) + D[4](f)(r, s, t, a, b)^2 * D[3, 4](f)(r, s, t, a, b) * D[2, \\
& 3](f)(r, s, t, a, b) - D[2](f)(r, s, t, a, b) * \\
& D[2, 4](f)(r, s, t, a, b) * D[2, 3](f)(r, s, t, a, b) - D[3, 4](f)(r, s, t, a, b) * D[2](f)(r, s, \\
& t, a, b) * D[2, 2](f)(r, s, t, a, b) - 2 * D[4, 5](f)(r, s, t, a, b) * \\
& D[3](f)(r, s, t, a, b) * D[3, 4](f)(r, s, t, a, b) * D[1](f)(r, s, t, a, b) + D[5](f)(r, s, t, a, \\
& b) * D[3, 4](f)(r, s, t, a, b)^2 * \\
& D[1](f)(r, s, t, a, b) + D[5](f)(r, s, t, a, b) * D[3, 4](f)(r, s, t, a, b) * D[2, 5](f)(r, s, t, \\
& a, b) * D[1](f)(r, s, t, a, b) + \\
& D[5](f)(r, s, t, a, b) * D[3, 5](f)(r, s, t, a, b) * D[2, 4](f)(r, s, t, a, b) * D[1](f)(r, s, t, \\
& a, b) + 2 * D[3, 3](f)(r, s, t, a, b) * \\
& D[2, 4](f)(r, s, t, a, b) * D[1](f)(r, s, t, a, b) + 2 * D[3, 4](f)(r, s, t, a, b) * D[2, \\
& 3](f)(r, s, t, a, b) * D[1](f)(r, s, t, a, b) - 4 * D[4, 5](f)(r, s, t, a, b) * \\
& D[3](f)(r, s, t, a, b) * D[2](f)(r, s, t, a, b) * D[1, 5](f)(r, s, t, a, b) - 2 * D[3](f)(r, s, t, \\
& a, b) * \\
& D[2, 2](f)(r, s, t, a, b) * D[1, 5](f)(r, s, t, a, b) + 2 * D[3, 3](f)(r, s, t, a, b) \\
& * D[1](f)(r, s, t, a, b) * D[1, 5](f)(r, s, t, a, b) + 2 * D[4, 5](f)(r, s, t, a, b) * \\
& D[3](f)(r, s, t, a, b)^2 * D[1, 4](f)(r, s, t, a, b) - D[5](f)(r, s, t, a, b) * D[3](f)(r, s, t, \\
& a, b) * D[3, 4](f)(r, s, t, a, b) * \\
& D[1, 4](f)(r, s, t, a, b) + 4 * D[5, 5](f)(r, s, t, a, b) * D[3](f)(r, s, t, a, b) * D[2](f)(r, \\
& s, t, a, b) * D[1, 4](f)(r, s, t, a, b) - \\
& D[5](f)(r, s, t, a, b) * D[3, 5](f)(r, s, t, a, b) * D[2](f)(r, s, t, a, b) * D[1, 4](f)(r, s, t, \\
& a, b) + 3 * D[3, 3](f)(r, s, t, a, b) * \\
& D[2](f)(r, s, t, a, b) * D[1, 4](f)(r, s, t, a, b) - D[5](f)(r, s, t, a, b) * D[3](f)(r, s, t, a, \\
& b) * D[2, 5](f)(r, s, t, a, b) * D[1, 4](f)(r, s, t, a, b) + \\
& D[5](f)(r, s, t, a, b)^2 * D[2, 3](f)(r, s, t, a, b) * D[1, 4](f)(r, s, t, a, b) + 2 \\
& * D[3](f)(r, s, t, a, b) * \\
& D[2, 3](f)(r, s, t, a, b) * D[1, 4](f)(r, s, t, a, b) + D[5](f)(r, s, t, a, b) * D[4, 5](f)(r, \\
& s, t, a, b) * D[2](f)(r, s, t, a, b) * D[1, 3](f)(r, s, t, a, b) - \\
& 3 * D[3, 4](f)(r, s, t, a, b) * D[2](f)(r, s, t, a, b) * D[1, 3](f)(r, s, t, a, b) - D[2](f)(r, \\
& s, t, a, b) * \\
& D[2, 5](f)(r, s, t, a, b) * D[1, 3](f)(r, s, t, a, b) + D[5](f)(r, s, t, a, b) * D[2, 2](f)(r, \\
& s, t, a, b) * D[1, 3](f)(r, s, t, a, b) - 2 * D[3, 5](f)(r, s, t, a, b) *
\end{aligned}$$

$$\begin{aligned}
& D[1](f)(r, s, t, a, b) * D[1, 3](f)(r, s, t, a, b) - 4 * D[3](f)(r, s, t, a, b) * D[1, 5](f)(r, \\
& \quad s, t, a, b) * D[1, 3](f)(r, s, t, a, b) + 2 * D[5](f)(r, s, t, a, b) * \\
& D[1, 3](f)(r, s, t, a, b)^2 + D[4, 4](f)(r, s, t, a, b) * (D[3, 5](f)(r, s, t, a, b) \\
& \quad * (D[2](f)(r, s, t, a, b)^2 + 2 * D[3](f)(r, s, t, a, b) * \\
& D[1](f)(r, s, t, a, b)) - D[5](f)(r, s, t, a, b) * (D[2](f)(r, s, t, a, b) * D[2, 3](f)(r, s, t, \\
& \quad a, b) + D[3, 3](f)(r, s, t, a, b) * \\
& D[1](f)(r, s, t, a, b)) - 2 * D[3](f)(r, s, t, a, b)^2 * D[1, 5](f)(r, s, t, a, b) \\
& \quad + D[3](f)(r, s, t, a, b) * (D[2](f)(r, s, t, a, b) * \\
& D[2, 5](f)(r, s, t, a, b) + D[5](f)(r, s, t, a, b) * D[1, 3](f)(r, s, t, a, b))) + D[5](f)(r, \\
& \quad s, t, a, b) * D[4, 5](f)(r, s, t, a, b) * D[3](f)(r, s, t, a, b) * \\
& D[1, 2](f)(r, s, t, a, b) + 2 * D[3](f)(r, s, t, a, b) * D[3, 4](f)(r, s, t, a, b) * D[1, \\
& \quad 2](f)(r, s, t, a, b) + D[3, 5](f)(r, s, t, a, b) * \\
& D[2](f)(r, s, t, a, b) * D[1, 2](f)(r, s, t, a, b) + 2 * D[3](f)(r, s, t, a, b) * D[2, 5](f)(r, \\
& \quad s, t, a, b) * D[1, 2](f)(r, s, t, a, b) - D[5](f)(r, s, t, a, b) * \\
& D[2, 3](f)(r, s, t, a, b) * D[1, 2](f)(r, s, t, a, b) + D[4](f)(r, s, t, a, b) * (-2 * D[4, \\
& \quad 5](f)(r, s, t, a, b)^2 * D[3](f)(r, s, t, a, b) * D[2](f)(r, s, t, a, b) + \\
& 2 * D[5, 5](f)(r, s, t, a, b) * D[4, 4](f)(r, s, t, a, b) * D[3](f)(r, s, t, a, b) * D[2](f)(r, s, \\
& \quad t, a, b) - D[3, 4](f)(r, s, t, a, b)^2 * D[2](f)(r, s, t, a, b) + \\
& D[4, 4](f)(r, s, t, a, b) * D[3, 3](f)(r, s, t, a, b) * D[2](f)(r, s, t, a, b) - D[3, 4](f)(r, s, \\
& \quad t, a, b) * D[2](f)(r, s, t, a, b) * D[2, 5](f)(r, s, t, a, b) + \\
& D[3](f)(r, s, t, a, b) * D[3, 4](f)(r, s, t, a, b) * D[2, 4](f)(r, s, t, a, b) + D[3](f)(r, s, t, \\
& \quad a, b) * D[2, 5](f)(r, s, t, a, b) * D[2, 4](f)(r, s, t, a, b) + \\
& D[4, 4](f)(r, s, t, a, b) * D[3](f)(r, s, t, a, b) * D[2, 3](f)(r, s, t, a, b) - D[5](f)(r, s, t, \\
& \quad a, b) * D[2, 4](f)(r, s, t, a, b) * D[2, 3](f)(r, s, t, a, b) - \\
& D[3, 5](f)(r, s, t, a, b) * D[3, 4](f)(r, s, t, a, b) * D[1](f)(r, s, t, a, b) + D[3](f)(r, s, t, \\
& \quad a, b) * D[3, 5](f)(r, s, t, a, b) * D[1, 4](f)(r, s, t, a, b) + \\
& D[2, 3](f)(r, s, t, a, b) * D[1, 3](f)(r, s, t, a, b) - D[4, 5](f)(r, s, t, a, b) * (- (D[3, \\
& \quad 3](f)(r, s, t, a, b) * D[1](f)(r, s, t, a, b)) + D[3](f)(r, s, t, a, b) * \\
& (D[2, 2](f)(r, s, t, a, b) + D[1, 3](f)(r, s, t, a, b))) - D[3, 3](f)(r, s, t, a, b) * D[1, \\
& \quad 2](f)(r, s, t, a, b)) + 4 * D[3](f)(r, s, t, a, b) * \\
& D[3, 5](f)(r, s, t, a, b) * D[1, 1](f)(r, s, t, a, b) - 2 * D[5](f)(r, s, t, a, b) * D[3, \\
& \quad 3](f)(r, s, t, a, b) * D[1, 1](f)(r, s, t, a, b)) / \\
& (D[4](f)(r, s, t, a, b)^2 * D[3](f)(r, s, t, a, b) - D[5](f)(r, s, t, a, b) * D[4](f)(r, s, t, a, \\
& \quad b) * D[2](f)(r, s, t, a, b) - \\
& D[2](f)(r, s, t, a, b)^2 + (D[5](f)(r, s, t, a, b)^2 + 4 * D[3](f)(r, s, t, a, b)) \\
& \quad * D[1](f)(r, s, t, a, b)), \\
& D[2, 3, 5](f)(r, s, t, a, b) = \\
& \quad (4 * D[4, 4](f)(r, s, t, a, b) * D[3](f)(r, s, t, a, b) * D[3, 5](f)(r, s, t, a, b) * D[2](f)(r, \\
& \quad s, t, a, b) - 4 * D[4, 5](f)(r, s, t, a, b) * \\
& D[3](f)(r, s, t, a, b) * D[3, 4](f)(r, s, t, a, b) * D[2](f)(r, s, t, a, b) - D[4](f)(r, s, t, a, \\
& \quad b) * D[3, 5](f)(r, s, t, a, b) * D[3, 4](f)(r, s, t, a, b) * \\
& D[2](f)(r, s, t, a, b) + D[4](f)(r, s, t, a, b) * D[4, 5](f)(r, s, t, a, b) * D[3, 3](f)(r, s, t, \\
& \quad a, b) * D[2](f)(r, s, t, a, b) + \\
& D[4, 5](f)(r, s, t, a, b) * D[3, 5](f)(r, s, t, a, b) * D[2](f)(r, s, t, a, b)^2 - D[5, \\
& \quad 5](f)(r, s, t, a, b) * D[3, 4](f)(r, s, t, a, b) * D[2](f)(r, s, t, a, b)^2 + \\
& D[4](f)(r, s, t, a, b) * D[3](f)(r, s, t, a, b) * D[3, 4](f)(r, s, t, a, b) * D[2, 5](f)(r, s, t, \\
& \quad a, b) - 3 * D[4, 5](f)(r, s, t, a, b) * \\
& D[3](f)(r, s, t, a, b) * D[2](f)(r, s, t, a, b) * D[2, 5](f)(r, s, t, a, b) - D[4](f)(r, s, t, a,
\end{aligned}$$

$$\begin{aligned}
& b) * D[3, 5](f)(r, s, t, a, b) * D[2](f)(r, s, t, a, b) * \\
& D[2, 5](f)(r, s, t, a, b) + D[4](f)(r, s, t, a, b) * D[3](f)(r, s, t, a, b) * D[2, 5](f)(r, s, t, \\
& a, b)^2 + 3 * D[5, 5](f)(r, s, t, a, b) * \\
& D[3](f)(r, s, t, a, b) * D[2](f)(r, s, t, a, b) * D[2, 4](f)(r, s, t, a, b) + 3 * D[3, 3](f)(r, \\
& s, t, a, b) * \\
& D[2](f)(r, s, t, a, b) * D[2, 4](f)(r, s, t, a, b) + D[4](f)(r, s, t, a, b) * D[4, 5](f)(r, s, t, \\
& a, b) * D[3](f)(r, s, t, a, b) * D[2, 3](f)(r, s, t, a, b) + \\
& D[4](f)(r, s, t, a, b)^2 * D[3, 5](f)(r, s, t, a, b) * D[2, 3](f)(r, s, t, a, b) - 3 * D[3, \\
& 4](f)(r, s, t, a, b) * \\
& D[2](f)(r, s, t, a, b) * D[2, 3](f)(r, s, t, a, b) - 2 * D[2](f)(r, s, t, a, b) * D[2, 5](f)(r, \\
& s, t, a, b) * D[2, 3](f)(r, s, t, a, b) + D[4](f)(r, s, t, a, b) * \\
& D[2, 3](f)(r, s, t, a, b)^2 - D[5, 5](f)(r, s, t, a, b) * D[4](f)(r, s, t, a, b) * D[3](f)(r, s, \\
& t, a, b) * D[2, 2](f)(r, s, t, a, b) - \\
& D[4](f)(r, s, t, a, b) * D[3, 3](f)(r, s, t, a, b) * D[2, 2](f)(r, s, t, a, b) + 2 * D[4, \\
& 5](f)(r, s, t, a, b) * \\
& D[3](f)(r, s, t, a, b) * D[3, 5](f)(r, s, t, a, b) * D[1](f)(r, s, t, a, b) - D[4](f)(r, s, t, a, \\
& b) * D[3, 5](f)(r, s, t, a, b)^2 * D[1](f)(r, s, t, a, b) - \\
& 2 * D[5, 5](f)(r, s, t, a, b) * D[3](f)(r, s, t, a, b) * D[3, 4](f)(r, s, t, a, b) * D[1](f)(r, s, \\
& t, a, b) + D[5, 5](f)(r, s, t, a, b) * D[4](f)(r, s, t, a, b) * D[3, 3](f)(r, s, t, a, b) * \\
& D[1](f)(r, s, t, a, b) + 4 * D[3, 3](f)(r, s, t, a, b) * D[2, 5](f)(r, s, t, a, b) * D[1](f)(r, \\
& s, t, a, b) - 2 * D[4, 5](f)(r, s, t, a, b) * \\
& D[3](f)(r, s, t, a, b)^2 * D[1, 5](f)(r, s, t, a, b) + D[4](f)(r, s, t, a, b) * D[3](f)(r, s, t, \\
& a, b) * D[3, 5](f)(r, s, t, a, b) * \\
& D[1, 5](f)(r, s, t, a, b) + D[3, 3](f)(r, s, t, a, b) * D[2](f)(r, s, t, a, b) * D[1, 5](f)(r, \\
& s, t, a, b) + D[5](f)(r, s, t, a, b)^2 * \\
& D[2, 3](f)(r, s, t, a, b) * D[1, 5](f)(r, s, t, a, b) - 2 * D[3](f)(r, s, t, a, b) * D[2, \\
& 3](f)(r, s, t, a, b) * D[1, 5](f)(r, s, t, a, b) + 2 * D[5, 5](f)(r, s, t, a, b) * \\
& D[3](f)(r, s, t, a, b)^2 * D[1, 4](f)(r, s, t, a, b) + 2 * D[3](f)(r, s, t, a, b) * \\
& D[3, 3](f)(r, s, t, a, b) * D[1, 4](f)(r, s, t, a, b) - D[5, 5](f)(r, s, t, a, b) * D[4](f)(r, s, \\
& t, a, b) * D[3](f)(r, s, t, a, b) * D[1, 3](f)(r, s, t, a, b) - \\
& 2 * D[3](f)(r, s, t, a, b) * D[3, 4](f)(r, s, t, a, b) * D[1, 3](f)(r, s, t, a, b) - D[3, \\
& 5](f)(r, s, t, a, b) * \\
& D[2](f)(r, s, t, a, b) * D[1, 3](f)(r, s, t, a, b) - 2 * D[3](f)(r, s, t, a, b) * D[2, 5](f)(r, \\
& s, t, a, b) * D[1, 3](f)(r, s, t, a, b) + 8 * D[3](f)(r, s, t, a, b) * \\
& D[3, 5](f)(r, s, t, a, b) * D[1, 2](f)(r, s, t, a, b) - D[5](f)(r, s, t, a, b) * (2 * D[4, \\
& 5](f)(r, s, t, a, b)^2 * D[3](f)(r, s, t, a, b) * \\
& D[2](f)(r, s, t, a, b) + D[4](f)(r, s, t, a, b) * D[2, 5](f)(r, s, t, a, b) * D[2, 3](f)(r, s, t, \\
& a, b) - D[3, 5](f)(r, s, t, a, b) * D[3, 4](f)(r, s, t, a, b) * \\
& D[1](f)(r, s, t, a, b) - 2 * D[3, 5](f)(r, s, t, a, b) * D[2, 5](f)(r, s, t, a, b) * D[1](f)(r, \\
& s, t, a, b) + D[3](f)(r, s, t, a, b) * \\
& D[3, 4](f)(r, s, t, a, b) * D[1, 5](f)(r, s, t, a, b) + D[3, 5](f)(r, s, t, a, b) * D[2](f)(r, \\
& s, t, a, b) * D[1, 5](f)(r, s, t, a, b) + D[3](f)(r, s, t, a, b) * \\
& D[2, 5](f)(r, s, t, a, b) * D[1, 5](f)(r, s, t, a, b) - 3 * D[2, 3](f)(r, s, t, a, b) * D[1, \\
& 3](f)(r, s, t, a, b) + D[4, 5](f)(r, s, t, a, b) * \\
& (D[2](f)(r, s, t, a, b) * D[2, 3](f)(r, s, t, a, b) + D[3, 3](f)(r, s, t, a, b) * D[1](f)(r, s, \\
& t, a, b) - D[3](f)(r, s, t, a, b) * D[1, 3](f)(r, s, t, a, b)) + \\
& 3 * D[3, 3](f)(r, s, t, a, b) * D[1, 2](f)(r, s, t, a, b) - D[5, 5](f)(r, s, t, a, b) * (2 * D[4, \\
& 4](f)(r, s, t, a, b) * D[3](f)(r, s, t, a, b) *
\end{aligned}$$



$$\begin{aligned}
& D[2](f)(r, s, t, a, b) + D[2](f)(r, s, t, a, b) * D[1, 3](f)(r, s, t, a, b) + D[3](f)(r, s, t, a, b) * D[1, 2](f)(r, s, t, a, b) / \\
& (D[4](f)(r, s, t, a, b)^2 * D[3](f)(r, s, t, a, b) - D[5](f)(r, s, t, a, b) * D[4](f)(r, s, t, a, b) * D[2](f)(r, s, t, a, b) - \\
& D[2](f)(r, s, t, a, b)^2 + (D[5](f)(r, s, t, a, b)^2 + 4 * D[3](f)(r, s, t, a, b)) \\
& * D[1](f)(r, s, t, a, b)), \\
D[2, 4, 4](f)(r, s, t, a, b) = & (D[4](f)(r, s, t, a, b)^2 * (-2 * D[4, 5](f)(r, s, t, a, b)^2 * D[2](f)(r, s, t, a, b) + D[4, \\
& 4](f)(r, s, t, a, b) * (2 * D[5, 5](f)(r, s, t, a, b) * \\
& D[2](f)(r, s, t, a, b) + D[2, 3](f)(r, s, t, a, b))) + D[5](f)(r, s, t, a, b)^2 * D[4, \\
& 4](f)(r, s, t, a, b) * D[1, 2](f)(r, s, t, a, b) + D[4](f)(r, s, t, a, b) * \\
& (D[4, 4](f)(r, s, t, a, b) * (3 * D[2](f)(r, s, t, a, b) * D[2, 5](f)(r, s, t, a, b) \\
& - D[5](f)(r, s, t, a, b) * D[2, 2](f)(r, s, t, a, b) + \\
& 2 * D[3, 5](f)(r, s, t, a, b) * D[1](f)(r, s, t, a, b) + 2 * D[3](f)(r, s, t, a, b) * (D[2, \\
& 4](f)(r, s, t, a, b) - D[1, 5](f)(r, s, t, a, b))) + \\
& 2 * (2 * D[5, 5](f)(r, s, t, a, b) * D[2](f)(r, s, t, a, b) * D[1, 4](f)(r, s, t, a, b) + D[2, \\
& 3](f)(r, s, t, a, b) * D[1, 4](f)(r, s, t, a, b) - \\
& D[4, 5](f)(r, s, t, a, b) * (D[3, 4](f)(r, s, t, a, b) * D[1](f)(r, s, t, a, b) + 2 \\
& * D[2](f)(r, s, t, a, b) * (D[2, 4](f)(r, s, t, a, b) + \\
& D[1, 5](f)(r, s, t, a, b)) - D[3](f)(r, s, t, a, b) * D[1, 4](f)(r, s, t, a, b)) - D[3, \\
& 4](f)(r, s, t, a, b) * D[1, 2](f)(r, s, t, a, b))) + \\
& D[5](f)(r, s, t, a, b) * (- (D[4, 4](f)(r, s, t, a, b) * D[2](f)(r, s, t, a, b) * (D[2, 4](f)(r, \\
& s, t, a, b) + 2 * D[1, 5](f)(r, s, t, a, b))) + \\
& 2 * (- (D[2, 2](f)(r, s, t, a, b) * D[1, 4](f)(r, s, t, a, b)) + D[4, 5](f)(r, s, t, a, b) \\
& * (D[2, 4](f)(r, s, t, a, b) * D[1](f)(r, s, t, a, b) + \\
& D[2](f)(r, s, t, a, b) * D[1, 4](f)(r, s, t, a, b)) + D[2, 4](f)(r, s, t, a, b) * D[1, 2](f)(r, \\
& s, t, a, b))) - \\
& 2 * (D[2](f)(r, s, t, a, b) * (D[2, 4](f)(r, s, t, a, b)^2 + D[4, 5](f)(r, s, t, a, b)^2 \\
& * D[1](f)(r, s, t, a, b) - D[5, 5](f)(r, s, t, a, b) * \\
& D[4, 4](f)(r, s, t, a, b) * D[1](f)(r, s, t, a, b) + 2 * D[2, 4](f)(r, s, t, a, b) * D[1, \\
& 5](f)(r, s, t, a, b) + D[1, 5](f)(r, s, t, a, b)^2 - \\
& D[3, 4](f)(r, s, t, a, b) * D[1, 4](f)(r, s, t, a, b) - 3 * D[2, 5](f)(r, s, t, a, b) * D[1, \\
& 4](f)(r, s, t, a, b) + D[4, 4](f)(r, s, t, a, b) * D[1, 3](f)(r, s, t, a, b) + \\
& D[4, 5](f)(r, s, t, a, b) * D[1, 2](f)(r, s, t, a, b) - D[5, 5](f)(r, s, t, a, b) * D[1, \\
& 1](f)(r, s, t, a, b)) - 2 * (D[4, 4](f)(r, s, t, a, b) * \\
& D[2, 3](f)(r, s, t, a, b) * D[1](f)(r, s, t, a, b) + D[3, 5](f)(r, s, t, a, b) * D[1](f)(r, s, t, \\
& a, b) * D[1, 4](f)(r, s, t, a, b) - D[4, 5](f)(r, s, t, a, b) * \\
& D[1](f)(r, s, t, a, b) * D[1, 3](f)(r, s, t, a, b) - D[1, 3](f)(r, s, t, a, b) * D[1, 2](f)(r, s, \\
& t, a, b) + D[2, 3](f)(r, s, t, a, b) * D[1, 1](f)(r, s, t, a, b) + \\
& D[3](f)(r, s, t, a, b) * (D[2, 4](f)(r, s, t, a, b) * D[1, 4](f)(r, s, t, a, b) - D[1, 5](f)(r, \\
& s, t, a, b) * D[1, 4](f)(r, s, t, a, b) + \\
& D[4, 5](f)(r, s, t, a, b) * D[1, 1](f)(r, s, t, a, b)))) / \\
& (D[4](f)(r, s, t, a, b)^2 * D[3](f)(r, s, t, a, b) - D[5](f)(r, s, t, a, b) * D[4](f)(r, s, t, a, \\
& b) * D[2](f)(r, s, t, a, b) - \\
& D[2](f)(r, s, t, a, b)^2 + (D[5](f)(r, s, t, a, b)^2 + 4 * D[3](f)(r, s, t, a, b)) \\
& * D[1](f)(r, s, t, a, b)), \\
D[2, 4, 5](f)(r, s, t, a, b) = & (- (D[4, 5](f)(r, s, t, a, b)^2 * D[2](f)(r, s, t, a, b)^2) + D[5, 5](f)(r, s, t, a, b) * D[4,
\end{aligned}$$

$$\begin{aligned}
& 4](f)(r, s, t, a, b) * D[2](f)(r, s, t, a, b)^2 - \\
& D[3, 4](f)(r, s, t, a, b) * D[2](f)(r, s, t, a, b) * D[2, 4](f)(r, s, t, a, b) - D[2](f)(r, s, t, \\
& a, b) * D[2, 5](f)(r, s, t, a, b) * D[2, 4](f)(r, s, t, a, b) + \\
& D[4](f)(r, s, t, a, b)^2 * D[4, 5](f)(r, s, t, a, b) * D[2, 3](f)(r, s, t, a, b) + D[4, \\
& 4](f)(r, s, t, a, b) * \\
& D[2](f)(r, s, t, a, b) * D[2, 3](f)(r, s, t, a, b) - D[4, 5](f)(r, s, t, a, b) * D[2](f)(r, s, t, \\
& a, b) * D[2, 2](f)(r, s, t, a, b) - 2 * D[3, 4](f)(r, s, t, a, b)^2 * \\
& D[1](f)(r, s, t, a, b) + 2 * D[4, 4](f)(r, s, t, a, b) * D[3, 3](f)(r, s, t, a, b) * D[1](f)(r, \\
& s, t, a, b) + 2 * D[3, 5](f)(r, s, t, a, b) * \\
& D[2, 4](f)(r, s, t, a, b) * D[1](f)(r, s, t, a, b) + 2 * D[4, 5](f)(r, s, t, a, b) * \\
& D[2, 3](f)(r, s, t, a, b) * D[1](f)(r, s, t, a, b) - 3 * D[3, 4](f)(r, s, t, a, b) * D[2](f)(r, \\
& s, t, a, b) * D[1, 5](f)(r, s, t, a, b) - D[2](f)(r, s, t, a, b) * \\
& D[2, 5](f)(r, s, t, a, b) * D[1, 5](f)(r, s, t, a, b) + 2 * D[3, 5](f)(r, s, t, a, b) \\
& * D[1](f)(r, s, t, a, b) * D[1, 5](f)(r, s, t, a, b) - 2 * D[3](f)(r, s, t, a, b) * \\
& D[1, 5](f)(r, s, t, a, b)^2 + 2 * D[3](f)(r, s, t, a, b) * D[3, 4](f)(r, s, t, a, b) * D[1, \\
& 4](f)(r, s, t, a, b) + 7 * D[3, 5](f)(r, s, t, a, b) * \\
& D[2](f)(r, s, t, a, b) * D[1, 4](f)(r, s, t, a, b) + 2 * D[3](f)(r, s, t, a, b) * D[2, 5](f)(r, \\
& s, t, a, b) * D[1, 4](f)(r, s, t, a, b) - 2 * D[4, 4](f)(r, s, t, a, b) * \\
& D[3](f)(r, s, t, a, b) * D[1, 3](f)(r, s, t, a, b) - 4 * D[4, 5](f)(r, s, t, a, b) * D[2](f)(r, \\
& s, t, a, b) * D[1, 3](f)(r, s, t, a, b) - 2 * D[2, 2](f)(r, s, t, a, b) * \\
& D[1, 3](f)(r, s, t, a, b) - 2 * D[5, 5](f)(r, s, t, a, b) * D[1](f)(r, s, t, a, b) * D[1, \\
& 3](f)(r, s, t, a, b) - 2 * D[1, 3](f)(r, s, t, a, b)^2 + \\
& D[5](f)(r, s, t, a, b)^2 * D[4, 5](f)(r, s, t, a, b) * D[1, 2](f)(r, s, t, a, b) + 2 * D[4, \\
& 5](f)(r, s, t, a, b) * \\
& D[3](f)(r, s, t, a, b) * D[1, 2](f)(r, s, t, a, b) + D[5, 5](f)(r, s, t, a, b) * D[2](f)(r, s, t, \\
& a, b) * D[1, 2](f)(r, s, t, a, b) + 2 * D[2, 3](f)(r, s, t, a, b) * \\
& D[1, 2](f)(r, s, t, a, b) + D[4](f)(r, s, t, a, b) * (D[4, 4](f)(r, s, t, a, b) * (3 * D[3, \\
& 5](f)(r, s, t, a, b) * D[2](f)(r, s, t, a, b) + \\
& D[3](f)(r, s, t, a, b) * D[2, 5](f)(r, s, t, a, b)) + D[2, 4](f)(r, s, t, a, b) * D[2, 3](f)(r, \\
& s, t, a, b) - D[3, 4](f)(r, s, t, a, b) * \\
& D[2, 2](f)(r, s, t, a, b) - D[5, 5](f)(r, s, t, a, b) * D[3, 4](f)(r, s, t, a, b) * D[1](f)(r, s, \\
& t, a, b) + D[2, 3](f)(r, s, t, a, b) * \\
& D[1, 5](f)(r, s, t, a, b) + D[4, 5](f)(r, s, t, a, b) * (-3 * D[3, 4](f)(r, s, t, a, b) \\
& * D[2](f)(r, s, t, a, b) - D[2](f)(r, s, t, a, b) * \\
& D[2, 5](f)(r, s, t, a, b) + D[3](f)(r, s, t, a, b) * D[2, 4](f)(r, s, t, a, b) + D[3, 5](f)(r, \\
& s, t, a, b) * D[1](f)(r, s, t, a, b) - \\
& D[3](f)(r, s, t, a, b) * D[1, 5](f)(r, s, t, a, b)) + D[5, 5](f)(r, s, t, a, b) * D[3](f)(r, s, \\
& t, a, b) * D[1, 4](f)(r, s, t, a, b) - \\
& D[3, 5](f)(r, s, t, a, b) * D[1, 2](f)(r, s, t, a, b)) + D[5](f)(r, s, t, a, b) * ( \\
& - (D[4](f)(r, s, t, a, b) * (2 * D[4, 5](f)(r, s, t, a, b)^2 * \\
& D[2](f)(r, s, t, a, b) - 2 * D[5, 5](f)(r, s, t, a, b) * D[4, 4](f)(r, s, t, a, b) * D[2](f)(r, \\
& s, t, a, b) + D[4, 5](f)(r, s, t, a, b) * D[2, 2](f)(r, s, t, a, b))) + \\
& D[4, 4](f)(r, s, t, a, b) * D[3, 5](f)(r, s, t, a, b) * D[1](f)(r, s, t, a, b) + D[5, 5](f)(r, \\
& s, t, a, b) * D[2, 4](f)(r, s, t, a, b) * D[1](f)(r, s, t, a, b) - \\
& D[4, 4](f)(r, s, t, a, b) * D[3](f)(r, s, t, a, b) * D[1, 5](f)(r, s, t, a, b) - D[2, 2](f)(r, s, \\
& t, a, b) * D[1, 5](f)(r, s, t, a, b) + 3 * D[5, 5](f)(r, s, t, a, b) * \\
& D[2](f)(r, s, t, a, b) * D[1, 4](f)(r, s, t, a, b) - D[2, 3](f)(r, s, t, a, b) * D[1, 4](f)(r, s, \\
& t, a, b) + D[4, 5](f)(r, s, t, a, b) *
\end{aligned}$$

$$\begin{aligned}
& (- (D[3, 4](f)(r, s, t, a, b) * D[1](f)(r, s, t, a, b)) + D[2, 5](f)(r, s, t, a, b) \\
& \quad * D[1](f)(r, s, t, a, b) - D[2](f)(r, s, t, a, b) * \\
& (D[2, 4](f)(r, s, t, a, b) + 3 * D[1, 5](f)(r, s, t, a, b)) + D[3](f)(r, s, t, a, b) * D[1, \\
& \quad 4](f)(r, s, t, a, b)) + D[3, 4](f)(r, s, t, a, b) * \\
& D[1, 2](f)(r, s, t, a, b) + D[2, 5](f)(r, s, t, a, b) * D[1, 2](f)(r, s, t, a, b)) + 2 * D[5, \\
& \quad 5](f)(r, s, t, a, b) * \\
& D[3](f)(r, s, t, a, b) * D[1, 1](f)(r, s, t, a, b) + 2 * D[3, 3](f)(r, s, t, a, b) * D[1, \\
& \quad 1](f)(r, s, t, a, b)) / \\
& (D[4](f)(r, s, t, a, b)^2 * D[3](f)(r, s, t, a, b) - D[5](f)(r, s, t, a, b) * D[4](f)(r, s, t, a, \\
& \quad b) * D[2](f)(r, s, t, a, b) - \\
& D[2](f)(r, s, t, a, b)^2 + (D[5](f)(r, s, t, a, b)^2 + 4 * D[3](f)(r, s, t, a, b)) \\
& \quad * D[1](f)(r, s, t, a, b)), \\
D[2, 5, 5](f)(r, s, t, a, b) = \\
& (-2 * D[4, 5](f)(r, s, t, a, b)^2 * D[3](f)(r, s, t, a, b) * D[2](f)(r, s, t, a, b) + 2 * D[5, \\
& \quad 5](f)(r, s, t, a, b) * \\
& D[4, 4](f)(r, s, t, a, b) * D[3](f)(r, s, t, a, b) * D[2](f)(r, s, t, a, b) - 2 * D[5, 5](f)(r, \\
& \quad s, t, a, b) * \\
& D[4](f)(r, s, t, a, b) * D[3, 4](f)(r, s, t, a, b) * D[2](f)(r, s, t, a, b) - 2 * D[3, 4](f)(r, \\
& \quad s, t, a, b)^2 * D[2](f)(r, s, t, a, b) + \\
& 2 * D[4, 4](f)(r, s, t, a, b) * D[3, 3](f)(r, s, t, a, b) * D[2](f)(r, s, t, a, b) - D[5, \\
& \quad 5](f)(r, s, t, a, b) * D[4](f)(r, s, t, a, b) * D[2](f)(r, s, t, a, b) * D[2, 5](f)(r, s, t, a, b) \\
& \quad - \\
& 4 * D[3, 4](f)(r, s, t, a, b) * D[2](f)(r, s, t, a, b) * D[2, 5](f)(r, s, t, a, b) - 2 \\
& \quad * D[2](f)(r, s, t, a, b) * D[2, 5](f)(r, s, t, a, b)^2 + \\
& 6 * D[3, 5](f)(r, s, t, a, b) * D[2](f)(r, s, t, a, b) * D[2, 4](f)(r, s, t, a, b) + D[5, \\
& \quad 5](f)(r, s, t, a, b) * D[4](f)(r, s, t, a, b)^2 * \\
& D[2, 3](f)(r, s, t, a, b) + 2 * D[4](f)(r, s, t, a, b) * D[2, 5](f)(r, s, t, a, b) * D[2, \\
& \quad 3](f)(r, s, t, a, b) - 2 * D[4](f)(r, s, t, a, b) * \\
& D[3, 5](f)(r, s, t, a, b) * D[2, 2](f)(r, s, t, a, b) - 4 * D[3, 5](f)(r, s, t, a, b) * D[3, \\
& \quad 4](f)(r, s, t, a, b) * D[1](f)(r, s, t, a, b) + 4 * D[3, 5](f)(r, s, t, a, b) * \\
& D[2, 5](f)(r, s, t, a, b) * D[1](f)(r, s, t, a, b) + 2 * D[3, 5](f)(r, s, t, a, b) * D[2](f)(r, \\
& \quad s, t, a, b) * D[1, 5](f)(r, s, t, a, b) + 4 * D[3](f)(r, s, t, a, b) * \\
& D[3, 5](f)(r, s, t, a, b) * D[1, 4](f)(r, s, t, a, b) - 2 * D[5, 5](f)(r, s, t, a, b) \\
& \quad * D[2](f)(r, s, t, a, b) * D[1, 3](f)(r, s, t, a, b) - 4 * D[2, 3](f)(r, s, t, a, b) * \\
& D[1, 3](f)(r, s, t, a, b) + 2 * D[4, 5](f)(r, s, t, a, b) * (D[4](f)(r, s, t, a, b) * (D[3, \\
& \quad 5](f)(r, s, t, a, b) * D[2](f)(r, s, t, a, b) + \\
& D[3](f)(r, s, t, a, b) * D[2, 5](f)(r, s, t, a, b)) - D[2](f)(r, s, t, a, b) * D[2, 3](f)(r, s, \\
& \quad t, a, b) + 2 * D[3, 3](f)(r, s, t, a, b) * \\
& D[1](f)(r, s, t, a, b) - 2 * D[3](f)(r, s, t, a, b) * D[1, 3](f)(r, s, t, a, b)) + 4 * D[5, \\
& \quad 5](f)(r, s, t, a, b) * \\
& D[3](f)(r, s, t, a, b) * D[1, 2](f)(r, s, t, a, b) + 4 * D[3, 3](f)(r, s, t, a, b) * D[1, \\
& \quad 2](f)(r, s, t, a, b) + \\
& D[5](f)(r, s, t, a, b) * (4 * D[4, 4](f)(r, s, t, a, b) * D[3, 5](f)(r, s, t, a, b) * D[2](f)(r, \\
& \quad s, t, a, b) + 3 * D[5, 5](f)(r, s, t, a, b) * \\
& D[2](f)(r, s, t, a, b) * D[2, 4](f)(r, s, t, a, b) - D[5, 5](f)(r, s, t, a, b) * D[4](f)(r, s, t, \\
& \quad a, b) * D[2, 2](f)(r, s, t, a, b) - 2 * D[5, 5](f)(r, s, t, a, b) * \\
& D[3, 4](f)(r, s, t, a, b) * D[1](f)(r, s, t, a, b) + 2 * D[5, 5](f)(r, s, t, a, b) * D[2, \\
& \quad 5](f)(r, s, t, a, b) * D[1](f)(r, s, t, a, b) -
\end{aligned}$$

$$\begin{aligned}
& 2 * D[2, 3](f)(r, s, t, a, b) * D[1, 5](f)(r, s, t, a, b) - 2 * D[4, 5](f)(r, s, t, a, b) * (2 \\
& \quad * D[3, 4](f)(r, s, t, a, b) * D[2](f)(r, s, t, a, b) + \\
& 2 * D[2](f)(r, s, t, a, b) * D[2, 5](f)(r, s, t, a, b) - D[3, 5](f)(r, s, t, a, b) * D[1](f)(r, \\
& \quad s, t, a, b) + D[3](f)(r, s, t, a, b) * D[1, 5](f)(r, s, t, a, b)) + \\
& 2 * D[5, 5](f)(r, s, t, a, b) * D[3](f)(r, s, t, a, b) * D[1, 4](f)(r, s, t, a, b) + 2 * D[3, \\
& \quad 5](f)(r, s, t, a, b) * D[1, 2](f)(r, s, t, a, b)) + \\
& D[5](f)(r, s, t, a, b)^2 * (-2 * D[4, 5](f)(r, s, t, a, b)^2 * D[2](f)(r, s, t, a, b) + D[5, \\
& \quad 5](f)(r, s, t, a, b) * (2 * D[4, 4](f)(r, s, t, a, b) * \\
& \quad D[2](f)(r, s, t, a, b) + D[1, 2](f)(r, s, t, a, b))) / \\
& (D[4](f)(r, s, t, a, b)^2 * D[3](f)(r, s, t, a, b) - D[5](f)(r, s, t, a, b) * D[4](f)(r, s, t, a, \\
& \quad b) * D[2](f)(r, s, t, a, b) - \\
& D[2](f)(r, s, t, a, b)^2 + (D[5](f)(r, s, t, a, b)^2 + 4 * D[3](f)(r, s, t, a, b)) \\
& \quad * D[1](f)(r, s, t, a, b)), \\
D[3, 3, 3](f)(r, s, t, a, b) = & \\
& (-2 * D[4, 5](f)(r, s, t, a, b)^2 * D[3](f)(r, s, t, a, b)^3 - 2 * D[3](f)(r, s, t, a, b)^2 \\
& \quad * D[3, 4](f)(r, s, t, a, b)^2 + \\
& 2 * D[4, 4](f)(r, s, t, a, b) * D[3](f)(r, s, t, a, b)^2 * D[3, 3](f)(r, s, t, a, b) + 2 \\
& \quad * D[4](f)(r, s, t, a, b) * \\
& D[3](f)(r, s, t, a, b) * D[3, 4](f)(r, s, t, a, b) * D[3, 3](f)(r, s, t, a, b) + D[4](f)(r, s, t, \\
& \quad a, b)^2 * D[3, 3](f)(r, s, t, a, b)^2 - \\
& 2 * D[3](f)(r, s, t, a, b) * D[3, 5](f)(r, s, t, a, b) * D[3, 4](f)(r, s, t, a, b) * D[2](f)(r, s, \\
& \quad t, a, b) - \\
& D[4](f)(r, s, t, a, b) * D[3, 5](f)(r, s, t, a, b) * D[3, 3](f)(r, s, t, a, b) * D[2](f)(r, s, t, \\
& \quad a, b) - \\
& D[5](f)(r, s, t, a, b) * D[3, 4](f)(r, s, t, a, b) * D[3, 3](f)(r, s, t, a, b) * D[2](f)(r, s, t, \\
& \quad a, b) - 2 * D[3, 5](f)(r, s, t, a, b)^2 * \\
& D[2](f)(r, s, t, a, b)^2 - 4 * D[3](f)(r, s, t, a, b)^2 * D[3, 4](f)(r, s, t, a, b) * D[2, \\
& \quad 5](f)(r, s, t, a, b) + 2 * D[4](f)(r, s, t, a, b) * \\
& D[3](f)(r, s, t, a, b) * D[3, 3](f)(r, s, t, a, b) * D[2, 5](f)(r, s, t, a, b) + 4 * D[3](f)(r, \\
& \quad s, t, a, b) * \\
& D[3, 5](f)(r, s, t, a, b) * D[2](f)(r, s, t, a, b) * D[2, 5](f)(r, s, t, a, b) - 4 * D[5](f)(r, \\
& \quad s, t, a, b) * \\
& D[3, 3](f)(r, s, t, a, b) * D[2](f)(r, s, t, a, b) * D[2, 5](f)(r, s, t, a, b) - 2 * D[3](f)(r, \\
& \quad s, t, a, b)^2 * D[2, 5](f)(r, s, t, a, b)^2 + \\
& 8 * D[3](f)(r, s, t, a, b)^2 * D[3, 5](f)(r, s, t, a, b) * D[2, 4](f)(r, s, t, a, b) - 4 \\
& \quad * D[5](f)(r, s, t, a, b) * \\
& D[3](f)(r, s, t, a, b) * D[3, 3](f)(r, s, t, a, b) * D[2, 4](f)(r, s, t, a, b) - 2 * D[4](f)(r, \\
& \quad s, t, a, b) * \\
& D[3](f)(r, s, t, a, b) * D[3, 5](f)(r, s, t, a, b) * D[2, 3](f)(r, s, t, a, b) + 4 * D[5](f)(r, \\
& \quad s, t, a, b) * \\
& D[3](f)(r, s, t, a, b) * D[3, 4](f)(r, s, t, a, b) * D[2, 3](f)(r, s, t, a, b) - D[5](f)(r, s, t, \\
& \quad a, b) * D[4](f)(r, s, t, a, b) * D[3, 3](f)(r, s, t, a, b) * \\
& D[2, 3](f)(r, s, t, a, b) + 4 * D[5](f)(r, s, t, a, b) * D[3, 5](f)(r, s, t, a, b) * D[2](f)(r, \\
& \quad s, t, a, b) * D[2, 3](f)(r, s, t, a, b) - \\
& 2 * D[3, 3](f)(r, s, t, a, b) * D[2](f)(r, s, t, a, b) * D[2, 3](f)(r, s, t, a, b) + 4 \\
& \quad * D[5](f)(r, s, t, a, b) * \\
& D[3](f)(r, s, t, a, b) * D[2, 5](f)(r, s, t, a, b) * D[2, 3](f)(r, s, t, a, b) - 2 * D[5](f)(r, \\
& \quad s, t, a, b)^2 * D[2, 3](f)(r, s, t, a, b)^2 -
\end{aligned}$$

$$\begin{aligned}
& 2 * D[3](f)(r, s, t, a, b) * D[2, 3](f)(r, s, t, a, b)^2 + 2 * D[4, 5](f)(r, s, t, a, b) \\
& \quad * D[3](f)(r, s, t, a, b) * (D[3, 3](f)(r, s, t, a, b) * \\
& D[2](f)(r, s, t, a, b) - 2 * D[3](f)(r, s, t, a, b) * D[2, 3](f)(r, s, t, a, b)) - 4 \\
& \quad * D[5](f)(r, s, t, a, b) * \\
& D[3](f)(r, s, t, a, b) * D[3, 5](f)(r, s, t, a, b) * D[2, 2](f)(r, s, t, a, b) + 2 * D[5](f)(r, \\
& \quad s, t, a, b)^2 * \\
& D[3, 3](f)(r, s, t, a, b) * D[2, 2](f)(r, s, t, a, b) + 2 * D[3](f)(r, s, t, a, b) * D[3, \\
& \quad 3](f)(r, s, t, a, b) * D[2, 2](f)(r, s, t, a, b) + 2 * D[3](f)(r, s, t, a, b) * \\
& D[3, 5](f)(r, s, t, a, b)^2 * D[1](f)(r, s, t, a, b) + 2 * D[5](f)(r, s, t, a, b) * D[3, \\
& \quad 5](f)(r, s, t, a, b) * D[3, 3](f)(r, s, t, a, b) * D[1](f)(r, s, t, a, b) + \\
& 4 * D[3, 3](f)(r, s, t, a, b)^2 * D[1](f)(r, s, t, a, b) - 4 * D[3](f)(r, s, t, a, b)^2 * \\
& D[3, 5](f)(r, s, t, a, b) * D[1, 5](f)(r, s, t, a, b) + 2 * D[5](f)(r, s, t, a, b) * \\
& D[3](f)(r, s, t, a, b) * D[3, 3](f)(r, s, t, a, b) * D[1, 5](f)(r, s, t, a, b) - 2 * D[5](f)(r, \\
& \quad s, t, a, b) * \\
& D[3](f)(r, s, t, a, b) * D[3, 5](f)(r, s, t, a, b) * D[1, 3](f)(r, s, t, a, b) + D[5](f)(r, s, t, \\
& \quad a, b)^2 * \\
& D[3, 3](f)(r, s, t, a, b) * D[1, 3](f)(r, s, t, a, b) + 4 * D[3](f)(r, s, t, a, b) * D[3, \\
& \quad 3](f)(r, s, t, a, b) * D[1, 3](f)(r, s, t, a, b) + 2 * D[5, 5](f)(r, s, t, a, b) * \\
& (D[4, 4](f)(r, s, t, a, b) * D[3](f)(r, s, t, a, b)^3 + D[3, 3](f)(r, s, t, a, b) \\
& \quad * (D[2](f)(r, s, t, a, b)^2 - D[3](f)(r, s, t, a, b) * \\
& D[1](f)(r, s, t, a, b)) + D[3](f)(r, s, t, a, b) * (-2 * D[2](f)(r, s, t, a, b) * D[2, \\
& \quad 3](f)(r, s, t, a, b) + D[3](f)(r, s, t, a, b) * \\
& (D[2, 2](f)(r, s, t, a, b) + 2 * D[1, 3](f)(r, s, t, a, b)))) / \\
& (D[4](f)(r, s, t, a, b)^2 * D[3](f)(r, s, t, a, b) - D[5](f)(r, s, t, a, b) * D[4](f)(r, s, t, a, \\
& \quad b) * D[2](f)(r, s, t, a, b) - \\
& D[2](f)(r, s, t, a, b)^2 + (D[5](f)(r, s, t, a, b)^2 + 4 * D[3](f)(r, s, t, a, b)) \\
& \quad * D[1](f)(r, s, t, a, b)), \\
& D[3, 3, 4](f)(r, s, t, a, b) = \\
& (D[4](f)(r, s, t, a, b)^2 * D[3, 4](f)(r, s, t, a, b) * D[3, 3](f)(r, s, t, a, b) - 2 * D[4, \\
& \quad 5](f)(r, s, t, a, b) * D[3](f)(r, s, t, a, b) * D[3, 4](f)(r, s, t, a, b) * D[2](f)(r, s, t, a, b) \\
& \quad + \\
& D[4, 4](f)(r, s, t, a, b) * (2 * D[3](f)(r, s, t, a, b) * D[3, 5](f)(r, s, t, a, b) - D[5](f)(r, \\
& \quad s, t, a, b) * D[3, 3](f)(r, s, t, a, b)) * \\
& D[2](f)(r, s, t, a, b) - 2 * D[3, 4](f)(r, s, t, a, b) * D[2](f)(r, s, t, a, b) * D[2, 3](f)(r, \\
& \quad s, t, a, b) + D[4](f)(r, s, t, a, b) * \\
& (-2 * D[4, 5](f)(r, s, t, a, b)^2 * D[3](f)(r, s, t, a, b)^2 + 2 * D[5, 5](f)(r, s, t, a, b) \\
& \quad * D[4, 4](f)(r, s, t, a, b) * D[3](f)(r, s, t, a, b)^2 + \\
& 2 * D[4, 4](f)(r, s, t, a, b) * D[3](f)(r, s, t, a, b) * D[3, 3](f)(r, s, t, a, b) - 2 * D[3, \\
& \quad 5](f)(r, s, t, a, b) * D[3, 4](f)(r, s, t, a, b) * \\
& D[2](f)(r, s, t, a, b) + 2 * D[3](f)(r, s, t, a, b) * D[3, 5](f)(r, s, t, a, b) * D[2, 4](f)(r, \\
& \quad s, t, a, b) - D[5](f)(r, s, t, a, b) * D[3, 3](f)(r, s, t, a, b) * \\
& D[2, 4](f)(r, s, t, a, b) + D[4, 5](f)(r, s, t, a, b) * (D[3, 3](f)(r, s, t, a, b) * D[2](f)(r, \\
& \quad s, t, a, b) - 2 * D[3](f)(r, s, t, a, b) * D[2, 3](f)(r, s, t, a, b))) + \\
& 2 * D[5](f)(r, s, t, a, b) * D[3, 5](f)(r, s, t, a, b) * D[3, 4](f)(r, s, t, a, b) * D[1](f)(r, s, \\
& \quad t, a, b) + 4 * D[3, 4](f)(r, s, t, a, b) * \\
& D[3, 3](f)(r, s, t, a, b) * D[1](f)(r, s, t, a, b) - 4 * D[4, 5](f)(r, s, t, a, b) * D[3](f)(r, \\
& \quad s, t, a, b)^2 * D[1, 5](f)(r, s, t, a, b) + \\
& 2 * D[3, 3](f)(r, s, t, a, b) * D[2](f)(r, s, t, a, b) * D[1, 5](f)(r, s, t, a, b) - 4 \\
& \quad * D[3](f)(r, s, t, a, b) *
\end{aligned}$$

$$\begin{aligned}
& D[2, 3](f)(r, s, t, a, b) * D[1, 5](f)(r, s, t, a, b) + 4 * D[5, 5](f)(r, s, t, a, b) \\
& \quad * D[3](f)(r, s, t, a, b)^2 * D[1, 4](f)(r, s, t, a, b) - \\
& 2 * D[5](f)(r, s, t, a, b) * D[3](f)(r, s, t, a, b) * D[3, 5](f)(r, s, t, a, b) * D[1, 4](f)(r, s, \\
& \quad t, a, b) + \\
& D[5](f)(r, s, t, a, b)^2 * D[3, 3](f)(r, s, t, a, b) * D[1, 4](f)(r, s, t, a, b) + 4 \\
& \quad * D[3](f)(r, s, t, a, b) * D[3, 3](f)(r, s, t, a, b) * D[1, 4](f)(r, s, t, a, b) + 2 \\
& \quad * D[5](f)(r, s, t, a, b) * \\
& D[4, 5](f)(r, s, t, a, b) * D[3](f)(r, s, t, a, b) * D[1, 3](f)(r, s, t, a, b) - 2 * D[3, \\
& \quad 5](f)(r, s, t, a, b) * \\
& D[2](f)(r, s, t, a, b) * D[1, 3](f)(r, s, t, a, b) + 2 * D[5](f)(r, s, t, a, b) * D[2, 3](f)(r, \\
& \quad s, t, a, b) * D[1, 3](f)(r, s, t, a, b) + 4 * D[3](f)(r, s, t, a, b) * \\
& D[3, 5](f)(r, s, t, a, b) * D[1, 2](f)(r, s, t, a, b) - 2 * D[5](f)(r, s, t, a, b) * D[3, \\
& \quad 3](f)(r, s, t, a, b) * D[1, 2](f)(r, s, t, a, b) / \\
& (D[4](f)(r, s, t, a, b)^2 * D[3](f)(r, s, t, a, b) - D[5](f)(r, s, t, a, b) * D[4](f)(r, s, t, a, \\
& \quad b) * D[2](f)(r, s, t, a, b) - D[2](f)(r, s, t, a, b)^2 \\
& \quad + (D[5](f)(r, s, t, a, b)^2 + 4 * D[3](f)(r, s, t, a, b)) * D[1](f)(r, s, t, a, b)), \\
& D[3, 3, 5](f)(r, s, t, a, b) = \\
& (4 * D[4, 4](f)(r, s, t, a, b) * D[3](f)(r, s, t, a, b)^2 * D[3, 5](f)(r, s, t, a, b) - 4 * D[4, \\
& \quad 5](f)(r, s, t, a, b) * \\
& D[3](f)(r, s, t, a, b)^2 * D[3, 4](f)(r, s, t, a, b) + 2 * D[4](f)(r, s, t, a, b) * D[4, \\
& \quad 5](f)(r, s, t, a, b) * D[3](f)(r, s, t, a, b) * D[3, 3](f)(r, s, t, a, b) + \\
& D[4](f)(r, s, t, a, b)^2 * D[3, 5](f)(r, s, t, a, b) * D[3, 3](f)(r, s, t, a, b) + 2 * D[4, \\
& \quad 5](f)(r, s, t, a, b) * \\
& D[3](f)(r, s, t, a, b) * D[3, 5](f)(r, s, t, a, b) * D[2](f)(r, s, t, a, b) - 2 * D[4](f)(r, s, t, \\
& \quad a, b) * D[3, 5](f)(r, s, t, a, b)^2 * \\
& D[2](f)(r, s, t, a, b) - 2 * D[5, 5](f)(r, s, t, a, b) * D[3](f)(r, s, t, a, b) * D[3, 4](f)(r, \\
& \quad s, t, a, b) * D[2](f)(r, s, t, a, b) + \\
& D[5, 5](f)(r, s, t, a, b) * D[4](f)(r, s, t, a, b) * D[3, 3](f)(r, s, t, a, b) * D[2](f)(r, s, t, \\
& \quad a, b) - 4 * D[4, 5](f)(r, s, t, a, b) * \\
& D[3](f)(r, s, t, a, b)^2 * D[2, 5](f)(r, s, t, a, b) + 2 * D[4](f)(r, s, t, a, b) * \\
& D[3](f)(r, s, t, a, b) * D[3, 5](f)(r, s, t, a, b) * D[2, 5](f)(r, s, t, a, b) + 2 * D[3, \\
& \quad 3](f)(r, s, t, a, b) * \\
& D[2](f)(r, s, t, a, b) * D[2, 5](f)(r, s, t, a, b) + 4 * D[5, 5](f)(r, s, t, a, b) * D[3](f)(r, \\
& \quad s, t, a, b)^2 * D[2, 4](f)(r, s, t, a, b) + \\
& 4 * D[3](f)(r, s, t, a, b) * D[3, 3](f)(r, s, t, a, b) * D[2, 4](f)(r, s, t, a, b) - 2 * D[5, \\
& \quad 5](f)(r, s, t, a, b) * \\
& D[4](f)(r, s, t, a, b) * D[3](f)(r, s, t, a, b) * D[2, 3](f)(r, s, t, a, b) - 4 * D[3](f)(r, s, t, \\
& \quad a, b) * \\
& D[3, 4](f)(r, s, t, a, b) * D[2, 3](f)(r, s, t, a, b) - 4 * D[3, 5](f)(r, s, t, a, b) \\
& \quad * D[2](f)(r, s, t, a, b) * D[2, 3](f)(r, s, t, a, b) - 4 * D[3](f)(r, s, t, a, b) * \\
& D[2, 5](f)(r, s, t, a, b) * D[2, 3](f)(r, s, t, a, b) + 4 * D[3](f)(r, s, t, a, b) * D[3, \\
& \quad 5](f)(r, s, t, a, b) * D[2, 2](f)(r, s, t, a, b) + 4 * D[3, 5](f)(r, s, t, a, b) * \\
& D[3, 3](f)(r, s, t, a, b) * D[1](f)(r, s, t, a, b) + D[5](f)(r, s, t, a, b)^2 * D[3, 3](f)(r, \\
& \quad s, t, a, b) * D[1, 5](f)(r, s, t, a, b) + 4 * D[3](f)(r, s, t, a, b) * \\
& D[3, 5](f)(r, s, t, a, b) * D[1, 3](f)(r, s, t, a, b) - D[5](f)(r, s, t, a, b) * (2 * D[4, \\
& \quad 5](f)(r, s, t, a, b)^2 * \\
& D[3](f)(r, s, t, a, b)^2 + D[4, 5](f)(r, s, t, a, b) * D[3, 3](f)(r, s, t, a, b) * D[2](f)(r, \\
& \quad s, t, a, b) + D[4](f)(r, s, t, a, b) *
\end{aligned}$$

$$\begin{aligned}
& D[3, 3](f)(r, s, t, a, b) * D[2, 5](f)(r, s, t, a, b) - 2 * D[2, 3](f)(r, s, t, a, b)^2 + 2 \\
& \quad * D[3, 3](f)(r, s, t, a, b) * D[2, 2](f)(r, s, t, a, b) - \\
& 2 * D[3, 5](f)(r, s, t, a, b)^2 * D[1](f)(r, s, t, a, b) + 2 * D[3](f)(r, s, t, a, b) * D[3, \\
& \quad 5](f)(r, s, t, a, b) * D[1, 5](f)(r, s, t, a, b) - \\
& 2 * D[5, 5](f)(r, s, t, a, b) * D[3](f)(r, s, t, a, b) * (D[4, 4](f)(r, s, t, a, b) * D[3](f)(r, \\
& \quad s, t, a, b) + D[1, 3](f)(r, s, t, a, b))) / \\
& (D[4](f)(r, s, t, a, b)^2 * D[3](f)(r, s, t, a, b) - D[5](f)(r, s, t, a, b) * D[4](f)(r, s, t, a, \\
& \quad b) * D[2](f)(r, s, t, a, b) - \\
& D[2](f)(r, s, t, a, b)^2 + (D[5](f)(r, s, t, a, b)^2 + 4 * D[3](f)(r, s, t, a, b)) \\
& \quad * D[1](f)(r, s, t, a, b)), \\
& D[3, 4, 4](f)(r, s, t, a, b) = \\
& (D[4](f)(r, s, t, a, b)^2 * (-2 * D[4, 5](f)(r, s, t, a, b)^2 * D[3](f)(r, s, t, a, b) + D[4, \\
& \quad 4](f)(r, s, t, a, b) * (2 * D[5, 5](f)(r, s, t, a, b) * \\
& D[3](f)(r, s, t, a, b) + D[3, 3](f)(r, s, t, a, b))) + D[5](f)(r, s, t, a, b)^2 * D[4, \\
& \quad 4](f)(r, s, t, a, b) * D[1, 3](f)(r, s, t, a, b) + D[4](f)(r, s, t, a, b) * \\
& (D[4, 4](f)(r, s, t, a, b) * (D[3, 5](f)(r, s, t, a, b) * D[2](f)(r, s, t, a, b) + 2 \\
& \quad * D[3](f)(r, s, t, a, b) * (D[3, 4](f)(r, s, t, a, b) + \\
& D[2, 5](f)(r, s, t, a, b)) - D[5](f)(r, s, t, a, b) * D[2, 3](f)(r, s, t, a, b)) - 2 * (D[4, \\
& \quad 5](f)(r, s, t, a, b) * (D[3, 4](f)(r, s, t, a, b) * \\
& D[2](f)(r, s, t, a, b) + D[3](f)(r, s, t, a, b) * (D[2, 4](f)(r, s, t, a, b) + 2 * D[1, \\
& \quad 5](f)(r, s, t, a, b))) - 2 * D[5, 5](f)(r, s, t, a, b) * \\
& D[3](f)(r, s, t, a, b) * D[1, 4](f)(r, s, t, a, b) - D[3, 3](f)(r, s, t, a, b) * D[1, 4](f)(r, s, \\
& \quad t, a, b) + D[3, 4](f)(r, s, t, a, b) * \\
& D[1, 3](f)(r, s, t, a, b))) + D[5](f)(r, s, t, a, b) * (- (D[4, 4](f)(r, s, t, a, b) * (D[3, \\
& \quad 4](f)(r, s, t, a, b) * D[2](f)(r, s, t, a, b) + \\
& 2 * D[3](f)(r, s, t, a, b) * D[1, 5](f)(r, s, t, a, b))) + 2 * (- (D[2, 3](f)(r, s, t, a, b) \\
& \quad * D[1, 4](f)(r, s, t, a, b)) + D[4, 5](f)(r, s, t, a, b) * \\
& (D[3, 4](f)(r, s, t, a, b) * D[1](f)(r, s, t, a, b) + D[3](f)(r, s, t, a, b) * D[1, 4](f)(r, s, \\
& \quad t, a, b)) + D[2, 4](f)(r, s, t, a, b) * \\
& D[1, 3](f)(r, s, t, a, b))) + 2 * (- (D[4, 5](f)(r, s, t, a, b)^2 * D[3](f)(r, s, t, a, b) \\
& \quad * D[1](f)(r, s, t, a, b)) + D[5, 5](f)(r, s, t, a, b) * \\
& D[4, 4](f)(r, s, t, a, b) * D[3](f)(r, s, t, a, b) * D[1](f)(r, s, t, a, b) + D[3, 4](f)(r, s, t, \\
& \quad a, b)^2 * D[1](f)(r, s, t, a, b) + D[4, 4](f)(r, s, t, a, b) * \\
& D[3, 3](f)(r, s, t, a, b) * D[1](f)(r, s, t, a, b) - 2 * D[3](f)(r, s, t, a, b) * D[2, 4](f)(r, \\
& \quad s, t, a, b) * D[1, 5](f)(r, s, t, a, b) - \\
& D[3](f)(r, s, t, a, b) * D[1, 5](f)(r, s, t, a, b)^2 + D[3, 5](f)(r, s, t, a, b) * D[2](f)(r, \\
& \quad s, t, a, b) * D[1, 4](f)(r, s, t, a, b) + 2 * D[3](f)(r, s, t, a, b) * \\
& D[2, 5](f)(r, s, t, a, b) * D[1, 4](f)(r, s, t, a, b) + D[3, 4](f)(r, s, t, a, b) * ( \\
& \quad - (D[2](f)(r, s, t, a, b) * D[2, 4](f)(r, s, t, a, b)) + \\
& 2 * D[3](f)(r, s, t, a, b) * D[1, 4](f)(r, s, t, a, b)) - D[4, 5](f)(r, s, t, a, b) * D[2](f)(r, \\
& \quad s, t, a, b) * D[1, 3](f)(r, s, t, a, b) - D[1, 3](f)(r, s, t, a, b)^2 + \\
& D[5, 5](f)(r, s, t, a, b) * D[3](f)(r, s, t, a, b) * D[1, 1](f)(r, s, t, a, b) + D[3, 3](f)(r, \\
& \quad s, t, a, b) * D[1, 1](f)(r, s, t, a, b))) / \\
& (D[4](f)(r, s, t, a, b)^2 * D[3](f)(r, s, t, a, b) - D[5](f)(r, s, t, a, b) * D[4](f)(r, s, t, a, \\
& \quad b) * D[2](f)(r, s, t, a, b) - D[2](f)(r, s, t, a, b)^2 + \\
& (D[5](f)(r, s, t, a, b)^2 + 4 * D[3](f)(r, s, t, a, b)) * D[1](f)(r, s, t, a, b)), \\
& D[3, 4, 5](f)(r, s, t, a, b) = \\
& (D[4](f)(r, s, t, a, b)^2 * D[4, 5](f)(r, s, t, a, b) * D[3, 3](f)(r, s, t, a, b) - D[4,
\end{aligned}$$

$$\begin{aligned}
& 5](f)(r, s, t, a, b)^2 * \\
& D[3](f)(r, s, t, a, b) * D[2](f)(r, s, t, a, b) + D[5, 5](f)(r, s, t, a, b) * D[4, 4](f)(r, s, t, \\
& a, b) * D[3](f)(r, s, t, a, b) * D[2](f)(r, s, t, a, b) - \\
& D[3, 4](f)(r, s, t, a, b)^2 * D[2](f)(r, s, t, a, b) + D[4, 4](f)(r, s, t, a, b) * D[3, \\
& 3](f)(r, s, t, a, b) * D[2](f)(r, s, t, a, b) - \\
& D[3, 4](f)(r, s, t, a, b) * D[2](f)(r, s, t, a, b) * D[2, 5](f)(r, s, t, a, b) - D[4, 5](f)(r, s, \\
& t, a, b) * D[2](f)(r, s, t, a, b) * D[2, 3](f)(r, s, t, a, b) + \\
& 2 * D[3, 5](f)(r, s, t, a, b) * D[3, 4](f)(r, s, t, a, b) * D[1](f)(r, s, t, a, b) + 2 * D[4, \\
& 5](f)(r, s, t, a, b) * D[3, 3](f)(r, s, t, a, b) * D[1](f)(r, s, t, a, b) - 2 * D[3](f)(r, s, t, \\
& a, b) * \\
& D[3, 4](f)(r, s, t, a, b) * D[1, 5](f)(r, s, t, a, b) + D[3, 5](f)(r, s, t, a, b) * D[2](f)(r, \\
& s, t, a, b) * D[1, 5](f)(r, s, t, a, b) - 2 * D[3](f)(r, s, t, a, b) * \\
& D[2, 5](f)(r, s, t, a, b) * D[1, 5](f)(r, s, t, a, b) + 8 * D[3](f)(r, s, t, a, b) * D[3, \\
& 5](f)(r, s, t, a, b) * D[1, 4](f)(r, s, t, a, b) + D[5](f)(r, s, t, a, b)^2 * \\
& D[4, 5](f)(r, s, t, a, b) * D[1, 3](f)(r, s, t, a, b) - 2 * D[4, 5](f)(r, s, t, a, b) \\
& * D[3](f)(r, s, t, a, b) * D[1, 3](f)(r, s, t, a, b) - D[5, 5](f)(r, s, t, a, b) * \\
& D[2](f)(r, s, t, a, b) * D[1, 3](f)(r, s, t, a, b) - 2 * D[2, 3](f)(r, s, t, a, b) * D[1, \\
& 3](f)(r, s, t, a, b) + D[4](f)(r, s, t, a, b) * \\
& (4 * D[4, 4](f)(r, s, t, a, b) * D[3](f)(r, s, t, a, b) * D[3, 5](f)(r, s, t, a, b) - D[5, \\
& 5](f)(r, s, t, a, b) * D[3, 4](f)(r, s, t, a, b) * D[2](f)(r, s, t, a, b) - \\
& D[4, 5](f)(r, s, t, a, b) * D[3](f)(r, s, t, a, b) * (2 * D[3, 4](f)(r, s, t, a, b) + D[2, \\
& 5](f)(r, s, t, a, b)) + D[5, 5](f)(r, s, t, a, b) * \\
& D[3](f)(r, s, t, a, b) * D[2, 4](f)(r, s, t, a, b) + D[3, 3](f)(r, s, t, a, b) * D[2, 4](f)(r, \\
& s, t, a, b) - D[3, 4](f)(r, s, t, a, b) * D[2, 3](f)(r, s, t, a, b) + \\
& D[3, 3](f)(r, s, t, a, b) * D[1, 5](f)(r, s, t, a, b) - D[3, 5](f)(r, s, t, a, b) * D[1, \\
& 3](f)(r, s, t, a, b) + D[5](f)(r, s, t, a, b) * \\
& (- (D[4](f)(r, s, t, a, b) * (2 * D[4, 5](f)(r, s, t, a, b)^2 * D[3](f)(r, s, t, a, b) - 2 * D[5, \\
& 5](f)(r, s, t, a, b) * D[4, 4](f)(r, s, t, a, b) * \\
& D[3](f)(r, s, t, a, b) + D[4, 5](f)(r, s, t, a, b) * D[2, 3](f)(r, s, t, a, b))) + D[5, \\
& 5](f)(r, s, t, a, b) * D[3, 4](f)(r, s, t, a, b) * \\
& D[1](f)(r, s, t, a, b) - D[2, 3](f)(r, s, t, a, b) * D[1, 5](f)(r, s, t, a, b) + D[4, 5](f)(r, \\
& s, t, a, b) * (- (D[3, 4](f)(r, s, t, a, b) * \\
& D[2](f)(r, s, t, a, b) + D[3, 5](f)(r, s, t, a, b) * D[1](f)(r, s, t, a, b) - 3 * D[3](f)(r, \\
& s, t, a, b) * D[1, 5](f)(r, s, t, a, b)) + \\
& 3 * D[5, 5](f)(r, s, t, a, b) * D[3](f)(r, s, t, a, b) * D[1, 4](f)(r, s, t, a, b) - D[3, \\
& 3](f)(r, s, t, a, b) * D[1, 4](f)(r, s, t, a, b) + \\
& D[3, 4](f)(r, s, t, a, b) * D[1, 3](f)(r, s, t, a, b) + D[2, 5](f)(r, s, t, a, b) * D[1, \\
& 3](f)(r, s, t, a, b) + 2 * D[5, 5](f)(r, s, t, a, b) * \\
& D[3](f)(r, s, t, a, b) * D[1, 2](f)(r, s, t, a, b) + 2 * D[3, 3](f)(r, s, t, a, b) * D[1, \\
& 2](f)(r, s, t, a, b)) / \\
& (D[4](f)(r, s, t, a, b)^2 * D[3](f)(r, s, t, a, b) - D[5](f)(r, s, t, a, b) * D[4](f)(r, s, t, a, \\
& b) * D[2](f)(r, s, t, a, b) - \\
& D[2](f)(r, s, t, a, b)^2 + (D[5](f)(r, s, t, a, b)^2 + 4 * D[3](f)(r, s, t, a, b)) \\
& * D[1](f)(r, s, t, a, b)), \\
& D[3, 5, 5](f)(r, s, t, a, b) = \\
& (-2 * D[4, 5](f)(r, s, t, a, b)^2 * D[3](f)(r, s, t, a, b)^2 + 2 * D[5, 5](f)(r, s, t, a, b) \\
& * D[4, 4](f)(r, s, t, a, b) * \\
& D[3](f)(r, s, t, a, b)^2 - 2 * D[5, 5](f)(r, s, t, a, b) * D[4](f)(r, s, t, a, b) * D[3](f)(r, \\
& s, t, a, b) * D[3, 4](f)(r, s, t, a, b) - 2 * D[3](f)(r, s, t, a, b) *
\end{aligned}$$



$$\begin{aligned}
& D[3, 4](f)(r, s, t, a, b)^2 + D[5, 5](f)(r, s, t, a, b) * D[4](f)(r, s, t, a, b)^2 * D[3, \\
& 3](f)(r, s, t, a, b) + 2 * D[4, 4](f)(r, s, t, a, b) * \\
& D[3](f)(r, s, t, a, b) * D[3, 3](f)(r, s, t, a, b) - D[5, 5](f)(r, s, t, a, b) * D[4](f)(r, s, t, \\
& a, b) * D[3, 5](f)(r, s, t, a, b) * D[2](f)(r, s, t, a, b) - \\
& 2 * D[3, 5](f)(r, s, t, a, b) * D[3, 4](f)(r, s, t, a, b) * D[2](f)(r, s, t, a, b) - 4 \\
& * D[3](f)(r, s, t, a, b) * \\
& D[3, 4](f)(r, s, t, a, b) * D[2, 5](f)(r, s, t, a, b) + 2 * D[4](f)(r, s, t, a, b) * D[3, \\
& 3](f)(r, s, t, a, b) * D[2, 5](f)(r, s, t, a, b) - 2 * D[3](f)(r, s, t, a, b) * \\
& D[2, 5](f)(r, s, t, a, b)^2 + 8 * D[3](f)(r, s, t, a, b) * D[3, 5](f)(r, s, t, a, b) * D[2, \\
& 4](f)(r, s, t, a, b) - 2 * D[4](f)(r, s, t, a, b) * \\
& D[3, 5](f)(r, s, t, a, b) * D[2, 3](f)(r, s, t, a, b) - 2 * D[5, 5](f)(r, s, t, a, b) \\
& * D[2](f)(r, s, t, a, b) * D[2, 3](f)(r, s, t, a, b) - 2 * D[2, 3](f)(r, s, t, a, b)^2 + \\
& 2 * D[4, 5](f)(r, s, t, a, b) * (2 * D[4](f)(r, s, t, a, b) * D[3](f)(r, s, t, a, b) * D[3, \\
& 5](f)(r, s, t, a, b) + D[3, 3](f)(r, s, t, a, b) * \\
& D[2](f)(r, s, t, a, b) - 2 * D[3](f)(r, s, t, a, b) * D[2, 3](f)(r, s, t, a, b)) + 2 * D[5, \\
& 5](f)(r, s, t, a, b) * \\
& D[3](f)(r, s, t, a, b) * D[2, 2](f)(r, s, t, a, b) + 2 * D[3, 3](f)(r, s, t, a, b) * D[2, \\
& 2](f)(r, s, t, a, b) + 2 * D[3, 5](f)(r, s, t, a, b)^2 * \\
& D[1](f)(r, s, t, a, b) + 2 * D[5, 5](f)(r, s, t, a, b) * D[3, 3](f)(r, s, t, a, b) * D[1](f)(r, \\
& s, t, a, b) + 4 * D[3](f)(r, s, t, a, b) * \\
& D[3, 5](f)(r, s, t, a, b) * D[1, 5](f)(r, s, t, a, b) + D[5](f)(r, s, t, a, b) * (4 * D[4, \\
& 4](f)(r, s, t, a, b) * D[3](f)(r, s, t, a, b) * \\
& D[3, 5](f)(r, s, t, a, b) - D[5, 5](f)(r, s, t, a, b) * D[3, 4](f)(r, s, t, a, b) * D[2](f)(r, s, \\
& t, a, b) - 4 * D[4, 5](f)(r, s, t, a, b) * \\
& D[3](f)(r, s, t, a, b) * (D[3, 4](f)(r, s, t, a, b) + D[2, 5](f)(r, s, t, a, b)) + 4 * D[5, \\
& 5](f)(r, s, t, a, b) * D[3](f)(r, s, t, a, b) * \\
& D[2, 4](f)(r, s, t, a, b) - D[5, 5](f)(r, s, t, a, b) * D[4](f)(r, s, t, a, b) * D[2, 3](f)(r, s, \\
& t, a, b) + 2 * D[5, 5](f)(r, s, t, a, b) * \\
& D[3, 5](f)(r, s, t, a, b) * D[1](f)(r, s, t, a, b) - 2 * D[3, 3](f)(r, s, t, a, b) * D[1, \\
& 5](f)(r, s, t, a, b) + 2 * D[3, 5](f)(r, s, t, a, b) * \\
& D[1, 3](f)(r, s, t, a, b)) + D[5](f)(r, s, t, a, b)^2 * (-2 * D[4, 5](f)(r, s, t, a, b)^2 \\
& * D[3](f)(r, s, t, a, b) + D[5, 5](f)(r, s, t, a, b) * \\
& (2 * D[4, 4](f)(r, s, t, a, b) * D[3](f)(r, s, t, a, b) + D[1, 3](f)(r, s, t, a, b))) / \\
& (D[4](f)(r, s, t, a, b)^2 * D[3](f)(r, s, t, a, b) - D[5](f)(r, s, t, a, b) * D[4](f)(r, s, t, a, \\
& b) * D[2](f)(r, s, t, a, b) - \\
& D[2](f)(r, s, t, a, b)^2 + (D[5](f)(r, s, t, a, b)^2 + 4 * D[3](f)(r, s, t, a, b)) \\
& * D[1](f)(r, s, t, a, b)), \\
& D[4, 4, 4](f)(r, s, t, a, b) = \\
& (-2 * D[4](f)(r, s, t, a, b)^3 * (D[4, 5](f)(r, s, t, a, b)^2 - D[5, 5](f)(r, s, t, a, b) \\
& * D[4, 4](f)(r, s, t, a, b)) - 2 * D[4, 4](f)(r, s, t, a, b) * \\
& D[2](f)(r, s, t, a, b) * D[2, 4](f)(r, s, t, a, b) + 4 * D[4, 4](f)(r, s, t, a, b) * D[3, \\
& 4](f)(r, s, t, a, b) * D[1](f)(r, s, t, a, b) + 4 * D[4, 4](f)(r, s, t, a, b) * \\
& D[2, 5](f)(r, s, t, a, b) * D[1](f)(r, s, t, a, b) - 4 * D[4, 5](f)(r, s, t, a, b) * D[2, \\
& 4](f)(r, s, t, a, b) * D[1](f)(r, s, t, a, b) - 2 * D[4, 4](f)(r, s, t, a, b) * \\
& D[2](f)(r, s, t, a, b) * D[1, 5](f)(r, s, t, a, b) - 4 * D[4, 5](f)(r, s, t, a, b) * D[1](f)(r, \\
& s, t, a, b) * D[1, 5](f)(r, s, t, a, b) + D[5](f)(r, s, t, a, b)^2 * \\
& D[4, 4](f)(r, s, t, a, b) * D[1, 4](f)(r, s, t, a, b) + 4 * D[4, 4](f)(r, s, t, a, b) \\
& * D[3](f)(r, s, t, a, b) * D[1, 4](f)(r, s, t, a, b) + 2 * D[4, 5](f)(r, s, t, a, b) *
\end{aligned}$$

$$\begin{aligned}
& D[2](f)(r, s, t, a, b) * D[1, 4](f)(r, s, t, a, b) + 4 * D[2, 2](f)(r, s, t, a, b) * D[1, \\
& 4](f)(r, s, t, a, b) + 4 * D[5, 5](f)(r, s, t, a, b) * \\
& D[1](f)(r, s, t, a, b) * D[1, 4](f)(r, s, t, a, b) + D[4](f)(r, s, t, a, b)^2 * (D[4, 4](f)(r, \\
& s, t, a, b) * (D[3, 4](f)(r, s, t, a, b) + \\
& 4 * D[2, 5](f)(r, s, t, a, b)) - 4 * (D[4, 5](f)(r, s, t, a, b) * (D[2, 4](f)(r, s, t, a, b) \\
& + D[1, 5](f)(r, s, t, a, b)) - D[5, 5](f)(r, s, t, a, b) * \\
& D[1, 4](f)(r, s, t, a, b))) - 4 * D[1, 4](f)(r, s, t, a, b) * D[1, 3](f)(r, s, t, a, b) - 4 \\
& * D[2, 4](f)(r, s, t, a, b) * D[1, 2](f)(r, s, t, a, b) - \\
& 4 * D[1, 5](f)(r, s, t, a, b) * D[1, 2](f)(r, s, t, a, b) + 4 * D[3, 4](f)(r, s, t, a, b) * D[1, \\
& 1](f)(r, s, t, a, b) + 4 * D[2, 5](f)(r, s, t, a, b) * \\
& D[1, 1](f)(r, s, t, a, b) + D[5](f)(r, s, t, a, b) * (- (D[4, 4](f)(r, s, t, a, b)^2 \\
& * D[2](f)(r, s, t, a, b)) + 2 * D[2, 4](f)(r, s, t, a, b) * \\
& D[1, 4](f)(r, s, t, a, b) - 4 * D[1, 5](f)(r, s, t, a, b) * D[1, 4](f)(r, s, t, a, b) + 2 * D[4, \\
& 4](f)(r, s, t, a, b) * (D[4, 5](f)(r, s, t, a, b) * \\
& D[1](f)(r, s, t, a, b) - D[1, 2](f)(r, s, t, a, b)) + 4 * D[4, 5](f)(r, s, t, a, b) * D[1, \\
& 1](f)(r, s, t, a, b)) + D[4](f)(r, s, t, a, b) * \\
& (2 * D[4, 4](f)(r, s, t, a, b)^2 * D[3](f)(r, s, t, a, b) - D[4, 4](f)(r, s, t, a, b) * (D[4, \\
& 5](f)(r, s, t, a, b) * D[2](f)(r, s, t, a, b) + \\
& D[5](f)(r, s, t, a, b) * (D[2, 4](f)(r, s, t, a, b) + 4 * D[1, 5](f)(r, s, t, a, b)) - 2 * (D[2, \\
& 2](f)(r, s, t, a, b) + 2 * D[5, 5](f)(r, s, t, a, b) * \\
& D[1](f)(r, s, t, a, b) - D[1, 3](f)(r, s, t, a, b))) - 2 * (D[2, 4](f)(r, s, t, a, b)^2 + 2 \\
& * D[4, 5](f)(r, s, t, a, b)^2 * D[1](f)(r, s, t, a, b) + \\
& 2 * D[2, 4](f)(r, s, t, a, b) * D[1, 5](f)(r, s, t, a, b) + D[1, 5](f)(r, s, t, a, b)^2 - D[3, \\
& 4](f)(r, s, t, a, b) * D[1, 4](f)(r, s, t, a, b) - \\
& 4 * D[2, 5](f)(r, s, t, a, b) * D[1, 4](f)(r, s, t, a, b) + D[4, 5](f)(r, s, t, a, b) * (-2 \\
& * D[5](f)(r, s, t, a, b) * D[1, 4](f)(r, s, t, a, b) + \\
& 2 * D[1, 2](f)(r, s, t, a, b)) - D[5, 5](f)(r, s, t, a, b) * D[1, 1](f)(r, s, t, a, b))) / \\
& (D[4](f)(r, s, t, a, b)^2 * D[3](f)(r, s, t, a, b) - D[5](f)(r, s, t, a, b) * D[4](f)(r, s, t, a, \\
& b) * D[2](f)(r, s, t, a, b) - \\
& D[2](f)(r, s, t, a, b)^2 + (D[5](f)(r, s, t, a, b)^2 + 4 * D[3](f)(r, s, t, a, b)) \\
& * D[1](f)(r, s, t, a, b)), \\
& D[4, 4, 5](f)(r, s, t, a, b) = \\
& (D[4](f)(r, s, t, a, b)^2 * (3 * D[4, 4](f)(r, s, t, a, b) * D[3, 5](f)(r, s, t, a, b) - 2 * D[4, \\
& 5](f)(r, s, t, a, b) * D[3, 4](f)(r, s, t, a, b)) - \\
& 2 * D[4, 5](f)(r, s, t, a, b) * D[2](f)(r, s, t, a, b) * D[2, 4](f)(r, s, t, a, b) + 4 * D[4, \\
& 4](f)(r, s, t, a, b) * \\
& D[3, 5](f)(r, s, t, a, b) * D[1](f)(r, s, t, a, b) - 2 * D[4, 5](f)(r, s, t, a, b) * D[2](f)(r, \\
& s, t, a, b) * D[1, 5](f)(r, s, t, a, b) + 4 * D[4, 5](f)(r, s, t, a, b) * \\
& D[3](f)(r, s, t, a, b) * D[1, 4](f)(r, s, t, a, b) + 2 * D[5, 5](f)(r, s, t, a, b) * D[2](f)(r, \\
& s, t, a, b) * D[1, 4](f)(r, s, t, a, b) + 4 * D[2, 3](f)(r, s, t, a, b) * \\
& D[1, 4](f)(r, s, t, a, b) + D[5](f)(r, s, t, a, b)^2 * (- (D[4, 4](f)(r, s, t, a, b) * D[1, \\
& 5](f)(r, s, t, a, b)) + 2 * D[4, 5](f)(r, s, t, a, b) * \\
& D[1, 4](f)(r, s, t, a, b)) + D[4](f)(r, s, t, a, b) * (-2 * D[4, 5](f)(r, s, t, a, b)^2 \\
& * D[2](f)(r, s, t, a, b) + D[5, 5](f)(r, s, t, a, b) * \\
& D[4, 4](f)(r, s, t, a, b) * D[2](f)(r, s, t, a, b) - 2 * D[3, 4](f)(r, s, t, a, b) * D[2, \\
& 4](f)(r, s, t, a, b) + 2 * D[4, 4](f)(r, s, t, a, b) * D[2, 3](f)(r, s, t, a, b) - \\
& 2 * D[3, 4](f)(r, s, t, a, b) * D[1, 5](f)(r, s, t, a, b) + 6 * D[3, 5](f)(r, s, t, a, b) * D[1, \\
& 4](f)(r, s, t, a, b) + 2 * D[4, 5](f)(r, s, t, a, b) *
\end{aligned}$$

$$\begin{aligned}
& (D[4, 4](f)(r, s, t, a, b) * D[3](f)(r, s, t, a, b) - 2 * D[1, 3](f)(r, s, t, a, b))) - 4 * D[2, \\
& 4](f)(r, s, t, a, b) * D[1, 3](f)(r, s, t, a, b) - \\
& 4 * D[1, 5](f)(r, s, t, a, b) * D[1, 3](f)(r, s, t, a, b) + 4 * D[3, 5](f)(r, s, t, a, b) * D[1, \\
& 1](f)(r, s, t, a, b) + D[5](f)(r, s, t, a, b) * \\
& (-2 * D[4](f)(r, s, t, a, b)^2 * (D[4, 5](f)(r, s, t, a, b)^2 - D[5, 5](f)(r, s, t, a, b) \\
& * D[4, 4](f)(r, s, t, a, b)) - D[4, 5](f)(r, s, t, a, b) * \\
& D[4, 4](f)(r, s, t, a, b) * D[2](f)(r, s, t, a, b) + D[4](f)(r, s, t, a, b) * (D[4, 4](f)(r, s, \\
& t, a, b) * D[2, 5](f)(r, s, t, a, b) - 2 * D[4, 5](f)(r, s, t, a, b) * \\
& (D[2, 4](f)(r, s, t, a, b) + 2 * D[1, 5](f)(r, s, t, a, b))) + 4 * D[5, 5](f)(r, s, t, a, b) \\
& * D[1, 4](f)(r, s, t, a, b)) + 2 * (- (D[2, 4](f)(r, s, t, a, b) * \\
& D[1, 5](f)(r, s, t, a, b)) - D[1, 5](f)(r, s, t, a, b)^2 + D[3, 4](f)(r, s, t, a, b) * D[1, \\
& 4](f)(r, s, t, a, b) + D[2, 5](f)(r, s, t, a, b) * \\
& D[1, 4](f)(r, s, t, a, b) - D[4, 4](f)(r, s, t, a, b) * D[1, 3](f)(r, s, t, a, b) + D[5, \\
& 5](f)(r, s, t, a, b) * (D[4, 4](f)(r, s, t, a, b) * \\
& D[1](f)(r, s, t, a, b) + D[1, 1](f)(r, s, t, a, b)))) / \\
& (D[4](f)(r, s, t, a, b)^2 * D[3](f)(r, s, t, a, b) - D[5](f)(r, s, t, a, b) * D[4](f)(r, s, t, a, \\
& b) * D[2](f)(r, s, t, a, b) - \\
& D[2](f)(r, s, t, a, b)^2 + (D[5](f)(r, s, t, a, b)^2 + 4 * D[3](f)(r, s, t, a, b)) \\
& * D[1](f)(r, s, t, a, b)), \\
& D[4, 5, 5](f)(r, s, t, a, b) = \\
& (D[5](f)(r, s, t, a, b)^2 * (-2 * D[4](f)(r, s, t, a, b) * (D[4, 5](f)(r, s, t, a, b)^2 - D[5, \\
& 5](f)(r, s, t, a, b) * D[4, 4](f)(r, s, t, a, b)) - \\
& 2 * D[4, 5](f)(r, s, t, a, b) * D[1, 5](f)(r, s, t, a, b) + 3 * D[5, 5](f)(r, s, t, a, b) * D[1, \\
& 4](f)(r, s, t, a, b)) - D[5, 5](f)(r, s, t, a, b) * \\
& (D[4](f)(r, s, t, a, b)^2 * D[3, 4](f)(r, s, t, a, b) - 4 * D[3](f)(r, s, t, a, b) * D[1, \\
& 4](f)(r, s, t, a, b) + D[4](f)(r, s, t, a, b) * \\
& (-2 * D[4, 4](f)(r, s, t, a, b) * D[3](f)(r, s, t, a, b) + D[4, 5](f)(r, s, t, a, b) \\
& * D[2](f)(r, s, t, a, b) + 2 * D[1, 3](f)(r, s, t, a, b))) + \\
& D[5](f)(r, s, t, a, b) * (-2 * D[4, 5](f)(r, s, t, a, b)^2 * D[2](f)(r, s, t, a, b) + D[5, \\
& 5](f)(r, s, t, a, b) * D[4, 4](f)(r, s, t, a, b) * \\
& D[2](f)(r, s, t, a, b) + D[4](f)(r, s, t, a, b) * (4 * D[4, 4](f)(r, s, t, a, b) * D[3, \\
& 5](f)(r, s, t, a, b) - 2 * D[4, 5](f)(r, s, t, a, b) * \\
& (2 * D[3, 4](f)(r, s, t, a, b) + D[2, 5](f)(r, s, t, a, b)) + D[5, 5](f)(r, s, t, a, b) * D[2, \\
& 4](f)(r, s, t, a, b)) + \\
& 2 * D[5, 5](f)(r, s, t, a, b) * D[4, 5](f)(r, s, t, a, b) * D[1](f)(r, s, t, a, b) - 2 * D[3, \\
& 4](f)(r, s, t, a, b) * D[1, 5](f)(r, s, t, a, b) - \\
& 2 * D[2, 5](f)(r, s, t, a, b) * D[1, 5](f)(r, s, t, a, b) + 6 * D[3, 5](f)(r, s, t, a, b) * D[1, \\
& 4](f)(r, s, t, a, b) - 4 * D[4, 5](f)(r, s, t, a, b) * \\
& D[1, 3](f)(r, s, t, a, b) + 2 * D[5, 5](f)(r, s, t, a, b) * D[1, 2](f)(r, s, t, a, b)) + 2 \\
& * (D[4](f)(r, s, t, a, b)^2 * D[4, 5](f)(r, s, t, a, b) * \\
& D[3, 5](f)(r, s, t, a, b) + D[4, 4](f)(r, s, t, a, b) * D[3, 5](f)(r, s, t, a, b) * D[2](f)(r, \\
& s, t, a, b) - D[4, 5](f)(r, s, t, a, b) * \\
& D[3, 4](f)(r, s, t, a, b) * D[2](f)(r, s, t, a, b) - D[4, 5](f)(r, s, t, a, b) * D[2](f)(r, s, t, \\
& a, b) * D[2, 5](f)(r, s, t, a, b) + \\
& 2 * D[4, 5](f)(r, s, t, a, b) * D[3, 5](f)(r, s, t, a, b) * D[1](f)(r, s, t, a, b) + D[4](f)(r, \\
& s, t, a, b) * (-D[3, 4](f)(r, s, t, a, b)^2 + \\
& D[4, 4](f)(r, s, t, a, b) * D[3, 3](f)(r, s, t, a, b) - D[3, 4](f)(r, s, t, a, b) * D[2, \\
& 5](f)(r, s, t, a, b) + D[3, 5](f)(r, s, t, a, b) *
\end{aligned}$$

$$\begin{aligned}
& (D[2, 4](f)(r, s, t, a, b) + D[1, 5](f)(r, s, t, a, b)) + 2 * D[3, 3](f)(r, s, t, a, b) * D[1, \\
& 4](f)(r, s, t, a, b) - 2 * D[3, 4](f)(r, s, t, a, b) * \\
& D[1, 3](f)(r, s, t, a, b) - 2 * D[2, 5](f)(r, s, t, a, b) * D[1, 3](f)(r, s, t, a, b) + 2 * D[3, \\
& 5](f)(r, s, t, a, b) * D[1, 2](f)(r, s, t, a, b)) / \\
& (D[4](f)(r, s, t, a, b)^2 * D[3](f)(r, s, t, a, b) - D[5](f)(r, s, t, a, b) * D[4](f)(r, s, t, a, \\
& b) * D[2](f)(r, s, t, a, b) - \\
& D[2](f)(r, s, t, a, b)^2 + (D[5](f)(r, s, t, a, b)^2 + 4 * D[3](f)(r, s, t, a, b)) \\
& * D[1](f)(r, s, t, a, b)), \\
D[5, 5, 5](f)(r, s, t, a, b) = \\
& (-2 * D[5](f)(r, s, t, a, b)^3 * (D[4, 5](f)(r, s, t, a, b)^2 - D[5, 5](f)(r, s, t, a, b) \\
& * D[4, 4](f)(r, s, t, a, b)) - \\
& D[5, 5](f)(r, s, t, a, b)^2 * D[4](f)(r, s, t, a, b) * D[2](f)(r, s, t, a, b) + D[5, 5](f)(r, \\
& s, t, a, b) * (D[4](f)(r, s, t, a, b)^2 * D[3, 5](f)(r, s, t, a, b) - \\
& 2 * D[3, 4](f)(r, s, t, a, b) * D[2](f)(r, s, t, a, b) - 2 * D[2](f)(r, s, t, a, b) * D[2, \\
& 5](f)(r, s, t, a, b) + 4 * D[3](f)(r, s, t, a, b) * D[2, 4](f)(r, s, t, a, b) + \\
& 2 * D[4](f)(r, s, t, a, b) * (D[4, 5](f)(r, s, t, a, b) * D[3](f)(r, s, t, a, b) - D[2, 3](f)(r, \\
& s, t, a, b)) + 4 * D[3, 5](f)(r, s, t, a, b) * \\
& D[1](f)(r, s, t, a, b) + 4 * D[3](f)(r, s, t, a, b) * D[1, 5](f)(r, s, t, a, b)) + D[5](f)(r, \\
& s, t, a, b)^2 * (4 * D[4, 4](f)(r, s, t, a, b) * \\
& D[3, 5](f)(r, s, t, a, b) - 4 * D[4, 5](f)(r, s, t, a, b) * (D[3, 4](f)(r, s, t, a, b) + D[2, \\
& 5](f)(r, s, t, a, b)) + D[5, 5](f)(r, s, t, a, b) * \\
& (4 * D[2, 4](f)(r, s, t, a, b) + D[1, 5](f)(r, s, t, a, b))) + 2 * (2 * D[4, 4](f)(r, s, t, a, b) \\
& * D[3](f)(r, s, t, a, b) * D[3, 5](f)(r, s, t, a, b) - \\
& 2 * D[4](f)(r, s, t, a, b) * D[3, 5](f)(r, s, t, a, b) * D[3, 4](f)(r, s, t, a, b) + D[4](f)(r, \\
& s, t, a, b) * D[3, 5](f)(r, s, t, a, b) * \\
& D[2, 5](f)(r, s, t, a, b) + D[4, 5](f)(r, s, t, a, b) * (2 * D[4](f)(r, s, t, a, b) * D[3, \\
& 3](f)(r, s, t, a, b) + D[3, 5](f)(r, s, t, a, b) * \\
& D[2](f)(r, s, t, a, b) - 2 * D[3](f)(r, s, t, a, b) * (D[3, 4](f)(r, s, t, a, b) + D[2, \\
& 5](f)(r, s, t, a, b))) + 2 * D[3, 3](f)(r, s, t, a, b) * \\
& D[2, 4](f)(r, s, t, a, b) - 2 * D[3, 4](f)(r, s, t, a, b) * D[2, 3](f)(r, s, t, a, b) - 2 * D[2, \\
& 5](f)(r, s, t, a, b) * D[2, 3](f)(r, s, t, a, b) + \\
& 2 * D[3, 5](f)(r, s, t, a, b) * D[2, 2](f)(r, s, t, a, b) + 2 * D[3, 3](f)(r, s, t, a, b) * D[1, \\
& 5](f)(r, s, t, a, b) - 2 * D[3, 5](f)(r, s, t, a, b) * \\
& D[1, 3](f)(r, s, t, a, b)) - D[5](f)(r, s, t, a, b) * (4 * D[4, 5](f)(r, s, t, a, b)^2 \\
& * D[3](f)(r, s, t, a, b) + D[4, 5](f)(r, s, t, a, b) * \\
& (-4 * D[4](f)(r, s, t, a, b) * D[3, 5](f)(r, s, t, a, b) + D[5, 5](f)(r, s, t, a, b) \\
& * D[2](f)(r, s, t, a, b) + 4 * D[2, 3](f)(r, s, t, a, b)) - \\
& 2 * D[5, 5](f)(r, s, t, a, b)^2 * D[1](f)(r, s, t, a, b) + 2 * (D[3, 4](f)(r, s, t, a, b)^2 \\
& - D[4, 4](f)(r, s, t, a, b) * D[3, 3](f)(r, s, t, a, b) + \\
& 2 * D[3, 4](f)(r, s, t, a, b) * D[2, 5](f)(r, s, t, a, b) + D[2, 5](f)(r, s, t, a, b)^2 - 4 \\
& * D[3, 5](f)(r, s, t, a, b) * D[2, 4](f)(r, s, t, a, b) - \\
& D[3, 5](f)(r, s, t, a, b) * D[1, 5](f)(r, s, t, a, b)) + D[5, 5](f)(r, s, t, a, b) * (-4 * D[4, \\
& 4](f)(r, s, t, a, b) * D[3](f)(r, s, t, a, b) + \\
& D[4](f)(r, s, t, a, b) * (4 * D[3, 4](f)(r, s, t, a, b) + D[2, 5](f)(r, s, t, a, b)) - 2 * D[2, \\
& 2](f)(r, s, t, a, b) + 2 * D[1, 3](f)(r, s, t, a, b))) / \\
& (D[4](f)(r, s, t, a, b)^2 * D[3](f)(r, s, t, a, b) - D[5](f)(r, s, t, a, b) * D[4](f)(r, s, t, a, \\
& b) * D[2](f)(r, s, t, a, b) - \\
& D[2](f)(r, s, t, a, b)^2 + (D[5](f)(r, s, t, a, b)^2 + 4 * D[3](f)(r, s, t, a, b))
\end{aligned}$$

[ \*D[1](f) (r, s, t, a, b) ) } :

[ Ready? Go:

$$\begin{aligned} & \text{> simplify(subs(convert(IC, diff), Rest1))} \\ & \quad \quad \quad 0 \end{aligned} \quad (14)$$

$$\begin{aligned} & \text{> simplify(subs(convert(IC, diff), subs([u_{2,2}=r, u_{2,3}=s, u_{3,3}=t, u_{1,2}=a, u_{1,3}=b], Eq1)))} \\ & \quad \quad \quad 0 \end{aligned} \quad (15)$$

$$\begin{aligned} & \text{> simplify(subs(convert(IC, diff), subs([u_{2,2}=r, u_{2,3}=s, u_{3,3}=t, u_{1,2}=a, u_{1,3}=b], Eq2)))} \\ & \quad \quad \quad 0 \end{aligned} \quad (16)$$

$$\begin{aligned} & \text{> simplify(subs(convert(IC, diff), subs([u_{2,2}=r, u_{2,3}=s, u_{3,3}=t, u_{1,2}=a, u_{1,3}=b], Eq3)))} \\ & \quad \quad \quad 0 \end{aligned} \quad (17)$$

$$\begin{aligned} & \text{> simplify(subs(convert(IC, diff), subs([u_{2,2}=r, u_{2,3}=s, u_{3,3}=t, u_{1,2}=a, u_{1,3}=b], Eq4)))} \\ & \quad \quad \quad 0 \end{aligned} \quad (18)$$

$$\begin{aligned} & \text{> simplify(subs(convert(IC, diff), subs([u_{2,2}=r, u_{2,3}=s, u_{3,3}=t, u_{1,2}=a, u_{1,3}=b], Eq5)))} \\ & \quad \quad \quad 0 \end{aligned} \quad (19)$$

[ Hurrah! Hurrah! Hurrah!

[ Thus we see that IC is a solution to all equations Eq\_i, which can be considered (count the amount of all coefficients of the quadratic terms in 3-jets:  $5 \cdot \text{Binomial}(7+1,2)=5 \cdot 28=140$ ) as a system of 140 (algebraic-differential but formally only algebraic on jets, while for the highest jets they are) linear (inhomogeneous) equations on 35 unknowns (derivatives of f by (u\_xx, u\_xy, u\_yy, u\_tx, u\_ty) of order 3).

[ To check this solution is unique we have to prove that the matrix of the coefficients has rank 35. The coefficients are polynomials of 1-jets of f, so calculating the rank of 140x35 matrix over polynomials in 5 variables can be cumbersome. In fact, all of the coefficients have the common factor  $\Delta^3$  ( $\Delta$  appears in the denominator of the IC), so we can cancel it and get 140\*35 quite simple expressions.

[ Below we write several versions of the substitutions, which are due to various hiding procedures. On one run I used alias command from the beginning, on the other I forgot to do it, so the simplification did not want to cancel the identical expressions  $\Delta^3$  (in fact they were identical only in the visible output; in the machine representation it remembered all the data which looked differently - see several changes: various writing D vs diff, u\_ij vs (r,s,t,a,b) etc). In any case one of these expressions work and it allows to have nice cancellation and the output - 140x35 polynomial matrix.

$$\text{> Ch} := \{D[1](f) (r, s, t, a, b) = \text{diff}(f(r, s, t, a, b), r), D[2](f) (r, s, t, a, b) = \text{diff}(f(r, s, t, a,$$

$$\begin{aligned}
& b), s), D[3](f)(r, s, t, a, b) = \text{diff}(f(r, s, t, a, b), t), D[4](f)(r, s, t, a, b) = \text{diff}(f(r, s, t, \\
& a, b), a), D[5](f)(r, s, t, a, b) = \text{diff}(f(r, s, t, a, b), b), \\
& D[1, 1](f)(r, s, t, a, b) = \text{diff}(f(r, s, t, a, b), r, r), D[1, 2](f)(r, s, t, a, b) = \text{diff}(f(r, s, t, a, \\
& b), r, s), D[1, 3](f)(r, s, t, a, b) = \text{diff}(f(r, s, t, a, b), r, t), D[1, 4](f)(r, s, t, a, b) \\
& = \text{diff}(f(r, s, t, a, b), r, a), D[1, 5](f)(r, s, t, a, b) = \text{diff}(f(r, s, t, a, b), r, b), D[2, \\
& 2](f)(r, s, t, a, b) = \text{diff}(f(r, s, t, a, b), s, s), D[2, 3](f)(r, s, t, a, b) = \text{diff}(f(r, s, t, a, b), \\
& s, t), D[2, 4](f)(r, s, t, a, b) = \text{diff}(f(r, s, t, a, b), s, a), D[2, 5](f)(r, s, t, a, b) \\
& = \text{diff}(f(r, s, t, a, b), s, b), D[3, 3](f)(r, s, t, a, b) = \text{diff}(f(r, s, t, a, b), t, t), D[3, \\
& 4](f)(r, s, t, a, b) = \text{diff}(f(r, s, t, a, b), t, a), D[3, 5](f)(r, s, t, a, b) = \text{diff}(f(r, s, t, a, \\
& b), t, b), D[4, 4](f)(r, s, t, a, b) = \text{diff}(f(r, s, t, a, b), a, a), D[4, 5](f)(r, s, t, a, b) \\
& = \text{diff}(f(r, s, t, a, b), a, b), D[5, 5](f)(r, s, t, a, b) = \text{diff}(f(r, s, t, a, b), b, b), \\
& D[1, 1, 1](f)(r, s, t, a, b) = \text{diff}(f(r, s, t, a, b), r, r, r), D[1, 1, 2](f)(r, s, t, a, b) = \text{diff}(f(r, \\
& s, t, a, b), r, r, s), D[1, 1, 3](f)(r, s, t, a, b) = \text{diff}(f(r, s, t, a, b), r, r, t), D[1, 1, 4](f)(r, \\
& s, t, a, b) = \text{diff}(f(r, s, t, a, b), r, r, a), D[1, 1, 5](f)(r, s, t, a, b) = \text{diff}(f(r, s, t, a, b), r, r, \\
& b), D[1, 2, 2](f)(r, s, t, a, b) = \text{diff}(f(r, s, t, a, b), r, s, s), D[1, 2, 3](f)(r, s, t, a, b) \\
& = \text{diff}(f(r, s, t, a, b), r, s, t), D[1, 2, 4](f)(r, s, t, a, b) = \text{diff}(f(r, s, t, a, b), r, s, a), D[1, \\
& 2, 5](f)(r, s, t, a, b) = \text{diff}(f(r, s, t, a, b), r, s, b), D[1, 3, 3](f)(r, s, t, a, b) = \text{diff}(f(r, s, \\
& t, a, b), r, t, t), D[1, 3, 4](f)(r, s, t, a, b) = \text{diff}(f(r, s, t, a, b), r, t, a), D[1, 3, 5](f)(r, s, \\
& t, a, b) = \text{diff}(f(r, s, t, a, b), r, t, b), D[1, 4, 4](f)(r, s, t, a, b) = \text{diff}(f(r, s, t, a, b), r, a, \\
& a), D[1, 4, 5](f)(r, s, t, a, b) = \text{diff}(f(r, s, t, a, b), r, a, b), D[1, 5, 5](f)(r, s, t, a, b) \\
& = \text{diff}(f(r, s, t, a, b), r, b, b), D[2, 2, 2](f)(r, s, t, a, b) = \text{diff}(f(r, s, t, a, b), s, s, s), D[2, \\
& 2, 3](f)(r, s, t, a, b) = \text{diff}(f(r, s, t, a, b), s, s, t), D[2, 2, 4](f)(r, s, t, a, b) = \text{diff}(f(r, s, \\
& t, a, b), s, s, a), D[2, 2, 5](f)(r, s, t, a, b) = \text{diff}(f(r, s, t, a, b), s, s, b), D[2, 3, 3](f)(r, s, \\
& t, a, b) = \text{diff}(f(r, s, t, a, b), s, t, t), D[2, 3, 4](f)(r, s, t, a, b) = \text{diff}(f(r, s, t, a, b), s, t, a), \\
& D[2, 3, 5](f)(r, s, t, a, b) = \text{diff}(f(r, s, t, a, b), s, t, b), D[2, 4, 4](f)(r, s, t, a, b) \\
& = \text{diff}(f(r, s, t, a, b), s, a, a), D[2, 4, 5](f)(r, s, t, a, b) = \text{diff}(f(r, s, t, a, b), s, a, b), \\
& D[2, 5, 5](f)(r, s, t, a, b) = \text{diff}(f(r, s, t, a, b), s, b, b), D[3, 3, 3](f)(r, s, t, a, b) \\
& = \text{diff}(f(r, s, t, a, b), t, t, t), D[3, 3, 4](f)(r, s, t, a, b) = \text{diff}(f(r, s, t, a, b), t, t, a), D[3, \\
& 3, 5](f)(r, s, t, a, b) = \text{diff}(f(r, s, t, a, b), t, t, b), D[3, 4, 4](f)(r, s, t, a, b) = \text{diff}(f(r, s, \\
& t, a, b), t, a, a), D[3, 4, 5](f)(r, s, t, a, b) = \text{diff}(f(r, s, t, a, b), t, a, b), D[3, 5, 5](f)(r, s, \\
& t, a, b) = \text{diff}(f(r, s, t, a, b), t, b, b), D[4, 4, 4](f)(r, s, t, a, b) = \text{diff}(f(r, s, t, a, b), a, a, \\
& a), D[4, 4, 5](f)(r, s, t, a, b) = \text{diff}(f(r, s, t, a, b), a, a, b), D[4, 5, 5](f)(r, s, t, a, b) \\
& = \text{diff}(f(r, s, t, a, b), a, b, b), D[5, 5, 5](f)(r, s, t, a, b) = \text{diff}(f(r, s, t, a, b), b, b, b) \} :
\end{aligned}$$

**J2** > subs(Ch, IC[35])

$IC_{35}$

(20)

**J2** > [denom(rhs(subs(Ch, IC[31]))), denom(rhs(subs(Ch, IC[32]))),  
denom(rhs(subs(Ch, IC[33]))), denom(rhs(subs(Ch, IC[34])))]

$$\begin{aligned}
& [f_a^2 f_t - f_b f_a f_s - f_s^2 + f_r f_b^2 + 4 f_t f_r f_a^2 f_t - f_b f_a f_s - f_s^2 + f_r f_b^2 + 4 f_t f_r f_a^2 f_t - f_b f_a f_s - f_s^2 + f_r f_b^2 \\
& + 4 f_t f_r f_a^2 f_t - f_b f_a f_s - f_s^2 + f_r f_b^2 + 4 f_t f_r]
\end{aligned} \tag{21}$$

**J2** >  $\Delta := (f_s^2 + f_b f_a f_s - f_a^2 f_t - 4 f_t f_r - f_r f_b^2)^3$

$$\Delta := (f_s^2 + f_b f_a f_s - f_a^2 f_t - 4 f_t f_r - f_r f_b^2)^3$$

(22)

$$\begin{aligned}
\text{J2} > \Delta := \text{subs}\left([u_{2,2}=r, u_{2,3}=s, u_{3,3}=t, u_{1,2}=a, u_{1,3}=b], \right. \\
& \left( \text{diff}\left(f(u_{2,2}, u_{2,3}, u_{3,3}, u_{1,2}, u_{1,3}), u_{2,3}\right)^2 + \text{diff}\left(f(u_{2,2}, u_{2,3}, u_{3,3}, u_{1,2}, \right. \right. \\
& u_{1,3}), u_{1,3}) \cdot \text{diff}\left(f(u_{2,2}, u_{2,3}, u_{3,3}, u_{1,2}, u_{1,3}), u_{1,2}\right) \cdot \text{diff}\left(f(u_{2,2}, u_{2,3}, u_{3,3}, u_{1,2}, \right. \\
& u_{1,3}), u_{2,3}) - \text{diff}\left(f(u_{2,2}, u_{2,3}, u_{3,3}, u_{1,2}, u_{1,3}), u_{1,2}\right)^2 \cdot \text{diff}\left(f(u_{2,2}, u_{2,3}, u_{3,3}, \right. \\
& u_{1,2}, u_{1,3}), u_{3,3}) - 4 \text{diff}\left(f(u_{2,2}, u_{2,3}, u_{3,3}, u_{1,2}, u_{1,3}), u_{3,3}\right) \cdot \text{diff}\left(f(u_{2,2}, u_{2,3}, \right. \\
& u_{3,3}, u_{1,2}, u_{1,3}), u_{2,2}) - \text{diff}\left(f(u_{2,2}, u_{2,3}, u_{3,3}, u_{1,2}, u_{1,3}), u_{2,2}\right) \\
& \left. \cdot \text{diff}\left(f(u_{2,2}, u_{2,3}, u_{3,3}, u_{1,2}, u_{1,3}), u_{1,3}\right)^2 \right)^3 \\
& \Delta := (f_s^2 + f_b f_a f_s - f_a^2 f_t - 4 f_t f_r - f_r f_b^2)^3
\end{aligned} \tag{23}$$

$$\begin{aligned}
\text{J2} > \text{factor}\left(\frac{1}{\Delta} \text{coeff}(\text{Rest1}, \text{diff}(f(r, s, t, a, b), r, r, r))\right) \\
& 8 f_r f_t (f_s f_b - 2 f_a f_t)
\end{aligned} \tag{24}$$

$$\begin{aligned}
\text{J2} > \text{factor}\left(\frac{1}{\Delta} \text{coeff}(\text{Rest1}, \text{diff}(f(r, s, t, a, b), r, r, b))\right) \\
& -2 f_s f_r (4 f_t f_r - f_s^2)
\end{aligned} \tag{25}$$

$$\begin{aligned}
\text{J2} > \text{factor}\left(\frac{1}{\Delta} \text{coeff}(\text{Rest1}, \text{diff}(f(r, s, t, a, b), a, a, a))\right) \\
& -4 f_r^2 f_t (4 f_t f_r - f_s^2)
\end{aligned} \tag{26}$$

$$\begin{aligned}
\text{J2} > \text{factor}\left(\frac{1}{\Delta} \text{coeff}(\text{Rest1}, \text{diff}(f(r, s, t, a, b), a, a, b))\right) \\
& 2 f_r^2 f_s (4 f_t f_r - f_s^2)
\end{aligned} \tag{27}$$

$$\begin{aligned}
\text{J2} > \text{factor}\left(\text{coeff}\left(\text{subs}\left([u_{2,2}=r, u_{2,3}=s, u_{3,3}=t, u_{1,2}=a, u_{1,3}=b], \text{diff}(Eq1, u_{1,2,3}, \right. \right. \right. \\
& u_{1,2,3})), \text{diff}(f(r, s, t, a, b), b, b, b))\right) \\
\text{J2} > \text{factor}\left(\frac{1}{\Delta} \cdot \text{coeff}\left(\text{subs}\left([u_{2,2}=r, u_{2,3}=s, u_{3,3}=t, u_{1,2}=a, u_{1,3}=b], \text{diff}(Eq1, u_{1,2,3}, \right. \right. \right. \\
& u_{1,2,3})), \text{subs}\left([u_{2,2}=r, u_{2,3}=s, u_{3,3}=t, u_{1,2}=a, u_{1,3}=b], \text{diff}(f(u_{2,2}, u_{2,3}, \right. \\
& u_{3,3}, u_{1,2}, u_{1,3}), u_{1,3}, u_{1,3}, u_{1,3}))\right) \\
& 2 f_s f_r (f_s^2 - 4 f_t f_r)
\end{aligned} \tag{28}$$

$$\begin{aligned}
\text{J2} > \text{simplify}\left(\text{factor}\left(\frac{1}{\Delta} \text{coeff}\left(\text{subs}\left([u_{2,2}=r, u_{2,3}=s, u_{3,3}=t, u_{1,2}=a, u_{1,3}=b], \right. \right. \right. \\
& \left. \left. \text{diff}(Eq1, u_{1,2,3}, u_{1,2,3}), \text{diff}(f(r, s, t, a, b), b, b, b))\right)\right) \\
& 0
\end{aligned} \tag{29}$$

$$\text{J2} > \text{simplify}\left(\text{subs}\left([u_{1,2,2}=0, u_{1,2,3}=0, u_{1,3,3}=0, u_{2,2,2}=0, u_{2,2,3}=0, u_{2,3,3}=0, u_{3,3,3}=0, \right. \right.$$

$$= 0], \text{subs}([u_{2,2}=r, u_{2,3}=s, u_{3,3}=t, u_{1,2}=a, u_{1,3}=b], \text{diff}(Eq5, u_{3,3,3})) \quad 0 \quad (30)$$

$$\text{J2} > \text{simplify}(\text{subs}([u_{1,2,2}=0, u_{1,2,3}=0, u_{1,3,3}=0, u_{2,2,2}=0, u_{2,2,3}=0, u_{2,3,3}=0, u_{3,3,3}=0], \text{subs}([u_{2,2}=r, u_{2,3}=s, u_{3,3}=t, u_{1,2}=a, u_{1,3}=b], [Eq1, Eq2, Eq3, Eq4, Eq5]))) \quad [0, 0, 0, 0, 0] \quad (31)$$

Thus Yes, at this point we check that Eq\_s are purely quadratic in the 3-jets  $u_{ijk}$ , sorry for the improper place - this should be higher up...

Now let's go to the calculation of the huge matrix

$$\text{J2} > \text{Vara} := [\text{diff}(f(u_{2,2}, u_{2,3}, u_{3,3}, u_{1,2}, u_{1,3}), r, r, r), \text{diff}(f(u_{2,2}, u_{2,3}, u_{3,3}, u_{1,2}, u_{1,3}), r, r, s), \text{diff}(f(u_{2,2}, u_{2,3}, u_{3,3}, u_{1,2}, u_{1,3}), r, r, t), \text{diff}(f(u_{2,2}, u_{2,3}, u_{3,3}, u_{1,2}, u_{1,3}), r, r, a), \text{diff}(f(u_{2,2}, u_{2,3}, u_{3,3}, u_{1,2}, u_{1,3}), r, r, b), \text{diff}(f(u_{2,2}, u_{2,3}, u_{3,3}, u_{1,2}, u_{1,3}), r, s, s), \text{diff}(f(u_{2,2}, u_{2,3}, u_{3,3}, u_{1,2}, u_{1,3}), r, s, t), \text{diff}(f(u_{2,2}, u_{2,3}, u_{3,3}, u_{1,2}, u_{1,3}), r, s, a), \text{diff}(f(u_{2,2}, u_{2,3}, u_{3,3}, u_{1,2}, u_{1,3}), r, s, b), \text{diff}(f(u_{2,2}, u_{2,3}, u_{3,3}, u_{1,2}, u_{1,3}), r, t, t), \text{diff}(f(u_{2,2}, u_{2,3}, u_{3,3}, u_{1,2}, u_{1,3}), r, t, a), \text{diff}(f(u_{2,2}, u_{2,3}, u_{3,3}, u_{1,2}, u_{1,3}), r, t, b), \text{diff}(f(u_{2,2}, u_{2,3}, u_{3,3}, u_{1,2}, u_{1,3}), r, a, a), \text{diff}(f(u_{2,2}, u_{2,3}, u_{3,3}, u_{1,2}, u_{1,3}), r, a, b), \text{diff}(f(u_{2,2}, u_{2,3}, u_{3,3}, u_{1,2}, u_{1,3}), r, b, b), \text{diff}(f(u_{2,2}, u_{2,3}, u_{3,3}, u_{1,2}, u_{1,3}), s, s, s), \text{diff}(f(u_{2,2}, u_{2,3}, u_{3,3}, u_{1,2}, u_{1,3}), s, s, t), \text{diff}(f(u_{2,2}, u_{2,3}, u_{3,3}, u_{1,2}, u_{1,3}), s, s, a), \text{diff}(f(u_{2,2}, u_{2,3}, u_{3,3}, u_{1,2}, u_{1,3}), s, s, b), \text{diff}(f(u_{2,2}, u_{2,3}, u_{3,3}, u_{1,2}, u_{1,3}), s, t, t), \text{diff}(f(u_{2,2}, u_{2,3}, u_{3,3}, u_{1,2}, u_{1,3}), s, t, a), \text{diff}(f(u_{2,2}, u_{2,3}, u_{3,3}, u_{1,2}, u_{1,3}), s, t, b), \text{diff}(f(u_{2,2}, u_{2,3}, u_{3,3}, u_{1,2}, u_{1,3}), s, a, a), \text{diff}(f(u_{2,2}, u_{2,3}, u_{3,3}, u_{1,2}, u_{1,3}), s, a, b), \text{diff}(f(u_{2,2}, u_{2,3}, u_{3,3}, u_{1,2}, u_{1,3}), s, b, b), \text{diff}(f(u_{2,2}, u_{2,3}, u_{3,3}, u_{1,2}, u_{1,3}), t, t, t), \text{diff}(f(u_{2,2}, u_{2,3}, u_{3,3}, u_{1,2}, u_{1,3}), t, t, a), \text{diff}(f(u_{2,2}, u_{2,3}, u_{3,3}, u_{1,2}, u_{1,3}), t, t, b), \text{diff}(f(u_{2,2}, u_{2,3}, u_{3,3}, u_{1,2}, u_{1,3}), t, a, a), \text{diff}(f(u_{2,2}, u_{2,3}, u_{3,3}, u_{1,2}, u_{1,3}), t, a, b), \text{diff}(f(u_{2,2}, u_{2,3}, u_{3,3}, u_{1,2}, u_{1,3}), t, b, b), \text{diff}(f(u_{2,2}, u_{2,3}, u_{3,3}, u_{1,2}, u_{1,3}), a, a, a), \text{diff}(f(u_{2,2}, u_{2,3}, u_{3,3}, u_{1,2}, u_{1,3}), a, a, b), \text{diff}(f(r, s, t, a, b), a, b, b), \text{diff}(f(r, s, t, a, b), b, b, b)]:$$

$$\text{J2} > \text{Vara} := [\text{diff}(f(u[2,2], u[2,3], u[3,3], u[1,2], u[1,3]), u[2,2], u[2,2], u[2,2]), \text{diff}(f(u[2,2], u[2,3], u[3,3], u[1,2], u[1,3]), u[2,2], u[2,2], u[2,3]), \text{diff}(f(u[2,2], u[2,3], u[3,3], u[1,2], u[1,3]), u[2,2], u[2,2], u[3,3]), \text{diff}(f(u[2,2], u[2,3], u[3,3], u[1,2], u[1,3]), u[2,2], u[2,2], u[1,2]), \text{diff}(f(u[2,2], u[2,3], u[3,3], u[1,2], u[1,3]), u[2,2], u[2,2], u[1,3]), \text{diff}(f(u[2,2], u[2,3], u[3,3], u[1,2], u[1,3]), u[2,2], u[2,3], u[2,3]), \text{diff}(f(u[2,2], u[2,3], u[3,3], u[1,2], u[1,3]), u[2,2], u[2,3], u[3,3]), \text{diff}(f(u[2,2], u[2,3], u[3,3], u[1,2], u[1,3]), u[2,2], u[2,3], u[1,2]), \text{diff}(f(u[2,2], u[2,3], u[3,3], u[1,2], u[1,3]), u[2,2], u[2,3], u[1,3]), \text{diff}(f(u[2,2], u[2,3], u[3,3], u[1,2], u[1,3]), u[2,2], u[3,3], u[3,3]), \text{diff}(f(u[2,2], u[2,3], u[3,3], u[1,2], u[1,3]), u[2,2], u[3,3], u[1,2]), \text{diff}(f(u[2,2], u[2,3], u[3,3], u[1,2], u[1,3]), u[2,2], u[3,3], u[1,3]), \text{diff}(f(u[2,2], u[2,3], u[3,3], u[1,2], u[1,3]), u[2,2], u[1,2], u[1,2]), \text{diff}(f(u[2,2], u[2,3], u[3,3], u[1,2], u[1,3]), u[2,2], u[1,2], u[1,3]), \text{diff}(f(u[2,2], u[2,3], u[3,3], u[1,2], u[1,3]), u[2,2], u[1,3], u[1,3]), \text{diff}(f(u[2,2], u[2,3], u[3,3], u[1,2], u[1,3]), u[2,3], u[2,3], u[2,3])]$$



$\text{diff}(f(u[2, 2], u[2, 3], u[3, 3], u[1, 2], u[1, 3]), u[2, 3], u[2, 3], u[3, 3]),$   
 $\text{diff}(f(u[2, 2], u[2, 3], u[3, 3], u[1, 2], u[1, 3]), u[2, 3], u[2, 3], u[1, 2]),$   
 $\text{diff}(f(u[2, 2], u[2, 3], u[3, 3], u[1, 2], u[1, 3]), u[2, 3], u[2, 3], u[1, 3]),$   
 $\text{diff}(f(u[2, 2], u[2, 3], u[3, 3], u[1, 2], u[1, 3]), u[2, 3], u[3, 3], u[3, 3]),$   
 $\text{diff}(f(u[2, 2], u[2, 3], u[3, 3], u[1, 2], u[1, 3]), u[2, 3], u[3, 3], u[1, 2]),$   
 $\text{diff}(f(u[2, 2], u[2, 3], u[3, 3], u[1, 2], u[1, 3]), u[2, 3], u[3, 3], u[1, 3]),$   
 $\text{diff}(f(u[2, 2], u[2, 3], u[3, 3], u[1, 2], u[1, 3]), u[2, 3], u[1, 2], u[1, 2]),$   
 $\text{diff}(f(u[2, 2], u[2, 3], u[3, 3], u[1, 2], u[1, 3]), u[2, 3], u[1, 2], u[1, 3]),$   
 $\text{diff}(f(u[2, 2], u[2, 3], u[3, 3], u[1, 2], u[1, 3]), u[2, 3], u[1, 3], u[1, 3]),$   
 $\text{diff}(f(u[2, 2], u[2, 3], u[3, 3], u[1, 2], u[1, 3]), u[3, 3], u[3, 3], u[3, 3]),$   
 $\text{diff}(f(u[2, 2], u[2, 3], u[3, 3], u[1, 2], u[1, 3]), u[3, 3], u[3, 3], u[1, 2]),$   
 $\text{diff}(f(u[2, 2], u[2, 3], u[3, 3], u[1, 2], u[1, 3]), u[3, 3], u[3, 3], u[1, 3]),$   
 $\text{diff}(f(u[2, 2], u[2, 3], u[3, 3], u[1, 2], u[1, 3]), u[3, 3], u[1, 2], u[1, 2]),$   
 $\text{diff}(f(u[2, 2], u[2, 3], u[3, 3], u[1, 2], u[1, 3]), u[3, 3], u[1, 2], u[1, 3]),$   
 $\text{diff}(f(u[2, 2], u[2, 3], u[3, 3], u[1, 2], u[1, 3]), u[3, 3], u[1, 3], u[1, 3]),$   
 $\text{diff}(f(u[2, 2], u[2, 3], u[3, 3], u[1, 2], u[1, 3]), u[1, 2], u[1, 2], u[1, 2]),$   
 $\text{diff}(f(u[2, 2], u[2, 3], u[3, 3], u[1, 2], u[1, 3]), u[1, 2], u[1, 2], u[1, 3]),$   
 $\text{diff}(f(u[2, 2], u[2, 3], u[3, 3], u[1, 2], u[1, 3]), u[1, 2], u[1, 3], u[1, 3]),$   
 $\text{diff}(f(u[2, 2], u[2, 3], u[3, 3], u[1, 2], u[1, 3]), u[1, 3], u[1, 3], u[1, 3]) ] :$

**J2** >  $\text{Var} := \text{subs}([u_{2,2}=r, u_{2,3}=s, u_{3,3}=t, u_{1,2}=a, u_{1,3}=b], \text{Vara})$

$\text{Var} := [f_{r,r,r}, r, r, f_{r,r,s}, f_{r,r,s}, f_{a,r,r}, r, r, f_{b,r,r}, r, r, f_{r,s,s}, f_{r,s,s}, f_{a,r,s}, f_{b,r,s}, f_{r,t,r}, f_{a,r,t}, f_{b,r,t}, f_{a,a,r}, f_{a,b,r},$   
 $f_{b,b,r}, r, f_{s,s,s}, f_{s,s,s}, f_{a,s,s}, f_{b,s,s}, f_{s,t,t}, f_{a,s,t}, f_{b,s,t}, f_{a,a,s}, f_{a,b,s}, f_{b,b,s}, f_{t,t,t}, f_{a,t,t}, f_{b,t,t}, f_{a,a,t},$   
 $f_{a,b,t}, f_{b,b,t}, f_{a,a,a}, f_{a,a,b}, f_{a,b,b}, f_{b,b,b}]$

(32)

**J2** >  $\text{Varb} := [\text{diff}(f(r, s, t, a, b), r, r, r), \text{diff}(f(r, s, t, a, b), r, r, s), \text{diff}(f(r, s, t, a, b), r,$   
 $r, t), \text{diff}(f(r, s, t, a, b), r, r, a), \text{diff}(f(r, s, t, a, b), r, r, b), \text{diff}(f(r, s, t, a, b), r,$   
 $s, s), \text{diff}(f(r, s, t, a, b), r, s, t), \text{diff}(f(r, s, t, a, b), r, s, a), \text{diff}(f(r, s, t, a, b), r,$   
 $s, b), \text{diff}(f(r, s, t, a, b), r, t, t), \text{diff}(f(r, s, t, a, b), r, t, a), \text{diff}(f(r, s, t, a, b), r, t,$   
 $b), \text{diff}(f(r, s, t, a, b), r, a, a), \text{diff}(f(r, s, t, a, b), r, a, b), \text{diff}(f(r, s, t, a, b), r,$   
 $b, b), \text{diff}(f(r, s, t, a, b), s, s, s), \text{diff}(f(r, s, t, a, b), s, s, t), \text{diff}(f(r, s, t, a, b), s,$   
 $s, a), \text{diff}(f(r, s, t, a, b), s, s, b), \text{diff}(f(r, s, t, a, b), s, t, t), \text{diff}(f(r, s, t, a, b), s,$   
 $t, a), \text{diff}(f(r, s, t, a, b), s, t, b), \text{diff}(f(r, s, t, a, b), s, a, a), \text{diff}(f(r, s, t, a, b), s,$   
 $a, b), \text{diff}(f(r, s, t, a, b), s, b, b), \text{diff}(f(r, s, t, a, b), t, t, t), \text{diff}(f(r, s, t, a, b), t,$   
 $t, a), \text{diff}(f(r, s, t, a, b), t, t, b), \text{diff}(f(r, s, t, a, b), t, a, a), \text{diff}(f(r, s, t, a, b), t,$   
 $a, b), \text{diff}(f(r, s, t, a, b), t, b, b), \text{diff}(f(r, s, t, a, b), a, a, a), \text{diff}(f(r, s, t, a, b),$   
 $a, a, b), \text{diff}(f(r, s, t, a, b), a, b, b), \text{diff}(f(r, s, t, a, b), b, b, b)] :$

**J2** >  $\text{ThP} := \text{subs}([u_{2,2}=r, u_{2,3}=s, u_{3,3}=t, u_{1,2}=a, u_{1,3}=b], [\text{diff}(Eq1, u_{1,2,2}, u_{1,2,2}),$   
 $\text{diff}(Eq1, u_{1,2,3}, u_{1,2,3}), \text{diff}(Eq1, u_{1,3,3}, u_{1,3,3}), \text{diff}(Eq1, u_{2,2,2}, u_{2,2,2}),$   
 $\text{diff}(Eq1, u_{2,2,3}, u_{2,2,3}), \text{diff}(Eq1, u_{2,3,3}, u_{2,3,3}), \text{diff}(Eq1, u_{3,3,3}, u_{3,3,3}),$   
 $\text{diff}(Eq2, u_{1,2,2}, u_{1,2,2}), \text{diff}(Eq2, u_{1,2,3}, u_{1,2,3}), \text{diff}(Eq2, u_{1,3,3}, u_{1,3,3}),$   
 $\text{diff}(Eq2, u_{2,2,2}, u_{2,2,2}), \text{diff}(Eq2, u_{2,2,3}, u_{2,2,3}), \text{diff}(Eq2, u_{2,3,3}, u_{2,3,3}),$   
 $\text{diff}(Eq2, u_{3,3,3}, u_{3,3,3}), \text{diff}(Eq3, u_{1,2,2}, u_{1,2,2}), \text{diff}(Eq3, u_{1,2,3}, u_{1,2,3}),$   
 $\text{diff}(Eq3, u_{1,3,3}, u_{1,3,3}), \text{diff}(Eq3, u_{2,2,2}, u_{2,2,2}), \text{diff}(Eq3, u_{2,2,3}, u_{2,2,3}),$   
 $\text{diff}(Eq3, u_{2,3,3}, u_{2,3,3}), \text{diff}(Eq3, u_{3,3,3}, u_{3,3,3}), \text{diff}(Eq4, u_{1,2,2}, u_{1,2,2}),$   
 $\text{diff}(Eq4, u_{1,2,3}, u_{1,2,3}), \text{diff}(Eq4, u_{1,3,3}, u_{1,3,3}), \text{diff}(Eq4, u_{2,2,2}, u_{2,2,2}),$   
 $\text{diff}(Eq4, u_{2,2,3}, u_{2,2,3}), \text{diff}(Eq4, u_{2,3,3}, u_{2,3,3}), \text{diff}(Eq4, u_{3,3,3}, u_{3,3,3}),$   
 $\text{diff}(Eq5, u_{1,2,2}, u_{1,2,2}), \text{diff}(Eq5, u_{1,2,3}, u_{1,2,3}), \text{diff}(Eq5, u_{1,3,3}, u_{1,3,3}),$

L

1

---

---

---

---

$$\begin{aligned}
& u_{1,2,2}, u_{3,3,3}), \text{diff}(Eq4, u_{1,2,3}, u_{1,2,3}), \text{diff}(Eq4, u_{1,2,3}, u_{1,3,3}), \text{diff}(Eq4, \\
& u_{1,2,3}, u_{2,2,2}), \text{diff}(Eq4, u_{1,2,3}, u_{2,2,3}), \text{diff}(Eq4, u_{1,2,3}, u_{2,3,3}), \text{diff}(Eq4, \\
& u_{1,2,3}, u_{3,3,3}), \text{diff}(Eq4, u_{1,3,3}, u_{1,3,3}), \text{diff}(Eq4, u_{1,3,3}, u_{2,2,2}), \text{diff}(Eq4, \\
& u_{1,3,3}, u_{2,2,3}), \text{diff}(Eq4, u_{1,3,3}, u_{2,3,3}), \text{diff}(Eq4, u_{1,3,3}, u_{3,3,3}), \text{diff}(Eq4, \\
& u_{2,2,2}, u_{2,2,2}), \text{diff}(Eq4, u_{2,2,2}, u_{2,2,3}), \text{diff}(Eq4, u_{2,2,2}, u_{2,3,3}), \text{diff}(Eq4, \\
& u_{2,2,2}, u_{3,3,3}), \text{diff}(Eq4, u_{2,2,3}, u_{2,2,3}), \text{diff}(Eq4, u_{2,2,3}, u_{2,3,3}), \text{diff}(Eq4, \\
& u_{2,2,3}, u_{3,3,3}), \text{diff}(Eq4, u_{2,3,3}, u_{2,3,3}), \text{diff}(Eq4, u_{2,3,3}, u_{3,3,3}), \text{diff}(Eq4, \\
& u_{3,3,3}, u_{3,3,3}), \\
& \text{diff}(Eq5, u_{1,2,2}, u_{1,2,2}), \text{diff}(Eq5, u_{1,2,2}, u_{1,2,3}), \text{diff}(Eq5, u_{1,2,2}, u_{1,3,3}), \text{diff}(Eq5, \\
& u_{1,2,2}, u_{2,2,2}), \text{diff}(Eq5, u_{1,2,2}, u_{2,2,3}), \text{diff}(Eq5, u_{1,2,2}, u_{2,3,3}), \text{diff}(Eq5, \\
& u_{1,2,2}, u_{3,3,3}), \text{diff}(Eq5, u_{1,2,3}, u_{1,2,3}), \text{diff}(Eq5, u_{1,2,3}, u_{1,3,3}), \text{diff}(Eq5, \\
& u_{1,2,3}, u_{2,2,2}), \text{diff}(Eq5, u_{1,2,3}, u_{2,2,3}), \text{diff}(Eq5, u_{1,2,3}, u_{2,3,3}), \text{diff}(Eq5, \\
& u_{1,2,3}, u_{3,3,3}), \text{diff}(Eq5, u_{1,3,3}, u_{1,3,3}), \text{diff}(Eq5, u_{1,3,3}, u_{2,2,2}), \text{diff}(Eq5, \\
& u_{1,3,3}, u_{2,2,3}), \text{diff}(Eq5, u_{1,3,3}, u_{2,3,3}), \text{diff}(Eq5, u_{1,3,3}, u_{3,3,3}), \text{diff}(Eq5, \\
& u_{2,2,2}, u_{2,2,2}), \text{diff}(Eq5, u_{2,2,2}, u_{2,2,3}), \text{diff}(Eq5, u_{2,2,2}, u_{2,3,3}), \text{diff}(Eq5, \\
& u_{2,2,2}, u_{3,3,3}), \text{diff}(Eq5, u_{2,2,3}, u_{2,2,3}), \text{diff}(Eq5, u_{2,2,3}, u_{2,3,3}), \text{diff}(Eq5, \\
& u_{2,2,3}, u_{3,3,3}), \text{diff}(Eq5, u_{2,3,3}, u_{2,3,3}), \text{diff}(Eq5, u_{2,3,3}, u_{3,3,3}), \text{diff}(Eq5, \\
& u_{3,3,3}, u_{3,3,3})) :
\end{aligned}$$

Finally we are ready for the matrix:

**J2** > interface(rtablesize = 140)

140

(33)

**J2** > MaQ := (i, j) → simplify $\left(\frac{1}{\Delta} \text{coeff}(ThP[i], \text{Var}[j])\right)$  :

**J2** > MEQ := Matrix(140, 35, MaQ)

$$\begin{aligned}
MEQ := & \left[ \left[ -8f_t(f_b f_s - 2f_a f_t), 2f_b f_s^2 - 8f_a f_t f_s + 8f_b f_t f_r, 4f_s(f_a f_s - 2f_b f_r), 4f_t(f_s^2 - 2f_b f_a f_s \right. \right. \\
& + 4f_a^2 f_t - 4f_t f_r), -2f_s(f_s^2 - 4f_t f_r), 0, 0, 2f_a(f_b f_s^2 - 4f_a f_t f_s + 4f_b f_t f_r), 0, 0, 4f_a f_s(f_a f_s \\
& - 2f_b f_r), 0, 4f_t(f_a f_s^2 + 2f_b f_r f_s - 8f_a f_t f_r), -2f_a f_s(f_s^2 - 4f_t f_r), 0, 0, 0, 0, 0, 0, 0, \\
& -2f_r(f_b f_s^2 - 4f_a f_t f_s + 4f_b f_t f_r), 0, 0, 0, 0, 0, -4f_r f_s(f_a f_s - 2f_b f_r), 0, 0, -4f_r f_t(f_s^2 \\
& - 4f_t f_r), 2f_r f_s(f_s^2 - 4f_t f_r), 0, 0 \left. \right], \\
& \left[ 0, -8f_t(f_b f_s - 2f_a f_t), 0, -4f_b f_t(f_b f_s - 2f_a f_t), -4f_a f_t(f_b f_s - 2f_a f_t), 2f_b f_s^2 - 8f_a f_t f_s \right. \\
& + 8f_b f_t f_r, 4f_s(f_a f_s - 2f_b f_r), f_s^2 f_b^2 + 4f_s^2 f_t - 8f_b f_a f_t f_s + 4f_b^2 f_r f_t - 16f_r f_t^2 + 8f_a^2 f_t^2, -2f_s^3 \\
& + f_b f_a f_s^2 + 8f_s f_r f_t - 4f_s f_a^2 f_t + 4f_b f_a f_t f_r, 0, 2f_b f_s(f_a f_s - 2f_b f_r), 2f_a f_s(f_a f_s - 2f_b f_r), \\
& 2f_t(3f_b f_s^2 - 4f_a f_t f_s - 4f_b f_t f_r), -f_b f_s^3 + 2f_s^2 f_a f_t + 12f_s f_b f_t f_r - 24f_a f_t^2 f_r - f_a f_s(f_s^2 \\
& - 4f_t f_r), 0, 0, f_a(f_b f_s^2 - 4f_a f_t f_s + 4f_b f_t f_r), 0, 0, 2f_a f_s(f_a f_s - 2f_b f_r), 0, -f_b f_s^3 + 6f_s^2 f_a f_t \\
& - 4f_s f_b f_t f_r - 8f_a f_t^2 f_r - f_a f_s^3 - 2f_s^2 f_b f_r + 12f_r f_a f_t f_s - 8f_b f_t f_r^2, 0, 0, 0, 0, -2f_s^2(f_a f_s
\end{aligned}$$

$$-2f_b f_r), -4f_r f_s (f_a f_s - 2f_b f_r), 0, -2f_s f_t (f_s^2 - 4f_t f_r), 16f_r^2 f_t^2 - 8f_s^2 f_r f_t + f_s^4, 2f_r f_s (f_s^2 - 4f_t f_r), 0],$$

$$[0, 0, -8f_t (f_b f_s - 2f_a f_t), 0, -4f_b f_t (f_b f_s - 2f_a f_t), 0, 2f_b f_s^2 - 8f_a f_t f_s + 8f_b f_t f_r, 0, f_b (f_b f_s^2 - 4f_a f_t f_s + 4f_b f_t f_r), 4f_s (f_a f_s - 2f_b f_r), 4f_t (f_s^2 - f_b f_a f_s - 4f_t f_r + 2f_a^2 f_t), -2f_s (f_s^2 - f_b f_a f_s - 4f_t f_r + 2f_r f_b^2), 0, 2f_t (3f_b f_s^2 - 4f_a f_t f_s - 4f_b f_t f_r), -f_b f_s (f_s^2 - 4f_t f_r), 0, 0, 0, 0, 0, f_a (f_b f_s^2 - 4f_a f_t f_s + 4f_b f_t f_r), 0, 0, -f_s (f_b f_s^2 - 4f_a f_t f_s + 4f_b f_t f_r), 0, 0, 2f_a f_s (f_a f_s - 2f_b f_r), 0, 2f_a f_t (f_s^2 - 4f_t f_r), -f_s (3f_a f_s^2 - 4f_b f_r f_s - 4f_a f_t f_r), 0, 0, -2f_s f_t (f_s^2 - 4f_t f_r), f_s^2 (f_s^2 - 4f_t f_r), 0],$$

$$[4f_a f_t (f_b f_s - 2f_a f_t), -f_a (f_b f_s^2 - 4f_a f_t f_s + 4f_b f_t f_r), -2f_a f_s (f_a f_s - 2f_b f_r), -2f_a f_t (f_s^2 - 2f_b f_a f_s + 4f_a^2 f_t - 4f_t f_r), f_a f_s (f_s^2 - 4f_t f_r), 0, 0, -f_a^2 (f_b f_s^2 - 4f_a f_t f_s + 4f_b f_t f_r), 0, 0, -2f_s f_a^2 (f_a f_s - 2f_b f_r), 0, -2f_a f_t (f_a f_s^2 + 2f_b f_r f_s - 8f_a f_t f_r), f_s f_a^2 (f_s^2 - 4f_t f_r), 0, 0, 0, 0, 0, 0, 0, f_a f_r (f_b f_s^2 - 4f_a f_t f_s + 4f_b f_t f_r), 0, 0, 0, 0, 0, 2f_s f_a f_r (f_a f_s - 2f_b f_r), 0, 0, 2f_a f_t f_r (f_s^2 - 4f_t f_r), -f_s f_a f_r (f_s^2 - 4f_t f_r), 0, 0],$$

$$[4f_b f_t (f_b f_s - 2f_a f_t), -f_s^2 f_b^2 + 8f_b f_a f_t f_s - 8f_a^2 f_t^2 - 4f_b^2 f_r f_r - 2f_b f_s (f_a f_s - 2f_b f_r), -2f_t (3f_b f_s^2 - 2f_s f_a f_b^2 - 4f_a f_t f_s - 4f_b f_t f_r + 4f_b f_a^2 f_t), f_b f_s^3 - 12f_s f_b f_t f_r + 16f_a f_t^2 f_r - f_a (f_b f_s^2 - 4f_a f_t f_s + 4f_b f_t f_r), -2f_a f_s (f_a f_s - 2f_b f_r), f_b f_s^3 - 6f_s^2 f_a f_t - f_b^2 f_a f_s^2 + 12f_s f_b f_t f_r + 8f_b f_a^2 f_s f_t - 8f_a f_t^2 f_r - 4f_r f_a f_t f_b^2 - 8f_a^3 f_t^2, f_a f_s^3 + 2f_s^2 f_b f_r - 12f_r f_a f_t f_s + 8f_b f_t f_r^2, 0, 2f_s (f_a f_s^2 - f_a^2 f_s f_b - 2f_b f_r f_s + 2f_r f_a f_b^2), 4f_r f_s (f_a f_s - 2f_b f_r), 2f_t (f_s^3 - 3f_b f_a f_s^2 - 4f_s f_r f_t + 4f_s f_a^2 f_t + 4f_b f_a f_t f_r), -f_s^4 + f_b f_a f_s^3 + 8f_s^2 f_r f_t - 8f_s f_b f_a f_t f_r - 16f_r^2 f_t^2 + 8f_a^2 f_t^2 f_r - 2f_r f_s (f_s^2 - 4f_t f_r), 0, 0, -f_a^2 f_s^2 f_b - 2f_s^2 f_b f_r + 8f_r f_a f_t f_s + 4f_a^3 f_s f_t - 4f_r f_b f_a^2 f_t - 8f_b f_t f_r^2, 0, 0, -2f_s (f_a^3 f_s + 2f_r f_s f_a - 4f_b f_r^2 - 2f_r f_b f_a^2), 0, f_b f_a f_s^3 - 4f_s^2 f_r f_t - 6f_s^2 f_a^2 f_t + 4f_s f_b f_a f_t f_r + 16f_r^2 f_t^2 + 8f_a^2 f_t^2 f_r^2 f_a^2 f_s^3 + 2f_r f_s^3 + f_r f_a f_s^2 f_b - 8f_r^2 f_t f_s - 8f_r f_a^2 f_s f_t + 4f_r^2 f_a f_t f_b, 0, 0, 0, 0, 2f_a f_s^2 (f_a f_s - 2f_b f_r), 2f_s f_a f_r (f_a f_s - 2f_b f_r), 0, 2f_a f_t f_s (f_s^2 - 4f_t f_r), -f_a (f_s^4 - 6f_s^2 f_r f_t + 8f_r^2 f_t^2), -f_s f_a f_r (f_s^2 - 4f_t f_r), 0],$$

$$[0, 4f_b f_t (f_b f_s - 2f_a f_t), 4f_a f_t (f_b f_s - 2f_a f_t), -8f_t^2 (f_b f_s - 2f_a f_t), -8f_t f_s (f_b f_s - 2f_a f_t), -f_b (f_b f_s^2 - 4f_a f_t f_s + 4f_b f_t f_r), -3f_b f_a f_s^2 + 4f_s f_r f_b^2 + 4f_s f_a^2 f_t - 4f_b f_a f_t f_r, 4f_t (f_b f_s^2 + f_s f_a f_b^2 - 4f_a f_t f_s - 2f_b f_a^2 f_t + 4f_b f_t f_r), f_s (3f_b f_s^2 - 8f_a f_t f_s + 4f_b f_t f_r), -2f_a f_s (f_a f_s - 2f_b f_r), 2f_a f_t (f_s^2 + 2f_b f_a f_s - 4f_t f_r - 4f_a^2 f_t), f_s (5f_a f_s^2 - 8f_b f_r f_s - 4f_a f_t f_r), 4f_t^2 (f_s^2 - f_b f_a f_s - 4f_t f_r + 2f_a^2 f_t), 2f_s f_t (f_s^2 - 2f_b f_a f_s + 4f_a^2 f_t - 4f_t f_r), -2f_s^2 (f_s^2 - 4f_t f_r), 0, 0, -f_b f_s^3 -$$

$$\begin{aligned}
& f_b^2 f_a f_s^2 + 4 f_s^2 f_a f_t + 4 f_b f_a^2 f_s f_t - 4 f_s f_b f_t f_r - 4 f_r f_a f_t f_b^2, 0, 0, -2 f_a f_s^3 + 2 f_s^2 f_b f_r - 3 f_a^2 f_s^2 f_b \\
& + 4 f_r f_a f_s f_b^2 + 8 f_r f_a f_t f_s + 4 f_a^3 f_s f_t - 4 f_r f_b f_a^2 f_t - 8 f_b f_t f_r^2, 0, -f_t (2 f_s^3 + f_b f_a f_s^2 - 8 f_s f_r f_t \\
& + 4 f_s f_a^2 f_t - 12 f_b f_a f_t f_r), f_s^2 (f_s^2 + 2 f_b f_a f_s - 4 f_t f_r - 4 f_a^2 f_t), 0, 0, -2 f_s (f_a^3 f_s + 2 f_r f_s f_a \\
& - 4 f_b f_r^2 - 2 f_r f_b f_a^2), 0, -4 f_r f_t (f_s^2 + f_b f_a f_s - 4 f_t f_r - 2 f_a^2 f_t), f_s (3 f_s^2 f_a^2 + 2 f_s^2 f_r \\
& - 4 f_b f_a f_r f_s - 4 f_a^2 f_t f_r - 8 f_r^2 f_t), 0, 2 f_a f_t^2 (f_s^2 - 4 f_t f_r), f_a f_t f_s (f_s^2 - 4 f_t f_r), -f_a f_s^2 (f_s^2 \\
& - 4 f_t f_r), 0], \\
& [0, 0, 4 f_b f_t (f_b f_s - 2 f_a f_t), 0, -8 f_t^2 (f_b f_s - 2 f_a f_t), 0, -f_b (f_b f_s^2 - 4 f_a f_t f_s + 4 f_b f_t f_r), 0, \\
& 2 f_t (f_b f_s^2 - 4 f_a f_t f_s + 4 f_b f_t f_r), -2 f_b f_s (f_a f_s - 2 f_b f_r), 2 f_t (f_b f_s^2 + 2 f_s f_a f_b^2 - 4 f_a f_t f_s \\
& - 4 f_b f_a^2 f_t + 4 f_b f_t f_r), f_s (f_b f_s^2 + 4 f_a f_t f_s - 12 f_b f_t f_r), 0, 4 f_t^2 (f_s^2 - f_b f_a f_s - 4 f_t f_r + 2 \\
& f_a^2 f_t), -2 f_s f_t (f_s^2 - 4 f_t f_r), 0, 0, 0, 0, 0, -f_b f_s^3 - f_b^2 f_a f_s^2 + 4 f_s^2 f_a f_t + 4 f_b f_a^2 f_s f_t - 4 f_s f_b f_t f_r \\
& - 4 f_r f_a f_t f_b^2, 0, 0, f_a f_t (f_b f_s^2 - 4 f_a f_t f_s + 4 f_b f_t f_r), 0, 0, -2 f_s (f_a f_s^2 - 2 f_b f_r f_s + f_a^2 f_s f_b \\
& - 2 f_r f_a f_b^2), 0, -2 f_t (f_s^3 + f_b f_a f_s^2 - 4 f_s f_r f_t - 4 f_b f_a f_t f_r), f_s (f_s^3 + f_b f_a f_s^2 - 4 f_s f_r f_t + 2 f_s f_a^2 f_t \\
& - 8 f_b f_a f_t f_r), 0, 0, 2 f_a f_t^2 (f_s^2 - 4 f_t f_r), -f_a f_t f_s (f_s^2 - 4 f_t f_r), 0], \\
& [0, 0, 0, 0, 0, -8 f_t (f_b f_s - 2 f_a f_t), 0, -8 f_b f_t (f_b f_s - 2 f_a f_t), -8 f_a f_t (f_b f_s - 2 f_a f_t), 0, 0, 0, \\
& 8 f_t^2 (f_b f_s - 2 f_a f_t), 8 f_t f_s (f_b f_s - 2 f_a f_t), 8 f_r f_t (f_b f_s - 2 f_a f_t), 2 f_b f_s^2 - 8 f_a f_t f_s + 8 f_b f_t f_r \\
& 4 f_s (f_a f_s - 2 f_b f_r), 2 f_s^2 f_b^2 + 4 f_s^2 f_t - 8 f_b f_a f_t f_s - 16 f_r f_t^2 + 8 f_b^2 f_r f_r, 8 f_b f_a f_t f_r + 8 f_s f_r f_t \\
& + 2 f_b f_a f_s^2 - 8 f_s f_a^2 f_t - 2 f_s^3, 0, 4 f_b f_s (f_a f_s - 2 f_b f_r), 4 f_a f_s (f_a f_s - 2 f_b f_r), 2 f_t (f_b f_s^2 \\
& + 4 f_a f_t f_s - 12 f_b f_t f_r), -16 f_a f_t^2 f_r - 4 f_b f_s^3 + 12 f_s^2 f_a f_r - 8 f_b f_t f_r^2 - 2 f_s^2 f_b f_r + 16 f_r f_a f_t f_s \\
& - 2 f_a f_s^3, 0, 0, 0, -4 f_t f_s (f_a f_s - 2 f_b f_r), -4 f_s^2 (f_a f_s - 2 f_b f_r), -4 f_r f_s (f_a f_s - 2 f_b f_r), -4 \\
& f_t^2 (f_s^2 - 4 f_t f_r), -2 f_s f_t (f_s^2 - 4 f_t f_r), 16 f_r^2 f_t^2 - 12 f_s^2 f_r f_t + 2 f_s^4, 2 f_r f_s (f_s^2 - 4 f_t f_r)], \\
& [0, 0, 0, 0, 0, -8 f_t (f_b f_s - 2 f_a f_t), 0, -4 f_b f_t (f_b f_s - 2 f_a f_t), 0, -4 f_b f_t (f_b f_s - 2 f_a f_t), \\
& -4 f_a f_t (f_b f_s - 2 f_a f_t), 0, 8 f_t^2 (f_b f_s - 2 f_a f_t), 4 f_t f_s (f_b f_s - 2 f_a f_t), 0, 2 f_b f_s^2 - 8 f_a f_t f_s \\
& + 8 f_b f_t f_r, 0, f_b (f_b f_s^2 - 4 f_a f_t f_s + 4 f_b f_t f_r), 4 f_s (f_a f_s - 2 f_b f_r), f_s^2 f_b^2 + 4 f_s^2 f_t - 4 f_b f_a f_t f_s \\
& - 16 f_r f_t^2 + 4 f_b^2 f_r f_r - 2 f_s^3 + 3 f_b f_a f_s^2 + 8 f_s f_r f_t - 4 f_s f_r f_b^2 - 4 f_s f_a^2 f_t + 4 f_b f_a f_t f_r, 0, 8 \\
& f_t^2 (f_a f_s - 2 f_b f_r), -2 f_s^2 (f_b f_s - 2 f_a f_t), 0, 2 f_b f_s (f_a f_s - 2 f_b f_r), 2 f_a f_s (f_a f_s - 2 f_b f_r), \\
& 2 f_b f_t (f_s^2 - 4 f_t f_r), -f_b f_s^3 - 2 f_s^2 f_a f_t + 12 f_s f_b f_t f_r - 8 f_a f_t^2 f_r, -f_s (3 f_a f_s^2 - 4 f_b f_r f_s \\
& - 4 f_a f_t f_r), 0, -4 f_t^2 (f_s^2 - 4 f_t f_r), 0, f_s^2 (f_s^2 - 4 f_t f_r)], \\
& [0, 4 f_a f_t (f_b f_s - 2 f_a f_t), 0, 4 f_t (f_b f_s^2 - 2 f_a f_t f_s + f_s f_a f_b^2 - 2 f_b f_a^2 f_t), 4 f_t (f_a^2 f_s f_b + 2 f_b f_r f_s \\
& - 4 f_a f_t f_r - 2 f_a^3 f_t), -f_a (f_b f_s^2 - 4 f_a f_t f_s + 4 f_b f_t f_r), -2 f_a f_s (f_a f_s - 2 f_b f_r), -f_b f_s^3 + 2
\end{aligned}$$

$$\begin{aligned}
& f_s^2 f_a f_t - f_b^2 f_a f_s^2 - 12 f_s f_b f_t f_r + 4 f_b f_a^2 f_s f_t + 24 f_a f_t^2 f_r - 4 f_r f_a f_t f_b^2, f_a f_s^3 - f_a^2 f_s^2 f_b - 2 f_s^2 f_b f_r \\
& + 4 f_a^3 f_s f_t + 4 f_r f_a f_t f_s - 4 f_r f_b f_a^2 f_t - 8 f_b f_t f_r^2, 0, -2 f_s (f_a f_s^2 - 2 f_b f_r f_s + f_a^2 f_s f_b - 2 f_r f_a \\
& f_b^2), -2 f_s (f_a^3 f_s + 2 f_r f_s f_a - 4 f_b f_r^2 - 2 f_r f_b f_a^2), -2 f_t (f_s^3 + f_b f_a f_s^2 - 4 f_s f_r f_t + 2 f_s f_r f_b^2 \\
& - 8 f_b f_a f_t f_r), f_s^4 + f_b f_a f_s^3 - 8 f_s^2 f_r f_t - 2 f_s^2 f_a^2 f_t - 8 f_s f_b f_a f_t f_r + 16 f_a^2 f_t^2 f_r + 16 f_r^2 f_t^2, f_s (f_s^2 \\
& f_a^2 + 2 f_s^2 f_r - 4 f_a^2 f_t f_r - 8 f_r^2 f_t), 0, 0, 2 f_r (f_b f_s^2 - 4 f_a f_t f_s + 4 f_b f_t f_r), 0, 0, 4 f_r f_s (f_a f_s \\
& - 2 f_b f_r), 0, f_r (f_s^2 f_b^2 + 4 f_s^2 f_t - 4 f_b f_a f_t f_s - 16 f_r f_t^2 + 4 f_b^2 f_r f_t), -f_r (2 f_s^3 - f_b f_a f_s^2 - 8 f_s f_r f_t \\
& + 4 f_s f_a^2 f_t - 4 f_b f_a f_t f_r), 0, 0, 0, 0, 2 f_b f_r f_s (f_a f_s - 2 f_b f_r), 2 f_s f_a f_r (f_a f_s - 2 f_b f_r), 0, \\
& 2 f_b f_t f_r (f_s^2 - 4 f_t f_r), -f_r (f_b f_s^3 - 2 f_s^2 f_a f_t - 4 f_s f_b f_t f_r + 8 f_a f_t^2 f_r), -f_s f_a f_r (f_s^2 - 4 f_t f_r), 0], \\
& [0, 4 f_b f_t (f_b f_s - 2 f_a f_t), 0, 4 f_t (2 f_t f_s f_b + f_s f_b^3 - 4 f_t^2 f_a - 2 f_a f_t f_b^2), 4 f_t (f_b f_s^2 - 2 f_a f_t f_s \\
& + f_s f_a f_b^2 - 2 f_b f_a^2 f_t), -f_s^2 f_b^2 + 8 f_b f_a f_t f_s - 8 f_a^2 f_t^2 - 4 f_b^2 f_r f_r - 2 f_b f_s (f_a f_s - 2 f_b f_r), -8 \\
& f_s^2 f_b f_t - f_s^2 f_b^3 + 16 f_s f_a f_t^2 + 8 f_s f_a f_t f_b^2 - 4 f_b^3 f_r f_t - 8 f_a^2 f_t^2 f_b, -f_b^2 f_a f_s^2 + 4 f_s^2 f_a f_t - 8 f_s f_b f_t f_r \\
& + 8 f_b f_a^2 f_s f_t - 4 f_r f_a f_t f_b^2 - 8 f_a^3 f_t^2, 0, -2 f_s (2 f_a f_t f_s + f_s f_a f_b^2 - 2 f_b^3 f_r - 4 f_b f_t f_r), -2 f_s (f_a \\
& f_s^2 - 2 f_b f_r f_s + f_a^2 f_s f_b - 2 f_r f_a f_b^2), -2 f_t (3 f_s^2 f_b^2 + 2 f_s^2 f_t - 4 f_b f_a f_t f_s - 4 f_b^2 f_r f_t - 8 f_r f_t^2), f_b^2 \\
& f_s^3 - 6 f_a f_t f_b f_s^2 + 8 f_s f_a^2 f_t^2 - 8 f_r f_t f_s f_b^2 + 16 f_r f_t^2 f_a f_b, f_s^4 + f_b f_a f_s^3 - 4 f_s^2 f_r f_t - 8 f_s f_b f_a f_t f_r \\
& + 8 f_a^2 f_t^2 f_r - f_a (f_b f_s^2 - 4 f_a f_t f_s + 4 f_b f_t f_r), -2 f_a f_s (f_a f_s - 2 f_b f_r), f_b f_s^3 - 6 f_s^2 f_a f_t - f_b^2 f_a f_s^2 \\
& + 4 f_b f_a^2 f_s f_t + 4 f_s f_b f_t f_r + 8 f_a f_t^2 f_r - 4 f_r f_a f_t f_b^2, f_a (f_s^3 - f_b f_a f_s^2 - 4 f_s f_r f_t + 4 f_s f_a^2 f_t \\
& - 4 f_b f_a f_t f_r), 0, 2 f_s (f_a f_s^2 - f_a^2 f_s f_b - 2 f_b f_r f_s + 2 f_r f_a f_b^2), -2 f_s f_a^2 (f_a f_s - 2 f_b f_r), f_b^2 f_s^3 \\
& + 2 f_t f_s^3 - 6 f_a f_t f_b f_s^2 - 8 f_r f_t^2 f_s + 4 f_r f_t f_s f_b^2 + 8 f_r f_t^2 f_a f_b, -f_s^4 + 2 f_b f_a f_s^3 + 4 f_s^2 f_r f_t - 6 f_s^2 \\
& f_a^2 f_t + f_s^2 f_r f_b^2 - 4 f_s f_b f_a f_t f_r + 4 f_r^2 f_t f_b^2 + 8 f_a^2 f_t^2 f_r f_a (4 f_b f_t f_r^2 + f_s^2 f_b f_r - 8 f_r f_a f_t f_s + f_a^3 f_s), \\
& 0, 0, 0, 2 f_b f_s^2 (f_a f_s - 2 f_b f_r), 2 f_s (f_s^2 f_a^2 - f_b f_a f_r f_s - 2 f_r^2 f_b^2), 2 f_s f_a f_r (f_a f_s - 2 f_b f_r), \\
& 2 f_s f_b f_t (f_s^2 - 4 f_t f_r), -f_b f_s^4 + 2 f_s^3 f_a f_t + 6 f_s^2 f_b f_t f_r - 8 f_s f_a f_t^2 f_r - 8 f_b f_r^2 f_t^2, -f_s^4 f_a - f_r f_b f_s^3 \\
& + 6 f_r f_a f_t f_s^2 + 4 f_r^2 f_s f_t f_b - 8 f_r^2 f_a f_t^2, -f_s f_a f_r (f_s^2 - 4 f_t f_r)], \\
& [0, 0, 0, 0, 0, 4 f_b f_t (f_b f_s - 2 f_a f_t), 4 f_a f_t (f_b f_s - 2 f_a f_t), 4 f_b^2 f_t (f_b f_s - 2 f_a f_t), -4 f_t (f_b f_s^2 \\
& - 2 f_a f_t f_s - f_s f_a f_b^2 + 2 f_b f_a^2 f_t), 0, 4 f_t (f_b f_s^2 - 2 f_a f_t f_s + f_s f_a f_b^2 - 2 f_b f_a^2 f_t), 4 f_t (f_a^2 f_s f_b \\
& + 2 f_b f_r f_s - 4 f_a f_t f_r - 2 f_a^3 f_t), -4 f_t^2 f_b (f_b f_s - 2 f_a f_t), -4 f_t (f_s^2 f_b^2 - f_b f_a f_t f_s - 2 f_a^2 f_t^2), \\
& -4 f_a f_t f_s (f_b f_s - 2 f_a f_t), -f_b (f_b f_s^2 - 4 f_a f_t f_s + 4 f_b f_t f_r), -3 f_b f_a f_s^2 + 4 f_s f_r f_b^2 + 4 f_s f_a^2 f_t \\
& - 4 f_b f_a f_t f_r, -f_b (f_s^2 f_b^2 + 2 f_s^2 f_t - 4 f_b f_a f_t f_s - 8 f_r f_t^2 + 4 f_b^2 f_r f_t), 2 f_b f_s^3 - f_b^2 f_a f_s^2 - 4 f_s^2 f_a f_t \\
& + 4 f_b f_a^2 f_s f_t - 4 f_r f_a f_t f_b^2, -2 f_a f_s (f_a f_s - 2 f_b f_r), -f_b f_s^3 - 3 f_b^2 f_a f_s^2 + 2 f_s^2 f_a f_t + 4 f_b f_a^2 f_s f_t \\
& + 4 f_r f_s f_b^3 - 4 f_s f_b f_t f_r - 4 f_r f_a f_t f_b^2 + 8 f_a f_t^2 f_r, 3 f_a f_s^3 - 6 f_s^2 f_b f_r - 3 f_a^2 f_s^2 f_b + 4 f_a^3 f_s f_t
\end{aligned}$$

$$\begin{aligned}
& + 4f_r f_a f_s f_b^2 + 4f_r f_a f_t f_s - 8f_b f_t f_r^2 - 4f_r f_b f_a^2 f_r - f_b f_t (f_b f_s^2 + 4f_a f_t f_s - 12f_b f_t f_r), 2f_b^2 f_s^3 \\
& + 2f_t f_s^3 - 5f_a f_t f_b f_s^2 - 8f_r f_t^2 f_s - 4f_s f_a^2 f_t^2 + 12f_r f_t^2 f_a f_b, -f_s^2 (f_s^2 - 2f_b f_a f_s + 4f_a^2 f_t \\
& - 4f_t f_r), 0, -2f_s (f_a f_s^2 - 2f_b f_r f_s + f_a^2 f_s f_b - 2f_r f_a f_b^2), -2f_s (f_a^3 f_s + 2f_r f_s f_a - 4f_b f_r^2 \\
& - 2f_r f_b f_a^2), -2f_t (f_s^3 - 4f_s f_r f_t + 2f_s f_r f_b^2 - 4f_b f_a f_t f_r), f_s^4 + 3f_b f_a f_s^3 - 4f_s^2 f_r f_b^2 - 8f_s^2 f_r f_t \\
& - 8f_s f_b f_a f_t f_r + 8f_a^2 f_t^2 f_r + 16f_r^2 f_t^2, f_s (3f_s^2 f_a^2 + 2f_s^2 f_r - 4f_b f_a f_r f_s - 4f_a^2 f_t f_r - 8f_r^2 f_t), \\
& 2f_b f_t^2 (f_s^2 - 4f_t f_r), f_t (f_b f_s^3 + 2f_s^2 f_a f_t - 4f_s f_b f_t f_r - 8f_a f_t^2 f_r), -f_s (f_b f_s^3 - f_s^2 f_a f_t \\
& - 4f_s f_b f_t f_r + 4f_a f_t^2 f_r), -f_a f_s^2 (f_s^2 - 4f_t f_r) \Big], \\
& \Big[ 0, 0, 0, 0, 0, 0, 4f_b f_t (f_b f_s - 2f_a f_t), 0, -8f_t^2 (f_b f_s - 2f_a f_t), 0, 4f_t (2f_t f_s f_b + f_s f_b^3 - 4f_t^2 f_a \\
& - 2f_a f_t f_b^2), 4f_t (f_b f_s^2 - 2f_a f_t f_s + f_s f_a f_b^2 - 2f_b f_a^2 f_t), 0, -4f_t^2 f_b (f_b f_s - 2f_a f_t), -4f_a \\
& f_t^2 (f_b f_s - 2f_a f_t), 0, -f_b (f_b f_s^2 - 4f_a f_t f_s + 4f_b f_t f_r), 0, 2f_t (f_b f_s^2 - 4f_a f_t f_s + 4f_b f_t f_r), \\
& -2f_b f_s (f_a f_s - 2f_b f_r), -f_s^2 f_b^3 - 4f_s^2 f_b f_t + 8f_s f_a f_t^2 + 4f_s f_a f_t f_b^2 - 4f_b^3 f_r f_r - f_b^2 f_a f_s^2 + 8 \\
& f_s^2 f_a f_t + 4f_b f_a^2 f_s f_t - 16f_s f_b f_t f_r - 4f_r f_a f_t f_b^2, 0, f_t (f_s^2 f_b^2 + 4f_s^2 f_t - 4f_b f_a f_t f_s - 16f_r f_t^2 + 4 \\
& f_b^2 f_r f_t), -f_t (2f_s^3 - f_b f_a f_s^2 - 8f_s f_r f_t + 4f_s f_a^2 f_t - 4f_b f_a f_t f_r), 0, -2f_s (2f_a f_t f_s + f_s f_a f_b^2 - 2 \\
& f_b^3 f_r - 4f_b f_t f_r), -2f_s (f_a f_s^2 - 2f_b f_r f_s + f_a^2 f_s f_b - 2f_r f_a f_b^2), -2f_t (f_s^2 f_b^2 + 2f_s^2 f_t - 8f_r f_t^2 \\
& - 4f_b^2 f_r f_t), f_b (f_b f_s^3 - 8f_s f_b f_t f_r + 8f_a f_t^2 f_r), f_s (f_s^3 + f_b f_a f_s^2 - 4f_s f_r f_t + 2f_s f_a^2 f_t \\
& - 8f_b f_a f_t f_r), 0, 2f_b f_t^2 (f_s^2 - 4f_t f_r), -f_t (f_b f_s^3 - 2f_s^2 f_a f_t - 4f_s f_b f_t f_r + 8f_a f_t^2 f_r), -f_a f_t f_s ( \\
& f_s^2 - 4f_t f_r) \Big], \\
& \Big[ 0, 0, 0, 0, 0, 0, 0, 0, 0, -8f_t (f_b f_s - 2f_a f_t), 0, -8f_b f_t (f_b f_s - 2f_a f_t), 0, 0, 8f_t^2 (f_b f_s \\
& - 2f_a f_t), 0, 0, 0, 0, 2f_b f_s^2 - 8f_a f_t f_s + 8f_b f_t f_r, 0, 2f_b (f_b f_s^2 - 4f_a f_t f_s + 4f_b f_t f_r), 0, 0, \\
& -2f_t (f_b f_s^2 - 4f_a f_t f_s + 4f_b f_t f_r), 4f_s (f_a f_s - 2f_b f_r), 4f_t (f_s^2 - 4f_t f_r), -2f_s (4f_r f_b^2 - 4f_t f_r \\
& - 2f_b f_a f_s + f_s^2), 0, 4f_b f_t (f_s^2 - 4f_t f_r), -2f_s (f_b f_s^2 + 2f_a f_t f_s - 8f_b f_t f_r), 0, 0, -4f_t^2 (f_s^2 \\
& - 4f_t f_r), 2f_s f_t (f_s^2 - 4f_t f_r) \Big], \\
& \Big[ 0, 0, 4f_a f_t (f_b f_s - 2f_a f_t), 0, 4f_t (f_b f_s^2 - 2f_a f_t f_s + f_s f_a f_b^2 - 2f_b f_a^2 f_t), 0, -f_a (f_b f_s^2 \\
& - 4f_a f_t f_s + 4f_b f_t f_r), 0, -f_b f_s^3 - f_b^2 f_a f_s^2 + 4f_s^2 f_a f_t + 4f_b f_a^2 f_s f_t - 4f_s f_b f_t f_r - 4f_r f_a f_t f_b^2, \\
& -2f_a f_s (f_a f_s - 2f_b f_r), -2f_t (4f_b f_r f_s - 12f_a f_t f_r + f_a f_s^2), -f_s (f_a f_s^2 + 2f_a^2 f_s f_b - 4f_b f_r f_s \\
& - 4f_r f_a f_b^2 + 4f_a f_t f_r), 0, -2f_t (f_s^3 + f_b f_a f_s^2 - 4f_s f_r f_t + 2f_s f_r f_b^2 - 8f_b f_a f_t f_r), f_s (f_s^3 + f_b f_a \\
& f_s^2 - 4f_s f_r f_t - 4f_b f_a f_t f_r), 0, 0, 0, 0, 0, 2f_r (f_b f_s^2 - 4f_a f_t f_s + 4f_b f_t f_r), 0, 0, f_b f_r (f_b f_s^2 \\
& - 4f_a f_t f_s + 4f_b f_t f_r), 0, 0, 4f_r f_s (f_a f_s - 2f_b f_r), 0, 4f_r f_t (f_s^2 - 4f_t f_r), -2f_s f_r (f_s^2 - f_b f_a f_s \\
& - 4f_t f_r + 2f_r f_b^2), 0, 0, 2f_b f_t f_r (f_s^2 - 4f_t f_r), -f_s f_b f_r (f_s^2 - 4f_t f_r), 0 \Big],
\end{aligned}$$

$$\begin{aligned}
& [0, 0, 4f_b f_t (f_b f_s - 2f_a f_t), 0, 4f_t (2f_t f_s f_b + f_s f_b^3 - 4f_t^2 f_a - 2f_a f_t f_b^2), 0, -f_s^2 f_b^2 + 8f_b f_a f_t f_s \\
& - 8f_a^2 f_t^2 - 4f_b^2 f_r f_r, 0, -f_b (-2f_s^2 f_t + f_s^2 f_b^2 - 8f_b f_a f_t f_s + 8f_r f_t^2 + 8f_a^2 f_t^2 + 4f_b^2 f_r f_t), \\
& -2f_b f_s (f_a f_s - 2f_b f_r), -2f_t (5f_b f_s^2 - 8f_a f_t f_s - 4f_b f_t f_r), f_b f_s^3 - 2f_b^2 f_a f_s^2 - 4f_s^2 f_a f_t \\
& - 4f_s f_b f_t f_r + 4f_r f_s f_b^3 + 16f_a f_t^2 f_r, 0, -2f_t (3f_s^2 f_b^2 + 2f_s^2 f_t - 4f_b f_a f_t f_s - 4f_b^2 f_r f_t - 8f_r \\
& f_t^2), f_b^2 f_s^3 + 2f_t f_s^3 - 8f_r f_t f_s f_b^2 - 8f_r f_t^2 f_s + 8f_r f_t^2 f_a f_b, 0, -f_a (f_b f_s^2 - 4f_a f_t f_s + 4f_b f_t f_r), 0, \\
& -f_b f_s^3 - f_b^2 f_a f_s^2 + 4f_s^2 f_a f_t + 4f_b f_a^2 f_s f_t - 4f_s f_b f_t f_r - 4f_r f_a f_t f_b^2, -2f_a f_s (f_a f_s - 2f_b f_r), 2f_b \\
& f_s^3 - 10f_s^2 f_a f_t + 8f_s f_b f_t f_r + 8f_a f_t^2 f_r, -f_a f_s^3 + 6f_s^2 f_b f_r - 2f_a^2 f_s^2 f_b - 12f_r f_a f_t f_s + 4f_r f_a f_s f_b^2 \\
& + 8f_b f_t f_r^2, 0, -2f_t f_s^3 + f_b^2 f_s^3 - 6f_a f_t f_b f_s^2 + 8f_r f_t^2 f_s + 4f_r f_t f_s f_b^2 + 8f_r f_t^2 f_a f_b, f_s^4 + f_b f_a f_s^3 \\
& - 4f_s^2 f_r f_t + f_s^2 f_r f_b^2 - 8f_s f_b f_a f_t f_r + 4f_r^2 f_t f_b^2, 0, 4f_s^2 (f_a f_s - 2f_b f_r), 4f_r f_s (f_a f_s - 2f_b f_r), \\
& 4f_s f_t (f_s^2 - 4f_t f_r), -2f_s^4 + 2f_b f_a f_s^3 + 12f_s^2 f_r f_t - 4f_s^2 f_r f_b^2 - 16f_r^2 f_t^2, -2f_s f_r (f_s^2 - f_b f_a f_s \\
& - 4f_t f_r + 2f_r f_b^2), 0, 2f_s f_b f_t (f_s^2 - 4f_t f_r), -f_b (f_s^4 - 6f_s^2 f_r f_t + 8f_r^2 f_t^2), -f_s f_b f_r (f_s^2 \\
& - 4f_t f_r) ],
\end{aligned}$$

$$\begin{aligned}
& [0, 0, 0, 0, 0, 0, 4f_b f_t (f_b f_s - 2f_a f_t), 0, 4f_t (2f_t f_s f_b + f_s f_b^3 - 4f_t^2 f_a - 2f_a f_t f_b^2), 4f_a f_t (f_b f_s \\
& - 2f_a f_t), -8f_t^2 (f_b f_s - 2f_a f_t), -4f_t (f_b f_s^2 - 2f_a f_t f_s - f_s f_a f_b^2 + 2f_b f_a^2 f_t), 0, -4f_t^2 f_b (f_b f_s \\
& - 2f_a f_t), -4f_s f_b f_t (f_b f_s - 2f_a f_t), 0, -f_b (f_b f_s^2 - 4f_a f_t f_s + 4f_b f_t f_r), 0, -f_s^2 f_b^3 - 2f_s^2 f_b f_t \\
& + 8f_s f_a f_t^2 + 4f_s f_a f_t f_b^2 - 4f_b^3 f_r f_t - 8f_r f_t^2 f_b, -3f_b f_a f_s^2 + 4f_s f_r f_b^2 + 4f_s f_a^2 f_t - 4f_b f_a f_t f_r \\
& - 8f_t^2 (f_a f_s - 2f_b f_r), 2f_b f_s^3 - 3f_b^2 f_a f_s^2 - 8f_s^2 f_a f_t + 4f_b f_a^2 f_s f_t + 4f_r f_s f_b^3 + 8f_s f_b f_t f_r \\
& - 4f_r f_a f_t f_b^2, 0, -f_t (f_s^2 f_b^2 + 4f_s^2 f_t + 4f_b f_a f_t f_s - 12f_b^2 f_r f_t - 16f_r f_t^2), 2f_s (f_s^2 f_b^2 + f_s^2 f_t \\
& - 2f_b f_a f_t f_s - 4f_r f_t^2), -2f_a f_s (f_a f_s - 2f_b f_r), 2f_t (f_a f_s^2 - 4f_b f_r f_s + 4f_a f_t f_r), f_s (3f_a f_s^2 \\
& - 4f_b f_r f_s - 2f_a^2 f_s f_b + 4f_r f_a f_b^2 - 4f_a f_t f_r), 4f_t^2 (f_s^2 - 4f_t f_r), -4f_b f_t f_r (f_b f_s - 2f_a f_t), \\
& -f_s (f_s^3 - 3f_b f_a f_s^2 + 4f_s f_r f_b^2 - 4f_s f_r f_t + 4f_b f_a f_t f_r), 0, 2f_b f_t^2 (f_s^2 - 4f_t f_r), f_s f_b f_t (f_s^2 \\
& - 4f_t f_r), -f_b f_s^2 (f_s^2 - 4f_t f_r) ],
\end{aligned}$$

$$\begin{aligned}
& [0, 0, 0, 0, 0, 0, 0, 0, 0, 4f_b f_t (f_b f_s - 2f_a f_t), 0, 4f_b^2 f_t (f_b f_s - 2f_a f_t), 0, 0, -4f_t^2 f_b (f_b f_s \\
& - 2f_a f_t), 0, 0, 0, 0, -f_b (f_b f_s^2 - 4f_a f_t f_s + 4f_b f_t f_r), 0, -f_b^2 (f_b f_s^2 - 4f_a f_t f_s + 4f_b f_t f_r), 0, \\
& 0, f_b f_t (f_b f_s^2 - 4f_a f_t f_s + 4f_b f_t f_r), -2f_b f_s (f_a f_s - 2f_b f_r), -2f_b f_t (f_s^2 - 4f_t f_r), f_b f_s (4f_r f_b^2 \\
& - 4f_t f_r - 2f_b f_a f_s + f_s^2), 0, -2f_b^2 f_t (f_s^2 - 4f_t f_r), f_b f_s (f_b f_s^2 + 2f_a f_t f_s - 8f_b f_t f_r), 0, 0, 2f_b \\
& f_t^2 (f_s^2 - 4f_t f_r), -f_s f_b f_t (f_s^2 - 4f_t f_r) ],
\end{aligned}$$

$$\begin{aligned}
& [8f_r f_t (f_b f_s - 2f_a f_t), -2f_r (f_b f_s^2 - 4f_a f_t f_s + 4f_b f_t f_r), -4f_r f_s (f_a f_s - 2f_b f_r), -4f_r f_t (f_s^2 \\
& - 2f_b f_a f_s + 4f_a^2 f_t - 4f_t f_r), 2f_r f_s (f_s^2 - 4f_t f_r), 0, 0, -2f_a f_r (f_b f_s^2 - 4f_a f_t f_s + 4f_b f_t f_r), 0,
\end{aligned}$$



$$\begin{aligned}
& 0, -4f_s f_a f_r (f_a f_s - 2f_b f_r), 0, -4f_r f_t (f_a f_s^2 + 2f_b f_r f_s - 8f_a f_t f_r), 2f_s f_a f_r (f_s^2 - 4f_t f_r), 0, \\
& 0, 0, 0, 0, 0, 0, 0, 0, 2f_r^2 (f_b f_s^2 - 4f_a f_t f_s + 4f_b f_t f_r), 0, 0, 0, 0, 0, 4f_s f_r^2 (f_a f_s - 2f_b f_r), 0, 0, \\
& 4f_t f_r^2 (f_s^2 - 4f_t f_r), -2f_s f_r^2 (f_s^2 - 4f_t f_r), 0, 0], \\
& [4f_t f_s (f_b f_s - 2f_a f_t), -f_b f_s^3 + 4f_s^2 f_a f_t + 4f_s f_b f_t f_r - 16f_a f_t^2 f_r - 2f_s^2 (f_a f_s - 2f_b f_r), \\
& -2f_t (f_s^3 - 2f_b f_a f_s^2 - 4f_s f_r f_t + 4f_s f_a^2 f_t - 2f_s f_r f_b^2 + 4f_b f_a f_t f_r), f_s^4 - 4f_s^2 f_r f_t + 4f_s f_b f_a f_t f_r \\
& - 8f_a^2 f_t^2 f_r - 2f_r (f_b f_s^2 - 4f_a f_t f_s + 4f_b f_t f_r), -4f_r f_s (f_a f_s - 2f_b f_r), -f_b f_a f_s^3 - 4f_s^2 f_r f_t - \\
& f_s^2 f_r f_b^2 + 4f_s^2 f_a^2 f_t + 4f_s f_b f_a f_t f_r - 4f_r^2 f_t f_b^2 - 8f_a^2 f_t^2 f_r + 16f_r^2 f_t^2, f_r (2f_s^3 - f_b f_a f_s^2 - 8f_s f_r f_t \\
& + 4f_s f_a^2 f_t - 4f_b f_a f_t f_r), 0, -2f_s (f_s^2 f_a^2 - f_b f_a f_r f_s - 2f_r^2 f_b^2), -2f_s f_a f_r (f_a f_s - 2f_b f_r), \\
& -2f_t (f_a f_s^3 + 5f_s^2 f_b f_r - 12f_r f_a f_t f_s - 4f_b f_t f_r^2), f_s^4 f_a + f_r f_b f_s^3 - 6f_r f_a f_t f_s^2 - 12f_r^2 f_s f_s f_b \\
& + 24f_r^2 f_a f_t^2, f_s f_a f_r (f_s^2 - 4f_t f_r), 0, 0, -f_a f_r (f_b f_s^2 - 4f_a f_t f_s + 4f_b f_t f_r), 0, 0, -2f_s f_a f_r (f_a f_s \\
& - 2f_b f_r), 0, 2f_r (f_b f_s^3 - 5f_s^2 f_a f_t + 4f_s f_b f_t f_r + 4f_a f_t^2 f_r), f_r (f_a f_s^3 + 2f_s^2 f_b f_r - 12f_r f_a f_t f_s \\
& + 8f_b f_t f_r^2), 0, 0, 0, 0, 4f_s^2 f_r (f_a f_s - 2f_b f_r), 4f_s f_r^2 (f_a f_s - 2f_b f_r), 0, 4f_s f_r f_t (f_s^2 - 4f_t f_r), \\
& -2f_r (f_s^4 - 6f_s^2 f_r f_t + 8f_r^2 f_t^2), -2f_s f_r^2 (f_s^2 - 4f_t f_r), 0], \\
& [0, 4f_t f_s (f_b f_s - 2f_a f_t), 8f_r f_t (f_b f_s - 2f_a f_t), 4f_a f_t^2 (f_b f_s - 2f_a f_t), 4f_a f_t f_s (f_b f_s - 2f_a f_t), \\
& -f_s (f_b f_s^2 - 4f_a f_t f_s + 4f_b f_t f_r), -2f_a f_s^3 + 2f_s^2 f_b f_r + 8f_r f_a f_t f_s - 8f_b f_t f_r^2, -f_t (2f_s^3 + f_b f_a f_s^2 \\
& - 4f_s f_a^2 f_t - 8f_s f_r f_t - 4f_s f_r f_b^2 + 12f_b f_a f_t f_r), f_s (f_s^3 - f_b f_a f_s^2 - 4f_s f_r f_t + 4f_s f_a^2 f_t \\
& - 4f_b f_a f_t f_r), -4f_r f_s (f_a f_s - 2f_b f_r), -2f_t (f_s^2 f_a^2 + 2f_s^2 f_r - 4f_b f_a f_r f_s - 8f_r^2 f_t + 4f_a^2 f_t f_r), \\
& -2f_s (f_s^2 f_a^2 - f_s^2 f_r - 2f_b f_a f_r f_s + 4f_r^2 f_t), -2f_t^2 (4f_b f_r f_s - 12f_a f_t f_r + f_a f_s^2), -f_s f_t (f_a f_s^2 \\
& + 8f_b f_r f_s - 20f_a f_t f_r), f_a f_s^2 (f_s^2 - 4f_t f_r), 0, 0, -f_b f_r (f_b f_s^2 - 4f_a f_t f_s + 4f_b f_t f_r), 0, 0, \\
& -f_r (3f_b f_a f_s^2 - 4f_s f_a^2 f_t - 4f_s f_r f_b^2 + 4f_b f_a f_t f_r), 0, -8f_r f_t^2 (f_a f_s - 2f_b f_r), f_r f_s (3f_b f_s^2 \\
& - 8f_a f_t f_s + 4f_b f_t f_r), 0, 0, -2f_s f_a f_r (f_a f_s - 2f_b f_r), 0, 2f_r f_t (f_a f_s^2 - 4f_b f_r f_s + 4f_a f_t f_r), \\
& f_s f_r (5f_a f_s^2 - 8f_b f_r f_s - 4f_a f_t f_r), 0, 4f_r f_t^2 (f_s^2 - 4f_t f_r), 2f_s f_r f_t (f_s^2 - 4f_t f_r), -2f_s^2 f_r (f_s^2 \\
& - 4f_t f_r), 0], \\
& [0, 0, 4f_t f_s (f_b f_s - 2f_a f_t), 0, 4f_a f_t^2 (f_b f_s - 2f_a f_t), 0, -f_s (f_b f_s^2 - 4f_a f_t f_s + 4f_b f_t f_r), 0, \\
& -f_a f_t (f_b f_s^2 - 4f_a f_t f_s + 4f_b f_t f_r), -2f_s^2 (f_a f_s - 2f_b f_r), -2f_t (f_s^3 - 2f_s f_r f_b^2 - 4f_s f_r f_t \\
& + 4f_b f_a f_t f_r), f_s (f_s^3 - 2f_s f_a^2 f_t - 4f_s f_r f_t + 4f_b f_a f_t f_r), 0, -2f_t^2 (4f_b f_r f_s - 12f_a f_t f_r + f_a \\
& f_s^2), f_a f_t f_s (f_s^2 - 4f_t f_r), 0, 0, 0, 0, 0, -f_b f_r (f_b f_s^2 - 4f_a f_t f_s + 4f_b f_t f_r), 0, 0, 2f_r f_t (f_b f_s^2 \\
& - 4f_a f_t f_s + 4f_b f_t f_r), 0, 0, -2f_b f_r f_s (f_a f_s - 2f_b f_r), 0, -2f_b f_t f_r (f_s^2 - 4f_t f_r), f_s f_r (f_b f_s^2 \\
& + 4f_a f_t f_s - 12f_b f_t f_r), 0, 0, 4f_r f_t^2 (f_s^2 - 4f_t f_r), -2f_s f_r f_t (f_s^2 - 4f_t f_r), 0],
\end{aligned}$$

$$\begin{aligned}
& \left[ 8f_t^2 (f_b f_s - 2f_a f_t), 2f_t (3f_b f_s^2 - 4f_a f_t f_s - 4f_b f_t f_r), -4f_t f_s (f_a f_s - 2f_b f_r), 4f_t (-f_s^2 f_t \right. \\
& + 2f_s^2 f_b^2 - 4f_b f_a f_t f_s + 4f_r f_t^2), 2f_t (f_s^3 + 4f_s f_r f_b^2 - 4f_s f_r f_t - 8f_b f_a f_t f_r), -2f_b f_s^3 + 8 \\
& f_s^2 f_a f_t - 16f_a f_t^2 f_r - 4f_s^2 (f_a f_s - 2f_b f_r), -2f_s (f_s^2 f_b^2 + 2f_s^2 f_t - 8f_b f_a f_t f_s + 4f_b^2 f_r f_t - 8f_r f_t^2 \\
& + 8f_a^2 f_t^2), 2f_s^4 - 8f_s^2 f_r f_t - 2f_s^2 f_r f_b^2 + 16f_s f_b f_a f_t f_r - 8f_r^2 f_t f_b^2 - 16f_a^2 f_t^2 f_r, 0, -4f_b \\
& f_s^2 (f_a f_s - 2f_b f_r), -4f_b f_r f_s (f_a f_s - 2f_b f_r), -4f_t f_s (3f_b f_s^2 - 4f_a f_t f_s - 4f_b f_t f_r), 2f_b f_s^4 \\
& - 28f_s^2 f_b f_t f_r + 32f_s f_a f_t^2 f_r + 16f_b f_r^2 f_t^2, 2f_r (f_b f_s^3 - 8f_s f_b f_t f_r + 8f_a f_t^2 f_r), -2f_r (f_b f_s^2 \\
& - 4f_a f_t f_s + 4f_b f_t f_r), -4f_r f_s (f_a f_s - 2f_b f_r), -2f_b f_a f_s^3 - 4f_s^2 f_r f_t + 8f_s^2 f_a^2 f_t - 8f_s f_b f_a f_t f_r \\
& + 16f_r^2 f_t^2, 2f_r (f_s^3 - f_b f_a f_s^2 - 4f_s f_r f_t + 4f_s f_a^2 f_t - 4f_b f_a f_t f_r), 0, -4f_a f_s^2 (f_a f_s - 2f_b f_r), \\
& -4f_s f_a f_r (f_a f_s - 2f_b f_r), 2f_s (4f_s f_b f_t f_r + 8f_a f_t^2 f_r + f_b f_s^3 - 6f_s^2 f_a f_t), 16f_r^2 f_s f_t f_b + 16f_r^2 f_a \\
& f_t^2 + 4f_r f_b f_s^3 - 28f_r f_a f_t f_s^2 + 2f_s^4 f_a^2 2f_r (4f_b f_t f_r^2 + f_s^2 f_b f_r - 8f_r f_a f_t f_s + f_a f_s^3), 0, 0, 0, 4 \\
& f_s^3 (f_a f_s - 2f_b f_r), 8f_s^2 f_r (f_a f_s - 2f_b f_r), 4f_s f_r^2 (f_a f_s - 2f_b f_r), 4f_s^2 f_t (f_s^2 - 4f_t f_r), \\
& -2f_s (16f_r^2 f_t^2 - 8f_s^2 f_r f_t + f_s^4), -4f_r (4f_r^2 f_t^2 - 5f_s^2 f_r f_t + f_s^4), -2f_s f_r^2 (f_s^2 - 4f_t f_r) \Big], \\
& \left[ 0, 8f_t^2 (f_b f_s - 2f_a f_t), 4f_t f_s (f_b f_s - 2f_a f_t), 4f_t^2 f_b (f_b f_s - 2f_a f_t), 4f_s f_b f_t (f_b f_s - 2f_a f_t), \right. \\
& 2f_b f_t (f_s^2 - 4f_t f_r), -f_b f_s^3 + 12f_s f_b f_t f_r - 16f_a f_t^2 f_r f_t (-4f_s^2 f_t + 3f_s^2 f_b^2 + 16f_r f_t^2 - 4f_b^2 f_r f_t \\
& - 8f_a^2 f_t^2), 2f_t f_s^3 - f_b^2 f_s^3 + 8f_a f_t f_b f_s^2 - 8f_r f_t^2 f_s - 8f_s f_a^2 f_t^2 - 8f_r f_t^2 f_a f_b, -2f_s^2 (f_a f_s \\
& - 2f_b f_r), -2f_s f_t (f_s^2 - f_b f_a f_s - 4f_t f_r + 4f_a^2 f_t - 2f_r f_b^2), f_s^4 - 2f_b f_a f_s^3 + 4f_s^2 f_r f_b^2 - 4f_s^2 f_r f_t \\
& + 4f_s f_b f_a f_t f_r - 8f_a^2 f_t^2 f_r - 2f_t^2 (5f_b f_s^2 - 8f_a f_t f_s - 4f_b f_t f_r), -f_t (9f_b f_s^3 - 16f_s^2 f_a f_t \\
& + 4f_s f_b f_t f_r - 16f_a f_t^2 f_r), f_s (f_b f_s^3 - 12f_s f_b f_t f_r + 16f_a f_t^2 f_r), -f_s (f_b f_s^2 - 4f_a f_t f_s \\
& + 4f_b f_t f_r), -2f_a f_s^3 + 2f_s^2 f_b f_r + 8f_r f_a f_t f_s - 8f_b f_t f_r^2, -f_b^2 f_s^3 - 2f_t f_s^3 + 3f_a f_t f_b f_s^2 - 4f_r f_t f_s \\
& f_b^2 + 4f_s f_a^2 f_t^2 + 8f_r f_t^2 f_s - 4f_r f_t^2 f_a f_b f_s^4 - f_b f_a f_s^3 - 4f_s^2 f_r f_t - f_s^2 f_r f_b^2 + 4f_s^2 f_a^2 f_t - 4f_r^2 f_t f_b^2, \\
& -4f_r f_s (f_a f_s - 2f_b f_r), -3f_b f_a f_s^3 + 4f_s^2 f_r f_b^2 - 4f_s^2 f_r f_t + 2f_s^2 f_a^2 f_t + 16f_r^2 f_t^2, -2f_a^2 f_s^3 + 2f_r \\
& f_s^3 + f_r f_a f_s^2 f_b + 4f_r f_a^2 f_s f_t - 8f_r^2 f_t f_s + 4f_s f_r^2 f_b^2 - 4f_r^2 f_a f_t f_b, -2f_t^2 (5f_a f_s^2 - 8f_b f_r f_s \\
& - 4f_a f_t f_r), 3f_b f_s^4 - 9f_s^3 f_a f_t + 4f_s^2 f_b f_t f_r - 4f_s f_a f_t^2 f_r + 16f_b f_r^2 f_t^2, f_s (f_a f_s^3 + 3f_s^2 f_b f_r \\
& - 12f_r f_a f_t f_s + 4f_b f_t f_r^2), 0, -2f_a f_s^2 (f_a f_s - 2f_b f_r), -2f_s f_a f_r (f_a f_s - 2f_b f_r), 2f_s f_t (f_a f_s^2 \\
& - 4f_b f_r f_s + 4f_a f_t f_r), 5f_s^4 f_a - 8f_r f_b f_s^3 - 2f_r f_a f_t f_s^2 - 8f_r^2 f_s f_t f_b + 8f_r^2 f_a f_t^2 f_s f_r (5f_a f_s^2 \\
& - 8f_b f_r f_s - 4f_a f_t f_r), 4f_s f_t^2 (f_s^2 - 4f_t f_r), 2f_t (f_s^4 - 2f_s^2 f_r f_t - 8f_r^2 f_t^2), -2f_s (4f_r^2 f_t^2 - 5 \\
& f_s^2 f_r f_t + f_s^4), -2f_s^2 f_r (f_s^2 - 4f_t f_r) \Big], \\
& \left[ 0, 0, 8f_t^2 (f_b f_s - 2f_a f_t), 0, 4f_t^2 f_b (f_b f_s - 2f_a f_t), 0, 2f_b f_t (f_s^2 - 4f_t f_r), 0, -f_t (f_s^2 f_b^2 \right. \\
& - 8f_b f_a f_t f_s + 8f_a^2 f_t^2 + 4f_b^2 f_r f_t), -4f_t f_s (f_a f_s - 2f_b f_r), 4f_t (f_s^2 f_b^2 - f_s^2 f_t - 2f_b f_a f_t f_s + 4f_r
\end{aligned}$$

$$\begin{aligned}
& f_t^2), 2f_t(f_s^3 - f_b f_a f_s^2 + 4f_s f_r f_b^2 - 4f_s f_r f_t - 4f_b f_a f_t f_r), 0, -2f_t^2(5f_b f_s^2 - 8f_a f_t f_s \\
& - 4f_b f_t f_r), f_t(f_b f_s^3 - 12f_s f_b f_t f_r + 16f_a f_t^2 f_r), 0, -f_s(f_b f_s^2 - 4f_a f_t f_s + 4f_b f_t f_r), 0, \\
& -f_a f_t(f_b f_s^2 - 4f_a f_t f_s + 4f_b f_t f_r), -2f_s^2(f_a f_s - 2f_b f_r), -f_s(f_s^2 f_b^2 + 2f_s^2 f_t - 4f_b f_a f_t f_s \\
& - 8f_r f_t^2 + 4f_b^2 f_r f_t), f_s^4 - 4f_s^2 f_r f_t - 2f_s^2 f_a^2 f_t - f_s^2 f_r f_b^2 + 8f_s f_b f_a f_t f_r - 4f_r^2 f_t f_b^2, 0, 2f_t(f_b f_s^3 \\
& - 5f_s^2 f_a f_t + 4f_s f_b f_t f_r + 4f_a f_t^2 f_r), f_t(f_a f_s^3 + 2f_s^2 f_b f_r - 12f_r f_a f_t f_s + 8f_b f_t f_r^2), 0, -2f_b \\
& f_s^2(f_a f_s - 2f_b f_r), -2f_b f_r f_s(f_a f_s - 2f_b f_r), -2f_s f_b f_t(f_s^2 - 4f_t f_r), f_b f_s^4 + 4f_s^3 f_a f_t - 14 \\
& f_s^2 f_b f_t f_r + 8f_b f_r^2 f_t^2, f_s f_r(f_b f_s^2 + 4f_a f_t f_s - 12f_b f_t f_r), 0, 4f_s f_t^2(f_s^2 - 4f_t f_r), -2f_t(f_s^4 - 6 \\
& f_s^2 f_r f_t + 8f_r^2 f_t^2), -2f_s f_r f_t(f_s^2 - 4f_t f_r) \Big], \\
& \Big[ 0, 0, 0, 0, 0, 8f_t^2(f_b f_s - 2f_a f_t), 8f_t f_s(f_b f_s - 2f_a f_t), 8f_t^2 f_b(f_b f_s - 2f_a f_t), 8f_s f_b f_t(f_b f_s \\
& - 2f_a f_t), 8f_r f_t(f_b f_s - 2f_a f_t), 8f_a f_t^2(f_b f_s - 2f_a f_t), 8f_a f_t f_s(f_b f_s - 2f_a f_t), -8f_t^3(f_b f_s \\
& - 2f_a f_t), -16f_t^2 f_s(f_b f_s - 2f_a f_t), -8f_s^2 f_t(f_b f_s - 2f_a f_t), -2f_t(f_b f_s^2 - 4f_a f_t f_s \\
& + 4f_b f_t f_r), -2f_s^2(f_b f_s - 2f_a f_t), -2f_t(f_s^2 f_b^2 + 2f_s^2 f_t - 4f_b f_a f_t f_s - 8f_r f_t^2 + 4f_b^2 f_r f_t), \\
& -2f_s(4f_b^2 f_r f_t + 4f_r f_t^2 + f_s^2 f_b^2 - 4f_b f_a f_t f_s - f_s^2 f_t), -8f_b f_t f_r^2 + 6f_s^2 f_b f_r + 8f_r f_a f_t f_s - 4f_a \\
& f_s^3, -2f_t(2f_s^3 + 3f_b f_a f_s^2 - 4f_s f_a^2 f_t - 8f_s f_r f_t - 4f_s f_r f_b^2 + 4f_b f_a f_t f_r), 2f_s(f_s^3 - 3f_b f_a f_s^2 \\
& + 4f_s f_r f_b^2 + 4f_s f_a^2 f_t - 4f_s f_r f_t - 4f_b f_a f_t f_r), -2f_t^2(f_b f_s^2 + 4f_a f_t f_s - 12f_b f_t f_r), \\
& 2f_s f_t(12f_b f_t f_r + f_b f_s^2 - 8f_a f_t f_s), 4f_s^3(f_b f_s - 2f_a f_t), -4f_r f_s(f_a f_s - 2f_b f_r), -4f_t(f_s^2 f_a^2 \\
& + f_s^2 f_r - 2f_b f_a f_r f_s - 4f_r^2 f_t), -2f_s(4f_r^2 f_t - 4f_b f_a f_r f_s - f_s^2 f_r + 2f_s^2 f_a^2), -8f_r f_t^2(f_b f_s \\
& - 2f_a f_t), 2f_t f_s(3f_a f_s^2 - 8f_b f_r f_s + 4f_a f_t f_r), 2f_s^2(3f_a f_s^2 - 4f_b f_r f_s - 4f_a f_t f_r), 4f_t^3(f_s^2 \\
& - 4f_t f_r), 6f_s f_t^2(f_s^2 - 4f_t f_r), 0, -2f_s^3(f_s^2 - 4f_t f_r) \Big], \\
& \Big[ 0, 0, 0, 0, 0, 0, 8f_t^2(f_b f_s - 2f_a f_t), 0, 4f_t^2 f_b(f_b f_s - 2f_a f_t), 4f_t f_s(f_b f_s - 2f_a f_t), 4 \\
& f_t^2 f_b(f_b f_s - 2f_a f_t), 4f_t(f_s^2 f_b^2 - f_b f_a f_t f_s - 2f_a^2 f_t^2), 0, -8f_t^3(f_b f_s - 2f_a f_t), -8f_t^2 f_s(f_b f_s \\
& - 2f_a f_t), 0, -2f_t(f_b f_s^2 - 4f_a f_t f_s + 4f_b f_t f_r), 0, -f_b f_t(f_b f_s^2 - 4f_a f_t f_s + 4f_b f_t f_r), -f_b f_s(f_s^2 \\
& - 4f_t f_r), -f_t(f_s^2 f_b^2 + 4f_s^2 f_t - 4f_b f_a f_t f_s - 16f_r f_t^2 + 4f_b^2 f_r f_t), 2f_t f_s^3 - f_b^2 f_s^3 + f_a f_t f_b f_s^2 \\
& - 8f_r f_t^2 f_s + 4f_s f_a^2 f_t - 4f_r f_t^2 f_a f_b, 0, -8f_t^3(f_a f_s - 2f_b f_r), f_t f_s(3f_b f_s^2 - 8f_a f_t f_s \\
& + 4f_b f_t f_r), -2f_s^2(f_a f_s - 2f_b f_r), -2f_t f_s(f_s^2 + f_b f_a f_s - 2f_r f_b^2 - 4f_t f_r), f_s(f_s^3 - 2f_b f_a f_s^2 \\
& - 2f_s f_a^2 f_t - 4f_s f_r f_t + 4f_s f_r f_b^2 + 4f_b f_a f_t f_r), -2f_b f_t^2(f_s^2 - 4f_t f_r), -f_t(f_b f_s^3 - 2f_s^2 f_a f_t \\
& + 4f_s f_b f_t f_r - 8f_a f_t^2 f_r), f_s(f_b f_s^3 + 5f_s^2 f_a f_t - 12f_s f_b f_t f_r - 4f_a f_t^2 f_r), 0, 4f_t^3(f_s^2 - 4f_t f_r), \\
& 2f_s f_t^2(f_s^2 - 4f_t f_r), -2f_s^2 f_t(f_s^2 - 4f_t f_r) \Big], \\
& \Big[ 0, 0, 0, 0, 0, 0, 0, 0, 0, 8f_t^2(f_b f_s - 2f_a f_t), 0, 8f_t^2 f_b(f_b f_s - 2f_a f_t), 0, 0, -8f_t^3(f_b f_s
\end{aligned}$$

$$\begin{aligned}
& -2f_a f_t), 0, 0, 0, 0, -2f_t (f_b f_s^2 - 4f_a f_t f_s + 4f_b f_t f_r), 0, -2f_b f_t (f_b f_s^2 - 4f_a f_t f_s \\
& + 4f_b f_t f_r), 0, 0, 2f_t^2 (f_b f_s^2 - 4f_a f_t f_s + 4f_b f_t f_r), -4f_t f_s (f_a f_s - 2f_b f_r), -4f_t^2 (f_s^2 \\
& - 4f_t f_r), 2f_s f_t (4f_r f_b^2 - 4f_t f_r - 2f_b f_a f_s + f_s^2), 0, -4f_b f_t^2 (f_s^2 - 4f_t f_r), 2f_t f_s (f_b f_s^2 \\
& + 2f_a f_t f_s - 8f_b f_t f_r), 0, 0, 4f_t^3 (f_s^2 - 4f_t f_r), -2f_s f_t^2 (f_s^2 - 4f_t f_r) \Big], \\
& [4f_s (f_b f_s - 2f_a f_t), 2f_a f_s^2 - 8f_b f_r f_s + 8f_a f_t f_r - 8f_r (f_a f_s - 2f_b f_r), -2f_s (f_s^2 - 2f_b f_a f_s \\
& + 4f_a^2 f_t - 4f_t f_r), 4f_r (f_s^2 - 4f_t f_r), 0, 0, 2f_a (f_a f_s^2 - 4f_b f_r f_s + 4f_a f_t f_r), 0, 0, -8f_a f_r (f_a f_s \\
& - 2f_b f_r), 0, -2f_s (f_a f_s^2 + 2f_b f_r f_s - 8f_a f_t f_r), 4f_a f_r (f_s^2 - 4f_t f_r), 0, 0, 0, 0, 0, 0, 0, \\
& -2f_r (f_a f_s^2 - 4f_b f_r f_s + 4f_a f_t f_r), 0, 0, 0, 0, 0, 8f_r^2 (f_a f_s - 2f_b f_r), 0, 0, 2f_r f_s (f_s^2 - 4f_t f_r), \\
& -4f_r^2 (f_s^2 - 4f_t f_r), 0, 0 \Big], \\
& [0, 4f_s (f_b f_s - 2f_a f_t), 0, 2f_b f_s (f_b f_s - 2f_a f_t), 2f_a f_s (f_b f_s - 2f_a f_t), 2f_a f_s^2 - 8f_b f_r f_s \\
& + 8f_a f_t f_r - 8f_r (f_a f_s - 2f_b f_r), -2f_s^3 + 3f_b f_a f_s^2 + 8f_s f_r f_t - 4f_s f_r f_b^2 - 4f_s f_a^2 f_t \\
& + 4f_b f_a f_t f_r f_s^2 f_a^2 + 4f_s^2 f_r - 4f_b f_a f_r f_s + 4f_a^2 f_t f_r - 16f_r^2 f_r, 0, -4f_b f_r (f_a f_s - 2f_b f_r), \\
& -4f_a f_r (f_a f_s - 2f_b f_r), -f_s (3f_b f_s^2 - 4f_a f_t f_s - 4f_b f_t f_r), -f_a f_s^3 - 2f_s^2 f_b f_r + 12f_r f_a f_t f_s \\
& - 8f_b f_t f_r^2, 2f_a f_r (f_s^2 - 4f_t f_r), 0, 0, f_a (f_a f_s^2 - 4f_b f_r f_s + 4f_a f_t f_r), 0, 0, -4f_a f_r (f_a f_s \\
& - 2f_b f_r), 0, -2f_s^2 (f_a f_s - 2f_b f_r), 8f_r^2 (f_b f_s - 2f_a f_t), 0, 0, 0, 0, 4f_r f_s (f_a f_s - 2f_b f_r), 8 \\
& f_r^2 (f_a f_s - 2f_b f_r), 0, f_s^2 (f_s^2 - 4f_t f_r), 0, -4f_r^2 (f_s^2 - 4f_t f_r), 0 \Big], \\
& [0, 0, 4f_s (f_b f_s - 2f_a f_t), 0, 2f_b f_s (f_b f_s - 2f_a f_t), 0, 2f_a f_s^2 - 8f_b f_r f_s + 8f_a f_t f_r, 0, f_b (f_a f_s^2 \\
& - 4f_b f_r f_s + 4f_a f_t f_r), -8f_r (f_a f_s - 2f_b f_r), -2f_s (f_s^2 - f_b f_a f_s - 4f_t f_r + 2f_a^2 f_t), 4f_r (f_s^2 \\
& - f_b f_a f_s - 4f_t f_r + 2f_r f_b^2), 0, -f_s (3f_b f_s^2 - 4f_a f_t f_s - 4f_b f_t f_r), 2f_b f_r (f_s^2 - 4f_t f_r), 0, 0, 0, \\
& 0, 0, f_a (f_a f_s^2 - 4f_b f_r f_s + 4f_a f_t f_r), 0, 0, -f_s (f_a f_s^2 - 4f_b f_r f_s + 4f_a f_t f_r), 0, 0, -4f_a f_r (f_a f_s \\
& - 2f_b f_r), 0, -f_a f_s (f_s^2 - 4f_t f_r), 2f_r (3f_a f_s^2 - 4f_b f_r f_s - 4f_a f_t f_r), 0, 0, f_s^2 (f_s^2 - 4f_t f_r), \\
& -2f_r f_s (f_s^2 - 4f_t f_r), 0 \Big], \\
& [-2f_a f_s (f_b f_s - 2f_a f_t), -f_a (f_a f_s^2 - 4f_b f_r f_s + 4f_a f_t f_r), 4f_a f_r (f_a f_s - 2f_b f_r), f_a f_s (f_s^2 \\
& - 2f_b f_a f_s + 4f_a^2 f_t - 4f_t f_r), -2f_a f_r (f_s^2 - 4f_t f_r), 0, 0, -f_a^2 (f_a f_s^2 - 4f_b f_r f_s + 4f_a f_t f_r), 0, \\
& 0, 4f_a^2 f_r (f_a f_s - 2f_b f_r), 0, f_a f_s (f_a f_s^2 + 2f_b f_r f_s - 8f_a f_t f_r), -2f_a^2 f_r (f_s^2 - 4f_t f_r), 0, 0, 0, 0, \\
& 0, 0, 0, 0, f_a f_r (f_a f_s^2 - 4f_b f_r f_s + 4f_a f_t f_r), 0, 0, 0, 0, 0, -4f_a f_r^2 (f_a f_s - 2f_b f_r), 0, 0, \\
& -f_s f_a f_r (f_s^2 - 4f_t f_r), 2f_a f_r^2 (f_s^2 - 4f_t f_r), 0, 0 \Big], \\
& [-2f_b f_s (f_b f_s - 2f_a f_t), -3f_b f_a f_s^2 + 4f_s f_r f_b^2 + 4f_s f_a^2 f_t - 4f_b f_a f_t f_r - 4f_b f_r (f_a f_s - 2f_b f_r), \\
& f_s (3f_b f_s^2 - 2f_s f_a f_b^2 - 4f_a f_t f_s - 4f_b f_t f_r + 4f_b f_a^2 f_t), 2f_r (f_b f_s^2 - 4f_a f_t f_s + 4f_b f_t f_r),
\end{aligned}$$

$$\begin{aligned}
& -f_a (f_a f_s^2 - 4f_b f_r f_s + 4f_a f_t f_r), 4f_a f_r (f_a f_s - 2f_b f_r), 2f_a f_s^3 - 8f_s^2 f_b f_r - 3f_a^2 f_s^2 f_b \\
& + 4f_r f_a f_s f_b^2 + 4f_a^3 f_s f_t + 8f_r f_a f_t f_s - 4f_r f_b f_a^2 f_r - 8f_r^2 (f_b f_s - 2f_a f_t), 0, -4f_r (f_a f_s^2 - \\
& f_a^2 f_s f_b - 2f_b f_r f_s + 2f_r f_a f_b^2), -8f_r^2 (f_a f_s - 2f_b f_r), -f_s (f_s^3 - 3f_b f_a f_s^2 - 4f_s f_r f_t + 4f_s f_a^2 f_t \\
& + 4f_b f_a f_t f_r), -4f_a f_t f_r (f_a f_s - 2f_b f_r), 4f_r^2 (f_s^2 - 4f_t f_r), 0, 0, -f_s^2 f_a^3 - 2f_s^2 f_a f_r + 8f_s f_b f_r^2 \\
& + 4f_s f_b f_a^2 f_r - 4f_a^3 f_t f_r - 8f_a f_t f_r^2, 0, 0, 4f_r (f_a^3 f_s + 2f_r f_s f_a - 4f_b f_r^2 - 2f_r f_b f_a^2), 0, 2f_s (f_s^2 \\
& f_a^2 + f_s^2 f_r - 2f_b f_a f_r f_s - 4f_r^2 f_t), -f_r (f_s^2 f_a^2 + 4f_s^2 f_r + 4f_b f_a f_r f_s - 16f_r^2 f_t - 12f_a^2 f_t f_r), 0, 0, \\
& 0, 0, -4f_s f_a f_r (f_a f_s - 2f_b f_r), -4f_a f_r^2 (f_a f_s - 2f_b f_r), 0, -f_a f_s^2 (f_s^2 - 4f_t f_r), f_s f_a f_r (f_s^2 \\
& - 4f_t f_r), 2f_a f_r^2 (f_s^2 - 4f_t f_r), 0], \\
& [0, -2f_b f_s (f_b f_s - 2f_a f_t), -2f_a f_s (f_b f_s - 2f_a f_t), 4f_t f_s (f_b f_s - 2f_a f_t), 4f_s^2 (f_b f_s - 2f_a f_t), \\
& -f_b (f_a f_s^2 - 4f_b f_r f_s + 4f_a f_t f_r), -f_s^2 f_a^2 + 8f_b f_a f_r f_s - 8f_r^2 f_b^2 - 4f_a^2 f_t f_r, -f_b f_s^3 + 6f_s^2 f_a f_t \\
& - 2f_b^2 f_a f_s^2 - 12f_s f_b f_t f_r + 4f_b f_a^2 f_s f_t + 8f_a f_t^2 f_r, 2f_a f_s^3 - 10f_s^2 f_b f_r + 8f_r f_a f_t f_s + 8f_b f_t f_r^2, \\
& 4f_a f_r (f_a f_s - 2f_b f_r), f_a f_s^3 - 4f_s^2 f_b f_r - 2f_a^2 f_s^2 f_b - 4f_r f_a f_t f_s + 4f_a^3 f_s f_t + 16f_b f_t f_r^2, \\
& -2f_r (5f_a f_s^2 - 8f_b f_r f_s - 4f_a f_t f_r), -2f_t f_s (f_s^2 - f_b f_a f_s - 4f_t f_r + 2f_a^2 f_t), -2f_s^4 + 2f_b f_a f_s^3 \\
& + 12f_s^2 f_r f_t - 4f_s^2 f_a^2 f_t - 16f_r^2 f_t^2, 4f_r f_s (f_s^2 - 4f_t f_r), 0, 0, -f_a f_s^3 + 4f_s^2 f_b f_r - f_a^2 f_s^2 f_b \\
& + 4f_r f_a f_s f_b^2 - 4f_r f_a f_t f_s - 4f_r f_b f_a^2 f_r, 0, 0, -f_a (f_s^2 f_a^2 - 2f_s^2 f_r - 8f_b f_a f_r f_s + 8f_r^2 f_b^2 + 8f_r^2 f_t \\
& + 4f_a^2 f_t f_r), 0, f_s^4 + f_b f_a f_s^3 - 4f_s^2 f_r f_t + f_s^2 f_a^2 f_t - 8f_s f_b f_a f_t f_r + 4f_a^2 f_t^2 f_r, f_a^2 f_s^3 - 2f_r f_s^3 \\
& - 6f_r f_a f_s^2 f_b + 8f_r^2 f_t f_s + 4f_r f_a^2 f_s f_t + 8f_r^2 f_a f_t f_b, 0, 0, 4f_r (f_a^3 f_s + 2f_r f_s f_a - 4f_b f_r^2 - 2f_r f_b \\
& f_a^2), 0, 2f_r f_s^3 + f_a^2 f_s^3 - 8f_r^2 f_t f_s - 8f_r f_a^2 f_s f_t + 8f_r^2 f_a f_t f_b, -2f_r (3f_s^2 f_a^2 + 2f_s^2 f_r - 4f_b f_a f_r f_s \\
& - 4f_a^2 f_t f_r - 8f_r^2 f_t), 0, -f_a f_t f_s (f_s^2 - 4f_t f_r), -f_a (f_s^4 - 6f_s^2 f_r f_t + 8f_r^2 f_t^2), 2f_s f_a f_r (f_s^2 \\
& - 4f_t f_r), 0], \\
& [0, 0, -2f_b f_s (f_b f_s - 2f_a f_t), 0, 4f_t f_s (f_b f_s - 2f_a f_t), 0, -f_b (f_a f_s^2 - 4f_b f_r f_s + 4f_a f_t f_r), 0, \\
& 2f_t (f_a f_s^2 - 4f_b f_r f_s + 4f_a f_t f_r), 4f_b f_r (f_a f_s - 2f_b f_r), -f_s (f_b f_s^2 + 2f_s f_a f_b^2 - 4f_a f_t f_s - 4f_b \\
& f_a^2 f_t + 4f_b f_t f_r), -2f_r (f_b f_s^2 + 4f_a f_t f_s - 12f_b f_t f_r), 0, -2f_t f_s (f_s^2 - f_b f_a f_s - 4f_t f_r + 2f_a^2 f_t), \\
& 4f_r f_t (f_s^2 - 4f_t f_r), 0, 0, 0, 0, 0, -f_a f_s^3 + 4f_s^2 f_b f_r - f_a^2 f_s^2 f_b + 4f_r f_a f_s f_b^2 - 4f_r f_a f_t f_s - 4f_r f_b \\
& f_a^2 f_r, 0, 0, f_a f_t (f_a f_s^2 - 4f_b f_r f_s + 4f_a f_t f_r), 0, 0, 4f_r (f_a f_s^2 - 2f_b f_r f_s + f_a^2 f_s f_b - 2f_r f_a f_b^2), 0, \\
& f_s (f_s^3 + f_b f_a f_s^2 - 4f_s f_r f_t - 4f_b f_a f_t f_r), -2f_r (f_s^3 + f_b f_a f_s^2 - 4f_s f_r f_t + 2f_s f_a^2 f_t - 8f_b f_a f_t f_r), \\
& 0, 0, -f_a f_t f_s (f_s^2 - 4f_t f_r), 2f_a f_t f_r (f_s^2 - 4f_t f_r), 0], \\
& [0, 0, 0, 0, 0, 4f_s (f_b f_s - 2f_a f_t), 0, 4f_b f_s (f_b f_s - 2f_a f_t), 4f_a f_s (f_b f_s - 2f_a f_t), 0, 0, 0, \\
& -4f_t f_s (f_b f_s - 2f_a f_t), -4f_s^2 (f_b f_s - 2f_a f_t), -4f_r f_s (f_b f_s - 2f_a f_t), 2f_a f_s^2 - 8f_b f_r f_s
\end{aligned}$$

$$\begin{aligned}
& + 8f_a f_t f_r - 8f_r (f_a f_s - 2f_b f_r), -2f_s^3 + 2f_b f_a f_s^2 - 8f_s f_r f_b^2 + 8f_s f_r f_t + 8f_b f_a f_t f_r - 16f_r^2 f_t \\
& - 8f_b f_a f_r f_s + 8f_a^2 f_t f_r + 4f_s^2 f_r + 2f_s^2 f_a^2, 0, -8f_b f_r (f_a f_s - 2f_b f_r), -8f_a f_r (f_a f_s - 2f_b f_r), \\
& 16f_s f_b f_t f_r - 8f_a f_t^2 f_r - 2f_b f_s^3 - 2f_s^2 f_a f_r - 16f_b f_t f_r^2 + 12f_s^2 f_b f_r - 4f_a f_s^3, 2f_r (4f_b f_r f_s \\
& - 12f_a f_t f_r + f_a f_s^2), 0, 0, 0, 8f_r f_t (f_a f_s - 2f_b f_r), 8f_r f_s (f_a f_s - 2f_b f_r), 8f_r^2 (f_a f_s - 2f_b f_r), \\
& 2f_s f_t (f_s^2 - 4f_t f_r), 16f_r^2 f_t^2 - 12f_s^2 f_r f_t + 2f_s^4, -2f_r f_s (f_s^2 - 4f_t f_r), -4f_r^2 (f_s^2 - 4f_t f_r) \Big], \\
& \Big[ 0, 0, 0, 0, 0, 0, 4f_s (f_b f_s - 2f_a f_t), 0, 2f_b f_s (f_b f_s - 2f_a f_t), 0, 2f_b f_s (f_b f_s - 2f_a f_t), \\
& 2f_a f_s (f_b f_s - 2f_a f_t), 0, -4f_t f_s (f_b f_s - 2f_a f_t), -2f_s^2 (f_b f_s - 2f_a f_t), 0, 2f_a f_s^2 - 8f_b f_r f_s \\
& + 8f_a f_t f_r, 0, f_b (f_a f_s^2 - 4f_b f_r f_s + 4f_a f_t f_r), -8f_r (f_a f_s - 2f_b f_r), -2f_s^3 + f_b f_a f_s^2 + 8f_s f_r f_t \\
& - 4f_s f_r f_b^2 + 4f_b f_a f_t f_r f_s^2 f_a^2 + 4f_s^2 f_r - 8f_b f_a f_r f_s - 16f_r^2 f_t + 4f_a^2 f_t f_r + 8f_r^2 f_b^2, 0, -f_b f_s^3 \\
& - 2f_s^2 f_a f_t + 12f_s f_b f_t f_r - 8f_a f_t^2 f_r - f_a f_s^3 + 6f_s^2 f_b f_r - 4f_r f_a f_t f_s - 8f_b f_t f_r^2, 0, -4f_b f_r (f_a f_s \\
& - 2f_b f_r), -4f_a f_r (f_a f_s - 2f_b f_r), -f_b f_s (f_s^2 - 4f_t f_r), -f_a f_s^3 + 2f_s^2 f_b f_r + 12f_r f_a f_t f_s \\
& - 24f_b f_t f_r^2, 2f_r (3f_a f_s^2 - 4f_b f_r f_s - 4f_a f_t f_r), 0, 2f_s f_t (f_s^2 - 4f_t f_r), 16f_r^2 f_t^2 - 8f_s^2 f_r f_t + \\
& f_s^4, -2f_r f_s (f_s^2 - 4f_t f_r) \Big], \\
& \Big[ 0, -2f_a f_s (f_b f_s - 2f_a f_t), 0, -2f_s (f_b f_s^2 - 2f_a f_t f_s + f_s f_a f_b^2 - 2f_b f_a^2 f_t), -2f_s (f_a^2 f_s f_b \\
& + 2f_b f_r f_s - 4f_a f_t f_r - 2f_a^3 f_t), -f_a (f_a f_s^2 - 4f_b f_r f_s + 4f_a f_t f_r), 4f_a f_r (f_a f_s - 2f_b f_r), 8 \\
& f_s^2 f_b f_r - f_a^2 f_s^2 f_b - 16f_r f_a f_t f_s + 4f_r f_a f_s f_b^2 - 4f_r f_b f_a^2 f_r - 4f_s^2 f_a f_r - f_s^2 f_a^3 + 8f_s f_b f_r^2 + 4f_s f_b \\
& f_a^2 f_r - 4f_a^3 f_t f_r, 0, 4f_r (f_a f_s^2 - 2f_b f_r f_s + f_a^2 f_s f_b - 2f_r f_a f_b^2), 4f_r (f_a^3 f_s + 2f_r f_s f_a - 4f_b f_r^2 \\
& - 2f_r f_b f_a^2), f_s (f_s^3 + f_b f_a f_s^2 - 4f_s f_r f_t + 2f_s f_r f_b^2 - 8f_b f_a f_t f_r), f_a (8f_b f_t f_r^2 - 8f_r f_a f_t f_s + f_a \\
& f_s^3), -2f_r (f_s^2 f_a^2 + 2f_s^2 f_r - 4f_a^2 f_t f_r - 8f_r^2 f_t), 0, 0, 2f_r (f_a f_s^2 - 4f_b f_r f_s + 4f_a f_t f_r), 0, 0, -8 \\
& f_r^2 (f_a f_s - 2f_b f_r), 0, -f_r (2f_s^3 - f_b f_a f_s^2 - 8f_s f_r f_t + 4f_s f_r f_b^2 - 4f_b f_a f_t f_r), f_r (f_s^2 f_a^2 + 4f_s^2 f_r \\
& - 4f_b f_a f_r f_s + 4f_a^2 f_t f_r - 16f_r^2 f_t), 0, 0, 0, 0, -4f_b f_r^2 (f_a f_s - 2f_b f_r), -4f_a f_r^2 (f_a f_s \\
& - 2f_b f_r), 0, -f_s f_b f_r (f_s^2 - 4f_t f_r), -f_r (f_a f_s^3 - 2f_s^2 f_b f_r - 4f_r f_a f_t f_s + 8f_b f_t f_r^2), 2f_a f_r^2 (f_s^2 \\
& - 4f_t f_r), 0 \Big], \\
& \Big[ 0, -2f_b f_s (f_b f_s - 2f_a f_t), 0, -2f_s (2f_t f_s f_b + f_s f_b^3 - 4f_t^2 f_a - 2f_a f_t f_b^2), -2f_s (f_b f_s^2 \\
& - 2f_a f_t f_s + f_s f_a f_b^2 - 2f_b f_a^2 f_t), -3f_b f_a f_s^2 + 4f_s f_r f_b^2 + 4f_s f_a^2 f_t - 4f_b f_a f_t f_r, 4f_b f_r (f_a f_s \\
& - 2f_b f_r), 3f_b f_s^3 - 6f_s^2 f_a f_t - 3f_b^2 f_a f_s^2 + 4f_r f_s f_b^3 + 4f_b f_a^2 f_s f_t + 4f_s f_b f_t f_r - 8f_a f_t^2 f_r \\
& - 4f_r f_a f_t f_b^2, -f_a f_s^3 + 2f_s^2 f_b f_r - 3f_a^2 f_s^2 f_b + 4f_r f_a f_s f_b^2 + 4f_a^3 f_s f_t - 4f_r f_a f_t f_s - 4f_r f_b f_a^2 f_t \\
& + 8f_b f_t f_r^2, 0, 4f_r (2f_a f_t f_s + f_s f_a f_b^2 - 2f_b^3 f_r - 4f_b f_t f_r), 4f_r (f_a f_s^2 - 2f_b f_r f_s + f_a^2 f_s f_b \\
& - 2f_r f_a f_b^2), f_s (3f_s^2 f_b^2 + 2f_s^2 f_t - 4f_b f_a f_t f_s - 4f_b^2 f_r f_t - 8f_r f_t^2), f_s^4 + 3f_b f_a f_s^3 - 8f_s^2 f_r f_t
\end{aligned}$$

$$\begin{aligned}
& -4f_s^2 f_a^2 f_t - 8f_s f_b f_a f_t f_r + 16f_r^2 f_t^2 + 8f_r^2 f_t f_b^2, -2f_r (f_s^3 - 4f_s f_r f_t + 2f_s f_a^2 f_t - 4f_b f_a f_t f_r), \\
& -f_a (f_a f_s^2 - 4f_b f_r f_s + 4f_a f_t f_r), 4f_a f_r (f_a f_s - 2f_b f_r), 2f_a f_s^3 - 4f_s^2 f_b f_r - f_a^2 f_s^2 f_b + 4f_r f_a f_s \\
& f_b^2 - 4f_r f_b f_a^2 f_r - f_a (f_s^2 f_a + 2f_s^2 f_r - 4f_b f_a f_r f_s - 8f_r^2 f_t + 4f_a^2 f_t f_r), 0, -4f_r (f_a f_s^2 - f_a^2 f_s f_b \\
& - 2f_b f_r f_s + 2f_r f_a f_b^2), 4f_a^2 f_r (f_a f_s - 2f_b f_r), -f_s^2 (4f_r f_b^2 - 4f_t f_r - 2f_b f_a f_s + f_s^2), 2f_a^2 f_s^3 \\
& + 2f_r f_s^3 - 5f_r f_a f_s^2 f_b - 8f_r^2 f_t f_s - 4f_s f_r^2 f_b^2 + 12f_r^2 f_a f_t f_b, -f_a f_r (4f_b f_r f_s - 12f_a f_t f_r + f_a \\
& f_s^2), 0, 0, 0, -4f_b f_r f_s (f_a f_s - 2f_b f_r), -4f_r (f_s^2 f_a^2 - f_b f_a f_r f_s - 2f_r^2 f_b^2), -4f_a f_r^2 (f_a f_s \\
& - 2f_b f_r), -f_b f_s^2 (f_s^2 - 4f_t f_r), -f_s (f_a f_s^3 - f_s^2 f_b f_r - 4f_r f_a f_t f_s + 4f_b f_t f_r^2), f_r (f_a f_s^3 + 2 \\
& f_s^2 f_b f_r - 4f_r f_a f_t f_s - 8f_b f_t f_r^2), 2f_a f_r^2 (f_s^2 - 4f_t f_r) \Big], \\
& \Big[ 0, 0, 0, 0, 0, -2f_b f_s (f_b f_s - 2f_a f_t), -2f_a f_s (f_b f_s - 2f_a f_t), -2f_s f_b^2 (f_b f_s - 2f_a f_t), 2f_s (f_b \\
& f_s^2 - 2f_a f_t f_s - f_s f_a f_b^2 + 2f_b f_a^2 f_t), 0, -2f_s (f_b f_s^2 - 2f_a f_t f_s + f_s f_a f_b^2 - 2f_b f_a^2 f_t), -2f_s (f_a^2 f_s f_b \\
& + 2f_b f_r f_s - 4f_a f_t f_r - 2f_a^3 f_t), 2f_s f_b f_t (f_b f_s - 2f_a f_t), 2f_s (f_s^2 f_b^2 - f_b f_a f_t f_s - 2f_a^2 f_t^2), 2f_a \\
& f_s^2 (f_b f_s - 2f_a f_t), -f_b (f_a f_s^2 - 4f_b f_r f_s + 4f_a f_t f_r), -f_s^2 f_a^2 + 8f_b f_a f_r f_s - 8f_r^2 f_b^2 - 4f_a^2 f_t f_r \\
& f_b (f_s^3 - f_b f_a f_s^2 + 4f_s f_r f_b^2 - 4f_s f_r f_t - 4f_b f_a f_t f_r), f_a f_s^3 - 6f_s^2 f_b f_r - f_a^2 f_s^2 f_b + 4f_r f_a f_s f_b^2 \\
& + 4f_r f_a f_t f_s - 4f_r f_b f_a^2 f_t + 8f_b f_t f_r^2, 4f_a f_r (f_a f_s - 2f_b f_r), 4f_s^2 f_b f_r - f_a^2 f_s^2 f_b + 8f_r f_a f_s f_b^2 \\
& - 8f_r f_a f_t f_s - 4f_r f_b f_a^2 f_t - 8f_b^3 f_r^2, -f_s^2 f_a^3 - 8f_s^2 f_a f_r + 16f_s f_b f_r^2 + 8f_s f_b f_a^2 f_r - 4f_a^3 f_t f_r \\
& - 8f_a^2 f_b^2 f_r^2, f_b (f_b f_s^3 + f_s^2 f_a f_t - 8f_s f_b f_t f_r + 4f_a^2 f_t f_r), -f_s^4 + 2f_b f_a f_s^3 + f_s^2 f_a^2 f_t - 6f_s^2 f_r f_b^2 \\
& + 4f_s^2 f_r f_t - 4f_s f_b f_a f_t f_r + 4f_a^2 f_t^2 f_r + 8f_r^2 f_t f_b^2, 2f_r f_s^3 + f_a^2 f_s^3 - 6f_r f_a f_s^2 f_b + 4f_r f_a^2 f_s f_t - 8 \\
& f_r^2 f_t f_s + 8f_r^2 f_a f_t f_b, 0, 4f_r (f_a f_s^2 - 2f_b f_r f_s + f_a^2 f_s f_b - 2f_r f_a f_b^2), 4f_r (f_a^3 f_s + 2f_r f_s f_a - 4f_b f_r^2 \\
& - 2f_r f_b f_a^2), f_s^4 + f_b f_a f_s^3 - 4f_s^2 f_r f_t - 8f_s f_b f_a f_t f_r + 8f_r^2 f_t f_b^2, f_a^2 f_s^3 - 6f_r f_a f_s^2 f_b + 8f_s f_r^2 f_b^2 \\
& - 8f_r f_a^2 f_s f_t + 16f_r^2 f_a f_t f_b, -2f_r (3f_s^2 f_a^2 + 2f_s^2 f_r - 4f_b f_a f_r f_s - 4f_a^2 f_t f_r - 8f_r^2 f_t), -f_s f_b f_t ( \\
& f_s^2 - 4f_t f_r), -f_b f_s^4 - f_s^3 f_a f_t + 6f_s^2 f_b f_t f_r + 4f_s f_a f_t^2 f_r - 8f_b f_r^2 f_t^2, -f_s^4 f_a + 2f_r f_b f_s^3 + 6f_r f_a f_t \\
& f_s^2 - 8f_r^2 f_s f_t f_b - 8f_r^2 f_a f_t^2, 2f_s f_a f_r (f_s^2 - 4f_t f_r) \Big], \\
& \Big[ 0, 0, 0, 0, 0, 0, -2f_b f_s (f_b f_s - 2f_a f_t), 0, 4f_t f_s (f_b f_s - 2f_a f_t), 0, -2f_s (2f_t f_s f_b + f_s f_b^3 - 4 \\
& f_t^2 f_a - 2f_a f_t f_b^2), -2f_s (f_b f_s^2 - 2f_a f_t f_s + f_s f_a f_b^2 - 2f_b f_a^2 f_t), 0, 2f_s f_b f_t (f_b f_s - 2f_a f_t), \\
& 2f_a f_t f_s (f_b f_s - 2f_a f_t), 0, -f_b (f_a f_s^2 - 4f_b f_r f_s + 4f_a f_t f_r), 0, 2f_t (f_a f_s^2 - 4f_b f_r f_s \\
& + 4f_a f_t f_r), 4f_b f_r (f_a f_s - 2f_b f_r), f_b f_s^3 - 2f_s^2 f_a f_t - f_b^2 f_a f_s^2 + 4f_r f_s f_b^3 + 4f_s f_b f_t f_r - 8f_a f_t^2 f_r \\
& - 4f_r f_a f_t f_b^2, -f_a f_s^3 + 2f_s^2 f_b f_r - f_a^2 f_s^2 f_b + 4f_r f_a f_s f_b^2 - 12f_r f_a f_t f_s + 24f_b f_t f_r^2 - 4f_r f_b f_a^2 f_r \\
& 0, -f_t (2f_s^3 - f_b f_a f_s^2 - 8f_s f_r f_t + 4f_s f_r f_b^2 - 4f_b f_a f_t f_r), f_t (f_s^2 f_a^2 + 4f_s^2 f_r - 4f_b f_a f_r f_s + 4 \\
& f_a^2 f_t f_r - 16f_r^2 f_t), 0, 4f_r (2f_a f_t f_s + f_s f_a f_b^2 - 2f_b^3 f_r - 4f_b f_t f_r), 4f_r (f_a f_s^2 - 2f_b f_r f_s + f_a^2 f_s f_b
\end{aligned}$$

$$\begin{aligned}
& -2f_r f_a f_b^2), f_s (f_s^2 f_b^2 + 2f_s^2 f_t - 8f_r f_t^2 - 4f_b^2 f_r f_t), f_s^4 + f_b f_a f_s^3 - 2f_s^2 f_r f_b^2 - 8f_s^2 f_r f_t \\
& -8f_s f_b f_a f_t f_r + 16f_r^2 f_t^2 + 16f_r^2 f_t f_b^2, -2f_r (f_s^3 + f_b f_a f_s^2 - 4f_s f_r f_t + 2f_s f_a f_t - 8f_b f_a f_t f_r), \\
& 0, -f_s f_b f_t (f_s^2 - 4f_t f_r), -f_t (f_a f_s^3 - 2f_s^2 f_b f_r - 4f_r f_a f_t f_s + 8f_b f_t f_r^2), 2f_a f_t f_r (f_s^2 - 4f_t f_r) \Big], \\
& \Big[ 0, 0, 0, 0, 0, 0, 0, 0, 0, 4f_s (f_b f_s - 2f_a f_t), 0, 4f_b f_s (f_b f_s - 2f_a f_t), 0, 0, -4f_t f_s (f_b f_s \\
& - 2f_a f_t), 0, 0, 0, 0, 2f_a f_s^2 - 8f_b f_r f_s + 8f_a f_t f_r, 0, 2f_b (f_a f_s^2 - 4f_b f_r f_s + 4f_a f_t f_r), 0, 0, \\
& -2f_t (f_a f_s^2 - 4f_b f_r f_s + 4f_a f_t f_r), -8f_r (f_a f_s - 2f_b f_r), -2f_s (f_s^2 - 4f_t f_r), 4f_r (4f_r f_b^2 \\
& - 4f_t f_r - 2f_b f_a f_s + f_s^2), 0, -2f_b f_s (f_s^2 - 4f_t f_r), 4f_r (f_b f_s^2 + 2f_a f_t f_s - 8f_b f_t f_r), 0, 0, \\
& 2f_s f_t (f_s^2 - 4f_t f_r), -4f_r f_t (f_s^2 - 4f_t f_r) \Big], \\
& \Big[ 0, 0, -2f_a f_s (f_b f_s - 2f_a f_t), 0, -2f_s (f_b f_s^2 - 2f_a f_t f_s + f_s f_a f_b^2 - 2f_b f_a^2 f_t), 0, -f_a (f_a f_s^2 \\
& - 4f_b f_r f_s + 4f_a f_t f_r), 0, -f_a f_s^3 + 4f_s^2 f_b f_r - f_a^2 f_s^2 f_b + 4f_r f_a f_s f_b^2 - 4f_r f_a f_t f_s - 4f_r f_b f_a^2 f_r \\
& 4f_a f_r (f_a f_s - 2f_b f_r), f_s (4f_b f_r f_s - 12f_a f_t f_r + f_a f_s^2), 2f_r (f_a f_s^2 + 2f_a^2 f_s f_b - 4f_b f_r f_s \\
& - 4f_r f_a f_b^2 + 4f_a f_t f_r), 0, f_s (f_s^3 + f_b f_a f_s^2 - 4f_s f_r f_t + 2f_s f_r f_b^2 - 8f_b f_a f_t f_r), -2f_r (f_s^3 + f_b f_a \\
& f_s^2 - 4f_s f_r f_t - 4f_b f_a f_t f_r), 0, 0, 0, 0, 0, 2f_r (f_a f_s^2 - 4f_b f_r f_s + 4f_a f_t f_r), 0, 0, f_b f_r (f_a f_s^2 \\
& - 4f_b f_r f_s + 4f_a f_t f_r), 0, 0, -8f_r^2 (f_a f_s - 2f_b f_r), 0, -2f_r f_s (f_s^2 - 4f_t f_r), 4f_r^2 (f_s^2 - f_b f_a f_s \\
& - 4f_t f_r + 2f_r f_b^2), 0, 0, -f_s f_b f_r (f_s^2 - 4f_t f_r), 2f_b f_r^2 (f_s^2 - 4f_t f_r), 0 \Big], \\
& \Big[ 0, 0, -2f_b f_s (f_b f_s - 2f_a f_t), 0, -2f_s (2f_t f_s f_b + f_s f_b^3 - 4f_t^2 f_a - 2f_a f_t f_b^2), 0, -3f_b f_a f_s^2 \\
& + 4f_s f_r f_b^2 + 4f_s f_a^2 f_t - 4f_b f_a f_t f_r, 0, -2f_b f_s^3 - 3f_b^2 f_a f_s^2 + 2f_s^2 f_a f_t + 8f_s f_b f_t f_r + 4f_r f_s f_b^3 \\
& + 4f_b f_a^2 f_s f_t - 4f_r f_a f_t f_b^2 - 8f_a f_t^2 f_r, 4f_b f_r (f_a f_s - 2f_b f_r), f_s (5f_b f_s^2 - 8f_a f_t f_s - 4f_b f_t f_r), \\
& 2f_b f_r (f_s^2 + 2f_b f_a f_s - 4f_t f_r - 4f_r f_b^2), 0, f_s (3f_s^2 f_b^2 + 2f_s^2 f_t - 4f_b f_a f_t f_s - 4f_b^2 f_r f_t - 8f_r \\
& f_t^2), -4f_r f_t (f_s^2 + f_b f_a f_s - 2f_r f_b^2 - 4f_t f_r), 0, -f_a (f_a f_s^2 - 4f_b f_r f_s + 4f_a f_t f_r), 0, -f_a f_s^3 + 4 \\
& f_s^2 f_b f_r - f_a^2 f_s^2 f_b + 4f_r f_a f_s f_b^2 - 4f_r f_a f_t f_s - 4f_r f_b f_a^2 f_r, 4f_a f_r (f_a f_s - 2f_b f_r), f_s (3f_a f_s^2 \\
& - 8f_b f_r f_s + 4f_a f_t f_r), 4f_r (f_a f_s^2 - 4f_b f_r f_s + f_a^2 f_s f_b - 2f_r f_a f_b^2 + 4f_a f_t f_r), 0, f_s^2 (f_s^2 \\
& + 2f_b f_a f_s - 4f_t f_r - 4f_r f_b^2), -f_r (2f_s^3 + f_b f_a f_s^2 - 8f_s f_r f_t + 4f_s f_r f_b^2 - 12f_b f_a f_t f_r), 0, \\
& -8f_r f_s (f_a f_s - 2f_b f_r), -8f_r^2 (f_a f_s - 2f_b f_r), -2f_s^2 (f_s^2 - 4f_t f_r), 2f_s f_r (4f_r f_b^2 - 4f_t f_r \\
& - 2f_b f_a f_s + f_s^2), 4f_r^2 (f_s^2 - f_b f_a f_s - 4f_t f_r + 2f_r f_b^2), 0, -f_b f_s^2 (f_s^2 - 4f_t f_r), f_s f_b f_r (f_s^2 \\
& - 4f_t f_r), 2f_b f_r^2 (f_s^2 - 4f_t f_r) \Big], \\
& \Big[ 0, 0, 0, 0, 0, 0, -2f_b f_s (f_b f_s - 2f_a f_t), 0, -2f_s (2f_t f_s f_b + f_s f_b^3 - 4f_t^2 f_a - 2f_a f_t f_b^2), \\
& -2f_a f_s (f_b f_s - 2f_a f_t), 4f_t f_s (f_b f_s - 2f_a f_t), 2f_s (f_b f_s^2 - 2f_a f_t f_s - f_s f_a f_b^2 + 2f_b f_a^2 f_t), 0, \\
& 2f_s f_b f_t (f_b f_s - 2f_a f_t), 2f_b f_s^2 (f_b f_s - 2f_a f_t), 0, -f_b (f_a f_s^2 - 4f_b f_r f_s + 4f_a f_t f_r), 0, -f_b^2 f_a f_s^2
\end{aligned}$$



$$\begin{aligned}
& -2f_s^2 f_a f_t + 8f_s f_b f_t f_r + 4f_r f_s f_b^3 - 4f_r f_a f_t f_b^2 - 8f_a f_t^2 f_r - f_s^2 f_a^2 + 8f_b f_a f_r f_s - 8f_r^2 f_b^2 - 4 \\
& f_a^2 f_t f_r f_b f_s^3 + 2f_s^2 f_a f_t - 12f_s f_b f_t f_r + 8f_a f_t^2 f_r f_a f_s^3 - 6f_s^2 f_b f_r - f_a^2 f_s^2 f_b + 8f_r f_a f_s f_b^2 \\
& + 12f_r f_a f_t f_s - 8f_b f_t f_r^2 - 4f_r f_b f_a^2 f_t - 8f_b^3 f_r^2, 0, f_b^2 f_s^3 + 2f_t f_s^3 + f_a f_t f_b f_s^2 - 8f_r f_t f_s f_b^2 - 8f_r \\
& f_t^2 f_s + 4f_r f_t^2 f_a f_b f_b f_a f_s^3 - 4f_s^2 f_r f_t - 6f_s^2 f_r f_b^2 + 4f_s f_b f_a f_t f_r + 8f_r^2 f_t f_b^2 + 16f_r^2 f_t^2, \\
& 4f_a f_r (f_a f_s - 2f_b f_r), f_a f_s^3 - 12f_r f_a f_t f_s + 16f_b f_t f_r^2, -2f_r (3f_a f_s^2 - 4f_b f_r f_s - 2f_a^2 f_s f_b \\
& + 4f_r f_a f_b^2 - 4f_a f_t f_r), -2f_s f_t (f_s^2 - 4f_t f_r), -f_s^4 + f_b f_a f_s^3 + 8f_s^2 f_r f_t - 8f_s f_b f_a f_t f_r - 16f_r^2 f_t^2 \\
& + 8f_r^2 f_t f_b^2, 2f_r (f_s^3 - 3f_b f_a f_s^2 + 4f_s f_r f_b^2 - 4f_s f_r f_t + 4f_b f_a f_t f_r), 0, -f_s f_b f_t (f_s^2 - 4f_t f_r), \\
& -f_b (f_s^4 - 6f_s^2 f_r f_t + 8f_r^2 f_t^2), 2f_s f_b f_r (f_s^2 - 4f_t f_r) \Big], \\
& \Big[ 0, 0, 0, 0, 0, 0, 0, 0, 0, -2f_b f_s (f_b f_s - 2f_a f_t), 0, -2f_s f_b^2 (f_b f_s - 2f_a f_t), 0, 0, 2f_s f_b f_t (f_b f_s \\
& - 2f_a f_t), 0, 0, 0, 0, -f_b (f_a f_s^2 - 4f_b f_r f_s + 4f_a f_t f_r), 0, -f_b^2 (f_a f_s^2 - 4f_b f_r f_s + 4f_a f_t f_r), 0, \\
& 0, f_b f_t (f_a f_s^2 - 4f_b f_r f_s + 4f_a f_t f_r), 4f_b f_r (f_a f_s - 2f_b f_r), f_b f_s (f_s^2 - 4f_t f_r), -2f_b f_r (4f_r f_b^2 \\
& - 4f_t f_r - 2f_b f_a f_s + f_s^2), 0, f_s f_b^2 (f_s^2 - 4f_t f_r), -2f_b f_r (f_b f_s^2 + 2f_a f_t f_s - 8f_b f_t f_r), 0, 0, \\
& -f_s f_b f_t (f_s^2 - 4f_t f_r), 2f_b f_t f_r (f_s^2 - 4f_t f_r) \Big], \\
& \Big[ -4f_r f_s (f_b f_s - 2f_a f_t), -2f_r (f_a f_s^2 - 4f_b f_r f_s + 4f_a f_t f_r), 8f_r^2 (f_a f_s - 2f_b f_r), 2f_r f_s (f_s^2 \\
& - 2f_b f_a f_s + 4f_a^2 f_t - 4f_t f_r), -4f_r^2 (f_s^2 - 4f_t f_r), 0, 0, -2f_a f_r (f_a f_s^2 - 4f_b f_r f_s + 4f_a f_t f_r), \\
& 0, 0, 8f_a f_r^2 (f_a f_s - 2f_b f_r), 0, 2f_r f_s (f_a f_s^2 + 2f_b f_r f_s - 8f_a f_t f_r), -4f_a f_r^2 (f_s^2 - 4f_t f_r), 0, 0, \\
& 0, 0, 0, 0, 0, 2f_r^2 (f_a f_s^2 - 4f_b f_r f_s + 4f_a f_t f_r), 0, 0, 0, 0, 0, -8f_r^3 (f_a f_s - 2f_b f_r), 0, 0, \\
& -2f_s f_r^2 (f_s^2 - 4f_t f_r), 4f_r^3 (f_s^2 - 4f_t f_r), 0, 0 \Big], \\
& \Big[ -2f_s^2 (f_b f_s - 2f_a f_t), -f_a f_s (f_s^2 - 4f_t f_r), 4f_r f_s (f_a f_s - 2f_b f_r), f_s (f_s^3 - 2f_b f_a f_s^2 - 4f_s f_r f_t \\
& + 4f_s f_a^2 f_t - 2f_s f_r f_b^2 + 4f_b f_a f_t f_r), -2f_s f_r (f_s^2 + f_b f_a f_s - 4f_t f_r - 2f_a^2 f_t), -2f_r (f_a f_s^2 \\
& - 4f_b f_r f_s + 4f_a f_t f_r), 8f_r^2 (f_a f_s - 2f_b f_r), -f_a^2 f_s^3 + 2f_r f_s^3 + f_r f_a f_s^2 f_b - 8f_r^2 f_t f_s + 4f_s f_r^2 f_b^2 \\
& - 4f_r^2 f_a f_t f_b, -f_r (f_s^2 f_a^2 + 4f_s^2 f_r - 4f_b f_a f_r f_s + 4f_a^2 f_t f_r - 16f_r^2 f_t), 0, 4f_r (f_s^2 f_a^2 - f_b f_a f_r f_s \\
& - 2f_r^2 f_b^2), 4f_a f_r^2 (f_a f_s - 2f_b f_r), f_s (f_a f_s^3 + 5f_s^2 f_b f_r - 12f_r f_a f_t f_s - 4f_b f_t f_r^2), -f_r (f_a f_s^3 \\
& - 2f_s^2 f_b f_r + 4f_r f_a f_t f_s - 8f_b f_t f_r^2), -2f_a f_r^2 (f_s^2 - 4f_t f_r), 0, 0, -f_a f_r (f_a f_s^2 - 4f_b f_r f_s \\
& + 4f_a f_t f_r), 0, 0, 4f_a f_r^2 (f_a f_s - 2f_b f_r), 0, f_s f_r (3f_a f_s^2 - 8f_b f_r f_s + 4f_a f_t f_r), -8f_r^3 (f_b f_s \\
& - 2f_a f_t), 0, 0, 0, 0, -8f_s f_r^2 (f_a f_s - 2f_b f_r), -8f_r^3 (f_a f_s - 2f_b f_r), 0, -2f_s^2 f_r (f_s^2 - 4f_t f_r), \\
& 2f_s f_r^2 (f_s^2 - 4f_t f_r), 4f_r^3 (f_s^2 - 4f_t f_r), 0 \Big], \\
& \Big[ 0, -2f_s^2 (f_b f_s - 2f_a f_t), -4f_r f_s (f_b f_s - 2f_a f_t), -2f_a f_t f_s (f_b f_s - 2f_a f_t), -2f_a f_s^2 (f_b f_s \\
& - 2f_a f_t), -f_s (f_a f_s^2 - 4f_b f_r f_s + 4f_a f_t f_r), 2f_a f_r (f_s^2 - 4f_t f_r), f_s^4 - f_s^2 f_a^2 f_t - 2f_s^2 f_r f_b^2 - 4
\end{aligned}$$

$$\begin{aligned}
& f_s^2 f_r f_t + 8 f_s f_b f_a f_t f_r - 4 f_a^2 f_t^2 f_r - f_s (f_s^2 f_a^2 + 2 f_s^2 f_r - 4 f_b f_a f_r f_s - 8 f_r^2 f_t + 4 f_a^2 f_t f_r), 8 \\
& f_r^2 (f_a f_s - 2 f_b f_r), 2 f_r (f_s^3 - f_b f_a f_s^2 - 4 f_s f_r f_t + 4 f_s f_a^2 f_t - 4 f_b f_a f_t f_r), 4 f_r (f_s^2 f_a^2 - f_s^2 f_r \\
& - 2 f_b f_a f_r f_s + 4 f_r^2 f_t), f_s f_t (4 f_b f_r f_s - 12 f_a f_t f_r + f_a f_s^2), f_s^4 f_a + 4 f_r f_b f_s^3 - 14 f_r f_a f_t f_s^2 + 8 \\
& f_r^2 f_a f_t^2, -2 f_s f_a f_r (f_s^2 - 4 f_t f_r), 0, 0, -f_b f_r (f_a f_s^2 - 4 f_b f_r f_s + 4 f_a f_t f_r), 0, 0, -f_r (f_s^2 f_a^2 \\
& - 8 f_b f_a f_r f_s + 8 f_r^2 f_b^2 + 4 f_a^2 f_t f_r), 0, f_r (f_b f_s^3 + 2 f_s^2 f_a f_t - 12 f_s f_b f_t f_r + 8 f_a f_t^2 f_r), 2 f_r (f_a f_s^3 \\
& - 5 f_s^2 f_b f_r + 4 f_r f_a f_t f_s + 4 f_b f_t f_r^2), 0, 0, 4 f_a f_r^2 (f_a f_s - 2 f_b f_r), 0, f_r (f_a f_s^3 - 12 f_r f_a f_t f_s \\
& + 16 f_b f_t f_r^2), -2 f_r^2 (5 f_a f_s^2 - 8 f_b f_r f_s - 4 f_a f_t f_r), 0, -2 f_s f_r f_t (f_s^2 - 4 f_t f_r), -2 f_r (f_s^4 - 6 \\
& f_s^2 f_r f_t + 8 f_r^2 f_t^2), 4 f_s f_r^2 (f_s^2 - 4 f_t f_r), 0], \\
& [0, 0, -2 f_s^2 (f_b f_s - 2 f_a f_t), 0, -2 f_a f_t f_s (f_b f_s - 2 f_a f_t), 0, -f_s (f_a f_s^2 - 4 f_b f_r f_s + 4 f_a f_t f_r), \\
& 0, -f_a f_t (f_a f_s^2 - 4 f_b f_r f_s + 4 f_a f_t f_r), 4 f_r f_s (f_a f_s - 2 f_b f_r), f_s (f_s^3 - 2 f_s f_r f_b^2 - 4 f_s f_r f_t \\
& + 4 f_b f_a f_t f_r), -2 f_r (f_s^3 - 2 f_s f_a^2 f_t - 4 f_s f_r f_t + 4 f_b f_a f_t f_r), 0, f_s f_t (4 f_b f_r f_s - 12 f_a f_t f_r + f_a \\
& f_s^2), -2 f_a f_t f_r (f_s^2 - 4 f_t f_r), 0, 0, 0, 0, 0, -f_b f_r (f_a f_s^2 - 4 f_b f_r f_s + 4 f_a f_t f_r), 0, 0, 2 f_r f_t (f_a f_s^2 \\
& - 4 f_b f_r f_s + 4 f_a f_t f_r), 0, 0, 4 f_b f_r^2 (f_a f_s - 2 f_b f_r), 0, f_s f_b f_r (f_s^2 - 4 f_t f_r), -2 f_r^2 (f_b f_s^2 \\
& + 4 f_a f_t f_s - 12 f_b f_t f_r), 0, 0, -2 f_s f_r f_t (f_s^2 - 4 f_t f_r), 4 f_t f_r^2 (f_s^2 - 4 f_t f_r), 0], \\
& [-4 f_t f_s (f_b f_s - 2 f_a f_t), -4 f_b f_s^3 + 6 f_s^2 f_a f_t + 8 f_s f_b f_t f_r - 8 f_a f_t^2 f_r, 8 f_r f_t (f_a f_s - 2 f_b f_r), \\
& -2 f_s (-f_s^2 f_t + 2 f_s^2 f_b^2 - 4 f_b f_a f_t f_s + 4 f_r f_t^2), -4 f_r (f_s^2 f_b^2 + f_s^2 f_t - 2 f_b f_a f_t f_s - 4 f_r f_t^2), -2 \\
& f_s^2 (f_a f_s - 2 f_b f_r), 8 f_r f_s (f_a f_s - 2 f_b f_r), 2 f_s (f_s^3 - 3 f_b f_a f_s^2 + 4 f_s f_r f_b^2 + 4 f_s f_a^2 f_t - 4 f_s f_r f_t \\
& - 4 f_b f_a f_t f_r), -2 f_r (2 f_s^3 + 3 f_b f_a f_s^2 - 4 f_s f_a^2 f_t - 8 f_s f_r f_t - 4 f_s f_r f_b^2 + 4 f_b f_a f_t f_r), 0, \\
& 8 f_b f_r f_s (f_a f_s - 2 f_b f_r), 8 f_b f_r^2 (f_a f_s - 2 f_b f_r), 2 f_s^2 (3 f_b f_s^2 - 4 f_a f_t f_s - 4 f_b f_t f_r), 2 f_r f_s (3 f_b \\
& f_s^2 - 8 f_a f_t f_s + 4 f_b f_t f_r), -8 f_r^2 f_t (f_a f_s - 2 f_b f_r), -2 f_r (f_a f_s^2 - 4 f_b f_r f_s + 4 f_a f_t f_r), 8 f_r^2 (f_a f_s \\
& - 2 f_b f_r), -2 f_s (-f_s^2 f_r + f_s^2 f_a^2 - 4 f_b f_a f_r f_s + 4 f_r^2 f_t + 4 f_a^2 f_t f_r), -2 f_r (f_s^2 f_a^2 + 2 f_s^2 f_r \\
& - 4 f_b f_a f_r f_s - 8 f_r^2 f_t + 4 f_a^2 f_t f_r), 0, 8 f_s f_a f_r (f_a f_s - 2 f_b f_r), 8 f_a f_r^2 (f_a f_s - 2 f_b f_r), 4 f_s^3 (f_a f_s \\
& - 2 f_b f_r), 2 f_s f_r (f_a f_s^2 - 8 f_b f_r f_s + 12 f_a f_t f_r), -2 f_r^2 (4 f_b f_r f_s - 12 f_a f_t f_r + f_a f_s^2), 0, 0, 0, \\
& -8 f_s^2 f_r (f_a f_s - 2 f_b f_r), -16 f_s f_r^2 (f_a f_s - 2 f_b f_r), -8 f_r^3 (f_a f_s - 2 f_b f_r), -2 f_s^3 (f_s^2 - 4 f_t f_r), \\
& 0, 6 f_s f_r^2 (f_s^2 - 4 f_t f_r), 4 f_r^3 (f_s^2 - 4 f_t f_r)], \\
& [0, -4 f_t f_s (f_b f_s - 2 f_a f_t), -2 f_s^2 (f_b f_s - 2 f_a f_t), -2 f_s f_b f_t (f_b f_s - 2 f_a f_t), -2 f_b f_s^2 (f_b f_s \\
& - 2 f_a f_t), -2 f_b f_s^3 + 2 f_s^2 f_a f_t + 8 f_s f_b f_t f_r - 8 f_a f_t^2 f_r - f_a f_s^3 + 12 f_r f_a f_t f_s - 16 f_b f_t f_r^2, -2 f_b^2 f_s^3 \\
& + 2 f_t f_s^3 + f_a f_t f_b f_s^2 - 8 f_r f_t^2 f_s + 4 f_r f_t f_s f_b^2 + 4 f_s f_a^2 f_t^2 - 4 f_r f_t^2 f_a f_b, -3 f_b f_a f_s^3 + 2 f_s^2 f_r f_b^2 \\
& - 4 f_s^2 f_r f_t + 4 f_s^2 f_a^2 f_t + 16 f_r^2 f_t^2, 4 f_r f_s (f_a f_s - 2 f_b f_r), f_s^4 - 2 f_b f_a f_s^3 - 4 f_s^2 f_r f_t + 4 f_s^2 f_a^2 f_t
\end{aligned}$$

$$\begin{aligned}
& + 4f_s f_b f_a f_t f_r - 8f_r^2 f_t f_b^2, -2f_s f_r (f_s^2 - f_b f_a f_s + 4f_r f_b^2 - 4f_t f_r - 2f_a^2 f_t), f_s f_t (5f_b f_s^2 \\
& - 8f_a f_t f_s - 4f_b f_t f_r), 5f_b f_s^4 - 8f_s^3 f_a f_t - 2f_s^2 f_b f_t f_r - 8f_s f_a f_t^2 f_r + 8f_b f_r^2 f_t^2, 2f_s f_r (f_b f_s^2 \\
& - 4f_a f_t f_s + 4f_b f_t f_r), -f_s (f_a f_s^2 - 4f_b f_r f_s + 4f_a f_t f_r), 2f_a f_r (f_s^2 - 4f_t f_r), f_s^4 - f_b f_a f_s^3 - 4 \\
& f_s^2 f_r f_t + 4f_s^2 f_r f_b^2 - f_s^2 f_a^2 f_t - 4f_a^2 f_t^2 f_r - 2f_r f_s^3 - f_a^2 f_s^3 + 3f_r f_a f_s^2 f_b + 4f_s f_r^2 f_b^2 - 4f_r f_a^2 f_s f_t \\
& + 8f_r^2 f_t f_s - 4f_r^2 f_a f_t f_b, 8f_r^2 (f_a f_s - 2f_b f_r), -f_a^2 f_s^3 + 2f_r f_s^3 + 8f_r f_a f_s^2 f_b - 8f_s f_r^2 f_b^2 - 8 \\
& f_r^2 f_t f_s - 8f_r^2 f_a f_t f_b, f_r (-4f_s^2 f_r + 3f_s^2 f_a^2 + 16f_r^2 f_t - 4f_a^2 f_t f_r - 8f_r^2 f_b^2), f_s (f_b f_s^3 + 3f_s^2 f_a f_t \\
& - 12f_s f_b f_t f_r + 4f_a f_t^2 f_r), 3f_s^4 f_a - 9f_r f_b f_s^3 + 4f_r f_a f_t f_s^2 - 4f_r^2 f_s f_t f_b + 16f_r^2 f_a f_t^2, -2 \\
& f_r^2 (5f_b f_s^2 - 8f_a f_t f_s - 4f_b f_t f_r), 0, 4f_s f_a f_r (f_a f_s - 2f_b f_r), 4f_a f_r^2 (f_a f_s - 2f_b f_r), f_s (f_a f_s^3 \\
& - 12f_r f_a f_t f_s + 16f_b f_t f_r^2), -f_r (9f_a f_s^3 - 16f_s^2 f_b f_r + 4f_r f_a f_t f_s - 16f_b f_t f_r^2), -2f_r^2 (5f_a f_s^2 \\
& - 8f_b f_r f_s - 4f_a f_t f_r), -2f_s^2 f_t (f_s^2 - 4f_t f_r), -2f_s (4f_r^2 f_t^2 - 5f_s^2 f_r f_t + f_s^4), 2f_r (f_s^4 - 2 \\
& f_s^2 f_r f_t - 8f_r^2 f_t^2), 4f_s f_r^2 (f_s^2 - 4f_t f_r) \Big], \\
& \Big[ 0, 0, -4f_t f_s (f_b f_s - 2f_a f_t), 0, -2f_s f_b f_t (f_b f_s - 2f_a f_t), 0, -2f_b f_s^3 + 2f_s^2 f_a f_t + 8f_s f_b f_t f_r \\
& - 8f_a f_t^2 f_r, 0, -f_t (3f_b f_a f_s^2 - 4f_s f_a^2 f_t - 4f_s f_r f_b^2 + 4f_b f_a f_t f_r), 8f_r f_t (f_a f_s - 2f_b f_r), -2f_s ( \\
& f_s^2 f_b^2 - f_s^2 f_t - 2f_b f_a f_t f_s + 4f_r f_t^2), -2f_r (f_s^2 f_b^2 + 2f_s^2 f_t - 4f_b f_a f_t f_s - 8f_r f_t^2 + 4f_b^2 f_r f_t), 0, \\
& f_s f_t (5f_b f_s^2 - 8f_a f_t f_s - 4f_b f_t f_r), 2f_r f_t (f_b f_s^2 - 4f_a f_t f_s + 4f_b f_t f_r), 0, -f_s (f_a f_s^2 - 4f_b f_r f_s \\
& + 4f_a f_t f_r), 0, -f_a f_t (f_a f_s^2 - 4f_b f_r f_s + 4f_a f_t f_r), 4f_r f_s (f_a f_s - 2f_b f_r), f_s (f_s^3 - f_b f_a f_s^2 \\
& + 4f_s f_r f_b^2 - 4f_s f_r f_t - 4f_b f_a f_t f_r), -f_r (2f_s^3 + f_b f_a f_s^2 - 4f_s f_a^2 f_t - 8f_s f_r f_t - 4f_s f_r f_b^2 \\
& + 12f_b f_a f_t f_r), 0, f_t f_s (3f_a f_s^2 - 8f_b f_r f_s + 4f_a f_t f_r), -8f_r^2 f_t (f_b f_s - 2f_a f_t), 0, 4f_b f_r f_s (f_a f_s \\
& - 2f_b f_r), 4f_b f_r^2 (f_a f_s - 2f_b f_r), f_b f_s^2 (f_s^2 - 4f_t f_r), -f_s f_r (f_b f_s^2 + 8f_a f_t f_s - 20f_b f_t f_r), -2 \\
& f_r^2 (f_b f_s^2 + 4f_a f_t f_s - 12f_b f_t f_r), 0, -2f_s^2 f_t (f_s^2 - 4f_t f_r), 2f_s f_r f_t (f_s^2 - 4f_t f_r), 4f_t f_r^2 (f_s^2 \\
& - 4f_t f_r) \Big], \\
& \Big[ 0, 0, 0, 0, 0, -4f_t f_s (f_b f_s - 2f_a f_t), -4f_s^2 (f_b f_s - 2f_a f_t), -4f_s f_b f_t (f_b f_s - 2f_a f_t), -4f_b \\
& f_s^2 (f_b f_s - 2f_a f_t), -4f_r f_s (f_b f_s - 2f_a f_t), -4f_a f_t f_s (f_b f_s - 2f_a f_t), -4f_a f_s^2 (f_b f_s - 2f_a f_t), \\
& 4f_t^2 f_s (f_b f_s - 2f_a f_t), 8f_s^2 f_t (f_b f_s - 2f_a f_t), 4f_s^3 (f_b f_s - 2f_a f_t), -2f_t (f_a f_s^2 - 4f_b f_r f_s \\
& + 4f_a f_t f_r), -2f_a f_s^3 + 8f_s^2 f_b f_r - 16f_b f_t f_r^2, 2f_t (f_s^3 - f_b f_a f_s^2 + 4f_s f_r f_b^2 - 4f_s f_r f_t \\
& - 4f_b f_a f_t f_r), 16f_r^2 f_t^2 + 8f_s^2 f_r f_b^2 - 8f_s f_b f_a f_t f_r - 4f_s^2 f_r f_t - 2f_b f_a f_s^3, 2f_r (3f_a f_s^2 - 4f_b f_r f_s \\
& - 4f_a f_t f_r), -16f_r^2 f_t f_b^2 + 16f_s f_b f_a f_t f_r - 8f_a^2 f_t^2 f_r - 8f_s^2 f_r f_t - 2f_s^2 f_a^2 f_t + 2f_s^4, -2f_s (8f_r^2 f_b^2 \\
& - 8f_r^2 f_t - 8f_b f_a f_r f_s + 4f_a^2 f_t f_r + 2f_s^2 f_r + f_s^2 f_a^2), 2f_t (f_b f_s^3 + f_s^2 f_a f_t - 8f_s f_b f_t f_r + 4f_a \\
& f_t^2 f_r), 16f_b f_r^2 f_t^2 - 28f_s^2 f_b f_t f_r + 16f_s f_a f_t^2 f_r + 2f_b f_s^4 + 4f_s^3 f_a f_r - 2f_s (8f_b f_t f_r^2 - 6f_s^2 f_b f_r
\end{aligned}$$

$$\begin{aligned}
& + 4f_r f_a f_t f_s + f_a f_s^3), 8f_r^2 (f_a f_s - 2f_b f_r), 2f_r (f_s^3 - 4f_s f_r f_t + 4f_s f_a^2 f_t - 8f_b f_a f_t f_r), 4f_r (4 \\
& f_r^2 f_t - 4f_b f_a f_r f_s - f_s^2 f_r + 2f_s^2 f_a^2), 2f_t (8f_b f_t f_r^2 - 8f_r f_a f_t f_s + f_a f_s^3), 32f_r^2 f_s f_t f_b + 16f_r^2 f_a f_t^2 \\
& - 28f_r f_a f_t f_s^2 + 2f_s^4 f_a - 4f_s f_r (3f_a f_s^2 - 4f_b f_r f_s - 4f_a f_t f_r), -2f_s f_t^2 (f_s^2 - 4f_t f_r), -4f_t (4 \\
& f_r^2 f_t^2 - 5f_s^2 f_r f_t + f_s^4), -2f_s (16f_r^2 f_t^2 - 8f_s^2 f_r f_t + f_s^4), 4f_s^2 f_r (f_s^2 - 4f_t f_r) \Big], \\
& [0, 0, 0, 0, 0, 0, -4f_t f_s (f_b f_s - 2f_a f_t), 0, -2f_s f_b f_t (f_b f_s - 2f_a f_t), -2f_s^2 (f_b f_s - 2f_a f_t), \\
& -2f_s f_b f_t (f_b f_s - 2f_a f_t), -2f_s (f_s^2 f_b^2 - f_b f_a f_t f_s - 2f_a^2 f_t^2), 0, 4f_t^2 f_s (f_b f_s - 2f_a f_t), 4 \\
& f_s^2 f_t (f_b f_s - 2f_a f_t), 0, -2f_t (f_a f_s^2 - 4f_b f_r f_s + 4f_a f_t f_r), 0, -f_b f_t (f_a f_s^2 - 4f_b f_r f_s \\
& + 4f_a f_t f_r), -f_a f_s^3 + 4f_s^2 f_b f_r + 4f_r f_a f_t f_s - 16f_b f_t f_r^2, f_t (2f_s^3 - f_b f_a f_s^2 - 8f_s f_r f_t + 4f_s f_r f_b^2 \\
& - 4f_b f_a f_t f_r), -f_b f_a f_s^3 + 4f_s^2 f_r f_b^2 - f_s^2 f_a^2 f_t - 4f_s^2 f_r f_t + 4f_s f_b f_a f_t f_r - 8f_r^2 f_t f_b^2 - 4f_a^2 f_t^2 f_r \\
& + 16f_r^2 f_t^2, 0, f_t (f_b f_s^3 + 2f_s^2 f_a f_t - 12f_s f_b f_t f_r + 8f_a f_t^2 f_r), 2f_t (f_a f_s^3 - 5f_s^2 f_b f_r + 4f_r f_a f_t f_s \\
& + 4f_b f_t f_r^2), 4f_r f_s (f_a f_s - 2f_b f_r), f_s^4 - 4f_s^2 f_r f_t + 4f_s f_b f_a f_t f_r - 8f_r^2 f_t f_b^2, -2f_r (f_s^3 - 2f_b f_a \\
& f_s^2 - 2f_s f_a^2 f_t - 4f_s f_r f_t + 4f_s f_r f_b^2 + 4f_b f_a f_t f_r), f_s f_b f_t (f_s^2 - 4f_t f_r), f_b f_s^4 + f_s^3 f_a f_t - 6f_s^2 f_b f_t f_r \\
& - 12f_s f_a f_t^2 f_r + 24f_b f_r^2 f_t^2, -2f_r (f_b f_s^3 + 5f_s^2 f_a f_t - 12f_s f_b f_t f_r - 4f_a f_t^2 f_r), 0, -2f_s f_t^2 (f_s^2 \\
& - 4f_t f_r), -2f_t (f_s^4 - 6f_s^2 f_r f_t + 8f_r^2 f_t^2), 4f_s f_r f_t (f_s^2 - 4f_t f_r) \Big], \\
& [0, 0, 0, 0, 0, 0, 0, 0, 0, -4f_t f_s (f_b f_s - 2f_a f_t), 0, -4f_s f_b f_t (f_b f_s - 2f_a f_t), 0, 0, 4f_t^2 f_s (f_b f_s \\
& - 2f_a f_t), 0, 0, 0, 0, -2f_t (f_a f_s^2 - 4f_b f_r f_s + 4f_a f_t f_r), 0, -2f_b f_t (f_a f_s^2 - 4f_b f_r f_s \\
& + 4f_a f_t f_r), 0, 0, 2f_t^2 (f_a f_s^2 - 4f_b f_r f_s + 4f_a f_t f_r), 8f_r f_t (f_a f_s - 2f_b f_r), 2f_s f_t (f_s^2 - 4f_t f_r), \\
& -4f_r f_t (4f_r f_b^2 - 4f_t f_r - 2f_b f_a f_s + f_s^2), 0, 2f_s f_b f_t (f_s^2 - 4f_t f_r), -4f_r f_t (f_b f_s^2 + 2f_a f_t f_s \\
& - 8f_b f_t f_r), 0, 0, -2f_s f_t^2 (f_s^2 - 4f_t f_r), 4f_r f_t^2 (f_s^2 - 4f_t f_r) \Big], \\
& [4f_t (f_b^2 + 4f_t), -2f_s (f_b^2 + 4f_t), 4f_s^2 + 4f_r f_b^2, 4f_a f_t (f_b^2 + 4f_t), 2f_b (f_s^2 - 4f_t f_r), 0, 0, \\
& -2f_a f_s (f_b^2 + 4f_t), 0, 0, 4f_a (f_s^2 + f_r f_b^2), 0, -4f_r f_t (f_b^2 + 4f_t), 2f_b f_a (f_s^2 - 4f_t f_r), 0, 0, 0, \\
& 0, 0, 0, 0, 2f_r f_s (f_b^2 + 4f_t), 0, 0, 0, 0, 0, -4f_r (f_s^2 + f_r f_b^2), 0, 0, 0, -2f_b f_r (f_s^2 - 4f_t f_r), 0, \\
& 0], \\
& [0, 4f_t (f_b^2 + 4f_t), 0, 2f_b f_t (f_b^2 + 4f_t), 2f_a f_t (f_b^2 + 4f_t), -2f_s (f_b^2 + 4f_t), 4f_s^2 + 4f_r f_b^2, \\
& -4f_t f_s f_b - f_s f_b^3 + 2f_a f_t f_b^2 + 8f_t^2 f_a, 2f_b f_s^2 - f_s f_a f_b^2 - 4f_a f_t f_s - 8f_b f_t f_r, 0, 2f_b (f_s^2 + f_r f_b^2), \\
& 2f_a (f_s^2 + f_r f_b^2), -2f_t f_s (f_b^2 + 4f_t), f_s^2 f_b^2 - 8f_b^2 f_r f_t - 16f_r f_t^2, f_b f_a (f_s^2 - 4f_t f_r), 0, 0, -f_a f_s ( \\
& f_b^2 + 4f_t), 0, 0, 2f_a (f_s^2 + f_r f_b^2), 0, (f_b^2 + 4f_t) f_s^2, 2f_s f_r f_b^2 - 4f_b f_a f_t f_r + 8f_s f_r f_t + f_b f_a f_s^2, 0, \\
& 0, 0, 0, -2f_s (f_s^2 + f_r f_b^2), -4f_r (f_s^2 + f_r f_b^2), 0, 0, -f_b f_s (f_s^2 - 4f_t f_r), -2f_b f_r (f_s^2 - 4f_t f_r), 0 \\
& ]
\end{aligned}$$

$$\begin{aligned}
& [0, 0, 4f_t(f_b^2 + 4f_t), 0, 2f_b f_t(f_b^2 + 4f_t), 0, -2f_s(f_b^2 + 4f_t), 0, -f_b f_s(f_b^2 + 4f_t), 4f_s^2 + 4f_r f_b^2, 2f_a f_t(f_b^2 + 4f_t), 2f_b(f_r f_b^2 - 4f_t f_r + 2f_s^2), 0, -2f_t f_s(f_b^2 + 4f_t), f_b^2(f_s^2 - 4f_t f_r), 0, 0, \\
& 0, 0, 0, -f_a f_s(f_b^2 + 4f_t), 0, 0, (f_b^2 + 4f_t)f_s^2, 0, 0, 2f_a(f_s^2 + f_r f_b^2), 0, 0, -2f_s^3 + f_b f_a f_s^2 \\
& - 2f_s f_r f_b^2 - 4f_b f_a f_t f_r, 0, 0, 0, -f_b f_s(f_s^2 - 4f_t f_r), 0], \\
& [-2f_a f_t(f_b^2 + 4f_t), f_a f_s(f_b^2 + 4f_t), -2f_a(f_s^2 + f_r f_b^2), -2f_a^2 f_t(f_b^2 + 4f_t), -f_b f_a(f_s^2 \\
& - 4f_t f_r), 0, 0, f_s f_a^2(f_b^2 + 4f_t), 0, 0, -2f_a^2(f_s^2 + f_r f_b^2), 0, 2f_a f_t f_r(f_b^2 + 4f_t), -f_b f_a^2(f_s^2 \\
& - 4f_t f_r), 0, 0, 0, 0, 0, 0, 0, 0, -f_s f_a f_r(f_b^2 + 4f_t), 0, 0, 0, 0, 0, 2f_a f_r(f_s^2 + f_r f_b^2), 0, 0, 0, \\
& f_b f_a f_r(f_s^2 - 4f_t f_r), 0, 0], \\
& [-2f_b f_t(f_b^2 + 4f_t), f_s f_b^3 - 2f_a f_t f_b^2 + 4f_t f_s f_b - 8f_t^2 f_a - 2f_b(f_s^2 + f_r f_b^2), 2f_t(4f_t f_s + f_s f_b^2 \\
& - 4f_a f_t f_b - f_b^3 f_a), 8f_b^2 f_r f_t + 16f_r f_t^2 - f_s^2 f_b^2, f_a f_s(f_b^2 + 4f_t), -2f_a(f_s^2 + f_r f_b^2), -4f_s^2 f_t - \\
& f_s^2 f_b^2 + 4f_b f_a f_t f_s + f_s f_b^3 f_a - 4f_b^2 f_r f_t - 2f_b^2 f_a^2 f_t - 8f_a^2 f_t^2 - 16f_r f_t^2, -f_b f_a f_s^2 - 2f_s f_r f_b^2 \\
& - 8f_s f_r f_t + 4f_b f_a f_t f_r, 0, 2f_s^3 - 2f_b f_a f_s^2 + 2f_s f_r f_b^2 - 2f_b^3 f_r f_a, 4f_r(f_s^2 + f_r f_b^2), 2f_s f_a f_t(f_b^2 \\
& + 4f_t), f_b f_s^3 - f_b^2 f_a f_s^2 - 4f_s f_b f_t f_r + 6f_r f_a f_t f_b^2 + 8f_a f_t^2 f_r, 2f_b f_r(f_s^2 - 4f_t f_r), 0, 0, f_s(f_b^2 f_a^2 \\
& + 2f_r f_b^2 + 4f_a^2 f_t + 8f_t f_r), 0, 0, -2f_s^2 f_a^2 - 4f_s^2 f_r - 2f_b^2 f_a^2 f_r - 4f_r^2 f_b^2, 0, -f_a f_s^2(f_b^2 + 4f_t), \\
& -2f_s^2 f_b f_r - f_a^2 f_s^2 f_b - f_r f_a f_s f_b^2 - 4f_r f_a f_t f_s + 8f_b f_t f_r^2 + 4f_r f_b f_a^2 f_r, 0, 0, 0, 0, 2f_a f_s(f_s^2 + f_r \\
& f_b^2), 2f_a f_r(f_s^2 + f_r f_b^2), 0, 0, f_s f_b f_a(f_s^2 - 4f_t f_r), f_b f_a f_r(f_s^2 - 4f_t f_r), 0], \\
& [0, -2f_b f_t(f_b^2 + 4f_t), -2f_a f_t(f_b^2 + 4f_t), 4f_t^2(f_b^2 + 4f_t), 4f_t f_s(f_b^2 + 4f_t), f_b f_s(f_b^2 + 4f_t), \\
& -2f_b f_s^2 + f_s f_a f_b^2 + 4f_a f_t f_s - 2f_b^3 f_r - 2f_t(2f_s f_b^2 + 8f_t f_s + f_b^3 f_a + 4f_a f_t f_b), 4f_b^2 f_r f_t - 3f_s^2 \\
& f_b^2 - 8f_s^2 f_r - 2f_a(f_s^2 + f_r f_b^2), 2f_t(2f_s^2 - 4f_a^2 f_t - f_b^2 f_a^2 - 8f_t f_r), 4f_s f_r f_b^2 + 4f_b f_a f_t f_r - f_b f_a \\
& f_s^2 + 4f_s^3, 2f_t^2 f_a(f_b^2 + 4f_t), 2f_t(f_b f_s^2 + f_s f_a f_b^2 + 4f_a f_t f_s - 4f_b f_t f_r), 2f_b f_s(f_s^2 - 4f_t f_r), 0, \\
& 0, f_s(4f_t f_s + f_s f_b^2 + f_b^3 f_a + 4f_a f_t f_b), 0, 0, -2f_s^3 - 2f_b f_a f_s^2 + 4f_s f_a^2 f_t + f_s f_b^2 f_a^2 + 8f_s f_r f_t \\
& - 2f_b^3 f_r f_a, 0, -f_s f_a f_t(f_b^2 + 4f_t), -f_b f_s^3 - 2f_b^2 f_a f_s^2 - 4f_s^2 f_a f_t + 4f_s f_b f_t f_r + 4f_r f_a f_t f_b^2, 0, 0, \\
& -2f_s^2 f_a^2 - 4f_s^2 f_r - 2f_b^2 f_a^2 f_r - 4f_r^2 f_b^2, 0, 2f_a f_t(f_s^2 + f_r f_b^2), 2f_a f_s^3 - 2f_s^2 f_b f_r - f_a^2 f_s^2 f_b \\
& + 2f_r f_a f_s f_b^2 + 8f_b f_t f_r^2 + 4f_r f_b f_a^2 f_r, 0, 0, f_a f_t f_b(f_s^2 - 4f_t f_r), f_s f_b f_a(f_s^2 - 4f_t f_r), 0], \\
& [0, 0, -2f_b f_t(f_b^2 + 4f_t), 0, 4f_t^2(f_b^2 + 4f_t), 0, f_b f_s(f_b^2 + 4f_t), 0, -2f_t f_s(f_b^2 + 4f_t), -2f_b(f_s^2 + f_r f_b^2), \\
& -2f_t(4f_t f_s + f_s f_b^2 + f_b^3 f_a + 4f_a f_t f_b), -f_s^2 f_b^2 + 4f_s^2 f_t + 8f_b^2 f_r f_r, 0, 2f_t^2 f_a(f_b^2 + 4f_t) \\
& + 4f_t), 2f_b f_t(f_s^2 - 4f_t f_r), 0, 0, 0, 0, 0, f_s(4f_t f_s + f_s f_b^2 + f_b^3 f_a + 4f_a f_t f_b), 0, 0, -f_s f_a f_t(f_b^2 + 4f_t), \\
& 0, 0, -2f_s^3 - 2f_b f_a f_s^2 - 2f_s f_r f_b^2 - 2f_b^3 f_r f_a, 0, 0, -f_b f_s^3 + 2f_s^2 f_a f_t - f_b^2 f_a f_s^2 \\
& + 4f_s f_b f_t f_r + 6f_r f_a f_t f_b^2, 0, 0, 0, f_a f_t f_b(f_s^2 - 4f_t f_r), 0],
\end{aligned}$$

$$\begin{aligned}
& \left[ 0, 0, 0, 0, 0, 4f_t(f_b^2 + 4f_t), 0, 4f_b f_t(f_b^2 + 4f_t), 4f_a f_t(f_b^2 + 4f_t), 0, 0, 0, -4f_t^2(f_b^2 + 4f_t), -4f_t f_s(f_b^2 + 4f_t), -4f_r f_t(f_b^2 + 4f_t), -2f_s(f_b^2 + 4f_t), 4f_s^2 + 4f_r f_b^2, -2f_b f_s(f_b^2 + 4f_t), -8f_b f_t f_r - 2f_s f_a f_b^2 + 2f_b f_s^2 - 8f_a f_t f_s, 0, 4f_b(f_s^2 + f_r f_b^2), 4f_a(f_s^2 + f_r f_b^2), 2f_t f_s(f_b^2 + 4f_t), -8f_b^2 f_r f_t + 4f_s^2 f_b^2 + 8f_s^2 f_r - 2f_s f_r f_b^2 - 8f_b f_a f_t f_r + 8f_s f_r f_t + 2f_b f_a f_s^2, 0, 0, 0, -4f_t(f_s^2 + f_r f_b^2), -4f_s(f_s^2 + f_r f_b^2), -4f_r(f_s^2 + f_r f_b^2), 0, -2f_b f_t(f_s^2 - 4f_t f_r), -2f_b f_s(f_s^2 - 4f_t f_r), -2f_b f_r(f_s^2 - 4f_t f_r) \right], \\
& \left[ 0, 0, 0, 0, 0, 4f_t(f_b^2 + 4f_t), 0, 2f_b f_t(f_b^2 + 4f_t), 0, 2f_b f_t(f_b^2 + 4f_t), 2f_a f_t(f_b^2 + 4f_t), 0, -4f_t^2(f_b^2 + 4f_t), -2f_t f_s(f_b^2 + 4f_t), 0, -2f_s(f_b^2 + 4f_t), 0, -f_b f_s(f_b^2 + 4f_t), 4f_s^2 + 4f_r f_b^2, -f_b f_s(f_b^2 + 4f_t), 4f_b f_s^2 - f_s f_a f_b^2 - 4f_a f_t f_s - 8f_b f_t f_r + 2f_b^3 f_r, 0, 2f_t f_s(f_b^2 + 4f_t), -4f_b^2 f_r f_t + 2f_s^2 f_b^2 + 4f_s^2 f_r, 0, 2f_b(f_s^2 + f_r f_b^2), 2f_a(f_s^2 + f_r f_b^2), 0, f_s^2 f_b^2 - 4f_s^2 f_t - 8f_b^2 f_r f_r - 2f_s^3 + f_b f_a f_s^2 - 2f_s f_r f_b^2 - 4f_b f_a f_t f_r, 0, 0, -2f_b f_t(f_s^2 - 4f_t f_r), -f_b f_s(f_s^2 - 4f_t f_r) \right], \\
& \left[ 0, -2f_a f_t(f_b^2 + 4f_t), 0, -2f_t(4f_t f_s + f_s f_b^2 + f_b^3 f_a + 4f_a f_t f_b), -2f_t(f_b^2 f_a^2 + 2f_r f_b^2 + 4f_a^2 f_t + 8f_t f_r), f_a f_s(f_b^2 + 4f_t), -2f_a(f_s^2 + f_r f_b^2), 4f_s^2 f_t + f_s^2 f_b^2 + f_s f_b^3 f_a + 4f_b f_a f_t f_s + 4f_b^2 f_r f_t + 16f_r f_t^2, -f_b f_a f_s^2 + f_s f_b^2 f_a^2 + 2f_s f_r f_b^2 + 4f_s f_a^2 f_t + 8f_s f_r f_t + 4f_b f_a f_t f_r, 0, -2f_s^3 - 2f_b f_a f_s^2 - 2f_s f_r f_b^2 - 2f_b^3 f_r f_a - 2f_s^2 f_a^2 - 4f_s^2 f_r - 2f_b^2 f_a^2 f_r - 4f_r^2 f_b^2, 2f_b f_t f_r(f_b^2 + 4f_t), -f_b f_s^3 - f_b^2 f_a f_s^2 + 4f_s f_b f_t f_r + 6f_r f_a f_t f_b^2 + 8f_a f_t^2 f_r - f_b(f_s^2 f_a^2 + 2f_s^2 f_r - 4f_a^2 f_t f_r - 8f_r^2 f_t), 0, 0, -2f_r f_s(f_b^2 + 4f_t), 0, 0, 4f_r(f_s^2 + f_r f_b^2), 0, -f_b f_r f_s(f_b^2 + 4f_t), f_r(2f_b f_s^2 - f_s f_a f_b^2 - 4f_a f_t f_s - 8f_b f_t f_r), 0, 0, 0, 0, 2f_b f_r(f_s^2 + f_r f_b^2), 2f_a f_r(f_s^2 + f_r f_b^2), 0, 0, f_r f_b^2(f_s^2 - 4f_t f_r), f_b f_a f_r(f_s^2 - 4f_t f_r), 0 \right], \\
& \left[ 0, -2f_b f_t(f_b^2 + 4f_t), 0, -2f_t(8f_t^2 + f_b^4 + 6f_t f_b^2), -2f_t(4f_t f_s + f_s f_b^2 + f_b^3 f_a + 4f_a f_t f_b), f_s f_b^3 - 2f_a f_t f_b^2 + 4f_t f_s f_b - 8f_t^2 f_a - 2f_b(f_s^2 + f_r f_b^2), 8f_s f_t f_b^2 + 16f_t^2 f_s + f_s f_b^4 - 8f_t^2 f_b f_a - 2f_b^3 f_a f_r - 4f_s^2 f_t + f_s f_b^3 f_a + 4f_b f_a f_t f_s - 8f_a^2 f_t^2 - 2f_b^2 f_a^2 f_t + 4f_b^2 f_r f_r, 0, -2f_s^2 f_b^2 - 4f_s^2 f_t - 4f_b^2 f_r f_t - 2f_b^4 f_r - 2f_s^3 - 2f_b f_a f_s^2 - 2f_s f_r f_b^2 - 2f_b^3 f_r f_a - 2f_t f_s f_b(f_b^2 + 4f_t), -2f_s^2 f_b f_t - f_s^2 f_b^3 + 8f_s f_a f_t^2 + 2f_s f_a f_t f_b^2 + 6f_b^3 f_r f_t + 16f_r f_t^2 f_b, -f_b f_s^3 - f_b^2 f_a f_s^2 + 4f_s f_b f_t f_r + 6f_r f_a f_t f_b^2 + 8f_a f_t^2 f_r f_a f_s(f_b^2 + 4f_t), -2f_a(f_s^2 + f_r f_b^2), -f_s(4f_t f_s + f_s f_b^2 - 4f_a f_t f_b - f_b^3 f_a), -f_a(f_b f_s^2 - f_s f_a f_b^2 - 4f_a f_t f_s - 4f_b f_t f_r), 0, 2f_s^3 - 2f_b f_a f_s^2 + 2f_s f_r f_b^2 - 2f_b^3 f_r f_a - 2f_a^2(f_s^2 + f_r f_b^2), -f_b f_s^2(f_b^2 + 4f_t), f_b f_s^3 - 2f_b^2 f_a f_s^2 - 4f_s^2 f_a f_t - 8f_s f_b f_t f_r - f_r f_s f_b^3 + 4f_r f_a f_t f_b^2, -f_a(f_s f_r f_b^2 - 4f_b f_a f_t f_r + 4f_s f_r f_t + f_b f_a f_s^2), 0, 0, 0, 2f_s f_b(f_s^2 + f_r f_b^2), 2f_a f_s^3 + 2f_s^2 f_b f_r + 2f_r f_a f_s f_b^2 + 2f_b^3 f_r^2, 2f_a f_r(f_s^2 + f_r f_b^2), 0, f_s f_b^2(f_s^2 - 4f_t f_r), f_b(f_a f_s^3 + f_s^2 f_b f_r - 4f_r f_a f_t f_s - 4f_b f_t f_r^2),
\end{aligned}$$

$$\begin{aligned}
& f_b f_a f_r (f_s^2 - 4 f_t f_r) \Big], \\
& \Big[ 0, 0, 0, 0, 0, -2 f_b f_t (f_b^2 + 4 f_t), -2 f_a f_t (f_b^2 + 4 f_t), -2 f_t f_b^2 (f_b^2 + 4 f_t), 2 f_t (4 f_t f_s + f_s f_b^2 \\
& - 4 f_a f_t f_b - f_b^3 f_a), 0, -2 f_t (4 f_t f_s + f_s f_b^2 + f_b^3 f_a + 4 f_a f_t f_b), -2 f_t (f_b^2 f_a^2 + 2 f_r f_b^2 + 4 f_a^2 f_t \\
& + 8 f_t f_r), 2 f_t^2 f_b (f_b^2 + 4 f_t), 2 f_t (f_s f_b^3 + 4 f_t f_s f_b + f_a f_t f_b^2 + 4 f_t^2 f_a), 2 f_s f_a f_t (f_b^2 + 4 f_t), \\
& f_b f_s (f_b^2 + 4 f_t), -2 f_b f_s^2 + f_s f_a f_b^2 + 4 f_a f_t f_s - 2 f_b^3 f_r f_s f_b^2 (f_b^2 + 4 f_t), -2 f_s^2 f_b^2 - 4 f_s^2 f_t \\
& + 4 f_b f_a f_t f_s + f_s f_b^3 f_a + 4 f_b^2 f_r f_r - 2 f_a (f_s^2 + f_r f_b^2), -f_s^2 f_b^2 + 4 f_s^2 f_t + 4 f_b f_a f_t f_s + f_s f_b^3 f_a - 2 \\
& f_b^4 f_r - 2 f_s^3 - 3 f_b f_a f_s^2 + f_s f_b^2 f_a^2 + 4 f_s f_r f_b^2 + 4 f_s f_a^2 f_t + 8 f_s f_r f_t - 2 f_b^3 f_r f_a + 4 f_b f_a f_t f_r \\
& - f_t f_s f_b (f_b^2 + 4 f_t), -2 f_s^2 f_b^3 - 4 f_s^2 f_b f_t - f_s f_a f_t f_b^2 - 4 f_s f_a f_t^2 + 4 f_b^3 f_r f_r f_b f_s^3 - 2 f_b^2 f_a f_s^2 - 4 \\
& f_s^2 f_a f_t - 4 f_s f_b f_t f_r + 4 f_r f_a f_t f_b^2, 0, -2 f_s^3 - 2 f_b f_a f_s^2 - 2 f_s f_r f_b^2 - 2 f_b^3 f_r f_a - 2 f_s^2 f_a^2 - 4 f_s^2 f_r \\
& - 2 f_b^2 f_a^2 f_r - 4 f_r^2 f_b^2, 2 f_t f_b (f_s^2 + f_r f_b^2), f_b f_s^3 + 2 f_s^2 f_a f_t - f_b^2 f_a f_s^2 + 2 f_r f_s f_b^3 + 4 f_s f_b f_t f_r \\
& + 6 f_r f_a f_t f_b^2, 2 f_a f_s^3 - 2 f_s^2 f_b f_r - f_a^2 f_s^2 f_b + 2 f_r f_a f_s f_b^2 + 8 f_b f_t f_r^2 + 4 f_r f_b f_a^2 f_r, 0, f_b^2 f_t (f_s^2 \\
& - 4 f_t f_r), f_b (f_b f_s^3 + f_s^2 f_a f_t - 4 f_s f_b f_t f_r - 4 f_a f_t^2 f_r), f_s f_b f_a (f_s^2 - 4 f_t f_r) \Big], \\
& \Big[ 0, 0, 0, 0, 0, 0, -2 f_b f_t (f_b^2 + 4 f_t), 0, 4 f_t^2 (f_b^2 + 4 f_t), 0, -2 f_t (8 f_t^2 + f_b^4 + 6 f_t f_b^2), \\
& -2 f_t (4 f_t f_s + f_s f_b^2 + f_b^3 f_a + 4 f_a f_t f_b), 0, 2 f_t^2 f_b (f_b^2 + 4 f_t), 2 f_t^2 f_a (f_b^2 + 4 f_t), 0, f_b f_s (f_b^2 \\
& + 4 f_t), 0, -2 f_t f_s (f_b^2 + 4 f_t), -2 f_b (f_s^2 + f_r f_b^2), f_s (8 f_t^2 + f_b^4 + 6 f_t f_b^2), 8 f_s^2 f_t + f_s f_b^3 f_a \\
& + 4 f_b f_a f_t f_s + 8 f_b^2 f_r f_r, 0, -f_t f_s f_b (f_b^2 + 4 f_t), f_t (2 f_b f_s^2 - f_s f_a f_b^2 - 4 f_a f_t f_s - 8 f_b f_t f_r), 0, -2 \\
& f_s^2 f_b^2 - 4 f_s^2 f_t - 4 f_b^2 f_r f_t - 2 f_b^4 f_r - 2 f_s^3 - 2 f_b f_a f_s^2 - 2 f_s f_r f_b^2 - 2 f_b^3 f_r f_a, 0, -f_b (f_s^2 f_b^2 - 6 \\
& f_b^2 f_r f_t - 8 f_r f_t^2), -f_b f_s^3 + 2 f_s^2 f_a f_t - f_b^2 f_a f_s^2 + 4 f_s f_b f_t f_r + 6 f_r f_a f_t f_b^2, 0, 0, f_b^2 f_t (f_s^2 - 4 f_t f_r), \\
& f_a f_t f_b (f_s^2 - 4 f_t f_r) \Big], \\
& \Big[ 0, 0, 0, 0, 0, 0, 0, 0, 0, 4 f_t (f_b^2 + 4 f_t), 0, 4 f_b f_t (f_b^2 + 4 f_t), 0, 0, -4 f_t^2 (f_b^2 + 4 f_t), 0, 0, 0, 0, \\
& -2 f_s (f_b^2 + 4 f_t), 0, -2 f_b f_s (f_b^2 + 4 f_t), 0, 0, 2 f_t f_s (f_b^2 + 4 f_t), 4 f_s^2 + 4 f_r f_b^2, 0, 2 f_b (2 f_r f_b^2 \\
& - 4 f_t f_r + 3 f_s^2), 0, 0, -12 f_b^2 f_r f_t + 2 f_s^2 f_b^2 - 4 f_s^2 f_r, 0, 0, 0, -2 f_b f_t (f_s^2 - 4 f_t f_r) \Big], \\
& \Big[ 0, 0, -2 f_a f_t (f_b^2 + 4 f_t), 0, -2 f_t (4 f_t f_s + f_s f_b^2 + f_b^3 f_a + 4 f_a f_t f_b), 0, f_a f_s (f_b^2 + 4 f_t), 0, \\
& f_s (4 f_t f_s + f_s f_b^2 + f_b^3 f_a + 4 f_a f_t f_b), -2 f_a (f_s^2 + f_r f_b^2), 4 f_r f_t (f_b^2 + 4 f_t), -2 f_s^3 - 3 f_b f_a f_s^2 \\
& - 2 f_s f_r f_b^2 - 2 f_b^3 f_r f_a + 4 f_b f_a f_t f_r, 0, 2 f_b f_t f_r (f_b^2 + 4 f_t), -f_b (f_s^3 + f_b f_a f_s^2 - 4 f_s f_r f_t \\
& - 4 f_b f_a f_t f_r), 0, 0, 0, 0, 0, -2 f_r f_s (f_b^2 + 4 f_t), 0, 0, -f_b f_r f_s (f_b^2 + 4 f_t), 0, 0, 4 f_r (f_s^2 + f_r \\
& f_b^2), 0, 0, 2 f_b f_r (f_r f_b^2 - 4 f_t f_r + 2 f_s^2), 0, 0, 0, f_r f_b^2 (f_s^2 - 4 f_t f_r), 0 \Big], \\
& \Big[ 0, 0, -2 f_b f_t (f_b^2 + 4 f_t), 0, -2 f_t (8 f_t^2 + f_b^4 + 6 f_t f_b^2), 0, f_s f_b^3 - 2 f_a f_t f_b^2 + 4 f_t f_s f_b - 8 f_t^2 f_a \\
& 0, f_b (f_s f_b^3 - 2 f_a f_t f_b^2 + 4 f_t f_s f_b - 8 f_t^2 f_a), -2 f_b (f_s^2 + f_r f_b^2), 4 f_t f_s (f_b^2 + 4 f_t), -4 f_s^2 f_t - 3
\end{aligned}$$

$$\begin{aligned}
& f_s^2 f_b^2 + 16 f_r f_t^2 - 2 f_b^4 f_r + 4 f_b^2 f_r f_r, 0, 2 f_t f_s f_b (f_b^2 + 4 f_t), -f_b (f_s^2 f_b^2 + 2 f_s^2 f_t - 6 f_b^2 f_r f_t \\
& - 16 f_r f_t^2), 0, f_a f_s (f_b^2 + 4 f_t), 0, f_s (4 f_t f_s + f_s f_b^2 + f_b^3 f_a + 4 f_a f_t f_b), -2 f_a (f_s^2 + f_r f_b^2), -2 ( \\
& f_b^2 + 4 f_t) f_s^2, -2 f_s^3 - 3 f_b f_a f_s^2 - 4 f_s f_r f_b^2 - 8 f_s f_r f_t - 2 f_b^3 f_r f_a + 4 f_b f_a f_t f_r, 0, -f_b f_s^2 (f_b^2 \\
& + 4 f_t), -f_b (f_s^3 + f_b f_a f_s^2 + f_s f_r f_b^2 - 4 f_b f_a f_t f_r), 0, 4 f_s (f_s^2 + f_r f_b^2), 4 f_r (f_s^2 + f_r f_b^2), 0, \\
& 2 f_b f_s (f_r f_b^2 - 4 f_t f_r + 2 f_s^2), 2 f_b f_r (f_r f_b^2 - 4 f_t f_r + 2 f_s^2), 0, 0, f_s f_b^2 (f_s^2 - 4 f_t f_r), f_r f_b^2 (f_s^2 \\
& - 4 f_t f_r) \Big], \\
& [0, 0, 0, 0, 0, 0, -2 f_b f_t (f_b^2 + 4 f_t), 0, -2 f_t (8 f_t^2 + f_b^4 + 6 f_t f_b^2), -2 f_a f_t (f_b^2 + 4 f_t), 4 f_t^2 (f_b^2 \\
& + 4 f_t), 2 f_t (4 f_t f_s + f_s f_b^2 - 4 f_a f_t f_b - f_b^3 f_a), 0, 2 f_t^2 f_b (f_b^2 + 4 f_t), 2 f_t f_s f_b (f_b^2 + 4 f_t), 0, \\
& f_b f_s (f_b^2 + 4 f_t), 0, f_s (8 f_t^2 + f_b^4 + 6 f_t f_b^2), -2 f_b f_s^2 + f_s f_a f_b^2 + 4 f_a f_t f_s - 2 f_b^3 f_r, -2 f_t f_s (f_b^2 \\
& + 4 f_t), -4 f_s^2 f_b^2 - 8 f_s^2 f_t + 4 f_b f_a f_t f_s + f_s f_b^3 f_a - 2 f_b^4 f_r, 0, -f_t f_s f_b (f_b^2 + 4 f_t), -2 f_b (f_s^2 f_b^2 \\
& + 3 f_s^2 f_t - 2 f_b^2 f_r f_t - 4 f_r f_t^2), -2 f_a (f_s^2 + f_r f_b^2), 4 f_t (f_s^2 + f_r f_b^2), 2 f_s^3 - 3 f_b f_a f_s^2 + 2 f_s f_r f_b^2 \\
& - 2 f_b^3 f_r f_a + 4 f_b f_a f_t f_r, 0, 2 f_t f_b (f_r f_b^2 - 4 f_t f_r + 2 f_s^2), f_b (3 f_s^3 - f_b f_a f_s^2 - 4 f_s f_r f_t + 2 f_s f_r f_b^2 \\
& + 4 f_b f_a f_t f_r), 0, 0, f_b^2 f_t (f_s^2 - 4 f_t f_r), f_s f_b^2 (f_s^2 - 4 f_t f_r) \Big], \\
& [0, 0, 0, 0, 0, 0, 0, 0, 0, -2 f_b f_t (f_b^2 + 4 f_t), 0, -2 f_t f_b^2 (f_b^2 + 4 f_t), 0, 0, 2 f_t^2 f_b (f_b^2 + 4 f_t), 0, \\
& 0, 0, 0, f_b f_s (f_b^2 + 4 f_t), 0, f_s f_b^2 (f_b^2 + 4 f_t), 0, 0, -f_t f_s f_b (f_b^2 + 4 f_t), -2 f_b (f_s^2 + f_r f_b^2), 0, - \\
& f_b^2 (2 f_r f_b^2 - 4 f_t f_r + 3 f_s^2), 0, 0, -f_b (-2 f_s^2 f_t + f_s^2 f_b^2 - 6 f_b^2 f_r f_t), 0, 0, 0, f_b^2 f_t (f_s^2 - 4 f_t f_r) \Big], \\
& [-4 f_r f_t (f_b^2 + 4 f_t), 2 f_r f_s (f_b^2 + 4 f_t), -4 f_r (f_s^2 + f_r f_b^2), -4 f_a f_t f_r (f_b^2 + 4 f_t), -2 f_b f_r (f_s^2 \\
& - 4 f_t f_r), 0, 0, 2 f_s f_a f_r (f_b^2 + 4 f_t), 0, 0, -4 f_a f_r (f_s^2 + f_r f_b^2), 0, 4 f_r^2 f_t (f_b^2 + 4 f_t), -2 f_b f_a f_r ( \\
& f_s^2 - 4 f_t f_r), 0, 0, 0, 0, 0, 0, 0, 0, -2 f_s f_r^2 (f_b^2 + 4 f_t), 0, 0, 0, 0, 0, 4 f_r^2 (f_s^2 + f_r f_b^2), 0, 0, 0, \\
& 2 f_b f_r^2 (f_s^2 - 4 f_t f_r), 0, 0 \Big], \\
& [-2 f_t f_s (f_b^2 + 4 f_t), 4 f_s^2 f_t + f_s^2 f_b^2 - 4 f_b^2 f_r f_t - 16 f_r f_t^2, -2 f_s (f_s^2 + f_r f_b^2), -2 f_t (f_s f_a f_b^2 \\
& + 4 f_a f_t f_s + 4 f_b f_t f_r + f_b^3 f_r), -f_b f_s^3 + 4 f_s f_b f_t f_r - 2 f_r f_a f_t f_b^2 - 8 f_a f_t^2 f_r, 2 f_r f_s (f_b^2 + 4 f_t), \\
& -4 f_r (f_s^2 + f_r f_b^2), f_b^2 f_a f_s^2 + 4 f_s^2 f_a f_t + 4 f_s f_b f_t f_r + f_r f_s f_b^3 - 2 f_r f_a f_t f_b^2 - 8 f_a f_t^2 f_r, -f_r (2 f_b f_s^2 \\
& - f_s f_a f_b^2 - 4 f_a f_t f_s - 8 f_b f_t f_r), 0, -2 f_a f_s^3 - 2 f_s^2 f_b f_r - 2 f_r f_a f_s f_b^2 - 2 f_b^3 f_r^2, -2 f_a f_r (f_s^2 + f_r \\
& f_b^2), 4 f_t f_r f_s (f_b^2 + 4 f_t), -f_b f_a f_s^3 - f_s^2 f_r f_b^2 + 4 f_s f_b f_a f_t f_r + 8 f_r^2 f_t f_b^2 + 16 f_r^2 f_t^2, -f_b f_a f_r (f_s^2 \\
& - 4 f_t f_r), 0, 0, f_s f_a f_r (f_b^2 + 4 f_t), 0, 0, -2 f_a f_r (f_s^2 + f_r f_b^2), 0, -2 f_r f_s^2 (f_b^2 + 4 f_t), -f_r (2 f_s f_r \\
& f_b^2 - 4 f_b f_a f_t f_r + 8 f_s f_r f_t + f_b f_a f_s^2), 0, 0, 0, 0, 4 f_s f_r (f_s^2 + f_r f_b^2), 4 f_r^2 (f_s^2 + f_r f_b^2), 0, 0, \\
& 2 f_s f_b f_r (f_s^2 - 4 f_t f_r), 2 f_b f_r^2 (f_s^2 - 4 f_t f_r), 0 \Big], \\
& [0, -2 f_t f_s (f_b^2 + 4 f_t), -4 f_r f_t (f_b^2 + 4 f_t), -2 f_t^2 f_a (f_b^2 + 4 f_t), -2 f_s f_a f_t (f_b^2 + 4 f_t), (f_b^2
\end{aligned}$$



[illegible]

$$\begin{aligned}
& f_s^2 + f_r f_b^2), -2f_a f_r (f_s^2 + f_r f_b^2), 4f_t f_s (f_s^2 + f_r f_b^2), 4f_s^4 - f_b f_a f_s^3 + 4f_s^2 f_r f_t + 4f_s^2 f_r f_b^2 \\
& + 4f_s f_b f_a f_t f_r + 4f_r^2 f_t f_b^2, f_r (4f_s f_r f_b^2 + 4f_b f_a f_t f_r - f_b f_a f_s^2 + 4f_s^3), 0, 2f_s f_b f_t (f_s^2 - 4f_t f_r), \\
& 2f_b (f_s^4 - 3f_s^2 f_r f_t - 4f_r^2 f_t^2), 2f_s f_b f_r (f_s^2 - 4f_t f_r) ], \\
& [0, 0, -4f_t^2 (f_b^2 + 4f_t), 0, -2f_t^2 f_b (f_b^2 + 4f_t), 0, 0, 0, f_t (f_s f_b^3 - 2f_a f_t f_b^2 + 4f_t f_s f_b - 8 \\
& f_t^2 f_a), -4f_t (f_s^2 + f_r f_b^2), -2f_t f_s f_b (f_b^2 + 4f_t), -4f_t f_b (f_s^2 + f_r f_b^2), 0, 4f_t^2 f_s (f_b^2 + 4f_t), -f_t ( \\
& f_s^2 f_b^2 - 8f_b^2 f_r f_t - 16f_r f_t^2), 0, (f_b^2 + 4f_t) f_s^2, 0, f_s f_a f_t (f_b^2 + 4f_t), -2f_s (f_s^2 + f_r f_b^2), f_b f_s^2 (f_b^2 \\
& + 4f_t), -f_b f_s^3 - 2f_s^2 f_a f_t + f_r f_s f_b^3 + 8f_s f_b f_t f_r - 2f_r f_a f_t f_b^2, 0, -2f_t f_s^2 (f_b^2 + 4f_t), -f_t (2f_s f_r \\
& f_b^2 - 4f_b f_a f_t f_r + 8f_s f_r f_t + f_b f_a f_s^2), 0, -2f_s f_b (f_s^2 + f_r f_b^2), -2f_b f_r (f_s^2 + f_r f_b^2), 0, -f_s (f_s^2 f_b^2 \\
& - 4f_s^2 f_t - 8f_b^2 f_r f_t), -f_r (f_s^2 f_b^2 - 4f_s^2 f_t - 8f_b^2 f_r f_t), 0, 0, 2f_s f_b f_t (f_s^2 - 4f_t f_r), 2f_b f_t f_r (f_s^2 \\
& - 4f_t f_r) ], \\
& [0, 0, 0, 0, 0, -4f_t^2 (f_b^2 + 4f_t), -4f_t f_s (f_b^2 + 4f_t), -4f_t^2 f_b (f_b^2 + 4f_t), -4f_t f_s f_b (f_b^2 + 4f_t), \\
& -4f_r f_t (f_b^2 + 4f_t), -4f_t^2 f_a (f_b^2 + 4f_t), -4f_s f_a f_t (f_b^2 + 4f_t), 4f_t^3 (f_b^2 + 4f_t), 8f_t^2 f_s (f_b^2 \\
& + 4f_t), 4f_t f_s^2 (f_b^2 + 4f_t), 2f_t f_s (f_b^2 + 4f_t), -4f_b^2 f_r f_t + 2f_s^2 f_b^2 + 4f_s^2 f_r 2f_t f_s f_b (f_b^2 + 4f_t), \\
& 2f_b (4f_r f_t^2 + f_s^2 f_b^2 + 3f_s^2 f_t), -2f_s (f_r f_b^2 - 4f_t f_r + 2f_s^2), -2f_t (2f_b^3 f_r - f_s f_a f_b^2 + 2f_b f_s^2 \\
& - 4f_a f_t f_s), -2f_s (2f_b^3 f_r - 4f_b f_t f_r - f_s f_a f_b^2 + 3f_b f_s^2 - 4f_a f_t f_s), -2f_t^2 f_s (f_b^2 + 4f_t), \\
& -2f_t (3f_s^2 f_b^2 + 8f_s^2 f_t - 4f_b^2 f_r f_t), -4f_s (2f_s^2 f_t + f_s^2 f_b^2 - 2f_b^2 f_r f_t), -4f_r (f_s^2 + f_r f_b^2), \\
& -4f_a f_t (f_s^2 + f_r f_b^2), 8f_b f_t f_r^2 - 4f_r f_a f_s f_b^2 - 2f_s^2 f_b f_r - 4f_a f_s^3, 4f_t^2 (f_s^2 + f_r f_b^2), 2f_t (4f_s f_r f_b^2 \\
& + 4f_b f_a f_t f_r - f_b f_a f_s^2 + 4f_s^3), 2f_s (2f_s f_r f_b^2 + 4f_b f_a f_t f_r - f_b f_a f_s^2 + 2f_s^3), 0, 2f_b f_t^2 (f_s^2 \\
& - 4f_t f_r), 4f_s f_b f_t (f_s^2 - 4f_t f_r), 2f_b f_s^2 (f_s^2 - 4f_t f_r) ], \\
& [0, 0, 0, 0, 0, 0, -4f_t^2 (f_b^2 + 4f_t), 0, -2f_t^2 f_b (f_b^2 + 4f_t), -2f_t f_s (f_b^2 + 4f_t), -2f_t^2 f_b (f_b^2 \\
& + 4f_t), -2f_t (f_s f_b^3 + 4f_t f_s f_b + f_a f_t f_b^2 + 4f_t^2 f_a), 0, 4f_t^3 (f_b^2 + 4f_t), 4f_t^2 f_s (f_b^2 + 4f_t), 0, \\
& 2f_t f_s (f_b^2 + 4f_t), 0, f_t f_s f_b (f_b^2 + 4f_t), f_b^2 (f_s^2 - 4f_t f_r), f_t f_s f_b (f_b^2 + 4f_t), f_s^2 f_b^3 + 4f_s f_a f_t^2 \\
& + f_s f_a f_t f_b^2 - 2f_b^3 f_r f_t + 8f_r f_t^2 f_b, 0, -2f_t^2 f_s (f_b^2 + 4f_t), -f_t (3f_s^2 f_b^2 + 8f_s^2 f_t - 4f_b^2 f_r f_t), \\
& -2f_s (f_s^2 + f_r f_b^2), -2f_t f_b (f_s^2 + f_r f_b^2), -3f_b f_s^3 - 2f_s^2 f_a f_t - 2f_r f_s f_b^3 + 4f_s f_b f_t f_r - 2f_r f_a f_t \\
& f_b^2, 0, -f_t (f_s^2 f_b^2 - 4f_s^2 f_t - 8f_b^2 f_r f_t), 4f_t f_s^3 - f_b^2 f_s^3 - f_a f_t f_b f_s^2 + 8f_r f_t f_s f_b^2 + 4f_r f_t^2 f_a f_b, 0, 0, \\
& 2f_b f_t^2 (f_s^2 - 4f_t f_r), 2f_s f_b f_t (f_s^2 - 4f_t f_r) ], \\
& [0, 0, 0, 0, 0, 0, 0, 0, 0, -4f_t^2 (f_b^2 + 4f_t), 0, -4f_t^2 f_b (f_b^2 + 4f_t), 0, 0, 4f_t^3 (f_b^2 + 4f_t), 0, 0, \\
& 0, 0, 2f_t f_s (f_b^2 + 4f_t), 0, 2f_t f_s f_b (f_b^2 + 4f_t), 0, 0, -2f_t^2 f_s (f_b^2 + 4f_t), -4f_t (f_s^2 + f_r f_b^2), 0, \\
& -2f_b f_t (2f_r f_b^2 - 4f_t f_r + 3f_s^2), 0, 0, -2f_t (-2f_s^2 f_t + f_s^2 f_b^2 - 6f_b^2 f_r f_t), 0, 0, 0, 2f_b f_t^2 (f_s^2
\end{aligned}$$

$$-4f_t f_r) \Big],$$

$$\begin{aligned} & [8f_t (f_a f_b + 2f_s), -16f_t f_r - 4f_b f_a f_s - 4f_s^2, 8f_r (f_a f_b + 2f_s), -8f_b f_t f_r + 2f_b f_s^2 + 8f_b f_a^2 f_t \\ & + 16f_a f_t f_s, 2f_a (f_s^2 - 4f_t f_r), 0, 0, -4f_a (4f_t f_r + f_b f_a f_s + f_s^2), 0, 0, 8f_a f_r (f_a f_b + 2f_s), 0, \\ & -16f_b f_a f_t f_r - 16f_s f_r f_t + 2f_b f_a f_s^2, 2f_a^2 (f_s^2 - 4f_t f_r), 0, 0, 0, 0, 0, 0, 0, 0, 4f_r (4f_t f_r + f_b f_a f_s \\ & + f_s^2), 0, 0, 0, 0, 0, -8f_r^2 (f_a f_b + 2f_s), 0, 0, -2f_b f_r (f_s^2 - 4f_t f_r), -2f_a f_r (f_s^2 - 4f_t f_r), 0, 0 \\ & ] \end{aligned}$$

$$\begin{aligned} & [0, 8f_t (f_a f_b + 2f_s), 0, 4f_b f_t (f_a f_b + 2f_s), 4f_a f_t (f_a f_b + 2f_s), -16f_t f_r - 4f_b f_a f_s - 4f_s^2, \\ & 8f_r (f_a f_b + 2f_s), 8f_a f_t f_s - 2f_s f_a f_b^2 + 4f_b f_a^2 f_t - 16f_b f_t f_r - 2f_a (f_b f_a f_s + 8f_t f_r), 0, \\ & 4f_b f_r (f_a f_b + 2f_s), 4f_a f_r (f_a f_b + 2f_s), -8f_s^2 f_t + f_s^2 f_b^2 - 4f_b f_a f_t f_s - 4f_b^2 f_r f_r - 16f_b f_a f_t f_r \\ & - 16f_s f_r f_t + 2f_b f_a f_s^2, f_a^2 (f_s^2 - 4f_t f_r), 0, 0, -2f_a (4f_t f_r + f_b f_a f_s + f_s^2), 0, 0, 4f_a f_r (f_a f_b \\ & + 2f_s), 0, 2f_s^3 + 3f_b f_a f_s^2 + 8f_s f_r f_t - 4f_b f_a f_t f_r, 4f_s^2 f_r + f_s^2 f_a^2 + 4f_b f_a f_r f_s - 4f_a^2 f_t f_r + 16 \\ & f_r^2 f_r, 0, 0, 0, 0, -4f_s f_r (f_a f_b + 2f_s), -8f_r^2 (f_a f_b + 2f_s), 0, -f_b f_s (f_s^2 - 4f_t f_r), 8f_b f_t f_r^2 - 2 \\ & f_s^2 f_b f_r + 4f_r f_a f_t f_s - f_a f_s^3, -2f_a f_r (f_s^2 - 4f_t f_r), 0] \end{aligned}$$

$$\begin{aligned} & [0, 0, 8f_t (f_a f_b + 2f_s), 0, 4f_b f_t (f_a f_b + 2f_s), 0, -16f_t f_r - 4f_b f_a f_s - 4f_s^2, 0, -2f_b (4f_t f_r \\ & + f_b f_a f_s + f_s^2), 8f_r (f_a f_b + 2f_s), 2f_b f_s^2 + 8f_a f_t f_s + 4f_b f_a^2 f_t - 8f_b f_t f_r, 2f_a f_s^2 + 8f_b f_r f_s \\ & + 4f_r f_a f_b^2 - 8f_a f_t f_r, 0, -8f_s^2 f_t + f_s^2 f_b^2 - 4f_b f_a f_t f_s - 4f_b^2 f_r f_r f_b f_a (f_s^2 - 4f_t f_r), 0, 0, 0, 0, \\ & 0, -2f_a (4f_t f_r + f_b f_a f_s + f_s^2), 0, 0, 2f_s (4f_t f_r + f_b f_a f_s + f_s^2), 0, 0, 4f_a f_r (f_a f_b + 2f_s), 0, \\ & f_b f_a (f_s^2 - 4f_t f_r), f_s^2 f_a^2 - 8f_s^2 f_r - 4f_b f_a f_r f_s - 4f_a^2 f_t f_r, 0, 0, -f_b f_s (f_s^2 - 4f_t f_r), -f_a f_s (f_s^2 \\ & - 4f_t f_r), 0] \end{aligned}$$

$$\begin{aligned} & [-4f_a f_t (f_a f_b + 2f_s), 2f_a (4f_t f_r + f_b f_a f_s + f_s^2), -4f_a f_r (f_a f_b + 2f_s), -f_a (f_b f_s^2 + 8f_a f_t f_s \\ & + 4f_b f_a^2 f_t - 4f_b f_t f_r), -f_a^2 (f_s^2 - 4f_t f_r), 0, 0, 2f_a^2 (4f_t f_r + f_b f_a f_s + f_s^2), 0, 0, -4f_a^2 f_r (f_a f_b \\ & + 2f_s), 0, -f_a (f_b f_a f_s^2 - 8f_s f_r f_t - 8f_b f_a f_t f_r), -f_a^3 (f_s^2 - 4f_t f_r), 0, 0, 0, 0, 0, 0, 0, 0, \\ & -2f_a f_r (4f_t f_r + f_b f_a f_s + f_s^2), 0, 0, 0, 0, 0, 4f_a f_r^2 (f_a f_b + 2f_s), 0, 0, f_b f_a f_r (f_s^2 - 4f_t f_r), \\ & f_a^2 f_r (f_s^2 - 4f_t f_r), 0, 0] \end{aligned}$$

$$\begin{aligned} & [-4f_b f_t (f_a f_b + 2f_s), 2f_b f_s^2 - 8f_a f_t f_s + 2f_s f_a f_b^2 - 4f_b f_a^2 f_t + 8f_b f_t f_r - 4f_b f_r (f_a f_b \\ & + 2f_s), 8f_s^2 f_t - f_s^2 f_b^2 - 4f_b f_a f_t f_s - 4f_b^2 f_a^2 f_t + 4f_b^2 f_r f_r - f_b f_a f_s^2 + 16f_s f_r f_t + 12f_b f_a f_t f_r \\ & 2f_a (4f_t f_r + f_b f_a f_s + f_s^2), -4f_a f_r (f_a f_b + 2f_s), -2f_s^3 - f_b f_a f_s^2 - 24f_s f_r f_t - 8f_s f_a^2 f_t + 2f_s \\ & f_b^2 f_a^2 - 4f_b f_t f_a^3 + 4f_b f_a f_t f_r - 4f_s^2 f_r - f_s^2 f_a^2 - 4f_b f_a f_r f_s + 4f_a^2 f_t f_r - 16f_r^2 f_r, 0, 4f_r (2f_s^2 \\ & - f_b f_a f_s - f_b^2 f_a^2), 8f_r^2 (f_a f_b + 2f_s), f_b f_s^3 + 8f_s^2 f_a f_t - f_b^2 f_a f_s^2 + 4f_b f_a^2 f_s f_t - 4f_s f_b f_t f_r \end{aligned}$$

$$\begin{aligned}
& + 4f_r f_a f_t f_b^2, f_a f_s^3 + 2f_s^2 f_b f_r - f_a^2 f_s^2 f_b + 4f_r f_a f_t f_s - 8f_b f_t f_r^2 + 8f_r f_b f_a^2 f_r - 2f_a f_r (f_s^2 \\
& - 4f_t f_r), 0, 0, 4f_s^2 f_r + 2f_s^2 f_a^2 + 4f_b f_a f_r f_s + 2f_s f_b f_a^3 + 8f_a^2 f_t f_r + 16f_r^2 f_p, 0, 0, -4f_r (2f_s f_a^2 \\
& + 4f_r f_s + 2f_b f_r f_a + f_b f_a^3), 0, -2f_a f_s^3 - 2f_s^2 f_b f_r - 3f_a^2 f_s^2 f_b - 8f_r f_a f_t f_s + 8f_b f_t f_r^2 + 4f_r f_b \\
& f_a^2 f_p - f_a (4f_s^2 f_r + f_s^2 f_a^2 + 2f_b f_a f_r f_s - 4f_a^2 f_t f_r), 0, 0, 0, 0, 4f_r f_s f_a (f_a f_b + 2f_s), 4f_a f_r^2 (f_a f_b \\
& + 2f_s), 0, f_s f_b f_a (f_s^2 - 4f_t f_r), f_a (f_a f_s^3 + f_s^2 f_b f_r - 4f_r f_a f_t f_s - 4f_b f_t f_r^2), f_a^2 f_r (f_s^2 - 4f_t f_r), \\
& 0],
\end{aligned}$$

$$\begin{aligned}
& [0, -4f_b f_t (f_a f_b + 2f_s), -4f_a f_t (f_a f_b + 2f_s), 8f_t^2 (f_a f_b + 2f_s), 8f_t f_s (f_a f_b + 2f_s), \\
& 2f_b (4f_t f_r + f_b f_a f_s + f_s^2), 2f_a f_s^2 - 8f_b f_r f_s + 2f_a^2 f_s f_b - 4f_r f_a f_b^2 + 8f_a f_t f_r - f_s^2 f_b^2 - 12f_s^2 f_t \\
& - 16f_b f_a f_t f_s - 4f_b^2 f_a^2 f_t - 16f_r f_t^2 + 4f_b^2 f_r f_p - 4f_s^3 - 5f_b f_a f_s^2 - 16f_s f_r f_t + 4f_b f_a f_t f_p \\
& - 4f_a f_r (f_a f_b + 2f_s), -f_a (f_b f_s^2 + 8f_a f_t f_s + 4f_b f_a^2 f_t - 4f_b f_t f_r), -f_s^2 f_a^2 + 16f_s^2 f_r \\
& + 8f_b f_a f_r f_s + 4f_a^2 f_t f_r, 2f_t (f_b f_s^2 + 4f_a f_t f_s + 2f_b f_a^2 f_t - 4f_b f_t f_r), 2f_b f_s^3 + 10f_s^2 f_a f_t + 4f_b \\
& f_a^2 f_s f_t - 8f_s f_b f_t f_r - 8f_a f_t^2 f_r - 2f_a f_s (f_s^2 - 4f_t f_r), 0, 0, 2f_s^3 + 4f_b f_a f_s^2 + 2f_s f_b^2 f_a^2 + 8f_s f_r f_t \\
& + 8f_b f_a f_t f_r, 0, 0, -4f_s^2 f_r + 2f_s^2 f_a^2 - 8f_b f_a f_r f_s + 2f_s f_b f_a^3 + 16f_r^2 f_t - 4f_b^2 f_a^2 f_r + 8f_a^2 f_t f_r \\
& 0, -f_b f_s^3 - f_b^2 f_a f_s^2 - 2f_s^2 f_a f_t - 2f_b f_a^2 f_s f_t + 4f_s f_b f_t f_r + 4f_r f_a f_t f_b^2 - 8f_a f_t^2 f_r - f_a (3f_s^3 \\
& + 3f_b f_a f_s^2 + 4f_s f_r f_t - 4f_b f_a f_t f_r), 0, 0, -4f_r (2f_s f_a^2 + 4f_r f_s + 2f_b f_r f_a + f_b f_a^3), 0, -2 \\
& f_s^2 f_b f_r - f_a^2 f_s^2 f_b + 8f_r f_a f_t f_s + 8f_b f_t f_r^2 + 8f_r f_b f_a^2 f_p - f_a (-6f_s^2 f_r + f_s^2 f_a^2 - 4f_b f_a f_r f_s - 4 \\
& f_a^2 f_t f_r - 8f_r^2 f_t), 0, f_a f_t f_b (f_s^2 - 4f_t f_r), f_a (f_b f_s^3 + f_s^2 f_a f_t - 4f_s f_b f_t f_r - 4f_a f_t^2 f_r), f_s f_a^2 (f_s^2 \\
& - 4f_t f_r), 0],
\end{aligned}$$

$$\begin{aligned}
& [0, 0, -4f_b f_t (f_a f_b + 2f_s), 0, 8f_t^2 (f_a f_b + 2f_s), 0, 2f_b (4f_t f_r + f_b f_a f_s + f_s^2), 0, -4f_t (4f_t f_r \\
& + f_b f_a f_s + f_s^2), -4f_b f_r (f_a f_b + 2f_s), -f_s^2 f_b^2 - 8f_s^2 f_t - 12f_b f_a f_t f_s - 4f_b^2 f_a^2 f_t + 4f_b^2 f_r f_p \\
& - f_b f_a f_s^2 + 16f_s f_r f_t + 12f_b f_a f_t f_r, 0, 2f_t (f_b f_s^2 + 4f_a f_t f_s + 2f_b f_a^2 f_t - 4f_b f_t f_r), 2f_a f_t (f_s^2 \\
& - 4f_t f_r), 0, 0, 0, 0, 0, 2f_s^3 + 4f_b f_a f_s^2 + 2f_s f_b^2 f_a^2 + 8f_s f_r f_t + 8f_b f_a f_t f_r, 0, 0, -2f_a f_t (4f_t f_r \\
& + f_b f_a f_s + f_s^2), 0, 0, -4f_r (2f_s^2 + 3f_b f_a f_s + f_b^2 f_a^2), 0, -f_b (f_s^3 + f_b f_a f_s^2 - 4f_s f_r f_t \\
& - 4f_b f_a f_t f_r), -f_a (f_s^3 + f_b f_a f_s^2 - 12f_s f_r f_t - 8f_b f_a f_t f_r), 0, 0, f_a f_t f_b (f_s^2 - 4f_t f_r), f_a^2 f_t (f_s^2 \\
& - 4f_t f_r), 0],
\end{aligned}$$

$$\begin{aligned}
& [0, 0, 0, 0, 0, 8f_t (f_a f_b + 2f_s), 0, 8f_b f_t (f_a f_b + 2f_s), 8f_a f_t (f_a f_b + 2f_s), 0, 0, 0, -8 \\
& f_t^2 (f_a f_b + 2f_s), -8f_t f_s (f_a f_b + 2f_s), -8f_r f_t (f_a f_b + 2f_s), -16f_t f_r - 4f_b f_a f_s - 4f_s^2, \\
& 8f_r (f_a f_b + 2f_s), -2f_b (12f_t f_r + 2f_b f_a f_s + f_s^2), -2f_a (12f_t f_r + 2f_b f_a f_s + f_s^2), 0, \\
& 8f_b f_r (f_a f_b + 2f_s), 8f_a f_r (f_a f_b + 2f_s), -8f_b^2 f_r f_t + 16f_r f_t^2 + 2f_s^2 f_b^2 + 4f_b f_a f_t f_s + 4f_s^2 f_p
\end{aligned}$$

$$\begin{aligned}
& -16f_b f_a f_t f_r + 16f_s f_r f_t + 8f_b f_a f_s^2 + 4f_s^3, 16f_r^2 f_t + 4f_b f_a f_r f_s + 4f_s^2 f_r - 8f_a^2 f_t f_r + 2f_s^2 f_a^2, \\
& 0, 0, 0, -8f_r f_t (f_a f_b + 2f_s), -8f_s f_r (f_a f_b + 2f_s), -8f_r^2 (f_a f_b + 2f_s), -2f_b f_t (f_s^2 - 4f_t f_r), \\
& 8f_s f_b f_t f_r + 8f_a f_t^2 f_r - 2f_b f_s^3 - 2f_s^2 f_a f_r, 8f_b f_t f_r^2 - 2f_s^2 f_b f_r + 8f_r f_a f_t f_s - 2f_a f_s^3, -2f_a f_r (f_s^2 \\
& - 4f_t f_r) \Big], \\
& \Big[ 0, 0, 0, 0, 0, 0, 8f_t (f_a f_b + 2f_s), 0, 4f_b f_t (f_a f_b + 2f_s), 0, 4f_b f_t (f_a f_b + 2f_s), 4f_a f_t (f_a f_b \\
& + 2f_s), 0, -8f_t^2 (f_a f_b + 2f_s), -4f_t f_s (f_a f_b + 2f_s), 0, -16f_t f_r - 4f_b f_a f_s - 4f_s^2, 0, \\
& -2f_b (4f_t f_r + f_b f_a f_s + f_s^2), 8f_r (f_a f_b + 2f_s), -2f_b (f_b f_a f_s + 8f_t f_r), 8f_b f_r f_s - 2f_a^2 f_s f_b \\
& + 4f_r f_a f_b^2 - 16f_a f_t f_r, 0, f_s^2 f_b^2 + 4f_s^2 f_t + 4f_b f_a f_t f_s + 16f_r f_t^2 - 4f_b^2 f_r f_r, 2f_s^3 + 3f_b f_a f_s^2 \\
& + 8f_s f_r f_t - 4f_b f_a f_t f_r, 0, 4f_b f_r (f_a f_b + 2f_s), 4f_a f_r (f_a f_b + 2f_s), f_b^2 (f_s^2 - 4f_t f_r), \\
& -16f_b f_a f_t f_r - 16f_s f_r f_t + 2f_b f_a f_s^2, f_s^2 f_a^2 - 8f_s^2 f_r - 4f_b f_a f_r f_s - 4f_a^2 f_t f_r, 0, -2f_b f_t (f_s^2 \\
& - 4f_t f_r), 4f_s f_b f_t f_r + 8f_a f_t^2 f_r - f_b f_s^3 - 2f_s^2 f_a f_r - f_a f_s (f_s^2 - 4f_t f_r) \Big], \\
& \Big[ 0, -4f_a f_t (f_a f_b + 2f_s), 0, -4f_t (2f_s^2 + 3f_b f_a f_s + f_b^2 f_a^2), -4f_t (2f_s f_a^2 + 4f_r f_s + 2f_b f_r f_a \\
& + f_b f_a^3), 2f_a (4f_t f_r + f_b f_a f_s + f_s^2), -4f_a f_r (f_a f_b + 2f_s), 2f_s^3 + 3f_b f_a f_s^2 + 2f_s f_b^2 f_a^2 \\
& + 24f_s f_r f_t + 20f_b f_a f_t f_r, 4f_s^2 f_r + f_s^2 f_a^2 + 4f_b f_a f_r f_s + 2f_s f_b f_a^3 + 12f_a^2 f_t f_r + 16f_r^2 f_r, 0, \\
& -4f_r (2f_s^2 + 3f_b f_a f_s + f_b^2 f_a^2), -4f_r (2f_s f_a^2 + 4f_r f_s + 2f_b f_r f_a + f_b f_a^3), -f_b (f_s^3 + f_b f_a f_s^2 \\
& - 12f_s f_r f_t - 8f_b f_a f_t f_r), -f_a f_s^3 - 2f_s^2 f_b f_r - 2f_a^2 f_s^2 f_b + 12f_r f_a f_t f_s + 12f_r f_b f_a^2 f_t + 8f_b f_t f_r^2, \\
& -f_a (f_s^2 f_a^2 + 2f_s^2 f_r - 4f_a^2 f_t f_r - 8f_r^2 f_t), 0, 0, -4f_r (4f_t f_r + f_b f_a f_s + f_s^2), 0, 0, 8f_r^2 (f_a f_b \\
& + 2f_s), 0, -2f_b f_r (f_b f_a f_s + 8f_t f_r), -2f_r f_a (f_b f_a f_s + 8f_t f_r), 0, 0, 0, 0, 4f_b f_r^2 (f_a f_b \\
& + 2f_s), 4f_a f_r^2 (f_a f_b + 2f_s), 0, f_r f_b^2 (f_s^2 - 4f_t f_r), 2f_b f_a f_r (f_s^2 - 4f_t f_r), f_a^2 f_r (f_s^2 - 4f_t f_r), 0 \\
& \Big], \\
& \Big[ 0, -4f_b f_t (f_a f_b + 2f_s), 0, -4f_t (4f_t f_s + 2f_s f_b^2 + 2f_a f_t f_b + f_b^3 f_a), -4f_t (2f_s^2 + 3f_b f_a f_s + \\
& f_b^2 f_a^2), 2f_b f_s^2 - 8f_a f_t f_s + 2f_s f_a f_b^2 - 4f_b f_a^2 f_t + 8f_b f_t f_r, -4f_b f_r (f_a f_b + 2f_s), f_s^2 f_b^2 + 12f_s^2 f_t \\
& + 2f_s f_b^3 f_a + 12f_b^2 f_r f_t - 4f_b^2 f_a^2 f_t + 16f_r f_t^2, 2f_s^3 + 3f_b f_a f_s^2 + 2f_s f_b^2 f_a^2 - 8f_s f_a^2 f_t + 8f_s f_r f_t \\
& - 4f_b f_t f_a^3 + 12f_b f_a f_t f_r, 0, -4f_r (4f_t f_s + 2f_s f_b^2 + 2f_a f_t f_b + f_b^3 f_a), -4f_r (2f_s^2 + 3f_b f_a f_s + \\
& f_b^2 f_a^2), -f_b (f_s^2 f_b^2 - 6f_s^2 f_t - 4f_b f_a f_t f_s - 8f_r f_t^2 - 4f_b^2 f_r f_t), -f_b f_s^3 - 2f_b^2 f_a f_s^2 + 6f_s^2 f_a f_t \\
& + 12f_s f_b f_t f_r + 4f_b f_a^2 f_s f_t + 12f_r f_a f_t f_b^2 + 8f_a f_t^2 f_r - f_a (f_s^3 + f_b f_a f_s^2 - 12f_s f_r f_t \\
& - 8f_b f_a f_t f_r), 2f_a (4f_t f_r + f_b f_a f_s + f_s^2), -4f_a f_r (f_a f_b + 2f_s), -2f_s^3 - f_b f_a f_s^2 + 2f_s f_b^2 f_a^2 \\
& - 8f_s f_r f_t + 12f_b f_a f_t f_r, f_a^2 (12f_t f_r + 2f_b f_a f_s + f_s^2), 0, 4f_r (2f_s^2 - f_b f_a f_s - f_b^2 f_a^2), -4 \\
& f_a^2 f_r (f_a f_b + 2f_s), -f_b (f_s^3 + 3f_b f_a f_s^2 + 12f_s f_r f_t - 4f_b f_a f_t f_r), -f_a f_s^3 - 2f_s^2 f_b f_r - 4f_a^2 f_s^2 f_b
\end{aligned}$$

$$\begin{aligned}
& -2f_r f_a f_s f_b^2 - 12f_r f_a f_t f_s + 8f_r f_b f_a^2 f_t - 8f_b f_t f_r^2, -f_a (8f_r^2 f_t + 2f_b f_a f_r f_s + 2f_s^2 f_r - 4f_a^2 f_t f_r \\
& + f_s^2 f_a), 0, 0, 0, 4f_b f_r f_s (f_a f_b + 2f_s), 4f_r (2f_a f_s^2 + 2f_b f_r f_s + f_a^2 f_s f_b + f_r f_a f_b^2), 4f_a \\
& f_r^2 (f_a f_b + 2f_s), f_s f_b^2 (f_s^2 - 4f_t f_r), f_b (2f_a f_s^3 + f_s^2 f_b f_r - 8f_r f_a f_t f_s - 4f_b f_t f_r^2), f_a (f_a f_s^3 + 2 \\
& f_s^2 f_b f_r - 4f_r f_a f_t f_s - 8f_b f_t f_r^2), f_a^2 f_r (f_s^2 - 4f_t f_r) ], \\
& [0, 0, 0, 0, 0, -4f_b f_t (f_a f_b + 2f_s), -4f_a f_t (f_a f_b + 2f_s), -4f_b^2 f_t (f_a f_b + 2f_s), 4f_t (2f_s^2 \\
& - f_b f_a f_s - f_b^2 f_a^2), 0, -4f_t (2f_s^2 + 3f_b f_a f_s + f_b^2 f_a^2), -4f_t (2f_s f_a^2 + 4f_r f_s + 2f_b f_r f_a + f_b \\
& f_a^3), 4f_t^2 f_b (f_a f_b + 2f_s), 4f_t (2f_b f_s^2 + f_s f_a f_b^2 + 2f_a f_t f_s + f_b f_a^2 f_t), 4f_s f_a f_t (f_a f_b + 2f_s), \\
& 2f_b (4f_t f_r + f_b f_a f_s + f_s^2), 2f_a f_s^2 - 8f_b f_r f_s + 2f_a^2 f_s f_b - 4f_r f_a f_b^2 + 8f_a f_t f_r f_b^2 (12f_t f_r \\
& + 2f_b f_a f_s + f_s^2), -2f_s^3 - f_b f_a f_s^2 + 2f_s f_b^2 f_a^2 - 8f_s f_r f_t + 12f_b f_a f_t f_r - 4f_a f_r (f_a f_b + 2f_s), 2 \\
& f_s^3 + 3f_b f_a f_s^2 + 2f_s f_b^2 f_a^2 - 8f_s f_r f_b^2 + 8f_s f_r f_t + 12f_b f_a f_t f_r - 4f_b^3 f_r f_a, 12f_s^2 f_r + f_s^2 f_a^2 \\
& + 2f_s f_b f_a^3 + 16f_r^2 f_t + 12f_a^2 f_t f_r - 4f_b^2 f_a^2 f_r - f_b (2f_s^2 f_t + f_s^2 f_b^2 + 2f_b f_a f_t f_s - 4f_b^2 f_r f_t + 8f_r \\
& f_t^2), -f_b f_s^3 - 4f_b^2 f_a f_s^2 - 2f_s^2 f_a f_t - 2f_b f_a^2 f_s f_t - 12f_s f_b f_t f_r + 8f_r f_a f_t f_b^2 - 8f_a f_t^2 f_r - f_a (f_s^3 \\
& + 3f_b f_a f_s^2 + 12f_s f_r f_t - 4f_b f_a f_t f_r), 0, -4f_r (2f_s^2 + 3f_b f_a f_s + f_b^2 f_a^2), -4f_r (2f_s f_a^2 + 4f_r f_s \\
& + 2f_b f_r f_a + f_b f_a^3), -f_b (f_s^3 + f_b f_a f_s^2 - 12f_s f_r f_t - 8f_b f_a f_t f_r), -f_a f_s^3 + 6f_s^2 f_b f_r - 2f_a^2 f_s^2 f_b \\
& + 4f_r f_a f_s f_b^2 + 12f_r f_a f_t f_s + 8f_b f_t f_r^2 + 12f_r f_b f_a^2 f_r - f_a (-6f_s^2 f_r + f_s^2 f_a^2 - 4f_b f_a f_r f_s - 4 \\
& f_a^2 f_t f_r - 8f_r^2 f_t), f_b^2 f_t (f_s^2 - 4f_t f_r), f_b (f_b f_s^3 + 2f_s^2 f_a f_t - 4f_s f_b f_t f_r - 8f_a f_t^2 f_r), f_a (2f_b f_s^3 + \\
& f_s^2 f_a f_t - 8f_s f_b f_t f_r - 4f_a f_t^2 f_r), f_s f_a^2 (f_s^2 - 4f_t f_r) ], \\
& [0, 0, 0, 0, 0, 0, -4f_b f_t (f_a f_b + 2f_s), 0, 8f_t^2 (f_a f_b + 2f_s), 0, -4f_t (4f_t f_s + 2f_s f_b^2 + 2f_a f_t f_b \\
& + f_b^3 f_a), -4f_t (2f_s^2 + 3f_b f_a f_s + f_b^2 f_a^2), 0, 4f_t^2 f_b (f_a f_b + 2f_s), 4f_t^2 f_a (f_a f_b + 2f_s), 0, \\
& 2f_b (4f_t f_r + f_b f_a f_s + f_s^2), 0, -4f_t (4f_t f_r + f_b f_a f_s + f_s^2), -4f_b f_r (f_a f_b + 2f_s), f_s^2 f_b^2 + 4f_s^2 f_t \\
& + 4f_b f_a f_t f_s + 2f_s f_b^3 f_a + 12f_b^2 f_r f_t + 16f_r f_t^2, 2f_s^3 + 3f_b f_a f_s^2 + 2f_s f_b^2 f_a^2 + 24f_s f_r f_t \\
& + 20f_b f_a f_t f_r, 0, -2f_b f_t (f_b f_a f_s + 8f_t f_r), -2f_a f_t (f_b f_a f_s + 8f_t f_r), 0, -4f_r (4f_t f_s + 2f_s f_b^2 \\
& + 2f_a f_t f_b + f_b^3 f_a), -4f_r (2f_s^2 + 3f_b f_a f_s + f_b^2 f_a^2), -f_b (f_s^2 f_b^2 + 2f_s^2 f_t - 8f_r f_t^2 - 4f_b^2 f_r f_t), \\
& -f_b f_s^3 - 2f_b^2 f_a f_s^2 - 2f_s^2 f_a f_t + 12f_s f_b f_t f_r + 12f_r f_a f_t f_b^2 + 8f_a f_t^2 f_r - f_a (f_s^3 + f_b f_a f_s^2 \\
& - 12f_s f_r f_t - 8f_b f_a f_t f_r), 0, f_b^2 f_t (f_s^2 - 4f_t f_r), 2f_a f_t f_b (f_s^2 - 4f_t f_r), f_a^2 f_t (f_s^2 - 4f_t f_r) ], \\
& [0, 0, 0, 0, 0, 0, 0, 0, 0, 8f_t (f_a f_b + 2f_s), 0, 8f_b f_t (f_a f_b + 2f_s), 0, 0, -8f_t^2 (f_a f_b + 2f_s), 0, \\
& 0, 0, 0, -16f_t f_r - 4f_b f_a f_s - 4f_s^2, 0, -4f_b (4f_t f_r + f_b f_a f_s + f_s^2), 0, 0, 4f_t (4f_t f_r + f_b f_a f_s + \\
& f_s^2), 8f_r (f_a f_b + 2f_s), 2f_b (f_s^2 - 4f_t f_r), 8f_r f_a f_b^2 + 16f_b f_r f_s - 8f_a f_t f_r + 2f_a f_s^2, 0, 2f_b^2 (f_s^2 \\
& - 4f_t f_r), -16f_b f_a f_t f_r - 16f_s f_r f_t + 2f_b f_a f_s^2, 0, 0, -2f_b f_t (f_s^2 - 4f_t f_r), -2f_a f_t (f_s^2 - 4f_t f_r) ]
\end{aligned}$$

$$\begin{aligned}
& \left. \begin{aligned}
& [0, 0, -4f_a f_t (f_a f_b + 2f_s), 0, -4f_t (2f_s^2 + 3f_b f_a f_s + f_b^2 f_a^2), 0, 2f_a (4f_t f_r + f_b f_a f_s + f_s^2), \\
& 0, 2f_s^3 + 4f_b f_a f_s^2 + 2f_s f_b^2 f_a^2 + 8f_s f_r f_t + 8f_b f_a f_t f_r - 4f_a f_r (f_a f_b + 2f_s), -f_b f_a f_s^2 + 16f_s f_r f_t \\
& + 12f_b f_a f_t f_r - f_s^2 f_a^2 - 8f_s^2 f_r - 12f_b f_a f_r f_s - 4f_b^2 f_a^2 f_r + 4f_a^2 f_t f_r, 0, -f_b (f_s^3 + f_b f_a f_s^2 \\
& - 12f_s f_r f_t - 8f_b f_a f_t f_r), -f_a (f_s^3 + f_b f_a f_s^2 - 4f_s f_r f_t - 4f_b f_a f_t f_r), 0, 0, 0, 0, 0, -4f_r (4f_t f_r \\
& + f_b f_a f_s + f_s^2), 0, 0, -2f_b f_r (4f_t f_r + f_b f_a f_s + f_s^2), 0, 0, 8f_r^2 (f_a f_b + 2f_s), 0, 2f_b f_r (f_s^2 \\
& - 4f_t f_r), 2f_r (f_a f_s^2 + 4f_b f_r f_s - 4f_a f_t f_r + 2f_r f_a f_b^2), 0, 0, f_r f_b^2 (f_s^2 - 4f_t f_r), f_b f_a f_r (f_s^2 \\
& - 4f_t f_r), 0] \\
& [0, 0, -4f_b f_t (f_a f_b + 2f_s), 0, -4f_t (4f_t f_s + 2f_s f_b^2 + 2f_a f_t f_b + f_b^3 f_a), 0, 2f_b f_s^2 - 8f_a f_t f_s \\
& + 2f_s f_a f_b^2 - 4f_b f_a^2 f_t + 8f_b f_t f_r, 0, 2f_s^2 f_b^2 - 4f_s^2 f_t + 2f_s f_b^3 f_a - 8f_b f_a f_t f_s + 16f_r f_t^2 - 4f_b^2 \\
& f_a^2 f_t + 8f_b^2 f_r f_r - 4f_b f_r (f_a f_b + 2f_s), -f_s^2 f_b^2 + 16f_s^2 f_t + 8f_b f_a f_t f_s + 4f_b^2 f_r f_r - f_b (4f_r f_a f_b^2 \\
& + 8f_b f_r f_s - 4f_a f_t f_r + f_a f_s^2), 0, -f_b (f_s^2 f_b^2 - 6f_s^2 f_t - 4f_b f_a f_t f_s - 8f_r f_t^2 - 4f_b^2 f_r f_t), -f_b^2 f_a f_s^2 \\
& - 2f_s^2 f_a f_t + 8f_s f_b f_t f_r + 8f_a f_t^2 f_r + 8f_r f_a f_t f_b^2, 0, 2f_a (4f_t f_r + f_b f_a f_s + f_s^2), 0, 2f_s^3 + 4f_b f_a \\
& f_s^2 + 2f_s f_b^2 f_a^2 + 8f_s f_r f_t + 8f_b f_a f_t f_r - 4f_a f_r (f_a f_b + 2f_s), -4f_s^3 - 5f_b f_a f_s^2 - 16f_s f_r f_t \\
& + 4f_b f_a f_t f_r - 12f_s^2 f_r - f_s^2 f_a^2 - 16f_b f_a f_r f_s - 4f_b^2 f_a^2 f_r - 16f_r^2 f_t + 4f_a^2 f_t f_r, 0, -f_b (3f_s^3 \\
& + 3f_b f_a f_s^2 + 4f_s f_r f_t - 4f_b f_a f_t f_r), -f_a f_s^3 - 2f_s^2 f_b f_r - f_a^2 f_s^2 f_b + 4f_r f_a f_t f_s - 2f_r f_a f_s f_b^2 \\
& + 4f_r f_b f_a^2 f_t - 8f_b f_t f_r^2, 0, 8f_s f_r (f_a f_b + 2f_s), 8f_r^2 (f_a f_b + 2f_s), 2f_b f_s (f_s^2 - 4f_t f_r), 2f_a f_s^3 \\
& + 10f_s^2 f_b f_r - 8f_r f_a f_t f_s + 4f_r f_a f_s f_b^2 - 8f_b f_t f_r^2, 2f_r (f_a f_s^2 + 4f_b f_r f_s - 4f_a f_t f_r + 2f_r f_a f_b^2), \\
& 0, f_s f_b^2 (f_s^2 - 4f_t f_r), f_b (f_a f_s^3 + f_s^2 f_b f_r - 4f_r f_a f_t f_s - 4f_b f_t f_r^2), f_b f_a f_r (f_s^2 - 4f_t f_r) ] \\
& [0, 0, 0, 0, 0, 0, -4f_b f_t (f_a f_b + 2f_s), 0, -4f_t (4f_t f_s + 2f_s f_b^2 + 2f_a f_t f_b + f_b^3 f_a), \\
& -4f_a f_t (f_a f_b + 2f_s), 8f_t^2 (f_a f_b + 2f_s), 4f_t (2f_s^2 - f_b f_a f_s - f_b^2 f_a^2), 0, 4f_t^2 f_b (f_a f_b + 2f_s), \\
& 4f_t f_s f_b (f_a f_b + 2f_s), 0, 2f_b (4f_t f_r + f_b f_a f_s + f_s^2), 0, 4f_s^2 f_t + 2f_s^2 f_b^2 + 4f_b f_a f_t f_s + 2f_s f_b^3 f_a \\
& + 16f_r f_t^2 + 8f_b^2 f_r f_r - 2f_a f_s^2 - 8f_b f_r f_s + 2f_a^2 f_s f_b - 4f_r f_a f_b^2 + 8f_a f_t f_r - f_s^2 f_b^2 - 4f_s^2 f_t \\
& - 4f_b f_a f_t f_s + 4f_b^2 f_r f_t - 16f_r f_t^2, -2f_s^3 - f_b f_a f_s^2 + 2f_s f_b^2 f_a^2 - 8f_s f_r f_b^2 - 24f_s f_r f_t \\
& + 4f_b f_a f_t f_r - 4f_b^3 f_r f_r, 0, -f_b (f_s^2 f_b^2 + 4f_s^2 f_t + 2f_b f_a f_t f_s - 4f_b^2 f_r f_t), -2f_b f_s^3 - 3f_b^2 f_a f_s^2 \\
& - 2f_s^2 f_a f_t - 8f_s f_b f_t f_r + 4f_r f_a f_t f_b^2 + 8f_a f_t^2 f_r - 4f_a f_r (f_a f_b + 2f_s), -f_b f_a f_s^2 + 16f_s f_r f_t \\
& + 12f_b f_a f_t f_r - 8f_s^2 f_r - f_s^2 f_a^2 - 4f_b f_a f_r f_s - 4f_b^2 f_a^2 f_r + 4f_a^2 f_t f_r, 2f_b f_t (f_s^2 - 4f_t f_r), f_b f_s^3 + 2 \\
& f_s^2 f_a f_t - f_b^2 f_a f_s^2 + 4f_s f_b f_t f_r + 8f_r f_a f_t f_b^2 - 8f_a f_t^2 f_r f_a f_s^3 + 8f_s^2 f_b f_r - f_a^2 f_s^2 f_b + 4f_r f_a f_s f_b^2 \\
& - 4f_r f_a f_t f_s + 4f_r f_b f_a^2 f_r, 0, f_b^2 f_t (f_s^2 - 4f_t f_r), f_b (f_b f_s^3 + f_s^2 f_a f_t - 4f_s f_b f_t f_r - 4f_a f_t^2 f_r),
\end{aligned}
\right]
\end{aligned}$$

$$\begin{aligned}
& f_s f_b f_a (f_s^2 - 4 f_t f_r) \Big], \\
& \Big[ 0, 0, 0, 0, 0, 0, 0, 0, 0, -4 f_b f_t (f_a f_b + 2 f_s), 0, -4 f_b^2 f_t (f_a f_b + 2 f_s), 0, 0, 4 f_t^2 f_b (f_a f_b \\
& + 2 f_s), 0, 0, 0, 0, 2 f_b (4 f_t f_r + f_b f_a f_s + f_s^2), 0, 2 f_b^2 (4 f_t f_r + f_b f_a f_s + f_s^2), 0, 0, \\
& -2 f_b f_t (4 f_t f_r + f_b f_a f_s + f_s^2), -4 f_b f_r (f_a f_b + 2 f_s), -f_b^2 (f_s^2 - 4 f_t f_r), -f_b (4 f_r f_a f_b^2 + 8 f_b f_r f_s \\
& - 4 f_a f_t f_r + f_a f_s^2), 0, -f_b^3 (f_s^2 - 4 f_t f_r), -f_b (f_b f_a f_s^2 - 8 f_s f_r f_t - 8 f_b f_a f_t f_r), 0, 0, f_b^2 f_t (f_s^2 \\
& - 4 f_t f_r), f_a f_t f_b (f_s^2 - 4 f_t f_r) \Big], \\
& \Big[ -8 f_r f_t (f_a f_b + 2 f_s), 4 f_r (4 f_t f_r + f_b f_a f_s + f_s^2), -8 f_r^2 (f_a f_b + 2 f_s), -2 f_r (f_b f_s^2 + 8 f_a f_t f_s \\
& + 4 f_b f_a^2 f_t - 4 f_b f_t f_r), -2 f_a f_r (f_s^2 - 4 f_t f_r), 0, 0, 4 f_a f_r (4 f_t f_r + f_b f_a f_s + f_s^2), 0, 0, -8 f_a \\
& f_r^2 (f_a f_b + 2 f_s), 0, -2 f_r (f_b f_a f_s^2 - 8 f_s f_r f_t - 8 f_b f_a f_t f_r), -2 f_a^2 f_r (f_s^2 - 4 f_t f_r), 0, 0, 0, 0, 0, \\
& 0, 0, 0, -4 f_r^2 (4 f_t f_r + f_b f_a f_s + f_s^2), 0, 0, 0, 0, 0, 8 f_r^3 (f_a f_b + 2 f_s), 0, 0, 2 f_b f_r^2 (f_s^2 - 4 f_t f_r), \\
& 2 f_a f_r^2 (f_s^2 - 4 f_t f_r), 0, 0 \Big], \\
& \Big[ -4 f_t f_s (f_a f_b + 2 f_s), 2 f_s^3 + 2 f_b f_a f_s^2 - 8 f_s f_r f_t - 8 f_b f_a f_t f_r, -4 f_s f_r (f_a f_b + 2 f_s), -f_b f_s^3 - 8 \\
& f_s^2 f_a f_t - 4 f_b f_a^2 f_s f_t - 4 f_s f_b f_t f_r - 4 f_r f_a f_t f_b, -f_a (f_s^3 + 4 f_s f_r f_t + 4 f_b f_a f_t f_r), 4 f_r (4 f_t f_r \\
& + f_b f_a f_s + f_s^2), -8 f_r^2 (f_a f_b + 2 f_s), 2 f_a f_s^3 + 2 f_a^2 f_s^2 f_b + 2 f_r f_a f_s f_b^2 + 16 f_b f_t f_r^2 - 4 f_r f_b f_a^2 f_r \\
& 2 f_r f_a (f_b f_a f_s + 8 f_t f_r), 0, -4 f_r (2 f_a f_s^2 + 2 f_b f_r f_s + f_a^2 f_s f_b + f_r f_a f_b^2), -4 f_a f_r^2 (f_a f_b + 2 f_s), \\
& -f_b f_a f_s^3 + 16 f_s^2 f_r f_t - f_s^2 f_r f_b^2 + 12 f_s f_b f_a f_t f_r + 4 f_r^2 f_t f_b^2, -f_a^2 f_s^3 - 2 f_r f_a f_s^2 f_b + 16 f_r^2 f_t f_s \\
& + 4 f_r f_a^2 f_s f_t + 16 f_r^2 f_a f_t f_b, -f_a^2 f_r (f_s^2 - 4 f_t f_r), 0, 0, 2 f_a f_r (4 f_t f_r + f_b f_a f_s + f_s^2), 0, 0, -4 f_a \\
& f_r^2 (f_a f_b + 2 f_s), 0, -f_r (4 f_s^3 + 5 f_b f_a f_s^2 + 16 f_s f_r f_t - 4 f_b f_a f_t f_r), -f_r (4 f_s^2 f_r + f_s^2 f_a^2 \\
& + 4 f_b f_a f_r f_s - 4 f_a^2 f_t f_r + 16 f_r^2 f_t), 0, 0, 0, 0, 8 f_s f_r^2 (f_a f_b + 2 f_s), 8 f_r^3 (f_a f_b + 2 f_s), 0, \\
& 2 f_s f_b f_r (f_s^2 - 4 f_t f_r), 2 f_r (f_a f_s^3 + f_s^2 f_b f_r - 4 f_r f_a f_t f_s - 4 f_b f_t f_r^2), 2 f_a f_r^2 (f_s^2 - 4 f_t f_r), 0 \Big], \\
& \Big[ 0, -4 f_t f_s (f_a f_b + 2 f_s), -8 f_r f_t (f_a f_b + 2 f_s), -4 f_t^2 f_a (f_a f_b + 2 f_s), -4 f_s f_a f_t (f_a f_b + 2 f_s), \\
& 2 f_s (4 f_t f_r + f_b f_a f_s + f_s^2), -4 f_r (f_s^2 - 4 f_t f_r), -f_b f_s^3 + 2 f_s^2 f_a f_t + 2 f_b f_a^2 f_s f_t - 4 f_s f_b f_t f_r \\
& - 4 f_r f_a f_t f_b^2 + 8 f_a f_t^2 f_r f_s f_a (12 f_t f_r + 2 f_b f_a f_s + f_s^2), -8 f_r^2 (f_a f_b + 2 f_s), -2 f_r (f_b f_s^2 \\
& + 8 f_a f_t f_s + 4 f_b f_a^2 f_t - 4 f_b f_t f_r), -2 f_r f_a (5 f_s^2 + 2 f_b f_a f_s - 4 f_t f_r), -f_t (f_b f_a f_s^2 - 16 f_s f_r f_t \\
& - 12 f_b f_a f_t f_r), -f_b f_a f_s^3 + 16 f_s^2 f_r f_t - f_s^2 f_a^2 f_t + 12 f_s f_b f_a f_t f_r + 4 f_a^2 f_t^2 f_r - f_s f_a^2 (f_s^2 - 4 f_t f_r), \\
& 0, 0, 2 f_b f_r (4 f_t f_r + f_b f_a f_s + f_s^2), 0, 0, 2 f_r (f_a f_s^2 - 4 f_b f_r f_s + f_a^2 f_s f_b - 2 f_r f_a f_b^2 + 4 f_a f_t f_r), \\
& 0, -f_r (f_s^2 f_b^2 + 4 f_s^2 f_t + 4 f_b f_a f_t f_s + 16 f_r f_t^2 - 4 f_b^2 f_r f_t), -f_r (4 f_s^3 + 5 f_b f_a f_s^2 + 16 f_s f_r f_t \\
& - 4 f_b f_a f_t f_r), 0, 0, -4 f_a f_r^2 (f_a f_b + 2 f_s), 0, -f_r (f_b f_a f_s^2 - 16 f_s f_r f_t - 12 f_b f_a f_t f_r), -f_r ( \\
& - 16 f_s^2 f_r + f_s^2 f_a^2 - 8 f_b f_a f_r f_s - 4 f_a^2 f_t f_r), 0, 2 f_b f_t f_r (f_s^2 - 4 f_t f_r), 2 f_r (f_b f_s^3 + f_s^2 f_a f_t
\end{aligned}$$



$$\begin{aligned}
& -4f_s f_b f_t f_r - 4f_a f_t^2 f_r), 2f_s f_a f_r (f_s^2 - 4f_t f_r), 0], \\
& [0, 0, -4f_t f_s (f_a f_b + 2f_s), 0, -4f_t^2 f_a (f_a f_b + 2f_s), 0, 2f_s (4f_t f_r + f_b f_a f_s + f_s^2), 0, \\
& 2f_a f_t (4f_t f_r + f_b f_a f_s + f_s^2), -4f_s f_r (f_a f_b + 2f_s), -f_b (f_s^3 + 4f_s f_r f_t + 4f_b f_a f_t f_r), -f_a (f_s^3 \\
& + 4f_s f_r f_t + 4f_b f_a f_t f_r), 0, -f_t (f_b f_a f_s^2 - 16f_s f_r f_t - 12f_b f_a f_t f_r), -f_a^2 f_t (f_s^2 - 4f_t f_r), 0, 0, 0, \\
& 0, 0, 2f_b f_r (4f_t f_r + f_b f_a f_s + f_s^2), 0, 0, -4f_r f_t (4f_t f_r + f_b f_a f_s + f_s^2), 0, 0, -4f_b f_r^2 (f_a f_b \\
& + 2f_s), 0, -f_r f_b^2 (f_s^2 - 4f_t f_r), -f_r (f_b f_a f_s^2 - 16f_s f_r f_t - 12f_b f_a f_t f_r), 0, 0, 2f_b f_t f_r (f_s^2 \\
& - 4f_t f_r), 2f_a f_t f_r (f_s^2 - 4f_t f_r), 0], \\
& [-8f_t^2 (f_a f_b + 2f_s), -4f_t (3f_s^2 + f_b f_a f_s - 4f_t f_r), -8f_r f_t (f_a f_b + 2f_s), -2f_b f_t (9f_s^2 \\
& + 4f_b f_a f_s - 4f_t f_r), -2f_t (4f_r f_a f_b^2 + 8f_b f_r f_s - 4f_a f_t f_r + f_a f_s^2), -8f_b f_a f_t f_r + 4f_b f_a f_s^2 + 4 \\
& f_s^3, -8f_s f_r (f_a f_b + 2f_s), 2f_s (12f_b f_t f_r + 2f_s f_a f_b^2 + f_b f_s^2 - 4f_b f_a^2 f_t - 8f_a f_t f_s), 16f_b f_t f_r^2 \\
& + 4f_r f_a f_s f_b^2 + 4f_s^2 f_b f_r - 8f_r f_b f_a^2 f_t - 8f_r f_a f_t f_s - 2f_a f_s^3, 0, -8f_b f_r f_s (f_a f_b + 2f_s), -8f_b \\
& f_r^2 (f_a f_b + 2f_s), -2f_s (-8f_s^2 f_t + f_s^2 f_b^2 - 4f_b f_a f_t f_s - 4f_b^2 f_r f_t), 8f_r^2 f_t f_b^2 - 2f_s^2 f_r f_b^2 \\
& + 24f_s f_b f_a f_t f_r + 32f_s^2 f_r f_t - 2f_b f_a f_s^3, -2f_r (f_b f_a f_s^2 - 8f_s f_r f_t - 8f_b f_a f_t f_r), 4f_r (4f_t f_r \\
& + f_b f_a f_s + f_s^2), -8f_r^2 (f_a f_b + 2f_s), 8f_b f_t f_r^2 - 2f_s^2 f_b f_r + 16f_r f_a f_t f_s + 4f_a^2 f_s^2 f_b + 4f_a f_s^3, \\
& 2f_a f_r (12f_t f_r + 2f_b f_a f_s + f_s^2), 0, -8f_r f_s f_a (f_a f_b + 2f_s), -8f_a f_r^2 (f_a f_b + 2f_s), -2f_s (2f_s^3 \\
& + 3f_b f_a f_s^2 + 8f_s f_r f_t - 4f_b f_a f_t f_r), 8f_r^2 f_a f_t f_b - 32f_r^2 f_t f_s - 10f_r f_a f_s^2 f_b + 8f_r f_a^2 f_s f_t - 8f_r f_s^3 \\
& - 2f_a^2 f_s^3, -2f_r (8f_r^2 f_t + 2f_b f_a f_r f_s + 2f_s^2 f_r - 4f_a^2 f_t f_r + f_s^2 f_a^2), 0, 0, 0, 8f_r f_s^2 (f_a f_b + 2f_s), \\
& 16f_s f_r^2 (f_a f_b + 2f_s), 8f_r^3 (f_a f_b + 2f_s), 2f_b f_s^2 (f_s^2 - 4f_t f_r), 2f_s (f_a f_s^3 + 2f_s^2 f_b f_r \\
& - 4f_r f_a f_t f_s - 8f_b f_t f_r^2), 2f_r (2f_a f_s^3 + f_s^2 f_b f_r - 8f_r f_a f_t f_s - 4f_b f_t f_r^2), 2f_a f_r^2 (f_s^2 - 4f_t f_r)], \\
& [0, -8f_t^2 (f_a f_b + 2f_s), -4f_t f_s (f_a f_b + 2f_s), -4f_t^2 f_b (f_a f_b + 2f_s), -4f_t f_s f_b (f_a f_b + 2f_s), \\
& -4f_t (f_s^2 - 4f_t f_r), 2f_s^3 + 2f_b f_a f_s^2 - 24f_s f_r f_t - 16f_b f_a f_t f_r, -2f_t (4f_b f_s^2 + 4f_a f_t f_s + f_s f_a f_b^2 \\
& - 8f_b f_t f_r + 2f_b f_a^2 f_t), 2f_b f_s^3 - 10f_s^2 f_a f_t + 2f_b^2 f_a f_s^2 - 4f_b f_a^2 f_s f_t - 4f_r f_a f_t f_b^2 + 8f_a f_t^2 f_r \\
& - 4f_s f_r (f_a f_b + 2f_s), -f_b f_s^3 - 8f_s^2 f_a f_t - 4f_b f_a^2 f_s f_t - 4f_s f_b f_t f_r - 4f_r f_a f_t f_b^2, -f_a f_s^3 - 8f_s^2 f_b f_r \\
& - 4f_r f_a f_s f_b^2 - 4f_r f_a f_t f_s - 4f_r f_b f_a^2 f_r, -f_t (f_s^2 f_b^2 - 16f_s^2 f_t - 8f_b f_a f_t f_s - 4f_b^2 f_r f_t), -f_b^2 f_s^3 \\
& + 16f_t f_s^3 + 7f_a f_t f_b f_s^2 + 16f_r f_t^2 f_s + 4f_r f_t f_s f_b^2 + 12f_r f_t^2 f_a f_b, -f_s (f_b f_a f_s^2 - 16f_s f_r f_t \\
& - 12f_b f_a f_t f_r), 2f_s (4f_t f_r + f_b f_a f_s + f_s^2), -4f_r (f_s^2 - 4f_t f_r), f_b f_s^3 + 2f_b^2 f_a f_s^2 + 2f_s^2 f_a f_t \\
& + 2f_b f_a^2 f_s f_t + 12f_s f_b f_t f_r + 8f_a f_t^2 f_r f_a f_s^3 + 2f_s^2 f_b f_r + 2f_a^2 f_s^2 f_b + 2f_r f_a f_s f_b^2 + 12f_r f_a f_t f_s \\
& + 8f_b f_t f_r^2, -8f_r^2 (f_a f_b + 2f_s), 2f_a f_s^3 - 10f_s^2 f_b f_r + 2f_a^2 f_s^2 f_b - 4f_r f_a f_s f_b^2 - 4f_r f_b f_a^2 f_t \\
& + 8f_b f_t f_r^2, -2f_r (4f_a f_s^2 + f_a^2 f_s f_b + 4f_b f_r f_s + 2f_r f_a f_b^2 - 8f_a f_t f_r), -f_b^2 f_s^3 - 4f_t f_s^3 - 5f_a f_t f_b
\end{aligned}$$

$$\begin{aligned}
& f_s^2 + 4f_r f_t f_s f_b^2 - 16f_r f_t^2 f_s + 4f_r f_t^2 f_a f_b - 4f_s^4 - 6f_b f_a f_s^3 - 20f_s^2 f_r f_t - f_s^2 f_a^2 f_t - f_s^2 f_r f_b^2 \\
& + 4f_s f_b f_a f_t f_r + 4f_r^2 f_t f_b^2 - 16f_r^2 f_t^2 + 4f_a^2 f_t^2 f_r - 4f_r f_s^3 - f_a^2 f_s^3 - 5f_r f_a f_s^2 f_b - 16f_r^2 f_t f_s \\
& + 4f_r f_a^2 f_s f_t + 4f_r^2 f_a f_t f_b, 0, -4f_r f_s f_a (f_a f_b + 2f_s), -4f_a f_r^2 (f_a f_b + 2f_s), -f_s (f_b f_a f_s^2 \\
& - 16f_s f_r f_t - 12f_b f_a f_t f_r), 16f_r f_s^3 - f_a^2 f_s^3 + 7f_r f_a f_s^2 f_b + 16f_r^2 f_t f_s + 4f_r f_a^2 f_s f_t + 12 \\
& f_r^2 f_a f_t f_b - f_r (-16f_s^2 f_r + f_s^2 f_a^2 - 8f_b f_a f_r f_s - 4f_a^2 f_t f_r), 2f_s f_b f_t (f_s^2 - 4f_t f_r), 2f_b f_s^4 + 2 \\
& f_s^3 f_a f_t - 6f_s^2 f_b f_t f_r - 8f_s f_a f_t^2 f_r - 8f_b f_r^2 f_t^2, 2f_s^4 f_a + 2f_r f_b f_s^3 - 6f_r f_a f_t f_s^2 - 8f_r^2 f_s f_t f_b - 8 \\
& f_r^2 f_a f_t^2, 2f_s f_a f_r (f_s^2 - 4f_t f_r) ], \\
& [0, 0, -8f_t^2 (f_a f_b + 2f_s), 0, -4f_t^2 f_b (f_a f_b + 2f_s), 0, -4f_t (f_s^2 - 4f_t f_r), 0, 2f_t (f_b f_s^2 + f_s f_a \\
& f_b^2 - 4f_a f_t f_s - 2f_b f_a^2 f_t + 4f_b f_t f_r), -8f_r f_t (f_a f_b + 2f_s), -2f_b f_t (5f_s^2 + 2f_b f_a f_s - 4f_t f_r), \\
& -2f_t (4f_r f_a f_b^2 + 8f_b f_r f_s - 4f_a f_t f_r + f_a f_s^2), 0, -f_t (f_s^2 f_b^2 - 16f_s^2 f_t - 8f_b f_a f_t f_s - 4f_b^2 f_r f_t), \\
& -f_t (f_b f_a f_s^2 - 16f_s f_r f_t - 12f_b f_a f_t f_r), 0, 2f_s (4f_t f_r + f_b f_a f_s + f_s^2), 0, 2f_a f_t (4f_t f_r + f_b f_a f_s \\
& + f_s^2), -4f_s f_r (f_a f_b + 2f_s), f_b f_s (12f_t f_r + 2f_b f_a f_s + f_s^2), -f_a f_s^3 + 2f_s^2 f_b f_r - 4f_r f_a f_t f_s \\
& + 2f_r f_a f_s f_b^2 - 4f_r f_b f_a^2 f_t + 8f_b f_t f_r^2, 0, -f_t (4f_s^3 + 5f_b f_a f_s^2 + 16f_s f_r f_t - 4f_b f_a f_t f_r), -f_t (4 \\
& f_s^2 f_r + f_s^2 f_a^2 + 4f_b f_a f_r f_s - 4f_a^2 f_t f_r + 16f_r^2 f_t), 0, -4f_b f_r f_s (f_a f_b + 2f_s), -4f_b f_r^2 (f_a f_b \\
& + 2f_s), -f_s f_b^2 (f_s^2 - 4f_t f_r), -f_b f_a f_s^3 + 16f_s^2 f_r f_t - f_s^2 f_r f_b^2 + 12f_s f_b f_a f_t f_r + 4f_r^2 f_t f_b^2, \\
& -f_r (f_b f_a f_s^2 - 16f_s f_r f_t - 12f_b f_a f_t f_r), 0, 2f_s f_b f_t (f_s^2 - 4f_t f_r), 2f_t (f_a f_s^3 + f_s^2 f_b f_r - 4f_r f_a f_t f_s \\
& - 4f_b f_t f_r^2), 2f_a f_t f_r (f_s^2 - 4f_t f_r) ], \\
& [0, 0, 0, 0, 0, -8f_t^2 (f_a f_b + 2f_s), -8f_t f_s (f_a f_b + 2f_s), -8f_t^2 f_b (f_a f_b + 2f_s), -8f_t f_s f_b (f_a f_b \\
& + 2f_s), -8f_r f_t (f_a f_b + 2f_s), -8f_t^2 f_a (f_a f_b + 2f_s), -8f_s f_a f_t (f_a f_b + 2f_s), 8f_t^3 (f_a f_b \\
& + 2f_s), 16f_t^2 f_s (f_a f_b + 2f_s), 8f_t f_s^2 (f_a f_b + 2f_s), 4f_t (4f_t f_r + f_b f_a f_s + f_s^2), -8f_b f_a f_t f_r \\
& + 4f_b f_a f_s^2 + 4f_s^3, 2f_b f_t (12f_t f_r + 2f_b f_a f_s + f_s^2), 16f_s f_b f_t f_r + 8f_a f_t^2 f_r + 4f_b^2 f_a f_s^2 + 4f_b f_s^3 \\
& - 2f_s^2 f_a f_r - 4f_r (3f_s^2 + f_b f_a f_s - 4f_t f_r), -8f_r f_a f_t f_b^2 - 8f_s f_b f_t f_r + 16f_a f_t^2 f_r - 2f_b f_s^3 + 4f_b \\
& f_a^2 f_s f_t + 4f_s^2 f_a f_r, 2f_s (f_a f_s^2 + 2f_a^2 f_s f_b - 8f_b f_r f_s - 4f_r f_a f_b^2 + 12f_a f_t f_r), -2f_t (2f_s^2 f_t + f_s^2 f_b^2 \\
& + 2f_b f_a f_t f_s - 4f_b^2 f_r f_t + 8f_r f_t^2), 8f_r f_t f_s f_b^2 + 8f_r f_t^2 f_a f_b - 32f_r f_t^2 f_s - 2f_b^2 f_s^3 - 10f_a f_t f_b f_s^2 \\
& - 8f_t f_s^3, -2f_s (2f_s^3 + 3f_b f_a f_s^2 + 8f_s f_r f_t - 4f_b f_a f_t f_r), -8f_r^2 (f_a f_b + 2f_s), -2f_r (f_b f_s^2 \\
& + 8f_a f_t f_s + 4f_b f_a^2 f_t - 4f_b f_t f_r), -2f_a f_r (9f_s^2 + 4f_b f_a f_s - 4f_t f_r), -2f_t (f_b f_a f_s^2 - 8f_s f_r f_t \\
& - 8f_b f_a f_t f_r), 24f_s f_b f_a f_t f_r + 32f_s^2 f_r f_t + 8f_a^2 f_t^2 f_r - 2f_b f_a f_s^3 - 2f_s^2 f_a^2 f_r - 2f_s (f_s^2 f_a^2 - 8 \\
& f_s^2 f_r - 4f_b f_a f_r f_s - 4f_a^2 f_t f_r), 2f_b f_t^2 (f_s^2 - 4f_t f_r), 2f_t (2f_b f_s^3 + f_s^2 f_a f_t - 8f_s f_b f_t f_r - 4f_a \\
& f_t^2 f_r), 2f_s (f_b f_s^3 + 2f_s^2 f_a f_t - 4f_s f_b f_t f_r - 8f_a f_t^2 f_r), 2f_a f_s^2 (f_s^2 - 4f_t f_r) ],
\end{aligned}$$

$$\begin{aligned}
& [0, 0, 0, 0, 0, 0, -8f_t^2(f_af_b + 2f_s), 0, -4f_t^2f_b(f_af_b + 2f_s), -4f_tf_s(f_af_b + 2f_s), -4 \\
& f_t^2f_b(f_af_b + 2f_s), -4f_t(2f_bf_s^2 + f_sf_af_b^2 + 2f_af_tf_s + f_bf_a^2f_t), 0, 8f_t^3(f_af_b + 2f_s), 8 \\
& f_t^2f_s(f_af_b + 2f_s), 0, 4f_t(4f_tf_r + f_bf_af_s + f_s^2), 0, 2f_bf_t(4f_tf_r + f_bf_af_s + f_s^2), 2f_s^3 + 2f_bf_af_s^2 \\
& - 8f_sf_rf_t - 8f_bf_af_tf_r, 2f_bf_t(f_bf_af_s + 8f_tf_r), 2f_bf_s^3 + 2f_b^2f_af_s^2 + 2f_bf_a^2f_sf_t - 4f_rf_af_tf_b^2 \\
& + 16f_af_t^2f_r, 0, -f_t(f_s^2f_b^2 + 4f_s^2f_t + 4f_bf_af_tf_s + 16f_rf_t^2 - 4f_b^2f_rf_t), -f_t(4f_s^3 + 5f_bf_af_s^2 \\
& + 16f_sf_rf_t - 4f_bf_af_tf_r), -4f_sf_r(f_af_b + 2f_s), -f_b(f_s^3 + 4f_sf_rf_t + 4f_bf_af_tf_r), -f_af_s^3 - 8 \\
& f_s^2f_bf_r - 4f_rf_af_sf_b^2 - 4f_rf_af_tf_s - 4f_rf_bf_af_r^2 - f_b^2f_t(f_s^2 - 4f_tf_r), -f_b^2f_s^3 - 2f_af_tf_bf_s^2 \\
& + 4f_rf_tf_sf_b^2 + 16f_rf_t^2f_s + 16f_rf_t^2f_af_b, -f_bf_af_s^3 + 16f_s^2f_rf_t - f_s^2f_a^2f_t + 12f_sf_bf_af_tf_r + 4f_a^2 \\
& f_t^2f_rf_r, 0, 2f_bf_t^2(f_s^2 - 4f_tf_r), 2f_t(f_bf_s^3 + f_s^2f_af_t - 4f_sf_bf_tf_r - 4f_af_t^2f_r), 2f_af_tf_s(f_s^2 - 4f_tf_r) \\
& ], \\
& [0, 0, 0, 0, 0, 0, 0, 0, 0, -8f_t^2(f_af_b + 2f_s), 0, -8f_t^2f_b(f_af_b + 2f_s), 0, 0, 8f_t^3(f_af_b \\
& + 2f_s), 0, 0, 0, 0, 4f_t(4f_tf_r + f_bf_af_s + f_s^2), 0, 4f_bf_t(4f_tf_r + f_bf_af_s + f_s^2), 0, 0, -4f_t^2(4f_tf_r \\
& + f_bf_af_s + f_s^2), -8f_rf_t(f_af_b + 2f_s), -2f_bf_t(f_s^2 - 4f_tf_r), -2f_t(4f_rf_af_b^2 + 8f_bf_rf_s \\
& - 4f_af_tf_r + f_af_s^2), 0, -2f_b^2f_t(f_s^2 - 4f_tf_r), -2f_t(f_bf_af_s^2 - 8f_sf_rf_t - 8f_bf_af_tf_r), 0, 0, 2f_b \\
& f_t^2(f_s^2 - 4f_tf_r), 2f_af_t^2(f_s^2 - 4f_tf_r)], \\
& [-4f_a^2f_t - 4f_s^2, 2f_s(4f_r + f_a^2), -4f_r(4f_r + f_a^2), -2f_a(3f_s^2 + 2f_a^2f_t - 4f_tf_r), 0, 0, 0, \\
& 2f_af_s(4f_r + f_a^2), 0, 0, -4f_af_r(4f_r + f_a^2), 0, 12f_a^2f_tf_r + 4f_s^2f_r - 2f_s^2f_a^2, 0, 0, 0, 0, 0, 0, \\
& 0, 0, -2f_sf_r(4f_r + f_a^2), 0, 0, 0, 0, 0, 4f_r^2(4f_r + f_a^2), 0, 0, 2f_af_r(f_s^2 - 4f_tf_r), 0, 0, 0], \\
& [0, -4f_a^2f_t - 4f_s^2, 0, -2f_b(f_a^2f_t + f_s^2), -2f_a(f_a^2f_t + f_s^2), 2f_s(4f_r + f_a^2), -4f_r(4f_r + f_a^2), \\
& -4f_af_s^2 + 4f_bf_rf_s + f_a^2f_sf_b + 8f_af_tf_r - 2f_af_rf_af_s(4f_r + f_a^2), 0, -2f_bf_r(4f_r + f_a^2), \\
& -2f_af_r(4f_r + f_a^2), 4f_bf_af_tf_r - f_bf_af_s^2 + 2f_s^3 + 2f_sf_a^2f_r - f_s^2f_a^2 + 4f_s^2f_r + 8f_a^2f_tf_r, 0, 0, 0, \\
& f_af_s(4f_r + f_a^2), 0, 0, -2f_af_r(4f_r + f_a^2), 0, -4f_s^2f_r + 4f_a^2f_tf_r - 2f_s^2f_a^2, -2f_sf_r(4f_r + f_a^2), \\
& 0, 0, 0, 0, 2f_sf_r(4f_r + f_a^2), 4f_r^2(4f_r + f_a^2), 0, f_af_s(f_s^2 - 4f_tf_r), 2f_af_r(f_s^2 - 4f_tf_r), 0, 0], \\
& [0, 0, -4f_a^2f_t - 4f_s^2, 0, -2f_b(f_a^2f_t + f_s^2), 0, 2f_s(4f_r + f_a^2), 0, f_sf_b(4f_r + f_a^2), -4f_r(4f_r + \\
& f_a^2), -2f_a(2f_s^2 - 4f_tf_r + f_a^2f_t), -2f_bf_r(4f_r + f_a^2), 0, 4f_bf_af_tf_r - f_bf_af_s^2 + 2f_s^3 + 2f_sf_a^2f_r \\
& 0, 0, 0, 0, 0, 0, f_af_s(4f_r + f_a^2), 0, 0, -(4f_r + f_a^2)f_s^2, 0, 0, -2f_af_r(4f_r + f_a^2), 0, -f_a^2(f_s^2 \\
& - 4f_tf_r), 2f_sf_r(4f_r + f_a^2), 0, 0, f_af_s(f_s^2 - 4f_tf_r), 0, 0], \\
& [2f_a(f_a^2f_t + f_s^2), -f_af_s(4f_r + f_a^2), 2f_af_r(4f_r + f_a^2), f_a^2(3f_s^2 + 2f_a^2f_t - 4f_tf_r), 0, 0, 0, -f_s \\
& f_a^2(4f_r + f_a^2), 0, 0, 2f_a^2f_r(4f_r + f_a^2), 0, f_a(f_s^2f_a^2 - 2f_s^2f_r - 6f_a^2f_tf_r), 0, 0, 0, 0, 0, 0, 0, 0,
\end{aligned}$$

$$\begin{aligned}
& 0, f_r f_s f_a (4f_r + f_a^2), 0, 0, 0, 0, 0, -2f_a f_r^2 (4f_r + f_a^2), 0, 0, -f_a^2 f_r (f_s^2 - 4f_t f_r), 0, 0, 0], \\
& [2f_b (f_a^2 f_t + f_s^2), 2f_a f_s^2 - 4f_b f_r f_s - f_a^2 f_s f_b + 2f_a^3 f_r, 2f_b f_r (4f_r + f_a^2), -2f_s^3 + 3f_b f_a f_s^2 \\
& - 2f_s f_a^2 f_t - 4f_b f_a f_t f_r + 2f_b f_t f_a^3, -4f_r (f_a^2 f_t + f_s^2), -f_a f_s (4f_r + f_a^2), 2f_a f_r (4f_r + f_a^2), 4f_s^2 \\
& f_a^2 + 8f_s^2 f_r - 4f_b f_a f_r f_s - f_s f_b f_a^3 + 2f_t f_a^4, 2f_s f_r (4f_r + f_a^2), 0, -2f_r (4f_r f_s + f_s f_a^2 - 4f_b f_r f_a \\
& - f_b f_a^3), -4f_r^2 (4f_r + f_a^2), -f_a (3f_s^3 - f_b f_a f_s^2 + 2f_s f_a^2 f_t - 4f_s f_r f_t + 4f_b f_a f_t f_r), -2f_a f_r (2 \\
& f_s^2 - 4f_t f_r + f_a^2 f_t), 0, 0, 0, -f_s (f_a^4 + 8f_r^2 + 6f_a^2 f_r), 0, 0, 2f_r (f_a^4 + 8f_r^2 + 6f_a^2 f_r), 0, 2f_a (3 \\
& f_s^2 f_r + f_s^2 f_a^2 - 2f_a^2 f_t f_r - 4f_r^2 f_t), f_r f_s f_a (4f_r + f_a^2), 0, 0, 0, 0, -2f_r f_s f_a (4f_r + f_a^2), -2f_a \\
& f_r^2 (4f_r + f_a^2), 0, -f_s f_a^2 (f_s^2 - 4f_t f_r), -f_a^2 f_r (f_s^2 - 4f_t f_r), 0, 0], \\
& [0, 2f_b (f_a^2 f_t + f_s^2), 2f_a (f_a^2 f_t + f_s^2), -4f_t (f_a^2 f_t + f_s^2), -4f_s (f_a^2 f_t + f_s^2), -f_s f_b (4f_r + f_a^2), \\
& 8f_b f_r^2 + 2f_r f_b f_a^2 - 4f_r f_s f_a - f_a^3 f_s, 2f_s^3 + 3f_b f_a f_s^2 + 4f_s f_a^2 f_t + 8f_s f_r f_t - 4f_b f_a f_t f_r + 2f_b f_t \\
& f_a^3, 2(4f_r + f_a^2)f_s^2, 2f_a f_r (4f_r + f_a^2), 4f_s^2 f_r + 3f_s^2 f_a^2 - 4f_a^2 f_t f_r - 16f_r^2 f_t + 2f_t f_a^4, \\
& -4f_s f_r (4f_r + f_a^2), -2f_a f_t (2f_s^2 - 4f_t f_r + f_a^2 f_t), -2f_s f_a (2f_s^2 - 4f_t f_r + f_a^2 f_t), 0, 0, 0, \\
& -f_s (4f_r f_s + f_s f_a^2 + 4f_b f_r f_a + f_b f_a^3), 0, 0, -f_a (4f_r f_s f_a + f_a^3 f_s - 8f_b f_r^2 - 2f_r f_b f_a^2), 0, f_a (f_s^3 \\
& + f_b f_a f_s^2 + f_s f_a^2 f_t - 4f_b f_a f_t f_r), f_a f_s^2 (4f_r + f_a^2), 0, 0, 2f_r (f_a^4 + 8f_r^2 + 6f_a^2 f_r), 0, f_a (f_s^2 f_a^2 \\
& + 2f_s^2 f_r - 6f_a^2 f_t f_r - 16f_r^2 f_t), -2f_r f_s f_a (4f_r + f_a^2), 0, -f_a^2 f_t (f_s^2 - 4f_t f_r), -f_s f_a^2 (f_s^2 \\
& - 4f_t f_r), 0, 0], \\
& [0, 0, 2f_b (f_a^2 f_t + f_s^2), 0, -4f_t (f_a^2 f_t + f_s^2), 0, -f_s f_b (4f_r + f_a^2), 0, 2f_t f_s (4f_r + f_a^2), \\
& 2f_b f_r (4f_r + f_a^2), 2f_s^3 + 3f_b f_a f_s^2 + 2f_s f_a^2 f_t - 4f_b f_a f_t f_r + 2f_b f_t f_a^3, -4f_r f_t (4f_r + f_a^2), 0, \\
& -2f_a f_t (2f_s^2 - 4f_t f_r + f_a^2 f_t), 0, 0, 0, 0, 0, 0, -f_s (4f_r f_s + f_s f_a^2 + 4f_b f_r f_a + f_b f_a^3), 0, 0, \\
& f_s f_a f_t (4f_r + f_a^2), 0, 0, 2f_r (4f_r f_s + f_s f_a^2 + 4f_b f_r f_a + f_b f_a^3), 0, f_a (f_s^3 + f_b f_a f_s^2 - 4f_s f_r f_t \\
& - 4f_b f_a f_t f_r), -2f_a f_r f_t (4f_r + f_a^2), 0, 0, -f_a^2 f_t (f_s^2 - 4f_t f_r), 0, 0], \\
& [0, 0, 0, 0, 0, -4f_a^2 f_t - 4f_s^2, 0, -4f_b (f_a^2 f_t + f_s^2), -4f_a (f_a^2 f_t + f_s^2), 0, 0, 0, 4f_t (f_a^2 f_t + f_s^2), \\
& 4f_s (f_a^2 f_t + f_s^2), 4f_r (f_a^2 f_t + f_s^2), 2f_s (4f_r + f_a^2), -4f_r (4f_r + f_a^2), 8f_b f_r f_s + 8f_a f_t f_r + 2 \\
& f_a^2 f_s f_b - 2f_a f_s^2, 2f_a f_s (4f_r + f_a^2), 0, -4f_b f_r (4f_r + f_a^2), -4f_a f_r (4f_r + f_a^2), 8f_b f_a f_t f_r \\
& - 8f_s f_r f_t - 2f_b f_a f_s^2 - 2f_s f_a^2 f_r - 8f_s^2 f_r + 8f_a^2 f_t f_r - 4f_s^2 f_a^2, -2f_s f_r (4f_r + f_a^2), 0, 0, 0, \\
& 4f_r f_t (4f_r + f_a^2), 4f_s f_r (4f_r + f_a^2), 4f_r^2 (4f_r + f_a^2), 2f_a f_t (f_s^2 - 4f_t f_r), 2f_a f_s (f_s^2 - 4f_t f_r), \\
& 2f_a f_r (f_s^2 - 4f_t f_r), 0], \\
& [0, 0, 0, 0, 0, 0, -4f_a^2 f_t - 4f_s^2, 0, -2f_b (f_a^2 f_t + f_s^2), 0, -2f_b (f_a^2 f_t + f_s^2), -2f_a (f_a^2 f_t + f_s^2), \\
& 0, 4f_t (f_a^2 f_t + f_s^2), 2f_s (f_a^2 f_t + f_s^2), 0, 2f_s (4f_r + f_a^2), 0, f_s f_b (4f_r + f_a^2), -4f_r (4f_r + f_a^2),
\end{aligned}$$

$$\begin{aligned}
& -2f_a f_s^2 + 4f_b f_r f_s + f_a^2 f_s f_b + 8f_a f_t f_r + 4f_r f_s f_a + f_a^3 f_s - 8f_b f_r^2 - 2f_r f_b f_a^2, 0, 4f_b f_a f_t f_r \\
& - 8f_s f_r f_t - f_b f_a f_s^2 - 2f_s f_a^2 f_r - (4f_r + f_a^2) f_s^2, 0, -2f_b f_r (4f_r + f_a^2), -2f_a f_r (4f_r + f_a^2), \\
& -f_b f_a (f_s^2 - 4f_t f_r), 16f_r^2 f_t + 8f_a^2 f_t f_r - f_s^2 f_a^2, 2f_s f_r (4f_r + f_a^2), 0, 2f_a f_t (f_s^2 - 4f_t f_r), f_a f_s (f_s^2 \\
& - 4f_t f_r), 0],
\end{aligned}$$

$$\begin{aligned}
& [0, 2f_a (f_a^2 f_t + f_s^2), 0, 2f_s^3 + 2f_b f_a f_s^2 + 2f_s f_a^2 f_t + 2f_b f_t f_a^3, 2f_s^2 f_a^2 + 4f_s^2 f_r + 4f_a^2 f_t f_r + 2f_t \\
& f_a^4, -f_a f_s (4f_r + f_a^2), 2f_a f_r (4f_r + f_a^2), -8f_s^2 f_r - 4f_b f_a f_r f_s - f_s f_b f_a^3 - 8f_a^2 f_t f_r - f_s (f_a^4 + 8 \\
& f_r^2 + 6f_a^2 f_r), 0, 2f_r (4f_r f_s + f_s f_a^2 + 4f_b f_r f_a + f_b f_a^3), 2f_r (f_a^4 + 8f_r^2 + 6f_a^2 f_r), f_a f_s^3 + f_a^2 f_s^2 f_b \\
& - 2f_s^2 f_b f_r - 4f_r f_a f_t f_s - 6f_r f_b f_a^2 f_r f_a (f_s^2 f_a^2 - 8f_r^2 f_t - 6f_a^2 f_t f_r), 0, 0, 0, 2f_s f_r (4f_r + f_a^2), \\
& 0, 0, -4f_r^2 (4f_r + f_a^2), 0, -f_r (2f_a f_s^2 - 4f_b f_r f_s - f_a^2 f_s f_b - 8f_a f_t f_r), f_r f_s f_a (4f_r + f_a^2), 0, 0, \\
& 0, 0, -2f_b f_r^2 (4f_r + f_a^2), -2f_a f_r^2 (4f_r + f_a^2), 0, -f_b f_a f_r (f_s^2 - 4f_t f_r), -f_a f_r (f_s^2 - 4f_t f_r), 0, \\
& 0],
\end{aligned}$$

$$\begin{aligned}
& [0, 2f_b (f_a^2 f_t + f_s^2), 0, 4f_s^2 f_t + 2f_s^2 f_b^2 + 4f_a^2 f_t^2 + 2f_b^2 f_a^2 f_r + 2f_s^3 + 2f_b f_a f_s^2 + 2f_s f_a^2 f_t \\
& + 2f_b f_t f_a^3, 2f_a f_s^2 - 4f_b f_r f_s - f_a^2 f_s f_b + 2f_a^3 f_r + 2f_b f_r (4f_r + f_a^2), -2f_s^3 + 3f_b f_a f_s^2 - 4f_s f_r f_b^2 \\
& - 4f_s f_a^2 f_t - f_s f_b^2 f_a^2 - 8f_s f_r f_t - 4f_b f_a f_t f_r + 2f_b f_t f_a^3, f_s^2 f_a^2 - 4f_s^2 f_r - 4f_b f_a f_r f_s - f_s f_b f_a^3 \\
& + 2f_t f_a^4, 0, 2f_r (f_b^2 f_a^2 + 4f_r f_b^2 + 2f_a^2 f_t + 8f_t f_r), 2f_r (4f_r f_s + f_s f_a^2 + 4f_b f_r f_a + f_b f_a^3), -2f_b \\
& f_s^3 + 2f_s^2 f_a f_t + f_b^2 f_a f_s^2 - 2f_b f_a^2 f_s f_t - 8f_a f_t^2 f_r - 4f_r f_a f_t f_b^2, -f_a f_s^3 + f_a^2 f_s^2 f_b - 2f_s^2 f_b f_r - 2 \\
& f_a^3 f_s f_t - 4f_r f_a f_t f_s - 6f_r f_b f_a^2 f_r - 2f_a f_r (f_a^2 f_t + f_s^2), -f_a f_s (4f_r + f_a^2), 2f_a f_r (4f_r + f_a^2), 2f_s^2 \\
& f_a^2 + 4f_s^2 f_r - 4f_b f_a f_r f_s - f_s f_b f_a^3 - 4f_a^2 f_t f_r - f_s f_a^2 (4f_r + f_a^2), 0, -2f_r (4f_r f_s + f_s f_a^2 \\
& - 4f_b f_r f_a - f_b f_a^3), 2f_a^2 f_r (4f_r + f_a^2), -f_a f_s^3 + 4f_s^2 f_b f_r + 2f_a^2 f_s^2 f_b + 4f_r f_a f_t f_s - 4f_r f_b f_a^2 f_r \\
& 4f_s^2 f_a f_r + 2f_s^2 f_a^3 + 4f_s f_b f_r^2 + f_s f_b f_a^2 f_r - 4f_a^3 f_t f_r + f_r f_s f_a (4f_r + f_a^2), 0, 0, 0, -2f_b f_r f_s (4f_r \\
& + f_a^2), -2f_r (4f_r f_s f_a + f_a^3 f_s + 4f_b f_r^2 + f_r f_b f_a^2), -2f_a f_r^2 (4f_r + f_a^2), -f_s f_b f_a (f_s^2 - 4f_t f_r), \\
& -f_a (f_a f_s^3 + f_s^2 f_b f_r - 4f_r f_a f_t f_s - 4f_b f_t f_r^2), -f_a^2 f_r (f_s^2 - 4f_t f_r), 0],
\end{aligned}$$

$$\begin{aligned}
& [0, 0, 0, 0, 0, 2f_b (f_a^2 f_t + f_s^2), 2f_a (f_a^2 f_t + f_s^2), 2f_b^2 (f_a^2 f_t + f_s^2), -2f_s^3 + 2f_b f_a f_s^2 - 2f_s f_a^2 f_t \\
& + 2f_b f_t f_a^3, 0, 2f_s^3 + 2f_b f_a f_s^2 + 2f_s f_a^2 f_t + 2f_b f_t f_a^3, 2f_s^2 f_a^2 + 4f_s^2 f_r + 4f_a^2 f_t f_r + 2f_t f_a^4, \\
& -2f_b f_t (f_a^2 f_t + f_s^2), -2f_b f_s^3 - 2f_s^2 f_a f_t - 2f_b f_a^2 f_s f_t - 2f_a^3 f_t^2, -2f_a f_s (f_a^2 f_t + f_s^2), -f_s f_b (4f_r \\
& + f_a^2), 8f_b f_r^2 + 2f_r f_b f_a^2 - 4f_r f_s f_a - f_a^3 f_s f_b (f_a f_s^2 - 4f_b f_r f_s - f_a^2 f_s f_b - 4f_a f_t f_r), f_s (4f_r f_s \\
& + f_s f_a^2 - 4f_b f_r f_a - f_b f_a^3), 2f_a f_r (4f_r + f_a^2), -4f_s^2 f_r - 4f_b f_a f_r f_s - f_s f_b f_a^3 + 2f_b^2 f_a^2 f_r + 8f_r^2 \\
& f_b^2 - 4f_a^2 f_t f_r - 8f_s f_a^2 f_r - f_s f_a^4 - 16f_s f_r^2 + 2f_r f_b f_a^3 + 8f_b f_a f_r^2, f_b (f_b f_a f_s^2 + 4f_s f_r f_t + f_s f_a^2 f_t \\
& - 4f_b f_a f_t f_r), -f_a f_s^3 + 4f_s^2 f_b f_r + 2f_a^2 f_s^2 f_b + 8f_r f_a f_t f_s + f_a^3 f_s f_t - 4f_r f_b f_a^2 f_r f_a f_s^2 (4f_r +
\end{aligned}$$

$$\begin{aligned}
& f_a^2), 0, 2f_r(4f_rf_s + f_sf_a^2 + 4f_bf_rf_a + f_bf_a^3), 2f_r(f_a^4 + 8f_r^2 + 6f_a^2f_r), f_af_s^3 + f_a^2f_s^2f_b \\
& - 4f_rf_af_tf_s - 6f_rf_bf_a^2f_t - 8f_bf_tf_r^2, 2f_s^2f_af_r + f_s^2f_a^3 - 8f_sf_bf_r^2 - 2f_sf_bf_a^2f_r - 16f_af_tf_r^2 - 6 \\
& f_a^3f_tf_r - 2f_rf_sf_a(4f_r + f_a^2), -f_af_tf_b(f_s^2 - 4f_tf_r), -f_a(f_bf_s^3 + f_s^2f_af_t - 4f_sf_bf_tf_r - 4f_a \\
& f_t^2f_r), -f_sf_a^2(f_s^2 - 4f_tf_r), 0], \\
& [0, 0, 0, 0, 0, 0, 2f_b(f_a^2f_t + f_s^2), 0, -4f_t(f_a^2f_t + f_s^2), 0, 4f_s^2f_t + 2f_s^2f_b^2 + 4f_a^2f_t^2 + 2f_b^2f_a^2f_p \\
& 2f_s^3 + 2f_bf_af_s^2 + 2f_sf_a^2f_t + 2f_bf_tf_a^3, 0, -2f_bf_t(f_a^2f_t + f_s^2), -2f_af_t(f_a^2f_t + f_s^2), 0, -f_sf_b(4f_r \\
& + f_a^2), 0, 2f_tf_s(4f_r + f_a^2), 2f_bf_r(4f_r + f_a^2), f_bf_af_s^2 - f_sf_b^2f_a^2 - 4f_sf_rf_b^2 - 2f_sf_a^2f_t - 8f_sf_rf_t \\
& - 4f_bf_af_tf_r - 4f_s^2f_r - f_s^2f_a^2 - 4f_bf_af_rf_s - f_sf_bf_a^3 - 4f_a^2f_tf_r - 16f_r^2f_p, 0, -f_t(2f_af_s^2 \\
& - 4f_bf_rf_s - f_a^2f_sf_b - 8f_af_tf_r), f_sf_af_t(4f_r + f_a^2), 0, 2f_r(f_b^2f_a^2 + 4f_rf_b^2 + 2f_a^2f_t + 8f_tf_r), \\
& 2f_r(4f_rf_s + f_sf_a^2 + 4f_bf_rf_a + f_bf_a^3), f_a(f_s^2f_b^2 + 2f_s^2f_t - 8f_rf_t^2 - 4f_b^2f_rf_t), f_af_s^3 + f_a^2f_s^2f_b \\
& - 4f_rf_af_tf_s - 6f_rf_bf_a^2f_t - 8f_bf_tf_r^2, -2f_af_rf_t(4f_r + f_a^2), 0, -f_af_tf_b(f_s^2 - 4f_tf_r), -f_a^2f_t(f_s^2 \\
& - 4f_tf_r), 0], \\
& [0, 0, 0, 0, 0, 0, 0, 0, 0, -4f_a^2f_t - 4f_s^2, 0, -4f_b(f_a^2f_t + f_s^2), 0, 0, 4f_t(f_a^2f_t + f_s^2), 0, 0, 0, 0, \\
& 2f_s(4f_r + f_a^2), 0, 2f_sf_b(4f_r + f_a^2), 0, 0, -2f_tf_s(4f_r + f_a^2), -4f_r(4f_r + f_a^2), -2f_a(f_s^2 \\
& - 4f_tf_r), -4f_bf_r(4f_r + f_a^2), 0, -2f_bf_a(f_s^2 - 4f_tf_r), 4f_rf_t(4f_r + f_a^2), 0, 0, 2f_af_t(f_s^2 \\
& - 4f_tf_r), 0], \\
& [0, 0, 2f_a(f_a^2f_t + f_s^2), 0, 2f_s^3 + 2f_bf_af_s^2 + 2f_sf_a^2f_t + 2f_bf_tf_a^3, 0, -f_af_s(4f_r + f_a^2), 0, \\
& -f_s(4f_rf_s + f_sf_a^2 + 4f_bf_rf_a + f_bf_a^3), 2f_af_r(4f_r + f_a^2), f_s^2f_a^2 - 4f_s^2f_r - 8f_a^2f_tf_r, 2f_r(4f_rf_s \\
& + f_sf_a^2 + 4f_bf_rf_a + f_bf_a^3), 0, f_af_s^3 + f_a^2f_s^2f_b - 2f_s^2f_bf_r - 4f_rf_af_tf_s - 6f_rf_bf_a^2f_p, 0, 0, 0, 0, 0, \\
& 0, 2f_sf_r(4f_r + f_a^2), 0, 0, f_bf_rf_s(4f_r + f_a^2), 0, 0, -4f_r^2(4f_r + f_a^2), 0, -2f_af_r(f_s^2 - 4f_tf_r), \\
& -2f_bf_r^2(4f_r + f_a^2), 0, 0, -f_bf_af_r(f_s^2 - 4f_tf_r), 0, 0], \\
& [0, 0, 2f_b(f_a^2f_t + f_s^2), 0, 4f_s^2f_t + 2f_s^2f_b^2 + 4f_a^2f_t^2 + 2f_b^2f_a^2f_p, 0, 2f_af_s^2 - 4f_bf_rf_s - f_a^2f_sf_b \\
& + 2f_a^3f_p, 0, 2f_s^3 + 2f_bf_af_s^2 - 4f_sf_rf_b^2 - f_sf_b^2f_a^2 - 8f_sf_rf_t + 2f_bf_tf_a^3, 2f_bf_r(4f_r + f_a^2), -4f_s^3 \\
& + f_bf_af_s^2 - 4f_sf_a^2f_t - 4f_bf_af_tf_r - 2f_r(2f_s^2 - 4f_rf_b^2 - f_b^2f_a^2 - 8f_tf_r), 0, -2f_bf_s^3 + 2f_s^2f_af_t \\
& + f_b^2f_af_s^2 - 2f_bf_a^2f_sf_t - 8f_af_t^2f_r - 4f_rf_af_tf_b^2, -2f_bf_r(f_a^2f_t + f_s^2), 0, -f_af_s(4f_r + f_a^2), 0, \\
& -f_s(4f_rf_s + f_sf_a^2 + 4f_bf_rf_a + f_bf_a^3), 2f_af_r(4f_r + f_a^2), -4f_a^2f_tf_r + 8f_s^2f_r + 3f_s^2f_a^2, 2f_r(2f_s \\
& f_a^2 + 8f_rf_s + 4f_bf_rf_a + f_bf_a^3), 0, f_af_s^3 + 4f_s^2f_bf_r + 2f_a^2f_s^2f_b - 4f_rf_af_tf_s - 4f_rf_bf_a^2f_p \\
& f_bf_rf_s(4f_r + f_a^2), 0, -4f_sf_r(4f_r + f_a^2), -4f_r^2(4f_r + f_a^2), -2f_af_s(f_s^2 - 4f_tf_r), -2f_r(f_af_s^2 \\
& + f_a^2f_sf_b + 4f_bf_rf_s - 4f_af_tf_r), -2f_bf_r^2(4f_r + f_a^2), 0, -f_sf_bf_a(f_s^2 - 4f_tf_r), -f_bf_af_r(f_s^2
\end{aligned}$$

$$-4f_t f_r), 0],$$

$$\begin{aligned} & [0, 0, 0, 0, 0, 0, 2f_b(f_a^2 f_t + f_s^2), 0, 4f_s^2 f_t + 2f_s^2 f_b^2 + 4f_a^2 f_t^2 + 2f_b^2 f_a^2 f_r, 2f_a(f_a^2 f_t + f_s^2), \\ & -4f_t(f_a^2 f_t + f_s^2), -2f_s^3 + 2f_b f_a f_s^2 - 2f_s f_a^2 f_t + 2f_b f_t f_a^3, 0, -2f_b f_t(f_a^2 f_t + f_s^2), -2f_s f_b(f_a^2 f_t \\ & + f_s^2), 0, -f_s f_b(4f_r + f_a^2), 0, -f_s(f_b^2 f_a^2 + 4f_r f_b^2 + 2f_a^2 f_t + 8f_t f_r), 8f_b f_r^2 + 2f_r f_b f_a^2 \\ & -4f_r f_s f_a - f_a^3 f_s f_b f_a f_s^2 + 8f_s f_r f_t + 2f_s f_a^2 f_t - 4f_b f_a f_t f_r, 4f_s^2 f_r + f_s^2 f_a^2 - 4f_b f_a f_r f_s - f_s f_b f_a^3 \\ & + 2f_b^2 f_a^2 f_r + 4f_a^2 f_t f_r + 8f_r^2 f_b^2 + 16f_r^2 f_r, 0, 2f_s^2 f_a f_t + f_b^2 f_a f_s^2 + 4f_s f_b f_t f_r + f_b f_a^2 f_s f_t - 8f_a \\ & f_t^2 f_r - 4f_r f_a f_t f_b^2, f_s^2 f_b(4f_r + f_a^2), 2f_a f_r(4f_r + f_a^2), f_s^2 f_a^2 - 8f_a^2 f_t f_r - 16f_r^2 f_r, -2f_r(4f_r f_s \\ & + f_s f_a^2 - 4f_b f_r f_a - f_b f_a^3), -2f_a f_t(f_s^2 - 4f_t f_r), -f_a f_s^3 + f_a^2 f_s^2 f_b + 4f_r f_a f_t f_s - 6f_r f_b f_a^2 f_t \\ & - 8f_b f_t f_r^2, -2f_b f_r f_s(4f_r + f_a^2), 0, -f_a f_t f_b(f_s^2 - 4f_t f_r), -f_s f_b f_a(f_s^2 - 4f_t f_r), 0], \end{aligned}$$

$$\begin{aligned} & [0, 0, 0, 0, 0, 0, 0, 0, 0, 2f_b(f_a^2 f_t + f_s^2), 0, 2f_b^2(f_a^2 f_t + f_s^2), 0, 0, -2f_b f_t(f_a^2 f_t + f_s^2), 0, 0, 0, \\ & 0, -f_s f_b(4f_r + f_a^2), 0, -f_b^2 f_s(4f_r + f_a^2), 0, 0, f_b f_s f_t(4f_r + f_a^2), 2f_b f_r(4f_r + f_a^2), f_b f_a(f_s^2 \\ & - 4f_t f_r), 2f_r f_b^2(4f_r + f_a^2), 0, f_b^2 f_a(f_s^2 - 4f_t f_r), -2f_r f_t f_b(4f_r + f_a^2), 0, 0, -f_a f_t f_b(f_s^2 \\ & - 4f_t f_r), 0], \end{aligned}$$

$$\begin{aligned} & [4f_r(f_a^2 f_t + f_s^2), -2f_s f_r(4f_r + f_a^2), 4f_r^2(4f_r + f_a^2), 2f_a f_r(3f_s^2 + 2f_a^2 f_t - 4f_t f_r), 0, 0, 0, \\ & -2f_r f_s f_a(4f_r + f_a^2), 0, 0, 4f_a f_r^2(4f_r + f_a^2), 0, 2f_r(f_s^2 f_a^2 - 2f_s^2 f_r - 6f_a^2 f_t f_r), 0, 0, 0, 0, 0, \\ & 0, 0, 0, 0, 2f_s f_r^2(4f_r + f_a^2), 0, 0, 0, 0, 0, -4f_r^3(4f_r + f_a^2), 0, 0, -2f_a f_r^2(f_s^2 - 4f_t f_r), 0, 0, 0 \\ & ], \end{aligned}$$

$$\begin{aligned} & [2f_s(f_a^2 f_t + f_s^2), -f_a^2(f_s^2 - 4f_t f_r), 2f_s f_r(4f_r + f_a^2), 3f_a f_s^3 + 2f_s^2 f_b f_r - 4f_r f_a f_t f_s + 2f_a^3 f_s f_t \\ & + 2f_r f_b f_a^2 f_r, 2f_a f_r(f_a^2 f_t + f_s^2), -2f_s f_r(4f_r + f_a^2), 4f_r^2(4f_r + f_a^2), -f_s^2 f_a^3 - f_s f_b f_a^2 f_r \\ & - 4f_s f_b f_r^2 + 2f_a^3 f_t f_r - 8f_a f_t f_r^2, -f_r f_s f_a(4f_r + f_a^2), 0, 2f_r(4f_r f_s f_a + f_a^3 f_s + 4f_b f_r^2 + f_r f_b \\ & f_a^2), 2f_a f_r^2(4f_r + f_a^2), f_a^2 f_s^3 - 4f_r f_s^3 + f_r f_a f_s^2 f_b - 8f_r f_a^2 f_s f_t - 4f_r^2 f_a f_t f_b f_r(f_s^2 f_a^2 - 4f_s^2 f_r \\ & - 8f_a^2 f_t f_r), 0, 0, 0, -f_r f_s f_a(4f_r + f_a^2), 0, 0, 2f_a f_r^2(4f_r + f_a^2), 0, f_r(-4f_a^2 f_t f_r + 8f_s^2 f_r + 3 \\ & f_s^2 f_a^2), 2f_s f_r^2(4f_r + f_a^2), 0, 0, 0, 0, -4f_s f_r^2(4f_r + f_a^2), -4f_r^3(4f_r + f_a^2), 0, -2f_s f_a f_r(f_s^2 \\ & - 4f_t f_r), -2f_a f_r^2(f_s^2 - 4f_t f_r), 0, 0], \end{aligned}$$

$$\begin{aligned} & [0, 2f_s(f_a^2 f_t + f_s^2), 4f_r(f_a^2 f_t + f_s^2), 2f_a f_t(f_a^2 f_t + f_s^2), 2f_a f_s(f_a^2 f_t + f_s^2), -(4f_r + f_a^2)f_s^2, 0, \\ & f_a f_s^3 + 2f_s^2 f_b f_r - f_a^3 f_s f_t - 8f_r f_a f_t f_s + 2f_r f_b f_a^2 f_r, -f_a f_s^2(4f_r + f_a^2), 4f_r^2(4f_r + f_a^2), 4f_a f_r(f_a^2 f_t + f_s^2), \\ & 2f_r f_s f_a(4f_r + f_a^2), f_t(f_s^2 f_a^2 - 4f_s^2 f_r - 8f_a^2 f_t f_r), f_s(f_s^2 f_a^2 - 4f_s^2 f_r - 8f_a^2 f_t f_r), 0, \\ & 0, 0, -f_b f_r f_s(4f_r + f_a^2), 0, 0, -f_r(4f_r f_s f_a + f_a^3 f_s - 8f_b f_r^2 - 2f_r f_b f_a^2), 0, f_r(f_b f_a f_s^2 \\ & + 8f_s f_r f_t + 2f_s f_a^2 f_t - 4f_b f_a f_t f_r), 2f_r f_s^2(4f_r + f_a^2), 0, 0, 2f_a f_r^2(4f_r + f_a^2), 0, f_r(f_s^2 f_a^2 - 8 \end{aligned}$$

$$\begin{aligned}
& f_a^2 f_t f_r - 16 f_r^2 f_t), -4 f_s f_r^2 (4 f_r + f_a^2), 0, -2 f_a f_t f_r (f_s^2 - 4 f_t f_r), -2 f_s f_a f_r (f_s^2 - 4 f_t f_r), 0, 0 \\
& ], \\
& [0, 0, 2 f_s (f_a^2 f_t + f_s^2), 0, 2 f_a f_t (f_a^2 f_t + f_s^2), 0, -(4 f_r + f_a^2) f_s^2, 0, -f_s f_a f_t (4 f_r + f_a^2), \\
& 2 f_s f_r (4 f_r + f_a^2), f_a f_s^3 + 2 f_s^2 f_b f_r - 4 f_r f_a f_t f_s + 2 f_r f_b f_a^2 f_r, 2 f_a f_r f_t (4 f_r + f_a^2), 0, f_t (f_s^2 f_a^2 \\
& - 4 f_s^2 f_r - 8 f_a^2 f_t f_r), 0, 0, 0, 0, 0, 0, -f_b f_r f_s (4 f_r + f_a^2), 0, 0, 2 f_s f_r f_t (4 f_r + f_a^2), 0, 0, 2 f_b \\
& f_r^2 (4 f_r + f_a^2), 0, f_b f_a f_r (f_s^2 - 4 f_t f_r), -4 f_r^2 f_t (4 f_r + f_a^2), 0, 0, -2 f_a f_t f_r (f_s^2 - 4 f_t f_r), 0, 0], \\
& [4 f_t (f_a^2 f_t + f_s^2), 2 f_s (2 f_s^2 - 4 f_t f_r + f_a^2 f_t), 4 f_r f_t (4 f_r + f_a^2), -8 f_a f_t^2 f_r + 4 f_b f_s^3 + 4 f_b f_a^2 f_s f_t \\
& + 2 f_s^2 f_a f_r, 4 f_b f_r (f_a^2 f_t + f_s^2), -4 f_s^2 f_r + 4 f_a^2 f_t f_r - 2 f_s^2 f_a^2, 4 f_s f_r (4 f_r + f_a^2), 2 f_s (3 f_a f_s^2 - \\
& f_a^2 f_s f_b - 4 f_b f_r f_s - 4 f_a f_t f_r + 2 f_a^3 f_t), 2 f_r (2 f_a f_s^2 - 4 f_b f_r f_s - f_a^2 f_s f_b + 2 f_a^3 f_t), 0, \\
& 4 f_b f_r f_s (4 f_r + f_a^2), 4 f_b f_r^2 (4 f_r + f_a^2), -2 f_s (4 f_b f_a f_t f_r - f_b f_a f_s^2 + 2 f_s^3 + 2 f_s f_a^2 f_t), \\
& -2 f_r (4 f_b f_a f_t f_r - f_b f_a f_s^2 + 4 f_s f_a^2 f_t + 4 f_s^3), -4 f_r^2 (f_a^2 f_t + f_s^2), -2 f_s f_r (4 f_r + f_a^2), 4 f_r^2 (4 f_r \\
& + f_a^2), -2 f_a (4 f_r^2 f_t + 3 f_s^2 f_r + f_s^2 f_a^2), -2 f_r f_s f_a (4 f_r + f_a^2), 0, 4 f_r f_s f_a (4 f_r + f_a^2), 4 f_a \\
& f_r^2 (4 f_r + f_a^2), 4 f_s (2 f_s^2 f_r - 2 f_a^2 f_t f_r + f_s^2 f_a^2), 2 f_r (-4 f_a^2 f_t f_r + 8 f_s^2 f_r + 3 f_s^2 f_a^2), 2 f_s f_r^2 (4 f_r \\
& + f_a^2), 0, 0, 0, -4 f_r f_s^2 (4 f_r + f_a^2), -8 f_s f_r^2 (4 f_r + f_a^2), -4 f_r^3 (4 f_r + f_a^2), -2 f_a f_s^2 (f_s^2 \\
& - 4 f_t f_r), -4 f_s f_a f_r (f_s^2 - 4 f_t f_r), -2 f_a f_r^2 (f_s^2 - 4 f_t f_r), 0], \\
& [0, 4 f_t (f_a^2 f_t + f_s^2), 2 f_s (f_a^2 f_t + f_s^2), 2 f_b f_t (f_a^2 f_t + f_s^2), 2 f_s f_b (f_a^2 f_t + f_s^2), 2 f_s (f_s^2 - 4 f_t f_r), \\
& 16 f_r^2 f_t + 8 f_a^2 f_t f_r - f_s^2 f_a^2, 2 f_b f_s^3 + 4 f_s^2 f_a f_t + f_b f_a^2 f_s f_t - 4 f_s f_b f_t f_r + 2 f_a^3 f_t^2 - 8 f_a f_t^2 f_r, 2 f_a f_s^3 \\
& - f_a^2 f_s^2 f_b - 2 f_s^2 f_b f_r + 2 f_a^3 f_s f_t + 2 f_r f_b f_a^2 f_r, 2 f_s f_r (4 f_r + f_a^2), 3 f_a f_s^3 - 4 f_r f_a f_t f_s + 2 f_a^3 f_s f_t \\
& + 2 f_r f_b f_a^2 f_t + 8 f_b f_t f_r^2, 2 f_r (f_a f_s^2 + f_a^2 f_s f_b + 4 f_b f_r f_s + f_a^3 f_t), -f_t (4 f_b f_a f_t f_r - f_b f_a f_s^2 + 4 f_s \\
& f_a^2 f_t + 4 f_s^3), -4 f_s^4 + f_b f_a f_s^3 - 4 f_s^2 f_r f_t - 4 f_s^2 f_a^2 f_t - 4 f_s f_b f_a f_t f_r - 4 f_a^2 f_t^2 f_r - 4 f_s f_r (f_a^2 f_t + \\
& f_s^2), -(4 f_r + f_a^2) f_s^2, 0, f_s (f_a f_s^2 - f_a^2 f_s f_b - 4 f_b f_r f_s - f_a^3 f_t - 8 f_a f_t f_r), -f_s (4 f_r f_s f_a + f_a^3 f_s \\
& + 4 f_b f_r^2 + f_r f_b f_a^2), 4 f_r^2 (4 f_r + f_a^2), -f_s^2 f_a^3 - 2 f_s^2 f_a f_r + 8 f_s f_b f_r^2 + 2 f_s f_b f_a^2 f_r + 2 f_a^3 f_t f_r, \\
& f_r (4 f_r f_s f_a + f_a^3 f_s + 8 f_b f_r^2 + 2 f_r f_b f_a^2), f_b f_a f_s^3 + 8 f_s^2 f_r f_t + 3 f_s^2 f_a^2 f_t - 4 f_s f_b f_a f_t f_r - 4 f_a^2 \\
& f_t^2 f_r, 3 f_a^2 f_s^3 + 8 f_r f_s^3 + f_r f_a f_s^2 f_b - 2 f_r f_a^2 f_s f_t + 8 f_r^2 f_t f_s - 4 f_r^2 f_a f_t f_b, 2 f_r f_s^2 (4 f_r + f_a^2), 0, \\
& 2 f_r f_s f_a (4 f_r + f_a^2), 2 f_a f_r^2 (4 f_r + f_a^2), f_s (f_s^2 f_a^2 - 8 f_a^2 f_t f_r - 16 f_r^2 f_t), -f_r (3 f_s^2 f_a^2 + 16 f_s^2 f_r \\
& + 8 f_a^2 f_t f_r + 16 f_r^2 f_t), -4 f_s f_r^2 (4 f_r + f_a^2), -2 f_a f_t f_s (f_s^2 - 4 f_t f_r), -2 f_a (f_s^4 - 3 f_s^2 f_r f_t - 4 \\
& f_r^2 f_t^2), -2 f_s f_a f_r (f_s^2 - 4 f_t f_r), 0], \\
& [0, 0, 4 f_t (f_a^2 f_t + f_s^2), 0, 2 f_b f_t (f_a^2 f_t + f_s^2), 0, 2 f_s (f_s^2 - 4 f_t f_r), 0, f_t (2 f_a f_s^2 - 4 f_b f_r f_s - \\
& f_a^2 f_s f_b + 2 f_a^3 f_t), 4 f_r f_t (4 f_r + f_a^2), 2 f_b f_s^3 + 2 f_s^2 f_a f_t + 2 f_b f_a^2 f_s f_t - 8 f_a f_t^2 f_r, 2 f_b f_r (4 f_t f_r + 2
\end{aligned}$$



$$\begin{aligned}
& f_a^2 f_t + f_s^2), 0, -f_t (4 f_b f_a f_t f_r - f_b f_a f_s^2 + 4 f_s f_a^2 f_t + 4 f_s^3), -4 f_r f_t (f_a^2 f_t + f_s^2), 0, - (4 f_r + f_a^2) \\
& f_s^2, 0, -f_s f_a f_t (4 f_r + f_a^2), 2 f_s f_r (4 f_r + f_a^2), f_s (f_a f_s^2 - 4 f_b f_r f_s - f_a^2 f_s f_b - 4 f_a f_t f_r), -f_r ( \\
& f_a^2 f_s f_b + 4 f_b f_r f_s - 8 f_a f_t f_r - 2 f_a^3 f_t), 0, f_t (-4 f_a^2 f_t f_r + 8 f_s^2 f_r + 3 f_s^2 f_a^2), 2 f_s f_r f_t (4 f_r + f_a^2), \\
& 0, 2 f_b f_r f_s (4 f_r + f_a^2), 2 f_b f_r^2 (4 f_r + f_a^2), f_s f_b f_a (f_s^2 - 4 f_t f_r), f_r (f_b f_a f_s^2 - 16 f_s f_r f_t - 4 f_s f_a^2 f_t \\
& - 4 f_b f_a f_t f_r), -4 f_r^2 f_t (4 f_r + f_a^2), 0, -2 f_a f_t f_s (f_s^2 - 4 f_t f_r), -2 f_a f_t f_r (f_s^2 - 4 f_t f_r), 0], \\
& [0, 0, 0, 0, 0, 4 f_t (f_a^2 f_t + f_s^2), 4 f_s (f_a^2 f_t + f_s^2), 4 f_b f_t (f_a^2 f_t + f_s^2), 4 f_s f_b (f_a^2 f_t + f_s^2), 4 f_r (f_a^2 f_t \\
& + f_s^2), 4 f_a f_t (f_a^2 f_t + f_s^2), 4 f_a f_s (f_a^2 f_t + f_s^2), -4 f_t^2 (f_a^2 f_t + f_s^2), -8 f_t f_s (f_a^2 f_t + f_s^2), -4 f_s^2 ( \\
& f_a^2 f_t + f_s^2), -2 f_t f_s (4 f_r + f_a^2), 16 f_r^2 f_t - 8 f_s^2 f_r + 4 f_a^2 f_t f_r - 2 f_s^2 f_a^2, 2 f_t (f_a f_s^2 - 4 f_b f_r f_s - \\
& f_a^2 f_s f_b - 4 f_a f_t f_r), -2 f_s^2 f_b (4 f_r + f_a^2), 2 f_s f_r (4 f_r + f_a^2), 16 f_b f_t f_r^2 + 4 f_r f_b f_a^2 f_t - 16 f_r f_a f_t f_s \\
& + 2 f_a f_s^3 - 2 f_a^3 f_s f_r - 2 f_s (4 f_r f_s f_a + f_a^3 f_s - 8 f_b f_r^2 - 2 f_r f_b f_a^2), 2 f_t (f_b f_a f_s^2 + 4 f_s f_r f_t + f_s \\
& f_a^2 f_t - 4 f_b f_a f_t f_r), 2 f_s (f_b f_a f_s^2 + 8 f_s f_r f_t + 2 f_s f_a^2 f_t - 4 f_b f_a f_t f_r), 2 f_s^3 (4 f_r + f_a^2), 4 f_r^2 (4 f_r \\
& + f_a^2), 2 f_a f_r (4 f_t f_r + 2 f_a^2 f_t + f_s^2), 4 f_r f_s f_a (4 f_r + f_a^2), 2 f_t (f_s^2 f_a^2 - 8 f_r^2 f_t - 6 f_a^2 f_t f_r), 2 f_s ( \\
& f_s^2 f_a^2 - 8 f_a^2 f_t f_r - 16 f_r^2 f_t), -4 f_r f_s^2 (4 f_r + f_a^2), -2 f_a f_t^2 (f_s^2 - 4 f_t f_r), -4 f_a f_t f_s (f_s^2 - 4 f_t f_r), \\
& -2 f_a f_s^2 (f_s^2 - 4 f_t f_r), 0], \\
& [0, 0, 0, 0, 0, 0, 4 f_t (f_a^2 f_t + f_s^2), 0, 2 f_b f_t (f_a^2 f_t + f_s^2), 2 f_s (f_a^2 f_t + f_s^2), 2 f_b f_t (f_a^2 f_t + f_s^2), 2 f_b \\
& f_s^3 + 2 f_s^2 f_a f_t + 2 f_b f_a^2 f_s f_t + 2 f_a^3 f_t^2, 0, -4 f_t^2 (f_a^2 f_t + f_s^2), -4 f_t f_s (f_a^2 f_t + f_s^2), 0, -2 f_t f_s (4 f_r \\
& + f_a^2), 0, -f_b f_s f_t (4 f_r + f_a^2), -4 f_s^2 f_r - f_s^2 f_a^2 + 16 f_r^2 f_t + 4 f_a^2 f_t f_r f_t (2 f_a f_s^2 - 4 f_b f_r f_s - \\
& f_a^2 f_s f_b - 8 f_a f_t f_r), -f_a^2 f_s^2 f_b - 4 f_s^2 f_b f_r - f_a^3 f_s f_t - 4 f_r f_a f_t f_s + 2 f_r f_b f_a^2 f_t + 8 f_b f_t f_r^2, 0, f_t (f_b f_a \\
& f_s^2 + 8 f_s f_r f_t + 2 f_s f_a^2 f_t - 4 f_b f_a f_t f_r), 2 f_s^2 f_t (4 f_r + f_a^2), 2 f_s f_r (4 f_r + f_a^2), f_a f_s^3 - 4 f_r f_a f_t f_s \\
& + 2 f_r f_b f_a^2 f_t + 8 f_b f_t f_r^2, 2 f_r (f_a^2 f_s f_b + 4 f_b f_r f_s + f_a^3 f_t + 4 f_a f_t f_r), f_a f_t f_b (f_s^2 - 4 f_t f_r), f_b f_a f_s^3 \\
& + f_s^2 f_a^2 f_t - 4 f_s f_b f_a f_t f_r - 16 f_r^2 f_t^2 - 8 f_a^2 f_t^2 f_r - 4 f_s f_r f_t (4 f_r + f_a^2), 0, -2 f_a f_t^2 (f_s^2 - 4 f_t f_r), \\
& -2 f_a f_t f_s (f_s^2 - 4 f_t f_r), 0], \\
& [0, 0, 0, 0, 0, 0, 0, 0, 0, 4 f_t (f_a^2 f_t + f_s^2), 0, 4 f_b f_t (f_a^2 f_t + f_s^2), 0, 0, -4 f_t^2 (f_a^2 f_t + f_s^2), 0, 0, 0, \\
& 0, -2 f_t f_s (4 f_r + f_a^2), 0, -2 f_b f_s f_t (4 f_r + f_a^2), 0, 0, 2 f_t^2 f_s (4 f_r + f_a^2), 4 f_r f_t (4 f_r + f_a^2), \\
& 2 f_a f_t (f_s^2 - 4 f_t f_r), 4 f_r f_t f_b (4 f_r + f_a^2), 0, 2 f_a f_t f_b (f_s^2 - 4 f_t f_r), -4 f_r f_t^2 (4 f_r + f_a^2), 0, 0, \\
& -2 f_a f_t^2 (f_s^2 - 4 f_t f_r), 0]]
\end{aligned}$$

It's hopeless to calculate its rank or to check the determinant of a sub-matrix is nonzero (in fact, at this place my computer was working at the edge of its capabilities for 4 hours). Instead we substitute as values of the 1-jet of  $f$  a random (our choice) set of rational numbers. The matrix becomes rational, so calculating its rank is an easy problem via Gaussian elimination.

$$\begin{aligned}
\mathbf{J2} > MEQa := \text{subs}\left(\text{subs}\left(\left[u_{2,2}=r, u_{2,3}=s, u_{3,3}=t, u_{1,2}=a, u_{1,3}=b\right], \left[\text{diff}\left(f\left(u_{2,2}, u_{2,3}, \right.\right.\right.\right. \\
& \left.\left.\left.\left. u_{3,3}, u_{1,2}, u_{1,3}\right), u_{2,2}\right)=2, \text{diff}\left(f\left(u_{2,2}, u_{2,3}, u_{3,3}, u_{1,2}, u_{1,3}\right), u_{2,3}\right)=-\frac{7}{2}, \right.\right.\right. \\
& \left.\left.\left.\left. \text{diff}\left(f\left(u_{2,2}, u_{2,3}, u_{3,3}, u_{1,2}, u_{1,3}\right), u_{3,3}\right)=5, \text{diff}\left(f\left(u_{2,2}, u_{2,3}, u_{3,3}, u_{1,2}, u_{1,3}\right), \right.\right.\right.\right. \\
& \left.\left.\left.\left. u_{1,2}\right)=-3, \text{diff}\left(f\left(u_{2,2}, u_{2,3}, u_{3,3}, u_{1,2}, u_{1,3}\right), u_{1,3}\right)=\frac{1}{2}\right]\right], MEQ\right) \\
MEQa := & \left[\left[-1130, -\frac{1471}{4}, -119, 2835, -\frac{777}{4}, 0, 0, \frac{4413}{4}, 0, 0, 357, 0, 3925, \frac{2331}{4}, 0, 0, \right.\right. \\
& 0, 0, 0, 0, 0, 0, \frac{1471}{2}, 0, 0, 0, 0, 0, 238, 0, 0, 1110, \frac{777}{2}, 0, 0\Big], \\
& \left[0, -1130, 0, -\frac{565}{2}, 1695, -\frac{1471}{4}, -119, \frac{16769}{16}, \frac{2859}{8}, 0, -\frac{119}{4}, \frac{357}{2}, -\frac{8465}{4}, \right. \\
& \frac{48703}{16}, \frac{2331}{8}, 0, 0, \frac{4413}{8}, 0, 0, \frac{357}{2}, 0, \frac{3023}{16}, \frac{8215}{8}, 0, 0, 0, 0, -\frac{833}{4}, 238, 0, \\
& \left.-\frac{3885}{4}, \frac{12321}{16}, \frac{777}{2}, 0\right], \\
& \left[0, 0, -1130, 0, -\frac{565}{2}, 0, -\frac{1471}{4}, 0, -\frac{1471}{16}, -119, 1140, -224, 0, -\frac{8465}{4}, -\frac{777}{16}, 0, \right. \\
& 0, 0, 0, 0, \frac{4413}{8}, 0, 0, -\frac{10297}{16}, 0, 0, \frac{357}{2}, 0, \frac{1665}{2}, \frac{665}{8}, 0, 0, -\frac{3885}{4}, -\frac{5439}{16}, 0\Big], \\
& \left[-1695, -\frac{4413}{8}, -\frac{357}{2}, \frac{8505}{2}, -\frac{2331}{8}, 0, 0, \frac{13239}{8}, 0, 0, \frac{1071}{2}, 0, \frac{11775}{2}, \frac{6993}{8}, \right. \\
& 0, 0, 0, 0, 0, 0, 0, \frac{4413}{4}, 0, 0, 0, 0, 0, 357, 0, 0, 1665, \frac{2331}{4}, 0, 0\Big], \\
& \left[\frac{565}{2}, -\frac{25649}{16}, \frac{119}{4}, \frac{5075}{4}, -\frac{35383}{16}, -\frac{4413}{8}, -\frac{357}{2}, \frac{27521}{4}, -\frac{8215}{8}, 0, 119, \right. \\
& -238, -\frac{10755}{2}, \frac{9897}{4}, -\frac{777}{2}, 0, 0, \frac{19123}{8}, 0, 0, \frac{1547}{2}, 0, \frac{26829}{16}, \frac{18927}{8}, 0, 0, 0, 0, \\
& \left.-\frac{2499}{4}, 357, 0, -\frac{11655}{4}, \frac{10323}{16}, \frac{2331}{4}, 0\right], \\
& \left[0, \frac{565}{2}, -1695, -5650, 3955, \frac{1471}{16}, -\frac{4175}{8}, -4525, \frac{21371}{16}, -\frac{357}{2}, \frac{11835}{2}, \frac{1001}{8}, \right. \\
& 5700, -\frac{19845}{4}, \frac{5439}{8}, 0, 0, -\frac{7355}{8}, 0, 0, \frac{16743}{8}, 0, \frac{10965}{8}, -\frac{38661}{16}, 0, 0, \frac{1547}{2}, 0, \\
& 4500, \frac{5103}{8}, 0, \frac{8325}{2}, -\frac{11655}{8}, -\frac{16317}{16}, 0\Big], \\
& \left[0, 0, \frac{565}{2}, 0, -5650, 0, \frac{1471}{16}, 0, -\frac{7355}{4}, \frac{119}{4}, -\frac{10745}{4}, -\frac{8743}{16}, 0, 5700, -\frac{3885}{4}, \right. \\
& 0, 0, 0, 0, 0, -\frac{7355}{8}, 0, 0, \frac{22065}{8}, 0, 0, -\frac{595}{2}, 0, -\frac{2775}{2}, \frac{3255}{8}, 0, 0, \frac{8325}{2}, \frac{11655}{8}, 0 \\
& \Big],
\end{aligned} \tag{35}$$

$$\begin{aligned}
& \left[ 0, 0, 0, 0, 0, -1130, 0, -565, 3390, 0, 0, 0, 5650, -3955, 2260, -\frac{1471}{4}, -119, -\frac{5911}{8}, \right. \\
& 909, 0, -\frac{119}{2}, 357, \frac{6245}{4}, \frac{1123}{4}, \frac{5273}{4}, 0, 0, 0, 595, -\frac{833}{2}, 238, 2775, -\frac{3885}{4}, \\
& \left. \frac{3441}{8}, \frac{777}{2} \right], \\
& \left[ 0, 0, 0, 0, 0, 0, -1130, 0, -\frac{565}{2}, 0, -\frac{565}{2}, 1695, 0, 5650, -\frac{3955}{2}, 0, -\frac{1471}{4}, 0, \right. \\
& -\frac{1471}{16}, -119, -\frac{10351}{16}, \frac{2621}{8}, 0, 1700, -\frac{5537}{8}, 0, -\frac{119}{4}, \frac{357}{2}, -\frac{555}{4}, \frac{22063}{16}, \\
& \left. \frac{665}{8}, 0, 2775, 0, -\frac{5439}{16} \right], \\
& \left[ 0, -1695, 0, -2825, 7345, -\frac{4413}{8}, -\frac{357}{2}, -\frac{32095}{8}, 2099, 0, -\frac{595}{2}, \frac{1547}{2}, -\frac{3905}{2}, \right. \\
& \frac{52095}{8}, \frac{10101}{8}, 0, 0, -\frac{1471}{2}, 0, 0, -238, 0, -\frac{10351}{8}, \frac{2859}{4}, 0, 0, 0, 0, -\frac{119}{2}, 357, 0, \\
& \left. -\frac{555}{2}, \frac{12543}{8}, \frac{2331}{4}, 0 \right], \\
& \left[ 0, \frac{565}{2}, 0, \frac{23165}{4}, -2825, -\frac{25649}{16}, \frac{119}{4}, \frac{100911}{32}, \frac{67427}{16}, 0, \frac{4879}{8}, -\frac{595}{2}, \right. \\
& \frac{30665}{8}, -\frac{220463}{32}, \frac{23235}{8}, -\frac{4413}{8}, -\frac{357}{2}, -\frac{1859}{4}, \frac{2727}{2}, 0, 119, \frac{1071}{2}, \frac{28057}{32}, \\
& \left. \frac{9235}{16}, \frac{15819}{8}, 0, 0, 0, \frac{833}{8}, -\frac{2737}{4}, 357, \frac{3885}{8}, -\frac{96681}{32}, \frac{8769}{16}, \frac{2331}{4} \right], \\
& \left[ 0, 0, 0, 0, 0, \frac{565}{2}, -1695, \frac{565}{4}, 1130, 0, -2825, 7345, -\frac{2825}{2}, \frac{37855}{4}, -\frac{11865}{2}, \right. \\
& \frac{1471}{16}, -\frac{4175}{8}, \frac{5911}{32}, \frac{6661}{16}, -\frac{357}{2}, -1737, 2218, -\frac{6245}{16}, \frac{58547}{16}, -\frac{27783}{16}, 0, \\
& \left. -\frac{595}{2}, \frac{1547}{2}, -\frac{6145}{4}, \frac{8237}{2}, \frac{5103}{8}, -\frac{2775}{4}, \frac{70485}{16}, -\frac{41181}{32}, -\frac{16317}{16} \right], \\
& \left[ 0, 0, 0, 0, 0, 0, \frac{565}{2}, 0, -5650, 0, \frac{23165}{4}, -2825, 0, -\frac{2825}{2}, 8475, 0, \frac{1471}{16}, 0, \right. \\
& -\frac{7355}{4}, \frac{119}{4}, \frac{64751}{32}, -\frac{23453}{16}, 0, -\frac{51755}{16}, \frac{14295}{8}, 0, \frac{4879}{8}, -\frac{595}{2}, \frac{22755}{8}, \\
& \left. -\frac{17303}{32}, \frac{3255}{8}, 0, -\frac{2775}{4}, \frac{62715}{16}, \frac{11655}{8} \right], \\
& \left[ 0, 0, 0, 0, 0, 0, 0, 0, 0, -1130, 0, -565, 0, 0, 5650, 0, 0, 0, 0, -\frac{1471}{4}, 0, -\frac{1471}{8}, 0, 0, \right. \\
& \left. \frac{7355}{4}, -119, -555, -\frac{1015}{4}, 0, -\frac{555}{2}, \frac{3983}{8}, 0, 0, 2775, \frac{3885}{4} \right], \\
& \left[ 0, 0, -1695, 0, -2825, 0, -\frac{4413}{8}, 0, -\frac{7355}{8}, -\frac{357}{2}, -\frac{6185}{2}, -\frac{4711}{8}, 0, -\frac{3905}{2}, \right. \\
& \left. -\frac{3885}{8}, 0, 0, 0, 0, 0, -\frac{1471}{2}, 0, 0, -\frac{1471}{8}, 0, 0, -238, 0, -1110, -448, 0, 0, -\frac{555}{2}, \right.
\end{aligned}$$

$$\begin{aligned}
& -\frac{777}{8}, 0], \\
& \left[ 0, 0, \frac{565}{2}, 0, \frac{23165}{4}, 0, -\frac{25649}{16}, 0, -\frac{30089}{32}, \frac{119}{4}, \frac{16375}{4}, -\frac{25625}{16}, 0, \frac{30665}{8}, \right. \\
& \frac{13777}{32}, 0, -\frac{4413}{8}, 0, -\frac{7355}{8}, -\frac{357}{2}, \frac{3637}{8}, -\frac{10595}{8}, 0, -\frac{34103}{32}, -\frac{1339}{2}, 0, \frac{833}{2}, \\
& \left. -238, \frac{3885}{2}, -326, -448, 0, \frac{3885}{8}, -\frac{3441}{32}, -\frac{777}{8} \right], \\
& \left[ 0, 0, 0, 0, 0, 0, \frac{565}{2}, 0, \frac{23165}{4}, -1695, -5650, 1130, 0, -\frac{2825}{2}, \frac{3955}{4}, 0, \frac{1471}{16}, 0, \right. \\
& \frac{60311}{32}, -\frac{4175}{8}, -1700, \frac{16419}{16}, 0, \frac{38155}{16}, \frac{21077}{16}, -\frac{357}{2}, -\frac{2855}{2}, -\frac{1379}{8}, -2775, \\
& \left. -565, \frac{2387}{8}, 0, -\frac{2775}{4}, \frac{3885}{16}, \frac{5439}{32} \right], \\
& \left[ 0, 0, 0, 0, 0, 0, 0, 0, 0, 0, \frac{565}{2}, 0, \frac{565}{4}, 0, 0, -\frac{2825}{2}, 0, 0, 0, 0, \frac{1471}{16}, 0, \frac{1471}{32}, 0, 0, \right. \\
& \left. -\frac{7355}{16}, \frac{119}{4}, \frac{555}{4}, \frac{1015}{16}, 0, \frac{555}{8}, -\frac{3983}{32}, 0, 0, -\frac{2775}{4}, -\frac{3885}{16} \right], \\
& \left[ 2260, \frac{1471}{2}, 238, -5670, \frac{777}{2}, 0, 0, -\frac{4413}{2}, 0, 0, -714, 0, -7850, -\frac{2331}{2}, 0, 0, 0, 0, \right. \\
& \left. 0, 0, 0, 0, -1471, 0, 0, 0, 0, 0, -476, 0, 0, -2220, -777, 0, 0 \right], \\
& \left[ -\frac{3955}{2}, \frac{25863}{16}, -\frac{833}{4}, \frac{22105}{4}, -\frac{59679}{16}, \frac{1471}{2}, 238, -\frac{2647}{16}, -\frac{2859}{4}, 0, \frac{2737}{4}, \right. \\
& -357, \frac{44405}{4}, -\frac{81089}{16}, -\frac{2331}{4}, 0, 0, -\frac{4413}{4}, 0, 0, -357, 0, \frac{3637}{4}, -\frac{8215}{4}, 0, 0, 0, 0, \\
& \left. 833, -476, 0, 3885, -\frac{3441}{4}, -777, 0 \right], \\
& \left[ 0, -\frac{3955}{2}, 2260, -8475, \frac{11865}{2}, -\frac{10297}{16}, \frac{2109}{4}, -\frac{25315}{8}, \frac{6363}{4}, 238, -\frac{6345}{2}, \right. \\
& \frac{4053}{4}, -\frac{30925}{2}, \frac{74935}{8}, \frac{16317}{16}, 0, 0, \frac{1471}{8}, 0, 0, -\frac{4175}{4}, 0, -3400, \frac{21371}{8}, 0, 0, \\
& \left. -357, 0, -2855, \frac{1001}{4}, 0, -5550, \frac{3885}{2}, \frac{5439}{4}, 0 \right], \\
& \left[ 0, 0, -\frac{3955}{2}, 0, -8475, 0, -\frac{10297}{16}, 0, -\frac{22065}{8}, -\frac{833}{4}, -\frac{1625}{4}, -\frac{19719}{16}, 0, \right. \\
& -\frac{30925}{2}, -\frac{11655}{8}, 0, 0, 0, 0, 0, \frac{1471}{8}, 0, 0, -\frac{7355}{2}, 0, 0, \frac{119}{2}, 0, \frac{555}{2}, -\frac{8743}{8}, 0, 0, \\
& \left. -5550, -\frac{3885}{2}, 0 \right], \\
& \left[ 5650, -\frac{8465}{4}, 595, \frac{1595}{2}, \frac{8405}{4}, \frac{7783}{8}, -\frac{833}{2}, \frac{148463}{16}, -\frac{56737}{8}, 0, -\frac{833}{4}, 119, \right. \\
& \left. -\frac{59255}{4}, \frac{256561}{16}, -\frac{17303}{4}, \frac{1471}{2}, 238, \frac{39771}{8}, -1818, 0, \frac{2499}{2}, -714, \frac{21161}{16}, \right.
\end{aligned}$$

$$\begin{aligned}
& \left[ \frac{30865}{8}, -\frac{5273}{2}, 0, 0, 0, -\frac{5831}{4}, 1666, -476, -\frac{27195}{4}, \frac{86247}{16}, \frac{999}{2}, -777 \right], \\
& \left[ 0, 5650, -\frac{3955}{2}, \frac{2825}{2}, -\frac{3955}{4}, -\frac{555}{4}, \frac{35383}{16}, -\frac{99665}{16}, \frac{228703}{32}, -\frac{833}{4}, 5110, \right. \\
& -\frac{61345}{16}, \frac{81875}{4}, -\frac{406165}{16}, \frac{247681}{32}, -\frac{10297}{16}, \frac{2109}{4}, -\frac{129637}{32}, \frac{14197}{8}, 238, \\
& \frac{32705}{16}, -\frac{61}{2}, \frac{3575}{2}, -\frac{211777}{32}, \frac{59059}{16}, 0, \frac{2499}{4}, -357, \frac{19985}{4}, -\frac{52687}{16}, \frac{1001}{4}, \\
& \left. \frac{19425}{2}, -\frac{71595}{8}, -\frac{6993}{16}, \frac{5439}{4} \right], \\
& \left[ 0, 0, 5650, 0, \frac{2825}{2}, 0, -\frac{555}{4}, 0, -\frac{128245}{16}, 595, \frac{7145}{4}, 1685, 0, \frac{81875}{4}, -\frac{176915}{16}, \right. \\
& 0, -\frac{10297}{16}, 0, -\frac{22065}{8}, -\frac{833}{4}, -\frac{41377}{32}, -\frac{16777}{16}, 0, \frac{18185}{8}, -\frac{41075}{8}, 0, -\frac{833}{8}, \\
& \left. \frac{119}{2}, -\frac{3885}{8}, \frac{70081}{32}, -\frac{8743}{8}, 0, \frac{19425}{2}, -\frac{17205}{8}, -\frac{3885}{2} \right], \\
& \left[ 0, 0, 0, 0, 0, 5650, -3955, 2825, -\frac{3955}{2}, 2260, -16950, 11865, -28250, 39550, \right. \\
& -\frac{27685}{2}, \frac{7355}{4}, -\frac{5537}{8}, \frac{29555}{8}, \frac{5243}{16}, 319, -\frac{28645}{4}, \frac{11893}{4}, -\frac{31225}{4}, \frac{99085}{8}, \\
& \left. -\frac{38759}{8}, 238, -675, 1638, -11300, \frac{28315}{4}, \frac{4655}{8}, -13875, \frac{58275}{4}, 0, -\frac{38073}{16} \right], \\
& \left[ 0, 0, 0, 0, 0, 0, 5650, 0, \frac{2825}{2}, -\frac{3955}{2}, \frac{2825}{2}, -\frac{37855}{4}, 0, -28250, 19775, 0, \frac{7355}{4}, \right. \\
& 0, \frac{7355}{16}, -\frac{777}{16}, \frac{51755}{16}, -\frac{62717}{32}, 0, -8500, \frac{106855}{16}, -\frac{833}{4}, -\frac{1645}{2}, -\frac{21385}{16}, \\
& \left. \frac{2775}{4}, -\frac{118085}{16}, \frac{14581}{32}, 0, -13875, \frac{19425}{4}, \frac{27195}{8} \right], \\
& \left[ 0, 0, 0, 0, 0, 0, 0, 0, 0, 5650, 0, 2825, 0, 0, -28250, 0, 0, 0, 0, \frac{7355}{4}, 0, \frac{7355}{8}, 0, 0, \right. \\
& \left. -\frac{36775}{4}, 595, 2775, \frac{5075}{4}, 0, \frac{2775}{2}, -\frac{19915}{8}, 0, 0, -13875, -\frac{19425}{4} \right], \\
& \left[ -\frac{791}{2}, -\frac{571}{2}, -136, \frac{3969}{4}, -222, 0, 0, \frac{1713}{2}, 0, 0, 408, 0, \frac{5495}{4}, 666, 0, 0, 0, 0, 0, 0, \right. \\
& \left. 0, 0, 571, 0, 0, 0, 0, 0, 272, 0, 0, \frac{777}{2}, 444, 0, 0 \right], \\
& \left[ 0, -\frac{791}{2}, 0, -\frac{791}{8}, \frac{2373}{4}, -\frac{571}{2}, -136, \frac{2621}{8}, \frac{825}{4}, 0, -34, 204, -\frac{11851}{16}, \frac{8215}{8}, \right. \\
& 333, 0, 0, \frac{1713}{4}, 0, 0, 204, 0, -\frac{833}{4}, 904, 0, 0, 0, 0, -238, 272, 0, -\frac{5439}{16}, 0, 444, 0 \left. \right], \\
& \left[ 0, 0, -\frac{791}{2}, 0, -\frac{791}{8}, 0, -\frac{571}{2}, 0, -\frac{571}{8}, -136, 399, -256, 0, -\frac{11851}{16}, -\frac{111}{2}, 0, 0, \right. \\
& \left. 0, 0, 0, \frac{1713}{4}, 0, 0, -\frac{3997}{8}, 0, 0, 204, 0, \frac{2331}{8}, 95, 0, 0, -\frac{5439}{16}, -\frac{777}{2}, 0 \right],
\end{aligned}$$

$$\begin{aligned}
& \left[ -\frac{2373}{4}, -\frac{1713}{4}, -204, \frac{11907}{8}, -333, 0, 0, \frac{5139}{4}, 0, 0, 612, 0, \frac{16485}{8}, 999, 0, 0, 0, 0, \right. \\
& 0, 0, 0, 0, \frac{1713}{2}, 0, 0, 0, 0, 0, 408, 0, 0, \frac{2331}{4}, 666, 0, 0 \Big], \\
& \left[ \frac{791}{8}, -\frac{4175}{8}, 34, \frac{7105}{16}, -\frac{1471}{2}, -\frac{1713}{4}, -204, \frac{20519}{8}, -904, 0, 136, -272, \right. \\
& -\frac{15057}{8}, 1020, -444, 0, 0, \frac{7423}{4}, 0, 0, 884, 0, -\frac{945}{4}, \frac{4599}{2}, 0, 0, 0, 0, -714, 408, 0, \\
& \left. -\frac{16317}{16}, -\frac{2331}{4}, 666, 0 \right], \\
& \left[ 0, \frac{791}{8}, -\frac{2373}{4}, -\frac{3955}{2}, \frac{5537}{4}, \frac{571}{8}, -\frac{1577}{4}, -\frac{37883}{16}, \frac{4219}{4}, -204, \frac{12795}{8}, \right. \\
& 143, 1995, -\frac{5013}{2}, 777, 0, 0, -\frac{2855}{4}, 0, 0, \frac{6063}{4}, 0, \frac{13245}{8}, -\frac{16431}{8}, 0, 0, 884, 0, \\
& \frac{18261}{8}, 729, 0, \frac{11655}{8}, \frac{10323}{16}, -\frac{2331}{2}, 0 \Big], \\
& \left[ 0, 0, \frac{791}{8}, 0, -\frac{3955}{2}, 0, \frac{571}{8}, 0, -\frac{2855}{2}, 34, -\frac{15043}{16}, -\frac{1249}{2}, 0, 1995, -1110, 0, 0, \right. \\
& 0, 0, 0, -\frac{2855}{4}, 0, 0, \frac{8565}{4}, 0, 0, -340, 0, -\frac{3885}{8}, 465, 0, 0, \frac{11655}{8}, 1665, 0 \Big], \\
& \left[ 0, 0, 0, 0, 0, -\frac{791}{2}, 0, -\frac{791}{4}, \frac{2373}{2}, 0, 0, 0, \frac{3955}{2}, -\frac{5537}{4}, 791, -\frac{571}{2}, -136, -337, \right. \\
& \frac{1269}{2}, 0, -68, 408, \frac{10643}{8}, -\frac{1055}{2}, 1237, 0, 0, 0, 680, -476, 272, \frac{3885}{4}, \frac{3441}{8}, \\
& \left. -\frac{777}{2}, 444 \right], \\
& \left[ 0, 0, 0, 0, 0, 0, -\frac{791}{2}, 0, -\frac{791}{8}, 0, -\frac{791}{8}, \frac{2373}{4}, 0, \frac{3955}{2}, -\frac{5537}{8}, 0, -\frac{571}{2}, 0, \right. \\
& -\frac{571}{8}, -136, -\frac{2125}{8}, \frac{689}{4}, 0, \frac{22063}{16}, -\frac{4441}{8}, 0, -34, 204, -\frac{777}{16}, \frac{7327}{8}, 95, 0, \\
& \frac{3885}{4}, \frac{12321}{16}, -\frac{777}{2} \Big], \\
& \left[ 0, -\frac{2373}{4}, 0, -\frac{3955}{4}, \frac{10283}{4}, -\frac{1713}{4}, -204, -\frac{14369}{8}, \frac{6091}{4}, 0, -340, 884, \right. \\
& -\frac{5467}{8}, \frac{15153}{8}, 1443, 0, 0, -571, 0, 0, -272, 0, -\frac{2125}{4}, \frac{825}{2}, 0, 0, 0, 0, -68, 408, 0, \\
& \left. -\frac{777}{8}, \frac{1887}{4}, 666, 0 \right], \\
& \left[ 0, \frac{791}{8}, 0, \frac{32431}{16}, -\frac{3955}{4}, -\frac{4175}{8}, 34, \frac{7629}{4}, \frac{2243}{2}, 0, 697, -340, \frac{42931}{32}, -1622, \right. \\
& \frac{1263}{2}, -\frac{1713}{4}, -204, -\frac{47}{8}, \frac{3807}{4}, 0, 136, 612, \frac{7105}{16}, -\frac{1091}{2}, \frac{3711}{2}, 0, 0, 0, 119, \\
& \left. -782, 408, \frac{5439}{32}, -\frac{14763}{16}, -\frac{2775}{4}, 666 \right],
\end{aligned}$$

$$\begin{aligned}
& \left[ 0, 0, 0, 0, 0, \frac{791}{8}, -\frac{2373}{4}, \frac{791}{16}, \frac{791}{2}, 0, -\frac{3955}{4}, \frac{10283}{4}, -\frac{3955}{8}, \frac{52997}{16}, \right. \\
& -\frac{16611}{8}, \frac{571}{8}, -\frac{1577}{4}, \frac{337}{4}, 341, -204, -\frac{7905}{8}, \frac{6635}{4}, -\frac{10643}{32}, \frac{41809}{16}, \\
& \left. -\frac{10215}{8}, 0, -340, 884, -\frac{5245}{8}, \frac{14773}{8}, 729, -\frac{3885}{16}, \frac{43179}{32}, \frac{13431}{16}, -\frac{2331}{2} \right], \\
& \left[ 0, 0, 0, 0, 0, 0, \frac{791}{8}, 0, -\frac{3955}{2}, 0, \frac{32431}{16}, -\frac{3955}{4}, 0, -\frac{3955}{8}, \frac{11865}{4}, 0, \frac{571}{8}, 0, \right. \\
& -\frac{2855}{2}, 34, \frac{6047}{4}, -\frac{5353}{4}, 0, -\frac{10625}{8}, \frac{4125}{4}, 0, 697, -340, \frac{31857}{32}, \frac{3857}{8}, 465, 0, \\
& \left. -\frac{3885}{16}, \frac{9435}{8}, 1665 \right], \\
& \left[ 0, 0, 0, 0, 0, 0, 0, 0, 0, -\frac{791}{2}, 0, -\frac{791}{4}, 0, 0, \frac{3955}{2}, 0, 0, 0, 0, -\frac{571}{2}, 0, -\frac{571}{4}, 0, 0, \right. \\
& \frac{2855}{2}, -136, -\frac{777}{4}, -290, 0, -\frac{777}{8}, 569, 0, 0, \frac{3885}{4}, 1110 \left. \right], \\
& \left[ 0, 0, -\frac{2373}{4}, 0, -\frac{3955}{4}, 0, -\frac{1713}{4}, 0, -\frac{2855}{4}, -204, -\frac{8659}{8}, -673, 0, -\frac{5467}{8}, \right. \\
& -555, 0, 0, 0, 0, 0, -571, 0, 0, -\frac{571}{4}, 0, 0, -272, 0, -\frac{777}{2}, -512, 0, 0, -\frac{777}{8}, -111, 0 \left. \right], \\
& \left[ 0, 0, \frac{791}{8}, 0, \frac{32431}{16}, 0, -\frac{4175}{8}, 0, \frac{7591}{16}, 34, \frac{22925}{16}, -\frac{77}{2}, 0, \frac{42931}{32}, 940, 0, \right. \\
& -\frac{1713}{4}, 0, -\frac{2855}{4}, -204, \frac{5663}{8}, -1244, 0, -\frac{3773}{16}, -\frac{2791}{4}, 0, 476, -272, \frac{5439}{8}, \\
& \left. \frac{1015}{2}, -512, 0, \frac{5439}{32}, \frac{777}{8}, -111 \right], \\
& \left[ 0, 0, 0, 0, 0, 0, \frac{791}{8}, 0, \frac{32431}{16}, -\frac{2373}{4}, -\frac{3955}{2}, \frac{791}{2}, 0, -\frac{3955}{8}, \frac{5537}{16}, 0, \frac{571}{8}, 0, \right. \\
& \frac{23411}{16}, -\frac{1577}{4}, -\frac{22063}{16}, 1038, 0, \frac{20437}{32}, \frac{22201}{16}, -204, -\frac{7771}{8}, -197, -\frac{3885}{4}, \\
& \left. -\frac{4343}{4}, 341, 0, -\frac{3885}{16}, -\frac{3441}{32}, \frac{777}{4} \right], \\
& \left[ 0, 0, 0, 0, 0, 0, 0, 0, 0, \frac{791}{8}, 0, \frac{791}{16}, 0, 0, -\frac{3955}{8}, 0, 0, 0, 0, \frac{571}{8}, 0, \frac{571}{16}, 0, 0, \right. \\
& -\frac{2855}{8}, 34, \frac{777}{16}, \frac{145}{2}, 0, \frac{777}{32}, -\frac{569}{4}, 0, 0, -\frac{3885}{16}, -\frac{555}{2} \left. \right], \\
& \left[ 791, 571, 272, -\frac{3969}{2}, 444, 0, 0, -1713, 0, 0, -816, 0, -\frac{5495}{2}, -1332, 0, 0, 0, 0, 0, 0, \right. \\
& 0, 0, -1142, 0, 0, 0, 0, 0, -544, 0, 0, -777, -888, 0, 0 \left. \right], \\
& \left[ -\frac{5537}{8}, \frac{2331}{8}, -238, \frac{30947}{16}, -1575, 571, 272, \frac{6749}{8}, -\frac{825}{2}, 0, 782, -408, \frac{62167}{16}, \right. \\
& \left. -\frac{3553}{4}, -666, 0, 0, -\frac{1713}{2}, 0, 0, -408, 0, \frac{5663}{4}, -1808, 0, 0, 0, 0, 952, -544, 0, \right.
\end{aligned}$$

$$\begin{aligned}
& \left[ \frac{5439}{4}, 777, -888, 0 \right], \\
& \left[ 0, -\frac{5537}{8}, 791, -\frac{11865}{4}, \frac{16611}{8}, -\frac{3997}{8}, 333, -\frac{36535}{16}, \frac{8883}{8}, 272, -1818, 1158, \right. \\
& -\frac{43295}{8}, \frac{33973}{16}, \frac{2331}{2}, 0, 0, \frac{571}{4}, 0, 0, -\frac{1577}{2}, 0, -\frac{22063}{8}, \frac{4219}{2}, 0, 0, -408, 0, \\
& \left. -\frac{7771}{4}, 286, 0, -\frac{3885}{2}, -\frac{3441}{4}, 1554, 0 \right], \\
& \left[ 0, 0, -\frac{5537}{8}, 0, -\frac{11865}{4}, 0, -\frac{3997}{8}, 0, -\frac{8565}{4}, -238, -\frac{2275}{16}, -\frac{2817}{2}, 0, -\frac{43295}{8}, \right. \\
& -1665, 0, 0, 0, 0, 0, \frac{571}{4}, 0, 0, -2855, 0, 0, 68, 0, \frac{777}{8}, -1249, 0, 0, -\frac{3885}{2}, -2220, 0 \left. \right], \\
& \left[ \frac{3955}{2}, \frac{173}{4}, 680, \frac{2233}{8}, \frac{3011}{2}, -\frac{833}{4}, -476, \frac{11893}{4}, -\frac{5729}{2}, 0, -238, 136, \right. \\
& -\frac{82957}{16}, \frac{21371}{4}, -1360, 571, 272, \frac{13545}{4}, -1269, 0, 1428, -816, -\frac{5831}{4}, \frac{10325}{2}, \\
& -2474, 0, 0, 0, -1666, 1904, -544, -\frac{38073}{16}, 0, 2331, -888 \left. \right], \\
& \left[ 0, \frac{3955}{2}, -\frac{5537}{8}, \frac{3955}{8}, -\frac{5537}{16}, \frac{5883}{8}, \frac{7771}{8}, -\frac{31747}{16}, \frac{50149}{16}, -238, \frac{30503}{16}, \right. \\
& -1694, \frac{114625}{16}, -\frac{278155}{32}, \frac{10297}{4}, -\frac{3997}{8}, 333, -2731, \frac{10025}{8}, 272, \frac{5987}{8}, \frac{739}{2}, \\
& \frac{107821}{32}, -\frac{113515}{16}, 3275, 0, 714, -408, \frac{54397}{16}, -\frac{9773}{4}, 286, \frac{27195}{8}, -\frac{6993}{16}, \\
& \left. -\frac{14319}{4}, 1554 \right], \\
& \left[ 0, 0, \frac{3955}{2}, 0, \frac{3955}{8}, 0, \frac{5883}{8}, 0, -\frac{20875}{8}, 680, \frac{10003}{16}, \frac{5911}{4}, 0, \frac{114625}{16}, \right. \\
& -\frac{7355}{2}, 0, -\frac{3997}{8}, 0, -\frac{8565}{4}, -238, -\frac{2359}{4}, -\frac{5063}{4}, 0, \frac{28315}{8}, -4520, 0, -119, 68, \\
& \left. -\frac{5439}{32}, \frac{18263}{8}, -1249, 0, \frac{27195}{8}, \frac{3885}{2}, -2220 \right], \\
& \left[ 0, 0, 0, 0, 0, \frac{3955}{2}, -\frac{5537}{4}, \frac{3955}{4}, -\frac{5537}{8}, 791, -\frac{11865}{2}, \frac{16611}{4}, -\frac{19775}{2}, \right. \\
& \frac{27685}{2}, -\frac{38759}{8}, \frac{2855}{2}, -\frac{1277}{4}, 1685, \frac{4883}{8}, 95, -\frac{36979}{8}, \frac{7931}{4}, -\frac{53215}{8}, \\
& \frac{163321}{16}, -\frac{31087}{8}, 272, -\frac{3303}{2}, 1872, -\frac{25255}{4}, \frac{27757}{8}, 665, -\frac{19425}{4}, \frac{4995}{4}, \\
& \left. \frac{86247}{16}, -\frac{5439}{2} \right], \\
& \left[ 0, 0, 0, 0, 0, 0, \frac{3955}{2}, 0, \frac{3955}{8}, -\frac{5537}{8}, \frac{3955}{8}, -\frac{52997}{16}, 0, -\frac{19775}{2}, \frac{27685}{4}, 0, \right. \\
& \frac{2855}{2}, 0, \frac{2855}{8}, \frac{1443}{8}, \frac{10625}{8}, -\frac{17777}{16}, 0, -\frac{110315}{16}, \frac{21095}{4}, -238, -\frac{2719}{16},
\end{aligned}$$



$$\begin{aligned}
& -\frac{3055}{2}, \frac{3885}{16}, -\frac{151979}{32}, \frac{2083}{4}, 0, -\frac{19425}{4}, -\frac{17205}{8}, 3885 \Big], \\
& \Big[ 0, 0, 0, 0, 0, 0, 0, 0, 0, \frac{3955}{2}, 0, \frac{3955}{4}, 0, 0, -\frac{19775}{2}, 0, 0, 0, 0, \frac{2855}{2}, 0, \frac{2855}{4}, 0, 0, \\
& -\frac{14275}{2}, 680, \frac{3885}{4}, 1450, 0, \frac{3885}{8}, -2845, 0, 0, -\frac{19425}{4}, -5550 \Big], \\
& \Big[ 405, \frac{567}{4}, 51, -1215, -\frac{111}{4}, 0, 0, -\frac{1701}{4}, 0, 0, -153, 0, -810, \frac{333}{4}, 0, 0, 0, 0, 0, 0, 0, \\
& 0, -\frac{567}{2}, 0, 0, 0, 0, 0, -102, 0, 0, 0, \frac{111}{2}, 0, 0 \Big], \\
& \Big[ 0, 405, 0, \frac{405}{4}, -\frac{1215}{2}, \frac{567}{4}, 51, -\frac{9153}{16}, -\frac{1923}{8}, 0, \frac{51}{4}, -\frac{153}{2}, \frac{2835}{4}, -\frac{13071}{16}, \\
& \frac{333}{8}, 0, 0, -\frac{1701}{8}, 0, 0, -\frac{153}{2}, 0, \frac{3969}{16}, -\frac{1935}{8}, 0, 0, 0, 0, \frac{357}{4}, -102, 0, 0, -\frac{777}{16}, \\
& \frac{111}{2}, 0 \Big], \\
& \Big[ 0, 0, 405, 0, \frac{405}{4}, 0, \frac{567}{4}, 0, \frac{567}{16}, 51, -\frac{1215}{2}, -15, 0, \frac{2835}{4}, -\frac{111}{16}, 0, 0, 0, 0, 0, \\
& -\frac{1701}{8}, 0, 0, \frac{3969}{16}, 0, 0, -\frac{153}{2}, 0, 0, \frac{1047}{8}, 0, 0, 0, -\frac{777}{16}, 0 \Big], \\
& \Big[ \frac{1215}{2}, \frac{1701}{8}, \frac{153}{2}, -\frac{3645}{2}, -\frac{333}{8}, 0, 0, -\frac{5103}{8}, 0, 0, -\frac{459}{2}, 0, -1215, \frac{999}{8}, 0, 0, \\
& 0, 0, 0, 0, 0, 0, -\frac{1701}{4}, 0, 0, 0, 0, 0, -153, 0, 0, 0, \frac{333}{4}, 0, 0 \Big], \\
& \Big[ -\frac{405}{4}, \frac{9153}{16}, -\frac{51}{4}, -405, \frac{13071}{16}, \frac{1701}{8}, \frac{153}{2}, -\frac{11097}{4}, \frac{1935}{8}, 0, -51, 102, \\
& \frac{8505}{4}, -\frac{4749}{4}, -\frac{111}{2}, 0, 0, -\frac{7371}{8}, 0, 0, -\frac{663}{2}, 0, \frac{11907}{16}, -\frac{1959}{8}, 0, 0, 0, 0, \\
& \frac{1071}{4}, -153, 0, 0, -\frac{2331}{16}, \frac{333}{4}, 0 \Big], \\
& \Big[ 0, -\frac{405}{4}, \frac{1215}{2}, 2025, -\frac{2835}{2}, -\frac{567}{16}, \frac{1599}{8}, \frac{6885}{4}, -\frac{7827}{16}, \frac{153}{2}, -\frac{4755}{2}, \\
& -\frac{1761}{8}, -\frac{6075}{2}, \frac{3975}{2}, \frac{777}{8}, 0, 0, \frac{2835}{8}, 0, 0, -\frac{6351}{8}, 0, -\frac{8505}{8}, \frac{10797}{16}, 0, 0, \\
& -\frac{663}{2}, 0, -\frac{765}{2}, \frac{3585}{8}, 0, 0, \frac{1665}{8}, -\frac{2331}{16}, 0 \Big], \\
& \Big[ 0, 0, -\frac{405}{4}, 0, 2025, 0, -\frac{567}{16}, 0, \frac{2835}{4}, -\frac{51}{4}, \frac{2025}{2}, \frac{4191}{16}, 0, -\frac{6075}{2}, -\frac{555}{4}, 0, \\
& 0, 0, 0, 0, \frac{2835}{8}, 0, 0, -\frac{8505}{8}, 0, 0, \frac{255}{2}, 0, 0, -\frac{3615}{8}, 0, 0, 0, \frac{1665}{8}, 0 \Big], \\
& \Big[ 0, 0, 0, 0, 0, 405, 0, \frac{405}{2}, -1215, 0, 0, 0, -2025, \frac{2835}{2}, -810, \frac{567}{4}, 51, \frac{567}{8}, -453, 0, \\
& \frac{51}{2}, -153, -\frac{2835}{4}, \frac{1929}{4}, -\frac{801}{4}, 0, 0, 0, -255, \frac{357}{2}, -102, 0, \frac{555}{4}, -\frac{777}{8}, \frac{111}{2} \Big],
\end{aligned}$$

$$\begin{aligned}
& \left[ 0, 0, 0, 0, 0, 0, 405, 0, \frac{405}{4}, 0, \frac{405}{4}, -\frac{1215}{2}, 0, -2025, \frac{2835}{4}, 0, \frac{567}{4}, 0, \frac{567}{16}, 51, \right. \\
& \left. \frac{567}{16}, -\frac{1821}{8}, 0, -\frac{2835}{4}, \frac{1929}{8}, 0, \frac{51}{4}, -\frac{153}{2}, 0, -\frac{4191}{16}, \frac{1047}{8}, 0, 0, \frac{555}{4}, -\frac{777}{16} \right], \\
& \left[ 0, \frac{1215}{2}, 0, \frac{2025}{2}, -\frac{5265}{2}, \frac{1701}{8}, \frac{153}{2}, \frac{9315}{8}, -963, 0, \frac{255}{2}, -\frac{663}{2}, \frac{405}{2}, \right. \\
& \left. -\frac{10275}{8}, \frac{1443}{8}, 0, 0, \frac{567}{2}, 0, 0, 102, 0, \frac{567}{8}, -\frac{1923}{4}, 0, 0, 0, 0, \frac{51}{2}, -153, 0, 0, \right. \\
& \left. -\frac{111}{8}, \frac{333}{4}, 0 \right], \\
& \left[ 0, -\frac{405}{4}, 0, -\frac{16605}{8}, \frac{2025}{2}, \frac{9153}{16}, -\frac{51}{4}, -\frac{36207}{32}, -\frac{23379}{16}, 0, -\frac{2091}{8}, \frac{255}{2}, \right. \\
& \left. -\frac{2835}{8}, \frac{79071}{32}, -\frac{10275}{8}, \frac{1701}{8}, \frac{153}{2}, -\frac{567}{4}, -\frac{1359}{2}, 0, -51, -\frac{459}{2}, -\frac{3969}{32}, \right. \\
& \left. \frac{13485}{16}, -\frac{2403}{8}, 0, 0, 0, -\frac{357}{8}, \frac{1173}{4}, -153, 0, \frac{777}{32}, -\frac{2553}{16}, \frac{333}{4} \right], \\
& \left[ 0, 0, 0, 0, 0, -\frac{405}{4}, \frac{1215}{2}, -\frac{405}{8}, -405, 0, \frac{2025}{2}, -\frac{5265}{2}, \frac{2025}{4}, -\frac{27135}{8}, \frac{8505}{4}, \right. \\
& \left. -\frac{567}{16}, \frac{1599}{8}, -\frac{567}{32}, -\frac{2157}{16}, \frac{153}{2}, 348, -1014, \frac{2835}{16}, -\frac{18939}{16}, \frac{12351}{16}, 0, \frac{255}{2}, \right. \\
& \left. -\frac{663}{2}, \frac{255}{4}, -\frac{993}{2}, \frac{3585}{8}, 0, -\frac{555}{16}, \frac{7437}{32}, -\frac{2331}{16} \right], \\
& \left[ 0, 0, 0, 0, 0, 0, -\frac{405}{4}, 0, 2025, 0, -\frac{16605}{8}, \frac{2025}{2}, 0, \frac{2025}{4}, -\frac{6075}{2}, 0, -\frac{567}{16}, 0, \right. \\
& \left. \frac{2835}{4}, -\frac{51}{4}, -\frac{23247}{32}, \frac{9861}{16}, 0, \frac{2835}{16}, -\frac{9615}{8}, 0, -\frac{2091}{8}, \frac{255}{2}, 0, \frac{6591}{32}, -\frac{3615}{8}, \right. \\
& \left. 0, 0, -\frac{555}{16}, \frac{1665}{8} \right], \\
& \left[ 0, 0, 0, 0, 0, 0, 0, 0, 0, 405, 0, \frac{405}{2}, 0, 0, -2025, 0, 0, 0, 0, \frac{567}{4}, 0, \frac{567}{8}, 0, 0, -\frac{2835}{4}, \right. \\
& \left. 51, 0, -\frac{9}{4}, 0, 0, -\frac{2151}{8}, 0, 0, 0, \frac{555}{4} \right], \\
& \left[ 0, 0, \frac{1215}{2}, 0, \frac{2025}{2}, 0, \frac{1701}{8}, 0, \frac{2835}{8}, \frac{153}{2}, 810, \frac{687}{8}, 0, \frac{405}{2}, -\frac{555}{8}, 0, 0, 0, 0, \right. \\
& \left. 0, \frac{567}{2}, 0, 0, \frac{567}{8}, 0, 0, 102, 0, 0, -30, 0, 0, 0, -\frac{111}{8}, 0 \right], \\
& \left[ 0, 0, -\frac{405}{4}, 0, -\frac{16605}{8}, 0, \frac{9153}{16}, 0, \frac{9153}{32}, -\frac{51}{4}, -\frac{2835}{2}, \frac{8889}{16}, 0, -\frac{2835}{8}, \right. \\
& \left. \frac{11031}{32}, 0, \frac{1701}{8}, 0, \frac{2835}{8}, \frac{153}{2}, -\frac{3969}{8}, \frac{2955}{8}, 0, -\frac{3969}{32}, \frac{3}{2}, 0, -\frac{357}{2}, 102, 0, \right. \\
& \left. \frac{105}{2}, -30, 0, 0, \frac{777}{32}, -\frac{111}{8} \right],
\end{aligned}$$

$$\left[ 0, 0, 0, 0, 0, 0, -\frac{405}{4}, 0, -\frac{16605}{8}, \frac{1215}{2}, 2025, -405, 0, \frac{2025}{4}, -\frac{2835}{8}, 0, -\frac{567}{16}, 0, -\frac{23247}{32}, \frac{1599}{8}, \frac{2835}{4}, -\frac{6339}{16}, 0, \frac{2835}{16}, \frac{291}{16}, \frac{153}{2}, 255, -\frac{741}{8}, 0, -75, -\frac{135}{8}, 0, 0, -\frac{555}{16}, \frac{777}{32} \right],$$

$$\left[ 0, 0, 0, 0, 0, 0, 0, 0, 0, -\frac{405}{4}, 0, -\frac{405}{8}, 0, 0, \frac{2025}{4}, 0, 0, 0, 0, -\frac{567}{16}, 0, -\frac{567}{32}, 0, 0, \frac{2835}{16}, -\frac{51}{4}, 0, \frac{9}{16}, 0, 0, \frac{2151}{32}, 0, 0, 0, -\frac{555}{16} \right],$$

$$\left[ -810, -\frac{567}{2}, -102, 2430, \frac{111}{2}, 0, 0, \frac{1701}{2}, 0, 0, 306, 0, 1620, -\frac{333}{2}, 0, 0, 0, 0, 0, 0, 0, 0, 567, 0, 0, 0, 0, 0, 204, 0, 0, 0, -111, 0, 0 \right],$$

$$\left[ \frac{2835}{4}, -\frac{8991}{16}, \frac{357}{4}, -\frac{9315}{4}, \frac{18663}{16}, -\frac{567}{2}, -102, \frac{6399}{16}, \frac{1923}{4}, 0, -\frac{1173}{4}, 153, -2835, \frac{28473}{16}, -\frac{333}{4}, 0, 0, \frac{1701}{4}, 0, 0, 153, 0, -\frac{3969}{4}, \frac{1935}{4}, 0, 0, 0, 0, -357, 204, 0, 0, \frac{777}{4}, -111, 0 \right],$$

$$\left[ 0, \frac{2835}{4}, -810, \frac{6075}{2}, -\frac{8505}{4}, \frac{3969}{16}, -\frac{777}{4}, \frac{6885}{8}, -\frac{3171}{4}, -102, \frac{3195}{2}, -\frac{849}{4}, 4050, -\frac{24345}{8}, \frac{2331}{16}, 0, 0, -\frac{567}{8}, 0, 0, \frac{1599}{4}, 0, \frac{2835}{2}, -\frac{7827}{8}, 0, 0, 153, 0, 510, -\frac{1761}{4}, 0, 0, -\frac{555}{2}, \frac{777}{4}, 0 \right],$$

$$\left[ 0, 0, \frac{2835}{4}, 0, \frac{6075}{2}, 0, \frac{3969}{16}, 0, \frac{8505}{8}, \frac{357}{4}, -\frac{405}{2}, \frac{5343}{16}, 0, 4050, -\frac{1665}{8}, 0, 0, 0, 0, 0, -\frac{567}{8}, 0, 0, \frac{2835}{2}, 0, 0, -\frac{51}{2}, 0, 0, \frac{4191}{8}, 0, 0, 0, -\frac{555}{2}, 0 \right],$$

$$\left[ -2025, \frac{2835}{4}, -255, \frac{2835}{4}, -\frac{1065}{4}, -\frac{2511}{8}, \frac{357}{2}, -\frac{64071}{16}, \frac{17529}{8}, 0, \frac{357}{4}, -51, \frac{19845}{4}, -\frac{91497}{16}, \frac{6591}{4}, -\frac{567}{2}, -102, -\frac{11907}{8}, 906, 0, -\frac{1071}{2}, 306, \frac{27783}{16}, -\frac{13545}{8}, \frac{801}{2}, 0, 0, 0, \frac{2499}{4}, -714, 204, 0, -\frac{5439}{16}, \frac{777}{2}, -111 \right],$$

$$\left[ 0, -2025, \frac{2835}{4}, -\frac{2025}{4}, \frac{2835}{8}, 0, -\frac{13071}{16}, \frac{51435}{16}, -\frac{66111}{32}, \frac{357}{4}, -2190, \frac{19377}{16}, -\frac{14175}{2}, \frac{144735}{16}, -\frac{91497}{32}, \frac{3969}{16}, -\frac{777}{4}, \frac{37989}{32}, -\frac{6909}{8}, -102, -\frac{5073}{16}, \frac{375}{2}, -\frac{19845}{8}, \frac{93489}{32}, -\frac{13323}{16}, 0, -\frac{1071}{4}, 153, -\frac{1785}{2}, \frac{20487}{16}, -\frac{1761}{4}, 0, \frac{3885}{8}, -\frac{9879}{16}, \frac{777}{4} \right],$$

$$\begin{aligned}
& \left[ 0, 0, -2025, 0, -\frac{2025}{4}, 0, 0, 0, \frac{45765}{16}, -255, \frac{2835}{8}, -\frac{255}{2}, 0, -\frac{14175}{2}, \frac{65355}{16}, 0, \right. \\
& \frac{3969}{16}, 0, \frac{8505}{8}, \frac{357}{4}, \frac{3969}{32}, \frac{4209}{16}, 0, -\frac{19845}{8}, \frac{9675}{8}, 0, \frac{357}{8}, -\frac{51}{2}, 0, -\frac{29337}{32}, \\
& \left. \frac{4191}{8}, 0, 0, \frac{3885}{8}, -\frac{555}{2} \right], \\
& \left[ 0, 0, 0, 0, 0, -2025, \frac{2835}{2}, -\frac{2025}{2}, \frac{2835}{4}, -810, 6075, -\frac{8505}{2}, 10125, -14175, \right. \\
& \frac{19845}{4}, -\frac{2835}{4}, \frac{1929}{8}, -\frac{2835}{8}, \frac{6189}{16}, -105, \frac{7995}{4}, -\frac{5985}{4}, \frac{14175}{4}, -\frac{39135}{8}, \\
& \left. \frac{13503}{8}, -102, 765, -480, 1275, -\frac{8805}{4}, \frac{7329}{8}, 0, -\frac{2775}{4}, \frac{3885}{4}, -\frac{5439}{16} \right], \\
& \left[ 0, 0, 0, 0, 0, 0, -2025, 0, -\frac{2025}{4}, \frac{2835}{4}, -\frac{2025}{4}, \frac{27135}{8}, 0, 10125, -\frac{14175}{2}, 0, \right. \\
& -\frac{2835}{4}, 0, -\frac{2835}{16}, -\frac{111}{16}, -\frac{2835}{16}, \frac{40389}{32}, 0, \frac{14175}{4}, -\frac{39135}{16}, \frac{357}{4}, -\frac{255}{4}, \\
& \left. \frac{6057}{16}, 0, \frac{20955}{16}, -\frac{35997}{32}, 0, 0, -\frac{2775}{4}, \frac{3885}{8} \right], \\
& \left[ 0, 0, 0, 0, 0, 0, 0, 0, 0, -2025, 0, -\frac{2025}{2}, 0, 0, 10125, 0, 0, 0, 0, -\frac{2835}{4}, 0, -\frac{2835}{8}, 0, \right. \\
& 0, \frac{14175}{4}, -255, 0, \frac{45}{4}, 0, 0, \frac{10755}{8}, 0, 0, 0, -\frac{2775}{4} \left. \right], \\
& \left[ -340, -230, -136, \frac{3969}{4}, \frac{333}{2}, 0, 0, 690, 0, 0, 408, 0, \frac{3053}{4}, -\frac{999}{2}, 0, 0, 0, 0, 0, 0, \right. \\
& 0, 460, 0, 0, 0, 0, 0, 272, 0, 0, \frac{111}{2}, -333, 0, 0 \left. \right], \\
& \left[ 0, -340, 0, -85, 510, -230, -136, \frac{1699}{4}, \frac{1023}{2}, 0, -34, 204, -\frac{9631}{16}, \frac{3053}{4}, -\frac{999}{4}, \right. \\
& 0, 0, 345, 0, 0, 204, 0, -\frac{2887}{8}, \frac{841}{4}, 0, 0, 0, 0, -238, 272, 0, -\frac{777}{16}, \frac{2775}{8}, -333, 0 \left. \right], \\
& \left[ 0, 0, -340, 0, -85, 0, -230, 0, -\frac{115}{2}, -136, \frac{1929}{4}, \frac{265}{2}, 0, -\frac{9631}{16}, \frac{333}{8}, 0, 0, 0, 0, \right. \\
& 0, 345, 0, 0, -\frac{805}{2}, 0, 0, 204, 0, \frac{333}{8}, -\frac{1951}{4}, 0, 0, -\frac{777}{16}, \frac{2331}{8}, 0 \left. \right], \\
& \left[ -510, -345, -204, \frac{11907}{8}, \frac{999}{4}, 0, 0, 1035, 0, 0, 612, 0, \frac{9159}{8}, -\frac{2997}{4}, 0, 0, 0, 0, 0, \right. \\
& 0, 0, 0, 690, 0, 0, 0, 0, 0, 408, 0, 0, \frac{333}{4}, -\frac{999}{2}, 0, 0 \left. \right], \\
& \left[ 85, -\frac{905}{2}, 34, \frac{5551}{16}, -\frac{5773}{8}, -345, -204, \frac{19187}{8}, -\frac{841}{4}, 0, 136, -272, -\frac{7029}{4}, \right. \\
& 798, 333, 0, 0, 1495, 0, 0, 884, 0, -\frac{8217}{8}, -\frac{1569}{4}, 0, 0, 0, 0, -714, 408, 0, -\frac{2331}{16}, \\
& \left. \frac{7659}{8}, -\frac{999}{2}, 0 \right],
\end{aligned}$$

$$\begin{aligned}
& \left[ 0, 85, -510, -1700, 1190, \frac{115}{2}, -311, -\frac{31889}{16}, \frac{6107}{8}, -204, \frac{11907}{8}, \frac{2903}{4}, \frac{9645}{4}, \right. \\
& -\frac{6843}{8}, -\frac{2331}{4}, 0, 0, -575, 0, 0, 1155, 0, \frac{13245}{8}, -\frac{3165}{4}, 0, 0, 884, 0, \frac{9603}{8}, \\
& \left. -\frac{7185}{4}, 0, \frac{1665}{8}, -\frac{22311}{16}, \frac{6993}{8}, 0 \right], \\
& \left[ 0, 0, 85, 0, -1700, 0, \frac{115}{2}, 0, -1150, 34, -\frac{13489}{16}, -\frac{5773}{8}, 0, \frac{9645}{4}, \frac{1665}{2}, 0, 0, 0, 0, \right. \\
& 0, -575, 0, 0, 1725, 0, 0, -340, 0, -\frac{555}{8}, \frac{5745}{4}, 0, 0, \frac{1665}{8}, -\frac{4995}{4}, 0 \left. \right], \\
& \left[ 0, 0, 0, 0, 0, -340, 0, -170, 1020, 0, 0, 0, 1700, -1190, 680, -230, -136, -\frac{571}{4}, \frac{1713}{2}, \right. \\
& 0, -68, 408, \frac{9089}{8}, -\frac{1277}{2}, -\frac{79}{2}, 0, 0, 0, 680, -476, 272, \frac{555}{4}, -\frac{7437}{8}, \frac{2553}{4}, -333 \\
& \left. \right], \\
& \left[ 0, 0, 0, 0, 0, 0, -340, 0, -85, 0, -85, 510, 0, 1700, -595, 0, -230, 0, -\frac{115}{2}, -136, \right. \\
& -\frac{341}{4}, \frac{955}{2}, 0, \frac{18289}{16}, -\frac{2887}{8}, 0, -34, 204, -\frac{111}{16}, \frac{3053}{4}, -\frac{1951}{4}, 0, \frac{555}{4}, \\
& \left. -\frac{14097}{16}, \frac{2331}{8} \right], \\
& \left[ 0, -510, 0, -850, 2210, -345, -204, -\frac{10373}{8}, \frac{6979}{4}, 0, -340, 884, -\frac{1915}{8}, \frac{12933}{8}, \right. \\
& -\frac{4329}{4}, 0, 0, -460, 0, 0, -272, 0, -\frac{341}{2}, 1023, 0, 0, 0, 0, -68, 408, 0, -\frac{111}{8}, \frac{333}{2}, \\
& \left. -\frac{999}{2}, 0 \right], \\
& \left[ 0, 85, 0, \frac{3485}{2}, -850, -\frac{905}{2}, 34, \frac{24411}{16}, \frac{7307}{8}, 0, 697, -340, \frac{14071}{32}, -\frac{46043}{16}, \right. \\
& \frac{5745}{4}, -345, -204, \frac{1507}{8}, \frac{5139}{4}, 0, 136, 612, 229, -\frac{10913}{8}, -\frac{237}{4}, 0, 0, 0, 119, \\
& \left. -782, 408, \frac{777}{32}, -\frac{1221}{4}, \frac{8325}{8}, -\frac{999}{2} \right], \\
& \left[ 0, 0, 0, 0, 0, 85, -510, \frac{85}{2}, 340, 0, -850, 2210, -425, \frac{5695}{2}, -1785, \frac{115}{2}, -311, \frac{571}{16}, \right. \\
& \frac{1507}{8}, -204, -\frac{4797}{8}, \frac{7523}{4}, -\frac{9089}{32}, \frac{30931}{16}, -1374, 0, -340, 884, -\frac{1915}{8}, \frac{13885}{8}, \\
& \left. -\frac{7185}{4}, -\frac{555}{16}, \frac{14097}{32}, -\frac{12321}{8}, \frac{6993}{8} \right], \\
& \left[ 0, 0, 0, 0, 0, 0, 85, 0, -1700, 0, \frac{3485}{2}, -850, 0, -425, 2550, 0, \frac{115}{2}, 0, -1150, 34, \right. \\
& \frac{18971}{16}, -\frac{10373}{8}, 0, -\frac{1705}{4}, \frac{5115}{2}, 0, 697, -340, \frac{4551}{32}, -\frac{17483}{16}, \frac{5745}{4}, 0, -\frac{555}{16},
\end{aligned}$$

$$\begin{aligned}
& \left[ \frac{1665}{4}, -\frac{4995}{4} \right], \\
& \left[ 0, 0, 0, 0, 0, 0, 0, 0, 0, -340, 0, -170, 0, 0, 1700, 0, 0, 0, 0, -230, 0, -115, 0, 0, 1150, \right. \\
& \left. -136, -\frac{111}{4}, \frac{197}{2}, 0, -\frac{111}{8}, \frac{3053}{4}, 0, 0, \frac{555}{4}, -\frac{1665}{2} \right], \\
& \left[ 0, 0, -510, 0, -850, 0, -345, 0, -575, -204, -\frac{5773}{8}, -\frac{361}{4}, 0, -\frac{1915}{8}, \frac{1665}{4}, 0, 0, 0, \right. \\
& \left. 0, 0, -460, 0, 0, -115, 0, 0, -272, 0, -\frac{111}{2}, 265, 0, 0, -\frac{111}{8}, \frac{333}{4}, 0 \right], \\
& \left[ 0, 0, 85, 0, \frac{3485}{2}, 0, -\frac{905}{2}, 0, \frac{1315}{4}, 34, \frac{19151}{16}, -\frac{197}{8}, 0, \frac{14071}{32}, -\frac{16373}{16}, 0, \right. \\
& \left. -345, 0, -575, -204, \frac{6107}{8}, -\frac{2201}{4}, 0, \frac{1055}{8}, \frac{1205}{4}, 0, 476, -272, \frac{777}{8}, -\frac{2077}{4}, \right. \\
& \left. 265, 0, \frac{777}{32}, -\frac{2553}{16}, \frac{333}{4} \right], \\
& \left[ 0, 0, 0, 0, 0, 0, 85, 0, \frac{3485}{2}, -510, -1700, 340, 0, -425, \frac{595}{2}, 0, \frac{115}{2}, 0, \frac{4715}{4}, -311, \right. \\
& \left. -\frac{18289}{16}, \frac{7083}{8}, 0, -\frac{4649}{32}, -\frac{10433}{16}, -204, -\frac{5773}{8}, \frac{1543}{4}, -\frac{555}{4}, \frac{2761}{4}, -\frac{95}{2}, 0, \right. \\
& \left. -\frac{555}{16}, \frac{7437}{32}, -\frac{2331}{16} \right], \\
& \left[ 0, 0, 0, 0, 0, 0, 0, 0, 0, 85, 0, \frac{85}{2}, 0, 0, -425, 0, 0, 0, 0, \frac{115}{2}, 0, \frac{115}{4}, 0, 0, -\frac{575}{2}, 34, \right. \\
& \left. \frac{111}{16}, -\frac{197}{8}, 0, \frac{111}{32}, -\frac{3053}{16}, 0, 0, -\frac{555}{16}, \frac{1665}{8} \right], \\
& \left[ 680, 460, 272, -\frac{3969}{2}, -333, 0, 0, -1380, 0, 0, -816, 0, -\frac{3053}{2}, 999, 0, 0, 0, 0, 0, 0, 0, \right. \\
& \left. 0, -920, 0, 0, 0, 0, 0, -544, 0, 0, -111, 666, 0, 0 \right], \\
& \left[ -595, \frac{555}{2}, -238, \frac{30503}{16}, -\frac{5829}{8}, 460, 272, 358, -1023, 0, 782, -408, \frac{40633}{16}, \right. \\
& \left. -\frac{19205}{8}, \frac{999}{2}, 0, 0, -690, 0, 0, -408, 0, \frac{6107}{4}, -\frac{841}{2}, 0, 0, 0, 0, 952, -544, 0, \frac{777}{4}, \right. \\
& \left. -\frac{2553}{2}, 666, 0 \right], \\
& \left[ 0, -595, 680, -2550, 1785, -\frac{805}{2}, 222, -\frac{25657}{16}, \frac{11991}{8}, 272, -\frac{3969}{2}, 381, \right. \\
& \left. -\frac{28865}{8}, \frac{60391}{16}, -\frac{6993}{8}, 0, 0, 115, 0, 0, -622, 0, -\frac{18289}{8}, \frac{6107}{4}, 0, 0, -408, 0, \right. \\
& \left. -\frac{5773}{4}, \frac{2903}{2}, 0, -\frac{555}{2}, \frac{7437}{4}, -\frac{2331}{2}, 0 \right], \\
& \left[ 0, 0, -595, 0, -2550, 0, -\frac{805}{2}, 0, -1725, -238, \frac{1943}{16}, -\frac{5829}{8}, 0, -\frac{28865}{8}, \frac{4995}{4}, 0, \right.
\end{aligned}$$

$$\begin{aligned}
& 0, 0, 0, 0, 115, 0, 0, -2300, 0, 0, 68, 0, \frac{111}{8}, -\frac{5773}{4}, 0, 0, -\frac{555}{2}, 1665, 0 \Big], \\
& \Big[ 1700, -40, 680, -\frac{1825}{4}, -\frac{985}{2}, -125, -476, \frac{24563}{8}, -\frac{4909}{4}, 0, -238, 136, \\
& -\frac{67417}{16}, \frac{40633}{8}, -\frac{3053}{2}, 460, 272, \frac{4941}{2}, -1713, 0, 1428, -816, -\frac{20209}{8}, \frac{5221}{4}, \\
& 79, 0, 0, 0, -1666, 1904, -544, -\frac{5439}{16}, \frac{19425}{8}, -2442, 666 \Big], \\
& \Big[ 0, 1700, -595, 425, -\frac{595}{2}, 555, \frac{1915}{2}, -\frac{9685}{4}, \frac{3685}{4}, -238, \frac{30503}{16}, -\frac{6781}{8}, \\
& \frac{95755}{16}, -\frac{249517}{32}, \frac{40411}{16}, -\frac{805}{2}, 222, -\frac{31597}{16}, \frac{12911}{8}, 272, 124, -241, \frac{121363}{32}, \\
& -\frac{7127}{2}, \frac{5221}{8}, 0, 714, -408, \frac{40411}{16}, -\frac{31867}{8}, \frac{2903}{2}, \frac{3885}{8}, -\frac{56499}{16}, \frac{31191}{8}, \\
& -\frac{2331}{2} \Big], \\
& \Big[ 0, 0, 1700, 0, 425, 0, 555, 0, -\frac{4525}{2}, 680, -\frac{635}{4}, -\frac{985}{2}, 0, \frac{95755}{16}, -\frac{28865}{8}, 0, \\
& -\frac{805}{2}, 0, -1725, -238, -\frac{3997}{16}, -\frac{4909}{8}, 0, \frac{30535}{8}, -\frac{4205}{4}, 0, -119, 68, -\frac{777}{32}, \\
& \frac{40633}{16}, -\frac{5773}{4}, 0, \frac{3885}{8}, -\frac{12765}{4}, 1665 \Big], \\
& \Big[ 0, 0, 0, 0, 0, 1700, -1190, 850, -595, 680, -5100, 3570, -8500, 11900, -4165, 1150, \\
& -125, \frac{2855}{4}, -1235, -16, -\frac{25657}{8}, \frac{11039}{4}, -\frac{45445}{8}, \frac{121363}{16}, -\frac{20209}{8}, 272, \\
& -\frac{3969}{2}, 1095, -\frac{15265}{4}, \frac{60391}{8}, -\frac{13657}{4}, -\frac{2775}{4}, \frac{20535}{4}, -\frac{98679}{16}, \frac{16317}{8} \Big], \\
& \Big[ 0, 0, 0, 0, 0, 0, 1700, 0, 425, -595, 425, -\frac{5695}{2}, 0, -8500, 5950, 0, 1150, 0, \frac{575}{2}, \frac{555}{2}, \\
& \frac{1705}{4}, -\frac{10355}{4}, 0, -\frac{91445}{16}, \frac{30535}{8}, -238, \frac{1943}{16}, -\frac{6781}{8}, \frac{555}{16}, -\frac{122897}{32}, \\
& \frac{60391}{16}, 0, -\frac{2775}{4}, \frac{37185}{8}, -\frac{11655}{4} \Big], \\
& \Big[ 0, 0, 0, 0, 0, 0, 0, 0, 0, 1700, 0, 850, 0, 0, -8500, 0, 0, 0, 0, 1150, 0, 575, 0, 0, -5750, 680, \\
& \frac{555}{4}, -\frac{985}{2}, 0, \frac{555}{8}, -\frac{15265}{4}, 0, 0, -\frac{2775}{4}, \frac{8325}{2} \Big], \\
& \Big[ -229, -119, -136, \frac{1041}{2}, 0, 0, 0, 357, 0, 0, 408, 0, \frac{1915}{2}, 0, 0, 0, 0, 0, 0, 0, 0, 238, 0, \\
& 0, 0, 0, 0, 272, 0, 0, 333, 0, 0, 0 \Big], \\
& \Big[ 0, -229, 0, -\frac{229}{4}, \frac{687}{2}, -119, -136, \frac{589}{4}, \frac{357}{2}, 0, -34, 204, -\frac{3539}{8}, \frac{2831}{4}, 0, 0, 0,
\end{aligned}$$

$$\begin{aligned}
& \left[ \frac{357}{2}, 0, 0, 204, 0, \frac{83}{2}, 238, 0, 0, 0, 0, -238, 272, 0, -\frac{2331}{8}, 333, 0, 0 \right], \\
& \left[ 0, 0, -229, 0, -\frac{229}{4}, 0, -119, 0, -\frac{119}{4}, -136, 177, -34, 0, -\frac{3539}{8}, 0, 0, 0, 0, 0, 0, \right. \\
& \left. \frac{357}{2}, 0, 0, -\frac{833}{4}, 0, 0, 204, 0, \frac{999}{4}, -238, 0, 0, -\frac{2331}{8}, 0, 0 \right], \\
& \left[ -\frac{687}{2}, -\frac{357}{2}, -204, \frac{3123}{4}, 0, 0, 0, \frac{1071}{2}, 0, 0, 612, 0, \frac{5745}{4}, 0, 0, 0, 0, 0, 0, 0, 0, \right. \\
& \left. 357, 0, 0, 0, 0, 0, 408, 0, 0, \frac{999}{2}, 0, 0, 0 \right], \\
& \left[ \frac{229}{4}, -\frac{1255}{4}, 34, \frac{2165}{8}, -458, -\frac{357}{2}, -204, \frac{5431}{4}, -238, 0, 136, -272, -\frac{4143}{4}, \right. \\
& \left. 354, 0, 0, 0, \frac{1547}{2}, 0, 0, 884, 0, \frac{915}{2}, 357, 0, 0, 0, 0, -714, 408, 0, -\frac{6993}{8}, \frac{999}{2}, 0, 0 \right], \\
& \left[ 0, \frac{229}{4}, -\frac{687}{2}, -1145, \frac{1603}{2}, \frac{119}{4}, -\frac{289}{2}, -\frac{9007}{8}, \frac{833}{2}, -204, \frac{2235}{4}, 476, 885, \right. \\
& \left. -\frac{1239}{2}, 0, 0, 0, -\frac{595}{2}, 0, 0, \frac{867}{2}, 0, \frac{1905}{4}, -\frac{2499}{4}, 0, 0, 884, 0, \frac{8409}{4}, -714, 0, \right. \\
& \left. \frac{4995}{4}, -\frac{6993}{8}, 0, 0 \right], \\
& \left[ 0, 0, \frac{229}{4}, 0, -1145, 0, \frac{119}{4}, 0, -595, 34, -\frac{4247}{8}, -680, 0, 885, 0, 0, 0, 0, 0, 0, -\frac{595}{2}, \right. \\
& \left. 0, 0, \frac{1785}{2}, 0, 0, -340, 0, -\frac{1665}{4}, 1020, 0, 0, \frac{4995}{4}, 0, 0 \right], \\
& \left[ 0, 0, 0, 0, 0, -229, 0, -\frac{229}{2}, 687, 0, 0, 0, 1145, -\frac{1603}{2}, 458, -119, -136, -226, 357, 0, \right. \\
& \left. -68, 408, \frac{2047}{4}, 83, 238, 0, 0, 0, 680, -476, 272, \frac{1665}{2}, -\frac{2331}{4}, 333, 0 \right], \\
& \left[ 0, 0, 0, 0, 0, 0, -229, 0, -\frac{229}{4}, 0, -\frac{229}{4}, \frac{687}{2}, 0, 1145, -\frac{1603}{4}, 0, -119, 0, -\frac{119}{4}, \right. \\
& \left. -136, -\frac{785}{4}, \frac{289}{2}, 0, \frac{4427}{8}, -\frac{833}{4}, 0, -34, 204, -\frac{333}{8}, \frac{3719}{4}, -238, 0, \frac{1665}{2}, \right. \\
& \left. -\frac{2331}{8}, 0 \right], \\
& \left[ 0, -\frac{687}{2}, 0, -\frac{1145}{2}, \frac{2977}{2}, -\frac{357}{2}, -204, -\frac{4021}{4}, \frac{1547}{2}, 0, -340, 884, -\frac{2123}{4}, \right. \\
& \left. \frac{7077}{4}, 0, 0, 0, -238, 0, 0, -272, 0, -\frac{785}{2}, 357, 0, 0, 0, 0, -68, 408, 0, -\frac{333}{4}, \frac{999}{2}, 0, 0 \right. \\
& \left. \right], \\
& \left[ 0, \frac{229}{4}, 0, \frac{9389}{8}, -\frac{1145}{2}, -\frac{1255}{4}, 34, \frac{1761}{2}, 733, 0, 697, -340, \frac{16859}{16}, -1733, \right. \\
& \left. 687, -\frac{357}{2}, -204, -\frac{523}{4}, \frac{1071}{2}, 0, 136, 612, \frac{2165}{8}, 65, 357, 0, 0, 0, 119, -782, 408, \right.
\end{aligned}$$



$$\begin{aligned}
& \left[ \frac{2331}{16}, -\frac{7659}{8}, \frac{999}{2}, 0 \right], \\
& \left[ 0, 0, 0, 0, 0, \frac{229}{4}, -\frac{687}{2}, \frac{229}{8}, 229, 0, -\frac{1145}{2}, \frac{2977}{2}, -\frac{1145}{4}, \frac{15343}{8}, -\frac{4809}{4}, \right. \\
& \frac{119}{4}, -\frac{289}{2}, \frac{113}{2}, 119, -204, -\frac{2121}{4}, \frac{1819}{2}, -\frac{2047}{16}, \frac{9305}{8}, -\frac{2499}{4}, 0, -340, 884, \\
& \left. -\frac{2345}{4}, \frac{8885}{4}, -714, -\frac{1665}{8}, \frac{22311}{16}, -\frac{6993}{8}, 0 \right], \\
& \left[ 0, 0, 0, 0, 0, 0, \frac{229}{4}, 0, -1145, 0, \frac{9389}{8}, -\frac{1145}{2}, 0, -\frac{1145}{4}, \frac{3435}{2}, 0, \frac{119}{4}, 0, -595, \right. \\
& 34, \frac{1303}{2}, -\frac{1955}{2}, 0, -\frac{3925}{4}, \frac{1785}{2}, 0, 697, -340, \frac{13653}{16}, -\frac{2345}{4}, 1020, 0, -\frac{1665}{8}, \\
& \left. \frac{4995}{4}, 0 \right], \\
& \left[ 0, 0, 0, 0, 0, 0, 0, 0, 0, -229, 0, -\frac{229}{2}, 0, 0, 1145, 0, 0, 0, 0, -119, 0, -\frac{119}{2}, 0, 0, 595, \right. \\
& \left. -136, -\frac{333}{2}, -68, 0, -\frac{333}{4}, 680, 0, 0, \frac{1665}{2}, 0 \right], \\
& \left[ 0, 0, -\frac{687}{2}, 0, -\frac{1145}{2}, 0, -\frac{357}{2}, 0, -\frac{595}{2}, -204, -\frac{2831}{4}, -340, 0, -\frac{2123}{4}, 0, 0, 0, \right. \\
& 0, 0, 0, -238, 0, 0, -\frac{119}{2}, 0, 0, -272, 0, -333, -68, 0, 0, -\frac{333}{4}, 0, 0 \left. \right], \\
& \left[ 0, 0, \frac{229}{4}, 0, \frac{9389}{8}, 0, -\frac{1255}{4}, 0, \frac{299}{8}, 34, \frac{6745}{8}, 239, 0, \frac{16859}{16}, -\frac{229}{2}, 0, -\frac{357}{2}, \right. \\
& 0, -\frac{595}{2}, -204, \frac{667}{4}, -578, 0, -\frac{2497}{8}, -\frac{119}{2}, 0, 476, -272, \frac{2331}{4}, -214, -68, 0, \\
& \left. \frac{2331}{16}, -\frac{333}{4}, 0 \right], \\
& \left[ 0, 0, 0, 0, 0, 0, \frac{229}{4}, 0, \frac{9389}{8}, -\frac{687}{2}, -1145, 229, 0, -\frac{1145}{4}, \frac{1603}{8}, 0, \frac{119}{4}, 0, \right. \\
& \frac{4879}{8}, -\frac{289}{2}, -\frac{4427}{8}, 816, 0, \frac{11273}{16}, \frac{833}{8}, -204, -\frac{3719}{4}, 136, -\frac{1665}{2}, -\frac{7}{2}, 119, \\
& \left. 0, -\frac{1665}{8}, \frac{2331}{16}, 0 \right], \\
& \left[ 0, 0, 0, 0, 0, 0, 0, 0, 0, \frac{229}{4}, 0, \frac{229}{8}, 0, 0, -\frac{1145}{4}, 0, 0, 0, 0, \frac{119}{4}, 0, \frac{119}{8}, 0, 0, \right. \\
& \left. -\frac{595}{4}, 34, \frac{333}{8}, 17, 0, \frac{333}{16}, -170, 0, 0, -\frac{1665}{8}, 0 \right], \\
& \left[ 458, 238, 272, -1041, 0, 0, 0, -714, 0, 0, -816, 0, -1915, 0, 0, 0, 0, 0, 0, 0, 0, -476, 0, \right. \\
& \left. 0, 0, 0, 0, -544, 0, 0, -666, 0, 0, 0 \right], \\
& \left[ -\frac{1603}{4}, \frac{999}{4}, -238, \frac{8203}{8}, -687, 238, 272, \frac{1321}{4}, -357, 0, 782, -408, \frac{20483}{8}, \right.
\end{aligned}$$

$$\begin{aligned}
& -\frac{2831}{2}, 0, 0, 0, -357, 0, 0, -408, 0, \frac{667}{2}, -476, 0, 0, 0, 0, 952, -544, 0, \frac{2331}{2}, -666, 0, \\
& 0], \\
& \left[ 0, -\frac{1603}{4}, 458, -\frac{3435}{2}, \frac{4809}{4}, -\frac{833}{4}, 0, -\frac{8555}{8}, \frac{2499}{4}, 272, -1374, 714, \right. \\
& -\frac{14155}{4}, \frac{19817}{8}, 0, 0, 0, \frac{119}{2}, 0, 0, -289, 0, -\frac{4427}{4}, 833, 0, 0, -408, 0, -\frac{3719}{2}, 952, \\
& 0, -1665, \frac{2331}{2}, 0, 0], \\
& \left[ 0, 0, -\frac{1603}{4}, 0, -\frac{3435}{2}, 0, -\frac{833}{4}, 0, -\frac{1785}{2}, -238, -\frac{1415}{8}, -1020, 0, -\frac{14155}{4}, 0, \right. \\
& 0, 0, 0, 0, 0, \frac{119}{2}, 0, 0, -1190, 0, 0, 68, 0, \frac{333}{4}, -1360, 0, 0, -1665, 0, 0], \\
& \left[ 1145, -\frac{413}{2}, 680, \frac{1727}{4}, 229, \frac{83}{2}, -476, \frac{3227}{2}, -1255, 0, -238, 136, -\frac{24773}{8}, \right. \\
& \frac{6745}{2}, -916, 238, 272, \frac{3165}{2}, -714, 0, 1428, -816, \frac{581}{2}, 667, -476, 0, 0, 0, -1666, \\
& 1904, -544, -\frac{16317}{8}, 2331, -666, 0], \\
& \left[ 0, 1145, -\frac{1603}{4}, \frac{1145}{4}, -\frac{1603}{8}, \frac{777}{4}, \frac{3719}{4}, -\frac{7493}{8}, \frac{9701}{8}, -238, \frac{8647}{8}, -806, \right. \\
& \frac{33725}{8}, -\frac{83855}{16}, 1603, -\frac{833}{4}, 0, -1288, \frac{2737}{4}, 272, -\frac{725}{4}, 425, \frac{11009}{16}, -\frac{13523}{8}, \\
& 833, 0, 714, -408, \frac{26033}{8}, -\frac{7051}{2}, 952, \frac{11655}{4}, -\frac{29637}{8}, \frac{2331}{2}, 0], \\
& \left[ 0, 0, 1145, 0, \frac{1145}{4}, 0, \frac{777}{4}, 0, -\frac{6275}{4}, 680, \frac{5057}{8}, \frac{569}{2}, 0, \frac{33725}{8}, -2290, 0, \right. \\
& -\frac{833}{4}, 0, -\frac{1785}{2}, -238, -\frac{791}{2}, -\frac{1921}{2}, 0, \frac{3335}{4}, -1190, 0, -119, 68, -\frac{2331}{16}, \\
& \frac{9853}{4}, -1360, 0, \frac{11655}{4}, -1665, 0], \\
& \left[ 0, 0, 0, 0, 0, 1145, -\frac{1603}{2}, \frac{1145}{2}, -\frac{1603}{4}, 458, -3435, \frac{4809}{2}, -5725, 8015, \right. \\
& -\frac{11221}{4}, 595, \frac{527}{2}, 1130, -\frac{833}{4}, -238, -\frac{8111}{4}, \frac{2023}{2}, -\frac{10235}{4}, \frac{30989}{8}, -\frac{5831}{4}, \\
& 272, -1707, 1428, -\frac{11795}{2}, \frac{26033}{4}, -1666, -\frac{8325}{2}, \frac{11655}{2}, -\frac{16317}{8}, 0], \\
& \left[ 0, 0, 0, 0, 0, 1145, 0, \frac{1145}{4}, -\frac{1603}{4}, \frac{1145}{4}, -\frac{15343}{8}, 0, -5725, \frac{8015}{2}, 0, 595, 0, \right. \\
& \frac{595}{4}, \frac{1887}{4}, \frac{3925}{4}, -\frac{6613}{8}, 0, -\frac{22135}{8}, \frac{4165}{2}, -238, -\frac{971}{8}, -1139, \frac{1665}{8}, \\
& -\frac{76711}{16}, 2380, 0, -\frac{8325}{2}, \frac{11655}{4}, 0],
\end{aligned}$$

$$\left[ 0, 0, 0, 0, 0, 0, 0, 0, 0, 1145, 0, \frac{1145}{2}, 0, 0, -5725, 0, 0, 0, 0, 595, 0, \frac{595}{2}, 0, 0, -2975, 680, \frac{1665}{2}, 340, 0, \frac{1665}{4}, -3400, 0, 0, -\frac{8325}{2}, 0 \right]$$

**J2** > Rank(MEQa)

35

(36)

Hurrah! Hurrah! Hurrah!

P.S. Notice that the calculation of the rank over Q is an exact operation in Maple (no round-offs), so our calculation, even though computer assisted, is mathematically rigorous.

Thus we conclude: integrability of PDE in Hirota form = EW property of its linearization.
