# Supplementary material for: Dispersionless integrable systems in 3D and Einstein-Weyl geometry
Source: arXiv:1208.2728 ancillary file (2013-05-09)
Supplement: Supplementary file 7 [file BKEF-2012-III-Hirota_form_linearization.pdf]

This is the worksheet accompanying the paper E.Ferapontov & B.Kruglikov "Dispersionless integrable systems in 3D and Einstein-Weyl geometry".

The file ran on *Maple* version 16, the package **DifferentialGeometry** was used.

```
> with(DifferentialGeometry):with(Tensor):with(Tools):with
(JetCalculus):with(LinearAlgebra):
```

```
E > # Proof that in 3D conformal flatness of the linearization metric of a Hirota type equation
      implies Monge-Ampere condition
      (and consequently is equivalent to linearization)
```

```
E >
```

```
E > DGsetup([x, y, z], [u], E, 5)
```

frame name: E

(1)

```
E > EQ := u3,3 - F(u1,1, u1,2, u1,3, u2,2, u2,3)
```

$$EQ := u_{3,3} - F(u_{1,1}, u_{1,2}, u_{1,3}, u_{2,2}, u_{2,3})$$

(2)

```
M > BB := Matrix([ [ diff(EQ, u[1,1]), 1/2 * diff(EQ, u[1,2]), 1/2 * diff(EQ, u[1,3]) ], [ 1/2
      * diff(EQ, u[1,2]), diff(EQ, u[2,2]), 1/2 * diff(EQ, u[2,3]) ], [ 1/2 * diff(EQ, u[1,3]),
      1/2 * diff(EQ, u[2,3]), diff(EQ, u[3,3]) ] ] ] )
```

$$BB := \left[ \left[ - \left( \frac{\partial}{\partial u_{1,1}} F(u_{1,1}, u_{1,2}, u_{1,3}, u_{2,2}, u_{2,3}) \right), - \frac{1}{2} \frac{\partial}{\partial u_{1,2}} F(u_{1,1}, u_{1,2}, u_{1,3}, u_{2,2}, u_{2,3}), \right. \right. \\ \left. \left. - \frac{1}{2} \frac{\partial}{\partial u_{1,3}} F(u_{1,1}, u_{1,2}, u_{1,3}, u_{2,2}, u_{2,3}) \right], \right.$$

(3)

$$\left[ - \frac{1}{2} \frac{\partial}{\partial u_{1,2}} F(u_{1,1}, u_{1,2}, u_{1,3}, u_{2,2}, u_{2,3}), - \left( \frac{\partial}{\partial u_{2,2}} F(u_{1,1}, u_{1,2}, u_{1,3}, u_{2,2}, u_{2,3}) \right), \right. \\ \left. - \frac{1}{2} \frac{\partial}{\partial u_{2,3}} F(u_{1,1}, u_{1,2}, u_{1,3}, u_{2,2}, u_{2,3}) \right],$$

$$\left[ - \frac{1}{2} \frac{\partial}{\partial u_{1,3}} F(u_{1,1}, u_{1,2}, u_{1,3}, u_{2,2}, u_{2,3}), - \frac{1}{2} \frac{\partial}{\partial u_{2,3}} F(u_{1,1}, u_{1,2}, u_{1,3}, u_{2,2}, u_{2,3}), 1 \right] \Bigg]$$

```
M > B := Adjoint(BB) :
```

```
E > dB := Determinant(BB) :
```

```
E > Bg := dB-1 · B :
```

```
E > simplify(Multiply(Bg, BB))
```

$$\begin{bmatrix} 1 & 0 & 0 \\ 0 & 1 & 0 \\ 0 & 0 & 1 \end{bmatrix}$$

(4)

```
> # Here I define the dual metric BB (with upper indices), the metric Bg
      and the adjoint matrix B (of linearization)
```

```

>
E > smbl5 := Z→add(add(add(add(add(diff(Z, u[k, l, p, q, r])·u[k, l, p, q, r], r=q..3), q=p
..3), p=l..3), l=k..3), k=1..3) :
E > smbl5(u[1]·u[1, 2, 3] + u[2]·u[1, 2, 2, 3]2 + u[3]·u[1, 1, 2, 3, 3])
u3 u1, 1, 2, 3, 3 (5)

```

```

M > G1 := (i, j, s) → -add(add(add(add(Bg[i, a]·diff(BB[a, b], u[p, q])·TotalDiff(u[p,
q], s)·Bg[b, j], q=p..3), p=1..3), b=1..3), a=1..3) :
E > G2 := (i, j, s, t) → -add(add(add(add(Bg[i, a]·diff(BB[a, b], u[p, q])·TotalDiff(u[p,
q], [s, t])·Bg[b, j], q=p..3), p=1..3), b=1..3), a=1..3) :
E > G3 := (i, j, s, t, m) → -add(add(add(add(Bg[i, a]·diff(BB[a, b], u[p, q])
·TotalDiff(u[p, q], [s, t, m])·Bg[b, j], q=p..3), p=1..3), b=1..3), a=1..3) :
E > Ric := (i, j) →  $\frac{1}{2}$ ·add(add(BB[k, l]·(G2(i, j, k, l) + G2(k, l, i, j) - G2(i, k, j, l) - G2(j,
l, i, k)), l=1..3), k=1..3) :
E > Ric2 := (i, j, m) →  $\frac{1}{2}$ ·add(add(BB[k, l]·(G3(i, j, k, l, m) + G3(k, l, i, j, m) - G3(i, k, j, l,
m) - G3(j, l, i, k, m)), l=1..3), k=1..3) :
E > Sc := add(add(BB[i, j]·Ric(i, j), j=1..3), i=1..3) :
E > Sc2 := k→add(add(BB[i, j]·Ric2(i, j, k), j=1..3), i=1..3) :
E > Cot := (i, j, p) → smbl5(Ric2(i, j, p) - Ric2(i, p, j) -  $\frac{1}{4}$ Bg[i, j]·Sc2(p) +  $\frac{1}{4}$ Bg[i, p]
·Sc2(j)) :
> # Here I define the symbol of the Cotton tensor - it has order 3 in the entries of the metric,
so order 5 in the function F

```

```

>
M > DE := DifferentialEquationData([EQ], [u[3, 3]]) :
M > DE3 := Prolong(DE, 3) :
M > alpha := Transformation(DE3) :
E >
E > with(PDEtools) : declare(F(u1, 1, u1, 2, u2, 2, u1, 3, u2, 3)) :
F(u1, 1, u1, 2, u2, 2, u1, 3, u2, 3) will now be displayed as F (6)

```

```

E > simplify(Pullback(alpha, u[1, 3, 3]))
Fu1, 1 u1, 1, 1 + Fu1, 2 u1, 1, 2 + Fu1, 3 u1, 1, 3 + Fu2, 2 u1, 2, 2 + Fu2, 3 u1, 2, 3 (7)

```

```

E > Sub := {Fu1, 1 = fr, Fu1, 2 = fs, Fu2, 2 = fr, Fu1, 3 = fa, Fu2, 3 = fb, Fu1, 1, u1, 1 = frr, Fu1, 1, u1, 2 = frs,
Fu1, 1, u2, 2 = frr, Fu1, 2, u1, 2 = fss, Fu1, 2, u2, 2 = fsr, Fu2, 2, u2, 2 = ftt, Fu1, 1, u1, 3 = far, Fu1, 2, u1, 3
= fas, Fu1, 3, u2, 2 = far, Fu1, 1, u2, 3 = fbr, Fu1, 2, u2, 3 = fbs, Fu2, 2, u2, 3 = fbr, Fu1, 3, u1, 3 = faa,
Fu1, 3, u2, 3 = fab, Fu2, 3, u2, 3 = fbb} :

```

```

> # Here I make setup for substitution of F instead of uii and simplifying the notations

```

**for patial derivatives** ( $r = u_{xx}$ ,  $s = u_{xy}$ ,  $t = u_{yy}$ ,  $a = u_{tx}$ ,  $b = u_{ty}$ ).

What is done below is the following :

we evaluate via the above substitution the components of the symbol of the Cotton tensor, they will yield Monge-Ampere conditions.

**E >**

**E >**  $Res112 := simplify(smb15(dB \cdot Pullback(alpha, Cot(1, 1, 2)))) :$

**E >**  $Res112a := factor([diff(Res112, u[1, 1, 1, 1, 1]), \blacklozenge, diff(Res112, u[1, 1, 1, 1, 2]), \blacklozenge, diff(Res112, u[1, 1, 1, 2, 2]), \blacklozenge, diff(Res112, u[1, 1, 2, 2, 2]), \blacklozenge, diff(Res112, u[2, 2, 2, 2, 2])])$

$$\begin{aligned}
 Res112a := & \left[ \frac{1}{16} F_{u_{2,3}} F_{u_{1,3}} F_{u_{1,1}'} u_{1,1} - \frac{1}{8} F_{u_{2,3}} F_{u_{1,1}} F_{u_{1,1}'} u_{1,3} - \frac{1}{16} F_{u_{1,3}}^2 F_{u_{1,1}'} u_{1,2} \right. \\
 & - \frac{1}{4} F_{u_{1,3}'} u_{2,3} F_{u_{1,1}}^2 - \frac{1}{16} F_{u_{1,3}}^2 F_{u_{1,1}} F_{u_{1,3}'} u_{2,3} - \frac{1}{4} F_{u_{1,1}} F_{u_{1,1}'} u_{1,2} \\
 & + \frac{1}{8} F_{u_{1,2}} F_{u_{1,1}'} u_{1,1} + \frac{1}{16} F_{u_{1,2}} F_{u_{1,3}} F_{u_{1,1}'} u_{1,3}, \blacklozenge, \frac{1}{16} F_{u_{2,3}}^2 F_{u_{1,1}'} u_{1,1} \\
 & + \frac{1}{4} F_{u_{2,2}} F_{u_{1,1}'} u_{1,1} - \frac{1}{2} F_{u_{1,1}} F_{u_{1,1}'} u_{2,2} - \frac{1}{8} F_{u_{1,3}} F_{u_{2,3}} F_{u_{1,1}} F_{u_{1,3}'} u_{2,3} \\
 & - \frac{1}{8} F_{u_{1,2}'} u_{1,3} F_{u_{2,3}} F_{u_{1,1}} - \frac{1}{16} F_{u_{1,2}} F_{u_{2,3}} F_{u_{1,1}'} u_{1,3} + \frac{1}{16} F_{u_{1,1}'} u_{2,3} F_{u_{1,3}} F_{u_{1,2}} \\
 & - \frac{1}{2} F_{u_{1,1}} F_{u_{1,3}'} u_{2,3} F_{u_{1,2}} - \frac{1}{16} F_{u_{1,3}}^2 F_{u_{1,2}'} u_{1,2} - \frac{1}{8} F_{u_{1,3}}^2 F_{u_{1,1}'} u_{2,2} \\
 & - \frac{1}{4} F_{u_{1,2}'} u_{1,2} F_{u_{1,1}} - \frac{1}{8} F_{u_{2,3}} F_{u_{1,1}} F_{u_{1,1}'} u_{2,3} - \frac{1}{4} F_{u_{2,3}'} u_{2,3} F_{u_{1,1}}^2 - \frac{1}{16} \\
 & F_{u_{1,3}}^2 F_{u_{1,2}} F_{u_{1,3}'} u_{2,3} - \frac{1}{16} F_{u_{1,3}}^2 F_{u_{2,3}'} u_{2,3} F_{u_{1,1}} + \frac{1}{16} F_{u_{1,3}} F_{u_{1,2}} F_{u_{1,2}'} u_{1,3} \\
 & + \frac{1}{8} F_{u_{2,2}} F_{u_{1,3}} F_{u_{1,1}'} u_{1,3}, \blacklozenge, -\frac{1}{8} F_{u_{1,2}} F_{u_{1,2}'} u_{1,2} - \frac{1}{2} F_{u_{1,1}} F_{u_{1,3}'} u_{2,3} F_{u_{2,2}} \\
 & + \frac{1}{8} F_{u_{1,1}'} u_{2,3} F_{u_{1,3}} F_{u_{2,2}} - \frac{1}{16} F_{u_{1,3}'} u_{2,3} F_{u_{2,3}}^2 F_{u_{1,1}} - \frac{1}{8} F_{u_{1,3}'} u_{2,2} F_{u_{2,3}} F_{u_{1,1}} \\
 & - \frac{1}{8} F_{u_{1,3}} F_{u_{2,3}} F_{u_{1,1}'} u_{2,2} - \frac{1}{16} F_{u_{1,3}}^2 F_{u_{2,3}'} u_{2,3} F_{u_{1,2}} - \frac{1}{8} F_{u_{1,3}} F_{u_{2,3}} F_{u_{1,1}} F_{u_{2,3}'} u_{2,3} \\
 & - \frac{1}{16} F_{u_{1,1}'} u_{2,3} F_{u_{2,3}} F_{u_{1,2}} - \frac{1}{2} F_{u_{1,1}} F_{u_{2,3}'} u_{2,3} F_{u_{1,2}} + \frac{1}{16} F_{u_{2,3}}^2 F_{u_{1,1}'} u_{1,2} - \frac{3}{16} \\
 & F_{u_{1,3}}^2 F_{u_{1,2}'} u_{2,2} - \frac{1}{4} F_{u_{1,2}} F_{u_{1,1}'} u_{2,2} - \frac{3}{4} F_{u_{1,2}'} u_{2,2} F_{u_{1,1}} + \frac{1}{4} F_{u_{2,2}} F_{u_{1,1}'} u_{1,2} \\
 & - \frac{1}{8} F_{u_{1,3}} F_{u_{2,3}} F_{u_{1,2}} F_{u_{1,3}'} u_{2,3} - \frac{1}{4} F_{u_{1,3}'} u_{2,3} F_{u_{1,2}}^2 - \frac{1}{16} F_{u_{1,2}'} u_{1,3} F_{u_{2,3}} F_{u_{1,2}} \\
 & + \frac{1}{16} F_{u_{1,3}} F_{u_{1,2}'} u_{2,3} F_{u_{1,2}} - \frac{1}{16} F_{u_{1,3}} F_{u_{2,3}} F_{u_{1,2}'} u_{1,2} - \frac{1}{16} F_{u_{1,3}}^2 F_{u_{2,2}} F_{u_{1,3}'} u_{2,3}
 \end{aligned} \tag{8}$$

$$\begin{aligned}
& + \frac{1}{16} F_{u_{1,3}} F_{u_{1,2}} F_{u_{1,3},u_{2,2}} + \frac{1}{8} F_{u_{1,3}} F_{u_{2,2}} F_{u_{1,2},u_{1,3}} - \frac{1}{8} F_{u_{2,3}} F_{u_{1,1}} F_{u_{1,2},u_{2,3}}, \blacklozenge, \\
& - \frac{1}{2} F_{u_{1,2}} F_{u_{1,3},u_{2,3}} F_{u_{2,2}} - \frac{1}{16} F_{u_{1,3},u_{2,3}} F_{u_{2,3}}^2 F_{u_{1,2}} - \frac{1}{16} F_{u_{1,3},u_{2,2}} F_{u_{2,3}} F_{u_{1,2}} \\
& + \frac{1}{16} F_{u_{1,3}} F_{u_{2,2},u_{2,3}} F_{u_{1,2}} - \frac{1}{16} F_{u_{1,3}}^2 F_{u_{2,3},u_{2,3}} F_{u_{2,2}} - \frac{1}{8} F_{u_{1,3}} F_{u_{2,3}} F_{u_{1,2}} F_{u_{2,3},u_{2,3}} \\
& - \frac{1}{2} F_{u_{1,1}} F_{u_{2,3},u_{2,3}} F_{u_{2,2}} - \frac{1}{8} F_{u_{1,3}}^2 F_{u_{2,2},u_{2,2}} - \frac{1}{2} F_{u_{2,2},u_{2,2}} F_{u_{1,1}} \\
& - \frac{1}{2} F_{u_{1,2}} F_{u_{1,2},u_{2,2}} - \frac{1}{4} F_{u_{2,3},u_{2,3}} F_{u_{1,2}}^2 - \frac{1}{8} F_{u_{1,3}} F_{u_{2,3}} F_{u_{2,2}} F_{u_{1,3},u_{2,3}} \\
& + \frac{1}{8} F_{u_{1,3}} F_{u_{1,2},u_{2,3}} F_{u_{2,2}} - \frac{1}{4} F_{u_{1,3}} F_{u_{2,3}} F_{u_{1,2},u_{2,2}} - \frac{1}{16} F_{u_{2,3}}^2 F_{u_{1,1}} F_{u_{2,3},u_{2,3}} \\
& - \frac{1}{8} F_{u_{2,3}} F_{u_{1,1}} F_{u_{2,2},u_{2,3}} + \frac{1}{8} F_{u_{1,3}} F_{u_{2,2}} F_{u_{1,3},u_{2,2}} - \frac{1}{16} F_{u_{2,3}} F_{u_{1,2}} F_{u_{1,2},u_{2,3}}, \blacklozenge, \\
& - \frac{1}{4} F_{u_{2,2}} F_{u_{1,2},u_{2,2}} - \frac{1}{16} F_{u_{1,3},u_{2,3}} F_{u_{2,3}}^2 F_{u_{2,2}} + \frac{1}{8} F_{u_{1,3}} F_{u_{2,2},u_{2,3}} F_{u_{2,2}} \\
& - \frac{3}{16} F_{u_{1,3}} F_{u_{2,3}} F_{u_{2,2},u_{2,2}} - \frac{1}{8} F_{u_{1,3}} F_{u_{2,3}} F_{u_{2,2}} F_{u_{2,3},u_{2,3}} - \frac{1}{2} F_{u_{1,2}} F_{u_{2,3},u_{2,3}} F_{u_{2,2}} \\
& - \frac{1}{16} F_{u_{2,3}}^2 F_{u_{1,2},u_{2,2}} - \frac{3}{8} F_{u_{1,2}} F_{u_{2,2},u_{2,2}} - \frac{1}{16} F_{u_{2,3}}^2 F_{u_{1,2}} F_{u_{2,3},u_{2,3}} - \frac{1}{4} F_{u_{1,3},u_{2,3}} \\
& F_{u_{2,2}}^2 - \frac{1}{16} F_{u_{2,3}} F_{u_{1,2}} F_{u_{2,2},u_{2,3}}, \blacklozenge, - \frac{1}{16} \left( 4 F_{u_{2,2}} + F_{u_{2,3}}^2 \right) \left( F_{u_{2,2},u_{2,2}} \right. \\
& \left. + F_{u_{2,2}} F_{u_{2,3},u_{2,3}} \right) \Big]
\end{aligned}$$

**E** > *Res112b* := factor([diff(*Res112*, u[1, 1, 1, 1, 3]),  $\blacklozenge$ , diff(*Res112*, u[1, 1, 1, 2, 3]),  $\blacklozenge$ ,  
diff(*Res112*, u[1, 1, 2, 2, 3]),  $\blacklozenge$ , diff(*Res112*, u[1, 2, 2, 2, 3]),  $\blacklozenge$ , diff(*Res112*, u[2,  
2, 2, 2, 3]))]

$$\begin{aligned}
\text{Res112b} := & \left[ -\frac{1}{16} F_{u_{1,3}}^2 F_{u_{1,2},u_{1,3}} - \frac{1}{8} F_{u_{2,3}} F_{u_{1,1}} F_{u_{1,3},u_{1,3}} + \frac{1}{8} F_{u_{1,2}} F_{u_{1,1},u_{1,3}} \right. \\
& - \frac{1}{4} F_{u_{1,1}} F_{u_{1,1},u_{2,3}} - \frac{1}{4} F_{u_{1,1}} F_{u_{1,3}} F_{u_{1,3},u_{2,3}} + \frac{1}{16} F_{u_{2,3}} F_{u_{1,3}} F_{u_{1,1},u_{1,3}} \\
& - \frac{1}{4} F_{u_{1,1}} F_{u_{1,2},u_{1,3}} - \frac{1}{16} F_{u_{1,3}}^3 F_{u_{1,3},u_{2,3}} - \frac{1}{16} F_{u_{1,1},u_{2,3}} F_{u_{1,3}}^2 \\
& + \frac{1}{16} F_{u_{1,2}} F_{u_{1,3}} F_{u_{1,3},u_{1,3}}, \blacklozenge, \frac{1}{8} F_{u_{2,2}} F_{u_{1,3}} F_{u_{1,3},u_{1,3}} + \frac{1}{16} F_{u_{2,3}}^2 F_{u_{1,1},u_{1,3}} \\
& \left. + \frac{1}{4} F_{u_{2,2}} F_{u_{1,1},u_{1,3}} - \frac{1}{16} F_{u_{1,1},u_{2,3}} F_{u_{1,3}} F_{u_{2,3}} - \frac{1}{2} F_{u_{1,1}} F_{u_{1,3},u_{2,3}} F_{u_{2,3}} \right]
\end{aligned} \tag{9}$$

$$\begin{aligned}
& -\frac{1}{4} F_{u_{1,1}} F_{u_{1,3}} F_{u_{2,3}'} u_{2,3} - \frac{1}{16} F_{u_{1,2}} F_{u_{2,3}} F_{u_{1,3}'} u_{1,3} - \frac{1}{8} F_{u_{1,3}}^2 F_{u_{1,2}'} u_{2,3} - \frac{1}{16} \\
& F_{u_{1,3}}^3 F_{u_{2,3}'} u_{2,3} - \frac{1}{8} F_{u_{1,3}}^2 F_{u_{1,3}'} u_{2,2} - \frac{1}{2} F_{u_{1,1}} F_{u_{1,3}'} u_{2,2} - \frac{1}{8} F_{u_{1,2}} F_{u_{1,2}'} u_{1,3} \\
& - \frac{1}{2} F_{u_{1,1}} F_{u_{1,2}'} u_{2,3} - \frac{1}{8} F_{u_{1,2}} F_{u_{1,3}} F_{u_{1,3}'} u_{2,3} - \frac{3}{16} F_{u_{1,3}}^2 F_{u_{2,3}} F_{u_{1,3}'} u_{2,3} \\
& - \frac{1}{8} F_{u_{1,1}'} u_{2,3} F_{u_{1,2}} - \frac{1}{16} F_{u_{1,3}} F_{u_{2,3}} F_{u_{1,2}'} u_{1,3}, \blacklozenge, -\frac{3}{8} F_{u_{1,2}} F_{u_{1,3}'} u_{2,3} F_{u_{2,3}} \\
& - \frac{3}{16} F_{u_{1,2}} F_{u_{1,3}} F_{u_{2,3}'} u_{2,3} - \frac{3}{4} F_{u_{1,1}} F_{u_{2,2}'} u_{2,3} - \frac{3}{8} F_{u_{1,2}} F_{u_{1,3}'} u_{2,2} - \frac{3}{16} \\
& F_{u_{1,3}}^2 F_{u_{2,2}'} u_{2,3} - \frac{3}{8} F_{u_{1,2}} F_{u_{1,2}'} u_{2,3} - \frac{3}{16} F_{u_{1,3}} F_{u_{2,3}}^2 F_{u_{1,3}'} u_{2,3} - \frac{3}{16} \\
& F_{u_{1,3}}^2 F_{u_{2,3}} F_{u_{2,3}'} u_{2,3} - \frac{3}{16} F_{u_{1,3}} F_{u_{2,3}} F_{u_{1,3}'} u_{2,2} - \frac{3}{16} F_{u_{1,3}} F_{u_{2,3}} F_{u_{1,2}'} u_{2,3} \\
& - \frac{3}{8} F_{u_{1,1}} F_{u_{2,3}} F_{u_{2,3}'} u_{2,3}, \blacklozenge, -\frac{1}{16} F_{u_{2,3}}^2 F_{u_{1,2}'} u_{2,3} - \frac{1}{4} F_{u_{2,2}} F_{u_{1,2}'} u_{2,3} \\
& - \frac{5}{8} F_{u_{1,2}} F_{u_{2,2}'} u_{2,3} - \frac{1}{16} F_{u_{1,3}'} u_{2,2} F_{u_{2,3}}^2 - \frac{1}{16} F_{u_{1,3}'} u_{2,3} F_{u_{2,3}}^3 - \frac{1}{4} F_{u_{2,2}} F_{u_{1,3}'} u_{2,2} \\
& - \frac{5}{16} F_{u_{1,2}} F_{u_{2,3}} F_{u_{2,3}'} u_{2,3} - \frac{1}{8} F_{u_{2,2}} F_{u_{1,3}} F_{u_{2,3}'} u_{2,3} - \frac{3}{16} F_{u_{1,3}} F_{u_{2,3}}^2 F_{u_{2,3}'} u_{2,3} \\
& - \frac{1}{4} F_{u_{2,2}} F_{u_{1,3}'} u_{2,3} F_{u_{2,3}} - \frac{5}{16} F_{u_{1,3}} F_{u_{2,3}} F_{u_{2,2}'} u_{2,3}, \blacklozenge, -\frac{1}{16} \left( F_{u_{2,3}'} u_{2,3} F_{u_{2,3}} \right. \\
& \left. + 2 F_{u_{2,2}'} u_{2,3} \right) \left( 4 F_{u_{2,2}}^2 + F_{u_{2,3}}^2 \right) \Big]
\end{aligned}$$

$$\begin{aligned}
\mathbf{E} & > \text{simplify}([ \text{diff}(Res112, u[1, 1, 1, 3, 3]), \blacklozenge, \text{diff}(Res112, u[1, 1, 2, 3, 3]), \blacklozenge, \\
& \text{diff}(Res112, u[1, 2, 2, 3, 3]), \blacklozenge, \text{diff}(Res112, u[2, 2, 2, 3, 3]), \blacklozenge, \text{diff}(Res112, u[1, \\
& 1, 3, 3, 3]), \blacklozenge, \text{diff}(Res112, u[1, 2, 3, 3, 3]), \blacklozenge, \text{diff}(Res112, u[2, 2, 3, 3, 3]), \blacklozenge, \\
& \text{diff}(Res112, u[1, 3, 3, 3, 3]), \blacklozenge, \text{diff}(Res112, u[2, 2, 3, 3, 3]), \blacklozenge, \text{diff}(Res112, u[3, \\
& 3, 3, 3, 3]) ]) \\
& [0, \blacklozenge, 0, \blacklozenge, 0, \blacklozenge, 0, \blacklozenge, 0, \blacklozenge, 0, \blacklozenge, 0, \blacklozenge, 0, \blacklozenge, 0]
\end{aligned} \tag{10}$$

$\mathbf{E} >$

$$\mathbf{E} > \text{subs}(\text{Sub}, Res112b[7])$$

$$\begin{aligned}
& -\frac{1}{16} F_{u_{2,3}}^2 F_{u_{1,2}'} u_{2,3} - \frac{1}{4} F_{u_{2,2}} F_{u_{1,2}'} u_{2,3} - \frac{5}{8} F_{u_{1,2}} F_{u_{2,2}'} u_{2,3} - \frac{1}{16} F_{u_{1,3}'} u_{2,2} F_{u_{2,3}}^2 \\
& - \frac{1}{16} F_{u_{1,3}'} u_{2,3} F_{u_{2,3}}^3 - \frac{1}{4} F_{u_{2,2}} F_{u_{1,3}'} u_{2,2} - \frac{5}{16} F_{u_{1,2}} F_{u_{2,3}} F_{u_{2,3}'} u_{2,3} \\
& - \frac{1}{8} F_{u_{2,2}} F_{u_{1,3}} F_{u_{2,3}'} u_{2,3} - \frac{3}{16} F_{u_{1,3}} F_{u_{2,3}}^2 F_{u_{2,3}'} u_{2,3} - \frac{1}{4} F_{u_{2,2}} F_{u_{1,3}'} u_{2,3} F_{u_{2,3}}
\end{aligned} \tag{11}$$

$$-\frac{5}{16} F_{u_{1,3}} F_{u_{2,3}} F_{u_{2,2} u_{2,3}}$$

> # Let us suppose at first that  $f_b^2 + 4f_t \neq 0$  and similarly (by symmetry)  $f_a^2 + 4f_r \neq 0$ .

Then

from the factorizable components above together with symmetric equations we get MAE conditions 1, 2, 5, 6 :

$$f_{ar} = -\frac{f_a f_{aa}}{2}, f_{bt} = -\frac{f_b f_{bb}}{2}, f_{rr} = -f_{aa}, f_{tt} = -f_{bb}. \text{ These we use as follows :}$$

>

$$\begin{aligned} \mathbf{E} > \text{factor} \left( \text{subs} \left( \left\{ f_{ar} = -\frac{f_a f_{aa}}{2}, f_{bt} = -\frac{f_b f_{bb}}{2} \right\}, \text{subs} \left( \text{Sub}, -\frac{1}{16} F_{u_{1,3}} F_{u_{2,2}} F_{u_{2,3}}^2 \right. \right. \right. \\ & - \frac{5}{16} F_{u_{2,3}} F_{u_{1,3}} F_{u_{2,2} u_{2,3}} - \frac{5}{8} F_{u_{1,2}} F_{u_{2,2} u_{2,3}} - \frac{1}{4} F_{u_{2,2}} F_{u_{1,3} u_{2,2}} - \frac{3}{16} F_{u_{1,3}} \\ & F_{u_{2,3}}^2 F_{u_{2,3} u_{2,3}} - \frac{1}{4} F_{u_{2,2}} F_{u_{1,2} u_{2,3}} - \frac{1}{4} F_{u_{2,2}} F_{u_{2,3}} F_{u_{1,3} u_{2,3}} \\ & - \frac{1}{8} F_{u_{2,2}} F_{u_{1,3}} F_{u_{2,3} u_{2,3}} - \frac{1}{16} F_{u_{2,3}}^3 F_{u_{1,3} u_{2,3}} - \frac{5}{16} F_{u_{2,3}} F_{u_{1,2}} F_{u_{2,3} u_{2,3}} - \frac{1}{16} \\ & \left. \left. \left. F_{u_{2,3}}^2 F_{u_{1,2} u_{2,3}} \right) \right) \right) \\ & - \frac{1}{32} (4f_t + f_b^2) (2f_{ab} f_b + 2f_{at} + 2f_{bs} + f_a f_{bb}) \end{aligned} \quad (12)$$

> # This equation ( ...=0 ) and its symmetric counterpart give the MAE conditions 3, 4. We add them to our substitution — simplification of vanishing of the other Cotton tensor components ( in fact we use only components [112], [212] and all coefficients in them with the fifth derivatives ).

$\mathbf{E} >$

$\mathbf{E} > \text{Res112a}[1]$

$$\begin{aligned} & \frac{1}{16} F_{u_{2,3}} F_{u_{1,3}} F_{u_{1,1} u_{1,1}} - \frac{1}{8} F_{u_{2,3}} F_{u_{1,1}} F_{u_{1,1} u_{1,3}} - \frac{1}{16} F_{u_{1,3}}^2 F_{u_{1,1} u_{1,2}} - \frac{1}{4} F_{u_{1,3} u_{2,3}} \\ & F_{u_{1,1}}^2 - \frac{1}{16} F_{u_{1,3}}^2 F_{u_{1,1}} F_{u_{1,3} u_{2,3}} - \frac{1}{4} F_{u_{1,1}} F_{u_{1,1} u_{1,2}} + \frac{1}{8} F_{u_{1,2}} F_{u_{1,1} u_{1,1}} \\ & + \frac{1}{16} F_{u_{1,2}} F_{u_{1,3}} F_{u_{1,1} u_{1,3}} \end{aligned} \quad (13)$$

$$\begin{aligned} \mathbf{E} > \text{Rela1} := \text{factor} \left( \text{subs} \left( \left\{ f_{ar} = -\frac{f_a f_{aa}}{2}, f_{bt} = -\frac{f_b f_{bb}}{2}, f_{at} = -f_{ab} f_b - \frac{f_a f_{bb}}{2} - f_{bs}, f_{br} = -f_{ab} f_a \right. \right. \right. \\ & - \frac{f_b f_{aa}}{2} - f_{as}, f_{rr} = -f_{aa}, f_{tt} = -f_{bb} \left. \right\}, \text{subs} \left( \text{Sub}, \frac{1}{16} F_{u_{2,3}} F_{u_{1,3}} F_{u_{1,1} u_{1,1}} \right. \\ & - \frac{1}{8} F_{u_{2,3}} F_{u_{1,1}} F_{u_{1,1} u_{1,3}} - \frac{1}{16} F_{u_{1,3}}^2 F_{u_{1,1} u_{1,2}} - \frac{1}{4} F_{u_{1,3} u_{2,3}} F_{u_{1,1}}^2 - \frac{1}{16} \\ & \left. \left. \left. F_{u_{1,3}}^2 F_{u_{1,1}} F_{u_{1,3} u_{2,3}} - \frac{1}{4} F_{u_{1,1}} F_{u_{1,1} u_{1,2}} + \frac{1}{8} F_{u_{1,2}} F_{u_{1,1} u_{1,1}} \right) \right) \right) \end{aligned}$$

$$+ \frac{1}{16} F_{u_{1,2}} F_{u_{1,3}} F_{u_{1,1}'} F_{u_{1,3}} \Big) \Big) \Big) \\ Rel1 := -\frac{1}{32} (4f_r + f_a^2) (2f_r f_{ab} + 2f_{rs} + f_s f_{aa}) \quad (14)$$

**E** > # This equation and its symemtric counterpart give the MAE conditions 7,8. Let's add them

**E** > Res112a[3]

$$\begin{aligned} & \frac{1}{16} F_{u_{1,1}'} F_{u_{2,3}} F_{u_{1,3}} F_{u_{1,2}} - \frac{1}{2} F_{u_{1,1}} F_{u_{1,3}'} F_{u_{2,3}} F_{u_{1,2}} - \frac{1}{16} F_{u_{1,3}}^2 F_{u_{2,3}'} F_{u_{2,3}} F_{u_{1,1}} - \frac{1}{8} \\ & F_{u_{1,3}}^2 F_{u_{1,1}'} F_{u_{2,2}} + \frac{1}{16} F_{u_{1,1}'} F_{u_{1,1}} F_{u_{2,3}}^2 - \frac{1}{4} F_{u_{1,1}} F_{u_{1,2}'} F_{u_{1,2}} - \frac{1}{16} F_{u_{1,3}}^2 F_{u_{1,2}'} F_{u_{1,2}} \\ & - \frac{1}{8} F_{u_{1,2}'} F_{u_{1,3}} F_{u_{2,3}} F_{u_{1,1}} + \frac{1}{4} F_{u_{2,2}} F_{u_{1,1}'} F_{u_{1,1}} - \frac{1}{16} F_{u_{1,1}'} F_{u_{1,3}} F_{u_{1,2}} F_{u_{2,3}} \\ & + \frac{1}{8} F_{u_{2,2}} F_{u_{1,1}'} F_{u_{1,3}} F_{u_{1,3}} - \frac{1}{2} F_{u_{1,1}} F_{u_{1,1}'} F_{u_{2,2}} - \frac{1}{8} F_{u_{1,3}} F_{u_{2,3}} F_{u_{1,1}} F_{u_{1,3}'} F_{u_{2,3}} \\ & - \frac{1}{8} F_{u_{2,3}} F_{u_{1,1}} F_{u_{1,1}'} F_{u_{2,3}} - \frac{1}{16} F_{u_{1,3}}^2 F_{u_{1,2}} F_{u_{1,3}'} F_{u_{2,3}} - \frac{1}{4} F_{u_{2,3}'} F_{u_{2,3}} F_{u_{1,1}}^2 \\ & + \frac{1}{16} F_{u_{1,3}} F_{u_{1,2}} F_{u_{1,2}'} F_{u_{1,3}} \end{aligned} \quad (15)$$

$$\begin{aligned} \mathbf{E} > factor \Big( subs \Big( \Big\{ f_{ar} = -\frac{f_a f_{aa}}{2}, f_{bt} = -\frac{f_b f_{bb}}{2}, f_{at} = -f_{ab} f_b - \frac{f_a f_{bb}}{2} - f_{bs}, f_{br} = -f_{ab} f_a - \frac{f_b f_{aa}}{2} - f_{as}, \\ f_{rr} = -f_r f_{aa}, f_{tt} = -f_{bb} f_r f_{rs} = -\frac{f_{aa} f_s}{2} - f_r f_{ab}, f_{st} = -\frac{f_{bb} f_s}{2} - f_t f_{ab} \Big\}, subs \Big( Sub, \\ & \frac{1}{16} F_{u_{1,1}'} F_{u_{2,3}} F_{u_{1,3}} F_{u_{1,2}} - \frac{1}{2} F_{u_{1,1}} F_{u_{1,3}'} F_{u_{2,3}} F_{u_{1,2}} - \frac{1}{16} F_{u_{1,3}}^2 F_{u_{2,3}'} F_{u_{2,3}} F_{u_{1,1}} \\ & - \frac{1}{8} F_{u_{1,3}}^2 F_{u_{1,1}'} F_{u_{2,2}} + \frac{1}{16} F_{u_{1,1}'} F_{u_{1,1}} F_{u_{2,3}}^2 - \frac{1}{4} F_{u_{1,1}} F_{u_{1,2}'} F_{u_{1,2}} - \frac{1}{16} \\ & F_{u_{1,3}}^2 F_{u_{1,2}'} F_{u_{1,2}} - \frac{1}{8} F_{u_{1,2}'} F_{u_{1,3}} F_{u_{2,3}} F_{u_{1,1}} + \frac{1}{4} F_{u_{2,2}} F_{u_{1,1}'} F_{u_{1,1}} \\ & - \frac{1}{16} F_{u_{1,1}'} F_{u_{1,3}} F_{u_{1,2}} F_{u_{2,3}} + \frac{1}{8} F_{u_{2,2}} F_{u_{1,1}'} F_{u_{1,3}} F_{u_{1,3}} - \frac{1}{2} F_{u_{1,1}} F_{u_{1,1}'} F_{u_{2,2}} \\ & - \frac{1}{8} F_{u_{1,3}} F_{u_{2,3}} F_{u_{1,1}} F_{u_{1,3}'} F_{u_{2,3}} - \frac{1}{8} F_{u_{2,3}} F_{u_{1,1}} F_{u_{1,1}'} F_{u_{2,3}} - \frac{1}{16} \\ & F_{u_{1,3}}^2 F_{u_{1,2}} F_{u_{1,3}'} F_{u_{2,3}} - \frac{1}{4} F_{u_{2,3}'} F_{u_{2,3}} F_{u_{1,1}}^2 + \frac{1}{16} F_{u_{1,3}} F_{u_{1,2}} F_{u_{1,2}'} F_{u_{1,3}} \Big) \Big) \Big) \\ & - \frac{1}{16} (f_a^2 + 4f_r) (2f_{rt} + f_{bb} f_r + f_t f_{aa} + 2f_{ab} f_s + f_{ss}) \end{aligned} \quad (16)$$

**E** > # This is the final MAE condition 9, so on the generic stratum the claim is poved.  
Let us consider now the singular cases, when some 1 st order equation holds.

**E** >

**E** >

**E** > # Now we can check the condition  $f_a^2 + 4f_r = 0$ , **and** assume  $f_b^2 + 4f_t$   
 $\neq 0$  (the other follows **by** symmetry); we add the differential corollaries  
**and** check what are the remaining MAE conditions

$$\begin{aligned} \mathbf{E} > \text{factor} \left( \text{subs} \left( \left\{ f_r = -\frac{1}{4}f_a^2, f_{ar} = -\frac{1}{2}f_af_{aa}, f_{br} = -\frac{1}{2}f_af_{ab}, f_{rr} = \frac{1}{4}f_a^2f_{aa}, f_{rs} = -\frac{1}{2}f_af_{as}, f_{rt} = \right. \right. \right. \\ \left. \left. \left. -\frac{1}{2}f_af_{at} \right\}, [f_{aa}f_a + 2f_{ar}, \blacklozenge, f_{bb}f_b + 2f_{br}, \blacklozenge, f_{aa}f_b + 2f_{ab}f_a + 2f_{as} + 2f_{br}, \blacklozenge, f_{bb}f_a \right. \right. \\ \left. \left. + 2f_{ab}f_b + 2f_{bs} + 2f_{ar}, \blacklozenge, f_{aa}f_r + f_{rr}, \blacklozenge, f_{bb}f_t + f_{tt}, \blacklozenge, f_{aa}f_s + 2f_{ab}f_r + 2f_{rs}, \blacklozenge, f_{bb}f_s \right. \right. \\ \left. \left. + 2f_{ab}f_t + 2f_{st}, \blacklozenge, f_{aa}f_t + f_{bb}f_r + 2f_{ab}f_s + 2f_{rt} + f_{ss}] \right) \right) \\ \left[ 0, \blacklozenge, f_bf_{bb} + 2f_{br}, \blacklozenge, f_bf_{aa} + f_{ab}f_a + 2f_{as}, \blacklozenge, f_af_{bb} + 2f_{ab}f_b + 2f_{bs} + 2f_{ar}, \blacklozenge, 0, \blacklozenge, f_{tt} \right. \\ \left. + f_tf_{bb}, \blacklozenge, -\frac{1}{2}f_a^2f_{ab} - f_af_{as} + f_sf_{aa}, \blacklozenge, f_{bb}f_s + 2f_{ab}f_t + 2f_{st}, \blacklozenge, f_{aa}f_t - \frac{1}{4}f_{bb}f_a^2 + 2f_{ab}f_s \right. \\ \left. - f_af_{at} + f_{ss} \right] \end{aligned} \quad (17)$$

$$\mathbf{E} > \text{Res112a}[11] \\ -\frac{1}{16} \left( 4F_{u_{2,2}} + F_{u_{2,3}}^2 \right) \left( F_{u_{2,2},u_{2,2}} + F_{u_{2,2}}F_{u_{2,3},u_{2,3}} \right) \quad (18)$$

$$\begin{aligned} \mathbf{E} > \text{factor} \left( \text{subs} \left( \left\{ f_r = -\frac{1}{4}f_a^2, f_{ar} = -\frac{1}{2}f_af_{aa}, f_{br} = -\frac{1}{2}f_af_{ab}, f_{rr} = \frac{1}{4}f_a^2f_{aa}, f_{rs} = -\frac{1}{2}f_af_{as}, f_{rt} = \right. \right. \right. \\ \left. \left. \left. -\frac{1}{2}f_af_{at} \right\}, \text{subs} \left( \text{Sub}, -\frac{1}{16} \left( 4F_{u_{2,2}} + F_{u_{2,3}}^2 \right) \left( F_{u_{2,2},u_{2,2}} + F_{u_{2,2}}F_{u_{2,3},u_{2,3}} \right) \right) \right) \right) \\ -\frac{1}{16} \left( 4f_t + f_b^2 \right) \left( f_{tt} + f_tf_{bb} \right) \end{aligned} \quad (19)$$

$$\mathbf{E} > \text{Res112b}[9] \\ -\frac{1}{16} \left( F_{u_{2,3},u_{2,3}}F_{u_{2,3}} + 2F_{u_{2,2},u_{2,3}} \right) \left( 4F_{u_{2,2}} + F_{u_{2,3}}^2 \right) \quad (20)$$

$$\begin{aligned} \mathbf{E} > \text{factor} \left( \text{subs} \left( \left\{ f_r = -\frac{1}{4}f_a^2, f_{ar} = -\frac{1}{2}f_af_{aa}, f_{br} = -\frac{1}{2}f_af_{ab}, f_{rr} = \frac{1}{4}f_a^2f_{aa}, f_{rs} = -\frac{1}{2}f_af_{as}, f_{rt} = \right. \right. \right. \\ \left. \left. \left. -\frac{1}{2}f_af_{at} \right\}, \text{subs} \left( \text{Sub}, -\frac{1}{16} \left( F_{u_{2,3},u_{2,3}}F_{u_{2,3}} + 2F_{u_{2,2},u_{2,3}} \right) \left( 4F_{u_{2,2}} + F_{u_{2,3}}^2 \right) \right) \right) \right) \\ -\frac{1}{16} \left( f_{bb}f_b + 2f_{bt} \right) \left( 4f_t + f_b^2 \right) \end{aligned} \quad (21)$$

**E** > # This gives two more vanishing conditions (the second **and** the first factors respectively)

$$\begin{aligned} \mathbf{E} > \text{Res112a}[9] \\ -\frac{1}{4}F_{u_{2,2}}F_{u_{1,2},u_{2,2}} - \frac{1}{16}F_{u_{1,3},u_{2,3}}F_{u_{2,3}}^2F_{u_{2,2}} + \frac{1}{8}F_{u_{1,3}}F_{u_{2,2},u_{2,3}}F_{u_{2,2}} \\ -\frac{3}{16}F_{u_{1,3}}F_{u_{2,3}}F_{u_{2,2},u_{2,2}} - \frac{1}{8}F_{u_{1,3}}F_{u_{2,3}}F_{u_{2,2}}F_{u_{2,3},u_{2,3}} - \frac{1}{2}F_{u_{1,2}}F_{u_{2,3},u_{2,3}}F_{u_{2,2}} \end{aligned} \quad (22)$$



$$-\frac{1}{16} F_{u_{2,3}}^2 F_{u_{1,2},u_{2,2}} - \frac{3}{8} F_{u_{1,2}} F_{u_{2,2},u_{2,2}} - \frac{1}{16} F_{u_{2,3}}^2 F_{u_{1,2}} F_{u_{2,3},u_{2,3}} - \frac{1}{4} F_{u_{1,3},u_{2,3}} F_{u_{2,2}}^2 - \frac{1}{16} F_{u_{2,3}} F_{u_{1,2}} F_{u_{2,2},u_{2,3}}$$

$$\begin{aligned} \mathbf{E} > \text{factor}\left(\text{subs}\left(\left\{f_r = -\frac{1}{4}f_a^2, f_{ar} = -\frac{1}{2}f_a f_{aa}, f_{br} = -\frac{1}{2}f_a f_{ab}, f_{rr} = \frac{1}{4}f_a^2 f_{aa}, f_{rs} = -\frac{1}{2}f_a f_{as}, f_{rt} = \right. \right. \\ & -\frac{1}{2}f_a f_{ar} f_{tt} = -f_{fbb}, f_{bt} = -\frac{1}{2}f_{fbb}\left.\right\}, \text{subs}\left(\text{Sub}, -\frac{1}{4} F_{u_{2,2}} F_{u_{1,2},u_{2,2}} - \frac{1}{16} F_{u_{1,3},u_{2,3}} F_{u_{2,3}}^2 F_{u_{2,2}} + \frac{1}{8} F_{u_{1,3}} F_{u_{2,2},u_{2,3}} F_{u_{2,2}} - \frac{3}{16} F_{u_{1,3}} F_{u_{2,3}} F_{u_{2,2},u_{2,2}} \right. \\ & -\frac{1}{8} F_{u_{1,3}} F_{u_{2,3}} F_{u_{2,2}} F_{u_{2,3},u_{2,3}} - \frac{1}{2} F_{u_{1,2}} F_{u_{2,3},u_{2,3}} F_{u_{2,2}} - \frac{1}{16} F_{u_{2,3}}^2 F_{u_{1,2},u_{2,2}} \\ & -\frac{3}{8} F_{u_{1,2}} F_{u_{2,2},u_{2,2}} - \frac{1}{16} F_{u_{2,3}}^2 F_{u_{1,2}} F_{u_{2,3},u_{2,3}} - \frac{1}{4} F_{u_{1,3},u_{2,3}} F_{u_{2,2}}^2 \\ & \left. \left. - \frac{1}{16} F_{u_{2,3}} F_{u_{1,2}} F_{u_{2,2},u_{2,3}}\right)\right)\right) \\ & -\frac{1}{32} (f_b^2 + 4f_t) (2f_{st} + f_{bb}f_s + 2f_{ab}f_t) \end{aligned} \quad (23)$$

$\mathbf{E} > \# \text{ more vanishing factors to add - one more vanishing obtained}$

$\mathbf{E} > \text{Res112b}[7]$

$$\begin{aligned} & -\frac{1}{16} F_{u_{2,3}}^2 F_{u_{1,2},u_{2,3}} - \frac{1}{4} F_{u_{2,2}} F_{u_{1,2},u_{2,3}} - \frac{5}{8} F_{u_{1,2}} F_{u_{2,2},u_{2,3}} - \frac{1}{16} F_{u_{1,3},u_{2,2}} F_{u_{2,3}}^2 \\ & -\frac{1}{16} F_{u_{1,3},u_{2,3}} F_{u_{2,3}}^3 - \frac{1}{4} F_{u_{2,2}} F_{u_{1,3},u_{2,2}} - \frac{5}{16} F_{u_{1,2}} F_{u_{2,3}} F_{u_{2,3},u_{2,3}} \\ & -\frac{1}{8} F_{u_{2,2}} F_{u_{1,3}} F_{u_{2,3},u_{2,3}} - \frac{3}{16} F_{u_{1,3}} F_{u_{2,3}}^2 F_{u_{2,3},u_{2,3}} - \frac{1}{4} F_{u_{2,2}} F_{u_{1,3},u_{2,3}} F_{u_{2,3}} \\ & -\frac{5}{16} F_{u_{1,3}} F_{u_{2,3}} F_{u_{2,2},u_{2,3}} \end{aligned} \quad (24)$$

$$\begin{aligned} \mathbf{E} > \text{factor}\left(\text{subs}\left(\left\{f_r = -\frac{1}{4}f_a^2, f_{ar} = -\frac{1}{2}f_a f_{aa}, f_{br} = -\frac{1}{2}f_a f_{ab}, f_{rr} = \frac{1}{4}f_a^2 f_{aa}, f_{rs} = -\frac{1}{2}f_a f_{as}, f_{rt} = \right. \right. \\ & -\frac{1}{2}f_a f_{ar} f_{tt} = -f_{fbb}, f_{bt} = -\frac{1}{2}f_{fbb}, f_{st} = -\frac{1}{2}f_{fbb} - f_{fab}\left.\right\}, \text{subs}\left(\text{Sub}, -\frac{1}{16} F_{u_{2,3}}^2 F_{u_{1,2},u_{2,3}} - \frac{1}{4} F_{u_{2,2}} F_{u_{1,2},u_{2,3}} - \frac{5}{8} F_{u_{1,2}} F_{u_{2,2},u_{2,3}} - \frac{1}{16} F_{u_{1,3},u_{2,2}} F_{u_{2,3}}^2 \right. \\ & -\frac{1}{16} F_{u_{1,3},u_{2,3}} F_{u_{2,3}}^3 - \frac{1}{4} F_{u_{2,2}} F_{u_{1,3},u_{2,2}} - \frac{5}{16} F_{u_{1,2}} F_{u_{2,3}} F_{u_{2,3},u_{2,3}} \\ & -\frac{1}{8} F_{u_{2,2}} F_{u_{1,3}} F_{u_{2,3},u_{2,3}} - \frac{3}{16} F_{u_{1,3}} F_{u_{2,3}}^2 F_{u_{2,3},u_{2,3}} - \frac{1}{4} F_{u_{2,2}} F_{u_{1,3},u_{2,3}} F_{u_{2,3}} \\ & \left. \left. - \frac{5}{16} F_{u_{1,3}} F_{u_{2,3}} F_{u_{2,2},u_{2,3}}\right)\right)\right) \end{aligned} \quad (25)$$

$$-\frac{1}{32} (f_b^2 + 4f_t) (f_a f_{bb} + 2f_b f_{ab} + 2f_{bs} + 2f_{at}) \quad (25)$$

**E** > *Res112b*[3]

$$\begin{aligned} & \frac{1}{8} F_{u,2,2} F_{u,1,3} F_{u,1,3,u,1,3} + \frac{1}{16} F_{u,2,3}^2 F_{u,1,1,u,1,3} + \frac{1}{4} F_{u,2,2} F_{u,1,1,u,1,3} \\ & - \frac{1}{16} F_{u,1,1,u,2,3} F_{u,1,3} F_{u,2,3} - \frac{1}{2} F_{u,1,1} F_{u,1,3,u,2,3} F_{u,2,3} - \frac{1}{4} F_{u,1,1} F_{u,1,3} F_{u,2,3,u,2,3} \\ & - \frac{1}{16} F_{u,1,2} F_{u,2,3} F_{u,1,3,u,1,3} - \frac{1}{8} F_{u,1,3}^2 F_{u,1,2,u,2,3} - \frac{1}{16} F_{u,1,3}^3 F_{u,2,3,u,2,3} - \frac{1}{8} \\ & F_{u,1,3}^2 F_{u,1,3,u,2,2} - \frac{1}{2} F_{u,1,1} F_{u,1,3,u,2,2} - \frac{1}{8} F_{u,1,2} F_{u,1,2,u,1,3} - \frac{1}{2} F_{u,1,1} F_{u,1,2,u,2,3} \\ & - \frac{1}{8} F_{u,1,2} F_{u,1,3} F_{u,1,3,u,2,3} - \frac{3}{16} F_{u,1,3}^2 F_{u,2,3} F_{u,1,3,u,2,3} - \frac{1}{8} F_{u,1,1,u,2,3} F_{u,1,2} \\ & - \frac{1}{16} F_{u,1,3} F_{u,2,3} F_{u,1,2,u,1,3} \end{aligned} \quad (26)$$

$$\begin{aligned} \mathbf{E} > \text{factor} \left( \text{subs} \left( \left\{ f_r = -\frac{1}{4} f_a^2, f_{ar} = -\frac{1}{2} f_a f_{aa}, f_{br} = -\frac{1}{2} f_a f_{ab}, f_{rr} = \frac{1}{4} f_a^2 f_{aa}, f_{rs} = -\frac{1}{2} f_a f_{as}, f_{rt} = \right. \right. \\ & \left. \left. -\frac{1}{2} f_a f_{ar} f_{tt} = -f f_{bb}, f_{bt} = -\frac{1}{2} f f_{bb}, f_{st} = -\frac{1}{2} f f_{bb} - f f_{ab}, f_{bs} = -f_{at} - f f_{ab} - \frac{1}{2} f f_{bb} \right\}, \right. \\ & \text{subs} \left( \text{Sub}, \frac{1}{8} F_{u,2,2} F_{u,1,3} F_{u,1,3,u,1,3} + \frac{1}{16} F_{u,2,3}^2 F_{u,1,1,u,1,3} + \frac{1}{4} F_{u,2,2} F_{u,1,1,u,1,3} \right. \\ & - \frac{1}{16} F_{u,1,1,u,2,3} F_{u,1,3} F_{u,2,3} - \frac{1}{2} F_{u,1,1} F_{u,1,3,u,2,3} F_{u,2,3} - \frac{1}{4} F_{u,1,1} F_{u,1,3} F_{u,2,3,u,2,3} \\ & - \frac{1}{16} F_{u,1,2} F_{u,2,3} F_{u,1,3,u,1,3} - \frac{1}{8} F_{u,1,3}^2 F_{u,1,2,u,2,3} - \frac{1}{16} F_{u,1,3}^3 F_{u,2,3,u,2,3} - \frac{1}{8} \\ & F_{u,1,3}^2 F_{u,1,3,u,2,2} - \frac{1}{2} F_{u,1,1} F_{u,1,3,u,2,2} - \frac{1}{8} F_{u,1,2} F_{u,1,2,u,1,3} - \frac{1}{2} F_{u,1,1} F_{u,1,2,u,2,3} \\ & - \frac{1}{8} F_{u,1,2} F_{u,1,3} F_{u,1,3,u,2,3} - \frac{3}{16} F_{u,1,3}^2 F_{u,2,3} F_{u,1,3,u,2,3} - \frac{1}{8} F_{u,1,1,u,2,3} F_{u,1,2} \\ & \left. \left. \left. - \frac{1}{16} F_{u,1,3} F_{u,2,3} F_{u,1,2,u,1,3} \right) \right) \right) \\ & - \frac{1}{32} (2f_s + f_a f_b) (f_a f_{ab} + f_{aa} f_b + 2f_{as}) \end{aligned} \quad (27)$$

**E** > *Res112a*[5]

$$\begin{aligned} & -\frac{1}{8} F_{u,1,2} F_{u,1,2,u,1,2} - \frac{1}{2} F_{u,1,1} F_{u,1,3,u,2,3} F_{u,2,2} + \frac{1}{8} F_{u,1,1,u,2,3} F_{u,1,3} F_{u,2,2} - \frac{1}{16} F_{u,1,3,u,2,3} \\ & F_{u,2,3}^2 F_{u,1,1} - \frac{1}{8} F_{u,1,3,u,2,2} F_{u,2,3} F_{u,1,1} - \frac{1}{8} F_{u,1,3} F_{u,2,3} F_{u,1,1,u,2,2} - \frac{1}{16} \\ & F_{u,1,3}^2 F_{u,2,3,u,2,3} F_{u,1,2} - \frac{1}{8} F_{u,1,3} F_{u,2,3} F_{u,1,1} F_{u,2,3,u,2,3} - \frac{1}{16} F_{u,1,1,u,2,3} F_{u,2,3} F_{u,1,2} \end{aligned} \quad (28)$$

$$\begin{aligned}
& -\frac{1}{2} F_{u_{1,1}} F_{u_{2,3}'} F_{u_{2,3}} F_{u_{1,2}} + \frac{1}{16} F_{u_{2,3}}^2 F_{u_{1,1}'} F_{u_{1,2}} - \frac{3}{16} F_{u_{1,3}}^2 F_{u_{1,2}'} F_{u_{2,2}} \\
& -\frac{1}{4} F_{u_{1,2}} F_{u_{1,1}'} F_{u_{2,2}} - \frac{3}{4} F_{u_{1,2}'} F_{u_{2,2}} F_{u_{1,1}} + \frac{1}{4} F_{u_{2,2}} F_{u_{1,1}'} F_{u_{1,2}} \\
& -\frac{1}{8} F_{u_{1,3}} F_{u_{2,3}} F_{u_{1,2}} F_{u_{1,3}'} F_{u_{2,3}} - \frac{1}{4} F_{u_{1,3}'} F_{u_{2,3}} F_{u_{1,2}}^2 - \frac{1}{16} F_{u_{1,2}'} F_{u_{1,3}} F_{u_{2,3}} F_{u_{1,2}} \\
& + \frac{1}{16} F_{u_{1,3}} F_{u_{1,2}'} F_{u_{2,3}} F_{u_{1,2}} - \frac{1}{16} F_{u_{1,3}} F_{u_{2,3}} F_{u_{1,2}'} F_{u_{1,2}} - \frac{1}{16} F_{u_{1,3}}^2 F_{u_{2,2}} F_{u_{1,3}'} F_{u_{2,3}} \\
& + \frac{1}{16} F_{u_{1,3}} F_{u_{1,2}} F_{u_{1,3}'} F_{u_{2,2}} + \frac{1}{8} F_{u_{1,3}} F_{u_{2,2}} F_{u_{1,2}'} F_{u_{1,3}} - \frac{1}{8} F_{u_{2,3}} F_{u_{1,1}} F_{u_{1,2}'} F_{u_{2,3}}
\end{aligned}$$

$$\begin{aligned}
\mathbf{E} & > \text{factor} \left( \text{subs} \left( \left\{ f_r = -\frac{1}{4} f_a^2, f_{ar} = -\frac{1}{2} f_a f_{aa}, f_{br} = -\frac{1}{2} f_a f_{ab}, f_{rr} = \frac{1}{4} f_a^2 f_{aa}, f_{rs} = -\frac{1}{2} f_a f_{as}, f_{rt} = \right. \right. \\
& \quad \left. \left. -\frac{1}{2} f_a f_{ar}, f_{tt} = -f_{bb}, f_{bt} = -\frac{1}{2} f_{bb}, f_{st} = -\frac{1}{2} f_{bb} - f_{ab}, f_{bs} = -f_{at} - f_{ab} - \frac{1}{2} f_{bb} \right\}, \right. \\
& \quad \text{subs} \left( \text{Sub}, -\frac{1}{8} F_{u_{1,2}} F_{u_{1,2}'} F_{u_{1,2}} - \frac{1}{2} F_{u_{1,1}} F_{u_{1,3}'} F_{u_{2,3}} F_{u_{2,2}} + \frac{1}{8} F_{u_{1,1}'} F_{u_{2,3}} F_{u_{1,3}} F_{u_{2,2}} \right. \\
& \quad - \frac{1}{16} F_{u_{1,3}'} F_{u_{2,3}} F_{u_{1,1}}^2 F_{u_{1,1}} - \frac{1}{8} F_{u_{1,3}'} F_{u_{2,2}} F_{u_{2,3}} F_{u_{1,1}} - \frac{1}{8} F_{u_{1,3}} F_{u_{2,3}} F_{u_{1,1}'} F_{u_{2,2}} \\
& \quad - \frac{1}{16} F_{u_{1,3}}^2 F_{u_{2,3}} F_{u_{1,2}} F_{u_{1,2}} - \frac{1}{8} F_{u_{1,3}} F_{u_{2,3}} F_{u_{1,1}} F_{u_{2,3}'} F_{u_{2,3}} \\
& \quad - \frac{1}{16} F_{u_{1,1}'} F_{u_{2,3}} F_{u_{2,3}} F_{u_{1,2}} - \frac{1}{2} F_{u_{1,1}} F_{u_{2,3}'} F_{u_{2,3}} F_{u_{1,2}} + \frac{1}{16} F_{u_{2,3}}^2 F_{u_{1,1}'} F_{u_{1,2}} - \frac{3}{16} \\
& \quad F_{u_{1,3}}^2 F_{u_{1,2}'} F_{u_{2,2}} - \frac{1}{4} F_{u_{1,2}} F_{u_{1,1}'} F_{u_{2,2}} - \frac{3}{4} F_{u_{1,2}'} F_{u_{2,2}} F_{u_{1,1}} + \frac{1}{4} F_{u_{2,2}} F_{u_{1,1}'} F_{u_{1,2}} \\
& \quad - \frac{1}{8} F_{u_{1,3}} F_{u_{2,3}} F_{u_{1,2}} F_{u_{1,3}'} F_{u_{2,3}} - \frac{1}{4} F_{u_{1,3}'} F_{u_{2,3}} F_{u_{1,2}}^2 - \frac{1}{16} F_{u_{1,2}'} F_{u_{1,3}} F_{u_{2,3}} F_{u_{1,2}} \\
& \quad + \frac{1}{16} F_{u_{1,3}} F_{u_{1,2}'} F_{u_{2,3}} F_{u_{1,2}} - \frac{1}{16} F_{u_{1,3}} F_{u_{2,3}} F_{u_{1,2}'} F_{u_{1,2}} - \frac{1}{16} F_{u_{1,3}}^2 F_{u_{2,2}} F_{u_{1,3}'} F_{u_{2,3}} \\
& \quad \left. \left. + \frac{1}{16} F_{u_{1,3}} F_{u_{1,2}} F_{u_{1,3}'} F_{u_{2,2}} + \frac{1}{8} F_{u_{1,3}} F_{u_{2,2}} F_{u_{1,2}'} F_{u_{1,3}} - \frac{1}{8} F_{u_{2,3}} F_{u_{1,1}} F_{u_{1,2}'} F_{u_{2,3}} \right) \right) \\
& \quad \left. \right) \\
& \quad \frac{1}{64} (2f_s + f_a f_b) (f_{bb} f_a^2 - f_a f_{ab} f_b + 4f_a f_{at} - 2f_{as} f_b - 8f_s f_{ab} - 4f_{ss})
\end{aligned} \tag{29}$$

$\mathbf{E} > \#$  if in addition  $2f_s + f_a f_b \neq 0$  we get two more conditions

. Let us substitute these all into MAE conditions :

$$\begin{aligned}
\mathbf{E} & > \text{factor} \left( \text{subs} \left( \left\{ f_r = -\frac{1}{4} f_a^2, f_{ar} = -\frac{1}{2} f_a f_{aa}, f_{br} = -\frac{1}{2} f_a f_{ab}, f_{rr} = \frac{1}{4} f_a^2 f_{aa}, f_{rs} = -\frac{1}{2} f_a \left( -\frac{1}{2} f_{bb} f_{aa} \right. \right. \right. \right. \\
& \quad \left. \left. \left. - \frac{1}{2} f_a f_{ab} \right), f_{rt} = -\frac{1}{2} f_a f_{ar}, f_{tt} = -f_{bb}, f_{bt} = -\frac{1}{2} f_{bb}, f_{st} = -\frac{1}{2} f_{bb} - f_{ab}, f_{bs} = -f_{at} - f_{ab} \right. \right. \\
& \quad \left. \left. - \frac{1}{2} f_{bb}, f_{as} = -\frac{1}{2} f_{bb} - \frac{1}{2} f_a f_{ab}, f_{ss} = \frac{1}{4} f_{bb} f_a^2 + f_a f_{at} + \frac{1}{4} f_{aa} f_b^2 - 2f_s f_{ab} \right\}, [f_{aa} f_a \right. \right.
\end{aligned}$$

$$\begin{aligned}
& + 2f_{ar}, \blacklozenge, f_{bb}f_b + 2f_{bt}, \blacklozenge, f_{aa}f_b + 2f_{ab}f_a + 2f_{as} + 2f_{br}, \blacklozenge, f_{bb}f_a + 2f_{ab}f_b + 2f_{bs} \\
& + 2f_{ar}, \blacklozenge, f_{aa}f_r + f_{rr}, \blacklozenge, f_{bb}f_t + f_{tr}, \blacklozenge, f_{aa}f_s + 2f_{ab}f_r + 2f_{rs}, \blacklozenge, f_{bb}f_s + 2f_{ab}f_t + 2f_{st}, \blacklozenge, \\
& f_{aa}f_t + f_{bb}f_r + 2f_{ab}f_s + 2f_{rt} + f_{ss} ] )
\end{aligned}$$

$$\left[ 0, \blacklozenge, 0, \blacklozenge, 0, \blacklozenge, 0, \blacklozenge, 0, \blacklozenge, \frac{1}{2} f_{aa} (2f_s + f_a f_b), \blacklozenge, 0, \blacklozenge, \frac{1}{4} f_{aa} (4f_t + f_b^2) \right] \quad (30)$$

**E** > #... so we need to show  $f_{aa}=0$ . [112] component of Cotton is **not** enough, so let us use [212] component

**E** >

**E** >  $Res212 := simplify(smb15(dB \cdot Pullback(alpha, Cot(2, 1, 2)))) :$

**E** >  $Res212a := factor([diff(Res212, u[1, 1, 1, 1, 1]), \blacklozenge, diff(Res212, u[1, 1, 1, 1, 2]), \blacklozenge, diff(Res212, u[1, 1, 1, 2, 2]), \blacklozenge, diff(Res212, u[1, 1, 2, 2, 2]), \blacklozenge, diff(Res212, u[1, 2, 2, 2, 2])])$

$$Res212a := \left[ \frac{1}{16} \left( 4F_{u_{1,1}}^2 + F_{u_{1,3}}^2 \right) \left( F_{u_{1,3}, u_{1,3}} F_{u_{1,1}} + F_{u_{1,1}, u_{1,1}} \right), \blacklozenge, \frac{1}{16} \right] \quad (31)$$

$$\begin{aligned}
& F_{u_{1,3}}^2 F_{u_{1,1}} F_{u_{1,3}, u_{2,3}} + \frac{3}{16} F_{u_{2,3}} F_{u_{1,3}} F_{u_{1,1}, u_{1,1}} - \frac{1}{8} F_{u_{2,3}} F_{u_{1,1}} F_{u_{1,1}, u_{1,3}} \\
& + \frac{1}{16} F_{u_{1,2}} F_{u_{1,3}} F_{u_{1,1}, u_{1,3}} + \frac{1}{8} F_{u_{1,3}} F_{u_{2,3}} F_{u_{1,1}} F_{u_{1,3}, u_{1,3}} + \frac{1}{16} F_{u_{1,3}}^2 F_{u_{1,2}} F_{u_{1,3}, u_{1,3}} \\
& + \frac{1}{16} F_{u_{1,3}}^2 F_{u_{1,1}, u_{1,2}} + \frac{1}{4} F_{u_{1,3}, u_{2,3}} F_{u_{1,1}}^2 + \frac{1}{2} F_{u_{1,1}} F_{u_{1,3}, u_{1,3}} F_{u_{1,2}} \\
& + \frac{1}{4} F_{u_{1,1}} F_{u_{1,1}, u_{1,2}} + \frac{3}{8} F_{u_{1,2}} F_{u_{1,1}, u_{1,1}}, \blacklozenge, \frac{1}{2} F_{u_{1,2}} F_{u_{1,1}, u_{1,2}} \\
& - \frac{1}{8} F_{u_{2,3}} F_{u_{1,1}} F_{u_{1,1}, u_{2,3}} + \frac{1}{16} F_{u_{1,3}} F_{u_{1,2}} F_{u_{1,2}, u_{1,3}} + \frac{1}{16} F_{u_{1,3}}^2 F_{u_{2,2}} F_{u_{1,3}, u_{1,3}} \\
& + \frac{1}{16} F_{u_{1,3}, u_{1,3}} F_{u_{2,3}}^2 F_{u_{1,1}} - \frac{1}{8} F_{u_{1,2}, u_{1,3}} F_{u_{2,3}} F_{u_{1,1}} + \frac{1}{8} F_{u_{2,2}} F_{u_{1,3}} F_{u_{1,1}, u_{1,3}} + \frac{1}{16} \\
& F_{u_{1,3}}^2 F_{u_{1,2}} F_{u_{1,3}, u_{2,3}} + \frac{1}{8} F_{u_{1,3}} F_{u_{2,3}} F_{u_{1,2}} F_{u_{1,3}, u_{1,3}} + \frac{1}{8} F_{u_{1,3}} F_{u_{2,3}} F_{u_{1,1}} F_{u_{1,3}, u_{2,3}} \\
& + \frac{1}{2} F_{u_{1,1}} F_{u_{1,3}, u_{1,3}} F_{u_{2,2}} + \frac{1}{8} F_{u_{2,3}}^2 F_{u_{1,1}, u_{1,1}} + \frac{1}{4} F_{u_{1,3}, u_{1,3}} F_{u_{1,2}}^2 \\
& - \frac{1}{16} F_{u_{1,2}} F_{u_{2,3}} F_{u_{1,1}, u_{1,3}} + \frac{1}{4} F_{u_{1,3}} F_{u_{2,3}} F_{u_{1,1}, u_{1,2}} + \frac{1}{16} F_{u_{1,1}, u_{2,3}} F_{u_{1,3}} F_{u_{1,2}} \\
& + \frac{1}{2} F_{u_{2,2}} F_{u_{1,1}, u_{1,1}} + \frac{1}{2} F_{u_{1,1}} F_{u_{1,3}, u_{2,3}} F_{u_{1,2}}, \blacklozenge, -\frac{1}{16} F_{u_{1,1}, u_{2,3}} F_{u_{2,3}} F_{u_{1,2}} - \frac{1}{16} \\
& F_{u_{1,3}}^2 F_{u_{1,2}, u_{2,2}} - \frac{1}{8} F_{u_{2,3}} F_{u_{1,1}} F_{u_{1,2}, u_{2,3}} + \frac{1}{8} F_{u_{1,3}} F_{u_{2,2}} F_{u_{1,2}, u_{1,3}} + \frac{1}{8} F_{u_{1,2}} F_{u_{1,2}, u_{1,2}} \\
& + \frac{1}{16} F_{u_{1,3}, u_{1,3}} F_{u_{2,3}}^2 F_{u_{1,2}} - \frac{1}{16} F_{u_{1,2}, u_{1,3}} F_{u_{2,3}} F_{u_{1,2}} + \frac{1}{16} F_{u_{1,3}} F_{u_{2,3}} F_{u_{1,2}, u_{1,2}}
\end{aligned}$$

$$\begin{aligned}
& + \frac{1}{16} F_{u_{1,3}} F_{u_{1,2}'} F_{u_{2,3}} F_{u_{1,2}} + \frac{1}{16} F_{u_{1,3}}^2 F_{u_{2,2}} F_{u_{1,3}'} F_{u_{2,3}} + \frac{1}{8} F_{u_{1,3}} F_{u_{2,3}} F_{u_{2,2}} F_{u_{1,3}'} F_{u_{1,3}} \\
& + \frac{1}{8} F_{u_{1,3}} F_{u_{2,3}} F_{u_{1,2}} F_{u_{1,3}'} F_{u_{2,3}} + \frac{1}{16} F_{u_{1,3}'} F_{u_{2,3}} F_{u_{1,1}}^2 - \frac{1}{4} F_{u_{1,2}'} F_{u_{2,2}} F_{u_{1,1}} \\
& + \frac{1}{2} F_{u_{1,2}} F_{u_{1,3}'} F_{u_{1,3}} F_{u_{2,2}} + \frac{1}{16} F_{u_{1,3}} F_{u_{1,2}} F_{u_{1,3}'} F_{u_{2,2}} + \frac{3}{16} F_{u_{2,3}}^2 F_{u_{1,1}'} F_{u_{1,2}} \\
& + \frac{1}{4} F_{u_{1,3}'} F_{u_{2,3}} F_{u_{1,2}}^2 + \frac{1}{8} F_{u_{1,3}} F_{u_{2,3}} F_{u_{1,1}'} F_{u_{2,2}} + \frac{1}{8} F_{u_{1,1}'} F_{u_{2,3}} F_{u_{1,3}} F_{u_{2,2}} \\
& + \frac{3}{4} F_{u_{2,2}} F_{u_{1,1}'} F_{u_{1,2}} + \frac{1}{4} F_{u_{1,2}} F_{u_{1,1}'} F_{u_{2,2}} + \frac{1}{2} F_{u_{1,1}} F_{u_{1,3}'} F_{u_{2,3}} F_{u_{2,2}} \\
& - \frac{1}{8} F_{u_{1,3}'} F_{u_{2,2}} F_{u_{2,3}} F_{u_{1,1}}', \blacklozenge, \frac{1}{2} F_{u_{2,2}} F_{u_{1,1}'} F_{u_{2,2}} - \frac{1}{4} F_{u_{2,2}} F_{u_{2,2}} F_{u_{1,1}} - \frac{1}{16} \\
& F_{u_{1,3}}^2 F_{u_{2,2}} F_{u_{2,2}} - \frac{1}{16} F_{u_{2,3}} F_{u_{1,2}} F_{u_{1,2}'} F_{u_{2,3}} + \frac{1}{16} F_{u_{1,3}'} F_{u_{1,3}} F_{u_{2,3}}^2 F_{u_{2,2}} \\
& + \frac{1}{4} F_{u_{1,2}'} F_{u_{1,2}} F_{u_{2,2}} + \frac{1}{2} F_{u_{1,2}} F_{u_{1,3}'} F_{u_{2,3}} F_{u_{2,2}} - \frac{1}{16} F_{u_{1,3}'} F_{u_{2,2}} F_{u_{2,3}} F_{u_{1,2}} \\
& + \frac{1}{8} F_{u_{1,3}} F_{u_{1,2}'} F_{u_{2,3}} F_{u_{2,2}} + \frac{1}{8} F_{u_{1,3}} F_{u_{2,2}} F_{u_{1,3}'} F_{u_{2,2}} + \frac{1}{16} F_{u_{2,3}}^2 F_{u_{1,2}'} F_{u_{1,2}} \\
& + \frac{1}{8} F_{u_{1,3}} F_{u_{2,3}} F_{u_{2,2}} F_{u_{1,3}'} F_{u_{2,3}} + \frac{1}{16} F_{u_{1,3}'} F_{u_{2,3}} F_{u_{1,2}}^2 + \frac{1}{4} F_{u_{1,3}'} F_{u_{1,3}} F_{u_{2,2}}^2 + \frac{1}{8} \\
& F_{u_{2,3}}^2 F_{u_{1,1}'} F_{u_{2,2}} + \frac{1}{16} F_{u_{1,3}} F_{u_{2,2}} F_{u_{2,3}} F_{u_{1,2}} - \frac{1}{8} F_{u_{2,3}} F_{u_{1,1}} F_{u_{2,2}} F_{u_{2,3}}', \blacklozenge, \\
& - \frac{1}{8} F_{u_{1,2}} F_{u_{2,2}} F_{u_{2,2}} + \frac{1}{16} F_{u_{2,3}}^2 F_{u_{1,2}} F_{u_{2,2}} + \frac{1}{16} F_{u_{1,3}'} F_{u_{2,3}} F_{u_{2,2}}^2 + \frac{1}{4} F_{u_{1,3}'} F_{u_{2,3}} \\
& F_{u_{2,2}}^2 + \frac{1}{4} F_{u_{2,2}} F_{u_{1,2}'} F_{u_{2,2}} + \frac{1}{8} F_{u_{1,3}} F_{u_{2,2}} F_{u_{2,3}} F_{u_{2,2}} - \frac{1}{16} F_{u_{1,3}} F_{u_{2,3}} F_{u_{2,2}} F_{u_{2,2}} \\
& - \frac{1}{16} F_{u_{2,3}} F_{u_{1,2}} F_{u_{2,2}} F_{u_{2,3}} \Big]
\end{aligned}$$

**E** >  $\text{Res212b} := \text{factor}([\text{diff}(\text{Res212}, u[1, 1, 1, 1, 3]), \blacklozenge, \text{diff}(\text{Res212}, u[1, 1, 1, 2, 3]), \blacklozenge, \text{diff}(\text{Res212}, u[1, 1, 2, 2, 3]), \blacklozenge, \text{diff}(\text{Res212}, u[1, 2, 2, 2, 3]), \blacklozenge, \text{diff}(\text{Res212}, u[2, 2, 2, 2, 3])])$

$$\text{Res212b} := \left[ \frac{1}{16} \left( F_{u_{1,3}} F_{u_{1,3}'} F_{u_{1,3}} + 2 F_{u_{1,1}'} F_{u_{1,3}} \right) \left( 4 F_{u_{1,1}} + F_{u_{1,3}}^2 \right), \blacklozenge, \frac{3}{16} \right. \quad (32)$$

$$\begin{aligned}
& F_{u_{1,3}}^2 F_{u_{2,3}} F_{u_{1,3}'} F_{u_{1,3}} + \frac{5}{16} F_{u_{2,3}} F_{u_{1,3}} F_{u_{1,1}'} F_{u_{1,3}} + \frac{1}{4} F_{u_{1,1}} F_{u_{1,2}'} F_{u_{1,3}} \\
& + \frac{5}{16} F_{u_{1,2}} F_{u_{1,3}} F_{u_{1,3}'} F_{u_{1,3}} + \frac{1}{16} F_{u_{1,3}}^3 F_{u_{1,3}'} F_{u_{2,3}} + \frac{1}{8} F_{u_{2,3}} F_{u_{1,1}} F_{u_{1,3}'} F_{u_{1,3}}
\end{aligned}$$

$$\begin{aligned}
& + \frac{1}{4} F_{u_{1,1}} F_{u_{1,3}} F_{u_{1,3}u_{2,3}} + \frac{1}{16} F_{u_{1,1}u_{2,3}} F_{u_{1,3}}^2 + \frac{5}{8} F_{u_{1,2}} F_{u_{1,1}u_{1,3}} \\
& + \frac{1}{4} F_{u_{1,1}} F_{u_{1,1}u_{2,3}} + \frac{1}{16} F_{u_{1,3}}^2 F_{u_{1,2}u_{1,3}}, \blacklozenge, \frac{3}{16} F_{u_{1,3}} F_{u_{2,3}} F_{u_{1,2}u_{1,3}} \\
& + \frac{3}{8} F_{u_{1,2}} F_{u_{1,2}u_{1,3}} + \frac{3}{16} F_{u_{1,3}}^2 F_{u_{2,3}} F_{u_{1,3}u_{2,3}} + \frac{3}{16} F_{u_{1,3}} F_{u_{2,3}}^2 F_{u_{1,3}u_{1,3}} \\
& + \frac{3}{16} F_{u_{1,1}u_{2,3}} F_{u_{1,3}} F_{u_{2,3}} + \frac{3}{8} F_{u_{2,2}} F_{u_{1,3}} F_{u_{1,3}u_{1,3}} + \frac{3}{16} F_{u_{1,2}} F_{u_{2,3}} F_{u_{1,3}u_{1,3}} \\
& + \frac{3}{8} F_{u_{1,2}} F_{u_{1,3}} F_{u_{1,3}u_{2,3}} + \frac{3}{16} F_{u_{2,3}}^2 F_{u_{1,1}u_{1,3}} + \frac{3}{8} F_{u_{1,1}u_{2,3}} F_{u_{1,2}} \\
& + \frac{3}{4} F_{u_{2,2}} F_{u_{1,1}u_{1,3}}, \blacklozenge, \frac{1}{8} F_{u_{2,3}}^2 F_{u_{1,1}u_{2,3}} + \frac{1}{2} F_{u_{2,2}} F_{u_{1,1}u_{2,3}} - \frac{1}{4} F_{u_{1,1}} F_{u_{2,2}u_{2,3}} \\
& - \frac{1}{16} F_{u_{1,3}}^2 F_{u_{2,2}u_{2,3}} + \frac{1}{16} F_{u_{1,3}} F_{u_{2,3}} F_{u_{1,2}u_{2,3}} + \frac{1}{8} F_{u_{1,2}} F_{u_{1,2}u_{2,3}} + \frac{3}{16} F_{u_{1,3}} \\
& F_{u_{2,3}}^2 F_{u_{1,3}u_{2,3}} + \frac{1}{8} F_{u_{1,2}} F_{u_{1,3}u_{2,3}} F_{u_{2,3}} + \frac{1}{2} F_{u_{2,2}} F_{u_{1,3}} F_{u_{1,3}u_{2,3}} \\
& + \frac{1}{4} F_{u_{2,2}} F_{u_{1,3}u_{1,3}} F_{u_{2,3}} + \frac{1}{16} F_{u_{1,3}} F_{u_{2,3}} F_{u_{1,3}u_{2,2}} + \frac{1}{2} F_{u_{2,2}} F_{u_{1,2}u_{1,3}} \\
& + \frac{1}{8} F_{u_{1,2}} F_{u_{1,3}u_{2,2}} + \frac{1}{8} F_{u_{1,2}u_{1,3}} F_{u_{2,3}}^2 + \frac{1}{16} F_{u_{1,3}u_{1,3}} F_{u_{2,3}}^3 \\
& + \frac{1}{16} F_{u_{1,2}} F_{u_{1,3}} F_{u_{2,3}u_{2,3}} - \frac{1}{8} F_{u_{1,1}} F_{u_{2,3}} F_{u_{2,3}u_{2,3}}, \blacklozenge, -\frac{1}{8} F_{u_{1,2}} F_{u_{2,2}u_{2,3}} + \frac{1}{16} \\
& F_{u_{2,3}}^2 F_{u_{1,2}u_{2,3}} + \frac{1}{4} F_{u_{2,2}} F_{u_{1,3}u_{2,2}} + \frac{1}{4} F_{u_{2,2}} F_{u_{1,3}u_{2,3}} F_{u_{2,3}} + \frac{1}{4} F_{u_{2,2}} F_{u_{1,2}u_{2,3}} \\
& + \frac{1}{16} F_{u_{1,3}u_{2,2}} F_{u_{2,3}}^2 + \frac{1}{16} F_{u_{1,3}u_{2,3}} F_{u_{2,3}}^3 + \frac{1}{8} F_{u_{2,2}} F_{u_{1,3}} F_{u_{2,3}u_{2,3}} \\
& - \frac{1}{16} F_{u_{1,3}} F_{u_{2,3}} F_{u_{2,2}u_{2,3}} - \frac{1}{16} F_{u_{1,2}} F_{u_{2,3}} F_{u_{2,3}u_{2,3}} \Big]
\end{aligned}$$

**E** > *simplify*([*diff*(*Res212*, *u*[1, 1, 1, 3, 3]),  $\blacklozenge$ , *diff*(*Res212*, *u*[1, 1, 2, 3, 3]),  $\blacklozenge$ ,  
*diff*(*Res212*, *u*[1, 2, 2, 3, 3]),  $\blacklozenge$ , *diff*(*Res212*, *u*[2, 2, 2, 3, 3]),  $\blacklozenge$ , *diff*(*Res212*, *u*[1,  
1, 3, 3, 3]),  $\blacklozenge$ , *diff*(*Res212*, *u*[1, 2, 3, 3, 3]),  $\blacklozenge$ , *diff*(*Res212*, *u*[2, 2, 3, 3, 3]),  $\blacklozenge$ ,  
*diff*(*Res212*, *u*[1, 3, 3, 3, 3]),  $\blacklozenge$ , *diff*(*Res212*, *u*[2, 2, 3, 3, 3]),  $\blacklozenge$ , *diff*(*Res212*, *u*[3,  
3, 3, 3, 3])])  
[0,  $\blacklozenge$ , 0,  $\blacklozenge$ , 0,  $\blacklozenge$ , 0,  $\blacklozenge$ , 0,  $\blacklozenge$ , 0,  $\blacklozenge$ , 0,  $\blacklozenge$ , 0,  $\blacklozenge$ , 0]

(33)

**E** > *Res212a*[9]

$$\frac{1}{2} F_{u_{2,2}} F_{u_{1,1}u_{2,2}} - \frac{1}{4} F_{u_{2,2}u_{2,2}} F_{u_{1,1}} - \frac{1}{16} F_{u_{1,3}}^2 F_{u_{2,2}u_{2,2}} - \frac{1}{16} F_{u_{2,3}} F_{u_{1,2}} F_{u_{1,2}u_{2,3}}$$

(34)

$$\begin{aligned}
& + \frac{1}{16} F_{u_{1,3}, u_{1,3}} F_{u_{2,3}}^2 F_{u_{2,2}} + \frac{1}{4} F_{u_{1,2}, u_{1,2}} F_{u_{2,2}} + \frac{1}{2} F_{u_{1,2}} F_{u_{1,3}, u_{2,3}} F_{u_{2,2}} \\
& - \frac{1}{16} F_{u_{1,3}, u_{2,2}} F_{u_{2,3}} F_{u_{1,2}} + \frac{1}{8} F_{u_{1,3}} F_{u_{1,2}, u_{2,3}} F_{u_{2,2}} + \frac{1}{8} F_{u_{1,3}} F_{u_{2,2}} F_{u_{1,3}, u_{2,2}} + \frac{1}{16} \\
& F_{u_{2,3}}^2 F_{u_{1,2}, u_{1,2}} + \frac{1}{8} F_{u_{1,3}} F_{u_{2,3}} F_{u_{2,2}} F_{u_{1,3}, u_{2,3}} + \frac{1}{16} F_{u_{1,3}, u_{2,3}} F_{u_{2,3}}^2 F_{u_{1,2}} \\
& + \frac{1}{4} F_{u_{1,3}, u_{1,3}} F_{u_{2,2}}^2 + \frac{1}{8} F_{u_{2,3}}^2 F_{u_{1,1}, u_{2,2}} + \frac{1}{16} F_{u_{1,3}} F_{u_{2,2}, u_{2,3}} F_{u_{1,2}} \\
& - \frac{1}{8} F_{u_{2,3}} F_{u_{1,1}} F_{u_{2,2}, u_{2,3}}
\end{aligned}$$

$$\begin{aligned}
\mathbf{E} & > \text{factor} \left( \text{subs} \left( \left\{ f_r = -\frac{1}{4} f_a^2, f_{ar} = -\frac{1}{2} f_a f_{aa}, f_{br} = -\frac{1}{2} f_a f_{ab}, f_{rr} = \frac{1}{4} f_a^2 f_{aa}, f_{rs} = -\frac{1}{2} f_a \left( -\frac{1}{2} f_b f_{aa} \right. \right. \right. \\
& \left. \left. \left. - \frac{1}{2} f_a f_{ab} \right), f_{rt} = -\frac{1}{2} f_a f_{ar} f_{tt} = -f_b f_{bb}, f_{bt} = -\frac{1}{2} f_b f_{bb}, f_{st} = -\frac{1}{2} f_s f_{bb} - f_b f_{ab}, f_{bs} = -f_{at} - f_b f_{ab} \right. \right. \\
& \left. \left. - \frac{1}{2} f_b f_{bb}, f_{as} = -\frac{1}{2} f_b f_{aa} - \frac{1}{2} f_a f_{ab}, f_{ss} = \frac{1}{4} f_{bb} f_a^2 + f_a f_{at} + \frac{1}{4} f_{aa} f_b^2 - 2 f_s f_{ab} \right\}, \right. \\
& \text{subs} \left( \text{Sub}, \frac{1}{2} F_{u_{2,2}} F_{u_{1,1}, u_{2,2}} - \frac{1}{4} F_{u_{2,2}, u_{2,2}} F_{u_{1,1}} - \frac{1}{16} F_{u_{1,3}}^2 F_{u_{2,2}, u_{2,2}} \right. \\
& \left. - \frac{1}{16} F_{u_{2,3}} F_{u_{1,2}} F_{u_{1,2}, u_{2,3}} + \frac{1}{16} F_{u_{1,3}, u_{1,3}} F_{u_{2,3}}^2 F_{u_{2,2}} + \frac{1}{4} F_{u_{1,2}, u_{1,2}} F_{u_{2,2}} \right. \\
& \left. + \frac{1}{2} F_{u_{1,2}} F_{u_{1,3}, u_{2,3}} F_{u_{2,2}} - \frac{1}{16} F_{u_{1,3}, u_{2,2}} F_{u_{2,3}} F_{u_{1,2}} + \frac{1}{8} F_{u_{1,3}} F_{u_{1,2}, u_{2,3}} F_{u_{2,2}} \right. \\
& \left. + \frac{1}{8} F_{u_{1,3}} F_{u_{2,2}} F_{u_{1,3}, u_{2,2}} + \frac{1}{16} F_{u_{2,3}}^2 F_{u_{1,2}, u_{1,2}} + \frac{1}{8} F_{u_{1,3}} F_{u_{2,3}} F_{u_{2,2}} F_{u_{1,3}, u_{2,3}} \right. \\
& \left. + \frac{1}{16} F_{u_{1,3}, u_{2,3}} F_{u_{2,3}}^2 F_{u_{1,2}} + \frac{1}{4} F_{u_{1,3}, u_{1,3}} F_{u_{2,2}}^2 + \frac{1}{8} F_{u_{2,3}}^2 F_{u_{1,1}, u_{2,2}} \right. \\
& \left. + \frac{1}{16} F_{u_{1,3}} F_{u_{2,2}, u_{2,3}} F_{u_{1,2}} - \frac{1}{8} F_{u_{2,3}} F_{u_{1,1}} F_{u_{2,2}, u_{2,3}} \right) \left. \right) \left. \right) \\
& \frac{1}{64} f_{aa} \left( 4 f_t + f_b^2 \right)^2
\end{aligned} \tag{35}$$

$\mathbf{E} > \#$  So **finally** the MAE condition is checked here as well!

$\mathbf{E} >$

$\mathbf{E} > \#$  The one case which is left over is  $2 f_s + f_a f_b = 0$

in the presence of the previous conditions  $\left\{ f_r = -\frac{1}{4} f_a^2, f_{ar} = -\frac{1}{2} f_a f_{aa}, f_{br} = -\frac{1}{2} f_a f_{ab}, f_{rr} = \frac{1}{4} f_a^2 f_{aa}, f_{rs} = -\frac{1}{2} f_a f_{as}, f_{rt} = -\frac{1}{2} f_a f_{ar} f_{tt} = -f_b f_{bb}, f_{bt} = -\frac{1}{2} f_b f_{bb}, f_{st} = -\frac{1}{2} f_s f_{bb} - f_b f_{ab}, f_{bs} = -f_{at} - f_b f_{ab} - \frac{1}{2} f_b f_{bb} \right\}$ . This is easy (the last condition

in the substitutions below is added on the basis of compatibility-equation  $f_{rs} = f_{sr}$

and the equation  $f_{ss} = \dots$  is deduced by prolongation). We first check what MAE are left :

$$\begin{aligned}
\mathbf{E} &> \text{factor}\left(\text{subs}\left(\left\{f_r = -\frac{1}{4}f_a^2, f_s = -\frac{1}{2}f_a f_b, f_{ar} = -\frac{1}{2}f_a f_{aa}, f_{br} = -\frac{1}{2}f_a f_{ab}, f_{rr} = \frac{1}{4}f_a^2 f_{aa}, f_{rs} = \right. \right. \\
&\quad \left. \left. -\frac{1}{2}f_a \left(-\frac{1}{2}f_b f_{aa} - \frac{1}{2}f_a f_{ab}\right), f_{rt} = -\frac{1}{2}f_a f_{at}, f_{tt} = -f_b f_{bb}, f_{bt} = -\frac{1}{2}f_b f_{bb}, f_{st} = -\frac{1}{2} \left( \right. \right. \\
&\quad \left. \left. -\frac{1}{2}f_a f_b \right) f_{bb} - f_b f_{ab}, f_{bs} = -f_{at} - f_b f_{ab} - \frac{1}{2}f_a f_{bb}, f_{as} = -\frac{1}{2}f_b f_{aa} - \frac{1}{2}f_a f_{ab} \right\}, [f_{aa}f_a + 2f_{ar}, \\
&\quad \blacklozenge, f_{bb}f_b + 2f_{br}, \blacklozenge, f_{aa}f_b + 2f_{ab}f_a + 2f_{as} + 2f_{br}, \blacklozenge, f_{bb}f_a + 2f_{ab}f_b + 2f_{bs} + 2f_{at}, \blacklozenge, f_{aa}f_r \\
&\quad + f_{rr}, \blacklozenge, f_{bb}f_t + f_{tt}, \blacklozenge, f_{aa}f_s + 2f_{ab}f_r + 2f_{rs}, \blacklozenge, f_{bb}f_s + 2f_{ab}f_t + 2f_{st}, \blacklozenge, f_{aa}f_t + f_{bb}f_r \\
&\quad + 2f_{ab}f_s + 2f_{rt} + f_{ss}]) \right) \\
&\quad \left[ 0, \blacklozenge, 0, \blacklozenge, 0, \blacklozenge, 0, \blacklozenge, 0, \blacklozenge, 0, \blacklozenge, 0, \blacklozenge, f_{aa}f_t - \frac{1}{4}f_{bb}f_a^2 - f_{ab}f_a f_b - f_a f_{at} + f_{ss} \right]
\end{aligned} \tag{36}$$

$$\begin{aligned}
\mathbf{E} &> \text{factor}\left(\text{subs}\left(\left\{f_r = -\frac{1}{4}f_a^2, f_s = -\frac{1}{2}f_a f_b, f_{ss} = -\frac{1}{2}f_a \left(-f_{at} - f_b f_{ab} - \frac{1}{2}f_a f_{bb}\right) - \frac{1}{2}f_b \left(-\frac{1}{2}f_b f_{aa} \right. \right. \right. \\
&\quad \left. \left. - \frac{1}{2}f_a f_{ab}\right), f_{ar} = -\frac{1}{2}f_a f_{aa}, f_{br} = -\frac{1}{2}f_a f_{ab}, f_{rr} = \frac{1}{4}f_a^2 f_{aa}, f_{rs} = -\frac{1}{2}f_a \left(-\frac{1}{2}f_b f_{aa} \right. \right. \\
&\quad \left. \left. - \frac{1}{2}f_a f_{ab}\right), f_{rt} = -\frac{1}{2}f_a f_{at}, f_{tt} = -f_b f_{bb}, f_{bt} = -\frac{1}{2}f_b f_{bb}, f_{st} = -\frac{1}{2} \left(-\frac{1}{2}f_a f_b\right) f_{bb} - f_b f_{ab}, f_{bs} = \\
&\quad -f_{at} - f_b f_{ab} - \frac{1}{2}f_a f_{bb}, f_{as} = -\frac{1}{2}f_b f_{aa} - \frac{1}{2}f_a f_{ab} \right\}, [f_{aa}f_a + 2f_{ar}, \blacklozenge, f_{bb}f_b + 2f_{br}, \blacklozenge, f_{aa}f_b \\
&\quad + 2f_{ab}f_a + 2f_{as} + 2f_{br}, \blacklozenge, f_{bb}f_a + 2f_{ab}f_b + 2f_{bs} + 2f_{at}, \blacklozenge, f_{aa}f_r + f_{rr}, \blacklozenge, f_{bb}f_t + f_{tt}, \blacklozenge, \\
&\quad f_{aa}f_s + 2f_{ab}f_r + 2f_{rs}, \blacklozenge, f_{bb}f_s + 2f_{ab}f_t + 2f_{st}, \blacklozenge, f_{aa}f_t + f_{bb}f_r + 2f_{ab}f_s + 2f_{rt} + f_{ss}]) \right) \\
&\quad \left[ 0, \blacklozenge, 0, \blacklozenge, 0, \blacklozenge, 0, \blacklozenge, 0, \blacklozenge, 0, \blacklozenge, 0, \blacklozenge, f_{aa}f_t - \frac{1}{4}f_{ab}f_a f_b - \frac{1}{2}f_a f_{at} + \frac{1}{4}f_{aa}f_b^2 \right]
\end{aligned} \tag{37}$$

$\mathbf{E} > \#$  Thus only the last MAE condition must be obtained. Here it is :

$\mathbf{E} > \text{Res212a}[9]$

$$\begin{aligned}
&\frac{1}{2}F_{u,2,2}F_{u,1,1}u_{2,2} - \frac{1}{4}F_{u,2,2}u_{2,2}F_{u,1,1} - \frac{1}{16}F_{u,1,3}^2F_{u,2,2}u_{2,2} - \frac{1}{16}F_{u,2,3}F_{u,1,2}F_{u,1,2}u_{2,3} \\
&+ \frac{1}{16}F_{u,1,3}u_{1,3}F_{u,2,3}^2F_{u,2,2} + \frac{1}{4}F_{u,1,2}u_{1,2}F_{u,2,2} + \frac{1}{2}F_{u,1,2}F_{u,1,3}u_{2,3}F_{u,2,2} \\
&- \frac{1}{16}F_{u,1,3}u_{2,2}F_{u,2,3}F_{u,1,2} + \frac{1}{8}F_{u,1,3}F_{u,1,2}u_{2,3}F_{u,2,2} + \frac{1}{8}F_{u,1,3}F_{u,2,2}F_{u,1,3}u_{2,2} + \frac{1}{16} \\
&F_{u,2,3}^2F_{u,1,2}u_{1,2} + \frac{1}{8}F_{u,1,3}F_{u,2,3}F_{u,2,2}F_{u,1,3}u_{2,3} + \frac{1}{16}F_{u,1,3}u_{2,3}F_{u,2,3}^2F_{u,1,2} \\
&+ \frac{1}{4}F_{u,1,3}u_{1,3}F_{u,2,2}^2 + \frac{1}{8}F_{u,2,3}^2F_{u,1,1}u_{2,2} + \frac{1}{16}F_{u,1,3}F_{u,2,2}u_{2,3}F_{u,1,2} \\
&- \frac{1}{8}F_{u,2,3}F_{u,1,1}F_{u,2,2}u_{2,3}
\end{aligned} \tag{38}$$

$$\begin{aligned}
\mathbf{E} &> \text{factor}\left(\text{subs}\left(\left\{f_r = -\frac{1}{4}f_a^2, f_s = -\frac{1}{2}f_a f_b, f_{ss} = -\frac{1}{2}f_a \left(-f_{at} - f_b f_{ab} - \frac{1}{2}f_a f_{bb}\right) - \frac{1}{2}f_b \left(-\frac{1}{2}f_b f_{aa} \right. \right. \right. \\
&\quad \left. \left. - \frac{1}{2}f_a f_{ab}\right), f_{ar} = -\frac{1}{2}f_a f_{aa}, f_{br} = -\frac{1}{2}f_a f_{ab}, f_{rr} = \frac{1}{4}f_a^2 f_{aa}, f_{rs} = -\frac{1}{2}f_a \left(-\frac{1}{2}f_b f_{aa} \right. \right.
\end{aligned}$$



$$\begin{aligned}
& -\frac{1}{2}f_{ab}) , f_{rt} = -\frac{1}{2}f_a f_{ar}, f_{tt} = -f_{bb}, f_{bt} = -\frac{1}{2}f_{bb}, f_{st} = -\frac{1}{2} \left( -\frac{1}{2}f_{ab} \right) f_{bb} - f_{ab}, f_{bs} = \\
& -f_{at} - f_{bb} - \frac{1}{2}f_{bb}, f_{as} = -\frac{1}{2}f_{ba} - \frac{1}{2}f_{ab} \}, subs \left( Sub, \frac{1}{2} F_{u_{2,2}} F_{u_{1,1}}^{u_{2,2}} \right. \\
& -\frac{1}{4} F_{u_{2,2}}^{u_{2,2}} F_{u_{1,1}} - \frac{1}{16} F_{u_{1,3}}^2 F_{u_{2,2}}^{u_{2,2}} - \frac{1}{16} F_{u_{2,3}} F_{u_{1,2}} F_{u_{1,2}}^{u_{2,3}} \\
& + \frac{1}{16} F_{u_{1,3}}^{u_{1,3}} F_{u_{2,3}}^2 F_{u_{2,2}} + \frac{1}{4} F_{u_{1,2}}^{u_{1,2}} F_{u_{2,2}} + \frac{1}{2} F_{u_{1,2}} F_{u_{1,3}}^{u_{2,3}} F_{u_{2,2}} \\
& - \frac{1}{16} F_{u_{1,3}}^{u_{2,2}} F_{u_{2,3}} F_{u_{1,2}} + \frac{1}{8} F_{u_{1,3}} F_{u_{1,2}}^{u_{2,3}} F_{u_{2,2}} + \frac{1}{8} F_{u_{1,3}} F_{u_{2,2}} F_{u_{1,3}}^{u_{2,2}} \\
& + \frac{1}{16} F_{u_{2,3}}^2 F_{u_{1,2}}^{u_{1,2}} + \frac{1}{8} F_{u_{1,3}} F_{u_{2,3}} F_{u_{2,2}} F_{u_{1,3}}^{u_{2,3}} + \frac{1}{16} F_{u_{1,3}}^{u_{2,3}} F_{u_{2,3}}^2 F_{u_{1,2}} \\
& + \frac{1}{4} F_{u_{1,3}}^{u_{1,3}} F_{u_{2,2}}^2 + \frac{1}{8} F_{u_{2,3}}^2 F_{u_{1,1}}^{u_{2,2}} + \frac{1}{16} F_{u_{1,3}} F_{u_{2,2}}^{u_{2,3}} F_{u_{1,2}} \\
& \left. \left. \left. - \frac{1}{8} F_{u_{2,3}} F_{u_{1,1}} F_{u_{2,2}}^{u_{2,3}} \right) \right) \right) \\
& - \frac{1}{64} (f_b^2 + 4f_t) (-f_{aa}f_b^2 + f_a f_{ab} f_b + 2f_a f_{at} - 4f_{aa}f_t)
\end{aligned} \tag{39}$$

**E** > # Therefore we are done with the first singular case!

**E** >

**E** > # Now we shall check the second singular case given by the condition  $f_a^2 + 4f_r = f_b^2 + 4f_t = 0$

**E** > factor  $\left( subs \left( \left\{ f_r = -\frac{1}{4}f_a^2, f_t = -\frac{1}{4}f_b^2, f_{ar} = -\frac{1}{2}f_a f_{aa}, f_{at} = -\frac{1}{2}f_b f_{ab}, f_{br} = -\frac{1}{2}f_a f_{ab}, f_{bt} = \right. \right.$   
 $\left. -\frac{1}{2}f_b f_{bb}, f_{rr} = \frac{1}{4}f_a^2 f_{aa}, f_{rs} = -\frac{1}{2}f_a f_{as}, f_{rt} = \frac{1}{4}f_a f_b f_{ab}, f_{st} = -\frac{1}{2}f_b f_{bs}, f_{tt} = \frac{1}{4}f_b^2 f_{bb} \right\},$   
 $[f_{aa}f_a + 2f_{ar}, \blacklozenge, f_{bb}f_b + 2f_{br}, \blacklozenge, f_{aaf_b} + 2f_{ab}f_a + 2f_{as} + 2f_{br}, \blacklozenge, f_{bbf_a} + 2f_{ab}f_b + 2f_{bs}$   
 $+ 2f_{ar}, \blacklozenge, f_{aaf_r} + f_{rr}, \blacklozenge, f_{bbf_t} + f_{tt}, \blacklozenge, f_{aaf_s} + 2f_{ab}f_r + 2f_{rs}, \blacklozenge, f_{bbf_s} + 2f_{ab}f_t + 2f_{st}, \blacklozenge,$   
 $f_{aaf_t} + f_{bbf_r} + 2f_{ab}f_s + 2f_{rt} + f_{ss}]) \right)$

$$\begin{aligned}
& \left[ 0, \blacklozenge, 0, \blacklozenge, f_a f_{ab} + f_{aa}f_b + 2f_{as}, \blacklozenge, f_{bb}f_a + f_b f_{ab} + 2f_{bs}, \blacklozenge, 0, \blacklozenge, 0, \blacklozenge, f_{aa}f_s - \frac{1}{2}f_{ab}f_a^2 \right. \\
& \left. - f_a f_{as}, \blacklozenge, f_{bb}f_s - \frac{1}{2}f_{ab}f_b^2 - f_b f_{bs}, \blacklozenge, -\frac{1}{4}f_{aa}f_b^2 - \frac{1}{4}f_{bb}f_a^2 + 2f_{ab}f_s + \frac{1}{2}f_a f_b f_{ab} + f_{ss} \right]
\end{aligned} \tag{40}$$

**E** >

**E** > Res112a[3]

$$\begin{aligned}
& \frac{1}{16} F_{u_{1,1}}^{u_{2,3}} F_{u_{1,3}} F_{u_{1,2}} - \frac{1}{2} F_{u_{1,1}} F_{u_{1,3}}^{u_{2,3}} F_{u_{1,2}} - \frac{1}{16} F_{u_{1,3}}^2 F_{u_{2,3}}^{u_{2,3}} F_{u_{1,1}} - \frac{1}{8} \\
& F_{u_{1,3}}^2 F_{u_{1,1}}^{u_{2,2}} + \frac{1}{16} F_{u_{1,1}}^{u_{1,1}} F_{u_{2,3}}^2 - \frac{1}{4} F_{u_{1,1}} F_{u_{1,2}}^{u_{1,2}} - \frac{1}{16} F_{u_{1,3}}^2 F_{u_{1,2}}^{u_{1,2}} \\
& - \frac{1}{8} F_{u_{1,2}}^{u_{1,3}} F_{u_{2,3}} F_{u_{1,1}} + \frac{1}{4} F_{u_{2,2}} F_{u_{1,1}}^{u_{1,1}} - \frac{1}{16} F_{u_{1,1}}^{u_{1,3}} F_{u_{1,2}} F_{u_{2,3}}
\end{aligned} \tag{41}$$

$$\begin{aligned}
& + \frac{1}{8} F_{u,2,2} F_{u,1,1} u_{1,3} F_{u,1,3} - \frac{1}{2} F_{u,1,1} F_{u,1,1} u_{2,2} - \frac{1}{8} F_{u,1,3} F_{u,2,3} F_{u,1,1} F_{u,1,3} u_{2,3} \\
& - \frac{1}{8} F_{u,2,3} F_{u,1,1} F_{u,1,1} u_{2,3} - \frac{1}{16} F_{u,1,3}^2 F_{u,1,2} F_{u,1,3} u_{2,3} - \frac{1}{4} F_{u,2,3} u_{2,3} F_{u,1,1}^2 \\
& + \frac{1}{16} F_{u,1,3} F_{u,1,2} F_{u,1,2} u_{1,3}
\end{aligned}$$

$$\begin{aligned}
\mathbf{E} > \text{factor} \left( \text{subs} \left( \left\{ f_r = -\frac{1}{4} f_a^2, f_t = -\frac{1}{4} f_b^2, f_{ar} = -\frac{1}{2} f_a f_{aa}, f_{at} = -\frac{1}{2} f_b f_{ab}, f_{br} = -\frac{1}{2} f_a f_{ab}, f_{bt} = \right. \right. \\
& \left. \left. -\frac{1}{2} f_b f_{bb}, f_{rr} = \frac{1}{4} f_a^2 f_{aa}, f_{rs} = -\frac{1}{2} f_a f_{as}, f_{rt} = \frac{1}{4} f_a f_b f_{ab}, f_{st} = -\frac{1}{2} f_b f_{bs}, f_{tt} = \frac{1}{4} f_b^2 f_{bb} \right\}, \right. \\
& \text{subs} \left( \text{Sub}, \frac{1}{16} F_{u,1,1} u_{2,3} F_{u,1,3} F_{u,1,2} - \frac{1}{2} F_{u,1,1} F_{u,1,3} u_{2,3} F_{u,1,2} - \frac{1}{16} \right. \\
& F_{u,1,3}^2 F_{u,2,3} u_{2,3} F_{u,1,1} - \frac{1}{8} F_{u,1,3}^2 F_{u,1,1} u_{2,2} + \frac{1}{16} F_{u,1,1} u_{1,1} F_{u,2,3}^2 - \frac{1}{4} F_{u,1,1} F_{u,1,2} u_{1,2} \\
& - \frac{1}{16} F_{u,1,3}^2 F_{u,1,2} u_{1,2} - \frac{1}{8} F_{u,1,2} u_{1,3} F_{u,2,3} F_{u,1,1} + \frac{1}{4} F_{u,2,2} F_{u,1,1} u_{1,1} \\
& - \frac{1}{16} F_{u,1,1} u_{1,3} F_{u,1,2} F_{u,2,3} + \frac{1}{8} F_{u,2,2} F_{u,1,1} u_{1,3} F_{u,1,3} - \frac{1}{2} F_{u,1,1} F_{u,1,1} u_{2,2} \\
& - \frac{1}{8} F_{u,1,3} F_{u,2,3} F_{u,1,1} F_{u,1,3} u_{2,3} - \frac{1}{8} F_{u,2,3} F_{u,1,1} F_{u,1,1} u_{2,3} - \frac{1}{16} \\
& \left. \left. F_{u,1,3}^2 F_{u,1,2} F_{u,1,3} u_{2,3} - \frac{1}{4} F_{u,2,3} u_{2,3} F_{u,1,1}^2 + \frac{1}{16} F_{u,1,3} F_{u,1,2} F_{u,1,2} u_{1,3} \right) \right) \right) \\
& \frac{1}{64} f_a (f_a f_b + 2 f_s) (f_a f_{ab} + f_{aa} f_b + 2 f_{as}) \quad (42)
\end{aligned}$$

$\mathbf{E} > \#$  assuming presently  $(f_a, f_b) \neq (0, 0)$  and  $f_a f_b + 2 f_s \neq 0$

$$\begin{aligned}
\mathbf{E} > \text{factor} \left( \text{subs} \left( \left\{ f_r = -\frac{1}{4} f_a^2, f_t = -\frac{1}{4} f_b^2, f_{ar} = -\frac{1}{2} f_a f_{aa}, f_{at} = -\frac{1}{2} f_b f_{ab}, f_{br} = -\frac{1}{2} f_a f_{ab}, f_{bt} = \right. \right. \right. \\
& \left. \left. -\frac{1}{2} f_b f_{bb}, f_{rr} = \frac{1}{4} f_a^2 f_{aa}, f_{rr} = \frac{1}{4} f_a^2 f_{aa}, f_{rs} = f_a \frac{f_a f_{ab} + f_{aa} f_b}{4}, f_{rt} = \frac{1}{4} f_a f_b f_{ab}, f_{st} \right. \right. \\
& \left. \left. = f_b \frac{f_b f_{ab} + f_{bb} f_a}{4}, f_{tt} = \frac{1}{4} f_b^2 f_{bb}, f_{as} = -\frac{f_a f_{ab} + f_{aa} f_b}{2}, f_{bs} = -\frac{f_b f_{ab} + f_{bb} f_a}{2} \right\}, [f_{aa} f_a \right. \\
& + 2 f_{ar}, \blacklozenge, f_{bb} f_b + 2 f_{br}, \blacklozenge, f_{aa} f_b + 2 f_{ab} f_a + 2 f_{as} + 2 f_{br}, \blacklozenge, f_{bb} f_a + 2 f_{ab} f_b + 2 f_{bs} \\
& + 2 f_{ar}, \blacklozenge, f_{aa} f_r + f_{rr}, \blacklozenge, f_{bb} f_t + f_{tt}, \blacklozenge, f_{aa} f_s + 2 f_{ab} f_r + 2 f_{rs}, \blacklozenge, f_{bb} f_s + 2 f_{ab} f_t + 2 f_{st}, \blacklozenge, \\
& \left. \left. f_{aa} f_t + f_{bb} f_r + 2 f_{ab} f_s + 2 f_{rt} + f_{ss} \right] \right) \\
& \left[ 0, \blacklozenge, 0, \blacklozenge, 0, \blacklozenge, 0, \blacklozenge, 0, \blacklozenge, \frac{1}{2} f_{aa} (f_a f_b + 2 f_s), \blacklozenge, \frac{1}{2} f_{bb} (f_a f_b + 2 f_s), \blacklozenge, -\frac{1}{4} f_{aa} f_b^2 \right. \\
& \left. - \frac{1}{4} f_{bb} f_a^2 + 2 f_{ab} f_s + \frac{1}{2} f_a f_b f_{ab} + f_{ss} \right] \quad (43)
\end{aligned}$$

$\mathbf{E} >$

$\mathbf{E} > \text{Res112a}[5]$

(44)

$$\begin{aligned}
& \frac{1}{8} F_{u_{1,1},u_{2,3}} F_{u_{1,3}} F_{u_{2,2}} - \frac{1}{2} F_{u_{1,1}} F_{u_{1,3},u_{2,3}} F_{u_{2,2}} - \frac{1}{16} F_{u_{1,1},u_{2,3}} F_{u_{2,3}} F_{u_{1,2}} \\
& - \frac{1}{2} F_{u_{1,1}} F_{u_{2,3},u_{2,3}} F_{u_{1,2}} - \frac{1}{16} F_{u_{1,3}}^2 F_{u_{2,3},u_{2,3}} F_{u_{1,2}} - \frac{3}{4} F_{u_{1,1}} F_{u_{1,2},u_{2,2}} \\
& + \frac{1}{4} F_{u_{1,1},u_{1,2}} F_{u_{2,2}} - \frac{1}{8} F_{u_{1,2}} F_{u_{1,2},u_{1,2}} - \frac{1}{8} F_{u_{1,3},u_{2,2}} F_{u_{2,3}} F_{u_{1,1}} + \frac{1}{16} \\
& F_{u_{2,3}}^2 F_{u_{1,1},u_{1,2}} - \frac{3}{16} F_{u_{1,3}}^2 F_{u_{1,2},u_{2,2}} - \frac{1}{16} F_{u_{1,3}}^2 F_{u_{2,2}} F_{u_{1,3},u_{2,3}} \\
& + \frac{1}{16} F_{u_{1,3}} F_{u_{1,2},u_{2,3}} F_{u_{1,2}} - \frac{1}{16} F_{u_{1,2},u_{1,3}} F_{u_{2,3}} F_{u_{1,2}} - \frac{1}{16} F_{u_{1,3}} F_{u_{2,3}} F_{u_{1,2},u_{1,2}} \\
& - \frac{1}{4} F_{u_{1,1},u_{2,2}} F_{u_{1,2}} - \frac{1}{8} F_{u_{1,3}} F_{u_{2,3}} F_{u_{1,1},u_{2,2}} - \frac{1}{8} F_{u_{1,3}} F_{u_{2,3}} F_{u_{1,2}} F_{u_{1,3},u_{2,3}} \\
& - \frac{1}{4} F_{u_{1,3},u_{2,3}} F_{u_{1,2}}^2 - \frac{1}{8} F_{u_{1,3}} F_{u_{2,3}} F_{u_{1,1}} F_{u_{2,3},u_{2,3}} + \frac{1}{16} F_{u_{1,3}} F_{u_{1,2}} F_{u_{1,3},u_{2,2}} \\
& - \frac{1}{16} F_{u_{1,3},u_{2,3}} F_{u_{2,3}}^2 F_{u_{1,1}} - \frac{1}{8} F_{u_{2,3}} F_{u_{1,1}} F_{u_{1,2},u_{2,3}} + \frac{1}{8} F_{u_{1,3}} F_{u_{2,2}} F_{u_{1,2},u_{1,3}}
\end{aligned}
\tag{44}$$

$$\begin{aligned}
\mathbf{E} & > factor \left( subs \left( \left\{ f_r = -\frac{1}{4} f_a^2, f_t = -\frac{1}{4} f_b^2, f_{ar} = -\frac{1}{2} f_a f_{aa}, f_{at} = -\frac{1}{2} f_b f_{ab}, f_{br} = -\frac{1}{2} f_a f_{ab}, f_{bt} = \right. \right. \\
& - \frac{1}{2} f_b f_{bb}, f_{rr} = \frac{1}{4} f_a^2 f_{aa}, f_{rs} = f_a \frac{f_a f_{ab} + f_{aa} f_b}{4}, f_{rt} = \frac{1}{4} f_a f_b f_{ab}, f_{st} = f_b \frac{f_b f_{ab} + f_{bb} f_a}{4}, f_{tt} \\
& = \frac{1}{4} f_b^2 f_{bb}, f_{as} = -\frac{f_a f_{ab} + f_{aa} f_b}{2}, f_{bs} = -\frac{f_b f_{ab} + f_{bb} f_a}{2} \left. \right\}, subs \left( Sub, \right. \\
& \frac{1}{8} F_{u_{1,1},u_{2,3}} F_{u_{1,3}} F_{u_{2,2}} - \frac{1}{2} F_{u_{1,1}} F_{u_{1,3},u_{2,3}} F_{u_{2,2}} - \frac{1}{16} F_{u_{1,1},u_{2,3}} F_{u_{2,3}} F_{u_{1,2}} \\
& - \frac{1}{2} F_{u_{1,1}} F_{u_{2,3},u_{2,3}} F_{u_{1,2}} - \frac{1}{16} F_{u_{1,3}}^2 F_{u_{2,3},u_{2,3}} F_{u_{1,2}} - \frac{3}{4} F_{u_{1,1}} F_{u_{1,2},u_{2,2}} \\
& + \frac{1}{4} F_{u_{1,1},u_{1,2}} F_{u_{2,2}} - \frac{1}{8} F_{u_{1,2}} F_{u_{1,2},u_{1,2}} - \frac{1}{8} F_{u_{1,3},u_{2,2}} F_{u_{2,3}} F_{u_{1,1}} + \frac{1}{16} \\
& F_{u_{2,3}}^2 F_{u_{1,1},u_{1,2}} - \frac{3}{16} F_{u_{1,3}}^2 F_{u_{1,2},u_{2,2}} - \frac{1}{16} F_{u_{1,3}}^2 F_{u_{2,2}} F_{u_{1,3},u_{2,3}} \\
& + \frac{1}{16} F_{u_{1,3}} F_{u_{1,2},u_{2,3}} F_{u_{1,2}} - \frac{1}{16} F_{u_{1,2},u_{1,3}} F_{u_{2,3}} F_{u_{1,2}} - \frac{1}{16} F_{u_{1,3}} F_{u_{2,3}} F_{u_{1,2},u_{1,2}} \\
& - \frac{1}{4} F_{u_{1,1},u_{2,2}} F_{u_{1,2}} - \frac{1}{8} F_{u_{1,3}} F_{u_{2,3}} F_{u_{1,1},u_{2,2}} - \frac{1}{8} F_{u_{1,3}} F_{u_{2,3}} F_{u_{1,2}} F_{u_{1,3},u_{2,3}} \\
& - \frac{1}{4} F_{u_{1,3},u_{2,3}} F_{u_{1,2}}^2 - \frac{1}{8} F_{u_{1,3}} F_{u_{2,3}} F_{u_{1,1}} F_{u_{2,3},u_{2,3}} + \frac{1}{16} F_{u_{1,3}} F_{u_{1,2}} F_{u_{1,3},u_{2,2}} \\
& - \frac{1}{16} F_{u_{1,3},u_{2,3}} F_{u_{2,3}}^2 F_{u_{1,1}} - \frac{1}{8} F_{u_{2,3}} F_{u_{1,1}} F_{u_{1,2},u_{2,3}} + \frac{1}{8} F_{u_{1,3}} F_{u_{2,2}} F_{u_{1,2},u_{1,3}} \left. \right) \left. \right)
\end{aligned}$$

$$\frac{1}{64} (f_a f_b + 2 f_s) (f_{bb} f_a^2 - 2 f_a f_b f_{ab} + f_{aa} f_b^2 - 8 f_{ab} f_s - 4 f_{ss}) \quad (45)$$

**E** > *Res112a*[7]

$$\begin{aligned} & -\frac{1}{8} F_{u,2,3} F_{u,1,1} F_{u,2,2}^{u,2,3} - \frac{1}{16} F_{u,1,3}^2 F_{u,2,3} F_{u,2,2}^{u,2,3} F_{u,2,2} - \frac{1}{2} F_{u,1,2} F_{u,1,2}^{u,2,2} \\ & - \frac{1}{4} F_{u,1,3} F_{u,2,3} F_{u,1,2}^{u,2,2} + \frac{1}{8} F_{u,1,3} F_{u,1,2}^{u,2,3} F_{u,2,2} - \frac{1}{2} F_{u,1,1} F_{u,2,2}^{u,2,2} - \frac{1}{8} \\ & F_{u,1,3}^2 F_{u,2,2}^{u,2,2} - \frac{1}{16} F_{u,2,3}^2 F_{u,1,1} F_{u,2,3}^{u,2,3} - \frac{1}{16} F_{u,1,3} F_{u,2,2} F_{u,2,3} F_{u,1,2} \\ & + \frac{1}{16} F_{u,1,3} F_{u,2,2}^{u,2,3} F_{u,1,2} + \frac{1}{8} F_{u,1,3} F_{u,2,2} F_{u,1,3}^{u,2,2} - \frac{1}{8} F_{u,1,3} F_{u,2,3} F_{u,2,2} F_{u,1,3}^{u,2,3} \\ & - \frac{1}{2} F_{u,1,2} F_{u,1,3}^{u,2,3} F_{u,2,2} - \frac{1}{4} F_{u,2,3}^{u,2,3} F_{u,1,2}^2 - \frac{1}{2} F_{u,1,1} F_{u,2,3}^{u,2,3} F_{u,2,2} \\ & - \frac{1}{8} F_{u,1,3} F_{u,2,3} F_{u,1,2} F_{u,2,3}^{u,2,3} - \frac{1}{16} F_{u,1,3}^{u,2,3} F_{u,2,3}^2 F_{u,1,2} - \frac{1}{16} F_{u,2,3} F_{u,1,2} F_{u,1,2}^{u,2,3} \end{aligned} \quad (46)$$

$$\begin{aligned} & \mathbf{E} > \text{factor} \left( \text{subs} \left( \left\{ f_r = -\frac{1}{4} f_a^2, f_t = -\frac{1}{4} f_b^2, f_{ar} = -\frac{1}{2} f_a f_{aa}, f_{at} = -\frac{1}{2} f_b f_{ab}, f_{br} = -\frac{1}{2} f_a f_{ab}, f_{bt} = \right. \right. \\ & -\frac{1}{2} f_b f_{bb}, f_{rr} = \frac{1}{4} f_a^2 f_{aa}, f_{rs} = f_a \frac{f_a f_{ab} + f_{aa} f_b}{4}, f_{rt} = \frac{1}{4} f_a f_b f_{ab}, f_{st} = f_b \frac{f_b f_{ab} + f_{bb} f_a}{4}, f_{tt} \\ & = \frac{1}{4} f_b^2 f_{bb}, f_{as} = -\frac{f_a f_{ab} + f_{aa} f_b}{2}, f_{bs} = -\frac{f_b f_{ab} + f_{bb} f_a}{2}, f_{ss} = \frac{1}{4} f_{aa} f_b^2 + \frac{1}{4} f_{bb} f_a^2 - 2 f_{ab} f_s \\ & \left. \left. - \frac{1}{2} f_a f_b f_{ab} \right\}, \text{subs} \left( \text{Sub}, -\frac{1}{8} F_{u,2,3} F_{u,1,1} F_{u,2,2}^{u,2,3} - \frac{1}{16} F_{u,1,3}^2 F_{u,2,3} F_{u,2,2}^{u,2,3} F_{u,2,2} \right. \right. \\ & - \frac{1}{2} F_{u,1,2} F_{u,1,2}^{u,2,2} - \frac{1}{4} F_{u,1,3} F_{u,2,3} F_{u,1,2}^{u,2,2} + \frac{1}{8} F_{u,1,3} F_{u,1,2}^{u,2,3} F_{u,2,2} \\ & - \frac{1}{2} F_{u,1,1} F_{u,2,2}^{u,2,2} - \frac{1}{8} F_{u,1,3}^2 F_{u,2,2}^{u,2,2} - \frac{1}{16} F_{u,2,3}^2 F_{u,1,1} F_{u,2,3}^{u,2,3} \\ & - \frac{1}{16} F_{u,1,3} F_{u,2,2} F_{u,2,3} F_{u,1,2} + \frac{1}{16} F_{u,1,3} F_{u,2,2}^{u,2,3} F_{u,1,2} + \frac{1}{8} F_{u,1,3} F_{u,2,2} F_{u,1,3}^{u,2,2} \\ & - \frac{1}{8} F_{u,1,3} F_{u,2,3} F_{u,2,2} F_{u,1,3}^{u,2,3} - \frac{1}{2} F_{u,1,2} F_{u,1,3}^{u,2,3} F_{u,2,2} - \frac{1}{4} F_{u,2,3}^{u,2,3} F_{u,1,2}^2 \\ & - \frac{1}{2} F_{u,1,1} F_{u,2,3}^{u,2,3} F_{u,2,2} - \frac{1}{8} F_{u,1,3} F_{u,2,3} F_{u,1,2} F_{u,2,3}^{u,2,3} - \frac{1}{16} F_{u,1,3}^{u,2,3} F_{u,2,3}^2 \\ & \left. \left. F_{u,2,3} F_{u,1,2} - \frac{1}{16} F_{u,2,3} F_{u,1,2} F_{u,1,2}^{u,2,3} \right) \right) \right) \\ & - \frac{1}{16} f_{bb} (f_a f_b + 2 f_s)^2 \quad (47) \end{aligned}$$

**E** > # Thus we are done in the case as well!

**E** >

**E** > # Finally consider two more overdetermined cases  $(f_a, f_b) \neq (0, 0)$  and  $f_a f_b + 2f_s = 0$ ,  $f_a^2 + 4f_r = f_b^2 + 4f_t = 0$

$$\begin{aligned} \mathbf{E} > \text{factor}\left(\text{subs}\left(\left\{f_r = -\frac{1}{4}f_a^2, f_s = -\frac{1}{2}f_a f_b, f_t = -\frac{1}{4}f_b^2, f_{ar} = -\frac{1}{2}f_a f_{aa}, f_{as} = -\frac{1}{2}(f_a f_{ab} + f_b f_{aa}), f_{at} = \right.\right.\right. \\ & -\frac{1}{2}f_b f_{ab}, f_{br} = -\frac{1}{2}f_a f_{ab}, f_{bs} = -\frac{1}{2}(f_a f_{bb} + f_b f_{ab}), f_{bt} = -\frac{1}{2}f_b f_{bb}, f_{rr} = \frac{1}{4}f_a^2 f_{aa}, f_{rs} \\ & = \frac{1}{4}f_a(f_a f_{ab} + f_b f_{aa}), f_{rt} = \frac{1}{4}f_a f_b f_{ab}, f_{ss} = \frac{1}{4}(f_a^2 f_{bb} + 2f_a f_b f_{ab} + f_b^2 f_{aa}), f_{st} \\ & = \frac{1}{4}f_b(f_b f_{ab} + f_a f_{bb}), f_{tt} = \frac{1}{4}f_b^2 f_{bb}\left.\right\}, [f_{aa}f_a + 2f_{ar}, \diamond, f_{bb}f_b + 2f_{br}, \diamond, f_{aa}f_b + 2f_{ab}f_a \\ & + 2f_{as} + 2f_{br}, \diamond, f_{bb}f_a + 2f_{ab}f_b + 2f_{bs} + 2f_{ar}, \diamond, f_{aa}f_r + f_{rr}, \diamond, f_{bb}f_t + f_{tt}, \diamond, f_{aa}f_s \\ & + 2f_{ab}f_r + 2f_{rs}, \diamond, f_{bb}f_s + 2f_{ab}f_t + 2f_{st}, \diamond, f_{aa}f_t + f_{bb}f_r + 2f_{ab}f_s + 2f_{rt} + f_{ss}])\left.\right) \\ & [0, \diamond, 0, \diamond, 0, \diamond, 0, \diamond, 0, \diamond, 0, \diamond, 0, \diamond, 0] \end{aligned} \quad (48)$$

**E** > # and the case  $f_a = f_b = f_r = f_t = 0$

$$\begin{aligned} \mathbf{E} > \text{factor}\left(\text{subs}\left(\left\{f_r = 0, f_t = 0, f_a = 0, f_b = 0, f_{aa} = 0, f_{ab} = 0, f_{bb} = 0, f_{ar} = 0, f_{as} = 0, f_{at} = 0, f_{br} = 0, \right.\right.\right. \\ & f_{bs} = 0, f_{bt} = 0, f_{rr} = 0, f_{rs} = 0, f_{rt} = 0, f_{st} = 0, f_{tt} = 0\left.\right\}, [f_{aa}f_a + 2f_{ar}, \diamond, f_{bb}f_b + 2f_{br}, \diamond, \\ & f_{aa}f_b + 2f_{ab}f_a + 2f_{as} + 2f_{br}, \diamond, f_{bb}f_a + 2f_{ab}f_b + 2f_{bs} + 2f_{ar}, \diamond, f_{aa}f_r + f_{rr}, \diamond, f_{bb}f_t + f_{tt}, \\ & \diamond, f_{aa}f_s + 2f_{ab}f_r + 2f_{rs}, \diamond, f_{bb}f_s + 2f_{ab}f_t + 2f_{st}, \diamond, f_{aa}f_t + f_{bb}f_r + 2f_{ab}f_s + 2f_{rt} + f_{ss}])\left.\right) \\ & [0, \diamond, 0, \diamond, 0, \diamond, 0, \diamond, 0, \diamond, 0, \diamond, 0, \diamond, f_{ss}] \end{aligned} \quad (49)$$

**E** > Res112a[5]

$$\begin{aligned} & \frac{1}{8} F_{u_{1,1}, u_{2,3}} F_{u_{1,3}} F_{u_{2,2}} - \frac{1}{2} F_{u_{1,1}} F_{u_{1,3}, u_{2,3}} F_{u_{2,2}} - \frac{1}{16} F_{u_{1,1}, u_{2,3}} F_{u_{2,3}} F_{u_{1,2}} \\ & - \frac{1}{2} F_{u_{1,1}} F_{u_{2,3}, u_{2,3}} F_{u_{1,2}} - \frac{1}{16} F_{u_{1,3}}^2 F_{u_{2,3}, u_{2,3}} F_{u_{1,2}} - \frac{3}{4} F_{u_{1,1}} F_{u_{1,2}, u_{2,2}} \\ & + \frac{1}{4} F_{u_{1,1}, u_{1,2}} F_{u_{2,2}} - \frac{1}{8} F_{u_{1,2}} F_{u_{1,2}, u_{1,2}} - \frac{1}{8} F_{u_{1,3}, u_{2,2}} F_{u_{2,3}} F_{u_{1,1}} + \frac{1}{16} \\ & F_{u_{2,3}}^2 F_{u_{1,1}, u_{1,2}} - \frac{3}{16} F_{u_{1,3}}^2 F_{u_{1,2}, u_{2,2}} - \frac{1}{16} F_{u_{1,3}}^2 F_{u_{2,2}} F_{u_{1,3}, u_{2,3}} \\ & + \frac{1}{16} F_{u_{1,3}} F_{u_{1,2}, u_{2,3}} F_{u_{1,2}} - \frac{1}{16} F_{u_{1,2}, u_{1,3}} F_{u_{2,3}} F_{u_{1,2}} - \frac{1}{16} F_{u_{1,3}} F_{u_{2,3}} F_{u_{1,2}, u_{1,2}} \\ & - \frac{1}{4} F_{u_{1,1}, u_{2,2}} F_{u_{1,2}} - \frac{1}{8} F_{u_{1,3}} F_{u_{2,3}} F_{u_{1,1}, u_{2,2}} - \frac{1}{8} F_{u_{1,3}} F_{u_{2,3}} F_{u_{1,2}} F_{u_{1,3}, u_{2,3}} \\ & - \frac{1}{4} F_{u_{1,3}, u_{2,3}} F_{u_{1,2}}^2 - \frac{1}{8} F_{u_{1,3}} F_{u_{2,3}} F_{u_{1,1}} F_{u_{2,3}, u_{2,3}} + \frac{1}{16} F_{u_{1,3}} F_{u_{1,2}} F_{u_{1,3}, u_{2,2}} \\ & - \frac{1}{16} F_{u_{1,3}, u_{2,3}} F_{u_{2,3}}^2 F_{u_{1,1}} - \frac{1}{8} F_{u_{2,3}} F_{u_{1,1}} F_{u_{1,2}, u_{2,3}} + \frac{1}{8} F_{u_{1,3}} F_{u_{2,2}} F_{u_{1,2}, u_{1,3}} \end{aligned} \quad (50)$$

$$\mathbf{E} > \text{factor}\left(\text{subs}\left(\left\{f_r = 0, f_t = 0, f_a = 0, f_b = 0, f_{aa} = 0, f_{ab} = 0, f_{bb} = 0, f_{ar} = 0, f_{as} = 0, f_{at} = 0, f_{br} = 0, \right.\right.\right.$$

$$\begin{aligned}
& f_{bs}=0, f_{bt}=0, f_{rr}=0, f_{rs}=0, f_{rt}=0, f_{st}=0, f_{tt}=0 \}, subs \left( Sub, \frac{1}{8} F_{u_{1,1}, u_{2,3}} F_{u_{1,3}} F_{u_{2,2}} \right. \\
& - \frac{1}{2} F_{u_{1,1}} F_{u_{1,3}, u_{2,3}} F_{u_{2,2}} - \frac{1}{16} F_{u_{1,1}, u_{2,3}} F_{u_{2,3}} F_{u_{1,2}} - \frac{1}{2} F_{u_{1,1}} F_{u_{2,3}, u_{2,3}} F_{u_{1,2}} \\
& - \frac{1}{16} F_{u_{1,3}}^2 F_{u_{2,3}, u_{2,3}} F_{u_{1,2}} - \frac{3}{4} F_{u_{1,1}} F_{u_{1,2}, u_{2,2}} + \frac{1}{4} F_{u_{1,1}, u_{1,2}} F_{u_{2,2}} \\
& - \frac{1}{8} F_{u_{1,2}} F_{u_{1,2}, u_{1,2}} - \frac{1}{8} F_{u_{1,3}, u_{2,2}} F_{u_{2,3}} F_{u_{1,1}} + \frac{1}{16} F_{u_{2,3}}^2 F_{u_{1,1}, u_{1,2}} - \frac{3}{16} \\
& F_{u_{1,3}}^2 F_{u_{1,2}, u_{2,2}} - \frac{1}{16} F_{u_{1,3}}^2 F_{u_{2,2}} F_{u_{1,3}, u_{2,3}} + \frac{1}{16} F_{u_{1,3}} F_{u_{1,2}, u_{2,3}} F_{u_{1,2}} \\
& - \frac{1}{16} F_{u_{1,2}, u_{1,3}} F_{u_{2,3}} F_{u_{1,2}} - \frac{1}{16} F_{u_{1,3}} F_{u_{2,3}} F_{u_{1,2}, u_{1,2}} - \frac{1}{4} F_{u_{1,1}, u_{2,2}} F_{u_{1,2}} \\
& - \frac{1}{8} F_{u_{1,3}} F_{u_{2,3}} F_{u_{1,1}, u_{2,2}} - \frac{1}{8} F_{u_{1,3}} F_{u_{2,3}} F_{u_{1,2}} F_{u_{1,3}, u_{2,3}} - \frac{1}{4} F_{u_{1,3}, u_{2,3}} F_{u_{1,2}}^2 \\
& - \frac{1}{8} F_{u_{1,3}} F_{u_{2,3}} F_{u_{1,1}} F_{u_{2,3}, u_{2,3}} + \frac{1}{16} F_{u_{1,3}} F_{u_{1,2}} F_{u_{1,3}, u_{2,2}} - \frac{1}{16} F_{u_{1,3}, u_{2,3}} \\
& F_{u_{2,3}}^2 F_{u_{1,1}} - \frac{1}{8} F_{u_{2,3}} F_{u_{1,1}} F_{u_{1,2}, u_{2,3}} + \frac{1}{8} F_{u_{1,3}} F_{u_{2,2}} F_{u_{1,2}, u_{1,3}} \left. \right) \left. \right) \left. \right) \\
& - \frac{1}{8} f_s f_{ss}
\end{aligned} \tag{51}$$

**E** > # The very last case (up to symmetry) that is left is:  $f_a \neq 0, f_a^2 + 4f_r = 0, f_b = f_t = 0$ .

$$\begin{aligned}
\mathbf{E} > factor \left( subs \left( \left\{ f_r = -\frac{1}{4} f_a^2, f_t = 0, f_b = 0, f_{ar} = -\frac{1}{2} f_a f_{aa}, f_{at} = 0, f_{br} = 0, f_{bt} = 0, f_{rr} = \frac{1}{4} f_a^2 f_{aa}, f_{rs} \right. \right. \right. \\
& = -\frac{1}{2} f_a f_{as}, f_{rt} = 0, f_{st} = 0, f_{tt} = 0, f_{ab} = 0, f_{bb} = 0, f_{bs} = 0 \left. \right\}, [f_{aa} f_a + 2f_{ar}, \blacklozenge, f_{bb} f_b + 2f_{br}, \\
& \blacklozenge, f_{aa} f_b + 2f_{ab} f_a + 2f_{as} + 2f_{br}, \blacklozenge, f_{bb} f_a + 2f_{ab} f_b + 2f_{bs} + 2f_{ar}, \blacklozenge, f_{aa} f_r + f_{rr}, \blacklozenge, f_{bb} f_t \\
& + f_{tt}, \blacklozenge, f_{aa} f_s + 2f_{ab} f_r + 2f_{rs}, \blacklozenge, f_{bb} f_s + 2f_{ab} f_t + 2f_{st}, \blacklozenge, f_{aa} f_t + f_{bb} f_r + 2f_{ab} f_s + 2f_{rt} \\
& + f_{ss}] \left. \right) \left. \right) \\
& [0, \blacklozenge, 0, \blacklozenge, 2f_{as}, \blacklozenge, 0, \blacklozenge, 0, \blacklozenge, 0, \blacklozenge, -f_a f_{as} + f_s f_{aa}, \blacklozenge, 0, \blacklozenge, f_{ss}]
\end{aligned} \tag{52}$$

**E** > Res112a[5]

$$\begin{aligned}
& \frac{1}{8} F_{u_{1,1}, u_{2,3}} F_{u_{1,3}} F_{u_{2,2}} - \frac{1}{2} F_{u_{1,1}} F_{u_{1,3}, u_{2,3}} F_{u_{2,2}} - \frac{1}{16} F_{u_{1,1}, u_{2,3}} F_{u_{2,3}} F_{u_{1,2}} \\
& - \frac{1}{2} F_{u_{1,1}} F_{u_{2,3}, u_{2,3}} F_{u_{1,2}} - \frac{1}{16} F_{u_{1,3}}^2 F_{u_{2,3}, u_{2,3}} F_{u_{1,2}} - \frac{3}{4} F_{u_{1,1}} F_{u_{1,2}, u_{2,2}} \\
& + \frac{1}{4} F_{u_{1,1}, u_{1,2}} F_{u_{2,2}} - \frac{1}{8} F_{u_{1,2}} F_{u_{1,2}, u_{1,2}} - \frac{1}{8} F_{u_{1,3}, u_{2,2}} F_{u_{2,3}} F_{u_{1,1}} + \frac{1}{16} \\
& F_{u_{2,3}}^2 F_{u_{1,1}, u_{1,2}} - \frac{3}{16} F_{u_{1,3}}^2 F_{u_{1,2}, u_{2,2}} - \frac{1}{16} F_{u_{1,3}}^2 F_{u_{2,2}} F_{u_{1,3}, u_{2,3}} \\
& + \frac{1}{16} F_{u_{1,3}} F_{u_{1,2}, u_{2,3}} F_{u_{1,2}} - \frac{1}{16} F_{u_{1,2}, u_{1,3}} F_{u_{2,3}} F_{u_{1,2}} - \frac{1}{16} F_{u_{1,3}} F_{u_{2,3}} F_{u_{1,2}, u_{1,2}}
\end{aligned} \tag{53}$$

$$\begin{aligned}
& -\frac{1}{4} F_{u_{1,1},u_{2,2}} F_{u_{1,2}} - \frac{1}{8} F_{u_{1,3}} F_{u_{2,3}} F_{u_{1,1},u_{2,2}} - \frac{1}{8} F_{u_{1,3}} F_{u_{2,3}} F_{u_{1,2}} F_{u_{1,3},u_{2,3}} \\
& -\frac{1}{4} F_{u_{1,3},u_{2,3}} F_{u_{1,2}}^2 - \frac{1}{8} F_{u_{1,3}} F_{u_{2,3}} F_{u_{1,1}} F_{u_{2,3},u_{2,3}} + \frac{1}{16} F_{u_{1,3}} F_{u_{1,2}} F_{u_{1,3},u_{2,2}} \\
& -\frac{1}{16} F_{u_{1,3},u_{2,3}} F_{u_{2,3}}^2 F_{u_{1,1}} - \frac{1}{8} F_{u_{2,3}} F_{u_{1,1}} F_{u_{1,2},u_{2,3}} + \frac{1}{8} F_{u_{1,3}} F_{u_{2,2}} F_{u_{1,2},u_{1,3}}
\end{aligned}$$

**E** >  $factor\left(subs\left(\left\{f_r=-\frac{1}{4}f_a^2, f_t=0, f_b=0, f_{ar}=-\frac{1}{2}f_a f_{aa}, f_{at}=0, f_{br}=0, f_{bt}=0, f_{rr}=\frac{1}{4}f_a^2 f_{aa}, f_{rs}\right.\right.\right.$

$=-\frac{1}{2}f_a f_{as}, f_{rt}=0, f_{st}=0, f_{tt}=0, f_{ab}=0, f_{bb}=0, f_{bs}=0\left.\right\}, subs\left( Sub,$

$\frac{1}{8} F_{u_{1,1},u_{2,3}} F_{u_{1,3}} F_{u_{2,2}} - \frac{1}{2} F_{u_{1,1}} F_{u_{1,3},u_{2,3}} F_{u_{2,2}} - \frac{1}{16} F_{u_{1,1},u_{2,3}} F_{u_{2,3}} F_{u_{1,2}}$

$- \frac{1}{2} F_{u_{1,1}} F_{u_{2,3},u_{2,3}} F_{u_{1,2}} - \frac{1}{16} F_{u_{1,3}}^2 F_{u_{2,3},u_{2,3}} F_{u_{1,2}} - \frac{3}{4} F_{u_{1,1}} F_{u_{1,2},u_{2,2}}$

$+ \frac{1}{4} F_{u_{1,1},u_{1,2}} F_{u_{2,2}} - \frac{1}{8} F_{u_{1,2}} F_{u_{1,2},u_{1,2}} - \frac{1}{8} F_{u_{1,3},u_{2,2}} F_{u_{2,3}} F_{u_{1,1}} + \frac{1}{16}$

$F_{u_{2,3}}^2 F_{u_{1,1},u_{1,2}} - \frac{3}{16} F_{u_{1,3}}^2 F_{u_{1,2},u_{2,2}} - \frac{1}{16} F_{u_{1,3}}^2 F_{u_{2,2}} F_{u_{1,3},u_{2,3}}$

$+ \frac{1}{16} F_{u_{1,3}} F_{u_{1,2},u_{2,3}} F_{u_{1,2}} - \frac{1}{16} F_{u_{1,2},u_{1,3}} F_{u_{2,3}} F_{u_{1,2}} - \frac{1}{16} F_{u_{1,3}} F_{u_{2,3}} F_{u_{1,2},u_{1,2}}$

$- \frac{1}{4} F_{u_{1,1},u_{2,2}} F_{u_{1,2}} - \frac{1}{8} F_{u_{1,3}} F_{u_{2,3}} F_{u_{1,1},u_{2,2}} - \frac{1}{8} F_{u_{1,3}} F_{u_{2,3}} F_{u_{1,2}} F_{u_{1,3},u_{2,3}}$

$- \frac{1}{4} F_{u_{1,3},u_{2,3}} F_{u_{1,2}}^2 - \frac{1}{8} F_{u_{1,3}} F_{u_{2,3}} F_{u_{1,1}} F_{u_{2,3},u_{2,3}} + \frac{1}{16} F_{u_{1,3}} F_{u_{1,2}} F_{u_{1,3},u_{2,2}}$

$- \frac{1}{16} F_{u_{1,3},u_{2,3}} F_{u_{2,3}}^2 F_{u_{1,1}} - \frac{1}{8} F_{u_{2,3}} F_{u_{1,1}} F_{u_{1,2},u_{2,3}} + \frac{1}{8} F_{u_{1,3}} F_{u_{2,2}} F_{u_{1,2},u_{1,3}}\left.\right)\left.\right)$

$\left.\right)$

$-\frac{1}{8} f_s f_{ss}$  (54)

**E** > # If  $f_s=0$  all follows, so let us assume  $f_{ss}=0$ . Then  $D_s(f_{rs}=..)$  gives  $f_{as}=0$ . We have

**E** > Res212a[5]

$$\begin{aligned}
& \frac{1}{2} F_{u_{1,2}} F_{u_{1,1},u_{1,2}} - \frac{1}{8} F_{u_{2,3}} F_{u_{1,1}} F_{u_{1,1},u_{2,3}} + \frac{1}{16} F_{u_{1,3}} F_{u_{1,2}} F_{u_{1,2},u_{1,3}} + \frac{1}{16} \\
& F_{u_{1,3}}^2 F_{u_{2,2}} F_{u_{1,3},u_{1,3}} + \frac{1}{16} F_{u_{1,3},u_{1,3}} F_{u_{2,3}}^2 F_{u_{1,1}} - \frac{1}{8} F_{u_{1,2},u_{1,3}} F_{u_{2,3}} F_{u_{1,1}} \\
& + \frac{1}{8} F_{u_{2,2}} F_{u_{1,3}} F_{u_{1,1},u_{1,3}} + \frac{1}{16} F_{u_{1,3}}^2 F_{u_{1,2}} F_{u_{1,3},u_{2,3}} + \frac{1}{8} F_{u_{1,3}} F_{u_{2,3}} F_{u_{1,2}} F_{u_{1,3},u_{1,3}} \\
& + \frac{1}{8} F_{u_{1,3}} F_{u_{2,3}} F_{u_{1,1}} F_{u_{1,3},u_{2,3}} + \frac{1}{2} F_{u_{1,1}} F_{u_{1,3},u_{1,3}} F_{u_{2,2}} + \frac{1}{8} F_{u_{2,3}}^2 F_{u_{1,1},u_{1,1}}
\end{aligned}$$
(55)

$$\begin{aligned}
& + \frac{1}{4} F_{u_{1,3}, u_{1,3}} F_{u_{1,2}}^2 - \frac{1}{16} F_{u_{1,2}} F_{u_{2,3}} F_{u_{1,1}, u_{1,3}} + \frac{1}{4} F_{u_{1,3}} F_{u_{2,3}} F_{u_{1,1}, u_{1,2}} \\
& + \frac{1}{16} F_{u_{1,1}, u_{2,3}} F_{u_{1,3}} F_{u_{1,2}} + \frac{1}{2} F_{u_{2,2}} F_{u_{1,1}, u_{1,1}} + \frac{1}{2} F_{u_{1,1}} F_{u_{1,3}, u_{2,3}} F_{u_{1,2}}
\end{aligned}$$

$$\begin{aligned}
\mathbf{E} > \text{factor} \left( \text{subs} \left( \left\{ f_r = -\frac{1}{4} f_a^2, f_t = 0, f_b = 0, f_{ar} = -\frac{1}{2} f_a f_{aa}, f_{at} = 0, f_{br} = 0, f_{bt} = 0, f_{rr} = \frac{1}{4} f_a^2 f_{aa}, f_{rs} \right. \right. \right. \\
& = 0, f_{rt} = 0, f_{st} = 0, f_{tt} = 0, f_{ab} = 0, f_{bb} = 0, f_{bs} = 0, f_{ss} = 0, f_{as} = 0 \left. \right\}, \text{subs} \left( \text{Sub}, \right. \\
& \frac{1}{2} F_{u_{1,2}} F_{u_{1,1}, u_{1,2}} - \frac{1}{8} F_{u_{2,3}} F_{u_{1,1}} F_{u_{1,1}, u_{2,3}} + \frac{1}{16} F_{u_{1,3}} F_{u_{1,2}} F_{u_{1,2}, u_{1,3}} + \frac{1}{16} \\
& F_{u_{1,3}}^2 F_{u_{2,2}} F_{u_{1,3}, u_{1,3}} + \frac{1}{16} F_{u_{1,3}, u_{1,3}} F_{u_{2,3}}^2 F_{u_{1,1}} - \frac{1}{8} F_{u_{1,2}, u_{1,3}} F_{u_{2,3}} F_{u_{1,1}} \\
& + \frac{1}{8} F_{u_{2,2}} F_{u_{1,3}} F_{u_{1,1}, u_{1,3}} + \frac{1}{16} F_{u_{1,3}}^2 F_{u_{1,2}} F_{u_{1,3}, u_{2,3}} \\
& + \frac{1}{8} F_{u_{1,3}} F_{u_{2,3}} F_{u_{1,2}} F_{u_{1,3}, u_{1,3}} + \frac{1}{8} F_{u_{1,3}} F_{u_{2,3}} F_{u_{1,1}} F_{u_{1,3}, u_{2,3}} \\
& + \frac{1}{2} F_{u_{1,1}} F_{u_{1,3}, u_{1,3}} F_{u_{2,2}} + \frac{1}{8} F_{u_{2,3}}^2 F_{u_{1,1}, u_{1,1}} + \frac{1}{4} F_{u_{1,3}, u_{1,3}} F_{u_{1,2}}^2 \\
& - \frac{1}{16} F_{u_{1,2}} F_{u_{2,3}} F_{u_{1,1}, u_{1,3}} + \frac{1}{4} F_{u_{1,3}} F_{u_{2,3}} F_{u_{1,1}, u_{1,2}} + \frac{1}{16} F_{u_{1,1}, u_{2,3}} F_{u_{1,3}} F_{u_{1,2}} \\
& \left. \left. \left. + \frac{1}{2} F_{u_{2,2}} F_{u_{1,1}, u_{1,1}} + \frac{1}{2} F_{u_{1,1}} F_{u_{1,3}, u_{2,3}} F_{u_{1,2}} \right) \right) \right) \right) \\
& \frac{1}{4} f_{aa} f_s^2
\end{aligned} \tag{56}$$

$\mathbf{E} > \# \dots$  and so get the last MAE condition.

$\mathbf{E} >$

$\mathbf{E} >$

$\mathbf{E} > \# \text{ Conclusion: condition Cotton}=0 \text{ implies Monge-Ampere condition !!!}$

$\mathbf{E} >$

$\mathbf{E} >$
