# Supplementary material for: Dispersionless integrable systems in 3D and Einstein-Weyl geometry
Source: arXiv:1208.2728 ancillary file (2013-05-09)
Supplement: Supplementary file 8 [file BKEF-2012-IV-2D_component_quasilinear_integrability-Lax.pdf]

This is the worksheet accompanying the paper E.Ferapontov & B.Kruglikov "Dispersionless integrable systems in 3D and Einstein-Weyl geometry".

The file ran on *Maple* version 16, the package **DifferentialGeometry** was used.

We consider the 2 component systems of hydrodynamic type and study its integrability in Lax/pseudopotential sense via EW property of the linearization conformal structure

>

We first check that the fields X,Y form a Lax pair in 4D (t,x,y,w=λ), as well as the similar property for their 3D analogs (when we let λ=λ(t,x,y)).

We start by deriving the compatibility condition for the system {w\_t=D\_y[f(u,v,w)],w\_x=D\_y[g(u,v,w)]}.

>

> restart : with(DifferentialGeometry) : with(Tensor) : with(Tools) : with(JetCalculus) :  
with(LinearAlgebra) : with(PDEtools, D\_Dx, declare, ToJet, FromJet) :

> DGsetup([t, x, y], [u, v, w], L2, 2) :

> declare(a(u[\_], v[\_])) : declare(b(u[\_], v[\_])) : declare(p(u[\_], v[\_])) : declare(q(u[\_], v[\_])) :  
declare(r(u[\_], v[\_])) : declare(s(u[\_], v[\_])) :

*a(u[\_], v[\_]) will now be displayed as a*

*b(u[\_], v[\_]) will now be displayed as b*

*p(u[\_], v[\_]) will now be displayed as p*

*q(u[\_], v[\_]) will now be displayed as q*

*r(u[\_], v[\_]) will now be displayed as r*

*s(u[\_], v[\_]) will now be displayed as s*

(1)

>

> S1 := {w1 =  $\frac{\partial}{\partial u_{[ ]}} f(u_{[ ]}, v_{[ ]}, w_{[ ]}) \cdot u_3 + \frac{\partial}{\partial v_{[ ]}} f(u_{[ ]}, v_{[ ]}, w_{[ ]}) \cdot v_3 + \frac{\partial}{\partial w_{[ ]}} f(u_{[ ]}, v_{[ ]}, w_{[ ]}) \cdot w_3,$   
w2 =  $\frac{\partial}{\partial u_{[ ]}} g(u_{[ ]}, v_{[ ]}, w_{[ ]}) \cdot u_3 + \frac{\partial}{\partial v_{[ ]}} g(u_{[ ]}, v_{[ ]}, w_{[ ]}) \cdot v_3 + \frac{\partial}{\partial w_{[ ]}} g(u_{[ ]}, v_{[ ]}, w_{[ ]}) \cdot w_3$  } :

>

> S2x := {w1,1 = TotalDiff(subs(S1, w1), 1), w1,2 = TotalDiff(subs(S1, w1), 2), w1,3  
= TotalDiff(subs(S1, w1), 3), w2,2 = TotalDiff(subs(S1, w2), 2), w2,3  
= TotalDiff(subs(S1, w2), 3) } :

>

> F := u1 + a(u[\_], v[\_]) · u2 + p(u[\_], v[\_]) · u3 + q(u[\_], v[\_]) · v3 :

G := v1 + b(u[\_], v[\_]) · v2 + r(u[\_], v[\_]) · u3 + s(u[\_], v[\_]) · v3 :

> de := DifferentialEquationData([F, G, S1[1]], [u1, v1, w1])

de := [ {u1, v1, w1}, [u1 + a u2 + p u3 + q v3, v1 + b v2 + r u3 + s v3, w1 - f\_u u3 - f\_v v3  
- f\_w w3] ]

(2)

> de1 := Prolong(de, 1) : deTR := Transformation(de1) :

>

$$\begin{aligned}
& \triangleright S2a := \{w_{2,3} = \text{TotalDiff}(\text{subs}(SI, w_2), 3)\} : \\
& \triangleright S2 := \{\text{subs}(S2a, w_{2,2} = \text{Pullback}(\text{deTR}, \text{TotalDiff}(\text{subs}(SI, w_2), 2))), S2a[1], SI[2]\} \\
& S2 := \{w_2 = g_{u, \square} u_3 + g_{v, \square} v_3 + g_{w, \square} w_3, w_{2,2} = (g_{u, \square, u} u_3 + g_{u, \square, v} v_3 + g_{u, \square, w} w_3) u_2
\end{aligned} \tag{3}$$

$$\begin{aligned}
& + g_{u, \square} u_{2,3} + (g_{u, \square, v} u_3 + g_{v, \square, v} v_3 + g_{v, \square, w} w_3) v_2 + g_{v, \square} v_{2,3} + (g_{u, \square, w} u_3 \\
& + g_{v, \square, w} v_3 + g_{w, \square, w} w_3) w_2 + g_{w, \square} ((g_{u, \square, u} u_3 + g_{u, \square, v} v_3 + g_{u, \square, w} w_3) u_3 \\
& + g_{u, \square} u_{3,3} + (g_{u, \square, v} u_3 + g_{v, \square, v} v_3 + g_{v, \square, w} w_3) v_3 + g_{v, \square} v_{3,3} + (g_{u, \square, w} u_3 \\
& + g_{v, \square, w} v_3 + g_{w, \square, w} w_3) w_3 + g_{w, \square} w_{3,3}), w_{2,3} = (g_{u, \square, u} u_3 + g_{u, \square, v} v_3 \\
& + g_{u, \square, w} w_3) u_3 + g_{u, \square} u_{3,3} + (g_{u, \square, v} u_3 + g_{v, \square, v} v_3 + g_{v, \square, w} w_3) v_3 + g_{v, \square} v_{3,3} \\
& + (g_{u, \square, w} u_3 + g_{v, \square, w} v_3 + g_{w, \square, w} w_3) w_3 + g_{w, \square} w_{3,3}\}
\end{aligned}$$

$$\begin{aligned}
& \triangleright S2x \\
& \{w_{1,1} = (f_{u, \square, u} u_3 + f_{u, \square, v} v_3 + f_{u, \square, w} w_3) u_1 + f_{u, \square} u_{1,3} + (f_{u, \square, v} u_3 + f_{v, \square, v} v_3 \\
& + f_{v, \square, w} w_3) v_1 + f_{v, \square} v_{1,3} + (f_{u, \square, w} u_3 + f_{v, \square, w} v_3 + f_{w, \square, w} w_3) w_1 + f_{w, \square} w_{1,3}, w_{1,2} \\
& = (f_{u, \square, u} u_3 + f_{u, \square, v} v_3 + f_{u, \square, w} w_3) u_2 + f_{u, \square} u_{2,3} + (f_{u, \square, v} u_3 + f_{v, \square, v} v_3 \\
& + f_{v, \square, w} w_3) v_2 + f_{v, \square} v_{2,3} + (f_{u, \square, w} u_3 + f_{v, \square, w} v_3 + f_{w, \square, w} w_3) w_2 + f_{w, \square} w_{2,3}, w_{1,3} \\
& = (f_{u, \square, u} u_3 + f_{u, \square, v} v_3 + f_{u, \square, w} w_3) u_3 + f_{u, \square} u_{3,3} + (f_{u, \square, v} u_3 + f_{v, \square, v} v_3 \\
& + f_{v, \square, w} w_3) v_3 + f_{v, \square} v_{3,3} + (f_{u, \square, w} u_3 + f_{v, \square, w} v_3 + f_{w, \square, w} w_3) w_3 + f_{w, \square} w_{3,3}, w_{2,2} \\
& = (g_{u, \square, u} u_3 + g_{u, \square, v} v_3 + g_{u, \square, w} w_3) u_2 + g_{u, \square} u_{2,3} + (g_{u, \square, v} u_3 + g_{v, \square, v} v_3 \\
& + g_{v, \square, w} w_3) v_2 + g_{v, \square} v_{2,3} + (g_{u, \square, w} u_3 + g_{v, \square, w} v_3 + g_{w, \square, w} w_3) w_2 + g_{w, \square} w_{2,3}, \\
& w_{2,3} = (g_{u, \square, u} u_3 + g_{u, \square, v} v_3 + g_{u, \square, w} w_3) u_3 + g_{u, \square} u_{3,3} + (g_{u, \square, v} u_3 + g_{v, \square, v} v_3 \\
& + g_{v, \square, w} w_3) v_3 + g_{v, \square} v_{3,3} + (g_{u, \square, w} u_3 + g_{v, \square, w} v_3 + g_{w, \square, w} w_3) w_3 + g_{w, \square} w_{3,3}\}
\end{aligned} \tag{4}$$

$$\begin{aligned}
& \triangleright \\
& \triangleright DeS := \text{simplify}(\text{subs}(S2, \text{Pullback}(\text{deTR}, w_{1,2} - \text{TotalDiff}(\text{subs}(SI, w_2), 1))))
\end{aligned}$$

$$\begin{aligned}
DeS := & f_{u, \square} u_{2,3} + f_{v, \square} v_{2,3} + g_{v, \square} b v_{2,3} + g_{v, \square} s v_{3,3} - g_{u, \square, w} u_3^2 f_u - g_{v, \square, w} v_3^2 f_v \\
& - g_{w, \square} f_{u, \square, u} u_3^2 - g_{w, \square} f_{u, \square} u_{3,3} - g_{w, \square} f_{v, \square, v} v_3^2 - g_{w, \square} f_{v, \square} v_{3,3} + f_{u, \square, w} u_3^2 g_u + f_{v, \square, w} v_3^2 g_v \\
& + f_{w, \square} g_{u, \square, u} u_3^2 + f_{w, \square} g_{u, \square} u_{3,3} + f_{w, \square} g_{v, \square, v} v_3^2 + f_{w, \square} g_{v, \square} v_{3,3} + g_{u, \square, u} u_3^2 p \\
& + g_{u, \square, v} v_3^2 q + u_2 f_{u, \square, u} u_3 + u_2 f_{u, \square, v} v_3 + u_2 f_{u, \square, w} w_3 + v_2 f_{u, \square, v} u_3 + v_2 f_{v, \square, v} v_3
\end{aligned} \tag{5}$$

$$\begin{aligned}
& + v_2 f_{v, w} w_3 + g_{u, p} u_3^2 + g_{u, a} u_{2, 3} + g_{u, p} u_{3, 3} + g_{u, q} v_3^2 + g_{u, q} v_{3, 3} \\
& + g_{u, v} u_3^2 r + g_{v, v} v_3^2 s + g_{v, r} u_3^2 + g_{v, r} u_{3, 3} + g_{v, s} v_3^2 + f_{u, w} u_3 g_{v, v} v_3 \\
& - f_{u, w} u_3 g_{w, w} w_3 + f_{v, w} v_3 g_{u, u} u_3 - f_{v, w} v_3 g_{w, w} w_3 + f_{w, w} w_3 g_{u, u} u_3 \\
& + f_{w, w} w_3 g_{v, v} v_3 + 2 f_{w, u} u_3 g_{u, v} v_3 + f_{w, u} u_3 g_{u, w} w_3 + f_{w, v} v_3 g_{v, w} w_3 \\
& + g_{u, u} u_3 a u_2 + g_{u, u} u_3 q v_3 + g_{u, v} v_3 a u_2 + g_{u, v} v_3 p u_3 + g_{u, w} w_3 a u_2 \\
& + g_{u, w} w_3 p u_3 + g_{u, w} w_3 q v_3 + g_{u, u} u_3 a_u u_2 + g_{u, u} u_3 q_u v_3 + g_{u, v} v_3 p_v u_3 \\
& + g_{u, v} v_3 a_v u_2 + g_{u, v} u_3 b v_2 + g_{u, v} u_3 s v_3 + g_{v, v} v_3 b v_2 + g_{v, v} v_3 r u_3 \\
& + g_{v, w} w_3 b v_2 + g_{v, w} w_3 r u_3 + g_{v, w} w_3 s v_3 + g_{v, u} u_3 b_u v_2 + g_{v, u} u_3 s_u v_3 \\
& + g_{v, v} v_3 b_v v_2 + g_{v, v} v_3 r_v u_3 - g_{u, w} u_3 f_{v, v} v_3 - g_{v, w} v_3 f_{u, u} u_3 - g_{w, w} w_3 f_{u, u} u_3 \\
& - g_{w, w} w_3 f_{v, v} v_3 - 2 g_{w, u} u_3 f_{u, v} v_3
\end{aligned}$$

This is the compatibility constraint, but it contains many conditions: all the coefficients of jets of u

>

$$> Qn1 := \text{diff}(DeS, u_{2, 3})$$

$$Qn1 := g_{u, a} a + f_{u, p} \quad (6)$$

$$> Qn2 := \text{diff}(DeS, v_{2, 3})$$

$$Qn2 := g_{v, b} b + f_{v, r} \quad (7)$$

$$> Qn3 := \text{diff}(DeS, u_{3, 3})$$

$$Qn3 := f_{w, g} g_{u, p} + g_{u, p} p + g_{v, r} r - g_{w, f} f_{u, u} \quad (8)$$

$$> Qn4 := \text{diff}(DeS, v_{3, 3})$$

$$Qn4 := -g_{w, f} f_{v, v} + f_{w, g} g_{v, s} + g_{u, q} q + g_{v, s} s \quad (9)$$

$$> \text{diff}(DeS, w_{3, 3})$$

$$0 \quad (10)$$

$$> \text{diff}(DeS, u_2, u_2)$$

$$0 \quad (11)$$

$$> Qn5 := \text{diff}(DeS, u_2, u_3)$$

$$Qn5 := g_{u, u} a + g_{u, a} a_u + f_{u, u} \quad (12)$$

$$> \text{diff}(DeS, u_2, v_2)$$

$$0 \quad (13)$$

$$> Qn6 := \text{diff}(DeS, u_2, v_3)$$

$$Qn6 := g_{u, v} a + g_{u, a} a_v + f_{u, v} \quad (14)$$

$$\begin{aligned} &> Qn7 := \text{diff}(DeS, u_2, w_3) \\ &Qn7 := g_{u, w} a + f_{u, w} \end{aligned} \quad (15)$$

$$\begin{aligned} &> Qn8 := \text{diff}(DeS, u_3, u_3) \\ &Qn8 := 2 g_{u, p} p_u + 2 f_{u, w} g_{u, r} + 2 g_{u, v} r + 2 g_{u, u} p + 2 f_w g_{u, u} - 2 g_{u, w} f_u \\ &\quad + 2 g_v r_u - 2 g_w f_{u, u} \end{aligned} \quad (16)$$

$$\begin{aligned} &> Qn9 := \text{diff}(DeS, u_3, v_2) \\ &Qn9 := g_{u, v} b + g_v b_u + f_{u, v} \end{aligned} \quad (17)$$

$$\begin{aligned} &> Qn10 := \text{diff}(DeS, u_3, v_3) \\ &Qn10 := f_{u, w} g_v + f_{v, w} g_u + 2 f_w g_{u, v} + g_{u, u} q + g_{u, v} p + g_u q_u \\ &\quad + g_u p_v + g_{u, v} s + g_{v, v} r + g_v s_u + g_v r_v - g_{u, w} f_v - g_{v, w} f_u \\ &\quad - 2 g_w f_{u, v} \end{aligned} \quad (18)$$

$$\begin{aligned} &> Qn11 := \text{diff}(DeS, u_3, w_3) \\ &Qn11 := -f_{u, w} g_w + f_{w, w} g_u + f_w g_{u, w} + g_{u, w} p + g_{v, w} r - g_{w, w} f_u \end{aligned} \quad (19)$$

$$\begin{aligned} &> \text{diff}(DeS, v_2, v_2) \\ &0 \end{aligned} \quad (20)$$

$$\begin{aligned} &> Qn12 := \text{diff}(DeS, v_2, v_3) \\ &Qn12 := g_{v, v} b + g_v b_v + f_{v, v} \end{aligned} \quad (21)$$

$$\begin{aligned} &> Qn13 := \text{diff}(DeS, v_2, w_3) \\ &Qn13 := g_{v, w} b + f_{v, w} \end{aligned} \quad (22)$$

$$\begin{aligned} &> Qn14 := \text{diff}(DeS, v_3, v_3) \\ &Qn14 := 2 g_{u, v} q + 2 g_{v, v} s - 2 g_w f_{v, v} + 2 f_{v, w} g_v + 2 g_v s_v + 2 g_u q_v \\ &\quad + 2 f_w g_{v, v} - 2 g_{v, w} f_v \end{aligned} \quad (23)$$

$$\begin{aligned} &> Qn15 := \text{diff}(DeS, v_3, w_3) \\ &Qn15 := -f_{v, w} g_w + f_{w, w} g_v + f_w g_{v, w} + g_{u, w} q + g_{v, w} s - g_{w, w} f_v \end{aligned} \quad (24)$$

$$\begin{aligned} &> \text{diff}(DeS, w_3, w_3) \\ &0 \end{aligned} \quad (25)$$

$$\begin{aligned} &> \\ &> \\ &> DpVar := [f(u, v, w), g(u, v, w)]: \\ &> Qn := \text{ToJet}([Qn1, Qn2, Qn3, Qn4, Qn5, Qn6, Qn7, Qn8, Qn9, Qn10, Qn11, Qn12, Qn13, Qn14, \\ &\quad Qn15], DpVar, \text{notation} = \text{jetnumbers}) \end{aligned} \quad (26)$$

$$\begin{aligned}
Qn := & \left[ g_1 a + f_1, g_2 b + f_2, f_3 g_1 + g_1 p + g_2 r - g_3 f_1, -g_3 f_2 + f_3 g_2 + g_1 q + g_2 s, g_{1,1} a + g_1 a_{u[]} \right. \\
& + f_{1,1}, g_{1,2} a + g_1 a_{v[]} + f_{1,2}, g_{1,3} a + f_{1,3}, 2 g_1 p_{u[]} + 2 f_{1,3} g_1 + 2 g_{1,2} r + 2 g_{1,1} p \\
& + 2 f_3 g_{1,1} - 2 g_{1,3} f_1 + 2 g_2 r_{u[]} - 2 g_3 f_{1,1}, g_{1,2} b + g_2 b_{u[]} + f_{1,2}, f_{1,3} g_2 + f_{2,3} g_1 \\
& + 2 f_3 g_{1,2} + g_{1,1} q + g_{1,2} p + g_1 q_{u[]} + g_1 p_{v[]} + g_{1,2} s + g_{2,2} r + g_2 s_{u[]} + g_2 r_{v[]} - g_{1,3} f_2 \\
& - g_{2,3} f_1 - 2 g_3 f_{1,2}, -f_{1,3} g_3 + f_{3,3} g_1 + f_3 g_{1,3} + g_{1,3} p + g_{2,3} r - g_{3,3} f_1, g_{2,2} b + g_2 b_{v[]} \\
& + f_{2,2}, g_{2,3} b + f_{2,3}, 2 g_{1,2} q + 2 g_{2,2} s - 2 g_3 f_{2,2} + 2 f_{2,3} g_2 + 2 g_2 s_{v[]} + 2 g_1 q_{v[]} \\
& \left. + 2 f_3 g_{2,2} - 2 g_{2,3} f_2, -f_{2,3} g_3 + f_{3,3} g_2 + f_3 g_{2,3} + g_{1,3} q + g_{2,3} s - g_{3,3} f_2 \right]
\end{aligned} \tag{26}$$

> We got the required eqns and hereafter we shall resolve them, making the compatibility into a substitution

> DGsetup([u, v, w], [f, g], TEQ, 2) :

$$\begin{aligned}
> Qn := & \text{subs}([u[] = u, v[] = v], [f_1 + g_1 a, f_2 + g_2 b, f_3 g_1 + g_1 p + g_2 r - g_3 f_1, f_3 g_2 + g_1 q + g_2 s \\
& - g_3 f_2, f_{1,1} + g_{1,1} a + g_1 a_{u[]}, f_{1,2} + g_1 a_{v[]} + g_{1,2} a, f_{1,3} + g_{1,3} a, 2 f_3 g_{1,1} + 2 g_1 p_{u[]} \\
& + 2 g_{1,1} p - 2 g_3 f_{1,1} - 2 g_{1,3} f_1 + 2 g_{1,2} r + 2 g_2 r_{u[]} + 2 f_{1,3} g_1, f_{1,2} + g_{1,2} b + g_2 b_{u[]} \\
& + g_1 p_{v[]} + g_{1,2} s + g_{2,2} r + g_2 s_{u[]} + g_2 r_{v[]} - g_{1,3} f_2 - g_{2,3} f_1 - 2 g_3 f_{1,2} + f_{1,3} g_2 + f_{2,3} g_1 \\
& + 2 f_3 g_{1,2} + g_{1,1} q + g_{1,2} p + g_1 q_{u[]}, g_{2,3} r - g_{3,3} f_1 - f_{1,3} g_3 + f_{3,3} g_1 + f_3 g_{1,3} + g_{1,3} p, \\
& f_{2,2} + g_{2,2} b + g_2 b_{v[]}, f_{2,3} + g_{2,3} b, 2 g_2 s_{v[]} + 2 g_1 q_{v[]} - 2 g_{2,3} f_2 + 2 g_{2,2} s + 2 f_3 g_{2,2} \\
& + 2 g_{1,2} q + 2 f_{2,3} g_2 - 2 g_3 f_{2,2}, g_{2,3} s - g_{3,3} f_2 - f_{2,3} g_3 + f_{3,3} g_2 + f_3 g_{2,3} + g_{1,3} q]) :
\end{aligned}$$

> Svll := solve(Qn, [f\_1, f\_2, f\_3, g\_3, f\_{1,1}, f\_{1,2}, f\_{1,3}, f\_{2,2}, f\_{2,3}, f\_{3,3}, g\_{1,1}, g\_{1,2}, g\_{1,3}, g\_{2,2}, g\_{2,3}, g\_{3,3}])[1] :

> Svll[4]

$$g_3 = - \frac{-g_1^2 q - g_1 g_2 s + g_1 p g_2 + g_2^2 r}{g_1 g_2 (a - b)} \tag{27}$$

> declare(a(u, v)) : declare(b(u, v)) : declare(p(u, v)) : declare(q(u, v)) : declare(r(u, v)) :  
declare(s(u, v)) :

*a(u, v) will now be displayed as a*

*b(u, v) will now be displayed as b*

*p(u, v) will now be displayed as p*

*q(u, v) will now be displayed as q*

*r(u, v) will now be displayed as r*

*s(u, v) will now be displayed as s*

(28)

> G23 := simplify(subs(Svll, TotalDiff(subs([a = a(u, v), b = b(u, v), p = p(u, v), q = q(u, v), r = r(u, v), s = s(u, v)], subs(Svll, g\_3)), 2)))

(29)

$$G23 := \frac{1}{g_2 g_1^3 (a-b)^3 q} \left( -g_1^2 q g_2^2 r_v b^2 - g_1^3 q g_2 s a_v a + g_1^3 q g_2 s a_v b + g_1^3 q p g_2 a_v a - \right. \quad (29)$$

$$g_1^3 q p g_2 a_v b + g_1^2 q g_2^2 r a_v a - g_1^2 q g_2^2 r a_v b + g_1^2 q g_2^2 b_v r b - g_2^2 r b_v g_1^2 q a - g_2^3 r b_v g_1 s a$$

$$+ g_2^3 r b_v g_1 s b + g_2^3 r b_v g_1 p a - g_2^3 r b_v g_1 p b - g_1^3 q p_v g_2 a^2 + 2 g_1^3 q p_v g_2 a b -$$

$$g_1^3 q p_v g_2 b^2 - g_1^2 q g_2^2 r_v a^2 + 2 g_1^2 q g_2^2 r_v a b - g_2^3 r s_v a^2 g_1 + 2 g_2^3 r s_v a g_1 b - g_2^3 r s_v b^2 g_1 -$$

$$g_2^2 r g_1^2 q_v a^2 + 2 g_2^2 r g_1^2 q_v a b - g_2^2 r g_1^2 q_v b^2 + g_2^4 r^2 b_v a - g_2^4 r^2 b_v b - g_1^4 q^2 a_v a +$$

$$g_1^4 q^2 a_v b \Big)$$

$$\text{> } Svl := \text{simplify}\left(\left[\text{op}\left(\text{subs}\left(g_{2,3} = G23, [SvII[1], SvII[2], SvII[3], SvII[4], SvII[5], SvII[6], \right.\right.\right. \quad (30)$$

$$SvII[7], SvII[8], SvII[9], SvII[10], SvII[11], SvII[12], SvII[13], SvII[14]]\right)\right], g_{2,3} = G23,$$

$$\text{subs}\left(g_{2,3} = G23, SvII[16]\right)\Big]$$

$$Svl := \left[ f_1 = -g_1 a, f_2 = -g_2 b, f_3 = -\frac{-b g_1 p g_2 - b g_2^2 r + a g_1^2 q + g_1 g_2 s a}{g_1 g_2 (a-b)}, g_3 = \right.$$

$$-\frac{-g_1^2 q - g_1 g_2 s + g_1 p g_2 + g_2^2 r}{g_1 g_2 (a-b)}, f_{1,1} = -\frac{1}{g_2^2 r (a-b)} \left( g_1 \left( a g_1^2 a_u q + a g_1 a_u g_2 s \right. \right.$$

$$- a g_1 a_u p g_2 - a r g_1 a_v g_2 + a r g_2^2 b_u + g_1 p_u a^2 g_2 - a g_1 p_u b g_2 + g_2^2 r_u a^2 - a g_2^2 r_u b$$

$$\left. - a_u g_2^2 r b \right) \Big), f_{1,2} = -\frac{a g_2 b_u - g_1 a_v b}{a-b}, f_{1,3} =$$

$$-\frac{1}{(b^2 + a^2 - 2ab) q r g_1^2 g_2^3 (a-b)^2} \left( a \left( a^2 q^3 a_u g_1^5 + b^2 q^3 a_u g_1^5 + a^2 q^2 r b_u g_1^3 g_2^2 \right. \right.$$

$$+ a^2 q^2 s a_u g_1^4 g_2 - a^2 q r^2 b_u g_1 g_2^4 - b^3 q^2 g_1^4 g_2 p_u - b^3 q^2 g_1^3 g_2^2 r_u - b^2 p q^2 a_u g_1^4 g_2$$

$$- b^2 q^2 r a_u g_1^3 g_2^2 + b^2 q^2 r b_u g_1^3 g_2^2 + b^2 q^2 s a_u g_1^4 g_2 - b^2 q r^2 b_u g_1 g_2^4 + a^3 q^2 g_1^4 g_2 p_u$$

$$+ a^3 q^2 g_1^3 g_2^2 r_u - a^2 p q^2 a_u g_1^4 g_2 - a^2 q^2 r a_u g_1^3 g_2^2 - 2ab q r s b_u g_1^2 g_2^3 + 2ab p q r b_u g_1^2$$

$$g_2^3 - b^3 q r g_1^2 g_2^3 s_u - b^2 p q r b_u g_1^2 g_2^3 + b^2 q r s b_u g_1^2 g_2^3 - a^2 p q r b_u g_1^2 g_2^3 + a^2 q r s b_u g_1^2 g_2^3$$

$$\left. - 3a^2 b q^2 g_1^4 g_2 p_u - 3a^2 b q^2 g_1^3 g_2^2 r_u + 3ab^2 q^2 g_1^4 g_2 p_u + 3ab^2 q^2 g_1^3 g_2^2 r_u \right)$$

$$\begin{aligned}
& + 2 a b p q^2 a_u g_1^4 g_2 + 2 a b q^2 r a_u g_1^3 g_2^2 - 2 a b q^2 r b_u g_1^3 g_2^2 - 2 a b q^2 s a_u g_1^4 g_2 \\
& + 2 a b q r^2 b_u g_1 g_2^4 + 3 b^2 a q r g_1^3 g_2^2 q_u + 3 b^2 a q r g_1^2 g_2^3 s_u - b^3 q r g_1^3 g_2^2 q_u + a^3 q r g_1^3 \\
& g_2^2 q_u + a^3 q r g_1^2 g_2^3 s_u - 3 a^2 b q r g_1^3 g_2^2 q_u - 3 a^2 b q r g_1^2 g_2^3 s_u - 2 a b q^3 a_u g_1^5 \Big) \Big), f_{2,2} = \\
& - \frac{1}{g_1^2 q (a-b)} \Big( g_2 \Big( b g_2 b_v g_1 s - b g_2 b_v g_1 p - b g_2^2 b_v r - b g_1^2 a_v q + b g_2 b_u g_1 q \\
& + b g_2 s_v a g_1 - g_2 s_v b^2 g_1 + b g_1^2 q_v a - g_1^2 q_v b^2 + b_v g_1^2 q a \Big) \Big), f_{2,3} = \\
& - \frac{1}{g_2 g_1^3 (a-b)^3 q} \Big( \Big( -g_1^2 q g_2^2 r_v b^2 - g_1^3 q g_2 s a_v a + g_1^3 q g_2 s a_v b + g_1^3 q p g_2 a_v a - \\
& g_1^3 q p g_2 a_v b + g_1^2 q g_2^2 r a_v a - g_1^2 q g_2^2 r a_v b + g_1^2 q g_2^2 b_v r b - g_2^2 r b_v g_1^2 q a - g_2^3 r b_v g_1 s a \\
& + g_2^3 r b_v g_1 s b + g_2^3 r b_v g_1 p a - g_2^3 r b_v g_1 p b - g_1^3 q p_v g_2 a^2 + 2 g_1^3 q p_v g_2 a b - \\
& g_1^3 q p_v g_2 b^2 - g_1^2 q g_2^2 r_v a^2 + 2 g_1^2 q g_2^2 r_v a b - g_2^3 r s_v a^2 g_1 + 2 g_2^3 r s_v a g_1 b - g_2^3 r s_v b^2 g_1 - \\
& g_2^2 r g_1^2 q_v a^2 + 2 g_2^2 r g_1^2 q_v a b - g_2^2 r g_1^2 q_v b^2 + g_2^4 r^2 b_v a - g_2^4 r^2 b_v b - g_1^4 q^2 a_v a + \\
& g_1^4 q^2 a_v b \Big) b \Big), f_{3,3} = - \frac{1}{g_2^4 r (b^2 + a^2 - 2 a b) g_1^4 q (a-b)} \Big( g_1^7 q^4 a_u a - b g_2^7 r^4 b_v - \\
& g_1^2 q r^3 g_2^5 b_v a + g_1^2 q r^3 g_2^5 b_v b + g_1^5 q^2 q_u a^2 g_2^2 r + g_1^5 q^2 p_v a^2 g_2^2 r + g_1^4 q^2 g_2^3 s_u a^2 r + g_1^4 q^2 \\
& g_2^3 r_v a^2 r - g_1^3 q^2 g_2^4 b_u r^2 a + g_1^3 q^2 g_2^4 b_u r^2 b + g_1^6 q^3 a_v g_2 r a + g_1^6 q^3 a_u g_2 s a - \\
& g_1^6 q^3 a_u p g_2 a - g_1^5 q^3 a_u g_2^2 r a + g_1^5 q^3 a_u g_2^2 r b + g_1^5 q^3 r g_2^2 b_u a - g_1^6 q^3 p_u a g_2 b - g_1^5 q^3 \\
& g_2^2 r_u a b + g_1^4 q^2 r^2 g_2^3 b_v a - g_1^4 q^2 r^2 g_2^3 a_v a + g_1^4 q^2 r^2 g_2^3 a_v b + g_1^3 q r^2 g_2^4 s_v a^2 + g_1^4 q r^2
\end{aligned}$$

$$\begin{aligned}
& g_2^3 q_v a^2 - g_2^4 r^2 g_1^3 q_u b^2 q - g_2^4 r^2 g_1^3 p_v b^2 q - g_2^5 r^2 s_u b^2 g_1^2 q - g_2^5 r^2 r_v b^2 g_1^2 q - g_2^3 r \\
& g_1^4 q^2 p_u b^2 - g_2^4 r g_1^3 q^2 r_u b^2 - b g_2^6 r^3 b_u g_1 q - b g_2^4 r^2 g_1^3 q^2 a_u + b g_2^6 r^3 b_v g_1 s - b \\
& g_2^6 r^3 b_v g_1 p - b g_2^5 r^3 g_1^2 a_v q + b g_2^6 r^3 s_v a g_1 + b g_2^5 r^3 g_1^2 q_v a + g_1^3 q r^2 g_2^4 b_v s a - g_1^3 q r^2 \\
& g_2^4 b_v p a - g_1^3 q r^2 g_2^4 s_v a b - g_1^4 q r^2 g_2^3 q_v a b - g_1^5 q^2 q_u a g_2^2 r b - g_1^5 q^2 p_v a g_2^2 r b - \\
& g_1^5 q^2 p a_v g_2^2 r a + g_1^5 q^2 s a_v g_2^2 r a - g_1^4 q^2 g_2^3 s_u a r b - g_1^4 q^2 g_2^3 r_v a r b - g_1^4 q^2 p g_2^3 b_u r a + \\
& g_1^4 q^2 s g_2^3 b_u r a + b g_2^4 r^2 g_1^3 q_u a q + b g_2^4 r^2 g_1^3 p_v a q - b g_2^4 r^2 p g_1^3 a_v q + b g_2^4 r^2 s g_1^3 a_v q \\
& + b g_2^5 r^2 s_u a g_1^2 q + b g_2^5 r^2 r_v a g_1^2 q - b g_2^5 r^2 p b_u g_1^2 q + b g_2^5 r^2 s b_u g_1^2 q + b g_2^3 r g_1^4 q^2 a_u s \\
& - b g_2^3 r g_1^4 q^2 a_u p + b g_2^3 r g_1^4 q^2 p_u a + b g_2^4 r g_1^3 q^2 r_u a + g_1^6 q^3 p_u a^2 g_2 + g_1^5 q^3 g_2^2 r_u a^2 - \\
& g_2^6 r^3 s_v b^2 g_1 - g_2^5 r^3 g_1^2 q_v b^2), g_{1,1} = \frac{1}{g_2^2 r (a-b)} \left( g_1 \left( g_1^2 a_u q + g_1 a_u g_2 s - g_1 a_u p g_2 \right. \right. \\
& \left. \left. - a_u g_2^2 r - r g_1 a_v g_2 + r g_2^2 b_u + g_1 p_u a g_2 - g_1 p_u b g_2 + g_2^2 r_u a - g_2^2 r_u b \right) \right), g_{1,2} = \\
& - \frac{g_1 a_v - g_2 b_u}{a-b}, g_{1,3} = \frac{1}{(b^2 + a^2 - 2ab) q r g_1^2 g_2^3 (a-b)^2} \left( a^2 q^3 a_u g_1^5 + b^2 q^3 a_u g_1^5 \right. \\
& + a^2 q^2 r b_u g_1^3 g_2^2 + a^2 q^2 s a_u g_1^4 g_2 - a^2 q r^2 b_u g_1 g_2^4 - b^3 q^2 g_1^4 g_2 p_u - b^3 q^2 g_1^3 g_2^2 r_u \\
& - b^2 p q^2 a_u g_1^4 g_2 - b^2 q^2 r a_u g_1^3 g_2^2 + b^2 q^2 r b_u g_1^3 g_2^2 + b^2 q^2 s a_u g_1^4 g_2 - b^2 q r^2 b_u g_1 g_2^4 \\
& + a^3 q^2 g_1^4 g_2 p_u + a^3 q^2 g_1^3 g_2^2 r_u - a^2 p q^2 a_u g_1^4 g_2 - a^2 q^2 r a_u g_1^3 g_2^2 - 2ab q r s b_u g_1^2 g_2^3 \\
& \left. + 2ab p q r b_u g_1^2 g_2^3 - b^3 q r g_1^2 g_2^3 s_u - b^2 p q r b_u g_1^2 g_2^3 + b^2 q r s b_u g_1^2 g_2^3 - a^2 p q r b_u g_1^2 g_2^3 \right)
\end{aligned}$$



$$\begin{aligned}
& + a^2 q r s b_u g_1^2 g_2^3 - 3 a^2 b q^2 g_1^4 g_2 p_u - 3 a^2 b q^2 g_1^3 g_2^2 r_u + 3 a b^2 q^2 g_1^4 g_2 p_u + 3 a b^2 q^2 g_1^3 g_2^2 r_u \\
& + 2 a b p q^2 a_u g_1^4 g_2 + 2 a b q^2 r a_u g_1^3 g_2^2 - 2 a b q^2 r b_u g_1^3 g_2^2 - 2 a b q^2 s a_u g_1^4 g_2 \\
& + 2 a b q r^2 b_u g_1^4 g_2 + 3 b^2 a q r g_1^3 g_2^2 q_u + 3 b^2 a q r g_1^2 g_2^3 s_u - b^3 q r g_1^3 g_2^2 q_u + a^3 q r g_1^3 g_2^2 q_u \\
& + a^3 q r g_1^2 g_2^3 s_u - 3 a^2 b q r g_1^3 g_2^2 q_u - 3 a^2 b q r g_1^2 g_2^3 s_u - 2 a b q^3 a_u g_1^5 \Big), g_{2,2} \\
& = \frac{1}{g_1^2 q (a-b)} \Big( g_2 \Big( b_v g_1^2 q + g_2 b_v g_1 s - g_2 b_v g_1 p - g_2^2 b_v r - g_1^2 a_v q + g_2 b_u g_1 q \\
& + g_2 s_v a g_1 - g_2 s_v b g_1 + g_1^2 q_v a - g_1^2 q_v b \Big) \Big), g_{2,3} = \frac{1}{g_2 g_1^3 (a-b)^3 q} \Big( -g_1^2 q g_2^2 r_v b^2 \\
& - g_1^3 q g_2 s a_v a + g_1^3 q g_2 s a_v b + g_1^3 q p g_2 a_v a - g_1^3 q p g_2 a_v b + g_1^2 q g_2^2 r a_v a - g_1^2 q \\
& g_2^2 r a_v b + g_1^2 q g_2^2 b_v r b - g_2^2 r b_v g_1^2 q a - g_2^3 r b_v g_1 s a + g_2^3 r b_v g_1 s b + g_2^3 r b_v g_1 p a - \\
& g_2^3 r b_v g_1 p b - g_1^3 q p_v g_2 a^2 + 2 g_1^3 q p_v g_2 a b - g_1^3 q p_v g_2 b^2 - g_1^2 q g_2^2 r_v a^2 + 2 g_1^2 q g_2^2 r_v a b \\
& - g_2^3 r s_v a^2 g_1 + 2 g_2^3 r s_v a g_1 b - g_2^3 r s_v b^2 g_1 - g_2^2 r g_1^2 q_v a^2 + 2 g_2^2 r g_1^2 q_v a b - g_2^2 r g_1^2 q_v b^2 \\
& + g_2^4 r^2 b_v a - g_2^4 r^2 b_v b - g_1^4 q^2 a_v a + g_1^4 q^2 a_v b \Big), g_{3,3} \\
& = \frac{1}{g_2^4 r (b^2 + a^2 - 2 a b) g_1^4 q (a-b)} \Big( g_1^5 q^2 q_u a g_2^2 r - g_1^5 q^2 q_u b g_2^2 r + g_1^5 q^2 p_v a g_2^2 r - \\
& g_1^5 q^2 p_v b g_2^2 r - g_1^5 q^2 p a_v g_2^2 r + g_1^5 q^2 s a_v g_2^2 r + g_1^4 q^2 g_2^3 s_u a r - g_1^4 q^2 g_2^3 s_u b r + g_1^4 q^2 \\
& g_2^3 r_v a r - g_1^4 q^2 g_2^3 r_v b r - g_1^4 q^2 p g_2^3 b_u r + g_1^4 q^2 s g_2^3 b_u r + g_1^3 q r^2 g_2^4 b_v s - g_1^3 q r^2 g_2^4 b_v p + \\
& g_1^3 q r^2 g_2^4 s_v a - g_1^3 q r^2 g_2^4 s_v b + g_1^4 q r^2 g_2^3 q_v a - g_1^4 q r^2 g_2^3 q_v b + g_2^4 r^2 g_1^3 q_u a q - g_2^4 r^2 \\
& g_1^3 q_u b q + g_2^4 r^2 g_1^3 p_v a q - g_2^4 r^2 g_1^3 p_v b q - g_2^4 r^2 p g_1^3 a_v q + g_2^4 r^2 s g_1^3 a_v q + g_2^5 r^2 s_u a g_1^2 q \\
& - g_2^5 r^2 s_u b g_1^2 q + g_2^5 r^2 r_v a g_1^2 q - g_2^5 r^2 r_v b g_1^2 q - g_2^5 r^2 p b_u g_1^2 q + g_2^5 r^2 s b_u g_1^2 q + g_2^3 r \\
& g_1^4 q^2 a_u s - g_2^3 r g_1^4 q^2 a_u p + g_2^3 r g_1^4 q^2 p_u a - g_2^3 r g_1^4 q^2 p_u b + g_2^4 r g_1^3 q^2 r_u a - g_2^4 r g_1^3 q^2 r_u b \\
& + g_1^6 q^3 a_v g_2 r + g_1^6 q^3 a_u g_2 s - g_1^6 q^3 a_u p g_2 + g_1^5 q^3 r g_2^2 b_u + g_1^6 q^3 p_u a g_2 - g_1^6 q^3 p_u b g_2
\end{aligned}$$

$$+ g_1^5 q^3 g_2^2 r_u a - g_1^5 q^3 g_2^2 r_u b + g_1^4 q^2 r^2 g_2^3 b_v - g_2^6 r^3 b_u g_1 q - g_2^4 r^2 g_1^3 q^2 a_u + g_2^6 r^3 b_v g_1 s - g_2^6 r^3 b_v g_1 p - g_2^5 r^3 g_1^2 a_v q + g_2^6 r^3 s_v a g_1 - g_2^6 r^3 s_v b g_1 + g_2^5 r^3 g_1^2 q_v a - g_2^5 r^3 g_1^2 q_v b + g_1^7 q^4 a_u - g_2^7 r^4 b_v) ]$$

Done: this Sv1 is the complete compatibility (a bit more detailed but equivalent to the condions from Ferapontov and Khusnutdinova [2004])

>

Now that we get compatibility (which we can substitute to check vanishing modulo the eqn) we start computing with 3D pair

>

> DGsetup([t, x, y], [u, v, w], L2, 2) :

> alias(a = a(u[], v[]), p = p(u[], v[]), b = b(u[], v[]), q = q(u[], v[]), r = r(u[], v[]), s = s(u[], v[])) :

$$\begin{aligned} > SeD0 := \text{simplify}\left(\text{subs}\left(S2, \text{Pullback}\left(\text{deTR}, -\text{TotalDiff}\left(\frac{\partial}{\partial w[]} g(u[], v[], w[]), 1\right) \right.\right.\right. \\ &\quad \left.\left. + \frac{\partial}{\partial w[]} f(u[], v[], w[]) \cdot \text{TotalDiff}\left(\frac{\partial}{\partial w[]} g(u[], v[], w[]), 3\right) + \text{TotalDiff}\left(\frac{\partial}{\partial w[]} f(u[], v[], w[]), 2\right) \right.\right. \\ &\quad \left.\left. - \frac{\partial}{\partial w[]} g(u[], v[], w[]) \cdot \text{TotalDiff}\left(\frac{\partial}{\partial w[]} f(u[], v[], w[]), 3\right)\right)\right) \\ SeD0 := & -f_{u[], w[]} u_3 g_{w[]} - f_{v[], w[]} v_3 g_{w[]} + f_{w[], w[]} g_{u[]} u_3 + f_{w[], w[]} g_{v[]} v_3 + f_{w[]} u_3 g_{u[], w[]} \\ & + f_{w[]} v_3 g_{v[], w[]} + g_{u[], w[]} a u_2 + g_{u[], w[]} p u_3 + g_{u[], w[]} q v_3 + g_{v[], w[]} b v_2 \\ & + g_{v[], w[]} r u_3 + g_{v[], w[]} s v_3 - g_{w[], w[]} f_{u[]} u_3 - g_{w[], w[]} f_{v[]} v_3 + u_2 f_{u[], w[]} + v_2 f_{v[], w[]} \end{aligned} \quad (31)$$

> SeD0a := simplify(subs([u[] = u, v[] = v, w[] = w], SeD0))

$$\begin{aligned} SeD0a := & -f_{u, w} u_3 g_w - f_{v, w} v_3 g_w + f_{w, w} g_u u_3 + f_{w, w} g_v v_3 + f_w u_3 g_{u, w} + f_w v_3 g_{v, w} + g_{u, w} a u_2 \\ & + g_{u, w} p u_3 + g_{u, w} q v_3 + g_{v, w} b v_2 + g_{v, w} r u_3 + g_{v, w} s v_3 - g_{w, w} f_u u_3 - g_{w, w} f_v v_3 + u_2 f_{u, w} \\ & + v_2 f_{v, w} \end{aligned} \quad (32)$$

> SED0 := ToJet(SeD0a, [f(u, v, w), g(u, v, w)], notation = jetnumbers)

$$\begin{aligned} SED0 := & -f_{1,3} u_3 g_3 - f_{2,3} v_3 g_3 + f_{3,3} g_1 u_3 + f_{3,3} g_2 v_3 + f_3 u_3 g_{1,3} + f_3 v_3 g_{2,3} + g_{1,3} a u_2 \\ & + g_{1,3} p u_3 + g_{1,3} q v_3 + g_{2,3} b v_2 + g_{2,3} r u_3 + g_{2,3} s v_3 - g_{3,3} f_1 u_3 - g_{3,3} f_2 v_3 + u_2 f_{1,3} \\ & + v_2 f_{2,3} \end{aligned} \quad (33)$$

> simplify(subs(Sv1, SED0))

0

(34)

Thus we see the Lax pair condition in 3D

This worked perfect, so we also do the 4D pair

>

> DGsetup([t, x, y], [u, v], L1, 2) :

> SeD1 := simplify(subs(S2, Pullback(deTR, -TotalDiff( $\frac{\partial}{\partial w} g(u[], v[], w)$ ), 1) +  $\frac{\partial}{\partial w} f(u[],$

$$v_{[ ]}, w) \cdot \text{TotalDiff} \left( \frac{\partial}{\partial w} g(u_{[ ]}, v_{[ ]}, w), 3 \right) - \left( \left( \frac{\partial}{\partial u_{[ ]}} f(u_{[ ]}, v_{[ ]}, w) \right) u_3 + \left( \frac{\partial}{\partial v_{[ ]}} f(u_{[ ]}, v_{[ ]}, w) \right) v_3 \right) \cdot \frac{\partial^2}{\partial w^2} g(u_{[ ]}, v_{[ ]}, w) + \text{TotalDiff} \left( \frac{\partial}{\partial w} f(u_{[ ]}, v_{[ ]}, w), 2 \right) - \frac{\partial}{\partial w} g(u_{[ ]}, v_{[ ]}, w) \cdot \text{TotalDiff} \left( \frac{\partial}{\partial w} f(u_{[ ]}, v_{[ ]}, w), 3 \right) + \left( \left( \frac{\partial}{\partial u_{[ ]}} g(u_{[ ]}, v_{[ ]}, w) \right) u_3 + \left( \frac{\partial}{\partial v_{[ ]}} g(u_{[ ]}, v_{[ ]}, w) \right) v_3 \right) \cdot \frac{\partial^2}{\partial w^2} f(u_{[ ]}, v_{[ ]}, w) \right) \right)$$

$$\text{SeD1} := g_{w, u} a u_2 + g_{w, u} p u_3 + g_{w, u} q v_3 + g_{w, v} b v_2 + g_{w, v} r u_3 + g_{w, v} s v_3 \quad (35)$$

$$+ f_w g_{w, u} u_3 + f_w g_{w, v} v_3 - g_{w, w} f_u u_3 - g_{w, w} f_v v_3 + f_{w, u} u_2 + f_{w, v} v_2 - g_w f_{w, u} u_3 - g_w f_{w, v} v_3 + f_{w, w} g_u u_3 + f_{w, w} g_v v_3$$

$$> \text{SeD1a} := \text{simplify}(\text{subs}([u_{[ ]} = u, v_{[ ]} = v], \text{SeD1}))$$

$$\text{SeD1a} := g_{w, u} a u_2 + g_{w, u} p u_3 + g_{w, u} q v_3 + g_{w, v} b v_2 + g_{w, v} r u_3 + g_{w, v} s v_3 + f_w g_{w, u} u_3 \quad (36)$$

$$+ f_w g_{w, v} v_3 - g_{w, w} f_u u_3 - g_{w, w} f_v v_3 + f_{w, u} u_2 + f_{w, v} v_2 - g_w f_{w, u} u_3 - g_w f_{w, v} v_3 + f_{w, w} g_u u_3 + f_{w, w} g_v v_3$$

$$> \text{SED1} := \text{ToJet}(\text{SeD1a}, [f(u, v, w), g(u, v, w)], \text{notation} = \text{jetnumbers})$$

$$\text{SED1} := -f_{1,3} u_3 g_3 - f_{2,3} v_3 g_3 + f_{3,3} g_1 u_3 + f_{3,3} g_2 v_3 + f_3 u_3 g_{1,3} + f_3 v_3 g_{2,3} + g_{1,3} a u_2 \quad (37)$$

$$+ g_{1,3} p u_3 + g_{1,3} q v_3 + g_{2,3} b v_2 + g_{2,3} r u_3 + g_{2,3} s v_3 - g_{3,3} f_1 u_3 - g_{3,3} f_2 v_3 + u_2 f_{1,3} + v_2 f_{2,3}$$

$$> \text{SED1} - \text{SED0}$$

$$0 \quad (38)$$

$$> \text{simplify}(\text{subs}(\text{Svl}, \text{SED1}))$$

$$0 \quad (39)$$

>

$$\begin{aligned} > \text{SeD2} := \text{simplify} \left( \text{subs} \left( \text{S2}, \text{Pullback} \left( \text{deTR}, \text{TotalDiff} \left( \left( \left( \frac{\partial}{\partial u_{[ ]}} g(u_{[ ]}, v_{[ ]}, w) \right) u_3 + \left( \frac{\partial}{\partial v_{[ ]}} g(u_{[ ]}, v_{[ ]}, w) \right) v_3 \right), 1 \right) - \frac{\partial}{\partial w} f(u_{[ ]}, v_{[ ]}, w) \cdot \text{TotalDiff} \left( \left( \left( \frac{\partial}{\partial u_{[ ]}} g(u_{[ ]}, v_{[ ]}, w) \right) u_3 + \left( \frac{\partial}{\partial v_{[ ]}} g(u_{[ ]}, v_{[ ]}, w) \right) v_3 \right), 3 \right) + \left( \left( \frac{\partial}{\partial u_{[ ]}} f(u_{[ ]}, v_{[ ]}, w) \right) u_3 + \left( \frac{\partial}{\partial v_{[ ]}} f(u_{[ ]}, v_{[ ]}, w) \right) v_3 \right) \cdot \left( \left( \frac{\partial^2}{\partial u_{[ ]} \partial w} g(u_{[ ]}, v_{[ ]}, w) \right) u_3 + \left( \frac{\partial^2}{\partial v_{[ ]} \partial w} g(u_{[ ]}, v_{[ ]}, w) \right) v_3 \right) \right. \right. \\ & \quad \left. - \text{TotalDiff} \left( \left( \left( \frac{\partial}{\partial u_{[ ]}} f(u_{[ ]}, v_{[ ]}, w) \right) u_3 + \left( \frac{\partial}{\partial v_{[ ]}} f(u_{[ ]}, v_{[ ]}, w) \right) v_3 \right), 2 \right) + \frac{\partial}{\partial w} g(u_{[ ]}, v_{[ ]}, w) \cdot \text{TotalDiff} \left( \left( \left( \frac{\partial}{\partial u_{[ ]}} f(u_{[ ]}, v_{[ ]}, w) \right) u_3 + \left( \frac{\partial}{\partial v_{[ ]}} f(u_{[ ]}, v_{[ ]}, w) \right) v_3 \right), 3 \right) \right. \\ & \quad \left. - \left( \left( \frac{\partial}{\partial u_{[ ]}} g(u_{[ ]}, v_{[ ]}, w) \right) u_3 + \left( \frac{\partial}{\partial v_{[ ]}} g(u_{[ ]}, v_{[ ]}, w) \right) v_3 \right) \cdot \left( \left( \frac{\partial^2}{\partial u_{[ ]} \partial w} f(u_{[ ]}, v_{[ ]}, w) \right) u_3 + \left( \frac{\partial^2}{\partial v_{[ ]} \partial w} f(u_{[ ]}, v_{[ ]}, w) \right) v_3 \right) \right) \end{aligned}$$

$$\begin{aligned}
& w) \Big) u_3 + \left( \frac{\partial^2}{\partial v_{[]} \partial w} f(u_{[]}, v_{[]}, w) \Big) v_3 \Big) \Big) \Big) \right) \\
\text{SeD2} := & -g_{u_{[]}, u_{[]}} u_3^2 p - g_{u_{[]}, v_{[]}} v_3^2 q - g_{u_{[]}} p_{u_{[]}} u_3^2 - g_{u_{[]}} a u_{2,3} - g_{u_{[]}} p u_{3,3} - g_{u_{[]}} q_{v_{[]}} v_3^2 \\
& - g_{u_{[]}} q v_{3,3} - g_{u_{[]}, v_{[]}} u_3^2 r - g_{v_{[]}, v_{[]}} v_3^2 s - g_{v_{[]}} r_{u_{[]}} u_3^2 - g_{v_{[]}} r u_{3,3} - g_{v_{[]}} s_{v_{[]}} v_3^2 \\
& - g_{v_{[]}} b v_{2,3} - g_{v_{[]}} s v_{3,3} - f_w g_{u_{[]}, u_{[]}} u_3^2 - f_w g_{u_{[]}} u_{3,3} - f_w g_{v_{[]}, v_{[]}} v_3^2 - f_w g_{v_{[]}} v_{3,3} + f_{u_{[]}} \\
& u_3^2 g_{w, u_{[]}} + f_{v_{[]}} v_3^2 g_{w, v_{[]}} - v_2 f_{v_{[]}, v_{[]}} v_3 + g_w f_{u_{[]}, u_{[]}} u_3^2 + g_w f_{u_{[]}} u_{3,3} + g_w f_{v_{[]}, v_{[]}} v_3^2 \\
& + g_w f_{v_{[]}} v_{3,3} - g_{u_{[]}} u_3^2 f_{w, u_{[]}} - g_{v_{[]}} v_3^2 f_{w, v_{[]}} - u_2 f_{u_{[]}, u_{[]}} u_3 - u_2 f_{u_{[]}, v_{[]}} v_3 - v_2 f_{u_{[]}, v_{[]}} u_3 \\
& - f_{u_{[]}} u_{2,3} - f_{v_{[]}} v_{2,3} - g_{u_{[]}, u_{[]}} u_3 a u_2 - g_{u_{[]}, u_{[]}} u_3 q v_3 - g_{u_{[]}, v_{[]}} v_3 a u_2 - g_{u_{[]}, v_{[]}} v_3 p u_3 \\
& - g_{u_{[]}} u_3 a_{u_{[]}} u_2 - g_{u_{[]}} u_3 q_{u_{[]}} v_3 - g_{u_{[]}} v_3 p_{v_{[]}} u_3 - g_{u_{[]}} v_3 a_{v_{[]}} u_2 - g_{u_{[]}, v_{[]}} u_3 b v_2 \\
& - g_{u_{[]}, v_{[]}} u_3 s v_3 - g_{v_{[]}, v_{[]}} v_3 b v_2 - g_{v_{[]}, v_{[]}} v_3 r u_3 - g_{v_{[]}} u_3 b_{u_{[]}} v_2 - g_{v_{[]}} u_3 s_{u_{[]}} v_3 \\
& - g_{v_{[]}} v_3 b_{v_{[]}} v_2 - g_{v_{[]}} v_3 r_{v_{[]}} u_3 - 2 f_w u_3 g_{u_{[]}, v_{[]}} v_3 + f_{u_{[]}} u_3 g_{w, v_{[]}} v_3 + f_{v_{[]}} v_3 g_{w, u_{[]}} u_3 \\
& + 2 g_w u_3 f_{u_{[]}, v_{[]}} v_3 - g_{u_{[]}} u_3 f_{w, v_{[]}} v_3 - g_{v_{[]}} v_3 f_{w, u_{[]}} u_3
\end{aligned} \tag{40}$$

> *SeD2a* := *simplify*(*subs*( $[u_{[]} = u, v_{[]} = v]$ , *SeD2*))

$$\begin{aligned}
\text{SeD2a} := & -g_{u, u} u_3 a u_2 - g_{u, u} u_3 q v_3 - g_{u, v} v_3 a u_2 - g_{u, v} v_3 p u_3 - g_{u, v} u_3 a_{u_{[]}} u_2 - g_{u, v} u_3 q_{u_{[]}} v_3 \\
& - g_{u, v} v_3 p_{v_{[]}} u_3 - g_{u, v} v_3 a_{v_{[]}} u_2 - g_{u, v} u_3 b v_2 - g_{u, v} u_3 s v_3 - g_{v, v} v_3 b v_2 - g_{v, v} v_3 r u_3 \\
& - g_{v, v} u_3 b_{u_{[]}} v_2 - g_{v, v} u_3 s_{u_{[]}} v_3 - g_{v, v} v_3 b_{v_{[]}} v_2 - g_{v, v} v_3 r_{v_{[]}} u_3 - 2 f_w u_3 g_{u, v} v_3 + f_{u, v} u_3 g_{w, v} v_3 \\
& + f_{v, v} v_3 g_{w, u} u_3 + 2 g_w u_3 f_{u, v} v_3 - g_{u, v} u_3 f_{w, v} v_3 - g_{v, v} v_3 f_{w, u} u_3 - f_w g_{u, v} u_{3,3} - g_{u, u} u_3^2 p \\
& + g_w f_{u, v} u_{3,3} - g_{u, v} u_3^2 f_{w, u} - g_{v, v} v_3^2 f_{w, v} - g_{u, v} p_{u_{[]}} u_3^2 - g_{u, v} a u_{2,3} - g_{u, v} p u_{3,3} - g_{u, v} v_3^2 q - v_2 f_{v, v} v_3 \\
& - g_{u, v} u_3^2 r - g_{v, v} b v_{2,3} + f_{u, v} u_3^2 g_{w, u} + f_{v, v} v_3^2 g_{w, v} - g_{v, v} r_{u_{[]}} u_3^2 - u_2 f_{u, v} u_3 + g_w f_{v, v} v_{3,3} - f_w g_{u, v} u_3^2 \\
& - g_{u, v} q_{v_{[]}} v_3^2 - g_{v, v} s v_{3,3} - f_w g_{v, v} v_3^2 - u_2 f_{u, v} v_3 - g_{v, v} v_3^2 s - f_w g_{v, v} v_{3,3} + g_w f_{v, v} v_3^2 - g_{v, v} r u_{3,3} \\
& - v_2 f_{u, v} u_3 + g_w f_{u, v} u_3^2 - g_{u, v} q v_{3,3} - g_{v, v} s_{v_{[]}} v_3^2 - f_{u, v} u_{2,3} - f_{v, v} v_{2,3}
\end{aligned} \tag{41}$$

> *SED2* := *ToJet*(*SeD2a*,  $[f(u, v, w), g(u, v, w)]$ , *notation* = *jetnumbers*)

$$\begin{aligned}
\text{SED2} := & f_1 u_3 g_{2,3} v_3 + f_2 v_3 g_{1,3} u_3 - g_1 u_3 f_{2,3} v_3 - g_2 v_3 f_{1,3} u_3 - 2 f_3 u_3 g_{1,2} v_3 + 2 g_3 u_3 f_{1,2} v_3 \\
& - g_{1,1} u_3 a u_2 - g_{1,1} u_3 q v_3 - g_{1,2} v_3 a u_2 - g_{1,2} v_3 p u_3 - g_{1,2} u_3 b v_2 - g_{1,2} u_3 s v_3 \\
& - g_{2,2} v_3 b v_2 - g_{2,2} v_3 r u_3 - g_1 u_3 a_{u_{[]}} u_2 - g_1 u_3 q_{u_{[]}} v_3 - g_1 v_3 p_{v_{[]}} u_3 - g_1 v_3 a_{v_{[]}} u_2 \\
& - g_2 u_3 b_{u_{[]}} v_2 - g_2 u_3 s_{u_{[]}} v_3 - g_2 v_3 b_{v_{[]}} v_2 - g_2 v_3 r_{v_{[]}} u_3 - g_1 p_{u_{[]}} u_3^2 - g_2 s v_{3,3} - g_2 r u_{3,3} \\
& - g_1 q v_{3,3} - g_1 a u_{2,3} - g_1 p u_{3,3} - g_2 b v_{2,3} - g_{1,1} u_3^2 p - g_{1,2} u_3^2 r - g_{1,2} v_3^2 q - g_{2,2} v_3^2 s \\
& - g_2 r_{u_{[]}} u_3^2 - g_1 q_{v_{[]}} v_3^2 - g_2 s_{v_{[]}} v_3^2 + f_2 v_3^2 g_{2,3} - g_1 u_3^2 f_{1,3} - g_2 v_3^2 f_{2,3} + f_1 u_3^2 g_{1,3} - f_3 g_{1,3} u_{3,3} \\
& + g_3 f_1 u_{3,3} - v_2 f_{2,2} v_3 - u_2 f_{1,1} u_3 + g_3 f_2 v_{3,3} - f_3 g_{1,1} u_3^2 - f_3 g_{2,2} v_3^2 - u_2 f_{1,2} v_3
\end{aligned} \tag{42}$$

$$-f_3 g_2 v_{3,3} + g_3 f_{2,2} v_3^2 - v_2 f_{1,2} u_3 + g_3 f_{1,1} u_3^2 - f_1 u_{2,3} - f_2 v_{2,3}$$

> simplify(subs(Svl, SED2))

0

(43)

Yes, we got commutativity modulo the equation. Now we are ready to check that the surfaces wipped by X,Y in 3D are totally geodesic.

>

We at first check that the covector  $\theta = f_\lambda dt + g_\lambda dx + dy$ , annihilating the plane in 3D spanned by X,Y, is null (below  $K = g_v/g_u$ ):

$$\begin{aligned} > \text{simplify} \left( p \cdot s - q \cdot r + \frac{(p+s)}{a-b} \cdot \left( b \cdot (p+r \cdot K) - a \cdot \left( s + \frac{q}{K} \right) \right) + \frac{(a \cdot s + b \cdot p)}{a-b} \cdot \left( s + \frac{q}{K} - p \right. \right. \\ & \quad \left. \left. - r \cdot K \right) + \frac{(a+b)}{(a-b)^2} \cdot \left( b \cdot (p+r \cdot K) - a \cdot \left( s + \frac{q}{K} \right) \right) \cdot \left( s + \frac{q}{K} - p - r \cdot K \right) + \frac{1}{(a-b)^2} \right. \\ & \quad \left. \cdot \left( b \cdot (p+r \cdot K) - a \cdot \left( s + \frac{q}{K} \right) \right)^2 + \frac{a \cdot b}{(a-b)^2} \cdot \left( s + \frac{q}{K} - p - r \cdot K \right)^2 \right) \end{aligned}$$

0

(44)

>

Now let us specify the equation and calculate the connection

> DGsetup([t, x, y], [u, v], J2, 3) :

> F := u<sub>1</sub> + a(u<sub>[1]</sub>, v<sub>[1]</sub>) · u<sub>2</sub> + p(u<sub>[1]</sub>, v<sub>[1]</sub>) · u<sub>3</sub> + q(u<sub>[1]</sub>, v<sub>[1]</sub>) · v<sub>3</sub>;

G := v<sub>1</sub> + b(u<sub>[1]</sub>, v<sub>[1]</sub>) · v<sub>2</sub> + r(u<sub>[1]</sub>, v<sub>[1]</sub>) · u<sub>3</sub> + s(u<sub>[1]</sub>, v<sub>[1]</sub>) · v<sub>3</sub>;

$$F := u_1 + a u_2 + p u_3 + q v_3$$

$$G := v_1 + b v_2 + r u_3 + s v_3$$

(45)

$$\begin{aligned} > DR := & \left( \text{diff}(F, u_1) \cdot \xi_1 + \text{diff}(F, u_2) \cdot \xi_2 + \text{diff}(F, u_3) \cdot \xi_3 \right) \cdot \left( \text{diff}(G, v_1) \cdot \xi_1 + \text{diff}(G, v_2) \cdot \xi_2 \right. \\ & \left. + \text{diff}(G, v_3) \cdot \xi_3 \right) - \left( \text{diff}(F, v_1) \cdot \xi_1 + \text{diff}(F, v_2) \cdot \xi_2 + \text{diff}(F, v_3) \cdot \xi_3 \right) \cdot \left( \text{diff}(G, u_1) \cdot \xi_1 \right. \\ & \left. + \text{diff}(G, u_2) \cdot \xi_2 + \text{diff}(G, u_3) \cdot \xi_3 \right) \end{aligned}$$

$$DR := (\xi_1 + a \xi_2 + p \xi_3) (\xi_1 + b \xi_2 + s \xi_3) - q \xi_3^2 r$$

(46)

$$\begin{aligned} > A := & 2 \cdot \text{Matrix} \left( \left[ \left[ \frac{1}{2} \text{diff}(DR, \xi_1, \xi_1), \frac{1}{2} \text{diff}(DR, \xi_1, \xi_2), \frac{1}{2} \text{diff}(DR, \xi_1, \xi_3) \right], \left[ \frac{1}{2} \text{diff}(DR, \right. \right. \right. \\ & \left. \left. \xi_1, \xi_2), \frac{1}{2} \text{diff}(DR, \xi_2, \xi_2), \frac{1}{2} \text{diff}(DR, \xi_2, \xi_3) \right], \left[ \frac{1}{2} \text{diff}(DR, \xi_1, \xi_3), \frac{1}{2} \text{diff}(DR, \xi_2, \xi_3), \right. \right. \\ & \left. \left. \frac{1}{2} \text{diff}(DR, \xi_3, \xi_3) \right] \right] \right) \end{aligned}$$

$$A := \begin{bmatrix} 2 & a+b & p+s \\ a+b & 2ab & as+bp \\ p+s & as+bp & 2ps-2qr \end{bmatrix}$$

(47)

> AA := expand(MatrixInverse(A)); factor(Determinant(A))

$$AA := \left[ \left[ -\frac{1}{2} \frac{-2bpas + 4abqr + a^2s^2 + b^2p^2}{qr(a^2 - 2ab + b^2)}, \right. \right]$$

$$\begin{aligned} & \left[ \frac{1}{2} \frac{-a p s + 2 a q r - b p s + 2 b q r + b p^2 + a s^2}{q r (a^2 - 2 a b + b^2)}, -\frac{1}{2} \frac{-a s + b p}{(a - b) q r} \right], \\ & \left[ \frac{1}{2} \frac{-a p s + 2 a q r - b p s + 2 b q r + b p^2 + a s^2}{q r (a^2 - 2 a b + b^2)}, -\frac{1}{2} \frac{-2 p s + 4 q r + p^2 + s^2}{q r (a^2 - 2 a b + b^2)}, \right. \\ & \left. \frac{1}{2} \frac{-s + p}{(a - b) q r} \right], \\ & \left[ -\frac{1}{2} \frac{-a s + b p}{(a - b) q r}, \frac{1}{2} \frac{-s + p}{(a - b) q r}, -\frac{1}{2 q r} \right] \Bigg] \\ & 2 q r (a - b)^2 \end{aligned} \quad (48)$$

```
> AM := simplify(Adjoint(A))
AM := [ [2 b p a s - 4 a b q r - a^2 s^2 - b^2 p^2, -a p s + 2 a q r - b p s + 2 b q r + b p^2 + a s^2,
a^2 s - a b p - b a s + b^2 p],
[-a p s + 2 a q r - b p s + 2 b q r + b p^2 + a s^2, 2 p s - 4 q r - p^2 - s^2, -a s - b p + p a
+ s b],
[a^2 s - a b p - b a s + b^2 p, -a s - b p + p a + s b, 2 a b - a^2 - b^2]]
```

Here A is the matrix of the linearized operator, AA - the inverse (metric) and AJ=AM the adjoint matrix (which we use as a representative for the conformal class)

```
> aA := [TotalDiff(A[1, 1], 1) + TotalDiff(A[1, 2], 2) + TotalDiff(A[1, 3], 3), TotalDiff(A[2,
1], 1) + TotalDiff(A[2, 2], 2) + TotalDiff(A[2, 3], 3), TotalDiff(A[3, 1], 1)
+ TotalDiff(A[3, 2], 2) + TotalDiff(A[3, 3], 3)]:
> omega := 2 * [AA[1, 1] * aA[1] + AA[1, 2] * aA[2] + AA[1, 3] * aA[3], AA[2, 1] * aA[1] + AA[2, 2]
* aA[2] + AA[2, 3] * aA[3], AA[3, 1] * aA[1] + AA[3, 2] * aA[2] + AA[3, 3] * aA[3]]:
```

This is our form connection Omega, but we will use the general form U below

```
> DepVars := [u(t, x, y), v(t, x, y)]: AJ := simplify(FromJet(AM, DepVars)):
```

```
> DGsetup([t, x, y], M):
```

```
> gg := evalDG(AJ[1, 1] * dt &t dt + AJ[1, 2] * dt &t dx + AJ[1, 3] * dt &t dy + AJ[2, 1] * dx &t dt
+ AJ[2, 2] * dx &t dx + AJ[2, 3] * dx &t dy + AJ[3, 1] * dy &t dt + AJ[3, 2] * dy &t dx
+ AJ[3, 3] * dy &t dy):
```

```
> C := Connection(a000 * dt &t D_t &t dt + a111 * dx &t D_x &t dx + a222 * dy &t D_y &t dy
+ a001 * (dt &t D_t &t dx + dx &t D_t &t dt) + a002 * (dt &t D_t &t dy + dy &t D_t
&t dt) + a102 * (dx &t D_t &t dy + dy &t D_t &t dx) + a011 * (dt &t D_x &t dx + dx
&t D_x &t dt) + a012 * (dt &t D_x &t dy + dy &t D_x &t dt) + a112 * (dx &t D_x &t dy
+ dy &t D_x &t dx) + a021 * (dt &t D_y &t dx + dx &t D_y &t dt) + a022 * (dt &t D_y
&t dy + dy &t D_y &t dt) + a122 * (dx &t D_y &t dy + dy &t D_y &t dx) + a010 * dt
&t D_x &t dt + a121 * dx &t D_y &t dx + a202 * dy &t D_t &t dy + a020 * dt &t D_y &t dt
+ a101 * dx &t D_t &t dx + a212 * dy &t D_x &t dy):
```

```
> TorsionTensor(C);
```

$$0 \, dt \, D_t \, dt$$

(50)

```

> Ω1 := simplify(FromJet(ω[1], DepVars)) :
Ω2 := simplify(FromJet(ω[2], DepVars)) :
Ω3 := simplify(FromJet(ω[3], DepVars)) :

```

Here we determine the connection C and define the covector Ω. However we wait to let U=Ω, we want to obtain this from the total geodesicity condition.

```

> Et := evalDG(DirectionalCovariantDerivative(D_t, gg, C) - U1·gg) :
Ex := evalDG(DirectionalCovariantDerivative(D_x, gg, C) - U2·gg) :
Ey := evalDG(DirectionalCovariantDerivative(D_y, gg, C) - U3·gg) :
> Eq000 := TensorInnerProduct(gg, Et, dt &t dt) :
Eq001 := TensorInnerProduct(gg, Et, dt &t dx) :
Eq002 := TensorInnerProduct(gg, Et, dt &t dy) :
Eq011 := TensorInnerProduct(gg, Et, dx &t dx) :
Eq012 := TensorInnerProduct(gg, Et, dx &t dy) :
Eq022 := TensorInnerProduct(gg, Et, dy &t dy) :
Eq100 := TensorInnerProduct(gg, Ex, dt &t dt) :
Eq101 := TensorInnerProduct(gg, Ex, dt &t dx) :
Eq102 := TensorInnerProduct(gg, Ex, dt &t dy) :
Eq111 := TensorInnerProduct(gg, Ex, dx &t dx) :
Eq112 := TensorInnerProduct(gg, Ex, dx &t dy) :
Eq122 := TensorInnerProduct(gg, Ex, dy &t dy) :
Eq200 := TensorInnerProduct(gg, Ey, dt &t dt) :
Eq201 := TensorInnerProduct(gg, Ey, dt &t dx) :
Eq202 := TensorInnerProduct(gg, Ey, dt &t dy) :
Eq211 := TensorInnerProduct(gg, Ey, dx &t dx) :
Eq212 := TensorInnerProduct(gg, Ey, dx &t dy) :
Eq222 := TensorInnerProduct(gg, Ey, dy &t dy) :
> sA := solve( {Eq000=0, Eq001=0, Eq002=0, Eq011=0, Eq012=0, Eq022=0, Eq100=0,
Eq101=0, Eq102=0, Eq111=0, Eq112=0, Eq122=0, Eq200=0, Eq201=0, Eq202=0,
Eq211=0, Eq212=0, Eq222=0}, [a000, a001, a002, a010, a011, a012, a020, a021, a022,
a101, a102, a111, a112, a121, a122, a202, a212, a222]) :
> C1 := evalDG( subs( {op(op(sA))}, C) ) :
> evalDG( CovariantDerivative(gg, C1) - gg &t (U1·dt + U2·dx + U3·dy) );
0 dt dt dt
(51)

```

We want to check that the connection preserves the conformal class of the form θ in the direction of Ann(θ)

```

> θ := evalDG( dy + D3(f)(u(t, x, y), v(t, x, y), w(t, x, y))·dt + D3(g)(u(t, x, y), v(t, x, y), w(t,
x, y))·dx )
θ := D3(f)(u(t, x, y), v(t, x, y), w(t, x, y)) dt + D3(g)(u(t, x, y), v(t, x, y), w(t, x, y)) dx + dy (52)
> X := evalDG( D_t - D3(f)(u(t, x, y), v(t, x, y), w(t, x, y))·D_y ) : Y := evalDG( D_x
- D3(g)(u(t, x, y), v(t, x, y), w(t, x, y))·D_y ) :
> [Hook(X, θ), Hook(Y, θ)]
[0, 0]
(53)

```

```

> XθX := ContractIndices( evalDG( DirectionalCovariantDerivative(X, θ, C1) ), X, [[1, 1]] ) :
XθY := ContractIndices( evalDG( DirectionalCovariantDerivative(X, θ, C1) ), Y, [[1, 1]] ) :

```

$Y\theta X := \text{ContractIndices}(\text{evalDG}(\text{DirectionalCovariantDerivative}(Y, \theta, C1)), X, [[1, 1]]) :$   
 $Y\theta Y := \text{ContractIndices}(\text{evalDG}(\text{DirectionalCovariantDerivative}(Y, \theta, C1)), Y, [[1, 1]]) :$

These are the 4 condtions to check and determine the connection for U (=Omega).  
 Let us restrict them to the equations of the Lax pair and their compatibility conditions

>  $\text{ChangeFrame}(L2);$  (54)

>  $\text{Tools:-DGinfo}(\text{"CurrentFrame"});$  (55)

>  $\text{de} := \text{DifferentialEquationData}([F, G, w_1 = w_1], [u_1, v_1, w_1])$   
 $\text{de} := [\{u_1, v_1, w_1\}, [u_1 + a u_2 + p u_3 + q v_3, v_1 + b v_2 + r u_3 + s v_3, 0]]$  (56)

>  $\text{de1} := \text{Prolong}(\text{de}, 1) : \text{deTRA} := \text{Transformation}(\text{de1}) :$

>  $\text{DepVarsP} := [\text{op}(\text{DepVars}), w(t, x, y)]$   
 $\text{DepVarsP} := [u(t, x, y), v(t, x, y), w(t, x, y)]$  (57)

>  $\text{XX1} := \text{Pullback}(\text{deTRA}, \text{subs}(S1, \text{ToJet}(X\theta X, \text{DepVarsP}, \text{notation} = \text{jetnumbers}))) :$   
 $\text{XX2} := \text{ToJet}(\text{subs}([u_{[]} = u, v_{[]} = v, w_{[]} = w], \text{XX1}), [f(u, v, w), g(u, v, w)], \text{notation} = \text{jetnumbers}) :$

$\text{XX3} := \text{simplify}(\text{subs}(\text{Svl}, \text{XX2})) :$

>  $\text{XY1} := \text{Pullback}(\text{deTRA}, \text{subs}(S1, \text{ToJet}(X\theta Y, \text{DepVarsP}, \text{notation} = \text{jetnumbers}))) :$   
 $\text{XY2} := \text{ToJet}(\text{subs}([u_{[]} = u, v_{[]} = v, w_{[]} = w], \text{XY1}), [f(u, v, w), g(u, v, w)], \text{notation} = \text{jetnumbers}) :$

$\text{XY3} := \text{simplify}(\text{subs}(\text{Svl}, \text{XY2})) :$

>  $\text{YX1} := \text{Pullback}(\text{deTRA}, \text{subs}(S1, \text{ToJet}(Y\theta X, \text{DepVarsP}, \text{notation} = \text{jetnumbers}))) :$   
 $\text{YX2} := \text{ToJet}(\text{subs}([u_{[]} = u, v_{[]} = v, w_{[]} = w], \text{YX1}), [f(u, v, w), g(u, v, w)], \text{notation} = \text{jetnumbers}) :$

$\text{YX3} := \text{simplify}(\text{subs}(\text{Svl}, \text{YX2})) :$

>  $\text{YY1} := \text{Pullback}(\text{deTRA}, \text{subs}(S1, \text{ToJet}(Y\theta Y, \text{DepVarsP}, \text{notation} = \text{jetnumbers}))) :$   
 $\text{YY2} := \text{ToJet}(\text{subs}([u_{[]} = u, v_{[]} = v, w_{[]} = w], \text{YY1}), [f(u, v, w), g(u, v, w)], \text{notation} = \text{jetnumbers}) :$

$\text{YY3} := \text{simplify}(\text{subs}(\text{Svl}, \text{YY2})) :$

These are the final 4 equations (to this end all our information was used) that allow to determined the connection form.

Let us first check that our  $\Omega$  is a solution.

>  $\Omega := \text{subs}([u_{[]} = u, v_{[]} = v], \text{Pullback}(\text{deTRA}, \text{ToJet}([\Omega 1, \Omega 2, \Omega 3], \text{DepVars}, \text{notation} = \text{jetnumbers}))) :$

>  $\text{simplify}(\text{subs}([U1 = \Omega[1], U2 = \Omega[2], U3 = \Omega[3]], \text{XX3}))$  (58)



$$\text{> simplify}(\text{subs}([U1 = \Omega[1], U2 = \Omega[2], U3 = \Omega[3]], XY3)) \quad (59)$$

$$\text{> simplify}(\text{subs}([U1 = \Omega[1], U2 = \Omega[2], U3 = \Omega[3]], YX3)) \quad (60)$$

$$\text{> simplify}(\text{subs}([U1 = \Omega[1], U2 = \Omega[2], U3 = \Omega[3]], YY3)) \quad (61)$$

Great - as expected!

$$\text{> } \Omega[3] \quad (62)$$

$$\frac{1}{(a-b)qr} \left( -v_2 a^2 s_v + v_2 b^2 p_v - u_3 a_u s^2 - v_3 a_v s^2 + p(-a u_2 - p u_3 - q v_3) a_u + p(-a u_2 - p u_3 - q v_3) b_u + p(-b v_2 - r u_3 - s v_3) a_v + p(-b v_2 - r u_3 - s v_3) b_v - (-a u_2 - p u_3 - q v_3) p_u a + (-a u_2 - p u_3 - q v_3) p_u b - (-a u_2 - p u_3 - q v_3) s_u a + (-a u_2 - p u_3 - q v_3) s_u b - (-b v_2 - r u_3 - s v_3) p_v a + (-b v_2 - r u_3 - s v_3) p_v b - (-b v_2 - r u_3 - s v_3) s_v a + (-b v_2 - r u_3 - s v_3) s_v b + u_3 b_u p^2 + v_3 b_v p^2 - u_2 a^2 s_u + u_2 b^2 p_u - s(-a u_2 - p u_3 - q v_3) a_u - s(-b v_2 - r u_3 - s v_3) b_v - s(-b v_2 - r u_3 - s v_3) a_v - s(-a u_2 - p u_3 - q v_3) b_u - a s u_3 p_u - a s v_3 p_v + b p u_2 a_u + b p v_2 a_v + b p u_3 s_u + b p v_3 s_v - s u_2 a_u b - s v_2 a_v b - s u_3 b_u p + s u_3 b p_u - s v_3 b_v p + s v_3 b p_v + p u_2 a b_u + p v_2 a b_v + p u_3 a_u s - p u_3 a s_u + p v_3 a_v s - p v_3 a s_v + u_2 a s_u b - u_2 b p_u a + v_2 a s_v b - v_2 b p_v a + 2 u_3 q_u r a - 2 u_3 q_u r b + 2 u_3 q r_u a - 2 u_3 q r_u b + 2 v_3 q_v r a - 2 v_3 q_v r b + 2 v_3 q r_v a - 2 v_3 q r_v b - a s u_2 b_u - a s v_2 b_v \right)$$

This how one of the components looks like, and we want to prove that any solution U coincide with this  $\Omega$ .

But direct approach does not work - no unique solution:

$$\text{> solve}([XX3, XY3, YX3, YY3], [U1, U2, U3]) \quad (63)$$

$$\text{> } SU := \text{solve}([\text{numer}(XX3), \text{numer}(XY3), \text{numer}(YX3)], [U1, U2, U3]) \quad (64)$$

$$\text{> } MAT := \text{Matrix}([\text{diff}(\text{numer}(XX3), U1), \text{diff}(\text{numer}(XX3), U2), \text{diff}(\text{numer}(XX3), U3)], [\text{diff}(\text{numer}(XY3), U1), \text{diff}(\text{numer}(XY3), U2), \text{diff}(\text{numer}(XY3), U3)], [\text{diff}(\text{numer}(YX3), U1), \text{diff}(\text{numer}(YX3), U2), \text{diff}(\text{numer}(YX3), U3)], [\text{diff}(\text{numer}(YY3), U1), \text{diff}(\text{numer}(YY3), U2), \text{diff}(\text{numer}(YY3), U3)]) : \quad (65)$$

$$\text{> } sDelta := (i, k, j, l) \rightarrow \text{simplify}(MAT[i, j] \cdot MAT[k, l] - MAT[i, l] \cdot MAT[k, j]) :$$

$$\text{> } [sDelta(1, 2, 1, 2), sDelta(1, 2, 1, 3), sDelta(1, 2, 2, 3), sDelta(1, 3, 1, 2), sDelta(1, 3, 1, 3), sDelta(1, 3, 2, 3), sDelta(1, 4, 1, 2), sDelta(1, 4, 1, 3), sDelta(1, 4, 2, 3), sDelta(2, 3, 2, 1, 2), sDelta(2, 3, 1, 3), sDelta(2, 3, 2, 3), sDelta(2, 4, 1, 2), sDelta(2, 4, 1, 3), sDelta(2, 4, 2, 3), sDelta(3, 4, 1, 2), sDelta(3, 4, 1, 3), sDelta(3, 4, 2, 3)]$$

$$[0, 0, 0, 0, 0, 0, 0, 0, 0, 0, 0, 0, 0, 0, 0, 0, 0, 0]$$

and even worse: the system shows to have a 2D family of solutions (up to addition of  $\theta \perp$ ).

However this happens at any fixed  $(t,x,y,\lambda=w)$  (i.e. a point in the mini-twistor space) and in our 3D manifold a curve of possible  $\lambda$  hangs over a point  $(t,x,y)$  of  $M$ . Thus we can decompose by  $\lambda$  and get more equations (in fact 7 of them); it is enough to work only with the coefficients of the equation XX3, as the others are proportional.  
The equation does not depend on  $\lambda$  explicitly, but via the functions  $g_u, g_v$  of which it is a homogeneous function.

>

>  $Leq1 := \text{simplify}(\text{diff}(\text{numer}(XX3), g_1\$7))$

$$\begin{aligned} Leq1 := & -5040 a q \left( 4 b^3 q^3 a r a_u u_2 + 2 a_u s a^3 q^3 r u_3 + 3 b^2 p a^2 U3 q^3 r - 3 b p a^3 U3 q^3 r \right. \\ & - 2 b_v b^2 s a q^3 r v_3 + 2 b_v b^2 p a q^3 r v_3 + 6 b_v b^2 a^2 q^3 r v_2 - 2 b_v b^2 r^2 a q^3 u_3 \\ & + 4 b_v b s a^2 q^3 r v_3 - 4 b_v b p a^2 q^3 r v_3 - 6 b_v b a^3 q^3 r v_2 + 4 b_v b r^2 a^2 q^3 u_3 \\ & + 4 b_u b q^4 a^2 r v_3 - 4 a_u b s a^2 q^3 r u_3 + 4 a_u b p a^2 q^3 r u_3 + 12 a_u b a^3 q^3 r u_2 \\ & - 2 a_u q^4 a^3 r v_3 - 2 b_u b^2 q^4 a r v_3 - 2 a_u p a^3 q^3 r u_3 - 2 b_u q^4 a^3 r v_3 + 4 a_v b r^2 a^2 q^3 u_3 \\ & - 2 a_v q^3 r^2 a^3 u_3 - 6 p_u b^2 a^2 q^3 r u_3 + 6 p_u b a^3 q^3 r u_3 - 4 q^3 a^4 r a_u u_2 - 2 b_v s a^3 q^3 r v_3 \\ & - 6 p_v b^2 a^2 q^3 r v_3 + 6 p_v b a^3 q^3 r v_3 - 6 a_v b^2 a^2 q^3 r v_2 - 2 a_v b^2 r^2 a q^3 u_3 \\ & + 6 a_v b a^3 q^3 r v_2 + 2 b_v p a^3 q^3 r v_3 - 2 b_v a^3 r^2 q^3 u_3 - 2 a_u b^2 q^4 a r v_3 + 2 a_u b^2 s a q^3 r u_3 \\ & - 2 a_u b^2 p a q^3 r u_3 - 12 a_u b^2 a^2 q^3 r u_2 + 4 a_u b q^4 a^2 r v_3 + 3 b^2 a^3 U2 q^3 r \\ & - 3 b a^4 U2 q^3 r + p a^4 U3 q^3 r - 3 b a^3 U1 q^3 r - 2 b_v b^3 a q^3 r v_2 + 2 b_v a^4 q^3 r v_2 \\ & - 2 p_u a^4 q^3 r u_3 - 2 p_v a^4 q^3 r v_3 + 2 a_v b^3 a q^3 r v_2 - 2 a_v a^4 q^3 r v_2 + 2 p_u b^3 a q^3 r u_3 \\ & + 2 p_v b^3 a q^3 r v_3 - b^3 p U3 a q^3 r + a^4 U1 q^3 r - b^3 U2 a^2 q^3 r + a^5 U2 q^3 r - b^3 U1 a q^3 r \\ & \left. + 3 b^2 U1 a^2 q^3 r \right) \end{aligned} \quad (66)$$

>  $Leq2 := \text{simplify}(\text{diff}(\text{numer}(XX3), g_1\$6, g_2))$

$$\begin{aligned} Leq2 := & 720 a \left( -8 p_u b^3 a^2 q^3 r u_2 + 2 p_u a^5 q^3 r u_2 + 8 s_v b^3 a^2 q^3 r v_2 - 2 s_v a^5 q^3 r v_2 \right. \\ & - 4 r_u b^3 q^4 a r u_3 - 4 q_u b^3 r^2 a q^3 u_3 - 4 r_v b^3 q^4 a r v_3 - 12 r_v b q^4 a^3 r v_3 + 2 b^3 q^4 r^2 U3 a \\ & - 12 r_u b q^4 a^3 r u_3 - 12 q_u a^3 r^2 b q^3 u_3 + 2 b_u q^4 s a^3 r v_3 - 2 b_u q^4 p a^3 r v_3 \\ & - 6 s_u q^4 a^3 b r v_3 - 2 a_u q^4 p a^3 r v_3 - 4 b_v p a^3 q^3 r s v_3 + 2 a_u q^4 a^3 r s v_3 \\ & - 6 b_v b p a^3 q^3 r v_2 - 2 a_u b^2 s^2 a q^3 r u_3 + 6 b_v b a^3 q^3 r s v_2 + 2 b_v p^2 a^3 q^3 r v_3 \\ & - 2 b_v a^4 q^3 r s v_2 + 2 b_v s^2 a^3 q^3 r v_3 + 2 b_v p a^4 q^3 r v_2 + 2 p_u p a^4 q^3 r u_3 + 4 q_v a^4 r^2 q^3 v_3 \\ & + 2 p_u q^4 a^4 r v_3 + 6 s_u b^2 q^4 a^2 r v_3 - 8 p_u b a^4 q^3 r u_2 - 2 q^4 a^4 r^2 U3 + 2 s_v a^4 r^2 q^3 u_3 \\ & + 2 p_v a^4 r^2 q^3 u_3 - 2 s_v b^4 a q^3 r v_2 + 6 s_v a^3 b p q^3 r v_3 - 6 s_v s a^3 b q^3 r v_3 \\ & - 12 s_v b^2 a^3 q^3 r v_2 + 8 s_v a^4 b q^3 r v_2 - 2 s_v a^4 p q^3 r v_3 + 2 s_v a^4 q^3 r s v_3 + 4 r_v q^4 a^4 r v_3 \\ & \left. + 4 q_u a^4 r^2 q^3 u_3 + 4 r_u q^4 a^4 r u_3 + 2 s_u q^4 a^4 r v_3 + 2 a_u a^4 q^3 r s u_2 + 2 p_u b^4 a q^3 r u_2 \right) \end{aligned} \quad (67)$$

$$\begin{aligned}
& + 2 s_v b^3 a p q^3 r v_3 - 2 s_v b^3 s a q^3 r v_3 - 2 b^3 q^4 a r p_u v_3 - 6 a_u b^2 a^2 p q^3 r u_2 \\
& + 6 a_u b^2 s a^2 q^3 r u_2 + 2 a_u b^3 a p q^3 r u_2 - 2 a_u b^3 s a q^3 r u_2 - 2 p_v b^3 a r^2 q^3 u_3 \\
& - 4 b_v p^2 a^2 b q^3 r v_3 + 8 b_v s a^2 b p q^3 r v_3 - 6 q^4 a^3 r b p_u v_3 - 2 q^3 a^3 r s^2 a_u u_3 \\
& + 6 q^4 a^3 r^2 U3 b - 2 q^3 a^4 r s p_u u_3 - 2 q^3 a^4 r p a_u u_2 + 6 b_v b^2 p a^2 q^3 r v_2 \\
& + 2 b_v b^2 p^2 a q^3 r v_3 + 2 b_v b^3 s a q^3 r v_2 - 2 s_u b^3 q^4 a r v_3 - 4 a_u q^4 s a^2 b r v_3 \\
& + 4 a_u q^4 a^2 b p r v_3 - 4 b_v b^2 s a p q^3 r v_3 + 2 b_v b^2 s^2 a q^3 r v_3 - 2 b_v b^3 a p q^3 r v_2 \\
& + 12 r_u b^2 q^4 a^2 r u_3 + 12 q_u b^2 a^2 r^2 q^3 u_3 + 12 r_v b^2 q^4 a^2 r v_3 + 4 b_u q^4 a^2 b p r v_3 \\
& - 4 b_u q^4 s a^2 b r v_3 - 2 b_u b^2 q^4 a p r v_3 + 2 b_u b^2 q^4 s a r v_3 + 4 b q^3 a^2 r s^2 a_u u_3 \\
& + 12 b^2 q^3 a^3 r p_u u_2 + 6 b q^3 a^3 r p a_u u_2 - 6 b q^3 a^3 r s a_u u_2 + 2 b^3 q^3 r a s p_u u_3 \\
& - 6 p_v q^3 a^3 r^2 b u_3 + 6 p_v q^3 a^2 r^2 b^2 u_3 - 4 q_v b^3 q^3 r^2 a v_3 + 2 a_v q^3 s r^2 a b^2 u_3 \\
& - 6 b_v b^2 s a^2 q^3 r v_2 - 6 s_v b^2 p a^2 q^3 r v_3 - 2 s_v b^3 q^3 r^2 a u_3 + 6 s_v b^2 s a^2 q^3 r v_3 \\
& - 2 b^3 q^3 a r p p_u u_3 - 6 b^2 q^4 a^2 r^2 U3 + 6 b q^3 a^3 r s p_u u_3 + 6 b^2 q^4 a^2 r p_u v_3 \\
& + 2 q^3 a^3 r^2 s a_v u_3 + 2 b^2 q^4 a r s a_u v_3 - 2 b^2 q^4 a r p a_u v_3 - 2 q^3 p^2 a^3 r a_u u_3 \\
& + 4 q^3 p a^3 r s a_u u_3 - 6 q^3 p a^3 r b p_u u_3 - 2 q^3 p a^3 r^2 a_v u_3 - 12 q^3 a^3 r^2 b q_v v_3 \\
& - 6 q^3 a^3 r^2 b s_v u_3 - 2 q^3 a^3 r^2 p b_v u_3 + 12 q^3 a^2 r^2 b^2 q_v v_3 + 6 q^3 a^2 r^2 b^2 s_v u_3 \\
& + 2 q^3 a^3 r^2 s b_v u_3 - 4 b_v s^2 a^2 b q^3 r v_3 - 2 b^2 q^3 p^2 a r a_u u_3 - 6 b^2 q^3 a^2 r s p_u u_3 \\
& + 4 b q^3 p^2 a^2 r a_u u_3 - 4 q^3 a^2 r^2 b s b_v u_3 + 4 q^3 p a^2 r^2 b b_v u_3 - 4 b q^3 a^2 r^2 s a_v u_3 \\
& + 2 b^2 q^3 r^2 a s b_v u_3 + 4 b q^3 p a^2 r^2 a_v u_3 - 8 b q^3 p a^2 r s a_u u_3 + 6 b^2 q^3 p a^2 r p_u u_3 \\
& - 2 b^2 q^3 p r^2 a b_v u_3 - 2 b^2 q^3 a r^2 p a_v u_3 + 4 b^2 q^3 a r p s a_u u_3)
\end{aligned}$$

$$\begin{aligned}
& \text{> [diff(Leq2, U1), diff(Leq2, U2), diff(Leq2, U3)]} \\
& \quad [0, 0, 720 a (-6 b^2 q^4 r^2 a^2 - 2 q^4 a^4 r^2 + 2 b^3 q^4 r^2 a + 6 b q^4 a^3 r^2)] \quad (68)
\end{aligned}$$

$$\begin{aligned}
& \text{> simplify(solve(Leq2, U3) - \Omega[3])} \\
& \quad 0 \quad (69)
\end{aligned}$$

$$\begin{aligned}
& \text{> Leq3 := simplify(diff(numer(XX3), g1$5, g2$2))} \\
& \text{Leq3 := } 960 b^3 q^3 r^2 a p a_u u_3 - 960 b^3 q^3 r^2 a s a_u u_3 - 2400 b^2 q^3 a^2 r^3 a_v u_3 \quad (70)
\end{aligned}$$

$$\begin{aligned}
& + 1920 q^3 a^3 r^2 b p a_u u_3 - 1920 q^3 a^3 r^2 b s a_u u_3 + 1920 b_v q^3 a^3 r^2 b s v_3 \\
& - 1920 b_v q^3 a^3 r^2 b p v_3 - 720 b q^3 a^5 r^2 U2 + 480 q^3 a^5 r^2 b_u u_2 - 480 q^4 a^4 r^2 b_u v_3 \\
& + 720 b^2 q^3 a^3 r^2 U1 + 480 b^4 q^3 a r^2 U1 - 480 q^3 a^4 r^3 b_v u_3 - 2400 q^4 a^2 r^2 b^2 a_u v_3 \\
& - 240 q^3 a^5 r^2 U3 s - 480 q^3 a^5 r^2 a_u u_2 + 240 b q^3 a^4 r^2 U1 - 1200 b^3 q^3 a^2 r^2 U1 \\
& - 3840 b_v b^3 a^2 q^3 r^2 v_2 + 960 b_v b^3 s a q^3 r^2 v_3 - 960 b_v b^3 p a q^3 r^2 v_3 \\
& + 5760 b_v b^2 q^3 r^2 a^3 v_2 + 2160 b^2 a^4 U2 q^3 r^2 - 480 p a^4 U3 b q^3 r^2 + 720 s a^4 U3 b q^3 r^2
\end{aligned}$$

$$\begin{aligned}
& + 480 q^3 a^5 r^2 s_v v_3 - 1440 b q^3 r^2 a^4 s_v v_3 - 2400 b_v b^2 s a^2 q^3 r^2 v_3 - 7200 a_u b^2 a^3 q^3 r^2 u_2 \\
& + 6240 a_u b^3 a^2 q^3 r^2 u_2 + 3360 a_u b a^4 q^3 r^2 u_2 - 480 a_u q^4 a^4 r^2 v_3 + 480 b_v p a^4 q^3 r^2 v_3 \\
& - 3840 b_v a^4 b q^3 r^2 v_2 + 2400 a_u b^2 s a^2 q^3 r^2 u_3 - 480 b_v s a^4 q^3 r^2 v_3 - 2400 b_v b^2 r^3 a^2 q^3 u_3 \\
& + 2400 b_v b^2 p a^2 q^3 r^2 v_3 + 960 b_v b^4 a q^3 r^2 v_2 - 2400 a_u b^2 p a^2 q^3 r^2 u_3 - 240 a^5 U1 q^3 r^2 \\
& - 1920 a_u b^4 q^3 a r^2 u_2 + 960 b_v q^3 a^5 r^2 v_2 + 1440 s_u b^2 a^3 q^3 r^2 u_3 - 480 s_u b^3 a^2 q^3 r^2 u_3 \\
& - 960 a_v b^4 q^3 r^2 a v_2 - 2880 a_v b^2 q^3 a^3 r^2 v_2 - 1440 s_u a^4 b q^3 r^2 u_3 - 480 a_v a^4 r^3 q^3 u_3 \\
& + 2880 a_v b^3 a^2 q^3 r^2 v_2 + 960 a_v a^4 b q^3 r^2 v_2 - 2400 b_u b^2 q^4 a^2 r^2 v_3 - 480 b_u b^3 a^2 q^3 r^2 u_2 \\
& + 480 s_u a^5 q^3 r^2 u_3 - 960 b^4 q^3 r^2 a p_u u_3 + 480 b^4 q^3 r^2 U3 a p + 2880 b^3 q^3 r^2 a^2 p_u u_3 \\
& + 2880 b^3 q^3 r^2 a^2 p_v v_3 + 720 b^4 q^3 a^2 r^2 U2 + 1440 b^2 q^3 a^3 r^2 b_u u_2 - 1440 b^3 q^3 r^2 U3 a^2 p \\
& + 960 b^3 q^4 r^2 a b_u v_3 + 960 b^3 q^3 r^3 a a_v u_3 - 960 b^4 q^3 r^2 a p_v v_3 + 240 b^3 q^3 s a^2 r^2 U3 \\
& + 960 b^3 q^4 a r^2 a_u v_3 + 960 b^3 q^3 r^3 a b_v u_3 - 2160 b^3 q^3 a^3 r^2 U2 - 480 q^3 a^2 r^2 b^3 s_v v_3 \\
& - 720 q^3 s a^3 r^2 U3 b^2 - 480 q^3 p a^4 r^2 a_u u_3 + 1440 q^3 a^3 r^2 b^2 s_v v_3 + 480 q^3 a^4 r^2 s a_u u_3 \\
& - 2880 q^3 a^3 r^2 b^2 p_u u_3 - 2880 q^3 a^3 r^2 b^2 p_v v_3 + 1440 q^3 a^3 r^2 U3 b^2 p + 960 q^3 a^4 r^2 b p_v v_3 \\
& + 960 q^3 a^4 r^2 b p_u u_3 - 1440 q^3 a^4 r^2 b b_u u_2 + 1920 q^3 a^3 r^3 b b_v u_3 + 1920 q^4 a^3 r^2 b a_u v_3 \\
& + 1920 q^4 a^3 r^2 b b_u v_3 + 1920 q^3 a^3 r^3 b a_v u_3
\end{aligned}$$

> Leq4 := simplify(diff(numer(XX3), g1\$4, g2\$3))

$$\begin{aligned}
\text{Leq4} := & 144 r \left( -8 b^2 q^2 a^2 r^2 s a_v u_3 - 16 a_u b^2 q^2 s a^2 r p u_3 + 8 a_u b^2 q^2 s^2 a^2 r u_3 \right. \\
& + 8 a_u b^2 q^2 p^2 a^2 r u_3 + 16 b_v b^2 q^2 s a^2 r p v_3 - 8 b_v b^2 q^2 s^2 a^2 r v_3 - 8 b_v b^2 q^2 p^2 a^2 r v_3 \\
& + 8 b^2 q^2 a^2 r^2 p a_v u_3 + 8 b^2 q^2 a^2 r^2 p b_v u_3 - 4 q^2 a r^2 b^4 s_v u_3 + 8 b q^2 r^2 a^4 q_v v_3 \\
& - 4 q^3 a^4 r^2 U3 b + 12 q^3 a^3 r^2 U3 b^2 - 12 b^3 q^3 r^2 U3 a^2 + 4 b^4 q^3 r^2 U3 a \\
& - 24 q_u a^3 r^2 b^2 q^2 u_3 + 8 r_u q^3 a^4 b r u_3 + 24 r_u b^3 q^3 a^2 r u_3 - 8 r_u b^4 q^3 a r u_3 \\
& + 24 q_u b^3 r^2 a^2 q^2 u_3 - 8 q_u b^4 r^2 a q^2 u_3 + 8 q_u b q^2 a^4 r^2 u_3 - 8 r_v b^4 q^3 a r v_3 \\
& + 8 r_v b q^3 r a^4 v_3 + 4 b_v b^4 q^2 a r s v_2 - 4 b_v b^4 q^2 p r a v_2 - 24 r_u b^2 q^3 a^3 r u_3 \\
& - 4 p_u b q^2 s a^4 r u_3 + 4 p_u b^4 q^2 s a r u_3 + 4 p_u b q^2 p a^4 r u_3 - 4 p_u b^4 q^2 p a r u_3 \\
& - 16 p_u b^2 q^2 a^4 r u_2 - 12 p_u b^2 q^3 a^3 r v_3 + 12 p_u b^3 q^3 a^2 r v_3 + 24 p_u b^3 q^2 a^3 r u_2 \\
& - 16 p_u b^4 q^2 a^2 r u_2 + 24 q_v q^2 a^2 r^2 b^3 v_3 - 8 q_v b^4 q^2 r^2 a v_3 - 24 r_v b^2 q^3 a^3 r v_3 \\
& + 24 r_v b^3 q^3 a^2 r v_3 - 4 b_u q^3 a^3 b p r v_3 + 4 b_u q^3 s a^3 b r v_3 - 8 b_u q^3 s a^2 b^2 r v_3 \\
& + 4 b_u b^3 q^3 s a r v_3 + 8 b_u b^2 q^3 p a^2 r v_3 - 4 b_u b^3 q^3 p a r v_3 - 24 q_v q^2 a^3 r^2 b^2 v_3 \\
& + 4 p_u b q^3 a^4 r v_3 + 4 p_u b q^2 a^5 r u_2 + 4 p_u b^5 q^2 a r u_2 - 4 p_u b^4 q^3 r a v_3 \\
& \left. - 4 a_v b q^2 p r^2 a^3 u_3 + 4 a_v b q^2 r^2 a^3 s u_3 - 4 s_v b q^2 a^5 r v_2 - 4 s_v b^5 q^2 a r v_2 \right)
\end{aligned} \tag{71}$$

$$\begin{aligned}
& + 4 p_v a^4 r^2 b q^2 u_3 + 12 p_v b^3 a^2 r^2 q^2 u_3 - 12 p_v b^2 a^3 r^2 q^2 u_3 - 4 p_v b^4 a r^2 q^2 u_3 \\
& + 4 s_v b a^4 q^2 r s v_3 - 24 s_v b^3 a^3 q^2 r v_2 - 4 s_v p a^4 b q^2 r v_3 + 12 s_v p a^3 b^2 q^2 r v_3 \\
& + 16 s_v b^4 a^2 q^2 r v_2 - 12 s_v b^3 p a^2 q^2 r v_3 - 12 s_u b^2 q^3 a^3 r v_3 - 4 s_u b^4 q^3 a r v_3 \\
& - 4 a_u b^3 p^2 a q^2 r u_3 + 4 s_v b a^4 r^2 q^2 u_3 + 12 s_v b^3 a^2 r^2 q^2 u_3 + 16 s_v b^2 a^4 q^2 r v_2 \\
& + 12 s_v b^3 a^2 q^2 r s v_3 + 4 s_v b^4 a p q^2 r v_3 - 12 s_v b^2 a^3 r^2 q^2 u_3 - 12 s_v b^2 s a^3 q^2 r v_3 \\
& - 4 s_v b^4 s a q^2 r v_3 - 4 a_u a^4 b p q^2 r u_2 + 4 s_u b q^3 a^4 r v_3 + 12 s_u b^3 q^3 a^2 r v_3 \\
& + 4 a_u b^4 a p q^2 r u_2 + 4 a_u b s a^4 q^2 r u_2 - 4 b_v a^4 b q^2 r s v_2 - 4 a_u q^2 s^2 a r b^3 u_3 \\
& - 12 a_u q^2 a^2 r b^3 p u_2 - 4 a_u b^4 s a q^2 r u_2 + 4 b_v p a^4 b q^2 r v_2 - 4 a_u q^3 a r b^3 p v_3 \\
& + 4 a_u q^3 s a r b^3 v_3 - 4 a_u b q^2 r a^3 s^2 u_3 - 4 a_u b q^2 p^2 r a^3 u_3 + 12 a_u q^2 s a^2 r b^3 u_2 \\
& - 4 a_u b q^3 p r a^3 v_3 + 4 a_u b q^3 r a^3 s v_3 - 12 a_u b^2 q^2 r a^3 s u_2 + 8 a_u b^2 q^3 r a^2 p v_3 \\
& - 8 a_u b^2 q^3 r a^2 s v_3 + 12 a_u b^2 q^2 p r a^3 u_2 + 12 b_v q^2 a^2 r b^3 p v_2 - 12 b_v q^2 s a^2 r b^3 v_2 \\
& - 4 b_v q^2 a r^2 b^3 p u_3 + 4 b_v q^2 a r b^3 p^2 v_3 - 8 b_v q^2 s r^2 a^2 b^2 u_3 + 4 b_v q^2 s r^2 a b^3 u_3 \\
& + 4 b_v q^2 s^2 a r b^3 v_3 + 4 b_v q^2 s^2 r a^3 b v_3 + 4 b_v b q^2 p^2 r a^3 v_3 - 4 b_v b q^2 p r^2 a^3 u_3 \\
& + 4 b_v b q^2 r^2 a^3 s u_3 - 12 b_v b^2 q^2 p r a^3 v_2 + 12 b_v b^2 q^2 r a^3 s v_2 - 12 p_u b^2 a^3 p q^2 r u_3 \\
& + 12 p_u b^2 a^3 q^2 r s u_3 + 12 p_u b^3 a^2 p q^2 r u_3 - 12 p_u b^3 s a^2 q^2 r u_3 - 4 a_v b^3 r^2 a p q^2 u_3 \\
& + 4 a_v b^3 r^2 a q^2 s u_3 + 8 a_u s p a^3 b q^2 r u_3 + 8 a_u b^3 s a p q^2 r u_3 - 8 b_v p a^3 b q^2 r s v_3 \\
& - 8 b_v b^3 p a q^2 r s v_3)
\end{aligned}$$

> *Leq5 := simplify(diff(numer(XX3), g1\$3, g2\$4))*

$$\begin{aligned}
& Leq5 := 144 r \left( b^5 U1 q^2 r^2 + 4 q^2 a^4 r^2 b s_u u_3 + 4 q^2 a^4 r^2 b s_v v_3 + 6 q^2 a^3 r^2 U3 b^2 s \right. \\
& - 3 b^2 q^2 a^4 r^2 U2 - 2 b q^2 s a^4 r^2 U3 - 4 b^4 q^2 r^2 a s_u u_3 + 2 b^4 q^2 r^2 U3 a s \\
& - b^2 q^2 p a^3 r^2 U3 - 3 b^4 q^2 p a r^2 U3 + 3 b^3 q^2 p r^2 U3 a^2 + 9 b^3 q^2 a^3 r^2 U2 \\
& - 9 b^4 q^2 a^2 r^2 U2 - 6 b^3 q^2 r^2 U3 a^2 s + 4 b_u b q^2 a^4 r^2 u_2 - 4 b_u b^4 q^2 a r^2 u_2 \\
& + 6 a_v b^4 q^2 a r^2 v_2 + b^5 q^2 r^2 U3 p + 3 b^5 q^2 a r^2 U2 - 4 b_u q^3 a^3 b r^2 v_3 - 12 b_u b^2 a^3 q^2 r^2 u_2 \\
& + 2 b_u b^4 q^3 r^2 v_3 + 10 b_u q^3 a^2 r^2 b^2 v_3 - 8 b_u q^3 a r^2 b^3 v_3 + 12 b_u b^3 a^2 q^2 r^2 u_2 \\
& - 6 p_u b^3 a^2 q^2 r^2 u_3 + 2 p_u b^2 a^3 q^2 r^2 u_3 - 8 a_v q^2 a r^3 b^3 u_3 - 4 a_v q^2 r^3 a^3 b u_3 \\
& + 2 a_v b^2 a^3 q^2 r^2 v_2 + 10 a_v b^2 q^2 r^3 a^2 u_3 + 2 a_v b^4 q^2 r^3 u_3 - 6 a_v b^3 q^2 r^2 a^2 v_2 \\
& - 2 a_v b^5 q^2 r^2 v_2 + 6 p_v q^2 a r^2 b^4 v_3 - 2 p_v b^5 q^2 r^2 v_3 + 2 p_v b^2 a^3 q^2 r^2 v_3 - 6 p_v b^3 a^2 q^2 r^2 v_3 \\
& - 12 s_v b^2 a^3 q^2 r^2 v_3 - 4 s_v q^2 a r^2 b^4 v_3 + 12 s_v b^3 a^2 q^2 r^2 v_3 - 12 s_u b^2 a^3 q^2 r^2 u_3 \\
& - 10 a_u s a^2 b^2 q^2 r^2 u_3 + 12 s_u b^3 a^2 q^2 r^2 u_3 + 16 a_u b^2 a^3 q^2 r^2 u_2 + 10 a_u p a^2 b^2 q^2 r^2 u_3 \\
& \left. - 4 a_u p a^3 b q^2 r^2 u_3 + 4 a_u s a^3 b q^2 r^2 u_3 - 2 b_v q^2 p r^2 b^4 v_3 - 4 a_u b^5 q^2 r^2 u_2 \right)
\end{aligned} \tag{72}$$

$$\begin{aligned}
& -4 a_u q^3 a^3 b r^2 v_3 + 4 b_v p a^3 b q^2 r^2 v_3 + 8 a_u b^3 s a q^2 r^2 u_3 - 8 a_u b^3 p a q^2 r^2 u_3 \\
& -24 a_u b^3 a^2 q^2 r^2 u_2 - 4 a_u b q^2 a^4 r^2 u_2 + 2 a_u b^4 q^2 p r^2 u_3 - 2 a_u b^4 q^2 s r^2 u_3 \\
& + 16 a_u b^4 q^2 a r^2 u_2 + 8 b_v b q^2 a^4 r^2 v_2 + 6 p_u b^4 a q^2 r^2 u_3 - 8 a_u b^3 q^3 a r^2 v_3 \\
& + 10 a_u b^2 q^3 r^2 a^2 v_3 + 2 a_u b^4 q^3 r^2 v_3 - 10 b_v p a^2 b^2 q^2 r^2 v_3 - 4 b_v q^2 r^3 a^3 b u_3 \\
& + 2 b_v q^2 s r^2 b^4 v_3 + 10 b_v q^2 r^3 a^2 b^2 u_3 + 8 b_v b^3 p a q^2 r^2 v_3 - 8 b_v b^3 r^3 a q^2 u_3 \\
& + 2 b_v b^4 q^2 r^3 u_3 + 2 b_v b^5 q^2 r^2 v_2 - 8 b_v q^2 s r^2 a b^3 v_3 - 26 b_v b^2 q^2 r^2 a^3 v_2 \\
& + 30 b_v b^3 q^2 r^2 a^2 v_2 - 14 b_v b^4 q^2 r^2 a v_2 - 2 b q^2 a^4 r^2 U1 - 3 b^3 q^2 a^2 r^2 U1 - b^4 q^2 a r^2 U1 \\
& + 5 b^2 q^2 a^3 r^2 U1 - 4 b_v q^2 s r^2 a^3 b v_3 + 10 b_v q^2 s r^2 a^2 b^2 v_3 - 2 p_u b^5 q^2 r^2 u_3)
\end{aligned}$$

$$\begin{aligned}
& \text{> [diff(Leq5, U1), diff(Leq5, U2), diff(Leq5, U3)]} \\
& [144 r (-2 b q^2 a^4 r^2 - b^4 q^2 a r^2 + 5 a^3 b^2 q^2 r^2 + b^5 q^2 r^2 - 3 b^3 a^2 q^2 r^2), 144 r (3 b^5 q^2 a r^2 \\
& - 9 b^4 a^2 q^2 r^2 - 3 b^2 a^4 q^2 r^2 + 9 b^3 a^3 q^2 r^2), 144 r (3 b^3 q^2 a^2 r^2 p - b^2 q^2 a^3 r^2 p \\
& - 2 b q^2 s a^4 r^2 - 6 b^3 q^2 a^2 r^2 s - 3 b^4 q^2 p a r^2 + 6 b^2 q^2 a^3 r^2 s + 2 b^4 q^2 a r^2 s + b^5 p q^2 r^2) \\
& ]
\end{aligned} \tag{73}$$

$$\begin{aligned}
& \text{> Leq6 := simplify(diff(numer(XX3), g1$2, g2$5))} \\
& \text{Leq6 := } 240 r (2 b_v p^2 a^2 b^2 q r^2 v_3 - 4 b_v b^3 p^2 a q r^2 v_3 - 4 b_v b^4 s p q r^2 v_3 + 6 b_v b^4 a p q r^2 v_2 \\
& - 6 b_v b^4 a q r^2 s v_2 - 2 b_v b^4 p r^3 q u_3 + 2 b_v b^4 s^2 q r^2 v_3 - 2 q^2 a^3 r^3 U3 b^2 \\
& + 4 r_u q^2 a^3 b^2 r^2 u_3 + 12 r_u b^4 q^2 a r^2 u_3 + 4 q_u a^3 r^3 b^2 q u_3 + 12 q_u b^4 r^3 a q u_3 \\
& + 4 q_v a^3 r^3 b^2 q v_3 - 2 b_u b^4 q^2 p r^2 v_3 + 2 b_u b^4 q^2 r^2 s v_3 + 12 q_v b^4 a r^3 q v_3 \\
& - 2 p_u a^3 b^2 q r^2 s u_3 - 6 p_u b^3 a^2 p q r^2 u_3 + 6 p_u b^3 a^2 q r^2 s u_3 + 2 p_u p a^3 b^2 q r^2 u_3 \\
& - 4 b^5 q^2 r^2 r_v v_3 - 2 b^5 q^2 r^2 s_u v_3 - 6 b^4 q^2 r^3 U3 a - 6 p_u b^3 q^2 a^2 r^2 v_3 - 6 p_u b^4 s a q r^2 u_3 \\
& + 4 a_v a r^3 b^3 p q u_3 + 6 p_u b^4 q^2 a r^2 v_3 + 6 p_u b^4 p a q r^2 u_3 + 12 p_u b^4 a^2 q r^2 u_2 \\
& - 2 a_v a^2 r^3 b^2 p q u_3 + 2 a_v a^2 r^3 b^2 q s u_3 - 4 a_v s a r^3 b^3 q u_3 + 2 p_v a^3 r^3 b^2 q u_3 \\
& - 6 p_v b^3 a^2 r^3 q u_3 + 2 p_u q^2 a^3 b^2 r^2 v_3 + 2 p_u b^2 a^4 q r^2 u_2 - 2 s_v p a^3 b^2 q r^2 v_3 \\
& - 2 a_v b^4 p r^3 q u_3 - 12 s_v b^4 a^2 q r^2 v_2 + 2 a_v b^4 r^3 q s u_3 + 6 p_v b^4 r^3 a q u_3 \\
& + 4 a_u p a^2 b^2 q r^2 s u_3 - 2 a_u p a^3 b^2 q r^2 u_2 - 8 a_u s a b^3 p q r^2 u_3 + 2 s_v s a^3 b^2 q r^2 v_3 \\
& - 2 s_v b^2 a^4 q r^2 v_2 + 6 s_v b^3 a^2 p q r^2 v_3 - 6 s_v b^3 a^2 q r^2 s v_3 - 6 s_v b^4 a p q r^2 v_3 \\
& + 2 a_u b^4 q^2 s r^2 v_3 - 2 b_v s a^3 b^2 q r^2 v_2 + 2 b_v s^2 a^2 b^2 q r^2 v_3 - 2 a_u q^2 a^2 b^2 p r^2 v_3 \\
& + 2 a_u q^2 a^2 b^2 r^2 s v_3 - 2 a_u s^2 a^2 b^2 q r^2 u_3 - 4 a_u q^2 s a b^3 r^2 v_3 + 4 a_u b^3 p^2 a q r^2 u_3 \\
& + 4 a_u q^2 p a b^3 r^2 v_3 + 4 a_u b^4 s p q r^2 u_3 - 6 a_u b^3 s a^2 q r^2 u_2 + 6 a_u b^3 a^2 p q r^2 u_2 \\
& - 2 a_u b^4 q^2 p r^2 v_3 - 6 s_v b^3 a^2 r^3 q u_3 + 6 s_v b^4 a q r^2 s v_3 + 6 a_u b^4 a q r^2 s u_2 \\
& - 6 a_u b^4 p a q r^2 u_2 - 2 a_u b^4 p^2 q r^2 u_3 + 4 a_u b^3 s^2 a q r^2 u_3 + 2 a_u a^3 b^2 q r^2 s u_2)
\end{aligned} \tag{74}$$

$$\begin{aligned}
& -2 a_u p^2 a^2 b^2 q r^2 u_3 + 8 b_v s a b^3 p q r^2 v_3 - 4 b_v s p a^2 b^2 q r^2 v_3 + 2 b_v p a^3 b^2 q r^2 v_2 \\
& + 2 a_u b^5 p q r^2 u_2 - 2 a_u b^4 s^2 q r^2 u_3 - 2 a_u b^5 s q r^2 u_2 - 4 r_u b^5 q^2 r^2 u_3 - 4 q_u b^5 r^3 q u_3 \\
& - 4 q_v b^5 r^3 q v_3 + 2 p_u b^5 q r^2 s u_3 - 2 p_v b^5 r^3 q u_3 + 2 b^5 q^2 r^3 U3 + 2 b^4 q r^2 p^2 b_v v_3 \\
& + 2 b^4 q r^3 s b_v u_3 - 2 b^5 q s r^2 s_v v_3 - 2 p_u b^5 q^2 r^2 v_3 - 2 p_u b^5 p q r^2 u_3 - 8 p_u b^5 a q r^2 u_2 \\
& + 8 b^5 q r^2 a s_v v_2 - 2 b^5 q r^2 p b_v v_2 + 2 b^5 q r^2 s b_v v_2 + 2 s_v b^5 p q r^2 v_3 - 6 b^3 q a^2 r^2 p b_v v_2 \\
& + 6 b^3 q a^2 r^2 s b_v v_2 - 4 b_v b^3 s^2 a q r^2 v_3 - 12 b^3 q a^2 r^3 q_v v_3 + 2 q^2 a^3 r^2 b^2 s_u v_3 \\
& - 2 q p a^2 r^3 b^2 b_v u_3 + 6 b^4 q^2 a r^2 s_u v_3 + 6 b^3 q^2 a^2 r^3 U3 + 2 q a^2 r^3 b^2 s b_v u_3 \\
& + 4 b^3 q p r^3 a b_v u_3 - 4 b^3 q r^3 a s b_v u_3 - 12 r_u b^3 q^2 a^2 r^2 u_3 - 12 q_u b^3 a^2 r^3 q u_3 \\
& + 4 r_v q^2 a^3 r^2 b^2 v_3 - 12 r_v q^2 a^2 r^2 b^3 v_3 + 12 r_v b^4 q^2 r^2 a v_3 + 2 b_u q^2 a^2 b^2 r^2 s v_3 \\
& - 2 b_u q^2 p a^2 b^2 r^2 v_3 + 2 b^2 q a^3 r^3 s_v u_3 + 4 b^3 q^2 a r^2 p b_u v_3 - 4 b^3 q^2 a r^2 s b_u v_3 \\
& - 6 b^3 q^2 a^2 r^2 s_u v_3 + 6 q a r^3 b^4 s_v u_3 - 2 b^5 q r^3 s_v u_3 - 2 b^6 q r^2 s_v v_2 + 2 p_u b^6 q r^2 u_2 \\
& - 8 p_u a^3 b^3 q r^2 u_2 + 8 s_v a^3 b^3 q r^2 v_2)
\end{aligned}$$

$$\begin{aligned}
& \text{> } [\text{diff}(\text{Leq6}, U1), \text{diff}(\text{Leq6}, U2), \text{diff}(\text{Leq6}, U3)] \\
& \quad [0, 0, 240 r (-2 a^3 b^2 q^2 r^3 + 2 b^5 q^2 r^3 + 6 b^3 q^2 a^2 r^3 - 6 b^4 a q^2 r^3)] \quad (75)
\end{aligned}$$

$$\begin{aligned}
& \text{> } \text{Leq7} := \text{simplify}(\text{diff}(\text{numer}(\text{XX3}), g_1\$1, g_2\$6)) \\
& \text{Leq7} := 720 b r^2 (-4 a_u s a b^2 q r^2 u_3 - 2 a_u b^3 p q r^2 u_3 - 6 a_u b^3 a q r^2 u_2 - 2 a_u b^3 q^2 r^2 v_3 \quad (76)
\end{aligned}$$

$$\begin{aligned}
& + 2 a_u b^3 s q r^2 u_3 - 2 a_u q^2 a^2 b r^2 v_3 + 4 a_u q^2 a b^2 r^2 v_3 + 12 b_v b^3 a q r^2 v_2 \\
& + 4 b q a^3 r^2 b_v v_2 + 6 s_u b^3 a q r^2 u_3 - 2 a_u p a^2 b q r^2 u_3 + 4 a_u p a b^2 q r^2 u_3 \\
& - 3 b^3 s a U3 q r^2 + 6 b_u b^3 a q r^2 u_2 - 2 a_v a^2 r^3 b q u_3 - 2 a_v b^3 r^3 q u_3 + 4 a_v a r^3 b^2 q u_3 \\
& + 2 a_u s a^2 b q r^2 u_3 - 2 b^3 q^2 r^2 b_u v_3 - 2 b^3 q r^2 s b_v v_3 + 2 b^3 q r^2 p b_v v_3 - 2 q^2 a^2 r^2 b b_u v_3 \\
& + 2 q a^2 r^2 b p b_v v_3 - 2 q a^2 r^2 b s b_v v_3 - s a^3 U3 b q r^2 + 3 s a^2 U3 b^2 q r^2 \\
& - 2 a_u a^3 b q r^2 u_2 + 6 a_u a^2 b^2 q r^2 u_2 - 2 s_u b^4 q r^2 u_3 - 2 b q r^3 a^2 b_v u_3 + 4 q a r^3 b^2 b_v u_3 \\
& + 6 q a r^2 b^3 s_v v_3 - 2 b^3 q r^3 b_v u_3 - 2 b^4 q r^2 s_v v_3 - 4 b^4 q r^2 b_v v_2 + b^4 s U3 q r^2 \\
& + 3 b^3 a^2 U2 q r^2 - 3 b^4 a U2 q r^2 - 3 b^3 a U1 q r^2 - b^2 a^3 U2 q r^2 - 12 b_v a^2 b^2 q r^2 v_2 \\
& + 2 a_u b^4 q r^2 u_2 - 2 b_u b^4 q r^2 u_2 + 2 b_u a^3 b q r^2 u_2 - 6 b_u a^2 b^2 q r^2 u_2 + 2 s_u a^3 b q r^2 u_3 \\
& - 6 s_u a^2 b^2 q r^2 u_3 + 2 s_v a^3 b q r^2 v_3 + 3 b^2 a^2 U1 q r^2 - 4 b^2 q a r^2 p b_v v_3 - 6 b^2 q a^2 r^2 s_v v_3 \\
& + 4 b^2 q^2 a r^2 b_u v_3 + 4 b^2 q a r^2 s b_v v_3 + b^4 U1 q r^2 - a^3 U1 b q r^2 + b^5 U2 q r^2)
\end{aligned}$$

$$\begin{aligned}
& \text{> } [\text{diff}(\text{Leq7}, U1), \text{diff}(\text{Leq7}, U2), \text{diff}(\text{Leq7}, U3)] \\
& \quad [720 b r^2 (-3 b^3 a q r^2 + 3 b^2 a^2 q r^2 + b^4 q r^2 - a^3 b q r^2), 720 b r^2 (3 b^3 a^2 q r^2 - 3 b^4 a q r^2 \\
& \quad - b^2 a^3 q r^2 + b^5 q r^2), 720 b r^2 (b^4 s q r^2 - s a^3 b q r^2 + 3 s a^2 b^2 q r^2 - 3 b^3 s a q r^2)] \quad (77)
\end{aligned}$$

$$\text{> } \text{Leq8} := \text{simplify}(\text{diff}(\text{numer}(\text{XX3}), g_2\$7))$$

$$\text{Leq8} := 0 \quad (78)$$

As we saw above we can solve some equations, and check the equality (above  $U3=\Omega[3]$ ); however if we try to do this with the whole set of 7 (linear inhomogeneous) equations on 3 unknowns, the system refuses (probably because of simplification complexity)

$$\begin{aligned} &> \text{solve}([ \text{Leq1}, \text{Leq2}, \text{Leq3}, \text{Leq4}, \text{Leq5}, \text{Leq6}, \text{Leq7}], [U1, U2, U3]) \\ &\quad [ ] \end{aligned} \quad (79)$$

$$\begin{aligned} &> \text{solve}([ \text{Leq1}, \text{Leq2}, \text{Leq3}], [U1, U2, U3]) \\ &\quad [ \text{Length of output exceeds limit of 1000000} ] \end{aligned} \quad (80)$$

But this is not a big deal. 1. We check that  $U=\Omega$  is a solution (double-checking the above calculation). 2. Check that there is no more than one solution, i.e. that the rank of the 7x3 matrix of the homogeneous part of the system is 3.

$$\begin{aligned} &> \text{simplify}(\text{subs}([U1 = \Omega[1], U2 = \Omega[2], U3 = \Omega[3]], [\text{Leq1}, \text{Leq2}, \text{Leq3}, \text{Leq4}, \text{Leq5}, \text{Leq6}, \\ &\quad \text{Leq7}])) \\ &\quad [0, 0, 0, 0, 0, 0, 0] \end{aligned} \quad (81)$$

$$\begin{aligned} &> \text{Mat} := \text{Matrix}([[\text{diff}(\text{Leq1}, U1), \text{diff}(\text{Leq1}, U2), \text{diff}(\text{Leq1}, U3)], [\text{diff}(\text{Leq2}, U1), \\ &\quad \text{diff}(\text{Leq2}, U2), \text{diff}(\text{Leq2}, U3)], [\text{diff}(\text{Leq3}, U1), \text{diff}(\text{Leq3}, U2), \text{diff}(\text{Leq3}, U3)], \\ &\quad [\text{diff}(\text{Leq4}, U1), \text{diff}(\text{Leq4}, U2), \text{diff}(\text{Leq4}, U3)], [\text{diff}(\text{Leq5}, U1), \text{diff}(\text{Leq5}, U2), \\ &\quad \text{diff}(\text{Leq5}, U3)], [\text{diff}(\text{Leq6}, U1), \text{diff}(\text{Leq6}, U2), \text{diff}(\text{Leq6}, U3)], [\text{diff}(\text{Leq7}, U1), \\ &\quad \text{diff}(\text{Leq7}, U2), \text{diff}(\text{Leq7}, U3)]]): \\ &> \text{mMat} := \text{SubMatrix}(\text{Mat}, [1..3], [1..3]) \\ \text{mMat} := &[[-5040 a q (-b^3 a q^3 r + 3 b^2 a^2 q^3 r + a^4 q^3 r - 3 b a^3 q^3 r), -5040 a q (-b^3 a^2 q^3 r \\ &\quad + a^5 q^3 r + 3 b^2 a^3 q^3 r - 3 b a^4 q^3 r), -5040 a q (3 b^2 p a^2 q^3 r - 3 b p a^3 q^3 r - b^3 p a q^3 r \\ &\quad + p a^4 q^3 r)], \\ &[0, 0, 720 a (-2 q^4 a^4 r^2 - 6 b^2 q^4 a^2 r^2 + 2 b^3 q^4 r^2 a + 6 b q^4 a^3 r^2)], \\ &[720 b^2 a^3 q^3 r^2 - 1200 b^3 a^2 q^3 r^2 - 240 a^5 q^3 r^2 + 240 a^4 b q^3 r^2 + 480 b^4 a q^3 r^2, \\ &\quad -2160 b^3 a^3 q^3 r^2 + 720 b^4 a^2 q^3 r^2 + 2160 b^2 a^4 q^3 r^2 - 720 a^5 b q^3 r^2, 240 b^3 s a^2 q^3 r^2 \\ &\quad - 480 p a^4 b q^3 r^2 + 720 s a^4 b q^3 r^2 - 1440 b^3 p a^2 q^3 r^2 + 1440 b^2 p a^3 q^3 r^2 \\ &\quad + 480 b^4 p a q^3 r^2 - 720 b^2 s a^3 q^3 r^2 - 240 s a^5 q^3 r^2]] \\ &> \text{factor}(\text{Determinant}(\text{mMat})) \\ &\quad -1741824000 q^{11} r^5 a^6 (a-b)^2 (b-a)^8 \end{aligned} \quad (82)$$

$$\begin{aligned} &> \text{mMat2} := \text{SubMatrix}(\text{Mat}, [1, 3], [1, 2]) \\ \text{mMat2} := &[[-5040 a q (-b^3 a q^3 r + 3 b^2 a^2 q^3 r + a^4 q^3 r - 3 b a^3 q^3 r), -5040 a q (-b^3 a^2 q^3 r \\ &\quad + a^5 q^3 r + 3 b^2 a^3 q^3 r - 3 b a^4 q^3 r)], \\ &[720 b^2 a^3 q^3 r^2 - 1200 b^3 a^2 q^3 r^2 - 240 a^5 q^3 r^2 + 240 a^4 b q^3 r^2 + 480 b^4 a q^3 r^2, \\ &\quad -2160 b^3 a^3 q^3 r^2 + 720 b^4 a^2 q^3 r^2 + 2160 b^2 a^4 q^3 r^2 - 720 a^5 b q^3 r^2]] \end{aligned} \quad (84)$$

$$\begin{aligned} &> \text{factor}(\text{Determinant}(\text{mMat2})) \\ &\quad -1209600 a^3 q^6 r^2 (b-a)^4 (a-b) (-2 b a^2 q r + a^3 q r + b^2 a q r) \\ &> \text{factor}(-1209600 a^3 q^6 r^2 (b-a)^4 (a-b) (-2 b a^2 q r + a^3 q r + b^2 a q r)) \end{aligned} \quad (85)$$



|  
=  
Done!  
=  
>  
=  
>  
=  
>  
=  
>

$$-1209600\,a^4\,q^7\,r^3\,(a-b)^7$$

(86)
