# Supplementary material for: Dispersionless integrable systems in 3D and Einstein-Weyl geometry
Source: arXiv:1208.2728 ancillary file (2013-05-09)
Supplement: Supplementary file 9 [file BKEF-2012-IV-2D_component_quasilinear_integrability.pdf]

This is the worksheet accompanying the paper E.Ferapontov & B.Kruglikov "Dispersionless integrable systems in 3D and Einstein-Weyl geometry".

The file ran on **Maple** version 16, the package **DifferentialGeometry** was used.

We consider the 2 component systems of hydrodynamic type and study it's integrability via EW property of the linearization conformal structure

```
>
> with(DifferentialGeometry) : with(Tensor) : with(Tools) : with(JetCalculus) :
  with(LinearAlgebra) : with(PDEtools, D_Dx, declare, ToJet, FromJet) :
> alias(f=f(u2,2, u2,3, u3,3, u1,2, u1,3)) : declare(a(u[], v[])) : declare(b(u[], v[])) :
  declare(p(u[], v[])) : declare(q(u[], v[])) : declare(r(u[], v[])) : declare(s(u[], v[])) :

      a(u[], v[]) will now be displayed as a
      b(u[], v[]) will now be displayed as b
      p(u[], v[]) will now be displayed as p
      q(u[], v[]) will now be displayed as q
      r(u[], v[]) will now be displayed as r
      s(u[], v[]) will now be displayed as s
```

(1)

```
> DGsetup([t, x, y], [u, v], J2, 3) :
> F := u1 + a(u[], v[]) · u2 + p(u[], v[]) · u3 + q(u[], v[]) · v3;
  G := v1 + b(u[], v[]) · v2 + r(u[], v[]) · u3 + s(u[], v[]) · v3;
      F := u1 + a u2 + p u3 + q v3
      G := v1 + b v2 + r u3 + s v3
```

(2)

```
> DR := (diff(F, u1) · ξ1 + diff(F, u2) · ξ2 + diff(F, u3) · ξ3) · (diff(G, v1) · ξ1 + diff(G, v2) · ξ2
  + diff(G, v3) · ξ3) - (diff(F, v1) · ξ1 + diff(F, v2) · ξ2 + diff(F, v3) · ξ3) · (diff(G, u1) · ξ1
  + diff(G, u2) · ξ2 + diff(G, u3) · ξ3)
      DR := (ξ1 + a ξ2 + p ξ3) (ξ1 + b ξ2 + s ξ3) - q ξ32 r
```

(3)

```
> A := 2 · Matrix(⌈⌈⌈⌈ 1/2 diff(DR, ξ1, ξ1), 1/2 diff(DR, ξ1, ξ2), 1/2 diff(DR, ξ1, ξ3) ⌋, ⌈ 1/2 diff(DR,
  ξ1, ξ2), 1/2 diff(DR, ξ2, ξ2), 1/2 diff(DR, ξ2, ξ3) ⌋, ⌈ 1/2 diff(DR, ξ1, ξ3), 1/2 diff(DR, ξ2, ξ3),
  1/2 diff(DR, ξ3, ξ3) ⌋⌋⌋)
      A := ⌈ 2      b + a      s + p
      b + a      2 a b      a s + p b
      s + p      a s + p b      2 p s - 2 q r ⌋
```

(4)

```
> AA := expand(MatrixInverse(A)); factor(Determinant(A))
```

```
AA := ⌈⌈⌈ -1/2      -2 a s p b + 4 a b q r + a2 s2 + p2 b2
      q r (-2 a b + b2 + a2)
```

$$\begin{aligned} & \frac{1}{2} \frac{-b p s + 2 b q r - a p s + 2 a q r + a s^2 + p^2 b}{q r (-2 a b + b^2 + a^2)}, -\frac{1}{2} \frac{-p b + a s}{(-a + b) q r} \Big], \\ & \left[ \frac{1}{2} \frac{-b p s + 2 b q r - a p s + 2 a q r + a s^2 + p^2 b}{q r (-2 a b + b^2 + a^2)}, -\frac{1}{2} \frac{-2 p s + 4 q r + s^2 + p^2}{q r (-2 a b + b^2 + a^2)}, \right. \\ & \left. \frac{1}{2} \frac{-p + s}{(-a + b) q r} \right], \\ & \left[ -\frac{1}{2} \frac{-p b + a s}{(-a + b) q r}, \frac{1}{2} \frac{-p + s}{(-a + b) q r}, -\frac{1}{2 q r} \right] \Big] \\ & 2 q r (-a + b)^2 \end{aligned} \quad (5)$$

```
> AM := simplify(Adjoint(A))
AM := [ [2 a s p b - 4 a b q r - a^2 s^2 - p^2 b^2, -b p s + 2 b q r - a p s + 2 a q r + a s^2 + p^2 b,
-b a s + p b^2 + a^2 s - a p b],
[ -b p s + 2 b q r - a p s + 2 a q r + a s^2 + p^2 b, 2 p s - 4 q r - s^2 - p^2, -a s - p b + s b
+ p a],
[ -b a s + p b^2 + a^2 s - a p b, -a s - p b + s b + p a, 2 a b - b^2 - a^2]]
```

```
>
>
```

Here A is the matrix of the linearized operator (bivector=metric with upper indices),  
AA - the inverse (metric, which we remember is defined only up to conformal rescaling)  
and AJ=AM=AdA the adjoint matrix (which we use as a representative for the conformal class)

```
>
```

```
> aA := [TotalDiff(A[1, 1], 1) + TotalDiff(A[1, 2], 2) + TotalDiff(A[1, 3], 3), TotalDiff(A[2,
1], 1) + TotalDiff(A[2, 2], 2) + TotalDiff(A[2, 3], 3), TotalDiff(A[3, 1], 1)
+ TotalDiff(A[3, 2], 2) + TotalDiff(A[3, 3], 3)]:
```

```
> ω := 2·[AA[1, 1]·aA[1] + AA[1, 2]·aA[2] + AA[1, 3]·aA[3], AA[2, 1]·aA[1] + AA[2, 2]
·aA[2] + AA[2, 3]·aA[3], AA[3, 1]·aA[1] + AA[3, 2]·aA[2] + AA[3, 3]·aA[3]]:
```

```
>
```

```
> DepVars := [u(t, x, y), v(t, x, y)]: AJ := simplify(FromJet(AM, DepVars)):
```

```
>
```

```
> DGsetup([t, x, y], M):
```

```
> g := evalDG(AJ[1, 1]·dt &t dt + AJ[1, 2]·dt &t dx + AJ[1, 3]·dt &t dy + AJ[2, 1]·dx &t dt
+ AJ[2, 2]·dx &t dx + AJ[2, 3]·dx &t dy + AJ[3, 1]·dy &t dt + AJ[3, 2]·dy &t dx
+ AJ[3, 3]·dy &t dy):
```

```
>
```

```
> C := Connection(a000*dt &t D_t &t dt + a111*dx &t D_x &t dx + a222*dy &t D_y &t dy
+ a001*(dt &t D_t &t dx + dx &t D_t &t dt) + a002*(dt &t D_t &t dy + dy &t D_t
&t dt) + a102*(dx &t D_t &t dy + dy &t D_t &t dx) + a011*(dt &t D_x &t dx + dx
&t D_x &t dt) + a012*(dt &t D_x &t dy + dy &t D_x &t dt) + a112*(dx &t D_x &t dy
+ dy &t D_x &t dx) + a021*(dt &t D_y &t dx + dx &t D_y &t dt) + a022*(dt &t D_y
&t dy + dy &t D_y &t dt) + a122*(dx &t D_y &t dy + dy &t D_y &t dx) + a010*dt
&t D_x &t dt + a121*dx &t D_y &t dx + a202*dy &t D_t &t dy + a020*dt &t D_y &t dt
+ a101*dx &t D_t &t dx + a212*dy &t D_x &t dy):
```

```
> TorsionTensor(C);
```

$$0 \, dt \, D_t \, dt$$

(7)

```
> U1 := simplify(FromJet(omega[1], DepVars)) :
U2 := simplify(FromJet(omega[2], DepVars)) :
U3 := simplify(FromJet(omega[3], DepVars)) :
```

Here we determine the connection C and define the covector U=omega.

That this choice of omega is the only natural is indicated by the absence of the terms of the 2nd order in u(t,x,y) in the expression Ric=V\*g (with V removed)

```
> Et := evalDG(DirectionalCovariantDerivative(D_t, g, C) - U1.g) :
Ex := evalDG(DirectionalCovariantDerivative(D_x, g, C) - U2.g) :
Ey := evalDG(DirectionalCovariantDerivative(D_y, g, C) - U3.g) :
```

```
> Eq000 := TensorInnerProduct(g, Et, dt &t dt) :
Eq001 := TensorInnerProduct(g, Et, dt &t dx) :
Eq002 := TensorInnerProduct(g, Et, dt &t dy) :
Eq011 := TensorInnerProduct(g, Et, dx &t dx) :
Eq012 := TensorInnerProduct(g, Et, dx &t dy) :
Eq022 := TensorInnerProduct(g, Et, dy &t dy) :
Eq100 := TensorInnerProduct(g, Ex, dt &t dt) :
Eq101 := TensorInnerProduct(g, Ex, dt &t dx) :
Eq102 := TensorInnerProduct(g, Ex, dt &t dy) :
Eq111 := TensorInnerProduct(g, Ex, dx &t dx) :
Eq112 := TensorInnerProduct(g, Ex, dx &t dy) :
Eq122 := TensorInnerProduct(g, Ex, dy &t dy) :
Eq200 := TensorInnerProduct(g, Ey, dt &t dt) :
Eq201 := TensorInnerProduct(g, Ey, dt &t dx) :
Eq202 := TensorInnerProduct(g, Ey, dt &t dy) :
Eq211 := TensorInnerProduct(g, Ey, dx &t dx) :
Eq212 := TensorInnerProduct(g, Ey, dx &t dy) :
Eq222 := TensorInnerProduct(g, Ey, dy &t dy) :
```

```
> sA := solve({Eq000=0, Eq001=0, Eq002=0, Eq011=0, Eq012=0, Eq022=0, Eq100=0,
Eq101=0, Eq102=0, Eq111=0, Eq112=0, Eq122=0, Eq200=0, Eq201=0, Eq202=0,
Eq211=0, Eq212=0, Eq222=0}, [a000, a001, a002, a010, a011, a012, a020, a021, a022,
a101, a102, a111, a112, a121, a122, a202, a212, a222]) :
```

```
> C1 := evalDG(subs({op(op(sA))}, C)) :
```

```
> evalDG(CovariantDerivative(g, C1) - g &t (U1.dt + U2.dx + U3.dy)) ;
```

$$0 \, dt \, dt \, dt$$

(8)

```
> R1 := CurvatureTensor(C1) : Ric1 := RicciTensor(R1) : T1 := SymmetrizeIndices(Ric1, [1, 2],
"Symmetric") : Res := evalDG(T1 - V.g) :
```

```
> NEQtt := ContractIndices(Res, D_t &t D_t, [[1, 1], [2, 2]]) : NEQtx := ContractIndices(Res,
D_t &t D_x, [[1, 1], [2, 2]]) :
NEQty := ContractIndices(Res, D_t &t D_y, [[1, 1], [2, 2]]) : NEQxx := ContractIndices(Res,
D_x &t D_x, [[1, 1], [2, 2]]) :
NEQxy := ContractIndices(Res, D_x &t D_y, [[1, 1], [2, 2]]) : NEQyy := ContractIndices(Res,
D_y &t D_y, [[1, 1], [2, 2]]) :
```

```
>
```

```
> DGsetup([t, x, y], [u, v], J2, 4) :
```

```
> de := DifferentialEquationData([F, G], [u1, v1])
```

$$de := [\{u_1, v_1\}, [u_1 + a u_2 + p u_3 + q v_3, v_1 + b v_2 + r u_3 + s v_3]]$$

(9)

```

>
> de2 := Prolong(de, 2) : deTRA := Transformation(de2) :
>
> Eq0 := Pullback(deTRA, ToJet(NEQtt, DepVars, notation = jetnumbers)) :
> VS := solve(Eq0, V) :
> factor(denom(simplify(VS)))

```

$$8 q^2 r^2 (a - b)^4 (-2 a s p b + 4 a b q r + a^2 s^2 + p^2 b^2) \quad (10)$$

Let us investigate when VS=0

```

> DepV := [a(u, v), b(u, v), p(u, v), q(u, v), r(u, v), s(u, v)] :
>
> simplify(ToJet(subs([u[] = u, v[] = v], diff(VS, u2, 2)), DepV, notation = jetnumbers))

```

$$-\frac{a_1}{q_{[]} r_{[]} (a_{[]} - b_{[]})} \quad (11)$$

```

> simplify(ToJet(subs([u[] = u, v[] = v], diff(VS, v2, 2)), DepV, notation = jetnumbers))

```

$$\frac{b_2}{r_{[]} q_{[]} (a_{[]} - b_{[]})} \quad (12)$$

```

> simplify(subs([a1=0, b2=0, a1,1=0], ToJet(subs([u[] = u, v[] = v], diff(VS, u2, u2)), DepV,
notation = jetnumbers)))

```

$$\frac{1}{4} \frac{p_1^2}{q_{[]}^2 r_{[]}^2} \quad (13)$$

```

> simplify(subs([a1=0, b2=0, a1,1=0, b2,2=0], ToJet(subs([u[] = u, v[] = v], diff(VS, v2,
v2)), DepV, notation = jetnumbers)))

```

$$\frac{1}{4} \frac{s_2^2}{q_{[]}^2 r_{[]}^2} \quad (14)$$

```

>
> simplify(subs([a1=0, b2=0, p1=0], ToJet(subs([u[] = u, v[] = v], diff(VS, u2, 3)), DepV,
notation = jetnumbers)))

```

$$-\frac{a_2}{q_{[]} (a_{[]}^2 - 2 b_{[]} a_{[]} + b_{[]}^2)} \quad (15)$$

```

> simplify(subs([a1=0, b2=0, s2=0], ToJet(subs([u[] = u, v[] = v], diff(VS, v2, 3)), DepV,
notation = jetnumbers)))

```

$$-\frac{b_1}{r_{[]} (a_{[]}^2 - 2 b_{[]} a_{[]} + b_{[]}^2)} \quad (16)$$

```

> simplify(subs([a1=0, b2=0, p1=0, s2=0], ToJet(subs([u[] = u, v[] = v], diff(VS, u3, 3)),
DepV, notation = jetnumbers)))

```

$$-\frac{q_{[]} r_1 + r_{[]} p_2 + r_{[]} q_1}{r_{[]} q_{[]} (a_{[]}^2 - 2 b_{[]} a_{[]} + b_{[]}^2)} \quad (17)$$

$$\begin{aligned}
& \text{> simplify}\left(\text{subs}\left(\left[a_1=0, b_2=0, p_1=0, s_2=0\right], \text{ToJet}\left(\text{subs}\left(\left[u_{[]} = u, v_{[]} = v\right], \text{diff}\left(VS, v_{3,3}\right)\right), \right.\right. \\
& \quad \left.\left.\text{DepV, notation=jetnumbers}\right)\right) \\
& \quad - \frac{q_{[]} s_1 + q_{[]} r_2 + r_{[]} q_2}{r_{[]} q_{[]} \left(a_{[]}^2 - 2 b_{[]} a_{[]} + b_{[]}^2\right)}
\end{aligned} \tag{18}$$

$$\begin{aligned}
& \text{> expand}\left(\text{solve}\left(r_{[]} p_2 + q_{[]} r_1 + r_{[]} q_1, p_2\right)\right) \\
& \quad - \frac{q_{[]} r_1}{r_{[]} } - q_1
\end{aligned} \tag{19}$$

$$\begin{aligned}
& \text{> expand}\left(\text{solve}\left(r_{[]} q_2 + q_{[]} r_2 + q_{[]} s_1, s_1\right)\right) \\
& \quad - \frac{r_{[]} q_2}{q_{[]} } - r_2
\end{aligned} \tag{20}$$

we see that several coefficients are constant, but we have to move forward

$$\begin{aligned}
& \text{> simplify}\left(\text{subs}\left(\left[a_1=0, a_2=0, b_1=0, b_2=0, p_1=0, s_2=0, a_{1,1}=0, a_{1,2}=0, a_{2,2}=0, b_{1,1}=0, b_{1,2}\right.\right.\right. \\
& \quad \left.\left.=0, b_{2,2}=0, p_{1,1}=0, p_{1,2}=0, s_{1,2}=0, s_{2,2}=0\right], \text{ToJet}\left(\text{subs}\left(\left[u_{[]} = u, v_{[]} = v\right], \text{diff}\left(VS, u_2,\right.\right.\right. \\
& \quad \left.\left.\left.u_3\right)\right), \text{DepV, notation=jetnumbers}\right)\right) \\
& \quad - \left(2 \left(-r_{[]}^2 q_1 q_2 + q_{[]} r_{[]}^2 q_{1,2} + r_{[]} r_{1,2} q_{[]}^2 - r_2 r_1 q_{[]}^2\right) a_{[]} b_{[]} \right) / \left(r_{[]} \left(a_{[]}^3 s_{[]}^2 - 2 a_{[]}^2 s_{[]} p_{[]} b_{[]} \right.\right. \\
& \quad \left.\left.+ 4 a_{[]}^2 r_{[]} q_{[]} b_{[]} - a_{[]}^2 s_{[]}^2 b_{[]} + 2 a_{[]} s_{[]} p_{[]} b_{[]}^2 - 4 a_{[]} r_{[]} q_{[]} b_{[]}^2 + a_{[]} p_{[]}^2 b_{[]}^2 - p_{[]}^2 b_{[]}^3\right) \right. \\
& \quad \left. q_{[]}^2\right)
\end{aligned} \tag{21}$$

$$\begin{aligned}
& \text{> simplify}\left(\text{subs}\left(\left[a_1=0, a_2=0, b_1=0, b_2=0, p_1=0, s_2=0, a_{1,1}=0, a_{1,2}=0, a_{2,2}=0, b_{1,1}=0, b_{1,2}\right.\right.\right. \\
& \quad \left.\left.=0, b_{2,2}=0, p_{1,1}=0, p_{1,2}=0, s_{1,2}=0, s_{2,2}=0\right], \text{ToJet}\left(\text{subs}\left(\left[u_{[]} = u, v_{[]} = v\right], \text{diff}\left(VS, v_2,\right.\right.\right. \\
& \quad \left.\left.\left.v_3\right)\right), \text{DepV, notation=jetnumbers}\right)\right) \\
& \quad \left(2 \left(-r_{[]}^2 q_1 q_2 + q_{[]} r_{[]}^2 q_{1,2} + r_{[]} r_{1,2} q_{[]}^2 - r_2 r_1 q_{[]}^2\right) a_{[]} b_{[]} \right) / \left(q_{[]} \left(a_{[]}^3 s_{[]}^2 - 2 a_{[]}^2 s_{[]} p_{[]} b_{[]} \right.\right. \\
& \quad \left.\left.+ 4 a_{[]}^2 r_{[]} q_{[]} b_{[]} - a_{[]}^2 s_{[]}^2 b_{[]} + 2 a_{[]} s_{[]} p_{[]} b_{[]}^2 - 4 a_{[]} r_{[]} q_{[]} b_{[]}^2 + a_{[]} p_{[]}^2 b_{[]}^2 - p_{[]}^2 b_{[]}^3\right) \right. \\
& \quad \left. r_{[]}^2\right)
\end{aligned} \tag{22}$$

$$\begin{aligned}
& \text{> solve}\left(r_{[]}^2 q_{[]} q_{1,2} - q_{[]}^2 r_2 r_1 + r_{[]} q_{[]}^2 r_{1,2} - r_{[]}^2 q_2 q_1, r_{1,2}\right) \\
& \quad \frac{r_{[]}^2 q_1 q_2 - q_{[]} r_{[]}^2 q_{1,2} + r_2 r_1 q_{[]}^2}{r_{[]} q_{[]}^2}
\end{aligned} \tag{23}$$

... and unite all we got so far ...

$$\begin{aligned}
& \text{> factor}\left(\text{subs}\left(\left[\left[q_{1,1} = -q_1 \frac{r_1}{r_{[]} } - q_{[]} \cdot \frac{r_{1,1} r_{[]} - r_1^2}{r_{[]}^2}, r_{1,2} = \frac{-r_{[]}^2 q_{[]} q_{1,2} + q_{[]}^2 r_2 r_1 + r_{[]}^2 q_2 q_1}{r_{[]} q_{[]}^2}\right], \right.\right. \\
& \quad \text{subs}\left(\left[a_1=0, a_2=0, b_1=0, b_2=0, p_1=0, p_2 = -\frac{q_{[]} r_1}{r_{[]} } - q_1, s_1 = -\frac{r_{[]} q_2}{q_{[]} } - r_2, s_2=0, a_{1,1}\right.\right. \\
& \quad \left.\left.=0, a_{1,2}=0, a_{2,2}=0, b_{1,1}=0, b_{1,2}=0, b_{2,2}=0, p_{1,1}=0, p_{1,2}=0, p_{2,2} = -\left(q_{1,2} + \frac{q_2 \cdot r_1}{r_{[]} }\right)\right.\right.
\end{aligned}$$

$$\begin{aligned}
& + q_{[]} \frac{r_{1,2} r_{[]} - r_1 r_2}{r_{[]}^2} \Bigg), s_{1,1} = - \left( r_{1,2} + \frac{q_2 \cdot r_1}{q_{[]}} + r_{[]} \frac{q_{2,2} q_{[]} - q_1 q_2}{q_{[]}^2} \right), s_{1,2} = 0, s_{2,2} = 0 \Bigg] \\
& ToJet(subs([u_{[]} = u, v_{[]} = v], diff(VS, u_2, v_3)), DepV, notation = jetnumbers) \Bigg) \Bigg) \Bigg) \\
& - \frac{(q_{1,2} - q_{2,2}) (a_{[]} s_{[]} - p_{[]} b_{[]} ) a_{[]}}{q_{[]} (a_{[]} - b_{[]} ) (a_{[]}^2 s_{[]}^2 - 2 a_{[]} s_{[]} p_{[]} b_{[]} + 4 a_{[]} r_{[]} q_{[]} b_{[]} + p_{[]}^2 b_{[]}^2 )} \quad (24)
\end{aligned}$$

$$\begin{aligned}
> factor \Bigg( subs \Bigg( \Bigg[ q_{1,1} = -q_1 \frac{r_1}{r_{[]}} - q_{[]} \cdot \frac{r_{1,1} r_{[]} - r_1^2}{r_{[]}^2}, q_{1,2} = q_{2,2}, r_{2,2} = -r_2 \frac{q_2}{q_{[]}} \\
& - r_{[]} \frac{q_{2,2} q_{[]} - q_2^2}{q_{[]}^2}, r_{1,2} = \frac{-r_{[]}^2 q_{[]} q_{2,2} + q_{[]}^2 r_2 r_1 + r_{[]}^2 q_2 q_1}{r_{[]} q_{[]}^2} \Bigg], subs \Bigg( \Bigg[ a_1 = 0, a_2 = 0, b_1 \\
& = 0, b_2 = 0, p_1 = 0, p_2 = -\frac{q_{[]} r_1}{r_{[]}} - q_1, s_1 = -\frac{r_{[]} q_2}{q_{[]}} - r_2, s_2 = 0, a_{1,1} = 0, a_{1,2} = 0, a_{2,2} = 0, \\
& b_{1,1} = 0, b_{1,2} = 0, b_{2,2} = 0, p_{1,1} = 0, p_{1,2} = 0, p_{2,2} = - \left( q_{1,2} + \frac{q_2 \cdot r_1}{r_{[]}} + q_{[]} \frac{r_{1,2} r_{[]} - r_1 r_2}{r_{[]}^2} \right), \\
& s_{1,1} = - \left( r_{1,2} + \frac{q_2 \cdot r_1}{q_{[]}} + r_{[]} \frac{q_{2,2} q_{[]} - q_1 q_2}{q_{[]}^2} \right), s_{1,2} = 0, s_{2,2} = 0 \Bigg], ToJet(subs([u_{[]} = u, v_{[]} \\
& = v], diff(VS, u_3, u_3)), DepV, notation = jetnumbers) \Bigg) \Bigg) \Bigg)
\end{aligned}$$

$$\frac{1}{4} \frac{(q_{[]} r_1 + r_{[]} q_1)^2}{(a_{[]} - b_{[]} )^2 q_{[]}^2 r_{[]}^2} \quad (25)$$

$$\begin{aligned}
> factor \Bigg( subs \Bigg( \Bigg[ q_{1,1} = -q_1 \frac{r_1}{r_{[]}} - q_{[]} \cdot \frac{r_{1,1} r_{[]} - r_1^2}{r_{[]}^2}, q_{1,2} = q_{2,2}, r_{2,2} = -r_2 \frac{q_2}{q_{[]}} \\
& - r_{[]} \frac{q_{2,2} q_{[]} - q_2^2}{q_{[]}^2}, r_{1,2} = \frac{-r_{[]}^2 q_{[]} q_{2,2} + q_{[]}^2 r_2 r_1 + r_{[]}^2 q_2 q_1}{r_{[]} q_{[]}^2} \Bigg], subs \Bigg( \Bigg[ a_1 = 0, a_2 = 0, b_1 \\
& = 0, b_2 = 0, p_1 = 0, p_2 = -\frac{q_{[]} r_1}{r_{[]}} - q_1, s_1 = -\frac{r_{[]} q_2}{q_{[]}} - r_2, s_2 = 0, a_{1,1} = 0, a_{1,2} = 0, a_{2,2} = 0, \\
& b_{1,1} = 0, b_{1,2} = 0, b_{2,2} = 0, p_{1,1} = 0, p_{1,2} = 0, p_{2,2} = - \left( q_{1,2} + \frac{q_2 \cdot r_1}{r_{[]}} + q_{[]} \frac{r_{1,2} r_{[]} - r_1 r_2}{r_{[]}^2} \right), \\
& s_{1,1} = - \left( r_{1,2} + \frac{q_2 \cdot r_1}{q_{[]}} + r_{[]} \frac{q_{2,2} q_{[]} - q_1 q_2}{q_{[]}^2} \right), s_{1,2} = 0, s_{2,2} = 0 \Bigg], ToJet(subs([u_{[]} = u, v_{[]} \\
& = v], diff(VS, v_3, v_3)), DepV, notation = jetnumbers) \Bigg) \Bigg) \Bigg)
\end{aligned}$$

$$(26)$$

$$\frac{1}{4} \frac{(r_{[]} q_2 + q_{[]} r_2)^2}{(a_{[]} - b_{[]} )^2 q_{[]}^2 r_{[]}^2} \quad (26)$$

connection great so  $q*r$  is constant, using which we get that also  $p$  and  $s$  are constants, and there is nothing more:

$$\begin{aligned} & \text{factor} \left( \text{subs} \left( \left[ q_{1,1} = -q_1 \frac{r_1}{r_{[]} } - q_{[]} \cdot \frac{r_{1,1} r_{[]} - r_1^2}{r_{[]}^2}, q_{1,2} = q_{2,2}, r_{2,2} = -r_2 \frac{q_2}{q_{[]} } \right. \right. \\ & \quad \left. \left. - r_{[]} \frac{q_{2,2} q_{[]} - q_2^2}{q_{[]}^2}, r_{1,2} = \frac{-r_{[]}^2 q_{[]} q_{2,2} + q_{[]}^2 r_2 r_1 + r_{[]}^2 q_2 q_1}{r_{[]} q_{[]}^2} \right], \text{subs} \left( \left[ a_1 = 0, a_2 = 0, b_1 \right. \right. \right. \\ & \quad = 0, b_2 = 0, p_1 = 0, p_2 = 0, s_1 = 0, s_2 = 0, r_1 = -r_{[]} \frac{q_1}{q_{[]} }, r_2 = -r_{[]} \frac{q_2}{q_{[]} }, a_{1,1} = 0, a_{1,2} = 0, a_{2,2} \\ & \quad = 0, b_{1,1} = 0, b_{1,2} = 0, b_{2,2} = 0, p_{1,1} = 0, p_{1,2} = 0, p_{2,2} = 0, s_{1,1} = 0, s_{1,2} = 0, s_{2,2} = 0, r_{1,1} = \\ & \quad \left. \left. - r_{[]} \frac{q_{1,1}}{q_{[]} } + 2 r_{[]} \frac{q_1^2}{q_{[]}^2}, r_{1,2} = -r_{[]} \frac{q_{1,2}}{q_{[]} } + 2 r_{[]} \frac{q_1 q_2}{q_{[]}^2}, r_{2,2} = -r_{[]} \frac{q_{2,2}}{q_{[]} } + 2 r_{[]} \frac{q_2^2}{q_{[]}^2} \right] \right. \\ & \quad \left. \left. \text{ToJet} \left( \text{subs} \left( [u_{[]} = u, v_{[]} = v], \text{VS} \right), \text{DepV}, \text{notation} = \text{jetnumbers} \right) \right) \right) \right) \right) \\ & \quad 0 \end{aligned} \quad (27)$$

In other words,  $\text{VS}=0$  iff the coefficients of the symbol matrix (or dispersion relation) are constants. This case being excluded, we continue to investigate integrability

```
>
>
> Eq1 := numer(subs(V=VS, Pullback(deTRA, ToJet(NEQtx, DepVars, notation
=jetnumbers)))) :
Eq2 := numer(subs(V=VS, Pullback(deTRA, ToJet(NEQty, DepVars, notation
=jetnumbers)))) :
Eq3 := numer(subs(V=VS, Pullback(deTRA, ToJet(NEQxx, DepVars, notation
=jetnumbers)))) :
Eq4 := numer(subs(V=VS, Pullback(deTRA, ToJet(NEQxy, DepVars, notation
=jetnumbers)))) :
Eq5 := numer(subs(V=VS, Pullback(deTRA, ToJet(NEQyy, DepVars, notation
=jetnumbers)))) :
```

These equations are expected a unique solution for the 16 of the 3rd derivatives of  $(a,b,p,q,r)$ , the same as in the integrability conditions, in this case it would be the same to find the solution or to check if the given set is a solution. We will address this issue rigorously later, and for now we write the integrability conditions and substitute them into the obtained eqns.

**J2 >**

```
J2 > IC := {D[1,1](a)(u,v) =
(r(u,v) * (- (r(u,v) * D[2](a)(u,v)^2) + D[1](a)(u,v) * ((-p(u,v) + s(u,v))
* D[2](a)(u,v) + 2 * (a(u,v)
- b(u,v)) * D[2](p)(u,v) + q(u,v) * (2 * D[1](a)(u,v) + D[1](b)(u,v))) + (
```

$$\begin{aligned}
& -a(u, v) + b(u, v)) * D[2](a)(u, v) * D[1](p)(u, v) \\
& + (a(u, v) - b(u, v)) * q(u, v) * D[1](a)(u, v) * D[1](r)(u, v) / ((a(u, v) - b(u, v)) * q(u, v) * r(u, v)), \\
D[1, 2](a)(u, v) = & ((a(u, v) - b(u, v)) * r(u, v) * D[2](q)(u, v) + q(u, v) * (r(u, v) * (D[2](a)(u, v) + D[2](b)(u, v)) + (a(u, v) - b(u, v)) * D[2](r)(u, v))) * D[1](a)(u, v) / ((a(u, v) - b(u, v)) * q(u, v) * r(u, v)), \\
D[2, 2](a)(u, v) = & ((a(u, v) - b(u, v)) * r(u, v) * D[2](a)(u, v) * D[2](q)(u, v) + q(u, v) * (r(u, v) * D[2](a)(u, v)^2 + ((-p(u, v) + s(u, v)) * D[2](b)(u, v) + (a(u, v) - b(u, v)) * D[2](s)(u, v)) * D[1](a)(u, v)) + q(u, v)^2 * D[1](a)(u, v) * D[1](b)(u, v)) / ((a(u, v) - b(u, v)) * q(u, v) * r(u, v)), \\
D[1, 1](b)(u, v) = & (r(u, v) * (- (q(u, v) * D[1](b)(u, v)^2 - D[2](b)(u, v) * (r(u, v) * D[2](a)(u, v) + (p(u, v) - s(u, v)) * D[1](a)(u, v) + (-a(u, v) + b(u, v)) * D[1](p)(u, v))) + (a(u, v) - b(u, v)) * q(u, v) * D[1](b)(u, v) * D[1](r)(u, v)) / ((a(u, v) - b(u, v)) * q(u, v) * r(u, v)), \\
D[1, 2](b)(u, v) = & D[2](b)(u, v) * (- ((D[1](a)(u, v) + D[1](b)(u, v)) / (a(u, v) - b(u, v))) + D[1](q)(u, v) / q(u, v) + D[1](r)(u, v) / r(u, v)), \\
D[2, 2](b)(u, v) = & ((a(u, v) - b(u, v)) * r(u, v) * D[2](b)(u, v) * D[2](q)(u, v) + q(u, v)^2 * D[1](b)(u, v)^2 + q(u, v) * (- (r(u, v) * D[2](b)(u, v) * (D[2](a)(u, v) + 2 * D[2](b)(u, v))) + ((-p(u, v) + s(u, v)) * D[2](b)(u, v) + (-a(u, v) + b(u, v)) * D[2](s)(u, v)) * D[1](b)(u, v) + 2 * (a(u, v) - b(u, v)) * D[2](b)(u, v) * D[1](s)(u, v))) / ((a(u, v) - b(u, v)) * q(u, v) * r(u, v)), \\
D[1, 1](p)(u, v) = & (2 * q(u, v) * r(u, v) * (r(u, v) * D[2](b)(u, v) * D[1](a)(u, v) - (r(u, v) * D[2](a)(u, v) + (p(u, v) - s(u, v)) * D[1](a)(u, v)) * D[1](b)(u, v)) + a(u, v)^2 * D[1](p)(u, v) * (r(u, v) * D[2](p)(u, v) + q(u, v) * D[1](r)(u, v)) + b(u, v)^2 * D[1](p)(u, v) * (r(u, v) * D[2](p)(u, v) + q(u, v) * D[1](r)(u, v)) + b(u, v) * r(u, v) * (s(u, v) * D[2](p)(u, v) * D[1](a)(u, v) - 2 * q(u, v) * D[2](r)(u, v) * D[1](a)(u, v) - 2 * s(u, v) * D[2](a)(u, v) * D[1](p)(u, v) - 2 * q(u, v) * D[1](a)(u, v) * D[1](p)(u, v) - q(u, v) * D[1](b)(u, v) * D[1](p)(u, v) + p(u, v) * (- (D[2](p)(u, v) * D[1](a)(u, v)) + 2 * D[2](a)(u, v) * D[1](p)(u, v)) + r(u, v) * (- 2 * D[2](q)(u, v) * D[1](a)(u, v) + D[2](a)(u, v) * (D[2](p)(u, v) + 2 * D[1](q)(u, v))) + 2 * q(u, v) * D[2](a)(u, v) * D[1](r)(u, v) - 2 * q(u, v) * D[1](a)(u, v) * D[1](s)(u, v)) + a(u, v) * (- (r(u, v)^2 * (- 2 * D[2](q)(u, v) * D[1](a)(u, v) + D[2](a)(u, v) * (D[2](p)(u, v) + 2 * D[1](q)(u, v))) - 2 * b(u, v) * q(u, v) *
\end{aligned}$$



$$\begin{aligned}
& D[1](p)(u, v) * D[1](r)(u, v) + r(u, v) * (-2 * b(u, v) * D[2](p)(u, v) \\
& \quad * D[1](p)(u, v) + p(u, v) * (D[2](p)(u, v) * D[1](a)(u, v) - \\
& \quad 2 * D[2](a)(u, v) * D[1](p)(u, v)) + s(u, v) * (- (D[2](p)(u, v) * D[1](a)(u, v)) \\
& \quad + 2 * D[2](a)(u, v) * D[1](p)(u, v)) + \\
& \quad q(u, v) * (2 * D[2](r)(u, v) * D[1](a)(u, v) + D[1](b)(u, v) * D[1](p)(u, v) - 2 \\
& \quad * D[2](a)(u, v) * D[1](r)(u, v) + \\
& \quad 2 * D[1](a)(u, v) * (D[1](p)(u, v) + D[1](s)(u, v))) / ((a(u, v) - b(u, v))^2 \\
& \quad * q(u, v) * r(u, v)),
\end{aligned}$$

$$\begin{aligned}
D[1, 2](p)(u, v) = & \\
& (q(u, v) * r(u, v) * (2 * (-p(u, v) + s(u, v)) * D[2](b)(u, v) + (a(u, v) - b(u, v)) \\
& \quad * (D[2](p)(u, v) + 2 * D[2](s)(u, v))) * D[1](a)(u, v) + \\
& \quad (a(u, v) - b(u, v)) * ((a(u, v) - b(u, v)) * r(u, v) * D[2](q)(u, v) + q(u, v) \\
& \quad * (r(u, v) * D[2](b)(u, v) + (a(u, v) \\
& \quad - b(u, v)) * D[2](r)(u, v))) * D[1](p)(u, v)) / ((a(u, v) - b(u, v))^2 * q(u, v) \\
& \quad * r(u, v)),
\end{aligned}$$

$$\begin{aligned}
D[2, 2](p)(u, v) = & \\
& (r(u, v) * (-2 * p(u, v) * q(u, v) * D[2](a)(u, v) * D[2](b)(u, v) + (a(u, v) - b(u, v) \\
& \quad v))^2 * D[2](p)(u, v) * D[2](q)(u, v) + \\
& \quad q(u, v) * D[2](a)(u, v) * (2 * s(u, v) * D[2](b)(u, v) + (a(u, v) - b(u, v)) \\
& \quad * (D[2](p)(u, v) + 2 * D[2](s)(u, v))) + \\
& \quad q(u, v)^2 * (-2 * D[2](b)(u, v) * D[1](a)(u, v) + 2 * D[2](a)(u, v) * D[1](b)(u, v) \\
& \quad v)) + (a(u, v) - b(u, v)) * q(u, v) * ((-p(u, v) + \\
& \quad s(u, v)) * D[2](b)(u, v) + (a(u, v) - b(u, v)) * D[2](s)(u, v) + q(u, v) \\
& \quad * D[1](b)(u, v)) * D[1](p)(u, v)) / ((a(u, v) - b(u, v))^2 * q(u, v) * r(u, v)),
\end{aligned}$$

$$\begin{aligned}
D[1, 1](s)(u, v) = & \\
& (r(u, v) * (2 * q(u, v) * (- (r(u, v) * D[2](b)(u, v) * D[1](a)(u, v)) + (r(u, v) \\
& \quad * D[2](a)(u, v) + (p(u, v) - s(u, v)) * D[1](a)(u, v)) * \\
& \quad D[1](b)(u, v)) + a(u, v)^2 * D[2](s)(u, v) * D[1](p)(u, v) + b(u, v)^2 \\
& \quad * D[2](s)(u, v) * D[1](p)(u, v) + b(u, v) * (D[2](s)(u, v) * \\
& \quad (r(u, v) * D[2](a)(u, v) + (p(u, v) - s(u, v)) * D[1](a)(u, v)) + 2 * q(u, v) \\
& \quad * D[1](b)(u, v) * D[1](p)(u, v)) + \\
& \quad a(u, v) * (- (D[2](s)(u, v) * (r(u, v) * D[2](a)(u, v) + (p(u, v) - s(u, v)) \\
& \quad * D[1](a)(u, v))) - \\
& \quad 2 * (b(u, v) * D[2](s)(u, v) + q(u, v) * D[1](b)(u, v)) * D[1](p)(u, v)) + (a(u, v) \\
& \quad - b(u, v)) * q(u, v) * (- (r(u, v) * D[1](b)(u, v)) \\
& \quad + (a(u, v) - b(u, v)) * D[1](r)(u, v)) * D[1](s)(u, v)) / ((a(u, v) - b(u, v))^2 \\
& \quad * q(u, v) * r(u, v)),
\end{aligned}$$

$$\begin{aligned}
D[1, 2](s)(u, v) = & \\
& (2 * p(u, v) * q(u, v) * r(u, v) * D[2](b)(u, v) * D[1](a)(u, v) + (a(u, v) - b(u, v) \\
& \quad v))^2 * r(u, v) * D[2](s)(u, v) * D[1](q)(u, v) + \\
& \quad q(u, v) * ((a(u, v) - b(u, v))^2 * D[2](s)(u, v) * D[1](r)(u, v) + r(u, v) * (-2 \\
& \quad * s(u, v) * D[2](b)(u, v) * D[1](a)(u, v) - (a(u, v) - \\
& \quad b(u, v)) * (D[2](s)(u, v) * D[1](a)(u, v) + D[2](b)(u, v) * (2 * D[1](p)(u, v) \\
& \quad + D[1](s)(u, v)))))) / ((a(u, v) - b(u, v))^2 * q(u, v) * r(u, v)),
\end{aligned}$$

$$\begin{aligned}
D[2, 2](s)(u, v) = & \\
& ((a(u, v) - b(u, v))^2 * r(u, v) * D[2](q)(u, v) * D[2](s)(u, v) + p(u, v) * q(u, v) \\
& \quad * (2 * r(u, v) * D[2](a)(u, v) * D[2](b)(u, v) - \\
& \quad (a(u, v) - b(u, v)) * (2 * D[2](s)(u, v) * D[1](b)(u, v) - D[2](b)(u, v)
\end{aligned}$$

$$\begin{aligned}
& *D[1](s)(u, v)) + q(u, v) * (r(u, v) * (-2 * s(u, v) * D[2](a)(u, v) * \\
& D[2](b)(u, v) - (a(u, v) - b(u, v)) * (D[2](a)(u, v) * D[2](s)(u, v) - 2 \\
& * D[2](q)(u, v) * D[1](b)(u, v) + 2 * D[2](b)(u, v) * (D[2](p)(u, v) + \\
& D[2](s)(u, v) + D[1](q)(u, v))) + (a(u, v) - b(u, v)) * (2 * s(u, v) \\
& * D[2](s)(u, v) * D[1](b)(u, v) - (s(u, v) * D[2](b)(u, v) + \\
& (-a(u, v) + b(u, v)) * D[2](s)(u, v)) * D[1](s)(u, v)) + q(u, v)^2 * (2 * r(u, v) \\
& * (D[2](b)(u, v) * D[1](a)(u, v) - D[2](a)(u, v) * D[1](b)(u, v)) + \\
& (a(u, v) - b(u, v)) * (-2 * D[2](b)(u, v) * D[1](r)(u, v) + D[1](b)(u, v) * (2 \\
& * D[2](r)(u, v) \\
& + D[1](s)(u, v)))) / ((a(u, v) - b(u, v))^2 * q(u, v) * r(u, v)), \\
D[1, 2](q)(u, v) = & \\
& (p(u, v)^2 * q(u, v) * D[2](b)(u, v) * D[1](a)(u, v) + p(u, v) * q(u, v) * (-r(u, \\
& v) * D[2](a)(u, v) * D[2](b)(u, v)) - \\
& D[1](a)(u, v) * (2 * s(u, v) * D[2](b)(u, v) + (a(u, v) - b(u, v)) * D[2](s)(u, v) \\
& + q(u, v) * D[1](b)(u, v)) + (-a(u, v) + b(u, v)) * \\
& D[2](b)(u, v) * D[1](p)(u, v)) + q(u, v) * (r(u, v) * (s(u, v) * D[2](a)(u, v) \\
& * D[2](b)(u, v) + (a(u, v) - b(u, v)) * (D[2](a)(u, v) * \\
& D[2](s)(u, v) + D[2](q)(u, v) * D[1](a)(u, v))) + D[1](a)(u, v) * ((a(u, v) \\
& - b(u, v)) * q(u, v) * D[2](r)(u, v) + \\
& s(u, v) * (s(u, v) * D[2](b)(u, v) + (a(u, v) - b(u, v)) * D[2](s)(u, v) + q(u, v) \\
& * D[1](b)(u, v))) + (a(u, v) - b(u, v)) * (s(u, v) * D[2](b)(u, v) + \\
& (a(u, v) - b(u, v)) * D[2](s)(u, v) + q(u, v) * D[1](b)(u, v)) * D[1](p)(u, v)) \\
& + (a(u, v) - b(u, v))^2 * r(u, v) * D[2](q)(u, v) * \\
& D[1](q)(u, v)) / ((a(u, v) - b(u, v))^2 * q(u, v) * r(u, v)), \\
D[1, 1](r)(u, v) = & \\
& (2 * q(u, v) * r(u, v) * (p(u, v) - s(u, v)) * (-r(u, v) * D[2](b)(u, v) \\
& * D[1](a)(u, v)) + (r(u, v) * D[2](a)(u, v) + (p(u, v) - s(u, v)) * \\
& D[1](a)(u, v)) * D[1](b)(u, v) + b(u, v) * r(u, v) * (r(u, v)^2 * D[2](a)(u, v) \\
& * D[2](q)(u, v) + \\
& q(u, v) * (q(u, v) * (-2 * D[1](a)(u, v) + D[1](b)(u, v)) * D[1](r)(u, v) + p(u, \\
& v) * (2 * D[1](b)(u, v) * D[1](p)(u, v) + \\
& D[1](a)(u, v) * (D[2](r)(u, v) + 2 * D[1](s)(u, v))) - s(u, v) * (2 * D[1](b)(u, \\
& v) * D[1](p)(u, v) + D[1](a)(u, v) * (D[2](r)(u, v) + \\
& 2 * D[1](s)(u, v)))) + r(u, v) * ((p(u, v) - s(u, v)) * D[2](q)(u, v) * D[1](a)(u, \\
& v) + q(u, v) * (-2 * (D[2](p)(u, v) + D[2](s)(u, v)) * \\
& D[1](a)(u, v) + (-2 * D[1](a)(u, v) + D[1](b)(u, v)) * D[1](q)(u, v) \\
& + D[2](a)(u, v) * (D[2](r)(u, v) + 2 * (D[1](p)(u, v) + D[1](s)(u, v)))))) + \\
& + \\
& a(u, v)^2 * (q(u, v)^2 * D[1](r)(u, v)^2 + q(u, v) * r(u, v) * (-D[1](q)(u, v) \\
& * D[1](r)(u, v) + D[1](p)(u, v) * (D[2](r)(u, v) + \\
& 2 * D[1](s)(u, v))) + r(u, v)^2 * (D[2](q)(u, v) * D[1](p)(u, v) - q(u, v) * D[1, \\
& 1](q)(u, v))) + b(u, v)^2 * (q(u, v)^2 * D[1](r)(u, v)^2 + \\
& q(u, v) * r(u, v) * (-D[1](q)(u, v) * D[1](r)(u, v) + D[1](p)(u, v) \\
& * (D[2](r)(u, v) + 2 * D[1](s)(u, v))) + \\
& r(u, v)^2 * (D[2](q)(u, v) * D[1](p)(u, v) - q(u, v) * D[1, 1](q)(u, v)) - a(u, v) \\
& * (r(u, v)^3 * D[2](a)(u, v) * D[2](q)(u, v) + \\
& 2 * b(u, v) * q(u, v)^2 * D[1](r)(u, v)^2 + q(u, v) * r(u, v) * (q(u, v) * (-2 \\
& * D[1](a)(u, v) + D[1](b)(u, v)) * D[1](r)(u, v) +
\end{aligned}$$

$$\begin{aligned}
& p(u, v) * (2 * D[1](b)(u, v) * D[1](p)(u, v) + D[1](a)(u, v) * (D[2](r)(u, v) + 2 \\
& \quad * D[1](s)(u, v))) - s(u, v) * (2 * D[1](b)(u, v) * D[1](p)(u, v) + \\
& \quad D[1](a)(u, v) * (D[2](r)(u, v) + 2 * D[1](s)(u, v))) + 2 * b(u, v) * ( \\
& \quad - (D[1](q)(u, v) * D[1](r)(u, v)) + D[1](p)(u, v) * (D[2](r)(u, v) + \\
& \quad 2 * D[1](s)(u, v))) + r(u, v)^2 * (D[2](q)(u, v) * ((p(u, v) - s(u, v)) \\
& \quad * D[1](a)(u, v) + 2 * b(u, v) * D[1](p)(u, v)) + \\
& \quad q(u, v) * (-2 * (D[2](p)(u, v) + D[2](s)(u, v)) * D[1](a)(u, v) + (-2 \\
& \quad * D[1](a)(u, v) + D[1](b)(u, v)) * D[1](q)(u, v) + \\
& \quad D[2](a)(u, v) * (D[2](r)(u, v) + 2 * (D[1](p)(u, v) + D[1](s)(u, v))) - 2 \\
& \quad * b(u, v) * D[1, 1](q)(u, v))) / ((a(u, v) - b(u, v))^2 * q(u, v)^2 * r(u, v)), \\
& D[1, 2](r)(u, v) =
\end{aligned}$$

$$\begin{aligned}
& (p(u, v)^2 * r(u, v) * D[2](b)(u, v) * D[1](a)(u, v) + p(u, v) * r(u, v) * (r(u, v) \\
& \quad * D[2](a)(u, v) * D[2](b)(u, v) + \\
& \quad D[1](a)(u, v) * (-2 * s(u, v) * D[2](b)(u, v) + (-a(u, v) + b(u, v)) * D[2](s)(u, \\
& \quad v) + q(u, v) * D[1](b)(u, v)) + (-a(u, v) + b(u, v)) * \\
& \quad D[2](b)(u, v) * D[1](p)(u, v)) + r(u, v) * ((s(u, v) * D[2](b)(u, v) + (a(u, v) \\
& \quad - b(u, v)) * D[2](s)(u, v) - q(u, v) * D[1](b)(u, v)) * \\
& \quad (s(u, v) * D[1](a)(u, v) + (a(u, v) - b(u, v)) * D[1](p)(u, v)) + r(u, v) * ( \\
& \quad - (s(u, v) * D[2](a)(u, v) * D[2](b)(u, v)) - (a(u, v) \\
& \quad - b(u, v)) * (D[2](a)(u, v) * D[2](s)(u, v) + D[2](b)(u, v) * D[1](q)(u, v))) \\
& \quad + (a(u, v) - b(u, v)) * q(u, v) * (-r(u, v) * D[2](b)(u, v)) \\
& \quad + (a(u, v) - b(u, v)) * D[2](r)(u, v)) * D[1](r)(u, v)) / ((a(u, v) - b(u, v))^2 \\
& \quad * q(u, v) * r(u, v)), \\
& D[2, 2](r)(u, v) =
\end{aligned}$$

$$\begin{aligned}
& (2 * p(u, v)^2 * q(u, v) * r(u, v) * D[2](a)(u, v) * D[2](b)(u, v) + (a(u, v) - b(u, \\
& \quad v))^2 * r(u, v)^2 * D[2](q)(u, v)^2 + q(u, v) * r(u, v) * \\
& \quad (2 * s(u, v)^2 * D[2](a)(u, v) * D[2](b)(u, v) + (a(u, v) - b(u, v)) * s(u, v) * (2 \\
& \quad * D[2](a)(u, v) * D[2](s)(u, v) + D[2](b)(u, v) * \\
& \quad (2 * D[2](p)(u, v) + D[1](q)(u, v))) + (a(u, v) - b(u, v)) * (r(u, v) \\
& \quad * ((D[2](a)(u, v) - 2 * D[2](b)(u, v)) * D[2](q)(u, v) + \\
& \quad (-a(u, v) + b(u, v)) * D[2, 2](q)(u, v)) - (a(u, v) - b(u, v)) * (D[2](q)(u, v) \\
& \quad * D[2](r)(u, v) - D[2](s)(u, v) * (2 * D[2](p)(u, v) + \\
& \quad D[1](q)(u, v)))) + (a(u, v) - b(u, v)) * q(u, v)^3 * D[1](b)(u, v) * D[1](r)(u, \\
& \quad v) + p(u, v) * q(u, v) * (r(u, v) * (-4 * s(u, v) * D[2](a)(u, v) * \\
& \quad D[2](b)(u, v) + 2 * (-a(u, v) * (D[2](b)(u, v) * D[2](p)(u, v) + D[2](a)(u, v) \\
& \quad * D[2](s)(u, v))) + b(u, v) * (D[2](b)(u, v) * D[2](p)(u, v) + \\
& \quad D[2](a)(u, v) * D[2](s)(u, v)) + q(u, v) * (D[2](b)(u, v) * D[1](a)(u, v) \\
& \quad - D[2](a)(u, v) * D[1](b)(u, v))) + \\
& \quad (-a(u, v) + b(u, v)) * D[2](b)(u, v) * D[1](q)(u, v)) + (-a(u, v) + b(u, v)) \\
& \quad * q(u, v) * D[2](b)(u, v) * D[1](r)(u, v)) + \\
& \quad q(u, v)^2 * (2 * r(u, v) * s(u, v) * (-D[2](b)(u, v) * D[1](a)(u, v)) \\
& \quad + D[2](a)(u, v) * D[1](b)(u, v)) + a(u, v)^2 * D[2](s)(u, v) * \\
& \quad D[1](r)(u, v) + b(u, v)^2 * D[2](s)(u, v) * D[1](r)(u, v) - b(u, v) * (s(u, v) \\
& \quad * D[2](b)(u, v) * D[1](r)(u, v) + r(u, v) * (D[2](a)(u, v) * \\
& \quad D[2](r)(u, v) + D[1](b)(u, v) * (2 * (D[2](p)(u, v) + D[2](s)(u, v)) \\
& \quad + D[1](q)(u, v)) - 2 * D[2](b)(u, v) * (D[2](r)(u, v) + D[1](p)(u, v) + \\
& \quad D[1](s)(u, v)))) + a(u, v) * ((s(u, v) * D[2](b)(u, v) - 2 * b(u, v) * D[2](s)(u, \\
& \quad v)) * D[1](r)(u, v) + r(u, v) * (D[2](a)(u, v) * D[2](r)(u, v) +
\end{aligned}$$

$$\begin{aligned} & D[1](b)(u, v) * (2 * (D[2](p)(u, v) + D[2](s)(u, v)) + D[1](q)(u, v)) - 2 \\ & * D[2](b)(u, v) * (D[2](r)(u, v) + \\ & D[1](p)(u, v) + D[1](s)(u, v))) / ((a(u, v) - b(u, v))^2 * q(u, v)^2 * r(u, \\ & v)) \} : \end{aligned}$$

**J2 >**

**J2 >** *convert(IC[3], diff)*

$$\begin{aligned} p_{u,u} = & \frac{1}{(a(u, v) - b(u, v))^2 q(u, v) r(u, v)} \left( 2 q(u, v) r(u, v) (r(u, v) b_v a_u - (r(u, v) a_v \right. \\ & + (p(u, v) - s(u, v)) a_u) b_u) + a(u, v)^2 p_u (r(u, v) p_v + q(u, v) r_u) + b(u, v)^2 p_u (r(u, \\ & v) p_v + q(u, v) r_u) + b(u, v) r(u, v) (s(u, v) p_v a_u - 2 q(u, v) r_v a_u - 2 s(u, v) a_v p_u \\ & - 2 q(u, v) a_u p_u - q(u, v) b_u p_u + p(u, v) (-p_v a_u + 2 a_v p_u) + r(u, v) (-2 q_v a_u + a_v (p_v \\ & + 2 q_u)) + 2 q(u, v) a_v r_u - 2 q(u, v) a_u s_u) + a(u, v) (-r(u, v)^2 (-2 q_v a_u + a_v (p_v \\ & + 2 q_u)) - 2 b(u, v) q(u, v) p_u r_u + r(u, v) (-2 b(u, v) p_v p_u + p(u, v) (p_v a_u - 2 a_v p_u) \\ & + s(u, v) (-p_v a_u + 2 a_v p_u) + q(u, v) (2 r_v a_u + b_u p_u - 2 a_v r_u + 2 a_u (p_u + s_u))) \right) \end{aligned} \quad (28)$$

**J2 >** *DepV := [a(u, v), b(u, v), p(u, v), q(u, v), r(u, v), s(u, v)] :*

*JIC := simplify(ToJet(convert(IC, diff), DepV, notation = jetnumbers)) :*

**J2 >**

**J2 >** *simplify(subs(JIC, ToJet(p\_u, DepV, notation = jetnumbers)))*

$$\begin{aligned} & \frac{1}{(a_{[]} - b_{[]})^2 q_{[]} r_{[]}} \left( 2 a_{[]} r_{[]}^2 q_2 a_1 - a_{[]} r_{[]}^2 a_2 p_2 - 2 a_{[]} r_{[]}^2 a_2 q_1 + 2 q_{[]} r_{[]}^2 b_2 a_1 - 2 q_{[]} \right. \\ & r_{[]}^2 b_1 a_2 + a_{[]}^2 p_1 r_{[]} p_2 + a_{[]}^2 p_1 q_{[]} r_1 + b_{[]}^2 p_1 r_{[]} p_2 + b_{[]}^2 p_1 q_{[]} r_1 - 2 b_{[]} r_{[]}^2 q_2 a_1 + b_{[]} \\ & r_{[]}^2 a_2 p_2 + 2 b_{[]} r_{[]}^2 a_2 q_1 - 2 q_{[]} r_{[]} b_1 a_1 p_{[]} + 2 q_{[]} r_{[]} b_1 s_{[]} a_1 + b_{[]} r_{[]} s_{[]} p_2 a_1 \\ & - 2 b_{[]} r_{[]} q_{[]} r_2 a_1 - 2 b_{[]} r_{[]} s_{[]} a_2 p_1 - 2 b_{[]} r_{[]} q_{[]} a_1 p_1 - b_{[]} r_{[]} q_{[]} b_1 p_1 \\ & - b_{[]} r_{[]} p_{[]} p_2 a_1 + 2 b_{[]} r_{[]} p_{[]} a_2 p_1 + 2 b_{[]} r_{[]} q_{[]} a_2 r_1 - 2 b_{[]} r_{[]} q_{[]} a_1 s_1 \\ & - 2 a_{[]} b_{[]} q_{[]} p_1 r_1 - 2 a_{[]} r_{[]} b_{[]} p_2 p_1 + a_{[]} r_{[]} p_{[]} p_2 a_1 - 2 a_{[]} r_{[]} p_{[]} a_2 p_1 \\ & - a_{[]} r_{[]} s_{[]} p_2 a_1 + 2 a_{[]} r_{[]} s_{[]} a_2 p_1 + 2 a_{[]} r_{[]} q_{[]} r_2 a_1 + a_{[]} r_{[]} q_{[]} b_1 p_1 \\ & \left. - 2 a_{[]} r_{[]} q_{[]} a_2 r_1 + 2 a_{[]} r_{[]} q_{[]} a_1 p_1 + 2 a_{[]} r_{[]} q_{[]} a_1 s_1 \right) \end{aligned} \quad (29)$$

**J2 >**

**J2 >** *simplify(subs(JIC, ToJet(subs([u\_{[]} = u, v\_{[]} = v], simplify(diff(Eq1, u\_3, u\_3))), DepV, notation = jetnumbers)))*

0

(30)

**J2 >** *simplify(subs(JIC, ToJet(subs([u\_{[]} = u, v\_{[]} = v], simplify(diff(Eq1, u\_2, u\_3))), DepV, notation = jetnumbers)))*

0

(31)

**J2 >** *simplify(subs(JIC, ToJet(subs([u\_{[]} = u, v\_{[]} = v], simplify(Eq1))), DepV, notation*

$$= \text{jetnumbers})))$$

0

(32)

$$\text{J2} > \text{simplify}(\text{subs}(\text{JIC}, \text{ToJet}(\text{subs}([u_{[]} = u, v_{[]} = v], \text{simplify}(\text{Eq2})), \text{DepV}, \text{notation} = \text{jetnumbers})))$$

0

(33)

$$\text{J2} > \text{simplify}(\text{subs}(\text{JIC}, \text{ToJet}(\text{subs}([u_{[]} = u, v_{[]} = v], \text{simplify}(\text{Eq3})), \text{DepV}, \text{notation} = \text{jetnumbers})))$$

0

(34)

$$\text{J2} > \text{simplify}(\text{subs}(\text{JIC}, \text{ToJet}(\text{subs}([u_{[]} = u, v_{[]} = v], \text{simplify}(\text{Eq4})), \text{DepV}, \text{notation} = \text{jetnumbers})))$$

0

(35)

$$\text{J2} > \text{simplify}(\text{subs}(\text{JIC}, \text{ToJet}(\text{subs}([u_{[]} = u, v_{[]} = v], \text{simplify}(\text{Eq5})), \text{DepV}, \text{notation} = \text{jetnumbers})))$$

0

(36)

Perfect, this means that integrability implies EW property. To check into the other side let us determine the rank of the system by substituting "arbitrary" rational values of (a,b,p,q,r,s) - due to large equivalence group we are basically independent of the choice - in the coefficients of the equations in  $u_i * u_j$  (the eqns are quadratic in the 2-jet of u); these are the 2nd order differential polynomials in (a,b,p,q,r,s) with the 2nd derivatives entering linearly with the coefficients depending on the 0-jet only.

J2 >

$$\text{J2} > \text{EQU} := \text{expand}(\{ \text{diff}(\text{Eq1}, u_2, u_2), \text{diff}(\text{Eq1}, u_2, u_3), \text{diff}(\text{Eq1}, u_2, v_2), \text{diff}(\text{Eq1}, u_2, v_3), \text{diff}(\text{Eq1}, u_3, u_3), \text{diff}(\text{Eq1}, u_3, v_2), \text{diff}(\text{Eq1}, u_3, v_3), \text{diff}(\text{Eq1}, v_2, v_2), \text{diff}(\text{Eq1}, v_2, v_3), \text{diff}(\text{Eq1}, v_3, v_3), \text{diff}(\text{Eq2}, u_2, u_2), \text{diff}(\text{Eq2}, u_2, u_3), \text{diff}(\text{Eq2}, u_2, v_2), \text{diff}(\text{Eq2}, u_2, v_3), \text{diff}(\text{Eq2}, u_3, u_3), \text{diff}(\text{Eq2}, u_3, v_2), \text{diff}(\text{Eq2}, u_3, v_3), \text{diff}(\text{Eq2}, v_2, v_2), \text{diff}(\text{Eq2}, v_2, v_3), \text{diff}(\text{Eq2}, v_3, v_3), \text{diff}(\text{Eq3}, u_2, u_2), \text{diff}(\text{Eq3}, u_2, u_3), \text{diff}(\text{Eq3}, u_2, v_2), \text{diff}(\text{Eq3}, u_2, v_3), \text{diff}(\text{Eq3}, u_3, u_3), \text{diff}(\text{Eq3}, u_3, v_2), \text{diff}(\text{Eq3}, u_3, v_3), \text{diff}(\text{Eq3}, v_2, v_2), \text{diff}(\text{Eq3}, v_2, v_3), \text{diff}(\text{Eq3}, v_3, v_3), \text{diff}(\text{Eq4}, u_2, u_2), \text{diff}(\text{Eq4}, u_2, u_3), \text{diff}(\text{Eq4}, u_2, v_2), \text{diff}(\text{Eq4}, u_2, v_3), \text{diff}(\text{Eq4}, u_3, u_3), \text{diff}(\text{Eq4}, u_3, v_2), \text{diff}(\text{Eq4}, u_3, v_3), \text{diff}(\text{Eq4}, v_2, v_2), \text{diff}(\text{Eq4}, v_2, v_3), \text{diff}(\text{Eq4}, v_3, v_3), \text{diff}(\text{Eq5}, u_2, u_2), \text{diff}(\text{Eq5}, u_2, u_3), \text{diff}(\text{Eq5}, u_2, v_2), \text{diff}(\text{Eq5}, u_2, v_3), \text{diff}(\text{Eq5}, u_3, u_3), \text{diff}(\text{Eq5}, u_3, v_2), \text{diff}(\text{Eq5}, u_3, v_3), \text{diff}(\text{Eq5}, v_2, v_2), \text{diff}(\text{Eq5}, v_2, v_3), \text{diff}(\text{Eq5}, v_3, v_3) \}) :$$

J2 >

$$\text{J2} > \text{nops}(\text{EQU})$$

41

(37)

$$\text{J2} > \text{EQUa} := \text{ToJet}(\text{subs}([u_{[]} = u, v_{[]} = v], \text{EQU}), \text{DepV}, \text{notation} = \text{jetnumbers}) :$$

$$\text{J2} > \text{SBS} := \left\{ a_{[]} = 1, b_{[]} = -\frac{5}{4}, p_{[]} = 3, q_{[]} = 2, r_{[]} = -\frac{1}{5}, s_{[]} = 7 \right\} :$$

$$\text{J2} > \text{EQU} := \text{simplify}(\text{subs}(\text{SBS}, \text{EQUa})) :$$

**J2** > *nops*(*EQU*)  
41 (38)

**J2** > *COF* := {*a*<sub>1,1</sub>, *a*<sub>1,2</sub>, *a*<sub>2,2</sub>, *b*<sub>1,1</sub>, *b*<sub>1,2</sub>, *b*<sub>2,2</sub>, *p*<sub>1,1</sub>, *p*<sub>1,2</sub>, *p*<sub>2,2</sub>, *q*<sub>1,1</sub>, *q*<sub>1,2</sub>, *q*<sub>2,2</sub>, *r*<sub>1,1</sub>, *r*<sub>1,2</sub>, *r*<sub>2,2</sub>,  
*s*<sub>1,1</sub>, *s*<sub>1,2</sub>, *s*<sub>2,2</sub>} :

**J2** > *nops*(*COF*)  
18 (39)

**J2** > *COF* := {*a*<sub>1,1</sub>, *a*<sub>1,2</sub>, *a*<sub>2,2</sub>, *b*<sub>1,1</sub>, *b*<sub>1,2</sub>, *b*<sub>2,2</sub>, *p*<sub>1,1</sub>, *p*<sub>1,2</sub>, *p*<sub>2,2</sub>, *r*<sub>1,1</sub>, *r*<sub>1,2</sub>, *r*<sub>2,2</sub>, *s*<sub>1,1</sub>, *s*<sub>1,2</sub>, *s*<sub>2,2</sub>} :

**J2** > *nops*(*COF*)  
15 (40)

**J2** > *M* := (*i*, *j*) → *coeff*(*EQU*[*i*], *COF*[*j*]) :

**J2** > *M*(4, 15)  
0 (41)

**J2** > *MAT* := *Matrix*(*nops*(*EQU*), *nops*(*COF*), *M*) :

**J2** > *Rank*(*MAT*)  
15 (42)

**J2** >  
We obtained that the rank is 15 not 16 as one could expect!  
Let us identify the 15x15 minor with non-zero determinant and solve for possible 2nd order derivatives  
of (a,b,p,q,r,s).

**J2** >  
**J2** > *interface*(*rtables*size = 41)  
10 (43)

**J2** > *MATs* := *SubMatrix*(*MAT*, [2, 5, 8, 11, 14, 17 .. 26], 1 .. 15) :

**J2** > *Rank*(*MATs*)  
15 (44)

**J2** >  
**J2** > *EQU**Ts* := {*EQU**T*[2], *EQU**T*[5], *EQU**T*[8], *EQU**T*[11], *EQU**T*[14], *EQU**T*[17],  
*EQU**T*[18], *EQU**T*[19], *EQU**T*[20], *EQU**T*[21], *EQU**T*[22], *EQU**T*[23],  
*EQU**T*[24], *EQU**T*[25], *EQU**T*[26]} :

**J2** > *EQU**Ts* := {*EQU**T*[2], *EQU**T*[5], *EQU**T*[7], *EQU**T*[11], *EQU**T*[13], *EQU**T*[17],  
*EQU**T*[18], *EQU**T*[21], *EQU**T*[22], *EQU**T*[25], *EQU**T*[28], *EQU**T*[30],  
*EQU**T*[31], *EQU**T*[32], *EQU**T*[33]} :

**J2** > *EQU**sa* := *ToJet*(*subs*([*u*<sub>[]</sub> = *u*, *v*<sub>[]</sub> = *v*], *EQU**Ts*), *DepV*, *notation* = *jetnumbers*) :  
*EQU**Us* := *simplify*(*subs*(*SBS*, *EQU**sa*)) :  
*Ms* := (*i*, *j*) → *coeff*(*EQU**Us*[*i*], *COF*[*j*]) : *MATs* := *Matrix*(*nops*(*EQU**Us*), *nops*(*COF*),  
*Ms*) :  
*Rank*(*MATs*)

15 (45)

**J2** > *nops*(*EQU**Ts*)  
15 (46)

**J2** > *nops*(*COF*)  
15 (47)

**J2** > *SQE* := *simplify*(*solve*(*EQU**sa*, *COF*))  
(48)

$$\begin{aligned}
SQE := & \left\{ a_{1,1} = \frac{1}{(a_{[]} - b_{[]}) q_{[]} r_{[]}} \left( -r_{[]}^2 a_2^2 - r_{[]} a_1 a_2 p_{[]} + r_{[]} a_1 a_2 s_{[]} + 2 r_{[]} a_1 p_2 a_{[]} \right. \right. \\
& - 2 r_{[]} a_1 p_2 b_{[]} + 2 r_{[]} q_{[]} a_1^2 + r_{[]} a_1 q_{[]} b_1 - r_{[]} a_2 p_1 a_{[]} + r_{[]} a_2 p_1 b_{[]} + q_{[]} a_1 r_1 a_{[]} \\
& \left. \left. - q_{[]} a_1 r_1 b_{[]} \right), a_{1,2} \right. \\
& = \frac{(r_{[]} q_2 a_{[]} - r_{[]} q_2 b_{[]} + q_{[]} r_{[]} a_2 + q_{[]} r_{[]} b_2 + q_{[]} r_2 a_{[]} - q_{[]} r_2 b_{[]}) a_1}{(a_{[]} - b_{[]}) q_{[]} r_{[]}}, a_{2,2} \\
& = \frac{1}{(a_{[]} - b_{[]}) q_{[]} r_{[]}} \left( r_{[]} a_2 q_2 a_{[]} - r_{[]} a_2 q_2 b_{[]} + q_{[]} r_{[]} a_2^2 - q_{[]} a_1 b_2 p_{[]} + q_{[]} s_{[]} b_2 a_1 \right. \\
& + q_{[]} a_1 s_2 a_{[]} - q_{[]} a_1 b_{[]} s_2 + q_{[]}^2 a_1 b_1 \left. \right), b_{1,1} = \frac{1}{(a_{[]} - b_{[]}) q_{[]} r_{[]}} \left( -r_{[]} q_{[]} b_1^2 - \right. \\
& r_{[]}^2 a_2 b_2 - r_{[]} a_1 b_2 p_{[]} + r_{[]} s_{[]} b_2 a_1 + r_{[]} b_2 p_1 a_{[]} - r_{[]} b_2 b_{[]} p_1 + q_{[]} b_1 r_1 a_{[]} \\
& \left. - q_{[]} b_1 r_1 b_{[]} \right), b_{1,2} \\
& = \frac{b_2 \left( -r_{[]} a_1 q_{[]} - q_{[]} r_{[]} b_1 + r_{[]} q_1 a_{[]} - r_{[]} q_1 b_{[]} + q_{[]} r_1 a_{[]} - q_{[]} r_1 b_{[]} \right)}{(a_{[]} - b_{[]}) q_{[]} r_{[]}}, b_{2,2} = \\
& - \frac{1}{(a_{[]} - b_{[]}) q_{[]} r_{[]}} \left( -r_{[]} b_2 q_2 a_{[]} + r_{[]} b_2 q_2 b_{[]} - q_{[]}^2 b_1^2 + q_{[]} r_{[]} a_2 b_2 + 2 q_{[]} r_{[]} b_2^2 \right. \\
& + q_{[]} b_1 b_2 p_{[]} - q_{[]} b_1 s_{[]} b_2 + q_{[]} b_1 s_2 a_{[]} - q_{[]} b_1 b_{[]} s_2 - 2 q_{[]} b_2 s_1 a_{[]} \\
& \left. + 2 q_{[]} b_2 s_1 b_{[]} \right), p_{1,1} = \frac{1}{r_{[]} q_{[]} (b_{[]}^2 + a_{[]}^2 - 2 a_{[]} b_{[]})} \left( 2 a_{[]} r_{[]}^2 q_2 a_1 - a_{[]} r_{[]}^2 a_2 p_2 \right. \\
& - 2 a_{[]} r_{[]}^2 a_2 q_1 + 2 q_{[]} r_{[]}^2 b_2 a_1 - 2 q_{[]} r_{[]}^2 b_1 a_2 + a_{[]}^2 p_1 r_{[]} p_2 + a_{[]}^2 p_1 q_{[]} r_1 + \\
& b_{[]}^2 p_1 r_{[]} p_2 + b_{[]}^2 p_1 q_{[]} r_1 - 2 b_{[]} r_{[]}^2 q_2 a_1 + b_{[]} r_{[]}^2 a_2 p_2 + 2 b_{[]} r_{[]}^2 a_2 q_1 \\
& \left. - 2 q_{[]} r_{[]} b_1 a_1 p_{[]} + 2 q_{[]} r_{[]} b_1 s_{[]} a_1 + b_{[]} r_{[]} s_{[]} p_2 a_1 - 2 b_{[]} r_{[]} q_{[]} r_2 a_1 \right.
\end{aligned}
\tag{48}$$

$$\begin{aligned}
& -2b_{[]}r_{[]}s_{[]}a_2p_1 - 2b_{[]}r_{[]}q_{[]}a_1p_1 - b_{[]}r_{[]}q_{[]}b_1p_1 - b_{[]}r_{[]}p_{[]}p_2a_1 \\
& + 2b_{[]}r_{[]}p_{[]}a_2p_1 + 2b_{[]}r_{[]}q_{[]}a_2r_1 - 2b_{[]}r_{[]}q_{[]}a_1s_1 - 2a_{[]}b_{[]}q_{[]}p_1r_1 \\
& - 2a_{[]}r_{[]}b_{[]}p_2p_1 + a_{[]}r_{[]}p_{[]}p_2a_1 - 2a_{[]}r_{[]}p_{[]}a_2p_1 - a_{[]}r_{[]}s_{[]}p_2a_1 \\
& + 2a_{[]}r_{[]}s_{[]}a_2p_1 + 2a_{[]}r_{[]}q_{[]}r_2a_1 + a_{[]}r_{[]}q_{[]}b_1p_1 - 2a_{[]}r_{[]}q_{[]}a_2r_1 \\
& + 2a_{[]}r_{[]}q_{[]}a_1p_1 + 2a_{[]}r_{[]}q_{[]}a_1s_1), p_{1,2} = \frac{1}{r_{[]}q_{[]} (b_{[]}^2 + a_{[]}^2 - 2a_{[]}b_{[]})} ( \\
& -2p_{[]}q_{[]}r_{[]}b_2a_1 + 2r_{[]}a_1q_{[]}s_{[]}b_2 + r_{[]}a_1q_{[]}p_2a_{[]} + 2r_{[]}a_1q_{[]}s_2a_{[]} \\
& - r_{[]}a_1q_{[]}p_2b_{[]} - 2r_{[]}a_1q_{[]}b_{[]}s_2 + p_1r_{[]}q_2a_{[]}^2 - 2p_1a_{[]}r_{[]}q_2b_{[]} + p_1a_{[]}q_{[]}r_{[]}b_2 \\
& + p_1q_{[]}r_2a_{[]}^2 - 2p_1a_{[]}q_{[]}r_2b_{[]} + p_1r_{[]}q_2b_{[]}^2 - p_1b_{[]}q_{[]}r_{[]}b_2 + p_1q_{[]}r_2b_{[]}^2), p_{2,2} \\
& = \frac{1}{r_{[]}q_{[]} (b_{[]}^2 + a_{[]}^2 - 2a_{[]}b_{[]})} ( -2r_{[]}p_{[]}q_{[]}a_2b_2 + r_{[]}p_2q_2a_{[]}^2 - 2r_{[]}p_2q_2a_{[]}b_{[]} \\
& + r_{[]}p_2q_2b_{[]}^2 + 2r_{[]}q_{[]}a_2s_{[]}b_2 + r_{[]}q_{[]}a_2p_2a_{[]} + 2r_{[]}q_{[]}a_2s_2a_{[]} - r_{[]}q_{[]}a_2p_2b_{[]} \\
& - 2r_{[]}q_{[]}a_2b_{[]}s_2 - 2r_{[]}q_{[]}^2b_2a_1 + 2r_{[]}q_{[]}^2a_2b_1 - q_{[]}p_1a_{[]}b_2p_{[]} + q_{[]}p_1a_{[]}s_{[]}b_2 \\
& + q_{[]}p_1s_2a_{[]}^2 - 2q_{[]}p_1a_{[]}b_{[]}s_2 + q_{[]}^2p_1a_{[]}b_1 + q_{[]}p_1b_{[]}b_2p_{[]} - q_{[]}p_1b_{[]}s_{[]}b_2 \\
& + q_{[]}p_1b_{[]}^2s_2 - q_{[]}^2p_1b_{[]}b_1), r_{1,1} = \frac{1}{r_{[]}q_{[]}^2 (b_{[]}^2 + a_{[]}^2 - 2a_{[]}b_{[]})} ( -a_{[]}r_{[]}^3a_2q_2 \\
& - 2a_{[]}b_{[]}q_{[]}^2r_1^2 + a_{[]}^2q_{[]}^2r_1^2 + b_{[]}^2q_{[]}^2r_1^2 + b_{[]}r_{[]}^3a_2q_2 + a_{[]}^2r_{[]}^2q_2p_1 - a_{[]}^2r_{[]}^2q_{[]}q_{1,1} + \\
& b_{[]}^2r_{[]}^2q_2p_1 - b_{[]}^2r_{[]}^2q_{[]}q_{1,1} - 4q_{[]}r_{[]}p_{[]}b_1s_{[]}a_1 + 2b_{[]}r_{[]}q_{[]}p_{[]}b_1p_1
\end{aligned}$$



$$\begin{aligned}
& + b_{[]} r_{[]} q_{[]} p_{[]} r_2 a_1 + 2 b_{[]} r_{[]} q_{[]} p_{[]} a_1 s_1 - 2 b_{[]} r_{[]} q_{[]} s_{[]} b_1 p_1 - b_{[]} r_{[]} q_{[]} s_{[]} r_2 a_1 \\
& - 2 b_{[]} r_{[]} q_{[]} s_{[]} a_1 s_1 - 2 a_{[]} q_{[]} r_{[]} p_{[]} b_1 p_1 - a_{[]} q_{[]} r_{[]} p_{[]} r_2 a_1 - 2 a_{[]} q_{[]} r_{[]} p_{[]} a_1 s_1 \\
& + 2 a_{[]} q_{[]} r_{[]} s_{[]} b_1 p_1 + a_{[]} q_{[]} r_{[]} s_{[]} r_2 a_1 + 2 a_{[]} q_{[]} r_{[]} s_{[]} a_1 s_1 + 2 a_{[]} q_{[]} r_{[]} b_{[]} q_1 r_1 \\
& - 2 a_{[]} q_{[]} r_{[]} b_{[]} p_1 r_2 - 4 a_{[]} q_{[]} r_{[]} b_{[]} p_1 s_1 - 2 q_{[]} r_{[]}^2 a_1 b_2 p_{[]} + 2 q_{[]} r_{[]}^2 p_{[]} b_1 a_2 \\
& + 2 q_{[]} r_{[]} b_1 a_1 p_{[]}^2 + 2 q_{[]} r_{[]}^2 s_{[]} b_2 a_1 - 2 q_{[]} r_{[]}^2 s_{[]} b_1 a_2 + 2 q_{[]} r_{[]} b_1 s_{[]}^2 a_1 - 2 b_{[]} r_{[]} \\
& q_{[]}^2 a_1 r_1 + b_{[]} r_{[]} q_{[]}^2 b_1 r_1 + b_{[]} r_{[]}^2 q_2 a_1 p_{[]} - b_{[]} r_{[]}^2 q_2 a_1 s_{[]} - 2 b_{[]} r_{[]}^2 q_{[]} p_2 a_1 - 2 b_{[]} \\
& r_{[]}^2 q_{[]} a_1 s_2 - 2 b_{[]} r_{[]}^2 q_{[]} q_1 a_1 + b_{[]} r_{[]}^2 q_{[]} q_1 b_1 + b_{[]} r_{[]}^2 q_{[]} a_2 r_2 + 2 b_{[]} r_{[]}^2 q_{[]} a_2 p_1 \\
& + 2 b_{[]} r_{[]}^2 q_{[]} a_2 s_1 - a_{[]}^2 q_{[]} r_{[]} q_1 r_1 + a_{[]}^2 q_{[]} r_{[]} p_1 r_2 + 2 a_{[]}^2 q_{[]} r_{[]} p_1 s_1 - b_{[]}^2 q_{[]} r_{[]} q_1 r_1 \\
& + b_{[]}^2 q_{[]} r_{[]} p_1 r_2 + 2 b_{[]}^2 q_{[]} r_{[]} p_1 s_1 + 2 a_{[]} q_{[]}^2 r_{[]} a_1 r_1 - a_{[]} q_{[]}^2 r_{[]} b_1 r_1 - a_{[]} r_{[]}^2 q_2 a_1 p_{[]} \\
& + a_{[]} r_{[]}^2 q_2 a_1 s_{[]} - 2 a_{[]} r_{[]}^2 q_2 b_{[]} p_1 + 2 a_{[]} r_{[]}^2 q_{[]} p_2 a_1 + 2 a_{[]} r_{[]}^2 q_{[]} a_1 s_2 + 2 a_{[]} \\
& r_{[]}^2 q_{[]} q_1 a_1 - a_{[]} r_{[]}^2 q_{[]} q_1 b_1 - a_{[]} r_{[]}^2 q_{[]} a_2 r_2 - 2 a_{[]} r_{[]}^2 q_{[]} a_2 p_1 - 2 a_{[]} r_{[]}^2 q_{[]} a_2 s_1 \\
& + 2 a_{[]} r_{[]}^2 q_{[]} b_{[]} q_{1,1}), r_{1,2} = \frac{1}{r_{[]} q_{[]}^2 (b_{[]}^2 + a_{[]}^2 - 2 a_{[]} b_{[]})} \left( -a_1 b_{[]} q_{[]}^2 r_{[]} r_2 \right. \\
& - a_1 b_{[]} q_{[]} q_2 r_{[]}^2 + 2 a_1 b_2 q_{[]} r_{[]} s_{[]}^2 + b_{[]} b_2 q_{[]}^2 r_{[]} r_1 + b_{[]} b_2 q_{[]} q_1 r_{[]}^2 + a_{[]} a_1 q_{[]}^2 r_{[]} r_2 \\
& + 2 a_{[]}^2 p_1 q_{[]} r_{[]} s_2 - 2 a_{[]} b_{[]} q_1 q_2 r_{[]}^2 - 2 a_{[]} b_{[]} q_{[]}^2 r_1 r_2 - a_{[]} b_2 q_{[]}^2 r_{[]} r_1 \\
& \left. + 2 a_{[]} b_{[]} q_{[]} q_{1,2} r_{[]}^2 - a_{[]} b_2 q_{[]} q_1 r_{[]}^2 + a_{[]} a_1 q_{[]} r_{[]}^2 q_2 + 2 b_{[]}^2 p_1 q_{[]} r_{[]} s_2 + 2 \right.
\end{aligned}$$

$$\begin{aligned}
& p_{[]}^2 a_1 b_2 q_{[]} r_{[]} - a_{[]}^2 q_{[]} q_{1,2} r_{[]}^2 + a_{[]}^2 q_{[]}^2 r_1 r_2 + a_{[]}^2 q_1 q_2 r_{[]}^2 + b_{[]}^2 q_1 q_2 r_{[]}^2 - b_{[]}^2 q_{[]} q_{1,2} r_{[]}^2 \\
& + b_{[]}^2 q_{[]}^2 r_1 r_2 + 2 b_{[]} b_2 p_{[]} p_1 q_{[]} r_{[]} - 2 b_{[]} b_2 p_1 q_{[]} r_{[]} s_{[]} + 2 a_1 b_{[]} p_{[]} q_{[]} r_{[]} s_2 \\
& - 2 a_1 b_{[]} q_{[]} r_{[]} s_{[]} s_2 - 4 a_1 b_2 p_{[]} q_{[]} r_{[]} s_{[]} - 4 a_{[]} b_{[]} p_1 q_{[]} r_{[]} s_2 + 2 a_{[]} b_2 p_1 q_{[]} r_{[]} s_{[]} \\
& + 2 a_{[]} a_1 q_{[]} r_{[]} s_{[]} s_2 - 2 a_{[]} p_{[]} a_1 q_{[]} r_{[]} s_2 - 2 a_{[]} p_{[]} b_2 p_1 q_{[]} r_{[]} \big), r_{2,2} \\
& = \frac{1}{r_{[]} q_{[]}^2 (b_{[]}^2 + a_{[]}^2 - 2 a_{[]} b_{[]})} \big( -2 r_{[]}^2 q_2^2 a_{[]} b_{[]} - q_{[]} r_{[]}^2 q_{2,2} a_{[]}^2 - q_{[]} r_{[]}^2 q_{2,2} b_{[]}^2 + \\
& q_{[]}^3 b_1 r_1 a_{[]} - q_{[]}^3 b_1 r_1 b_{[]} + q_{[]}^2 b_{[]}^2 s_2 r_1 + q_{[]}^2 a_{[]}^2 s_2 r_1 + r_{[]}^2 q_2^2 a_{[]}^2 + r_{[]}^2 q_2^2 b_{[]}^2 \\
& + 2 q_{[]} r_{[]} s_{[]} a_{[]} a_2 s_2 + 2 q_{[]} r_{[]} s_{[]} a_{[]} b_2 p_2 + q_{[]} r_{[]} s_{[]} a_{[]} b_2 q_1 - 2 q_{[]} r_{[]} s_{[]} b_{[]} a_2 s_2 \\
& - 2 q_{[]} r_{[]} s_{[]} b_{[]} b_2 p_2 - q_{[]} r_{[]} s_{[]} b_{[]} b_2 q_1 + 2 q_{[]} r_{[]} a_{[]} b_{[]} q_2 r_2 - 4 q_{[]} r_{[]} a_{[]} b_{[]} s_2 p_2 \\
& - 2 q_{[]} r_{[]} a_{[]} b_{[]} s_2 q_1 - 4 p_{[]} q_{[]} r_{[]} s_{[]} a_2 b_2 - 2 p_{[]} q_{[]} r_{[]} a_{[]} b_2 p_2 - 2 p_{[]} q_{[]} r_{[]} a_{[]} a_2 s_2 \\
& + 2 p_{[]} q_{[]} r_{[]} b_{[]} b_2 p_2 + 2 p_{[]} q_{[]} r_{[]} b_{[]} a_2 s_2 - p_{[]} q_{[]} r_{[]} a_{[]} b_2 q_1 + p_{[]} q_{[]} r_{[]} b_{[]} b_2 q_1 \\
& + q_{[]} r_{[]} b_{[]}^2 s_2 q_1 + 2 p_{[]} q_{[]}^2 r_{[]} b_2 a_1 - 2 p_{[]} q_{[]}^2 r_{[]} a_2 b_1 - p_{[]} q_{[]}^2 r_1 a_{[]} b_2 + p_{[]} \\
& q_{[]}^2 r_1 b_{[]} b_2 - 2 q_{[]}^2 r_{[]} s_{[]} b_2 a_1 + 2 q_{[]}^2 s_{[]} b_1 r_{[]} a_2 - q_{[]}^2 b_{[]} s_{[]} b_2 r_1 - q_{[]}^2 b_{[]} r_{[]} a_2 r_2 - 2 \\
& q_{[]}^2 b_{[]} r_{[]} b_1 p_2 - 2 q_{[]}^2 b_{[]} r_{[]} s_2 b_1 - q_{[]}^2 b_{[]} r_{[]} q_1 b_1 + 2 q_{[]}^2 b_{[]} r_{[]} b_2 r_2 + 2 q_{[]}^2 r_{[]} b_2 b_{[]} p_1 \\
& + 2 q_{[]}^2 b_{[]} r_{[]} b_2 s_1 + q_{[]}^2 a_{[]} s_{[]} b_2 r_1 - 2 q_{[]}^2 a_{[]} r_1 b_{[]} s_2 + q_{[]}^2 a_{[]} r_{[]} a_2 r_2 + 2 \\
& q_{[]}^2 a_{[]} r_{[]} b_1 p_2 + 2 q_{[]}^2 a_{[]} r_{[]} s_2 b_1 + q_{[]}^2 a_{[]} r_{[]} q_1 b_1 - 2 q_{[]}^2 a_{[]} r_{[]} b_2 r_2 - 2 q_{[]}^2 r_{[]} b_2 p_1 a_{[]}
\end{aligned}$$

$$\begin{aligned}
& -2q_{[]}^2a_{[]}r_{[]}b_2s_1+2p_{[]}^2q_{[]}r_{[]}a_2b_2+2q_{[]}r_{[]}s_{[]}^2a_2b_2+q_{[]}r_{[]}^2a_2q_2a_{[]} -2q_{[]} \\
& r_{[]}^2b_2q_2a_{[]}+2q_{[]}r_{[]}^2a_{[]}q_{2,2}b_{[]} -q_{[]}r_{[]}a_{[]}^2q_2r_2+2q_{[]}r_{[]}a_{[]}^2s_2p_2+q_{[]}r_{[]}a_{[]}^2s_2q_1 \\
& -q_{[]}r_{[]}^2a_2q_2b_{[]}+2q_{[]}r_{[]}^2b_2q_2b_{[]} -q_{[]}r_{[]}b_{[]}^2q_2r_2+2q_{[]}r_{[]}b_{[]}^2s_2p_2),s_{1,1} \\
& =\frac{1}{q_{[]}r_{[]}\left(b_{[]}^2+a_{[]}^2-2a_{[]}b_{[]}\right)}\left(-2q_{[]}r_{[]}^2b_2a_1+2q_{[]}r_{[]}^2b_1a_2+2q_{[]}r_{[]}b_1a_1p_{[]} \right. \\
& -2q_{[]}r_{[]}b_1s_{[]}a_1+r_{[]}a_{[]}^2s_2p_1+r_{[]}b_{[]}^2s_2p_1+r_{[]}^2b_{[]}a_2s_2+p_{[]}r_{[]}a_1b_{[]}s_2 \\
& -r_{[]}a_1s_{[]}b_{[]}s_2+2b_{[]}r_{[]}q_{[]}b_1p_1-r_{[]}^2a_{[]}a_2s_2-p_{[]}r_{[]}a_1s_2a_{[]}+r_{[]}a_1s_{[]}s_2a_{[]} \\
& -2r_{[]}p_1a_{[]}b_{[]}s_2-2a_{[]}r_{[]}q_{[]}b_1p_1-q_{[]}s_1a_{[]}r_{[]}b_1+q_{[]}s_1r_1a_{[]}^2-2q_{[]}s_1a_{[]}r_1b_{[]} \\
& \left.+q_{[]}s_1b_{[]}r_{[]}b_1+q_{[]}s_1r_1b_{[]}^2\right),s_{1,2} \\
& =\frac{1}{q_{[]}r_{[]}\left(b_{[]}^2+a_{[]}^2-2a_{[]}b_{[]}\right)}\left(2p_{[]}q_{[]}r_{[]}b_2a_1+r_{[]}s_2q_1a_{[]}^2-2r_{[]}s_2q_1a_{[]}b_{[]} \right. \\
& +r_{[]}s_2q_1b_{[]}^2+q_{[]}a_{[]}^2s_2r_1-2q_{[]}a_{[]}r_1b_{[]}s_2+q_{[]}b_{[]}^2s_2r_1-2r_{[]}a_1q_{[]}s_{[]}b_2 \\
& -r_{[]}a_1q_{[]}s_2a_{[]} -2p_1a_{[]}q_{[]}r_{[]}b_2-q_{[]}a_{[]}r_{[]}b_2s_1+r_{[]}a_1q_{[]}b_{[]}s_2 \\
& \left.+2p_1b_{[]}q_{[]}r_{[]}b_2+q_{[]}b_{[]}r_{[]}b_2s_1\right),s_{2,2}=\frac{1}{q_{[]}r_{[]}\left(b_{[]}^2+a_{[]}^2-2a_{[]}b_{[]}\right)}\left(r_{[]}q_2s_2 \right. \\
& a_{[]}^2+r_{[]}q_2s_2b_{[]}^2+q_{[]}s_1s_2a_{[]}^2+q_{[]}s_1b_{[]}^2s_2-2q_{[]}^2a_{[]}b_2r_1+2q_{[]}^2a_{[]}b_1r_2+q_{[]}^2a_{[]}b_1s_1 \\
& +2q_{[]}^2b_{[]}b_2r_1-2q_{[]}^2b_{[]}b_1r_2-q_{[]}^2b_{[]}b_1s_1+2r_{[]}q_{[]}^2b_2a_1-2r_{[]}q_{[]}^2a_2b_1 \\
& -2r_{[]}q_2s_2a_{[]}b_{[]} -2p_{[]}q_{[]}b_1s_2a_{[]}+p_{[]}q_{[]}b_2s_1a_{[]}+2p_{[]}q_{[]}b_1b_{[]}s_2 \\
& -p_{[]}q_{[]}b_2s_1b_{[]}+2q_{[]}r_{[]}a_{[]}q_2b_1-2q_{[]}r_{[]}a_{[]}b_2p_2-2q_{[]}r_{[]}a_{[]}b_2s_2 \\
& -2q_{[]}r_{[]}a_{[]}b_2q_1-2q_{[]}r_{[]}b_{[]}q_2b_1+2q_{[]}r_{[]}b_{[]}b_2p_2+2q_{[]}r_{[]}b_{[]}b_2s_2 \\
& \left.+2q_{[]}r_{[]}b_{[]}b_2q_1+2q_{[]}a_{[]}s_{[]}s_2b_1-q_{[]}a_{[]}s_1s_{[]}b_2-2q_{[]}a_{[]}s_1b_{[]}s_2\right)
\end{aligned}$$

$$\begin{aligned} & -2q_{[]}b_{[]}s_{[]}s_2b_1 + q_{[]}b_{[]}s_1s_{[]}b_2 + 2r_{[]}p_{[]}q_{[]}a_2b_2 - 2r_{[]}q_{[]}a_2s_{[]}b_2 \\ & -r_{[]}q_{[]}a_2s_2a_{[]} + r_{[]}q_{[]}a_2b_{[]}s_2) \} \end{aligned}$$

**J2 >**

Now we want to compare this to the Integrability Conditions written down above

**J2 >**

**J2 >** *JIC*[1]

$$\begin{aligned} a_{1,1} = & \frac{1}{(a_{[]} - b_{[]})q_{[]}r_{[]}} \left( -r_{[]}^2a_2^2 - r_{[]}a_1a_2p_{[]} + r_{[]}a_1a_2s_{[]} + 2r_{[]}a_1p_2a_{[]} - 2r_{[]}a_1p_2b_{[]} \right. \\ & \left. + 2r_{[]}q_{[]}a_1^2 + r_{[]}a_1q_{[]}b_1 - r_{[]}a_2p_1a_{[]} + r_{[]}a_2p_1b_{[]} + q_{[]}a_1r_1a_{[]} - q_{[]}a_1r_1b_{[]} \right) \end{aligned} \quad (49)$$

**J2 >** *SQE*[1]

$$\begin{aligned} a_{1,1} = & \frac{1}{(a_{[]} - b_{[]})q_{[]}r_{[]}} \left( -r_{[]}^2a_2^2 - r_{[]}a_1a_2p_{[]} + r_{[]}a_1a_2s_{[]} + 2r_{[]}a_1p_2a_{[]} - 2r_{[]}a_1p_2b_{[]} \right. \\ & \left. + 2r_{[]}q_{[]}a_1^2 + r_{[]}a_1q_{[]}b_1 - r_{[]}a_2p_1a_{[]} + r_{[]}a_2p_1b_{[]} + q_{[]}a_1r_1a_{[]} - q_{[]}a_1r_1b_{[]} \right) \end{aligned} \quad (50)$$

**J2 >** *simplify*(*JIC*[1] - *SQE*[1])

$$0 = 0$$

(51)

**J2 >** **for** *i* **to** 9 **do** *simplify*(*JIC*[*i*] - *SQE*[*i*]) **od**

$$0 = 0$$

$$0 = 0$$

$$0 = 0$$

$$0 = 0$$

$$0 = 0$$

$$0 = 0$$

$$0 = 0$$

$$0 = 0$$

$$0 = 0$$

(52)

**J2 >** **for** *i* **from** 10 **to** 15 **do** *simplify*(*JIC*[*i* + 1] - *SQE*[*i*]) **od**

$$0 = 0$$

$$\begin{aligned} 0 = & -\frac{1}{q_{[]}^2(b_{[]}^2 + a_{[]}^2 - 2a_{[]}b_{[]})} \left( 2a_{[]}b_{[]}q_{[]}q_{1,2}r_{[]} - a_{[]}^2q_{[]}q_{1,2}r_{[]} - b_{[]}^2q_{[]}q_{1,2}r_{[]} \right. \\ & + q_{[]}p_1s_2a_{[]}^2 + q_{[]}^2p_1a_{[]}b_1 + q_{[]}p_1b_{[]}^2s_2 - q_{[]}^2p_1b_{[]}b_1 - p_{[]}q_{[]}^2a_1b_1 + a_1q_{[]}^2r_2a_{[]} \\ & - a_1q_{[]}^2r_2b_{[]} + q_{[]}a_1s_{[]}^2b_2 + a_1s_{[]}q_{[]}^2b_1 + r_{[]}q_2q_1a_{[]}^2 + r_{[]}q_2q_1b_{[]}^2 + p_{[]}^2q_{[]}b_2a_1 \\ & - r_{[]}p_{[]}q_{[]}a_2b_2 + r_{[]}q_{[]}a_2s_{[]}b_2 + r_{[]}q_{[]}a_2s_2a_{[]} - r_{[]}q_{[]}a_2b_{[]}s_2 - q_{[]}p_1a_{[]}b_2p_{[]} \\ & + q_{[]}p_1a_{[]}s_{[]}b_2 - 2q_{[]}p_1a_{[]}b_{[]}s_2 + q_{[]}p_1b_{[]}b_2p_{[]} - q_{[]}p_1b_{[]}s_{[]}b_2 \\ & - 2p_{[]}q_{[]}s_{[]}b_2a_1 - p_{[]}q_{[]}a_1s_2a_{[]} + p_{[]}q_{[]}a_1b_{[]}s_2 + q_{[]}r_{[]}a_{[]}q_2a_1 - q_{[]}r_{[]}b_{[]}q_2a_1 \\ & \left. + q_{[]}a_1s_{[]}s_2a_{[]} - q_{[]}a_1s_{[]}b_{[]}s_2 - 2r_{[]}q_2q_1a_{[]}b_{[]} \right) \end{aligned}$$

$$0 = 0$$

$$0 = 0$$

$$0 = 0$$

$$0 = 0 \quad (53)$$

$$\text{J2} > \text{simplify}(\text{subs}(\text{JIC}[10], \text{JIC}[12] - \text{SQE}[11]))$$

$$0 = 0 \quad (54)$$

$$\text{J2} > \text{JIC}[10]$$

$$q_{1,2} = \frac{1}{(a_{[]} - b_{[]})^2 q_{[]} r_{[]}} \left( q_{[]} p_1 s_2 a_{[]}^2 + q_{[]}^2 p_1 a_{[]} b_1 + q_{[]} p_1 b_{[]}^2 s_2 - q_{[]}^2 p_1 b_{[]} b_1 - p_{[]} \right. \\ q_{[]}^2 a_1 b_1 + a_1 q_{[]}^2 r_2 a_{[]} - a_1 q_{[]}^2 r_2 b_{[]} + q_{[]} a_1 s_{[]}^2 b_2 + a_1 s_{[]} q_{[]}^2 b_1 + r_{[]} q_2 q_1 a_{[]}^2 + r_{[]} q_2 q_1 \\ b_{[]}^2 + p_{[]}^2 q_{[]} b_2 a_1 - r_{[]} p_{[]} q_{[]} a_2 b_2 + r_{[]} q_{[]} a_2 s_{[]} b_2 + r_{[]} q_{[]} a_2 s_2 a_{[]} - r_{[]} q_{[]} a_2 b_{[]} s_2 \\ - q_{[]} p_1 a_{[]} b_2 p_{[]} + q_{[]} p_1 a_{[]} s_{[]} b_2 - 2 q_{[]} p_1 a_{[]} b_{[]} s_2 + q_{[]} p_1 b_{[]} b_2 p_{[]} \\ - q_{[]} p_1 b_{[]} s_{[]} b_2 - 2 p_{[]} q_{[]} s_{[]} b_2 a_1 - p_{[]} q_{[]} a_1 s_2 a_{[]} + p_{[]} q_{[]} a_1 b_{[]} s_2 + q_{[]} r_{[]} a_{[]} q_2 a_1 \\ \left. - q_{[]} r_{[]} b_{[]} q_2 a_1 + q_{[]} a_1 s_{[]} s_2 a_{[]} - q_{[]} a_1 s_{[]} b_{[]} s_2 - 2 r_{[]} q_2 q_1 a_{[]} b_{[]} \right) \quad (55)$$

$$\text{J2} > \text{JIC}[12]$$

$$r_{1,2} = \frac{1}{(a_{[]} - b_{[]})^2 q_{[]} r_{[]}} \left( p_{[]} r_{[]}^2 a_2 b_2 + r_{[]} a_1 s_{[]}^2 b_2 + r_{[]} a_{[]}^2 s_2 p_1 + r_{[]} b_{[]}^2 s_2 p_1 - r_{[]}^2 s_{[]} a_2 b_2 \right. \\ - r_{[]}^2 a_{[]} a_2 s_2 - r_{[]}^2 a_{[]} b_2 q_1 + r_{[]}^2 b_{[]} a_2 s_2 + r_{[]}^2 b_{[]} b_2 q_1 + q_{[]} r_1 r_2 a_{[]}^2 + q_{[]} r_1 r_2 b_{[]}^2 + \\ p_{[]}^2 r_{[]} b_2 a_1 + q_{[]} r_{[]} b_1 a_1 p_{[]} - q_{[]} r_{[]} b_1 s_{[]} a_1 + b_{[]} r_{[]} q_{[]} b_1 p_1 - a_{[]} r_{[]} q_{[]} b_1 p_1 \\ - 2 p_{[]} r_{[]} s_{[]} b_2 a_1 - p_{[]} r_{[]} a_1 s_2 a_{[]} + p_{[]} r_{[]} a_1 b_{[]} s_2 - p_{[]} r_{[]} b_2 p_1 a_{[]} + p_{[]} r_{[]} b_2 b_{[]} p_1 \\ + r_{[]} p_1 a_{[]} s_{[]} b_2 - r_{[]} p_1 b_{[]} s_{[]} b_2 + r_{[]} a_1 s_{[]} s_2 a_{[]} - 2 r_{[]} p_1 a_{[]} b_{[]} s_2 - r_{[]} a_1 s_{[]} b_{[]} s_2 \\ \left. - q_{[]} r_1 a_{[]} r_{[]} b_2 - 2 q_{[]} r_1 a_{[]} r_2 b_{[]} + q_{[]} r_1 b_{[]} r_{[]} b_2 \right) \quad (56)$$

$$\text{J2} > \text{SQE}[11]$$

$$r_{1,2} = \frac{1}{r_{[]} q_{[]}^2 (b_{[]}^2 + a_{[]}^2 - 2 a_{[]} b_{[]})} \left( -a_1 b_{[]} q_{[]}^2 r_{[]} r_2 - a_1 b_{[]} q_{[]} q_2 r_{[]}^2 + 2 a_1 b_2 q_{[]} r_{[]} s_{[]}^2 \right. \\ + b_{[]} b_2 q_{[]}^2 r_{[]} r_1 + b_{[]} b_2 q_{[]} q_1 r_{[]}^2 + a_{[]} a_1 q_{[]}^2 r_{[]} r_2 + 2 a_{[]}^2 p_1 q_{[]} r_{[]} s_2 - 2 a_{[]} b_{[]} q_1 q_2 \\ r_{[]}^2 - 2 a_{[]} b_{[]} q_{[]}^2 r_1 r_2 - a_{[]} b_2 q_{[]}^2 r_{[]} r_1 + 2 a_{[]} b_{[]} q_{[]} q_{1,2} r_{[]}^2 - a_{[]} b_2 q_{[]} q_1 r_{[]}^2 \\ + a_{[]} a_1 q_{[]}^2 q_2 + 2 b_{[]}^2 p_1 q_{[]} r_{[]} s_2 + 2 p_{[]}^2 a_1 b_2 q_{[]} r_{[]} - a_{[]}^2 q_{[]} q_{1,2} r_{[]}^2 + a_{[]}^2 q_{[]}^2 r_1 r_2 + \\ a_{[]}^2 q_1 q_2 r_{[]}^2 + b_{[]}^2 q_1 q_2 r_{[]}^2 - b_{[]}^2 q_{[]} q_{1,2} r_{[]}^2 + b_{[]}^2 q_{[]}^2 r_1 r_2 + 2 b_{[]} b_2 p_{[]} p_1 q_{[]} r_{[]} \\ - 2 b_{[]} b_2 p_1 q_{[]} r_{[]} s_{[]} + 2 a_1 b_{[]} p_{[]} q_{[]} r_{[]} s_2 - 2 a_1 b_{[]} q_{[]} r_{[]} s_{[]} s_2 - 4 a_1 b_2 p_{[]} q_{[]} r_{[]} s_{[]} \\ - 4 a_{[]} b_{[]} p_1 q_{[]} r_{[]} s_2 + 2 a_{[]} b_2 p_1 q_{[]} r_{[]} s_{[]} + 2 a_{[]} a_1 q_{[]} r_{[]} s_{[]} s_2 - 2 a_{[]} p_{[]} a_1 q_{[]} r_{[]} s_2 \\ \left. - 2 a_{[]} p_{[]} b_2 p_1 q_{[]} r_{[]} \right) \quad (57)$$

$$\text{J2} > \text{simplify}(\text{coeff}(\text{subs}(\text{SQE}[11], r_{1,2}), q_{1,2}))$$

$$- \frac{r_{[]}}{q_{[]}} \quad (58)$$

$$\text{J2} >$$

Thus we see that the equations express  $(a_{ij}, b_{ij}, p_{ij}, (q*r)_{ij}, s_{ij})$ , precisely the same 15 equations that were obtained by Ferapontov and Khusnutdinova (2004) in the first round of the investigation of the integrability. Remark that the 16th equation was obtained from the first 15 by bringing the system to involution. As we also have to bring to involution, we obtain the above 16 equations IC and so the integrability of the system. Done!  
To conclude: provided that the matrix of the symbol is non-constant (another not identical to this version: that the equation is not linearizable) the EW property is equivalent to integrability.

**J2 >**

**J2 >**

Let us show to the end that IC conditions do not hold for linearizable equations (i.e. in IC conditions of Ferapontov and Khusnutdinova one has to assume integrability minus linearizability). Take for instance the equation  $a_{1,2}=0$  for the linear equation (constant coeffs) and get a non-zero identity...

$$\begin{aligned} \mathbf{J2} > \text{simplify} \left( \text{subs} \left( \left[ a_{[]} = a_1 \cdot t + a_2 \cdot x + a_3 \cdot y, b_{[]} = b_1 \cdot t + b_2 \cdot x + b_3 \cdot y, p_{[]} = p_1 \cdot t + p_2 \cdot x + p_3 \cdot y, \right. \right. \right. \\ \left. \left. \left. q_{[]} = q_1 \cdot t + q_2 \cdot x + q_2 \cdot y, r_{[]} = r_1 \cdot t + r_2 \cdot x + r_3 \cdot y, s_{[]} = s_1 \cdot t + s_2 \cdot x + s_3 \cdot y \right], \right. \right. \\ \left. \left. \frac{(r_{[]} q_2 a_{[]} - r_{[]} q_2 b_{[]} + q_{[]} r_{[]} a_2 + q_{[]} r_{[]} b_2 + q_{[]} r_2 a_{[]} - q_{[]} r_2 b_{[]} ) a_1}{(a_{[]} - b_{[]} ) q_{[]} r_{[]} }} \right) \right) \\ \left( \left( 2 a_2 q_1 t r_2 x + a_2 q_1 t r_3 y + a_2 q_2 y r_1 t + 2 a_2 q_2 y r_2 x + b_2 q_1 t r_3 y + b_2 q_2 y r_1 t + r_2 q_1 t a_3 y \right. \right. \quad (59) \\ \left. \left. + r_2 q_2 y a_1 t - r_2 q_1 t b_3 y - r_2 q_2 y b_1 t + 2 q_2 r_1 t a_2 x + q_2 r_1 t a_3 y + 2 q_2 r_2 x a_1 t \right. \right. \\ \left. \left. + 2 q_2 r_2 x a_3 y + q_2 r_3 y a_1 t + 2 q_2 r_3 y a_2 x - q_2 r_1 t b_3 y - 2 q_2 r_2 x b_1 t - 2 q_2 r_2 x b_3 y \right. \right. \\ \left. \left. - q_2 r_3 y b_1 t + q_2 r_1 t^2 a_1 + 3 q_2 r_2 x^2 a_2 + q_2 r_3 y^2 a_3 - q_2 r_1 t^2 b_1 - q_2 r_2 x^2 b_2 - q_2 r_3 y^2 b_3 \right. \right. \\ \left. \left. + a_2 q_1 t^2 r_1 + a_2 q_2 y^2 r_3 + b_2 q_1 t^2 r_1 + b_2 q_2 y^2 r_3 + r_2 q_1 t^2 a_1 + r_2 q_2 y^2 a_3 - r_2 q_1 t^2 b_1 \right. \right. \\ \left. \left. - r_2 q_2 y^2 b_3 \right) a_1 \right) / \left( (a_1 t + a_2 x + a_3 y - b_1 t - b_2 x - b_3 y) (q_1 t + q_2 x + q_2 y) (r_1 t \right. \\ \left. + r_2 x + r_3 y) \right) \end{aligned}$$

Now I want to check compatibility (bring to involution) for the obtained system of 15 equations

**J2 >**  $DGsetup([u, v], [a, b, p, q, r, s], D2)$   
frame name: D2 (60)

**D2 >**  $smb12 := Z \rightarrow \text{add}(\text{add}(\text{diff}(Z, a[i, j]) \cdot a[i, j], j = i..2), i = 1..2) + \text{add}(\text{add}(\text{diff}(Z, b[i, j]) \cdot b[i, j], j = i..2), i = 1..2) + \text{add}(\text{add}(\text{diff}(Z, p[i, j]) \cdot p[i, j], j = i..2), i = 1..2) + \text{add}(\text{add}(\text{diff}(Z, q[i, j]) \cdot q[i, j], j = i..2), i = 1..2) + \text{add}(\text{add}(\text{diff}(Z, r[i, j]) \cdot r[i, j], j = i..2), i = 1..2) + \text{add}(\text{add}(\text{diff}(Z, s[i, j]) \cdot s[i, j], j = i..2), i = 1..2) :$

**D2 >**  $smb13 := Z \rightarrow \text{add}(\text{add}(\text{add}(\text{diff}(Z, a[i, j, k]) \cdot a[i, j, k], k = j..2), j = i..2), i = 1..2) + \text{add}(\text{add}(\text{add}(\text{diff}(Z, b[i, j, k]) \cdot b[i, j, k], k = j..2), j = i..2), i = 1..2) + \text{add}(\text{add}(\text{add}(\text{diff}(Z, p[i, j, k]) \cdot p[i, j, k], k = j..2), j = i..2), i = 1..2) + \text{add}(\text{add}(\text{add}(\text{diff}(Z, q[i, j, k]) \cdot q[i, j, k], k = j..2), j = i..2), i = 1..2)$

+ add(add(add(diff(Z, r[i, j, k]) · r[i, j, k], k=j..2), j=i..2), i=1..2)  
+ add(add(add(diff(Z, s[i, j, k]) · s[i, j, k], k=j..2), j=i..2), i=1..2) :

**D2 >**

**J2 >**  $TMP := \text{simplify}(\text{subs}(SQE, \text{TotalDiff}(\text{subs}(SQE, a_{1,1}), 2) - \text{TotalDiff}(\text{subs}(SQE, a_{1,2}), 1)))$

$$TMP := \frac{1}{r_{[]} q_{[]}^2 (b_{[]}^2 + a_{[]}^2 - 2 a_{[]} b_{[]})} \left( (2 a_{[]} b_{[]} q_{[]} q_{1,2} r_{[]} - a_{[]}^2 q_{[]} q_{1,2} r_{[]} - b_{[]}^2 q_{[]} q_{1,2} r_{[]} \right. \quad (61)$$

$$+ q_{[]} p_1 s_2 a_{[]}^2 + q_{[]}^2 p_1 a_{[]} b_1 + q_{[]} p_1 b_{[]}^2 s_2 - q_{[]}^2 p_1 b_{[]} b_1 - p_{[]} q_{[]}^2 a_1 b_1 + a_1 q_{[]}^2 r_2 a_{[]} \\ - a_1 q_{[]}^2 r_2 b_{[]} + q_{[]} a_1 s_{[]}^2 b_2 + a_1 s_{[]} q_{[]}^2 b_1 + r_{[]} q_2 q_1 a_{[]}^2 + r_{[]} q_2 q_1 b_{[]}^2 + p_{[]}^2 q_{[]} b_2 a_1 \\ - r_{[]} p_{[]} q_{[]} a_2 b_2 + r_{[]} q_{[]} a_2 s_{[]} b_2 + r_{[]} q_{[]} a_2 s_2 a_{[]} - r_{[]} q_{[]} a_2 b_{[]} s_2 - q_{[]} p_1 a_{[]} b_2 p_{[]} \\ + q_{[]} p_1 a_{[]} s_{[]} b_2 - 2 q_{[]} p_1 a_{[]} b_{[]} s_2 + q_{[]} p_1 b_{[]} b_2 p_{[]} - q_{[]} p_1 b_{[]} s_{[]} b_2 \\ - 2 p_{[]} q_{[]} s_{[]} b_2 a_1 - p_{[]} q_{[]} a_1 s_2 a_{[]} + p_{[]} q_{[]} a_1 b_{[]} s_2 + q_{[]} r_{[]} a_{[]} q_2 a_1 - q_{[]} r_{[]} b_{[]} q_2 a_1 \\ \left. + q_{[]} a_1 s_{[]} s_2 a_{[]} - q_{[]} a_1 s_{[]} b_{[]} s_2 - 2 r_{[]} q_2 q_1 a_{[]} b_{[]} \right) a_1$$

So here compatibility fails, but there can be two reasons for this: the equation has two factors of order 1 or 2.

So I will be careful and resolve the first factor for the only 2-jet coordinate and add to this an indeterminate QQQ

**D2 >**  $\text{smb12}(TMP)$

$$\frac{(2 a_{[]} b_{[]} q_{[]} r_{[]} - a_{[]}^2 q_{[]} r_{[]} - b_{[]}^2 q_{[]} r_{[]}) a_1 q_{1,2}}{r_{[]} q_{[]}^2 (b_{[]}^2 + a_{[]}^2 - 2 a_{[]} b_{[]})} \quad (62)$$

**D2 >**  $\text{slvTMP} := \text{solve}(TMP, q_{1,2})$

$$\text{slvTMP} := \frac{1}{r_{[]} q_{[]} (b_{[]}^2 + a_{[]}^2 - 2 a_{[]} b_{[]})} \left( q_{[]} p_1 s_2 a_{[]}^2 + q_{[]}^2 p_1 a_{[]} b_1 + q_{[]} p_1 b_{[]}^2 s_2 - \right. \quad (63)$$

$$q_{[]}^2 p_1 b_{[]} b_1 - p_{[]} q_{[]}^2 a_1 b_1 + a_1 q_{[]}^2 r_2 a_{[]} - a_1 q_{[]}^2 r_2 b_{[]} + q_{[]} a_1 s_{[]}^2 b_2 + a_1 s_{[]} q_{[]}^2 b_1 \\ + r_{[]} q_2 q_1 a_{[]}^2 + r_{[]} q_2 q_1 b_{[]}^2 + p_{[]}^2 q_{[]} b_2 a_1 - r_{[]} p_{[]} q_{[]} a_2 b_2 + r_{[]} q_{[]} a_2 s_{[]} b_2 \\ + r_{[]} q_{[]} a_2 s_2 a_{[]} - r_{[]} q_{[]} a_2 b_{[]} s_2 - q_{[]} p_1 a_{[]} b_2 p_{[]} + q_{[]} p_1 a_{[]} s_{[]} b_2 - 2 q_{[]} p_1 a_{[]} b_{[]} s_2 \\ + q_{[]} p_1 b_{[]} b_2 p_{[]} - q_{[]} p_1 b_{[]} s_{[]} b_2 - 2 p_{[]} q_{[]} s_{[]} b_2 a_1 - p_{[]} q_{[]} a_1 s_2 a_{[]} + p_{[]} q_{[]} a_1 b_{[]} s_2 \\ + q_{[]} r_{[]} a_{[]} q_2 a_1 - q_{[]} r_{[]} b_{[]} q_2 a_1 + q_{[]} a_1 s_{[]} s_2 a_{[]} - q_{[]} a_1 s_{[]} b_{[]} s_2 \\ \left. - 2 r_{[]} q_2 q_1 a_{[]} b_{[]} \right)$$

**D2 >**  $SQEp := \text{simplify}([SQE[1], SQE[2], SQE[3], SQE[4], SQE[5], SQE[6], SQE[7],$   
 $SQE[8], SQE[9], SQE[10], \text{subs}(q_{1,2} = \text{slvTMP} + QQQ, SQE[11]), q_{1,2} = \text{slvTMP}$   
 $+ QQQ, SQE[12], SQE[13], SQE[14], SQE[15]]) :$

**D2 >**

**D2 >**  $\text{simplify}(\text{subs}(SQEp, \text{TotalDiff}(\text{subs}(SQEp, a_{1,1}), 2) - \text{TotalDiff}(\text{subs}(SQEp, a_{1,2}), 1)))$

$$- \frac{a_1 QQQ}{q_{[]}} \quad (64)$$

$$\text{J2} > \text{simplify}(\text{subs}(SQEp, \text{TotalDiff}(\text{subs}(SQEp, a_{1,2}), 2) - \text{TotalDiff}(\text{subs}(SQEp, a_{2,2}), 1)))$$

$$- \frac{QQQ a_2}{q_{[]}} \quad (65)$$

$$\text{J2} > \text{simplify}(\text{subs}(SQEp, \text{TotalDiff}(\text{subs}(SQEp, b_{1,1}), 2) - \text{TotalDiff}(\text{subs}(SQEp, b_{1,2}), 1)))$$

$$- \frac{QQQ b_1}{q_{[]}} \quad (66)$$

$$\text{J2} > \text{simplify}(\text{subs}(SQEp, \text{TotalDiff}(\text{subs}(SQEp, b_{1,2}), 2) - \text{TotalDiff}(\text{subs}(SQEp, b_{2,2}), 1)))$$

$$- \frac{b_2 QQQ}{q_{[]}} \quad (67)$$

$$\text{J2} > \text{simplify}(\text{subs}(SQEp, \text{TotalDiff}(\text{subs}(SQEp, p_{1,1}), 2) - \text{TotalDiff}(\text{subs}(SQEp, p_{1,2}), 1)))$$

$$- \frac{QQQ p_1}{q_{[]}} \quad (68)$$

$$\text{J2} > \text{simplify}(\text{subs}(SQEp, \text{TotalDiff}(\text{subs}(SQEp, p_{1,2}), 2) - \text{TotalDiff}(\text{subs}(SQEp, p_{2,2}), 1)))$$

$$- \frac{QQQ p_2}{q_{[]}} \quad (69)$$

$$\text{J2} > \text{simplify}(\text{subs}(SQEp, \text{TotalDiff}(\text{subs}(SQEp, s_{1,1}), 2) - \text{TotalDiff}(\text{subs}(SQEp, s_{1,2}), 1)))$$

$$- \frac{QQQ s_1}{q_{[]}} \quad (70)$$

$$\text{J2} > \text{simplify}(\text{subs}(SQEp, \text{TotalDiff}(\text{subs}(SQEp, s_{1,2}), 2) - \text{TotalDiff}(\text{subs}(SQEp, s_{2,2}), 1)))$$

$$- \frac{QQQ s_2}{q_{[]}} \quad (71)$$

$$\text{J2} > \text{simplify}(\text{subs}(SQEp, \text{TotalDiff}(\text{subs}(SQEp, \text{TotalDiff}(q_{[]} \cdot r_{[]}, [1, 1]), 2) - \text{TotalDiff}(\text{subs}(SQEp, \text{TotalDiff}(q_{[]} \cdot r_{[]}, [1, 2]), 1)))$$

$$- \frac{QQQ (q_{[]} r_1 + r_{[]} q_1)}{q_{[]}} \quad (72)$$

$$\text{J2} > \text{simplify}(\text{subs}(SQEp, \text{TotalDiff}(\text{subs}(SQEp, \text{TotalDiff}(q_{[]} \cdot r_{[]}, [1, 2]), 2) - \text{TotalDiff}(\text{subs}(SQEp, \text{TotalDiff}(q_{[]} \cdot r_{[]}, [2, 2]), 1)))$$



$$- \frac{QQQ (r_{[]} q_2 + q_{[]} r_2)}{q_{[]}} \quad (73)$$

Conclusion: we have an alternative: either the coefficients of the symbol matrix (=coefficients of the dispersion relation) are constant or  $QQQ=0$ .

The first condition leads to integrability if and only if the function  $q(u,v)$  is separable, in which case the equation is linearizable.

Otherwise we get the condition  $QQQ=0$ , leading to the 16th equation of the system. This new system coincides with the above IC (=JIC in jet-coordinates).

So let us add the 16th equation to JIC and continue checking compatibility conditions. The following shows that this might not be enough:

**D2 >**

**J2 >**  $\text{simplify}(\text{subs}(QQQ=0, \text{subs}(SQEp, \text{TotalDiff}(\text{subs}(SQEp, q_{1,2}), 2) \\ - \text{TotalDiff}(\text{subs}(SQEp, q_{2,2}), 1))))$

$$\frac{1}{q_{[]} (a_{[]} - b_{[]}) (b_{[]}^2 + a_{[]}^2 - 2 a_{[]} b_{[]}) r_{[]}^2} (r_{[]} p_2 a_{[]} q_{[]} a_1 b_2 p_{[]} - r_{[]} p_2 a_{[]} q_{[]} s_{[]} b_2 a_1 \quad (74)$$

$$- 4 r_{[]} p_2 a_{[]} q_{[]} a_1 b_{[]} s_2 - 2 r_{[]} q_1 a_{[]} q_{[]} a_1 b_{[]} s_2 - r_{[]} p_2 b_{[]} q_{[]} a_1 b_2 p_{[]} \\ + r_{[]} p_2 b_{[]} q_{[]} s_{[]} b_2 a_1 + 2 q_{[]} r_{[]}^2 b_1 a_2 q_2 a_{[]} - 2 q_{[]} r_{[]}^2 b_1 a_2 q_2 b_{[]} + 2 r_{[]} p_2 b_{[]}^2 q_{[]} a_1 s_2 \\ - 2 r_{[]} p_2 b_{[]} q_{[]}^2 a_1 b_1 + r_{[]} q_1 b_{[]}^2 q_{[]} a_1 s_2 - r_{[]} q_1 b_{[]} q_{[]}^2 a_1 b_1 - 2 q_{[]}^2 r_1 b_{[]} a_1 s_2 a_{[]} \\ + 2 r_{[]} p_2 a_{[]}^2 q_{[]} a_1 s_2 + 2 r_{[]} p_2 a_{[]} q_{[]}^2 a_1 b_1 + r_{[]} q_1 a_{[]}^2 q_{[]} a_1 s_2 + r_{[]} q_1 a_{[]} q_{[]}^2 a_1 b_1 - 2 \\ q_{[]}^2 r_{[]}^2 b_1 a_2^2 + q_{[]}^2 r_1 b_{[]}^2 a_1 s_2 - q_{[]}^3 r_1 b_{[]} a_1 b_1 + q_{[]}^2 r_1 a_{[]}^2 a_1 s_2 + q_{[]}^3 r_1 a_{[]} a_1 b_1 \\ - r_{[]} a_2 s_{[]} q_{[]} b_2 s_1 b_{[]} + 6 p_{[]} p_1 a_{[]} r_{[]} b_2 q_2 b_{[]} + 4 p_{[]} p_1 a_{[]} q_{[]} r_{[]} a_2 b_2 \\ - 2 p_{[]} p_1 a_{[]} q_{[]} b_1 s_{[]} b_2 + 2 p_{[]} p_1 a_{[]} q_{[]} b_1 b_{[]} s_2 + 2 p_{[]} p_1 a_{[]} q_{[]} b_2 s_1 b_{[]} \\ - 6 p_1 a_{[]} s_{[]} r_{[]} b_2 q_2 b_{[]} - 4 p_1 a_{[]} s_{[]} q_{[]} r_{[]} a_2 b_2 - 2 p_1 a_{[]} s_{[]} q_{[]} b_1 b_{[]} s_2 \\ - 2 p_1 a_{[]} s_{[]} q_{[]} b_2 s_1 b_{[]} - 4 p_{[]} b_{[]} p_1 q_{[]} r_{[]} a_2 b_2 + 2 p_{[]} b_{[]} p_1 q_{[]} b_1 s_{[]} b_2 \\ + 4 p_1 b_{[]} s_{[]} q_{[]} r_{[]} a_2 b_2 - 6 p_{[]} s_{[]} a_1 r_{[]} b_2 q_2 a_{[]} + 6 p_{[]} s_{[]} a_1 r_{[]} b_2 q_2 b_{[]} \\ + 4 p_{[]} s_{[]} a_1 q_{[]} r_{[]} a_2 b_2 - 2 p_{[]} s_{[]} a_1 q_{[]} b_1 s_2 a_{[]} + 2 p_{[]} s_{[]} a_1 q_{[]} b_1 b_{[]} s_2 \\ - 2 p_{[]} s_{[]} a_1 q_{[]} b_2 s_1 a_{[]} + 2 p_{[]} s_{[]} a_1 q_{[]} b_2 s_1 b_{[]} - 2 r_{[]} a_2 p_{[]} q_{[]} b_1 s_{[]} b_2 \\ - r_{[]} a_2 p_{[]} q_{[]} b_1 s_2 a_{[]} + r_{[]} a_2 p_{[]} q_{[]} b_1 b_{[]} s_2 - r_{[]} a_2 p_{[]} q_{[]} b_2 s_1 a_{[]} \\ + r_{[]} a_2 p_{[]} q_{[]} b_2 s_1 b_{[]} + r_{[]} a_2 s_{[]} q_{[]} b_1 s_2 a_{[]} - r_{[]} a_2 s_{[]} q_{[]} b_1 b_{[]} s_2 \\ + r_{[]} a_2 s_{[]} q_{[]} b_2 s_1 a_{[]} + a_1 s_{[]}^2 q_{[]}^2 b_1^2 + p_{[]}^2 a_1 q_{[]}^2 b_1^2 - 2 a_1 b_{[]} b_1 q_{[]}^2 r_2 s_{[]} - a_1 b_{[]} b_1 \\ q_{[]}^2 s_{[]} s_1 + a_1 b_{[]} b_2 p_1 q_{[]}^2 r_{[]} - a_2 b_{[]}^2 p_1 q_{[]} r_{[]} s_2 + a_2 b_{[]}^2 q_{[]} r_{[]} s_1 s_2 + 3 a_2 b_{[]} b_1 p_1 q_{[]}^2 r_{[]} \\ - 2 a_2 b_{[]} b_1 q_{[]}^2 r_{[]} r_2 - a_2 b_{[]} b_1 q_{[]}^2 r_{[]} s_1 + 3 a_2 b_{[]} b_2 p_2 q_{[]} r_{[]}^2 + 5 b_{[]}^2 b_1 p_1 q_{[]} q_2 r_{[]} \\ - 3 b_{[]}^2 b_2 p_1 p_2 q_{[]} r_{[]} - b_{[]}^2 b_2 p_1 q_{[]} q_1 r_{[]} - b_{[]} b_1 b_2 p_1 q_{[]}^2 r_{[]} + a_1 a_2 b_{[]} p_{[]} q_{[]} r_{[]} s_2 \\ - a_1 a_2 b_{[]} q_{[]} r_{[]} s_{[]} s_2 + 5 a_1 b_{[]} b_1 p_{[]} q_{[]} q_2 r_{[]} - 5 a_1 b_{[]} b_1 q_{[]} q_2 r_{[]} s_{[]}]$$

$$\begin{aligned}
& + 8 a_{\square} b_{\square} b_2 p_{\square} q_{\square} r_{\square} s_2 - 8 a_{\square} b_{\square} b_2 q_{\square} r_{\square} s_{\square} s_2 + 2 a_{\square} a_1 b_{\square} p_{\square} q_{\square} s_1 s_2 \\
& + 6 a_{\square} a_1 b_{\square} p_{\square} q_2 r_{\square} s_2 - 6 a_{\square} a_1 b_{\square} q_{\square} q_2 r_{\square} r_2 - 2 a_{\square} a_1 b_{\square} q_{\square} s_{\square} s_1 s_2 \\
& - 6 a_{\square} a_1 b_{\square} q_2 r_{\square} s_{\square} s_2 - 5 a_{\square} a_1 b_1 p_{\square} q_{\square} q_2 r_{\square} + 5 a_{\square} a_1 b_1 q_{\square} q_2 r_{\square} s_{\square} \\
& - 8 a_{\square} a_1 b_2 p_{\square} q_{\square} r_{\square} s_2 + 8 a_{\square} a_1 b_2 q_{\square} r_{\square} s_{\square} s_2 + 2 a_{\square} a_2 b_{\square} p_1 q_{\square} r_{\square} s_2 \\
& - 2 a_{\square} a_2 b_{\square} q_{\square} r_{\square} s_1 s_2 - 10 a_{\square} b_{\square} b_1 p_1 q_{\square} q_2 r_{\square} + 6 a_{\square} b_{\square} b_2 p_1 p_2 q_{\square} r_{\square} \\
& + 2 a_{\square} b_{\square} b_2 p_1 q_{\square} q_1 r_{\square} - a_{\square} a_1 a_2 p_{\square} q_{\square} r_{\square} s_2 + a_{\square} a_1 a_2 q_{\square} r_{\square} s_{\square} s_2 + a_{\square}^3 p_1 q_{\square} s_1 s_2 \\
& + 3 a_{\square}^3 p_1 q_2 r_{\square} s_2 + 4 a_{\square}^2 a_1 q_{\square} r_{\square} s_2^2 + 3 a_{\square}^2 a_2 q_2 r_{\square}^2 s_2 + 3 a_{\square}^2 b_{\square} q_{\square} q_{1,2} r_{\square}^2 - 3 \\
& a_{\square}^2 b_{\square} q_1 q_{2,2} r_{\square}^2 + 2 a_{\square}^2 b_1 p_1 q_{\square}^2 r_2 + a_{\square}^2 b_1 p_1 q_{\square}^2 s_1 - a_{\square}^2 b_2 p_1 q_{\square}^2 r_1 - 6 a_{\square} a_1 b_{\square} q_2^2 r_{\square}^2 \\
& - a_{\square} a_2^2 q_{\square} r_{\square}^2 s_2 - 3 a_{\square} b_{\square}^2 q_{\square} q_{1,2} r_{\square}^2 + 3 a_{\square} b_{\square}^2 q_1 q_{2,2} r_{\square}^2 + a_{\square}^2 b_2 p_{\square} q_{\square}^2 r_{\square} - a_{\square}^2 b_2 \\
& q_{\square}^2 r_{\square} s_{\square} + 4 a_1 b_{\square}^2 q_{\square} r_{\square} s_2^2 + a_2^2 b_{\square} q_{\square} r_{\square}^2 s_2 + 3 a_2 b_{\square}^2 q_2 r_{\square}^2 s_2 - b_{\square}^3 p_1 q_{\square} s_1 s_2 - 3 \\
& b_{\square}^3 p_1 q_2 r_{\square} s_2 + 2 b_{\square}^2 b_1 p_1 q_{\square}^2 r_2 + b_{\square}^2 b_1 p_1 q_{\square}^2 s_1 - b_{\square}^2 b_2 p_1 q_{\square}^2 r_1 - 6 a_{\square} a_2 b_{\square} q_2 r_{\square}^2 s_2 \\
& - 3 a_{\square} a_2 b_1 p_1 q_{\square}^2 r_{\square} + 2 a_{\square} a_2 b_1 q_{\square}^2 r_{\square} r_2 + a_{\square} a_2 b_1 q_{\square}^2 r_{\square} s_1 - 3 a_{\square} a_2 b_2 p_2 q_{\square} r_{\square}^2 \\
& + 3 a_{\square} b_{\square}^2 p_1 q_{\square} s_1 s_2 + 9 a_{\square} b_{\square}^2 p_1 q_2 r_{\square} s_2 - 4 a_{\square} b_{\square} b_1 p_1 q_{\square}^2 r_2 - 2 a_{\square} b_{\square} b_1 p_1 q_{\square}^2 s_1 \\
& + 2 a_{\square} b_{\square} b_2 p_1 q_{\square}^2 r_1 + a_{\square} b_1 b_2 p_1 q_{\square}^2 r_{\square} - a_1 a_2 b_{\square} q_{\square}^2 r_{\square} r_2 - a_1 a_2 b_{\square} q_{\square} q_2 r_{\square}^2 \\
& + a_1 a_2 b_1 p_{\square} q_{\square}^2 r_{\square} - a_1 a_2 b_1 q_{\square}^2 r_{\square} s_{\square} - a_1 b_{\square}^2 p_{\square} q_{\square} s_1 s_2 - 3 a_1 b_{\square}^2 p_{\square} q_2 r_{\square} s_2 + 3 a_1 \\
& b_{\square}^2 q_{\square} q_2 r_{\square} r_2 + a_1 b_{\square}^2 q_{\square} s_{\square} s_1 s_2 + 3 a_1 b_{\square}^2 q_2 r_{\square} s_{\square} s_2 + 2 a_1 b_{\square} b_1 p_{\square} q_{\square}^2 r_2 \\
& + a_1 b_{\square} b_1 p_{\square} q_{\square}^2 s_1 - a_{\square}^2 a_1 p_{\square} q_{\square} s_1 s_2 - 3 a_{\square}^2 a_1 p_{\square} q_2 r_{\square} s_2 + 3 a_{\square}^2 a_1 q_{\square} q_2 r_{\square} r_2 + \\
& a_{\square}^2 a_1 q_{\square} s_{\square} s_1 s_2 + 3 a_{\square}^2 a_1 q_2 r_{\square} s_{\square} s_2 - a_{\square}^2 a_2 p_1 q_{\square} r_{\square} s_2 + a_{\square}^2 a_2 q_{\square} r_{\square} s_1 s_2 - 3 \\
& a_{\square}^2 b_{\square} p_1 q_{\square} s_1 s_2 - 9 a_{\square}^2 b_{\square} p_1 q_2 r_{\square} s_2 + 5 a_{\square}^2 b_1 p_1 q_{\square} q_2 r_{\square} - 3 a_{\square}^2 b_2 p_1 p_2 q_{\square} r_{\square} - \\
& a_{\square}^2 b_2 p_1 q_{\square} q_1 r_{\square} + a_{\square} a_1 a_2 q_{\square}^2 r_{\square} r_2 + a_{\square} a_1 a_2 q_{\square} q_2 r_{\square}^2 - 8 a_{\square} a_1 b_{\square} q_{\square} r_{\square} s_2^2 \\
& - 2 a_{\square} a_1 b_1 p_{\square} q_{\square}^2 r_2 - a_{\square} a_1 b_1 p_{\square} q_{\square}^2 s_1 + 2 a_{\square} a_1 b_1 q_{\square}^2 r_2 s_{\square} + a_{\square} a_1 b_1 q_{\square}^2 s_{\square} s_1 \\
& - a_{\square} a_1 b_2 p_1 q_{\square}^2 r_{\square} - a_{\square}^3 q_{\square} q_{1,2} r_{\square}^2 + a_{\square}^3 q_1 q_{2,2} r_{\square}^2 + 3 a_{\square}^2 a_1 q_2^2 r_{\square}^2 + 3 a_1 b_{\square}^2 q_2^2 r_{\square}^2 + \\
& b_{\square}^3 q_{\square} q_{1,2} r_{\square}^2 - b_{\square}^3 q_1 q_{2,2} r_{\square}^2 + 4 a_1 s_{\square}^2 q_{\square} r_{\square} b_2^2 + a_1 s_{\square}^3 q_{\square} b_1 b_2 + 4 p_{\square}^2 a_1 q_{\square} r_{\square} b_2^2 - \\
& p_{\square}^3 a_1 q_{\square} b_1 b_2 - r_{\square} a_2 p_{\square} q_{\square}^2 b_1^2 + 4 r_{\square}^2 a_2^2 p_{\square} q_{\square} b_2 + r_{\square} a_2 s_{\square} q_{\square}^2 b_1^2 - 4 r_{\square}^2 a_2^2 s_{\square} q_{\square} b_2 \\
& - p_{\square} p_1 a_{\square} q_{\square}^2 b_1^2 + p_1 a_{\square} s_{\square} q_{\square}^2 b_1^2 + p_{\square} b_{\square} p_1 q_{\square}^2 b_1^2 - p_1 b_{\square} s_{\square} q_{\square}^2 b_1^2 - 2 p_{\square} s_{\square} a_1 q_{\square}^2 \\
& b_1^2 + 2 r_{\square}^2 a_1 q_{\square}^2 a_2 b_2 - 2 r_{\square}^2 q_1 a_{\square} q_{\square} a_2 b_2 + 2 r_{\square}^2 q_1 b_{\square} q_{\square} a_2 b_2 - 2 q_{\square}^2 r_1 a_{\square} r_{\square} a_2 b_2 \\
& + 2 q_{\square}^2 r_1 b_{\square} r_{\square} a_2 b_2 - 5 r_{\square} a_1 q_{\square}^2 b_1 b_2 p_{\square} + 5 r_{\square} a_1 q_{\square}^2 b_1 s_{\square} b_2 + 6 r_{\square} a_1 q_{\square}^2 b_1 s_2 a_{\square} \\
& - 6 r_{\square} a_1 q_{\square}^2 b_1 b_{\square} s_2 - 2 r_{\square} a_1 q_{\square}^2 b_2 s_1 a_{\square} + 2 r_{\square} a_1 q_{\square}^2 b_2 s_1 b_{\square} + p_1 a_{\square}^2 s_{\square} q_{\square} b_1 s_2 \\
& + p_1 a_{\square}^2 s_{\square} q_{\square} b_2 s_1 - 3 p_{\square} b_{\square}^2 p_1 r_{\square} b_2 q_2 - p_{\square}^2 b_{\square} p_1 q_{\square} b_1 b_2 - p_{\square} b_{\square}^2 p_1 q_{\square} b_1 s_2 - p_{\square}
\end{aligned}$$

$$\begin{aligned}
& b_{\square}^2 p_{\square} q_{\square} b_2 s_1 + 3 p_{\square} b_{\square}^2 s_{\square} r_{\square} b_2 q_2 - p_{\square} b_{\square} s_{\square}^2 q_{\square} b_1 b_2 + p_{\square} b_{\square}^2 s_{\square} q_{\square} b_1 s_2 + p_{\square} \\
& b_{\square}^2 s_{\square} q_{\square} b_2 s_1 - 8 p_{\square} s_{\square} a_{\square} q_{\square} r_{\square} b_2^2 + 3 a_{\square} s_{\square}^2 r_{\square} b_2 q_2 a_{\square} - 3 a_{\square} s_{\square}^2 r_{\square} b_2 q_2 b_{\square} - 2 a_{\square} \\
& s_{\square}^2 q_{\square} r_{\square} a_2 b_2 - 3 a_{\square} s_{\square}^2 q_{\square} b_1 b_2 p_{\square} + a_{\square} s_{\square}^2 q_{\square} b_1 s_2 a_{\square} - a_{\square} s_{\square}^2 q_{\square} b_1 b_{\square} s_2 + a_{\square} \\
& s_{\square}^2 q_{\square} b_2 s_1 a_{\square} - a_{\square} s_{\square}^2 q_{\square} b_2 s_1 b_{\square} + 3 p_{\square}^2 a_{\square} r_{\square} b_2 q_2 a_{\square} - 3 p_{\square}^2 a_{\square} r_{\square} b_2 q_2 b_{\square} - 2 \\
& p_{\square}^2 a_{\square} q_{\square} r_{\square} a_2 b_2 + 3 p_{\square}^2 a_{\square} q_{\square} b_1 s_{\square} b_2 + p_{\square}^2 a_{\square} q_{\square} b_1 s_2 a_{\square} - p_{\square}^2 a_{\square} q_{\square} b_1 b_{\square} s_2 + \\
& p_{\square}^2 a_{\square} q_{\square} b_2 s_1 a_{\square} - p_{\square}^2 a_{\square} q_{\square} b_2 s_1 b_{\square} - 3 r_{\square}^2 a_2 p_{\square} b_2 q_2 a_{\square} + 3 r_{\square}^2 a_2 p_{\square} b_2 q_2 b_{\square} + r_{\square} a_2 \\
& p_{\square}^2 q_{\square} b_1 b_2 + 3 r_{\square}^2 a_2 s_{\square} b_2 q_2 a_{\square} - 3 r_{\square}^2 a_2 s_{\square} b_2 q_2 b_{\square} + r_{\square} a_2 s_{\square}^2 q_{\square} b_1 b_2 - 3 p_{\square} p_1 \\
& a_{\square}^2 r_{\square} b_2 q_2 + p_{\square}^2 p_1 a_{\square} q_{\square} b_1 b_2 - p_{\square} p_1 a_{\square}^2 q_{\square} b_1 s_2 - p_{\square} p_1 a_{\square}^2 q_{\square} b_2 s_1 + 3 p_{\square} \\
& a_{\square}^2 s_{\square} r_{\square} b_2 q_2 + p_{\square} a_{\square} s_{\square}^2 q_{\square} b_1 b_2)
\end{aligned}$$

**D2** > [smb12(%), smb13(%)]

$$\left[ \frac{(-3 r_{\square}^2 a_{\square}^2 q_{\square} b_{\square} + 3 r_{\square}^2 a_{\square} q_{\square} b_{\square}^2 + r_{\square}^2 a_{\square}^3 q_{\square} - r_{\square}^2 b_{\square}^3 q_{\square}) q_{2,2}}{q_{\square} (a_{\square} - b_{\square}) r_{\square}^2 (b_{\square}^2 + a_{\square}^2 - 2 a_{\square} b_{\square})}, \right. \\
\left. \frac{(-a_{\square}^3 q_{\square} r_{\square}^2 + b_{\square}^3 q_{\square} r_{\square}^2 + 3 a_{\square}^2 b_{\square} q_{\square} r_{\square}^2 - 3 a_{\square} b_{\square}^2 q_{\square} r_{\square}^2) q_{1,2,2}}{q_{\square} (a_{\square} - b_{\square}) r_{\square}^2 (b_{\square}^2 + a_{\square}^2 - 2 a_{\square} b_{\square})} \right] \quad (75)$$

**D2** > JIC[12]

$$\begin{aligned}
r_{1,2} = & \frac{1}{(a_{\square} - b_{\square})^2 q_{\square} r_{\square}} (p_{\square} r_{\square}^2 a_2 b_2 + r_{\square} a_{\square} s_{\square}^2 b_2 + r_{\square} a_{\square}^2 s_2 p_1 + r_{\square} b_{\square}^2 s_2 p_1 - r_{\square} s_{\square} a_2 b_2 \\
& - r_{\square}^2 a_{\square} a_2 s_2 - r_{\square}^2 a_{\square} b_2 q_1 + r_{\square}^2 b_{\square} a_2 s_2 + r_{\square}^2 b_{\square} b_2 q_1 + q_{\square} r_1 r_2 a_{\square}^2 + q_{\square} r_1 r_2 b_{\square}^2 + \\
& p_{\square}^2 r_{\square} b_2 a_1 + q_{\square} r_{\square} b_1 a_1 p_{\square} - q_{\square} r_{\square} b_1 s_{\square} a_1 + b_{\square} r_{\square} q_{\square} b_1 p_1 - a_{\square} r_{\square} q_{\square} b_1 p_1 \\
& - 2 p_{\square} r_{\square} s_{\square} b_2 a_1 - p_{\square} r_{\square} a_1 s_2 a_{\square} + p_{\square} r_{\square} a_1 b_{\square} s_2 - p_{\square} r_{\square} b_2 p_1 a_{\square} + p_{\square} r_{\square} b_2 b_{\square} p_1 \\
& + r_{\square} p_1 a_{\square} s_{\square} b_2 - r_{\square} p_1 b_{\square} s_{\square} b_2 + r_{\square} a_1 s_{\square} s_2 a_{\square} - 2 r_{\square} p_1 a_{\square} b_{\square} s_2 - r_{\square} a_1 s_{\square} b_{\square} s_2 \\
& - q_{\square} r_1 a_{\square} r_{\square} b_2 - 2 q_{\square} r_1 a_{\square} r_2 b_{\square} + q_{\square} r_1 b_{\square} r_{\square} b_2)
\end{aligned} \quad (76)$$

**D2** > simplify(subs(QQQ=0, SQEP[11]))

$$\begin{aligned}
r_{1,2} = & \frac{1}{q_{\square} r_{\square} (b_{\square}^2 + a_{\square}^2 - 2 a_{\square} b_{\square})} (p_{\square} r_{\square}^2 a_2 b_2 + r_{\square} a_{\square} s_{\square}^2 b_2 + r_{\square} a_{\square}^2 s_2 p_1 + r_{\square} b_{\square}^2 s_2 p_1 - \\
& r_{\square}^2 s_{\square} a_2 b_2 - r_{\square}^2 a_{\square} a_2 s_2 - r_{\square}^2 a_{\square} b_2 q_1 + r_{\square}^2 b_{\square} a_2 s_2 + r_{\square}^2 b_{\square} b_2 q_1 + q_{\square} r_1 r_2 a_{\square}^2 \\
& + q_{\square} r_1 r_2 b_{\square}^2 + p_{\square}^2 r_{\square} b_2 a_1 + q_{\square} r_{\square} b_1 a_1 p_{\square} - q_{\square} r_{\square} b_1 s_{\square} a_1 + b_{\square} r_{\square} q_{\square} b_1 p_1 \\
& - a_{\square} r_{\square} q_{\square} b_1 p_1 - 2 p_{\square} r_{\square} s_{\square} b_2 a_1 - p_{\square} r_{\square} a_1 s_2 a_{\square} + p_{\square} r_{\square} a_1 b_{\square} s_2 - p_{\square} r_{\square} b_2 p_1 a_{\square} \\
& + p_{\square} r_{\square} b_2 b_{\square} p_1 + r_{\square} p_1 a_{\square} s_{\square} b_2 - r_{\square} p_1 b_{\square} s_{\square} b_2 + r_{\square} a_1 s_{\square} s_2 a_{\square} - 2 r_{\square} p_1 a_{\square} b_{\square} s_2 \\
& - r_{\square} a_1 s_{\square} b_{\square} s_2 - q_{\square} r_1 a_{\square} r_{\square} b_2 - 2 q_{\square} r_1 a_{\square} r_2 b_{\square} + q_{\square} r_1 b_{\square} r_{\square} b_2)
\end{aligned} \quad (77)$$

**D2** > simplify(subs(subs(QQQ=0, SQEP[11]), r1,2) - subs(JIC[12], r1,2))

**D2 >**

Similar story happens to 3 other compatibility equations involving q and r:  $(q_{\{1,1\}})_2 = (q_{\{1,2\}})_1$ ,  $(r_{\{1,1\}})_2 = (r_{\{1,2\}})_1$ ,  $(r_{\{1,2\}})_2 = (r_{\{2,2\}})_1$ .

Now we add the 16th equation and re-start. I do not introduce new notations since SQE+(new eqn)=JIC.

$$\mathbf{J2} > \text{simplify}(\text{subs}(JIC, \text{TotalDiff}(\text{subs}(JIC, a_{1,1}), 2) - \text{TotalDiff}(\text{subs}(JIC, a_{1,2}), 1))) \quad (79)$$

$$\mathbf{J2} > \text{simplify}(\text{subs}(JIC, \text{TotalDiff}(\text{subs}(JIC, a_{1,2}), 2) - \text{TotalDiff}(\text{subs}(JIC, a_{2,2}), 1))) \quad (80)$$

$$\mathbf{J2} > \text{simplify}(\text{subs}(JIC, \text{TotalDiff}(\text{subs}(JIC, b_{1,1}), 2) - \text{TotalDiff}(\text{subs}(JIC, b_{1,2}), 1))) \quad (81)$$

$$\mathbf{J2} > \text{simplify}(\text{subs}(JIC, \text{TotalDiff}(\text{subs}(JIC, b_{1,2}), 2) - \text{TotalDiff}(\text{subs}(JIC, b_{2,2}), 1))) \quad (82)$$

$$\mathbf{J2} > \text{simplify}(\text{subs}(JIC, \text{TotalDiff}(\text{subs}(JIC, p_{1,1}), 2) - \text{TotalDiff}(\text{subs}(JIC, p_{1,2}), 1))) \quad (83)$$

$$\mathbf{J2} > \text{simplify}(\text{subs}(JIC, \text{TotalDiff}(\text{subs}(JIC, p_{1,2}), 2) - \text{TotalDiff}(\text{subs}(JIC, p_{2,2}), 1))) \quad (84)$$

$$\mathbf{J2} > \text{simplify}(\text{subs}(JIC, \text{TotalDiff}(\text{subs}(JIC, s_{1,1}), 2) - \text{TotalDiff}(\text{subs}(JIC, s_{1,2}), 1))) \quad (85)$$

$$\mathbf{J2} > \text{simplify}(\text{subs}(JIC, \text{TotalDiff}(\text{subs}(JIC, s_{1,2}), 2) - \text{TotalDiff}(\text{subs}(JIC, s_{2,2}), 1))) \quad (86)$$

**D2 >**

**D2 >**

Here are the problematic compatibility conditions:

$$\mathbf{J2} > \text{NEq1} := \text{simplify}(\text{subs}(JIC, \text{TotalDiff}(\text{subs}(JIC, q_{1,1}), 2) - \text{TotalDiff}(\text{subs}(JIC, q_{1,2}), 1))) :$$

$$\mathbf{D2} > \text{simplify}([\text{smb12}(\text{NEq1}), \text{smb13}(\text{NEq1})]) \quad \left[ -\frac{q_{1,1} q_2}{q_{[]}}, q_{1,1,2} \right] \quad (87)$$

$$\mathbf{J2} > \text{NEq2} := \text{simplify}(\text{subs}(JIC, \text{TotalDiff}(\text{subs}(JIC, q_{1,2}), 2) - \text{TotalDiff}(\text{subs}(JIC, q_{2,2}), 1))) :$$

$$\mathbf{J2} > \text{simplify}([\text{smb12}(\text{NEq2}), \text{smb13}(\text{NEq2})]) \quad \left[ \frac{q_{2,2} q_1}{q_{[]}}, -q_{1,2,2} \right] \quad (88)$$

$$\mathbf{J2} > \text{NEq3} := \text{simplify}(\text{subs}(JIC, \text{TotalDiff}(\text{subs}(JIC, r_{1,1}), 2) - \text{TotalDiff}(\text{subs}(JIC, r_{1,2}), 1))) :$$

$$\mathbf{J2} > \text{simplify}([\text{smb12}(\text{NEq3}), \text{smb13}(\text{NEq3})]) \quad (89)$$

$$\left[ \frac{q_{1,1} r_{[]} q_2}{q_{[]}^2}, -\frac{q_{1,1,2} r_{[]}}{q_{[]}} \right] \quad (89)$$

**J2** >  $NEq4 := \text{simplify}(\text{subs}(JIC, \text{TotalDiff}(\text{subs}(JIC, r_{1,2}), 2) - \text{TotalDiff}(\text{subs}(JIC, r_{2,2}), 1))) :$

**J2** >  $\text{simplify}([\text{smb12}(NEq4), \text{smb13}(NEq4)])$

$$\left[ -\frac{q_{2,2} r_{[]} q_1}{q_{[]}^2}, \frac{q_{1,2,2} r_{[]}}{q_{[]}} \right] \quad (90)$$

However since the 3rd ord jets are involved, we have to take only those combinations of these that are of ord=2

**J2** >  $\text{simplify}(r_{[]} \cdot NEq1 + q_{[]} \cdot NEq3)$

0 (91)

**J2** >  $\text{simplify}(r_{[]} \cdot NEq2 + q_{[]} \cdot NEq4)$

0 (92)

This means precisely that the system is in involution!

**J2** >

Conclusion: Integrability => EW condition.  
 EW condition => either integrability or that the system has constant symbol (= constant coeffs of dispersion relations),  
 in which case integrability = linearizability

>  
 >
