# Supplementary material for: Dispersionless integrable systems in 3D and Einstein-Weyl geometry
Source: arXiv:1208.2728 ancillary file (2013-05-09)
Supplement: Supplementary file 10 [file BKEF-2012-IV-2D_component_quasilinear_linearization.pdf]

This is the worksheet accompanying the paper E.Ferapontov & B.Kruglikov "Dispersionless integrable systems in 3D and Einstein-Weyl geometry".

The file ran on **Maple** version 16, the package **DifferentialGeometry** was used.

```
> restart : with(DifferentialGeometry) : with(Tensor) : with(Tools) : with(JetCalculus) :
with(LinearAlgebra) : with(PDEtools, D_Dx, declare, ToJet, FromJet) :
```

We consider the 2 component systems of hydrodynamic type and study it's linearization via vanishing of the Cotton tensor of the linearization conformal structure

```
> alias(f=f(u2,2, u2,3, u3,3, u1,2, u1,3)) : declare(a(u[], v[])) : declare(b(u[], v[])) :
declare(p(u[], v[])) : declare(q(u[], v[])) : declare(r(u[], v[])) : declare(s(u[], v[])) :
```

$a(u_{[]} , v_{[]})$  will now be displayed as  $a$

$b(u_{[]} , v_{[]})$  will now be displayed as  $b$

$p(u_{[]} , v_{[]})$  will now be displayed as  $p$

$q(u_{[]} , v_{[]})$  will now be displayed as  $q$

$r(u_{[]} , v_{[]})$  will now be displayed as  $r$

$s(u_{[]} , v_{[]})$  will now be displayed as  $s$

(1)

```
> DGsetup([t, x, y], [u, v], J2, 3) :
```

```
> F := u1 + a(u[], v[])) · u2 + p(u[], v[])) · u3 + q(u[], v[])) · v3;
G := v1 + b(u[], v[])) · v2 + r(u[], v[])) · u3 + s(u[], v[])) · v3;
F := u1 + a u2 + p u3 + q v3
```

$G := v_1 + b v_2 + r u_3 + s v_3$

(2)

```
> DR := (diff(F, u1) · ξ1 + diff(F, u2) · ξ2 + diff(F, u3) · ξ3) · (diff(G, v1) · ξ1 + diff(G, v2) · ξ2
+ diff(G, v3) · ξ3) - (diff(F, v1) · ξ1 + diff(F, v2) · ξ2 + diff(F, v3) · ξ3) · (diff(G, u1) · ξ1
+ diff(G, u2) · ξ2 + diff(G, u3) · ξ3)
```

$DR := (\xi_1 + a \xi_2 + p \xi_3) (\xi_1 + b \xi_2 + s \xi_3) - q \xi_3^2 r$

(3)

```
> A := 2 · Matrix( [[ [ 1/2 diff(DR, ξ1, ξ1), 1/2 diff(DR, ξ1, ξ2), 1/2 diff(DR, ξ1, ξ3) ], [ 1/2 diff(DR,
ξ1, ξ2), 1/2 diff(DR, ξ2, ξ2), 1/2 diff(DR, ξ2, ξ3) ], [ 1/2 diff(DR, ξ1, ξ3), 1/2 diff(DR, ξ2, ξ3),
1/2 diff(DR, ξ3, ξ3) ] ] ] )
```

$A := \begin{bmatrix} 2 & b+a & s+p \\ b+a & 2ab & as+bp \\ s+p & as+bp & 2ps-2qr \end{bmatrix}$

(4)

```
> AA := expand(MatrixInverse(A)); factor(Determinant(A))
```

$$AA := \left[ \left[ -\frac{1}{2} \frac{-2aspb + 4abqr + a^2s^2 + p^2b^2}{qr(-2ab + b^2 + a^2)}, \right. \right. \\ \left. \frac{1}{2} \frac{-bps + 2bqr - a ps + 2aqr + as^2 + p^2b}{qr(-2ab + b^2 + a^2)}, \frac{1}{2} \frac{-pb + as}{(a-b)qr} \right], \\ \left[ \frac{1}{2} \frac{-bps + 2bqr - a ps + 2aqr + as^2 + p^2b}{qr(-2ab + b^2 + a^2)}, -\frac{1}{2} \frac{-2ps + 4qr + s^2 + p^2}{qr(-2ab + b^2 + a^2)}, \right. \\ \left. -\frac{1}{2} \frac{-p + s}{(a-b)qr} \right], \\ \left[ \frac{1}{2} \frac{-pb + as}{(a-b)qr}, -\frac{1}{2} \frac{-p + s}{(a-b)qr}, -\frac{1}{2qr} \right] \\ \left. \right] \\ 2qr(a-b)^2 \quad (5)$$

> *AM := simplify(Adjoint(A))*

$$AM := \left[ \left[ 2aspb - 4abqr - a^2s^2 - p^2b^2, -bps + 2bqr - a ps + 2aqr + as^2 + p^2b, \right. \right. \\ \left. -bas + pb^2 + a^2s - apb \right], \\ \left[ -bps + 2bqr - a ps + 2aqr + as^2 + p^2b, 2ps - 4qr - s^2 - p^2, -as - bp + sb \right. \\ \left. + ap \right], \\ \left[ -bas + pb^2 + a^2s - apb, -as - bp + sb + ap, 2ab - b^2 - a^2 \right] \quad (6)$$

>

>

Here A is the matrix of the linearized operator (bivector=metric with upper indices),  
AA - the inverse (metric, which we remember is defined only up to conformal rescaling)  
and AJ=AM=AdA the adjoint matrix (which we use as a representative for the conformal class)

>

> *aA := [TotalDiff(A[1,1],1) + TotalDiff(A[1,2],2) + TotalDiff(A[1,3],3), TotalDiff(A[2,1],1) + TotalDiff(A[2,2],2) + TotalDiff(A[2,3],3), TotalDiff(A[3,1],1) + TotalDiff(A[3,2],2) + TotalDiff(A[3,3],3)] :*

> *ω := 2·[AA[1,1]·aA[1] + AA[1,2]·aA[2] + AA[1,3]·aA[3], AA[2,1]·aA[1] + AA[2,2]·aA[2] + AA[2,3]·aA[3], AA[3,1]·aA[1] + AA[3,2]·aA[2] + AA[3,3]·aA[3]] :*

>

> *DepVars := [u(t,x,y), v(t,x,y)] : AJ := simplify(FromJet(AM, DepVars)) :*

>

> *DGsetup([t,x,y],M) :*

> *g := evalDG(AJ[1,1]·dt&tdt + AJ[1,2]·dt&tdx + AJ[1,3]·dt&tdy + AJ[2,1]·dx&tdt + AJ[2,2]·dx&tdx + AJ[2,3]·dx&tdy + AJ[3,1]·dy&tdt + AJ[3,2]·dy&tdx + AJ[3,3]·dy&tdy) :*

>

> *smb13 := Z→add(add(add(diff(Z,u[p,q,r])·u[p,q,r] + diff(Z,v[p,q,r])·v[p,q,r],r=q..3),q=p..3),p=1..3) :*

```

> G2 := (i, j, k, l) → diff (AA[i, j], u[]) · TotalDiff (u[], [k, l]) + diff (AA[i, j], v[])
    · TotalDiff (v[], [k, l]) :
=
> G3 := (i, j, k, l, m) → diff (AA[i, j], u[]) · TotalDiff (u[], [k, l, m]) + diff (AA[i, j], v[])
    · TotalDiff (v[], [k, l, m]) :
=
> Ric := (i, j) →  $\frac{1}{2} \cdot \text{add}(\text{add}(A[k, l] \cdot (G2(i, j, k, l) + G2(k, l, i, j) - G2(i, k, j, l) - G2(j, l, i, k)), l = 1 \dots 3), k = 1 \dots 3) :$ 
=
> Ric2 := (i, j, m) →  $\frac{1}{2} \cdot \text{add}(\text{add}(A[k, l] \cdot (G3(i, j, k, l, m) + G3(k, l, i, j, m) - G3(i, k, j, l, m) - G3(j, l, i, k, m)), l = 1 \dots 3), k = 1 \dots 3) :$ 
> Sc := add(add(A[i, j] · Ric(i, j), j = 1 .. 3), i = 1 .. 3) :
> Sc2 := k → add(add(A[i, j] · Ric2(i, j, k), j = 1 .. 3), i = 1 .. 3) :
> Cot := (i, j, t) → smbl3  $\left( Ric2(i, j, t) - Ric2(i, t, j) - \frac{1}{4} AA[i, j] \cdot Sc2(t) + \frac{1}{4} AA[i, t] \cdot Sc2(j) \right) :$ 

```

```

>
>
> # Here I define the symbol of the Cotton tensor - it has order 3 in the entries of the metric,
    so order 1 in the functions a(u, v), b(u, v), p(u, v), q(u, v), r(u, v), s(u, v) and order 3
    in u, v.
>

```

```

M > de := DifferentialEquationData([F, G], [u1, v1])
    de := [ {u1, v1}, [u1 + a u2 + p u3 + q v3, v1 + b v2 + r u3 + s v3] ]

```

(7)

```

M > DE2 := Prolong(de, 2) :
M > alpha := Transformation(DE2) :
E >
E > simplify(Pullback(alpha, v[1, 1, 3]))
>

```

```

> Res112 := simplify(smbl3(2 Determinant(A) · Pullback(alpha, Cot(1, 1, 2)))) :
> Res113 := simplify(smbl3(2 Determinant(A) · Pullback(alpha, Cot(1, 1, 3)))) :
> Res123 := simplify(smbl3(2 Determinant(A) · Pullback(alpha, Cot(1, 2, 3)))) :
> Res212 := simplify(smbl3(2 Determinant(A) · Pullback(alpha, Cot(2, 1, 2)))) :
> Res213 := simplify(smbl3(2 Determinant(A) · Pullback(alpha, Cot(2, 1, 3)))) :
> Res223 := simplify(smbl3(2 Determinant(A) · Pullback(alpha, Cot(2, 2, 3)))) :
> Res312 := simplify(smbl3(2 Determinant(A) · Pullback(alpha, Cot(3, 1, 2)))) :
> Res313 := simplify(smbl3(2 Determinant(A) · Pullback(alpha, Cot(3, 1, 3)))) :
> Res323 := simplify(smbl3(2 Determinant(A) · Pullback(alpha, Cot(3, 2, 3)))) :

```

Let us deduce some corollaries

```

J2 > simplify  $\left( \frac{\text{factor}(\text{diff}(Res323, u[2, 2, 2]))}{(a - b)^3} \right)$ 

```

$a_u$

(8)

$$\mathbf{J2} > \text{simplify}\left(-\frac{\text{factor}(\text{diff}(\text{Res323}, v[2, 2, 2]))}{(a-b)^3}\right) b_v[] \quad (9)$$

$$\mathbf{J2} > \text{simplify}\left(\frac{\text{factor}(\text{diff}(\text{Res323}, u[2, 2, 3]))}{(a-b)^2}\right) r a_v[] + r b_v[] + 3 p a_u[] - 3 a_u[] s \quad (10)$$

$$\mathbf{J2} > \text{simplify}\left(\frac{\text{factor}(\text{diff}(\text{Res323}, v[2, 2, 3]))}{(a-b)^2}\right) q a_u[] + q b_u[] - 3 p b_v[] + 3 s b_v[] \quad (11)$$

Thus  $a, b$  are constants ...

$$\mathbf{J2} > \text{simplify}\left(-\frac{\text{factor}(\text{diff}(\text{Res223}, u[2, 2, 2]))}{(a-b)^3}\right) p_u[] \quad (12)$$

$$\mathbf{J2} > \text{simplify}\left(\frac{\text{factor}(\text{diff}(\text{Res223}, v[2, 2, 2]))}{(a-b)^3}\right) s_v[] \quad (13)$$

... **and**  $p = p(v), s = s(u)$ . It is **not** easy to observe the other identities at the moment, so we substitute these data **and** check again

>

> restart : with(DifferentialGeometry) : with(Tensor) : with(Tools) : with(JetCalculus) :  
with(LinearAlgebra) : with(PDEtools, D\_Dx, declare, ToJet, FromJet) :

> alias(f=f(u<sub>2,2</sub>, u<sub>2,3</sub>, u<sub>3,3</sub>, u<sub>1,2</sub>, u<sub>1,3</sub>)) : declare(p(v<sub>[]</sub>)) : declare(q(u<sub>[]</sub>, v<sub>[]</sub>)) :  
declare(r(u<sub>[]</sub>, v<sub>[]</sub>)) : declare(s(u<sub>[]</sub>)) :

$p(v[]) \text{ will now be displayed as } p$

$q(u[], v[]) \text{ will now be displayed as } q$

$r(u[], v[]) \text{ will now be displayed as } r$

$s(u[]) \text{ will now be displayed as } s$

(14)

> DGsetup([t, x, y], [u, v], J2, 3) :

> F := u<sub>1</sub> + a·u<sub>2</sub> + p(v<sub>[]</sub>)·u<sub>3</sub> + q(u<sub>[]</sub>, v<sub>[]</sub>)·v<sub>3</sub>;

G := v<sub>1</sub> + b·v<sub>2</sub> + r(u<sub>[]</sub>, v<sub>[]</sub>)·u<sub>3</sub> + s(u<sub>[]</sub>)·v<sub>3</sub>;

$F := u_1 + a u_2 + p u_3 + q v_3$

$G := v_1 + b v_2 + r u_3 + s v_3$

(15)

> DR := (diff(F, u<sub>1</sub>)·ξ<sub>1</sub> + diff(F, u<sub>2</sub>)·ξ<sub>2</sub> + diff(F, u<sub>3</sub>)·ξ<sub>3</sub>)·(diff(G, v<sub>1</sub>)·ξ<sub>1</sub> + diff(G, v<sub>2</sub>)·ξ<sub>2</sub>

$$+ \text{diff}(G, v_3) \cdot \xi_3) - (\text{diff}(F, v_1) \cdot \xi_1 + \text{diff}(F, v_2) \cdot \xi_2 + \text{diff}(F, v_3) \cdot \xi_3) \cdot (\text{diff}(G, u_1) \cdot \xi_1 + \text{diff}(G, u_2) \cdot \xi_2 + \text{diff}(G, u_3) \cdot \xi_3)$$

$$DR := (\xi_1 + a \xi_2 + p \xi_3) (\xi_1 + b \xi_2 + s \xi_3) - q \xi_3^2 r \quad (16)$$

$$> A := 2 \cdot \text{Matrix} \left( \left[ \left[ \frac{1}{2} \text{diff}(DR, \xi_1, \xi_1), \frac{1}{2} \text{diff}(DR, \xi_1, \xi_2), \frac{1}{2} \text{diff}(DR, \xi_1, \xi_3) \right], \left[ \frac{1}{2} \text{diff}(DR, \xi_1, \xi_2), \frac{1}{2} \text{diff}(DR, \xi_2, \xi_2), \frac{1}{2} \text{diff}(DR, \xi_2, \xi_3) \right], \left[ \frac{1}{2} \text{diff}(DR, \xi_1, \xi_3), \frac{1}{2} \text{diff}(DR, \xi_2, \xi_3), \frac{1}{2} \text{diff}(DR, \xi_3, \xi_3) \right] \right] \right)$$

$$A := \begin{bmatrix} 2 & b+a & s+p \\ b+a & 2ab & as+pb \\ s+p & as+pb & 2ps-2qr \end{bmatrix} \quad (17)$$

$$> AA := \text{expand}(\text{MatrixInverse}(A)); \text{factor}(\text{Determinant}(A))$$

$$AA := \left[ \left[ -\frac{1}{2} \frac{-2aspb + 4abqr + a^2s^2 + p^2b^2}{qr(-2ab + b^2 + a^2)}, \frac{1}{2} \frac{-bps + 2bqr - aps + 2aqr + a^2s^2 + p^2b}{qr(-2ab + b^2 + a^2)}, \frac{1}{2} \frac{as - pb}{(a-b)qr} \right], \left[ \frac{1}{2} \frac{-bps + 2bqr - aps + 2aqr + a^2s^2 + p^2b}{qr(-2ab + b^2 + a^2)}, -\frac{1}{2} \frac{-2ps + 4qr + s^2 + p^2}{qr(-2ab + b^2 + a^2)}, -\frac{1}{2} \frac{s-p}{(a-b)qr} \right], \left[ \frac{1}{2} \frac{as - pb}{(a-b)qr}, -\frac{1}{2} \frac{s-p}{(a-b)qr}, -\frac{1}{2qr} \right] \right]$$

$$2qr(a-b)^2 \quad (18)$$

$$> AM := \text{simplify}(\text{Adjoint}(A))$$

$$AM := \left[ [2aspb - 4abqr - a^2s^2 - p^2b^2, -bps + 2bqr - aps + 2aqr + a^2s^2 + p^2b, -bas + pb^2 + a^2s - apb], [-bps + 2bqr - aps + 2aqr + a^2s^2 + p^2b, 2ps - 4qr - s^2 - p^2, -as - pb + sb + pa], [-bas + pb^2 + a^2s - apb, -as - pb + sb + pa, 2ab - b^2 - a^2] \right] \quad (19)$$

$$> \text{smbl3} := Z \rightarrow \text{add}(\text{add}(\text{add}(\text{diff}(Z, u[p, q, r]) \cdot u[p, q, r] + \text{diff}(Z, v[p, q, r]) \cdot v[p, q, r], r = q \dots 3), q = p \dots 3), p = 1 \dots 3) :$$

$$> G2 := (i, j, k, l) \rightarrow \text{diff}(AA[i, j], u_{[ ]}) \cdot \text{TotalDiff}(u_{[ ]}, [k, l]) + \text{diff}(AA[i, j], v_{[ ]}) \cdot \text{TotalDiff}(v_{[ ]}, [k, l]) :$$

$$> G3 := (i, j, k, l, m) \rightarrow \text{diff}(AA[i, j], u_{[ ]}) \cdot \text{TotalDiff}(u_{[ ]}, [k, l, m]) + \text{diff}(AA[i, j], v_{[ ]})$$

$\cdot TotalDiff(v_{[]}, [k, l, m]) :$

$> Ric := (i, j) \rightarrow \frac{1}{2} \cdot add(add(A[k, l] \cdot (G2(i, j, k, l) + G2(k, l, i, j) - G2(i, k, j, l) - G2(j, l, i, k)), l = 1 \dots 3), k = 1 \dots 3) :$

$> Ric2 := (i, j, m) \rightarrow \frac{1}{2} \cdot add(add(A[k, l] \cdot (G3(i, j, k, l, m) + G3(k, l, i, j, m) - G3(i, k, j, l, m) - G3(j, l, i, k, m)), l = 1 \dots 3), k = 1 \dots 3) :$

$> Sc := add(add(A[i, j] \cdot Ric(i, j), j = 1 \dots 3), i = 1 \dots 3) :$

$> Sc2 := k \rightarrow add(add(A[i, j] \cdot Ric2(i, j, k), j = 1 \dots 3), i = 1 \dots 3) :$

$> Cot := (i, j, t) \rightarrow smbl3\left(Ric2(i, j, t) - Ric2(i, t, j) - \frac{1}{4}AA[i, j] \cdot Sc2(t) + \frac{1}{4}AA[i, t] \cdot Sc2(j)\right) :$

**M**  $> de := DifferentialEquationData([F, G], [u_1, v_1])$

$de := [\{u_1, v_1\}, [u_1 + a u_2 + p u_3 + q v_3, v_1 + b v_2 + r u_3 + s v_3]]$

(20)

**M**  $> DE2 := Prolong(de, 2) :$

**M**  $> alpha := Transformation(DE2) :$

$> Res112 := simplify(smbl3(2 Determinant(A) \cdot Pullback(alpha, Cot(1, 1, 2)))) :$

$> Res113 := simplify(smbl3(2 Determinant(A) \cdot Pullback(alpha, Cot(1, 1, 3)))) :$

$> Res123 := simplify(smbl3(2 Determinant(A) \cdot Pullback(alpha, Cot(1, 2, 3)))) :$

$> Res212 := simplify(smbl3(2 Determinant(A) \cdot Pullback(alpha, Cot(2, 1, 2)))) :$

$> Res213 := simplify(smbl3(2 Determinant(A) \cdot Pullback(alpha, Cot(2, 1, 3)))) :$

$> Res223 := simplify(smbl3(2 Determinant(A) \cdot Pullback(alpha, Cot(2, 2, 3)))) :$

$> Res312 := simplify(smbl3(2 Determinant(A) \cdot Pullback(alpha, Cot(3, 1, 2)))) :$

$> Res313 := simplify(smbl3(2 Determinant(A) \cdot Pullback(alpha, Cot(3, 1, 3)))) :$

$> Res323 := simplify(smbl3(2 Determinant(A) \cdot Pullback(alpha, Cot(3, 2, 3)))) :$

*Let us deduce some corollaries*

$>$

$> simplify\left(-\frac{factor(diff(Res323, u[2, 3, 3]))}{(a-b)^2}\right)$

$q r_{u[]} + q_{u[]} r$

(21)

$> simplify\left(-\frac{factor(diff(Res323, v[2, 3, 3]))}{(a-b)^2}\right)$

$q r_{v[]} + q_{v[]} r$

(22)

$> simplify\left(-\frac{factor(diff(Res223, u[2, 2, 3]) - 2 \cdot diff(Res323, u[2, 3, 3]))}{(a-b)^2}\right)$

$r p_{v[]}$

(23)

$> simplify\left(-\frac{factor(diff(Res223, v[2, 2, 3]) - 2 \cdot diff(Res323, v[2, 3, 3]))}{(a-b)^2}\right)$

(24)

$$q s_{u_{[]}} \quad (24)$$

Thus  $p, s$  are constants **and** the product  $q \cdot r$  is constant too (but **not** individual  $q$  **and**  $r$ )  
. Let us again substitute this **and** run anew

>

> restart : with(DifferentialGeometry) : with(Tensor) : with(Tools) : with(JetCalculus) :  
with(LinearAlgebra) : with(PDEtools, D\_Dx, declare, ToJet, FromJet) :

> alias(f=f(u<sub>2,2</sub>, u<sub>2,3</sub>, u<sub>3,3</sub>, u<sub>1,2</sub>, u<sub>1,3</sub>)) : declare(q(u<sub>[]</sub>, v<sub>[])) :</sub>

$q(u_{[]}, v_{[]})$  will now be displayed as  $q$  (25)

> DGsetup([t, x, y], [u, v], J2, 3) :

> F := u<sub>1</sub> + a·u<sub>2</sub> + p·u<sub>3</sub> + q(u<sub>[]</sub>, v<sub>[]))·v<sub>3</sub>;</sub>

$$G := v_1 + b \cdot v_2 + \frac{r}{q(u_{[]}, v_{[]})} \cdot u_3 + s \cdot v_3;$$

$$F := u_1 + a u_2 + p u_3 + q v_3$$

$$G := v_1 + b v_2 + \frac{r u_3}{q} + s v_3 \quad (26)$$

> DR := (diff(F, u<sub>1</sub>)·ξ<sub>1</sub> + diff(F, u<sub>2</sub>)·ξ<sub>2</sub> + diff(F, u<sub>3</sub>)·ξ<sub>3</sub>)·(diff(G, v<sub>1</sub>)·ξ<sub>1</sub> + diff(G, v<sub>2</sub>)·ξ<sub>2</sub>  
+ diff(G, v<sub>3</sub>)·ξ<sub>3</sub>) - (diff(F, v<sub>1</sub>)·ξ<sub>1</sub> + diff(F, v<sub>2</sub>)·ξ<sub>2</sub> + diff(F, v<sub>3</sub>)·ξ<sub>3</sub>)·(diff(G, u<sub>1</sub>)·ξ<sub>1</sub>  
+ diff(G, u<sub>2</sub>)·ξ<sub>2</sub> + diff(G, u<sub>3</sub>)·ξ<sub>3</sub>)

$$DR := (\xi_1 + a \xi_2 + p \xi_3) (\xi_1 + b \xi_2 + s \xi_3) - \xi_3^2 r \quad (27)$$

> A := 2·Matrix([ [ 1/2 diff(DR, ξ<sub>1</sub>, ξ<sub>1</sub>), 1/2 diff(DR, ξ<sub>1</sub>, ξ<sub>2</sub>), 1/2 diff(DR, ξ<sub>1</sub>, ξ<sub>3</sub>) ], [ 1/2 diff(DR,  
ξ<sub>1</sub>, ξ<sub>2</sub>), 1/2 diff(DR, ξ<sub>2</sub>, ξ<sub>2</sub>), 1/2 diff(DR, ξ<sub>2</sub>, ξ<sub>3</sub>) ], [ 1/2 diff(DR, ξ<sub>1</sub>, ξ<sub>3</sub>), 1/2 diff(DR, ξ<sub>2</sub>, ξ<sub>3</sub>),  
1/2 diff(DR, ξ<sub>3</sub>, ξ<sub>3</sub>) ] ] ] )

$$A := \begin{bmatrix} 2 & b+a & s+p \\ b+a & 2ab & as+pb \\ s+p & as+pb & 2ps-2r \end{bmatrix} \quad (28)$$

> AA := expand(MatrixInverse(A)); factor(Determinant(A))

$$AA := \left[ \left[ -\frac{1}{2} \frac{-2aspb + 4abr + a^2s^2 + p^2b^2}{r(-2ab + b^2 + a^2)}, \right. \right. \\
\left. -\frac{1}{2} \frac{bps - 2br + aps - 2ar - as^2 - p^2b}{r(-2ab + b^2 + a^2)}, \frac{1}{2} \frac{as - pb}{(-b + a)r} \right], \\
\left[ -\frac{1}{2} \frac{bps - 2br + aps - 2ar - as^2 - p^2b}{r(-2ab + b^2 + a^2)}, -\frac{1}{2} \frac{-2ps + 4r + s^2 + p^2}{r(-2ab + b^2 + a^2)}, \right]$$

$$\left[ \frac{1}{2} \frac{-s+p}{(-b+a)r}, \frac{1}{2} \frac{as-pb}{(-b+a)r}, \frac{1}{2} \frac{-s+p}{(-b+a)r}, -\frac{1}{2r} \right]$$

$$2r(-b+a)^2 \quad (29)$$

> *AM := simplify(Adjoint(A))*

$$AM := \left[ \begin{aligned} &[2aspb - 4abrb - a^2s^2 - p^2b^2, -bps + 2br - apsb + 2ar + as^2 + p^2b, -bas \\ &+ pb^2 + a^2s - apb], \\ &[-bps + 2br - apsb + 2ar + as^2 + p^2b, 2ps - 4r - s^2 - p^2, -as - pb + sb + pa], \\ &[-bas + pb^2 + a^2s - apb, -as - pb + sb + pa, 2ab - b^2 - a^2] \end{aligned} \right] \quad (30)$$

> *DepVars := [u(t, x, y), v(t, x, y)]: AJ := simplify(FromJet(AM, DepVars)) :*

> *DGsetup([t, x, y], M) :*

> *g := evalDG(AJ[1, 1]·dt &t dt + AJ[1, 2]·dt &t dx + AJ[1, 3]·dt &t dy + AJ[2, 1]·dx &t dt + AJ[2, 2]·dx &t dx + AJ[2, 3]·dx &t dy + AJ[3, 1]·dy &t dt + AJ[3, 2]·dy &t dx + AJ[3, 3]·dy &t dy)*

$$g := -(-2aspb + 4abrb + a^2s^2 + p^2b^2) dt dt - (bps - 2br + apsb - 2ar - a^2s^2 - p^2b) dt dx + (-bas + pb^2 + a^2s - apb) dt dy - (bps - 2br + apsb - 2ar - a^2s^2 - p^2b) dx dt - (-2ps + 4r + s^2 + p^2) dx dx + (-as - pb + sb + pa) dx dy + (-bas + pb^2 + a^2s - apb) dy dt + (-as - pb + sb + pa) dy dx - (-2ab + b^2 + a^2) dy dy \quad (31)$$

> *CotTen := CottonTensor(g) :*

> *CotTen*

$$0 D_t D_t \quad (32)$$

*This says that no other conditions exists. And indeed the coefficients of the symbol matrix (or dispersion relation) are constant, so the corresponding metric is (conformally) flat.*

>

*Given that the symbol matrix is constant, the system can be easily brought to the form :*

$$u_t = q(u, v) \cdot v_y;$$

$$u_y = q(u, v) \cdot v_x$$

*This system is integrable iff q is separable : q(u, v) = U(u) · V(v),*

*in which case a change of variables brings all of the coefficients of the 2 component system (a, b, p, q, r, s) to constants. This is the desired linearization!*

>

**# Conclusion:** condition Cotton=0 does **not** imply **linearization**, but it does **if** we impose some other conditions, like existence of 3 conservation laws (Godunov's symmetrization) **or** existence of a pseudopotential  $\leftrightarrow$  integrability, we **do** obtain linearizability!

>

>
