# Supplementary material for: Dispersionless integrable systems in 3D and Einstein-Weyl geometry
Source: arXiv:1208.2728 ancillary file (2013-05-09)
Supplement: Supplementary file 11 [file Examples-1.pdf]

This is the worksheet accompanying the paper E.Ferapontov & B.Kruglikov "Dispersionless integrable systems in 3D and Einstein-Weyl geometry".

The file ran on **Maple** version 16, the package **DifferentialGeometry** was used.

Integrable equations of type I have 5 normal forms and for them we check that integrability is equivalent to EW property.

>

> with(DifferentialGeometry) : with(Tensor) : with(Tools) : with(JetCalculus) :  
with(LinearAlgebra) : with(PDEtools, D\_Dx, declare, ToJet, FromJet) :

[Equation 1]  $u_{xx} + u_{yy} - (\log(1 - e^u))_{yy} - (\log(1 - e^u))_{tt} = 0$

> DGsetup([t, x, y], [u], J2) :

>  $F := u[2, 2] + u[3, 3] - \text{TotalDiff}(\log(1 - \exp(u[1])), [3, 3]) - \text{TotalDiff}(\log(1 - \exp(u[1])), [1, 1])$

$$F := u_{2,2} + u_{3,3} - \left( -\frac{e^{u[1]} u_3}{1 - e^{u[1]}} - \frac{(e^{u[1]})^2 u_3}{(1 - e^{u[1]})^2} \right) u_3 + \frac{e^{u[1]} u_{3,3}}{1 - e^{u[1]}} - \left( -\frac{e^{u[1]} u_1}{1 - e^{u[1]}} - \frac{(e^{u[1]})^2 u_1}{(1 - e^{u[1]})^2} \right) u_1 + \frac{e^{u[1]} u_{1,1}}{1 - e^{u[1]}} \quad (1)$$

>  $A := \text{Matrix} \left( \left[ \left[ \text{diff}(F, u[1, 1]), \frac{1}{2} \text{diff}(F, u[1, 2]), \frac{1}{2} \text{diff}(F, u[1, 3]) \right], \left[ \frac{1}{2} \text{diff}(F, u[1, 2]), \text{diff}(F, u[2, 2]), \frac{1}{2} \text{diff}(F, u[2, 3]) \right], \left[ \frac{1}{2} \text{diff}(F, u[1, 3]), \frac{1}{2} \text{diff}(F, u[2, 3]), \text{diff}(F, u[3, 3]) \right] \right] \right) : AA := \text{expand}(\text{MatrixInverse}(A))$

$$AA := \begin{bmatrix} -\frac{-1 + e^{u[1]}}{e^{u[1]}} & 0 & 0 \\ 0 & 1 & 0 \\ 0 & 0 & 1 - e^{u[1]} \end{bmatrix} \quad (2)$$

> DepVars := [u(t, x, y)] : FromJet(AA, DepVars)

$$\begin{bmatrix} -\frac{-1 + e^{u(t, x, y)}}{e^{u(t, x, y)}} & 0 & 0 \\ 0 & 1 & 0 \\ 0 & 0 & 1 - e^{u(t, x, y)} \end{bmatrix} \quad (3)$$

A is the matrix of the symbol of the operator (bi-vector) and AA is the matrix of the inverse metric. Both are defined up to conformal factor.

> DGsetup([t, x, y], M) :

>  $g := \text{evalDG}((e^{-u(t, x, y)} - 1) \cdot dt \& dt + dx \& dx + (1 - e^{u(t, x, y)}) \cdot dy \& dy) :$

> CotTen := CottonTensor(g) :

> CTJ := ToJet(CotTen, DepVars, notation = jetnumbers)

We remove output of the Cotton tensor - it is large, does not simplify to zero, meaning the equation is not linearizable. Next we compute the connection.

> C := Connection(a000\*dt &t D\_t &t dt + a111\*dx &t D\_x &t dx + a222\*dy &t D\_y &t dy  
+ a001\*(dt &t D\_t &t dx + dx &t D\_t &t dt) + a002\*(dt &t D\_t &t dy + dy &t D\_t  
&t dt) + a102\*(dx &t D\_t &t dy + dy &t D\_t &t dx) + a011\*(dt &t D\_x &t dx + dx  
&t D\_x &t dt) + a012\*(dt &t D\_x &t dy + dy &t D\_x &t dt) + a112\*(dx &t D\_x &t dy  
+ dy &t D\_x &t dx) + a021\*(dt &t D\_y &t dx + dx &t D\_y &t dt) + a022\*(dt &t D\_y  
&t dy + dy &t D\_y &t dt) + a122\*(dx &t D\_y &t dy + dy &t D\_y &t dx) + a010\*dt  
&t D\_x &t dt + a121\*dx &t D\_y &t dx + a202\*dy &t D\_t &t dy + a020\*dt &t D\_y &t dt  
+ a101\*dx &t D\_t &t dx + a212\*dy &t D\_x &t dy) :

> TorsionTensor(C);

$$0 \, dt \, D_t \, dt$$

(4)

> U1 := x11(u(t, x, y))·diff(u(t, x, y), t) + x12(u(t, x, y))·diff(u(t, x, y), x) + x13(u(t, x, y))  
·diff(u(t, x, y), y) :

U2 := x21(u(t, x, y))·diff(u(t, x, y), t) + x22(u(t, x, y))·diff(u(t, x, y), x) + x23(u(t, x, y))  
·diff(u(t, x, y), y) :

U3 := x31(u(t, x, y))·diff(u(t, x, y), t) + x32(u(t, x, y))·diff(u(t, x, y), x) + x33(u(t, x, y))  
·diff(u(t, x, y), y) :

> Et := evalDG(DirectionalCovariantDerivative(D\_t, g, C) + U1·g) :

Ex := evalDG(DirectionalCovariantDerivative(D\_x, g, C) + U2·g) :

Ey := evalDG(DirectionalCovariantDerivative(D\_y, g, C) + U3·g) :

U1·dt+U2·dx+U3·dy=-ω is the 1-form (covector) defining the connection.

We have chosen them in the quasilinear 1st order form basing on the form of the PDE, but experiments show that we got the same answer for any general form.

We shall compute the coefficients U[i] from the EW condition.

> Eq000 := TensorInnerProduct(g, Et, dt &t dt) :

Eq001 := TensorInnerProduct(g, Et, dt &t dx) :

Eq002 := TensorInnerProduct(g, Et, dt &t dy) :

Eq011 := TensorInnerProduct(g, Et, dx &t dx) :

Eq012 := TensorInnerProduct(g, Et, dx &t dy) :

Eq022 := TensorInnerProduct(g, Et, dy &t dy) :

Eq100 := TensorInnerProduct(g, Ex, dt &t dt) :

Eq101 := TensorInnerProduct(g, Ex, dt &t dx) :

Eq102 := TensorInnerProduct(g, Ex, dt &t dy) :

Eq111 := TensorInnerProduct(g, Ex, dx &t dx) :

Eq112 := TensorInnerProduct(g, Ex, dx &t dy) :

Eq122 := TensorInnerProduct(g, Ex, dy &t dy) :

Eq200 := TensorInnerProduct(g, Ey, dt &t dt) :

Eq201 := TensorInnerProduct(g, Ey, dt &t dx) :

Eq202 := TensorInnerProduct(g, Ey, dt &t dy) :

Eq211 := TensorInnerProduct(g, Ey, dx &t dx) :

Eq212 := TensorInnerProduct(g, Ey, dx &t dy) :

Eq222 := TensorInnerProduct(g, Ey, dy &t dy) :

> sA := solve( {Eq000=0, Eq001=0, Eq002=0, Eq011=0, Eq012=0, Eq022=0, Eq100=0,  
Eq101=0, Eq102=0, Eq111=0, Eq112=0, Eq122=0, Eq200=0, Eq201=0, Eq202=0,  
Eq211=0, Eq212=0, Eq222=0}, [a000, a001, a002, a010, a011, a012, a020, a021, a022,  
a101, a102, a111, a112, a121, a122, a202, a212, a222]) :

> C1 := evalDG( subs( {op(op(sA))}, C) ) :

$$\begin{aligned} &> \text{evalDG}(\text{CovariantDerivative}(g, C1) + g \&t (U1 \cdot dt + U2 \cdot dx + U3 \cdot dy)); \\ &\quad 0 \text{ } dt \text{ } dt \text{ } dt \end{aligned} \quad (5)$$

$$\begin{aligned} &> R1 := \text{CurvatureTensor}(C1) : Ric1 := \text{RicciTensor}(R1) : T1 := \text{SymmetrizeIndices}(Ric1, [1, 2], \\ &\quad \text{"Symmetric"}) : Res := \text{evalDG}(T1 - V \cdot g) : \end{aligned}$$

$$\begin{aligned} &> NEQtt := \text{TensorInnerProduct}(g, Res, dt \&t dt) : NEQtx := \text{TensorInnerProduct}(g, Res, dt \\ &\quad \&t dx) : \\ &NEQty := \text{TensorInnerProduct}(g, Res, dt \&t dy) : NEQxx := \text{TensorInnerProduct}(g, Res, dx \\ &\quad \&t dx) : \\ &NEQxy := \text{TensorInnerProduct}(g, Res, dx \&t dy) : NEQyy := \text{TensorInnerProduct}(g, Res, dy \\ &\quad \&t dy) : \end{aligned}$$

$$\begin{aligned} &> \\ &> NEQtt := \text{ContractIndices}(Res, D\_t \&t D\_t, [[1, 1], [2, 2]]) : NEQtx := \text{ContractIndices}(Res, \\ &\quad D\_t \&t D\_x, [[1, 1], [2, 2]]) : \\ &NEQty := \text{ContractIndices}(Res, D\_t \&t D\_y, [[1, 1], [2, 2]]) : NEQxx := \text{ContractIndices}(Res, \\ &\quad D\_x \&t D\_x, [[1, 1], [2, 2]]) : \\ &NEQxy := \text{ContractIndices}(Res, D\_x \&t D\_y, [[1, 1], [2, 2]]) : NEQyy := \text{ContractIndices}(Res, \\ &\quad D\_y \&t D\_y, [[1, 1], [2, 2]]) : \end{aligned}$$

Thus we got 5 equations specifying EW condition  $\text{Ricci}(\nabla) = V \cdot g$  for some scalar function  $V$ .

Next we restrict everything to the equation, and for this we pass to jet-notations. Then we solve for the terms  $\kappa[ij]$  of the coefficients  $U[i]$  of the covector.

$$> \text{DGsetup}([t, x, y], [u], J2, 4) :$$

$$> \text{de} := \text{DifferentialEquationData}([F], [u_{1,1}])$$

$$\begin{aligned} \text{de} := & \left[ \{u_{1,1}\}, \left[ u_{2,2} + u_{3,3} - \left( -\frac{e^{u_{[]}} u_3}{1 - e^{u_{[]}}} - \frac{(e^{u_{[]}})^2 u_3}{(1 - e^{u_{[]}})^2} \right) u_3 + \frac{e^{u_{[]}} u_{3,3}}{1 - e^{u_{[]}}} - \left( -\frac{e^{u_{[]}} u_1}{1 - e^{u_{[]}}} \right. \right. \right. \\ & \left. \left. - \frac{(e^{u_{[]}})^2 u_1}{(1 - e^{u_{[]}})^2} \right) u_1 + \frac{e^{u_{[]}} u_{1,1}}{1 - e^{u_{[]}}} \right] \end{aligned} \quad (6)$$

$$> \text{de2} := \text{Prolong}(\text{de}, 2) : \text{deTRA} := \text{Transformation}(\text{de2}) :$$

>

$$> \text{Eq0} := \text{Pullback}(\text{deTRA}, \text{ToJet}(NEQtt, \text{DepVars}, \text{notation} = \text{jetnumbers})) :$$

$$> \text{VS} := \text{solve}(\text{Eq0}, V) :$$

$$> \text{Eq1} := \text{numer}(\text{subs}(V = \text{VS}, \text{Pullback}(\text{deTRA}, \text{ToJet}(NEQtx, \text{DepVars}, \text{notation} = \text{jetnumbers})))) :$$

$$\text{Eq2} := \text{numer}(\text{subs}(V = \text{VS}, \text{Pullback}(\text{deTRA}, \text{ToJet}(NEQty, \text{DepVars}, \text{notation} = \text{jetnumbers})))) :$$

$$\text{Eq3} := \text{numer}(\text{subs}(V = \text{VS}, \text{Pullback}(\text{deTRA}, \text{ToJet}(NEQxx, \text{DepVars}, \text{notation} = \text{jetnumbers})))) :$$

$$\text{Eq4} := \text{numer}(\text{subs}(V = \text{VS}, \text{Pullback}(\text{deTRA}, \text{ToJet}(NEQxy, \text{DepVars}, \text{notation} = \text{jetnumbers})))) :$$

$$\text{Eq5} := \text{numer}(\text{subs}(V = \text{VS}, \text{Pullback}(\text{deTRA}, \text{ToJet}(NEQyy, \text{DepVars}, \text{notation} = \text{jetnumbers})))) :$$

$$\text{J2 } > \text{SQE1} := \text{simplify}(\text{diff}(\text{Eq1}, u_{1,2}))$$

$$\text{SQE1} := -6 e^{3u_{[]}} - 4 \kappa_{11}(u_{[]}) e^{3u_{[]}} - 4 \kappa_{22}(u_{[]}) e^{3u_{[]}} + \kappa_{11}(u_{[]}) - 4 \kappa_{11}(u_{[]}) e^{u_{[]}} \quad (7)$$

$$\begin{aligned}
& + \kappa_{22}(u_{[]}) - 4 \kappa_{22}(u_{[]}) e^u_{[]} + 6 e^{2u}_{[]} - 2 e^u_{[]} + 6 \kappa_{22}(u_{[]}) e^{2u}_{[]} + \kappa_{11}(u_{[]}) e^{4u}_{[]} \\
& + \kappa_{22}(u_{[]}) e^{4u}_{[]} + 6 \kappa_{11}(u_{[]}) e^{2u}_{[]} + 2 e^{4u}_{[]}
\end{aligned}$$

> *simplify*(*diff*(*Eq1*, *u*<sub>1,3</sub>))

$$\kappa_{23}(u_{[]}) \left( -4 e^{3u}_{[]} + 1 - 4 e^u_{[]} + 6 e^{2u}_{[]} + e^{4u}_{[]} \right) \quad (8)$$

> *simplify*(*diff*(*Eq1*, *u*<sub>2,2</sub>))

$$\begin{aligned}
& -4 \kappa_{12}(u_{[]}) e^{3u}_{[]} + \kappa_{12}(u_{[]}) - 4 \kappa_{12}(u_{[]}) e^u_{[]} - 5 \kappa_{21}(u_{[]}) e^{3u}_{[]} - \kappa_{21}(u_{[]}) e^{-u}_{[]} \\
& + 10 \kappa_{21}(u_{[]}) e^{2u}_{[]} + \kappa_{21}(u_{[]}) e^{4u}_{[]} - 10 \kappa_{21}(u_{[]}) e^u_{[]} + \kappa_{12}(u_{[]}) e^{4u}_{[]} \\
& + 6 \kappa_{12}(u_{[]}) e^{2u}_{[]} + 5 \kappa_{21}(u_{[]})
\end{aligned} \quad (9)$$

> *simplify*(*diff*(*Eq1*, *u*<sub>2,3</sub>))

$$\kappa_{13}(u_{[]}) \left( -4 e^{3u}_{[]} + 1 - 4 e^u_{[]} + 6 e^{2u}_{[]} + e^{4u}_{[]} \right) \quad (10)$$

> *simplify*(*diff*(*Eq1*, *u*<sub>3,3</sub>))

$$-\kappa_{21}(u_{[]}) \left( e^{3u}_{[]} + e^{-u}_{[]} - 4 e^{2u}_{[]} + 6 e^u_{[]} - 4 \right) \quad (11)$$

> *simplify*(*diff*(*Eq2*, *u*<sub>1,2</sub>))

$$\kappa_{32}(u_{[]}) \left( 3 e^{2u}_{[]} - 3 e^u_{[]} + 1 - e^{3u}_{[]} \right) \quad (12)$$

> *SQE2* := *simplify*(*diff*(*Eq2*, *u*<sub>1,3</sub>))

$$\begin{aligned}
\text{SQE2} := & 3 \kappa_{11}(u_{[]}) e^{2u}_{[]} + 3 \kappa_{33}(u_{[]}) e^{2u}_{[]} - 3 \kappa_{11}(u_{[]}) e^u_{[]} - 3 \kappa_{33}(u_{[]}) e^u_{[]} + \kappa_{11}(u_{[]}) \\
& - \kappa_{11}(u_{[]}) e^{3u}_{[]} + \kappa_{33}(u_{[]}) - \kappa_{33}(u_{[]}) e^{3u}_{[]}
\end{aligned} \quad (13)$$

> *simplify*(*diff*(*Eq2*, *u*<sub>2,2</sub>))

$$-\kappa_{31}(u_{[]}) \left( e^{3u}_{[]} + e^{-u}_{[]} - 4 e^{2u}_{[]} + 6 e^u_{[]} - 4 \right) \quad (14)$$

> *simplify*(*diff*(*Eq2*, *u*<sub>2,3</sub>))

$$\kappa_{12}(u_{[]}) \left( 3 e^{2u}_{[]} - 3 e^u_{[]} + 1 - e^{3u}_{[]} \right) \quad (15)$$

> *simplify*(*diff*(*Eq2*, *u*<sub>3,3</sub>))

$$\begin{aligned}
& 3 \kappa_{31}(u_{[]}) + 3 \kappa_{13}(u_{[]}) e^{2u}_{[]} - 3 \kappa_{31}(u_{[]}) e^u_{[]} - \kappa_{31}(u_{[]}) e^{-u}_{[]} + \kappa_{31}(u_{[]}) e^{2u}_{[]} \\
& - 3 \kappa_{13}(u_{[]}) e^u_{[]} + \kappa_{13}(u_{[]}) - \kappa_{13}(u_{[]}) e^{3u}_{[]}
\end{aligned} \quad (16)$$

> *simplify*(*diff*(*Eq3*, *u*<sub>1,2</sub>))

$$-252 \kappa_{12}(u_{[]}) e^{3u}_{[]} - 504 \kappa_{21}(u_{[]}) e^{3u}_{[]} + 420 \kappa_{21}(u_{[]}) e^{4u}_{[]} + 252 \kappa_{12}(u_{[]}) e^{4u}_{[]} \quad (17)$$

$$\begin{aligned}
& + 90 \kappa 21(u_{[]}) + 18 \kappa 12(u_{[]}) - 72 \kappa 12(u_{[]}) e^u_{[]} + 168 \kappa 12(u_{[]}) e^{2u}_{[]} \\
& - 20 \kappa 21(u_{[]}) e^{-u}_{[]} - 240 \kappa 21(u_{[]}) e^u_{[]} + 420 \kappa 21(u_{[]}) e^{2u}_{[]} - 2 \kappa 12(u_{[]}) e^{-u}_{[]} \\
& + 2 \kappa 12(u_{[]}) e^{8u}_{[]} + 2 \kappa 21(u_{[]}) e^{8u}_{[]} + 72 \kappa 12(u_{[]}) e^{6u}_{[]} - 18 \kappa 12(u_{[]}) e^{7u}_{[]} \\
& - 240 \kappa 21(u_{[]}) e^{5u}_{[]} + 90 \kappa 21(u_{[]}) e^{6u}_{[]} - 20 \kappa 21(u_{[]}) e^{7u}_{[]} + 2 \kappa 21(u_{[]}) e^{-2u}_{[]} \\
& - 168 \kappa 12(u_{[]}) e^{5u}_{[]}
\end{aligned}$$

> *simplify(diff(Eq3, u<sub>1,3</sub>))*

$$\begin{aligned}
& -2 \kappa 13(u_{[]}) \left( -9 + e^{-u}_{[]} - 36 e^{6u}_{[]} - e^{8u}_{[]} + 84 e^{5u}_{[]} + 9 e^{7u}_{[]} - 84 e^{2u}_{[]} + 126 e^{3u}_{[]} \right. \\
& \quad \left. - 126 e^{4u}_{[]} + 36 e^u_{[]} \right)
\end{aligned} \tag{18}$$

> *SQE3 := simplify(diff(Eq3, u<sub>2,2</sub>))*

$$\begin{aligned}
& SQE3 := 36 - 144 e^u_{[]} + 90 \kappa 22(u_{[]}) + 90 \kappa 11(u_{[]}) - 4 e^{-u}_{[]} - 504 e^{3u}_{[]} + 2 \kappa 22(u_{[]}) e^{8u}_{[]} \\
& + 2 \kappa 11(u_{[]}) e^{8u}_{[]} + 2 \kappa 22(u_{[]}) e^{-2u}_{[]} + 90 \kappa 22(u_{[]}) e^{6u}_{[]} - 20 \kappa 22(u_{[]}) e^{7u}_{[]} \\
& - 240 \kappa 22(u_{[]}) e^{5u}_{[]} - 240 \kappa 11(u_{[]}) e^{5u}_{[]} + 90 \kappa 11(u_{[]}) e^{6u}_{[]} - 20 \kappa 11(u_{[]}) e^{7u}_{[]} \\
& - 20 \kappa 22(u_{[]}) e^{-u}_{[]} + 2 e^{-2u}_{[]} \kappa 11(u_{[]}) - 20 e^{-u}_{[]} \kappa 11(u_{[]}) + 144 e^{6u}_{[]} + 336 e^{2u}_{[]} \\
& - 36 e^{7u}_{[]} - 336 e^{5u}_{[]} + 4 e^{8u}_{[]} + 420 \kappa 22(u_{[]}) e^{2u}_{[]} - 240 \kappa 22(u_{[]}) e^u_{[]} \\
& + 420 \kappa 11(u_{[]}) e^{2u}_{[]} - 504 \kappa 11(u_{[]}) e^{3u}_{[]} - 504 \kappa 22(u_{[]}) e^{3u}_{[]} + 420 \kappa 11(u_{[]}) e^{4u}_{[]} \\
& + 420 \kappa 22(u_{[]}) e^{4u}_{[]} - 240 \kappa 11(u_{[]}) e^u_{[]} + 504 e^{4u}_{[]}
\end{aligned} \tag{19}$$

> *simplify(diff(Eq3, u<sub>2,3</sub>))*

$$\begin{aligned}
& -2 \kappa 23(u_{[]}) \left( 10 e^{-u}_{[]} - e^{8u}_{[]} - 45 e^{6u}_{[]} + 120 e^{5u}_{[]} - e^{-2u}_{[]} + 10 e^{7u}_{[]} + 252 e^{3u}_{[]} \right. \\
& \quad \left. - 210 e^{4u}_{[]} - 45 + 120 e^u_{[]} - 210 e^{2u}_{[]} \right)
\end{aligned} \tag{20}$$

> *SQE4 := simplify(diff(Eq3, u<sub>3,3</sub>))*

$$\begin{aligned}
& SQE4 := 72 - 168 e^u_{[]} + 72 \kappa 11(u_{[]}) + 2 e^{-2u}_{[]} - 18 e^{-u}_{[]} - 252 e^{3u}_{[]} - 72 \kappa 11(u_{[]}) e^{5u}_{[]} \\
& + 18 \kappa 11(u_{[]}) e^{6u}_{[]} - 2 \kappa 11(u_{[]}) e^{7u}_{[]} + 2 e^{-2u}_{[]} \kappa 11(u_{[]}) - 18 e^{-u}_{[]} \kappa 11(u_{[]}) \\
& + 18 e^{6u}_{[]} + 252 e^{2u}_{[]} - 2 e^{7u}_{[]} - 72 e^{5u}_{[]} + 252 \kappa 11(u_{[]}) e^{2u}_{[]} - 252 \kappa 11(u_{[]}) e^{3u}_{[]} \\
& + 168 \kappa 11(u_{[]}) e^{4u}_{[]} - 168 \kappa 11(u_{[]}) e^u_{[]} + 168 e^{4u}_{[]}
\end{aligned} \tag{21}$$

$$\begin{aligned} &> \text{simplify}(\text{diff}(Eq4, u_{1,2})) \\ &\quad \kappa31(u_{[]}) \left( 3 e^{-u_{[]}} + e^{u_{[]}} - e^{-2u_{[]}} - 3 \right) \end{aligned} \quad (22)$$

$$\begin{aligned} &> \text{simplify}(\text{diff}(Eq4, u_{1,3})) \\ &\quad \kappa21(u_{[]}) \left( 3 e^{-u_{[]}} + e^{u_{[]}} - e^{-2u_{[]}} - 3 \right) \end{aligned} \quad (23)$$

$$\begin{aligned} &> \text{simplify}(\text{diff}(Eq4, u_{2,2})) \\ &\quad \kappa32(u_{[]}) \left( 3 e^{-u_{[]}} + e^{u_{[]}} - e^{-2u_{[]}} - 3 \right) \end{aligned} \quad (24)$$

$$\begin{aligned} &> SQE5 := \text{simplify}(\text{diff}(Eq4, u_{2,3})) \\ SQE5 &:= \kappa22(u_{[]}) e^{u_{[]}} + 3 \kappa33(u_{[]}) e^{-u_{[]}} - \kappa22(u_{[]}) e^{-2u_{[]}} + 3 \kappa22(u_{[]}) e^{-u_{[]}} \\ &\quad - \kappa33(u_{[]}) e^{-2u_{[]}} + \kappa33(u_{[]}) e^{u_{[]}} - 3 \kappa33(u_{[]}) - 3 \kappa22(u_{[]}) + 2 e^{-2u_{[]}} - 4 e^{-u_{[]}} + 2 \end{aligned} \quad (25)$$

$$\begin{aligned} &> \text{simplify}(\text{diff}(Eq4, u_{3,3})) \\ &\quad \kappa23(u_{[]}) \left( 3 e^{-u_{[]}} + e^{u_{[]}} - e^{-2u_{[]}} - 3 \right) \end{aligned} \quad (26)$$

$$\begin{aligned} &> \text{simplify}(\text{diff}(Eq5, u_{1,2})) \\ 2 \kappa12(u_{[]}) &\left( -9 + e^{-u_{[]}} - 36 e^{6u_{[]}} - e^{8u_{[]}} + 84 e^{5u_{[]}} + 9 e^{7u_{[]}} - 84 e^{2u_{[]}} + 126 e^{3u_{[]}} \right. \\ &\quad \left. - 126 e^{4u_{[]}} + 36 e^{u_{[]}} \right) \end{aligned} \quad (27)$$

$$\begin{aligned} &> \text{simplify}(\text{diff}(Eq5, u_{1,3})) \\ 252 \kappa31(u_{[]}) e^{3u_{[]}} &+ 72 e^{5u_{[]}} \kappa31(u_{[]}) + 2 \kappa31(u_{[]}) e^{7u_{[]}} - 168 \kappa31(u_{[]}) e^{4u_{[]}} \\ &- 18 \kappa31(u_{[]}) e^{6u_{[]}} - 252 \kappa31(u_{[]}) e^{2u_{[]}} - 72 \kappa31(u_{[]}) - 18 \kappa13(u_{[]}) \\ &+ 2 \kappa13(u_{[]}) e^{-u_{[]}} - 72 \kappa13(u_{[]}) e^{6u_{[]}} - 2 \kappa13(u_{[]}) e^{8u_{[]}} + 168 \kappa13(u_{[]}) e^{5u_{[]}} \\ &+ 18 \kappa13(u_{[]}) e^{7u_{[]}} - 2 \kappa31(u_{[]}) e^{-2u_{[]}} + 18 \kappa31(u_{[]}) e^{-u_{[]}} + 168 \kappa31(u_{[]}) e^{u_{[]}} \\ &- 168 \kappa13(u_{[]}) e^{2u_{[]}} + 72 \kappa13(u_{[]}) e^{u_{[]}} + 252 \kappa13(u_{[]}) e^{3u_{[]}} - 252 \kappa13(u_{[]}) e^{4u_{[]}} \end{aligned} \quad (28)$$

$$\begin{aligned} &> SQE6 := \text{simplify}(\text{diff}(Eq5, u_{2,2})) \\ SQE6 &:= -90 + 240 e^{u_{[]}} - 90 \kappa11(u_{[]}) - 2 e^{-2u_{[]}} + 20 e^{-u_{[]}} + 504 e^{3u_{[]}} - 2 \kappa11(u_{[]}) e^{8u_{[]}} \\ &\quad + 240 \kappa11(u_{[]}) e^{5u_{[]}} - 90 \kappa11(u_{[]}) e^{6u_{[]}} + 20 \kappa11(u_{[]}) e^{7u_{[]}} - 2 e^{-2u_{[]}} \kappa11(u_{[]}) \\ &\quad + 20 e^{-u_{[]}} \kappa11(u_{[]}) - 90 e^{6u_{[]}} - 420 e^{2u_{[]}} + 20 e^{7u_{[]}} + 240 e^{5u_{[]}} - 2 e^{8u_{[]}} \\ &\quad - 420 \kappa11(u_{[]}) e^{2u_{[]}} + 504 \kappa11(u_{[]}) e^{3u_{[]}} - 420 \kappa11(u_{[]}) e^{4u_{[]}} + 240 \kappa11(u_{[]}) e^{u_{[]}} \\ &\quad - 420 e^{4u_{[]}} \end{aligned} \quad (29)$$

$$\begin{aligned} &> \text{simplify}(\text{diff}(Eq5, u_{2,3})) \\ &2 \kappa_{32}(u_{[]}) \left( 126 e^{3u_{[]}} + 84 e^{u_{[]}} - 126 e^{2u_{[]}} + 36 e^{5u_{[]}} - 9 e^{6u_{[]}} + e^{7u_{[]}} - 84 e^{4u_{[]}} - 36 \right. \\ &\quad \left. + 9 e^{-u_{[]}} - e^{-2u_{[]}} \right) \end{aligned} \quad (30)$$

$$\begin{aligned} &> SQE7 := \text{simplify}(\text{diff}(Eq5, u_{3,3})) \\ &SQE7 := 252 \kappa_{33}(u_{[]}) e^{3u_{[]}} + 72 e^{5u_{[]}} \kappa_{33}(u_{[]}) + 2 \kappa_{33}(u_{[]}) e^{7u_{[]}} - 168 \kappa_{33}(u_{[]}) e^{4u_{[]}} \\ &\quad - 18 \kappa_{33}(u_{[]}) e^{6u_{[]}} - 72 \kappa_{33}(u_{[]}) - 72 \kappa_{11}(u_{[]}) + 18 \kappa_{33}(u_{[]}) e^{-u_{[]}} \\ &\quad - 2 \kappa_{33}(u_{[]}) e^{-2u_{[]}} + 72 \kappa_{11}(u_{[]}) e^{5u_{[]}} - 18 \kappa_{11}(u_{[]}) e^{6u_{[]}} + 2 \kappa_{11}(u_{[]}) e^{7u_{[]}} \\ &\quad - 2 e^{-2u_{[]}} \kappa_{11}(u_{[]}) + 18 e^{-u_{[]}} \kappa_{11}(u_{[]}) + 168 \kappa_{33}(u_{[]}) e^{u_{[]}} - 252 \kappa_{33}(u_{[]}) e^{2u_{[]}} \\ &\quad - 252 \kappa_{11}(u_{[]}) e^{2u_{[]}} + 252 \kappa_{11}(u_{[]}) e^{3u_{[]}} - 168 \kappa_{11}(u_{[]}) e^{4u_{[]}} + 168 \kappa_{11}(u_{[]}) e^{u_{[]}} \end{aligned} \quad (31)$$

$$\begin{aligned} &> \text{solve}([SQE1, SQE2, SQE3, SQE4, SQE5, SQE6], \{\kappa_{11}(u_{[]}), \kappa_{22}(u_{[]}), \kappa_{33}(u_{[]})\}) \\ &\quad \left\{ \kappa_{11}(u_{[]}) = -1, \kappa_{22}(u_{[]}) = \frac{e^{-u_{[]}} - e^{u_{[]}} - e^{-2u_{[]}} + 1}{3 e^{-u_{[]}} + e^{u_{[]}} - e^{-2u_{[]}} - 3}, \kappa_{33}(u_{[]}) = 1 \right\} \end{aligned} \quad (32)$$

Finally, by only studying the symbols of the EW equations, we determined completely the covector  $\omega$ . Now let us check the EW property in full.

**M** > DGsetup([t, x, y], M) :

> U1 := -diff(u(t, x, y), t) :

$$U2 := \frac{e^{-u(t, x, y)} - e^{u(t, x, y)} - e^{-2u(t, x, y)} + 1}{3 e^{-u(t, x, y)} + e^{u(t, x, y)} - e^{-2u(t, x, y)} - 3} \cdot \text{diff}(u(t, x, y), x) :$$

U3 := diff(u(t, x, y), y) :

> Et := evalDG(DirectionalCovariantDerivative(D\_t, g, C) + U1·g) :

Ex := evalDG(DirectionalCovariantDerivative(D\_x, g, C) + U2·g) :

Ey := evalDG(DirectionalCovariantDerivative(D\_y, g, C) + U3·g) :

> Eq000 := TensorInnerProduct(g, Et, dt &t dt) :

Eq001 := TensorInnerProduct(g, Et, dt &t dx) :

Eq002 := TensorInnerProduct(g, Et, dt &t dy) :

Eq011 := TensorInnerProduct(g, Et, dx &t dx) :

Eq012 := TensorInnerProduct(g, Et, dx &t dy) :

Eq022 := TensorInnerProduct(g, Et, dy &t dy) :

Eq100 := TensorInnerProduct(g, Ex, dt &t dt) :

Eq101 := TensorInnerProduct(g, Ex, dt &t dx) :

Eq102 := TensorInnerProduct(g, Ex, dt &t dy) :

Eq111 := TensorInnerProduct(g, Ex, dx &t dx) :

Eq112 := TensorInnerProduct(g, Ex, dx &t dy) :

Eq122 := TensorInnerProduct(g, Ex, dy &t dy) :

Eq200 := TensorInnerProduct(g, Ey, dt &t dt) :

Eq201 := TensorInnerProduct(g, Ey, dt &t dx) :

Eq202 := TensorInnerProduct(g, Ey, dt &t dy) :

Eq211 := TensorInnerProduct(g, Ey, dx &t dx) :

Eq212 := TensorInnerProduct(g, Ey, dx &t dy) :

Eq222 := TensorInnerProduct(g, Ey, dy &t dy) :

> sA := solve( {Eq000=0, Eq001=0, Eq002=0, Eq011=0, Eq012=0, Eq022=0, Eq100=0, Eq101=0, Eq102=0, Eq111=0, Eq112=0, Eq122=0, Eq200=0, Eq201=0, Eq202=0, Eq211=0, Eq212=0, Eq222=0}, [a000, a001, a002, a010, a011, a012, a020, a021, a022, a101, a102, a111, a112, a121, a122, a202, a212, a222] ) :

> C1 := evalDG( subs( {op(op(sA))}, C) ) :

> evalDG( CovariantDerivative(g, C1) + g &t (U1·dt + U2·dx + U3 ·dy) );  
0 dt dt dt

(33)

> R1 := CurvatureTensor(C1) : Ric1 := RicciTensor(R1) : T1 := SymmetrizeIndices(Ric1, [1, 2], "Symmetric") : Res := evalDG(T1 - V·g) :

> NEQtt := TensorInnerProduct(g, Res, dt &t dt) : NEQtx := TensorInnerProduct(g, Res, dt &t dx) :

NEQty := TensorInnerProduct(g, Res, dt &t dy) : NEQxx := TensorInnerProduct(g, Res, dx &t dx) :

NEQxy := TensorInnerProduct(g, Res, dx &t dy) : NEQyy := TensorInnerProduct(g, Res, dy &t dy) :

>

> DGsetup([t, x, y], [u], J2, 4) :

> de := DifferentialEquationData([F], [u<sub>1,1</sub>])

$$de := \left[ \{u_{1,1}\}, \left[ u_{2,2} + u_{3,3} - \left( -\frac{e^{u_{[]}} u_3}{1 - e^{u_{[]}}} - \frac{(e^{u_{[]}})^2 u_3}{(1 - e^{u_{[]}})^2} \right) u_3 + \frac{e^{u_{[]}} u_{3,3}}{1 - e^{u_{[]}}} - \left( -\frac{e^{u_{[]}} u_1}{1 - e^{u_{[]}}} - \frac{(e^{u_{[]}})^2 u_1}{(1 - e^{u_{[]}})^2} \right) u_1 + \frac{e^{u_{[]}} u_{1,1}}{1 - e^{u_{[]}}} \right] \right] \quad (34)$$

> de2 := Prolong(de, 2) : deTRA := Transformation(de2) :

>

> Eq0 := Pullback(deTRA, ToJet(NEQtt, DepVars, notation = jetnumbers)) :

> VS := solve(Eq0, V) :

> Eq1 := numer(subs(V=VS, Pullback(deTRA, ToJet(NEQtx, DepVars, notation = jetnumbers)))) :

Eq2 := numer(subs(V=VS, Pullback(deTRA, ToJet(NEQty, DepVars, notation = jetnumbers)))) :

Eq3 := numer(subs(V=VS, Pullback(deTRA, ToJet(NEQxx, DepVars, notation = jetnumbers)))) :

Eq4 := numer(subs(V=VS, Pullback(deTRA, ToJet(NEQxy, DepVars, notation = jetnumbers)))) :

Eq5 := numer(subs(V=VS, Pullback(deTRA, ToJet(NEQyy, DepVars, notation = jetnumbers)))) :

> simplify([Eq1, Eq2, Eq3, Eq4, Eq5])

[0, 0, 0, 0, 0]

(35)

> simplify(VS)

$$\frac{1}{2} \left( 22880 u_{2,2} + 22880 u_{3,3} - 2 u_{3,3} e^{7u_{[]}} - 3003 u_2^2 e^{2u_{[]}} + e^{7u_{[]}} u_2^2 + 5005 e^{u_{[]}} u_2^2 \right) \quad (36)$$



$$\begin{aligned}
& + 1365 e^{3u} u_2^2 + e^{7u} u_1^2 - 2 e^{7u} u_{2,2} - 6435 u_2^2 + e^{7u} u_3^2 - 6435 u_3^2 - 6435 u_1^2 \\
& - 16016 u_{2,2} e^u - 16016 e^u u_{3,3} + 5005 e^u u_3^2 + 5005 e^u u_1^2 + 8736 e^{2u} u_{3,3} \\
& - 3003 e^{2u} u_3^2 - 3003 e^{2u} u_1^2 - 3640 e^{3u} u_{2,2} + 32 u_{3,3} e^{-8u} - 240 u_{2,2} e^{-7u} \\
& + 3003 u_1^2 e^{-3u} - 5005 u_1^2 e^{-2u} + 455 u_2^2 e^{-5u} - 1365 u_2^2 e^{-4u} + 1365 u_1^2 e^{3u} \\
& + 3003 u_2^2 e^{-3u} + 6435 u_1^2 e^{-u} - 455 u_1^2 e^{4u} - 455 u_2^2 e^{4u} + 105 u_2^2 e^{5u} - 455 \\
& u_3^2 e^{4u} - 1365 u_3^2 e^{-4u} + 15 u_3^2 e^{-7u} + 455 u_3^2 e^{-5u} - 105 u_3^2 e^{-6u} + 15 u_1^2 e^{-7u} \\
& + 3003 u_3^2 e^{-3u} + 15 u_2^2 e^{-7u} - 1365 u_1^2 e^{-4u} + 455 u_1^2 e^{-5u} - 105 u_1^2 e^{-6u} - 105 \\
& u_2^2 e^{-6u} - u_2^2 e^{-8u} - u_3^2 e^{-8u} - u_1^2 e^{-8u} + 1120 u_{2,2} e^{-6u} - 16016 u_{3,3} e^{-3u} \\
& + 1120 u_{3,3} e^{4u} + 8736 u_{3,3} e^{-4u} - 3640 u_{3,3} e^{-5u} + 1120 u_{3,3} e^{-6u} - 2 u_{3,3} e^{-9u} \\
& + 32 u_{2,2} e^{6u} - 3640 u_{2,2} e^{-5u} + 1120 u_{2,2} e^{4u} + 8736 u_{2,2} e^{-4u} \\
& - 16016 u_{2,2} e^{-3u} - 240 u_{2,2} e^{5u} - 240 u_{3,3} e^{5u} + 32 u_{2,2} e^{-8u} - 2 u_{2,2} e^{-9u} \\
& - 240 u_{3,3} e^{-7u} - 15 u_2^2 e^{6u} + 32 e^{6u} u_{3,3} + 105 u_1^2 e^{5u} + 105 u_3^2 e^{5u} - 15 u_1^2 e^{6u} \\
& - 15 u_3^2 e^{6u} - 3640 e^{3u} u_{3,3} + 1365 e^{3u} u_3^2 - 5005 u_3^2 e^{-2u} - 5005 u_2^2 e^{-2u} \\
& + 22880 u_{2,2} e^{-2u} - 25740 u_{2,2} e^{-u} + 6435 u_2^2 e^{-u} + 22880 u_{3,3} e^{-2u} \\
& - 25740 u_{3,3} e^{-u} + 6435 u_3^2 e^{-u} + 8736 u_{2,2} e^{2u} \Big) / \Big( -24310 + e^{-9u} - 17 e^{-8u} \\
& + 136 e^{-7u} - 680 e^{-6u} + 2380 e^{-5u} + 12376 e^{-3u} + 19448 e^u - 19448 e^{-2u} \\
& + 24310 e^{-u} + 6188 e^{3u} - 136 e^{6u} - 12376 e^{2u} - 6188 e^{-4u} + 17 e^{7u} \\
& + 680 e^{5u} - e^{8u} - 2380 e^{4u} \Big)
\end{aligned}$$

Perfect - the linerization metric is EW on the equation.

>

Let us checkd that the Coton tensor does not vanish

**J2** > *ToJet(ContractIndices(CotTen, dt & dt, [[1, 1], [2, 2]]), DepVars, notation = jetnumbers)*

$$\begin{aligned}
& \frac{1}{4} \frac{1}{\left( e^{-u} - 1 \right)^3 \left( -1 + e^u \right)^2} \Big( 4 u_3 u_2 u_1 e^{-u} - 2 u_2 u_3 u_1 - 2 u_1 e^u u_2 u_3 + 4 u_{2,3} u_1 e^{-u} \\
& - 9 u_{2,3} u_1 + 6 u_1 e^u u_{2,3} + 3 u_3 u_{1,2} e^{-u} - 6 u_{1,2} u_3 + 3 u_{1,2} u_3 e^u + 6 u_{1,2,3} e^u \Big)
\end{aligned} \tag{37}$$

$$\begin{aligned} & -7 u_2 u_{1,3} + 2 u_{1,2,3} e^{-u} + 5 u_2 u_{1,3} e^u + 3 u_{1,3} u_2 e^{-u} - 6 u_{1,2,3} - 2 u_{1,2,3} e^{2u} \\ & - u_2 u_{1,3} e^{2u} - u_1 e^{2u} u_{2,3} \end{aligned}$$

$$\begin{aligned} & \text{Pullback}\left(\text{deTRA}, 4 u_3 u_2 u_1 e^{-u} - 2 u_2 u_3 u_1 - 2 u_1 e^u u_2 u_3 + 4 u_{2,3} u_1 e^{-u} - 9 u_{2,3} u_1 \right. \\ & \quad + 6 u_1 e^u u_{2,3} + 3 u_3 u_{1,2} e^{-u} - 6 u_{1,2} u_3 + 3 u_{1,2} u_3 e^u + 6 u_{1,2,3} e^u - 7 u_2 u_{1,3} \\ & \quad + 2 u_{1,2,3} e^{-u} + 5 u_2 u_{1,3} e^u + 3 u_{1,3} u_2 e^{-u} - 6 u_{1,2,3} - 2 u_{1,2,3} e^{2u} - u_2 u_{1,3} e^{2u} \\ & \quad \left. - u_1 e^{2u} u_{2,3}\right) \\ & 4 u_3 u_2 u_1 e^{-u} - 2 u_2 u_3 u_1 - 2 u_1 e^u u_2 u_3 + 4 u_{2,3} u_1 e^{-u} - 9 u_{2,3} u_1 + 6 u_1 e^u u_{2,3} \\ & \quad + 3 u_3 u_{1,2} e^{-u} - 6 u_{1,2} u_3 + 3 u_{1,2} u_3 e^u + 6 u_{1,2,3} e^u - 7 u_2 u_{1,3} + 2 u_{1,2,3} e^{-u} \\ & \quad + 5 u_2 u_{1,3} e^u + 3 u_{1,3} u_2 e^{-u} - 6 u_{1,2,3} - 2 u_{1,2,3} e^{2u} - u_2 u_{1,3} e^{2u} - u_1 e^{2u} u_{2,3} \end{aligned} \quad (38)$$

In what follows we repeat the same procedure for the four other equations, so we will not write detailed comments.

```
> restart : with(DifferentialGeometry) : with(Tensor) : with(Tools) : with(JetCalculus) :
with(LinearAlgebra) : with(PDEtools, D_Dx, declare, ToJet, FromJet) :
```

[Equation 2]  $u_{xx} + u_{yy} + (e^u u)_{tt} = 0$

```
> DGsetup([t, x, y], [u], J2) :
```

```
> F := u[2, 2] + u[3, 3] + TotalDiff(exp(u), [1, 1])
```

$$F := u_{2,2} + u_{3,3} + e^u u_1^2 + e^u u_{1,1} \quad (39)$$

```
> A := Matrix( [[diff(F, u[1, 1]), 1/2 diff(F, u[1, 2]), 1/2 diff(F, u[1, 3])], [1/2 diff(F, u[1, 2]), diff(F, u[2, 2]), 1/2 diff(F, u[2, 3])], [1/2 diff(F, u[1, 3]), 1/2 diff(F, u[2, 3]), diff(F, u[3, 3])] ] ) : AA := expand(MatrixInverse(A))
```

$$AA := \begin{bmatrix} \frac{1}{e^u} & 0 & 0 \\ 0 & 1 & 0 \\ 0 & 0 & 1 \end{bmatrix} \quad (40)$$

> DepVars := [u(t, x, y)] : FromJet(AA, DepVars)

$$\begin{bmatrix} \frac{1}{e^{u(t, x, y)}} & 0 & 0 \\ 0 & 1 & 0 \\ 0 & 0 & 1 \end{bmatrix} \quad (41)$$

> DGsetup([t, x, y], M) :

> g := evalDG( $e^{-u(t, x, y)} \cdot dt \& dt + dx \& dx + dy \& dy$ ) :

> CotTen := CottonTensor(g) :

> CTJ := ToJet(CotTen, DepVars, notation = jetnumbers) :

> C := Connection(a000\*dt&t D\_t&t dt + a111\*dx&t D\_x&t dx + a222\*dy&t D\_y&t dy + a001\*(dt&t D\_t&t dx + dx&t D\_t&t dt) + a002\*(dt&t D\_t&t dy + dy&t D\_t&t dt) + a102\*(dx&t D\_t&t dy + dy&t D\_t&t dx) + a011\*(dt&t D\_x&t dx + dx&t D\_x&t dt) + a012\*(dt&t D\_x&t dy + dy&t D\_x&t dt) + a112\*(dx&t D\_x&t dy + dy&t D\_x&t dx) + a021\*(dt&t D\_y&t dx + dx&t D\_y&t dt) + a022\*(dt&t D\_y&t dy + dy&t D\_y&t dt) + a122\*(dx&t D\_y&t dy + dy&t D\_y&t dx) + a010\*dt&t D\_x&t dt + a121\*dx&t D\_y&t dx + a202\*dy&t D\_t&t dy + a020\*dt&t D\_y&t dt + a101\*dx&t D\_t&t dx + a212\*dy&t D\_x&t dy) :

> TorsionTensor(C);

$$0 \ dt \ D_t \ dt \quad (42)$$

> U1 :=  $\kappa_{11}(u(t, x, y)) \cdot \text{diff}(u(t, x, y), t) + \kappa_{12}(u(t, x, y)) \cdot \text{diff}(u(t, x, y), x) + \kappa_{13}(u(t, x, y)) \cdot \text{diff}(u(t, x, y), y)$  :

U2 :=  $\kappa_{21}(u(t, x, y)) \cdot \text{diff}(u(t, x, y), t) + \kappa_{22}(u(t, x, y)) \cdot \text{diff}(u(t, x, y), x) + \kappa_{23}(u(t, x, y)) \cdot \text{diff}(u(t, x, y), y)$  :

U3 :=  $\kappa_{31}(u(t, x, y)) \cdot \text{diff}(u(t, x, y), t) + \kappa_{32}(u(t, x, y)) \cdot \text{diff}(u(t, x, y), x) + \kappa_{33}(u(t, x, y)) \cdot \text{diff}(u(t, x, y), y)$  :

> Et := evalDG(DirectionalCovariantDerivative(D\_t, g, C) + U1·g) :

Ex := evalDG(DirectionalCovariantDerivative(D\_x, g, C) + U2·g) :

Ey := evalDG(DirectionalCovariantDerivative(D\_y, g, C) + U3·g) :

> Eq000 := TensorInnerProduct(g, Et, dt&t dt) :

Eq001 := TensorInnerProduct(g, Et, dt&t dx) :

Eq002 := TensorInnerProduct(g, Et, dt&t dy) :

Eq011 := TensorInnerProduct(g, Et, dx&t dx) :

Eq012 := TensorInnerProduct(g, Et, dx&t dy) :

Eq022 := TensorInnerProduct(g, Et, dy&t dy) :

Eq100 := TensorInnerProduct(g, Ex, dt&t dt) :

Eq101 := TensorInnerProduct(g, Ex, dt&t dx) :

Eq102 := TensorInnerProduct(g, Ex, dt&t dy) :

Eq111 := TensorInnerProduct(g, Ex, dx&t dx) :

Eq112 := TensorInnerProduct(g, Ex, dx&t dy) :

Eq122 := TensorInnerProduct(g, Ex, dy&t dy) :

```

Eq200 := TensorInnerProduct(g, Ey, dt &t dt) :
Eq201 := TensorInnerProduct(g, Ey, dt &t dx) :
Eq202 := TensorInnerProduct(g, Ey, dt &t dy) :
Eq211 := TensorInnerProduct(g, Ey, dx &t dx) :
Eq212 := TensorInnerProduct(g, Ey, dx &t dy) :
Eq222 := TensorInnerProduct(g, Ey, dy &t dy) :
> sA := solve( {Eq000=0, Eq001=0, Eq002=0, Eq011=0, Eq012=0, Eq022=0, Eq100=0,
Eq101=0, Eq102=0, Eq111=0, Eq112=0, Eq122=0, Eq200=0, Eq201=0, Eq202=0,
Eq211=0, Eq212=0, Eq222=0}, [a000, a001, a002, a010, a011, a012, a020, a021, a022,
a101, a102, a111, a112, a121, a122, a202, a212, a222] ) :
> C1 := evalDG( subs( {op(op(sA))}, C) ) :
> evalDG( CovariantDerivative(g, C1) + g &t (U1·dt + U2·dx + U3·dy));
0 dt dt dt
(43)

```

```

> R1 := CurvatureTensor(C1) : Ric1 := RicciTensor(R1) : T1 := SymmetrizeIndices(Ric1, [1, 2],
"Symmetric") : Res := evalDG(T1 - V·g) :
> NEQtt := ContractIndices(Res, D_t &t D_t, [[1, 1], [2, 2]]) : NEQtx := ContractIndices(Res,
D_t &t D_x, [[1, 1], [2, 2]]) :
NEQty := ContractIndices(Res, D_t &t D_y, [[1, 1], [2, 2]]) : NEQxx := ContractIndices(Res,
D_x &t D_x, [[1, 1], [2, 2]]) :
NEQxy := ContractIndices(Res, D_x &t D_y, [[1, 1], [2, 2]]) : NEQyy := ContractIndices(Res,
D_y &t D_y, [[1, 1], [2, 2]]) :
>
> DGsetup([t, x, y], [u], J2, 4) :
> de := DifferentialEquationData([F], [u1,1])

```

$$de := \left[ \{u_{1,1}\}, \left[ u_{2,2} + u_{3,3} + e^{u_{1,1}} u_1^2 + e^{u_{1,1}} u_{1,1} \right] \right] \quad (44)$$

```

> de2 := Prolong(de, 2) : deTRA := Transformation(de2) :
>
> Eq0 := Pullback(deTRA, ToJet(NEQtt, DepVars, notation = jetnumbers)) :
> VS := solve(Eq0, V) :
> Eq1 := numer(subs(V=VS, Pullback(deTRA, ToJet(NEQtx, DepVars, notation
= jetnumbers)))) :
Eq2 := numer(subs(V=VS, Pullback(deTRA, ToJet(NEQty, DepVars, notation
= jetnumbers)))) :
Eq3 := numer(subs(V=VS, Pullback(deTRA, ToJet(NEQxx, DepVars, notation
= jetnumbers)))) :
Eq4 := numer(subs(V=VS, Pullback(deTRA, ToJet(NEQxy, DepVars, notation
= jetnumbers)))) :
Eq5 := numer(subs(V=VS, Pullback(deTRA, ToJet(NEQyy, DepVars, notation
= jetnumbers)))) :
> simplify(diff(Eq1, u1,2))

```

$$-e^{u_{1,1}} (x_{22}(u_{1,1}) + x_{11}(u_{1,1})) \quad (45)$$

```

> simplify(diff(Eq1, u1,3))

```

$$-x_{23}(u_{1,1}) e^{u_{1,1}} \quad (46)$$

```

> simplify(diff(Eq1, u2,2))

```

$$-e^{u_{[1]}} \kappa_{12}(u_{[1]}) + \kappa_{21}(u_{[1]}) \quad (47)$$

> simplify(diff(Eq1, u<sub>2,3</sub>))

$$-\kappa_{13}(u_{[1]}) e^{u_{[1]}} \quad (48)$$

> simplify(diff(Eq1, u<sub>3,3</sub>))

$$\kappa_{21}(u_{[1]}) \quad (49)$$

> simplify(diff(Eq2, u<sub>1,2</sub>))

$$-\kappa_{32}(u_{[1]}) e^{u_{[1]}} \quad (50)$$

> simplify(diff(Eq2, u<sub>1,3</sub>))

$$-e^{u_{[1]}} (\kappa_{11}(u_{[1]}) + \kappa_{33}(u_{[1]})) \quad (51)$$

> simplify(diff(Eq2, u<sub>2,2</sub>))

$$\kappa_{31}(u_{[1]}) \quad (52)$$

> simplify(diff(Eq3, u<sub>3,3</sub>))

$$-2 - 2 \kappa_{11}(u_{[1]}) \quad (53)$$

**M** > DGsetup([t, x, y], M) :

> U1 := -diff(u(t, x, y), t) :

U2 := diff(u(t, x, y), x) :

U3 := diff(u(t, x, y), y) :

> Et := evalDG(DirectionalCovariantDerivative(D\_t, g, C) + U1·g) :

Ex := evalDG(DirectionalCovariantDerivative(D\_x, g, C) + U2·g) :

Ey := evalDG(DirectionalCovariantDerivative(D\_y, g, C) + U3·g) :

> Eq000 := TensorInnerProduct(g, Et, dt &t dt) :

Eq001 := TensorInnerProduct(g, Et, dt &t dx) :

Eq002 := TensorInnerProduct(g, Et, dt &t dy) :

Eq011 := TensorInnerProduct(g, Et, dx &t dx) :

Eq012 := TensorInnerProduct(g, Et, dx &t dy) :

Eq022 := TensorInnerProduct(g, Et, dy &t dy) :

Eq100 := TensorInnerProduct(g, Ex, dt &t dt) :

Eq101 := TensorInnerProduct(g, Ex, dt &t dx) :

Eq102 := TensorInnerProduct(g, Ex, dt &t dy) :

Eq111 := TensorInnerProduct(g, Ex, dx &t dx) :

Eq112 := TensorInnerProduct(g, Ex, dx &t dy) :

Eq122 := TensorInnerProduct(g, Ex, dy &t dy) :

Eq200 := TensorInnerProduct(g, Ey, dt &t dt) :

Eq201 := TensorInnerProduct(g, Ey, dt &t dx) :

Eq202 := TensorInnerProduct(g, Ey, dt &t dy) :

Eq211 := TensorInnerProduct(g, Ey, dx &t dx) :

Eq212 := TensorInnerProduct(g, Ey, dx &t dy) :

Eq222 := TensorInnerProduct(g, Ey, dy &t dy) :

> sA := solve({Eq000=0, Eq001=0, Eq002=0, Eq011=0, Eq012=0, Eq022=0, Eq100=0, Eq101=0, Eq102=0, Eq111=0, Eq112=0, Eq122=0, Eq200=0, Eq201=0, Eq202=0, Eq211=0, Eq212=0, Eq222=0}, [a000, a001, a002, a010, a011, a012, a020, a021, a022,

$$\begin{aligned}
& a101, a102, a111, a112, a121, a122, a202, a212, a222] : \\
& > C1 := evalDG( subs( \{ op( op( sA ) ) \}, C ) ) : \\
& > evalDG( CovariantDerivative(g, C1) + g \&t ( U1 \cdot dt + U2 \cdot dx + U3 \cdot dy ) ); \\
& \quad \quad \quad 0 \, dt \, dt \, dt
\end{aligned} \tag{54}$$

$$\begin{aligned}
& > R1 := CurvatureTensor(C1) : Ric1 := RicciTensor(R1) : T1 := SymmetrizeIndices(Ric1, [1, 2], \\
& \quad \text{"Symmetric"}) : Res := evalDG(T1 - V \cdot g) : \\
& > NEQtt := TensorInnerProduct(g, Res, dt \&t dt) : NEQtx := TensorInnerProduct(g, Res, dt \\
& \quad \&t dx) : \\
& NEQty := TensorInnerProduct(g, Res, dt \&t dy) : NEQxx := TensorInnerProduct(g, Res, dx \\
& \quad \&t dx) : \\
& NEQxy := TensorInnerProduct(g, Res, dx \&t dy) : NEQyy := TensorInnerProduct(g, Res, dy \\
& \quad \&t dy) : \\
& > \\
& > DGsetup([t, x, y], [u], J2, 4) : \\
& > de := DifferentialEquationData([F], [u_{1,1}]) \\
& \quad \quad \quad de := \left[ \{ u_{1,1} \}, \left[ u_{2,2} + u_{3,3} + e^{u_{1,1}} u_1^2 + e^{u_{1,1}} u_{1,1} \right] \right]
\end{aligned} \tag{55}$$

$$\begin{aligned}
& > de2 := Prolong(de, 2) : deTRA := Transformation(de2) : \\
& > \\
& > Eq0 := Pullback(deTRA, ToJet(NEQtt, DepVars, notation = jetnumbers)) : \\
& > VS := solve(Eq0, V) : \\
& > Eq1 := numer(subs(V = VS, Pullback(deTRA, ToJet(NEQtx, DepVars, notation \\
& \quad = jetnumbers)))) : \\
& Eq2 := numer(subs(V = VS, Pullback(deTRA, ToJet(NEQty, DepVars, notation \\
& \quad = jetnumbers)))) : \\
& Eq3 := numer(subs(V = VS, Pullback(deTRA, ToJet(NEQxx, DepVars, notation \\
& \quad = jetnumbers)))) : \\
& Eq4 := numer(subs(V = VS, Pullback(deTRA, ToJet(NEQxy, DepVars, notation \\
& \quad = jetnumbers)))) : \\
& Eq5 := numer(subs(V = VS, Pullback(deTRA, ToJet(NEQyy, DepVars, notation \\
& \quad = jetnumbers)))) : \\
& > simplify([Eq1, Eq2, Eq3, Eq4, Eq5]) \\
& \quad \quad \quad [0, 0, 0, 0, 0]
\end{aligned} \tag{56}$$

$$\begin{aligned}
& > \text{simplify}(VS) \\
& \quad \quad \quad -\frac{1}{2} e^{u_{1,1}} u_1^2 - u_{2,2} - u_{3,3}
\end{aligned} \tag{57}$$

Perfect - the linerization metric is again EW on the equation.

> Let us checkd that the Coton tensor does not vanish

$$\begin{aligned}
& \text{J2} > ToJet(ContractIndices(CotTen, dt \&t dx, [[1, 1], [2, 2]]), DepVars, notation \\
& \quad = jetnumbers) \\
& \quad \quad \quad \frac{1}{4} u_3 u_{2,2} - \frac{1}{4} u_{2,2,3} + \frac{1}{4} u_3 u_{3,3} - \frac{1}{4} u_{3,3,3}
\end{aligned} \tag{58}$$

$$\begin{aligned}
& > Pullback\left(deTRA, \frac{1}{4} u_3 u_{2,2} - \frac{1}{4} u_{2,2,3} + \frac{1}{4} u_3 u_{3,3} - \frac{1}{4} u_{3,3,3}\right) \\
& \quad \quad \quad \frac{1}{4} u_3 u_{2,2} - \frac{1}{4} u_{2,2,3} + \frac{1}{4} u_3 u_{3,3} - \frac{1}{4} u_{3,3,3}
\end{aligned} \tag{59}$$

```
> restart : with(DifferentialGeometry) : with(Tensor) : with(Tools) : with(JetCalculus) :
with(LinearAlgebra) : with(PDEtools, D_Dx, declare, ToJet, FromJet) :
```

[Equation 3]  $(e^u u)_{xx} + 2u_{xy} + (e^u u)_{tt} = 0$

```
> DGsetup([t, x, y], [u], J2) :
```

```
> F := TotalDiff(exp(u[]) - u[], [2, 2]) + 2 u[2, 3] + TotalDiff(exp(u[]), [1, 1])
```

$$F := e^{u_{[1]}} u_{2,2}^2 + (e^{u_{[1]}} - 1) u_{2,2} + 2 u_{2,3} + e^{u_{[1]}} u_1^2 + e^{u_{[1]}} u_{1,1} \quad (60)$$

```
> A := Matrix( [[ [diff(F, u[1, 1]), 1/2 diff(F, u[1, 2]), 1/2 diff(F, u[1, 3])], [1/2 diff(F, u[1, 2]), diff(F, u[2, 2]), 1/2 diff(F, u[2, 3])], [1/2 diff(F, u[1, 3]), 1/2 diff(F, u[2, 3]), diff(F, u[3, 3])]] ) : AA := expand(MatrixInverse(A))
```

$$AA := \begin{bmatrix} \frac{1}{e^{u_{[1]}}} & 0 & 0 \\ 0 & 0 & 1 \\ 0 & 1 & -e^{u_{[1]}} + 1 \end{bmatrix} \quad (61)$$

```
> DepVars := [u(t, x, y)] : FromJet(AA, DepVars)
```

$$\begin{bmatrix} \frac{1}{e^{u(t, x, y)}} & 0 & 0 \\ 0 & 0 & 1 \\ 0 & 1 & -e^{u(t, x, y)} + 1 \end{bmatrix} \quad (62)$$

```
> DGsetup([t, x, y], M) :
```

```
> g := evalDG(e^{-u(t, x, y)} . dt &t dt + (dx &t dy + dy &t dx) + (1 - e^{u(t, x, y)}) . dy &t dy) :
```

```
> CotTen := CottonTensor(g) :
```

```
> CTJ := ToJet(CotTen, DepVars, notation = jetnumbers) :
```

```
> C := Connection(a000 * dt &t D_t &t dt + a111 * dx &t D_x &t dx + a222 * dy &t D_y &t dy
+ a001 * (dt &t D_t &t dx + dx &t D_t &t dt) + a002 * (dt &t D_t &t dy + dy &t D_t
&t dt) + a102 * (dx &t D_t &t dy + dy &t D_t &t dx) + a011 * (dt &t D_x &t dx + dx
&t D_x &t dt) + a012 * (dt &t D_x &t dy + dy &t D_x &t dt) + a112 * (dx &t D_x &t dy
+ dy &t D_x &t dx) + a021 * (dt &t D_y &t dx + dx &t D_y &t dt) + a022 * (dt &t D_y
```

$$\begin{aligned} & \&t \, dy + dy \&t \, D\_y \&t \, dt) + a122 * (dx \&t \, D\_y \&t \, dy + dy \&t \, D\_y \&t \, dx) + a010 * dt \\ & \&t \, D\_x \&t \, dt + a121 * dx \&t \, D\_y \&t \, dx + a202 * dy \&t \, D\_t \&t \, dy + a020 * dt \&t \, D\_y \&t \, dt \\ & + a101 * dx \&t \, D\_t \&t \, dx + a212 * dy \&t \, D\_x \&t \, dy) : \end{aligned}$$

> TorsionTensor(C);

$0 \, dt \, D\_t \, dt$

(63)

> U1 :=  $\kappa11(u(t, x, y)) \cdot \text{diff}(u(t, x, y), t) + \kappa12(u(t, x, y)) \cdot \text{diff}(u(t, x, y), x) + \kappa13(u(t, x, y)) \cdot \text{diff}(u(t, x, y), y) :$   
U2 :=  $\kappa21(u(t, x, y)) \cdot \text{diff}(u(t, x, y), t) + \kappa22(u(t, x, y)) \cdot \text{diff}(u(t, x, y), x) + \kappa23(u(t, x, y)) \cdot \text{diff}(u(t, x, y), y) :$   
U3 :=  $\kappa31(u(t, x, y)) \cdot \text{diff}(u(t, x, y), t) + \kappa32(u(t, x, y)) \cdot \text{diff}(u(t, x, y), x) + \kappa33(u(t, x, y)) \cdot \text{diff}(u(t, x, y), y) :$

> Et := evalDG(DirectionalCovariantDerivative(D\_t, g, C) + U1·g) :  
Ex := evalDG(DirectionalCovariantDerivative(D\_x, g, C) + U2·g) :  
Ey := evalDG(DirectionalCovariantDerivative(D\_y, g, C) + U3·g) :

> Eq000 := TensorInnerProduct(g, Et, dt &t dt) :  
Eq001 := TensorInnerProduct(g, Et, dt &t dx) :  
Eq002 := TensorInnerProduct(g, Et, dt &t dy) :  
Eq011 := TensorInnerProduct(g, Et, dx &t dx) :  
Eq012 := TensorInnerProduct(g, Et, dx &t dy) :  
Eq022 := TensorInnerProduct(g, Et, dy &t dy) :  
Eq100 := TensorInnerProduct(g, Ex, dt &t dt) :  
Eq101 := TensorInnerProduct(g, Ex, dt &t dx) :  
Eq102 := TensorInnerProduct(g, Ex, dt &t dy) :  
Eq111 := TensorInnerProduct(g, Ex, dx &t dx) :  
Eq112 := TensorInnerProduct(g, Ex, dx &t dy) :  
Eq122 := TensorInnerProduct(g, Ex, dy &t dy) :  
Eq200 := TensorInnerProduct(g, Ey, dt &t dt) :  
Eq201 := TensorInnerProduct(g, Ey, dt &t dx) :  
Eq202 := TensorInnerProduct(g, Ey, dt &t dy) :  
Eq211 := TensorInnerProduct(g, Ey, dx &t dx) :  
Eq212 := TensorInnerProduct(g, Ey, dx &t dy) :  
Eq222 := TensorInnerProduct(g, Ey, dy &t dy) :

> sA := solve( {Eq000=0, Eq001=0, Eq002=0, Eq011=0, Eq012=0, Eq022=0, Eq100=0, Eq101=0, Eq102=0, Eq111=0, Eq112=0, Eq122=0, Eq200=0, Eq201=0, Eq202=0, Eq211=0, Eq212=0, Eq222=0}, [a000, a001, a002, a010, a011, a012, a020, a021, a022, a101, a102, a111, a112, a121, a122, a202, a212, a222] ) :

> C1 := evalDG( subs( {op(op(sA))}, C) ) :

> evalDG(CovariantDerivative(g, C1) + g &t (U1·dt + U2·dx + U3·dy));

$0 \, dt \, dt \, dt$

(64)

> R1 := CurvatureTensor(C1) : Ric1 := RicciTensor(R1) : T1 := SymmetrizeIndices(Ric1, [1, 2], "Symmetric") : Res := evalDG(T1 - V·g) :

> NEQt1 := ContractIndices(Res, D\_t &t D\_t, [[1, 1], [2, 2]]) : NEQt2 := ContractIndices(Res, D\_t &t D\_x, [[1, 1], [2, 2]]) :  
NEQty := ContractIndices(Res, D\_t &t D\_y, [[1, 1], [2, 2]]) : NEQxx := ContractIndices(Res, D\_x &t D\_x, [[1, 1], [2, 2]]) :  
NEQxy := ContractIndices(Res, D\_x &t D\_y, [[1, 1], [2, 2]]) : NEQyy := ContractIndices(Res, D\_y &t D\_y, [[1, 1], [2, 2]]) :

>

> DGsetup([t, x, y], [u], J2, 4) :



$$\begin{aligned} &> de := DifferentialEquationData([F], [u_{1,1}]) \\ &\quad de := \left[ \{u_{1,1}\}, \left[ e^{u_{1,1}} u_{2,2}^2 + (e^{u_{1,1}} - 1) u_{2,2} + 2 u_{2,3} + e^{u_{1,1}} u_1^2 + e^{u_{1,1}} u_{1,1} \right] \right] \end{aligned} \quad (65)$$

$$> de2 := Prolong(de, 2) : deTRA := Transformation(de2) :$$

>

$$> Eq0 := Pullback(deTRA, ToJet(NEQtt, DepVars, notation = jetnumbers)) :$$

$$> VS := solve(Eq0, V) :$$

$$> Eq1 := numer(subs(V=VS, Pullback(deTRA, ToJet(NEQtx, DepVars, notation = jetnumbers)))) :$$

$$Eq2 := numer(subs(V=VS, Pullback(deTRA, ToJet(NEQty, DepVars, notation = jetnumbers)))) :$$

$$Eq3 := numer(subs(V=VS, Pullback(deTRA, ToJet(NEQxx, DepVars, notation = jetnumbers)))) :$$

$$Eq4 := numer(subs(V=VS, Pullback(deTRA, ToJet(NEQxy, DepVars, notation = jetnumbers)))) :$$

$$Eq5 := numer(subs(V=VS, Pullback(deTRA, ToJet(NEQyy, DepVars, notation = jetnumbers)))) :$$

$$\text{J2 } > SQE1 := simplify(diff(Eq1, u_{1,2}))$$

$$SQE1 := -e^{u_{1,1}} (\kappa_{22}(u_{1,1}) + \kappa_{11}(u_{1,1})) \quad (66)$$

$$> simplify(diff(Eq1, u_{1,3}))$$

$$-\kappa_{23}(u_{1,1}) e^{u_{1,1}} \quad (67)$$

$$> simplify(diff(Eq1, u_{2,2}))$$

$$-e^{u_{1,1}} \kappa_{12}(u_{1,1}) + \kappa_{21}(u_{1,1}) e^{u_{1,1}} - \kappa_{21}(u_{1,1}) \quad (68)$$

$$> simplify(diff(Eq1, u_{2,3}))$$

$$-\kappa_{13}(u_{1,1}) e^{u_{1,1}} + 2 \kappa_{21}(u_{1,1}) \quad (69)$$

$$> simplify(diff(Eq2, u_{1,2}))$$

$$-\kappa_{32}(u_{1,1}) e^{u_{1,1}} - 2 e^{2u_{1,1}} \quad (70)$$

$$> simplify(diff(Eq2, u_{1,3}))$$

$$-e^{u_{1,1}} (\kappa_{33}(u_{1,1}) + \kappa_{11}(u_{1,1})) \quad (71)$$

$$> simplify(diff(Eq2, u_{2,2}))$$

$$\kappa_{31}(u_{1,1}) (e^{u_{1,1}} - 1) \quad (72)$$

$$> simplify(diff(Eq2, u_{2,3}))$$

$$-e^{u_{1,1}} \kappa_{12}(u_{1,1}) + 2 \kappa_{31}(u_{1,1}) \quad (73)$$

$$> simplify(diff(Eq3, u_{1,2}))$$

$$-2 \kappa_{21}(u_{1,1}) \quad (74)$$

$$\begin{aligned} &> \text{simplify}(\text{diff}(Eq3, u_{2,2})) \\ &\quad -2 \kappa_{22}(u_{[]}) + 2 \end{aligned} \quad (75)$$

$$\begin{aligned} &\mathbf{M} > \text{DGsetup}([t, x, y], M) : \\ &> U1 := -\text{diff}(u(t, x, y), t) : \\ &\quad U2 := \text{diff}(u(t, x, y), x) : \\ &\quad U3 := -2e^{u(t, x, y)} \cdot \text{diff}(u(t, x, y), x) + \text{diff}(u(t, x, y), y) : \\ &> Et := \text{evalDG}(\text{DirectionalCovariantDerivative}(D\_t, g, C) + U1 \cdot g) : \\ &\quad Ex := \text{evalDG}(\text{DirectionalCovariantDerivative}(D\_x, g, C) + U2 \cdot g) : \\ &\quad Ey := \text{evalDG}(\text{DirectionalCovariantDerivative}(D\_y, g, C) + U3 \cdot g) : \\ &> Eq000 := \text{TensorInnerProduct}(g, Et, dt \& t dt) : \\ &\quad Eq001 := \text{TensorInnerProduct}(g, Et, dt \& t dx) : \\ &\quad Eq002 := \text{TensorInnerProduct}(g, Et, dt \& t dy) : \\ &\quad Eq011 := \text{TensorInnerProduct}(g, Et, dx \& t dx) : \\ &\quad Eq012 := \text{TensorInnerProduct}(g, Et, dx \& t dy) : \\ &\quad Eq022 := \text{TensorInnerProduct}(g, Et, dy \& t dy) : \\ &\quad Eq100 := \text{TensorInnerProduct}(g, Ex, dt \& t dt) : \\ &\quad Eq101 := \text{TensorInnerProduct}(g, Ex, dt \& t dx) : \\ &\quad Eq102 := \text{TensorInnerProduct}(g, Ex, dt \& t dy) : \\ &\quad Eq111 := \text{TensorInnerProduct}(g, Ex, dx \& t dx) : \\ &\quad Eq112 := \text{TensorInnerProduct}(g, Ex, dx \& t dy) : \\ &\quad Eq122 := \text{TensorInnerProduct}(g, Ex, dy \& t dy) : \\ &\quad Eq200 := \text{TensorInnerProduct}(g, Ey, dt \& t dt) : \\ &\quad Eq201 := \text{TensorInnerProduct}(g, Ey, dt \& t dx) : \\ &\quad Eq202 := \text{TensorInnerProduct}(g, Ey, dt \& t dy) : \\ &\quad Eq211 := \text{TensorInnerProduct}(g, Ey, dx \& t dx) : \\ &\quad Eq212 := \text{TensorInnerProduct}(g, Ey, dx \& t dy) : \\ &\quad Eq222 := \text{TensorInnerProduct}(g, Ey, dy \& t dy) : \\ &> sA := \text{solve}(\{Eq000=0, Eq001=0, Eq002=0, Eq011=0, Eq012=0, Eq022=0, Eq100=0, \\ &\quad Eq101=0, Eq102=0, Eq111=0, Eq112=0, Eq122=0, Eq200=0, Eq201=0, Eq202=0, \\ &\quad Eq211=0, Eq212=0, Eq222=0\}, [a000, a001, a002, a010, a011, a012, a020, a021, a022, \\ &\quad a101, a102, a111, a112, a121, a122, a202, a212, a222]) : \\ &> C1 := \text{evalDG}(\text{subs}(\{\text{op}(\text{op}(sA))\}, C)) : \\ &> \text{evalDG}(\text{CovariantDerivative}(g, C1) + g \& t (U1 \cdot dt + U2 \cdot dx + U3 \cdot dy)); \\ &\quad 0 \, dt \, dt \, dt \end{aligned} \quad (76)$$

$$\begin{aligned} &> R1 := \text{CurvatureTensor}(C1) : Ric1 := \text{RicciTensor}(R1) : T1 := \text{SymmetrizeIndices}(Ric1, [1, 2], \\ &\quad \text{"Symmetric"}) : Res := \text{evalDG}(T1 - V \cdot g) : \\ &> NEQtt := \text{TensorInnerProduct}(g, Res, dt \& t dt) : NEQtx := \text{TensorInnerProduct}(g, Res, dt \\ &\quad \& t dx) : \\ &\quad NEQty := \text{TensorInnerProduct}(g, Res, dt \& t dy) : NEQxx := \text{TensorInnerProduct}(g, Res, dx \\ &\quad \& t dx) : \\ &\quad NEQxy := \text{TensorInnerProduct}(g, Res, dx \& t dy) : NEQyy := \text{TensorInnerProduct}(g, Res, dy \\ &\quad \& t dy) : \\ &> \\ &> \text{DGsetup}([t, x, y], [u], J2, 4) : \\ &> de := \text{DifferentialEquationData}([F], [u_{1,1}]) \\ &\quad de := \left[ \{u_{1,1}\}, \left[ e^{u_{[]}} u_{2,2}^2 + \left( e^{u_{[]}} - 1 \right) u_{2,2} + 2 u_{2,3} + e^{u_{[]}} u_1^2 + e^{u_{[]}} u_{1,1} \right] \right] \end{aligned} \quad (77)$$



$$F := u_{1,2} - u_{[,] } u_{2,2} - u_2^2 - u_{3,3} \quad (82)$$

>  $A := \text{Matrix}\left(\left[\left[\text{diff}(F, u[1, 1]), \frac{1}{2} \text{diff}(F, u[1, 2]), \frac{1}{2} \text{diff}(F, u[1, 3])\right], \left[\frac{1}{2} \text{diff}(F, u[1, 2]), \text{diff}(F, u[2, 2]), \frac{1}{2} \text{diff}(F, u[2, 3])\right], \left[\frac{1}{2} \text{diff}(F, u[1, 3]), \frac{1}{2} \text{diff}(F, u[2, 3]), \text{diff}(F, u[3, 3])\right]\right]\right) : AA := \text{expand}(\text{MatrixInverse}(A))$

$$AA := \begin{bmatrix} 4 u_{[,] } & 2 & 0 \\ 2 & 0 & 0 \\ 0 & 0 & -1 \end{bmatrix} \quad (83)$$

>  $\text{DepVars} := [u(t, x, y)] : \text{FromJet}(AA, \text{DepVars})$

$$\begin{bmatrix} 4 u(t, x, y) & 2 & 0 \\ 2 & 0 & 0 \\ 0 & 0 & -1 \end{bmatrix} \quad (84)$$

>  $\text{DGsetup}([t, x, y], M) :$

>  $g := \text{evalDG}(4 u(t, x, y) \cdot dt \& t dt + 2(dx \& t dt + dt \& t dx) - dy \& t dy) :$

>  $\text{CotTen} := \text{CottonTensor}(g) :$

>  $\text{CTJ} := \text{ToJet}(\text{CotTen}, \text{DepVars}, \text{notation} = \text{jetnumbers}) :$

>  $C := \text{Connection}(a000 \cdot dt \& t D\_t \& t dt + a111 \cdot dx \& t D\_x \& t dx + a222 \cdot dy \& t D\_y \& t dy + a001 \cdot (dt \& t D\_t \& t dx + dx \& t D\_t \& t dt) + a002 \cdot (dt \& t D\_t \& t dy + dy \& t D\_t \& t dt) + a102 \cdot (dx \& t D\_t \& t dy + dy \& t D\_t \& t dx) + a011 \cdot (dt \& t D\_x \& t dx + dx \& t D\_x \& t dt) + a012 \cdot (dt \& t D\_x \& t dy + dy \& t D\_x \& t dt) + a112 \cdot (dx \& t D\_x \& t dy + dy \& t D\_x \& t dx) + a021 \cdot (dt \& t D\_y \& t dx + dx \& t D\_y \& t dt) + a022 \cdot (dt \& t D\_y \& t dy + dy \& t D\_y \& t dt) + a122 \cdot (dx \& t D\_y \& t dy + dy \& t D\_y \& t dx) + a010 \cdot dt \& t D\_x \& t dt + a121 \cdot dx \& t D\_y \& t dx + a202 \cdot dy \& t D\_t \& t dy + a020 \cdot dt \& t D\_y \& t dt + a101 \cdot dx \& t D\_t \& t dx + a212 \cdot dy \& t D\_x \& t dy) :$

>  $\text{TorsionTensor}(C);$

$$0 dt D\_t dt \quad (85)$$

>  $U1 := \kappa11(u(t, x, y)) \cdot \text{diff}(u(t, x, y), t) + \kappa12(u(t, x, y)) \cdot \text{diff}(u(t, x, y), x) + \kappa13(u(t, x, y)) \cdot \text{diff}(u(t, x, y), y) :$

$U2 := \kappa21(u(t, x, y)) \cdot \text{diff}(u(t, x, y), t) + \kappa22(u(t, x, y)) \cdot \text{diff}(u(t, x, y), x) + \kappa23(u(t, x, y)) \cdot \text{diff}(u(t, x, y), y) :$

$U3 := \kappa31(u(t, x, y)) \cdot \text{diff}(u(t, x, y), t) + \kappa32(u(t, x, y)) \cdot \text{diff}(u(t, x, y), x) + \kappa33(u(t, x, y)) \cdot \text{diff}(u(t, x, y), y) :$

>  $Et := \text{evalDG}(\text{DirectionalCovariantDerivative}(D\_t, g, C) + U1 \cdot g) :$

$Ex := \text{evalDG}(\text{DirectionalCovariantDerivative}(D\_x, g, C) + U2 \cdot g) :$

$Ey := \text{evalDG}(\text{DirectionalCovariantDerivative}(D\_y, g, C) + U3 \cdot g) :$

>  $Eq000 := \text{TensorInnerProduct}(g, Et, dt \& t dt) :$

$Eq001 := \text{TensorInnerProduct}(g, Et, dt \& t dx) :$

$Eq002 := \text{TensorInnerProduct}(g, Et, dt \& t dy) :$

$Eq011 := \text{TensorInnerProduct}(g, Et, dx \& t dx) :$

$Eq012 := \text{TensorInnerProduct}(g, Et, dx \& t dy) :$

$Eq022 := \text{TensorInnerProduct}(g, Et, dy \& t dy) :$

$Eq100 := \text{TensorInnerProduct}(g, Ex, dt \& t dt) :$

```

Eq101 := TensorInnerProduct(g, Ex, dt &t dx) :
Eq102 := TensorInnerProduct(g, Ex, dt &t dy) :
Eq111 := TensorInnerProduct(g, Ex, dx &t dx) :
Eq112 := TensorInnerProduct(g, Ex, dx &t dy) :
Eq122 := TensorInnerProduct(g, Ex, dy &t dy) :
Eq200 := TensorInnerProduct(g, Ey, dt &t dt) :
Eq201 := TensorInnerProduct(g, Ey, dt &t dx) :
Eq202 := TensorInnerProduct(g, Ey, dt &t dy) :
Eq211 := TensorInnerProduct(g, Ey, dx &t dx) :
Eq212 := TensorInnerProduct(g, Ey, dx &t dy) :
Eq222 := TensorInnerProduct(g, Ey, dy &t dy) :

```

```

> sA := solve( {Eq000=0, Eq001=0, Eq002=0, Eq011=0, Eq012=0, Eq022=0, Eq100=0,
Eq101=0, Eq102=0, Eq111=0, Eq112=0, Eq122=0, Eq200=0, Eq201=0, Eq202=0,
Eq211=0, Eq212=0, Eq222=0}, [a000, a001, a002, a010, a011, a012, a020, a021, a022,
a101, a102, a111, a112, a121, a122, a202, a212, a222] ) :

```

```

> C1 := evalDG( subs( {op(op(sA))}, C) ) :

```

```

> evalDG( CovariantDerivative(g, C1) + g &t (U1·dt + U2·dx + U3·dy) );
0 dt dt dt

```

(86)

```

> R1 := CurvatureTensor(C1) : Ric1 := RicciTensor(R1) : T1 := SymmetrizeIndices(Ric1, [1, 2],
"Symmetric") : Res := evalDG(T1 - V·g) :

```

```

> NEQt1 := ContractIndices(Res, D_t &t D_t, [[1, 1], [2, 2]]) : NEQt2 := ContractIndices(Res,
D_t &t D_x, [[1, 1], [2, 2]]) :
NEQt3 := ContractIndices(Res, D_t &t D_y, [[1, 1], [2, 2]]) : NEQt4 := ContractIndices(Res,
D_x &t D_x, [[1, 1], [2, 2]]) :
NEQt5 := ContractIndices(Res, D_x &t D_y, [[1, 1], [2, 2]]) : NEQt6 := ContractIndices(Res,
D_y &t D_y, [[1, 1], [2, 2]]) :

```

```

> DGsetup([t, x, y], [u], J2, 4) :

```

```

> de := DifferentialEquationData([F], [u1,2])

```

$de := \left[ \{u_{1,2}\}, \left[ u_{1,2} - u_{\square} u_{2,2} - u_{2,2}^2 - u_{3,3} \right] \right]$

(87)

```

> de2 := Prolong(de, 2) : deTRA := Transformation(de2) :

```

```

> Eq0 := Pullback(deTRA, ToJet(NEQt1, DepVars, notation = jetnumbers)) :

```

```

> VS := solve(Eq0, V) :

```

```

> Eq1 := numer(subs(V=VS, Pullback(deTRA, ToJet(NEQt2, DepVars, notation
=jetnumbers)))) :

```

```

Eq2 := numer(subs(V=VS, Pullback(deTRA, ToJet(NEQt3, DepVars, notation
=jetnumbers)))) :

```

```

Eq3 := numer(subs(V=VS, Pullback(deTRA, ToJet(NEQt4, DepVars, notation
=jetnumbers)))) :

```

```

Eq4 := numer(subs(V=VS, Pullback(deTRA, ToJet(NEQt5, DepVars, notation
=jetnumbers)))) :

```

```

Eq5 := numer(subs(V=VS, Pullback(deTRA, ToJet(NEQt6, DepVars, notation
=jetnumbers)))) :

```

```

> simplify(diff(Eq1, u1,1))

```

$-2 u_{\square} \times 21(u_{\square}) + 2 \times 11(u_{\square})$

(88)

```

> simplify(diff(Eq1, u1,3))

```

```

=
-2 u[] x23(u[]) + 2 x13(u[]) (89)
> simplify(diff(Eq1, u2, 2))
-2 u[]^2 x11(u[]) - 2 u[]^2 x22(u[]) (90)
> simplify(diff(Eq1, u2, 3))
-2 u[] x13(u[]) (91)
> simplify(diff(Eq1, u3, 3))
-8 - 2 u[] x11(u[]) - 2 u[] x22(u[]) + 2 x12(u[]) (92)
> simplify(diff(Eq2, u1, 1))
-x31(u[]) (93)
> simplify(diff(Eq2, u1, 3))
-x11(u[]) - x33(u[]) (94)
> simplify(diff(Eq2, u2, 2))
-u[] x32(u[]) (95)
> simplify(diff(Eq2, u2, 3))
4 - x12(u[]) (96)
> simplify(diff(Eq3, u2, 2))
-2 u[] x21(u[]) - 2 x22(u[]) (97)
> simplify(diff(Eq3, u3, 3))
-2 x21(u[]) (98)
> simplify(diff(Eq4, u2, 3))
-x22(u[]) - x33(u[]) (99)
M > DGsetup([t, x, y], M) :
> U1 := 4 diff(u(t, x, y), x) :
U2 := 0 :
U3 := 0 :
> Et := evalDG(DirectionalCovariantDerivative(D_t, g, C) + U1.g) :
Ex := evalDG(DirectionalCovariantDerivative(D_x, g, C) + U2.g) :
Ey := evalDG(DirectionalCovariantDerivative(D_y, g, C) + U3.g) :
> Eq000 := TensorInnerProduct(g, Et, dt &t dt) :
Eq001 := TensorInnerProduct(g, Et, dt &t dx) :
Eq002 := TensorInnerProduct(g, Et, dt &t dy) :
Eq011 := TensorInnerProduct(g, Et, dx &t dx) :
Eq012 := TensorInnerProduct(g, Et, dx &t dy) :
Eq022 := TensorInnerProduct(g, Et, dy &t dy) :
Eq100 := TensorInnerProduct(g, Ex, dt &t dt) :
Eq101 := TensorInnerProduct(g, Ex, dt &t dx) :
Eq102 := TensorInnerProduct(g, Ex, dt &t dy) :
Eq111 := TensorInnerProduct(g, Ex, dx &t dx) :
Eq112 := TensorInnerProduct(g, Ex, dx &t dy) :
Eq122 := TensorInnerProduct(g, Ex, dy &t dy) :

```

```
Eq200 := TensorInnerProduct(g, Ey, dt &t dt) :
Eq201 := TensorInnerProduct(g, Ey, dt &t dx) :
Eq202 := TensorInnerProduct(g, Ey, dt &t dy) :
Eq211 := TensorInnerProduct(g, Ey, dx &t dx) :
Eq212 := TensorInnerProduct(g, Ey, dx &t dy) :
Eq222 := TensorInnerProduct(g, Ey, dy &t dy) :
```

```
> sA := solve( {Eq000=0, Eq001=0, Eq002=0, Eq011=0, Eq012=0, Eq022=0, Eq100=0,
Eq101=0, Eq102=0, Eq111=0, Eq112=0, Eq122=0, Eq200=0, Eq201=0, Eq202=0,
Eq211=0, Eq212=0, Eq222=0}, [a000, a001, a002, a010, a011, a012, a020, a021, a022,
a101, a102, a111, a112, a121, a122, a202, a212, a222] ) :
```

```
> C1 := evalDG( subs( {op(op(sA))}, C) ) :
```

```
> evalDG( CovariantDerivative(g, C1) + g &t (U1·dt + U2·dx + U3·dy) );
0 dt dt dt
```

(100)

```
> R1 := CurvatureTensor(C1) : Ric1 := RicciTensor(R1) : T1 := SymmetrizeIndices(Ric1, [1, 2],
"Symmetric") : Res := evalDG(T1 - V·g) :
```

```
> NEQt := TensorInnerProduct(g, Res, dt &t dt) : NEQtX := TensorInnerProduct(g, Res, dt
&t dx) :
```

```
NEQty := TensorInnerProduct(g, Res, dt &t dy) : NEQxx := TensorInnerProduct(g, Res, dx
&t dx) :
```

```
NEQxy := TensorInnerProduct(g, Res, dx &t dy) : NEQyy := TensorInnerProduct(g, Res, dy
&t dy) :
```

```
>
```

```
> DGsetup( [t, x, y], [u], J2, 4) :
```

```
> de := DifferentialEquationData( [F], [u1,2] )
```

$de := \left[ \{u_{1,2}\}, \left[ u_{1,2} - u_{[1} u_{2,2} - u_{2,2}^2 - u_{3,3} \right] \right]$

(101)

```
> de2 := Prolong(de, 2) : deTRA := Transformation(de2) :
```

```
>
```

```
> Eq0 := Pullback(deTRA, ToJet(NEQtX, DepVars, notation = jetnumbers)) :
```

```
> VS := solve(Eq0, V) :
```

```
> Eq1 := numer(subs(V=VS, Pullback(deTRA, ToJet(NEQty, DepVars, notation
= jetnumbers)))) :
```

```
Eq2 := numer(subs(V=VS, Pullback(deTRA, ToJet(NEQxx, DepVars, notation
= jetnumbers)))) :
```

```
Eq3 := numer(subs(V=VS, Pullback(deTRA, ToJet(NEQxy, DepVars, notation
= jetnumbers)))) :
```

```
Eq4 := numer(subs(V=VS, Pullback(deTRA, ToJet(NEQyy, DepVars, notation
= jetnumbers)))) :
```

```
Eq5 := numer(subs(V=VS, Pullback(deTRA, ToJet(NEQyy, DepVars, notation
= jetnumbers)))) :
```

```
> simplify( [Eq1, Eq2, Eq3, Eq4, Eq5] )
```

$[0, 0, 0, 0, 0]$

(102)

```
> simplify(VS)
```

$-u_{2,2}$

(103)

Perfect - the linerization metric is again EW on the equation.

```
>
```

Let us checdk that the Coton tensor does not vanish

```
J2 > ToJet(ContractIndices(CotTen, dt &t dx, [[1, 1], [2, 2]]), DepVars, notation
```

$$=jetnumbers)$$

$$-\frac{1}{4}u_{2,2,3} \quad (104)$$

$$\triangleright \text{Pullback}\left(deTRA, -\frac{1}{4} u_{2,2,3}\right)$$

$$-\frac{1}{4}u_{2,2,3} \quad (105)$$

```
> restart : with(DifferentialGeometry) : with(Tensor) : with(Tools) : with(JetCalculus) :
_ with(LinearAlgebra) : with(PDEtools, D_Dx, declare, ToJet, FromJet) :
```

[Equation 5]  $(u^2)_{xy}+u_{yy}+2u_{xt}=0$

```
> DGsetup([t, x, y], [u], J2) :
```

$$\triangleright F := TotalDiff(u_{[1]}^2, [2, 3]) + u[3, 3] + 2 u[1, 2]$$

$$F := 2 u_2 u_3 + 2 u_{[1} u_{2, 3} + u_{3, 3} + 2 u_{1, 2} \quad (106)$$

$$\begin{aligned} & \text{> } A := \text{Matrix}\left(\left[\left[\text{diff}(F, u[1, 1]), \frac{1}{2} \text{diff}(F, u[1, 2]), \frac{1}{2} \text{diff}(F, u[1, 3])\right], \left[\frac{1}{2} \text{diff}(F, u[1, 2]), \text{diff}(F, u[2, 2]), \frac{1}{2} \text{diff}(F, u[2, 3])\right], \left[\frac{1}{2} \text{diff}(F, u[1, 3]), \frac{1}{2} \text{diff}(F, u[2, 3]), \text{diff}(F, u[3, 3])\right]\right]\right) : AA := \text{expand}(\text{MatrixInverse}(A)) \end{aligned}$$

$$AA := \begin{bmatrix} u_{[]}^2 & 1 & -u_{[]} \\ 1 & 0 & 0 \\ -u_{[]} & 0 & 1 \end{bmatrix} \quad (107)$$

$$\triangleright \text{DepVars} := [u(t, x, y)] : \text{FromJet}(AA, \text{DepVars})$$

$$\begin{bmatrix} u(t, x, y)^2 & 1 & -u(t, x, y) \\ 1 & 0 & 0 \\ -u(t, x, y) & 0 & 1 \end{bmatrix} \quad (108)$$

$$\rightarrow DGsetup([t, x, y], M) :$$

$$g := evalDG(u(t,x,y)^2 \cdot dt \& dt + (dt \& dx + dx \& dt) \cdot u(t,x,y) \cdot (dt \& dy + dy \& dt) + dy \& dy) :$$

```
> CotTen := CottonTensor(g) :
```

$$\triangleright CTJ := ToJet(CotTen, DepVars, notation = jetnumbers) :$$



```
> C := Connection(a000*dt &t D_t &t dt + a111*dx &t D_x &t dx + a222*dy &t D_y &t dy
+ a001*(dt &t D_t &t dx + dx &t D_t &t dt) + a002*(dt &t D_t &t dy + dy &t D_t
&t dt) + a102*(dx &t D_t &t dy + dy &t D_t &t dx) + a011*(dt &t D_x &t dx + dx
&t D_x &t dt) + a012*(dt &t D_x &t dy + dy &t D_x &t dt) + a112*(dx &t D_x &t dy
+ dy &t D_x &t dx) + a021*(dt &t D_y &t dx + dx &t D_y &t dt) + a022*(dt &t D_y
&t dy + dy &t D_y &t dt) + a122*(dx &t D_y &t dy + dy &t D_y &t dx) + a010*dt
&t D_x &t dt + a121*dx &t D_y &t dx + a202*dy &t D_t &t dy + a020*dt &t D_y &t dt
+ a101*dx &t D_t &t dx + a212*dy &t D_x &t dy) :
```

```
> TorsionTensor(C);
```

$0 \, dt \, D_t \, dt$

(109)

```
> U1 := x11(u(t,x,y))·diff(u(t,x,y),t) + x12(u(t,x,y))·diff(u(t,x,y),x) + x13(u(t,x,y))
·diff(u(t,x,y),y) :
U2 := x21(u(t,x,y))·diff(u(t,x,y),t) + x22(u(t,x,y))·diff(u(t,x,y),x) + x23(u(t,x,y))
·diff(u(t,x,y),y) :
U3 := x31(u(t,x,y))·diff(u(t,x,y),t) + x32(u(t,x,y))·diff(u(t,x,y),x) + x33(u(t,x,y))
·diff(u(t,x,y),y) :
```

```
> Et := evalDG(DirectionalCovariantDerivative(D_t, g, C) + U1·g) :
```

```
Ex := evalDG(DirectionalCovariantDerivative(D_x, g, C) + U2·g) :
```

```
Ey := evalDG(DirectionalCovariantDerivative(D_y, g, C) + U3·g) :
```

```
> Eq000 := TensorInnerProduct(g, Et, dt &t dt) :
Eq001 := TensorInnerProduct(g, Et, dt &t dx) :
Eq002 := TensorInnerProduct(g, Et, dt &t dy) :
Eq011 := TensorInnerProduct(g, Et, dx &t dx) :
Eq012 := TensorInnerProduct(g, Et, dx &t dy) :
Eq022 := TensorInnerProduct(g, Et, dy &t dy) :
Eq100 := TensorInnerProduct(g, Ex, dt &t dt) :
Eq101 := TensorInnerProduct(g, Ex, dt &t dx) :
Eq102 := TensorInnerProduct(g, Ex, dt &t dy) :
Eq111 := TensorInnerProduct(g, Ex, dx &t dx) :
Eq112 := TensorInnerProduct(g, Ex, dx &t dy) :
Eq122 := TensorInnerProduct(g, Ex, dy &t dy) :
Eq200 := TensorInnerProduct(g, Ey, dt &t dt) :
Eq201 := TensorInnerProduct(g, Ey, dt &t dx) :
Eq202 := TensorInnerProduct(g, Ey, dt &t dy) :
Eq211 := TensorInnerProduct(g, Ey, dx &t dx) :
Eq212 := TensorInnerProduct(g, Ey, dx &t dy) :
Eq222 := TensorInnerProduct(g, Ey, dy &t dy) :
```

```
> sA := solve( {Eq000=0, Eq001=0, Eq002=0, Eq011=0, Eq012=0, Eq022=0, Eq100=0,
Eq101=0, Eq102=0, Eq111=0, Eq112=0, Eq122=0, Eq200=0, Eq201=0, Eq202=0,
Eq211=0, Eq212=0, Eq222=0}, [a000, a001, a002, a010, a011, a012, a020, a021, a022,
a101, a102, a111, a112, a121, a122, a202, a212, a222]) :
```

```
> C1 := evalDG( subs( {op(op(sA))}, C) ) :
```

```
> evalDG(CovariantDerivative(g, C1) + g &t (U1·dt + U2·dx + U3·dy));
```

$0 \, dt \, dt \, dt$

(110)

```
> R1 := CurvatureTensor(C1) : Ric1 := RicciTensor(R1) : T1 := SymmetrizeIndices(Ric1, [1, 2],
"Symmetric") : Res := evalDG(T1 - V·g) :
```

```
> NEQt := ContractIndices(Res, D_t &t D_t, [[1, 1], [2, 2]]) : NEQt := ContractIndices(Res,
D_t &t D_x, [[1, 1], [2, 2]]) :
```

```

NEQty := ContractIndices(Res, D_t &t D_y, [[1, 1], [2, 2]]) : NEQxx := ContractIndices(Res,
D_x &t D_x, [[1, 1], [2, 2]]) :
NEQxy := ContractIndices(Res, D_x &t D_y, [[1, 1], [2, 2]]) : NEQyy := ContractIndices(Res,
D_y &t D_y, [[1, 1], [2, 2]]) :

```

```

>
> DGsetup([t, x, y], [u], J2, 4) :
> de := DifferentialEquationData([F], [u3,3])
de := [{u3,3}, [2 u2 u3 + 2 u[] u2,3 + u3,3 + 2 u1,2]] (111)

```

```

> de2 := Prolong(de, 2) : deTRA := Transformation(de2) :
>
> Eq0 := Pullback(deTRA, ToJet(NEQtt, DepVars, notation = jetnumbers)) :
> VS := solve(Eq0, V) :
> Eq1 := numer(subs(V=VS, Pullback(deTRA, ToJet(NEQtx, DepVars, notation
= jetnumbers)))) :
Eq2 := numer(subs(V=VS, Pullback(deTRA, ToJet(NEQty, DepVars, notation
= jetnumbers)))) :
Eq3 := numer(subs(V=VS, Pullback(deTRA, ToJet(NEQxx, DepVars, notation
= jetnumbers)))) :
Eq4 := numer(subs(V=VS, Pullback(deTRA, ToJet(NEQxy, DepVars, notation
= jetnumbers)))) :
Eq5 := numer(subs(V=VS, Pullback(deTRA, ToJet(NEQyy, DepVars, notation
= jetnumbers)))) :

```

```

> simplify(diff(Eq1, u1,1))
-u[]2 x21(u[]) + 2 x11(u[]) (112)

```

```

> simplify(diff(Eq1, u1,2))
-4 u[] - u[]2 x11(u[]) - u[]2 x22(u[]) + 2 x12(u[]) (113)

```

```

> simplify(diff(Eq1, u1,3))
4 - u[]2 x23(u[]) + 2 x13(u[]) (114)

```

```

> simplify(diff(Eq1, u2,2))
-u[]2 x12(u[]) + 2 u[]3 (115)

```

```

> simplify(diff(Eq1, u2,3))
-2 u[]2 - u[]2 x13(u[]) (116)

```

```

> simplify(diff(Eq2, u1,1))
-u[] x31(u[]) - 2 x11(u[]) (117)

```

```

> simplify(diff(Eq2, u1,2))
6 u[] + 2 u[] x13(u[]) - u[] x32(u[]) - 2 x12(u[]) (118)

```

```

> simplify(diff(Eq2, u1,3))
-4 - u[] x33(u[]) - u[] x11(u[]) - 2 x13(u[]) (119)

```

```

> simplify(diff(Eq2, u2,3))
6 u[]2 + 2 u[]2 x13(u[]) - u[] x12(u[]) (120)

```

$$\begin{aligned} &> \text{simplify}(\text{diff}(Eq3, u_{1,2})) \\ &\quad -2 \kappa_{21}(u_{[]}) \end{aligned} \quad (121)$$

$$\begin{aligned} &> \text{simplify}(\text{diff}(Eq3, u_{2,2})) \\ &\quad -2 \kappa_{22}(u_{[]}) \end{aligned} \quad (122)$$

$$\begin{aligned} &> \text{simplify}(\text{diff}(Eq3, u_{2,3})) \\ &\quad -2 \kappa_{23}(u_{[]}) \end{aligned} \quad (123)$$

$$\begin{aligned} &> \text{simplify}(\text{diff}(Eq4, u_{1,2})) \\ &\quad -\kappa_{31}(u_{[]}) + 2 \kappa_{23}(u_{[]}) \end{aligned} \quad (124)$$

$$\begin{aligned} &> \text{simplify}(\text{diff}(Eq4, u_{2,3})) \\ &\quad 2 u_{[]} \kappa_{23}(u_{[]}) - \kappa_{33}(u_{[]}) - \kappa_{22}(u_{[]}) \end{aligned} \quad (125)$$

$$\begin{aligned} &> \text{simplify}(\text{diff}(Eq4, u_{2,2})) \\ &\quad -2 - \kappa_{32}(u_{[]}) \end{aligned} \quad (126)$$

>

**M** > DGsetup([t, x, y], M) :

> U1 := 2 u(t, x, y) · diff(u(t, x, y), x) - 2 · diff(u(t, x, y), y) :  
 U2 := 0 :  
 U3 := -2 · diff(u(t, x, y), x) :

> Et := evalDG(DirectionalCovariantDerivative(D\_t, g, C) + U1 · g) :  
 Ex := evalDG(DirectionalCovariantDerivative(D\_x, g, C) + U2 · g) :  
 Ey := evalDG(DirectionalCovariantDerivative(D\_y, g, C) + U3 · g) :

> Eq000 := TensorInnerProduct(g, Et, dt &t dt) :  
 Eq001 := TensorInnerProduct(g, Et, dt &t dx) :  
 Eq002 := TensorInnerProduct(g, Et, dt &t dy) :  
 Eq011 := TensorInnerProduct(g, Et, dx &t dx) :  
 Eq012 := TensorInnerProduct(g, Et, dx &t dy) :  
 Eq022 := TensorInnerProduct(g, Et, dy &t dy) :  
 Eq100 := TensorInnerProduct(g, Ex, dt &t dt) :  
 Eq101 := TensorInnerProduct(g, Ex, dt &t dx) :  
 Eq102 := TensorInnerProduct(g, Ex, dt &t dy) :  
 Eq111 := TensorInnerProduct(g, Ex, dx &t dx) :  
 Eq112 := TensorInnerProduct(g, Ex, dx &t dy) :  
 Eq122 := TensorInnerProduct(g, Ex, dy &t dy) :  
 Eq200 := TensorInnerProduct(g, Ey, dt &t dt) :  
 Eq201 := TensorInnerProduct(g, Ey, dt &t dx) :  
 Eq202 := TensorInnerProduct(g, Ey, dt &t dy) :  
 Eq211 := TensorInnerProduct(g, Ey, dx &t dx) :  
 Eq212 := TensorInnerProduct(g, Ey, dx &t dy) :  
 Eq222 := TensorInnerProduct(g, Ey, dy &t dy) :

> sA := solve({Eq000=0, Eq001=0, Eq002=0, Eq011=0, Eq012=0, Eq022=0, Eq100=0,  
 Eq101=0, Eq102=0, Eq111=0, Eq112=0, Eq122=0, Eq200=0, Eq201=0, Eq202=0,  
 Eq211=0, Eq212=0, Eq222=0}, [a000, a001, a002, a010, a011, a012, a020, a021, a022,  
 a101, a102, a111, a112, a121, a122, a202, a212, a222]) :

> C1 := evalDG(subs({op(op(sA))}, C)) :

> evalDG(CovariantDerivative(g, C1) + g &t (U1 · dt + U2 · dx + U3 · dy)) ;

$0 \, dt \, dt \, dt$

(127)

```
> R1 := CurvatureTensor(C1) : Ric1 := RicciTensor(R1) : T1 := SymmetrizeIndices(Ric1, [1, 2],
    "Symmetric") : Res := evalDG(T1 - V.g) :
> NEQtt := TensorInnerProduct(g, Res, dt &t dt) : NEQtx := TensorInnerProduct(g, Res, dt
    &t dx) :
    NEQty := TensorInnerProduct(g, Res, dt &t dy) : NEQxx := TensorInnerProduct(g, Res, dx
    &t dx) :
    NEQxy := TensorInnerProduct(g, Res, dx &t dy) : NEQyy := TensorInnerProduct(g, Res, dy
    &t dy) :
```

```
> DGsetup([t, x, y], [u], J2, 4) :
```

```
> de := DifferentialEquationData([F], [u3,3])
```

$de := [\{u_{3,3}\}, [2 \, u_2 \, u_3 + 2 \, u_{[} \, u_{2,3} + u_{3,3} + 2 \, u_{1,2}]]$

(128)

```
> de2 := Prolong(de, 2) : deTRA := Transformation(de2) :
```

```
> Eq0 := Pullback(deTRA, ToJet(NEQtx, DepVars, notation = jetnumbers)) :
```

```
> VS := solve(Eq0, V) :
```

```
> Eq1 := numer(subs(V=VS, Pullback(deTRA, ToJet(NEQtt, DepVars, notation
    = jetnumbers)))) :
```

```
Eq2 := numer(subs(V=VS, Pullback(deTRA, ToJet(NEQty, DepVars, notation
    = jetnumbers)))) :
```

```
Eq3 := numer(subs(V=VS, Pullback(deTRA, ToJet(NEQxx, DepVars, notation
    = jetnumbers)))) :
```

```
Eq4 := numer(subs(V=VS, Pullback(deTRA, ToJet(NEQxy, DepVars, notation
    = jetnumbers)))) :
```

```
Eq5 := numer(subs(V=VS, Pullback(deTRA, ToJet(NEQyy, DepVars, notation
    = jetnumbers)))) :
```

```
> simplify([Eq1, Eq2, Eq3, Eq4, Eq5])
```

$[0, 0, 0, 0, 0]$

(129)

```
> simplify(VS)
```

$-\frac{1}{2} \, u_2^2 + 2 \, u_{2,3}$

(130)

Excellent - the linerization metric is EW on the equation in all cases!

Let us checdk that the Coton tensor does not vanish

```
J2 > ToJet(ContractIndices(CotTen, dt &t dt, [[1, 1], [2, 2]]), DepVars, notation
    = jetnumbers)
```

$\frac{1}{2} \, u_{2,2,2}$

(131)

```
> Pullback(deTRA, u2,2,2)
```

$u_{2,2,2}$

(132)
