# Supplementary material for: Dispersionless integrable systems in 3D and Einstein-Weyl geometry
Source: arXiv:1208.2728 ancillary file (2013-05-09)
Supplement: Supplementary file 12 [file Examples-2.pdf]

This is the worksheet accompanying the paper E.Ferapontov & B.Kruglikov "Dispersionless integrable systems in 3D and Einstein-Weyl geometry".

The file ran on **Maple** version 16, the package **DifferentialGeometry** was used.

For integrable PDE of type II, quasilinear wave equations, we consider 3 examples and for them we check that integrability is equivalent to EW property.

For explanations of the steps consult file Examples-1, we write only basic comments here.

>

I. We are going to consider the 2nd order quasilinear PDE  $u_x \cdot u_{yt} + u_y \cdot u_{tx} + u_t \cdot u_{xy} = 0$  and check if the corresponding conformal metric is EW

> with(DifferentialGeometry) : with(Tensor) : with(Tools) : with(JetCalculus) :  
with(LinearAlgebra) : with(PDEtools, D\_Dx, declare, ToJet, FromJet) :

> DGsetup([t, x, y], [u], J2) :

> F :=  $u_1 \cdot u_{2,3} + u_2 \cdot u_{1,3} + u_3 \cdot u_{1,2}$

$$F := u_1 u_{2,3} + u_2 u_{1,3} + u_3 u_{1,2}$$

(1)

> A := Matrix( $\left( \left[ \left[ \text{diff}(F, u[1, 1]), \frac{1}{2} \text{diff}(F, u[1, 2]), \frac{1}{2} \text{diff}(F, u[1, 3]) \right], \left[ \frac{1}{2} \text{diff}(F, u[1, 2]), \text{diff}(F, u[2, 2]), \frac{1}{2} \text{diff}(F, u[2, 3]) \right], \left[ \frac{1}{2} \text{diff}(F, u[1, 3]), \frac{1}{2} \text{diff}(F, u[2, 3]), \text{diff}(F, u[3, 3]) \right] \right] \right)$ ); AA := expand(MatrixInverse(A)) : AM := simplify(Determinant(A) · AA) :

$$A := \begin{bmatrix} 0 & \frac{1}{2} u_3 & \frac{1}{2} u_2 \\ \frac{1}{2} u_3 & 0 & \frac{1}{2} u_1 \\ \frac{1}{2} u_2 & \frac{1}{2} u_1 & 0 \end{bmatrix}$$

(2)

> AA; Determinant(A);

$$\begin{bmatrix} -\frac{u_1}{u_2 u_3} & \frac{1}{u_3} & \frac{1}{u_2} \\ \frac{1}{u_3} & -\frac{u_2}{u_3 u_1} & \frac{1}{u_1} \\ \frac{1}{u_2} & \frac{1}{u_1} & -\frac{u_3}{u_2 u_1} \end{bmatrix}$$

$$\frac{1}{4} u_3 u_2 u_1$$

(3)

> DepVars := [u(t, x, y)] : AJ := FromJet(AM, DepVars)

$$AJ := \left[ \left[ -\frac{1}{4} \left( \frac{\partial}{\partial t} u(t, x, y) \right)^2, \frac{1}{4} \left( \frac{\partial}{\partial x} u(t, x, y) \right) \left( \frac{\partial}{\partial t} u(t, x, y) \right), \frac{1}{4} \left( \frac{\partial}{\partial y} u(t, x, y) \right) \left( \frac{\partial}{\partial t} u(t, x, y) \right), \right. \right. \\ \left. \left. \left( \frac{\partial}{\partial t} u(t, x, y) \right) \left( \frac{\partial}{\partial x} u(t, x, y) \right), \left( \frac{\partial}{\partial t} u(t, x, y) \right) \left( \frac{\partial}{\partial y} u(t, x, y) \right), \left( \frac{\partial}{\partial x} u(t, x, y) \right) \left( \frac{\partial}{\partial y} u(t, x, y) \right) \right] \right]$$

(4)

$$\left[ \frac{1}{4} \left( \frac{\partial}{\partial x} u(t, x, y) \right) \left( \frac{\partial}{\partial t} u(t, x, y) \right), -\frac{1}{4} \left( \frac{\partial}{\partial x} u(t, x, y) \right)^2, \frac{1}{4} \left( \frac{\partial}{\partial x} u(t, x, y) \right) \left( \frac{\partial}{\partial y} u(t, x, y) \right) \right],$$

$$\left[ \frac{1}{4} \left( \frac{\partial}{\partial y} u(t, x, y) \right) \left( \frac{\partial}{\partial t} u(t, x, y) \right), \frac{1}{4} \left( \frac{\partial}{\partial x} u(t, x, y) \right) \left( \frac{\partial}{\partial y} u(t, x, y) \right), -\frac{1}{4} \left( \frac{\partial}{\partial y} u(t, x, y) \right)^2 \right]$$

> DGsetup([t, x, y], M) :

> g := evalDG(AJ[1, 1]·dt &t dt + AJ[1, 2]·dt &t dx + AJ[1, 3]·dt &t dy + AJ[2, 1]·dx &t dt + AJ[2, 2]·dx &t dx + AJ[2, 3]·dx &t dy + AJ[3, 1]·dy &t dt + AJ[3, 2]·dy &t dx + AJ[3, 3]·dy &t dy) :

> C := Connection(a000\*dt &t D\_t &t dt + a111\*dx &t D\_x &t dx + a222\*dy &t D\_y &t dy + a001\*(dt &t D\_t &t dx + dx &t D\_t &t dt) + a002\*(dt &t D\_t &t dy + dy &t D\_t &t dt) + a102\*(dx &t D\_t &t dy + dy &t D\_t &t dx) + a011\*(dt &t D\_x &t dx + dx &t D\_x &t dt) + a012\*(dt &t D\_x &t dy + dy &t D\_x &t dt) + a112\*(dx &t D\_x &t dy + dy &t D\_x &t dx) + a021\*(dt &t D\_y &t dx + dx &t D\_y &t dt) + a022\*(dt &t D\_y &t dy + dy &t D\_y &t dt) + a122\*(dx &t D\_y &t dy + dy &t D\_y &t dx) + a010\*dt &t D\_x &t dt + a121\*dx &t D\_y &t dx + a202\*dy &t D\_t &t dy + a020\*dt &t D\_y &t dt + a101\*dx &t D\_t &t dx + a212\*dy &t D\_x &t dy) :

> TorsionTensor(C);

$$0 \, dt \, D_t \, dt$$

(5)

> U1 := V111(diff(u(t, x, y), t), diff(u(t, x, y), x), diff(u(t, x, y), y))·diff(u(t, x, y), t, t) + V112(diff(u(t, x, y), t), diff(u(t, x, y), x), diff(u(t, x, y), y))·diff(u(t, x, y), t, x) + V113(diff(u(t, x, y), t), diff(u(t, x, y), x), diff(u(t, x, y), y))·diff(u(t, x, y), t, y) + V122(diff(u(t, x, y), t), diff(u(t, x, y), x), diff(u(t, x, y), y))·diff(u(t, x, y), x, x) + V123(diff(u(t, x, y), t), diff(u(t, x, y), x), diff(u(t, x, y), y))·diff(u(t, x, y), x, y) + V133(diff(u(t, x, y), t), diff(u(t, x, y), x), diff(u(t, x, y), y))·diff(u(t, x, y), y, y) :

U2 := V211(diff(u(t, x, y), t), diff(u(t, x, y), x), diff(u(t, x, y), y))·diff(u(t, x, y), t, t) + V212(diff(u(t, x, y), t), diff(u(t, x, y), x), diff(u(t, x, y), y))·diff(u(t, x, y), t, x) + V213(diff(u(t, x, y), t), diff(u(t, x, y), x), diff(u(t, x, y), y))·diff(u(t, x, y), t, y) + V222(diff(u(t, x, y), t), diff(u(t, x, y), x), diff(u(t, x, y), y))·diff(u(t, x, y), x, x) + V223(diff(u(t, x, y), t), diff(u(t, x, y), x), diff(u(t, x, y), y))·diff(u(t, x, y), x, y) + V233(diff(u(t, x, y), t), diff(u(t, x, y), x), diff(u(t, x, y), y))·diff(u(t, x, y), y, y) :

U3 := V311(diff(u(t, x, y), t), diff(u(t, x, y), x), diff(u(t, x, y), y))·diff(u(t, x, y), t, t) + V312(diff(u(t, x, y), t), diff(u(t, x, y), x), diff(u(t, x, y), y))·diff(u(t, x, y), t, x) + V313(diff(u(t, x, y), t), diff(u(t, x, y), x), diff(u(t, x, y), y))·diff(u(t, x, y), t, y) + V322(diff(u(t, x, y), t), diff(u(t, x, y), x), diff(u(t, x, y), y))·diff(u(t, x, y), x, x) + V323(diff(u(t, x, y), t), diff(u(t, x, y), x), diff(u(t, x, y), y))·diff(u(t, x, y), x, y) + V333(diff(u(t, x, y), t), diff(u(t, x, y), x), diff(u(t, x, y), y))·diff(u(t, x, y), y, y) :

> Et := evalDG(DirectionalCovariantDerivative(D\_t, g, C) + U1·g) :

Ex := evalDG(DirectionalCovariantDerivative(D\_x, g, C) + U2·g) :

Ey := evalDG(DirectionalCovariantDerivative(D\_y, g, C) + U3·g) :

> Eq000 := TensorInnerProduct(g, Et, dt &t dt) :

Eq001 := TensorInnerProduct(g, Et, dt &t dx) :

Eq002 := TensorInnerProduct(g, Et, dt &t dy) :

Eq011 := TensorInnerProduct(g, Et, dx &t dx) :

```

Eq012 := TensorInnerProduct(g, Et, dx &t dy) :
Eq022 := TensorInnerProduct(g, Et, dy &t dy) :
Eq100 := TensorInnerProduct(g, Ex, dt &t dt) :
Eq101 := TensorInnerProduct(g, Ex, dt &t dx) :
Eq102 := TensorInnerProduct(g, Ex, dt &t dy) :
Eq111 := TensorInnerProduct(g, Ex, dx &t dx) :
Eq112 := TensorInnerProduct(g, Ex, dx &t dy) :
Eq122 := TensorInnerProduct(g, Ex, dy &t dy) :
Eq200 := TensorInnerProduct(g, Ey, dt &t dt) :
Eq201 := TensorInnerProduct(g, Ey, dt &t dx) :
Eq202 := TensorInnerProduct(g, Ey, dt &t dy) :
Eq211 := TensorInnerProduct(g, Ey, dx &t dx) :
Eq212 := TensorInnerProduct(g, Ey, dx &t dy) :
Eq222 := TensorInnerProduct(g, Ey, dy &t dy) :

```

```

> sA := solve( {Eq000=0, Eq001=0, Eq002=0, Eq011=0, Eq012=0, Eq022=0, Eq100=0,
Eq101=0, Eq102=0, Eq111=0, Eq112=0, Eq122=0, Eq200=0, Eq201=0, Eq202=0,
Eq211=0, Eq212=0, Eq222=0}, [a000, a001, a002, a010, a011, a012, a020, a021, a022,
a101, a102, a111, a112, a121, a122, a202, a212, a222] ) :

```

```

> C1 := evalDG( subs( {op(op(sA))}, C) ) :

```

```

> evalDG( CovariantDerivative(g, C1) + g &t (U1·dt + U2·dx + U3·dy));
0 dt dt dt

```

(6)

```

> R1 := CurvatureTensor(C1) : Ric1 := RicciTensor(R1) : T1 := SymmetrizeIndices(Ric1, [1, 2],
"Symmetric") : Res := evalDG(T1 - V·g) :

```

```

> NEQt1 := ContractIndices(Res, D_t &t D_t, [[1, 1], [2, 2]]) : NEQt1x := ContractIndices(Res,
D_t &t D_x, [[1, 1], [2, 2]]) :
NEQt1y := ContractIndices(Res, D_t &t D_y, [[1, 1], [2, 2]]) : NEQt1xx := ContractIndices(Res,
D_x &t D_x, [[1, 1], [2, 2]]) :
NEQt1xy := ContractIndices(Res, D_x &t D_y, [[1, 1], [2, 2]]) : NEQt1yy := ContractIndices(Res,
D_y &t D_y, [[1, 1], [2, 2]]) :

```

```

> DGsetup([t, x, y], [u], J2, 4) :
> de := DifferentialEquationData([F], [u1, 2])

```

$de := [\{u_{1,2}\}, [u_1 u_{2,3} + u_2 u_{1,3} + u_3 u_{1,2}]]$

(7)

```

> de2 := Prolong(de, 2) : deTRA := Transformation(de2) :

```

```

> Eq0 := Pullback(deTRA, ToJet(NEQt1, DepVars, notation = jetnumbers)) :

```

```

> VS := solve(Eq0, V) :

```

```

> Eq1 := numer(subs(V=VS, Pullback(deTRA, ToJet(NEQt1x, DepVars, notation
=jetnumbers)))) :

```

```

Eq2 := numer(subs(V=VS, Pullback(deTRA, ToJet(NEQt1y, DepVars, notation
=jetnumbers)))) :

```

```

Eq3 := numer(subs(V=VS, Pullback(deTRA, ToJet(NEQt1xx, DepVars, notation
=jetnumbers)))) :

```

```

Eq4 := numer(subs(V=VS, Pullback(deTRA, ToJet(NEQt1xy, DepVars, notation
=jetnumbers)))) :

```

```

Eq5 := numer(subs(V=VS, Pullback(deTRA, ToJet(NEQt1yy, DepVars, notation
=jetnumbers)))) :

```

```

>

```

**J2** >  $Eq := [numer(subs(V = VS, Pullback(deTRA, ToJet(NEQtx, DepVars, notation = jetnumbers))))), numer(subs(V = VS, Pullback(deTRA, ToJet(NEQty, DepVars, notation = jetnumbers))))), numer(subs(V = VS, Pullback(deTRA, ToJet(NEQxx, DepVars, notation = jetnumbers))))), numer(subs(V = VS, Pullback(deTRA, ToJet(NEQxy, DepVars, notation = jetnumbers))))), numer(subs(V = VS, Pullback(deTRA, ToJet(NEQyy, DepVars, notation = jetnumbers))))]$  :

**J2** >  $Q := (i, j, k, l) \rightarrow diff(Eq[i], u[j, k, l]) :$

**J2** >  $Q(1, 1, 1, 1)$

$$u_3 \left( -2 u_2^3 u_1 u_3^3 V111(u_1, u_2, u_3) - u_3^3 u_1^2 u_2^2 V211(u_1, u_2, u_3) \right) \quad (8)$$

**J2** >  $Qq := \{ \}$  :

**for**  $i$  **from** 1 **to** 3 **do** **for**  $j$  **from** 1 **to** 3 **do** **for**  $k$  **from**  $j$  **to** 3 **do** **for**  $l$  **from**  $k$  **to** 3 **do**

$Qq := \{op(Qq), Q(i, j, k, l)\}$  **od:od:od:od:**

**J2** >  $nops(Qq)$

$$19 \quad (9)$$

**J2** >  $Qq$

$$\{0, u_3 \left( -2 u_2^3 u_1 u_3^3 V111(u_1, u_2, u_3) - u_3^3 u_1^2 u_2^2 V211(u_1, u_2, u_3) \right), u_3 \left( -2 u_1^2 u_2^3 V122(u_1, u_2, u_3) u_3^2 - 2 u_2 u_3^3 u_1^3 V223(u_1, u_2, u_3) + 2 u_2 u_1^4 V212(u_1, u_2, u_3) u_3^2 \right), u_3 \left( 2 u_2^3 u_1 u_3^3 V113(u_1, u_2, u_3) - 2 u_2^4 u_1 V112(u_1, u_2, u_3) u_3^2 + 2 u_1^3 u_2^2 V211(u_1, u_2, u_3) u_3^2 \right), u_3 \left( -u_1^2 u_2^3 V123(u_1, u_2, u_3) + u_2^2 u_1^3 V112(u_1, u_2, u_3) u_3^2 + u_1^3 u_2^2 V222(u_1, u_2, u_3) u_3^2 + 2 u_1^2 u_2^3 V122(u_1, u_2, u_3) u_3^2 + 4 u_2^2 u_1^3 u_2 \right), u_3 \left( u_2^3 u_1^2 V212(u_1, u_2, u_3) u_3^2 - 2 u_2^3 u_1 u_3^3 V113(u_1, u_2, u_3) - u_3^3 u_1^2 u_2^2 V213(u_1, u_2, u_3) + u_1^2 u_2^3 V111(u_1, u_2, u_3) u_3^2 + 2 u_2^4 u_1 V112(u_1, u_2, u_3) u_3^2 + 4 u_2^2 u_1 u_3^3 \right), u_3 \left( -2 u_1^4 u_2^2 V212(u_1, u_2, u_3) u_3 + 2 u_2^3 u_1^3 V112(u_1, u_2, u_3) u_3 - 2 u_1^2 u_2^3 V123(u_1, u_2, u_3) u_3^2 + 2 u_2^4 u_1^2 V122(u_1, u_2, u_3) u_3 - 2 u_2 u_3^3 u_1^3 V233(u_1, u_2, u_3) - 2 u_2 u_1^5 V211(u_1, u_2, u_3) u_3 + 2 u_2 u_1^4 V213(u_1, u_2, u_3) u_3^2 \right), u_3 \left( 2 u_2^3 u_1 u_3^3 V133(u_1, u_2, u_3) - 2 u_1^3 u_2^3 V212(u_1, u_2, u_3) u_3 + 2 u_2^4 u_1^2 V112(u_1, u_2, u_3) u_3 - 2 u_2^4 u_1 V123(u_1, u_2, u_3) u_3^2 + 2 u_2^5 u_1 V122(u_1, u_2, u_3) u_3 - 2 u_2^2 u_1^4 V211(u_1, u_2, u_3) u_3 + 2 u_1^3 u_2^2 V213(u_1, u_2, u_3) u_3^2 \right), u_3 \left( u_1^3 u_2^2 V223(u_1, u_2, u_3) u_3^2 - u_1^2 u_2^2 u_3^3 V133(u_1, u_2, u_3) - u_1^4 u_2^2 V212(u_1, u_2, u_3) u_3 - u_2^2 u_1^4 V111(u_1, u_2, u_3) u_3 + u_2^2 u_1^3 V113(u_1, u_2, u_3) u_3^2 - 3 u_2^3 u_1^3 V112(u_1, u_2, u_3) u_3 - u_2^3 u_1^3 V222(u_1, u_2, u_3) u_3 + 2 u_1^2 u_2^3 V123(u_1, u_2, u_3) u_3^2 - 2 u_2^4 u_1^2 V122(u_1, u_2, u_3) u_3 - 8 u_2^2 u_1^3 u_3 \right), u_3 \left( u_2^3 u_1^2 V223(u_1, u_2, u_3) u_3^2 - 2 u_2^3 u_1 u_3^3 V133(u_1, u_2, u_3) - u_1^3 u_2^3 V212(u_1, u_2, u_3) u_3 - u_2^3 u_1^3 V111(u_1, u_2, u_3) u_3 - 3 u_2^4 u_1^2 V112(u_1, u_2, u_3) u_3 - u_2^4 u_1^2 V222(u_1, u_2, u_3) u_3 - u_3^3 u_1^2 u_2^2 V233(u_1, u_2, u_3) + u_1^2 u_2^3 V113(u_1, u_2, u_3) u_3^2 + 2 u_2^4 u_1 V123(u_1, u_2, u_3) u_3^2 - 2 u_2^5 u_1 V122(u_1, u_2, u_3) u_3 - 8 u_2^3 u_1^2 u_3 \right), -u_2 u_1^2 V133(u_1, u_2, u_3) u_3^3, -u_3^4 u_1^2 u_2^2 V122(u_1, u_2, u_3), -2 u_3^4 u_2 u_1^3 V222(u_1, u_2, u_3), 2 u_3^4 u_2 u_1 V111(u_1, u_2, u_3), -u_1^2 u_2 V311(u_1, u_2, u_3) u_3^3 - 2 u_1 u_3^4 u_2 V111(u_1, u_2, u_3), u_1^3 u_2 V322(u_1, u_2, u_3) u_3^2 + u_2 u_1^2 V122(u_1, u_2, u_3) u_3^3, -u_1^2$$

$$\begin{aligned}
& u_3^3 u_2 V111(u_1, u_2, u_3) - 4 u_1 u_2 u_3^3 + u_1^2 u_2^2 V312(u_1, u_2, u_3) u_3^2 + 2 u_1 u_2^2 V112(u_1, u_2, u_3) u_3^3 \\
& - u_1^2 u_2 V313(u_1, u_2, u_3) u_3^3 - 2 u_1 u_3^4 u_2 V113(u_1, u_2, u_3), -u_1^3 u_2^2 V322(u_1, u_2, u_3) u_3 + \\
& u_1^3 u_2 V323(u_1, u_2, u_3) u_3^2 - 2 u_1^2 u_2^2 V122(u_1, u_2, u_3) u_3^2 - u_1^4 V312(u_1, u_2, u_3) u_2 u_3 - \\
& u_1^3 V112(u_1, u_2, u_3) u_3^2 u_2 + u_2 u_1^2 V123(u_1, u_2, u_3) u_3^3, -u_1^2 u_3^3 u_2 V113(u_1, u_2, u_3) - \\
& u_1^3 V312(u_1, u_2, u_3) u_2^2 u_3 + 2 u_1 u_2^2 V123(u_1, u_2, u_3) u_3^3 - u_1^2 u_2^3 V322(u_1, u_2, u_3) u_3 + u_1^2 \\
& u_2^2 V323(u_1, u_2, u_3) u_3^2 - 2 u_1 u_2^3 V122(u_1, u_2, u_3) u_3^2 - u_1^2 u_2 V333(u_1, u_2, u_3) u_3^3 - \\
& u_1^2 V112(u_1, u_2, u_3) u_3^2 u_2^2 - 2 u_1 u_3^4 u_2 V133(u_1, u_2, u_3) - 4 u_3^2 u_1^2 u_2 \}
\end{aligned}$$

**J2** >  $SLV := solve(Qq, [V111(u_1, u_2, u_3), V112(u_1, u_2, u_3), V113(u_1, u_2, u_3), V122(u_1, u_2, u_3), V123(u_1, u_2, u_3), V133(u_1, u_2, u_3), V211(u_1, u_2, u_3), V212(u_1, u_2, u_3), V213(u_1, u_2, u_3), V222(u_1, u_2, u_3), V223(u_1, u_2, u_3), V233(u_1, u_2, u_3), V311(u_1, u_2, u_3), V312(u_1, u_2, u_3), V313(u_1, u_2, u_3), V322(u_1, u_2, u_3), V323(u_1, u_2, u_3), V333(u_1, u_2, u_3)])$

$$\begin{aligned}
SLV := & \left[ \left[ V111(u_1, u_2, u_3) = 0, V112(u_1, u_2, u_3) = \frac{V123(u_1, u_2, u_3) u_2 u_3 - 4 u_1}{u_1 u_2}, V113(u_1, u_2, u_3) = \right. \right. \quad (11) \\
& \left. \left. u_3 \right) = \frac{V123(u_1, u_2, u_3) u_2 u_3 - 4 u_1}{u_3 u_1}, V122(u_1, u_2, u_3) = 0, V123(u_1, u_2, u_3) = V123(u_1, \right. \\
& \left. u_2, u_3), V133(u_1, u_2, u_3) = 0, V211(u_1, u_2, u_3) = 0, V212(u_1, u_2, u_3) \right. \\
& \left. = \frac{u_3 u_1 V213(u_1, u_2, u_3) - 4 u_2}{u_2 u_1}, V213(u_1, u_2, u_3) = V213(u_1, u_2, u_3), V222(u_1, u_2, u_3) \right. \\
& \left. = 0, V223(u_1, u_2, u_3) = \frac{u_3 u_1 V213(u_1, u_2, u_3) - 4 u_2}{u_2 u_3}, V233(u_1, u_2, u_3) = 0, V311(u_1, u_2, \right. \\
& \left. u_3) = 0, V312(u_1, u_2, u_3) = \frac{u_3 (u_1 V313(u_1, u_2, u_3) + 4)}{u_2 u_1}, V313(u_1, u_2, u_3) = V313(u_1, \right. \\
& \left. u_2, u_3), V322(u_1, u_2, u_3) = 0, V323(u_1, u_2, u_3) = \frac{u_1 V313(u_1, u_2, u_3)}{u_2}, V333(u_1, u_2, u_3) \right. \\
& \left. = 0 \right] \left. \right]
\end{aligned}$$

We are looking for the general form of 1-form omega (it has coefficients  $U_i$ ) that depends linearly on 2nd derivatives with the coefficients depending on 1st derivatives, and then we see that this coincides with our general formula.

**J2** >  $U1a := subs(FromJet(SLV[1], DepVars), U1)$

$$U1a := \frac{1}{\left( \frac{\partial}{\partial t} u(t, x, y) \right) \left( \frac{\partial}{\partial x} u(t, x, y) \right)} \left( \left( V123 \left( \frac{\partial}{\partial t} u(t, x, y), \frac{\partial}{\partial x} u(t, x, y), \frac{\partial}{\partial y} u(t, x, \right. \right. \right. \quad (12)$$

$$\begin{aligned}
& y) \left( \frac{\partial}{\partial x} u(t, x, y) \right) \left( \frac{\partial}{\partial y} u(t, x, y) \right) - 4 \left( \frac{\partial}{\partial t} u(t, x, y) \right) \left( \frac{\partial^2}{\partial x \partial t} u(t, x, y) \right) \Bigg) \\
& + \frac{1}{\left( \frac{\partial}{\partial y} u(t, x, y) \right) \left( \frac{\partial}{\partial t} u(t, x, y) \right)} \left( \left( V123 \left( \frac{\partial}{\partial t} u(t, x, y), \frac{\partial}{\partial x} u(t, x, y), \frac{\partial}{\partial y} u(t, x, \right. \right. \right. \\
& y) \left( \frac{\partial}{\partial x} u(t, x, y) \right) \left( \frac{\partial}{\partial y} u(t, x, y) \right) - 4 \left( \frac{\partial}{\partial t} u(t, x, y) \right) \left( \frac{\partial^2}{\partial y \partial t} u(t, x, y) \right) \Bigg) \\
& + V123 \left( \frac{\partial}{\partial t} u(t, x, y), \frac{\partial}{\partial x} u(t, x, y), \frac{\partial}{\partial y} u(t, x, y) \right) \left( \frac{\partial^2}{\partial y \partial x} u(t, x, y) \right)
\end{aligned}$$

**J2** >  $U2a := \text{subs}(\text{FromJet}(\text{SLV}[1], \text{DepVars}), U2)$

$$\begin{aligned}
U2a := & \frac{1}{\left( \frac{\partial}{\partial x} u(t, x, y) \right) \left( \frac{\partial}{\partial t} u(t, x, y) \right)} \left( \left( \left( \frac{\partial}{\partial y} u(t, x, y) \right) \left( \frac{\partial}{\partial t} u(t, x, y) \right) V213 \left( \frac{\partial}{\partial t} u(t, \right. \right. \right. \quad (13) \\
& x, y), \frac{\partial}{\partial x} u(t, x, y), \frac{\partial}{\partial y} u(t, x, y) \Bigg) - 4 \left( \frac{\partial}{\partial x} u(t, x, y) \right) \left( \frac{\partial^2}{\partial x \partial t} u(t, x, y) \right) \Bigg) \\
& + V213 \left( \frac{\partial}{\partial t} u(t, x, y), \frac{\partial}{\partial x} u(t, x, y), \frac{\partial}{\partial y} u(t, x, y) \right) \left( \frac{\partial^2}{\partial y \partial t} u(t, x, y) \right) \\
& + \frac{1}{\left( \frac{\partial}{\partial x} u(t, x, y) \right) \left( \frac{\partial}{\partial y} u(t, x, y) \right)} \left( \left( \left( \frac{\partial}{\partial y} u(t, x, y) \right) \left( \frac{\partial}{\partial t} u(t, x, y) \right) V213 \left( \frac{\partial}{\partial t} u(t, \right. \right. \right. \\
& x, y), \frac{\partial}{\partial x} u(t, x, y), \frac{\partial}{\partial y} u(t, x, y) \Bigg) - 4 \left( \frac{\partial}{\partial x} u(t, x, y) \right) \left( \frac{\partial^2}{\partial y \partial x} u(t, x, y) \right) \Bigg)
\end{aligned}$$

**J2** >  $U3a := \text{subs}(\text{FromJet}(\text{SLV}[1], \text{DepVars}), U3)$

$$\begin{aligned}
U3a := & \frac{1}{\left( \frac{\partial}{\partial x} u(t, x, y) \right) \left( \frac{\partial}{\partial t} u(t, x, y) \right)} \left( \left( \frac{\partial}{\partial y} u(t, x, y) \right) \left( \frac{\partial}{\partial t} u(t, x, y) \right) V313 \left( \frac{\partial}{\partial t} u(t, \right. \right. \quad (14) \\
& x, y), \frac{\partial}{\partial x} u(t, x, y), \frac{\partial}{\partial y} u(t, x, y) \Bigg) + 4 \left( \frac{\partial^2}{\partial x \partial t} u(t, x, y) \right) \Bigg) + V313 \left( \frac{\partial}{\partial t} u(t, x, y), \right. \\
& \frac{\partial}{\partial x} u(t, x, y), \frac{\partial}{\partial y} u(t, x, y) \Bigg) \left( \frac{\partial^2}{\partial y \partial t} u(t, x, y) \right) \\
& + \frac{\left( \frac{\partial}{\partial t} u(t, x, y) \right) V313 \left( \frac{\partial}{\partial t} u(t, x, y), \frac{\partial}{\partial x} u(t, x, y), \frac{\partial}{\partial y} u(t, x, y) \right) \left( \frac{\partial^2}{\partial y \partial x} u(t, x, y) \right)}{\frac{\partial}{\partial x} u(t, x, y)}
\end{aligned}$$

>

$$\begin{aligned}
\textbf{J2} > U1a := & \frac{4 \left( \frac{\partial}{\partial t} u(t, x, y) \right) \left( \frac{\partial^2}{\partial x \partial y} u(t, x, y) \right)}{\left( \frac{\partial}{\partial x} u(t, x, y) \right) \left( \frac{\partial}{\partial y} u(t, x, y) \right)} : U2a \\
:= & \frac{4 \left( \frac{\partial}{\partial x} u(t, x, y) \right) \left( \frac{\partial^2}{\partial t \partial y} u(t, x, y) \right)}{\left( \frac{\partial}{\partial t} u(t, x, y) \right) \left( \frac{\partial}{\partial y} u(t, x, y) \right)} : U3a
\end{aligned}$$

$$:= \frac{4 \left( \frac{\partial}{\partial y} u(t, x, y) \right) \left( \frac{\partial^2}{\partial t \partial x} u(t, x, y) \right)}{\left( \frac{\partial}{\partial t} u(t, x, y) \right) \left( \frac{\partial}{\partial x} u(t, x, y) \right)} :$$

**J2** > DGsetup([t, x, y], M) :

> Et := evalDG(DirectionalCovariantDerivative(D\_t, g, C) + U1a·g) :

Ex := evalDG(DirectionalCovariantDerivative(D\_x, g, C) + U2a·g) :

Ey := evalDG(DirectionalCovariantDerivative(D\_y, g, C) + U3a·g) :

> Eq000 := TensorInnerProduct(g, Et, dt &t dt) :

Eq001 := TensorInnerProduct(g, Et, dt &t dx) :

Eq002 := TensorInnerProduct(g, Et, dt &t dy) :

Eq011 := TensorInnerProduct(g, Et, dx &t dx) :

Eq012 := TensorInnerProduct(g, Et, dx &t dy) :

Eq022 := TensorInnerProduct(g, Et, dy &t dy) :

Eq100 := TensorInnerProduct(g, Ex, dt &t dt) :

Eq101 := TensorInnerProduct(g, Ex, dt &t dx) :

Eq102 := TensorInnerProduct(g, Ex, dt &t dy) :

Eq111 := TensorInnerProduct(g, Ex, dx &t dx) :

Eq112 := TensorInnerProduct(g, Ex, dx &t dy) :

Eq122 := TensorInnerProduct(g, Ex, dy &t dy) :

Eq200 := TensorInnerProduct(g, Ey, dt &t dt) :

Eq201 := TensorInnerProduct(g, Ey, dt &t dx) :

Eq202 := TensorInnerProduct(g, Ey, dt &t dy) :

Eq211 := TensorInnerProduct(g, Ey, dx &t dx) :

Eq212 := TensorInnerProduct(g, Ey, dx &t dy) :

Eq222 := TensorInnerProduct(g, Ey, dy &t dy) :

> sA := solve({Eq000=0, Eq001=0, Eq002=0, Eq011=0, Eq012=0, Eq022=0, Eq100=0, Eq101=0, Eq102=0, Eq111=0, Eq112=0, Eq122=0, Eq200=0, Eq201=0, Eq202=0, Eq211=0, Eq212=0, Eq222=0}, [a000, a001, a002, a010, a011, a012, a020, a021, a022, a101, a102, a111, a112, a121, a122, a202, a212, a222]) :

> C1 := evalDG(subs({op(op(sA))}, C)) :

> evalDG(CovariantDerivative(g, C1) + g &t (U1a·dt + U2a·dx + U3a·dy)) ;

0 dt dt dt

(15)

> R1 := CurvatureTensor(C1) : Ric1 := RicciTensor(R1) : T1 := SymmetrizeIndices(Ric1, [1, 2], "Symmetric") : Res := evalDG(T1 - V·g) :

> NEQtt := ContractIndices(Res, D\_t &t D\_t, [[1, 1], [2, 2]]) : NEQtx := ContractIndices(Res, D\_t &t D\_x, [[1, 1], [2, 2]]) :

NEQty := ContractIndices(Res, D\_t &t D\_y, [[1, 1], [2, 2]]) : NEQxx := ContractIndices(Res, D\_x &t D\_x, [[1, 1], [2, 2]]) :

NEQxy := ContractIndices(Res, D\_x &t D\_y, [[1, 1], [2, 2]]) : NEQyy := ContractIndices(Res, D\_y &t D\_y, [[1, 1], [2, 2]]) :

> DGsetup([t, x, y], [u], J2, 4) :

> de := DifferentialEquationData([F], [u<sub>1,2</sub>])

de := [ {u<sub>1,2</sub>}, [u<sub>1</sub>u<sub>2,3</sub> + u<sub>2</sub>u<sub>1,3</sub> + u<sub>3</sub>u<sub>1,2</sub>] ]

(16)

> de2 := Prolong(de, 2) : deTRA := Transformation(de2) :





$$A := \begin{bmatrix} u_2 u_3 \left( \frac{d^2}{du_1^2} p(u_1) \right) & u_3 \left( \frac{d}{du_1} p(u_1) \right) & u_2 \left( \frac{d}{du_1} p(u_1) \right) \\ u_3 \left( \frac{d}{du_1} p(u_1) \right) & 0 & p(u_1) \\ u_2 \left( \frac{d}{du_1} p(u_1) \right) & p(u_1) & 0 \end{bmatrix} \quad (19)$$

> AA; Determinant(A);

$$\left[ \left[ -\frac{p(u_1)}{u_2 u_3 \left( 2 \left( \frac{d}{du_1} p(u_1) \right)^2 - \left( \frac{d^2}{du_1^2} p(u_1) \right) p(u_1) \right)}, \right. \right. \\ \left. \frac{\frac{d}{du_1} p(u_1)}{u_3 \left( 2 \left( \frac{d}{du_1} p(u_1) \right)^2 - \left( \frac{d^2}{du_1^2} p(u_1) \right) p(u_1) \right)}, \right. \\ \left. \frac{\frac{d}{du_1} p(u_1)}{u_2 \left( 2 \left( \frac{d}{du_1} p(u_1) \right)^2 - \left( \frac{d^2}{du_1^2} p(u_1) \right) p(u_1) \right)} \right], \\ \left[ \frac{\frac{d}{du_1} p(u_1)}{u_3 \left( 2 \left( \frac{d}{du_1} p(u_1) \right)^2 - \left( \frac{d^2}{du_1^2} p(u_1) \right) p(u_1) \right)}, \right. \\ \left. -\frac{u_2 \left( \frac{d}{du_1} p(u_1) \right)^2}{u_3 p(u_1) \left( 2 \left( \frac{d}{du_1} p(u_1) \right)^2 - \left( \frac{d^2}{du_1^2} p(u_1) \right) p(u_1) \right)}, \right. \\ \left. \frac{-\left( \frac{d^2}{du_1^2} p(u_1) \right) p(u_1) + \left( \frac{d}{du_1} p(u_1) \right)^2}{p(u_1) \left( 2 \left( \frac{d}{du_1} p(u_1) \right)^2 - \left( \frac{d^2}{du_1^2} p(u_1) \right) p(u_1) \right)} \right], \right]$$

$$\begin{aligned}
& \left[ \frac{\frac{d}{du_1} p(u_1)}{u_2 \left( 2 \left( \frac{d}{du_1} p(u_1) \right)^2 - \left( \frac{d^2}{du_1^2} p(u_1) \right) p(u_1) \right)} \right. \\
& \quad \left. - \frac{\left( \frac{d^2}{du_1^2} p(u_1) \right) p(u_1) + \left( \frac{d}{du_1} p(u_1) \right)^2}{p(u_1) \left( 2 \left( \frac{d}{du_1} p(u_1) \right)^2 - \left( \frac{d^2}{du_1^2} p(u_1) \right) p(u_1) \right)} \right. \\
& \quad \left. - \frac{u_3 \left( \frac{d}{du_1} p(u_1) \right)^2}{u_2 p(u_1) \left( 2 \left( \frac{d}{du_1} p(u_1) \right)^2 - \left( \frac{d^2}{du_1^2} p(u_1) \right) p(u_1) \right)} \right] \\
& \quad 2 u_2 \left( \frac{d}{du_1} p(u_1) \right)^2 u_3 p(u_1) - u_2 u_3 \left( \frac{d^2}{du_1^2} p(u_1) \right) p(u_1)^2
\end{aligned} \tag{20}$$

> *DepVars* := [*u*(*t*, *x*, *y*)] : *AJ* := *FromJet*(*AM*, *DepVars*)

$$\begin{aligned}
*AJ* := & \left[ \left[ -p \left( \frac{\partial}{\partial t} u(t, x, y) \right)^2, \left( \frac{\partial}{\partial x} u(t, x, y) \right) D(p) \left( \frac{\partial}{\partial t} u(t, x, y) \right) p \left( \frac{\partial}{\partial t} u(t, x, y) \right), \right. \right. \\
& \left. \left( \frac{\partial}{\partial y} u(t, x, y) \right) D(p) \left( \frac{\partial}{\partial t} u(t, x, y) \right) p \left( \frac{\partial}{\partial t} u(t, x, y) \right) \right], \\
& \left[ \left( \frac{\partial}{\partial x} u(t, x, y) \right) D(p) \left( \frac{\partial}{\partial t} u(t, x, y) \right) p \left( \frac{\partial}{\partial t} u(t, x, y) \right), - \left( \frac{\partial}{\partial x} u(t, x, \right. \right. \\
& \left. \left. y) \right)^2 D(p) \left( \frac{\partial}{\partial t} u(t, x, y) \right)^2, \left( \frac{\partial}{\partial x} u(t, x, y) \right) \left( \frac{\partial}{\partial y} u(t, x, y) \right) \left( -D^{(2)}(p) \left( \frac{\partial}{\partial t} u(t, x, \right. \right. \right. \\
& \left. \left. y) \right) p \left( \frac{\partial}{\partial t} u(t, x, y) \right) + D(p) \left( \frac{\partial}{\partial t} u(t, x, y) \right)^2 \right], \\
& \left[ \left( \frac{\partial}{\partial y} u(t, x, y) \right) D(p) \left( \frac{\partial}{\partial t} u(t, x, y) \right) p \left( \frac{\partial}{\partial t} u(t, x, y) \right), \left( \frac{\partial}{\partial x} u(t, x, y) \right) \left( \frac{\partial}{\partial y} u(t, x, \right. \right. \\
& \left. \left. y) \right) \left( -D^{(2)}(p) \left( \frac{\partial}{\partial t} u(t, x, y) \right) p \left( \frac{\partial}{\partial t} u(t, x, y) \right) + D(p) \left( \frac{\partial}{\partial t} u(t, x, y) \right)^2 \right), \right. \\
& \left. - \left( \frac{\partial}{\partial y} u(t, x, y) \right)^2 D(p) \left( \frac{\partial}{\partial t} u(t, x, y) \right)^2 \right]
\end{aligned} \tag{21}$$

> *DGsetup*( [*t*, *x*, *y*], *M*) :

> *g* := *evalDG*(*AJ*[1, 1]·*dt* & *dt* + *AJ*[1, 2]·*dt* & *dx* + *AJ*[1, 3]·*dt* & *dy* + *AJ*[2, 1]·*dx* & *dt* + *AJ*[2, 2]·*dx* & *dx* + *AJ*[2, 3]·*dx* & *dy* + *AJ*[3, 1]·*dy* & *dt* + *AJ*[3, 2]·*dy* & *dx* + *AJ*[3, 3]·*dy* & *dy*) :

> *C* := *Connection*(*a000*·*dt* & *D\_t* & *dt* + *a111*·*dx* & *D\_x* & *dx* + *a222*·*dy* & *D\_y* & *dy* + *a001*·(*dt* & *D\_t* & *dx* + *dx* & *D\_t* & *dt*) + *a002*·(*dt* & *D\_t* & *dy* + *dy* & *D\_t* & *dt*) + *a102*·(*dx* & *D\_t* & *dy* + *dy* & *D\_t* & *dx*) + *a011*·(*dt* & *D\_x* & *dx* + *dx*

$$\begin{aligned} & \& t D\_x \& t dt) + a012 * (dt \& t D\_x \& t dy + dy \& t D\_x \& t dt) + a112 * (dx \& t D\_x \& t dy \\ & + dy \& t D\_x \& t dx) + a021 * (dt \& t D\_y \& t dx + dx \& t D\_y \& t dt) + a022 * (dt \& t D\_y \\ & \& t dy + dy \& t D\_y \& t dt) + a122 * (dx \& t D\_y \& t dy + dy \& t D\_y \& t dx) + a010 * dt \\ & \& t D\_x \& t dt + a121 * dx \& t D\_y \& t dx + a202 * dy \& t D\_t \& t dy + a020 * dt \& t D\_y \& t dt \\ & + a101 * dx \& t D\_t \& t dx + a212 * dy \& t D\_x \& t dy) : \end{aligned}$$

> TorsionTensor(C);

$$0 \, dt \, D\_t \, dt$$

(22)

> U1 := V111(diff(u(t, x, y), t), diff(u(t, x, y), x), diff(u(t, x, y), y)) · diff(u(t, x, y), t, t)  
+ V112(diff(u(t, x, y), t), diff(u(t, x, y), x), diff(u(t, x, y), y)) · diff(u(t, x, y), t, x)  
+ V113(diff(u(t, x, y), t), diff(u(t, x, y), x), diff(u(t, x, y), y)) · diff(u(t, x, y), t, y)  
+ V122(diff(u(t, x, y), t), diff(u(t, x, y), x), diff(u(t, x, y), y)) · diff(u(t, x, y), x, x)  
+ V123(diff(u(t, x, y), t), diff(u(t, x, y), x), diff(u(t, x, y), y)) · diff(u(t, x, y), x, y)  
+ V133(diff(u(t, x, y), t), diff(u(t, x, y), x), diff(u(t, x, y), y)) · diff(u(t, x, y), y, y) :  
U2 := V211(diff(u(t, x, y), t), diff(u(t, x, y), x), diff(u(t, x, y), y)) · diff(u(t, x, y), t, t)  
+ V212(diff(u(t, x, y), t), diff(u(t, x, y), x), diff(u(t, x, y), y)) · diff(u(t, x, y), t, x)  
+ V213(diff(u(t, x, y), t), diff(u(t, x, y), x), diff(u(t, x, y), y)) · diff(u(t, x, y), t, y)  
+ V222(diff(u(t, x, y), t), diff(u(t, x, y), x), diff(u(t, x, y), y)) · diff(u(t, x, y), x, x)  
+ V223(diff(u(t, x, y), t), diff(u(t, x, y), x), diff(u(t, x, y), y)) · diff(u(t, x, y), x, y)  
+ V233(diff(u(t, x, y), t), diff(u(t, x, y), x), diff(u(t, x, y), y)) · diff(u(t, x, y), y, y) :  
U3 := V311(diff(u(t, x, y), t), diff(u(t, x, y), x), diff(u(t, x, y), y)) · diff(u(t, x, y), t, t)  
+ V312(diff(u(t, x, y), t), diff(u(t, x, y), x), diff(u(t, x, y), y)) · diff(u(t, x, y), t, x)  
+ V313(diff(u(t, x, y), t), diff(u(t, x, y), x), diff(u(t, x, y), y)) · diff(u(t, x, y), t, y)  
+ V322(diff(u(t, x, y), t), diff(u(t, x, y), x), diff(u(t, x, y), y)) · diff(u(t, x, y), x, x)  
+ V323(diff(u(t, x, y), t), diff(u(t, x, y), x), diff(u(t, x, y), y)) · diff(u(t, x, y), x, y)  
+ V333(diff(u(t, x, y), t), diff(u(t, x, y), x), diff(u(t, x, y), y)) · diff(u(t, x, y), y, y) :

> Et := evalDG(DirectionalCovariantDerivative(D\_t, g, C) + U1·g) :

Ex := evalDG(DirectionalCovariantDerivative(D\_x, g, C) + U2·g) :

Ey := evalDG(DirectionalCovariantDerivative(D\_y, g, C) + U3·g) :

> Eq000 := TensorInnerProduct(g, Et, dt & t dt) :  
Eq001 := TensorInnerProduct(g, Et, dt & t dx) :  
Eq002 := TensorInnerProduct(g, Et, dt & t dy) :  
Eq011 := TensorInnerProduct(g, Et, dx & t dx) :  
Eq012 := TensorInnerProduct(g, Et, dx & t dy) :  
Eq022 := TensorInnerProduct(g, Et, dy & t dy) :  
Eq100 := TensorInnerProduct(g, Ex, dt & t dt) :  
Eq101 := TensorInnerProduct(g, Ex, dt & t dx) :  
Eq102 := TensorInnerProduct(g, Ex, dt & t dy) :  
Eq111 := TensorInnerProduct(g, Ex, dx & t dx) :  
Eq112 := TensorInnerProduct(g, Ex, dx & t dy) :  
Eq122 := TensorInnerProduct(g, Ex, dy & t dy) :  
Eq200 := TensorInnerProduct(g, Ey, dt & t dt) :  
Eq201 := TensorInnerProduct(g, Ey, dt & t dx) :  
Eq202 := TensorInnerProduct(g, Ey, dt & t dy) :  
Eq211 := TensorInnerProduct(g, Ey, dx & t dx) :  
Eq212 := TensorInnerProduct(g, Ey, dx & t dy) :  
Eq222 := TensorInnerProduct(g, Ey, dy & t dy) :

> sA := solve( {Eq000=0, Eq001=0, Eq002=0, Eq011=0, Eq012=0, Eq022=0, Eq100=0,  
Eq101=0, Eq102=0, Eq111=0, Eq112=0, Eq122=0, Eq200=0, Eq201=0, Eq202=0,  
Eq211=0, Eq212=0, Eq222=0}, [a000, a001, a002, a010, a011, a012, a020, a021, a022,  
a101, a102, a111, a112, a121, a122, a202, a212, a222] ) :

```

> C1 := evalDG( subs( {op(op(sA))}, C) ) :
> evalDG( CovariantDerivative(g, C1) + g &t (U1·dt + U2·dx + U3 ·dy)) ;
0 dt dt dt
(23)

```

```

> R1 := CurvatureTensor(C1) : Ric1 := RicciTensor(R1) : T1 := SymmetrizeIndices(Ric1, [1, 2],
"Symmetric") : Res := evalDG(T1 - V·g) :
> NEQtt := ContractIndices(Res, D_t &t D_t, [[1, 1], [2, 2]]) : NEQtx := ContractIndices(Res,
D_t &t D_x, [[1, 1], [2, 2]]) :
NEQty := ContractIndices(Res, D_t &t D_y, [[1, 1], [2, 2]]) : NEQxx := ContractIndices(Res,
D_x &t D_x, [[1, 1], [2, 2]]) :
NEQxy := ContractIndices(Res, D_x &t D_y, [[1, 1], [2, 2]]) : NEQyy := ContractIndices(Res,
D_y &t D_y, [[1, 1], [2, 2]]) :

```

```

> DGsetup([t, x, y], [u], J2, 4) :
> de := DifferentialEquationData([F], [u1,2])
de := [ {u1,2}, [ 2 u2 ( d/d u1 p(u1) ) u1,3 + 2 p(u1) u2,3 + 2 u3 ( d/d u1 p(u1) ) u1,2
+ u2 u3 ( d2/du12 p(u1) ) u1,1 ] ]
(24)

```

```

> de2 := Prolong(de, 2) : deTRA := Transformation(de2) :
>
> Eq0 := Pullback(deTRA, ToJet(NEQtt, DepVars, notation = jetnumbers)) :
> VS := solve(Eq0, V) :
> Eq1 := numer(subs(V = VS, Pullback(deTRA, ToJet(NEQtx, DepVars, notation
= jetnumbers)))) :
Eq2 := numer(subs(V = VS, Pullback(deTRA, ToJet(NEQty, DepVars, notation
= jetnumbers)))) :
Eq3 := numer(subs(V = VS, Pullback(deTRA, ToJet(NEQxx, DepVars, notation
= jetnumbers)))) :
Eq4 := numer(subs(V = VS, Pullback(deTRA, ToJet(NEQxy, DepVars, notation
= jetnumbers)))) :
Eq5 := numer(subs(V = VS, Pullback(deTRA, ToJet(NEQyy, DepVars, notation
= jetnumbers)))) :

```

```

>
J2 > Eq := [ numer(subs(V = VS, Pullback(deTRA, ToJet(NEQtx, DepVars, notation
= jetnumbers)))) , numer(subs(V = VS, Pullback(deTRA, ToJet(NEQty, DepVars,
notation = jetnumbers)))) , numer(subs(V = VS, Pullback(deTRA, ToJet(NEQxx,
DepVars, notation = jetnumbers)))) , numer(subs(V = VS, Pullback(deTRA,
ToJet(NEQxy, DepVars, notation = jetnumbers)))) , numer(subs(V = VS,
Pullback(deTRA, ToJet(NEQyy, DepVars, notation = jetnumbers)))) ] :

```

```

J2 > Q := (i, j, k, l) → diff(Eq[i], u[j, k, l]) :

```

```

J2 > Q(1, 1, 1, 1)
-u3 ( -64 p(u1)5 u22 ( d2/du12 p(u1) )3 ( d/d u1 p(u1) )6 u33 V211(u1, u2, u3) - 32 p(u1)4
(25)

```

$$\begin{aligned}
& u_2^5 \left( \frac{d^2}{du_1^2} p(u_1) \right)^5 \left( \frac{d}{du_1} p(u_1) \right)^5 VI22(u_1, u_2, u_3) u_3^3 + 32 p(u_1)^5 \\
& u_2^3 \left( \frac{d^2}{du_1^2} p(u_1) \right)^4 \left( \frac{d}{du_1} p(u_1) \right)^5 V2I2(u_1, u_2, u_3) u_3^3 + 192 p(u_1)^4 \\
& u_2^2 \left( \frac{d^2}{du_1^2} p(u_1) \right)^2 \left( \frac{d}{du_1} p(u_1) \right)^8 u_3^3 V2II(u_1, u_2, u_3) - 192 p(u_1)^4 \\
& u_2^3 \left( \frac{d^2}{du_1^2} p(u_1) \right)^2 \left( \frac{d}{du_1} p(u_1) \right)^7 u_3^3 \left( \frac{d^3}{du_1^3} p(u_1) \right) + 48 p(u_1)^4 \\
& u_2^4 \left( \frac{d^2}{du_1^2} p(u_1) \right)^4 \left( \frac{d}{du_1} p(u_1) \right)^6 V222(u_1, u_2, u_3) u_3^3 + 48 p(u_1)^5 \\
& u_2^3 \left( \frac{d^2}{du_1^2} p(u_1) \right)^4 VIII(u_1, u_2, u_3) u_3^3 \left( \frac{d}{du_1} p(u_1) \right)^5 - 224 p(u_1)^4 \\
& u_2^3 \left( \frac{d^2}{du_1^2} p(u_1) \right)^3 VIII(u_1, u_2, u_3) u_3^3 \left( \frac{d}{du_1} p(u_1) \right)^7 + 512 p(u_1)^3 \\
& u_2^3 \left( \frac{d^2}{du_1^2} p(u_1) \right)^2 VIII(u_1, u_2, u_3) u_3^3 \left( \frac{d}{du_1} p(u_1) \right)^9 + 4 p(u_1)^5 \\
& u_2^5 \left( \frac{d^2}{du_1^2} p(u_1) \right)^6 \left( \frac{d}{du_1} p(u_1) \right)^3 VI22(u_1, u_2, u_3) u_3^3 - 16 p(u_1)^5 \\
& u_2^4 \left( \frac{d^2}{du_1^2} p(u_1) \right)^5 \left( \frac{d}{du_1} p(u_1) \right)^4 V222(u_1, u_2, u_3) u_3^3 + 32 \\
& u_2^4 \left( \frac{d}{du_1} p(u_1) \right)^{10} p(u_1)^2 V222(u_1, u_2, u_3) u_3^3 \left( \frac{d^2}{du_1^2} p(u_1) \right)^2 + 96 p(u_1)^3 \\
& u_2^5 \left( \frac{d^2}{du_1^2} p(u_1) \right)^4 \left( \frac{d}{du_1} p(u_1) \right)^7 VI22(u_1, u_2, u_3) u_3^3 - 128 u_2^5 p(u_1)^2 VI22(u_1, u_2, \\
& u_3) \left( \frac{d^2}{du_1^2} p(u_1) \right)^3 u_3^3 \left( \frac{d}{du_1} p(u_1) \right)^9 + 288 u_2^4 p(u_1)^2 VII2(u_1, u_2, \\
& u_3) \left( \frac{d^2}{du_1^2} p(u_1) \right)^2 u_3^3 \left( \frac{d}{du_1} p(u_1) \right)^{10} + 2 p(u_1)^6 u_2^4 \left( \frac{d^2}{du_1^2} p(u_1) \right)^6 VII2(u_1, u_2, u_3) \\
& u_3^3 \left( \frac{d}{du_1} p(u_1) \right)^2 - 4 p(u_1)^6 u_2^3 \left( \frac{d^2}{du_1^2} p(u_1) \right)^5 VIII(u_1, u_2, u_3) u_3^3 \left( \frac{d}{du_1} p(u_1) \right)^3
\end{aligned}$$

$$\begin{aligned}
& -24 u_2^4 p(u_1)^5 \left( \frac{d^2}{du_1^2} p(u_1) \right)^5 VII2(u_1, u_2, u_3) u_3^3 \left( \frac{d}{du_1} p(u_1) \right)^4 + 112 \\
& u_2^4 p(u_1)^4 \left( \frac{d^2}{du_1^2} p(u_1) \right)^4 VII2(u_1, u_2, u_3) u_3^3 \left( \frac{d}{du_1} p(u_1) \right)^6 - 256 \\
& u_2^4 p(u_1)^3 \left( \frac{d^2}{du_1^2} p(u_1) \right)^3 VII2(u_1, u_2, u_3) u_3^3 \left( \frac{d}{du_1} p(u_1) \right)^8 - 8 \\
& u_2^3 p(u_1)^6 \left( \frac{d^3}{du_1^3} p(u_1) \right) \left( \frac{d^2}{du_1^2} p(u_1) \right)^4 u_3^3 \left( \frac{d}{du_1} p(u_1) \right)^3 - 576 p(u_1)^2 \\
& u_2^3 \left( \frac{d}{du_1} p(u_1) \right)^{11} VIII(u_1, u_2, u_3) u_3^3 \left( \frac{d^2}{du_1^2} p(u_1) \right) + 64 \\
& u_2^5 \left( \frac{d}{du_1} p(u_1) \right)^{11} p(u_1) VI22(u_1, u_2, u_3) u_3^3 \left( \frac{d^2}{du_1^2} p(u_1) \right)^2 - 4 \\
& u_2^3 p(u_1)^6 \left( \frac{d^2}{du_1^2} p(u_1) \right)^5 V2I2(u_1, u_2, u_3) u_3^3 \left( \frac{d}{du_1} p(u_1) \right)^3 - 256 u_2^2 p(u_1)^3 \\
& u_3^3 \left( \frac{d}{du_1} p(u_1) \right)^{10} V2II(u_1, u_2, u_3) \left( \frac{d^2}{du_1^2} p(u_1) \right) + 2 \\
& u_2^4 p(u_1)^6 \left( \frac{d^2}{du_1^2} p(u_1) \right)^6 V222(u_1, u_2, u_3) u_3^3 \left( \frac{d}{du_1} p(u_1) \right)^2 + 256 \\
& u_2^3 p(u_1)^3 \left( \frac{d^3}{du_1^3} p(u_1) \right) u_3^3 \left( \frac{d}{du_1} p(u_1) \right)^9 \left( \frac{d^2}{du_1^2} p(u_1) \right) - 64 \\
& u_2^3 p(u_1)^2 \left( \frac{d}{du_1} p(u_1) \right)^{11} V2I2(u_1, u_2, u_3) u_3^3 \left( \frac{d^2}{du_1^2} p(u_1) \right) + 8 u_2^2 p(u_1)^6 \\
& u_3^3 \left( \frac{d^2}{du_1^2} p(u_1) \right)^4 V2II(u_1, u_2, u_3) \left( \frac{d}{du_1} p(u_1) \right)^4 + 128 u_2^3 p(u_1)^3 V2I2(u_1, u_2, \\
& u_3) \left( \frac{d^2}{du_1^2} p(u_1) \right)^2 u_3^3 \left( \frac{d}{du_1} p(u_1) \right)^9 - 64 u_2^4 p(u_1)^3 V222(u_1, u_2, u_3) \left( \frac{d^2}{du_1^2} p(u_1) \right)^3 \\
& u_3^3 \left( \frac{d}{du_1} p(u_1) \right)^8 - 128 u_2^4 \left( \frac{d}{du_1} p(u_1) \right)^{12} p(u_1) VII2(u_1, u_2, u_3) u_3^3 \left( \frac{d^2}{du_1^2} p(u_1) \right) \\
& - 96 p(u_1)^4 u_2^3 \left( \frac{d^2}{du_1^2} p(u_1) \right)^3 \left( \frac{d}{du_1} p(u_1) \right)^7 V2I2(u_1, u_2, u_3) u_3^3 + 64 p(u_1)^5
\end{aligned}$$

$$\begin{aligned}
& u_2^3 \left( \frac{d^2}{du_1^2} p(u_1) \right)^3 \left( \frac{d}{du_1} p(u_1) \right)^5 u_3^3 \left( \frac{d^3}{du_1^3} p(u_1) \right) + 128 u_2^3 p(u_1) \\
& u_3^3 \left( \frac{d^2}{du_1^2} p(u_1) \right) \left( \frac{d}{du_1} p(u_1) \right)^{12} + 8 u_2^3 p(u_1)^6 \left( \frac{d^2}{du_1^2} p(u_1) \right)^6 u_3^3 \left( \frac{d}{du_1} p(u_1) \right)^2 \\
& - 128 u_2^3 p(u_1)^2 u_3^3 \left( \frac{d^2}{du_1^2} p(u_1) \right)^2 \left( \frac{d}{du_1} p(u_1) \right)^{10} - 128 u_2^3 \\
& u_3^3 p(u_1)^2 \left( \frac{d}{du_1} p(u_1) \right)^{11} \left( \frac{d^3}{du_1^3} p(u_1) \right) - 56 p(u_1)^5 \\
& u_2^3 \left( \frac{d^2}{du_1^2} p(u_1) \right)^5 \left( \frac{d}{du_1} p(u_1) \right)^4 u_3^3 - 64 p(u_1)^3 u_2^3 \left( \frac{d^2}{du_1^2} p(u_1) \right)^3 \left( \frac{d}{du_1} p(u_1) \right)^8 u_3^3 \\
& + 128 p(u_1)^4 u_2^3 \left( \frac{d^2}{du_1^2} p(u_1) \right)^4 \left( \frac{d}{du_1} p(u_1) \right)^6 u_3^3 + 128 u_2^2 \left( \frac{d}{du_1} p(u_1) \right)^{12} \\
& u_3^3 p(u_1)^2 V211(u_1, u_2, u_3) + 256 u_2^3 \left( \frac{d}{du_1} p(u_1) \right)^{13} p(u_1) u_3^3 V111(u_1, u_2, u_3) \Big)
\end{aligned}$$

**J2** > Qq := { } :  
**for** *i* **from** 1 **to** 3 **do** **for** *j* **from** 1 **to** 3 **do** **for** *k* **from** *j* **to** 3 **do** **for** *l* **from** *k* **to** 3 **do**  
*Qq* := { *op*(*Qq*), *Q*(*i*, *j*, *k*, *l*) } **od:od:od:od:**

**J2** > nops(Qq)

19

(26)

**J2** > *Qq*

**J2** >

**J2** > *SLV* := solve(*Qq*, [*V111*(*u*<sub>1</sub>, *u*<sub>2</sub>, *u*<sub>3</sub>), *V112*(*u*<sub>1</sub>, *u*<sub>2</sub>, *u*<sub>3</sub>), *V113*(*u*<sub>1</sub>, *u*<sub>2</sub>, *u*<sub>3</sub>), *V122*(*u*<sub>1</sub>, *u*<sub>2</sub>, *u*<sub>3</sub>), *V123*(*u*<sub>1</sub>, *u*<sub>2</sub>, *u*<sub>3</sub>), *V133*(*u*<sub>1</sub>, *u*<sub>2</sub>, *u*<sub>3</sub>), *V211*(*u*<sub>1</sub>, *u*<sub>2</sub>, *u*<sub>3</sub>), *V212*(*u*<sub>1</sub>, *u*<sub>2</sub>, *u*<sub>3</sub>), *V213*(*u*<sub>1</sub>, *u*<sub>2</sub>, *u*<sub>3</sub>), *V222*(*u*<sub>1</sub>, *u*<sub>2</sub>, *u*<sub>3</sub>), *V223*(*u*<sub>1</sub>, *u*<sub>2</sub>, *u*<sub>3</sub>), *V233*(*u*<sub>1</sub>, *u*<sub>2</sub>, *u*<sub>3</sub>), *V311*(*u*<sub>1</sub>, *u*<sub>2</sub>, *u*<sub>3</sub>), *V312*(*u*<sub>1</sub>, *u*<sub>2</sub>, *u*<sub>3</sub>), *V313*(*u*<sub>1</sub>, *u*<sub>2</sub>, *u*<sub>3</sub>), *V322*(*u*<sub>1</sub>, *u*<sub>2</sub>, *u*<sub>3</sub>), *V323*(*u*<sub>1</sub>, *u*<sub>2</sub>, *u*<sub>3</sub>), *V333*(*u*<sub>1</sub>, *u*<sub>2</sub>, *u*<sub>3</sub>)] )

$$SLV := \left[ \left[ \begin{aligned}
& V111(u_1, u_2, u_3) = \frac{1}{2} \left( -u_2 \left( \frac{d^2}{du_1^2} p(u_1) \right)^2 u_3 V123(u_1, u_2, u_3) p(u_1) \right. \right. \\
& \left. \left. + 2 u_2 \left( \frac{d^2}{du_1^2} p(u_1) \right) u_3 V123(u_1, u_2, u_3) \left( \frac{d}{du_1} p(u_1) \right)^2 + 4 \left( \frac{d^3}{du_1^3} p(u_1) \right) p(u_1)^2 \right. \right.
\end{aligned} \right] \right]$$

(27)

$$-12 p(u_1) \left( \frac{d}{du_1} p(u_1) \right) \left( \frac{d^2}{du_1^2} p(u_1) \right) \Bigg/ \left( p(u_1) \left( 2 \left( \frac{d}{du_1} p(u_1) \right)^2 \right. \right.$$

$$\left. - \left( \frac{d^2}{du_1^2} p(u_1) \right) p(u_1) \right) \Bigg), VII2(u_1, u_2, u_3)$$

$$= \frac{\left( \frac{d}{du_1} p(u_1) \right) u_2 VI23(u_1, u_2, u_3) u_3 - 4 p(u_1)}{p(u_1) u_2}, VII3(u_1, u_2, u_3)$$

$$= \frac{\left( \frac{d}{du_1} p(u_1) \right) u_2 VI23(u_1, u_2, u_3) u_3 - 4 p(u_1)}{p(u_1) u_3}, VI22(u_1, u_2, u_3) = 0, VI23(u_1, u_2,$$

$$u_3) = VI23(u_1, u_2, u_3), VI33(u_1, u_2, u_3) = 0, V211(u_1, u_2, u_3) =$$

$$- \frac{1}{2} \left( u_2 \left( \left( \frac{d^2}{du_1^2} p(u_1) \right)^2 u_3 V223(u_1, u_2, u_3) p(u_1) - 2 \left( \frac{d^2}{du_1^2} p(u_1) \right) u_3 V223(u_1, u_2,$$

$$u_3) \left( \frac{d}{du_1} p(u_1) \right)^2 - 4 p(u_1) \left( \frac{d^2}{du_1^2} p(u_1) \right)^2 + 4 p(u_1) \left( \frac{d^3}{du_1^3} p(u_1) \right) \left( \frac{d}{du_1} p(u_1) \right)$$

$$- 4 \left( \frac{d}{du_1} p(u_1) \right)^2 \left( \frac{d^2}{du_1^2} p(u_1) \right) \Bigg) \Bigg/ \left( p(u_1) \left( 2 \left( \frac{d}{du_1} p(u_1) \right)^2 \right. \right.$$



$$- \left( \frac{d^2}{du_1^2} p(u_1) \right) p(u_1) \Bigg) \Bigg), V212(u_1, u_2, u_3) = \frac{u_3 \left( \frac{d}{du_1} p(u_1) \right) V223(u_1, u_2, u_3)}{p(u_1)},$$

$$V213(u_1, u_2, u_3) = \frac{u_2 \left( \frac{d}{du_1} p(u_1) \right) (V223(u_1, u_2, u_3) u_3 + 4)}{p(u_1) u_3}, V222(u_1, u_2, u_3) = 0,$$

$$V223(u_1, u_2, u_3) = V223(u_1, u_2, u_3), V233(u_1, u_2, u_3) = 0, V311(u_1, u_2, u_3)$$

$$\begin{aligned} &= \frac{1}{2} \frac{u_2 \left( \frac{d^2}{du_1^2} p(u_1) \right) u_3 V323(u_1, u_2, u_3)}{p(u_1)} - \left( 2 \left( -p(u_1) \left( \frac{d^2}{du_1^2} p(u_1) \right)^2 \right. \right. \\ &\quad \left. \left. + p(u_1) \left( \frac{d^3}{du_1^3} p(u_1) \right) \left( \frac{d}{du_1} p(u_1) \right) - \left( \frac{d}{du_1} p(u_1) \right)^2 \left( \frac{d^2}{du_1^2} p(u_1) \right) \right) u_3 \right) / \\ &\quad \left( p(u_1) \left( 2 \left( \frac{d}{du_1} p(u_1) \right)^2 - \left( \frac{d^2}{du_1^2} p(u_1) \right) p(u_1) \right) \right), V312(u_1, u_2, u_3) \\ &= \frac{u_3 \left( \frac{d}{du_1} p(u_1) \right) V323(u_1, u_2, u_3)}{p(u_1)} + \frac{4 u_3 \left( \frac{d}{du_1} p(u_1) \right)}{p(u_1) u_2}, V313(u_1, u_2, u_3) \\ &= \frac{\left( \frac{d}{du_1} p(u_1) \right) u_2 V323(u_1, u_2, u_3)}{p(u_1)}, V322(u_1, u_2, u_3) = 0, V323(u_1, u_2, u_3) = V323(u_1, \\ &\quad u_2, u_3), V333(u_1, u_2, u_3) = 0 \Bigg] \Bigg] \end{aligned}$$

**J2** >  $U1a := \text{subs}(\text{FromJet}(\text{SLV}[1], \text{DepVars}), U1)$

$$\begin{aligned} U1a := & \frac{1}{2} \left( \left( - \left( \frac{\partial}{\partial x} u(t, x, y) \right) D^{(2)}(p) \left( \frac{\partial}{\partial t} u(t, x, y) \right)^2 \left( \frac{\partial}{\partial y} u(t, x, y) \right) V123 \left( \frac{\partial}{\partial t} u(t, x, \right. \right. \right. \\ & \left. \left. \left. y \right), \frac{\partial}{\partial x} u(t, x, y), \frac{\partial}{\partial y} u(t, x, y) \right) p \left( \frac{\partial}{\partial t} u(t, x, y) \right) + 2 \left( \frac{\partial}{\partial x} u(t, x, y) \right) D^{(2)}(p) \left( \frac{\partial}{\partial t} u(t, \right. \right. \end{aligned} \quad (28)$$

$$\begin{aligned}
& x, y) \Big) \left( \frac{\partial}{\partial y} u(t, x, y) \right) VI23 \left( \frac{\partial}{\partial t} u(t, x, y), \frac{\partial}{\partial x} u(t, x, y), \frac{\partial}{\partial y} u(t, x, \right. \\
& y) \Big) D(p) \left( \frac{\partial}{\partial t} u(t, x, y) \right)^2 + 4 D^{(3)}(p) \left( \frac{\partial}{\partial t} u(t, x, y) \right) p \left( \frac{\partial}{\partial t} u(t, x, y) \right)^2 \\
& - 12 p \left( \frac{\partial}{\partial t} u(t, x, y) \right) D(p) \left( \frac{\partial}{\partial t} u(t, x, y) \right) D^{(2)}(p) \left( \frac{\partial}{\partial t} u(t, x, y) \right) \Big) \left( \frac{\partial^2}{\partial t^2} u(t, x, y) \right) \Big) \\
& \Big/ \left( p \left( \frac{\partial}{\partial t} u(t, x, y) \right) \left( -D^{(2)}(p) \left( \frac{\partial}{\partial t} u(t, x, y) \right) p \left( \frac{\partial}{\partial t} u(t, x, y) \right) \right. \right. \\
& \left. \left. + 2 D(p) \left( \frac{\partial}{\partial t} u(t, x, y) \right)^2 \right) \right) \\
& + \frac{1}{p \left( \frac{\partial}{\partial t} u(t, x, y) \right) \left( \frac{\partial}{\partial x} u(t, x, y) \right)} \left( \left( D(p) \left( \frac{\partial}{\partial t} u(t, x, y) \right) \left( \frac{\partial}{\partial x} u(t, x, \right. \right. \right. \\
& y) \Big) VI23 \left( \frac{\partial}{\partial t} u(t, x, y), \frac{\partial}{\partial x} u(t, x, y), \frac{\partial}{\partial y} u(t, x, y) \right) \left( \frac{\partial}{\partial y} u(t, x, y) \right) - 4 p \left( \frac{\partial}{\partial t} u(t, x, \right. \\
& y) \Big) \left( \frac{\partial^2}{\partial x \partial t} u(t, x, y) \right) \Big) + \frac{1}{p \left( \frac{\partial}{\partial t} u(t, x, y) \right) \left( \frac{\partial}{\partial y} u(t, x, y) \right)} \left( \left( D(p) \left( \frac{\partial}{\partial t} u(t, x, \right. \right. \right. \\
& y) \Big) \left( \frac{\partial}{\partial x} u(t, x, y) \right) VI23 \left( \frac{\partial}{\partial t} u(t, x, y), \frac{\partial}{\partial x} u(t, x, y), \frac{\partial}{\partial y} u(t, x, y) \right) \left( \frac{\partial}{\partial y} u(t, x, y) \right) \\
& - 4 p \left( \frac{\partial}{\partial t} u(t, x, y) \right) \Big) \left( \frac{\partial^2}{\partial y \partial t} u(t, x, y) \right) \Big) + VI23 \left( \frac{\partial}{\partial t} u(t, x, y), \frac{\partial}{\partial x} u(t, x, y), \right. \\
& \left. \frac{\partial}{\partial y} u(t, x, y) \right) \left( \frac{\partial^2}{\partial y \partial x} u(t, x, y) \right)
\end{aligned}$$

**J2** >  $U2a := \text{subs}(\text{FromJet}(\text{SLV}[1], \text{DepVars}), U2)$

$$\begin{aligned}
U2a := & -\frac{1}{2} \left( \left( \frac{\partial}{\partial x} u(t, x, y) \right) \left( D^{(2)}(p) \left( \frac{\partial}{\partial t} u(t, x, y) \right)^2 \left( \frac{\partial}{\partial y} u(t, x, y) \right) V223 \left( \frac{\partial}{\partial t} u(t, x, \right. \right. \right. \\
& y), \frac{\partial}{\partial x} u(t, x, y), \frac{\partial}{\partial y} u(t, x, y) \Big) p \left( \frac{\partial}{\partial t} u(t, x, y) \right) - 2 D^{(2)}(p) \left( \frac{\partial}{\partial t} u(t, x, y) \right) \left( \frac{\partial}{\partial y} u(t, \right. \\
& x, y) \Big) V223 \left( \frac{\partial}{\partial t} u(t, x, y), \frac{\partial}{\partial x} u(t, x, y), \frac{\partial}{\partial y} u(t, x, y) \right) D(p) \left( \frac{\partial}{\partial t} u(t, x, y) \right)^2 \\
& - 4 p \left( \frac{\partial}{\partial t} u(t, x, y) \right) D^{(2)}(p) \left( \frac{\partial}{\partial t} u(t, x, y) \right)^2 + 4 p \left( \frac{\partial}{\partial t} u(t, x, y) \right) D^{(3)}(p) \left( \frac{\partial}{\partial t} u(t, x, \right. \\
& y) \Big) D(p) \left( \frac{\partial}{\partial t} u(t, x, y) \right) - 4 D(p) \left( \frac{\partial}{\partial t} u(t, x, y) \right)^2 D^{(2)}(p) \left( \frac{\partial}{\partial t} u(t, x, y) \right) \Big) \left( \frac{\partial^2}{\partial t^2} u(t, \right. \\
& x, y) \Big) \Big/ \left( p \left( \frac{\partial}{\partial t} u(t, x, y) \right) \left( -D^{(2)}(p) \left( \frac{\partial}{\partial t} u(t, x, y) \right) p \left( \frac{\partial}{\partial t} u(t, x, y) \right) \right. \right.
\end{aligned} \tag{29}$$

$$\begin{aligned}
& + 2 D(p) \left( \left( \frac{\partial}{\partial t} u(t, x, y) \right)^2 \right) \Bigg) + \frac{1}{p \left( \frac{\partial}{\partial t} u(t, x, y) \right)} \left( \left( \frac{\partial}{\partial y} u(t, x, y) \right) D(p) \left( \frac{\partial}{\partial t} u(t, \right. \right. \\
& x, y) \Big) V223 \left( \frac{\partial}{\partial t} u(t, x, y), \frac{\partial}{\partial x} u(t, x, y), \frac{\partial}{\partial y} u(t, x, y) \right) \left( \frac{\partial^2}{\partial x \partial t} u(t, x, y) \right) \Bigg) \\
& + \frac{1}{p \left( \frac{\partial}{\partial t} u(t, x, y) \right) \left( \frac{\partial}{\partial y} u(t, x, y) \right)} \left( \left( \frac{\partial}{\partial x} u(t, x, y) \right) D(p) \left( \frac{\partial}{\partial t} u(t, x, \right. \right. \\
& y) \Big) \left( V223 \left( \frac{\partial}{\partial t} u(t, x, y), \frac{\partial}{\partial x} u(t, x, y), \frac{\partial}{\partial y} u(t, x, y) \right) \left( \frac{\partial}{\partial y} u(t, x, y) \right) \right. \\
& + 4 \left( \frac{\partial^2}{\partial y \partial t} u(t, x, y) \right) \Bigg) + V223 \left( \frac{\partial}{\partial t} u(t, x, y), \frac{\partial}{\partial x} u(t, x, y), \frac{\partial}{\partial y} u(t, x, \right. \\
& y) \Big) \left( \frac{\partial^2}{\partial y \partial x} u(t, x, y) \right)
\end{aligned}$$

**J2** >  $U3a := \text{subs}(\text{FromJet}(\text{SLV}[1], \text{DepVars}), U3)$

$$\begin{aligned}
U3a := & \left( \frac{1}{2} \frac{1}{p \left( \frac{\partial}{\partial t} u(t, x, y) \right)} \left( \left( \frac{\partial}{\partial x} u(t, x, y) \right) D^{(2)}(p) \left( \frac{\partial}{\partial t} u(t, x, y) \right) \left( \frac{\partial}{\partial y} u(t, x, \right. \right. \right. \quad (30) \\
& y) \Big) V323 \left( \frac{\partial}{\partial t} u(t, x, y), \frac{\partial}{\partial x} u(t, x, y), \frac{\partial}{\partial y} u(t, x, y) \right) \Big) - \left( 2 \left( -p \left( \frac{\partial}{\partial t} u(t, x, \right. \right. \right. \\
& y) \Big) D^{(2)}(p) \left( \frac{\partial}{\partial t} u(t, x, y) \right)^2 + p \left( \frac{\partial}{\partial t} u(t, x, y) \right) D^{(3)}(p) \left( \frac{\partial}{\partial t} u(t, x, y) \right) D(p) \left( \frac{\partial}{\partial t} u(t, \right. \\
& x, y) \Big) - D(p) \left( \frac{\partial}{\partial t} u(t, x, y) \right)^2 D^{(2)}(p) \left( \frac{\partial}{\partial t} u(t, x, y) \right) \left( \frac{\partial}{\partial y} u(t, x, y) \right) \Bigg) / \\
& \left( p \left( \frac{\partial}{\partial t} u(t, x, y) \right) \left( -D^{(2)}(p) \left( \frac{\partial}{\partial t} u(t, x, y) \right) p \left( \frac{\partial}{\partial t} u(t, x, y) \right) + 2 D(p) \left( \frac{\partial}{\partial t} u(t, x, \right. \right. \right. \\
& y) \Big)^2 \Bigg) \left( \frac{\partial^2}{\partial t^2} u(t, x, y) \right) \\
& + \left( \frac{1}{p \left( \frac{\partial}{\partial t} u(t, x, y) \right)} \left( \left( \frac{\partial}{\partial y} u(t, x, y) \right) D(p) \left( \frac{\partial}{\partial t} u(t, x, y) \right) V323 \left( \frac{\partial}{\partial t} u(t, x, y), \right. \right. \right. \\
& \frac{\partial}{\partial x} u(t, x, y), \frac{\partial}{\partial y} u(t, x, y) \Big) + \frac{4 \left( \frac{\partial}{\partial y} u(t, x, y) \right) D(p) \left( \frac{\partial}{\partial t} u(t, x, y) \right)}{p \left( \frac{\partial}{\partial t} u(t, x, y) \right) \left( \frac{\partial}{\partial x} u(t, x, y) \right)} \Bigg) \left( \frac{\partial^2}{\partial x \partial t} u(t, \right. \\
& x, y) \Big) + \frac{1}{p \left( \frac{\partial}{\partial t} u(t, x, y) \right)} \left( D(p) \left( \frac{\partial}{\partial t} u(t, x, y) \right) \left( \frac{\partial}{\partial x} u(t, x, y) \right) V323 \left( \frac{\partial}{\partial t} u(t, x, \right. \right.
\end{aligned}$$

$$y), \frac{\partial}{\partial x} u(t, x, y), \frac{\partial}{\partial y} u(t, x, y) \left( \frac{\partial^2}{\partial y \partial t} u(t, x, y) \right) \Big) + V323 \left( \frac{\partial}{\partial t} u(t, x, y), \frac{\partial}{\partial x} u(t, x, y), \frac{\partial}{\partial y} u(t, x, y) \right) \left( \frac{\partial^2}{\partial y \partial x} u(t, x, y) \right)$$

**M >**  $U1a := \text{FromJet}(\text{simplify}(\text{Pullback}(\text{deTRA}, \text{subs}(\text{SLV}[1], \text{ToJet}(U1, \text{DepVars}, \text{notation} = \text{jetnumbers}))) , \text{DepVars})$

$$\begin{aligned} U1a := & \left( 2 \left( D(p) \left( \frac{\partial}{\partial t} u(t, x, y) \right) \left( \frac{\partial}{\partial x} u(t, x, y) \right) \left( \frac{\partial}{\partial y} u(t, x, y) \right) D^{(3)}(p) \left( \frac{\partial}{\partial t} u(t, x, y) \right) \left( \frac{\partial^2}{\partial t^2} u(t, x, y) \right) p \left( \frac{\partial}{\partial t} u(t, x, y) \right) - D(p) \left( \frac{\partial}{\partial t} u(t, x, y) \right)^2 \left( \frac{\partial}{\partial x} u(t, x, y) \right) \left( \frac{\partial}{\partial y} u(t, x, y) \right) D^{(2)}(p) \left( \frac{\partial}{\partial t} u(t, x, y) \right) \left( \frac{\partial^2}{\partial t^2} u(t, x, y) \right) + 4 D(p) \left( \frac{\partial}{\partial t} u(t, x, y) \right)^2 p \left( \frac{\partial}{\partial t} u(t, x, y) \right) \left( \frac{\partial^2}{\partial y \partial x} u(t, x, y) \right) - 2 D^{(2)}(p) \left( \frac{\partial}{\partial t} u(t, x, y) \right) p \left( \frac{\partial}{\partial t} u(t, x, y) \right)^2 \left( \frac{\partial^2}{\partial y \partial x} u(t, x, y) \right) - p \left( \frac{\partial}{\partial t} u(t, x, y) \right) \left( \frac{\partial}{\partial x} u(t, x, y) \right) \left( \frac{\partial}{\partial y} u(t, x, y) \right) D^{(2)}(p) \left( \frac{\partial}{\partial t} u(t, x, y) \right)^2 \left( \frac{\partial^2}{\partial t^2} u(t, x, y) \right) \right) \Bigg) / \left( \left( -D^{(2)}(p) \left( \frac{\partial}{\partial t} u(t, x, y) \right) p \left( \frac{\partial}{\partial t} u(t, x, y) \right) + 2 D(p) \left( \frac{\partial}{\partial t} u(t, x, y) \right)^2 \right) \left( \frac{\partial}{\partial x} u(t, x, y) \right) \left( \frac{\partial}{\partial y} u(t, x, y) \right) D(p) \left( \frac{\partial}{\partial t} u(t, x, y) \right) \right) \end{aligned} \quad (31)$$

**J2 >**  $U2a := \text{FromJet}(\text{simplify}(\text{Pullback}(\text{deTRA}, \text{subs}(\text{SLV}[1], \text{ToJet}(U2, \text{DepVars}, \text{notation} = \text{jetnumbers}))) , \text{DepVars})$

$$\begin{aligned} U2a := & - \left( 2 \left( \frac{\partial}{\partial x} u(t, x, y) \right) \left( -p \left( \frac{\partial}{\partial t} u(t, x, y) \right) \left( \frac{\partial}{\partial y} u(t, x, y) \right) D^{(2)}(p) \left( \frac{\partial}{\partial t} u(t, x, y) \right)^2 \left( \frac{\partial^2}{\partial t^2} u(t, x, y) \right) + D(p) \left( \frac{\partial}{\partial t} u(t, x, y) \right) \left( \frac{\partial}{\partial y} u(t, x, y) \right) \left( \frac{\partial^2}{\partial t^2} u(t, x, y) \right) D^{(3)}(p) \left( \frac{\partial}{\partial t} u(t, x, y) \right) p \left( \frac{\partial}{\partial t} u(t, x, y) \right) - D(p) \left( \frac{\partial}{\partial t} u(t, x, y) \right)^2 \left( \frac{\partial}{\partial y} u(t, x, y) \right) \left( \frac{\partial^2}{\partial t^2} u(t, x, y) \right) D^{(2)}(p) \left( \frac{\partial}{\partial t} u(t, x, y) \right) - 4 D(p) \left( \frac{\partial}{\partial t} u(t, x, y) \right)^3 \left( \frac{\partial^2}{\partial y \partial t} u(t, x, y) \right) + 2 D(p) \left( \frac{\partial}{\partial t} u(t, x, y) \right) \left( \frac{\partial^2}{\partial y \partial t} u(t, x, y) \right) D^{(2)}(p) \left( \frac{\partial}{\partial t} u(t, x, y) \right) p \left( \frac{\partial}{\partial t} u(t, x, y) \right) \right) \Bigg) / \left( p \left( \frac{\partial}{\partial t} u(t, x, y) \right) \left( -D^{(2)}(p) \left( \frac{\partial}{\partial t} u(t, x, y) \right) p \left( \frac{\partial}{\partial t} u(t, x, y) \right) + 2 D(p) \left( \frac{\partial}{\partial t} u(t, x, y) \right)^2 \right) \left( \frac{\partial}{\partial y} u(t, x, y) \right) \right) \end{aligned} \quad (32)$$

**J2** >  $U3a := \text{FromJet}(\text{simplify}(\text{Pullback}(\text{deTRA}, \text{subs}(\text{SLV}[1], \text{ToJet}(U3, \text{DepVars}, \text{notation} = \text{jetnumbers}))) , \text{DepVars})$

$$\begin{aligned}
 U3a := & - \left( 2 \left( -2p \left( \frac{\partial}{\partial t} u(t, x, y) \right) \left( \frac{\partial}{\partial x} u(t, x, y) \right) \left( \frac{\partial}{\partial y} u(t, x, y) \right) D^{(2)}(p) \left( \frac{\partial}{\partial t} u(t, x, \right. \right. \\
 & \left. \left. y) \right)^2 \left( \frac{\partial^2}{\partial t^2} u(t, x, y) \right) + D(p) \left( \frac{\partial}{\partial t} u(t, x, y) \right) \left( \frac{\partial}{\partial x} u(t, x, y) \right) \left( \frac{\partial}{\partial y} u(t, x, \right. \right. \\
 & \left. \left. y) \right) D^{(3)}(p) \left( \frac{\partial}{\partial t} u(t, x, y) \right) \left( \frac{\partial^2}{\partial t^2} u(t, x, y) \right) p \left( \frac{\partial}{\partial t} u(t, x, y) \right) + D(p) \left( \frac{\partial}{\partial t} u(t, x, \right. \right. \\
 & \left. \left. y) \right)^2 \left( \frac{\partial}{\partial x} u(t, x, y) \right) \left( \frac{\partial}{\partial y} u(t, x, y) \right) D^{(2)}(p) \left( \frac{\partial}{\partial t} u(t, x, y) \right) \left( \frac{\partial^2}{\partial t^2} u(t, x, y) \right) \\
 & + 4 \left( \frac{\partial}{\partial x} u(t, x, y) \right) D(p) \left( \frac{\partial}{\partial t} u(t, x, y) \right)^3 \left( \frac{\partial^2}{\partial y \partial t} u(t, x, y) \right) - 2p \left( \frac{\partial}{\partial t} u(t, x, \right. \\
 & \left. y) \right) \left( \frac{\partial}{\partial x} u(t, x, y) \right) D(p) \left( \frac{\partial}{\partial t} u(t, x, y) \right) D^{(2)}(p) \left( \frac{\partial}{\partial t} u(t, x, y) \right) \left( \frac{\partial^2}{\partial y \partial t} u(t, x, y) \right) \\
 & + 4 D(p) \left( \frac{\partial}{\partial t} u(t, x, y) \right)^2 p \left( \frac{\partial}{\partial t} u(t, x, y) \right) \left( \frac{\partial^2}{\partial y \partial x} u(t, x, y) \right) - 2 D^{(2)}(p) \left( \frac{\partial}{\partial t} u(t, x, \right. \\
 & \left. y) \right) p \left( \frac{\partial}{\partial t} u(t, x, y) \right)^2 \left( \frac{\partial^2}{\partial y \partial x} u(t, x, y) \right) \Bigg) \Bigg/ \left( p \left( \frac{\partial}{\partial t} u(t, x, y) \right) \left( -D^{(2)}(p) \left( \frac{\partial}{\partial t} u(t, \right. \right. \right. \\
 & \left. \left. x, y) \right) p \left( \frac{\partial}{\partial t} u(t, x, y) \right) + 2 D(p) \left( \frac{\partial}{\partial t} u(t, x, y) \right)^2 \right) \left( \frac{\partial}{\partial x} u(t, x, y) \right) \Bigg)
 \end{aligned} \tag{33}$$

**J2** >  $\text{DGsetup}([t, x, y], M) :$

>  $Et := \text{evalDG}(\text{DirectionalCovariantDerivative}(D\_t, g, C) + U1a \cdot g) :$   
 $Ex := \text{evalDG}(\text{DirectionalCovariantDerivative}(D\_x, g, C) + U2a \cdot g) :$   
 $Ey := \text{evalDG}(\text{DirectionalCovariantDerivative}(D\_y, g, C) + U3a \cdot g) :$

>  $Eq000 := \text{TensorInnerProduct}(g, Et, dt \& t \, dt) :$   
 $Eq001 := \text{TensorInnerProduct}(g, Et, dt \& t \, dx) :$   
 $Eq002 := \text{TensorInnerProduct}(g, Et, dt \& t \, dy) :$   
 $Eq011 := \text{TensorInnerProduct}(g, Et, dx \& t \, dx) :$   
 $Eq012 := \text{TensorInnerProduct}(g, Et, dx \& t \, dy) :$   
 $Eq022 := \text{TensorInnerProduct}(g, Et, dy \& t \, dy) :$   
 $Eq100 := \text{TensorInnerProduct}(g, Ex, dt \& t \, dt) :$   
 $Eq101 := \text{TensorInnerProduct}(g, Ex, dt \& t \, dx) :$   
 $Eq102 := \text{TensorInnerProduct}(g, Ex, dt \& t \, dy) :$   
 $Eq111 := \text{TensorInnerProduct}(g, Ex, dx \& t \, dx) :$   
 $Eq112 := \text{TensorInnerProduct}(g, Ex, dx \& t \, dy) :$   
 $Eq122 := \text{TensorInnerProduct}(g, Ex, dy \& t \, dy) :$   
 $Eq200 := \text{TensorInnerProduct}(g, Ey, dt \& t \, dt) :$   
 $Eq201 := \text{TensorInnerProduct}(g, Ey, dt \& t \, dx) :$   
 $Eq202 := \text{TensorInnerProduct}(g, Ey, dt \& t \, dy) :$   
 $Eq211 := \text{TensorInnerProduct}(g, Ey, dx \& t \, dx) :$   
 $Eq212 := \text{TensorInnerProduct}(g, Ey, dx \& t \, dy) :$   
 $Eq222 := \text{TensorInnerProduct}(g, Ey, dy \& t \, dy) :$

>  $sa := \text{solve}(\{Eq000=0, Eq001=0, Eq002=0, Eq011=0, Eq012=0, Eq022=0, Eq100=0, Eq101=0, Eq102=0, Eq111=0, Eq112=0, Eq122=0, Eq200=0, Eq201=0, Eq202=0,$

$Eq211=0, Eq212=0, Eq222=0\}$ ,  $[a000, a001, a002, a010, a011, a012, a020, a021, a022, a101, a102, a111, a112, a121, a122, a202, a212, a222]$  ) :

>  $C1 := evalDG( subs( \{op(op(sA))\}, C) ) :$

>  $evalDG( CovariantDerivative(g, C1) + g \&t (U1a \cdot dt + U2a \cdot dx + U3a \cdot dy) );$   
 $0 \ dt \ dt \ dt$

(34)

>  $R1 := CurvatureTensor(C1) : Ric1 := RicciTensor(R1) : T1 := SymmetrizeIndices(Ric1, [1, 2], "Symmetric") : Res := evalDG(T1 - V \cdot g) :$

>  $NEQtt := ContractIndices(Res, D\_t \&t D\_t, [[1, 1], [2, 2]]) : NEQtx := ContractIndices(Res, D\_t \&t D\_x, [[1, 1], [2, 2]]) :$

$NEQty := ContractIndices(Res, D\_t \&t D\_y, [[1, 1], [2, 2]]) : NEQxx := ContractIndices(Res, D\_x \&t D\_x, [[1, 1], [2, 2]]) :$

$NEQxy := ContractIndices(Res, D\_x \&t D\_y, [[1, 1], [2, 2]]) : NEQyy := ContractIndices(Res, D\_y \&t D\_y, [[1, 1], [2, 2]]) :$

>

>  $DGsetup([t, x, y], [u], J2, 4) :$

>  $de := DifferentialEquationData([F], [u_1, 2])$

$$de := \left[ \{u_{1,2}\}, \left[ 2 u_2 \left( \frac{d}{du_1} p(u_1) \right) u_{1,3} + 2 p(u_1) u_{2,3} + 2 u_3 \left( \frac{d}{du_1} p(u_1) \right) u_{1,2} \right. \right. \\ \left. \left. + u_2 u_3 \left( \frac{d^2}{du_1^2} p(u_1) \right) u_{1,1} \right] \right] \quad (35)$$

>  $de2 := Prolong(de, 2) : deTRA := Transformation(de2) :$

>

>  $Eq0 := Pullback(deTRA, ToJet(NEQtt, DepVars, notation = jetnumbers)) :$

>  $VS := solve(Eq0, V) :$

>  $Eq1 := numer(subs(V = VS, Pullback(deTRA, ToJet(NEQtx, DepVars, notation = jetnumbers)))) :$

$Eq2 := numer(subs(V = VS, Pullback(deTRA, ToJet(NEQty, DepVars, notation = jetnumbers)))) :$

$Eq3 := numer(subs(V = VS, Pullback(deTRA, ToJet(NEQxx, DepVars, notation = jetnumbers)))) :$

$Eq4 := numer(subs(V = VS, Pullback(deTRA, ToJet(NEQxy, DepVars, notation = jetnumbers)))) :$

$Eq5 := numer(subs(V = VS, Pullback(deTRA, ToJet(NEQyy, DepVars, notation = jetnumbers)))) :$

**J2** >  $simplify([Eq1, Eq2, Eq3, Eq4, Eq5])$

$$\left[ 0, 0, 0, \right.$$

(36)

$$- \left( \frac{d}{du_1} p(u_1) \right)^2 u_2 p(u_1)^2 u_3 \left( 4 \left( \frac{d}{du_1} p(u_1) \right)^4 u_2 u_3 p(u_1)^2 \left( \frac{d^3}{du_1^3} p(u_1) \right)^2 u_{1,1} u_{1,3} \right. \\ \left. \left( \frac{d^2}{du_1^2} p(u_1) \right) \right]$$

$$\begin{aligned}
& -4 \left( \frac{d}{du_1} p(u_1) \right)^2 u_2 u_3 p(u_1)^3 \left( \frac{d^3}{du_1^3} p(u_1) \right)^2 u_{1,1} u_{1,3} \left( \frac{d^2}{du_1^2} p(u_1) \right)^2 \\
& -2 p(u_1)^3 \left( \frac{d^2}{du_1^2} p(u_1) \right)^4 \left( \frac{d}{du_1} p(u_1) \right) u_{1,3} u_2 u_3 \left( \frac{d^3}{du_1^3} p(u_1) \right) u_{1,1} \\
& +24 p(u_1) \left( \frac{d}{du_1} p(u_1) \right)^5 u_2 u_{1,3} u_3 \left( \frac{d^3}{du_1^3} p(u_1) \right) u_{1,1} \left( \frac{d^2}{du_1^2} p(u_1) \right)^2 \\
& -12 \left( \frac{d}{du_1} p(u_1) \right)^4 u_2 p(u_1)^2 u_3 \left( \frac{d^4}{du_1^4} p(u_1) \right) u_{1,3} \left( \frac{d^2}{du_1^2} p(u_1) \right)^2 u_{1,1} \\
& +6 \left( \frac{d}{du_1} p(u_1) \right)^2 u_2 p(u_1)^3 u_3 \left( \frac{d^4}{du_1^4} p(u_1) \right) u_{1,3} \left( \frac{d^2}{du_1^2} p(u_1) \right)^3 u_{1,1} \\
& +8 \left( \frac{d}{du_1} p(u_1) \right)^6 u_2 p(u_1) u_3 \left( \frac{d^4}{du_1^4} p(u_1) \right) u_{1,3} \left( \frac{d^2}{du_1^2} p(u_1) \right) u_{1,1} \\
& +18 p(u_1)^3 \left( \frac{d^2}{du_1^2} p(u_1) \right)^4 \left( \frac{d}{du_1} p(u_1) \right)^2 u_{1,3} u_{2,3} \\
& -72 p(u_1)^2 \left( \frac{d^2}{du_1^2} p(u_1) \right)^3 \left( \frac{d}{du_1} p(u_1) \right)^4 u_{1,3} u_{2,3} \\
& +72 p(u_1) \left( \frac{d}{du_1} p(u_1) \right)^6 u_{1,3} u_{2,3} \left( \frac{d^2}{du_1^2} p(u_1) \right)^2 \\
& +72 \left( \frac{d}{du_1} p(u_1) \right)^7 u_{2,3} u_3 \left( \frac{d^2}{du_1^2} p(u_1) \right)^2 u_{1,1} \\
& -64 \left( \frac{d}{du_1} p(u_1) \right)^8 u_3 \left( \frac{d^3}{du_1^3} p(u_1) \right) u_{1,1} u_{2,3} \\
& +16 \left( \frac{d}{du_1} p(u_1) \right)^6 p(u_1)^2 \left( \frac{d^4}{du_1^4} p(u_1) \right) u_{1,3} u_{2,3} \\
& -64 \left( \frac{d}{du_1} p(u_1) \right)^7 \left( \frac{d^3}{du_1^3} p(u_1) \right) u_{1,3} p(u_1) u_{2,3} \\
& +8 \left( \frac{d}{du_1} p(u_1) \right)^4 p(u_1)^3 \left( \frac{d^3}{du_1^3} p(u_1) \right)^2 u_{1,3} u_{2,3} \\
& +16 \left( \frac{d}{du_1} p(u_1) \right)^7 u_2 p(u_1) \left( \frac{d^4}{du_1^4} p(u_1) \right) u_{1,3}^2
\end{aligned}$$

$$\begin{aligned}
& + 8 \left( \frac{d}{du_1} p(u_1) \right)^5 u_2 p(u_1)^2 \left( \frac{d^3}{du_1^3} p(u_1) \right)^2 u_{1,3}^2 \\
& - 72 p(u_1) \left( \frac{d^2}{du_1^2} p(u_1) \right)^3 \left( \frac{d}{du_1} p(u_1) \right)^5 u_{1,3}^2 u_2 + 18 p(u_1)^2 \left( \frac{d^2}{du_1^2} p(u_1) \right)^4 \\
& u_{1,3}^2 \left( \frac{d}{du_1} p(u_1) \right)^3 u_2 + 2 p(u_1)^5 \left( \frac{d^3}{du_1^3} p(u_1) \right)^2 u_{1,3} u_{2,3} \left( \frac{d^2}{du_1^2} p(u_1) \right)^2 \\
& - 2 p(u_1)^5 \left( \frac{d^4}{du_1^4} p(u_1) \right) u_{1,3} \left( \frac{d^2}{du_1^2} p(u_1) \right)^3 u_{2,3} \\
& - 64 \left( \frac{d}{du_1} p(u_1) \right)^8 u_2 \left( \frac{d^3}{du_1^3} p(u_1) \right) u_{1,3}^2 + 72 u_2 \left( \frac{d}{du_1} p(u_1) \right)^7 \\
& u_{1,3}^2 \left( \frac{d^2}{du_1^2} p(u_1) \right)^2 \\
& - 24 \left( \frac{d}{du_1} p(u_1) \right)^5 u_3 p(u_1)^2 \left( \frac{d^4}{du_1^4} p(u_1) \right) u_{1,1} u_{2,3} \left( \frac{d^2}{du_1^2} p(u_1) \right) \\
& + 12 \left( \frac{d}{du_1} p(u_1) \right)^3 u_3 p(u_1)^3 \left( \frac{d^4}{du_1^4} p(u_1) \right) u_{1,1} u_{2,3} \left( \frac{d^2}{du_1^2} p(u_1) \right)^2 \\
& + 9 p(u_1)^2 \left( \frac{d^2}{du_1^2} p(u_1) \right)^5 u_{1,1} u_2 \left( \frac{d}{du_1} p(u_1) \right)^2 u_{1,3} u_3 \\
& - 36 p(u_1) \left( \frac{d^2}{du_1^2} p(u_1) \right)^4 \left( \frac{d}{du_1} p(u_1) \right)^4 u_{1,1} u_2 u_{1,3} u_3 \\
& - 8 \left( \frac{d}{du_1} p(u_1) \right)^3 u_3 p(u_1)^3 \left( \frac{d^3}{du_1^3} p(u_1) \right)^2 u_{1,1} u_{2,3} \left( \frac{d^2}{du_1^2} p(u_1) \right) \\
& + 2 \left( \frac{d}{du_1} p(u_1) \right) u_3 p(u_1)^4 \left( \frac{d^3}{du_1^3} p(u_1) \right)^2 u_{1,1} u_{2,3} \left( \frac{d^2}{du_1^2} p(u_1) \right)^2 \\
& + u_3 u_2 p(u_1)^4 \left( \frac{d^3}{du_1^3} p(u_1) \right)^2 u_{1,3} \left( \frac{d^2}{du_1^2} p(u_1) \right)^3 u_{1,1} \\
& - 4 p(u_1)^3 \left( \frac{d^2}{du_1^2} p(u_1) \right)^3 u_3 \left( \frac{d}{du_1} p(u_1) \right)^2 \left( \frac{d^3}{du_1^3} p(u_1) \right) u_{1,1} u_{2,3} \\
& - 32 \left( \frac{d}{du_1} p(u_1) \right)^7 u_2 u_{1,3} u_3 \left( \frac{d^3}{du_1^3} p(u_1) \right) u_{1,1} \left( \frac{d^2}{du_1^2} p(u_1) \right)
\end{aligned}$$



$$\begin{aligned}
& + 48 \left( \frac{d}{du_1} p(u_1) \right)^6 u_3 \left( \frac{d^3}{du_1^3} p(u_1) \right) u_{1,1} p(u_1) u_{2,3} \left( \frac{d^2}{du_1^2} p(u_1) \right) \\
& - u_2 p(u_1)^4 u_3 \left( \frac{d^4}{du_1^4} p(u_1) \right) u_{1,3} \left( \frac{d^2}{du_1^2} p(u_1) \right)^4 u_{1,1} \\
& - 2 \left( \frac{d}{du_1} p(u_1) \right) u_3 p(u_1)^4 \left( \frac{d^4}{du_1^4} p(u_1) \right) u_{1,1} \left( \frac{d^2}{du_1^2} p(u_1) \right)^3 u_{2,3} \\
& + 48 \left( \frac{d}{du_1} p(u_1) \right)^5 \left( \frac{d^3}{du_1^3} p(u_1) \right) u_{1,3} p(u_1)^2 u_{2,3} \left( \frac{d^2}{du_1^2} p(u_1) \right) \\
& + 18 p(u_1)^2 \left( \frac{d^2}{du_1^2} p(u_1) \right)^4 u_3 \left( \frac{d}{du_1} p(u_1) \right)^3 u_{1,1} u_{2,3} \\
& + 36 \left( \frac{d}{du_1} p(u_1) \right)^6 u_2 u_{1,3} \left( \frac{d^2}{du_1^2} p(u_1) \right)^3 u_3 u_{1,1} \\
& - 72 p(u_1) \left( \frac{d}{du_1} p(u_1) \right)^5 u_{2,3} u_3 \left( \frac{d^2}{du_1^2} p(u_1) \right)^3 u_{1,1} \\
& - 24 \left( \frac{d}{du_1} p(u_1) \right)^5 u_2 p(u_1)^2 \left( \frac{d^4}{du_1^4} p(u_1) \right) u_{1,3}^2 \left( \frac{d^2}{du_1^2} p(u_1) \right) \\
& + 12 \left( \frac{d}{du_1} p(u_1) \right)^3 u_2 p(u_1)^3 \left( \frac{d^4}{du_1^4} p(u_1) \right) u_{1,3}^2 \left( \frac{d^2}{du_1^2} p(u_1) \right)^2 \\
& + 48 \left( \frac{d}{du_1} p(u_1) \right)^6 u_2 \left( \frac{d^3}{du_1^3} p(u_1) \right) u_{1,3}^2 p(u_1) \left( \frac{d^2}{du_1^2} p(u_1) \right) \\
& + 16 \left( \frac{d}{du_1} p(u_1) \right)^7 u_3 p(u_1) \left( \frac{d^4}{du_1^4} p(u_1) \right) u_{1,1} u_{2,3} \\
& + 8 \left( \frac{d}{du_1} p(u_1) \right)^5 u_3 p(u_1)^2 \left( \frac{d^3}{du_1^3} p(u_1) \right)^2 u_{1,1} u_{2,3} \\
& - 8 \left( \frac{d}{du_1} p(u_1) \right)^3 u_2 p(u_1)^3 \left( \frac{d^3}{du_1^3} p(u_1) \right)^2 u_{1,3}^2 \left( \frac{d^2}{du_1^2} p(u_1) \right) \\
& + 2 \left( \frac{d}{du_1} p(u_1) \right) u_2 p(u_1)^4 \left( \frac{d^3}{du_1^3} p(u_1) \right)^2 u_{1,3}^2 \left( \frac{d^2}{du_1^2} p(u_1) \right)^2 \\
& - 4 u_2 p(u_1)^3 \left( \frac{d^3}{du_1^3} p(u_1) \right) \left( \frac{d^2}{du_1^2} p(u_1) \right)^3 \left( \frac{d}{du_1} p(u_1) \right)^2 u_{1,3}^2
\end{aligned}$$

$$\begin{aligned}
& -2 \left( \frac{d}{du_1} p(u_1) \right) u_2 p(u_1)^4 \left( \frac{d^4}{du_1^4} p(u_1) \right) u_{1,3}^2 \left( \frac{d^2}{du_1^2} p(u_1) \right)^3 \\
& -4 p(u_1)^4 \left( \frac{d^3}{du_1^3} p(u_1) \right) \left( \frac{d^2}{du_1^2} p(u_1) \right)^3 \left( \frac{d}{du_1} p(u_1) \right) u_{1,3} u_{2,3} \\
& -8 \left( \frac{d}{du_1} p(u_1) \right)^2 p(u_1)^4 \left( \frac{d^3}{du_1^3} p(u_1) \right)^2 u_{1,3} u_{2,3} \left( \frac{d^2}{du_1^2} p(u_1) \right) \\
& -24 \left( \frac{d}{du_1} p(u_1) \right)^4 p(u_1)^3 \left( \frac{d^4}{du_1^4} p(u_1) \right) u_{1,3} u_{2,3} \left( \frac{d^2}{du_1^2} p(u_1) \right) \\
& + 12 \left( \frac{d}{du_1} p(u_1) \right)^2 p(u_1)^4 \left( \frac{d^4}{du_1^4} p(u_1) \right) u_{1,3} u_{2,3} \left( \frac{d^2}{du_1^2} p(u_1) \right)^2, 0 \Big]
\end{aligned}$$

Now we don't get zero after substitution, so let us explore when this expression is zero depending on p(u<sub>1</sub>)

$$\begin{aligned}
\text{J2} > \text{tmp} := & \left( 4 \left( \frac{d}{du_1} p(u_1) \right)^4 u_2 u_3 p(u_1)^2 \left( \frac{d^3}{du_1^3} p(u_1) \right)^2 u_{1,1} u_{1,3} \left( \frac{d^2}{du_1^2} p(u_1) \right) \right. \\
& - 4 \left( \frac{d}{du_1} p(u_1) \right)^2 u_2 u_3 p(u_1)^3 \left( \frac{d^3}{du_1^3} p(u_1) \right)^2 u_{1,1} u_{1,3} \left( \frac{d^2}{du_1^2} p(u_1) \right)^2 \\
& - 2 p(u_1)^3 \left( \frac{d^2}{du_1^2} p(u_1) \right)^4 \left( \frac{d}{du_1} p(u_1) \right) u_{1,3} u_2 u_3 \left( \frac{d^3}{du_1^3} p(u_1) \right) u_{1,1} \\
& + 24 p(u_1) \left( \frac{d}{du_1} p(u_1) \right)^5 u_2 u_{1,3} u_3 \left( \frac{d^3}{du_1^3} p(u_1) \right) u_{1,1} \left( \frac{d^2}{du_1^2} p(u_1) \right)^2 \\
& - 12 \left( \frac{d}{du_1} p(u_1) \right)^4 u_2 p(u_1)^2 u_3 \left( \frac{d^4}{du_1^4} p(u_1) \right) u_{1,3} \left( \frac{d^2}{du_1^2} p(u_1) \right)^2 u_{1,1} \\
& + 6 \left( \frac{d}{du_1} p(u_1) \right)^2 u_2 p(u_1)^3 u_3 \left( \frac{d^4}{du_1^4} p(u_1) \right) u_{1,3} \left( \frac{d^2}{du_1^2} p(u_1) \right)^3 u_{1,1} \\
& + 8 \left( \frac{d}{du_1} p(u_1) \right)^6 u_2 p(u_1) u_3 \left( \frac{d^4}{du_1^4} p(u_1) \right) u_{1,3} \left( \frac{d^2}{du_1^2} p(u_1) \right) u_{1,1} \\
& + 18 p(u_1)^3 \left( \frac{d^2}{du_1^2} p(u_1) \right)^4 \left( \frac{d}{du_1} p(u_1) \right)^2 u_{1,3} u_{2,3} \\
& - 72 p(u_1)^2 \left( \frac{d^2}{du_1^2} p(u_1) \right)^3 \left( \frac{d}{du_1} p(u_1) \right)^4 u_{1,3} u_{2,3} \\
& \left. + 72 p(u_1) \left( \frac{d}{du_1} p(u_1) \right)^6 u_{1,3} u_{2,3} \left( \frac{d^2}{du_1^2} p(u_1) \right)^2 \right)
\end{aligned}$$

$$\begin{aligned}
& + 72 \left( \frac{d}{du_1} p(u_1) \right)^7 u_{2,3} u_3 \left( \frac{d^2}{du_1^2} p(u_1) \right)^2 u_{1,1} \\
& - 64 \left( \frac{d}{du_1} p(u_1) \right)^8 u_3 \left( \frac{d^3}{du_1^3} p(u_1) \right) u_{1,1} u_{2,3} \\
& + 16 \left( \frac{d}{du_1} p(u_1) \right)^6 p(u_1)^2 \left( \frac{d^4}{du_1^4} p(u_1) \right) u_{1,3} u_{2,3} \\
& - 64 \left( \frac{d}{du_1} p(u_1) \right)^7 \left( \frac{d^3}{du_1^3} p(u_1) \right) u_{1,3} p(u_1) u_{2,3} \\
& + 8 \left( \frac{d}{du_1} p(u_1) \right)^4 p(u_1)^3 \left( \frac{d^3}{du_1^3} p(u_1) \right)^2 u_{1,3} u_{2,3} \\
& + 16 \left( \frac{d}{du_1} p(u_1) \right)^7 u_2 p(u_1) \left( \frac{d^4}{du_1^4} p(u_1) \right) u_{1,3}^2 \\
& + 8 \left( \frac{d}{du_1} p(u_1) \right)^5 u_2 p(u_1)^2 \left( \frac{d^3}{du_1^3} p(u_1) \right)^2 u_{1,3}^2 \\
& - 72 p(u_1) \left( \frac{d^2}{du_1^2} p(u_1) \right)^3 \left( \frac{d}{du_1} p(u_1) \right)^5 u_{1,3}^2 u_2 \\
& + 18 p(u_1)^2 \left( \frac{d^2}{du_1^2} p(u_1) \right)^4 u_{1,3}^2 \left( \frac{d}{du_1} p(u_1) \right)^3 u_2 \\
& + 2 p(u_1)^5 \left( \frac{d^3}{du_1^3} p(u_1) \right)^2 u_{1,3} u_{2,3} \left( \frac{d^2}{du_1^2} p(u_1) \right)^2 \\
& - 2 p(u_1)^5 \left( \frac{d^4}{du_1^4} p(u_1) \right) u_{1,3} \left( \frac{d^2}{du_1^2} p(u_1) \right)^3 u_{2,3} \\
& - 64 \left( \frac{d}{du_1} p(u_1) \right)^8 u_2 \left( \frac{d^3}{du_1^3} p(u_1) \right) u_{1,3}^2 + 72 u_2 \left( \frac{d}{du_1} p(u_1) \right)^7 \\
& u_{1,3}^2 \left( \frac{d^2}{du_1^2} p(u_1) \right)^2 \\
& - 24 \left( \frac{d}{du_1} p(u_1) \right)^5 u_3 p(u_1)^2 \left( \frac{d^4}{du_1^4} p(u_1) \right) u_{1,1} u_{2,3} \left( \frac{d^2}{du_1^2} p(u_1) \right) \\
& + 12 \left( \frac{d}{du_1} p(u_1) \right)^3 u_3 p(u_1)^3 \left( \frac{d^4}{du_1^4} p(u_1) \right) u_{1,1} u_{2,3} \left( \frac{d^2}{du_1^2} p(u_1) \right)^2 \\
& + 9 p(u_1)^2 \left( \frac{d^2}{du_1^2} p(u_1) \right)^5 u_{1,1} u_2 \left( \frac{d}{du_1} p(u_1) \right)^2 u_{1,3} u_3
\end{aligned}$$

$$\begin{aligned}
& -36 p(u_1) \left( \frac{d^2}{du_1^2} p(u_1) \right)^4 \left( \frac{d}{du_1} p(u_1) \right)^4 u_{1,1} u_{2,3} u_3 \\
& -8 \left( \frac{d}{du_1} p(u_1) \right)^3 u_3 p(u_1)^3 \left( \frac{d^3}{du_1^3} p(u_1) \right)^2 u_{1,1} u_{2,3} \left( \frac{d^2}{du_1^2} p(u_1) \right) \\
& +2 \left( \frac{d}{du_1} p(u_1) \right) u_3 p(u_1)^4 \left( \frac{d^3}{du_1^3} p(u_1) \right)^2 u_{1,1} u_{2,3} \left( \frac{d^2}{du_1^2} p(u_1) \right)^2 \\
& +u_3 u_2 p(u_1)^4 \left( \frac{d^3}{du_1^3} p(u_1) \right)^2 u_{1,3} \left( \frac{d^2}{du_1^2} p(u_1) \right)^3 u_{1,1} \\
& -4 p(u_1)^3 \left( \frac{d^2}{du_1^2} p(u_1) \right)^3 u_3 \left( \frac{d}{du_1} p(u_1) \right)^2 \left( \frac{d^3}{du_1^3} p(u_1) \right) u_{1,1} u_{2,3} \\
& -32 \left( \frac{d}{du_1} p(u_1) \right)^7 u_{2,3} u_3 \left( \frac{d^3}{du_1^3} p(u_1) \right) u_{1,1} \left( \frac{d^2}{du_1^2} p(u_1) \right) \\
& +48 \left( \frac{d}{du_1} p(u_1) \right)^6 u_3 \left( \frac{d^3}{du_1^3} p(u_1) \right) u_{1,1} p(u_1) u_{2,3} \left( \frac{d^2}{du_1^2} p(u_1) \right) \\
& -u_2 p(u_1)^4 u_3 \left( \frac{d^4}{du_1^4} p(u_1) \right) u_{1,3} \left( \frac{d^2}{du_1^2} p(u_1) \right)^4 u_{1,1} \\
& -2 \left( \frac{d}{du_1} p(u_1) \right) u_3 p(u_1)^4 \left( \frac{d^4}{du_1^4} p(u_1) \right) u_{1,1} \left( \frac{d^2}{du_1^2} p(u_1) \right)^3 u_{2,3} \\
& +48 \left( \frac{d}{du_1} p(u_1) \right)^5 \left( \frac{d^3}{du_1^3} p(u_1) \right) u_{1,3} p(u_1)^2 u_{2,3} \left( \frac{d^2}{du_1^2} p(u_1) \right) \\
& +18 p(u_1)^2 \left( \frac{d^2}{du_1^2} p(u_1) \right)^4 u_3 \left( \frac{d}{du_1} p(u_1) \right)^3 u_{1,1} u_{2,3} \\
& +36 \left( \frac{d}{du_1} p(u_1) \right)^6 u_{2,3} u_3 \left( \frac{d^2}{du_1^2} p(u_1) \right)^3 u_{1,1} \\
& -72 p(u_1) \left( \frac{d}{du_1} p(u_1) \right)^5 u_{2,3} u_3 \left( \frac{d^2}{du_1^2} p(u_1) \right)^3 u_{1,1} \\
& -24 \left( \frac{d}{du_1} p(u_1) \right)^5 u_2 p(u_1)^2 \left( \frac{d^4}{du_1^4} p(u_1) \right) u_{1,3}^2 \left( \frac{d^2}{du_1^2} p(u_1) \right) \\
& +12 \left( \frac{d}{du_1} p(u_1) \right)^3 u_2 p(u_1)^3 \left( \frac{d^4}{du_1^4} p(u_1) \right) u_{1,3}^2 \left( \frac{d^2}{du_1^2} p(u_1) \right)^2 \\
& +48 \left( \frac{d}{du_1} p(u_1) \right)^6 u_2 \left( \frac{d^3}{du_1^3} p(u_1) \right) u_{1,3}^2 p(u_1) \left( \frac{d^2}{du_1^2} p(u_1) \right)
\end{aligned}$$

$$\begin{aligned}
& + 16 \left( \frac{d}{du_1} p(u_1) \right)^7 u_3 p(u_1) \left( \frac{d^4}{du_1^4} p(u_1) \right) u_{1,1} u_{2,3} \\
& + 8 \left( \frac{d}{du_1} p(u_1) \right)^5 u_3 p(u_1)^2 \left( \frac{d^3}{du_1^3} p(u_1) \right)^2 u_{1,1} u_{2,3} \\
& - 8 \left( \frac{d}{du_1} p(u_1) \right)^3 u_2 p(u_1)^3 \left( \frac{d^3}{du_1^3} p(u_1) \right)^2 u_{1,3}^2 \left( \frac{d^2}{du_1^2} p(u_1) \right) \\
& + 2 \left( \frac{d}{du_1} p(u_1) \right) u_2 p(u_1)^4 \left( \frac{d^3}{du_1^3} p(u_1) \right)^2 u_{1,3}^2 \left( \frac{d^2}{du_1^2} p(u_1) \right)^2 \\
& - 4 u_2 p(u_1)^3 \left( \frac{d^3}{du_1^3} p(u_1) \right) \left( \frac{d^2}{du_1^2} p(u_1) \right)^3 \left( \frac{d}{du_1} p(u_1) \right)^2 u_{1,3}^2 \\
& - 2 \left( \frac{d}{du_1} p(u_1) \right) u_2 p(u_1)^4 \left( \frac{d^4}{du_1^4} p(u_1) \right) u_{1,3}^2 \left( \frac{d^2}{du_1^2} p(u_1) \right)^3 \\
& - 4 p(u_1)^4 \left( \frac{d^3}{du_1^3} p(u_1) \right) \left( \frac{d^2}{du_1^2} p(u_1) \right)^3 \left( \frac{d}{du_1} p(u_1) \right) u_{1,3} u_{2,3} \\
& - 8 \left( \frac{d}{du_1} p(u_1) \right)^2 p(u_1)^4 \left( \frac{d^3}{du_1^3} p(u_1) \right)^2 u_{1,3} u_{2,3} \left( \frac{d^2}{du_1^2} p(u_1) \right) \\
& - 24 \left( \frac{d}{du_1} p(u_1) \right)^4 p(u_1)^3 \left( \frac{d^4}{du_1^4} p(u_1) \right) u_{1,3} u_{2,3} \left( \frac{d^2}{du_1^2} p(u_1) \right) \\
& + 12 \left( \frac{d}{du_1} p(u_1) \right)^2 p(u_1)^4 \left( \frac{d^4}{du_1^4} p(u_1) \right) u_{1,3} u_{2,3} \left( \frac{d^2}{du_1^2} p(u_1) \right)^2 \Bigg) :
\end{aligned}$$

**J2** > *simplify(diff(tmp, u<sub>1,3</sub>, u<sub>1,3</sub>, u<sub>2</sub>))*

$$\begin{aligned}
& -4 \left( \frac{d}{du_1} p(u_1) \right) \left( 12 \left( \frac{d}{du_1} p(u_1) \right)^4 p(u_1)^2 \left( \frac{d^4}{du_1^4} p(u_1) \right) \left( \frac{d^2}{du_1^2} p(u_1) \right) \right. \\
& \quad - 6 \left( \frac{d}{du_1} p(u_1) \right)^2 p(u_1)^3 \left( \frac{d^4}{du_1^4} p(u_1) \right) \left( \frac{d^2}{du_1^2} p(u_1) \right)^2 \\
& \quad - 24 \left( \frac{d}{du_1} p(u_1) \right)^5 \left( \frac{d^3}{du_1^3} p(u_1) \right) p(u_1) \left( \frac{d^2}{du_1^2} p(u_1) \right) \\
& \quad + 4 \left( \frac{d}{du_1} p(u_1) \right)^2 p(u_1)^3 \left( \frac{d^3}{du_1^3} p(u_1) \right)^2 \left( \frac{d^2}{du_1^2} p(u_1) \right) \\
& \quad \left. - p(u_1)^4 \left( \frac{d^3}{du_1^3} p(u_1) \right)^2 \left( \frac{d^2}{du_1^2} p(u_1) \right)^2 \right)
\end{aligned}$$

(37)

$$\begin{aligned}
& + 2 p(u_1)^3 \left( \frac{d^3}{du_1^3} p(u_1) \right) \left( \frac{d^2}{du_1^2} p(u_1) \right)^3 \left( \frac{d}{du_1} p(u_1) \right) \\
& + p(u_1)^4 \left( \frac{d^4}{du_1^4} p(u_1) \right) \left( \frac{d^2}{du_1^2} p(u_1) \right)^3 - 8 \left( \frac{d}{du_1} p(u_1) \right)^6 p(u_1) \left( \frac{d^4}{du_1^4} p(u_1) \right) \\
& - 4 \left( \frac{d}{du_1} p(u_1) \right)^4 p(u_1)^2 \left( \frac{d^3}{du_1^3} p(u_1) \right)^2 + 36 p(u_1) \left( \frac{d^2}{du_1^2} p(u_1) \right)^3 \left( \frac{d}{du_1} p(u_1) \right)^4 \\
& - 9 p(u_1)^2 \left( \frac{d^2}{du_1^2} p(u_1) \right)^4 \left( \frac{d}{du_1} p(u_1) \right)^2 + 32 \left( \frac{d}{du_1} p(u_1) \right)^7 \left( \frac{d^3}{du_1^3} p(u_1) \right) \\
& - 36 \left( \frac{d}{du_1} p(u_1) \right)^6 \left( \frac{d^2}{du_1^2} p(u_1) \right)^2
\end{aligned}$$

**J2** > subs( $\left[ \left[ \frac{d^4}{du_1^4} p(u_1) = p_4, \frac{d^3}{du_1^3} p(u_1) = p_3, \frac{d^2}{du_1^2} p(u_1) = p_2, \frac{d}{du_1} p(u_1) = p_1, p(u_1) = p \right], \% \right)$

$$\begin{aligned}
& -4 p_1 (12 p_1^4 p_2^2 p_4 p_2 - 6 p_1^2 p_3^2 p_4 p_2^2 - 24 p_1^5 p_3 p p_2 + 4 p_1^2 p_3^2 p_2^2 p_2 - p^4 p_3^2 p_2^2 + 2 p^3 p_3 p_2^3 p_1 \\
& + p^4 p_4 p_2^3 - 8 p_1^6 p p_4 - 4 p_1^4 p^2 p_3^2 + 36 p p_2^3 p_1^4 - 9 p^2 p_2^4 p_1^2 + 32 p_1^7 p_3 - 36 p_1^6 p_2^2)
\end{aligned} \tag{38}$$

**J2** > solve( $\% = 0, p_4$ )

$$\frac{p^2 p_3^2 - 2 p p_1 p_2 p_3 - 8 p_1^3 p_3 + 9 p_1^2 p_2^2}{(p p_2 - 2 p_1^2) p} \tag{39}$$

**J2** > simplify( $\left( \text{subs} \left( p_4 = \frac{p^2 \cdot p_3^2 - 2 p \cdot p_1 \cdot p_2 \cdot p_3 - 8 p_1^3 \cdot p_3 + 9 p_1^2 \cdot p_2^2}{p^2 \cdot p_2 - 2 p \cdot p_1^2}, \text{subs} \left( \left[ \frac{d^4}{du_1^4} p(u_1) = p_4, \frac{d^3}{du_1^3} p(u_1) = p_3, \frac{d^2}{du_1^2} p(u_1) = p_2, \frac{d}{du_1} p(u_1) = p_1, p(u_1) = p \right], tmp \right) \right) \right)$

$$0 \tag{40}$$

Thus we got a 4th order ODE governing EW property, and this is the same ODE that arises as the integrability condition!

**J2** > DGsetup([t, x, y], [u], J2, 4) :

**J2** > de := DifferentialEquationData([F], [u<sub>2,3</sub>])

$$\begin{aligned}
de := & \left[ \{u_{2,3}\}, \left[ 2 u_2 \left( \frac{d}{du_1} p(u_1) \right) u_{1,3} + 2 p(u_1) u_{2,3} + 2 u_3 \left( \frac{d}{du_1} p(u_1) \right) u_{1,2} \right. \right. \\
& \left. \left. + u_2 u_3 \left( \frac{d^2}{du_1^2} p(u_1) \right) u_{1,1} \right] \right]
\end{aligned} \tag{41}$$

**J2** > de2 := Prolong(de, 2) : deTRA := Transformation(de2) :

**J2** >

**J2** > simplify $\left( \text{subs}\left( \left[ \frac{d^4}{du_1^4} p(u_1) = p_4, \frac{d^3}{du_1^3} p(u_1) = p_3, \frac{d^2}{du_1^2} p(u_1) = p_2, \frac{d}{du_1} p(u_1) = p_1, p(u_1) = p \right], \text{Pullback}(\text{deTRA}, \text{subs}(\text{SLV}[1], \text{ToJet}([U1, U2, U3], \text{DepVars}, \text{notation} = \text{jetnumbers}))) \right) \right)$

$$\left[ -\frac{1}{(p p_2 - 2 p_1^2) u_2 u_3} \left( 2 (u_{1,1} u_2 u_3 p_3 p - 3 u_{1,1} u_2 u_3 p_1 p_2 + 2 u_3 u_{1,2} p p_2 - 4 u_3 u_{1,2} p_1^2 + 2 u_2 u_{1,3} p p_2 - 4 u_2 u_{1,3} p_1^2) \right), \right. \quad (42)$$

$$\frac{2 u_2 (-u_3 p_2^2 u_{1,1} p + u_{1,1} u_3 p p_3 p_1 - u_3 p_2 u_{1,1} p_1^2 + 2 p_1 u_{1,3} p p_2 - 4 p_1^3 u_{1,3})}{p (p p_2 - 2 p_1^2) u_3},$$

$$\left. \frac{2 u_3 (-u_2 p_2^2 u_{1,1} p + u_{1,1} u_2 p p_3 p_1 - u_2 p_2 u_{1,1} p_1^2 + 2 p_1 u_{1,2} p p_2 - 4 p_1^3 u_{1,2})}{u_2 p (p p_2 - 2 p_1^2)} \right]$$

**J2** > simplify $\left( \text{subs}\left( \left[ \frac{d^4}{du_1^4} p(u_1) = p_4, \frac{d^3}{du_1^3} p(u_1) = p_3, \frac{d^2}{du_1^2} p(u_1) = p_2, \frac{d}{du_1} p(u_1) = p_1, p(u_1) = p \right], \text{Pullback}(\text{deTRA}, \text{subs}(\text{SLV}[1], \text{ToJet}([-U1, -U2, -U3], \text{DepVars}, \text{notation} = \text{jetnumbers}))) \right) \right)$

$$\left[ \frac{1}{(p p_2 - 2 p_1^2) u_2 u_3} \left( 2 (u_{1,1} u_2 u_3 p_3 p - 3 u_{1,1} u_2 u_3 p_1 p_2 + 2 u_3 u_{1,2} p p_2 - 4 u_3 u_{1,2} p_1^2 + 2 u_2 u_{1,3} p p_2 - 4 u_2 u_{1,3} p_1^2) \right), \right. \quad (43)$$

$$\frac{2 u_2 (-u_3 p_2^2 u_{1,1} p + u_{1,1} u_3 p p_3 p_1 - u_3 p_2 u_{1,1} p_1^2 + 2 p_1 u_{1,3} p p_2 - 4 p_1^3 u_{1,3})}{p (p p_2 - 2 p_1^2) u_3},$$

$$\left. \frac{2 u_3 (-u_2 p_2^2 u_{1,1} p + u_{1,1} u_2 p p_3 p_1 - u_2 p_2 u_{1,1} p_1^2 + 2 p_1 u_{1,2} p p_2 - 4 p_1^3 u_{1,2})}{u_2 p (p p_2 - 2 p_1^2)} \right]$$

Here we expressed the 1-form omega (with coefficients U\_i; sorry in some files we get minus sign, meaning we write Weyl structure in the form Dg+omega\*g=0, not DG=omega\*g as in the paper) through the function p(u\_1). Done!

>  
>  
>

III. Finally we shall consider Example 3 of type 2 and check if the corresponding conformal metric is EW

> restart : with(DifferentialGeometry) : with(Tensor) : with(Tools) : with(JetCalculus) :  
with(LinearAlgebra) : with(PDEtools, D\_Dx, declare, ToJet, FromJet) :

> DGsetup([t, x, y], [u], J2) :

$$F := \alpha \cdot \frac{\text{diff}(p(u_2), u_2) - \text{diff}(p(u_3), u_3)}{p(u_2) \cdot p(u_3)} \cdot u_{2,3} + \beta \cdot \frac{\text{diff}(p(u_1), u_1) - \text{diff}(p(u_2), u_2)}{p(u_1) \cdot p(u_2)} \cdot u_{1,2} + \gamma \cdot \frac{\text{diff}(p(u_3), u_3) - \text{diff}(p(u_1), u_1)}{p(u_1) \cdot p(u_3)} \cdot u_{1,3}$$

$$F := \frac{\alpha \left( \frac{d}{du_2} p(u_2) - \left( \frac{d}{du_3} p(u_3) \right) \right) u_{2,3}}{p(u_2) p(u_3)} + \frac{\beta \left( \frac{d}{du_1} p(u_1) - \left( \frac{d}{du_2} p(u_2) \right) \right) u_{1,2}}{p(u_1) p(u_2)} + \frac{\gamma \left( \frac{d}{du_3} p(u_3) - \left( \frac{d}{du_1} p(u_1) \right) \right) u_{1,3}}{p(u_1) p(u_3)} \quad (44)$$

> A := Matrix( [[ [diff(F, u[1, 1]), 1/2 diff(F, u[1, 2]), 1/2 diff(F, u[1, 3])], [1/2 diff(F, u[1, 2]), diff(F, u[2, 2]), 1/2 diff(F, u[2, 3])], [1/2 diff(F, u[1, 3]), 1/2 diff(F, u[2, 3]), diff(F, u[3, 3])] ] ] ); AA := expand(MatrixInverse(A)) : AM := simplify(Determinant(A) \cdot AA) :

$$A := \begin{bmatrix} \left[ 0, \frac{1}{2} \frac{\beta \left( \frac{d}{du_1} p(u_1) - \left( \frac{d}{du_2} p(u_2) \right) \right)}{p(u_1) p(u_2)}, \frac{1}{2} \frac{\gamma \left( \frac{d}{du_3} p(u_3) - \left( \frac{d}{du_1} p(u_1) \right) \right)}{p(u_1) p(u_3)} \right], \\ \left[ \frac{1}{2} \frac{\beta \left( \frac{d}{du_1} p(u_1) - \left( \frac{d}{du_2} p(u_2) \right) \right)}{p(u_1) p(u_2)}, 0, \frac{1}{2} \frac{\alpha \left( \frac{d}{du_2} p(u_2) - \left( \frac{d}{du_3} p(u_3) \right) \right)}{p(u_2) p(u_3)} \right], \\ \left[ \frac{1}{2} \frac{\gamma \left( \frac{d}{du_3} p(u_3) - \left( \frac{d}{du_1} p(u_1) \right) \right)}{p(u_1) p(u_3)}, \frac{1}{2} \frac{\alpha \left( \frac{d}{du_2} p(u_2) - \left( \frac{d}{du_3} p(u_3) \right) \right)}{p(u_2) p(u_3)}, 0 \right] \end{bmatrix} \quad (45)$$

> simplify(AM); simplify(Determinant(A));



$$\begin{aligned}
& \left[ \left[ -\frac{1}{4} \frac{\alpha^2 \left( -\left( \frac{d}{du_2} p(u_2) \right) + \frac{d}{du_3} p(u_3) \right)^2}{p(u_3)^2 p(u_2)^2}, \right. \right. \\
& -\frac{1}{4} \frac{\gamma \left( \frac{d}{du_3} p(u_3) - \left( \frac{d}{du_1} p(u_1) \right) \right) \alpha \left( -\left( \frac{d}{du_2} p(u_2) \right) + \frac{d}{du_3} p(u_3) \right)}{p(u_1) p(u_3)^2 p(u_2)}, \\
& \left. -\frac{1}{4} \frac{\beta \left( \frac{d}{du_1} p(u_1) - \left( \frac{d}{du_2} p(u_2) \right) \right) \alpha \left( -\left( \frac{d}{du_2} p(u_2) \right) + \frac{d}{du_3} p(u_3) \right)}{p(u_1) p(u_3) p(u_2)^2} \right] \\
& \left[ -\frac{1}{4} \frac{\gamma \left( \frac{d}{du_3} p(u_3) - \left( \frac{d}{du_1} p(u_1) \right) \right) \alpha \left( -\left( \frac{d}{du_2} p(u_2) \right) + \frac{d}{du_3} p(u_3) \right)}{p(u_1) p(u_3)^2 p(u_2)}, \right. \\
& -\frac{1}{4} \frac{\gamma^2 \left( \frac{d}{du_3} p(u_3) - \left( \frac{d}{du_1} p(u_1) \right) \right)^2}{p(u_1)^2 p(u_3)^2}, \\
& \left. \frac{1}{4} \frac{\gamma \left( \frac{d}{du_3} p(u_3) - \left( \frac{d}{du_1} p(u_1) \right) \right) \beta \left( \frac{d}{du_1} p(u_1) - \left( \frac{d}{du_2} p(u_2) \right) \right)}{p(u_1)^2 p(u_3) p(u_2)} \right] \\
& \left[ -\frac{1}{4} \frac{\beta \left( \frac{d}{du_1} p(u_1) - \left( \frac{d}{du_2} p(u_2) \right) \right) \alpha \left( -\left( \frac{d}{du_2} p(u_2) \right) + \frac{d}{du_3} p(u_3) \right)}{p(u_1) p(u_3) p(u_2)^2}, \right. \\
& \frac{1}{4} \frac{\gamma \left( \frac{d}{du_3} p(u_3) - \left( \frac{d}{du_1} p(u_1) \right) \right) \beta \left( \frac{d}{du_1} p(u_1) - \left( \frac{d}{du_2} p(u_2) \right) \right)}{p(u_1)^2 p(u_3) p(u_2)}, \\
& \left. -\frac{1}{4} \frac{\beta^2 \left( \frac{d}{du_1} p(u_1) - \left( \frac{d}{du_2} p(u_2) \right) \right)^2}{p(u_1)^2 p(u_2)^2} \right] \\
& -\frac{1}{4} \frac{1}{p(u_1)^2 p(u_3)^2 p(u_2)^2} \left( \gamma \left( \frac{d}{du_3} p(u_3) - \left( \frac{d}{du_1} p(u_1) \right) \right) \beta \left( \frac{d}{du_1} p(u_1) \right. \right. \\
& \left. \left. - \left( \frac{d}{du_2} p(u_2) \right) \right) \alpha \left( -\left( \frac{d}{du_2} p(u_2) \right) + \frac{d}{du_3} p(u_3) \right) \right)
\end{aligned} \tag{46}$$


---

$\triangleright Qa := [TotalDiff(A[1, 1], 1) + TotalDiff(A[1, 2], 2) + TotalDiff(A[1, 3], 3),$   
 $TotalDiff(A[2, 1], 1) + TotalDiff(A[2, 2], 2) + TotalDiff(A[2, 3], 3),$   
 $TotalDiff(A[3, 1], 1) + TotalDiff(A[3, 2], 2) + TotalDiff(A[3, 3], 3)] :$

---

$\triangleright \Omega := simplify([2 (AA[1, 1] \cdot Qa[1] + AA[1, 2] \cdot Qa[2] + AA[1, 3] \cdot Qa[3]),$   
 $2 (AA[2, 1] \cdot Qa[1] + AA[2, 2] \cdot Qa[2] + AA[2, 3] \cdot Qa[3]),$

2 (AA[3, 1]·Qa[1] + AA[3, 2]·Qa[2] + AA[3, 3]·Qa[3]))):

DepVars := [u(t, x, y)]: AJ := FromJet(AM, DepVars):

DGsetup([t, x, y], M):

g := evalDG(AJ[1, 1]·dt &t dt + AJ[1, 2]·dt &t dx + AJ[1, 3]·dt &t dy + AJ[2, 1]·dx &t dt  
+ AJ[2, 2]·dx &t dx + AJ[2, 3]·dx &t dy + AJ[3, 1]·dy &t dt + AJ[3, 2]·dy &t dx  
+ AJ[3, 3]·dy &t dy):

C := Connection(a000\*dt &t D\_t &t dt + a111\*dx &t D\_x &t dx + a222\*dy &t D\_y &t dy  
+ a001\*(dt &t D\_t &t dx + dx &t D\_t &t dt) + a002\*(dt &t D\_t &t dy + dy &t D\_t  
&t dt) + a102\*(dx &t D\_t &t dy + dy &t D\_t &t dx) + a011\*(dt &t D\_x &t dx + dx  
&t D\_x &t dt) + a012\*(dt &t D\_x &t dy + dy &t D\_x &t dt) + a112\*(dx &t D\_x &t dy  
+ dy &t D\_x &t dx) + a021\*(dt &t D\_y &t dx + dx &t D\_y &t dt) + a022\*(dt &t D\_y  
&t dy + dy &t D\_y &t dt) + a122\*(dx &t D\_y &t dy + dy &t D\_y &t dx) + a010\*dt  
&t D\_x &t dt + a121\*dx &t D\_y &t dx + a202\*dy &t D\_t &t dy + a020\*dt &t D\_y &t dt  
+ a101\*dx &t D\_t &t dx + a212\*dy &t D\_x &t dy):

TorsionTensor(C);

0 dt D\_t dt

(47)

U1 := FromJet(Ω[1], DepVars):

U2 := FromJet(Ω[2], DepVars):

U3 := FromJet(Ω[3], DepVars):

Et := evalDG(DirectionalCovariantDerivative(D\_t, g, C) - U1·g):

Ex := evalDG(DirectionalCovariantDerivative(D\_x, g, C) - U2·g):

Ey := evalDG(DirectionalCovariantDerivative(D\_y, g, C) - U3·g):

Eq000 := TensorInnerProduct(g, Et, dt &t dt):

Eq001 := TensorInnerProduct(g, Et, dt &t dx):

Eq002 := TensorInnerProduct(g, Et, dt &t dy):

Eq011 := TensorInnerProduct(g, Et, dx &t dx):

Eq012 := TensorInnerProduct(g, Et, dx &t dy):

Eq022 := TensorInnerProduct(g, Et, dy &t dy):

Eq100 := TensorInnerProduct(g, Ex, dt &t dt):

Eq101 := TensorInnerProduct(g, Ex, dt &t dx):

Eq102 := TensorInnerProduct(g, Ex, dt &t dy):

Eq111 := TensorInnerProduct(g, Ex, dx &t dx):

Eq112 := TensorInnerProduct(g, Ex, dx &t dy):

Eq122 := TensorInnerProduct(g, Ex, dy &t dy):

Eq200 := TensorInnerProduct(g, Ey, dt &t dt):

Eq201 := TensorInnerProduct(g, Ey, dt &t dx):

Eq202 := TensorInnerProduct(g, Ey, dt &t dy):

Eq211 := TensorInnerProduct(g, Ey, dx &t dx):

Eq212 := TensorInnerProduct(g, Ey, dx &t dy):

Eq222 := TensorInnerProduct(g, Ey, dy &t dy):

sA := solve({Eq000=0, Eq001=0, Eq002=0, Eq011=0, Eq012=0, Eq022=0, Eq100=0,  
Eq101=0, Eq102=0, Eq111=0, Eq112=0, Eq122=0, Eq200=0, Eq201=0, Eq202=0,  
Eq211=0, Eq212=0, Eq222=0}, [a000, a001, a002, a010, a011, a012, a020, a021, a022,  
a101, a102, a111, a112, a121, a122, a202, a212, a222]):

C1 := evalDG(subs({op(op(sA))}, C)):

evalDG(CovariantDerivative(g, C1) - g &t (U1·dt + U2·dx + U3·dy));

(48)

```

> R1 := CurvatureTensor(C1) : Ric1 := RicciTensor(R1) : T1 := SymmetrizeIndices(Ric1, [1, 2],
  "Symmetric") : Res := evalDG(T1 - V.g) :
> NEQtt := ContractIndices(Res, D_t &t D_t, [[1, 1], [2, 2]]) : NEQtx := ContractIndices(Res,
  D_t &t D_x, [[1, 1], [2, 2]]) :
NEQty := ContractIndices(Res, D_t &t D_y, [[1, 1], [2, 2]]) : NEQxx := ContractIndices(Res,
  D_x &t D_x, [[1, 1], [2, 2]]) :
NEQxy := ContractIndices(Res, D_x &t D_y, [[1, 1], [2, 2]]) : NEQyy := ContractIndices(Res,
  D_y &t D_y, [[1, 1], [2, 2]]) :

```

```

> DGsetup([t, x, y], [u], J2, 4) :

```

```

> de := DifferentialEquationData([F], [u1, 2])

```

$$de := \left[ \{u_{1,2}\}, \left[ \frac{\alpha \left( \frac{d}{du_2} p(u_2) - \left( \frac{d}{du_3} p(u_3) \right) \right) u_{2,3}}{p(u_2) p(u_3)} + \frac{\beta \left( \frac{d}{du_1} p(u_1) - \left( \frac{d}{du_2} p(u_2) \right) \right) u_{1,2}}{p(u_1) p(u_2)} + \frac{\gamma \left( \frac{d}{du_3} p(u_3) - \left( \frac{d}{du_1} p(u_1) \right) \right) u_{1,3}}{p(u_1) p(u_3)} \right] \right] \quad (49)$$

```

> de2 := Prolong(de, 2) : deTRA := Transformation(de2) :

```

```

> Eq0 := Pullback(deTRA, ToJet(NEQtt, DepVars, notation = jetnumbers)) :

```

```

> VS := solve(Eq0, V) :

```

```

> Eq1 := numer(subs(V = VS, Pullback(deTRA, ToJet(NEQtx, DepVars, notation
  = jetnumbers)))) :

```

```

Eq2 := numer(subs(V = VS, Pullback(deTRA, ToJet(NEQty, DepVars, notation
  = jetnumbers)))) :

```

```

Eq3 := numer(subs(V = VS, Pullback(deTRA, ToJet(NEQxx, DepVars, notation
  = jetnumbers)))) :

```

```

Eq4 := numer(subs(V = VS, Pullback(deTRA, ToJet(NEQxy, DepVars, notation
  = jetnumbers)))) :

```

```

Eq5 := numer(subs(V = VS, Pullback(deTRA, ToJet(NEQyy, DepVars, notation
  = jetnumbers)))) :

```

```

J2 >

```

```

J2 > factor(simplify(diff(Eq5, u1, 3, u3, 3)))

```

$$-\alpha \gamma^2 p(u_2)^2 p(u_1) p(u_3) \left( \frac{d}{du_1} p(u_1) - \left( \frac{d}{du_2} p(u_2) \right) \right)^9 \left( - \left( \frac{d}{du_2} p(u_2) \right) + \frac{d}{du_3} p(u_3) \right)^2 \left( \frac{d}{du_3} p(u_3) - \left( \frac{d}{du_1} p(u_1) \right) \right)^3 \left( - \left( \frac{d}{du_3} p(u_3) \right)^2 \left( \frac{d^2}{du_3^2} p(u_3) \right) \left( \frac{d}{du_2} p(u_2) \right)^2 \beta + \left( \frac{d}{du_1} p(u_1) \right)^2 \left( \frac{d^2}{du_3^2} p(u_3) \right) \left( \frac{d}{du_2} p(u_2) \right)^2 \alpha \right) \quad (50)$$

$$\begin{aligned}
& - \left( \frac{d}{du_1} p(u_1) \right)^2 \left( \frac{d^2}{du_3^2} p(u_3) \right) \left( \frac{d}{du_2} p(u_2) \right)^2 \beta \\
& - \left( \frac{d}{du_1} p(u_1) \right) \left( \frac{d^2}{du_3^2} p(u_3) \right) \left( \frac{d}{du_2} p(u_2) \right)^3 \alpha \\
& + \left( \frac{d}{du_1} p(u_1) \right) \left( \frac{d^2}{du_3^2} p(u_3) \right) \left( \frac{d}{du_2} p(u_2) \right)^3 \beta \\
& - p(u_3) \left( \frac{d}{du_1} p(u_1) \right)^2 \left( \frac{d^2}{du_3^2} p(u_3) \right)^2 \beta + p(u_3) \left( \frac{d^2}{du_3^2} p(u_3) \right)^2 \left( \frac{d}{du_2} p(u_2) \right)^2 \beta \\
& - \left( \frac{d}{du_3} p(u_3) \right)^3 \left( \frac{d}{du_1} p(u_1) \right) \left( \frac{d^2}{du_3^2} p(u_3) \right) \beta \\
& + \left( \frac{d}{du_3} p(u_3) \right)^3 \left( \frac{d^2}{du_3^2} p(u_3) \right) \left( \frac{d}{du_2} p(u_2) \right) \beta \\
& + \left( \frac{d}{du_3} p(u_3) \right)^2 \left( \frac{d}{du_1} p(u_1) \right)^2 \left( \frac{d^2}{du_3^2} p(u_3) \right) \alpha \\
& - p(u_1) \left( \frac{d}{du_3} p(u_3) \right)^2 \left( \frac{d^2}{du_3^2} p(u_3) \right) \left( \frac{d^2}{du_1^2} p(u_1) \right) \alpha \\
& - p(u_1) \left( \frac{d^2}{du_3^2} p(u_3) \right) \left( \frac{d}{du_2} p(u_2) \right)^2 \left( \frac{d^2}{du_1^2} p(u_1) \right) \alpha \\
& - p(u_3) \left( \frac{d}{du_3} p(u_3) \right)^2 \left( \frac{d}{du_1} p(u_1) \right) \left( \frac{d^3}{du_3^3} p(u_3) \right) \beta \\
& + p(u_3) \left( \frac{d}{du_3} p(u_3) \right)^2 \left( \frac{d}{du_2} p(u_2) \right) \left( \frac{d^3}{du_3^3} p(u_3) \right) \beta \\
& + p(u_3) \left( \frac{d}{du_3} p(u_3) \right) \left( \frac{d}{du_1} p(u_1) \right)^2 \left( \frac{d^3}{du_3^3} p(u_3) \right) \beta \\
& + 2 p(u_3) \left( \frac{d}{du_3} p(u_3) \right) \left( \frac{d}{du_1} p(u_1) \right) \left( \frac{d^2}{du_3^2} p(u_3) \right)^2 \beta \\
& - 2 p(u_3) \left( \frac{d}{du_3} p(u_3) \right) \left( \frac{d^2}{du_3^2} p(u_3) \right)^2 \left( \frac{d}{du_2} p(u_2) \right) \beta \\
& - p(u_3) \left( \frac{d}{du_3} p(u_3) \right) \left( \frac{d}{du_2} p(u_2) \right)^2 \left( \frac{d^3}{du_3^3} p(u_3) \right) \beta
\end{aligned}$$

$$\begin{aligned}
& -p(u_3) \left( \frac{d}{du_1} p(u_1) \right)^2 \left( \frac{d}{du_2} p(u_2) \right) \left( \frac{d^3}{du_3^3} p(u_3) \right) \beta \\
& + p(u_3) \left( \frac{d}{du_1} p(u_1) \right) \left( \frac{d}{du_2} p(u_2) \right)^2 \left( \frac{d^3}{du_3^3} p(u_3) \right) \beta \\
& - \left( \frac{d}{du_3} p(u_3) \right)^2 \left( \frac{d}{du_1} p(u_1) \right) \left( \frac{d^2}{du_3^2} p(u_3) \right) \left( \frac{d}{du_2} p(u_2) \right) \alpha \\
& + \left( \frac{d}{du_3} p(u_3) \right)^2 \left( \frac{d}{du_1} p(u_1) \right) \left( \frac{d^2}{du_3^2} p(u_3) \right) \left( \frac{d}{du_2} p(u_2) \right) \beta \\
& - 2 \left( \frac{d}{du_3} p(u_3) \right) \left( \frac{d}{du_1} p(u_1) \right)^2 \left( \frac{d^2}{du_3^2} p(u_3) \right) \left( \frac{d}{du_2} p(u_2) \right) \alpha \\
& + \left( \frac{d}{du_3} p(u_3) \right) \left( \frac{d}{du_1} p(u_1) \right)^2 \left( \frac{d^2}{du_3^2} p(u_3) \right) \left( \frac{d}{du_2} p(u_2) \right) \beta \\
& + 2 \left( \frac{d}{du_3} p(u_3) \right) \left( \frac{d}{du_1} p(u_1) \right) \left( \frac{d^2}{du_3^2} p(u_3) \right) \left( \frac{d}{du_2} p(u_2) \right)^2 \alpha \\
& - \left( \frac{d}{du_3} p(u_3) \right) \left( \frac{d}{du_1} p(u_1) \right) \left( \frac{d^2}{du_3^2} p(u_3) \right) \left( \frac{d}{du_2} p(u_2) \right)^2 \beta \\
& + \gamma \left( \frac{d}{du_3} p(u_3) \right)^2 \left( \frac{d^2}{du_2^2} p(u_2) \right) \left( \frac{d^2}{du_3^2} p(u_3) \right) p(u_2) \\
& + \gamma \left( \frac{d}{du_1} p(u_1) \right)^2 \left( \frac{d^2}{du_2^2} p(u_2) \right) \left( \frac{d^2}{du_3^2} p(u_3) \right) p(u_2) \\
& - 2 \gamma \left( \frac{d}{du_3} p(u_3) \right) \left( \frac{d}{du_1} p(u_1) \right) \left( \frac{d^2}{du_2^2} p(u_2) \right) \left( \frac{d^2}{du_3^2} p(u_3) \right) p(u_2) \\
& + 2 p(u_1) \left( \frac{d}{du_3} p(u_3) \right) \left( \frac{d^2}{du_3^2} p(u_3) \right) \left( \frac{d}{du_2} p(u_2) \right) \left( \frac{d^2}{du_1^2} p(u_1) \right) \alpha
\end{aligned}$$

> simplify  $\left( \text{subs} \left( \left[ \frac{d}{du_1} p(u_1) = \sqrt{4 \cdot p(u_1)^3 - \rho}, \frac{d}{du_2} p(u_2) = \sqrt{4 \cdot p(u_2)^3 - \rho}, \frac{d}{du_3} p(u_3) = \sqrt{4 \cdot p(u_3)^3 - \rho} \right], \text{subs} \left( \left[ \frac{d^2}{du_1^2} p(u_1) = 6 \cdot p(u_1)^2, \frac{d^2}{du_2^2} p(u_2) = 6 \cdot p(u_2)^2, \frac{d^2}{du_3^2} p(u_3) = 6 \cdot p(u_3)^2 \right], \text{subs} \left( \left[ \frac{d^3}{du_1^3} p(u_1) = 12 p(u_1) \sqrt{4 \cdot p(u_1)^3 - \rho}, \frac{d^3}{du_2^3} p(u_2) = 12 p(u_2) \sqrt{4 \cdot p(u_2)^3 - \rho}, \frac{d^3}{du_3^3} p(u_3) = 12 p(u_3) \sqrt{4 \cdot p(u_3)^3 - \rho} \right], \text{diff} (Eq5, u_1, 3), \right. \right. \right.$

$$u_{3,3}) \Big) \Big) \Big) \Big)$$

output is visible, but too large and so is removed

>  $\Omega[1]$

$$\begin{aligned}
& - \left( \beta \alpha u_{2,3} p(u_1)^2 \left( \frac{d}{du_2} p(u_2) \right) \left( \frac{d}{du_3} p(u_3) \right) \left( \frac{d}{du_1} p(u_1) \right) \right. \\
& \quad + \gamma \alpha u_{2,3} p(u_1)^2 \left( \frac{d}{du_2} p(u_2) \right) \left( \frac{d}{du_3} p(u_3) \right) \left( \frac{d}{du_1} p(u_1) \right) \\
& \quad + 2 p(u_2) \gamma \beta u_{1,1} p(u_3) \left( \frac{d}{du_1} p(u_1) \right)^2 \left( \frac{d}{du_3} p(u_3) \right) \\
& \quad + 2 p(u_2) \gamma \beta u_{1,1} p(u_3) \left( \frac{d}{du_1} p(u_1) \right)^2 \left( \frac{d}{du_2} p(u_2) \right) \\
& \quad + p(u_1) \alpha \beta u_{1,2} p(u_3) \left( \frac{d}{du_1} p(u_1) \right) \left( \frac{d}{du_2} p(u_2) \right)^2 \\
& \quad + p(u_1) \alpha \left( \frac{d}{du_2} p(u_2) \right) \gamma u_{1,3} p(u_2) \left( \frac{d}{du_1} p(u_1) \right)^2 \\
& \quad + p(u_1) \alpha \left( \frac{d}{du_3} p(u_3) \right) \beta u_{1,2} p(u_3) \left( \frac{d}{du_1} p(u_1) \right)^2 \\
& \quad + p(u_1) \alpha \gamma u_{1,3} p(u_2) \left( \frac{d}{du_1} p(u_1) \right) \left( \frac{d}{du_3} p(u_3) \right)^2 \\
& \quad - p(u_1) \alpha \left( \frac{d}{du_3} p(u_3) \right) \gamma u_{1,3} p(u_2) \left( \frac{d}{du_1} p(u_1) \right)^2 \\
& \quad - \gamma \beta u_{1,2} p(u_1) p(u_3) \left( \frac{d}{du_1} p(u_1) \right)^2 \left( \frac{d}{du_2} p(u_2) \right) \\
& \quad - \gamma \beta u_{1,2} p(u_1) p(u_3) \left( \frac{d}{du_2} p(u_2) \right)^2 \left( \frac{d}{du_3} p(u_3) \right) \\
& \quad + \gamma \beta u_{1,2} p(u_1) p(u_3) \left( \frac{d}{du_2} p(u_2) \right)^2 \left( \frac{d}{du_1} p(u_1) \right) \\
& \quad - p(u_1) \alpha \left( \frac{d}{du_2} p(u_2) \right) \beta u_{1,2} p(u_3) \left( \frac{d}{du_1} p(u_1) \right)^2 \\
& \quad + \beta \gamma u_{1,3} p(u_1) p(u_2) \left( \frac{d}{du_3} p(u_3) \right)^2 \left( \frac{d}{du_1} p(u_1) \right) \\
& \quad \left. - \beta \gamma u_{1,3} p(u_1) p(u_2) \left( \frac{d}{du_3} p(u_3) \right)^2 \left( \frac{d}{du_2} p(u_2) \right) \right)
\end{aligned} \tag{51}$$

$$\begin{aligned}
& -\beta \gamma u_{1,3} p(u_1) p(u_2) \left( \frac{d}{du_1} p(u_1) \right)^2 \left( \frac{d}{du_3} p(u_3) \right) \\
& -2 p(u_2) \gamma \beta u_{1,1} p(u_3) \left( \frac{d}{du_1} p(u_1) \right)^3 \\
& + \gamma \alpha u_{2,3} p(u_1)^2 \left( \frac{d}{du_2} p(u_2) \right)^2 \left( \frac{d}{du_3} p(u_3) \right) \\
& - \gamma \alpha u_{2,3} p(u_1)^2 \left( \frac{d}{du_2} p(u_2) \right)^2 \left( \frac{d}{du_1} p(u_1) \right) \\
& - \gamma \alpha u_{2,3} p(u_1)^2 \left( \frac{d}{du_2} p(u_2) \right) \left( \frac{d}{du_3} p(u_3) \right)^2 \\
& - \beta \alpha u_{2,3} p(u_1)^2 \left( \frac{d}{du_2} p(u_2) \right)^2 \left( \frac{d}{du_3} p(u_3) \right) \\
& - \beta \alpha u_{2,3} p(u_1)^2 \left( \frac{d}{du_3} p(u_3) \right)^2 \left( \frac{d}{du_1} p(u_1) \right) \\
& + \beta \alpha u_{2,3} p(u_1)^2 \left( \frac{d}{du_3} p(u_3) \right)^2 \left( \frac{d}{du_2} p(u_2) \right) \\
& -2 p(u_2) \gamma \beta u_{1,1} p(u_3) \left( \frac{d}{du_1} p(u_1) \right) \left( \frac{d}{du_2} p(u_2) \right) \left( \frac{d}{du_3} p(u_3) \right) \\
& + \beta \gamma u_{1,3} p(u_1) p(u_2) \left( \frac{d}{du_1} p(u_1) \right) \left( \frac{d}{du_3} p(u_3) \right) \left( \frac{d}{du_2} p(u_2) \right) \\
& - p(u_1) \alpha \left( \frac{d}{du_2} p(u_2) \right) \gamma u_{1,3} p(u_2) \left( \frac{d}{du_1} p(u_1) \right) \left( \frac{d}{du_3} p(u_3) \right) \\
& - p(u_1) \alpha \left( \frac{d}{du_3} p(u_3) \right) \beta u_{1,2} p(u_3) \left( \frac{d}{du_1} p(u_1) \right) \left( \frac{d}{du_2} p(u_2) \right) \\
& + \gamma \beta u_{1,2} p(u_1) p(u_3) \left( \frac{d}{du_1} p(u_1) \right) \left( \frac{d}{du_2} p(u_2) \right) \left( \frac{d}{du_3} p(u_3) \right) \\
& + 2 p(u_2) \gamma \beta u_{1,1} p(u_3) \left( \frac{d^2}{du_1^2} p(u_1) \right) p(u_1) \left( \frac{d}{du_1} p(u_1) \right) \\
& + p(u_2) \gamma \beta u_{1,2} p(u_1) p(u_3) \left( \frac{d^2}{du_2^2} p(u_2) \right) \left( \frac{d}{du_3} p(u_3) \right) \\
& + p(u_3) \beta \gamma u_{1,3} p(u_1) p(u_2) \left( \frac{d^2}{du_3^2} p(u_3) \right) \left( \frac{d}{du_2} p(u_2) \right)
\end{aligned}$$

$$\begin{aligned}
& -p(u_2) \gamma \beta u_{1,1} p(u_3) \left( \frac{d^2}{du_1^2} p(u_1) \right) p(u_1) \left( \frac{d}{du_3} p(u_3) \right) \\
& -p(u_3) \beta \alpha u_{2,3} p(u_1)^2 \left( \frac{d^2}{du_3^2} p(u_3) \right) \left( \frac{d}{du_2} p(u_2) \right) \\
& -p(u_1)^2 \alpha \left( \frac{d}{du_2} p(u_2) \right) \gamma u_{1,3} p(u_2) \left( \frac{d^2}{du_1^2} p(u_1) \right) \\
& +p(u_1)^2 \alpha \left( \frac{d}{du_2} p(u_2) \right) \gamma u_{3,3} p(u_2) \left( \frac{d^2}{du_3^2} p(u_3) \right) \\
& -p(u_1)^2 \alpha \left( \frac{d}{du_3} p(u_3) \right) \beta u_{1,2} p(u_3) \left( \frac{d^2}{du_1^2} p(u_1) \right) \\
& +p(u_1)^2 \alpha \left( \frac{d}{du_3} p(u_3) \right) \beta u_{2,2} p(u_3) \left( \frac{d^2}{du_2^2} p(u_2) \right) \\
& +p(u_1)^2 \alpha \left( \frac{d}{du_3} p(u_3) \right) \gamma u_{1,3} p(u_2) \left( \frac{d^2}{du_1^2} p(u_1) \right) \\
& -p(u_2) \gamma \alpha u_{2,3} p(u_1)^2 \left( \frac{d^2}{du_2^2} p(u_2) \right) \left( \frac{d}{du_3} p(u_3) \right) \\
& +p(u_2) \gamma \alpha u_{2,3} p(u_1)^2 \left( \frac{d^2}{du_2^2} p(u_2) \right) \left( \frac{d}{du_1} p(u_1) \right) \\
& -p(u_2) \gamma \alpha u_{3,3} p(u_1)^2 \left( \frac{d^2}{du_3^2} p(u_3) \right) \left( \frac{d}{du_1} p(u_1) \right) \\
& +p(u_1)^2 \alpha \left( \frac{d}{du_2} p(u_2) \right) \beta u_{1,2} p(u_3) \left( \frac{d^2}{du_1^2} p(u_1) \right) \\
& -p(u_3) \beta \alpha u_{2,2} p(u_1)^2 \left( \frac{d^2}{du_2^2} p(u_2) \right) \left( \frac{d}{du_1} p(u_1) \right) \\
& +p(u_3) \beta \alpha u_{2,3} p(u_1)^2 \left( \frac{d^2}{du_3^2} p(u_3) \right) \left( \frac{d}{du_1} p(u_1) \right) \\
& -p(u_2) \gamma \beta u_{1,2} p(u_1) p(u_3) \left( \frac{d^2}{du_2^2} p(u_2) \right) \left( \frac{d}{du_1} p(u_1) \right) \\
& -p(u_3) \beta \gamma u_{1,3} p(u_1) p(u_2) \left( \frac{d^2}{du_3^2} p(u_3) \right) \left( \frac{d}{du_1} p(u_1) \right) \\
& -p(u_3) \beta \gamma u_{1,1} p(u_2) \left( \frac{d^2}{du_1^2} p(u_1) \right) p(u_1) \left( \frac{d}{du_2} p(u_2) \right) \Big) /
\end{aligned}$$



$$\left( p(u_1) p(u_3) p(u_2) \left( \frac{d}{du_1} p(u_1) - \left( \frac{d}{du_2} p(u_2) \right) \right) \beta \left( \frac{d}{du_3} p(u_3) - \left( \frac{d}{du_1} p(u_1) \right) \right) \gamma \right)$$

$$\begin{aligned} & \text{> simplify} \left( \text{subs} \left( \left[ \frac{d}{du_1} p(u_1) = \sqrt{4 \cdot p(u_1)^3 - \rho}, \frac{d}{du_2} p(u_2) = \sqrt{4 \cdot p(u_2)^3 - \rho}, \frac{d}{du_3} p(u_3) \right. \right. \right. \\ & \quad \left. \left. \left. = \sqrt{4 \cdot p(u_3)^3 - \rho} \right], \text{subs} \left( \left[ \frac{d^2}{du_1^2} p(u_1) = 6 \cdot p(u_1)^2, \frac{d^2}{du_2^2} p(u_2) = 6 \cdot p(u_2)^2, \frac{d^2}{du_3^2} p(u_3) \right. \right. \right. \right. \\ & \quad \left. \left. \left. = 6 \cdot p(u_3)^2 \right], \Omega[1] \right) \right) \right) \\ & \left( 6 p(u_1)^2 \alpha \sqrt{4 p(u_2)^3 - \rho} \gamma u_{3,3} p(u_2) p(u_3)^2 \right. \\ & \quad + 6 p(u_1)^2 \alpha \sqrt{4 p(u_3)^3 - \rho} \beta u_{2,2} p(u_3) p(u_2)^2 \\ & \quad - 6 p(u_2) \gamma \alpha u_{3,3} p(u_1)^2 p(u_3)^2 \sqrt{4 p(u_1)^3 - \rho} \\ & \quad - 6 p(u_3) \beta \alpha u_{2,2} p(u_1)^2 p(u_2)^2 \sqrt{4 p(u_1)^3 - \rho} \\ & \quad - 2 \gamma \beta u_{1,2} p(u_1) p(u_3) \sqrt{4 p(u_1)^3 - \rho} p(u_2)^3 \\ & \quad - \gamma \beta u_{1,2} p(u_1) p(u_3) \sqrt{4 p(u_1)^3 - \rho} \rho \\ & \quad + 2 \beta \gamma u_{1,3} p(u_1) p(u_2) \sqrt{4 p(u_2)^3 - \rho} p(u_3)^3 \\ & \quad + \beta \gamma u_{1,3} p(u_1) p(u_2) \sqrt{4 p(u_2)^3 - \rho} \rho + \beta \gamma u_{1,3} p(u_1) p(u_2) \sqrt{4 p(u_3)^3 - \rho} \rho \\ & \quad + p(u_1) \alpha \sqrt{4 p(u_3)^3 - \rho} \gamma u_{1,3} p(u_2) \rho + \gamma \beta u_{1,2} p(u_1) p(u_3) \sqrt{4 p(u_2)^3 - \rho} \rho \\ & \quad + 2 \gamma \beta u_{1,2} p(u_1) p(u_3) \sqrt{4 p(u_3)^3 - \rho} p(u_2)^3 \\ & \quad + \gamma \beta u_{1,2} p(u_1) p(u_3) \sqrt{4 p(u_3)^3 - \rho} \rho + p(u_1) \alpha \sqrt{4 p(u_2)^3 - \rho} \beta u_{1,2} p(u_3) \rho \\ & \quad - 2 \beta \gamma u_{1,3} p(u_1) p(u_2) \sqrt{4 p(u_1)^3 - \rho} p(u_3)^3 \\ & \quad - \beta \gamma u_{1,3} p(u_1) p(u_2) \sqrt{4 p(u_1)^3 - \rho} \rho \\ & \quad + 2 p(u_2) \gamma \beta u_{1,1} p(u_3) \sqrt{4 p(u_3)^3 - \rho} p(u_1)^3 \\ & \quad - 2 p(u_2) \gamma \beta u_{1,1} p(u_3) \sqrt{4 p(u_3)^3 - \rho} \rho \\ & \quad + 2 p(u_2) \gamma \beta u_{1,1} p(u_3) \sqrt{4 p(u_2)^3 - \rho} p(u_1)^3 \\ & \quad - 2 p(u_2) \gamma \beta u_{1,1} p(u_3) \sqrt{4 p(u_2)^3 - \rho} \rho \\ & \quad \left. + 4 p(u_1) \alpha \beta u_{1,2} p(u_3) \sqrt{4 p(u_1)^3 - \rho} p(u_2)^3 \right) \end{aligned} \tag{52}$$

$$\begin{aligned}
& -p(u_1) \alpha \beta u_{1,2} p(u_3) \sqrt{4p(u_1)^3 - \rho} \rho - p(u_1) \alpha \sqrt{4p(u_2)^3 - \rho} \gamma u_{1,3} p(u_2) \rho \\
& -p(u_1) \alpha \sqrt{4p(u_3)^3 - \rho} \beta u_{1,2} p(u_3) \rho \\
& + 4p(u_1) \alpha \gamma u_{1,3} p(u_2) \sqrt{4p(u_1)^3 - \rho} p(u_3)^3 \\
& -p(u_1) \alpha \gamma u_{1,3} p(u_2) \sqrt{4p(u_1)^3 - \rho} \rho \\
& + \beta \alpha u_{2,3} p(u_1)^2 \sqrt{4p(u_2)^3 - \rho} \sqrt{4p(u_3)^3 - \rho} \sqrt{4p(u_1)^3 - \rho} \\
& + \gamma \alpha u_{2,3} p(u_1)^2 \sqrt{4p(u_2)^3 - \rho} \sqrt{4p(u_3)^3 - \rho} \sqrt{4p(u_1)^3 - \rho} \\
& + 4p(u_2) \gamma \beta u_{1,1} p(u_3) \sqrt{4p(u_1)^3 - \rho} p(u_1)^3 \\
& + 2p(u_2) \gamma \beta u_{1,1} p(u_3) \sqrt{4p(u_1)^3 - \rho} \rho \\
& + \beta \gamma u_{1,3} p(u_1) p(u_2) \sqrt{4p(u_1)^3 - \rho} \sqrt{4p(u_3)^3 - \rho} \sqrt{4p(u_2)^3 - \rho} \\
& -p(u_1) \alpha \sqrt{4p(u_3)^3 - \rho} \beta u_{1,2} p(u_3) \sqrt{4p(u_1)^3 - \rho} \sqrt{4p(u_2)^3 - \rho} \\
& + \gamma \beta u_{1,2} p(u_1) p(u_3) \sqrt{4p(u_1)^3 - \rho} \sqrt{4p(u_2)^3 - \rho} \sqrt{4p(u_3)^3 - \rho} \\
& - 2p(u_2) \gamma \beta u_{1,1} p(u_3) \sqrt{4p(u_1)^3 - \rho} \sqrt{4p(u_2)^3 - \rho} \sqrt{4p(u_3)^3 - \rho} \\
& -p(u_1) \alpha \sqrt{4p(u_2)^3 - \rho} \gamma u_{1,3} p(u_2) \sqrt{4p(u_1)^3 - \rho} \sqrt{4p(u_3)^3 - \rho} \\
& - 2\gamma \alpha u_{2,3} p(u_1)^2 \sqrt{4p(u_3)^3 - \rho} p(u_2)^3 - \gamma \alpha u_{2,3} p(u_1)^2 \sqrt{4p(u_3)^3 - \rho} \rho \\
& - 2\beta \alpha u_{2,3} p(u_1)^2 \sqrt{4p(u_2)^3 - \rho} p(u_3)^3 - \beta \alpha u_{2,3} p(u_1)^2 \sqrt{4p(u_2)^3 - \rho} \rho \\
& - 4\beta \gamma u_{1,3} p(u_1)^4 p(u_2) \sqrt{4p(u_3)^3 - \rho} + 2p(u_1)^4 \alpha \sqrt{4p(u_3)^3 - \rho} \gamma u_{1,3} p(u_2) \\
& - 4\gamma \beta u_{1,2} p(u_1)^4 p(u_3) \sqrt{4p(u_2)^3 - \rho} + 2p(u_1)^4 \alpha \sqrt{4p(u_2)^3 - \rho} \beta u_{1,2} p(u_3) \\
& - 2p(u_1)^4 \alpha \sqrt{4p(u_2)^3 - \rho} \gamma u_{1,3} p(u_2) - 2p(u_1)^4 \alpha \sqrt{4p(u_3)^3 - \rho} \beta u_{1,2} p(u_3) \\
& + 2\gamma \alpha u_{2,3} p(u_1)^2 \sqrt{4p(u_1)^3 - \rho} p(u_2)^3 + \gamma \alpha u_{2,3} p(u_1)^2 \sqrt{4p(u_1)^3 - \rho} \rho \\
& - 4\gamma \alpha u_{2,3} p(u_1)^2 \sqrt{4p(u_2)^3 - \rho} p(u_3)^3 + \gamma \alpha u_{2,3} p(u_1)^2 \sqrt{4p(u_2)^3 - \rho} \rho \\
& - 4\beta \alpha u_{2,3} p(u_1)^2 \sqrt{4p(u_3)^3 - \rho} p(u_2)^3 + \beta \alpha u_{2,3} p(u_1)^2 \sqrt{4p(u_3)^3 - \rho} \rho \\
& + 2\beta \alpha u_{2,3} p(u_1)^2 \sqrt{4p(u_1)^3 - \rho} p(u_3)^3 + \beta \alpha u_{2,3} p(u_1)^2 \sqrt{4p(u_1)^3 - \rho} \rho \Big) / \\
& \left( p(u_1) p(u_3) p(u_2) \left( -\sqrt{4p(u_1)^3 - \rho} + \sqrt{4p(u_2)^3 - \rho} \right) \beta \left( \sqrt{4p(u_3)^3 - \rho} \right. \right. \\
& \left. \left. - \sqrt{4p(u_1)^3 - \rho} \right) \gamma \right)
\end{aligned}$$

> *simplify*(diff(%, u<sub>2,3</sub>))

$$\begin{aligned}
& - \left( \alpha p(u_1) \left( -\beta \sqrt{4p(u_2)^3 - \rho} \sqrt{4p(u_3)^3 - \rho} \sqrt{4p(u_1)^3 - \rho} \right. \right. \\
& \quad - \gamma \sqrt{4p(u_2)^3 - \rho} \sqrt{4p(u_3)^3 - \rho} \sqrt{4p(u_1)^3 - \rho} + 2\gamma \sqrt{4p(u_3)^3 - \rho} p(u_2)^3 \\
& \quad + \gamma \sqrt{4p(u_3)^3 - \rho} \rho + 2\beta \sqrt{4p(u_2)^3 - \rho} p(u_3)^3 + \beta \sqrt{4p(u_2)^3 - \rho} \rho \\
& \quad - 2\gamma \sqrt{4p(u_1)^3 - \rho} p(u_2)^3 - \gamma \sqrt{4p(u_1)^3 - \rho} \rho + 4\gamma \sqrt{4p(u_2)^3 - \rho} p(u_3)^3 \\
& \quad - \gamma \sqrt{4p(u_2)^3 - \rho} \rho + 4\beta \sqrt{4p(u_3)^3 - \rho} p(u_2)^3 - \beta \sqrt{4p(u_3)^3 - \rho} \rho \\
& \quad \left. \left. - 2\beta \sqrt{4p(u_1)^3 - \rho} p(u_3)^3 - \beta \sqrt{4p(u_1)^3 - \rho} \rho \right) \right) / \left( p(u_3) p(u_2) \left( \right. \right. \\
& \quad \left. \left. - \sqrt{4p(u_1)^3 - \rho} + \sqrt{4p(u_2)^3 - \rho} \right) \beta \left( \sqrt{4p(u_3)^3 - \rho} - \sqrt{4p(u_1)^3 - \rho} \right) \gamma \right)
\end{aligned} \tag{53}$$

This was a bit messy, we should have gotten the equation on the Weirstrass function...
