# Supplementary material for: Dispersionless integrable systems in 3D and Einstein-Weyl geometry
Source: arXiv:1208.2728 ancillary file (2013-05-09)
Supplement: Supplementary file 13 [file Examples-3.pdf]

This is the worksheet accompanying the paper E.Ferapontov & B.Kruglikov "Dispersionless integrable systems in 3D and Einstein-Weyl geometry".

The file ran on **Maple** version 16, the package **DifferentialGeometry** was used.

For integrable PDE of type III, dispersionless Hirota type equations, we consider 3 examples and for them we check that integrability is equivalent to EW property.

For explanations of the steps consult file Examples-1, we write only basic comments here.

>

I. We are going to consider the 2nd order PDE in Hirota form  $\exp(u_{tt})=\exp(u_{xx})+\exp(u_{yy})$  and check if the corresponding conformal metric is EW

>

> with(DifferentialGeometry) : with(Tensor) : with(Tools) : with(JetCalculus) :  
with(LinearAlgebra) : with(PDEtools, D\_Dx, declare, ToJet, FromJet) :

> DGsetup([t, x, y], [u], J2) :

>  $F := e^{u_{1,1}} - e^{u_{2,2}} - e^{u_{3,3}}$

$$F := e^{u_{1,1}} - e^{u_{2,2}} - e^{u_{3,3}} \quad (1)$$

>  $A := \text{Matrix}\left(\left[\left[\text{diff}(F, u[1, 1]), \frac{1}{2} \text{diff}(F, u[1, 2]), \frac{1}{2} \text{diff}(F, u[1, 3])\right], \left[\frac{1}{2} \text{diff}(F, u[1, 2]), \text{diff}(F, u[2, 2]), \frac{1}{2} \text{diff}(F, u[2, 3])\right], \left[\frac{1}{2} \text{diff}(F, u[1, 3]), \frac{1}{2} \text{diff}(F, u[2, 3]), \text{diff}(F, u[3, 3])\right]\right]\right);$   
 $AA := \text{expand}(\text{MatrixInverse}(A)) : AM := \text{simplify}(\text{Determinant}(A) \cdot AA) :$

$$A := \begin{bmatrix} e^{u_{1,1}} & 0 & 0 \\ 0 & -e^{u_{2,2}} & 0 \\ 0 & 0 & -e^{u_{3,3}} \end{bmatrix} \quad (2)$$

> simplify(AA); simplify(Determinant(A));

$$\begin{bmatrix} e^{-u_{1,1}} & 0 & 0 \\ 0 & -e^{-u_{2,2}} & 0 \\ 0 & 0 & -e^{-u_{3,3}} \end{bmatrix} e^{u_{1,1} + u_{2,2} + u_{3,3}} \quad (3)$$

> DepVars := [u(t, x, y)] : AJ := simplify(FromJet(AA, DepVars));

(4)

$$AJ := \begin{bmatrix} e^{-\left(\frac{\partial^2}{\partial t^2} u(t, x, y)\right)} & 0 & 0 \\ 0 & -e^{-\left(\frac{\partial^2}{\partial x^2} u(t, x, y)\right)} & 0 \\ 0 & 0 & -e^{-\left(\frac{\partial^2}{\partial y^2} u(t, x, y)\right)} \end{bmatrix} \quad (4)$$

> DGsetup([t, x, y], M) :

> g := evalDG(AJ[1, 1]·dt &t dt + AJ[1, 2]·dt &t dx + AJ[1, 3]·dt &t dy + AJ[2, 1]·dx &t dt + AJ[2, 2]·dx &t dx + AJ[2, 3]·dx &t dy + AJ[3, 1]·dy &t dt + AJ[3, 2]·dy &t dx + AJ[3, 3]·dy &t dy) :

> C := Connection(a000\*dt &t D\_t &t dt + a111\*dx &t D\_x &t dx + a222\*dy &t D\_y &t dy + a001\*(dt &t D\_t &t dx + dx &t D\_t &t dt) + a002\*(dt &t D\_t &t dy + dy &t D\_t &t dt) + a102\*(dx &t D\_t &t dy + dy &t D\_t &t dx) + a011\*(dt &t D\_x &t dx + dx &t D\_x &t dt) + a012\*(dt &t D\_x &t dy + dy &t D\_x &t dt) + a112\*(dx &t D\_x &t dy + dy &t D\_x &t dx) + a021\*(dt &t D\_y &t dx + dx &t D\_y &t dt) + a022\*(dt &t D\_y &t dy + dy &t D\_y &t dt) + a122\*(dx &t D\_y &t dy + dy &t D\_y &t dx) + a010\*dt &t D\_x &t dt + a121\*dx &t D\_y &t dx + a202\*dy &t D\_t &t dy + a020\*dt &t D\_y &t dt + a101\*dx &t D\_t &t dx + a212\*dy &t D\_x &t dy) :

> TorsionTensor(C);

$$0 \, dt \, D_t \, dt$$

(5)

> U1 := simplify(diff(ln(FromJet( $\frac{A[1, 1]}{A[2, 2] \cdot A[3, 3]}$ ), DepVars)), t);

U2 := simplify(diff(ln(FromJet( $\frac{A[2, 2]}{A[1, 1] \cdot A[3, 3]}$ ), DepVars)), x);

U3 := simplify(diff(ln(FromJet( $\frac{A[3, 3]}{A[1, 1] \cdot A[2, 2]}$ ), DepVars)), y);

$$U1 := \frac{\partial^3}{\partial t^3} u(t, x, y) - \left( \frac{\partial^3}{\partial x^2 \partial t} u(t, x, y) \right) - \left( \frac{\partial^3}{\partial y^2 \partial t} u(t, x, y) \right)$$

$$U2 := \frac{\partial^3}{\partial x^3} u(t, x, y) - \left( \frac{\partial^3}{\partial x \partial t^2} u(t, x, y) \right) - \left( \frac{\partial^3}{\partial y^2 \partial x} u(t, x, y) \right)$$

$$U3 := \frac{\partial^3}{\partial y^3} u(t, x, y) - \left( \frac{\partial^3}{\partial y \partial t^2} u(t, x, y) \right) - \left( \frac{\partial^3}{\partial y \partial x^2} u(t, x, y) \right)$$

(6)

> Et := evalDG(DirectionalCovariantDerivative(D\_t, g, C) - U1·g) :

Ex := evalDG(DirectionalCovariantDerivative(D\_x, g, C) - U2·g) :

Ey := evalDG(DirectionalCovariantDerivative(D\_y, g, C) - U3·g) :

> Eq000 := TensorInnerProduct(g, Et, dt &t dt) :

Eq001 := TensorInnerProduct(g, Et, dt &t dx) :

Eq002 := TensorInnerProduct(g, Et, dt &t dy) :

Eq011 := TensorInnerProduct(g, Et, dx &t dx) :

Eq012 := TensorInnerProduct(g, Et, dx &t dy) :

Eq022 := TensorInnerProduct(g, Et, dy &t dy) :

Eq100 := TensorInnerProduct(g, Ex, dt &t dt) :

Eq101 := TensorInnerProduct(g, Ex, dt &t dx) :

Eq102 := TensorInnerProduct(g, Ex, dt &t dy) :

```

Eq111 := TensorInnerProduct(g, Ex, dx &t dx) :
Eq112 := TensorInnerProduct(g, Ex, dx &t dy) :
Eq122 := TensorInnerProduct(g, Ex, dy &t dy) :
Eq200 := TensorInnerProduct(g, Ey, dt &t dt) :
Eq201 := TensorInnerProduct(g, Ey, dt &t dx) :
Eq202 := TensorInnerProduct(g, Ey, dt &t dy) :
Eq211 := TensorInnerProduct(g, Ey, dx &t dx) :
Eq212 := TensorInnerProduct(g, Ey, dx &t dy) :
Eq222 := TensorInnerProduct(g, Ey, dy &t dy) :

```

```

> sA := solve( {Eq000=0, Eq001=0, Eq002=0, Eq011=0, Eq012=0, Eq022=0, Eq100=0,
Eq101=0, Eq102=0, Eq111=0, Eq112=0, Eq122=0, Eq200=0, Eq201=0, Eq202=0,
Eq211=0, Eq212=0, Eq222=0}, [a000, a001, a002, a010, a011, a012, a020, a021, a022,
a101, a102, a111, a112, a121, a122, a202, a212, a222] ) :

```

```

> C1 := evalDG( subs( {op(op(sA))}, C) ) :

```

```

> evalDG( CovariantDerivative(g, C1) - g &t (U1·dt + U2·dx + U3·dy) );
0 dt dt dt

```

(7)

```

> R1 := CurvatureTensor(C1) : Ric1 := RicciTensor(R1) : T1 := SymmetrizeIndices(Ric1, [1, 2],
"Symmetric") : Res := evalDG(T1 - V·g) :

```

```

> NEQtt := ContractIndices(Res, D_t &t D_t, [[1, 1], [2, 2]]) : NEQtx := ContractIndices(Res,
D_t &t D_x, [[1, 1], [2, 2]]) :
NEQty := ContractIndices(Res, D_t &t D_y, [[1, 1], [2, 2]]) : NEQxx := ContractIndices(Res,
D_x &t D_x, [[1, 1], [2, 2]]) :
NEQxy := ContractIndices(Res, D_x &t D_y, [[1, 1], [2, 2]]) : NEQyy := ContractIndices(Res,
D_y &t D_y, [[1, 1], [2, 2]]) :

```

```

> DGsetup([t, x, y], [u], J2, 4) :

```

```

> de := DifferentialEquationData([F], [u1, 1])

```

$$de := \left[ \{u_{1,1}\}, \left[ e^{u_{1,1}} - e^{u_{2,2}} - e^{u_{3,3}} \right] \right]$$

(8)

```

> de2 := Prolong(de, 2) : deTRA := Transformation(de2) :

```

```

> Eq0 := Pullback(deTRA, ToJet(NEQtt, DepVars, notation = jetnumbers)) :

```

```

> VS := solve(Eq0, V) :

```

```

> Eq1 := numer(subs(V=VS, Pullback(deTRA, ToJet(NEQtx, DepVars, notation
=jetnumbers)))) :

```

```

Eq2 := numer(subs(V=VS, Pullback(deTRA, ToJet(NEQty, DepVars, notation
=jetnumbers)))) :

```

```

Eq3 := numer(subs(V=VS, Pullback(deTRA, ToJet(NEQxx, DepVars, notation
=jetnumbers)))) :

```

```

Eq4 := numer(subs(V=VS, Pullback(deTRA, ToJet(NEQxy, DepVars, notation
=jetnumbers)))) :

```

```

Eq5 := numer(subs(V=VS, Pullback(deTRA, ToJet(NEQyy, DepVars, notation
=jetnumbers)))) :

```

```

J2 > simplify([Eq1, Eq2, Eq3, Eq4, Eq5])

```

[0, 0, 0, 0, 0]

(9)

Perfect!

```

>

```

```

>

```

II. Now we shall consider the example:  $u_{tt}=u_{xy}/u_{xt}+1/6*(\eta(u_{xx}))u_{xt}^2$   
and check if the corresponding conformal metric is EW provided  $\eta()$  satisfies a 4th order ODE.  
( $\eta$  will be  $f$  in what follows)

```
> restart : with(DifferentialGeometry) : with(Tensor) : with(Tools) : with(JetCalculus) :
with(LinearAlgebra) : with(PDEtools, D_Dx, declare, ToJet, FromJet) :
> DGsetup([t, x, y], [u], J2) :
```

```
> F := u_{1,1} - \frac{u_{2,3}}{u_{1,2}} - \frac{1}{6} f(u_{2,2}) \cdot u_{1,2}^2
```

$$F := u_{1,1} - \frac{u_{2,3}}{u_{1,2}} - \frac{1}{6} f(u_{2,2}) u_{1,2}^2 \quad (10)$$

```
> A := Matrix([ [diff(F, u[1,1]), \frac{1}{2} diff(F, u[1,2]), \frac{1}{2} diff(F, u[1,3]) ], [ \frac{1}{2} diff(F, u[1,2]), diff(F, u[2,2]), \frac{1}{2} diff(F, u[2,3]) ], [ \frac{1}{2} diff(F, u[1,3]), \frac{1}{2} diff(F, u[2,3]), diff(F, u[3,3]) ] ] ); AA := expand(MatrixInverse(A)) : AM := simplify(Determinant(A) \cdot AA) :
```

$$A := \begin{bmatrix} 1 & \frac{1}{2} \frac{u_{2,3}}{u_{1,2}^2} - \frac{1}{6} f(u_{2,2}) u_{1,2} & 0 \\ \frac{1}{2} \frac{u_{2,3}}{u_{1,2}^2} - \frac{1}{6} f(u_{2,2}) u_{1,2} & -\frac{1}{6} \left( \frac{d}{du_{2,2}} f(u_{2,2}) \right) u_{1,2}^2 - \frac{1}{2 u_{1,2}} \\ 0 & -\frac{1}{2 u_{1,2}} & 0 \end{bmatrix} \quad (11)$$

```
> AA; ad := Determinant(A);
```

$$\begin{bmatrix} 1, 0, -\frac{1}{3} \frac{-3 u_{2,3} + f(u_{2,2}) u_{1,2}^3}{u_{1,2}} \end{bmatrix},$$

$$\begin{bmatrix} 0, 0, -2 u_{1,2} \end{bmatrix},$$

$$\left[ -\frac{1}{3} \frac{-3 u_{2,3} + f(u_{2,2}) u_{1,2}^3}{u_{1,2}}, -2 u_{1,2}, \frac{1}{9} \frac{6 \left( \frac{d}{du_{2,2}} f(u_{2,2}) \right) u_{1,2}^6 + 9 u_{2,3}^2 - 6 u_{2,3} f(u_{2,2}) u_{1,2}^3 + f(u_{2,2})^2 u_{1,2}^6}{u_{1,2}^2} \right] \\ ad := -\frac{1}{4 u_{1,2}^2} \quad (12)$$

$$\begin{aligned} & \text{DepVars} := [u(t, x, y)] : AJ := \text{simplify}(\text{FromJet}(AA, \text{DepVars})) \\ AJ := & \left[ \left[ 1, 0, \frac{1}{3} \frac{3 \left( \frac{\partial^2}{\partial y \partial x} u(t, x, y) \right) - f \left( \frac{\partial^2}{\partial x^2} u(t, x, y) \right) \left( \frac{\partial^2}{\partial x \partial t} u(t, x, y) \right)^3}{\frac{\partial^2}{\partial x \partial t} u(t, x, y)}, \right. \right. \\ & \left. \left[ 0, 0, -2 \left( \frac{\partial^2}{\partial x \partial t} u(t, x, y) \right) \right], \right. \\ & \left. \left[ \frac{1}{3} \frac{3 \left( \frac{\partial^2}{\partial y \partial x} u(t, x, y) \right) - f \left( \frac{\partial^2}{\partial x^2} u(t, x, y) \right) \left( \frac{\partial^2}{\partial x \partial t} u(t, x, y) \right)^3}{\frac{\partial^2}{\partial x \partial t} u(t, x, y)}, -2 \left( \frac{\partial^2}{\partial x \partial t} u(t, x, \right. \right. \\ & \left. \left. y \right) \right], \frac{1}{9} \frac{1}{D_{1,2}(u)(t, x, y)^2} \left( 6 D(f) (D_{2,2}(u)(t, x, y)) D_{1,2}(u)(t, x, y)^6 \right. \right. \\ & \left. \left. + 9 D_{2,3}(u)(t, x, y)^2 - 6 D_{2,3}(u)(t, x, y) f(D_{2,2}(u)(t, x, y)) D_{1,2}(u)(t, x, y)^3 \right. \right. \\ & \left. \left. + f(D_{2,2}(u)(t, x, y))^2 D_{1,2}(u)(t, x, y)^6 \right) \right] \end{aligned} \quad (13)$$

$$\begin{aligned} & \text{aa} := [TotalDiff(A[1, 1], 1) + TotalDiff(A[1, 2], 2) + TotalDiff(A[1, 3], 3), TotalDiff(A[2, \\ & 1], 1) + TotalDiff(A[2, 2], 2) + TotalDiff(A[2, 3], 3), TotalDiff(A[3, 1], 1) \\ & + TotalDiff(A[3, 2], 2) + TotalDiff(A[3, 3], 3)] \\ aa := & \left[ \left( -\frac{u_{2,3}}{u_{1,2}^3} - \frac{1}{6} f(u_{2,2}) \right) u_{1,2,2} - \frac{1}{6} \left( \frac{d}{du_{2,2}} f(u_{2,2}) \right) u_{1,2} u_{2,2,2} + \frac{1}{2} \frac{u_{2,2,3}}{u_{1,2}^2}, \left( \right. \right. \\ & \left. \left. -\frac{u_{2,3}}{u_{1,2}^3} - \frac{1}{6} f(u_{2,2}) \right) u_{1,1,2} - \frac{1}{2} \left( \frac{d}{du_{2,2}} f(u_{2,2}) \right) u_{1,2} u_{1,2,2} + \frac{u_{1,2,3}}{u_{1,2}^2} \right. \\ & \left. - \frac{1}{6} \left( \frac{d^2}{du_{2,2}^2} f(u_{2,2}) \right) u_{1,2}^2 u_{2,2,2}, \frac{1}{2} \frac{u_{1,2,2}}{u_{1,2}^2} \right] \quad (14) \end{aligned}$$

$$\begin{aligned} & \text{aA} := \text{FromJet}(aa, \text{DepVars}) : \\ & \text{aD} := [\text{FromJet}(TotalDiff(\ln(ad), 1), \text{DepVars}), \text{FromJet}(TotalDiff(\ln(ad), 2), \text{DepVars}), \\ & \text{FromJet}(TotalDiff(\ln(ad), 3), \text{DepVars})] : \end{aligned}$$

```

>
> DGsetup([t, x, y], M) :
> g := evalDG(AJ[1, 1]·dt &t dt + AJ[1, 2]·dt &t dx + AJ[1, 3]·dt &t dy + AJ[2, 1]·dx &t dt
+ AJ[2, 2]·dx &t dx + AJ[2, 3]·dx &t dy + AJ[3, 1]·dy &t dt + AJ[3, 2]·dy &t dx
+ AJ[3, 3]·dy &t dy) :
> C := Connection(a000*dt &t D_t &t dt + a111*dx &t D_x &t dx + a222*dy &t D_y &t dy
+ a001*(dt &t D_t &t dx + dx &t D_t &t dt) + a002*(dt &t D_t &t dy + dy &t D_t
&t dt) + a102*(dx &t D_t &t dy + dy &t D_t &t dx) + a011*(dt &t D_x &t dx + dx
&t D_x &t dt) + a012*(dt &t D_x &t dy + dy &t D_x &t dt) + a112*(dx &t D_x &t dy
+ dy &t D_x &t dx) + a021*(dt &t D_y &t dx + dx &t D_y &t dt) + a022*(dt &t D_y
&t dy + dy &t D_y &t dt) + a122*(dx &t D_y &t dy + dy &t D_y &t dx) + a010*dt
&t D_x &t dt + a121*dx &t D_y &t dx + a202*dy &t D_t &t dy + a020*dt &t D_y &t dt
+ a101*dx &t D_t &t dx + a212*dy &t D_x &t dy) :
> TorsionTensor(C);
0 dt D_t dt (15)
> U1 := simplify(2(AJ[1, 1]·aA[1] + AJ[1, 2]·aA[2] + AJ[1, 3]·aA[3]) - aD[1]) :
U2 := simplify(2(AJ[2, 1]·aA[1] + AJ[2, 2]·aA[2] + AJ[2, 3]·aA[3]) - aD[2]) :
U3 := simplify(2(AJ[3, 1]·aA[1] + AJ[3, 2]·aA[2] + AJ[3, 3]·aA[3]) - aD[3]) :
> Et := evalDG(DirectionalCovariantDerivative(D_t, g, C) - U1·g) :
Ex := evalDG(DirectionalCovariantDerivative(D_x, g, C) - U2·g) :
Ey := evalDG(DirectionalCovariantDerivative(D_y, g, C) - U3·g) :
> Eq000 := TensorInnerProduct(g, Et, dt &t dt) :
Eq001 := TensorInnerProduct(g, Et, dt &t dx) :
Eq002 := TensorInnerProduct(g, Et, dt &t dy) :
Eq011 := TensorInnerProduct(g, Et, dx &t dx) :
Eq012 := TensorInnerProduct(g, Et, dx &t dy) :
Eq022 := TensorInnerProduct(g, Et, dy &t dy) :
Eq100 := TensorInnerProduct(g, Ex, dt &t dt) :
Eq101 := TensorInnerProduct(g, Ex, dt &t dx) :
Eq102 := TensorInnerProduct(g, Ex, dt &t dy) :
Eq111 := TensorInnerProduct(g, Ex, dx &t dx) :
Eq112 := TensorInnerProduct(g, Ex, dx &t dy) :
Eq122 := TensorInnerProduct(g, Ex, dy &t dy) :
Eq200 := TensorInnerProduct(g, Ey, dt &t dt) :
Eq201 := TensorInnerProduct(g, Ey, dt &t dx) :
Eq202 := TensorInnerProduct(g, Ey, dt &t dy) :
Eq211 := TensorInnerProduct(g, Ey, dx &t dx) :
Eq212 := TensorInnerProduct(g, Ey, dx &t dy) :
Eq222 := TensorInnerProduct(g, Ey, dy &t dy) :
> sA := solve({Eq000=0, Eq001=0, Eq002=0, Eq011=0, Eq012=0, Eq022=0, Eq100=0,
Eq101=0, Eq102=0, Eq111=0, Eq112=0, Eq122=0, Eq200=0, Eq201=0, Eq202=0,
Eq211=0, Eq212=0, Eq222=0}, [a000, a001, a002, a010, a011, a012, a020, a021, a022,
a101, a102, a111, a112, a121, a122, a202, a212, a222]) :
> C1 := evalDG(subs({op(op(sA))}, C)) :
> evalDG(CovariantDerivative(g, C1) - g &t (U1·dt + U2·dx + U3·dy));
0 dt dt dt (16)
> R1 := CurvatureTensor(C1) : Ric1 := RicciTensor(R1) : T1 := SymmetrizeIndices(Ric1, [1, 2],
"Symmetric") : Res := evalDG(T1 - V·g) :

```

```

> NEQt := ContractIndices(Res, D_t &t D_t, [[1, 1], [2, 2]]) : NEQt := ContractIndices(Res,
    D_t &t D_x, [[1, 1], [2, 2]]) :
NEQty := ContractIndices(Res, D_t &t D_y, [[1, 1], [2, 2]]) : NEQxx := ContractIndices(Res,
    D_x &t D_x, [[1, 1], [2, 2]]) :
NEQxy := ContractIndices(Res, D_x &t D_y, [[1, 1], [2, 2]]) : NEQyy := ContractIndices(Res,
    D_y &t D_y, [[1, 1], [2, 2]]) :
>
> DGsetup([t, x, y], [u], J2, 4) :
> de := DifferentialEquationData([F], [u1,1])

```

$$de := \left[ \{u_{1,1}\}, \left[ u_{1,1} - \frac{u_{2,3}}{u_{1,2}} - \frac{1}{6} f(u_{2,2}) u_{1,2}^2 \right] \right] \quad (17)$$

```

> de2 := Prolong(de, 2) : deTRA := Transformation(de2) :
>
> Eq0 := Pullback(deTRA, ToJet(NEQt, DepVars, notation = jetnumbers)) :
> VS := solve(Eq0, V) :
> Eq1 := numer(subs(V = VS, Pullback(deTRA, ToJet(NEQt, DepVars, notation
    = jetnumbers)))) :
Eq2 := numer(subs(V = VS, Pullback(deTRA, ToJet(NEQty, DepVars, notation
    = jetnumbers)))) :
Eq3 := numer(subs(V = VS, Pullback(deTRA, ToJet(NEQxx, DepVars, notation
    = jetnumbers)))) :
Eq4 := numer(subs(V = VS, Pullback(deTRA, ToJet(NEQxy, DepVars, notation
    = jetnumbers)))) :
Eq5 := numer(subs(V = VS, Pullback(deTRA, ToJet(NEQyy, DepVars, notation
    = jetnumbers)))) :
J2 > simplify([Eq1, Eq2, Eq3, Eq4])

```

$$[0, 0, 0, 0] \quad (18)$$

```

J2 > simplify(Eq5)

```

$$\begin{aligned}
& u_{1,2}^{10} \left( u_{1,2}^4 \left( \frac{d}{du_{2,2}} f(u_{2,2}) \right) \left( \frac{d^3}{du_{2,2}^3} f(u_{2,2}) \right) u_{2,2,2}^2 + 18 \left( \frac{d}{du_{2,2}} f(u_{2,2}) \right)^2 u_{1,2}^2 u_{1,2,2}^2 \right. \\
& - 3 u_{1,2}^4 \left( \frac{d}{du_{2,2}} f(u_{2,2}) \right)^3 u_{2,2,2}^2 - 6 u_{1,2}^2 \left( \frac{d^3}{du_{2,2}^3} f(u_{2,2}) \right) u_{1,2,2}^2 \\
& - 12 \left( \frac{d^2}{du_{2,2}^2} f(u_{2,2}) \right) u_{2,2,2} u_{2,3} u_{1,2,2} f(u_{2,2}) \\
& + 6 u_{1,2} \left( \frac{d^3}{du_{2,2}^3} f(u_{2,2}) \right) u_{2,2,3} u_{2,2,2} - 18 u_{1,2} u_{2,2,3} \left( \frac{d}{du_{2,2}} f(u_{2,2}) \right)^2 u_{2,2,2} - 12 \\
& u_{1,2}^2 u_{1,2,2}^2 f(u_{2,2}) \left( \frac{d^2}{du_{2,2}^2} f(u_{2,2}) \right) + 18 \left( \frac{d}{du_{2,2}} f(u_{2,2}) \right)^2 u_{1,2,2} u_{2,3} u_{2,2,2} \\
& \left. - 6 \left( \frac{d}{du_{2,2}} f(u_{2,2}) \right)^2 u_{1,2}^3 u_{1,2,2} f(u_{2,2}) u_{2,2,2} + 4 \left( \frac{d^2}{du_{2,2}^2} f(u_{2,2}) \right) u_{2,2,2} \right) \quad (19)
\end{aligned}$$

$$\begin{aligned}
& u_{1,2}^3 f(u_{2,2})^2 u_{1,2,2} + 12 \left( \frac{d^2}{du_{2,2}^2} f(u_{2,2}) \right) u_{2,2,2} u_{1,2} f(u_{2,2}) u_{2,2,3} \\
& + 2 \left( \frac{d^2}{du_{2,2}^2} f(u_{2,2}) \right) u_{2,2,2}^2 u_{1,2}^4 f(u_{2,2}) \left( \frac{d}{du_{2,2}} f(u_{2,2}) \right) + 2 \\
& u_{1,2}^3 f(u_{2,2}) \left( \frac{d^3}{du_{2,2}^3} f(u_{2,2}) \right) u_{2,2,2} u_{1,2,2} - 6 u_{2,3} \left( \frac{d^3}{du_{2,2}^3} f(u_{2,2}) \right) u_{2,2,2} u_{1,2,2} \\
\text{J2} & > \text{solve} \left( \%, \frac{d^3}{du_{2,2}^3} f(u_{2,2}) \right) \\
& - 2 \left( \frac{d^2}{du_{2,2}^2} f(u_{2,2}) \right) f(u_{2,2}) + 3 \left( \frac{d}{du_{2,2}} f(u_{2,2}) \right)^2
\end{aligned} \tag{20}$$

Perfect! This means precisely that f is the solution to the Chazy equation

$$\begin{aligned}
& > \\
& > \\
& > \\
& > \\
& > \\
\text{J2} & > \text{ToJet}(U1, \text{DepVars}) \\
& - \frac{1}{3} \frac{1}{u_{t,x}^3} \left( 3 u_{t,x,x} u_{x,y} + 2 u_{t,x,x} f(u_{x,x}) u_{t,x}^3 + \left( \frac{d}{du_{x,x}} f(u_{x,x}) \right) u_{t,x}^4 u_{x,x,x} - 3 u_{x,x,y} u_{t,x} \right. \\
& \quad \left. - 6 u_{t,t,x} u_{t,x}^2 \right)
\end{aligned} \tag{21}$$

$$\text{J2} > \text{ToJet}(U2, \text{DepVars}) \tag{22}$$

$$\begin{aligned}
& \text{J2} > \text{collect}(\text{expand}(\text{ToJet}(U3, \text{DepVars})), \{u_{t,t,x}, u_{t,x,x}, u_{x,x,x}, u_{x,x,y}\}) \\
& \left( \frac{2}{3} u_{t,x} f(u_{x,x}) + \frac{4 u_{x,y}}{u_{t,x}^2} \right) u_{t,t,x} + \left( -\frac{u_{x,y}^2}{u_{t,x}^4} + \frac{2}{9} u_{t,x}^2 f(u_{x,x})^2 + \frac{8}{3} u_{t,x}^2 \left( \frac{d}{du_{x,x}} f(u_{x,x}) \right) \right. \\
& \quad \left. - \frac{1}{3} \frac{u_{x,y} f(u_{x,x})}{u_{t,x}} \right) u_{t,x,x} + \left( -\frac{1}{3} u_{x,y} \left( \frac{d}{du_{x,x}} f(u_{x,x}) \right) + \frac{1}{9} f(u_{x,x}) \right. \\
& \quad \left. u_{t,x}^3 \left( \frac{d}{du_{x,x}} f(u_{x,x}) \right) + \frac{2}{3} u_{t,x}^3 \left( \frac{d^2}{du_{x,x}^2} f(u_{x,x}) \right) \right) u_{x,x,x} + \left( -\frac{1}{3} f(u_{x,x}) + \frac{u_{x,y}}{u_{t,x}^3} \right) u_{x,x,y} \\
& \quad - \frac{2 u_{t,x,y}}{u_{t,x}}
\end{aligned} \tag{23}$$

J2 >

J2 > latex(%)  

$$\left( \frac{2}{3} u_{t,x} f(u_{x,x}) + \frac{4 u_{x,y}}{u_{t,x}^2} \right) u_{t,t,x} + \left( -\frac{u_{x,y}^2}{u_{t,x}^4} + \frac{2}{9} u_{t,x}^2 f(u_{x,x})^2 + \frac{8}{3} u_{t,x}^2 \left( \frac{d}{du_{x,x}} f(u_{x,x}) \right) \right.$$



```

y}}^{\{
2\}}{\{u_{\{t,x\}}\}^{\{4\}}\}+2/9\,{u_{\{t,x\}}\}^{\{2\}}\left(f\left(u_{\{x,x\}}\right)\right)^{\{2\}}+8/3\,{u_{\{t,x\}}\}^{\{2\}}\{\frac{d}{du_{\{x,x\}}}\}f\left(u_{\{x,x\}}\right)-1/3\,{\frac{u_{\{x,y\}}}{f}}\left(u_{\{x,x\}}\right)\right)\{u_{\{t,x\}}\}\right)u_{\{t,x,x\}}+\left(-1/3\,{u_{\{x,y\}}}\{\frac{d}{du_{\{x,x\}}}\}f\left(u_{\{x,x\}}\right)+1/9\,f\left(u_{\{x,x\}}\right)\right)\{u_{\{t,x\}}\}^{\{3\}}\{\frac{d}{du_{\{x,x\}}}\}f\left(u_{\{x,x\}}\right)+2/3\,{u_{\{t,x\}}\}^{\{3\}}\{\frac{d^2}{d^2u_{\{x,x\}}}\}d\{u_{\{x,x\}}\}^{\{2\}}\}f\left(u_{\{x,x\}}\right)\right)\right)u_{\{x,x,x\}}+\left(-1/3\,f\left(u_{\{x,x\}}\right)+{\frac{u_{\{x,y\}}}{f}}\{u_{\{t,x\}}\}^{\{3\}}\right)u_{\{x,y\}}\}-2\,{\frac{u_{\{t,x,y\}}}{f}}\{u_{\{t,x\}}\}\}

```

**J2** >
