# Supplementary material for: Dispersionless integrable systems in 3D and Einstein-Weyl geometry
Source: arXiv:1208.2728 ancillary file (2013-05-09)
Supplement: Supplementary file 14 [file Examples-4.pdf]

This is the worksheet accompanying the paper E.Ferapontov & B.Kruglikov "Dispersionless integrable systems in 3D and Einstein-Weyl geometry".

The file ran on **Maple** version 16, the package **DifferentialGeometry** was used.

For examples of integrable PDE of type IV and for some other types of equations we check that integrability is equivalent to EW property.

>

> restart :

I. To warm up, let us consider the Manakov-Santini system:  $u_{xt}=u_{yy}-(u \cdot u_x)_x - v_x \cdot u_{xy} + v_y \cdot u_{xx}$ ;  $v_{xt}=v_{yy} - u \cdot v_{xx} - v_x \cdot v_{xy} + v_y \cdot v_{xx}$

> alias(f=f(u<sub>2,2</sub>, u<sub>2,3</sub>, u<sub>3,3</sub>, u<sub>1,2</sub>, u<sub>1,3</sub>));

$f$

(1)

> with(DifferentialGeometry) : with(Tensor) : with(Tools) : with(JetCalculus) :  
with(LinearAlgebra) : with(PDEtools, D\_Dx, declare, ToJet, FromJet) :

> declare(h(u<sub>2,2</sub>, u<sub>2,3</sub>, u<sub>3,3</sub>)) : subs([h<sub>r</sub>(r, s, t) = haha], subs([u<sub>2,2</sub> = r, u<sub>2,3</sub> = s, u<sub>3,3</sub> = t, u<sub>1,2</sub> = a, u<sub>1,3</sub> = b],  $\frac{d^3}{du_{1,3}^3} f(u_{2,2}, u_{2,3}, u_{3,3}, u_{1,2}, u_{1,3})$ ))

$h(u_{2,2}, u_{2,3}, u_{3,3})$  will now be displayed as  $h$

$f_{b,b,b}$

(2)

> DGsetup([t, x, y], [u, v], J2) :

> F := u<sub>1,2</sub> - u<sub>3,3</sub> + TotalDiff(u<sub>[ ]</sub> · u<sub>2,2</sub>) + v<sub>2</sub> · u<sub>2,3</sub> - v<sub>3</sub> · u<sub>2,2</sub>;

G := v<sub>1,2</sub> - v<sub>3,3</sub> + u<sub>[ ]</sub> · v<sub>2,2</sub> + v<sub>2</sub> · v<sub>2,3</sub> - v<sub>3</sub> · v<sub>2,2</sub>;

$F := u_{1,2} - u_{3,3} + u_{[ ]}^2 + u_{[ ]} u_{2,2} + v_2 u_{2,3} - v_3 u_{2,2}$

$G := v_{1,2} - v_{3,3} + u_{[ ]} v_{2,2} + v_2 v_{2,3} - v_3 v_{2,2}$

(3)

> A := Matrix([ [diff(F, u[1,1]),  $\frac{1}{2}$  diff(F, u[1,2]),  $\frac{1}{2}$  diff(F, u[1,3]) ], [  $\frac{1}{2}$  diff(F, u[1,2]), diff(F, u[2,2]),  $\frac{1}{2}$  diff(F, u[2,3]) ], [  $\frac{1}{2}$  diff(F, u[1,3]),  $\frac{1}{2}$  diff(F, u[2,3]), diff(F, u[3,3]) ] ])

$$A := \begin{bmatrix} 0 & \frac{1}{2} & 0 \\ \frac{1}{2} u_{[ ]} - v_3 & \frac{1}{2} v_2 & \\ 0 & \frac{1}{2} v_2 & -1 \end{bmatrix}$$

(4)

> Av := Matrix([ [diff(G, v[1,1]),  $\frac{1}{2}$  diff(G, v[1,2]),  $\frac{1}{2}$  diff(G, v[1,3]) ], [  $\frac{1}{2}$  diff(G, v[1,2]), diff(G, v[2,2]),  $\frac{1}{2}$  diff(G, v[2,3]) ], [  $\frac{1}{2}$  diff(G, v[1,3]),  $\frac{1}{2}$  diff(G, v[2,3]),

$$diff(G, v[3, 3]) \big] \big])$$

$$Av := \begin{bmatrix} 0 & \frac{1}{2} & 0 \\ \frac{1}{2} & u_{[]} - v_3 & \frac{1}{2} v_2 \\ 0 & \frac{1}{2} v_2 & -1 \end{bmatrix} \quad (5)$$

```
J2 > AA := expand(MatrixInverse(A)); AM := simplify(Determinant(A) · AA); AdA
      := Adjoint(A);
```

$$\begin{aligned}
AA &:= \begin{bmatrix} -4u_{[]} + 4v_3 - v_2^2 & 2 & v_2 \\ 2 & 0 & 0 \\ v_2 & 0 & -1 \end{bmatrix} \\
AM &:= \begin{bmatrix} -u_{[]} + v_3 - \frac{1}{4}v_2^2 & \frac{1}{2} & \frac{1}{4}v_2 \\ \frac{1}{2} & 0 & 0 \\ \frac{1}{4}v_2 & 0 & -\frac{1}{4} \end{bmatrix} \\
AdA &:= \begin{bmatrix} -u_{[]} + v_3 - \frac{1}{4}v_2^2 & \frac{1}{2} & \frac{1}{4}v_2 \\ \frac{1}{2} & 0 & 0 \\ \frac{1}{4}v_2 & 0 & -\frac{1}{4} \end{bmatrix}
\end{aligned} \tag{6}$$

Here  $A$  is the matrix of the linearized operator (bivector=metric with upper indices),  
 $AA$  - the inverse (metric, which we remember is defined only up to conformal rescaling)  
and  $AJ=AM=AdA$  the adjoint matrix (which we use as a representative for the conformal class)

>

```
> aA := [TotalDiff(A[1, 1], 1) + TotalDiff(A[1, 2], 2) + TotalDiff(A[1, 3], 3), TotalDiff(A[2, 1], 1) + TotalDiff(A[2, 2], 2) + TotalDiff(A[2, 3], 3), TotalDiff(A[3, 1], 1) + TotalDiff(A[3, 2], 2) + TotalDiff(A[3, 3], 3)]:
```

$$\omega := 2 \cdot [AA[1, 1] \cdot aA[1] + AA[1, 2] \cdot aA[2] + AA[1, 3] \cdot aA[3], AA[2, 1] \cdot aA[1] + AA[2, 2] \cdot aA[2] + AA[2, 3] \cdot aA[3], AA[3, 1] \cdot aA[1] + AA[3, 2] \cdot aA[2] + AA[3, 3] \cdot aA[3]]:$$
$$J_2 > \omega$$

$$[4u_2 - 2v_{2,3} + v_2v_{2,2}, 0, -v_{2,2}] \quad (7)$$

**J2 >**

Let us re-write the system of hydrodynamic type from S5 through "polar" coordinates

**J2** > *alias*( $\rho = \rho(t, x, y)$ ,  $\phi = \phi(t, x, y)$ ); *declare*( $\rho(t, x, y)$ ); *declare*( $\phi(t, x, y)$ );

$\rho, \varphi$   
 $\text{declare}(\rho(t, x, y))$   
 $\text{declare}(\varphi(t, x, y))$

(8)

**J2** >  $U := \sqrt{\rho(t, x, y)} \cdot \cos(\varphi(t, x, y)) : V := \sqrt{\rho(t, x, y)} \cdot \sin(\varphi(t, x, y)) :$

>  $E1 := \text{numer}\left(\text{simplify}\left(\text{diff}(U, t) + \frac{U \cdot \text{diff}(U, x) + V \cdot \text{diff}(V, x) + U \cdot \text{diff}(V, y) - V \cdot \text{diff}(U, y)}{U^2 + V^2}\right)\right)$

$$E1 := \cos(\varphi) \left( \frac{\partial}{\partial t} \rho \right) \rho - 2 \rho^2 \sin(\varphi) \left( \frac{\partial}{\partial t} \varphi \right) + \sqrt{\rho} \left( \frac{\partial}{\partial x} \rho \right) + 2 \rho^{3/2} \left( \frac{\partial}{\partial y} \varphi \right)$$

(9)

>  $E2 := \text{numer}\left(\text{simplify}\left(\text{diff}(V, t) + \frac{V \cdot \text{diff}(U, x) - U \cdot \text{diff}(V, x) + U \cdot \text{diff}(U, y) + V \cdot \text{diff}(V, y)}{U^2 + V^2}\right)\right)$

$$E2 := \sin(\varphi) \left( \frac{\partial}{\partial t} \rho \right) \rho + 2 \rho^2 \cos(\varphi) \left( \frac{\partial}{\partial t} \varphi \right) - 2 \rho^{3/2} \left( \frac{\partial}{\partial x} \varphi \right) + \sqrt{\rho} \left( \frac{\partial}{\partial y} \rho \right)$$

(10)

>  $S := \text{solve}\left([E1 = 0, E2 = 0], \left[\frac{\partial}{\partial x} \varphi, \frac{\partial}{\partial y} \varphi\right]\right)[1]$

$$S := \left[ \frac{\partial}{\partial x} \varphi = \frac{1}{2} \frac{\sin(\varphi) \left( \frac{\partial}{\partial t} \rho \right) \rho + 2 \rho^2 \cos(\varphi) \left( \frac{\partial}{\partial t} \varphi \right) + \sqrt{\rho} \left( \frac{\partial}{\partial y} \rho \right)}{\rho^{3/2}}, \frac{\partial}{\partial y} \varphi = -\frac{1}{2} \frac{\cos(\varphi) \left( \frac{\partial}{\partial t} \rho \right) \rho - 2 \rho^2 \sin(\varphi) \left( \frac{\partial}{\partial t} \varphi \right) + \sqrt{\rho} \left( \frac{\partial}{\partial x} \rho \right)}{\rho^{3/2}} \right]$$

(11)

>  $\text{numer}\left(\text{simplify}\left(\text{subs}\left(S, \text{diff}\left(\text{subs}\left(S[1], \frac{\partial}{\partial x} \varphi\right), y\right) - \text{diff}\left(\text{subs}\left(S[1], \frac{\partial}{\partial y} \varphi\right), x\right)\right)\right)\right)$

$$\begin{aligned} & - \left( \frac{\partial}{\partial y} \rho \right) \sin(\varphi) \left( \frac{\partial}{\partial t} \rho \right) \rho + 2 \left( \frac{\partial}{\partial y} \rho \right) \rho^2 \cos(\varphi) \left( \frac{\partial}{\partial t} \varphi \right) - 2 \sqrt{\rho} \left( \frac{\partial}{\partial y} \rho \right)^2 \\ & - \rho^{3/2} \cos(\varphi)^2 \left( \frac{\partial}{\partial t} \rho \right)^2 + 4 \rho^{5/2} \cos(\varphi) \left( \frac{\partial}{\partial t} \rho \right) \sin(\varphi) \left( \frac{\partial}{\partial t} \varphi \right) \\ & - \cos(\varphi) \left( \frac{\partial}{\partial t} \rho \right) \rho \left( \frac{\partial}{\partial x} \rho \right) + 2 \sin(\varphi) \left( \frac{\partial^2}{\partial y \partial t} \rho \right) \rho^2 - 4 \rho^{7/2} \left( \frac{\partial}{\partial t} \varphi \right)^2 \\ & + 4 \rho^{7/2} \left( \frac{\partial}{\partial t} \varphi \right)^2 \cos(\varphi)^2 + 2 \rho^2 \sin(\varphi) \left( \frac{\partial}{\partial t} \varphi \right) \left( \frac{\partial}{\partial x} \rho \right) + 4 \rho^3 \cos(\varphi) \left( \frac{\partial^2}{\partial y \partial t} \varphi \right) \\ & + 2 \rho^{3/2} \left( \frac{\partial^2}{\partial y^2} \rho \right) \\ & - 4 \left( \frac{\partial}{\partial y} \left( \frac{1}{2} \frac{\sin(\varphi) \left( \frac{\partial}{\partial t} \rho \right) \rho + 2 \rho^2 \cos(\varphi) \left( \frac{\partial}{\partial t} \varphi \right) + \sqrt{\rho} \left( \frac{\partial}{\partial y} \rho \right)}{\rho^{3/2}} \right) \right) \rho^{5/2} \end{aligned}$$

(12)



$$\begin{aligned}
G &:= v_1 + \frac{v_{[]} \cdot u_2 - u_{[]} \cdot v_2 + u_{[]} \cdot u_3 + v_{[]} \cdot v_3}{u_{[]}^2 + v_{[]}^2}, \\
F &:= u_1 + \frac{u_{[]} u_2 + v_{[]} v_2 + u_{[]} v_3 - v_{[]} u_3}{u_{[]}^2 + v_{[]}^2} \\
G &:= v_1 + \frac{v_{[]} u_2 - u_{[]} v_2 + u_{[]} u_3 + v_{[]} v_3}{u_{[]}^2 + v_{[]}^2}
\end{aligned} \tag{16}$$

**J2** >  $A := \text{Matrix}\left(\left[\left[-\left(u_{[]}^2 + v_{[]}^2\right), 0, 0\right], [0, 1, 0], [0, 0, 1]\right]\right)$

$$A := \begin{bmatrix} -u_{[]}^2 - v_{[]}^2 & 0 & 0 \\ 0 & 1 & 0 \\ 0 & 0 & 1 \end{bmatrix} \tag{17}$$

**J2** >  $AA := \text{MatrixInverse}(A); Ad := \text{Adjoint}(A);$

$$\begin{aligned}
AA &:= \begin{bmatrix} -\frac{1}{u_{[]}^2 + v_{[]}^2} & 0 & 0 \\ 0 & 1 & 0 \\ 0 & 0 & 1 \end{bmatrix} \\
Ad &:= \begin{bmatrix} 1 & 0 & 0 \\ 0 & -u_{[]}^2 - v_{[]}^2 & 0 \\ 0 & 0 & -u_{[]}^2 - v_{[]}^2 \end{bmatrix}
\end{aligned} \tag{18}$$

Here A is the matrix of the linearized operator (bivector=metric with upper indices),  
AA - the inverse (metric, which we remember is defined only up to conformal rescaling)  
and AJ=AM=AdA the adjoint matrix (which we use as a representative for the conformal class)

>

>  $aA := [TotalDiff(A[1, 1], 1) + TotalDiff(A[1, 2], 2) + TotalDiff(A[1, 3], 3), TotalDiff(A[2, 1], 1) + TotalDiff(A[2, 2], 2) + TotalDiff(A[2, 3], 3), TotalDiff(A[3, 1], 1) + TotalDiff(A[3, 2], 2) + TotalDiff(A[3, 3], 3)] :$

>  $\omega := [AA[1, 1] \cdot aA[1] + AA[1, 2] \cdot aA[2] + AA[1, 3] \cdot aA[3], AA[2, 1] \cdot aA[1] + AA[2, 2] \cdot aA[2] + AA[2, 3] \cdot aA[3], AA[3, 1] \cdot aA[1] + AA[3, 2] \cdot aA[2] + AA[3, 3] \cdot aA[3]] :$

**J2** >  $2 \cdot \omega$

$$\left[ -\frac{2(-2u_{[]}u_1 - 2v_{[]}v_1)}{u_{[]}^2 + v_{[]}^2}, 0, 0 \right] \tag{19}$$

**J2** >

>  $DepVars := [u(t, x, y), v(t, x, y)] : AJ := \text{simplify}(\text{FromJet}(Ad, DepVars)) :$

>

>  $DGsetup([t, x, y], M) :$

>  $g := \text{evalDG}(AJ[1, 1] \cdot dt \& t \, dt + AJ[1, 2] \cdot dt \& t \, dx + AJ[1, 3] \cdot dt \& t \, dy + AJ[2, 1] \cdot dx \& t \, dt + AJ[2, 2] \cdot dx \& t \, dx + AJ[2, 3] \cdot dx \& t \, dy + AJ[3, 1] \cdot dy \& t \, dt + AJ[3, 2] \cdot dy \& t \, dx + AJ[3, 3] \cdot dy \& t \, dy) :$

```
> C := Connection(a000*dt &t D_t &t dt + a111*dx &t D_x &t dx + a222*dy &t D_y &t dy
+ a001*(dt &t D_t &t dx + dx &t D_t &t dt) + a002*(dt &t D_t &t dy + dy &t D_t
&t dt) + a102*(dx &t D_t &t dy + dy &t D_t &t dx) + a011*(dt &t D_x &t dx + dx
&t D_x &t dt) + a012*(dt &t D_x &t dy + dy &t D_x &t dt) + a112*(dx &t D_x &t dy
+ dy &t D_x &t dx) + a021*(dt &t D_y &t dx + dx &t D_y &t dt) + a022*(dt &t D_y
&t dy + dy &t D_y &t dt) + a122*(dx &t D_y &t dy + dy &t D_y &t dx) + a010*dt
&t D_x &t dt + a121*dx &t D_y &t dx + a202*dy &t D_t &t dy + a020*dt &t D_y &t dt
+ a101*dx &t D_t &t dx + a212*dy &t D_x &t dy) :
```

```
> TorsionTensor(C);
```

$0 \, dt \, D_t \, dt$

(20)

```
> U1 := simplify(2*FromJet(omega[1], DepVars)) :
```

```
U2 := simplify(2*FromJet(omega[2], DepVars)) :
```

```
U3 := simplify(2*FromJet(omega[3], DepVars)) :
```

Here we determine the connection C and define the covector U=omega. Later we will demonstrate that this choice of omega is the only natural

```
> Et := evalDG(DirectionalCovariantDerivative(D_t, g, C) - U1.g) :
```

```
Ex := evalDG(DirectionalCovariantDerivative(D_x, g, C) - U2.g) :
```

```
Ey := evalDG(DirectionalCovariantDerivative(D_y, g, C) - U3.g) :
```

```
> Eq000 := TensorInnerProduct(g, Et, dt &t dt) :
```

```
Eq001 := TensorInnerProduct(g, Et, dt &t dx) :
```

```
Eq002 := TensorInnerProduct(g, Et, dt &t dy) :
```

```
Eq011 := TensorInnerProduct(g, Et, dx &t dx) :
```

```
Eq012 := TensorInnerProduct(g, Et, dx &t dy) :
```

```
Eq022 := TensorInnerProduct(g, Et, dy &t dy) :
```

```
Eq100 := TensorInnerProduct(g, Ex, dt &t dt) :
```

```
Eq101 := TensorInnerProduct(g, Ex, dt &t dx) :
```

```
Eq102 := TensorInnerProduct(g, Ex, dt &t dy) :
```

```
Eq111 := TensorInnerProduct(g, Ex, dx &t dx) :
```

```
Eq112 := TensorInnerProduct(g, Ex, dx &t dy) :
```

```
Eq122 := TensorInnerProduct(g, Ex, dy &t dy) :
```

```
Eq200 := TensorInnerProduct(g, Ey, dt &t dt) :
```

```
Eq201 := TensorInnerProduct(g, Ey, dt &t dx) :
```

```
Eq202 := TensorInnerProduct(g, Ey, dt &t dy) :
```

```
Eq211 := TensorInnerProduct(g, Ey, dx &t dx) :
```

```
Eq212 := TensorInnerProduct(g, Ey, dx &t dy) :
```

```
Eq222 := TensorInnerProduct(g, Ey, dy &t dy) :
```

```
> sA := solve({Eq000=0, Eq001=0, Eq002=0, Eq011=0, Eq012=0, Eq022=0, Eq100=0,
Eq101=0, Eq102=0, Eq111=0, Eq112=0, Eq122=0, Eq200=0, Eq201=0, Eq202=0,
Eq211=0, Eq212=0, Eq222=0}, [a000, a001, a002, a010, a011, a012, a020, a021, a022,
a101, a102, a111, a112, a121, a122, a202, a212, a222]) :
```

```
> C1 := evalDG(subs({op(op(sA))}, C)) :
```

```
> evalDG(CovariantDerivative(g, C1) - g &t (U1*dt + U2*dx + U3*dy)) ;
```

$0 \, dt \, dt \, dt$

(21)

The connection C=C1 is uniquely determined by the 1st equation of EW property:  $D_C(g)=\omega \cdot g$ .  
Let us consider the main defining relation:  $\text{Ricci}(C)=V \cdot g$  (V is some scalar function).

```
> R1 := CurvatureTensor(C1) : Ric1 := RicciTensor(R1) : T1 := SymmetrizeIndices(Ric1, [1, 2],
"Symmetric") : Res := evalDG(T1 - V.g) :
```



### III. Next, let us treat the 2-component quasilinear system of PDEs - Hamiltonian systems of hydrodynamic type

> with(DifferentialGeometry) : with(Tensor) : with(Tools) : with(JetCalculus) :  
with(LinearAlgebra) : with(PDEtools, D\_Dx, declare, ToJet, FromJet) :

> declare( $h(u_{2,2}, u_{2,3}, u_{3,3})$ ) : subs( $\left[ h_r(r, s, t) = haha \right]$ , subs( $\left[ u_{2,2} = r, u_{2,3} = s, u_{3,3} = t, u_{1,2} = a, u_{1,3} = b \right]$ ,  $\frac{d^3}{du_{1,3}^3} f(u_{2,2}, u_{2,3}, u_{3,3}, u_{1,2}, u_{1,3})$ ))  
 $h(u_{2,2}, u_{2,3}, u_{3,3})$  will now be displayed as  $h$   
 $f_{b,b,b}$  (24)

> DGsetup([t, x, y], [v, w], J2) :

>  $F := v_1 + \text{TotalDiff}(\text{diff}(H(v_{[]}, w_{[]}), v_{[]}), 3);$

$G := w_2 + \text{TotalDiff}(\text{diff}(H(v_{[]}, w_{[]}), w_{[]}), 3);$

$$F := v_1 + H_{v_{[]}, v_{[]}} v_3 + H_{v_{[]}, w_{[]}} w_3$$

$$G := w_2 + H_{v_{[]}, w_{[]}} v_3 + H_{w_{[]}, w_{[]}} w_3$$

(25)

>  $DR := (\text{diff}(F, v_1) \cdot p_1 + \text{diff}(F, v_2) \cdot p_2 + \text{diff}(F, v_3) \cdot p_3) \cdot (\text{diff}(G, w_1) \cdot p_1 + \text{diff}(G, w_2) \cdot p_2 + \text{diff}(G, w_3) \cdot p_3) - (\text{diff}(F, w_1) \cdot p_1 + \text{diff}(F, w_2) \cdot p_2 + \text{diff}(F, w_3) \cdot p_3) \cdot (\text{diff}(G, v_1) \cdot p_1 + \text{diff}(G, v_2) \cdot p_2 + \text{diff}(G, v_3) \cdot p_3)$

$$DR := (p_1 + H_{v_{[]}, v_{[]}} p_3) (p_2 + H_{w_{[]}, w_{[]}} p_3) - H_{v_{[]}, w_{[]}}^2 p_3^2$$

(26)

>  $A := 2 \cdot \text{Matrix}\left(\left[\left[\frac{1}{2} \text{diff}(DR, p_1, p_1), \frac{1}{2} \text{diff}(DR, p_1, p_2), \frac{1}{2} \text{diff}(DR, p_1, p_3)\right], \left[\frac{1}{2} \text{diff}(DR, p_1, p_2), \frac{1}{2} \text{diff}(DR, p_2, p_2), \frac{1}{2} \text{diff}(DR, p_2, p_3)\right], \left[\frac{1}{2} \text{diff}(DR, p_1, p_3), \frac{1}{2} \text{diff}(DR, p_2, p_3), \frac{1}{2} \text{diff}(DR, p_3, p_3)\right]\right]\right)$

$$A := \begin{bmatrix} 0 & 1 & H_{w_{[]}, w_{[]}} \\ 1 & 0 & H_{v_{[]}, v_{[]}} \\ H_{w_{[]}, w_{[]}} & H_{v_{[]}, v_{[]}} & 2 H_{v_{[]}, v_{[]}} H_{w_{[]}, w_{[]}} - 2 H_{v_{[]}, w_{[]}}^2 \end{bmatrix}$$

(27)

**J2** >  $\text{det} := \text{simplify}(\text{Determinant}(A)); \text{AA} := \text{expand}(\text{MatrixInverse}(A));$   
 $\text{AM} := \text{simplify}(\text{Determinant}(A) \cdot \text{AA}); \text{AdA} := \text{Adjoint}(A);$

$$\text{det} := 2 H_{v_{[]}, w_{[]}}^2$$



$$\begin{aligned}
AM &:= \begin{bmatrix} -H_{v[\cdot], v[\cdot]}^2 & -H_{v[\cdot], v[\cdot]} H_{w[\cdot], w[\cdot]} + 2 H_{v[\cdot], w[\cdot]}^2 & H_{v[\cdot], v[\cdot]} \\ -H_{v[\cdot], v[\cdot]} H_{w[\cdot], w[\cdot]} + 2 H_{v[\cdot], w[\cdot]}^2 & -H_{w[\cdot], w[\cdot]}^2 & H_{w[\cdot], w[\cdot]} \\ H_{v[\cdot], v[\cdot]} & H_{w[\cdot], w[\cdot]} & -1 \end{bmatrix} \\
AdA &:= \begin{bmatrix} -H_{v[\cdot], v[\cdot]}^2 & -H_{v[\cdot], v[\cdot]} H_{w[\cdot], w[\cdot]} + 2 H_{v[\cdot], w[\cdot]}^2 & H_{v[\cdot], v[\cdot]} \\ -H_{v[\cdot], v[\cdot]} H_{w[\cdot], w[\cdot]} + 2 H_{v[\cdot], w[\cdot]}^2 & -H_{w[\cdot], w[\cdot]}^2 & H_{w[\cdot], w[\cdot]} \\ H_{v[\cdot], v[\cdot]} & H_{w[\cdot], w[\cdot]} & -1 \end{bmatrix}
\end{aligned} \tag{28}$$

Here A is the matrix of the linearized operator (bivector=metric with upper indices),  
AA - the inverse (metric, which we remember is defined only up to conformal rescaling)  
and AJ=AM=AdA the adjoint matrix (which we use as a representative for the conformal class)

>

>  $aA := [TotalDiff(A[1, 1], 1) + TotalDiff(A[1, 2], 2) + TotalDiff(A[1, 3], 3), TotalDiff(A[2, 1], 1) + TotalDiff(A[2, 2], 2) + TotalDiff(A[2, 3], 3), TotalDiff(A[3, 1], 1) + TotalDiff(A[3, 2], 2) + TotalDiff(A[3, 3], 3)] :$

>  $\omega := 2 \cdot [AA[1, 1] \cdot aA[1] + AA[1, 2] \cdot aA[2] + AA[1, 3] \cdot aA[3], AA[2, 1] \cdot aA[1] + AA[2, 2] \cdot aA[2] + AA[2, 3] \cdot aA[3], AA[3, 1] \cdot aA[1] + AA[3, 2] \cdot aA[2] + AA[3, 3] \cdot aA[3]] :$

**J2** > *simplify*( $\omega$ )

$$\begin{aligned}
& \left[ \frac{1}{H_{v[\cdot], w[\cdot]}^2} \left( H_{v[\cdot], v[\cdot]}^2 H_{v[\cdot], w[\cdot], w[\cdot]} v_3 + H_{v[\cdot], v[\cdot]}^2 H_{w[\cdot], w[\cdot], w[\cdot]} w_3 + H_{v[\cdot], v[\cdot]} H_{w[\cdot], w[\cdot]} H_{v[\cdot], v[\cdot], v[\cdot]} v_3 \right. \right. \\
& + H_{v[\cdot], v[\cdot]} H_{w[\cdot], w[\cdot]} H_{v[\cdot], v[\cdot], w[\cdot]} w_3 + 2 H_{v[\cdot], w[\cdot]}^2 H_{v[\cdot], v[\cdot], v[\cdot]} v_3 + 2 H_{v[\cdot], w[\cdot]}^2 H_{v[\cdot], v[\cdot], w[\cdot]} w_3 \\
& + H_{v[\cdot], v[\cdot]} H_{v[\cdot], w[\cdot], w[\cdot]} v_1 + H_{v[\cdot], v[\cdot]} H_{w[\cdot], w[\cdot], w[\cdot]} w_1 + H_{v[\cdot], v[\cdot]} H_{v[\cdot], v[\cdot], v[\cdot]} v_2 \\
& + H_{v[\cdot], v[\cdot]} H_{v[\cdot], v[\cdot], w[\cdot]} w_2 - 4 H_{v[\cdot], v[\cdot]} v_3 H_{v[\cdot], w[\cdot]} H_{v[\cdot], v[\cdot], w[\cdot]} \\
& \left. \left. - 4 H_{v[\cdot], v[\cdot]} w_3 H_{v[\cdot], w[\cdot]} H_{v[\cdot], w[\cdot], w[\cdot]} \right), \frac{1}{H_{v[\cdot], w[\cdot]}^2} \left( H_{v[\cdot], v[\cdot]} H_{w[\cdot], w[\cdot]} H_{v[\cdot], w[\cdot], w[\cdot]} v_3 \right. \right. \\
& \left. \left. - 4 H_{v[\cdot], v[\cdot]} w_3 H_{v[\cdot], w[\cdot]} H_{v[\cdot], w[\cdot], w[\cdot]} \right) \right]
\end{aligned} \tag{29}$$

$$\begin{aligned}
& + H_{v[], v[]} H_{w[], w[]} H_{w[], w[], w[]} w_3 + 2 H_{v[], w[]}^2 H_{v[], w[], w[]} v_3 + 2 H_{v[], w[]}^2 H_{w[], w[], w[]} w_3 \\
& + H_{w[], w[]}^2 H_{v[], v[], v[]} v_3 + H_{w[], w[]}^2 H_{v[], v[], w[]} w_3 + H_{w[], w[]} H_{v[], w[], w[]} v_1 \\
& + H_{w[], w[]} H_{w[], w[], w[]} w_1 + H_{w[], w[]} H_{v[], v[], v[]} v_2 + H_{w[], w[]} H_{v[], v[], w[]} w_2 \\
& - 4 H_{w[], w[]} v_3 H_{v[], w[]} H_{v[], v[], w[]} - 4 H_{w[], w[]} w_3 H_{v[], w[]} H_{v[], w[], w[]} \Big), \frac{1}{H_{v[], w[]}^2} \Big( \\
& - v_3 H_{v[], v[]} H_{v[], w[], w[]} - w_3 H_{v[], v[]} H_{w[], w[], w[]} - v_3 H_{v[], v[], v[]} H_{w[], w[]} \\
& - w_3 H_{v[], v[], w[]} H_{w[], w[]} - H_{v[], w[], w[]} v_1 - H_{w[], w[], w[]} w_1 - H_{v[], v[], v[]} v_2 \\
& - H_{v[], v[], w[]} w_2 + 4 v_3 H_{v[], w[]} H_{v[], v[], w[]} + 4 w_3 H_{v[], w[]} H_{v[], w[], w[]} \Big) \Big]
\end{aligned}$$

**J2** > *simplify*(*subs*([ $v_{[]} = v, w_{[]} = w$ ],  $\omega$ ))

$$\begin{aligned}
& \left[ \frac{1}{H_{v, w}^2} \left( H_{v, v}^2 H_{v, w, w} v_3 + H_{v, v}^2 H_{w, w, w} w_3 + H_{v, v} H_{w, w} H_{v, v, v} v_3 + H_{v, v} H_{w, w} H_{v, v, w} w_3 + 2 \right. \right. \\
& H_{v, w}^2 H_{v, v, v} v_3 + 2 H_{v, w}^2 H_{v, v, w} w_3 + H_{v, v} H_{v, w, w} v_1 + H_{v, v} H_{w, w, w} w_1 + H_{v, v} H_{v, v, v} v_2 \\
& + H_{v, v} H_{v, v, w} w_2 - 4 H_{v, v} v_3 H_{v, w} H_{v, v, w} - 4 H_{v, v} w_3 H_{v, w} H_{v, w, w} \Big), \\
& \frac{1}{H_{v, w}^2} \left( H_{v, v} H_{w, w} H_{v, w, w} v_3 + H_{v, v} H_{w, w} H_{w, w, w} w_3 + 2 H_{v, w}^2 H_{v, w, w} v_3 + 2 H_{v, w}^2 H_{w, w, w} w_3 \right. \\
& + H_{w, w}^2 H_{v, v, v} v_3 + H_{w, w}^2 H_{v, v, w} w_3 + H_{w, w} H_{v, w, w} v_1 + H_{w, w} H_{w, w, w} w_1 + H_{w, w} H_{v, v, v} v_2 \\
& + H_{w, w} H_{v, v, w} w_2 - 4 H_{w, w} v_3 H_{v, w} H_{v, v, w} - 4 H_{w, w} w_3 H_{v, w} H_{v, w, w} \Big), \\
& - \frac{1}{H_{v, w}^2} \left( v_3 H_{v, v} H_{v, w, w} + w_3 H_{v, v} H_{w, w, w} + v_3 H_{v, v, v} H_{w, w} + w_3 H_{v, v, w} H_{w, w} + H_{v, w, w} v_1 \right. \\
& \left. \left. + H_{w, w, w} w_1 + H_{v, v, v} v_2 + H_{v, v, w} w_2 - 4 v_3 H_{v, w} H_{v, v, w} - 4 w_3 H_{v, w} H_{v, w, w} \right) \right]
\end{aligned} \tag{30}$$

**J2** > *simplify*(*subs*([ $v_{[]} = v, w_{[]} = w$ ], *subs*(*solve*([ $F=0, G=0$ ], { $v_1, w_2$ }),  $\omega$ )))

$$\begin{aligned}
& \left[ \frac{1}{H_{v,w}^2} \left( H_{v,v}^2 H_{w,w,w} w_3 + H_{v,v} H_{w,w} H_{v,v,v} v_3 + 2 H_{v,w}^2 H_{v,v,v} v_3 + 2 H_{v,w}^2 H_{v,v,w} w_3 \right. \right. \\
& \quad \left. \left. - 5 H_{v,v} w_3 H_{v,w} H_{v,w,w} + H_{v,v} H_{w,w,w} w_1 + H_{v,v} H_{v,v,v} v_2 - 5 H_{v,v} v_3 H_{v,w} H_{v,v,w} \right), \right. \\
& \quad \frac{1}{H_{v,w}^2} \left( H_{v,v} H_{w,w} H_{w,w,w} w_3 + 2 H_{v,w}^2 H_{v,w,w} v_3 + 2 H_{v,w}^2 H_{w,w,w} w_3 + H_{w,w}^2 H_{v,v,v} v_3 \right. \\
& \quad \left. - 5 H_{w,w} w_3 H_{v,w} H_{v,w,w} + H_{w,w} H_{w,w,w} w_1 + H_{w,w} H_{v,v,v} v_2 \right. \\
& \quad \left. - 5 H_{w,w} v_3 H_{v,w} H_{v,v,w} \right), - \frac{1}{H_{v,w}^2} \left( w_3 H_{v,v} H_{w,w,w} + v_3 H_{v,v,v} H_{w,w} - 5 w_3 H_{v,w} H_{v,w,w} \right. \\
& \quad \left. + H_{w,w,w} w_1 + H_{v,v,v} v_2 - 5 v_3 H_{v,w} H_{v,v,w} \right) \left. \right]
\end{aligned} \tag{31}$$

$\text{DepVars} := [v(t, x, y), w(t, x, y)] : AJ := \text{simplify}(\text{FromJet}(\text{AdA}, \text{DepVars})) :$

$\text{DGsetup}([t, x, y], M) :$

$g := \text{evalDG}(AJ[1, 1] \cdot dt \& dt + AJ[1, 2] \cdot dt \& dx + AJ[1, 3] \cdot dt \& dy + AJ[2, 1] \cdot dx \& dt$   
 $+ AJ[2, 2] \cdot dx \& dx + AJ[2, 3] \cdot dx \& dy + AJ[3, 1] \cdot dy \& dt + AJ[3, 2] \cdot dy \& dx$   
 $+ AJ[3, 3] \cdot dy \& dy) :$

$C := \text{Connection}(a000 \cdot dt \& D\_t \& dt + a111 \cdot dx \& D\_x \& dx + a222 \cdot dy \& D\_y \& dy$   
 $+ a001 \cdot (dt \& D\_t \& dx + dx \& D\_t \& dt) + a002 \cdot (dt \& D\_t \& dy + dy \& D\_t \& dt)$   
 $+ a102 \cdot (dx \& D\_t \& dy + dy \& D\_t \& dx) + a011 \cdot (dt \& D\_x \& dx + dx \& D\_x \& dt)$   
 $+ a012 \cdot (dt \& D\_x \& dy + dy \& D\_x \& dt) + a112 \cdot (dx \& D\_x \& dy + dy \& D\_x \& dx)$   
 $+ a021 \cdot (dt \& D\_y \& dx + dx \& D\_y \& dt) + a022 \cdot (dt \& D\_y \& dy + dy \& D\_y \& dt)$   
 $+ a122 \cdot (dx \& D\_y \& dy + dy \& D\_y \& dx) + a010 \cdot dt \& D\_x \& dt + a121 \cdot dx \& D\_y \& dx + a202 \cdot dy \& D\_t \& dy + a020 \cdot dt \& D\_y \& dt$   
 $+ a101 \cdot dx \& D\_t \& dx + a212 \cdot dy \& D\_x \& dy) :$

$\text{TorsionTensor}(C);$

$0 \ dt \ D\_t \ dt$

(32)

$U1 := \text{simplify}(\text{FromJet}(\omega[1], \text{DepVars})) :$

$U2 := \text{simplify}(\text{FromJet}(\omega[2], \text{DepVars})) :$

$U3 := \text{simplify}(\text{FromJet}(\omega[3], \text{DepVars})) :$

Here we determine the connection C and define the covector U=omega. Later we will demonstrate that this choice of omega is the only natural

$Et := \text{evalDG}(\text{DirectionalCovariantDerivative}(D\_t, g, C) - U1 \cdot g) :$

$Ex := \text{evalDG}(\text{DirectionalCovariantDerivative}(D\_x, g, C) - U2 \cdot g) :$

$Ey := \text{evalDG}(\text{DirectionalCovariantDerivative}(D\_y, g, C) - U3 \cdot g) :$

$Eq000 := \text{TensorInnerProduct}(g, Et, dt \& dt) :$

$Eq001 := \text{TensorInnerProduct}(g, Et, dt \& dx) :$

$Eq002 := \text{TensorInnerProduct}(g, Et, dt \& dy) :$

$Eq011 := \text{TensorInnerProduct}(g, Et, dx \& dx) :$

$Eq012 := \text{TensorInnerProduct}(g, Et, dx \& dy) :$

```

Eq022 := TensorInnerProduct(g, Et, dy &t dy) :
Eq100 := TensorInnerProduct(g, Ex, dt &t dt) :
Eq101 := TensorInnerProduct(g, Ex, dt &t dx) :
Eq102 := TensorInnerProduct(g, Ex, dt &t dy) :
Eq111 := TensorInnerProduct(g, Ex, dx &t dx) :
Eq112 := TensorInnerProduct(g, Ex, dx &t dy) :
Eq122 := TensorInnerProduct(g, Ex, dy &t dy) :
Eq200 := TensorInnerProduct(g, Ey, dt &t dt) :
Eq201 := TensorInnerProduct(g, Ey, dt &t dx) :
Eq202 := TensorInnerProduct(g, Ey, dt &t dy) :
Eq211 := TensorInnerProduct(g, Ey, dx &t dx) :
Eq212 := TensorInnerProduct(g, Ey, dx &t dy) :
Eq222 := TensorInnerProduct(g, Ey, dy &t dy) :

```

```

> sA := solve( {Eq000=0, Eq001=0, Eq002=0, Eq011=0, Eq012=0, Eq022=0, Eq100=0,
Eq101=0, Eq102=0, Eq111=0, Eq112=0, Eq122=0, Eq200=0, Eq201=0, Eq202=0,
Eq211=0, Eq212=0, Eq222=0}, [a000, a001, a002, a010, a011, a012, a020, a021, a022,
a101, a102, a111, a112, a121, a122, a202, a212, a222] ) :

```

```

> C1 := evalDG( subs( {op(op(sA))}, C) ) :

```

```

> evalDG( CovariantDerivative(g, C1) - g &t (U1·dt + U2·dx + U3·dy) );
0 dt dt dt

```

(33)

The connection  $C=C1$  is uniquely determined by the 1st equation of EW property:  $D_C(g)=\omega g$ .  
Let us consider the main defining relation:  $Ricci(C)=V*g$  ( $V$  is some scalar function).

```

> R1 := CurvatureTensor(C1) : Ric1 := RicciTensor(R1) : T1 := SymmetrizeIndices(Ric1, [1, 2],
"Symmetric") : Res := evalDG(T1 - V·g) :
> NEQt1 := ContractIndices(Res, D_t &t D_t, [[1, 1], [2, 2]]) : NEQt1x := ContractIndices(Res,
D_t &t D_x, [[1, 1], [2, 2]]) :
NEQt1y := ContractIndices(Res, D_t &t D_y, [[1, 1], [2, 2]]) : NEQt1xx := ContractIndices(Res,
D_x &t D_x, [[1, 1], [2, 2]]) :
NEQt1xy := ContractIndices(Res, D_x &t D_y, [[1, 1], [2, 2]]) : NEQt1yy := ContractIndices(Res,
D_y &t D_y, [[1, 1], [2, 2]]) :

```

```

> DGsetup([t, x, y], [v, w], J2, 4) :

```

```

> de := DifferentialEquationData([F, G], [v1, w2])

```

```

de := [ {v1, w2}, [v1 + H_v, v v3 + H_v, w w3, w2 + H_v, w v3 + H_w, w w3] ]

```

(34)

```

> de2 := Prolong(de, 2) : deTRA := Transformation(de2) :

```

```

> Eq0 := Pullback(deTRA, ToJet(NEQt1, DepVars, notation = jetnumbers)) :

```

```

> VS := solve(Eq0, V) :

```

```

> Eq1 := numer(subs(V=VS, Pullback(deTRA, ToJet(NEQt1x, DepVars, notation
=jetnumbers)))) :

```

```

Eq2 := numer(subs(V=VS, Pullback(deTRA, ToJet(NEQt1y, DepVars, notation
=jetnumbers)))) :

```

```

Eq3 := numer(subs(V=VS, Pullback(deTRA, ToJet(NEQt1xx, DepVars, notation
=jetnumbers)))) :

```

```

Eq4 := numer(subs(V=VS, Pullback(deTRA, ToJet(NEQt1xy, DepVars, notation
=jetnumbers)))) :

```

```

Eq5 := numer(subs(V=VS, Pullback(deTRA, ToJet(NEQt1yy, DepVars, notation
=jetnumbers)))) :

```

The highest (2nd order) derivatives have zero coefficients, which indicates that the universal formula for the covector omega holds.

So let us consider the highest derivatives, which are of order 1 and are quadratic in 1-jets

**J2 >**  $Res1 := \text{simplify}([ \text{diff}(Eq1, v_2, w_1), \text{diff}(Eq1, v_3, v_3), \text{diff}(Eq1, v_3, w_3), \text{diff}(Eq1, w_3, w_3), \text{diff}(Eq2, v_2, w_1), \text{diff}(Eq2, v_3, v_3), \text{diff}(Eq2, v_3, w_3), \text{diff}(Eq2, w_3, w_3), \text{diff}(Eq3, v_2, w_1), \text{diff}(Eq3, v_3, v_3), \text{diff}(Eq3, v_3, w_3), \text{diff}(Eq3, w_3, w_3), \text{diff}(Eq4, v_2, w_1), \text{diff}(Eq4, v_3, v_3), \text{diff}(Eq4, v_3, w_3), \text{diff}(Eq4, w_3, w_3), \text{diff}(Eq5, v_2, w_1), \text{diff}(Eq5, v_3, v_3), \text{diff}(Eq5, v_3, w_3), \text{diff}(Eq5, w_3, w_3) ])$  :

**J2 >**  $DeVars := [H(v[], w[])] : \text{simplify}(\text{ToJet}(Res1[1], DeVars))$

$$\begin{aligned} H_{v[], w[]} & \left( H_{v[], w[]}^2 H_{v[], v[]}^2 H_{v[], w[], w[], w[]} - 4 H_{v[], w[]}^2 H_{v[], v[], w[], w[]} H_{v[], v[]} - 8 \right. \\ & H_{v[], w[]}^2 H_{v[], v[], v[]} H_{v[], w[], w[]} - 2 H_{v[], v[]}^2 H_{w[], w[], w[]} H_{v[], v[], w[]} + 4 \\ & H_{v[], w[]}^3 H_{v[], v[], v[], w[]} + 2 H_{w[], w[]} H_{v[], v[], v[]} H_{v[], w[], w[]} H_{v[], v[]} \\ & + 4 H_{v[], w[]} H_{v[], v[], w[]} H_{v[], w[], w[]} H_{v[], v[]} + 4 H_{w[], w[], w[]} H_{v[], w[]} H_{v[], v[], v[]} H_{v[], v[]} \\ & \left. - H_{v[], w[]} H_{w[], w[]} H_{v[], v[], v[], w[]} H_{v[], v[]} \right) \end{aligned} \quad (35)$$

**J2 >**  $ReS1 := \text{simplify}(\text{FromJet}(Res1, DepVars))$  :

**J2 >**  $SolV := \text{solve}(ReS1, [D_{1,1,1,1}(H)(v(t, x, y), w(t, x, y)), D_{1,1,1,2}(H)(v(t, x, y), w(t, x, y)), D_{1,1,2,2}(H)(v(t, x, y), w(t, x, y)), D_{1,2,2,2}(H)(v(t, x, y), w(t, x, y)), D_{2,2,2,2}(H)(v(t, x, y), w(t, x, y))][1])$  :

**J2 >**  $SolVt := \text{ToJet}(\text{solve}(ReS1, [D_{1,1,1,1}(H)(v(t, x, y), w(t, x, y)), D_{1,1,1,2}(H)(v(t, x, y), w(t, x, y)), D_{1,1,2,2}(H)(v(t, x, y), w(t, x, y)), D_{1,2,2,2}(H)(v(t, x, y), w(t, x, y)), D_{2,2,2,2}(H)(v(t, x, y), w(t, x, y))][1]), DepVars)[1])$

$$\begin{aligned} SolVt := & \left[ H_{v, v, v, v} = \frac{2 H_{v, v, w} H_{v, v, v}}{H_{v, w}}, H_{v, v, v, w} = \frac{2 H_{v, v, v} H_{v, w, w}}{H_{v, w}}, H_{v, v, w, w} \right. \\ & = \frac{H_{v, v, v} H_{w, w, w} + H_{v, w, w} H_{v, v, w}}{H_{v, w}}, H_{v, w, w, w} = \frac{2 H_{w, w, w} H_{v, v, w}}{H_{v, w}}, H_{w, w, w, w} \\ & \left. = \frac{2 H_{v, w, w} H_{w, w, w}}{H_{v, w}} \right] \end{aligned} \quad (36)$$

**J2 >**

**J2 >**  $\text{simplify}(\text{subs}(SolV, \text{FromJet}([Eq1, Eq2, Eq3, Eq4, Eq5], DepVars)))$

$$[0, 0, 0, 0, 0]$$

(37)

Perfect! We get that integrability condition precisely characterizes those Hamiltonian 2-component systems of hydrodynamic type that possess EW property

>  
>  
>  
>  
>

> restart :

IV. Now consider the 2-component generalization of BF, proposed by Bogdanov

> with(DifferentialGeometry) : with(Tensor) : with(Tools) : with(JetCalculus) :  
with(LinearAlgebra) : with(PDEtools, D\_Dx, declare, ToJet, FromJet) :

> declare( $h(u_{2,2}, u_{2,3}, u_{3,3})$ ) : subs( $\left[ h_r(r, s, t) = haha \right]$ , subs( $\left[ u_{2,2} = r, u_{2,3} = s, u_{3,3} = t, u_{1,2} = a, u_{1,3} = b \right]$ ,  $\frac{d^3}{du_{1,3}^3} f(u_{2,2}, u_{2,3}, u_{3,3}, u_{1,2}, u_{1,3})$ ))

$h(u_{2,2}, u_{2,3}, u_{3,3})$  will now be displayed as  $h$

$f_{b,b,b}$

(38)

> DGsetup([t, x, y], [ $\phi, m$ ], J2) :

>  $F := \text{TotalDiff}(\exp(-\phi(t, x, y)), [1, 1]) - \text{diff}(m(t, x, y), t) \cdot \text{diff}(\phi(t, x, y), x, y) + \text{diff}(m(t, x, y), x) \cdot \text{diff}(\phi(t, x, y), t, y)$ ;

$G := \text{diff}(m(t, x, y), t, t) \cdot \exp(-\phi(t, x, y)) - \text{diff}(m(t, x, y), x) \cdot \text{diff}(m(t, x, y), t, y) + \text{diff}(m(t, x, y), t) \cdot \text{diff}(m(t, x, y), x, y)$ ;

$F := -\phi_{t,t} e^{-\phi(t, x, y)} + \phi_t^2 e^{-\phi(t, x, y)} - m_t \phi_{x,y} + m_x \phi_{t,y}$

$G := m_{t,t} e^{-\phi(t, x, y)} - m_x m_{t,y} + m_t m_{x,y}$

(39)

> DepVars := [ $\phi(t, x, y), m(t, x, y)$ ] : AJ := simplify(ToJet([F, G], DepVars, jetnotation = jetnumbers))

$AJ := \left[ -\phi_{1,1} e^{-\phi_{[]}} + \phi_1^2 e^{-\phi_{[]}} - m_1 \phi_{2,3} + m_2 \phi_{1,3}, m_{1,1} e^{-\phi_{[]}} - m_2 m_{1,3} + m_1 m_{2,3} \right]$

(40)

>  $F := -\text{TotalDiff}(\exp(-\phi_{[]}), [1, 1]) - m_2 \cdot \phi_{1,3} + m_1 \cdot \phi_{2,3}$ ;

$G := m_{1,1} \cdot \exp(-\phi_{[]}) - m_2 \cdot m_{1,3} + m_1 \cdot m_{2,3}$ ;

$F := -\phi_1^2 e^{-\phi_{[]}} + \phi_{1,1} e^{-\phi_{[]}} - m_2 \phi_{1,3} + m_1 \phi_{2,3}$

$G := m_{1,1} e^{-\phi_{[]}} - m_2 m_{1,3} + m_1 m_{2,3}$

(41)

>  $A := 2 \cdot \text{Matrix}\left(\left[\left[\text{diff}(F, \phi[1, 1]), \frac{1}{2} \text{diff}(F, \phi[1, 2]), \frac{1}{2} \text{diff}(F, \phi[1, 3])\right], \left[\frac{1}{2} \text{diff}(F, \phi[1, 2]), \text{diff}(F, \phi[2, 2]), \frac{1}{2} \text{diff}(F, \phi[2, 3])\right], \left[\frac{1}{2} \text{diff}(F, \phi[1, 3]), \frac{1}{2} \text{diff}(F, \phi[2, 3]), \text{diff}(F, \phi[3, 3])\right]\right]\right)$

$$A := \begin{bmatrix} 2 e^{-\phi_{[]}} & 0 & -m_2 \\ 0 & 0 & m_1 \\ -m_2 & m_1 & 0 \end{bmatrix} \quad (42)$$

**>**  $A := 2 \cdot \text{Matrix} \left( \left[ \left[ \text{diff}(G, m[1, 1]), \frac{1}{2} \text{diff}(G, m[1, 2]), \frac{1}{2} \text{diff}(G, m[1, 3]) \right], \left[ \frac{1}{2} \text{diff}(G, m[1, 2]), \text{diff}(G, m[2, 2]), \frac{1}{2} \text{diff}(G, m[2, 3]) \right], \left[ \frac{1}{2} \text{diff}(G, m[1, 3]), \frac{1}{2} \text{diff}(G, m[2, 3]), \text{diff}(G, m[3, 3]) \right] \right] \right)$

$$A := \begin{bmatrix} 2 e^{-\phi_{[]}} & 0 & -m_2 \\ 0 & 0 & m_1 \\ -m_2 & m_1 & 0 \end{bmatrix} \quad (43)$$

**J2 >**  $\text{det} := \text{simplify}(\text{Determinant}(A)); \text{AA} := \text{expand}(\text{MatrixInverse}(A));$   
 $\text{AM} := \text{simplify}(\text{Determinant}(A) \cdot \text{AA}); \text{AdA} := \text{Adjoint}(A);$

$$\begin{aligned} \text{det} &:= -2 e^{-\phi_{[]}} m_1^2 \\ \text{AM} &:= \begin{bmatrix} -m_1^2 & -m_1 m_2 & 0 \\ -m_1 m_2 & -m_2^2 & -2 e^{-\phi_{[]}} m_1 \\ 0 & -2 e^{-\phi_{[]}} m_1 & 0 \end{bmatrix} \\ \text{AdA} &:= \begin{bmatrix} -m_1^2 & -m_1 m_2 & 0 \\ -m_1 m_2 & -m_2^2 & -2 e^{-\phi_{[]}} m_1 \\ 0 & -2 e^{-\phi_{[]}} m_1 & 0 \end{bmatrix} \end{aligned} \quad (44)$$

Here A is the matrix of the linearized operator (bivector=metric with upper indices),  
AA - the inverse (metric, which we remember is defined only up to conformal rescaling)  
and AJ=AM=AdA the adjoint matrix (which we use as a representative for the conformal class)

**>**  
**>**  $aA := [\text{TotalDiff}(A[1, 1], 1) + \text{TotalDiff}(A[1, 2], 2) + \text{TotalDiff}(A[1, 3], 3), \text{TotalDiff}(A[2, 1], 1) + \text{TotalDiff}(A[2, 2], 2) + \text{TotalDiff}(A[2, 3], 3), \text{TotalDiff}(A[3, 1], 1) + \text{TotalDiff}(A[3, 2], 2) + \text{TotalDiff}(A[3, 3], 3)]:$

**>**  $\omega := 2 \cdot [AA[1, 1] \cdot aA[1] + AA[1, 2] \cdot aA[2] + AA[1, 3] \cdot aA[3], AA[2, 1] \cdot aA[1] + AA[2, 2] \cdot aA[2] + AA[2, 3] \cdot aA[3], AA[3, 1] \cdot aA[1] + AA[3, 2] \cdot aA[2] + AA[3, 3] \cdot aA[3]]:$

**M >**  $\text{simplify}(\omega)$

$$\left[ -\frac{e^{\phi_{[1]}} \left( 2 m_1 e^{-\phi_{[1]}} \phi_1 + m_1 m_{2,3} - m_2 m_{1,3} \right)}{m_1}, -\frac{m_2 e^{\phi_{[1]}} \left( 2 m_1 e^{-\phi_{[1]}} \phi_1 + m_1 m_{2,3} - m_2 m_{1,3} \right)}{m_1^2}, \right. \\ \left. \frac{2 m_{1,3}}{m_1} \right] \quad (45)$$

the Alternatively we can use the following form omega, but then g should be changed to ...

**J2** > simplify( $\omega + 2 \cdot [\phi_1, \phi_2, \phi_3]$ )

$$\left[ -\frac{e^{\phi_{[1]}} (m_1 m_{2,3} - m_2 m_{1,3})}{m_1}, -\frac{-2 \phi_2 m_1^2 + 2 m_2 m_1 \phi_1 + m_2 e^{\phi_{[1]}} m_1 m_{2,3} - m_2^2 e^{\phi_{[1]}} m_{1,3}}{m_1^2}, \right. \\ \left. \frac{2 (\phi_3 m_1 + m_{1,3})}{m_1} \right] \quad (46)$$

>

> DepVars :=  $[\phi(t, x, y), m(t, x, y)]$  : AJ := simplify(FromJet(AdA, DepVars)) :

>

> DGsetup([t, x, y], M) :

> g := evalDG(AJ[1, 1]·dt &t dt + AJ[1, 2]·dt &t dx + AJ[1, 3]·dt &t dy + AJ[2, 1]·dx &t dt + AJ[2, 2]·dx &t dx + AJ[2, 3]·dx &t dy + AJ[3, 1]·dy &t dt + AJ[3, 2]·dy &t dx + AJ[3, 3]·dy &t dy)

$$g := -m_t^2 dt dt - m_t m_x dt dx - m_t m_x dx dt - m_x^2 dx dx - 2 e^{-\phi(t, x, y)} m_t dx dy - 2 e^{-\phi(t, x, y)} m_t dy dx \quad (47)$$

(prolongation of the above pink remark) ... g has to be changed to the following metric.

**M** > DGsimplify(evalDG(-exp(2  $\phi(t, x, y)$ ) · g))

$$e^{2\phi(t, x, y)} m_t^2 dt dt + e^{2\phi(t, x, y)} m_t m_x dt dx + e^{2\phi(t, x, y)} m_t m_x dx dt + e^{2\phi(t, x, y)} m_x^2 dx dx \\ + 2 m_t e^{\phi(t, x, y)} dx dy + 2 m_t e^{\phi(t, x, y)} dy dx \quad (48)$$

> C := Connection(a000\*dt &t D\_t &t dt + a111\*dx &t D\_x &t dx + a222\*dy &t D\_y &t dy + a001\*(dt &t D\_t &t dx + dx &t D\_t &t dt) + a002\*(dt &t D\_t &t dy + dy &t D\_t &t dt) + a102\*(dx &t D\_t &t dy + dy &t D\_t &t dx) + a011\*(dt &t D\_x &t dx + dx &t D\_x &t dt) + a012\*(dt &t D\_x &t dy + dy &t D\_x &t dt) + a112\*(dx &t D\_x &t dy + dy &t D\_x &t dx) + a021\*(dt &t D\_y &t dx + dx &t D\_y &t dt) + a022\*(dt &t D\_y &t dy + dy &t D\_y &t dt) + a122\*(dx &t D\_y &t dy + dy &t D\_y &t dx) + a010\*dt &t D\_x &t dt + a121\*dx &t D\_y &t dx + a202\*dy &t D\_t &t dy + a020\*dt &t D\_y &t dt + a101\*dx &t D\_t &t dx + a212\*dy &t D\_x &t dy) :

> TorsionTensor(C);

$$0 dt D_t dt \quad (49)$$

> U1 := simplify(FromJet( $\omega[1]$ , DepVars)) :

U2 := simplify(FromJet( $\omega[2]$ , DepVars)) :

U3 := simplify(FromJet( $\omega[3]$ , DepVars)) :

Here we determine the connection C and define the covector U=omega. Later we will demonstrate that this choice of omega is the only natural



```

> Et := evalDG(DirectionalCovariantDerivative(D_t, g, C) - U1.g) :
Ex := evalDG(DirectionalCovariantDerivative(D_x, g, C) - U2.g) :
Ey := evalDG(DirectionalCovariantDerivative(D_y, g, C) - U3.g) :
=
> Eq000 := TensorInnerProduct(g, Et, dt &t dt) :
Eq001 := TensorInnerProduct(g, Et, dt &t dx) :
Eq002 := TensorInnerProduct(g, Et, dt &t dy) :
Eq011 := TensorInnerProduct(g, Et, dx &t dx) :
Eq012 := TensorInnerProduct(g, Et, dx &t dy) :
Eq022 := TensorInnerProduct(g, Et, dy &t dy) :
Eq100 := TensorInnerProduct(g, Ex, dt &t dt) :
Eq101 := TensorInnerProduct(g, Ex, dt &t dx) :
Eq102 := TensorInnerProduct(g, Ex, dt &t dy) :
Eq111 := TensorInnerProduct(g, Ex, dx &t dx) :
Eq112 := TensorInnerProduct(g, Ex, dx &t dy) :
Eq122 := TensorInnerProduct(g, Ex, dy &t dy) :
Eq200 := TensorInnerProduct(g, Ey, dt &t dt) :
Eq201 := TensorInnerProduct(g, Ey, dt &t dx) :
Eq202 := TensorInnerProduct(g, Ey, dt &t dy) :
Eq211 := TensorInnerProduct(g, Ey, dx &t dx) :
Eq212 := TensorInnerProduct(g, Ey, dx &t dy) :
Eq222 := TensorInnerProduct(g, Ey, dy &t dy) :
=
> sA := solve( {Eq000=0, Eq001=0, Eq002=0, Eq011=0, Eq012=0, Eq022=0, Eq100=0,
Eq101=0, Eq102=0, Eq111=0, Eq112=0, Eq122=0, Eq200=0, Eq201=0, Eq202=0,
Eq211=0, Eq212=0, Eq222=0}, [a000, a001, a002, a010, a011, a012, a020, a021, a022,
a101, a102, a111, a112, a121, a122, a202, a212, a222]) :
=
> C1 := evalDG( subs( {op(op(sA))}, C) ) :
> evalDG( CovariantDerivative(g, C1) - g &t (U1.dt + U2.dx + U3.dy) );
0 dt dt dt
(50)

```

The connection  $C=C1$  is uniquely determined by the 1st equation of EW property:  $D_C(g)=\omega g$ .  
Let us consider the main defining relation:  $\text{Ricci}(C)=V*g$  ( $V$  is some scalar function).

```

> R1 := CurvatureTensor(C1) : Ric1 := RicciTensor(R1) : T1 := SymmetrizeIndices(Ric1, [1, 2],
"Symmetric") : Res := evalDG(T1 - V.g) :
=
> NEQt := ContractIndices(Res, D_t &t D_t, [[1, 1], [2, 2]]) : NEQtX := ContractIndices(Res,
D_t &t D_x, [[1, 1], [2, 2]]) :
NEQty := ContractIndices(Res, D_t &t D_y, [[1, 1], [2, 2]]) : NEQxx := ContractIndices(Res,
D_x &t D_x, [[1, 1], [2, 2]]) :
NEQxy := ContractIndices(Res, D_x &t D_y, [[1, 1], [2, 2]]) : NEQyy := ContractIndices(Res,
D_y &t D_y, [[1, 1], [2, 2]]) :
=
>
> DGsetup([t, x, y], [\phi, m], J2, 4) :
> de := DifferentialEquationData([F, G], [\phi_1, m_1])
de := [ {m_1, \phi_1}, [ -\phi_1^2 e^{-\phi} + \phi_1 e^{-\phi} - m_2 \phi_{1,3} + m_1 \phi_{2,3}, m_{1,1} e^{-\phi} - m_2 m_{1,3}
+ m_1 m_{2,3} ] ]
(51)
> de2 := Prolong(de, 2) : deTRA := Transformation(de2) :
>

```

```

> Eq0 := Pullback(deTRA, ToJet(NEQt, DepVars, notation = jetnumbers)) :
> VS := solve(Eq0, V) :
> Eq1 := numer(subs(V = VS, Pullback(deTRA, ToJet(NEQt, DepVars, notation
= jetnumbers)))) :
Eq2 := numer(subs(V = VS, Pullback(deTRA, ToJet(NEQy, DepVars, notation
= jetnumbers)))) :
Eq3 := numer(subs(V = VS, Pullback(deTRA, ToJet(NEQxx, DepVars, notation
= jetnumbers)))) :
Eq4 := numer(subs(V = VS, Pullback(deTRA, ToJet(NEQxy, DepVars, notation
= jetnumbers)))) :
Eq5 := numer(subs(V = VS, Pullback(deTRA, ToJet(NEQyy, DepVars, notation
= jetnumbers)))) :

J2 >
J2 > simplify([Eq1, Eq2, Eq3, Eq4, Eq5])
[0, 0, 0, 0, 0]

```

```

> restart :
V. Now consider the 1-component reduction of the Bogdanov generalization of BF
> with(DifferentialGeometry) : with(Tensor) : with(Tools) : with(JetCalculus) :
  with(LinearAlgebra) : with(PDEtools, D_Dx, declare, ToJet, FromJet) :
> declare(h(u_{2,2}, u_{2,3}, u_{3,3})) : subs([h_r(r, s, t) = haha], subs([u_{2,2} = r, u_{2,3} = s, u_{3,3} = t, u_{1,2}
= a, u_{1,3} = b], \frac{d^3}{du_{1,3}^3} f(u_{2,2}, u_{2,3}, u_{3,3}, u_{1,2}, u_{1,3}) ))
                                     h(u_{2,2}, u_{2,3}, u_{3,3}) will now be displayed as h
                                                                    f_{b,b,b}
> DGsetup([t, x, y], [m], J2) :
> F := m_1^0 \cdot m_{1,1} - m_2 \cdot m_{1,3} + m_1 \cdot m_{2,3}
                                     F := m_1^0 m_{1,1} - m_2 m_{1,3} + m_1 m_{2,3}

```

$$\begin{aligned}
& \text{> } A := 2 \cdot \text{Matrix} \left( \left[ \left[ \text{diff}(F, m[1, 1]), \frac{1}{2} \text{diff}(F, m[1, 2]), \frac{1}{2} \text{diff}(F, m[1, 3]) \right], \left[ \frac{1}{2} \text{diff}(F, m[1, 2]), \text{diff}(F, m[2, 2]), \frac{1}{2} \text{diff}(F, m[2, 3]) \right], \left[ \frac{1}{2} \text{diff}(F, m[1, 3]), \frac{1}{2} \text{diff}(F, m[2, 3]), \text{diff}(F, m[3, 3]) \right] \right] \right) \\
& A := \begin{bmatrix} 2 m_1^\rho & 0 & -m_2 \\ 0 & 0 & m_1 \\ -m_2 & m_1 & 0 \end{bmatrix} \quad (55)
\end{aligned}$$

$$\begin{aligned}
& \text{J2 > } \det := \text{simplify}(\text{Determinant}(A)); AA := \text{expand}(\text{MatrixInverse}(A)); \\
& AM := \text{simplify}(\text{Determinant}(A) \cdot AA); AdA := \text{simplify}(\text{Adjoint}(A)); \\
& \det := -2 m_1^{(\rho+2)} \\
& AM := \begin{bmatrix} -m_1^2 & -m_1 m_2 & 0 \\ -m_1 m_2 & -m_2^2 & -2 m_1^{(\rho+1)} \\ 0 & -2 m_1^{(\rho+1)} & 0 \end{bmatrix} \\
& AdA := \begin{bmatrix} -m_1^2 & -m_1 m_2 & 0 \\ -m_1 m_2 & -m_2^2 & -2 m_1^{(\rho+1)} \\ 0 & -2 m_1^{(\rho+1)} & 0 \end{bmatrix} \quad (56)
\end{aligned}$$

Here A is the matrix of the linearized operator (bivector=metric with upper indices),  
AA - the inverse (metric, which we remember is defined only up to conformal rescaling)  
and AJ=AM=AdA the adjoint matrix (which we use as a representative for the conformal class)

$$\begin{aligned}
& \text{> } aA := [\text{TotalDiff}(A[1, 1], 1) + \text{TotalDiff}(A[1, 2], 2) + \text{TotalDiff}(A[1, 3], 3), \text{TotalDiff}(A[2, 1], 1) + \text{TotalDiff}(A[2, 2], 2) + \text{TotalDiff}(A[2, 3], 3), \text{TotalDiff}(A[3, 1], 1) \\
& \quad + \text{TotalDiff}(A[3, 2], 2) + \text{TotalDiff}(A[3, 3], 3)]: \\
& \text{> } \omega := 2 \cdot [AA[1, 1] \cdot aA[1] + AA[1, 2] \cdot aA[2] + AA[1, 3] \cdot aA[3], AA[2, 1] \cdot aA[1] + AA[2, 2] \\
& \quad \cdot aA[2] + AA[2, 3] \cdot aA[3], AA[3, 1] \cdot aA[1] + AA[3, 2] \cdot aA[2] + AA[3, 3] \cdot aA[3]]: \\
& \text{M > } \text{simplify}(\omega) \\
& \left[ -\frac{-2 \rho m_{1,1} + m_1^{(-\rho+1)} m_{2,3} - m_1^{(-\rho)} m_2 m_{1,3}}{m_1}, \right. \\
& \quad \left. -\frac{m_2 (-2 \rho m_{1,1} + m_1^{(-\rho+1)} m_{2,3} - m_1^{(-\rho)} m_2 m_{1,3})}{m_1^2}, \frac{2 m_{1,3}}{m_1} \right] \quad (57)
\end{aligned}$$

$$\begin{aligned}
& \text{> } \text{DepVars} := [m(t, x, y)]: AJ := \text{simplify}(\text{FromJet}(AdA, \text{DepVars})) : \\
& \text{>}
\end{aligned}$$

```

> DGsetup([t, x, y], M) :
> g := - evalDG(AJ[1, 1]·dt &t dt + AJ[1, 2]·dt &t dx + AJ[1, 3]·dt &t dy + AJ[2, 1]·dx &t dt
+ AJ[2, 2]·dx &t dx + AJ[2, 3]·dx &t dy + AJ[3, 1]·dy &t dt + AJ[3, 2]·dy &t dx
+ AJ[3, 3]·dy &t dy)
g := m_t^2 dt dt + m_t m_x dt dx + m_t m_x dx dt + m_x^2 dx dx + 2 m_t^(p+1) dx dy + 2 m_t^(p+1) dy dx

```

(58)

```

> C := Connection(a000*dt &t D_t &t dt + a111*dx &t D_x &t dx + a222*dy &t D_y &t dy
+ a001*(dt &t D_t &t dx + dx &t D_t &t dt) + a002*(dt &t D_t &t dy + dy &t D_t
&t dt) + a102*(dx &t D_t &t dy + dy &t D_t &t dx) + a011*(dt &t D_x &t dx + dx
&t D_x &t dt) + a012*(dt &t D_x &t dy + dy &t D_x &t dt) + a112*(dx &t D_x &t dy
+ dy &t D_x &t dx) + a021*(dt &t D_y &t dx + dx &t D_y &t dt) + a022*(dt &t D_y
&t dy + dy &t D_y &t dt) + a122*(dx &t D_y &t dy + dy &t D_y &t dx) + a010*dt
&t D_x &t dt + a121*dx &t D_y &t dx + a202*dy &t D_t &t dy + a020*dt &t D_y &t dt
+ a101*dx &t D_t &t dx + a212*dy &t D_x &t dy) :

```

```

> TorsionTensor(C);

```

0 dt D\_t dt

(59)

```

> U1 := simplify(FromJet(ω[1], DepVars)) :
U2 := simplify(FromJet(ω[2], DepVars)) :
U3 := simplify(FromJet(ω[3], DepVars)) :

```

Here we determine the connection C and define the covector U=omega. Later we will demonstrate that this choice of omega is the only natural

```

> Et := evalDG(DirectionalCovariantDerivative(D_t, g, C) - U1·g) :
Ex := evalDG(DirectionalCovariantDerivative(D_x, g, C) - U2·g) :
Ey := evalDG(DirectionalCovariantDerivative(D_y, g, C) - U3·g) :

```

```

> Eq000 := TensorInnerProduct(g, Et, dt &t dt) :
Eq001 := TensorInnerProduct(g, Et, dt &t dx) :
Eq002 := TensorInnerProduct(g, Et, dt &t dy) :
Eq011 := TensorInnerProduct(g, Et, dx &t dx) :
Eq012 := TensorInnerProduct(g, Et, dx &t dy) :
Eq022 := TensorInnerProduct(g, Et, dy &t dy) :
Eq100 := TensorInnerProduct(g, Ex, dt &t dt) :
Eq101 := TensorInnerProduct(g, Ex, dt &t dx) :
Eq102 := TensorInnerProduct(g, Ex, dt &t dy) :
Eq111 := TensorInnerProduct(g, Ex, dx &t dx) :
Eq112 := TensorInnerProduct(g, Ex, dx &t dy) :
Eq122 := TensorInnerProduct(g, Ex, dy &t dy) :
Eq200 := TensorInnerProduct(g, Ey, dt &t dt) :
Eq201 := TensorInnerProduct(g, Ey, dt &t dx) :
Eq202 := TensorInnerProduct(g, Ey, dt &t dy) :
Eq211 := TensorInnerProduct(g, Ey, dx &t dx) :
Eq212 := TensorInnerProduct(g, Ey, dx &t dy) :
Eq222 := TensorInnerProduct(g, Ey, dy &t dy) :

```

```

> sA := solve({Eq000=0, Eq001=0, Eq002=0, Eq011=0, Eq012=0, Eq022=0, Eq100=0,
Eq101=0, Eq102=0, Eq111=0, Eq112=0, Eq122=0, Eq200=0, Eq201=0, Eq202=0,
Eq211=0, Eq212=0, Eq222=0}, [a000, a001, a002, a010, a011, a012, a020, a021, a022,
a101, a102, a111, a112, a121, a122, a202, a212, a222]) :

```

```

> C1 := evalDG(subs({op(op(sA))}, C)) :

```

```

> evalDG(CovariantDerivative(g, C1) - g &t (U1·dt + U2·dx + U3·dy));

```

0

The connection  $C=C1$  is uniquely determined by the 1st equation of EW property:  $D_C(g)=\omega g$ .  
Let us consider the main defining relation:  $\text{Ricci}(C)=V \cdot g$  ( $V$  is some scalar function).

```

> R1 := CurvatureTensor(C1) : Ric1 := RicciTensor(R1) : T1 := SymmetrizeIndices(Ric1, [1, 2],
  "Symmetric") : Res := evalDG(T1 - V·g) :
> NEQtt := ContractIndices(Res, D_t &t D_t, [[1, 1], [2, 2]]) : NEQtx := ContractIndices(Res,
  D_t &t D_x, [[1, 1], [2, 2]]) :
  NEQty := ContractIndices(Res, D_t &t D_y, [[1, 1], [2, 2]]) : NEQxx := ContractIndices(Res,
  D_x &t D_x, [[1, 1], [2, 2]]) :
  NEQxy := ContractIndices(Res, D_x &t D_y, [[1, 1], [2, 2]]) : NEQyy := ContractIndices(Res,
  D_y &t D_y, [[1, 1], [2, 2]]) :
>
> DGsetup([t, x, y], [m], J2, 4) :
> de := DifferentialEquationData([F], [m1,1])
  de := [ {m1,1}, [m1p m1,1 - m2 m1,3 + m1 m2,3] ]

```

(61)

```

> de2 := Prolong(de, 2) : deTRA := Transformation(de2) :
>
> Eq0 := Pullback(deTRA, ToJet(NEQtt, DepVars, notation = jetnumbers)) :
> VS := solve(Eq0, V) :
> Eq1 := numer(subs(V = VS, Pullback(deTRA, ToJet(NEQtx, DepVars, notation
  = jetnumbers)))) :
  Eq2 := numer(subs(V = VS, Pullback(deTRA, ToJet(NEQty, DepVars, notation
  = jetnumbers)))) :
  Eq3 := numer(subs(V = VS, Pullback(deTRA, ToJet(NEQxx, DepVars, notation
  = jetnumbers)))) :
  Eq4 := numer(subs(V = VS, Pullback(deTRA, ToJet(NEQxy, DepVars, notation
  = jetnumbers)))) :
  Eq5 := numer(subs(V = VS, Pullback(deTRA, ToJet(NEQyy, DepVars, notation
  = jetnumbers)))) :
J2 > simplify([Eq1, Eq2, Eq3, Eq4, Eq5])
  [0, 0, 0, 0, 0]

```

(62)

Done!

```

>
> simplify(Pullback(Transformation(DifferentialEquationData([F], [m2,3]]), ω))
  [ m1,1 (2 ρ + 1) / m1, m2 m1,1 (2 ρ + 1) / m12, 2 m1,3 / m1 ]

```

(63)

Via. Now I implement the contact change of variables from Section 6 and check that the equations and EW structures are mapped to each other

> restart : with(DifferentialGeometry) : with(JetCalculus) : with(Tensor) : with(Tools) :

> DGsetup([t, x, y], [m], P1, 2, verbose)

*The following coordinates have been protected:*

$[t, x, y, m_{[]}, m_1, m_2, m_3, m_{1,1}, m_{1,2}, m_{1,3}, m_{2,2}, m_{2,3}, m_{3,3}]$

*The following vector fields have been defined and protected:*

$[D_t, D_x, D_y, D_{m_{[]}}, D_{m_1}, D_{m_2}, D_{m_3}, D_{m_{1,1}}, D_{m_{1,2}}, D_{m_{1,3}}, D_{m_{2,2}}, D_{m_{2,3}}, D_{m_{3,3}}]$

*The following differential 1-forms have been defined and protected:*

$[dt, dx, dy, dm_{[]}, dm_1, dm_2, dm_3, dm_{1,1}, dm_{1,2}, dm_{1,3}, dm_{2,2}, dm_{2,3}, dm_{3,3}]$

*The following type [1,0] biforms have been defined and protected::*

$[Dt, Dx, Dy]$

*The following type [0,1] biforms (contact 1-forms) have been defined and protected::*

$[Cm_{[]}, Cm_1, Cm_2, Cm_3, Cm_{1,1}, Cm_{1,2}, Cm_{1,3}, Cm_{2,2}, Cm_{2,3}, Cm_{3,3}]$

*frame name: P1*

(64)

> DGsetup([T, X, Y], [M], Q1, 2, verbose)

*The following coordinates have been protected:*

$[T, X, Y, M_{[]}, M_1, M_2, M_3, M_{1,1}, M_{1,2}, M_{1,3}, M_{2,2}, M_{2,3}, M_{3,3}]$

*The following vector fields have been defined and protected:*

$[D_T, D_X, D_Y, D_{M_{[]}}, D_{M_1}, D_{M_2}, D_{M_3}, D_{M_{1,1}}, D_{M_{1,2}}, D_{M_{1,3}}, D_{M_{2,2}}, D_{M_{2,3}}, D_{M_{3,3}}]$

*The following differential 1-forms have been defined and protected:*

$[dT, dX, dY, dM_{[]}, dM_1, dM_2, dM_3, dM_{1,1}, dM_{1,2}, dM_{1,3}, dM_{2,2}, dM_{2,3}, dM_{3,3}]$

*The following type [1,0] biforms have been defined and protected::*

$[DT, DX, DY]$

*The following type [0,1] biforms (contact 1-forms) have been defined and protected::*

$[CM_{[]}, CM_1, CM_2, CM_3, CM_{1,1}, CM_{1,2}, CM_{1,3}, CM_{2,2}, CM_{2,3}, CM_{3,3}]$

*frame name: Q1*

(65)

>

>  $\Phi := \text{Transformation}\left(P1, Q1, \left[X = x, Y = y, T = \frac{1}{2} \cdot \ln(m_1), M_{[]} = \frac{m_{[]} - t \cdot m_1}{\sqrt{m_1}}, M_1 = -2 t \cdot \sqrt{m_1} - \frac{m_{[]} - t \cdot m_1}{\sqrt{m_1}}, M_2 = \frac{m_2}{\sqrt{m_1}}, M_3 = \frac{m_3}{\sqrt{m_1}}\right]\right)$

$\Phi := \left[T = \frac{1}{2} \ln(m_1), X = x, Y = y, M_{[]} = \frac{m_{[]} - t \cdot m_1}{\sqrt{m_1}}, M_1 = -2 t \sqrt{m_1} - \frac{m_{[]} - t \cdot m_1}{\sqrt{m_1}}, M_2 = \frac{m_2}{\sqrt{m_1}}, M_3 = \frac{m_3}{\sqrt{m_1}}\right]$  (66)

$$= \frac{m_2}{\sqrt{m_1}}, M_3 = \frac{m_3}{\sqrt{m_1}} \Big]$$

$$> \Omega_0 := evalDG(dM_{[]} - M_1 \cdot dT - M_2 \cdot dX - M_3 \cdot dY) : \Omega_1 := evalDG(dM_1 - M_{1,1} \cdot dT - M_{1,2} \cdot dX - M_{1,3} \cdot dY) :$$

$$\Omega_2 := evalDG(dM_2 - M_{1,2} \cdot dT - M_{2,2} \cdot dX - M_{2,3} \cdot dY) : \Omega_3 := evalDG(dM_3 - M_{1,3} \cdot dT - M_{2,3} \cdot dX - M_{3,3} \cdot dY) :$$

$$> V1 := D_T + M_1 \cdot D_{M_{[]}} + M_{1,1} \cdot D_{M_1} + M_{1,2} \cdot D_{M_2} + M_{1,3} \cdot D_{M_3} :$$

$$V2 := D_X + M_2 \cdot D_{M_{[]}} + M_{1,2} \cdot D_{M_1} + M_{2,2} \cdot D_{M_2} + M_{2,3} \cdot D_{M_3} :$$

$$V3 := D_Y + M_3 \cdot D_{M_{[]}} + M_{1,3} \cdot D_{M_1} + M_{2,3} \cdot D_{M_2} + M_{3,3} \cdot D_{M_3} :$$

$$> [Hook(V1, \Omega_0), Hook(V1, \Omega_1), Hook(V1, \Omega_2), Hook(V1, \Omega_3), Hook(V2, \Omega_0), Hook(V2, \Omega_1), Hook(V2, \Omega_2), Hook(V2, \Omega_3), Hook(V3, \Omega_0), Hook(V3, \Omega_1), Hook(V3, \Omega_2), Hook(V3, \Omega_3)]$$

$$[0, 0, 0, 0, 0, 0, 0, 0, 0, 0, 0, 0, 0] \quad (67)$$

$$> \Psi1 := InverseTransformation(\Phi)$$

$$\Psi1 := \left[ t = -\frac{1}{2} \frac{M_1 + M_{[]}}{\sqrt{e^{2T}}}, x = X, y = Y, m_{[]} = \frac{1}{2} M_{[]} \sqrt{e^{2T}} - \frac{1}{2} \sqrt{e^{2T}} M_1, m_1 = e^{2T}, m_2 \right. \quad (68)$$

$$\left. = M_2 \sqrt{e^{2T}}, m_3 = M_3 \sqrt{e^{2T}} \right]$$

$$> \theta_0 := evalDG(dm_{[]} - m_1 dt - m_2 dx - m_3 dy) :$$

$$> [Hook(V1, Pullback(\Psi1, \theta_0)), Hook(V2, Pullback(\Psi1, \theta_0)), Hook(V3, Pullback(\Psi1, \theta_0))] \quad (69)$$

$$[0, 0, 0]$$

$$> Pullback(\Phi, e^T \cdot \Omega_0)$$

$$-m_1 dt - m_2 dx - m_3 dy + dm_{[]} \quad (70)$$

$$> \Phi2 := Prolong(\Phi, 2)$$

$$\Phi2 := \left[ T = \frac{1}{2} \ln(m_1), X = x, Y = y, M_{[]} = \frac{m_{[]} - t m_1}{\sqrt{m_1}}, M_1 = -2 t \sqrt{m_1} - \frac{m_{[]} - t m_1}{\sqrt{m_1}}, M_2 \right. \quad (71)$$

$$\left. = \frac{m_2}{\sqrt{m_1}}, M_3 = \frac{m_3}{\sqrt{m_1}}, M_{1,1} = \frac{2 m_1 \left( -2 \sqrt{m_1} - \frac{1}{2} \frac{(-m_{[]} + t m_1) m_{1,1}}{m_1^{(3/2)}} \right)}{m_{1,1}}, M_{1,2} \right]$$

$$\begin{aligned}
&= \frac{2 m_1 \left( -\frac{1}{2} \frac{m_2 m_{1,1}}{m_1^{(3/2)}} + \frac{m_{1,2}}{\sqrt{m_1}} \right)}{m_{1,1}}, M_{1,3} = \frac{2 m_1 \left( -\frac{1}{2} \frac{m_3 m_{1,1}}{m_1^{(3/2)}} + \frac{m_{1,3}}{\sqrt{m_1}} \right)}{m_{1,1}}, M_{2,2} = \\
&- \frac{m_{1,2} \left( -\frac{1}{2} \frac{m_2 m_{1,1}}{m_1^{(3/2)}} + \frac{m_{1,2}}{\sqrt{m_1}} \right)}{m_{1,1}} - \frac{1}{2} \frac{m_2 m_{1,2}}{m_1^{(3/2)}} + \frac{m_{2,2}}{\sqrt{m_1}}, M_{2,3} = \\
&- \frac{m_{1,2} \left( -\frac{1}{2} \frac{m_3 m_{1,1}}{m_1^{(3/2)}} + \frac{m_{1,3}}{\sqrt{m_1}} \right)}{m_{1,1}} - \frac{1}{2} \frac{m_3 m_{1,2}}{m_1^{(3/2)}} + \frac{m_{2,3}}{\sqrt{m_1}}, M_{3,3} = \\
&- \frac{m_{1,3} \left( -\frac{1}{2} \frac{m_3 m_{1,1}}{m_1^{(3/2)}} + \frac{m_{1,3}}{\sqrt{m_1}} \right)}{m_{1,1}} - \frac{1}{2} \frac{m_3 m_{1,3}}{m_1^{(3/2)}} + \frac{m_{3,3}}{\sqrt{m_1}} \Bigg]
\end{aligned}$$

>  $\Psi2 := \text{InverseTransformation}(\Phi2)$

$$\begin{aligned}
\Psi2 &:= \left[ t = -\frac{1}{2} \frac{M_1 + M_{[]}}{\sqrt{e^{2T}}}, x = X, y = Y, m_{[]} = \frac{1}{2} M_{[]} \sqrt{e^{2T}} - \frac{1}{2} \sqrt{e^{2T}} M_1, m_1 = e^{2T}, m_2 \right. \\
&= M_2 \sqrt{e^{2T}}, m_3 = M_3 \sqrt{e^{2T}}, m_{1,1} = \frac{4 (e^{2T})^{3/2}}{-M_{1,1} + M_{[]}}, m_{1,2} = \frac{2 e^{2T} (M_{1,2} + M_2)}{-M_{1,1} + M_{[]}}, m_{1,3} \\
&= \frac{2 e^{2T} (M_{1,3} + M_3)}{-M_{1,1} + M_{[]}}, m_{2,2} = \frac{\sqrt{e^{2T}} (M_{[]} M_{2,2} + M_{1,2}^2 + 2 M_{1,2} M_2 + M_2^2 - M_{2,2} M_{1,1})}{-M_{1,1} + M_{[]}}, \\
m_{2,3} &= \frac{\sqrt{e^{2T}} (M_{[]} M_{2,3} + M_{1,2} M_3 + M_2 M_{1,3} + M_{1,2} M_{1,3} + M_2 M_3 - M_{2,3} M_{1,1})}{-M_{1,1} + M_{[]}}, m_{3,3} \\
&= \frac{\sqrt{e^{2T}} (M_{[]} M_{3,3} + M_{1,3}^2 + 2 M_{1,3} M_3 + M_3^2 - M_{3,3} M_{1,1})}{-M_{1,1} + M_{[]} \Bigg]
\end{aligned} \tag{72}$$

>

>  $G := \text{Pullback}(\Psi2, \text{evalDG}((m_1 \cdot dt + m_2 \cdot dx) \& t (m_1 \cdot dt + m_2 \cdot dx) + 2 m_1^0 + 1 \cdot (dx \& t dy + dy \& t dx)))$

$$\begin{aligned}
G &:= \frac{1}{4} e^{2T} (M_1 + M_{[]})^2 dT dT + \frac{1}{2} e^{2T} M_2 (M_1 + M_{[]}) dT dX - \frac{1}{4} e^{2T} (M_1 + M_{[]}) dT dM_{[]} \\
&- \frac{1}{4} e^{2T} (M_1 + M_{[]}) dT dM_1 + \frac{1}{2} e^{2T} M_2 (M_1 + M_{[]}) dX dT + M_2^2 e^{2T} dX dX \\
&+ 2 (e^{2T})^p e^{2T} dX dY - \frac{1}{2} e^{2T} M_2 dX dM_{[]} - \frac{1}{2} e^{2T} M_2 dX dM_1 + 2 (e^{2T})^p e^{2T} dY dX
\end{aligned} \tag{73}$$



$$\begin{aligned}
& -\frac{1}{4} e^{2T} (M_1 + M_{[]}) dM_{[]} dT - \frac{1}{2} e^{2T} M_2 dM_{[]} dX + \frac{1}{4} e^{2T} dM_{[]} dM_{[]} \\
& + \frac{1}{4} e^{2T} dM_{[]} dM_1 - \frac{1}{4} e^{2T} (M_1 + M_{[]}) dM_1 dT - \frac{1}{2} e^{2T} M_2 dM_1 dX + \frac{1}{4} e^{2T} dM_1 dM_{[]} \\
& + \frac{1}{4} e^{2T} dM_1 dM_1
\end{aligned}$$

$\text{G11} := \text{ContractIndices}(V1 \ \&t \ V1, G, [[1, 1], [2, 2]]); \text{G12} := \text{ContractIndices}(V1 \ \&t \ V2, G, [[1, 1], [2, 2]]);$   
 $\text{G13} := \text{ContractIndices}(V1 \ \&t \ V3, G, [[1, 1], [2, 2]]);$   
 $\text{G22} := \text{ContractIndices}(V2 \ \&t \ V2, G, [[1, 1], [2, 2]]); \text{G23} := \text{ContractIndices}(V2 \ \&t \ V3, G, [[1, 1], [2, 2]]);$   
 $\text{G33} := \text{ContractIndices}(V3 \ \&t \ V3, G, [[1, 1], [2, 2]]);$

$$\text{G11} := \frac{1}{4} e^{2T} (M_{1,1}^2 - 2 M_{1,1} M_{[]} + M_{[]}^2)$$

$$\text{G12} := \frac{1}{4} e^{2T} (M_{1,1} M_{1,2} - M_{1,1} M_2 - M_{1,2} M_{[]} + M_2 M_{[]})$$

$$\text{G13} := -\frac{1}{4} e^{2T} (-M_{1,1} M_{1,3} - M_{1,1} M_3 + M_{1,3} M_{[]} + M_3 M_{[]})$$

$$\text{G22} := \frac{1}{4} e^{2T} (M_{1,2}^2 + M_2^2 - 2 M_{1,2} M_2)$$

$$\text{G23} := \frac{1}{4} e^{2T} (M_{1,2} M_{1,3} + M_{1,2} M_3 - M_2 M_{1,3} - M_2 M_3 + 8 (e^{2T})^p)$$

$$\text{G33} := \frac{1}{4} e^{2T} (M_{1,3}^2 + 2 M_{1,3} M_3 + M_3^2)$$

(74)

$$\begin{aligned}
\omega := \text{evalDG} \left( -\frac{-2 \rho m_{1,1} + m_1^{1-\rho} m_{2,3} - m_1^{-\rho} m_2 m_{1,3}}{m_1} \cdot dt \right. \\
\left. - \frac{m_2 (-2 \rho m_{1,1} + m_1^{(-\rho+1)} m_{2,3} - m_1^{(-\rho)} m_2 m_{1,3})}{m_1^2} \cdot dx + \frac{2 m_{1,3}}{m_1} \cdot dy \right) :
\end{aligned}$$

$\text{de} := \text{DifferentialEquationData}([m_1^p \cdot m_{1,1} - m_2 \cdot m_{1,3} + m_1 \cdot m_{2,3}], [m_{1,1}]) : \text{deTRA}$   
 $:= \text{Transformation}(\text{de}) :$

$\omega 0 := \text{simplify}(\text{Pullback}(\text{deTRA}, \omega))$

$$\begin{aligned}
\omega 0 := & -\frac{(-2 \rho m_1^{(-\rho)} m_2 m_{1,3} + 2 \rho m_1^{(-\rho+1)} m_{2,3} + m_1^{(-\rho+1)} m_{2,3} - m_1^{(-\rho)} m_2 m_{1,3}) dt}{m_1} \\
& - \frac{m_2 (-2 \rho m_1^{(-\rho)} m_2 m_{1,3} + 2 \rho m_1^{(-\rho+1)} m_{2,3} + m_1^{(-\rho+1)} m_{2,3} - m_1^{(-\rho)} m_2 m_{1,3}) dx}{m_1^2} \\
& + \frac{2 m_{1,3} dy}{m_1}
\end{aligned}$$

(75)

$\text{simplify}(\text{Pullback}(\Psi 2, m_1^p \cdot m_{1,1} - m_2 \cdot m_{1,3} + m_1 \cdot m_{2,3}))$

$$\frac{(e^{2T})^{3/2} \left( 4 (e^{2T})^{\rho} - M_2 M_{1,3} - M_2 M_3 + M_{[1} M_{2,3} + M_{1,2} M_3 + M_{1,2} M_{1,3} - M_{2,3} M_{1,1} \right)}{-M_{1,1} + M_{[1}} \quad (76)$$

> *De* := DifferentialEquationData([ 4 e<sup>2ρT</sup> - M<sub>2</sub> M<sub>1,3</sub> - M<sub>2</sub> M<sub>3</sub> + M<sub>[1</sub> M<sub>2,3</sub> + M<sub>1,2</sub> M<sub>3</sub> + M<sub>1,2</sub> M<sub>1,3</sub> - M<sub>2,3</sub> M<sub>1,1</sub> ], [M<sub>1,1</sub>]) : *DeTRA* := Transformation(*De*) :

> *Om1* := simplify(Pullback(*DeTRA*, Hook(*V1*, Pullback(*Ψ2*, ω))));

*Om2* := simplify(Pullback(*DeTRA*, Hook(*V2*, Pullback(*Ψ2*, ω))));

*Om3* := simplify(Pullback(*DeTRA*, Hook(*V3*, Pullback(*Ψ2*, ω))));

$$Om1 := 4 \rho + 2 e^{2\rho T} (e^{2T})^{-\rho}$$

$$Om2 := - \frac{2 (2 \rho + e^{2\rho T} (e^{2T})^{-\rho}) (-M_{1,2} + M_2) M_{2,3}}{4 e^{2\rho T} - M_2 M_{1,3} - M_2 M_3 + M_{1,2} M_3 + M_{1,2} M_{1,3}}$$

*Om3* := (77)

$$\frac{2 (2 M_{1,3} \rho + M_{1,3} (e^{2T})^{-\rho} e^{2\rho T} + 2 M_3 \rho + M_3 (e^{2T})^{-\rho} e^{2\rho T} - 2 M_{1,3} - 2 M_3) M_{2,3}}{4 e^{2\rho T} - M_2 M_{1,3} - M_2 M_3 + M_{1,2} M_3 + M_{1,2} M_{1,3}}$$

> *Om1* := simplify(Pullback(*DeTRA*, Hook(*V1*, Pullback(*Ψ2*, ω0))));

*Om2* := simplify(Pullback(*DeTRA*, Hook(*V2*, Pullback(*Ψ2*, ω0))));

*Om3* := simplify(Pullback(*DeTRA*, Hook(*V3*, Pullback(*Ψ2*, ω0))));

$$Om1 := 2 (e^{2T})^{-\rho} e^{2\rho T} (2 \rho + 1)$$

$$Om2 := - \frac{2 e^{2\rho T} (2 \rho + 1) (e^{2T})^{-\rho} (-M_{1,2} + M_2) M_{2,3}}{4 e^{2\rho T} - M_2 M_{1,3} - M_2 M_3 + M_{1,2} M_3 + M_{1,2} M_{1,3}}$$

*Om3* := ( 2 ( -2 M<sub>1,3</sub> - 2 M<sub>3</sub> + M<sub>3</sub> (e<sup>2T</sup>)<sup>-ρ</sup> e<sup>2ρT</sup> + M<sub>1,3</sub> (e<sup>2T</sup>)<sup>-ρ</sup> e<sup>2ρT</sup> + 2 M<sub>1,3</sub> (e<sup>2T</sup>)<sup>-ρ</sup> ρ e<sup>2ρT</sup> (78)

$$+ 2 M_3 (e^{2T})^{-\rho} \rho e^{2\rho T} ) M_{2,3} ) / ( 4 e^{2\rho T} - M_2 M_{1,3} - M_2 M_3 + M_{1,2} M_3 + M_{1,2} M_{1,3} )$$

> simplify( -2 M<sub>1,3</sub> - 2 M<sub>3</sub> + M<sub>3</sub> + M<sub>1,3</sub> + 2 M<sub>1,3</sub> ρ + 2 M<sub>3</sub> ρ )

$$-M_{1,3} - M_3 + 2 M_{1,3} \rho + 2 M_3 \rho \quad (79)$$

> restart :

VIb. So I want to check how this formula for the pullback-omega agrees with the omega calculated by the usual formula

> with(DifferentialGeometry) : with(Tensor) : with(Tools) : with(JetCalculus) :  
with(LinearAlgebra) : with(PDEtools, D\_Dx, declare, ToJet, FromJet) :

$$\begin{aligned} & \textcolor{blue}{> \text{declare}(h(u_{2,2}, u_{2,3}, u_{3,3})) : \text{subs}\left(\left[h_r(r, s, t) = \text{haha}\right], \text{subs}\left(\left[u_{2,2} = r, u_{2,3} = s, u_{3,3} = t, u_{1,2} \right.\right.} \\ & \quad \left.\left. = a, u_{1,3} = b\right], \frac{d^3}{du_{1,3}^3} f(u_{2,2}, u_{2,3}, u_{3,3}, u_{1,2}, u_{1,3})\right)\right) \\ & \quad \textcolor{blue}{h(u_{2,2}, u_{2,3}, u_{3,3}) \text{ will now be displayed as } h} \\ & \quad \textcolor{blue}{f_{b,b,b}} \end{aligned} \tag{80}$$

$h(u_{2,2}, u_{2,3}, u_{3,3})$  will now be displayed as  $h$

$f_{b, b, b}$

(80)

```
> DGsetup( [T, X, Y], [M], J2) :
```

$$F := 4 e^{2\rho T} - M_2 M_{1,3} - M_2 M_3 + M_{[\cdot]} M_{2,3} + M_{1,2} M_3 + M_{1,2} M_{1,3} - M_{2,3} M_{1,1} \quad (81)$$

$$F := 4 e^{2\rho T} - M_2 M_{1,3} - M_2 M_3 + M_{[1} M_{2,3} + M_{1,2} M_3 + M_{1,2} M_{1,3} - M_{2,3} M_{1,1} \quad (81)$$

$$\begin{aligned} & \mathbf{A} := 2 \cdot \text{Matrix} \left( \left[ \left[ \text{diff}(F, M_{1,1}), \frac{1}{2} \text{diff}(F, M_{1,2}), \frac{1}{2} \text{diff}(F, M_{1,3}) \right], \left[ \frac{1}{2} \text{diff}(F, M_{1,2}), \right. \right. \\ & \quad \left. \left. \text{diff}(F, M_{2,2}), \frac{1}{2} \text{diff}(F, M_{2,3}) \right], \left[ \frac{1}{2} \text{diff}(F, M_{1,3}), \frac{1}{2} \text{diff}(F, M_{2,3}), \text{diff}(F, M_{3,3}) \right] \right] \right) \\ & \mathbf{A} := \begin{bmatrix} -2M_{2,3} & M_3 + M_{1,3} & -M_2 + M_{1,2} \\ M_3 + M_{1,3} & 0 & M_{[]} - M_{1,1} \\ -M_2 + M_{1,2} & M_{[]} - M_{1,1} & 0 \end{bmatrix} \end{aligned} \quad (82)$$

$$A := \begin{bmatrix} -2 M_{2,3} & M_3 + M_{1,3} & -M_2 + M_{1,2} \\ M_3 + M_{1,3} & 0 & M_{[\cdot]} - M_{1,1} \\ -M_2 + M_{1,2} & M_{[\cdot]} - M_{1,1} & 0 \end{bmatrix} \quad (82)$$

**J2** > *det := simplify(Determinant(A)); AA := expand(MatrixInverse(A)) :*

$$AM := \text{simplify}(\text{Determinant}(A) \cdot AA); AdA := \text{simplify}(\text{Adjoint}(A));$$

$$\begin{aligned} \det := & 2 M_{2,3} M_{[]}^2 - 4 M_{2,3} M_{[]} M_{1,1} + 2 M_{2,3} M_{1,1}^2 - 2 M_3 M_{[]} M_2 + 2 M_3 M_{[]} M_{1,2} \\ & + 2 M_3 M_{1,1} M_2 - 2 M_3 M_{1,1} M_{1,2} - 2 M_{1,3} M_{[]} M_2 + 2 M_{1,3} M_{[]} M_{1,2} + 2 M_{1,3} M_{1,1} M_2 \\ & - 2 M_{1,3} M_{1,1} M_{1,2} \end{aligned}$$

$$AM := \left[ \left[ - (M_{[]} - M_{1,1})^2, - (M_{[]} - M_{1,1}) (M_2 - M_{1,2}), (M_3 + M_{1,3}) (M_{[]} - M_{1,1}) \right], \right. \\ \left[ - (M_{[]} - M_{1,1}) (M_2 - M_{1,2}), - (M_2 - M_{1,2})^2, 2 M_{[]} M_{2,3} - 2 M_{2,3} M_{1,1} - M_2 M_3 \right. \\ \left. - M_2 M_{1,3} + M_{1,2} M_3 + M_{1,2} M_{1,3} \right], \\ \left[ (M_3 + M_{1,3}) (M_{[]} - M_{1,1}), 2 M_{[]} M_{2,3} - 2 M_{2,3} M_{1,1} - M_2 M_3 - M_2 M_{1,3} + M_{1,2} M_3 \right. \\ \left. + M_{1,2} M_{1,3}, - (M_3 + M_{1,3})^2 \right] \Big]$$

$$AdA := \left[ \left[ - (M_{[]} - M_{1,1})^2, - (M_{[]} - M_{1,1}) (M_2 - M_{1,2}), (M_3 + M_{1,3}) (M_{[]} - M_{1,1}) \right], \right. \quad (83)$$

$$\left[ - (M_{[]} - M_{1,1}) (M_2 - M_{1,2}), - (M_2 - M_{1,2})^2, 2 M_{[]} M_{2,3} - 2 M_{2,3} M_{1,1} - M_2 M_3 \right.$$

$$\left. - M_2 M_{1,3} + M_{1,2} M_3 + M_{1,2} M_{1,3} \right],$$

$$\left[ (M_3 + M_{1,3}) (M_{[]} - M_{1,1}), 2 M_{[]} M_{2,3} - 2 M_{2,3} M_{1,1} - M_2 M_3 - M_2 M_{1,3} + M_{1,2} M_3 \right.$$

$$\left. + M_{1,2} M_{1,3}, - (M_3 + M_{1,3})^2 \right]$$

>

$$\mathbf{N} > \text{simplify} \left( \text{subs} \left( M_{1,1} = \frac{4 e^{2\rho t} - M_2 M_{1,3} - M_2 M_3 + M_{[1]} M_{2,3} + M_{1,2} M_3 + M_{1,2} M_{1,3}}{M_{2,3}}, \right. \right. \\ \left. \left. (2 M_{[1]} M_{2,3} - 2 M_{2,3} M_{1,1} - M_2 M_3 - M_2 M_{1,3} + M_{1,2} M_3 + M_{1,2} M_{1,3}) + (M_3 + M_{1,3}) \cdot (M_{1,2} - M_2) + 8 e^{2\rho t} \right) \right) \\ 0 \quad (84)$$

> aA := [TotalDiff(A[1, 1], 1) + TotalDiff(A[1, 2], 2) + TotalDiff(A[1, 3], 3), TotalDiff(A[2, 1], 1) + TotalDiff(A[2, 2], 2) + TotalDiff(A[2, 3], 3), TotalDiff(A[3, 1], 1) + TotalDiff(A[3, 2], 2) + TotalDiff(A[3, 3], 3)] :

> ω := 2 · [AA[1, 1] · aA[1] + AA[1, 2] · aA[2] + AA[1, 3] · aA[3], AA[2, 1] · aA[1] + AA[2, 2] · aA[2] + AA[2, 3] · aA[3], AA[3, 1] · aA[1] + AA[3, 2] · aA[2] + AA[3, 3] · aA[3]] :

$$\mathbf{M} > \text{simplify}(\omega) \\ \left[ 0, \frac{2 (M_2 - M_{1,2})}{M_{[1]} - M_{1,1}}, \frac{2 (M_3 + M_{1,3})}{M_{[1]} - M_{1,1}} \right] \quad (85)$$

> restart :

VII. Finally let us check directly that the equations of Dunajski-Tod related hyper-Kähler metrics, which showed above as translation non-invariant PDEs, are not subject to our approach (I partially repeat)

> with(DifferentialGeometry) : with(Tensor) : with(Tools) : with(JetCalculus) :  
with(LinearAlgebra) : with(PDEtools, D\_Dx, declare, ToJet, FromJet) :

$$> \text{declare}(h(u_{2,2}, u_{2,3}, u_{3,3})) : \text{subs} \left( [h_r(r, s, t) = haha], \text{subs} \left( [u_{2,2} = r, u_{2,3} = s, u_{3,3} = t, u_{1,2} = a, u_{1,3} = b], \frac{d^3}{du_{1,3}^3} f(u_{2,2}, u_{2,3}, u_{3,3}, u_{1,2}, u_{1,3}) \right) \right) \\ h(u_{2,2}, u_{2,3}, u_{3,3}) \text{ will now be displayed as } h_{b,b,b} \quad (86)$$

> DGsetup([t, x, y], [M], J2) :

$$> F := 4 e^{2\rho t} - M_2 M_{1,3} - M_2 M_3 + M_{[1]} M_{2,3} + M_{1,2} M_3 + M_{1,2} M_{1,3} - M_{2,3} M_{1,1} \\ F := 4 e^{2\rho t} - M_2 M_{1,3} - M_2 M_3 + M_{[1]} M_{2,3} + M_{1,2} M_3 + M_{1,2} M_{1,3} - M_{2,3} M_{1,1} \quad (87)$$

$$\begin{aligned}
& \mathbf{A} := 2 \cdot \text{Matrix} \left( \left[ \left[ \text{diff}(F, M_{1,1}), \frac{1}{2} \text{diff}(F, M_{1,2}), \frac{1}{2} \text{diff}(F, M_{1,3}) \right], \left[ \frac{1}{2} \text{diff}(F, M_{1,2}), \right. \right. \right. \\
& \quad \left. \left. \text{diff}(F, M_{2,2}), \frac{1}{2} \text{diff}(F, M_{2,3}) \right], \left[ \frac{1}{2} \text{diff}(F, M_{1,3}), \frac{1}{2} \text{diff}(F, M_{2,3}), \text{diff}(F, M_{3,3}) \right] \right] \right) \\
& \mathbf{A} := \begin{bmatrix} -2 M_{2,3} & M_3 + M_{1,3} & -M_2 + M_{1,2} \\ M_3 + M_{1,3} & 0 & M_{[]} - M_{1,1} \\ -M_2 + M_{1,2} & M_{[]} - M_{1,1} & 0 \end{bmatrix} \tag{88}
\end{aligned}$$

$$\begin{aligned}
& \mathbf{J2} > \text{det} := \text{simplify}(\text{Determinant}(\mathbf{A})); \mathbf{AA} := \text{expand}(\text{MatrixInverse}(\mathbf{A})); \\
& \quad \mathbf{AM} := \text{simplify}(\text{Determinant}(\mathbf{A}) \cdot \mathbf{AA}); \mathbf{AdA} := \text{simplify}(\text{Adjoint}(\mathbf{A})); \\
& \text{det} := 2 M_{2,3} M_{[]}^2 - 4 M_{2,3} M_{[]} M_{1,1} + 2 M_{2,3} M_{1,1}^2 - 2 M_3 M_{[]} M_2 + 2 M_3 M_{[]} M_{1,2} \\
& \quad + 2 M_3 M_{1,1} M_2 - 2 M_3 M_{1,1} M_{1,2} - 2 M_{1,3} M_{[]} M_2 + 2 M_{1,3} M_{[]} M_{1,2} + 2 M_{1,3} M_{1,1} M_2 \\
& \quad - 2 M_{1,3} M_{1,1} M_{1,2} \\
& \mathbf{AM} := \left[ \left[ - (M_{[]} - M_{1,1})^2, - (M_{[]} - M_{1,1}) (M_2 - M_{1,2}), (M_3 + M_{1,3}) (M_{[]} - M_{1,1}) \right], \right. \\
& \quad \left[ - (M_{[]} - M_{1,1}) (M_2 - M_{1,2}), - (M_2 - M_{1,2})^2, 2 M_{[]} M_{2,3} - 2 M_{2,3} M_{1,1} - M_2 M_3 \right. \\
& \quad \left. - M_2 M_{1,3} + M_{1,2} M_3 + M_{1,2} M_{1,3} \right], \\
& \quad \left[ (M_3 + M_{1,3}) (M_{[]} - M_{1,1}), 2 M_{[]} M_{2,3} - 2 M_{2,3} M_{1,1} - M_2 M_3 - M_2 M_{1,3} + M_{1,2} M_3 \right. \\
& \quad \left. + M_{1,2} M_{1,3}, - (M_3 + M_{1,3})^2 \right] \Big] \\
& \mathbf{AdA} := \left[ \left[ - (M_{[]} - M_{1,1})^2, - (M_{[]} - M_{1,1}) (M_2 - M_{1,2}), (M_3 + M_{1,3}) (M_{[]} - M_{1,1}) \right], \right. \\
& \quad \left[ - (M_{[]} - M_{1,1}) (M_2 - M_{1,2}), - (M_2 - M_{1,2})^2, 2 M_{[]} M_{2,3} - 2 M_{2,3} M_{1,1} - M_2 M_3 \right. \\
& \quad \left. - M_2 M_{1,3} + M_{1,2} M_3 + M_{1,2} M_{1,3} \right], \\
& \quad \left[ (M_3 + M_{1,3}) (M_{[]} - M_{1,1}), 2 M_{[]} M_{2,3} - 2 M_{2,3} M_{1,1} - M_2 M_3 - M_2 M_{1,3} + M_{1,2} M_3 \right. \\
& \quad \left. + M_{1,2} M_{1,3}, - (M_3 + M_{1,3})^2 \right] \Big] \tag{89}
\end{aligned}$$

**N** >

**N** >

Here **A** is the matrix of the linearized operator (bivector=metric with upper indices),  
**AA** - the inverse (metric, which we remember is defined only up to conformal rescaling)  
and **AJ=AM=AdA** the adjoint matrix (which we use as a representative for the conformal class)

>

$$\begin{aligned}
& \mathbf{aA} := [\text{TotalDiff}(\mathbf{A}[1,1], 1) + \text{TotalDiff}(\mathbf{A}[1,2], 2) + \text{TotalDiff}(\mathbf{A}[1,3], 3), \text{TotalDiff}(\mathbf{A}[2, \\
& \quad 1], 1) + \text{TotalDiff}(\mathbf{A}[2,2], 2) + \text{TotalDiff}(\mathbf{A}[2,3], 3), \text{TotalDiff}(\mathbf{A}[3,1], 1) \\
& \quad + \text{TotalDiff}(\mathbf{A}[3,2], 2) + \text{TotalDiff}(\mathbf{A}[3,3], 3)] :
\end{aligned}$$

$$\begin{aligned}
& \omega := 2 \cdot [\mathbf{AA}[1,1] \cdot \mathbf{aA}[1] + \mathbf{AA}[1,2] \cdot \mathbf{aA}[2] + \mathbf{AA}[1,3] \cdot \mathbf{aA}[3], \mathbf{AA}[2,1] \cdot \mathbf{aA}[1] + \mathbf{AA}[2,2] \\
& \quad \cdot \mathbf{aA}[2] + \mathbf{AA}[2,3] \cdot \mathbf{aA}[3], \mathbf{AA}[3,1] \cdot \mathbf{aA}[1] + \mathbf{AA}[3,2] \cdot \mathbf{aA}[2] + \mathbf{AA}[3,3] \cdot \mathbf{aA}[3]] :
\end{aligned}$$

$$\mathbf{M} > \text{simplify}(\omega)$$

$$\left[ 0, \frac{2 (M_2 - M_{1,2})}{M_{[]} - M_{1,1}}, \frac{2 (M_3 + M_{1,3})}{M_{[]} - M_{1,1}} \right] \tag{90}$$

>

```

> DepVars := [M(t, x, y)] : AJ := simplify(FromJet(AdA, DepVars)) :
>
> DGsetup([t, x, y], N) :
> g := - evalDG(AJ[1, 1]·dt &t dt + AJ[1, 2]·dt &t dx + AJ[1, 3]·dt &t dy + AJ[2, 1]·dx &t dt
+ AJ[2, 2]·dx &t dx + AJ[2, 3]·dx &t dy + AJ[3, 1]·dy &t dt + AJ[3, 2]·dy &t dx
+ AJ[3, 3]·dy &t dy)
g := (M(t, x, y) - Mt,t)2 dt dt + (M(t, x, y) - Mt,t) (Mx - Mt,x) dt dx - (M(t, x, y)
- Mt,t) (My + Mt,y) dt dy + (M(t, x, y) - Mt,t) (Mx - Mt,x) dx dt + (Mx - Mt,x)2 dx dx
+ (-2 M(t, x, y) Mx,y + 2 Mx,y Mt,t + Mx My + Mx Mt,y - Mt,x My - Mt,x Mt,y) dx dy
- (M(t, x, y) - Mt,t) (My + Mt,y) dy dt + (-2 M(t, x, y) Mx,y + 2 Mx,y Mt,t + Mx My
+ Mx Mt,y - Mt,x My - Mt,x Mt,y) dy dx + (My + Mt,y)2 dy dy
>
> C := Connection(a000*dt &t D_t &t dt + a111*dx &t D_x &t dx + a222*dy &t D_y &t dy
+ a001*(dt &t D_t &t dx + dx &t D_t &t dt) + a002*(dt &t D_t &t dy + dy &t D_t
&t dt) + a102*(dx &t D_t &t dy + dy &t D_t &t dx) + a011*(dt &t D_x &t dx + dx
&t D_x &t dt) + a012*(dt &t D_x &t dy + dy &t D_x &t dt) + a112*(dx &t D_x &t dy
+ dy &t D_x &t dx) + a021*(dt &t D_y &t dx + dx &t D_y &t dt) + a022*(dt &t D_y
&t dy + dy &t D_y &t dt) + a122*(dx &t D_y &t dy + dy &t D_y &t dx) + a010*dt
&t D_x &t dt + a121*dx &t D_y &t dx + a202*dy &t D_t &t dy + a020*dt &t D_y &t dt
+ a101*dx &t D_t &t dx + a212*dy &t D_x &t dy) :
> TorsionTensor(C);
0 dt D_t dt

```

(91)

(92)

Here we determine the connection C and define the covector U=omega. Later we will demonstrate that this choice of omega is the only natural

```

> Et := evalDG(DirectionalCovariantDerivative(D_t, g, C) - U1·g) :
Ex := evalDG(DirectionalCovariantDerivative(D_x, g, C) - U2·g) :
Ey := evalDG(DirectionalCovariantDerivative(D_y, g, C) - U3·g) :
> Eq000 := TensorInnerProduct(g, Et, dt &t dt) :
Eq001 := TensorInnerProduct(g, Et, dt &t dx) :
Eq002 := TensorInnerProduct(g, Et, dt &t dy) :
Eq011 := TensorInnerProduct(g, Et, dx &t dx) :
Eq012 := TensorInnerProduct(g, Et, dx &t dy) :
Eq022 := TensorInnerProduct(g, Et, dy &t dy) :
Eq100 := TensorInnerProduct(g, Ex, dt &t dt) :
Eq101 := TensorInnerProduct(g, Ex, dt &t dx) :
Eq102 := TensorInnerProduct(g, Ex, dt &t dy) :
Eq111 := TensorInnerProduct(g, Ex, dx &t dx) :
Eq112 := TensorInnerProduct(g, Ex, dx &t dy) :
Eq122 := TensorInnerProduct(g, Ex, dy &t dy) :
Eq200 := TensorInnerProduct(g, Ey, dt &t dt) :
Eq201 := TensorInnerProduct(g, Ey, dt &t dx) :
Eq202 := TensorInnerProduct(g, Ey, dt &t dy) :

```

$Eq211 := \text{TensorInnerProduct}(g, Ey, dx \ \&t \ dx) :$

$Eq212 := \text{TensorInnerProduct}(g, Ey, dx \ \&t \ dy) :$

$Eq222 := \text{TensorInnerProduct}(g, Ey, dy \ \&t \ dy) :$

>  $sa := \text{solve}(\{Eq000=0, Eq001=0, Eq002=0, Eq011=0, Eq012=0, Eq022=0, Eq100=0, Eq101=0, Eq102=0, Eq111=0, Eq112=0, Eq122=0, Eq200=0, Eq201=0, Eq202=0, Eq211=0, Eq212=0, Eq222=0\}, [a000, a001, a002, a010, a011, a012, a020, a021, a022, a101, a102, a111, a112, a121, a122, a202, a212, a222]) :$

>  $C1 := \text{evalDG}(\text{subs}(\{op(op(sa))\}, C)) :$

>  $\text{evalDG}(\text{CovariantDerivative}(g, C1) - g \ \&t \ (U1 \cdot dt + U2 \cdot dx + U3 \cdot dy)) ;$   
 $0 \ dt \ dt \ dt$

(93)

The connection  $C=C1$  is uniquely determined by the 1st equation of EW property:  $D\_C(g)=\omega g$ .  
 Let us consider the main defining relation:  $\text{Ricci}(C)=V \cdot g$  ( $V$  is some scalar function).

>  $R1 := \text{CurvatureTensor}(C1) : Ric1 := \text{RicciTensor}(R1) : T1 := \text{SymmetrizeIndices}(Ric1, [1, 2],$   
 $"Symmetric") : Res := \text{evalDG}(T1 - V \cdot g) :$

>  $NEQtt := \text{ContractIndices}(Res, D\_t \ \&t \ D\_t, [[1, 1], [2, 2]]) : NEQtx := \text{ContractIndices}(Res,$   
 $D\_t \ \&t \ D\_x, [[1, 1], [2, 2]]) :$

$NEQty := \text{ContractIndices}(Res, D\_t \ \&t \ D\_y, [[1, 1], [2, 2]]) : NEQxx := \text{ContractIndices}(Res,$   
 $D\_x \ \&t \ D\_x, [[1, 1], [2, 2]]) :$

$NEQxy := \text{ContractIndices}(Res, D\_x \ \&t \ D\_y, [[1, 1], [2, 2]]) : NEQyy := \text{ContractIndices}(Res,$   
 $D\_y \ \&t \ D\_y, [[1, 1], [2, 2]]) :$

>

>  $DGsetup([t, x, y], [M], J2, 4) :$

>  $de := \text{DifferentialEquationData}([F], [M_{1,1}])$

$de := [\{M_{1,1}\}, [4 e^{2\rho t} - M_2 M_{1,3} - M_2 M_3 + M_{[1} M_{2,3} + M_{1,2} M_3 + M_{1,2} M_{1,3} - M_{2,3} M_{1,1}]]$  (94)

>  $de2 := \text{Prolong}(de, 2) : deTRA := \text{Transformation}(de2) :$

>

>  $Eq0 := \text{Pullback}(deTRA, \text{ToJet}(NEQtt, \text{DepVars}, \text{notation} = \text{jetnumbers})) :$

>  $VS := \text{solve}(Eq0, V) :$

>  $Eq1 := \text{numer}(\text{subs}(V=VS, \text{Pullback}(deTRA, \text{ToJet}(NEQtx, \text{DepVars}, \text{notation} = \text{jetnumbers})))) :$

$Eq2 := \text{numer}(\text{subs}(V=VS, \text{Pullback}(deTRA, \text{ToJet}(NEQty, \text{DepVars}, \text{notation} = \text{jetnumbers})))) :$

$Eq3 := \text{numer}(\text{subs}(V=VS, \text{Pullback}(deTRA, \text{ToJet}(NEQxx, \text{DepVars}, \text{notation} = \text{jetnumbers})))) :$

$Eq4 := \text{numer}(\text{subs}(V=VS, \text{Pullback}(deTRA, \text{ToJet}(NEQxy, \text{DepVars}, \text{notation} = \text{jetnumbers})))) :$

$Eq5 := \text{numer}(\text{subs}(V=VS, \text{Pullback}(deTRA, \text{ToJet}(NEQyy, \text{DepVars}, \text{notation} = \text{jetnumbers})))) :$

... the obtained expression is of the 3rd order but ...

J2 >  $\text{simplify}(Eq1)$

$-e^{4\rho t} \rho M_{2,3}^4 (4 e^{2\rho t} M_3^4 M_{1,2}^4 M_{2,2,3} + 4 e^{2\rho t} M_{1,2}^4 M_{1,3}^4 M_{2,2,3} + 4 M_2^4 M_3^4 e^{2\rho t} M_{2,2,3} + 16 M_2^5$  (95)  
 $M_3^3 e^{2\rho t} M_{2,3,3} + 4 M_2^4 M_{1,3}^4 e^{2\rho t} M_{2,2,3} + 16 M_2^5 M_{1,3}^3 e^{2\rho t} M_{2,3,3} - 16 M_{1,2}^5 e^{2\rho t} M_3^3 M_{2,3,3}$   
 $- 16 M_{1,2}^5 e^{2\rho t} M_{1,3}^3 M_{2,3,3} - 96 M_2^3 M_3^2 M_{1,2} M_{1,3} M_{2,3}^2 e^{2\rho t} \rho - 96 M_2^3 M_3 M_{1,2} M_{1,3}^2$   
 $M_{2,3}^2 e^{2\rho t} \rho + 144 M_2^2 M_3^2 M_{1,2}^2 M_{1,3}^2 M_{2,3}^2 e^{2\rho t} \rho + 144 M_2^2 M_3 M_{1,2}^2 M_{1,3}^2 M_{2,3}^2 e^{2\rho t} \rho - 72 M_2^2$

$$\begin{aligned}
& M_3^2 M_{1,2} M_{1,3}^2 M_{2,3} e^{2\rho t} M_{1,2,2} - 144 M_2^2 M_3 M_{1,2}^2 M_{1,3}^2 M_{2,3} e^{2\rho t} M_{1,2,3} + 96 M_2^3 \\
& M_3^2 M_{1,2} M_{1,3} M_{2,3} e^{2\rho t} M_{1,2,3} - 240 M_2^3 M_3 M_{1,2}^2 M_{1,3} M_{2,3} e^{2\rho t} M_{3,3} - 240 M_2^3 M_3 \\
& M_{1,2}^2 M_{1,3} M_{2,3} e^{2\rho t} M_{1,3,3} + 96 M_2^3 M_3 M_{1,2} M_{1,3}^2 M_{2,3} e^{2\rho t} M_{1,2,3} - 96 M_2 M_3^2 M_{1,2}^3 M_{1,3} \\
& M_{2,3}^2 e^{2\rho t} \rho - 96 M_2 M_3 M_{1,2}^3 M_{1,3}^2 M_{2,3}^2 e^{2\rho t} \rho - 144 M_2^2 M_3^2 M_{1,2}^2 M_{1,3} M_{2,3} e^{2\rho t} M_{1,2,3} + 72 \\
& M_2^2 M_3^2 M_{1,2} M_{1,3}^2 M_{2,3} e^{2\rho t} M_{2,2} + 120 M_2^4 M_3 M_{1,2} M_{1,3} M_{2,3} e^{2\rho t} M_{3,3} + 120 \\
& M_2^4 M_3 M_{1,2} M_{1,3} M_{2,3} e^{2\rho t} M_{1,3,3} + 48 M_2^2 M_3^3 M_{1,2} M_{1,3} M_{2,3} e^{2\rho t} M_{2,2} - 48 M_2^2 \\
& M_3^3 M_{1,2} M_{1,3} M_{2,3} e^{2\rho t} M_{1,2,2} + 96 M_2 M_3^2 M_{1,2}^3 M_{1,3} M_{2,3} e^{2\rho t} M_{1,2,3} - 72 M_2 M_3^2 M_{1,2}^2 \\
& M_{1,3}^2 M_{2,3} e^{2\rho t} M_{2,2} + 72 M_2 M_3^2 M_{1,2}^2 M_{1,3}^2 M_{2,3} e^{2\rho t} M_{1,2,2} + 96 M_2 M_3 M_{1,2}^3 \\
& M_{1,3}^2 M_{2,3} e^{2\rho t} M_{1,2,3} - 48 M_2 M_3^3 M_{1,2}^2 M_{1,3} M_{2,3} e^{2\rho t} M_{2,2} + 48 M_2 M_3^3 \\
& M_{1,2}^2 M_{1,3} M_{2,3} e^{2\rho t} M_{1,2,2} - 120 M_2 M_3 M_{1,2}^4 M_{1,3} M_{2,3} e^{2\rho t} M_{3,3} - 120 M_2 M_3 \\
& M_{1,2}^4 M_{1,3} M_{2,3} e^{2\rho t} M_{1,3,3} - 48 M_2 M_3 M_{1,2}^2 M_{1,3}^3 M_{2,3} e^{2\rho t} M_{2,2} + 48 M_2 M_3 M_{1,2}^2 \\
& M_{1,3}^3 M_{2,3} e^{2\rho t} M_{1,2,2} + 240 M_2^2 M_3 M_{1,2}^3 M_{1,3} M_{2,3} e^{2\rho t} M_{3,3} + 240 M_2^2 M_3 \\
& M_{1,2}^3 M_{1,3} M_{2,3} e^{2\rho t} M_{1,3,3} + 48 M_2^2 M_3 M_{1,2} M_{1,3}^3 M_{2,3} e^{2\rho t} M_{2,2} - 48 M_2^2 M_3 M_{1,2} \\
& M_{1,3}^3 M_{2,3} e^{2\rho t} M_{1,2,2} - M_{1,2}^6 M_3^4 M_{2,3,3} - M_{1,2}^6 M_{1,3}^4 M_{2,3,3} - M_2^6 M_{1,3}^4 M_{2,3,3} + M_2^6 \\
& M_{1,3}^3 M_{2,3} M_{3,3} + M_2^6 M_{1,3}^3 M_{2,3} M_{1,3,3} + 24 M_2^4 M_3 e^{2\rho t} \rho M_{1,3}^2 M_{2,3}^2 + 48 M_2^2 M_3^3 e^{2\rho t} \rho M_{1,2}^2 \\
& M_{2,3}^2 + 48 M_2^2 M_{1,3}^3 e^{2\rho t} \rho M_{1,2}^2 M_{2,3}^2 - 32 M_2^3 M_{1,3}^3 e^{2\rho t} \rho M_{1,2} M_{2,3}^2 + 480 M_2^3 M_3^2 \\
& M_{1,2}^2 M_{1,3} e^{2\rho t} M_{2,3,3} - 96 M_2^3 M_3^2 M_{1,2} M_{1,3}^2 e^{2\rho t} M_{2,2,3} + 480 M_2^3 M_3 M_{1,2}^2 M_{1,3}^2 e^{2\rho t} M_{2,3,3} \\
& + 144 M_2^2 M_3^2 M_{1,2}^2 M_{1,3}^2 e^{2\rho t} M_{2,2,3} - 32 e^{2\rho t} \rho M_2 M_3^3 M_{1,2}^2 M_{2,3}^2 - 32 e^{2\rho t} \rho M_2 M_{1,2}^3 M_{1,3}^3 \\
& M_{2,3}^2 + 24 e^{2\rho t} \rho M_3^3 M_{1,2}^4 M_{1,3} M_{2,3}^2 + 24 e^{2\rho t} \rho M_3 M_{1,2}^4 M_{1,3}^2 M_{2,3}^2 + 24 M_2^4 M_3^2 e^{2\rho t} \rho M_{1,3} \\
& M_{2,3}^2 - 32 M_2^3 M_3^3 e^{2\rho t} \rho M_{1,2} M_{2,3}^2 - 24 e^{2\rho t} M_2^4 M_3^2 M_{1,3} M_{2,3} M_{1,2,3} - 24 e^{2\rho t} M_2^4 M_3 \\
& M_{1,3}^2 M_{2,3} M_{1,2,3} - 24 e^{2\rho t} M_3^2 M_{1,2}^4 M_{1,3} M_{2,3} M_{1,2,3} + 24 e^{2\rho t} M_3^2 M_{1,2}^3 M_{1,3}^2 M_{2,2} M_{2,3} \\
& - 24 e^{2\rho t} M_3^2 M_{1,2}^3 M_{1,3}^2 M_{2,3} M_{1,2,2} + 24 e^{2\rho t} M_3 M_{1,2}^5 M_{1,3} M_{2,3} M_{3,3} + 24 e^{2\rho t} M_3 \\
& M_{1,2}^5 M_{1,3} M_{2,3} M_{1,3,3} - 24 e^{2\rho t} M_3 M_{1,2}^4 M_{1,3}^2 M_{2,3} M_{1,2,3} + 16 e^{2\rho t} M_3 M_{1,2}^3 M_{1,3}^3 M_{2,2} M_{2,3} \\
& - 16 e^{2\rho t} M_3 M_{1,2}^3 M_{1,3}^3 M_{2,3} M_{1,2,2} + 32 M_{1,2} e^{2\rho t} M_2^3 M_3^3 M_{2,3} M_{1,2,3} + 32 M_{1,2} e^{2\rho t} M_2^3 \\
& M_{1,3}^3 M_{2,3} M_{1,2,3} - 240 M_2^4 M_3^2 M_{1,2} M_{1,3} e^{2\rho t} M_{2,3,3} - 240 M_2^4 M_3 M_{1,2} M_{1,3}^2 e^{2\rho t} M_{2,3,3} \\
& - 64 M_2^3 M_3^3 M_{1,2} M_{1,3} e^{2\rho t} M_{2,2,3} - 64 M_2^2 M_3 M_{1,2} M_{1,3}^3 e^{2\rho t} M_{2,2,3} + 96 M_2^2 M_3^3 \\
& M_{1,2}^2 M_{1,3} e^{2\rho t} M_{2,2,3} - 480 M_2^2 M_3^2 M_{1,2}^3 M_{1,3} e^{2\rho t} M_{2,3,3} - 480 M_2^2 M_3 M_{1,2}^3 \\
& M_{1,3}^2 e^{2\rho t} M_{2,3,3} - 96 M_2 M_3^2 M_{1,2}^3 M_{1,3} e^{2\rho t} M_{2,2,3} - 64 M_2 M_3^3 M_{1,2}^3 M_{1,3} e^{2\rho t} M_{2,2,3}
\end{aligned}$$



$$\begin{aligned}
& + 240 M_2 M_3^2 M_{1,2}^4 M_{1,3} e^{2\rho t} M_{2,3,3} + 240 M_2 M_3 M_{1,2}^4 M_{1,3}^2 e^{2\rho t} M_{2,3,3} - 64 M_2 M_3 M_{1,2}^3 M_{1,3} e^{2\rho t} M_{2,2,3} + 96 M_2^2 M_3 M_{1,2}^2 M_{1,3}^3 e^{2\rho t} M_{2,2,3} - 24 M_2^5 M_3 e^{2\rho t} M_{1,3} M_{2,3} M_{1,3,3} - 16 \\
& M_2^3 M_3 e^{2\rho t} M_{1,3}^3 M_{2,2} M_{2,3} + 16 M_2^2 M_3 e^{2\rho t} M_{1,3}^3 M_{2,3} M_{1,2,2} + 12 M_2^2 M_3^2 e^{2\rho t} M_{1,2} M_{2,2} M_{2,3} - 12 M_2^2 M_3^4 e^{2\rho t} M_{1,2} M_{2,3} M_{1,2,2} + 120 M_2^2 M_3^2 e^{2\rho t} M_{1,2}^3 M_{2,3} M_{3,3} \\
& + 120 M_2^2 M_3^2 e^{2\rho t} M_{1,2}^3 M_{2,3} M_{1,3,3} - 24 M_2^5 M_3 e^{2\rho t} M_{1,3} M_{2,3} M_{3,3} + 60 M_2^4 M_{1,3}^2 e^{2\rho t} M_{1,2} M_{2,3} M_{3,3} - 48 e^{2\rho t} M_2^2 M_3^3 M_{1,2}^2 M_{2,3} M_{1,2,3} - 48 e^{2\rho t} M_2^2 M_{1,2}^2 \\
& M_{1,3}^3 M_{2,3} M_{1,2,3} - 12 e^{2\rho t} M_2 M_3^4 M_{1,2}^2 M_{2,2} M_{2,3} + 12 e^{2\rho t} M_2 M_3^4 M_{1,2}^2 M_{2,3} M_{1,2,2} + 32 e^{2\rho t} M_2 M_3^3 M_{1,2}^3 M_{2,3} M_{1,2,3} - 60 e^{2\rho t} M_2 M_3^3 M_{1,2}^4 M_{2,3} M_{3,3} - 60 e^{2\rho t} M_2 M_3^2 \\
& M_{1,2}^4 M_{2,3} M_{1,3,3} - 60 e^{2\rho t} M_2 M_{1,2}^4 M_{1,3}^2 M_{2,3} M_{3,3} - 60 e^{2\rho t} M_2 M_{1,2}^4 M_{1,3}^2 M_{2,3} M_{1,3,3} + 32 e^{2\rho t} M_2 M_{1,2}^3 M_{1,3}^3 M_{2,3} M_{1,2,3} - 12 e^{2\rho t} M_2 M_{1,2}^2 M_{1,3}^4 M_{2,2} M_{2,3} + 12 e^{2\rho t} M_2 M_{1,2}^2 \\
& M_{1,3}^4 M_{2,3} M_{1,2,2} + 16 e^{2\rho t} M_3^3 M_{1,2}^3 M_{1,3} M_{2,2} M_{2,3} - 16 e^{2\rho t} M_3^3 M_{1,2}^3 M_{1,3} M_{2,3} M_{1,2,2} + 60 M_2^4 M_{1,3}^2 e^{2\rho t} M_{1,2} M_{2,3} M_{1,3,3} - 120 M_2^3 M_{1,3}^2 e^{2\rho t} M_{1,2}^2 M_{2,3} M_{3,3} - 120 M_2^2 \\
& M_{1,3}^2 e^{2\rho t} M_{1,2}^2 M_{2,3} M_{1,3,3} + 120 M_2^2 M_{1,3}^2 e^{2\rho t} M_{1,2}^2 M_{2,3} M_{3,3} + 120 M_2^2 M_{1,3}^2 e^{2\rho t} M_{1,2}^2 M_{2,3} M_{1,3,3} + 12 M_2^2 M_{1,3}^4 e^{2\rho t} M_{1,2} M_{2,2} M_{2,3} - 12 M_2^2 M_{1,3}^4 e^{2\rho t} M_{1,2} M_{2,3} M_{1,2,2} \\
& - 16 M_2^3 M_3^3 e^{2\rho t} M_{1,3} M_{2,2} M_{2,3} + 16 M_2^3 M_3^3 e^{2\rho t} M_{1,3} M_{2,3} M_{1,2,2} - 120 M_2^3 M_3^2 e^{2\rho t} M_{1,2} M_{2,3} M_{3,3} - 120 M_2^3 M_3^2 e^{2\rho t} M_{1,2}^2 M_{2,3} M_{1,3,3} - 24 M_2^3 M_3^2 e^{2\rho t} M_{1,3}^2 M_{2,2} M_{2,3} + 24 \\
& M_2^3 M_3^2 e^{2\rho t} M_{1,3}^2 M_{2,3} M_{1,2,2} + 60 M_2^4 M_3^2 e^{2\rho t} M_{1,2} M_{2,3} M_{3,3} + 60 M_2^4 M_3^2 e^{2\rho t} M_{1,2} M_{2,3} M_{1,3,3} + 80 M_2^3 M_3^3 M_{1,2}^3 M_{1,3} M_{2,3,3} + 80 M_2^3 M_3^3 M_{1,2}^3 M_{1,3}^3 M_{2,3,3} - 90 \\
& M_2^2 M_3^2 M_{1,2}^4 M_{1,3}^2 M_{2,3,3} + 45 M_2^2 M_3^2 M_{1,2}^4 M_{1,3} M_{2,3} M_{3,3} + 45 M_2^2 M_3^2 M_{1,2}^4 M_{1,3} M_{2,3} M_{1,3,3} + 45 M_2^2 M_3 M_{1,2}^4 M_{1,3}^2 M_{2,3} M_{3,3} + 45 M_2^2 M_3 M_{1,2}^4 M_{1,3}^2 M_{2,3} M_{1,3,3} + M_3^3 M_{1,2}^6 M_{2,3} M_{3,3} \\
& + M_3^3 M_{1,2}^6 M_{2,3} M_{1,3,3} + M_{1,2}^6 M_{1,3}^3 M_{2,3} M_{3,3} + M_{1,2}^6 M_{1,3}^3 M_{2,3} M_{1,3,3} - M_2^6 M_3^4 M_{2,3,3} + M_2^6 M_3^3 M_{2,3} M_{3,3} + M_2^6 M_3^3 M_{2,3} M_{1,3,3} + 15 M_2^4 M_{1,3}^3 M_{1,2}^2 M_{2,3} M_{3,3} + 15 M_2^4 M_{1,3}^3 \\
& M_{1,2}^2 M_{2,3} M_{1,3,3} - 20 M_2^3 M_{1,3}^3 M_{1,2}^3 M_{2,3} M_{3,3} - 20 M_2^3 M_{1,3}^3 M_{1,2}^3 M_{2,3} M_{1,3,3} - 6 M_2 M_3^3 M_{1,2}^5 M_{2,3} M_{3,3} - 6 M_2 M_3^3 M_{1,2}^5 M_{2,3} M_{1,3,3} - 6 M_2 M_{1,2}^5 \\
& M_{1,3}^3 M_{2,3} M_{1,3,3} - 256 e^{8\rho t} M_2^2 M_{2,3,3} - 256 M_{1,2}^2 e^{8\rho t} M_{2,3,3} + 1024 e^{10\rho t} M_{2,2,3} - 160 M_{1,2}^3 e^{2\rho t} M_2^2 M_3^3 M_{2,3,3} - 160 M_{1,2}^3 e^{2\rho t} M_2^2 M_{1,3}^3 M_{2,3,3} + 80 M_{1,2}^4 e^{2\rho t} M_2 M_3^3 M_{2,3,3} + 80 \\
& M_{1,2}^4 e^{2\rho t} M_2 M_{1,3}^3 M_{2,3,3} - 48 M_{1,2}^5 e^{2\rho t} M_3^2 M_{1,3} M_{2,3,3} - 48 M_{1,2}^5 e^{2\rho t} M_3 M_{1,3}^2 M_{2,3,3} + 24 e^{2\rho t} M_3^2 M_{1,2}^4 M_{1,3}^2 M_{2,2,3} + 16 e^{2\rho t} M_3 M_{1,2}^4 M_{1,3}^3 M_{2,2,3} + 8 e^{2\rho t} M_3^3 M_{1,2}^4 M_{2,2,3}
\end{aligned}$$

$$\begin{aligned}
& + 8 e^{2\rho t} \rho M_{1,2}^4 M_{1,3}^3 M_{2,3}^2 + 8 M_2^4 M_{1,3}^3 e^{2\rho t} \rho M_{2,3}^2 + 8 M_2^4 M_3^3 e^{2\rho t} \rho M_{2,3}^2 + 160 M_{1,2}^2 e^{2\rho t} \\
& M_2^3 M_3^3 M_{2,3,3} + 160 M_{1,2}^2 e^{2\rho t} M_2^3 M_{1,3}^3 M_{2,3,3} + 4 e^{2\rho t} M_3^4 M_{1,2}^3 M_{2,2} M_{2,3} - 4 e^{2\rho t} M_3^4 \\
& M_{1,2}^3 M_{2,3} M_{1,2,2} - 8 e^{2\rho t} M_3^3 M_{1,2}^4 M_{2,3} M_{1,2,3} + 12 e^{2\rho t} M_3^2 M_{1,2}^5 M_{2,3} M_{3,3} + 12 e^{2\rho t} M_3^2 \\
& M_{1,2}^5 M_{2,3} M_{1,3,3} + 12 e^{2\rho t} M_{1,2}^5 M_{1,3}^2 M_{2,3} M_{3,3} + 12 e^{2\rho t} M_{1,2}^5 M_{1,3}^2 M_{2,3} M_{1,3,3} - 8 e^{2\rho t} \\
& M_{1,2}^4 M_{1,3}^3 M_{2,3} M_{1,2,3} + 4 e^{2\rho t} M_{1,2}^3 M_{1,3}^4 M_{2,2} M_{2,3} - 4 e^{2\rho t} M_{1,2}^3 M_{1,3}^4 M_{2,3} M_{1,2,2} - 4 M_2^3 \\
& M_3^4 e^{2\rho t} M_{2,2} M_{2,3} + 4 M_2^3 M_3^4 e^{2\rho t} M_{2,3} M_{1,2,2} - 12 M_2^5 M_3^2 e^{2\rho t} M_{2,3} M_{3,3} - 12 M_2^5 \\
& M_3^2 e^{2\rho t} M_{2,3} M_{1,3,3} - 12 M_2^5 M_{1,3}^2 e^{2\rho t} M_{2,3} M_{1,3,3} - 4 M_2^3 M_{1,3}^4 e^{2\rho t} M_{2,2} M_{2,3} + 4 M_2^3 \\
& M_{1,3}^4 e^{2\rho t} M_{2,3} M_{1,2,2} - 12 M_2^5 M_{1,3}^2 e^{2\rho t} M_{2,3} M_{3,3} - 8 e^{2\rho t} M_2^4 M_3^3 M_{2,3} M_{1,2,3} - 8 e^{2\rho t} M_2^4 \\
& M_{1,3}^3 M_{2,3} M_{1,2,3} + 24 M_2^4 M_3^2 e^{2\rho t} M_{1,3}^2 M_{2,2,3} - 90 M_2^4 M_3^2 M_{1,2}^2 M_{1,3}^2 M_{2,3,3} + 45 M_2^4 M_3^2 \\
& M_{1,2}^2 M_{1,3}^2 M_{2,3} M_{3,3} + 45 M_2^4 M_3^2 M_{1,2}^2 M_{1,3}^2 M_{2,3} M_{1,3,3} + 45 M_2^4 M_3^2 M_{1,2}^2 M_{1,3}^2 M_{2,3} M_{3,3} \\
& + 45 M_2^4 M_3^2 M_{1,2}^2 M_{1,3}^2 M_{2,3} M_{1,3,3} + 120 M_2^3 M_3^3 M_{1,2}^2 M_{1,3}^2 M_{2,3,3} - 60 M_2^3 M_3^3 \\
& M_{1,2}^3 M_{1,3}^2 M_{2,3} M_{3,3} - 60 M_2^3 M_3^3 M_{1,2}^3 M_{1,3}^2 M_{2,3} M_{1,3,3} - 60 M_2^3 M_3^3 M_{1,2}^3 M_{1,3}^2 M_{2,3} M_{3,3} \\
& - 60 M_2^3 M_3^3 M_{1,2}^3 M_{1,3}^2 M_{2,3} M_{1,3,3} + 24 M_2^5 M_3^3 M_{1,2} M_{1,3} M_{2,3,3} + 24 M_2^5 M_3^3 M_{1,2} \\
& M_{1,3} M_{2,3,3} - 60 M_2^2 M_3^3 M_{1,2}^4 M_{1,3} M_{2,3,3} - 60 M_2^2 M_3^3 M_{1,2}^4 M_{1,3} M_{2,3,3} + 36 M_2 M_3^2 M_{1,2}^5 \\
& M_{1,3}^2 M_{2,3,3} - 18 M_2 M_3^2 M_{1,2}^5 M_{1,3} M_{2,3} M_{3,3} - 18 M_2 M_3^2 M_{1,2}^5 M_{1,3} M_{2,3} M_{1,3,3} \\
& - 18 M_2 M_3^2 M_{1,2}^5 M_{1,3} M_{2,3} M_{3,3} - 18 M_2 M_3^2 M_{1,2}^5 M_{1,3} M_{2,3} M_{1,3,3} + 24 M_2 M_3^3 \\
& M_{1,2}^5 M_{1,3} M_{2,3,3} + 24 M_2 M_3^3 M_{1,2}^5 M_{1,3} M_{2,3,3} + 36 M_2^5 M_3^2 M_{1,2} M_{1,3}^2 M_{2,3,3} - 18 M_2^5 \\
& M_3^2 M_{1,2} M_{1,3} M_{2,3} M_{3,3} - 18 M_2^5 M_3^2 M_{1,2} M_{1,3} M_{2,3} M_{1,3,3} - 18 M_2^5 M_3^2 M_{1,2} M_{1,3} M_{2,3} M_{3,3} \\
& - 18 M_2^5 M_3^2 M_{1,2} M_{1,3} M_{2,3} M_{1,3,3} - 60 M_2^4 M_3^3 M_{1,2}^2 M_{1,3} M_{2,3,3} - 60 M_2^4 M_3^3 M_{1,2}^2 \\
& M_{1,3} M_{2,3,3} + 16 M_2^4 M_3^3 e^{2\rho t} M_{1,3}^3 M_{2,2,3} + 24 M_2^2 M_3^4 e^{2\rho t} M_{1,2}^2 M_{2,2,3} + 48 M_2^5 M_3^3 e^{2\rho t} \\
& M_{1,3}^2 M_{2,3,3} - 80 M_2^4 M_{1,3}^3 e^{2\rho t} M_{1,2} M_{2,3,3} - 16 e^{2\rho t} M_2 M_3^4 M_{1,2}^3 M_{2,2,3} - 16 e^{2\rho t} M_2 M_{1,2}^3 \\
& M_{2,2,3} + 16 e^{2\rho t} M_3^3 M_{1,2}^4 M_{1,3} M_{2,2,3} - 16 M_2^3 M_{1,3}^4 e^{2\rho t} M_{1,2} M_{2,2,3} + 24 M_2^2 \\
& M_{1,3}^4 e^{2\rho t} M_{1,2}^2 M_{2,2,3} - 16 M_2^3 M_3^4 e^{2\rho t} M_{1,2} M_{2,2,3} + 48 M_2^5 M_3^2 e^{2\rho t} M_{1,3} M_{2,3,3} - 80 M_2^4 \\
& M_3^3 e^{2\rho t} M_{1,2} M_{2,3,3} + 16 M_2^4 M_3^3 e^{2\rho t} M_{1,3} M_{2,2,3} + 288 M_2^2 M_{1,3}^4 e^{4\rho t} M_{1,2}^2 M_{2,3} M_{3,3} + 288 \\
& M_2^2 M_{1,3}^4 e^{4\rho t} M_{1,2}^2 M_{2,3} M_{1,3,3} + 192 M_2^3 M_3^4 e^{4\rho t} M_{1,3} M_{2,3} M_{1,2,3} - 288 M_2^2 \\
& M_3^2 e^{4\rho t} M_{1,2} M_{2,3} M_{1,2,3} + 144 M_2^2 M_3^2 e^{4\rho t} M_{1,3} M_{2,2} M_{2,3} - 144 M_2^2 \\
& M_3^2 e^{4\rho t} M_{1,3} M_{2,3} M_{1,2,2} - 192 M_2^3 M_3^4 e^{4\rho t} M_{1,2} M_{2,3} M_{3,3} - 192 \\
& M_2^3 M_3^4 e^{4\rho t} M_{1,2} M_{2,3} M_{1,3,3} - 1536 M_{1,2} e^{6\rho t} M_2 M_3 M_{1,3} M_{2,2,3} - 576 M_2 M_3^2
\end{aligned}$$

$$\begin{aligned}
& M_{1,2}^2 M_{1,3} e^{4\rho t} M_{2,2,3} + 768 M_2 M_3 M_{1,2}^3 M_{1,3} e^{4\rho t} M_{2,3,3} - 576 M_2 M_3 M_{1,2}^2 M_{1,3}^2 e^{4\rho t} M_{2,2,3} \\
& - 96 M_{1,2} e^{4\rho t} M_2 M_3^3 M_{2,2} M_{2,3} + 96 M_{1,2} e^{4\rho t} M_2 M_3^3 M_{2,3} M_{1,2,2} - 96 M_{1,2} e^{4\rho t} M_2 \\
& M_{1,3}^3 M_{2,2} M_{2,3} + 96 M_{1,2} e^{4\rho t} M_2 M_{1,3}^3 M_{2,3} M_{1,2,2} + 288 e^{4\rho t} M_2 M_3^2 M_{1,2}^2 M_{2,3} M_{1,2,3} \\
& - 192 e^{4\rho t} M_2 M_3 M_{1,2}^3 M_{2,3} M_{3,3} - 192 e^{4\rho t} M_2 M_3 M_{1,2}^2 M_{2,3} M_{1,3,3} - 192 e^{4\rho t} M_2 \\
& M_{1,2}^3 M_{1,3} M_{2,3} M_{3,3} - 192 e^{4\rho t} M_2 M_{1,2}^3 M_{1,3} M_{2,3} M_{1,3,3} + 288 e^{4\rho t} M_2 M_{1,2}^2 \\
& M_{1,3}^2 M_{2,3} M_{1,2,3} - 384 M_2 e^{6\rho t} M_3 M_{1,3} M_{2,2} M_{2,3} + 384 M_2 e^{6\rho t} M_3 M_{1,3} M_{2,3} M_{1,2,2} \\
& - 192 M_2^3 M_{1,3} e^{4\rho t} M_{1,2} M_{2,3} M_{3,3} - 192 M_2^3 M_{1,3} e^{4\rho t} M_{1,2} M_{2,3} M_{1,3,3} - 288 M_2^2 \\
& M_{1,3}^2 e^{4\rho t} M_{1,2} M_{2,3} M_{1,2,3} - 288 e^{4\rho t} \rho M_2 M_{1,2}^2 M_{1,3}^2 M_{2,3}^2 + 192 e^{4\rho t} \rho M_3 M_{1,2}^3 M_{1,3} M_{2,3}^2 \\
& + 144 e^{4\rho t} M_3^2 M_{1,2}^2 M_{1,3} M_{2,2} M_{2,3} - 144 e^{4\rho t} M_3^2 M_{1,2}^2 M_{1,3} M_{2,3} M_{1,2,2} - 192 e^{4\rho t} M_3 \\
& M_{1,2}^3 M_{1,3} M_{2,3} M_{1,2,3} + 144 e^{4\rho t} M_3 M_{1,2}^2 M_{1,3}^2 M_{2,2} M_{2,3} - 144 e^{4\rho t} M_3 M_{1,2}^2 \\
& M_{1,3}^2 M_{2,3} M_{1,2,2} + 768 M_{1,2} e^{6\rho t} M_2 M_3 M_{2,3} M_{1,2,3} + 768 M_{1,2} e^{6\rho t} M_2 M_{1,3} M_{2,3} M_{1,2,3} \\
& + 384 M_{1,2} e^{6\rho t} M_3 M_{1,3} M_{2,2} M_{2,3} - 384 M_{1,2} e^{6\rho t} M_3 M_{1,3} M_{2,3} M_{1,2,2} - 1152 M_2^2 M_3 \\
& M_{1,2}^2 M_{1,3} e^{4\rho t} M_{2,3,3} + 576 M_2^2 M_3 M_{1,2} M_{1,3}^2 e^{4\rho t} M_{2,2,3} - 288 e^{4\rho t} \rho M_2 M_3^2 M_{1,2}^2 M_{2,3}^2 \\
& + 144 M_2^2 M_3 e^{4\rho t} M_{1,3}^2 M_{2,2} M_{2,3} - 144 M_2^2 M_3 e^{4\rho t} M_{1,3}^2 M_{2,3} M_{1,2,2} - 192 \\
& M_2^3 M_3 e^{4\rho t} \rho M_{1,3} M_{2,3}^2 + 288 M_2^2 M_3^2 e^{4\rho t} \rho M_{1,2} M_{2,3}^2 + 288 M_2^2 M_{1,3}^2 e^{4\rho t} \rho M_{1,2} M_{2,3}^2 \\
& - 768 M_{1,2} e^{6\rho t} \rho M_2 M_3 M_{2,3}^2 - 768 M_{1,2} e^{6\rho t} \rho M_2 M_{1,3} M_{2,3}^2 + 768 \\
& M_2^3 M_3 M_{1,2} M_{1,3} e^{4\rho t} M_{2,3,3} + 576 M_2^2 M_3^2 M_{1,2} M_{1,3} e^{4\rho t} M_{2,2,3} + 288 M_2^2 M_3 e^{4\rho t} \\
& M_{1,2}^2 M_{2,3} M_{3,3} + 288 M_2^2 M_3 e^{4\rho t} M_{1,2}^2 M_{2,3} M_{1,3,3} + 576 M_2 M_3 M_{1,2}^2 M_{1,3} M_{2,3} e^{4\rho t} M_{1,2,3} \\
& - 576 M_2 M_3 M_{1,2}^2 M_{1,3} M_{2,3}^2 e^{4\rho t} \rho + 576 M_2^2 M_3 M_{1,2} M_{1,3} M_{2,3}^2 e^{4\rho t} \rho - 288 M_{1,2} e^{4\rho t} M_2 \\
& M_3^2 M_{1,3} M_{2,2} M_{2,3} + 288 M_{1,2} e^{4\rho t} M_2 M_3^2 M_{1,3} M_{2,3} M_{1,2,2} - 288 M_{1,2} e^{4\rho t} M_2 M_3 \\
& M_{1,3}^2 M_{2,2} M_{2,3} + 288 M_{1,2} e^{4\rho t} M_2 M_3 M_{1,3}^2 M_{2,3} M_{1,2,2} - 576 \\
& M_2^2 M_3 M_{1,2} M_{1,3} M_{2,3} e^{4\rho t} M_{1,2,3} + 96 e^{4\rho t} \rho M_{1,2}^3 M_{1,3}^2 M_{2,3}^2 + 384 e^{6\rho t} \rho M_3 M_{1,2}^2 M_{2,3}^2 \\
& + 384 e^{6\rho t} \rho M_{1,2}^2 M_{1,3} M_{2,3}^2 + 384 M_2^2 M_{1,3} e^{6\rho t} \rho M_{2,3}^2 - 96 M_2^3 M_{1,3}^2 e^{4\rho t} \rho M_{2,3}^2 - 96 M_2^3 \\
& M_3^2 e^{4\rho t} \rho M_{2,3}^2 + 384 M_2^2 M_3 e^{6\rho t} \rho M_{2,3}^2 + 768 M_{1,2}^2 e^{6\rho t} M_2 M_{1,3} M_{2,3,3} + 768 e^{6\rho t} M_3 \\
& M_{1,2}^2 M_{1,3} M_{2,2,3} - 768 M_{1,2} e^{6\rho t} M_2 M_{1,3}^2 M_{2,2,3} + 192 M_2^2 M_{1,3}^3 e^{4\rho t} M_{1,2} M_{2,2,3} - 576 \\
& M_{1,2}^2 e^{4\rho t} M_2^2 M_3^2 M_{2,3,3} - 576 M_{1,2}^2 e^{4\rho t} M_2^2 M_{1,3}^2 M_{2,3,3} - 768 M_{1,2} e^{6\rho t} M_2 M_3^2 M_{2,2,3} \\
& - 192 e^{4\rho t} M_2 M_3^3 M_{1,2}^2 M_{2,2,3} - 192 e^{4\rho t} M_2 M_{1,2}^2 M_{1,3}^3 M_{2,2,3} + 96 e^{4\rho t} \rho M_3^3 M_{1,2}^2 M_{2,3}^2 \\
& + 48 e^{4\rho t} M_{1,2}^4 M_{1,3} M_{2,3} M_{1,3,3} - 96 e^{4\rho t} M_{1,2}^3 M_{1,3}^2 M_{2,3} M_{1,2,3} + 48 e^{4\rho t} M_{1,2}^2
\end{aligned}$$

$$\begin{aligned}
& M_{1,3}^3 M_{2,2} M_{2,3} - 48 e^{4\rho t} M_{1,2}^2 M_{1,3}^3 M_{2,3} M_{1,2,2} - 192 e^{6\rho t} M_2 M_{1,2}^2 M_{2,3} M_{3,3} \\
& - 192 e^{6\rho t} M_2 M_{1,2}^2 M_{2,3} M_{1,3,3} - 384 e^{6\rho t} M_3 M_{1,2}^2 M_{2,3} M_{1,2,3} - 384 e^{6\rho t} \\
& M_{1,2}^2 M_{1,3} M_{2,3} M_{1,2,3} + 96 M_2^3 M_3^2 e^{4\rho t} M_{2,3} M_{1,2,3} + 192 e^{4\rho t} M_3^2 M_{1,2}^3 M_{1,3} M_{2,2,3} \\
& + 192 e^{4\rho t} M_3 M_{1,2}^3 M_{1,3}^2 M_{2,2,3} - 48 e^{4\rho t} M_3^3 M_{1,2}^2 M_{2,3} M_{1,2,2} - 96 e^{4\rho t} M_3^2 \\
& M_{1,2}^3 M_{2,3} M_{1,2,3} + 48 e^{4\rho t} M_3 M_{1,2}^4 M_{2,3} M_{3,3} + 48 e^{4\rho t} M_3 M_{1,2}^4 M_{2,3} M_{1,3,3} + 48 e^{4\rho t} \\
& M_{1,2}^4 M_{1,3} M_{2,3} M_{3,3} + 6 M_2^5 M_{1,3}^4 M_{1,2} M_{2,3,3} - 6 M_2^5 M_{1,3}^3 M_{1,2} M_{2,3} M_{3,3} - 6 M_2^5 \\
& M_{1,3}^3 M_{1,2} M_{2,3} M_{1,3,3} - 20 M_2^3 M_3^3 M_{1,2}^3 M_{2,3} M_{3,3} - 20 M_2^3 M_3^3 M_{1,2}^3 M_{2,3} M_{1,3,3} - 4 M_2^6 \\
& M_{1,3}^3 M_{1,3} M_{2,3,3} - 6 M_2^6 M_3^2 M_{1,3}^2 M_{2,3,3} + 3 M_2^6 M_3^2 M_{1,3} M_{2,3} M_{3,3} + 3 M_2^6 \\
& M_3^2 M_{1,3} M_{2,3} M_{1,3,3} + 6 M_2^5 M_3^4 M_{1,2} M_{2,3,3} - 6 M_2^5 M_3^3 M_{1,2} M_{2,3} M_{3,3} - 6 M_2^5 \\
& M_3^3 M_{1,2} M_{2,3} M_{1,3,3} + 15 M_2^4 M_3^3 M_{1,2}^2 M_{2,3} M_{3,3} + 15 M_2^4 M_3^3 M_{1,2}^2 M_{2,3} M_{1,3,3} \\
& + 512 M_{1,2} e^{8\rho t} \rho M_{2,3}^2 - 512 M_2 e^{8\rho t} \rho M_{2,3}^2 - 96 M_2^4 M_3^2 e^{4\rho t} M_{2,3,3} - 64 M_2^3 \\
& M_3^3 e^{4\rho t} M_{2,2,3} + 64 e^{6\rho t} M_{1,2}^3 M_{2,3} M_{3,3} + 64 e^{6\rho t} M_{1,2}^3 M_{2,3} M_{1,3,3} \\
& + 256 e^{8\rho t} M_3 M_{2,2} M_{2,3} - 256 e^{8\rho t} M_3 M_{2,3} M_{1,2,2} + 256 e^{8\rho t} M_{1,3} M_{2,2} M_{2,3} \\
& - 256 e^{8\rho t} M_{1,3} M_{2,3} M_{1,2,2} - 64 e^{6\rho t} M_2^3 M_{2,3} M_{3,3} - 64 e^{6\rho t} M_2^3 M_{2,3} M_{1,3,3} \\
& + 512 M_2 e^{8\rho t} M_{2,3} M_{1,2,3} - 512 M_{1,2} e^{8\rho t} M_{2,3} M_{1,2,3} - 4 M_2^6 M_3 M_{1,3}^3 M_{2,3,3} + 3 M_2^6 M_3 \\
& M_{1,3}^2 M_{2,3} M_{3,3} + 3 M_2^6 M_3 M_{1,3}^2 M_{2,3} M_{1,3,3} + 15 M_2^2 M_3^3 M_{1,2}^4 M_{2,3} M_{3,3} + 15 M_2^2 M_3^3 \\
& M_{1,2}^4 M_{2,3} M_{1,3,3} + 3 M_2^2 M_{1,2}^6 M_{1,3} M_{2,3} M_{3,3} + 3 M_2^2 M_{1,2}^6 M_{1,3} M_{2,3} M_{1,3,3} + 3 M_3 M_{1,2}^6 \\
& M_{1,3}^2 M_{2,3} M_{3,3} + 3 M_3 M_{1,2}^6 M_{1,3}^2 M_{2,3} M_{1,3,3} + 20 M_{1,2}^3 M_3^3 M_{2,3,3}^4 + 20 M_{1,2}^3 M_3^3 \\
& M_{1,2}^4 M_{2,3,3} - 15 M_{1,2}^4 M_2^2 M_3^4 M_{2,3,3} - 15 M_{1,2}^4 M_2^2 M_{1,3}^4 M_{2,3,3} + 6 M_{1,2}^5 M_2 M_3^4 M_{2,3,3} + 6 \\
& M_{1,2}^5 M_2 M_{1,3}^4 M_{2,3,3} - 4 M_{1,2}^6 M_3^3 M_{1,3} M_{2,3,3} - 6 M_{1,2}^6 M_3^2 M_{1,3}^2 M_{2,3,3} - 4 M_{1,2}^6 M_3 \\
& M_{1,3}^3 M_{2,3,3} - 15 M_{1,2}^2 M_2^4 M_3^4 M_{2,3,3} - 15 M_{1,2}^2 M_2^4 M_{1,3}^4 M_{2,3,3} - 96 M_{1,2}^4 e^{4\rho t} M_{1,3}^2 M_{2,3,3} \\
& + 64 e^{4\rho t} M_3^3 M_{1,2}^3 M_{2,2,3} + 64 e^{4\rho t} M_{1,2}^3 M_{1,3}^3 M_{2,2,3} + 384 e^{6\rho t} M_3^2 M_{1,2}^2 M_{2,2,3} \\
& + 384 e^{6\rho t} M_{1,2}^2 M_{1,3}^2 M_{2,2,3} - 256 M_{1,2}^3 e^{6\rho t} M_3 M_{2,3,3} - 256 M_{1,2}^3 e^{6\rho t} M_{1,3} M_{2,3,3} - 96 \\
& M_2^4 M_{1,3}^2 e^{4\rho t} M_{2,3,3} - 64 M_2^2 M_{1,3}^3 e^{4\rho t} M_{2,2,3} + 512 M_{1,2} e^{8\rho t} M_2 M_{2,3,3} \\
& + 1024 M_{1,2} e^{8\rho t} M_3 M_{2,2,3} + 1024 M_{1,2} e^{8\rho t} M_{1,3} M_{2,2,3} - 1024 M_2 e^{8\rho t} M_3 M_{2,2,3} \\
& - 1024 M_2 e^{8\rho t} M_{1,3} M_{2,2,3} - 96 M_{1,2}^4 e^{4\rho t} M_3^2 M_{2,3,3} + 256 M_2^3 M_3 e^{6\rho t} M_{2,3,3} + 384 M_2^2 \\
& M_3^2 e^{6\rho t} M_{2,2,3} + 256 M_2^3 M_{1,3} e^{6\rho t} M_{2,3,3} + 384 M_2^2 M_{1,3}^2 e^{6\rho t} M_{2,2,3} + 15 M_2^2 M_{1,3}^3 \\
& M_{1,2}^4 M_{2,3} M_{3,3} + 15 M_2^2 M_{1,3}^3 M_{1,2}^4 M_{2,3} M_{1,3,3} - 192 M_2^4 M_3 e^{4\rho t} M_{1,3} M_{2,3,3} - 192
\end{aligned}$$

$$\begin{aligned}
& M_2^3 M_3 e^{4\rho t} M_{1,3}^2 M_{2,2,3} + 192 M_2^2 M_3^3 e^{4\rho t} M_{1,2} M_{2,2,3} + 384 M_2^3 M_{1,3}^2 e^{4\rho t} M_{1,2} M_{2,3,3} \\
& - 768 M_2^2 M_{1,3} e^{6\rho t} M_{1,2} M_{2,3,3} + 384 M_2^3 M_3^2 e^{4\rho t} M_{1,2} M_{2,3,3} - 192 M_2^3 \\
& M_3^2 e^{4\rho t} M_{1,3} M_{2,2,3} - 192 M_{1,2} e^{6\rho t} M_{1,3}^2 M_{2,3} M_{1,2,2} - 192 M_2 e^{6\rho t} M_3^2 M_{2,2} M_{2,3} \\
& + 192 M_2 e^{6\rho t} M_3^2 M_{2,3} M_{1,2,2} - 192 M_2 e^{6\rho t} M_{1,3}^2 M_{2,2} M_{2,3} + 192 M_2 e^{6\rho t} \\
& M_{1,3}^2 M_{2,3} M_{1,2,2} + 48 e^{4\rho t} M_3^3 M_{1,2}^2 M_{2,2} M_{2,3} - 768 M_2^2 M_3 e^{6\rho t} M_{1,2} M_{2,3,3} + 768 \\
& M_2^2 M_3 e^{6\rho t} M_{1,3} M_{2,2,3} + 384 M_{1,2}^3 e^{4\rho t} M_2 M_3^2 M_{2,3,3} + 384 M_{1,2}^3 e^{4\rho t} M_2 M_{1,3}^2 M_{2,3,3} \\
& - 192 M_{1,2}^4 e^{4\rho t} M_3 M_{1,3} M_{2,3,3} + 768 M_{1,2}^2 e^{6\rho t} M_2 M_3 M_{2,3,3} + 48 M_2^4 M_{1,3} e^{4\rho t} M_{2,3} M_{3,3} \\
& + 48 M_2^4 M_{1,3} e^{4\rho t} M_{2,3} M_{1,3,3} + 48 M_2^2 M_{1,3}^3 e^{4\rho t} M_{2,2} M_{2,3} - 48 M_2^2 M_{1,3}^3 e^{4\rho t} M_{2,3} M_{1,2,2} \\
& - 384 M_2^2 M_{1,3} e^{6\rho t} M_{2,3} M_{1,2,3} + 96 M_2^3 M_{1,3}^2 e^{4\rho t} M_{2,3} M_{1,2,3} + 192 M_{1,2} e^{6\rho t} \\
& M_2^2 M_{2,3} M_{3,3} + 192 M_{1,2} e^{6\rho t} M_2^2 M_{2,3} M_{1,3,3} + 192 M_{1,2} e^{6\rho t} M_3^2 M_{2,2} M_{2,3} \\
& - 192 M_{1,2} e^{6\rho t} M_3^2 M_{2,3} M_{1,2,2} + 192 M_{1,2} e^{6\rho t} M_{1,3}^2 M_{2,2} M_{2,3} + 48 M_2^4 M_3 e^{4\rho t} M_{2,3} M_{3,3} \\
& + 48 M_2^4 M_3 e^{4\rho t} M_{2,3} M_{1,3,3} + 48 M_2^2 M_3^3 e^{4\rho t} M_{2,2} M_{2,3} - 48 M_2^2 M_3^3 e^{4\rho t} M_{2,3} M_{1,2,2} \\
& - 384 M_2^2 M_3 e^{6\rho t} M_{2,3} M_{1,2,3} )
\end{aligned}$$

>

Thus in this case the 'universal' formula does not apply :(

This is the consequence of breaking the assumption of translation-invariance of the PDE in question.

However condition that the conformal metric of linearization is EW on the equation is still valid, with a different type of the covector.

>

>
