# Supplementary material for: Dispersionless integrable systems in 3D and Einstein-Weyl geometry
Source: arXiv:1208.2728 ancillary file (2013-05-09)
Supplement: Supplementary file 15 [file Integrability_conditions-type_II.pdf]

```

> # Input;
> #
> #
> restart;
    u[xx] := 1;
    u[yy] := 1;
    u[zz] := -2*a;
    u[xy] := lambda*c;
    u[xz] := c-lambda*b;
    u[yz] := 0;
> #

> # Define notation
> f(2*x) := u[xx]: f(2*y) := u[yy]: f(2*z) := u[zz]: f(x+y) := u
    [xy]: f(x+z) := u[xz]: f(y+z) := u[yz]:

> HessUniv:= - f(2*z)*f(y + x)^2 + 2*f(y + x)*f(z + x)*f(z + y) - f
    (2*y)*f(z + x)^2 - f(2*x)*f(z + y)^2 + f(2*x)*f(2*y)*f(2*z);

> f(a+2*x) := diff(f(2*x), a):
    f(b+2*x) := diff(f(2*x), b):
    f(c+2*x) := diff(f(2*x), c):
    f(2*a+2*x) := diff(f(a+2*x), a):
    f(2*b+2*x) := diff(f(b+2*x), b):
    f(2*c+2*x) := diff(f(c+2*x), c):
    f(a+b+2*x) := diff(f(b+2*x), a):
    f(a+c+2*x) := diff(f(c+2*x), a):
    f(c+b+2*x) := diff(f(b+2*x), c):
    f(a+2*y) := diff(f(2*y), a):
    f(b+2*y) := diff(f(2*y), b):
    f(c+2*y) := diff(f(2*y), c):
    f(2*a+2*y) := diff(f(a+2*y), a):
    f(2*b+2*y) := diff(f(b+2*y), b):
    f(2*c+2*y) := diff(f(c+2*y), c):
    f(a+b+2*y) := diff(f(b+2*y), a):
    f(a+c+2*y) := diff(f(c+2*y), a):
    f(c+b+2*y) := diff(f(b+2*y), c):
    f(a+2*z) := diff(f(2*z), a):
    f(b+2*z) := diff(f(2*z), b):
    f(c+2*z) := diff(f(2*z), c):
    f(2*a+2*z) := diff(f(a+2*z), a):
    f(2*b+2*z) := diff(f(b+2*z), b):
    f(2*c+2*z) := diff(f(c+2*z), c):
    f(a+b+2*z) := diff(f(b+2*z), a):
    f(a+c+2*z) := diff(f(c+2*z), a):
    f(c+b+2*z) := diff(f(b+2*z), c):
    f(a+x+y) := diff(f(x+y), a):
    f(b+x+y) := diff(f(x+y), b):
    f(c+x+y) := diff(f(x+y), c):
    f(2*a+x+y) := diff(f(a+x+y), a):
    f(2*b+x+y) := diff(f(b+x+y), b):
    f(2*c+x+y) := diff(f(c+x+y), c):

```

```

f(a+b+x+y) := diff(f(b+x+y), a):
f(a+c+x+y) := diff(f(c+x+y), a):
f(c+b+x+y) := diff(f(b+x+y), c):
f(a+x+z)    := diff(f(x+z), a):
f(b+x+z)    := diff(f(x+z), b):
f(c+x+z)    := diff(f(x+z), c):
f(2*a+x+z) := diff(f(a+x+z), a):
f(2*b+x+z) := diff(f(b+x+z), b):
f(2*c+x+z) := diff(f(c+x+z), c):
f(a+b+x+z) := diff(f(b+x+z), a):
f(a+c+x+z) := diff(f(c+x+z), a):
f(c+b+x+z) := diff(f(b+x+z), c):
f(a+z+y)   := diff(f(y+z), a):
f(b+z+y)   := diff(f(y+z), b):
f(c+z+y)   := diff(f(y+z), c):
f(2*a+z+y) := diff(f(a+z+y), a):
f(2*b+z+y) := diff(f(b+z+y), b):
f(2*c+z+y) := diff(f(c+z+y), c):
f(a+b+z+y) := diff(f(b+z+y), a):
f(a+c+z+y) := diff(f(c+z+y), a):
f(c+b+z+y) := diff(f(b+z+y), c):

```

```

> #
> # Equations
> eq[1] :=
> (1/HessUniv) * ( f(2*z)*f(z + y)^2*f(a + 2*y)*f(c + 2*x) - 2*f(2*
> z)*
> f(z + x)*f(z + y)*f(a + 2*y)*f(c + y + x) + f(2*z)*f(z +
> x)^2*f(a + 2
> *y)*f(c + 2*y) - 1/2*f(2*z)^2*f(z + y)*f(a + 2*y)*f(b +
> 2*x) + 1/2*f(
> 2*z)^2*f(z + y)*f(a + 2*x)*f(b + 2*y) + f(2*z)^2*f(z +
> x)*f(b + 2*y)*
> f(a + y + x) - 1/2*f(2*z)^2*f(z + x)*f(b + 2*x)*f(b + 2*
> y) - 1/2*f(2*
> z)^2*f(z + x)*f(a + 2*y)^2 + 1/2*f(2*z)^2*f(y + x)*f(b +
> 2*y)*f(c + 2
> *x) - f(2*z)^2*f(y + x)*f(b + 2*y)*f(a + z + x) + 1/2*f
> (2*z)^2*f(y +
> x)*f(b + 2*x)*f(c + 2*y) + f(2*z)^2*f(y + x)*f(a + 2*y)*
> f(c + y + x)
> + f(2*z)^2*f(y + x)*f(a + 2*y)*f(a + z + y) - f(2*z)*f
> (y + x)*f(z +
> y)*f(c + 2*x)*f(c + 2*y) - f(2*z)*f(y + x)*f(z + y)*f(a
> + 2*y)*f(a +
> 2*z) - 2*f(2*z)*f(y + x)*f(z + x)*f(c + 2*y)*f(a + z +
> y) + 2*f(y + x
> )*f(z + x)*f(z + y)*f(a + 2*z)*f(c + 2*y) - f(2*y)*f(z +
> y)^2*f(a + 2
> *x)*f(c + 2*z) + 2*f(2*y)*f(z + x)*f(z + y)*f(c + 2*z)*f
> (a + y + x)
> - f(2*y)*f(z + x)^2*f(a + 2*z)*f(c + 2*y) - f(2*y)*f(z
> + x)^2*f(a +
> 2*y)*f(c + 2*z) - f(2*y)*f(2*z)*f(z + y)*f(c + 2*x)*f(a
> + z + y) - 1/
> 2*f(2*y)*f(2*z)*f(z + y)*f(a + 2*z)*f(b + 2*x) + f(2*y)*

```

```

f(2*z)*f(z +
> y)*f(a + 2*x)*f(c + z + y) + 1/2*f(2*y)*f(2*z)*f(z + y)*
f(a + 2*x)*f(
> b + 2*z) + 1/2*f(2*y)*f(2*z)*f(z + x)*f(c + 2*x)*f(c +
2*y) - f(2*y)*
> f(2*z)*f(z + x)*f(b + 2*z)*f(a + y + x) + 1/2*f(2*y)*f
(2*z)*f(z + x)*
> f(b + 2*x)*f(b + 2*z) + 2*f(2*y)*f(2*z)*f(z + x)*f(a + z
+ y)*f(c + y
> + x) - 2*f(2*y)*f(2*z)*f(z + x)*f(a + y + x)*f(c + z +
y) + f(2*y)*
> f(2*z)*f(z + x)*f(a + 2*y)*f(c + z + x) + f(2*y)*f(2*z)*
f(z + x)*f(a
> + 2*y)*f(a + 2*z) + f(2*y)*f(2*z)^2*f(b + 2*x)*f(a + z
+ y) - 1/2*f(
> 2*y)*f(2*z)^2*f(a + 2*y)*f(c + 2*x) - 1/2*f(2*y)*f(2*z)
^2*f(a + 2*x)*
> f(c + 2*y) - f(2*y)*f(2*z)^2*f(a + 2*x)*f(b + z + y) -
1/2*f(2*y)*f(2
> *z)*f(y + x)*f(b + 2*z)*f(c + 2*x) + f(2*y)*f(2*z)*f(y +
x)*f(b + 2*z
> )*f(a + z + x) - 1/2*f(2*y)*f(2*z)*f(y + x)*f(b + 2*x)*f
(c + 2*z) - 2
> *f(2*y)*f(2*z)*f(y + x)*f(a + z + y)*f(c + z + x) + 2*f
(2*y)*f(2*z)*
> f(y + x)*f(a + z + x)*f(c + z + y) - f(2*y)*f(2*z)*f(y +
x)*f(a + 2*z
> )*f(c + y + x) - f(2*y)*f(2*z)*f(y + x)*f(a + 2*z)*f(a +
z + y) - 2*
> f(2*y)*f(y + x)*f(z + y)*f(c + 2*z)*f(a + z + x) + f(2*
y)*f(y + x)*f(
> z + y)*f(c + 2*x)*f(c + 2*z) + 2*f(2*y)*f(y + x)*f(z +
y)*f(a + 2*z)*
> f(c + z + x) + f(2*y)*f(y + x)*f(z + y)*f(a + 2*z)^2 +
2*f(2*y)*f(y
> + x)*f(z + x)*f(c + 2*z)*f(a + z + y) - f(2*y)*f(y + x)
^2*f(a + 2*z)
> *f(c + 2*z) - 1/2*f(2*y)^2*f(z + x)*f(c + 2*x)*f(c + 2*
z) - f(2*y)^2*
> f(z + x)*f(a + 2*z)*f(c + z + x) - 1/2*f(2*y)^2*f(z + x)
*f(a + 2*z)^2
> + 1/2*f(2*y)^2*f(2*z)*f(a + 2*z)*f(c + 2*x) + 1/2*f(2*
y)^2*f(2*z)*f(
> a + 2*x)*f(c + 2*z) - f(2*x)*f(z + y)^2*f(a + 2*z)*f(c +
2*y) + f(2*x
> )*f(2*z)*f(z + y)*f(c + 2*y)*f(c + y + x) + f(2*x)*f(2*
z)*f(z + y)*f(
> c + 2*y)*f(a + z + y) - f(2*x)*f(2*z)*f(z + y)*f(b + 2*
y)*f(c + z + x
> ) + 1/2*f(2*x)*f(2*z)*f(z + y)*f(a + 2*z)*f(b + 2*y) +
1/2*f(2*x)*f(2
> *z)*f(z + y)*f(a + 2*y)*f(b + 2*z) - 1/2*f(2*x)*f(2*z)*f
(z + x)*f(c
> + 2*y)^2 + f(2*x)*f(2*z)*f(z + x)*f(b + 2*y)*f(c + z +
y) - 1/2*f(2*
> x)*f(2*z)*f(z + x)*f(b + 2*y)*f(b + 2*z) - f(2*x)*f(2*z)
^2*f(b + 2*y)

```

```

>      *f(c + y + x) + f(2*x)*f(2*z)^2*f(b + 2*y)*f(b + z + x)
> - f(2*x)*f(2*
>      z)^2*f(b + 2*y)*f(a + z + y) - 1/2*f(2*x)*f(2*z)*f(y +
> x)*f(b + 2*z)*
>      f(c + 2*y) + 1/2*f(2*x)*f(2*z)*f(y + x)*f(b + 2*y)*f(c +
> 2*z) - f(2*x
>      )*f(2*y)*f(z + y)*f(c + 2*z)*f(c + y + x) + 2*f(2*x)*f
> (2*y)*f(z + y)*
>      f(c + 2*z)*f(b + z + x) - f(2*x)*f(2*y)*f(z + y)*f(b +
> 2*z)*f(c + z
>      + x) - f(2*x)*f(2*y)*f(z + y)*f(a + 2*z)*f(c + z + y) -
> f(2*x)*f(2*y
>      )*f(z + y)*f(a + 2*z)*f(b + 2*z) - 2*f(2*x)*f(2*y)*f(z +
> x)*f(c + 2*z
>      )*f(b + z + y) + 1/2*f(2*x)*f(2*y)*f(z + x)*f(c + 2*y)*f
> (c + 2*z) +
>      f(2*x)*f(2*y)*f(z + x)*f(b + 2*z)*f(c + z + y) + 1/2*f
> (2*x)*f(2*y)*f(
>      z + x)*f(b + 2*z)^2 + 2*f(2*x)*f(2*y)*f(2*z)*f(b + z +
> y)*f(c + z + x
>      ) - 2*f(2*x)*f(2*y)*f(2*z)*f(b + z + x)*f(c + z + y) + f
> (2*x)*f(2*y)*
>      f(2*z)*f(b + 2*z)*f(c + y + x) - f(2*x)*f(2*y)*f(2*z)*f
> (b + 2*z)*f(b
>      + z + x) + 1/2*f(2*x)*f(2*y)*f(2*z)*f(a + 2*z)*f(c + 2*
> y) + f(2*x)*
>      f(2*y)*f(2*z)*f(a + 2*z)*f(b + z + y) - 1/2*f(2*x)*f(2*
> y)*f(2*z)*f(a
>      + 2*y)*f(c + 2*z) + f(2*x)*f(2*y)^2*f(a + 2*z)*f(c + 2*
> z) )
>
>      - f(a + 2*z)*f(c + 2*y) + f(2*z)*f(c + a + 2*y) - f(2*y)*f
> (c + a + 2*z)
>      :
>
> eq[2] :=
> (1/HessUniv) * ( 2*f(z + y)^3*f(a + 2*x)*f(a + 2*y) - 2*f(z + x)
> *f(z
>      + y)^2*f(a + 2*y)*f(b + 2*x) - 4*f(z + x)*f(z + y)^2*f
> (a + 2*y)*f(a
>      + y + x) + 2*f(z + x)*f(z + y)^2*f(a + 2*x)*f(b + 2*y)
> + 4*f(z + x)^
>      2*f(z + y)*f(b + 2*y)*f(a + y + x) - 2*f(z + x)^2*f(z +
> y)*f(b + 2*x)
>      *f(b + 2*y) + 4*f(2*z)*f(y + x)*f(z + y)*f(a + 2*y)*f(a
> + y + x) + 2*
>      f(y + x)*f(z + y)^2*f(a + 2*y)*f(c + 2*x) - 4*f(y + x)*f
> (z + y)^2*f(a
>      + 2*y)*f(a + z + x) - 2*f(y + x)*f(z + y)^2*f(a + 2*x)*
> f(c + 2*y) -
>      4*f(y + x)*f(z + x)*f(z + y)*f(c + 2*y)*f(a + y + x) +
> 2*f(y + x)*f(z
>      + x)*f(z + y)*f(b + 2*y)*f(c + 2*x) - 4*f(y + x)*f(z +
> x)*f(z + y)*
>      f(b + 2*y)*f(a + z + x) + 2*f(y + x)*f(z + x)*f(z + y)*f
> (b + 2*x)*f(c
>      + 2*y) + 4*f(y + x)^2*f(z + y)*f(c + 2*y)*f(a + z + x)

```

```

- 2*f(y + x)^
>      2*f(z + y)*f(c + 2*x)*f(c + 2*y) - 2*f(2*y)*f(z + y)^2*f
(a + 2*x)*f(a
>      + z + y) + 2*f(2*y)*f(z + x)*f(z + y)*f(b + 2*x)*f(a +
z + y) + 4*f(
>      2*y)*f(z + x)*f(z + y)*f(a + y + x)*f(a + z + y) + 4*f
(2*y)*f(z + x)*
>      f(z + y)*f(a + 2*y)*f(a + z + x) - 2*f(2*y)*f(z + x)*f(z
+ y)*f(a + 2
>      *x)*f(b + z + y) + 2*f(2*y)*f(z + x)^2*f(b + 2*x)*f(b +
z + y) - 4*f(
>      2*y)*f(z + x)^2*f(a + y + x)*f(b + z + y) - 2*f(2*y)*f
(2*z)*f(z + y)*
>      f(a + 2*x)*f(a + 2*y) + f(2*y)*f(2*z)*f(z + x)*f(a + 2*
y)*f(b + 2*x)
>      - f(2*y)*f(2*z)*f(z + x)*f(a + 2*x)*f(b + 2*y) - 4*f(2*
y)*f(2*z)*f(y
>      + x)*f(a + y + x)*f(a + z + y) - f(2*y)*f(2*z)*f(y + x)
*f(a + 2*y)*
>      f(c + 2*x) + f(2*y)*f(2*z)*f(y + x)*f(a + 2*x)*f(c + 2*
y) - 2*f(2*y)*
>      f(y + x)*f(z + y)*f(c + 2*x)*f(a + z + y) + 4*f(2*y)*f(y
+ x)*f(z + y
>      )*f(a + z + x)*f(a + z + y) + 2*f(2*y)*f(y + x)*f(z + y)
*f(a + 2*x)*
>      f(c + z + y) - 2*f(2*y)*f(y + x)*f(z + x)*f(c + 2*x)*f(b
+ z + y) - 2
>      *f(2*y)*f(y + x)*f(z + x)*f(b + 2*x)*f(c + z + y) + 4*f
(2*y)*f(y + x)
>      *f(z + x)*f(a + z + x)*f(b + z + y) + 4*f(2*y)*f(y + x)*
f(z + x)*f(a
>      + y + x)*f(c + z + y) + 2*f(2*y)*f(y + x)^2*f(c + 2*x)*
f(c + z + y)
>      - 4*f(2*y)*f(y + x)^2*f(a + z + x)*f(c + z + y) - 4*f
(2*y)^2*f(z + x
>      )*f(a + z + x)*f(a + z + y) - f(2*y)^2*f(z + x)*f(a + 2*
z)*f(b + 2*x)
>      + f(2*y)^2*f(z + x)*f(a + 2*x)*f(b + 2*z) + 2*f(2*y)^2*
f(2*z)*f(a +
>      2*x)*f(a + z + y) + f(2*y)^2*f(y + x)*f(a + 2*z)*f(c +
2*x) - f(2*y)^
>      2*f(y + x)*f(a + 2*x)*f(c + 2*z) + 4*f(2*x)*f(z + y)^2*f
(c + 2*y)*f(a
>      + y + x) - 2*f(2*x)*f(z + y)^2*f(b + 2*y)*f(c + 2*x) -
2*f(2*x)*f(z
>      + y)^2*f(a + 2*y)*f(c + y + x) + 2*f(2*x)*f(z + y)^2*f
(a + 2*y)*f(b
>      + z + x) + 2*f(2*x)*f(z + y)^2*f(a + 2*y)*f(a + z + y)
- 2*f(2*x)*f(
>      z + x)*f(z + y)*f(b + 2*y)*f(c + y + x) + 2*f(2*x)*f(z +
x)*f(z + y)*
>      f(b + 2*y)*f(b + z + x) - 2*f(2*x)*f(z + x)*f(z + y)*f(b
+ 2*y)*f(a
>      + z + y) + 2*f(2*x)*f(z + x)*f(z + y)*f(a + 2*y)*f(c +
2*y) - 2*f(2*
>      x)*f(2*z)*f(z + y)*f(b + 2*y)*f(a + y + x) + f(2*x)*f(2*
z)*f(z + y)*

```

```

>      f(b + 2*x)*f(b + 2*y) - f(2*x)*f(2*z)*f(z + y)*f(a + 2*
y)^2 + 2*f(2*x
>      )*f(y + x)*f(z + y)*f(c + 2*y)*f(c + y + x) - 2*f(2*x)*f
(y + x)*f(z
>      + y)*f(c + 2*y)*f(b + z + x) - 2*f(2*x)*f(y + x)*f(z +
y)*f(c + 2*y)
>      *f(a + z + y) + 2*f(2*x)*f(y + x)*f(z + y)*f(a + 2*z)*f
(b + 2*y) - 2*
>      f(2*x)*f(2*y)*f(z + y)*f(c + 2*y)*f(a + z + x) + f(2*x)*
f(2*y)*f(z +
>      y)*f(c + 2*x)*f(c + 2*y) + 2*f(2*x)*f(2*y)*f(z + y)*f(c
+ 2*x)*f(b +
>      z + y) + 2*f(2*x)*f(2*y)*f(z + y)*f(a + z + y)*f(c + y +
x) - 2*f(2*x
>      )*f(2*y)*f(z + y)*f(a + z + y)*f(b + z + x) - 2*f(2*x)*f
(2*y)*f(z + y
>      )*f(a + z + y)^2 - 4*f(2*x)*f(2*y)*f(z + y)*f(a + y + x)
*f(c + z + y)
>      - f(2*x)*f(2*y)*f(z + y)*f(a + 2*y)*f(a + 2*z) + 2*f(2*
x)*f(2*y)*f(z
>      + x)*f(b + z + y)*f(c + y + x) - 2*f(2*x)*f(2*y)*f(z +
x)*f(b + z +
>      x)*f(b + z + y) + 2*f(2*x)*f(2*y)*f(z + x)*f(a + z + y)*
f(b + z + y)
>      - 2*f(2*x)*f(2*y)*f(z + x)*f(a + 2*y)*f(c + z + y) - f
(2*x)*f(2*y)*
>      f(2*z)*f(c + 2*y)*f(a + y + x) + 1/2*f(2*x)*f(2*y)*f(2*
z)*f(b + 2*y)*
>      f(c + 2*x) + f(2*x)*f(2*y)*f(2*z)*f(b + 2*y)*f(a + z +
x) - 1/2*f(2*x
>      )*f(2*y)*f(2*z)*f(b + 2*x)*f(c + 2*y) - f(2*x)*f(2*y)*f
(2*z)*f(b + 2*
>      x)*f(b + z + y) + 2*f(2*x)*f(2*y)*f(2*z)*f(a + y + x)*f
(b + z + y) +
>      f(2*x)*f(2*y)*f(2*z)*f(a + 2*y)*f(c + y + x) - f(2*x)*f
(2*y)*f(2*z)*
>      f(a + 2*y)*f(b + z + x) + f(2*x)*f(2*y)*f(2*z)*f(a + 2*
y)*f(a + z + y
>      ) - 2*f(2*x)*f(2*y)*f(y + x)*f(c + y + x)*f(c + z + y) +
2*f(2*x)*f(2
>      *y)*f(y + x)*f(b + z + x)*f(c + z + y) + 2*f(2*x)*f(2*y)
*f(y + x)*f(a
>      + z + y)*f(c + z + y) - 2*f(2*x)*f(2*y)*f(y + x)*f(a +
2*z)*f(b + z
>      + y) + f(2*x)*f(2*y)^2*f(c + 2*z)*f(a + y + x) - f(2*x)
*f(2*y)^2*f(c
>      + 2*x)*f(c + z + y) - 1/2*f(2*x)*f(2*y)^2*f(b + 2*z)*f
(c + 2*x) - f(
>      2*x)*f(2*y)^2*f(b + 2*z)*f(a + z + x) + 1/2*f(2*x)*f(2*
y)^2*f(b + 2*x
>      )*f(c + 2*z) + 2*f(2*x)*f(2*y)^2*f(a + z + x)*f(c + z +
y) - f(2*x)*
>      f(2*y)^2*f(a + 2*z)*f(c + y + x) + f(2*x)*f(2*y)^2*f(a +
2*z)*f(b + z
>      + x) + f(2*x)*f(2*y)^2*f(a + 2*z)*f(a + z + y) - f(2*x)
^2*f(z + y)*
>      f(c + 2*y)^2 + 2*f(2*x)^2*f(z + y)*f(b + 2*y)*f(c + z +

```

```

y) - f(2*x)^2
>      *f(z + y)*f(b + 2*y)*f(b + 2*z) + f(2*x)^2*f(2*y)*f(c +
2*y)*f(c + z
>      + y) - 2*f(2*x)^2*f(2*y)*f(b + z + y)*f(c + z + y) +
1/2*f(2*x)^2*f(
>      2*y)*f(b + 2*z)*f(c + 2*y) + f(2*x)^2*f(2*y)*f(b + 2*z)*
f(b + z + y)
>      - 1/2*f(2*x)^2*f(2*y)*f(b + 2*y)*f(c + 2*z) )
>
>      + 2*f(z + y)*f(2*a + 2*y) - 2*f(2*y)*f(2*a + z + y):
> eq[3] :=
> (1/HessUniv) * ( f(2*z)*f(z + y)^2*f(b + 2*y)*f(c + 2*x) - 2*f(2*
z)*
>      f(z + x)*f(z + y)*f(b + 2*y)*f(c + y + x) + f(2*z)*f(z +
x)^2*f(b + 2
>      *y)*f(c + 2*y) + 2*f(2*z)^2*f(z + y)*f(b + 2*y)*f(a + y
+ x) - 1/2*f(
>      2*z)^2*f(z + y)*f(b + 2*x)*f(b + 2*y) - f(2*z)^2*f(z +
y)*f(a + 2*y)*
>      f(b + y + x) - 1/2*f(2*z)^2*f(z + y)*f(a + 2*y)^2 + f(2*
z)^2*f(y + x)
>      *f(c + 2*y)*f(b + y + x) + f(2*z)^2*f(y + x)*f(b + 2*y)*
f(b + z + x)
>      - 2*f(2*z)^2*f(y + x)*f(b + 2*y)*f(a + z + y) + f(2*z)
^2*f(y + x)*f(
>      a + 2*y)*f(c + 2*y) + f(2*z)^2*f(y + x)*f(a + 2*y)*f(b +
z + y) - 2*
>      f(2*z)*f(y + x)*f(z + y)*f(b + 2*y)*f(c + z + x) - f(2*
z)*f(y + x)*f(
>      z + x)*f(c + 2*y)^2 - 2*f(2*z)*f(y + x)*f(z + x)*f(c +
2*y)*f(b + z
>      + y) + 2*f(2*z)*f(y + x)*f(z + x)*f(b + 2*y)*f(c + z +
y) - f(2*z)*
>      f(y + x)*f(z + x)*f(b + 2*y)*f(b + 2*z) + 2*f(y + x)*f(z
+ x)*f(z + y
>      )*f(b + 2*y)*f(c + 2*z) - f(2*y)*f(z + y)^2*f(b + 2*x)*f
(c + 2*z) + 2
>      *f(2*y)*f(z + x)*f(z + y)*f(c + 2*z)*f(b + y + x) - 2*f
(2*y)*f(z + x)
>      ^2*f(b + 2*y)*f(c + 2*z) - 1/2*f(2*y)*f(2*z)*f(z + y)*f
(c + 2*x)*f(c
>      + 2*y) - f(2*y)*f(2*z)*f(z + y)*f(c + 2*x)*f(b + z + y)
+ f(2*y)*f(2
>      *z)*f(z + y)*f(b + 2*x)*f(c + z + y) + 1/2*f(2*y)*f(2*z)
*f(z + y)*f(b
>      + 2*x)*f(b + 2*z) - f(2*y)*f(2*z)*f(z + y)*f(a + 2*z)*f
(b + y + x)
>      + f(2*y)*f(2*z)*f(z + y)*f(a + 2*y)*f(c + z + x) + f(2*
y)*f(2*z)*f(z
>      + x)*f(c + 2*y)*f(c + y + x) + 2*f(2*y)*f(2*z)*f(z + x)
*f(b + z + y)
>      *f(c + y + x) - 2*f(2*y)*f(2*z)*f(z + x)*f(b + y + x)*f
(c + z + y) +
>      f(2*y)*f(2*z)*f(z + x)*f(b + 2*y)*f(c + z + x) + f(2*y)*
f(2*z)*f(z +
>      x)*f(a + 2*z)*f(b + 2*y) - f(2*y)*f(2*z)*f(z + x)*f(a +

```

```

2*y)*f(c + z
> + y) - f(2*y)*f(2*z)^2*f(c + 2*y)*f(a + y + x) - f(2*y)
*f(2*z)^2*f(b
> + 2*y)*f(a + z + x) + 2*f(2*y)*f(2*z)^2*f(a + z + y)*f
(b + y + x) -
> 2*f(2*y)*f(2*z)^2*f(a + y + x)*f(b + z + y) + f(2*y)*f
(2*z)^2*f(a + 2
> *y)*f(a + z + y) - f(2*y)*f(2*z)*f(y + x)*f(c + 2*z)*f(b
+ y + x) + 2
> *f(2*y)*f(2*z)*f(y + x)*f(b + z + y)*f(c + z + x) - 2*f
(2*y)*f(2*z)*
> f(y + x)*f(b + z + x)*f(c + z + y) - f(2*y)*f(2*z)*f(y +
x)*f(b + 2*z
> )*f(b + z + x) + f(2*y)*f(2*z)*f(y + x)*f(a + 2*z)*f(b +
z + y) - f(2
> *y)*f(2*z)*f(y + x)*f(a + 2*y)*f(c + 2*z) + 2*f(2*y)*f(y
+ x)*f(z + y
> )*f(c + 2*z)*f(b + z + x) - 2*f(2*y)*f(y + x)*f(z + x)*f
(c + 2*z)*f(b
> + z + y) + f(2*y)*f(y + x)*f(z + x)*f(c + 2*y)*f(c + 2*
z) + 2*f(2*y)
> *f(y + x)*f(z + x)*f(b + 2*z)*f(c + z + y) + f(2*y)*f(y
+ x)*f(z + x)
> *f(b + 2*z)^2 - f(2*y)*f(y + x)^2*f(b + 2*z)*f(c + 2*z)
- 2*f(2*y)^2*
> f(z + y)*f(c + 2*z)*f(a + z + x) + 1/2*f(2*y)^2*f(z + y)
*f(c + 2*x)*
> f(c + 2*z) + f(2*y)^2*f(z + y)*f(a + 2*z)*f(c + z + x) +
1/2*f(2*y)^2
> *f(z + y)*f(a + 2*z)^2 - f(2*y)^2*f(z + x)*f(c + 2*z)*f
(c + y + x) +
> 2*f(2*y)^2*f(z + x)*f(c + 2*z)*f(a + z + y) - f(2*y)^2*f
(z + x)*f(b
> + 2*z)*f(c + z + x) - f(2*y)^2*f(z + x)*f(a + 2*z)*f(c
+ z + y) - f(
> 2*y)^2*f(z + x)*f(a + 2*z)*f(b + 2*z) + f(2*y)^2*f(2*z)*
f(c + 2*z)*f(
> a + y + x) + f(2*y)^2*f(2*z)*f(b + 2*z)*f(a + z + x) -
2*f(2*y)^2*f(2
> *z)*f(a + z + y)*f(c + z + x) + 2*f(2*y)^2*f(2*z)*f(a +
z + x)*f(c +
> z + y) - f(2*y)^2*f(2*z)*f(a + 2*z)*f(a + z + y) - f(2*
x)*f(z + y)^2*
> f(b + 2*y)*f(c + 2*z) + 1/2*f(2*x)*f(2*z)*f(z + y)*f(c +
2*y)^2 + f(2
> *x)*f(2*z)*f(z + y)*f(c + 2*y)*f(b + z + y) + 1/2*f(2*x)
*f(2*z)*f(z
> + y)*f(b + 2*y)*f(b + 2*z) - f(2*x)*f(2*z)^2*f(b + 2*y)
*f(c + 2*y)
> - 1/2*f(2*x)*f(2*y)*f(z + y)*f(c + 2*y)*f(c + 2*z) - f
(2*x)*f(2*y)*
> f(z + y)*f(b + 2*z)*f(c + z + y) - 1/2*f(2*x)*f(2*y)*f(z
+ y)*f(b + 2
> *z)^2 + f(2*x)*f(2*y)*f(2*z)*f(b + 2*y)*f(c + 2*z) + f
(2*x)*f(2*y)^2*
> f(b + 2*z)*f(c + 2*z) )

```



```

>      - f(b + 2*y)*f(c + 2*z) + f(2*z)*f(c + b + 2*y) - f(2*y)*f
(c + b + 2*z)
>      :
> eq[4] :=
> (1/HessUniv) * ( 2*f(z + x)*f(z + y)^2*f(a + 2*x)*f(a + 2*y) -
2*f(z
>      + x)^2*f(z + y)*f(a + 2*y)*f(b + 2*x) - 4*f(z + x)^2*f
(z + y)*f(a +
>      2*y)*f(a + y + x) + 2*f(z + x)^2*f(z + y)*f(a + 2*x)*f(b
+ 2*y) + 4*
>      f(z + x)^3*f(b + 2*y)*f(a + y + x) - 2*f(z + x)^3*f(b +
2*x)*f(b + 2*
>      y) + 4*f(2*z)*f(y + x)*f(z + x)*f(a + 2*y)*f(a + y + x)
+ 2*f(y + x)*
>      f(z + x)*f(z + y)*f(a + 2*y)*f(c + 2*x) - 4*f(y + x)*f(z
+ x)*f(z + y
>      )*f(a + 2*y)*f(a + z + x) - 2*f(y + x)*f(z + x)*f(z + y)
*f(a + 2*x)*
>      f(c + 2*y) - 4*f(y + x)*f(z + x)^2*f(c + 2*y)*f(a + y +
x) + 2*f(y +
>      x)*f(z + x)^2*f(b + 2*y)*f(c + 2*x) - 4*f(y + x)*f(z +
x)^2*f(b + 2*y
>      )*f(a + z + x) + 2*f(y + x)*f(z + x)^2*f(b + 2*x)*f(c +
2*y) + 4*f(y
>      + x)^2*f(z + x)*f(c + 2*y)*f(a + z + x) - 2*f(y + x)^2*
f(z + x)*f(c
>      + 2*x)*f(c + 2*y) - 2*f(2*y)*f(z + y)^2*f(a + 2*x)*f(a
+ z + x) - 2*
>      f(2*y)*f(z + x)*f(z + y)*f(b + 2*x)*f(a + z + x) + 4*f
(2*y)*f(z + x)*
>      f(z + y)*f(a + y + x)*f(a + z + x) + 2*f(2*y)*f(z + x)*f
(z + y)*f(a
>      + 2*x)*f(b + z + x) + 2*f(2*y)*f(z + x)^2*f(b + 2*x)*f
(b + z + x) +
>      4*f(2*y)*f(z + x)^2*f(b + 2*x)*f(a + z + y) - 4*f(2*y)*f
(z + x)^2*f(a
>      + y + x)*f(b + z + x) + 4*f(2*y)*f(z + x)^2*f(a + 2*y)*
f(a + z + x)
>      - 4*f(2*y)*f(z + x)^2*f(a + 2*x)*f(b + z + y) + 2*f(2*
y)*f(2*z)*f(z
>      + x)*f(b + 2*x)*f(a + y + x) - 2*f(2*y)*f(2*z)*f(z + x)
*f(a + 2*x)*
>      f(b + y + x) - 2*f(2*y)*f(2*z)*f(z + x)*f(a + 2*x)*f(a
+ 2*y) - 2*f(2
>      *y)*f(2*z)*f(y + x)*f(c + 2*x)*f(a + y + x) - 4*f(2*y)*f
(2*z)*f(y + x
>      )*f(a + y + x)*f(a + z + x) + 2*f(2*y)*f(2*z)*f(y + x)*f
(a + 2*x)*f(c
>      + y + x) + 2*f(2*y)*f(y + x)*f(z + y)*f(c + 2*x)*f(a +
z + x) + 4*f(
>      2*y)*f(y + x)*f(z + y)*f(a + z + x)^2 - 2*f(2*y)*f(y +
x)*f(z + y)*f(
>      a + 2*x)*f(c + z + x) - 2*f(2*y)*f(y + x)*f(z + x)*f(c
+ 2*x)*f(b + z
>      + x) - 4*f(2*y)*f(y + x)*f(z + x)*f(c + 2*x)*f(a + z +
y) - 2*f(2*y)

```

```

>      *f(y + x)*f(z + x)*f(b + 2*x)*f(c + z + x) + 4*f(2*y)*f
(y + x)*f(z +
>      x)*f(a + z + x)*f(b + z + x) - 2*f(2*y)*f(y + x)*f(z +
x)*f(a + 2*z)*
>      f(b + 2*x) + 4*f(2*y)*f(y + x)*f(z + x)*f(a + y + x)*f(c
+ z + x) + 4
>      *f(2*y)*f(y + x)*f(z + x)*f(a + 2*x)*f(c + z + y) + 2*f
(2*y)*f(y + x)
>      *f(z + x)*f(a + 2*x)*f(b + 2*z) + 2*f(2*y)*f(y + x)^2*f
(c + 2*x)*f(c
>      + z + x) - 4*f(2*y)*f(y + x)^2*f(a + z + x)*f(c + z +
x) + 2*f(2*y)*
>      f(y + x)^2*f(a + 2*z)*f(c + 2*x) - 2*f(2*y)*f(y + x)^2*f
(a + 2*x)*f(c
>      + 2*z) - 4*f(2*y)^2*f(z + x)*f(a + z + x)^2 + 2*f(2*y)
^2*f(2*z)*f(a
>      + 2*x)*f(a + z + x) + 4*f(2*x)*f(z + x)*f(z + y)*f(c +
2*y)*f(a + y
>      + x) - 2*f(2*x)*f(z + x)*f(z + y)*f(b + 2*y)*f(c + 2*x)
- 2*f(2*x)*
>      f(z + x)*f(z + y)*f(a + 2*y)*f(c + y + x) + 2*f(2*x)*f(z
+ x)*f(z + y
>      )*f(a + 2*y)*f(b + z + x) + 2*f(2*x)*f(z + x)*f(z + y)*f
(a + 2*y)*f(a
>      + z + y) - 2*f(2*x)*f(z + x)^2*f(b + 2*y)*f(c + y + x)
+ 2*f(2*x)*f(
>      z + x)^2*f(b + 2*y)*f(b + z + x) - 2*f(2*x)*f(z + x)^2*f
(b + 2*y)*f(a
>      + z + y) + 2*f(2*x)*f(z + x)^2*f(a + 2*y)*f(c + 2*y) -
2*f(2*x)*f(2*
>      z)*f(z + x)*f(b + 2*y)*f(a + y + x) + f(2*x)*f(2*z)*f(z
+ x)*f(b + 2*
>      x)*f(b + 2*y) - f(2*x)*f(2*z)*f(z + x)*f(a + 2*y)^2 + 2*
f(2*x)*f(y +
>      x)*f(z + x)*f(c + 2*y)*f(c + y + x) - 2*f(2*x)*f(y + x)*
f(z + x)*f(c
>      + 2*y)*f(b + z + x) - 2*f(2*x)*f(y + x)*f(z + x)*f(c +
2*y)*f(a + z
>      + y) + 2*f(2*x)*f(y + x)*f(z + x)*f(a + 2*z)*f(b + 2*y)
+ 2*f(2*x)*
>      f(2*y)*f(z + y)*f(b + 2*x)*f(c + z + x) - 2*f(2*x)*f(2*
y)*f(z + y)*f(
>      a + z + x)*f(c + y + x) - 2*f(2*x)*f(2*y)*f(z + y)*f(a +
z + x)*f(b
>      + z + x) - 2*f(2*x)*f(2*y)*f(z + y)*f(a + z + x)*f(a +
z + y) + f(2*
>      x)*f(2*y)*f(z + y)*f(a + 2*z)*f(b + 2*x) - f(2*x)*f(2*y)
*f(z + y)*f(a
>      + 2*x)*f(b + 2*z) - 2*f(2*x)*f(2*y)*f(z + x)*f(c + 2*y)
*f(a + z + x)
>      + f(2*x)*f(2*y)*f(z + x)*f(c + 2*x)*f(c + 2*y) + 2*f(2*
x)*f(2*y)*f(z
>      + x)*f(c + 2*x)*f(b + z + y) + 2*f(2*x)*f(2*y)*f(z + x)
*f(b + z + x)
>      *f(c + y + x) - 2*f(2*x)*f(2*y)*f(z + x)*f(b + z + x)^2
- 2*f(2*x)*f(
>      2*y)*f(z + x)*f(b + 2*x)*f(c + z + y) + 4*f(2*x)*f(2*y)*

```

```

f(z + x)*f(a
> + z + y)*f(c + y + x) - 2*f(2*x)*f(2*y)*f(z + x)*f(a +
> z + y)*f(b +
> z + x) + 4*f(2*x)*f(2*y)*f(z + x)*f(a + z + x)*f(b + z +
> y) - 4*f(2*x
> )*f(2*y)*f(z + x)*f(a + y + x)*f(c + z + y) - 2*f(2*x)*f
> (2*y)*f(z + x
> )*f(a + 2*y)*f(c + z + x) - f(2*x)*f(2*y)*f(z + x)*f(a +
> 2*y)*f(a + 2
> *z) + f(2*x)*f(2*y)*f(2*z)*f(c + 2*x)*f(b + y + x) - f
> (2*x)*f(2*y)*f(
> 2*z)*f(b + 2*x)*f(c + y + x) - f(2*x)*f(2*y)*f(2*z)*f(b
> + 2*x)*f(b +
> z + x) - f(2*x)*f(2*y)*f(2*z)*f(b + 2*x)*f(a + z + y) +
> 2*f(2*x)*f(2*
> y)*f(2*z)*f(a + z + x)*f(b + y + x) + 1/2*f(2*x)*f(2*y)*
> f(2*z)*f(a +
> 2*y)*f(c + 2*x) + f(2*x)*f(2*y)*f(2*z)*f(a + 2*y)*f(a +
> z + x) - 1/2*
> f(2*x)*f(2*y)*f(2*z)*f(a + 2*x)*f(c + 2*y) + f(2*x)*f(2*
> y)*f(2*z)*f(a
> + 2*x)*f(b + z + y) + 2*f(2*x)*f(2*y)*f(y + x)*f(c + 2*
> z)*f(a + y +
> x) - 2*f(2*x)*f(2*y)*f(y + x)*f(c + y + x)*f(c + z + x)
> + 2*f(2*x)*f(
> 2*y)*f(y + x)*f(b + z + x)*f(c + z + x) - f(2*x)*f(2*y)*
> f(y + x)*f(b
> + 2*z)*f(c + 2*x) - 2*f(2*x)*f(2*y)*f(y + x)*f(b + 2*z)
> *f(a + z + x)
> + f(2*x)*f(2*y)*f(y + x)*f(b + 2*x)*f(c + 2*z) + 2*f(2*
> x)*f(2*y)*f(y
> + x)*f(a + z + y)*f(c + z + x) - 2*f(2*x)*f(2*y)*f(y +
> x)*f(a + 2*z)
> *f(c + y + x) - f(2*x)*f(2*y)^2*f(c + 2*x)*f(c + z + x)
> + 2*f(2*x)*f(
> 2*y)^2*f(a + z + x)*f(c + z + x) - 1/2*f(2*x)*f(2*y)^2*f
> (a + 2*z)*f(c
> + 2*x) + f(2*x)*f(2*y)^2*f(a + 2*z)*f(a + z + x) + 1/2*
> f(2*x)*f(2*y)
> ^2*f(a + 2*x)*f(c + 2*z) - f(2*x)^2*f(z + x)*f(c + 2*y)
> ^2 + 2*f(2*x)^
> 2*f(z + x)*f(b + 2*y)*f(c + z + y) - f(2*x)^2*f(z + x)*f
> (b + 2*y)*f(b
> + 2*z) - f(2*x)^2*f(2*y)*f(c + 2*z)*f(b + y + x) + f(2*
> x)^2*f(2*y)*
> f(c + 2*y)*f(c + z + x) - 2*f(2*x)^2*f(2*y)*f(b + z + y)
> *f(c + z + x)
> + f(2*x)^2*f(2*y)*f(b + 2*z)*f(c + y + x) + f(2*x)^2*f
> (2*y)*f(b + 2*
> z)*f(b + z + x) + f(2*x)^2*f(2*y)*f(b + 2*z)*f(a + z +
> y) + 1/2*f(2*x
> )^2*f(2*y)*f(a + 2*z)*f(c + 2*y) - f(2*x)^2*f(2*y)*f(a +
> 2*z)*f(b + z
> + y) - 1/2*f(2*x)^2*f(2*y)*f(a + 2*y)*f(c + 2*z) )
>
> + 2*f(z + x)*f(2*a + 2*y) - 2*f(2*y)*f(2*a + z + x):

```

```

> eq[5] :=
> (1/HessUniv) * ( 2*f(2*z)*f(z + y)^2*f(a + 2*y)*f(c + z + x) - f
> (2*z)
> *f(z + y)^2*f(a + 2*y)*f(a + 2*z) - 2*f(2*z)*f(z + x)*f
> (z + y)*f(b +
> 2*y)*f(c + z + x) + f(2*z)*f(z + x)*f(z + y)*f(a + 2*z)*
> f(b + 2*y) -
> 2*f(2*z)*f(z + x)*f(z + y)*f(a + 2*y)*f(c + z + y) + f
> (2*z)*f(z + x)*
> f(z + y)*f(a + 2*y)*f(b + 2*z) + 2*f(2*z)*f(z + x)^2*f(b
> + 2*y)*f(c
> + z + y) - f(2*z)*f(z + x)^2*f(b + 2*y)*f(b + 2*z) + f
> (2*z)^2*f(z +
> y)*f(b + 2*y)*f(c + 2*x) - f(2*z)^2*f(z + y)*f(a + 2*y)*
> f(c + y + x)
> - f(2*z)^2*f(z + y)*f(a + 2*y)*f(b + z + x) + f(2*z)^2*
> f(z + y)*f(a
> + 2*y)*f(a + z + y) - f(2*z)^2*f(z + x)*f(b + 2*y)*f(c
> + y + x) + f(
> 2*z)^2*f(z + x)*f(b + 2*y)*f(b + z + x) - f(2*z)^2*f(z +
> x)*f(b + 2*y
> )*f(a + z + y) + f(2*z)^2*f(z + x)*f(a + 2*y)*f(c + 2*y)
> + f(2*z)^3*
> f(b + 2*y)*f(a + y + x) - 1/2*f(2*z)^3*f(b + 2*x)*f(b +
> 2*y) - 1/2*f(
> 2*z)^3*f(a + 2*y)^2 + f(2*z)^2*f(y + x)*f(c + 2*y)*f(c +
> y + x) + f(2
> *z)^2*f(y + x)*f(c + 2*y)*f(b + z + x) - f(2*z)^2*f(y +
> x)*f(c + 2*y)
> *f(a + z + y) - f(2*z)^2*f(y + x)*f(a + 2*z)*f(b + 2*y)
> + 2*f(2*z)^2*
> f(y + x)*f(a + 2*y)*f(c + z + y) - 2*f(2*z)*f(y + x)*f(z
> + y)*f(c + 2
> *y)*f(c + z + x) + f(2*z)*f(y + x)*f(z + y)*f(a + 2*z)*f
> (c + 2*y) -
> f(2*z)*f(y + x)*f(z + y)*f(a + 2*y)*f(c + 2*z) - 2*f(2*
> z)*f(y + x)*f(
> z + x)*f(c + 2*y)*f(c + z + y) - f(2*z)*f(y + x)*f(z +
> x)*f(b + 2*z)*
> f(c + 2*y) + f(2*z)*f(y + x)*f(z + x)*f(b + 2*y)*f(c +
> 2*z) + 2*f(y
> + x)*f(z + x)*f(z + y)*f(c + 2*y)*f(c + 2*z) - 4*f(2*y)
> *f(z + y)^2*
> f(c + 2*z)*f(a + z + x) + 2*f(2*y)*f(z + y)^2*f(a + 2*z)
> *f(c + z + x)
> + f(2*y)*f(z + y)^2*f(a + 2*z)^2 + 4*f(2*y)*f(z + x)*f
> (z + y)*f(c +
> 2*z)*f(b + z + x) + 4*f(2*y)*f(z + x)*f(z + y)*f(c + 2*
> z)*f(a + z + y
> ) - 2*f(2*y)*f(z + x)*f(z + y)*f(b + 2*z)*f(c + z + x) -
> 2*f(2*y)*f(z
> + x)*f(z + y)*f(a + 2*z)*f(c + z + y) - 2*f(2*y)*f(z +
> x)*f(z + y)*
> f(a + 2*z)*f(b + 2*z) - 4*f(2*y)*f(z + x)^2*f(c + 2*z)*f
> (b + z + y)
> - f(2*y)*f(z + x)^2*f(c + 2*y)*f(c + 2*z) + 2*f(2*y)*f
> (z + x)^2*f(b

```

```

> + 2*z)*f(c + z + y) + f(2*y)*f(z + x)^2*f(b + 2*z)^2 +
2*f(2*y)*f(2*
> z)*f(z + y)*f(c + 2*z)*f(a + y + x) + 2*f(2*y)*f(2*z)*f
(z + y)*f(b +
> 2*z)*f(a + z + x) - f(2*y)*f(2*z)*f(z + y)*f(b + 2*x)*f
(c + 2*z) - 4*
> f(2*y)*f(2*z)*f(z + y)*f(a + z + y)*f(c + z + x) + 4*f
(2*y)*f(2*z)*f(
> z + y)*f(a + z + x)*f(c + z + y) - f(2*y)*f(2*z)*f(z +
y)*f(a + 2*z)*
> f(c + y + x) - f(2*y)*f(2*z)*f(z + y)*f(a + 2*z)*f(b + z
+ x) - f(2*y
> )*f(2*z)*f(z + y)*f(a + 2*z)*f(a + z + y) + 2*f(2*y)*f
(2*z)*f(z + x)*
> f(c + 2*y)*f(c + z + x) + 4*f(2*y)*f(2*z)*f(z + x)*f(b +
z + y)*f(c
> + z + x) - 4*f(2*y)*f(2*z)*f(z + x)*f(b + z + x)*f(c +
z + y) + f(2*
> y)*f(2*z)*f(z + x)*f(b + 2*z)*f(c + y + x) - f(2*y)*f(2*
z)*f(z + x)*
> f(b + 2*z)*f(b + z + x) - f(2*y)*f(2*z)*f(z + x)*f(b +
2*z)*f(a + z
> + y) + 2*f(2*y)*f(2*z)*f(z + x)*f(a + 2*z)*f(b + z + y)
- f(2*y)*f(2
> *z)*f(z + x)*f(a + 2*y)*f(c + 2*z) - f(2*y)*f(2*z)^2*f(c
+ 2*y)*f(a
> + z + x) - 1/2*f(2*y)*f(2*z)^2*f(c + 2*x)*f(c + 2*y) -
f(2*y)*f(2*z)
> ^2*f(c + 2*x)*f(b + z + y) - f(2*y)*f(2*z)^2*f(b + 2*z)*
f(a + y + x)
> + f(2*y)*f(2*z)^2*f(b + 2*x)*f(c + z + y) + 1/2*f(2*y)*
f(2*z)^2*f(b
> + 2*x)*f(b + 2*z) + 2*f(2*y)*f(2*z)^2*f(a + z + y)*f(c
+ y + x) + 2*
> f(2*y)*f(2*z)^2*f(a + z + y)*f(b + z + x) - 2*f(2*y)*f
(2*z)^2*f(a + z
> + x)*f(b + z + y) - 2*f(2*y)*f(2*z)^2*f(a + y + x)*f(c
+ z + y) + f(
> 2*y)*f(2*z)^2*f(a + 2*y)*f(a + 2*z) - f(2*y)*f(2*z)*f(y
+ x)*f(c + 2*
> z)*f(c + y + x) - f(2*y)*f(2*z)*f(y + x)*f(c + 2*z)*f(b
+ z + x) - f(
> 2*y)*f(2*z)*f(y + x)*f(c + 2*z)*f(a + z + y) + f(2*y)*f
(2*z)*f(y + x)
> *f(a + 2*z)*f(b + 2*z) + 2*f(2*y)*f(y + x)*f(z + y)*f(c
+ 2*z)*f(c +
> z + x) + 2*f(2*y)*f(y + x)*f(z + x)*f(c + 2*z)*f(c + z +
y) - f(2*y)*
> f(y + x)^2*f(c + 2*z)^2 - 2*f(2*y)^2*f(z + x)*f(c + 2*z)
*f(c + z + x)
> + f(2*y)^2*f(2*z)*f(c + 2*z)*f(a + z + x) + 1/2*f(2*y)
^2*f(2*z)*f(c
> + 2*x)*f(c + 2*z) - 1/2*f(2*y)^2*f(2*z)*f(a + 2*z)^2 -
f(2*x)*f(z +
> y)^2*f(c + 2*y)*f(c + 2*z) + 2*f(2*x)*f(2*z)*f(z + y)*f
(c + 2*y)*f(c
> + z + y) - 1/2*f(2*x)*f(2*z)^2*f(c + 2*y)^2 - f(2*x)*f

```

```

(2*z)^2*f(b +
>      2*y)*f(c + z + y) + 1/2*f(2*x)*f(2*z)^2*f(b + 2*y)*f(b +
2*z) - 2*f(2
>      *x)*f(2*y)*f(z + y)*f(c + 2*z)*f(c + z + y) + f(2*x)*f
(2*y)*f(2*z)*f(
>      c + 2*z)*f(b + z + y) + 1/2*f(2*x)*f(2*y)*f(2*z)*f(c +
2*y)*f(c + 2*z
>      ) - 1/2*f(2*x)*f(2*y)*f(2*z)*f(b + 2*z)^2 + f(2*x)*f(2*
y)^2*f(c + 2*z
>      )^2 )

>      - f(c + 2*y)*f(c + 2*z) + f(2*z)*f(2*c + 2*y) - f(2*y)*f
(2*c + 2*z):

> eq[6] :=
> (1/HessUniv) * ( 8*f(z + y)^3*f(b + 2*y)*f(a + y + x) - 4*f(z +
y)^3*
>      f(a + 2*y)*f(b + y + x) - 2*f(z + y)^3*f(a + 2*y)^2 - 4*
f(z + x)*f(z
>      + y)^2*f(b + 2*y)*f(b + y + x) + 2*f(z + x)^2*f(z + y)*
f(b + 2*y)^2
>      + 4*f(2*z)*f(y + x)*f(z + y)*f(b + 2*y)*f(b + y + x) +
4*f(y + x)*f(
>      z + y)^2*f(c + 2*y)*f(b + y + x) - 8*f(y + x)*f(z + y)
^2*f(b + 2*y)*
>      f(c + y + x) - 8*f(y + x)*f(z + y)^2*f(b + 2*y)*f(a + z
+ y) + 4*f(y
>      + x)*f(z + y)^2*f(a + 2*y)*f(c + 2*y) + 4*f(y + x)*f(z
+ y)^2*f(a +
>      2*y)*f(b + z + y) - 4*f(y + x)*f(z + x)*f(z + y)*f(b +
2*y)*f(b + z
>      + y) - 2*f(y + x)^2*f(z + y)*f(c + 2*y)^2 - 4*f(y + x)
^2*f(z + y)*f(
>      c + 2*y)*f(b + z + y) + 8*f(y + x)^2*f(z + y)*f(b + 2*y)
*f(c + z + y)
>      - 4*f(2*y)*f(z + y)^2*f(c + 2*y)*f(a + y + x) + 2*f(2*
y)*f(z + y)^2*
>      f(b + 2*y)*f(c + 2*x) - 4*f(2*y)*f(z + y)^2*f(b + 2*y)*f
(a + z + x)
>      + 4*f(2*y)*f(z + y)^2*f(a + z + y)*f(b + y + x) - 8*f
(2*y)*f(z + y)^
>      2*f(a + y + x)*f(b + z + y) + 2*f(2*y)*f(z + y)^2*f(a +
2*y)*f(c + y
>      + x) + 2*f(2*y)*f(z + y)^2*f(a + 2*y)*f(b + z + x) + 4*
f(2*y)*f(z +
>      y)^2*f(a + 2*y)*f(a + z + y) + 4*f(2*y)*f(z + x)*f(z +
y)*f(b + y + x
>      )*f(b + z + y) + 2*f(2*y)*f(z + x)*f(z + y)*f(b + 2*y)*f
(c + y + x)
>      + 2*f(2*y)*f(z + x)*f(z + y)*f(b + 2*y)*f(b + z + x) +
4*f(2*y)*f(z
>      + x)*f(z + y)*f(b + 2*y)*f(a + z + y) - 2*f(2*y)*f(z +
x)*f(z + y)*
>      f(a + 2*y)*f(c + 2*y) - 2*f(2*y)*f(z + x)*f(z + y)*f(a +
2*y)*f(b + z
>      + y) - 2*f(2*y)*f(z + x)^2*f(b + 2*y)*f(b + z + y) - 4*
f(2*y)*f(2*z)

```

```

>      *f(z + y)*f(b + 2*y)*f(a + y + x) - f(2*y)*f(2*z)*f(z +
> y)*f(b + 2*x)
>      *f(b + 2*y) + 2*f(2*y)*f(2*z)*f(z + y)*f(a + 2*y)*f(b +
> y + x) + f(2*
> y)*f(2*z)*f(z + y)*f(a + 2*y)^2 - 2*f(2*y)*f(2*z)*f(y +
> x)*f(c + 2*y)
>      *f(b + y + x) - 4*f(2*y)*f(2*z)*f(y + x)*f(b + y + x)*f
> (b + z + y) +
>      2*f(2*y)*f(2*z)*f(y + x)*f(b + 2*y)*f(c + y + x) + 2*f
> (2*y)*f(y + x)*
>      f(z + y)*f(c + 2*y)*f(c + y + x) - 2*f(2*y)*f(y + x)*f(z
> + y)*f(c + 2
> *y)*f(b + z + x) + 8*f(2*y)*f(y + x)*f(z + y)*f(b + z +
> y)*f(c + y +
> x) - 4*f(2*y)*f(y + x)*f(z + y)*f(b + y + x)*f(c + z +
> y) + 4*f(2*y)*
>      f(y + x)*f(z + y)*f(a + z + y)*f(b + z + y) + 4*f(2*y)*f
> (y + x)*f(z
> + y)*f(a + 2*z)*f(b + 2*y) - 6*f(2*y)*f(y + x)*f(z + y)
> *f(a + 2*y)*
>      f(c + z + y) - 2*f(2*y)*f(y + x)*f(z + y)*f(a + 2*y)*f(b
> + 2*z) + 2*
>      f(2*y)*f(y + x)*f(z + x)*f(c + 2*y)*f(b + z + y) + 4*f
> (2*y)*f(y + x)*
>      f(z + x)*f(b + z + y)^2 - 2*f(2*y)*f(y + x)*f(z + x)*f(b
> + 2*y)*f(c
> + z + y) + 2*f(2*y)*f(y + x)^2*f(c + 2*y)*f(c + z + y)
> - 4*f(2*y)*f(
>      y + x)^2*f(b + z + y)*f(c + z + y) + 2*f(2*y)*f(y + x)
> ^2*f(b + 2*z)*
>      f(c + 2*y) - 2*f(2*y)*f(y + x)^2*f(b + 2*y)*f(c + 2*z) +
> 2*f(2*y)^2*
>      f(z + y)*f(c + 2*y)*f(a + z + x) - f(2*y)^2*f(z + y)*f(c
> + 2*x)*f(c
> + 2*y) - 2*f(2*y)^2*f(z + y)*f(c + 2*x)*f(b + z + y) +
> 2*f(2*y)^2*f(
>      z + y)*f(b + 2*z)*f(a + y + x) - 2*f(2*y)^2*f(z + y)*f(a
> + z + y)*f(c
> + y + x) - 2*f(2*y)^
>      2*f(z + y)*f(a + z + y)^2 + 4*f(2*y)^2*f(z + y)*f(a + z
> + x)*f(b + z
> + y) - 2*f(2*y)^2*f(z + y)*f(a + 2*z)*f(b + y + x) + 4*
> f(2*y)^2*f(z
> + y)*f(a + y + x)*f(c + z + y) - f(2*y)^2*f(z + y)*f(a
> + 2*y)*f(a +
>      2*z) - 2*f(2*y)^2*f(z + x)*f(b + z + y)*f(c + y + x) -
> 2*f(2*y)^2*f(z
> + x)*f(b + z + x)*f(b + z + y) - 2*f(2*y)^2*f(z + x)*f
> (a + z + y)*f(
>      b + z + y) - f(2*y)^2*f(z + x)*f(a + 2*z)*f(b + 2*y) +
> 2*f(2*y)^2*f(z
> + x)*f(a + 2*y)*f(c + z + y) + f(2*y)^2*f(z + x)*f(a +
> 2*y)*f(b + 2*
>      z) + f(2*y)^2*f(2*z)*f(c + 2*y)*f(a + y + x) - 1/2*f(2*
> y)^2*f(2*z)*f(
>      b + 2*y)*f(c + 2*x) + f(2*y)^2*f(2*z)*f(b + 2*y)*f(a + z

```

```

+ x) + 1/2*
> f(2*y)^2*f(2*z)*f(b + 2*x)*f(c + 2*y) + f(2*y)^2*f(2*z)*
f(b + 2*x)*f(
> b + z + y) + 2*f(2*y)^2*f(2*z)*f(a + y + x)*f(b + z + y)
- f(2*y)^2*
> f(2*z)*f(a + 2*y)*f(c + y + x) - f(2*y)^2*f(2*z)*f(a +
2*y)*f(b + z
> + x) - f(2*y)^2*f(2*z)*f(a + 2*y)*f(a + z + y) + 2*f(2*
y)^2*f(y + x)
> *f(c + 2*z)*f(b + y + x) - 2*f(2*y)^2*f(y + x)*f(c + y +
x)*f(c + z
> + y) + 2*f(2*y)^2*f(y + x)*f(b + z + x)*f(c + z + y) -
2*f(2*y)^2*f(
> y + x)*f(b + 2*z)*f(c + y + x) + 2*f(2*y)^2*f(y + x)*f(a
+ z + y)*f(c
> + z + y) - f(2*y)^2*f(y + x)*f(a + 2*z)*f(c + 2*y) - 2*
f(2*y)^2*f(y
> + x)*f(a + 2*z)*f(b + z + y) + f(2*y)^2*f(y + x)*f(a +
2*y)*f(c + 2*
> z) - f(2*y)^3*f(c + 2*z)*f(a + y + x) + f(2*y)^3*f(c +
2*x)*f(c + z
> + y) + 1/2*f(2*y)^3*f(b + 2*z)*f(c + 2*x) - f(2*y)^3*f
(b + 2*z)*f(a
> + z + x) - 1/2*f(2*y)^3*f(b + 2*x)*f(c + 2*z) - 2*f(2*
y)^3*f(a + z
> + x)*f(c + z + y) + f(2*y)^3*f(a + 2*z)*f(c + y + x) +
f(2*y)^3*f(a
> + 2*z)*f(b + z + x) + f(2*y)^3*f(a + 2*z)*f(a + z + y)
+ 4*f(2*x)*f(
> z + y)^2*f(b + 2*y)*f(b + z + y) - 2*f(2*x)*f(2*z)*f(z +
y)*f(b + 2*y
> )^2 + f(2*x)*f(2*y)*f(z + y)*f(c + 2*y)^2 - 4*f(2*x)*f
(2*y)*f(z + y)*
> f(b + z + y)^2 - 2*f(2*x)*f(2*y)*f(z + y)*f(b + 2*y)*f(c
+ z + y) -
> f(2*x)*f(2*y)*f(z + y)*f(b + 2*y)*f(b + 2*z) + 2*f(2*x)*
f(2*y)*f(2*z)
> *f(b + 2*y)*f(b + z + y) - f(2*x)*f(2*y)^2*f(c + 2*y)*f
(c + z + y) +
> 2*f(2*x)*f(2*y)^2*f(b + z + y)*f(c + z + y) - 1/2*f(2*x)
*f(2*y)^2*f(b
> + 2*z)*f(c + 2*y) + f(2*x)*f(2*y)^2*f(b + 2*z)*f(b + z
+ y) + 1/2*f(
> 2*x)*f(2*y)^2*f(b + 2*y)*f(c + 2*z) )
>
> + 2*f(z + y)*f(2*b + 2*y) - 2*f(2*y)*f(2*b + z + y):
> eq[7] :=
> (1/HessUniv) * ( 2*f(z + x)*f(z + y)^2*f(a + 2*x)*f(b + 2*y) + 4*
f(z
> + x)^2*f(z + y)*f(b + 2*y)*f(a + y + x) - 2*f(z + x)^2*
f(z + y)*f(b
> + 2*x)*f(b + 2*y) - 4*f(z + x)^2*f(z + y)*f(a + 2*y)*f
(b + y + x) -
> 2*f(z + x)^2*f(z + y)*f(a + 2*y)^2 + 2*f(z + x)^3*f(a +
2*y)*f(b + 2*
> y) + f(2*z)*f(y + x)*f(z + x)*f(b + 2*x)*f(b + 2*y) + 2*

```



```

f(2*z)*f(y +
>      x)*f(z + x)*f(a + 2*y)*f(b + y + x) + f(2*z)*f(y + x)*f
(z + x)*f(a +
>      2*y)^2 - 4*f(y + x)*f(z + x)*f(z + y)*f(b + 2*y)*f(a + z
+ x) - 4*f(y
>      + x)*f(z + x)^2*f(b + 2*y)*f(a + z + y) + 2*f(y + x)^2*
f(z + x)*f(a
>      + 2*z)*f(b + 2*y) - 2*f(2*y)*f(z + y)^2*f(b + 2*x)*f(a
+ z + x) + 2*
>      f(2*y)*f(z + x)*f(z + y)*f(b + 2*x)*f(b + z + x) + 2*f
(2*y)*f(z + x)*
>      f(z + y)*f(b + 2*x)*f(a + z + y) + f(2*y)*f(z + x)*f(z +
y)*f(a + 2*y
>      )*f(c + 2*x) + 2*f(2*y)*f(z + x)*f(z + y)*f(a + 2*y)*f(a
+ z + x) -
>      f(2*y)*f(z + x)*f(z + y)*f(a + 2*x)*f(c + 2*y) - 2*f(2*
y)*f(z + x)*f(
>      z + y)*f(a + 2*x)*f(b + z + y) - 2*f(2*y)*f(z + x)^2*f(c
+ 2*y)*f(a
>      + y + x) + f(2*y)*f(z + x)^2*f(b + 2*y)*f(c + 2*x) + f
(2*y)*f(z + x)
>      ^2*f(b + 2*x)*f(c + 2*y) + 4*f(2*y)*f(z + x)^2*f(a + z +
y)*f(b + y
>      + x) - 4*f(2*y)*f(z + x)^2*f(a + y + x)*f(b + z + y) +
2*f(2*y)*f(z
>      + x)^2*f(a + 2*y)*f(a + z + y) + f(2*y)*f(2*z)*f(z + y)
*f(b + 2*x)*
>      f(a + y + x) - f(2*y)*f(2*z)*f(z + y)*f(a + 2*x)*f(b + y
+ x) - 1/2*
>      f(2*y)*f(2*z)*f(z + x)*f(a + 2*y)*f(b + 2*x) - 3/2*f(2*
y)*f(2*z)*f(z
>      + x)*f(a + 2*x)*f(b + 2*y) - f(2*y)*f(2*z)*f(y + x)*f(b
+ 2*x)*f(b
>      + z + x) - f(2*y)*f(2*z)*f(y + x)*f(b + 2*x)*f(a + z +
y) - 2*f(2*y)
>      *f(2*z)*f(y + x)*f(a + y + x)*f(b + z + x) - f(2*y)*f(2*
z)*f(y + x)*
>      f(a + 2*y)*f(a + z + x) + f(2*y)*f(2*z)*f(y + x)*f(a +
2*x)*f(b + z
>      + y) + 4*f(2*y)*f(y + x)*f(z + y)*f(a + z + x)*f(b + z
+ x) + 2*f(2*
>      y)*f(y + x)*f(z + x)*f(c + 2*y)*f(a + z + x) - f(2*y)*f
(y + x)*f(z +
>      x)*f(c + 2*x)*f(c + 2*y) + 2*f(2*y)*f(y + x)*f(z + x)*f
(b + 2*z)*f(a
>      + y + x) + 4*f(2*y)*f(y + x)*f(z + x)*f(a + z + x)*f(b
+ z + y) - 2*
>      f(2*y)*f(y + x)*f(z + x)*f(a + 2*z)*f(b + y + x) - f(2*
y)*f(y + x)*f(
>      z + x)*f(a + 2*y)*f(a + 2*z) - 2*f(2*y)*f(y + x)^2*f(b +
2*z)*f(a + z
>      + x) + f(2*y)^2*f(z + y)*f(c + 2*x)*f(a + z + x) - f(2*
y)^2*f(z + y)
>      *f(a + 2*x)*f(c + z + x) - f(2*y)^2*f(z + x)*f(c + 2*x)*
f(b + z + x)
>      - 2*f(2*y)^2*f(z + x)*f(c + 2*x)*f(a + z + y) - f(2*y)
^2*f(z + x)*f(

```

```

>      b + 2*x)*f(c + z + x) - 2*f(2*y)^2*f(z + x)*f(a + z + x)
>      *f(b + z + x)
>      - 2*f(2*y)^2*f(z + x)*f(a + z + x)*f(a + z + y) - 1/2*f
>      (2*y)^2*f(z
>      + x)*f(a + 2*z)*f(b + 2*x) + 2*f(2*y)^2*f(z + x)*f(a +
>      y + x)*f(c +
>      z + x) + 2*f(2*y)^2*f(z + x)*f(a + 2*x)*f(c + z + y) +
>      1/2*f(2*y)^2*
>      f(z + x)*f(a + 2*x)*f(b + 2*z) - f(2*y)^2*f(2*z)*f(c +
>      2*x)*f(a + y
>      + x) + f(2*y)^2*f(2*z)*f(b + 2*x)*f(a + z + x) + f(2*y)
>      ^2*f(2*z)*f(a
>      + 2*x)*f(c + y + x) + f(2*y)^2*f(2*z)*f(a + 2*x)*f(b +
>      z + x) + f(2*
>      y)^2*f(y + x)*f(c + 2*x)*f(c + z + x) - 2*f(2*y)^2*f(y +
>      x)*f(a + z
>      + x)*f(c + z + x) + f(2*y)^2*f(y + x)*f(a + 2*z)*f(c +
>      2*x) + f(2*y)
>      ^2*f(y + x)*f(a + 2*z)*f(a + z + x) - f(2*y)^2*f(y + x)*
>      f(a + 2*x)*f(
>      c + 2*z) + 2*f(2*x)*f(z + x)*f(z + y)*f(c + 2*y)*f(b + y
>      + x) - 4*f(2
>      *x)*f(z + x)*f(z + y)*f(b + 2*y)*f(c + y + x) + 2*f(2*x)
>      *f(z + x)*f(z
>      + y)*f(b + 2*y)*f(b + z + x) + 2*f(2*x)*f(z + x)*f(z +
>      y)*f(a + 2*y)
>      *f(c + 2*y) + 2*f(2*x)*f(z + x)*f(z + y)*f(a + 2*y)*f(b
>      + z + y) - 2*
>      f(2*x)*f(2*z)*f(z + x)*f(a + 2*y)*f(b + 2*y) - f(2*x)*f
>      (y + x)*f(z +
>      x)*f(c + 2*y)^2 - 2*f(2*x)*f(y + x)*f(z + x)*f(c + 2*y)*
>      f(b + z + y)
>      + 4*f(2*x)*f(y + x)*f(z + x)*f(b + 2*y)*f(c + z + y) -
>      f(2*x)*f(y +
>      x)*f(z + x)*f(b + 2*y)*f(b + 2*z) - f(2*x)*f(2*y)*f(z +
>      y)*f(c + 2*y)
>      *f(a + z + x) - 2*f(2*x)*f(2*y)*f(z + y)*f(b + z + x)^2
>      - f(2*x)*f(2*
>      y)*f(z + y)*f(b + 2*z)*f(a + y + x) + 2*f(2*x)*f(2*y)*f
>      (z + y)*f(b +
>      y + x)*f(c + z + x) - 2*f(2*x)*f(2*y)*f(z + y)*f(a + z +
>      y)*f(b + z
>      + x) + f(2*x)*f(2*y)*f(z + y)*f(a + 2*z)*f(b + y + x) -
>      f(2*x)*f(2*y
>      )*f(z + y)*f(a + 2*y)*f(c + z + x) + 2*f(2*x)*f(2*y)*f(z
>      + x)*f(c + 2
>      *y)*f(c + y + x) - f(2*x)*f(2*y)*f(z + x)*f(c + 2*y)*f(b
>      + z + x) + 4
>      *f(2*x)*f(2*y)*f(z + x)*f(b + z + y)*f(c + y + x) - 4*f
>      (2*x)*f(2*y)*
>      f(z + x)*f(b + y + x)*f(c + z + y) - f(2*x)*f(2*y)*f(z +
>      x)*f(b + 2*y
>      )*f(c + z + x) + 1/2*f(2*x)*f(2*y)*f(z + x)*f(a + 2*z)*f
>      (b + 2*y) - 2
>      *f(2*x)*f(2*y)*f(z + x)*f(a + 2*y)*f(c + z + y) - 1/2*f
>      (2*x)*f(2*y)*
>      f(z + x)*f(a + 2*y)*f(b + 2*z) + 1/2*f(2*x)*f(2*y)*f(2*

```

```

z)*f(b + 2*y)*
> f(c + 2*x) + f(2*x)*f(2*y)*f(2*z)*f(b + 2*y)*f(a + z +
x) - 1/2*f(2*x
> )*f(2*y)*f(2*z)*f(b + 2*x)*f(c + 2*y) + f(2*x)*f(2*y)*f
(2*z)*f(a + 2*
> y)*f(b + z + x) + f(2*x)*f(2*y)*f(y + x)*f(c + 2*y)*f(c
+ z + x) - 2*
> f(2*x)*f(2*y)*f(y + x)*f(b + z + y)*f(c + z + x) + f(2*
x)*f(2*y)*f(y
> + x)*f(b + 2*z)*f(b + z + x) + f(2*x)*f(2*y)*f(y + x)*f
(b + 2*z)*f(a
> + z + y) - f(2*x)*f(2*y)*f(y + x)*f(a + 2*z)*f(b + z +
y) + f(2*x)*
> f(2*y)^2*f(c + 2*z)*f(a + y + x) - 2*f(2*x)*f(2*y)^2*f(c
+ y + x)*f(c
> + z + x) + 2*f(2*x)*f(2*y)^2*f(b + z + x)*f(c + z + x)
- 1/2*f(2*x)*
> f(2*y)^2*f(b + 2*z)*f(c + 2*x) + 1/2*f(2*x)*f(2*y)^2*f(b
+ 2*x)*f(c
> + 2*z) + 2*f(2*x)*f(2*y)^2*f(a + z + y)*f(c + z + x) -
f(2*x)*f(2*y)
> ^2*f(a + 2*z)*f(c + y + x) + 1/2*f(2*x)^2*f(2*y)*f(b +
2*z)*f(c + 2*y
> ) - 1/2*f(2*x)^2*f(2*y)*f(b + 2*y)*f(c + 2*z) )
>
> + 2*f(z + x)*f(b + a + 2*y) - 2*f(2*y)*f(b + a + z + x):
>
> eq[8] :=
> (1/HessUniv) * ( 2*f(z + y)^3*f(a + 2*x)*f(b + 2*y) + 4*f(z + x)*
f(z
> + y)^2*f(b + 2*y)*f(a + y + x) - 2*f(z + x)*f(z + y)^2*
f(b + 2*x)*f(
> b + 2*y) - 4*f(z + x)*f(z + y)^2*f(a + 2*y)*f(b + y + x)
- 2*f(z + x)
> *f(z + y)^2*f(a + 2*y)^2 + 2*f(z + x)^2*f(z + y)*f(a +
2*y)*f(b + 2*y
> ) + f(2*z)*f(y + x)*f(z + y)*f(b + 2*x)*f(b + 2*y) + 2*f
(2*z)*f(y + x
> )*f(z + y)*f(a + 2*y)*f(b + y + x) + f(2*z)*f(y + x)*f(z
+ y)*f(a + 2
> *y)^2 - 4*f(y + x)*f(z + y)^2*f(b + 2*y)*f(a + z + x) -
4*f(y + x)*f(
> z + x)*f(z + y)*f(b + 2*y)*f(a + z + y) + 2*f(y + x)^2*f
(z + y)*f(a
> + 2*z)*f(b + 2*y) + f(2*y)*f(z + y)^2*f(a + 2*y)*f(c +
2*x) - f(2*y)
> *f(z + y)^2*f(a + 2*x)*f(c + 2*y) - 2*f(2*y)*f(z + y)^2*
f(a + 2*x)*f(
> b + z + y) - 2*f(2*y)*f(z + x)*f(z + y)*f(c + 2*y)*f(a +
y + x) + f(2
> *y)*f(z + x)*f(z + y)*f(b + 2*y)*f(c + 2*x) + f(2*y)*f(z
+ x)*f(z + y
> )*f(b + 2*x)*f(c + 2*y) + 2*f(2*y)*f(z + x)*f(z + y)*f(b
+ 2*x)*f(b
> + z + y) + 4*f(2*y)*f(z + x)*f(z + y)*f(a + z + y)*f(b
+ y + x) - 4*
> f(2*y)*f(z + x)*f(z + y)*f(a + y + x)*f(b + z + y) + 2*f

```

```

(2*y)*f(z + x
> )*f(z + y)*f(a + 2*y)*f(b + z + x) + 4*f(2*y)*f(z + x)*f
(z + y)*f(a
> + 2*y)*f(a + z + y) - 2*f(2*y)*f(z + x)^2*f(a + 2*y)*f
(b + z + y) -
> 1/2*f(2*y)*f(2*z)*f(z + y)*f(a + 2*y)*f(b + 2*x) - 3/2*f
(2*y)*f(2*z)*
> f(z + y)*f(a + 2*x)*f(b + 2*y) - f(2*y)*f(2*z)*f(z + x)*
f(b + 2*y)*f(
> a + y + x) + f(2*y)*f(2*z)*f(z + x)*f(a + 2*y)*f(b + y +
x) + f(2*y)*
> f(2*z)*f(y + x)*f(b + 2*y)*f(a + z + x) - f(2*y)*f(2*z)*
f(y + x)*f(b
> + 2*x)*f(b + z + y) - 2*f(2*y)*f(2*z)*f(y + x)*f(a + z
+ y)*f(b + y
> + x) - f(2*y)*f(2*z)*f(y + x)*f(a + 2*y)*f(b + z + x) -
f(2*y)*f(2*z
> )*f(y + x)*f(a + 2*y)*f(a + z + y) + 2*f(2*y)*f(y + x)*f
(z + y)*f(c
> + 2*y)*f(a + z + x) - f(2*y)*f(y + x)*f(z + y)*f(c + 2*
x)*f(c + 2*y)
> + 4*f(2*y)*f(y + x)*f(z + y)*f(a + z + x)*f(b + z + y)
- f(2*y)*f(y
> + x)*f(z + y)*f(a + 2*y)*f(a + 2*z) + 4*f(2*y)*f(y + x)
*f(z + x)*f(a
> + z + y)*f(b + z + y) - 2*f(2*y)*f(y + x)^2*f(a + 2*z)*
f(b + z + y)
> - f(2*y)^2*f(z + y)*f(c + 2*x)*f(a + z + y) - 1/2*f(2*
y)^2*f(z + y)*
> f(a + 2*z)*f(b + 2*x) + f(2*y)^2*f(z + y)*f(a + 2*x)*f(c
+ z + y) + 1/
> 2*f(2*y)^2*f(z + y)*f(a + 2*x)*f(b + 2*z) - f(2*y)^2*f(z
+ x)*f(c + 2
> *x)*f(b + z + y) + f(2*y)^2*f(z + x)*f(b + 2*z)*f(a + y
+ x) - f(2*y)
> ^2*f(z + x)*f(b + 2*x)*f(c + z + y) - 2*f(2*y)^2*f(z +
x)*f(a + z + y
> )*f(b + z + x) - 2*f(2*y)^2*f(z + x)*f(a + z + y)^2 - f
(2*y)^2*f(z +
> x)*f(a + 2*z)*f(b + y + x) + 2*f(2*y)^2*f(z + x)*f(a + y
+ x)*f(c + z
> + y) + f(2*y)^2*f(2*z)*f(b + 2*x)*f(a + z + y) - 1/2*f
(2*y)^2*f(2*z)
> *f(a + 2*y)*f(c + 2*x) + 1/2*f(2*y)^2*f(2*z)*f(a + 2*x)*
f(c + 2*y) +
> f(2*y)^2*f(2*z)*f(a + 2*x)*f(b + z + y) + f(2*y)^2*f(y +
x)*f(c + 2*x
> )*f(c + z + y) - f(2*y)^2*f(y + x)*f(b + 2*z)*f(a + z +
x) - 2*f(2*y)
> ^2*f(y + x)*f(a + z + x)*f(c + z + y) + f(2*y)^2*f(y +
x)*f(a + 2*z)*
> f(b + z + x) + f(2*y)^2*f(y + x)*f(a + 2*z)*f(a + z + y)
+ 1/2*f(2*y)
> ^3*f(a + 2*z)*f(c + 2*x) - 1/2*f(2*y)^3*f(a + 2*x)*f(c +
2*z) + 2*f(2
> *x)*f(z + y)^2*f(c + 2*y)*f(b + y + x) - 4*f(2*x)*f(z +
y)^2*f(b + 2*

```

```

> y)*f(c + y + x) + 2*f(2*x)*f(z + y)^2*f(b + 2*y)*f(b + z
+ x) + 2*f(2
> *x)*f(z + y)^2*f(a + 2*y)*f(c + 2*y) + 2*f(2*x)*f(z + y)
^2*f(a + 2*y)
> *f(b + z + y) - 2*f(2*x)*f(2*z)*f(z + y)*f(a + 2*y)*f(b
+ 2*y) - f(2*
> x)*f(y + x)*f(z + y)*f(c + 2*y)^2 - 2*f(2*x)*f(y + x)*f
(z + y)*f(c +
> 2*y)*f(b + z + y) + 4*f(2*x)*f(y + x)*f(z + y)*f(b + 2*
y)*f(c + z + y
> ) - f(2*x)*f(y + x)*f(z + y)*f(b + 2*y)*f(b + 2*z) + 2*f
(2*x)*f(2*y)*
> f(z + y)*f(c + 2*y)*f(c + y + x) - 2*f(2*x)*f(2*y)*f(z +
y)*f(c + 2*y
> )*f(b + z + x) - f(2*x)*f(2*y)*f(z + y)*f(c + 2*y)*f(a +
z + y) + 4*
> f(2*x)*f(2*y)*f(z + y)*f(b + z + y)*f(c + y + x) - 2*f
(2*x)*f(2*y)*f(
> z + y)*f(b + z + x)*f(b + z + y) - 2*f(2*x)*f(2*y)*f(z +
y)*f(b + y
> + x)*f(c + z + y) - 2*f(2*x)*f(2*y)*f(z + y)*f(a + z +
y)*f(b + z +
> y) + 1/2*f(2*x)*f(2*y)*f(z + y)*f(a + 2*z)*f(b + 2*y) -
3*f(2*x)*f(2*
> y)*f(z + y)*f(a + 2*y)*f(c + z + y) - 1/2*f(2*x)*f(2*y)*
f(z + y)*f(a
> + 2*y)*f(b + 2*z) + f(2*x)*f(2*y)*f(z + x)*f(c + 2*y)*f
(b + z + y)
> - f(2*x)*f(2*y)*f(z + x)*f(b + 2*y)*f(c + z + y) - f(2*
x)*f(2*y)*f(2
> *z)*f(c + 2*y)*f(b + y + x) + f(2*x)*f(2*y)*f(2*z)*f(b +
2*y)*f(c + y
> + x) + f(2*x)*f(2*y)*f(2*z)*f(b + 2*y)*f(a + z + y) + f
(2*x)*f(2*y)*
> f(2*z)*f(a + 2*y)*f(b + z + y) + f(2*x)*f(2*y)*f(y + x)*
f(c + 2*y)*f(
> c + z + y) - 2*f(2*x)*f(2*y)*f(y + x)*f(b + z + y)*f(c +
z + y) + f(2
> *x)*f(2*y)*f(y + x)*f(b + 2*z)*f(c + 2*y) + f(2*x)*f(2*
y)*f(y + x)*f(
> b + 2*z)*f(b + z + y) - f(2*x)*f(2*y)*f(y + x)*f(b + 2*
y)*f(c + 2*z)
> + f(2*x)*f(2*y)^2*f(c + 2*z)*f(b + y + x) - 2*f(2*x)*f
(2*y)^2*f(c +
> y + x)*f(c + z + y) + 2*f(2*x)*f(2*y)^2*f(b + z + x)*f(c
+ z + y) -
> f(2*x)*f(2*y)^2*f(b + 2*z)*f(c + y + x) + 2*f(2*x)*f(2*
y)^2*f(a + z
> + y)*f(c + z + y) - 1/2*f(2*x)*f(2*y)^2*f(a + 2*z)*f(c
+ 2*y) + 1/2*
> f(2*x)*f(2*y)^2*f(a + 2*y)*f(c + 2*z) )

> + 2*f(z + y)*f(b + a + 2*y) - 2*f(2*y)*f(b + a + z + y):

> eq[9] :=
> (1/HessUniv) * ( 4*f(2*z)*f(y + x)*f(z + y)*f(b + 2*y)*f(a + y +
x)

```

```

> - f(2*z)*f(y + x)*f(z + y)*f(b + 2*x)*f(b + 2*y) - 2*f
(2*z)*f(y + x)
> *f(z + y)*f(a + 2*y)*f(b + y + x) - f(2*z)*f(y + x)*f(z
+ y)*f(a + 2*
> y)^2 + 2*f(y + x)*f(z + y)^2*f(b + 2*y)*f(c + 2*x) + 4*f
(y + x)*f(z
> + x)*f(z + y)*f(c + 2*y)*f(b + y + x) - 4*f(y + x)*f(z
+ x)*f(z + y)
> *f(b + 2*y)*f(c + y + x) + 4*f(y + x)*f(z + x)*f(z + y)*
f(b + 2*y)*f(
> b + z + x) - 8*f(y + x)*f(z + x)*f(z + y)*f(b + 2*y)*f(a
+ z + y) + 4
> *f(y + x)*f(z + x)*f(z + y)*f(a + 2*y)*f(c + 2*y) + 4*f
(y + x)*f(z +
> x)*f(z + y)*f(a + 2*y)*f(b + z + y) + 2*f(y + x)*f(z +
x)^2*f(b + 2*y
> )*f(c + 2*y) - 4*f(y + x)^2*f(z + y)*f(b + 2*y)*f(c + z
+ x) - 2*f(y
> + x)^2*f(z + x)*f(c + 2*y)^2 - 4*f(y + x)^2*f(z + x)*f
(c + 2*y)*f(b
> + z + y) + 4*f(y + x)^2*f(z + x)*f(b + 2*y)*f(c + z +
y) - 2*f(y + x
> )^2*f(z + x)*f(b + 2*y)*f(b + 2*z) + 2*f(y + x)^3*f(b +
2*y)*f(c + 2*
> z) - 2*f(2*y)*f(z + y)^2*f(c + 2*x)*f(b + y + x) + 4*f
(2*y)*f(z + x)*
> f(z + y)*f(b + y + x)*f(c + y + x) - 4*f(2*y)*f(z + x)
^2*f(c + 2*y)*
> f(b + y + x) - 2*f(2*y)*f(z + x)^2*f(b + 2*y)*f(b + z +
x) + 4*f(2*y)
> *f(z + x)^2*f(b + 2*y)*f(a + z + y) - 2*f(2*y)*f(z + x)
^2*f(a + 2*y)*
> f(c + 2*y) - 2*f(2*y)*f(z + x)^2*f(a + 2*y)*f(b + z + y)
+ f(2*y)*f(2
> *z)*f(z + y)*f(b + 2*x)*f(b + y + x) - 2*f(2*y)*f(2*z)*f
(z + y)*f(a
> + y + x)*f(b + y + x) + f(2*y)*f(2*z)*f(z + y)*f(a + 2*
y)*f(b + 2*x)
> + f(2*y)*f(2*z)*f(z + y)*f(a + 2*y)*f(a + y + x) - f(2*
y)*f(2*z)*f(z
> + y)*f(a + 2*x)*f(b + 2*y) - f(2*y)*f(2*z)*f(z + x)*f(b
+ 2*y)*f(a
> + y + x) + f(2*y)*f(2*z)*f(z + x)*f(a + 2*y)*f(b + y +
x) - 3*f(2*y)
> *f(2*z)*f(y + x)*f(c + 2*y)*f(a + y + x) - 2*f(2*y)*f(2*
z)*f(y + x)*
> f(b + y + x)*f(c + y + x) - 2*f(2*y)*f(2*z)*f(y + x)*f(b
+ y + x)*f(b
> + z + x) + 1/2*f(2*y)*f(2*z)*f(y + x)*f(b + 2*y)*f(c +
2*x) - 1/2*f(
> 2*y)*f(2*z)*f(y + x)*f(b + 2*x)*f(c + 2*y) + 4*f(2*y)*f
(2*z)*f(y + x)
> *f(a + z + y)*f(b + y + x) - 2*f(2*y)*f(2*z)*f(y + x)*f
(a + y + x)*f(
> b + z + y) - f(2*y)*f(2*z)*f(y + x)*f(a + 2*y)*f(c + y +
x) - 2*f(2*y
> )*f(2*z)*f(y + x)*f(a + 2*y)*f(b + z + x) + 2*f(2*y)*f

```

```

(2*z)*f(y + x)*
> f(a + 2*y)*f(a + z + y) - f(2*y)*f(y + x)*f(z + y)*f(c +
2*x)*f(c + 2
> *y) + 4*f(2*y)*f(y + x)*f(z + y)*f(b + y + x)*f(c + z +
x) + 2*f(2*y)
> *f(y + x)*f(z + y)*f(a + 2*y)*f(c + z + x) - f(2*y)*f(y
+ x)*f(z + y)
> *f(a + 2*y)*f(a + 2*z) + 4*f(2*y)*f(y + x)*f(z + x)*f(c
+ 2*y)*f(c +
> y + x) + 2*f(2*y)*f(y + x)*f(z + x)*f(c + 2*y)*f(b + z +
x) + 4*f(2*y)
> )*f(y + x)*f(z + x)*f(b + z + y)*f(c + y + x) + 2*f(2*y)
*f(y + x)*f(z
> + x)*f(b + 2*z)*f(b + y + x) - 4*f(2*y)*f(y + x)*f(z +
x)*f(b + y +
> x)*f(c + z + y) + f(2*y)*f(y + x)*f(z + x)*f(a + 2*z)*f
(b + 2*y) - 2*
> f(2*y)*f(y + x)*f(z + x)*f(a + 2*y)*f(c + z + y) + f(2*
y)*f(y + x)*f(
> z + x)*f(a + 2*y)*f(b + 2*z) - 2*f(2*y)*f(y + x)^2*f(c +
2*z)*f(b + y
> + x) + f(2*y)*f(y + x)^2*f(a + 2*z)*f(c + 2*y) - f(2*y)
*f(y + x)^2*
> f(a + 2*y)*f(c + 2*z) + f(2*y)^2*f(z + y)*f(c + 2*x)*f(c
+ y + x) +
> f(2*y)^2*f(z + y)*f(c + 2*x)*f(b + z + x) - f(2*y)^2*f(z
+ y)*f(b + 2
> *x)*f(c + z + x) + f(2*y)^2*f(z + y)*f(a + 2*z)*f(a + y
+ x) - 2*f(2*
> y)^2*f(z + y)*f(a + y + x)*f(c + z + x) - 2*f(2*y)^2*f(z
+ x)*f(c + y
> + x)^2 - f(2*y)^2*f(z + x)*f(c + 2*x)*f(b + z + y) - 2*
f(2*y)^2*f(z
> + x)*f(b + z + x)*f(c + y + x) - f(2*y)^2*f(z + x)*f(b
+ 2*z)*f(a +
> y + x) + f(2*y)^2*f(z + x)*f(b + 2*x)*f(c + z + y) - f
(2*y)^2*f(z + x
> )*f(a + 2*z)*f(b + y + x) + 2*f(2*y)^2*f(z + x)*f(a + y
+ x)*f(c + z
> + y) - f(2*y)^2*f(2*z)*f(b + 2*x)*f(a + z + y) + 2*f(2*
y)^2*f(2*z)*
> f(a + y + x)*f(c + y + x) + 2*f(2*y)^2*f(2*z)*f(a + y +
x)*f(b + z +
> x) - 2*f(2*y)^2*f(2*z)*f(a + y + x)*f(a + z + y) - 1/2*f
(2*y)^2*f(2*z
> )*f(a + 2*y)*f(c + 2*x) + 1/2*f(2*y)^2*f(2*z)*f(a + 2*x)
*f(c + 2*y)
> + f(2*y)^2*f(2*z)*f(a + 2*x)*f(b + z + y) + f(2*y)^2*f
(y + x)*f(c +
> 2*z)*f(a + y + x) - 1/2*f(2*y)^2*f(y + x)*f(b + 2*z)*f(c
+ 2*x) + 1/2
> *f(2*y)^2*f(y + x)*f(b + 2*x)*f(c + 2*z) - f(2*y)^2*f(y
+ x)*f(a + 2*
> z)*f(c + y + x) + 1/2*f(2*y)^3*f(a + 2*z)*f(c + 2*x) -
1/2*f(2*y)^3*
> f(a + 2*x)*f(c + 2*z) - 2*f(2*x)*f(z + y)^2*f(c + 2*y)*f
(b + y + x)

```

```

> - 2*f(2*x)*f(z + y)^2*f(b + 2*y)*f(b + z + x) + 4*f(2*
x)*f(z + y)^2*
> f(b + 2*y)*f(a + z + y) - 2*f(2*x)*f(z + y)^2*f(a + 2*y)
*f(c + 2*y)
> - 2*f(2*x)*f(z + y)^2*f(a + 2*y)*f(b + z + y) - 2*f(2*
x)*f(2*z)*f(y
> + x)*f(b + 2*y)*f(c + 2*y) + f(2*x)*f(y + x)*f(z + y)*f
(c + 2*y)^2
> + 2*f(2*x)*f(y + x)*f(z + y)*f(c + 2*y)*f(b + z + y) +
f(2*x)*f(y +
> x)*f(z + y)*f(b + 2*y)*f(b + 2*z) - f(2*x)*f(2*y)*f(z +
y)*f(c + 2*y)
> *f(c + y + x) - f(2*x)*f(2*y)*f(z + y)*f(c + 2*y)*f(b +
z + x) - 2*f(
> 2*x)*f(2*y)*f(z + y)*f(b + z + y)*f(c + y + x) - f(2*x)*
f(2*y)*f(z +
> y)*f(b + 2*z)*f(b + y + x) + f(2*x)*f(2*y)*f(z + y)*f(b
+ 2*y)*f(c +
> z + x) + f(2*x)*f(2*y)*f(z + x)*f(c + 2*y)*f(b + z + y)
- f(2*x)*f(2*
> y)*f(z + x)*f(b + 2*y)*f(c + z + y) + 3*f(2*x)*f(2*y)*f
(2*z)*f(c + 2*
> y)*f(b + y + x) + f(2*x)*f(2*y)*f(2*z)*f(b + 2*y)*f(c +
y + x) + 2*f(
> 2*x)*f(2*y)*f(2*z)*f(b + 2*y)*f(b + z + x) - 3*f(2*x)*f
(2*y)*f(2*z)*
> f(b + 2*y)*f(a + z + y) + 2*f(2*x)*f(2*y)*f(2*z)*f(a +
2*y)*f(c + 2*y
> ) + f(2*x)*f(2*y)*f(2*z)*f(a + 2*y)*f(b + z + y) - 1/2*f
(2*x)*f(2*y)*
> f(y + x)*f(b + 2*z)*f(c + 2*y) - 3/2*f(2*x)*f(2*y)*f(y +
x)*f(b + 2*y
> )*f(c + 2*z) + f(2*x)*f(2*y)^2*f(c + 2*z)*f(b + y + x) +
f(2*x)*f(2*y
> )^2*f(b + 2*z)*f(c + y + x) - 1/2*f(2*x)*f(2*y)^2*f(a +
2*z)*f(c + 2*
> y) + 1/2*f(2*x)*f(2*y)^2*f(a + 2*y)*f(c + 2*z) )

> - 2*f(c + 2*y)*f(b + y + x) - 2*f(b + 2*y)*f(b + z + x) +
4*f(b + 2*y)*
> f(a + z + y) - 2*f(a + 2*y)*f(c + 2*y) - 2*f(a + 2*y)*f
(b + z + y) +
> 2*f(y + x)*f(c + b + 2*y) - 2*f(2*y)*f(c + b + y + x):

> eq[10] :=
> (1/HessUniv) * ( - f(2*z)*f(y + x)*f(z + y)*f(a + 2*y)*f(b + 2*
x) +
> f(2*z)*f(y + x)*f(z + y)*f(a + 2*x)*f(b + 2*y) + 2*f(2*
z)*f(y + x)*f(
> z + x)*f(b + 2*y)*f(a + y + x) - f(2*z)*f(y + x)*f(z +
x)*f(b + 2*x)*
> f(b + 2*y) - f(2*z)*f(y + x)*f(z + x)*f(a + 2*y)^2 + 2*f
(y + x)*f(z
> + y)^2*f(a + 2*y)*f(c + 2*x) + 2*f(y + x)*f(z + x)*f(z
+ y)*f(b + 2*
> y)*f(c + 2*x) - 4*f(y + x)*f(z + x)*f(z + y)*f(b + 2*y)*
f(a + z + x)

```



```

> + 2*f(y + x)*f(z + x)*f(z + y)*f(b + 2*x)*f(c + 2*y) +
4*f(y + x)*f(
> z + x)*f(z + y)*f(a + 2*y)*f(a + z + y) + 2*f(y + x)*f(z
+ x)^2*f(a
> + 2*y)*f(c + 2*y) - 2*f(y + x)^2*f(z + y)*f(c + 2*x)*f
(c + 2*y) - 2*
> f(y + x)^2*f(z + y)*f(a + 2*y)*f(a + 2*z) - 4*f(y + x)
^2*f(z + x)*f(c
> + 2*y)*f(a + z + y) + 2*f(y + x)^3*f(a + 2*z)*f(c + 2*
y) - 2*f(2*y)*
> f(z + y)^2*f(c + 2*x)*f(a + y + x) + 4*f(2*y)*f(z + x)*f
(z + y)*f(a
> + y + x)*f(c + y + x) - 2*f(2*y)*f(z + x)^2*f(c + 2*y)*
f(a + y + x)
> - f(2*y)*f(z + x)^2*f(b + 2*y)*f(c + 2*x) + 2*f(2*y)*f
(z + x)^2*f(b
> + 2*y)*f(a + z + x) - f(2*y)*f(z + x)^2*f(b + 2*x)*f(c
+ 2*y) - 2*f(
> 2*y)*f(z + x)^2*f(a + 2*y)*f(c + y + x) - 2*f(2*y)*f(z +
x)^2*f(a + 2
> *y)*f(a + z + y) + f(2*y)*f(2*z)*f(z + y)*f(b + 2*x)*f(a
+ y + x) -
> f(2*y)*f(2*z)*f(z + y)*f(a + 2*x)*f(b + y + x) + f(2*y)*
f(2*z)*f(z +
> x)*f(b + 2*x)*f(b + y + x) - 2*f(2*y)*f(2*z)*f(z + x)*f
(a + y + x)*f(
> b + y + x) + f(2*y)*f(2*z)*f(z + x)*f(a + 2*y)*f(b + 2*
x) + f(2*y)*f(
> 2*z)*f(z + x)*f(a + 2*y)*f(a + y + x) - f(2*y)*f(2*z)*f
(z + x)*f(a +
> 2*x)*f(b + 2*y) - f(2*y)*f(2*z)*f(y + x)*f(c + 2*x)*f(b
+ y + x) - f(
> 2*y)*f(2*z)*f(y + x)*f(b + 2*x)*f(c + y + x) + 2*f(2*y)*
f(2*z)*f(y +
> x)*f(a + z + x)*f(b + y + x) - 2*f(2*y)*f(2*z)*f(y + x)*
f(a + y + x)*
> f(c + y + x) - 2*f(2*y)*f(2*z)*f(y + x)*f(a + y + x)*f(a
+ z + y) - 3/
> 2*f(2*y)*f(2*z)*f(y + x)*f(a + 2*y)*f(c + 2*x) - 1/2*f
(2*y)*f(2*z)*f(
> y + x)*f(a + 2*x)*f(c + 2*y) + 2*f(2*y)*f(y + x)*f(z +
y)*f(c + 2*x)*
> f(c + y + x) + 2*f(2*y)*f(y + x)*f(z + y)*f(a + 2*z)*f(a
+ y + x) + 2
> *f(2*y)*f(y + x)*f(z + x)*f(c + 2*y)*f(a + z + x) + f(2*
y)*f(y + x)*
> f(z + x)*f(c + 2*x)*f(c + 2*y) + 4*f(2*y)*f(y + x)*f(z +
x)*f(a + z
> + y)*f(c + y + x) + f(2*y)*f(y + x)*f(z + x)*f(a + 2*y)
*f(a + 2*z)
> - 2*f(2*y)*f(y + x)^2*f(a + 2*z)*f(c + y + x) + f(2*y)
^2*f(z + y)*f(
> c + 2*x)*f(a + z + x) - f(2*y)^2*f(z + y)*f(a + 2*x)*f(c
+ z + x) -
> f(2*y)^2*f(z + x)*f(c + 2*x)*f(c + y + x) - f(2*y)^2*f(z
+ x)*f(c + 2
> *x)*f(a + z + y) - 2*f(2*y)^2*f(z + x)*f(a + z + x)*f(c

```

```

+ y + x) - f(
>      2*y)^2*f(z + x)*f(a + 2*z)*f(a + y + x) + f(2*y)^2*f(z +
x)*f(a + 2*x
>      )*f(c + z + y) + f(2*y)^2*f(2*z)*f(c + 2*x)*f(a + y + x)
- f(2*y)^2*
>      f(2*z)*f(b + 2*x)*f(a + z + x) + f(2*y)^2*f(2*z)*f(a +
2*x)*f(c + y
>      + x) + f(2*y)^2*f(2*z)*f(a + 2*x)*f(b + z + x) + 1/2*f
(2*y)^2*f(y +
>      x)*f(a + 2*z)*f(c + 2*x) - 1/2*f(2*y)^2*f(y + x)*f(a +
2*x)*f(c + 2*z
>      ) - f(2*x)*f(z + y)^2*f(b + 2*y)*f(c + 2*x) + 2*f(2*x)*f
(z + y)^2*f(b
>      + 2*y)*f(a + z + x) - f(2*x)*f(z + y)^2*f(b + 2*x)*f(c
+ 2*y) - 2*f(
>      2*x)*f(z + y)^2*f(a + 2*y)*f(c + y + x) - 2*f(2*x)*f(z +
y)^2*f(a + 2
>      *y)*f(a + z + y) - 2*f(2*x)*f(2*z)*f(y + x)*f(b + 2*y)*f
(c + y + x)
>      + 2*f(2*x)*f(2*z)*f(y + x)*f(b + 2*y)*f(b + z + x) - 2*
f(2*x)*f(2*z)
>      *f(y + x)*f(b + 2*y)*f(a + z + y) + 2*f(2*x)*f(y + x)*f
(z + y)*f(c +
>      2*y)*f(c + y + x) + 2*f(2*x)*f(y + x)*f(z + y)*f(c + 2*
y)*f(a + z + y
>      ) - 2*f(2*x)*f(y + x)*f(z + y)*f(b + 2*y)*f(c + z + x) +
f(2*x)*f(y
>      + x)*f(z + y)*f(a + 2*z)*f(b + 2*y) + f(2*x)*f(y + x)*f
(z + y)*f(a
>      + 2*y)*f(b + 2*z) - f(2*x)*f(y + x)*f(z + x)*f(c + 2*y)
^2 + 2*f(2*x)
>      *f(y + x)*f(z + x)*f(b + 2*y)*f(c + z + y) - f(2*x)*f(y
+ x)*f(z + x)
>      *f(b + 2*y)*f(b + 2*z) - f(2*x)*f(y + x)^2*f(b + 2*z)*f
(c + 2*y) + f(
>      2*x)*f(y + x)^2*f(b + 2*y)*f(c + 2*z) - 2*f(2*x)*f(2*y)*
f(z + y)*f(c
>      + y + x)^2 - f(2*x)*f(2*y)*f(z + y)*f(c + 2*y)*f(a + z
+ x) - f(2*x)
>      *f(2*y)*f(z + y)*f(b + 2*z)*f(a + y + x) + 2*f(2*x)*f(2*
y)*f(z + y)*
>      f(b + y + x)*f(c + z + x) - 2*f(2*x)*f(2*y)*f(z + y)*f(a
+ z + y)*f(c
>      + y + x) - f(2*x)*f(2*y)*f(z + y)*f(a + 2*z)*f(b + y +
x) + f(2*x)*
>      f(2*y)*f(z + y)*f(a + 2*y)*f(c + z + x) + f(2*x)*f(2*y)*
f(z + x)*f(c
>      + 2*y)*f(c + y + x) + f(2*x)*f(2*y)*f(z + x)*f(c + 2*y)
*f(a + z + y)
>      + f(2*x)*f(2*y)*f(z + x)*f(b + 2*z)*f(b + y + x) - 2*f
(2*x)*f(2*y)*
>      f(z + x)*f(b + y + x)*f(c + z + y) - f(2*x)*f(2*y)*f(z +
x)*f(a + 2*y
>      )*f(c + z + y) + 2*f(2*x)*f(2*y)*f(2*z)*f(b + y + x)*f(c
+ y + x) - 2
>      *f(2*x)*f(2*y)*f(2*z)*f(b + y + x)*f(b + z + x) + 3/2*f
(2*x)*f(2*y)*

```

```

>      f(2*z)*f(b + 2*y)*f(c + 2*x) - f(2*x)*f(2*y)*f(2*z)*f(b
> + 2*y)*f(a +
>      z + x) + 1/2*f(2*x)*f(2*y)*f(2*z)*f(b + 2*x)*f(c + 2*y)
> + 2*f(2*x)*f(
>      2*y)*f(2*z)*f(a + z + y)*f(b + y + x) + 2*f(2*x)*f(2*y)*
> f(2*z)*f(a +
>      2*y)*f(c + y + x) - f(2*x)*f(2*y)*f(2*z)*f(a + 2*y)*f(b
> + z + x) + 2*
>      f(2*x)*f(2*y)*f(2*z)*f(a + 2*y)*f(a + z + y) - f(2*x)*f
> (2*y)*f(y + x)
>      *f(c + 2*z)*f(b + y + x) + f(2*x)*f(2*y)*f(y + x)*f(b +
> 2*z)*f(c + y
>      + x) - 3/2*f(2*x)*f(2*y)*f(y + x)*f(a + 2*z)*f(c + 2*y)
> - 1/2*f(2*x)
>      *f(2*y)*f(y + x)*f(a + 2*y)*f(c + 2*z) + f(2*x)*f(2*y)
> ^2*f(c + 2*z)*
>      f(a + y + x) - 1/2*f(2*x)*f(2*y)^2*f(b + 2*z)*f(c + 2*x)
> + 1/2*f(2*x)
>      *f(2*y)^2*f(b + 2*x)*f(c + 2*z) + f(2*x)*f(2*y)^2*f(a +
> 2*z)*f(c + y
>      + x) + 1/2*f(2*x)^2*f(2*y)*f(b + 2*z)*f(c + 2*y) - 1/2*
> f(2*x)^2*f(2*
>      y)*f(b + 2*y)*f(c + 2*z) )
>
>      - f(b + 2*y)*f(c + 2*x) + 2*f(b + 2*y)*f(a + z + x) - f(b
> + 2*x)*f(c +
>      2*y) - 2*f(a + 2*y)*f(c + y + x) - 2*f(a + 2*y)*f(a + z
> + y) + 2*f(y
>      + x)*f(c + a + 2*y) - 2*f(2*y)*f(c + a + y + x):
> eq[11] :=
> (1/HessUniv) * ( - f(2*y)*f(z + y)^2*f(b + 2*x)*f(c + 2*x) + 2*f
> (2*y
>      )*f(z + x)*f(z + y)*f(b + 2*x)*f(c + y + x) - f(2*y)*f(z
> + x)^2*f(b
>      + 2*x)*f(c + 2*y) + 1/2*f(2*y)*f(2*z)*f(z + y)*f(b + 2*
> x)^2 - f(2*y)
>      *f(2*z)*f(z + y)*f(a + 2*x)*f(b + y + x) + 1/2*f(2*y)*f
> (2*z)*f(z + y)
>      *f(a + 2*x)*f(a + 2*y) + 1/2*f(2*y)*f(2*z)*f(z + x)*f(a
> + 2*y)*f(b +
>      2*x) - 1/2*f(2*y)*f(2*z)*f(z + x)*f(a + 2*x)*f(b + 2*y)
> - f(2*y)*f(2*
>      z)*f(y + x)*f(b + 2*x)*f(c + y + x) - f(2*y)*f(2*z)*f(y
> + x)*f(b + 2*
>      x)*f(b + z + x) - 1/2*f(2*y)*f(2*z)*f(y + x)*f(a + 2*y)*
> f(c + 2*x) -
>      1/2*f(2*y)*f(2*z)*f(y + x)*f(a + 2*x)*f(c + 2*y) + f(2*
> y)*f(2*z)*f(y
>      + x)*f(a + 2*x)*f(b + z + y) + 2*f(2*y)*f(y + x)*f(z +
> y)*f(c + 2*x)
>      *f(b + z + x) + f(2*y)*f(y + x)*f(z + x)*f(c + 2*x)*f(c
> + 2*y) + f(2*
>      y)*f(y + x)*f(z + x)*f(b + 2*x)*f(b + 2*z) - f(2*y)*f(y
> + x)^2*f(b +
>      2*z)*f(c + 2*x) + 1/2*f(2*y)^2*f(z + y)*f(c + 2*x)^2 - f
> (2*y)^2*f(z
>      + y)*f(a + 2*x)*f(c + z + x) + 1/2*f(2*y)^2*f(z + y)*f

```

```

(a + 2*x)*f(a
> + 2*z) - f(2*y)^2*f(z + x)*f(c + 2*x)*f(c + y + x) - f
(2*y)^2*f(z +
> x)*f(c + 2*x)*f(b + z + x) - 1/2*f(2*y)^2*f(z + x)*f(a +
2*z)*f(b + 2
> *x) + f(2*y)^2*f(z + x)*f(a + 2*x)*f(c + z + y) - 1/2*f
(2*y)^2*f(z +
> x)*f(a + 2*x)*f(b + 2*z) + f(2*y)^2*f(2*z)*f(a + 2*x)*f
(c + y + x) +
> f(2*y)^2*f(2*z)*f(a + 2*x)*f(b + z + x) - f(2*y)^2*f(2*
z)*f(a + 2*x)*
> f(a + z + y) + 1/2*f(2*y)^2*f(y + x)*f(a + 2*z)*f(c + 2*
x) - 1/2*f(2*
> y)^2*f(y + x)*f(a + 2*x)*f(c + 2*z) + f(2*x)*f(z + y)^2*
f(b + 2*y)*f(
> c + 2*x) - 2*f(2*x)*f(z + x)*f(z + y)*f(b + 2*y)*f(c + y
+ x) + f(2*x
> )*f(z + x)^2*f(b + 2*y)*f(c + 2*y) + 2*f(2*x)*f(2*z)*f(z
+ y)*f(b + 2
> *y)*f(a + y + x) - 1/2*f(2*x)*f(2*z)*f(z + y)*f(b + 2*x)
*f(b + 2*y)
> - f(2*x)*f(2*z)*f(z + y)*f(a + 2*y)*f(b + y + x) - 1/2*
f(2*x)*f(2*z)
> *f(z + y)*f(a + 2*y)^2 + f(2*x)*f(2*z)*f(y + x)*f(c + 2*
y)*f(b + y +
> x) + f(2*x)*f(2*z)*f(y + x)*f(b + 2*y)*f(b + z + x) - 2*
f(2*x)*f(2*z)
> *f(y + x)*f(b + 2*y)*f(a + z + y) + f(2*x)*f(2*z)*f(y +
x)*f(a + 2*y)
> *f(c + 2*y) + f(2*x)*f(2*z)*f(y + x)*f(a + 2*y)*f(b + z
+ y) - 2*f(2*
> x)*f(y + x)*f(z + y)*f(b + 2*y)*f(c + z + x) - f(2*x)*f
(y + x)*f(z +
> x)*f(c + 2*y)^2 - 2*f(2*x)*f(y + x)*f(z + x)*f(c + 2*y)*
f(b + z + y)
> + 2*f(2*x)*f(y + x)*f(z + x)*f(b + 2*y)*f(c + z + y) -
f(2*x)*f(y +
> x)*f(z + x)*f(b + 2*y)*f(b + 2*z) + f(2*x)*f(y + x)^2*f
(b + 2*y)*f(c
> + 2*z) - f(2*x)*f(2*y)*f(z + y)*f(c + 2*x)*f(c + 2*y) -
f(2*x)*f(2*y)
> )*f(z + y)*f(c + 2*x)*f(b + z + y) - 2*f(2*x)*f(2*y)*f(z
+ y)*f(b + z
> + x)*f(c + y + x) + 2*f(2*x)*f(2*y)*f(z + y)*f(b + y +
x)*f(c + z +
> x) - 1/2*f(2*x)*f(2*y)*f(z + y)*f(b + 2*x)*f(b + 2*z) +
f(2*x)*f(2*y)
> *f(z + y)*f(a + 2*y)*f(c + z + x) - 1/2*f(2*x)*f(2*y)*f
(z + y)*f(a +
> 2*y)*f(a + 2*z) + f(2*x)*f(2*y)*f(z + x)*f(c + 2*y)*f(c
+ y + x) + f(
> 2*x)*f(2*y)*f(z + x)*f(c + 2*y)*f(b + z + x) + 2*f(2*x)*
f(2*y)*f(z +
> x)*f(b + z + y)*f(c + y + x) - 2*f(2*x)*f(2*y)*f(z + x)*
f(b + y + x)*
> f(c + z + y) + 1/2*f(2*x)*f(2*y)*f(z + x)*f(a + 2*z)*f(b
+ 2*y) - f(2

```

```

>      *x)*f(2*y)*f(z + x)*f(a + 2*y)*f(c + z + y) + 1/2*f(2*x)
>      *f(2*y)*f(z
>      + x)*f(a + 2*y)*f(b + 2*z) - f(2*x)*f(2*y)*f(2*z)*f(c +
>      2*y)*f(a + y
>      + x) + 1/2*f(2*x)*f(2*y)*f(2*z)*f(b + 2*y)*f(c + 2*x) +
>      1/2*f(2*x)*
>      f(2*y)*f(2*z)*f(b + 2*x)*f(c + 2*y) + 2*f(2*x)*f(2*y)*f
>      (2*z)*f(a + z
>      + y)*f(b + y + x) - 2*f(2*x)*f(2*y)*f(2*z)*f(a + y + x)
>      *f(b + z + y)
>      - f(2*x)*f(2*y)*f(2*z)*f(a + 2*y)*f(b + z + x) + f(2*x)
>      *f(2*y)*f(2*z
>      )*f(a + 2*y)*f(a + z + y) - f(2*x)*f(2*y)*f(y + x)*f(c +
>      2*z)*f(b + y
>      + x) + f(2*x)*f(2*y)*f(y + x)*f(b + 2*z)*f(c + y + x) +
>      1/2*f(2*x)*
>      f(2*y)*f(y + x)*f(a + 2*z)*f(c + 2*y) - 1/2*f(2*x)*f(2*
>      y)*f(y + x)*f(
>      a + 2*y)*f(c + 2*z) + f(2*x)*f(2*y)^2*f(c + 2*z)*f(a + y
>      + x) + 1/2*
>      f(2*x)*f(2*y)^2*f(b + 2*z)*f(c + 2*x) + 1/2*f(2*x)*f(2*
>      y)^2*f(b + 2*x
>      )*f(c + 2*z) - f(2*x)*f(2*y)^2*f(a + 2*z)*f(c + y + x) +
>      1/2*f(2*x)^2
>      *f(z + y)*f(c + 2*y)^2 + f(2*x)^2*f(z + y)*f(c + 2*y)*f
>      (b + z + y) +
>      1/2*f(2*x)^2*f(z + y)*f(b + 2*y)*f(b + 2*z) - f(2*x)^2*f
>      (2*z)*f(b + 2
>      *y)*f(c + 2*y) - 1/2*f(2*x)^2*f(2*y)*f(b + 2*z)*f(c + 2*
>      y) - 1/2*f(2*
>      x)^2*f(2*y)*f(b + 2*y)*f(c + 2*z) )
>
>      - f(2*y)*f(c + b + 2*x) + f(2*x)*f(c + b + 2*y):
>
> eq[12] :=
> (1/HessUniv) * ( - f(2*y)*f(z + y)^2*f(a + 2*x)*f(c + 2*x) + 2*f
> (2*y
> )*f(z + x)*f(z + y)*f(a + 2*x)*f(c + y + x) - f(2*y)*f(z
> + x)^2*f(a
> + 2*x)*f(c + 2*y) + 1/2*f(2*y)*f(2*z)*f(z + x)*f(b + 2*
> x)^2 + f(2*y)
> *f(2*z)*f(z + x)*f(b + 2*x)*f(a + y + x) - 2*f(2*y)*f(2*
> z)*f(z + x)*
> f(a + 2*x)*f(b + y + x) + 1/2*f(2*y)*f(2*z)*f(z + x)*f(a
> + 2*x)*f(a
> + 2*y) - f(2*y)*f(2*z)*f(y + x)*f(c + 2*x)*f(a + y + x)
> - f(2*y)*f(2
> *z)*f(y + x)*f(b + 2*x)*f(c + 2*x) - f(2*y)*f(2*z)*f(y +
> x)*f(b + 2*x
> )*f(a + z + x) + 2*f(2*y)*f(2*z)*f(y + x)*f(a + 2*x)*f(b
> + z + x) -
> f(2*y)*f(2*z)*f(y + x)*f(a + 2*x)*f(a + z + y) + f(2*y)*
> f(y + x)*f(z
> + y)*f(c + 2*x)^2 + 2*f(2*y)*f(y + x)*f(z + y)*f(c + 2*
> x)*f(a + z +
> x) - 2*f(2*y)*f(y + x)*f(z + y)*f(a + 2*x)*f(c + z + x)
> + f(2*y)*f(y

```

```

> + x)*f(z + y)*f(a + 2*x)*f(a + 2*z) + 2*f(2*y)*f(y + x)
> *f(z + x)*f(a
> + 2*x)*f(c + z + y) - f(2*y)*f(y + x)^2*f(a + 2*x)*f(c
> + 2*z) - 1/2*
> f(2*y)^2*f(z + x)*f(c + 2*x)^2 - f(2*y)^2*f(z + x)*f(c +
> 2*x)*f(a + z
> + x) - 1/2*f(2*y)^2*f(z + x)*f(a + 2*x)*f(a + 2*z) + f
> (2*y)^2*f(2*z)
> *f(a + 2*x)*f(c + 2*x) + f(2*x)*f(z + y)^2*f(a + 2*y)*f
> (c + 2*x) - 2*
> f(2*x)*f(z + x)*f(z + y)*f(a + 2*y)*f(c + y + x) + f(2*
> x)*f(z + x)^2*
> f(a + 2*y)*f(c + 2*y) - 1/2*f(2*x)*f(2*z)*f(z + y)*f(a +
> 2*y)*f(b + 2
> *x) + 1/2*f(2*x)*f(2*z)*f(z + y)*f(a + 2*x)*f(b + 2*y) +
> f(2*x)*f(2*z
> )*f(z + x)*f(b + 2*y)*f(a + y + x) - 1/2*f(2*x)*f(2*z)*f
> (z + x)*f(b
> + 2*x)*f(b + 2*y) - 1/2*f(2*x)*f(2*z)*f(z + x)*f(a + 2*
> y)^2 + 1/2*f(
> 2*x)*f(2*z)*f(y + x)*f(b + 2*y)*f(c + 2*x) - f(2*x)*f(2*
> z)*f(y + x)*
> f(b + 2*y)*f(a + z + x) + 1/2*f(2*x)*f(2*z)*f(y + x)*f(b
> + 2*x)*f(c
> + 2*y) + f(2*x)*f(2*z)*f(y + x)*f(a + 2*y)*f(c + y + x)
> + f(2*x)*f(2
> *z)*f(y + x)*f(a + 2*y)*f(a + z + y) - f(2*x)*f(y + x)*f
> (z + y)*f(c
> + 2*x)*f(c + 2*y) - f(2*x)*f(y + x)*f(z + y)*f(a + 2*y)
> *f(a + 2*z)
> - 2*f(2*x)*f(y + x)*f(z + x)*f(c + 2*y)*f(a + z + y) +
> f(2*x)*f(y +
> x)^2*f(a + 2*z)*f(c + 2*y) - f(2*x)*f(2*y)*f(z + y)*f(c
> + 2*x)*f(c +
> y + x) - f(2*x)*f(2*y)*f(z + y)*f(c + 2*x)*f(a + z + y)
> + f(2*x)*f(2*
> y)*f(z + y)*f(b + 2*x)*f(c + z + x) - 2*f(2*x)*f(2*y)*f
> (z + y)*f(a +
> z + x)*f(c + y + x) - 1/2*f(2*x)*f(2*y)*f(z + y)*f(a +
> 2*z)*f(b + 2*x
> ) + 2*f(2*x)*f(2*y)*f(z + y)*f(a + y + x)*f(c + z + x) -
> 1/2*f(2*x)*
> f(2*y)*f(z + y)*f(a + 2*x)*f(b + 2*z) + f(2*x)*f(2*y)*f
> (z + x)*f(c +
> 2*y)*f(a + z + x) + f(2*x)*f(2*y)*f(z + x)*f(c + 2*x)*f
> (c + 2*y) - f(
> 2*x)*f(2*y)*f(z + x)*f(b + 2*x)*f(c + z + y) + 1/2*f(2*
> x)*f(2*y)*f(z
> + x)*f(b + 2*x)*f(b + 2*z) + 2*f(2*x)*f(2*y)*f(z + x)*f
> (a + z + y)*
> f(c + y + x) - 2*f(2*x)*f(2*y)*f(z + x)*f(a + y + x)*f(c
> + z + y) + 1/
> 2*f(2*x)*f(2*y)*f(z + x)*f(a + 2*y)*f(a + 2*z) + f(2*x)*
> f(2*y)*f(2*z)
> *f(c + 2*x)*f(b + y + x) - f(2*x)*f(2*y)*f(2*z)*f(b + 2*
> x)*f(b + z +
> x) + f(2*x)*f(2*y)*f(2*z)*f(b + 2*x)*f(a + z + y) + 2*f

```

```

(2*x)*f(2*y)*
> f(2*z)*f(a + z + x)*f(b + y + x) - 2*f(2*x)*f(2*y)*f(2*
z)*f(a + y + x
> )*f(b + z + x) - 1/2*f(2*x)*f(2*y)*f(2*z)*f(a + 2*y)*f(c
+ 2*x) - 1/2
> *f(2*x)*f(2*y)*f(2*z)*f(a + 2*x)*f(c + 2*y) + f(2*x)*f
(2*y)*f(y + x)*
> f(c + 2*z)*f(a + y + x) - 1/2*f(2*x)*f(2*y)*f(y + x)*f(b
+ 2*z)*f(c
> + 2*x) + 1/2*f(2*x)*f(2*y)*f(y + x)*f(b + 2*x)*f(c + 2*
z) - f(2*x)*
> f(2*y)*f(y + x)*f(a + 2*z)*f(c + y + x) + 1/2*f(2*x)*f
(2*y)^2*f(a + 2
> *z)*f(c + 2*x) + 1/2*f(2*x)*f(2*y)^2*f(a + 2*x)*f(c + 2*
z) + f(2*x)^2
> *f(z + y)*f(c + 2*y)*f(c + y + x) + f(2*x)^2*f(z + y)*f
(c + 2*y)*f(a
> + z + y) - f(2*x)^2*f(z + y)*f(b + 2*y)*f(c + z + x) +
1/2*f(2*x)^2*
> f(z + y)*f(a + 2*z)*f(b + 2*y) + 1/2*f(2*x)^2*f(z + y)*f
(a + 2*y)*f(b
> + 2*z) - 1/2*f(2*x)^2*f(z + x)*f(c + 2*y)^2 + f(2*x)^2*
f(z + x)*f(b
> + 2*y)*f(c + z + y) - 1/2*f(2*x)^2*f(z + x)*f(b + 2*y)*
f(b + 2*z) -
> f(2*x)^2*f(2*z)*f(b + 2*y)*f(c + y + x) + f(2*x)^2*f(2*
z)*f(b + 2*y)*
> f(b + z + x) - f(2*x)^2*f(2*z)*f(b + 2*y)*f(a + z + y) -
1/2*f(2*x)^2
> *f(y + x)*f(b + 2*z)*f(c + 2*y) + 1/2*f(2*x)^2*f(y + x)*
f(b + 2*y)*f(
> c + 2*z) - f(2*x)^2*f(2*y)*f(c + 2*z)*f(b + y + x) + f
(2*x)^2*f(2*y)*
> f(b + 2*z)*f(c + y + x) - 1/2*f(2*x)^2*f(2*y)*f(a + 2*z)
*f(c + 2*y)
> - 1/2*f(2*x)^2*f(2*y)*f(a + 2*y)*f(c + 2*z) )
>
> - f(2*y)*f(c + a + 2*x) + f(2*x)*f(c + a + 2*y):
>
> eq[13] :=
> (1/HessUniv) * ( 2*f(2*z)^2*f(y + x)*f(b + 2*y)*f(a + y + x) - f
(2*z)
> ^2*f(y + x)*f(b + 2*x)*f(b + 2*y) - f(2*z)^2*f(y + x)*f
(a + 2*y)^2 +
> 2*f(2*z)*f(y + x)*f(z + y)*f(b + 2*y)*f(c + 2*x) - 2*f
(2*z)*f(y + x)*
> f(z + y)*f(a + 2*y)*f(c + y + x) - 2*f(2*z)*f(y + x)*f(z
+ y)*f(a + 2
> *y)*f(b + z + x) + 2*f(2*z)*f(y + x)*f(z + y)*f(a + 2*y)
*f(a + z + y)
> - 2*f(2*z)*f(y + x)*f(z + x)*f(b + 2*y)*f(c + y + x) +
2*f(2*z)*f(y
> + x)*f(z + x)*f(b + 2*y)*f(b + z + x) - 2*f(2*z)*f(y +
x)*f(z + x)*
> f(b + 2*y)*f(a + z + y) + 2*f(2*z)*f(y + x)*f(z + x)*f(a
+ 2*y)*f(c
> + 2*y) + 4*f(y + x)*f(z + y)^2*f(a + 2*y)*f(c + z + x)

```

```

- 2*f(y + x)*
> f(z + y)^2*f(a + 2*y)*f(a + 2*z) + 4*f(y + x)*f(z + x)*f
(z + y)*f(c
> + 2*y)*f(c + y + x) + 4*f(y + x)*f(z + x)*f(z + y)*f(c
+ 2*y)*f(b +
> z + x) - 4*f(y + x)*f(z + x)*f(z + y)*f(c + 2*y)*f(a + z
+ y) - 4*f(y
> + x)*f(z + x)*f(z + y)*f(b + 2*y)*f(c + z + x) - 2*f(y
+ x)*f(z + x)
> *f(z + y)*f(a + 2*z)*f(b + 2*y) + 4*f(y + x)*f(z + x)*f
(z + y)*f(a +
> 2*y)*f(c + z + y) + 2*f(y + x)*f(z + x)*f(z + y)*f(a +
2*y)*f(b + 2*z
> ) + 4*f(y + x)*f(z + x)^2*f(b + 2*y)*f(c + z + y) - 2*f
(y + x)*f(z +
> x)^2*f(b + 2*y)*f(b + 2*z) - 4*f(y + x)^2*f(z + y)*f(c +
2*y)*f(c + z
> + x) + 2*f(y + x)^2*f(z + y)*f(a + 2*z)*f(c + 2*y) - 2*
f(y + x)^2*f(
> z + y)*f(a + 2*y)*f(c + 2*z) - 4*f(y + x)^2*f(z + x)*f(c
+ 2*y)*f(c
> + z + y) - 2*f(y + x)^2*f(z + x)*f(b + 2*z)*f(c + 2*y)
+ 2*f(y + x)^
> 2*f(z + x)*f(b + 2*y)*f(c + 2*z) + 2*f(y + x)^3*f(c + 2*
y)*f(c + 2*z)
> + 2*f(2*y)*f(z + y)^2*f(a + 2*z)*f(a + y + x) - 4*f(2*
y)*f(z + y)^2*
> f(a + y + x)*f(c + z + x) - 2*f(2*y)*f(z + x)*f(z + y)*f
(b + 2*z)*f(a
> + y + x) + 4*f(2*y)*f(z + x)*f(z + y)*f(b + y + x)*f(c
+ z + x) - 2*
> f(2*y)*f(z + x)*f(z + y)*f(a + 2*z)*f(b + y + x) + 4*f
(2*y)*f(z + x)*
> f(z + y)*f(a + y + x)*f(c + z + y) - 2*f(2*y)*f(z + x)
^2*f(c + 2*y)*
> f(c + y + x) - 2*f(2*y)*f(z + x)^2*f(c + 2*y)*f(b + z +
x) + 2*f(2*y)
> *f(z + x)^2*f(c + 2*y)*f(a + z + y) + 2*f(2*y)*f(z + x)
^2*f(b + 2*z)*
> f(b + y + x) - 4*f(2*y)*f(z + x)^2*f(b + y + x)*f(c + z
+ y) + 2*f(2*
> y)*f(z + x)^2*f(a + 2*z)*f(b + 2*y) - 4*f(2*y)*f(z + x)
^2*f(a + 2*y)*
> f(c + z + y) - 2*f(2*y)*f(2*z)*f(z + y)*f(c + 2*x)*f(b +
y + x) + 2*
> f(2*y)*f(2*z)*f(z + y)*f(a + y + x)*f(c + y + x) + 2*f
(2*y)*f(2*z)*f(
> z + y)*f(a + y + x)*f(b + z + x) - 2*f(2*y)*f(2*z)*f(z +
y)*f(a + y
> + x)*f(a + z + y) - 2*f(2*y)*f(2*z)*f(z + x)*f(c + 2*y)
*f(a + y + x)
> + 2*f(2*y)*f(2*z)*f(z + x)*f(b + y + x)*f(c + y + x) -
2*f(2*y)*f(2*
> z)*f(z + x)*f(b + y + x)*f(b + z + x) + 2*f(2*y)*f(2*z)*
f(z + x)*f(a
> + z + y)*f(b + y + x) + f(2*y)*f(2*z)^2*f(b + 2*x)*f(b
+ y + x) - 2*

```



```

>      f(2*y)*f(2*z)^2*f(a + y + x)*f(b + y + x) + 1/2*f(2*y)*f
(2*z)^2*f(a
>      + 2*y)*f(b + 2*x) + f(2*y)*f(2*z)^2*f(a + 2*y)*f(a + y
+ x) - 1/2*f(
>      2*y)*f(2*z)^2*f(a + 2*x)*f(b + 2*y) - 2*f(2*y)*f(2*z)*f
(y + x)*f(c +
>      y + x)^2 - f(2*y)*f(2*z)*f(y + x)*f(c + 2*x)*f(c + 2*y)
- 2*f(2*y)*f(
>      2*z)*f(y + x)*f(b + z + x)*f(c + y + x) + 2*f(2*y)*f(2*
z)*f(y + x)*f(
>      a + z + y)*f(c + y + x) + 2*f(2*y)*f(2*z)*f(y + x)*f(a +
2*z)*f(b + y
>      + x) - 4*f(2*y)*f(2*z)*f(y + x)*f(a + y + x)*f(c + z +
y) - 2*f(2*y)
>      *f(2*z)*f(y + x)*f(a + 2*y)*f(c + z + x) + f(2*y)*f(2*z)
*f(y + x)*f(a
>      + 2*y)*f(a + 2*z) + 2*f(2*y)*f(y + x)*f(z + y)*f(c + 2*
z)*f(a + y +
>      x) + 4*f(2*y)*f(y + x)*f(z + y)*f(c + y + x)*f(c + z +
x) - 2*f(2*y)*
>      f(y + x)*f(z + y)*f(a + 2*z)*f(c + y + x) - 2*f(2*y)*f(y
+ x)*f(z + x
>      )*f(c + 2*z)*f(b + y + x) + 4*f(2*y)*f(y + x)*f(z + x)*f
(c + y + x)*
>      f(c + z + y) + 4*f(2*y)*f(y + x)*f(z + x)*f(c + 2*y)*f(c
+ z + x) + 2
>      *f(2*y)*f(y + x)*f(z + x)*f(b + 2*z)*f(c + y + x) - 2*f
(2*y)*f(y + x)
>      ^2*f(c + 2*z)*f(c + y + x) + f(2*y)^2*f(z + y)*f(a + 2*
z)*f(c + 2*x)
>      - f(2*y)^2*f(z + y)*f(a + 2*x)*f(c + 2*z) - 4*f(2*y)^2*
f(z + x)*f(c
>      + y + x)*f(c + z + x) - f(2*y)^2*f(z + x)*f(b + 2*z)*f
(c + 2*x) + f(
>      2*y)^2*f(z + x)*f(b + 2*x)*f(c + 2*z) + f(2*y)^2*f(2*z)*
f(c + 2*x)*f(
>      c + y + x) + f(2*y)^2*f(2*z)*f(c + 2*x)*f(b + z + x) - f
(2*y)^2*f(2*z
>      )*f(c + 2*x)*f(a + z + y) - f(2*y)^2*f(2*z)*f(b + 2*x)*f
(c + z + x)
>      - 1/2*f(2*y)^2*f(2*z)*f(a + 2*z)*f(b + 2*x) - f(2*y)^2*
f(2*z)*f(a +
>      2*z)*f(a + y + x) + 2*f(2*y)^2*f(2*z)*f(a + y + x)*f(c +
z + x) + f(2
>      *y)^2*f(2*z)*f(a + 2*x)*f(c + z + y) + 1/2*f(2*y)^2*f(2*
z)*f(a + 2*x)
>      *f(b + 2*z) - 2*f(2*x)*f(z + y)^2*f(c + 2*y)*f(c + y +
x) - 2*f(2*x)*
>      f(z + y)^2*f(c + 2*y)*f(b + z + x) + 2*f(2*x)*f(z + y)
^2*f(c + 2*y)*
>      f(a + z + y) + 2*f(2*x)*f(z + y)^2*f(a + 2*z)*f(b + 2*y)
- 4*f(2*x)*
>      f(z + y)^2*f(a + 2*y)*f(c + z + y) - f(2*x)*f(2*z)*f(y +
x)*f(c + 2*y
>      )^2 - 2*f(2*x)*f(2*z)*f(y + x)*f(b + 2*y)*f(c + z + y) +
f(2*x)*f(2*z
>      )*f(y + x)*f(b + 2*y)*f(b + 2*z) + 4*f(2*x)*f(y + x)*f(z

```

```

+ y)*f(c + 2
>      *y)*f(c + z + y) - 4*f(2*x)*f(2*y)*f(z + y)*f(c + y + x)
>      *f(c + z + y)
>      - f(2*x)*f(2*y)*f(z + y)*f(a + 2*z)*f(c + 2*y) + f(2*x)
>      *f(2*y)*f(z
>      + y)*f(a + 2*y)*f(c + 2*z) + f(2*x)*f(2*y)*f(z + x)*f(b
>      + 2*z)*f(c
>      + 2*y) - f(2*x)*f(2*y)*f(z + x)*f(b + 2*y)*f(c + 2*z) +
>      3*f(2*x)*f(2
>      *y)*f(2*z)*f(c + 2*y)*f(c + y + x) + f(2*x)*f(2*y)*f(2*
>      z)*f(c + 2*y)*
>      f(b + z + x) - f(2*x)*f(2*y)*f(2*z)*f(c + 2*y)*f(a + z +
>      y) - f(2*x)*
>      f(2*y)*f(2*z)*f(b + 2*z)*f(b + y + x) + 2*f(2*x)*f(2*y)*
>      f(2*z)*f(b +
>      y + x)*f(c + z + y) + f(2*x)*f(2*y)*f(2*z)*f(b + 2*y)*f
>      (c + z + x) -
>      3/2*f(2*x)*f(2*y)*f(2*z)*f(a + 2*z)*f(b + 2*y) + 3*f(2*
>      x)*f(2*y)*f(2*
>      z)*f(a + 2*y)*f(c + z + y) - 1/2*f(2*x)*f(2*y)*f(2*z)*f
>      (a + 2*y)*f(b
>      + 2*z) - 2*f(2*x)*f(2*y)*f(y + x)*f(c + 2*y)*f(c + 2*z)
>      + 2*f(2*x)*
>      f(2*y)^2*f(c + 2*z)*f(c + y + x) )
>
>      - 2*f(c + 2*y)*f(c + y + x) - 2*f(c + 2*y)*f(b + z + x) +
>      2*f(c + 2*y)*
>      f(a + z + y) + 2*f(a + 2*z)*f(b + 2*y) - 4*f(a + 2*y)*f
>      (c + z + y) +
>      2*f(y + x)*f(2*c + 2*y) - 2*f(2*y)*f(2*c + y + x):
>
> eq[14] :=
> (1/HessUniv) * ( 4*f(2*z)*f(z + y)^2*f(b + 2*y)*f(a + y + x) - 2*
> f(2*
>      z)*f(z + y)^2*f(a + 2*y)*f(b + y + x) - f(2*z)*f(z + y)
>      ^2*f(a + 2*y)^
>      2 - 2*f(2*z)*f(z + x)*f(z + y)*f(b + 2*y)*f(b + y + x) +
>      f(2*z)*f(z
>      + x)^2*f(b + 2*y)^2 + 2*f(2*z)^2*f(y + x)*f(b + 2*y)*f
>      (b + y + x) +
>      2*f(2*z)*f(y + x)*f(z + y)*f(c + 2*y)*f(b + y + x) - 4*f
>      (2*z)*f(y + x
>      )*f(z + y)*f(b + 2*y)*f(c + y + x) - 4*f(2*z)*f(y + x)*f
>      (z + y)*f(b
>      + 2*y)*f(a + z + y) + 2*f(2*z)*f(y + x)*f(z + y)*f(a +
>      2*y)*f(c + 2*
>      y) + 2*f(2*z)*f(y + x)*f(z + y)*f(a + 2*y)*f(b + z + y)
>      - 2*f(2*z)*f(
>      y + x)*f(z + x)*f(b + 2*y)*f(b + z + y) - 2*f(y + x)*f(z
>      + x)*f(z + y
>      )*f(c + 2*y)^2 - 4*f(y + x)*f(z + x)*f(z + y)*f(c + 2*y)
>      *f(b + z + y)
>      + 8*f(y + x)*f(z + x)*f(z + y)*f(b + 2*y)*f(c + z + y)
>      - 2*f(2*y)*f(
>      z + y)^2*f(a + 2*z)*f(b + y + x) + f(2*y)*f(z + y)^2*f(a
>      + 2*y)*f(a
>      + 2*z) + 2*f(2*y)*f(z + x)*f(z + y)*f(b + 2*z)*f(b + y

```

```

+ x) + f(2*y)
>      *f(z + x)*f(z + y)*f(a + 2*z)*f(b + 2*y) - f(2*y)*f(z +
x)*f(z + y)*
>      f(a + 2*y)*f(b + 2*z) + f(2*y)*f(z + x)^2*f(c + 2*y)^2 +
2*f(2*y)*f(z
>      + x)^2*f(c + 2*y)*f(b + z + y) - 4*f(2*y)*f(z + x)^2*f
(b + 2*y)*f(c
>      + z + y) - f(2*y)*f(z + x)^2*f(b + 2*y)*f(b + 2*z) - 2*
f(2*y)*f(2*z)
>      *f(z + y)*f(c + 2*y)*f(a + y + x) + f(2*y)*f(2*z)*f(z +
y)*f(b + 2*y)
>      *f(c + 2*x) - 2*f(2*y)*f(2*z)*f(z + y)*f(b + 2*y)*f(a +
z + x) + 4*f(
>      2*y)*f(2*z)*f(z + y)*f(a + z + y)*f(b + y + x) - 4*f(2*
y)*f(2*z)*f(z
>      + y)*f(a + y + x)*f(b + z + y) + f(2*y)*f(2*z)*f(z + y)
*f(a + 2*y)*
>      f(c + y + x) + f(2*y)*f(2*z)*f(z + y)*f(a + 2*y)*f(b + z
+ x) + f(2*y
>      )*f(2*z)*f(z + y)*f(a + 2*y)*f(a + z + y) + f(2*y)*f(2*
z)*f(z + x)*f(
>      b + 2*y)*f(c + y + x) + f(2*y)*f(2*z)*f(z + x)*f(b + 2*
y)*f(b + z + x
>      ) + f(2*y)*f(2*z)*f(z + x)*f(b + 2*y)*f(a + z + y) - f
(2*y)*f(2*z)*f(
>      z + x)*f(a + 2*y)*f(c + 2*y) - f(2*y)*f(2*z)^2*f(b + 2*
y)*f(a + y + x
>      ) - 1/2*f(2*y)*f(2*z)^2*f(b + 2*x)*f(b + 2*y) + 1/2*f(2*
y)*f(2*z)^2*
>      f(a + 2*y)^2 + f(2*y)*f(2*z)*f(y + x)*f(c + 2*y)*f(c + y
+ x) - f(2*y
>      )*f(2*z)*f(y + x)*f(c + 2*y)*f(b + z + x) + f(2*y)*f(2*
z)*f(y + x)*f(
>      c + 2*y)*f(a + z + y) + 4*f(2*y)*f(2*z)*f(y + x)*f(b + z
+ y)*f(c + y
>      + x) - 2*f(2*y)*f(2*z)*f(y + x)*f(b + 2*z)*f(b + y + x)
- 4*f(2*y)*
>      f(2*z)*f(y + x)*f(b + y + x)*f(c + z + y) + f(2*y)*f(2*
z)*f(y + x)*f(
>      a + 2*z)*f(b + 2*y) - 2*f(2*y)*f(2*z)*f(y + x)*f(a + 2*
y)*f(c + z + y
>      ) + 2*f(2*y)*f(y + x)*f(z + y)*f(c + 2*z)*f(b + y + x) -
f(2*y)*f(y
>      + x)*f(z + y)*f(a + 2*z)*f(c + 2*y) + 2*f(2*y)*f(y + x)
*f(z + y)*f(a
>      + 2*z)*f(b + z + y) - f(2*y)*f(y + x)*f(z + y)*f(a + 2*
y)*f(c + 2*z)
>      + f(2*y)*f(y + x)*f(z + x)*f(b + 2*z)*f(c + 2*y) + 2*f
(2*y)*f(y + x)
>      *f(z + x)*f(b + 2*z)*f(b + z + y) - f(2*y)*f(y + x)*f(z
+ x)*f(b + 2*
>      y)*f(c + 2*z) - 2*f(2*y)*f(y + x)^2*f(c + 2*z)*f(b + z +
y) + f(2*y)*
>      f(y + x)^2*f(c + 2*y)*f(c + 2*z) - f(2*y)^2*f(z + y)*f(b
+ 2*x)*f(c
>      + 2*z) + f(2*y)^2*f(z + y)*f(a + 2*z)*f(c + y + x) + f
(2*y)^2*f(z +

```

```

> y)*f(a + 2*z)*f(b + z + x) - f(2*y)^2*f(z + y)*f(a + 2*
z)*f(a + z + y
> ) - f(2*y)^2*f(z + x)*f(b + 2*z)*f(c + y + x) - f(2*y)
^2*f(z + x)*f(b
> + 2*z)*f(b + z + x) + f(2*y)^2*f(z + x)*f(b + 2*z)*f(a
+ z + y) - 2*
> f(2*y)^2*f(z + x)*f(a + 2*z)*f(b + z + y) + f(2*y)^2*f(z
+ x)*f(a + 2
> *y)*f(c + 2*z) + f(2*y)^2*f(2*z)*f(c + 2*y)*f(a + z + x)
- 1/2*f(2*y)
> ^2*f(2*z)*f(c + 2*x)*f(c + 2*y) - f(2*y)^2*f(2*z)*f(c +
2*x)*f(b + z
> + y) + f(2*y)^2*f(2*z)*f(b + 2*z)*f(a + y + x) + f(2*y)
^2*f(2*z)*f(b
> + 2*x)*f(c + z + y) + 1/2*f(2*y)^2*f(2*z)*f(b + 2*x)*f
(b + 2*z) - 2*
> f(2*y)^2*f(2*z)*f(a + z + y)*f(c + y + x) - 2*f(2*y)^2*f
(2*z)*f(a + z
> + y)*f(b + z + x) + 2*f(2*y)^2*f(2*z)*f(a + z + x)*f(b
+ z + y) + 2*
> f(2*y)^2*f(2*z)*f(a + y + x)*f(c + z + y) - f(2*y)^2*f
(2*z)*f(a + 2*y
> )*f(a + 2*z) - f(2*y)^2*f(y + x)*f(c + 2*z)*f(c + y + x)
+ f(2*y)^2*
> f(y + x)*f(c + 2*z)*f(b + z + x) + f(2*y)^2*f(y + x)*f(c
+ 2*z)*f(a
> + z + y) - f(2*y)^2*f(y + x)*f(a + 2*z)*f(b + 2*z) - f
(2*y)^3*f(c +
> 2*z)*f(a + z + x) + 1/2*f(2*y)^3*f(c + 2*x)*f(c + 2*z) +
1/2*f(2*y)^3
> *f(a + 2*z)^2 + f(2*x)*f(z + y)^2*f(c + 2*y)^2 + 2*f(2*
x)*f(z + y)^2*
> f(c + 2*y)*f(b + z + y) - 4*f(2*x)*f(z + y)^2*f(b + 2*y)
*f(c + z + y)
> + 2*f(2*x)*f(2*z)*f(z + y)*f(b + 2*y)*f(b + z + y) - f
(2*x)*f(2*z)^2
> *f(b + 2*y)^2 - 2*f(2*x)*f(2*y)*f(z + y)*f(b + 2*z)*f(b
+ z + y) - 1/
> 2*f(2*x)*f(2*y)*f(2*z)*f(c + 2*y)^2 - 2*f(2*x)*f(2*y)*f
(2*z)*f(c + 2*
> y)*f(b + z + y) + 3*f(2*x)*f(2*y)*f(2*z)*f(b + 2*y)*f(c
+ z + y) + 1/
> 2*f(2*x)*f(2*y)*f(2*z)*f(b + 2*y)*f(b + 2*z) + f(2*x)*f
(2*y)^2*f(c +
> 2*z)*f(b + z + y) - 1/2*f(2*x)*f(2*y)^2*f(c + 2*y)*f(c +
2*z) + 1/2*
> f(2*x)*f(2*y)^2*f(b + 2*z)^2 )

> + f(c + 2*y)^2 + 2*f(c + 2*y)*f(b + z + y) - 4*f(b + 2*y)*
f(c + z + y)
> + f(2*z)*f(2*b + 2*y) - f(2*y)*f(2*b + 2*z):

> eq[15] :=
> (1/HessUniv) * ( f(2*z)*f(z + y)^2*f(a + 2*x)*f(b + 2*y) + 2*f(2*
z)*
> f(z + x)*f(z + y)*f(b + 2*y)*f(a + y + x) - f(2*z)*f(z +

```

```

x)*f(z + y)*
> f(b + 2*x)*f(b + 2*y) - 2*f(2*z)*f(z + x)*f(z + y)*f(a +
2*y)*f(b + y
> + x) - f(2*z)*f(z + x)*f(z + y)*f(a + 2*y)^2 + f(2*z)*f
(z + x)^2*f(a
> + 2*y)*f(b + 2*y) + 1/2*f(2*z)^2*f(y + x)*f(b + 2*x)*f
(b + 2*y) + f(
> 2*z)^2*f(y + x)*f(a + 2*y)*f(b + y + x) + 1/2*f(2*z)^2*f
(y + x)*f(a
> + 2*y)^2 - 2*f(2*z)*f(y + x)*f(z + y)*f(b + 2*y)*f(a +
z + x) - 2*f(
> 2*z)*f(y + x)*f(z + x)*f(b + 2*y)*f(a + z + y) + 2*f(y +
x)*f(z + x)*
> f(z + y)*f(a + 2*z)*f(b + 2*y) - f(2*y)*f(z + y)^2*f(a +
2*z)*f(b + 2
> *x) + f(2*y)*f(z + x)*f(z + y)*f(b + 2*x)*f(b + 2*z) + f
(2*y)*f(z + x
> )*f(z + y)*f(a + 2*y)*f(a + 2*z) - f(2*y)*f(z + x)^2*f(a
+ 2*z)*f(b
> + 2*y) - f(2*y)*f(z + x)^2*f(a + 2*y)*f(b + 2*z) + f(2*
y)*f(2*z)*f(z
> + y)*f(b + 2*x)*f(a + z + y) + 1/2*f(2*y)*f(2*z)*f(z +
y)*f(a + 2*y)
> *f(c + 2*x) - 1/2*f(2*y)*f(2*z)*f(z + y)*f(a + 2*x)*f(c
+ 2*y) - f(2*
> y)*f(2*z)*f(z + y)*f(a + 2*x)*f(b + z + y) - f(2*y)*f(2*
z)*f(z + x)*
> f(c + 2*y)*f(a + y + x) + 1/2*f(2*y)*f(2*z)*f(z + x)*f(b
+ 2*y)*f(c
> + 2*x) + 1/2*f(2*y)*f(2*z)*f(z + x)*f(b + 2*x)*f(c + 2*
y) + 2*f(2*y)
> *f(2*z)*f(z + x)*f(a + z + y)*f(b + y + x) - 2*f(2*y)*f
(2*z)*f(z + x)
> *f(a + y + x)*f(b + z + y) + f(2*y)*f(2*z)*f(z + x)*f(a
+ 2*y)*f(b +
> z + x) + f(2*y)*f(2*z)*f(z + x)*f(a + 2*y)*f(a + z + y)
- 1/2*f(2*y)*
> f(2*z)^2*f(a + 2*y)*f(b + 2*x) - 1/2*f(2*y)*f(2*z)^2*f(a
+ 2*x)*f(b
> + 2*y) + f(2*y)*f(2*z)*f(y + x)*f(c + 2*y)*f(a + z + x)
- 1/2*f(2*y)
> *f(2*z)*f(y + x)*f(c + 2*x)*f(c + 2*y) - 1/2*f(2*y)*f(2*
z)*f(y + x)*
> f(b + 2*x)*f(b + 2*z) - 2*f(2*y)*f(2*z)*f(y + x)*f(a + z
+ y)*f(b + z
> + x) + 2*f(2*y)*f(2*z)*f(y + x)*f(a + z + x)*f(b + z +
y) - f(2*y)*
> f(2*z)*f(y + x)*f(a + 2*z)*f(b + y + x) - f(2*y)*f(2*z)*
f(y + x)*f(a
> + 2*y)*f(a + 2*z) + 2*f(2*y)*f(y + x)*f(z + y)*f(a + 2*
z)*f(b + z +
> x) + 2*f(2*y)*f(y + x)*f(z + x)*f(b + 2*z)*f(a + z + y)
- f(2*y)*f(y
> + x)^2*f(a + 2*z)*f(b + 2*z) + 1/2*f(2*y)^2*f(z + y)*f
(a + 2*z)*f(c
> + 2*x) - 1/2*f(2*y)^2*f(z + y)*f(a + 2*x)*f(c + 2*z) +
f(2*y)^2*f(z

```

```

> + x)*f(c + 2*z)*f(a + y + x) - 1/2*f(2*y)^2*f(z + x)*f
(b + 2*z)*f(c
> + 2*x) - 1/2*f(2*y)^2*f(z + x)*f(b + 2*x)*f(c + 2*z) -
f(2*y)^2*f(z
> + x)*f(a + 2*z)*f(b + z + x) - f(2*y)^2*f(z + x)*f(a +
2*z)*f(a + z
> + y) - f(2*y)^2*f(2*z)*f(c + 2*x)*f(a + z + y) + 1/2*f
(2*y)^2*f(2*z)
> *f(a + 2*z)*f(b + 2*x) + f(2*y)^2*f(2*z)*f(a + 2*x)*f(c
+ z + y) + 1/
> 2*f(2*y)^2*f(2*z)*f(a + 2*x)*f(b + 2*z) - f(2*y)^2*f(y +
x)*f(c + 2*z
> )*f(a + z + x) + 1/2*f(2*y)^2*f(y + x)*f(c + 2*x)*f(c +
2*z) + 1/2*f(
> 2*y)^2*f(y + x)*f(a + 2*z)^2 - f(2*x)*f(z + y)^2*f(a +
2*z)*f(b + 2*y
> ) + f(2*x)*f(2*z)*f(z + y)*f(c + 2*y)*f(b + y + x) - 2*f
(2*x)*f(2*z)*
> f(z + y)*f(b + 2*y)*f(c + y + x) + f(2*x)*f(2*z)*f(z +
y)*f(b + 2*y)*
> f(b + z + x) + f(2*x)*f(2*z)*f(z + y)*f(a + 2*y)*f(c +
2*y) + f(2*x)*
> f(2*z)*f(z + y)*f(a + 2*y)*f(b + z + y) - f(2*x)*f(2*z)
^2*f(a + 2*y)*
> f(b + 2*y) - 1/2*f(2*x)*f(2*z)*f(y + x)*f(c + 2*y)^2 - f
(2*x)*f(2*z)*
> f(y + x)*f(c + 2*y)*f(b + z + y) + 2*f(2*x)*f(2*z)*f(y +
x)*f(b + 2*y
> )*f(c + z + y) - 1/2*f(2*x)*f(2*z)*f(y + x)*f(b + 2*y)*f
(b + 2*z) +
> f(2*x)*f(2*y)*f(z + y)*f(c + 2*z)*f(b + y + x) - f(2*x)*
f(2*y)*f(z +
> y)*f(b + 2*z)*f(b + z + x) - f(2*x)*f(2*y)*f(z + y)*f(b
+ 2*z)*f(a +
> z + y) - 1/2*f(2*x)*f(2*y)*f(z + y)*f(a + 2*z)*f(c + 2*
y) - 1/2*f(2*x
> )*f(2*y)*f(z + y)*f(a + 2*y)*f(c + 2*z) + 1/2*f(2*x)*f
(2*y)*f(z + x)*
> f(b + 2*z)*f(c + 2*y) - 1/2*f(2*x)*f(2*y)*f(z + x)*f(b +
2*y)*f(c + 2
> *z) + f(2*x)*f(2*y)*f(2*z)*f(c + 2*y)*f(c + y + x) - f
(2*x)*f(2*y)*f(
> 2*z)*f(c + 2*y)*f(b + z + x) + 2*f(2*x)*f(2*y)*f(2*z)*f
(b + z + y)*f(
> c + y + x) - 2*f(2*x)*f(2*y)*f(2*z)*f(b + y + x)*f(c + z
+ y) + 3/2*
> f(2*x)*f(2*y)*f(2*z)*f(a + 2*z)*f(b + 2*y) - f(2*x)*f(2*
y)*f(2*z)*f(a
> + 2*y)*f(c + z + y) + 1/2*f(2*x)*f(2*y)*f(2*z)*f(a + 2*
y)*f(b + 2*z)
> - f(2*x)*f(2*y)*f(y + x)*f(c + 2*z)*f(b + z + y) + 1/2*
f(2*x)*f(2*y)
> *f(y + x)*f(c + 2*y)*f(c + 2*z) + 1/2*f(2*x)*f(2*y)*f(y
+ x)*f(b + 2*
> z)^2 - f(2*x)*f(2*y)^2*f(c + 2*z)*f(c + y + x) + f(2*x)*
f(2*y)^2*f(c
> + 2*z)*f(b + z + x) + f(2*x)*f(2*y)^2*f(c + 2*z)*f(a +

```

```

z + y) )
>      - f(a + 2*z)*f(b + 2*y) + f(2*z)*f(b + a + 2*y) - f(2*y)*f
(b + a + 2*z)
>      :
> eq[16] :=
> (1/HessUniv) * ( f(2*z)*f(z + y)^2*f(a + 2*x)*f(a + 2*y) - f(2*z)
*f(z
>      + x)*f(z + y)*f(a + 2*y)*f(b + 2*x) - 2*f(2*z)*f(z + x)
*f(z + y)*f(a
>      + 2*y)*f(a + y + x) + f(2*z)*f(z + x)*f(z + y)*f(a + 2*
x)*f(b + 2*y)
>      + 2*f(2*z)*f(z + x)^2*f(b + 2*y)*f(a + y + x) - f(2*z)*
f(z + x)^2*f(
>      b + 2*x)*f(b + 2*y) + 2*f(2*z)^2*f(y + x)*f(a + 2*y)*f(a
+ y + x) +
>      f(2*z)*f(y + x)*f(z + y)*f(a + 2*y)*f(c + 2*x) - 2*f(2*
z)*f(y + x)*f(
>      z + y)*f(a + 2*y)*f(a + z + x) - f(2*z)*f(y + x)*f(z +
y)*f(a + 2*x)*
>      f(c + 2*y) - 2*f(2*z)*f(y + x)*f(z + x)*f(c + 2*y)*f(a +
y + x) + f(2
>      *z)*f(y + x)*f(z + x)*f(b + 2*y)*f(c + 2*x) - 2*f(2*z)*f
(y + x)*f(z
>      + x)*f(b + 2*y)*f(a + z + x) + f(2*z)*f(y + x)*f(z + x)
*f(b + 2*x)*
>      f(c + 2*y) + 4*f(y + x)*f(z + x)*f(z + y)*f(c + 2*y)*f(a
+ z + x) - 2
>      *f(y + x)*f(z + x)*f(z + y)*f(c + 2*x)*f(c + 2*y) - f(2*
y)*f(z + y)^2
>      *f(a + 2*x)*f(a + 2*z) - f(2*y)*f(z + x)*f(z + y)*f(a +
2*z)*f(b + 2*
>      x) + 2*f(2*y)*f(z + x)*f(z + y)*f(a + 2*z)*f(a + y + x)
+ f(2*y)*f(z
>      + x)*f(z + y)*f(a + 2*x)*f(b + 2*z) - 2*f(2*y)*f(z + x)
^2*f(c + 2*y)
>      *f(a + z + x) + f(2*y)*f(z + x)^2*f(c + 2*x)*f(c + 2*y)
- 2*f(2*y)*f(
>      z + x)^2*f(b + 2*z)*f(a + y + x) + f(2*y)*f(z + x)^2*f(b
+ 2*x)*f(b
>      + 2*z) + 2*f(2*y)*f(2*z)*f(z + x)*f(b + 2*x)*f(a + z +
y) + 2*f(2*y)
>      *f(2*z)*f(z + x)*f(a + 2*y)*f(a + z + x) - 2*f(2*y)*f(2*
z)*f(z + x)*
>      f(a + 2*x)*f(b + z + y) - f(2*y)*f(2*z)^2*f(a + 2*x)*f(a
+ 2*y) - 2*
>      f(2*y)*f(2*z)*f(y + x)*f(c + 2*x)*f(a + z + y) - 2*f(2*
y)*f(2*z)*f(y
>      + x)*f(a + 2*z)*f(a + y + x) + 2*f(2*y)*f(2*z)*f(y + x)
*f(a + 2*x)*
>      f(c + z + y) + f(2*y)*f(y + x)*f(z + y)*f(a + 2*z)*f(c +
2*x) + 2*f(2
>      *y)*f(y + x)*f(z + y)*f(a + 2*z)*f(a + z + x) - f(2*y)*f
(y + x)*f(z
>      + y)*f(a + 2*x)*f(c + 2*z) + 2*f(2*y)*f(y + x)*f(z + x)
*f(c + 2*z)*

```

```

>      f(a + y + x) - f(2*y)*f(y + x)*f(z + x)*f(b + 2*z)*f(c +
2*x) + 2*f(2
>      *y)*f(y + x)*f(z + x)*f(b + 2*z)*f(a + z + x) - f(2*y)*f
(y + x)*f(z
>      + x)*f(b + 2*x)*f(c + 2*z) - 2*f(2*y)*f(y + x)^2*f(c +
2*z)*f(a + z
>      + x) + f(2*y)*f(y + x)^2*f(c + 2*x)*f(c + 2*z) - 2*f(2*
y)^2*f(z + x)
>      *f(a + 2*z)*f(a + z + x) + f(2*y)^2*f(2*z)*f(a + 2*x)*f
(a + 2*z) - 2*
>      f(2*x)*f(z + y)^2*f(c + 2*y)*f(a + z + x) + f(2*x)*f(z +
y)^2*f(c + 2
>      *x)*f(c + 2*y) + 2*f(2*x)*f(2*z)*f(z + y)*f(c + 2*y)*f(a
+ y + x) -
>      f(2*x)*f(2*z)*f(z + y)*f(b + 2*y)*f(c + 2*x) - f(2*x)*f
(2*z)*f(z + y)
>      *f(a + 2*y)*f(c + y + x) + f(2*x)*f(2*z)*f(z + y)*f(a +
2*y)*f(b + z
>      + x) + f(2*x)*f(2*z)*f(z + y)*f(a + 2*y)*f(a + z + y) -
f(2*x)*f(2*z
>      )*f(z + x)*f(b + 2*y)*f(c + y + x) + f(2*x)*f(2*z)*f(z +
x)*f(b + 2*y
>      )*f(b + z + x) - f(2*x)*f(2*z)*f(z + x)*f(b + 2*y)*f(a +
z + y) + f(2
>      *x)*f(2*z)*f(z + x)*f(a + 2*y)*f(c + 2*y) - f(2*x)*f(2*
z)^2*f(b + 2*y
>      )*f(a + y + x) + 1/2*f(2*x)*f(2*z)^2*f(b + 2*x)*f(b + 2*
y) - 1/2*f(2*
>      x)*f(2*z)^2*f(a + 2*y)^2 + f(2*x)*f(2*z)*f(y + x)*f(c +
2*y)*f(c + y
>      + x) - f(2*x)*f(2*z)*f(y + x)*f(c + 2*y)*f(b + z + x) -
f(2*x)*f(2*z
>      )*f(y + x)*f(c + 2*y)*f(a + z + y) + f(2*x)*f(2*z)*f(y +
x)*f(a + 2*z
>      )*f(b + 2*y) - 2*f(2*x)*f(2*y)*f(z + y)*f(b + 2*z)*f(a +
z + x) + f(2
>      *x)*f(2*y)*f(z + y)*f(b + 2*x)*f(c + 2*z) - f(2*x)*f(2*
y)*f(z + y)*f(
>      a + 2*z)*f(c + y + x) + f(2*x)*f(2*y)*f(z + y)*f(a + 2*
z)*f(b + z + x
>      ) - f(2*x)*f(2*y)*f(z + y)*f(a + 2*z)*f(a + z + y) + f
(2*x)*f(2*y)*f(
>      z + x)*f(b + 2*z)*f(c + y + x) - f(2*x)*f(2*y)*f(z + x)*
f(b + 2*z)*f(
>      b + z + x) + f(2*x)*f(2*y)*f(z + x)*f(b + 2*z)*f(a + z +
y) - f(2*x)*
>      f(2*y)*f(z + x)*f(a + 2*y)*f(c + 2*z) + f(2*x)*f(2*y)*f
(2*z)*f(c + 2*
>      y)*f(a + z + x) - 1/2*f(2*x)*f(2*y)*f(2*z)*f(c + 2*x)*f
(c + 2*y) + f(
>      2*x)*f(2*y)*f(2*z)*f(c + 2*x)*f(b + z + y) + f(2*x)*f(2*
y)*f(2*z)*f(b
>      + 2*z)*f(a + y + x) - f(2*x)*f(2*y)*f(2*z)*f(b + 2*x)*f
(c + z + y)
>      - 1/2*f(2*x)*f(2*y)*f(2*z)*f(b + 2*x)*f(b + 2*z) + 2*f
(2*x)*f(2*y)*
>      f(2*z)*f(a + z + y)*f(c + y + x) - 2*f(2*x)*f(2*y)*f(2*

```



```

z)*f(a + z + y
> )*f(b + z + x) + 2*f(2*x)*f(2*y)*f(2*z)*f(a + z + x)*f(b
+ z + y) - 2
> *f(2*x)*f(2*y)*f(2*z)*f(a + y + x)*f(c + z + y) - f(2*x)
*f(2*y)*f(y
> + x)*f(c + 2*z)*f(c + y + x) + f(2*x)*f(2*y)*f(y + x)*f
(c + 2*z)*f(b
> + z + x) + f(2*x)*f(2*y)*f(y + x)*f(c + 2*z)*f(a + z +
y) - f(2*x)*
> f(2*y)*f(y + x)*f(a + 2*z)*f(b + 2*z) + f(2*x)*f(2*y)^2*
f(c + 2*z)*f(
> a + z + x) - 1/2*f(2*x)*f(2*y)^2*f(c + 2*x)*f(c + 2*z) +
1/2*f(2*x)*
> f(2*y)^2*f(a + 2*z)^2 - 1/2*f(2*x)^2*f(2*z)*f(c + 2*y)^2
+ f(2*x)^2*
> f(2*z)*f(b + 2*y)*f(c + z + y) - 1/2*f(2*x)^2*f(2*z)*f(b
+ 2*y)*f(b
> + 2*z) - f(2*x)^2*f(2*y)*f(c + 2*z)*f(b + z + y) + 1/2*
f(2*x)^2*f(2*
> y)*f(c + 2*y)*f(c + 2*z) + 1/2*f(2*x)^2*f(2*y)*f(b + 2*
z)^2 )
>
> - 2*f(c + 2*y)*f(a + z + x) + f(c + 2*x)*f(c + 2*y) + f(2*
z)*f(2*a + 2*
> y) - f(2*y)*f(2*a + 2*z):
>
> eq[17] :=
> (1/HessUniv) * ( 4*f(z + y)^3*f(a + 2*y)*f(c + z + x) - 2*f(z +
y)^3*
> f(a + 2*y)*f(a + 2*z) - 4*f(z + x)*f(z + y)^2*f(b + 2*y)
*f(c + z + x)
> + 2*f(z + x)*f(z + y)^2*f(a + 2*z)*f(b + 2*y) - 4*f(z +
x)*f(z + y)^
> 2*f(a + 2*y)*f(c + z + y) + 2*f(z + x)*f(z + y)^2*f(a +
2*y)*f(b + 2*
> z) + 4*f(z + x)^2*f(z + y)*f(b + 2*y)*f(c + z + y) - 2*f
(z + x)^2*f(z
> + y)*f(b + 2*y)*f(b + 2*z) + 2*f(2*z)*f(z + y)^2*f(b +
2*y)*f(c + 2*
> x) - 2*f(2*z)*f(z + y)^2*f(a + 2*y)*f(c + y + x) - 2*f
(2*z)*f(z + y)^
> 2*f(a + 2*y)*f(b + z + x) + 2*f(2*z)*f(z + y)^2*f(a + 2*
y)*f(a + z +
> y) - 2*f(2*z)*f(z + x)*f(z + y)*f(b + 2*y)*f(c + y + x)
+ 2*f(2*z)*f(
> z + x)*f(z + y)*f(b + 2*y)*f(b + z + x) - 2*f(2*z)*f(z +
x)*f(z + y)*
> f(b + 2*y)*f(a + z + y) + 2*f(2*z)*f(z + x)*f(z + y)*f(a
+ 2*y)*f(c
> + 2*y) + 2*f(2*z)^2*f(z + y)*f(b + 2*y)*f(a + y + x) -
f(2*z)^2*f(z
> + y)*f(b + 2*x)*f(b + 2*y) - f(2*z)^2*f(z + y)*f(a + 2*
y)^2 + 2*f(2*
> z)*f(y + x)*f(z + y)*f(c + 2*y)*f(c + y + x) + 2*f(2*z)*
f(y + x)*f(z
> + y)*f(c + 2*y)*f(b + z + x) - 2*f(2*z)*f(y + x)*f(z +
y)*f(c + 2*y)

```

```

>      *f(a + z + y) - 2*f(2*z)*f(y + x)*f(z + y)*f(a + 2*z)*f
>      (b + 2*y) + 4*
>      f(2*z)*f(y + x)*f(z + y)*f(a + 2*y)*f(c + z + y) - 4*f(y
>      + x)*f(z + y
>      )^2*f(c + 2*y)*f(c + z + x) + 2*f(y + x)*f(z + y)^2*f(a
>      + 2*z)*f(c +
>      2*y) - 2*f(y + x)*f(z + y)^2*f(a + 2*y)*f(c + 2*z) - 4*f
>      (y + x)*f(z
>      + x)*f(z + y)*f(c + 2*y)*f(c + z + y) - 2*f(y + x)*f(z
>      + x)*f(z + y)
>      *f(b + 2*z)*f(c + 2*y) + 2*f(y + x)*f(z + x)*f(z + y)*f
>      (b + 2*y)*f(c
>      + 2*z) + 2*f(y + x)^2*f(z + y)*f(c + 2*y)*f(c + 2*z) -
>      4*f(2*y)*f(z
>      + y)^2*f(a + z + y)*f(c + z + x) + 2*f(2*y)*f(z + y)^2*
>      f(a + 2*z)*f(
>      a + z + y) + 4*f(2*y)*f(z + x)*f(z + y)*f(c + 2*y)*f(c +
>      z + x) + 4*
>      f(2*y)*f(z + x)*f(z + y)*f(b + z + y)*f(c + z + x) - 2*f
>      (2*y)*f(z + x
>      )*f(z + y)*f(b + 2*z)*f(a + z + y) + 4*f(2*y)*f(z + x)*f
>      (z + y)*f(a
>      + z + y)*f(c + z + y) - 2*f(2*y)*f(z + x)*f(z + y)*f(a
>      + 2*z)*f(c +
>      2*y) - 2*f(2*y)*f(z + x)*f(z + y)*f(a + 2*z)*f(b + z +
>      y) + 2*f(2*y)*
>      f(z + x)*f(z + y)*f(a + 2*y)*f(c + 2*z) - 4*f(2*y)*f(z +
>      x)^2*f(b + z
>      + y)*f(c + z + y) + 2*f(2*y)*f(z + x)^2*f(b + 2*z)*f(c
>      + 2*y) + 2*f(
>      2*y)*f(z + x)^2*f(b + 2*z)*f(b + z + y) - 2*f(2*y)*f(z +
>      x)^2*f(b + 2
>      *y)*f(c + 2*z) - f(2*y)*f(2*z)*f(z + y)*f(c + 2*x)*f(c +
>      2*y) - 2*f(2
>      *y)*f(2*z)*f(z + y)*f(c + 2*x)*f(b + z + y) + 2*f(2*y)*f
>      (2*z)*f(z + y
>      )*f(a + z + y)*f(c + y + x) + 2*f(2*y)*f(2*z)*f(z + y)*f
>      (a + z + y)*
>      f(b + z + x) - 2*f(2*y)*f(2*z)*f(z + y)*f(a + z + y)^2 -
>      2*f(2*y)*f(2
>      *z)*f(z + y)*f(a + 2*y)*f(c + z + x) + f(2*y)*f(2*z)*f(z
>      + y)*f(a + 2
>      *y)*f(a + 2*z) - 2*f(2*y)*f(2*z)*f(z + x)*f(c + 2*y)*f(b
>      + z + x) + 2
>      *f(2*y)*f(2*z)*f(z + x)*f(b + z + y)*f(c + y + x) - 2*f
>      (2*y)*f(2*z)*
>      f(z + x)*f(b + z + x)*f(b + z + y) + 2*f(2*y)*f(2*z)*f(z
>      + x)*f(b + 2
>      *y)*f(c + z + x) + 2*f(2*y)*f(2*z)*f(z + x)*f(a + z + y)
>      *f(b + z + y)
>      + f(2*y)*f(2*z)*f(z + x)*f(a + 2*z)*f(b + 2*y) - 2*f(2*
>      y)*f(2*z)*f(z
>      + x)*f(a + 2*y)*f(c + z + y) - f(2*y)*f(2*z)*f(z + x)*f
>      (a + 2*y)*f(b
>      + 2*z) - f(2*y)*f(2*z)^2*f(c + 2*y)*f(a + y + x) - 1/2*
>      f(2*y)*f(2*z)
>      ^2*f(b + 2*y)*f(c + 2*x) - f(2*y)*f(2*z)^2*f(b + 2*y)*f

```

```

(a + z + x) +
> 1/2*f(2*y)*f(2*z)^2*f(b + 2*x)*f(c + 2*y) + f(2*y)*f(2*
z)^2*f(b + 2*x
> )*f(b + z + y) - 2*f(2*y)*f(2*z)^2*f(a + y + x)*f(b + z
+ y) + f(2*y)
> *f(2*z)^2*f(a + 2*y)*f(c + y + x) + f(2*y)*f(2*z)^2*f(a
+ 2*y)*f(b +
> z + x) + f(2*y)*f(2*z)^2*f(a + 2*y)*f(a + z + y) - 2*f
(2*y)*f(2*z)*f(
> y + x)*f(c + y + x)*f(c + z + y) - 2*f(2*y)*f(2*z)*f(y +
x)*f(b + z
> + x)*f(c + z + y) - 2*f(2*y)*f(2*z)*f(y + x)*f(a + z +
y)*f(c + z +
> y) + f(2*y)*f(2*z)*f(y + x)*f(a + 2*z)*f(c + 2*y) + 2*f
(2*y)*f(2*z)*
> f(y + x)*f(a + 2*z)*f(b + z + y) - f(2*y)*f(2*z)*f(y +
x)*f(a + 2*y)*
> f(c + 2*z) + 4*f(2*y)*f(y + x)*f(z + y)*f(c + z + x)*f(c
+ z + y) + 2
> *f(2*y)*f(y + x)*f(z + y)*f(c + 2*z)*f(a + z + y) - 2*f
(2*y)*f(y + x)
> *f(z + y)*f(a + 2*z)*f(c + z + y) + 4*f(2*y)*f(y + x)*f
(z + x)*f(c +
> z + y)^2 - 2*f(2*y)*f(y + x)*f(z + x)*f(c + 2*z)*f(b + z
+ y) + 2*f(2
> *y)*f(y + x)*f(z + x)*f(b + 2*z)*f(c + z + y) - 2*f(2*y)
*f(y + x)^2*
> f(c + 2*z)*f(c + z + y) - 2*f(2*y)^2*f(z + y)*f(c + 2*z)
*f(a + z + x)
> + 2*f(2*y)^2*f(z + y)*f(a + 2*z)*f(c + z + x) - 4*f(2*
y)^2*f(z + x)*
> f(c + z + x)*f(c + z + y) + 2*f(2*y)^2*f(z + x)*f(c + 2*
z)*f(b + z +
> x) - 2*f(2*y)^2*f(z + x)*f(b + 2*z)*f(c + z + x) + f(2*
y)^2*f(2*z)*f(
> c + 2*z)*f(a + y + x) + f(2*y)^2*f(2*z)*f(c + 2*x)*f(c +
z + y) + 1/2
> *f(2*y)^2*f(2*z)*f(b + 2*z)*f(c + 2*x) + f(2*y)^2*f(2*z)
*f(b + 2*z)*
> f(a + z + x) - 1/2*f(2*y)^2*f(2*z)*f(b + 2*x)*f(c + 2*z)
+ 2*f(2*y)^2
> *f(2*z)*f(a + z + x)*f(c + z + y) - f(2*y)^2*f(2*z)*f(a
+ 2*z)*f(c +
> y + x) - f(2*y)^2*f(2*z)*f(a + 2*z)*f(b + z + x) - f(2*
y)^2*f(2*z)*f(
> a + 2*z)*f(a + z + y) + 4*f(2*x)*f(z + y)^2*f(c + 2*y)*f
(c + z + y)
> - f(2*x)*f(2*z)*f(z + y)*f(c + 2*y)^2 - 2*f(2*x)*f(2*z)
*f(z + y)*f(b
> + 2*y)*f(c + z + y) + f(2*x)*f(2*z)*f(z + y)*f(b + 2*y)
*f(b + 2*z)
> - 4*f(2*x)*f(2*y)*f(z + y)*f(c + z + y)^2 - 2*f(2*x)*f
(2*y)*f(z + y)
> *f(c + 2*y)*f(c + 2*z) + f(2*x)*f(2*y)*f(2*z)*f(c + 2*y)
*f(c + z + y)
> + 2*f(2*x)*f(2*y)*f(2*z)*f(b + z + y)*f(c + z + y) -
1/2*f(2*x)*f(2*

```

```

> y)*f(2*z)*f(b + 2*z)*f(c + 2*y) - f(2*x)*f(2*y)*f(2*z)*f
(b + 2*z)*f(b
> + z + y) + 1/2*f(2*x)*f(2*y)*f(2*z)*f(b + 2*y)*f(c + 2*
z) + 2*f(2*x)
> *f(2*y)^2*f(c + 2*z)*f(c + z + y) )
>
> + 2*f(z + y)*f(2*c + 2*y) - 2*f(2*y)*f(2*c + z + y):
> eq[18] :=
> (1/HessUniv) * ( 4*f(z + x)*f(z + y)^2*f(a + 2*y)*f(c + z + x) -
2*f(
> z + x)*f(z + y)^2*f(a + 2*y)*f(a + 2*z) - 4*f(z + x)^2*f
(z + y)*f(b
> + 2*y)*f(c + z + x) + 2*f(z + x)^2*f(z + y)*f(a + 2*z)*
f(b + 2*y) -
> 4*f(z + x)^2*f(z + y)*f(a + 2*y)*f(c + z + y) + 2*f(z +
x)^2*f(z + y)
> *f(a + 2*y)*f(b + 2*z) + 4*f(z + x)^3*f(b + 2*y)*f(c + z
+ y) - 2*f(z
> + x)^3*f(b + 2*y)*f(b + 2*z) + 2*f(2*z)*f(z + x)*f(z +
y)*f(b + 2*y)
> *f(c + 2*x) - 2*f(2*z)*f(z + x)*f(z + y)*f(a + 2*y)*f(c
+ y + x) - 2*
> f(2*z)*f(z + x)*f(z + y)*f(a + 2*y)*f(b + z + x) + 2*f
(2*z)*f(z + x)*
> f(z + y)*f(a + 2*y)*f(a + z + y) - 2*f(2*z)*f(z + x)^2*f
(b + 2*y)*f(c
> + y + x) + 2*f(2*z)*f(z + x)^2*f(b + 2*y)*f(b + z + x)
- 2*f(2*z)*f(
> z + x)^2*f(b + 2*y)*f(a + z + y) + 2*f(2*z)*f(z + x)^2*f
(a + 2*y)*f(c
> + 2*y) + 2*f(2*z)^2*f(z + x)*f(b + 2*y)*f(a + y + x) -
f(2*z)^2*f(z
> + x)*f(b + 2*x)*f(b + 2*y) - f(2*z)^2*f(z + x)*f(a + 2*
y)^2 + 2*f(2*
> z)*f(y + x)*f(z + x)*f(c + 2*y)*f(c + y + x) + 2*f(2*z)*
f(y + x)*f(z
> + x)*f(c + 2*y)*f(b + z + x) - 2*f(2*z)*f(y + x)*f(z +
x)*f(c + 2*y)
> *f(a + z + y) - 2*f(2*z)*f(y + x)*f(z + x)*f(a + 2*z)*f
(b + 2*y) + 4*
> f(2*z)*f(y + x)*f(z + x)*f(a + 2*y)*f(c + z + y) - 4*f(y
+ x)*f(z + x)
> )*f(z + y)*f(c + 2*y)*f(c + z + x) + 2*f(y + x)*f(z + x)
*f(z + y)*f(a
> + 2*z)*f(c + 2*y) - 2*f(y + x)*f(z + x)*f(z + y)*f(a +
2*y)*f(c + 2*
> z) - 4*f(y + x)*f(z + x)^2*f(c + 2*y)*f(c + z + y) - 2*f
(y + x)*f(z
> + x)^2*f(b + 2*z)*f(c + 2*y) + 2*f(y + x)*f(z + x)^2*f
(b + 2*y)*f(c
> + 2*z) + 2*f(y + x)^2*f(z + x)*f(c + 2*y)*f(c + 2*z) -
4*f(2*y)*f(z
> + y)^2*f(a + z + x)*f(c + z + x) + 2*f(2*y)*f(z + y)^2*
f(a + 2*z)*f(
> c + 2*x) + 2*f(2*y)*f(z + y)^2*f(a + 2*z)*f(a + z + x) -
2*f(2*y)*f(z

```

```

> + y)^2*f(a + 2*x)*f(c + 2*z) + 4*f(2*y)*f(z + x)*f(z +
> y)*f(c + 2*z)
> *f(a + y + x) + 4*f(2*y)*f(z + x)*f(z + y)*f(b + z + x)*
> f(c + z + x)
> - 2*f(2*y)*f(z + x)*f(z + y)*f(b + 2*z)*f(c + 2*x) - 2*
> f(2*y)*f(z +
> x)*f(z + y)*f(b + 2*z)*f(a + z + x) + 2*f(2*y)*f(z + x)*
> f(z + y)*f(b
> + 2*x)*f(c + 2*z) + 4*f(2*y)*f(z + x)*f(z + y)*f(a + z
> + x)*f(c + z
> + y) - 4*f(2*y)*f(z + x)*f(z + y)*f(a + 2*z)*f(c + y +
> x) - 2*f(2*y)
> *f(z + x)*f(z + y)*f(a + 2*z)*f(b + z + x) - 4*f(2*y)*f
> (z + x)^2*f(c
> + 2*z)*f(b + y + x) + 4*f(2*y)*f(z + x)^2*f(c + 2*y)*f
> (c + z + x) -
> 4*f(2*y)*f(z + x)^2*f(b + z + x)*f(c + z + y) + 4*f(2*y)
> *f(z + x)^2*
> f(b + 2*z)*f(c + y + x) + 2*f(2*y)*f(z + x)^2*f(b + 2*z)
> *f(b + z + x)
> - 2*f(2*y)*f(2*z)*f(z + y)*f(c + 2*x)*f(a + z + y) - 2*
> f(2*y)*f(2*z)
> *f(z + y)*f(b + 2*x)*f(c + z + x) + 2*f(2*y)*f(2*z)*f(z
> + y)*f(a + z
> + x)*f(c + y + x) + 2*f(2*y)*f(2*z)*f(z + y)*f(a + z +
> x)*f(b + z +
> x) - 2*f(2*y)*f(2*z)*f(z + y)*f(a + z + x)*f(a + z + y)
> - f(2*y)*f(2*
> z)*f(z + y)*f(a + 2*z)*f(b + 2*x) + 2*f(2*y)*f(2*z)*f(z
> + y)*f(a + 2*
> x)*f(c + z + y) + f(2*y)*f(2*z)*f(z + y)*f(a + 2*x)*f(b
> + 2*z) - 2*f(
> 2*y)*f(2*z)*f(z + x)*f(c + 2*y)*f(a + z + x) - f(2*y)*f
> (2*z)*f(z + x)
> *f(c + 2*x)*f(c + 2*y) - 2*f(2*y)*f(2*z)*f(z + x)*f(b +
> z + x)*f(c +
> y + x) - 2*f(2*y)*f(2*z)*f(z + x)*f(b + z + x)^2 - 2*f
> (2*y)*f(2*z)*f(
> z + x)*f(b + 2*z)*f(a + y + x) + 4*f(2*y)*f(2*z)*f(z +
> x)*f(b + y + x
> )*f(c + z + x) + 4*f(2*y)*f(2*z)*f(z + x)*f(a + z + y)*f
> (c + y + x)
> + 2*f(2*y)*f(2*z)*f(z + x)*f(a + z + y)*f(b + z + x) +
> 2*f(2*y)*f(2*
> z)*f(z + x)*f(a + 2*z)*f(b + y + x) - 4*f(2*y)*f(2*z)*f
> (z + x)*f(a +
> y + x)*f(c + z + y) - 2*f(2*y)*f(2*z)*f(z + x)*f(a + 2*
> y)*f(c + z + x
> ) + f(2*y)*f(2*z)*f(z + x)*f(a + 2*y)*f(a + 2*z) - f(2*
> y)*f(2*z)^2*f(
> c + 2*x)*f(b + y + x) + f(2*y)*f(2*z)^2*f(b + 2*x)*f(c +
> y + x) + f(2
> *y)*f(2*z)^2*f(b + 2*x)*f(b + z + x) + f(2*y)*f(2*z)^2*f
> (b + 2*x)*f(a
> + z + y) - 2*f(2*y)*f(2*z)^2*f(a + z + x)*f(b + y + x)
> + 1/2*f(2*y)*
> f(2*z)^2*f(a + 2*y)*f(c + 2*x) + f(2*y)*f(2*z)^2*f(a +

```

```

2*y)*f(a + z
> + x) - 1/2*f(2*y)*f(2*z)^2*f(a + 2*x)*f(c + 2*y) - f(2*
y)*f(2*z)^2*
> f(a + 2*x)*f(b + z + y) - 2*f(2*y)*f(2*z)*f(y + x)*f(c +
y + x)*f(c
> + z + x) - 2*f(2*y)*f(2*z)*f(y + x)*f(b + z + x)*f(c +
z + x) + f(2*
> y)*f(2*z)*f(y + x)*f(b + 2*z)*f(c + 2*x) + 2*f(2*y)*f(2*
z)*f(y + x)*
> f(b + 2*z)*f(a + z + x) - f(2*y)*f(2*z)*f(y + x)*f(b +
2*x)*f(c + 2*z
> ) - 2*f(2*y)*f(2*z)*f(y + x)*f(a + z + y)*f(c + z + x) +
4*f(2*y)*f(y
> + x)*f(z + y)*f(c + z + x)^2 - 2*f(2*y)*f(y + x)*f(z +
y)*f(c + 2*z)
> *f(a + z + x) + 2*f(2*y)*f(y + x)*f(z + y)*f(a + 2*z)*f
(c + z + x) +
> 4*f(2*y)*f(y + x)*f(z + x)*f(c + z + x)*f(c + z + y) +
2*f(2*y)*f(y
> + x)*f(z + x)*f(c + 2*z)*f(b + z + x) - 2*f(2*y)*f(y +
x)*f(z + x)*
> f(b + 2*z)*f(c + z + x) - 2*f(2*y)*f(y + x)^2*f(c + 2*z)
*f(c + z + x)
> - 4*f(2*y)^2*f(z + x)*f(c + z + x)^2 + f(2*y)^2*f(2*z)*
f(c + 2*x)*f(
> c + z + x) + 2*f(2*y)^2*f(2*z)*f(a + z + x)*f(c + z + x)
- 1/2*f(2*y)
> ^2*f(2*z)*f(a + 2*z)*f(c + 2*x) - f(2*y)^2*f(2*z)*f(a +
2*z)*f(a + z
> + x) + 1/2*f(2*y)^2*f(2*z)*f(a + 2*x)*f(c + 2*z) + 4*f
(2*x)*f(z + x)
> *f(z + y)*f(c + 2*y)*f(c + z + y) - f(2*x)*f(2*z)*f(z +
x)*f(c + 2*y)
> ^2 - 2*f(2*x)*f(2*z)*f(z + x)*f(b + 2*y)*f(c + z + y) +
f(2*x)*f(2*z)
> *f(z + x)*f(b + 2*y)*f(b + 2*z) - 4*f(2*x)*f(2*y)*f(z +
y)*f(c + z +
> x)*f(c + z + y) + 2*f(2*x)*f(2*y)*f(z + y)*f(c + 2*z)*f
(a + z + y) -
> 2*f(2*x)*f(2*y)*f(z + y)*f(a + 2*z)*f(c + z + y) - 2*f
(2*x)*f(2*y)*f(
> z + x)*f(c + 2*z)*f(b + z + y) - 2*f(2*x)*f(2*y)*f(z +
x)*f(c + 2*y)*
> f(c + 2*z) + 2*f(2*x)*f(2*y)*f(z + x)*f(b + 2*z)*f(c + z
+ y) + f(2*x)
> )*f(2*y)*f(2*z)*f(c + 2*z)*f(b + y + x) + f(2*x)*f(2*y)*
f(2*z)*f(c +
> 2*y)*f(c + z + x) + 2*f(2*x)*f(2*y)*f(2*z)*f(b + z + y)*
f(c + z + x)
> - f(2*x)*f(2*y)*f(2*z)*f(b + 2*z)*f(c + y + x) - f(2*x)
*f(2*y)*f(2*z)
> )*f(b + 2*z)*f(b + z + x) - f(2*x)*f(2*y)*f(2*z)*f(b +
2*z)*f(a + z
> + y) + 1/2*f(2*x)*f(2*y)*f(2*z)*f(a + 2*z)*f(c + 2*y) +
f(2*x)*f(2*y)
> )*f(2*z)*f(a + 2*z)*f(b + z + y) - 1/2*f(2*x)*f(2*y)*f
(2*z)*f(a + 2*y

```

```

> ) * f(c + 2*z) + 2*f(2*x)*f(2*y)^2*f(c + 2*z)*f(c + z + x)
> )
> + 2*f(z + x)*f(2*c + 2*y) - 2*f(2*y)*f(2*c + z + x):
>
> eq[19] :=
> (1/HessUniv) * ( 8*f(z + x)*f(z + y)^2*f(b + 2*y)*f(a + y + x) -
> 4*f(
> z + x)*f(z + y)^2*f(a + 2*y)*f(b + y + x) - 2*f(z + x)*f
> (z + y)^2*f(a
> + 2*y)^2 - 4*f(z + x)^2*f(z + y)*f(b + 2*y)*f(b + y +
> x) + 2*f(z + x
> )^3*f(b + 2*y)^2 + 4*f(2*z)*f(y + x)*f(z + x)*f(b + 2*y)
> *f(b + y + x)
> + 4*f(y + x)*f(z + x)*f(z + y)*f(c + 2*y)*f(b + y + x)
> - 8*f(y + x)*
> f(z + x)*f(z + y)*f(b + 2*y)*f(c + y + x) - 8*f(y + x)*f
> (z + x)*f(z
> + y)*f(b + 2*y)*f(a + z + y) + 4*f(y + x)*f(z + x)*f(z
> + y)*f(a + 2*
> y)*f(c + 2*y) + 4*f(y + x)*f(z + x)*f(z + y)*f(a + 2*y)*
> f(b + z + y)
> - 4*f(y + x)*f(z + x)^2*f(b + 2*y)*f(b + z + y) - 2*f(y
> + x)^2*f(z
> + x)*f(c + 2*y)^2 - 4*f(y + x)^2*f(z + x)*f(c + 2*y)*f
> (b + z + y) +
> 8*f(y + x)^2*f(z + x)*f(b + 2*y)*f(c + z + y) - 4*f(2*y)
> *f(z + y)^2*
> f(a + z + x)*f(b + y + x) + 2*f(2*y)*f(z + y)^2*f(a + 2*
> y)*f(a + z +
> x) - 4*f(2*y)*f(z + x)*f(z + y)*f(c + 2*y)*f(a + y + x)
> + 4*f(2*y)*f(
> z + x)*f(z + y)*f(b + y + x)*f(b + z + x) + 2*f(2*y)*f(z
> + x)*f(z + y
> ) * f(b + 2*y)*f(c + 2*x) - 2*f(2*y)*f(z + x)*f(z + y)*f(b
> + 2*y)*f(a
> + z + x) + 8*f(2*y)*f(z + x)*f(z + y)*f(a + z + y)*f(b
> + y + x) - 8*
> f(2*y)*f(z + x)*f(z + y)*f(a + y + x)*f(b + z + y) + 2*f
> (2*y)*f(z + x
> ) * f(z + y)*f(a + 2*y)*f(c + y + x) + 2*f(2*y)*f(z + x)*f
> (z + y)*f(a
> + 2*y)*f(a + z + y) + 2*f(2*y)*f(z + x)^2*f(b + 2*y)*f
> (c + y + x) +
> 2*f(2*y)*f(z + x)^2*f(b + 2*y)*f(a + z + y) - 2*f(2*y)*f
> (z + x)^2*f(a
> + 2*y)*f(c + 2*y) + f(2*y)*f(2*z)*f(z + y)*f(a + 2*y)*f
> (b + 2*x) -
> f(2*y)*f(2*z)*f(z + y)*f(a + 2*x)*f(b + 2*y) - 2*f(2*y)*
> f(2*z)*f(z +
> x)*f(b + 2*y)*f(a + y + x) - f(2*y)*f(2*z)*f(z + x)*f(b
> + 2*x)*f(b +
> 2*y) + f(2*y)*f(2*z)*f(z + x)*f(a + 2*y)^2 - 4*f(2*y)*f
> (2*z)*f(y + x)
> *f(b + y + x)*f(b + z + x) + f(2*y)*f(2*z)*f(y + x)*f(b
> + 2*y)*f(c +

```

```

>      2*x) - f(2*y)*f(2*z)*f(y + x)*f(b + 2*x)*f(c + 2*y) - 2*
f(2*y)*f(y +
>      x)*f(z + y)*f(c + 2*y)*f(a + z + x) + 4*f(2*y)*f(y + x)*
f(z + y)*f(b
>      + y + x)*f(c + z + x) + 4*f(2*y)*f(y + x)*f(z + y)*f(a
+ z + x)*f(b
>      + z + y) - 2*f(2*y)*f(y + x)*f(z + y)*f(a + 2*y)*f(c +
z + x) + 2*f(
>      2*y)*f(y + x)*f(z + x)*f(c + 2*y)*f(c + y + x) + 2*f(2*
y)*f(y + x)*f(
>      z + x)*f(c + 2*y)*f(a + z + y) + 8*f(2*y)*f(y + x)*f(z +
x)*f(b + z
>      + y)*f(c + y + x) + 4*f(2*y)*f(y + x)*f(z + x)*f(b + z
+ x)*f(b + z
>      + y) - 8*f(2*y)*f(y + x)*f(z + x)*f(b + y + x)*f(c + z
+ y) - 2*f(2*
>      y)*f(y + x)*f(z + x)*f(b + 2*y)*f(c + z + x) + 2*f(2*y)*
f(y + x)*f(z
>      + x)*f(a + 2*z)*f(b + 2*y) - 4*f(2*y)*f(y + x)*f(z + x)
*f(a + 2*y)*
>      f(c + z + y) + 2*f(2*y)*f(y + x)^2*f(c + 2*y)*f(c + z +
x) - 4*f(2*y)
>      *f(y + x)^2*f(b + z + y)*f(c + z + x) - 2*f(2*y)^2*f(z +
y)*f(b + 2*x
>      )*f(c + z + x) + 2*f(2*y)^2*f(z + y)*f(a + z + x)*f(c +
y + x) + 2*f(
>      2*y)^2*f(z + y)*f(a + z + x)*f(b + z + x) - 2*f(2*y)^2*f
(z + y)*f(a
>      + z + x)*f(a + z + y) + 2*f(2*y)^2*f(z + x)*f(c + 2*y)*
f(a + z + x)
>      - f(2*y)^2*f(z + x)*f(c + 2*x)*f(c + 2*y) - 2*f(2*y)^2*
f(z + x)*f(c
>      + 2*x)*f(b + z + y) - 2*f(2*y)^2*f(z + x)*f(b + z + x)*
f(c + y + x)
>      - 2*f(2*y)^2*f(z + x)*f(b + z + x)^2 + 2*f(2*y)^2*f(z +
x)*f(b + 2*z
>      )*f(a + y + x) + 2*f(2*y)^2*f(z + x)*f(b + 2*x)*f(c + z
+ y) - 4*f(2*
>      y)^2*f(z + x)*f(a + z + y)*f(c + y + x) - 2*f(2*y)^2*f(z
+ x)*f(a + z
>      + y)*f(b + z + x) - 2*f(2*y)^2*f(z + x)*f(a + 2*z)*f(b
+ y + x) + 4*
>      f(2*y)^2*f(z + x)*f(a + y + x)*f(c + z + y) + 2*f(2*y)
^2*f(z + x)*f(a
>      + 2*y)*f(c + z + x) - f(2*y)^2*f(z + x)*f(a + 2*y)*f(a
+ 2*z) - f(2*
>      y)^2*f(2*z)*f(c + 2*x)*f(b + y + x) + f(2*y)^2*f(2*z)*f
(b + 2*x)*f(c
>      + y + x) + f(2*y)^2*f(2*z)*f(b + 2*x)*f(b + z + x) - f
(2*y)^2*f(2*z)
>      *f(b + 2*x)*f(a + z + y) + 2*f(2*y)^2*f(2*z)*f(a + z +
x)*f(b + y + x
>      ) - 1/2*f(2*y)^2*f(2*z)*f(a + 2*y)*f(c + 2*x) - f(2*y)
^2*f(2*z)*f(a
>      + 2*y)*f(a + z + x) + 1/2*f(2*y)^2*f(2*z)*f(a + 2*x)*f
(c + 2*y) + f(
>      2*y)^2*f(2*z)*f(a + 2*x)*f(b + z + y) - 2*f(2*y)^2*f(y +

```



```

x)*f(c + y
> + x)*f(c + z + x) + 2*f(2*y)^2*f(y + x)*f(b + z + x)*f
(c + z + x) -
> 2*f(2*y)^2*f(y + x)*f(b + 2*z)*f(a + z + x) + 2*f(2*y)
^2*f(y + x)*f(a
> + z + y)*f(c + z + x) + f(2*y)^3*f(c + 2*x)*f(c + z +
x) - 2*f(2*y)^
> 3*f(a + z + x)*f(c + z + x) + 1/2*f(2*y)^3*f(a + 2*z)*f
(c + 2*x) + f(
> 2*y)^3*f(a + 2*z)*f(a + z + x) - 1/2*f(2*y)^3*f(a + 2*x)
*f(c + 2*z)
> + 4*f(2*x)*f(z + x)*f(z + y)*f(b + 2*y)*f(b + z + y) -
2*f(2*x)*f(2*
> z)*f(z + x)*f(b + 2*y)^2 - 4*f(2*x)*f(2*y)*f(z + y)*f(b
+ z + x)*f(b
> + z + y) + f(2*x)*f(2*y)*f(z + y)*f(a + 2*z)*f(b + 2*y)
- f(2*x)*f(2
> *y)*f(z + y)*f(a + 2*y)*f(b + 2*z) + f(2*x)*f(2*y)*f(z +
x)*f(c + 2*y
> )^2 - 2*f(2*x)*f(2*y)*f(z + x)*f(b + 2*y)*f(c + z + y) -
f(2*x)*f(2*y
> )*f(z + x)*f(b + 2*y)*f(b + 2*z) + 2*f(2*x)*f(2*y)*f(2*
z)*f(b + 2*y)*
> f(b + z + x) + f(2*x)*f(2*y)*f(y + x)*f(b + 2*z)*f(c +
2*y) - f(2*x)*
> f(2*y)*f(y + x)*f(b + 2*y)*f(c + 2*z) + f(2*x)*f(2*y)^2*
f(c + 2*z)*f(
> b + y + x) - f(2*x)*f(2*y)^2*f(c + 2*y)*f(c + z + x) +
2*f(2*x)*f(2*y
> )^2*f(b + z + y)*f(c + z + x) - f(2*x)*f(2*y)^2*f(b + 2*
z)*f(c + y +
> x) + f(2*x)*f(2*y)^2*f(b + 2*z)*f(b + z + x) + f(2*x)*f
(2*y)^2*f(b +
> 2*z)*f(a + z + y) - 1/2*f(2*x)*f(2*y)^2*f(a + 2*z)*f(c +
2*y) - f(2*x
> )*f(2*y)^2*f(a + 2*z)*f(b + z + y) + 1/2*f(2*x)*f(2*y)
^2*f(a + 2*y)*
> f(c + 2*z) )
>
> + 2*f(z + x)*f(2*b + 2*y) - 2*f(2*y)*f(2*b + z + x):
>
> eq[20] :=
> (1/HessUniv) * ( - 2*f(2*y)*f(z + y)^2*f(a + 2*x)*f(c + z + x) +
f(2
> *y)*f(z + y)^2*f(a + 2*x)*f(a + 2*z) + 2*f(2*y)*f(z + x)
*f(z + y)*f(b
> + 2*x)*f(c + z + x) - f(2*y)*f(z + x)*f(z + y)*f(a + 2*
z)*f(b + 2*x)
> + 2*f(2*y)*f(z + x)*f(z + y)*f(a + 2*x)*f(c + z + y) -
f(2*y)*f(z +
> x)*f(z + y)*f(a + 2*x)*f(b + 2*z) - 2*f(2*y)*f(z + x)^2*
f(b + 2*x)*f(
> c + z + y) + f(2*y)*f(z + x)^2*f(b + 2*x)*f(b + 2*z) - f
(2*y)*f(2*z)*
> f(z + y)*f(b + 2*x)*f(c + 2*x) + f(2*y)*f(2*z)*f(z + y)*
f(a + 2*x)*f(
> c + y + x) + f(2*y)*f(2*z)*f(z + y)*f(a + 2*x)*f(b + z +

```

```

x) - f(2*y)*
> f(2*z)*f(z + y)*f(a + 2*x)*f(a + z + y) + f(2*y)*f(2*z)*
f(z + x)*f(b
> + 2*x)*f(c + y + x) - f(2*y)*f(2*z)*f(z + x)*f(b + 2*x)
*f(b + z + x)
> + f(2*y)*f(2*z)*f(z + x)*f(b + 2*x)*f(a + z + y) - f(2*
y)*f(2*z)*f(z
> + x)*f(a + 2*x)*f(c + 2*y) + 1/2*f(2*y)*f(2*z)^2*f(b +
2*x)^2 - f(2*
> y)*f(2*z)^2*f(a + 2*x)*f(b + y + x) + 1/2*f(2*y)*f(2*z)
^2*f(a + 2*x)*
> f(a + 2*y) - f(2*y)*f(2*z)*f(y + x)*f(c + 2*x)*f(c + y +
x) + f(2*y)*
> f(2*z)*f(y + x)*f(c + 2*x)*f(b + z + x) - f(2*y)*f(2*z)*
f(y + x)*f(c
> + 2*x)*f(a + z + y) - 2*f(2*y)*f(2*z)*f(y + x)*f(b + 2*
x)*f(c + z +
> x) + f(2*y)*f(2*z)*f(y + x)*f(a + 2*x)*f(b + 2*z) + 2*f
(2*y)*f(y + x)
> *f(z + y)*f(c + 2*x)*f(c + z + x) + f(2*y)*f(y + x)*f(z
+ y)*f(a + 2*
> z)*f(c + 2*x) - f(2*y)*f(y + x)*f(z + y)*f(a + 2*x)*f(c
+ 2*z) + 2*f(
> 2*y)*f(y + x)*f(z + x)*f(c + 2*x)*f(c + z + y) - f(2*y)*
f(y + x)*f(z
> + x)*f(b + 2*z)*f(c + 2*x) + f(2*y)*f(y + x)*f(z + x)*f
(b + 2*x)*f(c
> + 2*z) - f(2*y)*f(y + x)^2*f(c + 2*x)*f(c + 2*z) - 2*f
(2*y)^2*f(z +
> x)*f(c + 2*x)*f(c + z + x) + 1/2*f(2*y)^2*f(2*z)*f(c +
2*x)^2 + f(2*y
> )^2*f(2*z)*f(a + 2*x)*f(c + z + x) - 1/2*f(2*y)^2*f(2*z)
*f(a + 2*x)*
> f(a + 2*z) + 2*f(2*x)*f(z + y)^2*f(a + 2*y)*f(c + z + x)
- f(2*x)*f(z
> + y)^2*f(a + 2*y)*f(a + 2*z) - 2*f(2*x)*f(z + x)*f(z +
y)*f(b + 2*y)
> *f(c + z + x) + f(2*x)*f(z + x)*f(z + y)*f(a + 2*z)*f(b
+ 2*y) - 2*f(
> 2*x)*f(z + x)*f(z + y)*f(a + 2*y)*f(c + z + y) + f(2*x)*
f(z + x)*f(z
> + y)*f(a + 2*y)*f(b + 2*z) + 2*f(2*x)*f(z + x)^2*f(b +
2*y)*f(c + z
> + y) - f(2*x)*f(z + x)^2*f(b + 2*y)*f(b + 2*z) + f(2*x)
*f(2*z)*f(z
> + y)*f(b + 2*y)*f(c + 2*x) - f(2*x)*f(2*z)*f(z + y)*f(a
+ 2*y)*f(c
> + y + x) - f(2*x)*f(2*z)*f(z + y)*f(a + 2*y)*f(b + z +
x) + f(2*x)*
> f(2*z)*f(z + y)*f(a + 2*y)*f(a + z + y) - f(2*x)*f(2*z)*
f(z + x)*f(b
> + 2*y)*f(c + y + x) + f(2*x)*f(2*z)*f(z + x)*f(b + 2*y)
*f(b + z + x)
> - f(2*x)*f(2*z)*f(z + x)*f(b + 2*y)*f(a + z + y) + f(2*
x)*f(2*z)*f(z
> + x)*f(a + 2*y)*f(c + 2*y) + f(2*x)*f(2*z)^2*f(b + 2*y)
*f(a + y + x)

```

```

> - 1/2*f(2*x)*f(2*z)^2*f(b + 2*x)*f(b + 2*y) - 1/2*f(2*
x)*f(2*z)^2*f(
> a + 2*y)^2 + f(2*x)*f(2*z)*f(y + x)*f(c + 2*y)*f(c + y +
x) + f(2*x)*
> f(2*z)*f(y + x)*f(c + 2*y)*f(b + z + x) - f(2*x)*f(2*z)*
f(y + x)*f(c
> + 2*y)*f(a + z + y) - f(2*x)*f(2*z)*f(y + x)*f(a + 2*z)
*f(b + 2*y)
> + 2*f(2*x)*f(2*z)*f(y + x)*f(a + 2*y)*f(c + z + y) - 2*
f(2*x)*f(y +
> x)*f(z + y)*f(c + 2*y)*f(c + z + x) + f(2*x)*f(y + x)*f
(z + y)*f(a +
> 2*z)*f(c + 2*y) - f(2*x)*f(y + x)*f(z + y)*f(a + 2*y)*f
(c + 2*z) - 2*
> f(2*x)*f(y + x)*f(z + x)*f(c + 2*y)*f(c + z + y) - f(2*
x)*f(y + x)*f(
> z + x)*f(b + 2*z)*f(c + 2*y) + f(2*x)*f(y + x)*f(z + x)*
f(b + 2*y)*f(
> c + 2*z) + f(2*x)*f(y + x)^2*f(c + 2*y)*f(c + 2*z) + 2*f
(2*x)*f(2*y)*
> f(z + y)*f(c + 2*z)*f(a + y + x) - 2*f(2*x)*f(2*y)*f(z +
y)*f(c + 2*x
> )*f(c + z + y) - 2*f(2*x)*f(2*y)*f(z + y)*f(a + 2*z)*f(c
+ y + x) - 2
> *f(2*x)*f(2*y)*f(z + x)*f(c + 2*z)*f(b + y + x) + 2*f(2*
x)*f(2*y)*f(z
> + x)*f(c + 2*y)*f(c + z + x) + 2*f(2*x)*f(2*y)*f(z + x)
*f(b + 2*z)*
> f(c + y + x) - 2*f(2*x)*f(2*y)*f(2*z)*f(b + z + x)*f(c +
y + x) - f(2
> *x)*f(2*y)*f(2*z)*f(b + 2*z)*f(a + y + x) + 2*f(2*x)*f
(2*y)*f(2*z)*f(
> b + y + x)*f(c + z + x) + f(2*x)*f(2*y)*f(2*z)*f(b + 2*
x)*f(c + z + y
> ) - 1/2*f(2*x)*f(2*y)*f(2*z)*f(b + 2*x)*f(b + 2*z) + 2*f
(2*x)*f(2*y)*
> f(2*z)*f(a + z + y)*f(c + y + x) + f(2*x)*f(2*y)*f(2*z)*
f(a + 2*z)*f(
> b + y + x) - 2*f(2*x)*f(2*y)*f(2*z)*f(a + y + x)*f(c + z
+ y) - f(2*x
> )*f(2*y)*f(2*z)*f(a + 2*y)*f(c + z + x) + 1/2*f(2*x)*f
(2*y)*f(2*z)*f(
> a + 2*y)*f(a + 2*z) + f(2*x)*f(2*y)^2*f(c + 2*x)*f(c +
2*z) + 2*f(2*x
> )^2*f(z + y)*f(c + 2*y)*f(c + z + y) - 1/2*f(2*x)^2*f(2*
z)*f(c + 2*y)
> ^2 - f(2*x)^2*f(2*z)*f(b + 2*y)*f(c + z + y) + 1/2*f(2*
x)^2*f(2*z)*f(
> b + 2*y)*f(b + 2*z) - f(2*x)^2*f(2*y)*f(c + 2*y)*f(c +
2*z) )
> - f(2*y)*f(2*c + 2*x) + f(2*x)*f(2*c + 2*y):
> eq[21] :=
> (1/HessUniv) * ( 2*f(z + y)^3*f(b + 2*y)*f(c + 2*x) - 4*f(z + x)*
f(z
> + y)^2*f(b + 2*y)*f(c + y + x) + 2*f(z + x)^2*f(z + y)*

```

```

f(b + 2*y)*f(
> c + 2*y) + 4*f(2*z)*f(z + y)^2*f(b + 2*y)*f(a + y + x) -
f(2*z)*f(z
> + y)^2*f(b + 2*x)*f(b + 2*y) - 2*f(2*z)*f(z + y)^2*f(a
+ 2*y)*f(b +
> y + x) - f(2*z)*f(z + y)^2*f(a + 2*y)^2 + 2*f(2*z)*f(y +
x)*f(z + y)*
> f(c + 2*y)*f(b + y + x) + 2*f(2*z)*f(y + x)*f(z + y)*f(b
+ 2*y)*f(b
> + z + x) - 4*f(2*z)*f(y + x)*f(z + y)*f(b + 2*y)*f(a +
z + y) + 2*f(
> 2*z)*f(y + x)*f(z + y)*f(a + 2*y)*f(c + 2*y) + 2*f(2*z)*
f(y + x)*f(z
> + y)*f(a + 2*y)*f(b + z + y) - 4*f(y + x)*f(z + y)^2*f
(b + 2*y)*f(c
> + z + x) - 2*f(y + x)*f(z + x)*f(z + y)*f(c + 2*y)^2 -
4*f(y + x)*f(
> z + x)*f(z + y)*f(c + 2*y)*f(b + z + y) + 4*f(y + x)*f(z
+ x)*f(z + y
> )*f(b + 2*y)*f(c + z + y) - 2*f(y + x)*f(z + x)*f(z + y)
*f(b + 2*y)*
> f(b + 2*z) + 2*f(y + x)^2*f(z + y)*f(b + 2*y)*f(c + 2*z)
- f(2*y)*f(z
> + y)^2*f(c + 2*x)*f(c + 2*y) - 2*f(2*y)*f(z + y)^2*f(c
+ 2*x)*f(b +
> z + y) + 2*f(2*y)*f(z + y)^2*f(a + 2*y)*f(c + z + x) - f
(2*y)*f(z + y
> )^2*f(a + 2*y)*f(a + 2*z) + 2*f(2*y)*f(z + x)*f(z + y)*f
(c + 2*y)*f(c
> + y + x) + 4*f(2*y)*f(z + x)*f(z + y)*f(b + z + y)*f(c
+ y + x) + 2*
> f(2*y)*f(z + x)*f(z + y)*f(b + 2*y)*f(c + z + x) + f(2*
y)*f(z + x)*f(
> z + y)*f(a + 2*z)*f(b + 2*y) - 2*f(2*y)*f(z + x)*f(z +
y)*f(a + 2*y)*
> f(c + z + y) + f(2*y)*f(z + x)*f(z + y)*f(a + 2*y)*f(b +
2*z) - 2*f(2
> *y)*f(z + x)^2*f(b + 2*y)*f(c + z + y) - 2*f(2*y)*f(2*z)
*f(z + y)*f(c
> + 2*y)*f(a + y + x) - 1/2*f(2*y)*f(2*z)*f(z + y)*f(b +
2*y)*f(c + 2*
> x) - 2*f(2*y)*f(2*z)*f(z + y)*f(b + 2*y)*f(a + z + x) +
1/2*f(2*y)*f(
> 2*z)*f(z + y)*f(b + 2*x)*f(c + 2*y) + f(2*y)*f(2*z)*f(z
+ y)*f(b + 2*
> x)*f(b + z + y) + 2*f(2*y)*f(2*z)*f(z + y)*f(a + z + y)*
f(b + y + x)
> - 4*f(2*y)*f(2*z)*f(z + y)*f(a + y + x)*f(b + z + y) +
3*f(2*y)*f(2*
> z)*f(z + y)*f(a + 2*y)*f(a + z + y) - f(2*y)*f(2*z)*f(z
+ x)*f(c + 2*
> y)*f(b + y + x) + f(2*y)*f(2*z)*f(z + x)*f(b + 2*y)*f(c
+ y + x) + f(
> 2*y)*f(2*z)*f(z + x)*f(b + 2*y)*f(a + z + y) - f(2*y)*f
(2*z)*f(z + x)
> *f(a + 2*y)*f(b + z + y) - f(2*y)*f(2*z)^2*f(b + 2*y)*f
(a + y + x) +

```

```

> f(2*y)*f(2*z)^2*f(a + 2*y)*f(b + y + x) - f(2*y)*f(2*z)*
f(y + x)*f(c
> + 2*y)*f(b + z + x) - f(2*y)*f(2*z)*f(y + x)*f(c + 2*y)
*f(a + z + y)
> - 2*f(2*y)*f(2*z)*f(y + x)*f(b + z + x)*f(b + z + y) -
2*f(2*y)*f(2*
> z)*f(y + x)*f(b + y + x)*f(c + z + y) + f(2*y)*f(2*z)*f
(y + x)*f(b +
> 2*y)*f(c + z + x) + 2*f(2*y)*f(2*z)*f(y + x)*f(a + z +
y)*f(b + z + y
> ) + f(2*y)*f(2*z)*f(y + x)*f(a + 2*z)*f(b + 2*y) - f(2*
y)*f(2*z)*f(y
> + x)*f(a + 2*y)*f(c + z + y) - f(2*y)*f(2*z)*f(y + x)*f
(a + 2*y)*f(b
> + 2*z) + 4*f(2*y)*f(y + x)*f(z + y)*f(b + z + y)*f(c +
z + x) + f(2*
> y)*f(y + x)*f(z + y)*f(a + 2*z)*f(c + 2*y) - f(2*y)*f(y
+ x)*f(z + y)
> *f(a + 2*y)*f(c + 2*z) + 2*f(2*y)*f(y + x)*f(z + x)*f(c
+ 2*y)*f(c +
> z + y) + 2*f(2*y)*f(y + x)*f(z + x)*f(b + 2*z)*f(c + 2*
y) + 2*f(2*y)*
> f(y + x)*f(z + x)*f(b + 2*z)*f(b + z + y) - 2*f(2*y)*f(y
+ x)*f(z + x
> )*f(b + 2*y)*f(c + 2*z) - 2*f(2*y)*f(y + x)^2*f(c + 2*z)
*f(b + z + y)
> + f(2*y)^2*f(z + y)*f(c + 2*x)*f(c + z + y) + 1/2*f(2*
y)^2*f(z + y)*
> f(b + 2*z)*f(c + 2*x) - 1/2*f(2*y)^2*f(z + y)*f(b + 2*x)
*f(c + 2*z)
> - 2*f(2*y)^2*f(z + y)*f(a + z + y)*f(c + z + x) + f(2*
y)^2*f(z + y)*
> f(a + 2*z)*f(a + z + y) + f(2*y)^2*f(z + x)*f(c + 2*z)*f
(b + y + x)
> - 2*f(2*y)^2*f(z + x)*f(c + y + x)*f(c + z + y) - 2*f
(2*y)^2*f(z + x
> )*f(b + z + y)*f(c + z + x) - f(2*y)^2*f(z + x)*f(b + 2*
z)*f(c + y +
> x) - f(2*y)^2*f(z + x)*f(b + 2*z)*f(a + z + y) + 2*f(2*
y)^2*f(z + x)*
> f(a + z + y)*f(c + z + y) - f(2*y)^2*f(z + x)*f(a + 2*z)
*f(c + 2*y)
> - f(2*y)^2*f(z + x)*f(a + 2*z)*f(b + z + y) + f(2*y)^2*
f(z + x)*f(a
> + 2*y)*f(c + 2*z) + f(2*y)^2*f(2*z)*f(c + 2*y)*f(a + z
+ x) + f(2*y)
> ^2*f(2*z)*f(b + 2*z)*f(a + y + x) - 2*f(2*y)^2*f(2*z)*f
(a + z + y)^2
> + 2*f(2*y)^2*f(2*z)*f(a + z + x)*f(b + z + y) - f(2*y)
^2*f(2*z)*f(a
> + 2*z)*f(b + y + x) + 2*f(2*y)^2*f(2*z)*f(a + y + x)*f
(c + z + y) -
> f(2*y)^2*f(2*z)*f(a + 2*y)*f(c + z + x) + f(2*y)^2*f(y +
x)*f(c + 2*z
> )*f(b + z + x) + f(2*y)^2*f(y + x)*f(c + 2*z)*f(a + z +
y) - f(2*y)^2
> *f(y + x)*f(b + 2*z)*f(c + z + x) - f(2*y)^2*f(y + x)*f

```

```

(a + 2*z)*f(c
> + z + y) - f(2*y)^3*f(c + 2*z)*f(a + z + x) + f(2*y)^3*
f(a + 2*z)*f(
> c + z + x) + f(2*x)*f(z + y)^2*f(c + 2*y)^2 + 2*f(2*x)*f
(z + y)^2*f(c
> + 2*y)*f(b + z + y) + f(2*x)*f(z + y)^2*f(b + 2*y)*f(b
+ 2*z) - 2*f(
> 2*x)*f(2*z)*f(z + y)*f(b + 2*y)*f(c + 2*y) - f(2*x)*f(2*
y)*f(z + y)*
> f(c + 2*y)*f(c + z + y) - 2*f(2*x)*f(2*y)*f(z + y)*f(b +
z + y)*f(c
> + z + y) - 3/2*f(2*x)*f(2*y)*f(z + y)*f(b + 2*z)*f(c +
2*y) - f(2*x)
> *f(2*y)*f(z + y)*f(b + 2*z)*f(b + z + y) - 1/2*f(2*x)*f
(2*y)*f(z + y)
> *f(b + 2*y)*f(c + 2*z) + f(2*x)*f(2*y)*f(2*z)*f(c + 2*y)
*f(b + z + y)
> + f(2*x)*f(2*y)*f(2*z)*f(b + 2*y)*f(c + z + y) + f(2*x)
*f(2*y)^2*f(c
> + 2*z)*f(b + z + y) + f(2*x)*f(2*y)^2*f(b + 2*z)*f(c +
z + y) )
>
+ 2*f(z + y)*f(c + b + 2*y) - 2*f(2*y)*f(c + b + z + y):
> eq[22] :=
> (1/HessUniv) * ( 2*f(z + y)^3*f(a + 2*y)*f(c + 2*x) - 4*f(z + x)*
f(z
> + y)^2*f(a + 2*y)*f(c + y + x) + 2*f(z + x)^2*f(z + y)*
f(a + 2*y)*f(
> c + 2*y) - f(2*z)*f(z + y)^2*f(a + 2*y)*f(b + 2*x) + f
(2*z)*f(z + y)^
> 2*f(a + 2*x)*f(b + 2*y) + 2*f(2*z)*f(z + x)*f(z + y)*f(b
+ 2*y)*f(a
> + y + x) - f(2*z)*f(z + x)*f(z + y)*f(b + 2*x)*f(b + 2*
y) - f(2*z)*
> f(z + x)*f(z + y)*f(a + 2*y)^2 + f(2*z)*f(y + x)*f(z +
y)*f(b + 2*y)*
> f(c + 2*x) - 2*f(2*z)*f(y + x)*f(z + y)*f(b + 2*y)*f(a +
z + x) + f(2
> *z)*f(y + x)*f(z + y)*f(b + 2*x)*f(c + 2*y) + 2*f(2*z)*f
(y + x)*f(z
> + y)*f(a + 2*y)*f(c + y + x) + 2*f(2*z)*f(y + x)*f(z +
y)*f(a + 2*y)
> *f(a + z + y) - 2*f(y + x)*f(z + y)^2*f(c + 2*x)*f(c +
2*y) - 2*f(y
> + x)*f(z + y)^2*f(a + 2*y)*f(a + 2*z) - 4*f(y + x)*f(z
+ x)*f(z + y)
> *f(c + 2*y)*f(a + z + y) + 2*f(y + x)^2*f(z + y)*f(a +
2*z)*f(c + 2*y
> ) - 2*f(2*y)*f(z + y)^2*f(c + 2*x)*f(a + z + y) + f(2*y)
*f(z + x)*f(z
> + y)*f(c + 2*x)*f(c + 2*y) + 4*f(2*y)*f(z + x)*f(z + y)
*f(a + z + y)
> *f(c + y + x) + 2*f(2*y)*f(z + x)*f(z + y)*f(a + 2*y)*f
(c + z + x) +
> f(2*y)*f(z + x)*f(z + y)*f(a + 2*y)*f(a + 2*z) - 2*f(2*
y)*f(z + x)^2*

```

```

>      f(a + 2*y)*f(c + z + y) + f(2*y)*f(2*z)*f(z + y)*f(b +
>      2*x)*f(a + z
>      + y) - 3/2*f(2*y)*f(2*z)*f(z + y)*f(a + 2*y)*f(c + 2*x)
>      - 1/2*f(2*y)
>      *f(2*z)*f(z + y)*f(a + 2*x)*f(c + 2*y) - f(2*y)*f(2*z)*f
>      (z + y)*f(a
>      + 2*x)*f(b + z + y) - f(2*y)*f(2*z)*f(z + x)*f(c + 2*y)
>      *f(a + y + x)
>      + f(2*y)*f(2*z)*f(z + x)*f(b + 2*x)*f(b + z + y) - 2*f
>      (2*y)*f(2*z)*
>      f(z + x)*f(a + y + x)*f(b + z + y) + f(2*y)*f(2*z)*f(z +
>      x)*f(a + 2*y
>      )*f(c + y + x) + f(2*y)*f(2*z)*f(z + x)*f(a + 2*y)*f(a +
>      z + y) + 1/2
>      *f(2*y)*f(2*z)^2*f(a + 2*y)*f(b + 2*x) - 1/2*f(2*y)*f(2*
>      z)^2*f(a + 2*
>      x)*f(b + 2*y) + f(2*y)*f(2*z)*f(y + x)*f(c + 2*y)*f(a +
>      z + x) - f(2*
>      y)*f(2*z)*f(y + x)*f(c + 2*x)*f(b + z + y) - f(2*y)*f(2*
>      z)*f(y + x)*
>      f(b + 2*x)*f(c + z + y) - 2*f(2*y)*f(2*z)*f(y + x)*f(a +
>      z + y)*f(c
>      + y + x) - 2*f(2*y)*f(2*z)*f(y + x)*f(a + z + y)^2 + 2*
>      f(2*y)*f(2*z)
>      *f(y + x)*f(a + z + x)*f(b + z + y) - f(2*y)*f(2*z)*f(y
>      + x)*f(a + 2*
>      y)*f(c + z + x) + 2*f(2*y)*f(y + x)*f(z + y)*f(c + 2*x)*
>      f(c + z + y)
>      + 2*f(2*y)*f(y + x)*f(z + y)*f(a + 2*z)*f(a + z + y) +
>      4*f(2*y)*f(y
>      + x)*f(z + x)*f(a + z + y)*f(c + z + y) - 2*f(2*y)*f(y
>      + x)^2*f(a +
>      2*z)*f(c + z + y) + 1/2*f(2*y)^2*f(z + y)*f(a + 2*z)*f(c
>      + 2*x) - 1/2
>      *f(2*y)^2*f(z + y)*f(a + 2*x)*f(c + 2*z) + f(2*y)^2*f(z
>      + x)*f(c + 2*
>      z)*f(a + y + x) - f(2*y)^2*f(z + x)*f(c + 2*x)*f(c + z +
>      y) - 2*f(2*y
>      )^2*f(z + x)*f(a + z + y)*f(c + z + x) - f(2*y)^2*f(z +
>      x)*f(a + 2*z)
>      *f(c + y + x) - f(2*y)^2*f(z + x)*f(a + 2*z)*f(a + z +
>      y) + f(2*y)^2*
>      f(2*z)*f(c + 2*x)*f(a + z + y) - 1/2*f(2*y)^2*f(2*z)*f(a
>      + 2*z)*f(b
>      + 2*x) + f(2*y)^2*f(2*z)*f(a + 2*x)*f(c + z + y) + 1/2*
>      f(2*y)^2*f(2*
>      z)*f(a + 2*x)*f(b + 2*z) - f(2*y)^2*f(y + x)*f(c + 2*z)*
>      f(a + z + x)
>      + f(2*y)^2*f(y + x)*f(a + 2*z)*f(c + z + x) + 2*f(2*x)*
>      f(z + y)^2*f(
>      c + 2*y)*f(c + y + x) + 2*f(2*x)*f(z + y)^2*f(c + 2*y)*f
>      (a + z + y)
>      - 2*f(2*x)*f(z + y)^2*f(b + 2*y)*f(c + z + x) + f(2*x)*
>      f(z + y)^2*f(
>      a + 2*z)*f(b + 2*y) + f(2*x)*f(z + y)^2*f(a + 2*y)*f(b +
>      2*z) - f(2*x
>      )*f(z + x)*f(z + y)*f(c + 2*y)^2 + 2*f(2*x)*f(z + x)*f(z

```

```

+ y)*f(b + 2
>      *y)*f(c + z + y) - f(2*x)*f(z + x)*f(z + y)*f(b + 2*y)*f
(b + 2*z) - 2
>      *f(2*x)*f(2*z)*f(z + y)*f(b + 2*y)*f(c + y + x) + 2*f(2*
x)*f(2*z)*f(z
>      + y)*f(b + 2*y)*f(b + z + x) - 2*f(2*x)*f(2*z)*f(z + y)
*f(b + 2*y)*
>      f(a + z + y) - f(2*x)*f(y + x)*f(z + y)*f(b + 2*z)*f(c +
2*y) + f(2*x
>      )*f(y + x)*f(z + y)*f(b + 2*y)*f(c + 2*z) - 2*f(2*x)*f
(2*y)*f(z + y)*
>      f(c + y + x)*f(c + z + y) + 2*f(2*x)*f(2*y)*f(z + y)*f(b
+ z + y)*f(c
>      + z + x) - f(2*x)*f(2*y)*f(z + y)*f(b + 2*z)*f(a + z +
y) - 2*f(2*x)
>      *f(2*y)*f(z + y)*f(a + z + y)*f(c + z + y) - 3/2*f(2*x)*
f(2*y)*f(z +
>      y)*f(a + 2*z)*f(c + 2*y) - f(2*x)*f(2*y)*f(z + y)*f(a +
2*z)*f(b + z
>      + y) - 1/2*f(2*x)*f(2*y)*f(z + y)*f(a + 2*y)*f(c + 2*z)
+ f(2*x)*f(2
>      *y)*f(z + x)*f(c + 2*y)*f(c + z + y) - 2*f(2*x)*f(2*y)*f
(z + x)*f(b
>      + z + y)*f(c + z + y) + f(2*x)*f(2*y)*f(z + x)*f(b + 2*
z)*f(c + 2*y)
>      + f(2*x)*f(2*y)*f(z + x)*f(b + 2*z)*f(b + z + y) - f(2*
x)*f(2*y)*f(z
>      + x)*f(b + 2*y)*f(c + 2*z) - f(2*x)*f(2*y)*f(2*z)*f(c +
2*y)*f(b + z
>      + x) + 2*f(2*x)*f(2*y)*f(2*z)*f(b + z + y)*f(c + y + x)
- 2*f(2*x)*
>      f(2*y)*f(2*z)*f(b + z + x)*f(b + z + y) + f(2*x)*f(2*y)*
f(2*z)*f(b +
>      2*y)*f(c + z + x) + 2*f(2*x)*f(2*y)*f(2*z)*f(a + z + y)*
f(b + z + y)
>      + 1/2*f(2*x)*f(2*y)*f(2*z)*f(a + 2*z)*f(b + 2*y) - 1/2*
f(2*x)*f(2*y)
>      *f(2*z)*f(a + 2*y)*f(b + 2*z) - f(2*x)*f(2*y)*f(y + x)*f
(c + 2*z)*f(b
>      + z + y) + f(2*x)*f(2*y)*f(y + x)*f(b + 2*z)*f(c + z +
y) + f(2*x)*
>      f(2*y)^2*f(c + 2*z)*f(b + z + x) + f(2*x)*f(2*y)^2*f(c +
2*z)*f(a + z
>      + y) - f(2*x)*f(2*y)^2*f(b + 2*z)*f(c + z + x) + f(2*x)
*f(2*y)^2*f(a
>      + 2*z)*f(c + z + y) )
>
>      + 2*f(z + y)*f(c + a + 2*y) - 2*f(2*y)*f(c + a + z + y):
>
> eq[23] :=
> (1/HessUniv) * ( 2*f(z + x)*f(z + y)^2*f(b + 2*y)*f(c + 2*x) - 4*
f(z
>      + x)^2*f(z + y)*f(b + 2*y)*f(c + y + x) + 2*f(z + x)^3*
f(b + 2*y)*f(
>      c + 2*y) + 4*f(2*z)*f(z + x)*f(z + y)*f(b + 2*y)*f(a + y
+ x) - f(2*z
>      )*f(z + x)*f(z + y)*f(b + 2*x)*f(b + 2*y) - 2*f(2*z)*f(z

```



```

+ x)*f(z + y
> )*f(a + 2*y)*f(b + y + x) - f(2*z)*f(z + x)*f(z + y)*f(a
+ 2*y)^2 + 2
> *f(2*z)*f(y + x)*f(z + x)*f(c + 2*y)*f(b + y + x) + 2*f
(2*z)*f(y + x)
> *f(z + x)*f(b + 2*y)*f(b + z + x) - 4*f(2*z)*f(y + x)*f
(z + x)*f(b +
> 2*y)*f(a + z + y) + 2*f(2*z)*f(y + x)*f(z + x)*f(a + 2*
y)*f(c + 2*y)
> + 2*f(2*z)*f(y + x)*f(z + x)*f(a + 2*y)*f(b + z + y) -
4*f(y + x)*f(
> z + x)*f(z + y)*f(b + 2*y)*f(c + z + x) - 2*f(y + x)*f(z
+ x)^2*f(c
> + 2*y)^2 - 4*f(y + x)*f(z + x)^2*f(c + 2*y)*f(b + z +
y) + 4*f(y + x
> )*f(z + x)^2*f(b + 2*y)*f(c + z + y) - 2*f(y + x)*f(z +
x)^2*f(b + 2*
> y)*f(b + 2*z) + 2*f(y + x)^2*f(z + x)*f(b + 2*y)*f(c +
2*z) - 2*f(2*y
> )*f(z + y)^2*f(b + 2*x)*f(c + z + x) - f(2*y)*f(z + x)*f
(z + y)*f(c
> + 2*x)*f(c + 2*y) - 2*f(2*y)*f(z + x)*f(z + y)*f(c + 2*
x)*f(b + z +
> y) + 4*f(2*y)*f(z + x)*f(z + y)*f(b + y + x)*f(c + z +
x) + 2*f(2*y)*
> f(z + x)*f(z + y)*f(b + 2*x)*f(c + z + y) + 2*f(2*y)*f(z
+ x)*f(z + y
> )*f(a + 2*y)*f(c + z + x) - f(2*y)*f(z + x)*f(z + y)*f(a
+ 2*y)*f(a
> + 2*z) + 2*f(2*y)*f(z + x)^2*f(c + 2*y)*f(c + y + x) +
4*f(2*y)*f(z
> + x)^2*f(b + z + y)*f(c + y + x) - 4*f(2*y)*f(z + x)^2*
f(b + y + x)*
> f(c + z + y) + f(2*y)*f(z + x)^2*f(a + 2*z)*f(b + 2*y) -
2*f(2*y)*f(z
> + x)^2*f(a + 2*y)*f(c + z + y) + f(2*y)*f(z + x)^2*f(a
+ 2*y)*f(b +
> 2*z) - f(2*y)*f(2*z)*f(z + y)*f(c + 2*x)*f(b + y + x) +
f(2*y)*f(2*z)
> *f(z + y)*f(b + 2*x)*f(c + y + x) + f(2*y)*f(2*z)*f(z +
y)*f(b + 2*x)
> *f(b + z + x) - 2*f(2*y)*f(2*z)*f(z + y)*f(a + z + x)*f
(b + y + x) +
> f(2*y)*f(2*z)*f(z + y)*f(a + 2*y)*f(a + z + x) - 2*f(2*
y)*f(2*z)*f(z
> + x)*f(c + 2*y)*f(a + y + x) + 1/2*f(2*y)*f(2*z)*f(z +
x)*f(b + 2*y)
> *f(c + 2*x) - f(2*y)*f(2*z)*f(z + x)*f(b + 2*y)*f(a + z
+ x) - 1/2*f(
> 2*y)*f(2*z)*f(z + x)*f(b + 2*x)*f(c + 2*y) + 4*f(2*y)*f
(2*z)*f(z + x)
> *f(a + z + y)*f(b + y + x) - 4*f(2*y)*f(2*z)*f(z + x)*f
(a + y + x)*f(
> b + z + y) - f(2*y)*f(2*z)*f(z + x)*f(a + 2*y)*f(b + z +
x) + 2*f(2*y
> )*f(2*z)*f(z + x)*f(a + 2*y)*f(a + z + y) + 1/2*f(2*y)*f
(2*z)^2*f(a

```

```

> + 2*y)*f(b + 2*x) - 1/2*f(2*y)*f(2*z)^2*f(a + 2*x)*f(b
+ 2*y) - f(2*
> y)*f(2*z)*f(y + x)*f(c + 2*y)*f(a + z + x) + f(2*y)*f(2*
z)*f(y + x)*
> f(c + 2*x)*f(b + z + y) - 2*f(2*y)*f(2*z)*f(y + x)*f(b +
z + x)*f(c
> + y + x) - 2*f(2*y)*f(2*z)*f(y + x)*f(b + z + x)^2 - f
(2*y)*f(2*z)*
> f(y + x)*f(b + 2*x)*f(c + z + y) + 2*f(2*y)*f(2*z)*f(y +
x)*f(a + z
> + x)*f(b + z + y) - f(2*y)*f(2*z)*f(y + x)*f(a + 2*y)*f
(c + z + x)
> + 4*f(2*y)*f(y + x)*f(z + y)*f(b + z + x)*f(c + z + x)
- 2*f(2*y)*f(
> y + x)*f(z + x)*f(c + 2*z)*f(b + y + x) + 2*f(2*y)*f(y +
x)*f(z + x)*
> f(c + 2*y)*f(c + z + x) + 2*f(2*y)*f(y + x)*f(z + x)*f(b
+ 2*z)*f(c
> + y + x) + 2*f(2*y)*f(y + x)*f(z + x)*f(b + 2*z)*f(b +
z + x) + f(2*
> y)*f(y + x)*f(z + x)*f(a + 2*z)*f(c + 2*y) - f(2*y)*f(y
+ x)*f(z + x)
> *f(a + 2*y)*f(c + 2*z) - 2*f(2*y)*f(y + x)^2*f(b + 2*z)*
f(c + z + x)
> + f(2*y)^2*f(z + y)*f(c + 2*x)*f(c + z + x) - 2*f(2*y)
^2*f(z + y)*f(
> a + z + x)*f(c + z + x) + f(2*y)^2*f(z + y)*f(a + 2*z)*f
(c + 2*x) +
> f(2*y)^2*f(z + y)*f(a + 2*z)*f(a + z + x) - f(2*y)^2*f(z
+ y)*f(a + 2
> *x)*f(c + 2*z) + 2*f(2*y)^2*f(z + x)*f(c + 2*z)*f(a + y
+ x) - 2*f(2*
> y)^2*f(z + x)*f(c + y + x)*f(c + z + x) - 2*f(2*y)^2*f(z
+ x)*f(b + z
> + x)*f(c + z + x) - 1/2*f(2*y)^2*f(z + x)*f(b + 2*z)*f
(c + 2*x) - f(
> 2*y)^2*f(z + x)*f(b + 2*z)*f(a + z + x) + 1/2*f(2*y)^2*f
(z + x)*f(b
> + 2*x)*f(c + 2*z) + 2*f(2*y)^2*f(z + x)*f(a + z + x)*f
(c + z + y) -
> 2*f(2*y)^2*f(z + x)*f(a + 2*z)*f(c + y + x) - f(2*y)^2*f
(z + x)*f(a
> + 2*z)*f(b + z + x) - f(2*y)^2*f(2*z)*f(c + 2*x)*f(a +
z + y) + 2*f(
> 2*y)^2*f(2*z)*f(a + z + x)*f(c + y + x) + 2*f(2*y)^2*f
(2*z)*f(a + z
> + x)*f(b + z + x) - 2*f(2*y)^2*f(2*z)*f(a + z + x)*f(a
+ z + y) - 1/
> 2*f(2*y)^2*f(2*z)*f(a + 2*z)*f(b + 2*x) + f(2*y)^2*f(2*
z)*f(a + 2*x)*
> f(c + z + y) + 1/2*f(2*y)^2*f(2*z)*f(a + 2*x)*f(b + 2*z)
- f(2*y)^2*
> f(y + x)*f(c + 2*z)*f(a + z + x) + f(2*y)^2*f(y + x)*f(a
+ 2*z)*f(c
> + z + x) + f(2*x)*f(z + x)*f(z + y)*f(c + 2*y)^2 + 2*f
(2*x)*f(z + x)
> *f(z + y)*f(c + 2*y)*f(b + z + y) + f(2*x)*f(z + x)*f(z

```

```

+ y)*f(b + 2*
> y)*f(b + 2*z) - 2*f(2*x)*f(2*z)*f(z + x)*f(b + 2*y)*f(c
+ 2*y) + f(2*
> x)*f(2*y)*f(z + y)*f(c + 2*z)*f(b + y + x) - f(2*x)*f(2*
y)*f(z + y)*
> f(c + 2*y)*f(c + z + x) - 2*f(2*x)*f(2*y)*f(z + y)*f(b +
z + x)*f(c
> + z + y) - f(2*x)*f(2*y)*f(z + y)*f(b + 2*z)*f(c + y +
x) - f(2*x)*
> f(2*y)*f(z + y)*f(b + 2*z)*f(b + z + x) - 1/2*f(2*x)*f
(2*y)*f(z + x)*
> f(b + 2*z)*f(c + 2*y) - 3/2*f(2*x)*f(2*y)*f(z + x)*f(b +
2*y)*f(c + 2
> *z) + f(2*x)*f(2*y)*f(2*z)*f(c + 2*y)*f(b + z + x) + f
(2*x)*f(2*y)*f(
> 2*z)*f(b + 2*y)*f(c + z + x) + 1/2*f(2*x)*f(2*y)*f(2*z)*
f(a + 2*z)*f(
> b + 2*y) - 1/2*f(2*x)*f(2*y)*f(2*z)*f(a + 2*y)*f(b + 2*
z) - f(2*x)*f(
> 2*y)*f(y + x)*f(c + 2*z)*f(b + z + y) + f(2*x)*f(2*y)*f
(y + x)*f(b +
> 2*z)*f(c + z + y) + f(2*x)*f(2*y)^2*f(c + 2*z)*f(b + z +
x) + f(2*x)*
> f(2*y)^2*f(c + 2*z)*f(a + z + y) + f(2*x)*f(2*y)^2*f(b +
2*z)*f(c + z
> + x) - f(2*x)*f(2*y)^2*f(a + 2*z)*f(c + z + y) )
>
> + 2*f(z + x)*f(c + b + 2*y) - 2*f(2*y)*f(c + b + z + x):
>
> eq[24] :=
> (1/HessUniv) * ( 2*f(z + x)*f(z + y)^2*f(a + 2*y)*f(c + 2*x) - 4*
f(z
> + x)^2*f(z + y)*f(a + 2*y)*f(c + y + x) + 2*f(z + x)^3*
f(a + 2*y)*f(
> c + 2*y) - f(2*z)*f(z + x)*f(z + y)*f(a + 2*y)*f(b + 2*
x) + f(2*z)*f(
> z + x)*f(z + y)*f(a + 2*x)*f(b + 2*y) + 2*f(2*z)*f(z +
x)^2*f(b + 2*y
> )*f(a + y + x) - f(2*z)*f(z + x)^2*f(b + 2*x)*f(b + 2*y)
- f(2*z)*f(z
> + x)^2*f(a + 2*y)^2 + f(2*z)*f(y + x)*f(z + x)*f(b + 2*
y)*f(c + 2*x)
> - 2*f(2*z)*f(y + x)*f(z + x)*f(b + 2*y)*f(a + z + x) +
f(2*z)*f(y +
> x)*f(z + x)*f(b + 2*x)*f(c + 2*y) + 2*f(2*z)*f(y + x)*f
(z + x)*f(a +
> 2*y)*f(c + y + x) + 2*f(2*z)*f(y + x)*f(z + x)*f(a + 2*
y)*f(a + z + y
> ) - 2*f(y + x)*f(z + x)*f(z + y)*f(c + 2*x)*f(c + 2*y) -
2*f(y + x)*
> f(z + x)*f(z + y)*f(a + 2*y)*f(a + 2*z) - 4*f(y + x)*f(z
+ x)^2*f(c
> + 2*y)*f(a + z + y) + 2*f(y + x)^2*f(z + x)*f(a + 2*z)*
f(c + 2*y) -
> 2*f(2*y)*f(z + y)^2*f(a + 2*x)*f(c + z + x) - 2*f(2*y)*f
(z + x)*f(z
> + y)*f(c + 2*x)*f(a + z + y) + 4*f(2*y)*f(z + x)*f(z +

```

```

y)*f(a + y +
> x)*f(c + z + x) + 2*f(2*y)*f(z + x)*f(z + y)*f(a + 2*x)*
f(c + z + y)
> + f(2*y)*f(z + x)^2*f(c + 2*x)*f(c + 2*y) + 4*f(2*y)*f
(z + x)^2*f(a
> + z + y)*f(c + y + x) - 4*f(2*y)*f(z + x)^2*f(a + y +
x)*f(c + z + y
> ) + f(2*y)*f(z + x)^2*f(a + 2*y)*f(a + 2*z) - f(2*y)*f
(2*z)*f(z + y)*
> f(c + 2*x)*f(a + y + x) - f(2*y)*f(2*z)*f(z + y)*f(b +
2*x)*f(a + z
> + x) + f(2*y)*f(2*z)*f(z + y)*f(a + 2*x)*f(c + y + x) +
f(2*y)*f(2*z
> )*f(z + y)*f(a + 2*x)*f(b + z + x) + f(2*y)*f(2*z)*f(z +
x)*f(b + 2*x
> )*f(b + z + x) + 2*f(2*y)*f(2*z)*f(z + x)*f(b + 2*x)*f(a
+ z + y) - 2
> *f(2*y)*f(2*z)*f(z + x)*f(a + y + x)*f(b + z + x) - 1/2*
f(2*y)*f(2*z)
> *f(z + x)*f(a + 2*y)*f(c + 2*x) + f(2*y)*f(2*z)*f(z + x)
*f(a + 2*y)*
> f(a + z + x) - 3/2*f(2*y)*f(2*z)*f(z + x)*f(a + 2*x)*f(c
+ 2*y) - 2*
> f(2*y)*f(2*z)*f(z + x)*f(a + 2*x)*f(b + z + y) + f(2*y)*
f(2*z)^2*f(b
> + 2*x)*f(a + y + x) - f(2*y)*f(2*z)^2*f(a + 2*x)*f(b +
y + x) - f(2*
> y)*f(2*z)*f(y + x)*f(c + 2*x)*f(b + z + x) - f(2*y)*f(2*
z)*f(y + x)*
> f(c + 2*x)*f(a + z + y) - f(2*y)*f(2*z)*f(y + x)*f(b +
2*x)*f(c + z
> + x) + 2*f(2*y)*f(2*z)*f(y + x)*f(a + z + x)*f(b + z +
x) - 2*f(2*y)
> *f(2*z)*f(y + x)*f(a + z + x)*f(a + z + y) - f(2*y)*f(2*
z)*f(y + x)*
> f(a + 2*z)*f(b + 2*x) - 2*f(2*y)*f(2*z)*f(y + x)*f(a + y
+ x)*f(c + z
> + x) + f(2*y)*f(2*z)*f(y + x)*f(a + 2*x)*f(c + z + y) +
f(2*y)*f(2*z
> )*f(y + x)*f(a + 2*x)*f(b + 2*z) + 2*f(2*y)*f(y + x)*f(z
+ y)*f(c + 2
> *x)*f(c + z + x) + 2*f(2*y)*f(y + x)*f(z + y)*f(a + 2*z)
*f(c + 2*x)
> + 2*f(2*y)*f(y + x)*f(z + y)*f(a + 2*z)*f(a + z + x) -
2*f(2*y)*f(y
> + x)*f(z + y)*f(a + 2*x)*f(c + 2*z) + 2*f(2*y)*f(y + x)
*f(z + x)*f(c
> + 2*z)*f(a + y + x) + 4*f(2*y)*f(y + x)*f(z + x)*f(a +
z + x)*f(c +
> z + y) - 2*f(2*y)*f(y + x)*f(z + x)*f(a + 2*z)*f(c + y +
x) - 2*f(2*y
> )*f(y + x)^2*f(c + 2*z)*f(a + z + x) - f(2*y)^2*f(z + x)
*f(c + 2*x)*
> f(c + z + x) - 2*f(2*y)^2*f(z + x)*f(a + z + x)*f(c + z
+ x) - 1/2*f(
> 2*y)^2*f(z + x)*f(a + 2*z)*f(c + 2*x) - f(2*y)^2*f(z +
x)*f(a + 2*z)*

```

```

>      f(a + z + x) + 1/2*f(2*y)^2*f(z + x)*f(a + 2*x)*f(c + 2*
>      z) + f(2*y)^2
>      *f(2*z)*f(c + 2*x)*f(a + z + x) + f(2*y)^2*f(2*z)*f(a +
>      2*x)*f(c + z
>      + x) + 2*f(2*x)*f(z + x)*f(z + y)*f(c + 2*y)*f(c + y +
>      x) + 2*f(2*x)
>      *f(z + x)*f(z + y)*f(c + 2*y)*f(a + z + y) - 2*f(2*x)*f
>      (z + x)*f(z +
>      y)*f(b + 2*y)*f(c + z + x) + f(2*x)*f(z + x)*f(z + y)*f
>      (a + 2*z)*f(b
>      + 2*y) + f(2*x)*f(z + x)*f(z + y)*f(a + 2*y)*f(b + 2*z)
>      - f(2*x)*f(z
>      + x)^2*f(c + 2*y)^2 + 2*f(2*x)*f(z + x)^2*f(b + 2*y)*f
>      (c + z + y) -
>      f(2*x)*f(z + x)^2*f(b + 2*y)*f(b + 2*z) - 2*f(2*x)*f(2*
>      z)*f(z + x)*f(
>      b + 2*y)*f(c + y + x) + 2*f(2*x)*f(2*z)*f(z + x)*f(b +
>      2*y)*f(b + z
>      + x) - 2*f(2*x)*f(2*z)*f(z + x)*f(b + 2*y)*f(a + z + y)
>      - f(2*x)*f(y
>      + x)*f(z + x)*f(b + 2*z)*f(c + 2*y) + f(2*x)*f(y + x)*f
>      (z + x)*f(b
>      + 2*y)*f(c + 2*z) + f(2*x)*f(2*y)*f(z + y)*f(c + 2*z)*f
>      (a + y + x)
>      - 2*f(2*x)*f(2*y)*f(z + y)*f(c + y + x)*f(c + z + x) +
>      2*f(2*x)*f(2*
>      y)*f(z + y)*f(b + z + x)*f(c + z + x) - f(2*x)*f(2*y)*f
>      (z + y)*f(b +
>      2*z)*f(c + 2*x) - f(2*x)*f(2*y)*f(z + y)*f(b + 2*z)*f(a
>      + z + x) + f(
>      2*x)*f(2*y)*f(z + y)*f(b + 2*x)*f(c + 2*z) - 2*f(2*x)*f
>      (2*y)*f(z + y)
>      *f(a + z + x)*f(c + z + y) - f(2*x)*f(2*y)*f(z + y)*f(a
>      + 2*z)*f(c +
>      y + x) - f(2*x)*f(2*y)*f(z + y)*f(a + 2*z)*f(b + z + x)
>      - 2*f(2*x)*f(
>      2*y)*f(z + x)*f(c + 2*z)*f(b + y + x) + f(2*x)*f(2*y)*f
>      (z + x)*f(c +
>      2*y)*f(c + z + x) - 2*f(2*x)*f(2*y)*f(z + x)*f(b + z +
>      x)*f(c + z + y
>      ) + 2*f(2*x)*f(2*y)*f(z + x)*f(b + 2*z)*f(c + y + x) + f
>      (2*x)*f(2*y)*
>      f(z + x)*f(b + 2*z)*f(b + z + x) - 1/2*f(2*x)*f(2*y)*f(z
>      + x)*f(a + 2
>      *z)*f(c + 2*y) - 3/2*f(2*x)*f(2*y)*f(z + x)*f(a + 2*y)*f
>      (c + 2*z) +
>      f(2*x)*f(2*y)*f(2*z)*f(c + 2*x)*f(b + z + y) - 2*f(2*x)*
>      f(2*y)*f(2*z)
>      *f(b + z + x)^2 - f(2*x)*f(2*y)*f(2*z)*f(b + 2*z)*f(a +
>      y + x) + 2*f(
>      2*x)*f(2*y)*f(2*z)*f(b + y + x)*f(c + z + x) - f(2*x)*f
>      (2*y)*f(2*z)*
>      f(b + 2*x)*f(c + z + y) + 2*f(2*x)*f(2*y)*f(2*z)*f(a + z
>      + x)*f(b + z
>      + y) + f(2*x)*f(2*y)*f(2*z)*f(a + 2*z)*f(b + y + x) + f
>      (2*x)*f(2*y)*
>      f(y + x)*f(c + 2*z)*f(b + z + x) + f(2*x)*f(2*y)*f(y +

```

```

x)*f(c + 2*z)*
>      f(a + z + y) - f(2*x)*f(2*y)*f(y + x)*f(b + 2*z)*f(c + z
+ x) - f(2*x
>      )*f(2*y)*f(y + x)*f(a + 2*z)*f(c + z + y) + f(2*x)*f(2*
y)^2*f(c + 2*z
>      )*f(a + z + x) + f(2*x)*f(2*y)^2*f(a + 2*z)*f(c + z + x)
>      - f(2*x)^2*
>      f(2*y)*f(c + 2*z)*f(b + z + y) + f(2*x)^2*f(2*y)*f(b +
2*z)*f(c + z
>      + y) )
>
>      + 2*f(z + x)*f(c + a + 2*y) - 2*f(2*y)*f(c + a + z + x):
>
> eq[25] :=
> (1/HessUniv) * ( 8*f(y + x)*f(z + y)^2*f(b + 2*y)*f(a + y + x) -
4*f(
>      y + x)*f(z + y)^2*f(a + 2*y)*f(b + y + x) - 2*f(y + x)*f
(z + y)^2*f(a
>      + 2*y)^2 + 4*f(y + x)*f(z + x)*f(z + y)*f(b + 2*y)*f(b
+ y + x) + 2*
>      f(y + x)*f(z + x)^2*f(b + 2*y)^2 + 4*f(y + x)^2*f(z + y)
*f(c + 2*y)*
>      f(b + y + x) - 8*f(y + x)^2*f(z + y)*f(b + 2*y)*f(c + y
+ x) - 8*f(y
>      + x)^2*f(z + y)*f(b + 2*y)*f(a + z + y) + 4*f(y + x)^2*
f(z + y)*f(a
>      + 2*y)*f(c + 2*y) + 4*f(y + x)^2*f(z + y)*f(a + 2*y)*f
(b + z + y) -
>      4*f(y + x)^2*f(z + x)*f(b + 2*y)*f(b + z + y) - 2*f(y +
x)^3*f(c + 2*
>      y)^2 - 4*f(y + x)^3*f(c + 2*y)*f(b + z + y) + 8*f(y + x)
^3*f(b + 2*y)
>      *f(c + z + y) - 4*f(2*y)*f(z + y)^2*f(a + y + x)*f(b + y
+ x) + 2*f(2
>      *y)*f(z + y)^2*f(a + 2*y)*f(b + 2*x) + 2*f(2*y)*f(z + y)
^2*f(a + 2*y)
>      *f(a + y + x) - 2*f(2*y)*f(z + y)^2*f(a + 2*x)*f(b + 2*
y) + 4*f(2*y)*
>      f(z + x)*f(z + y)*f(b + y + x)^2 - 2*f(2*y)*f(z + x)*f(z
+ y)*f(b + 2
>      *y)*f(a + y + x) + 2*f(2*y)*f(z + x)*f(z + y)*f(a + 2*y)
*f(b + y + x)
>      - 6*f(2*y)*f(z + x)^2*f(b + 2*y)*f(b + y + x) - 4*f(2*
y)*f(2*z)*f(y
>      + x)*f(b + y + x)^2 - 2*f(2*y)*f(2*z)*f(y + x)*f(b + 2*
y)*f(a + y +
>      x) - f(2*y)*f(2*z)*f(y + x)*f(b + 2*x)*f(b + 2*y) + f(2*
y)*f(2*z)*f(y
>      + x)*f(a + 2*y)^2 - 6*f(2*y)*f(y + x)*f(z + y)*f(c + 2*
y)*f(a + y +
>      x) + 4*f(2*y)*f(y + x)*f(z + y)*f(b + y + x)*f(c + y +
x) + 4*f(2*y)*
>      f(y + x)*f(z + y)*f(b + 2*y)*f(c + 2*x) - 2*f(2*y)*f(y +
x)*f(z + y)*
>      f(b + 2*x)*f(c + 2*y) + 8*f(2*y)*f(y + x)*f(z + y)*f(a +
z + y)*f(b
>      + y + x) - 4*f(2*y)*f(y + x)*f(z + y)*f(a + y + x)*f(b

```

```

+ z + y) - 2*
> f(2*y)*f(y + x)*f(z + y)*f(a + 2*y)*f(b + z + x) + 2*f
(2*y)*f(y + x)*
> f(z + y)*f(a + 2*y)*f(a + z + y) - 2*f(2*y)*f(y + x)*f(z
+ x)*f(c + 2
> *y)*f(b + y + x) + 4*f(2*y)*f(y + x)*f(z + x)*f(b + y +
x)*f(b + z +
> y) + 4*f(2*y)*f(y + x)*f(z + x)*f(b + 2*y)*f(c + y + x)
+ 2*f(2*y)*f(
> y + x)*f(z + x)*f(b + 2*y)*f(b + z + x) + 2*f(2*y)*f(y +
x)*f(z + x)*
> f(b + 2*y)*f(a + z + y) - 2*f(2*y)*f(y + x)*f(z + x)*f(a
+ 2*y)*f(c
> + 2*y) + 4*f(2*y)*f(y + x)^2*f(c + 2*y)*f(c + y + x) +
2*f(2*y)*f(y
> + x)^2*f(c + 2*y)*f(b + z + x) + 2*f(2*y)*f(y + x)^2*f
(c + 2*y)*f(a
> + z + y) + 4*f(2*y)*f(y + x)^2*f(b + z + y)*f(c + y +
x) - 8*f(2*y)*
> f(y + x)^2*f(b + y + x)*f(c + z + y) - 4*f(2*y)*f(y + x)
^2*f(b + 2*y)
> *f(c + z + x) + 2*f(2*y)*f(y + x)^2*f(a + 2*z)*f(b + 2*
y) - 4*f(2*y)*
> f(y + x)^2*f(a + 2*y)*f(c + z + y) - 2*f(2*y)^2*f(z + y)
*f(c + 2*x)*
> f(b + y + x) - 2*f(2*y)^2*f(z + y)*f(b + 2*x)*f(a + z +
y) + 2*f(2*y)
> ^2*f(z + y)*f(a + y + x)*f(c + y + x) + 2*f(2*y)^2*f(z +
y)*f(a + y
> + x)*f(b + z + x) - 2*f(2*y)^2*f(z + y)*f(a + y + x)*f
(a + z + y) -
> f(2*y)^2*f(z + y)*f(a + 2*y)*f(c + 2*x) + f(2*y)^2*f(z +
y)*f(a + 2*x
> )*f(c + 2*y) + 2*f(2*y)^2*f(z + y)*f(a + 2*x)*f(b + z +
y) + 2*f(2*y)
> ^2*f(z + x)*f(c + 2*y)*f(a + y + x) - 2*f(2*y)^2*f(z +
x)*f(b + y + x
> )*f(c + y + x) - 2*f(2*y)^2*f(z + x)*f(b + y + x)*f(b +
z + x) - f(2*
> y)^2*f(z + x)*f(b + 2*y)*f(c + 2*x) + f(2*y)^2*f(z + x)*
f(b + 2*x)*f(
> c + 2*y) - 2*f(2*y)^2*f(z + x)*f(a + z + y)*f(b + y + x)
+ f(2*y)^2*
> f(2*z)*f(b + 2*x)*f(b + y + x) + 2*f(2*y)^2*f(2*z)*f(a +
y + x)*f(b
> + y + x) - 1/2*f(2*y)^2*f(2*z)*f(a + 2*y)*f(b + 2*x) -
f(2*y)^2*f(2*
> z)*f(a + 2*y)*f(a + y + x) + 1/2*f(2*y)^2*f(2*z)*f(a +
2*x)*f(b + 2*y
> ) - 2*f(2*y)^2*f(y + x)*f(c + y + x)^2 - f(2*y)^2*f(y +
x)*f(c + 2*x)
> *f(c + 2*y) - 2*f(2*y)^2*f(y + x)*f(c + 2*x)*f(b + z +
y) - 2*f(2*y)^
> 2*f(y + x)*f(b + z + x)*f(c + y + x) + 4*f(2*y)^2*f(y +
x)*f(b + y +
> x)*f(c + z + x) + 2*f(2*y)^2*f(y + x)*f(b + 2*x)*f(c + z
+ y) - 2*f(2

```

```

>      *y)^2*f(y + x)*f(a + z + y)*f(c + y + x) - 2*f(2*y)^2*f
> (y + x)*f(a +
>      2*z)*f(b + y + x) + 4*f(2*y)^2*f(y + x)*f(a + y + x)*f(c
> + z + y) + 2
>      *f(2*y)^2*f(y + x)*f(a + 2*y)*f(c + z + x) - f(2*y)^2*f
> (y + x)*f(a +
>      2*y)*f(a + 2*z) + f(2*y)^3*f(c + 2*x)*f(c + y + x) + f
> (2*y)^3*f(c + 2
>      *x)*f(b + z + x) + f(2*y)^3*f(c + 2*x)*f(a + z + y) - f
> (2*y)^3*f(b +
>      2*x)*f(c + z + x) + 1/2*f(2*y)^3*f(a + 2*z)*f(b + 2*x) +
> f(2*y)^3*f(a
>      + 2*z)*f(a + y + x) - 2*f(2*y)^3*f(a + y + x)*f(c + z +
> x) - f(2*y)^
>      3*f(a + 2*x)*f(c + z + y) - 1/2*f(2*y)^3*f(a + 2*x)*f(b
> + 2*z) - 4*f(
>      2*x)*f(z + y)^2*f(b + 2*y)*f(b + y + x) - 2*f(2*x)*f(2*
> z)*f(y + x)*f(
>      b + 2*y)^2 + 4*f(2*x)*f(y + x)*f(z + y)*f(b + 2*y)*f(b +
> z + y) - 4*
>      f(2*x)*f(2*y)*f(z + y)*f(b + y + x)*f(b + z + y) + 2*f
> (2*x)*f(2*y)*f(
>      z + y)*f(b + 2*y)*f(a + z + y) - 2*f(2*x)*f(2*y)*f(z +
> y)*f(a + 2*y)*
>      f(b + z + y) + 6*f(2*x)*f(2*y)*f(2*z)*f(b + 2*y)*f(b + y
> + x) + f(2*x
>      )*f(2*y)*f(y + x)*f(c + 2*y)^2 + 2*f(2*x)*f(2*y)*f(y +
> x)*f(c + 2*y)*
>      f(b + z + y) - 4*f(2*x)*f(2*y)*f(y + x)*f(b + 2*y)*f(c +
> z + y) - f(2
>      *x)*f(2*y)*f(y + x)*f(b + 2*y)*f(b + 2*z) - f(2*x)*f(2*
> y)^2*f(c + 2*y
>      )*f(c + y + x) - f(2*x)*f(2*y)^2*f(c + 2*y)*f(b + z + x)
> - f(2*x)*f(2
>      *y)^2*f(c + 2*y)*f(a + z + y) + f(2*x)*f(2*y)^2*f(b + 2*
> z)*f(b + y +
>      x) + 2*f(2*x)*f(2*y)^2*f(b + y + x)*f(c + z + y) + f(2*
> x)*f(2*y)^2*f(
>      b + 2*y)*f(c + z + x) - 1/2*f(2*x)*f(2*y)^2*f(a + 2*z)*f
> (b + 2*y) +
>      f(2*x)*f(2*y)^2*f(a + 2*y)*f(c + z + y) + 1/2*f(2*x)*f
> (2*y)^2*f(a + 2
>      *y)*f(b + 2*z) )
>
>      - 4*f(b + 2*y)*f(b + y + x) + 2*f(y + x)*f(2*b + 2*y) - 2*
> f(2*y)*f(2*b
>      + y + x):
>
> eq[26] :=
> (1/HessUniv) * ( 2*f(y + x)*f(z + y)^2*f(a + 2*x)*f(b + 2*y) + 4*
> f(y
>      + x)*f(z + x)*f(z + y)*f(b + 2*y)*f(a + y + x) + 2*f(y
> + x)*f(z + x)
>      ^2*f(a + 2*y)*f(b + 2*y) - 4*f(y + x)^2*f(z + y)*f(b +
> 2*y)*f(a + z
>      + x) - 4*f(y + x)^2*f(z + x)*f(b + 2*y)*f(a + z + y) +
> 2*f(y + x)^3*

```



```

>      f(a + 2*z)*f(b + 2*y) - 2*f(2*y)*f(z + y)^2*f(a + 2*x)*f
>      (b + y + x)
>      + 2*f(2*y)*f(z + x)*f(z + y)*f(b + 2*x)*f(b + y + x) +
>      2*f(2*y)*f(z
>      + x)*f(z + y)*f(a + 2*y)*f(b + 2*x) + 2*f(2*y)*f(z + x)
>      *f(z + y)*f(a
>      + 2*y)*f(a + y + x) - 2*f(2*y)*f(z + x)*f(z + y)*f(a +
>      2*x)*f(b + 2*
>      y) - 2*f(2*y)*f(z + x)^2*f(b + 2*y)*f(a + y + x) - f(2*
>      y)*f(z + x)^2*
>      f(b + 2*x)*f(b + 2*y) - 2*f(2*y)*f(z + x)^2*f(a + 2*y)*f
>      (b + y + x)
>      - f(2*y)*f(z + x)^2*f(a + 2*y)^2 - f(2*y)*f(2*z)*f(y +
>      x)*f(b + 2*x)
>      *f(b + y + x) - 2*f(2*y)*f(2*z)*f(y + x)*f(a + y + x)*f
>      (b + y + x) -
>      3/2*f(2*y)*f(2*z)*f(y + x)*f(a + 2*y)*f(b + 2*x) - f(2*
>      y)*f(2*z)*f(y
>      + x)*f(a + 2*y)*f(a + y + x) - 1/2*f(2*y)*f(2*z)*f(y +
>      x)*f(a + 2*x)
>      *f(b + 2*y) + 4*f(2*y)*f(y + x)*f(z + y)*f(a + z + x)*f
>      (b + y + x) +
>      f(2*y)*f(y + x)*f(z + y)*f(a + 2*y)*f(c + 2*x) - f(2*y)*
>      f(y + x)*f(z
>      + y)*f(a + 2*x)*f(c + 2*y) - 2*f(2*y)*f(y + x)*f(z + x)
>      *f(c + 2*y)*
>      f(a + y + x) + f(2*y)*f(y + x)*f(z + x)*f(b + 2*y)*f(c +
>      2*x) + 2*f(2
>      *y)*f(y + x)*f(z + x)*f(b + 2*y)*f(a + z + x) + f(2*y)*f
>      (y + x)*f(z
>      + x)*f(b + 2*x)*f(c + 2*y) + 4*f(2*y)*f(y + x)*f(z + x)
>      *f(a + z + y)
>      *f(b + y + x) + 2*f(2*y)*f(y + x)*f(z + x)*f(a + 2*y)*f
>      (a + z + y) +
>      2*f(2*y)*f(y + x)^2*f(c + 2*y)*f(a + z + x) - f(2*y)*f(y
>      + x)^2*f(c
>      + 2*x)*f(c + 2*y) - 2*f(2*y)*f(y + x)^2*f(a + 2*z)*f(b
>      + y + x) - f(
>      2*y)*f(y + x)^2*f(a + 2*y)*f(a + 2*z) - f(2*y)^2*f(z +
>      y)*f(c + 2*x)*
>      f(a + y + x) - f(2*y)^2*f(z + y)*f(b + 2*x)*f(a + z + x)
>      + f(2*y)^2*
>      f(z + y)*f(a + 2*x)*f(c + y + x) + f(2*y)^2*f(z + y)*f(a
>      + 2*x)*f(b
>      + z + x) - f(2*y)^2*f(z + x)*f(c + 2*x)*f(b + y + x) -
>      f(2*y)^2*f(z
>      + x)*f(b + 2*x)*f(c + y + x) - f(2*y)^2*f(z + x)*f(b +
>      2*x)*f(a + z
>      + y) - 2*f(2*y)^2*f(z + x)*f(a + z + x)*f(b + y + x) +
>      2*f(2*y)^2*f(
>      z + x)*f(a + y + x)*f(c + y + x) - 2*f(2*y)^2*f(z + x)*f
>      (a + y + x)*
>      f(a + z + y) - f(2*y)^2*f(z + x)*f(a + 2*y)*f(c + 2*x) +
>      f(2*y)^2*f(z
>      + x)*f(a + 2*x)*f(c + 2*y) + f(2*y)^2*f(z + x)*f(a + 2*
>      x)*f(b + z +
>      y) + f(2*y)^2*f(2*z)*f(b + 2*x)*f(a + y + x) + f(2*y)^2*

```

```

f(2*z)*f(a +
>      2*x)*f(b + y + x) + f(2*y)^2*f(y + x)*f(c + 2*x)*f(c + y
+ x) - 2*f(2
>      *y)^2*f(y + x)*f(a + z + x)*f(c + y + x) + 1/2*f(2*y)^2*
f(y + x)*f(a
>      + 2*z)*f(b + 2*x) + f(2*y)^2*f(y + x)*f(a + 2*z)*f(a +
y + x) - 1/2*
>      f(2*y)^2*f(y + x)*f(a + 2*x)*f(b + 2*z) + f(2*y)^3*f(c +
2*x)*f(a + z
>      + x) - f(2*y)^3*f(a + 2*x)*f(c + z + x) - f(2*x)*f(z +
y)^2*f(b + 2*
>      x)*f(b + 2*y) - 2*f(2*x)*f(z + y)^2*f(a + 2*y)*f(b + y +
x) - f(2*x)*
>      f(z + y)^2*f(a + 2*y)^2 - 2*f(2*x)*f(2*z)*f(y + x)*f(a +
2*y)*f(b + 2
>      *y) + 2*f(2*x)*f(y + x)*f(z + y)*f(c + 2*y)*f(b + y + x)
- 4*f(2*x)*
>      f(y + x)*f(z + y)*f(b + 2*y)*f(c + y + x) + 2*f(2*x)*f(y
+ x)*f(z + y
>      )*f(b + 2*y)*f(b + z + x) + 2*f(2*x)*f(y + x)*f(z + y)*f
(a + 2*y)*f(c
>      + 2*y) + 2*f(2*x)*f(y + x)*f(z + y)*f(a + 2*y)*f(b + z
+ y) - f(2*x)
>      *f(y + x)^2*f(c + 2*y)^2 - 2*f(2*x)*f(y + x)^2*f(c + 2*
y)*f(b + z + y
>      ) + 4*f(2*x)*f(y + x)^2*f(b + 2*y)*f(c + z + y) - f(2*x)
*f(y + x)^2*
>      f(b + 2*y)*f(b + 2*z) - f(2*x)*f(2*y)*f(z + y)*f(c + 2*
y)*f(a + y + x
>      ) + 2*f(2*x)*f(2*y)*f(z + y)*f(b + y + x)*f(c + y + x) -
2*f(2*x)*f(2
>      *y)*f(z + y)*f(b + y + x)*f(b + z + x) + f(2*x)*f(2*y)*f
(z + y)*f(b
>      + 2*y)*f(c + 2*x) + f(2*x)*f(2*y)*f(z + y)*f(b + 2*y)*f
(a + z + x)
>      - f(2*x)*f(2*y)*f(z + y)*f(b + 2*x)*f(c + 2*y) - 2*f(2*
x)*f(2*y)*f(z
>      + y)*f(a + y + x)*f(b + z + y) - f(2*x)*f(2*y)*f(z + y)
*f(a + 2*y)*
>      f(c + y + x) - f(2*x)*f(2*y)*f(z + y)*f(a + 2*y)*f(b + z
+ x) - f(2*x)
>      )*f(2*y)*f(z + x)*f(c + 2*y)*f(b + y + x) + f(2*x)*f(2*
y)*f(z + x)*f(
>      b + 2*y)*f(c + y + x) + f(2*x)*f(2*y)*f(z + x)*f(b + 2*
y)*f(a + z + y
>      ) - f(2*x)*f(2*y)*f(z + x)*f(a + 2*y)*f(b + z + y) + f
(2*x)*f(2*y)*f(
>      2*z)*f(b + 2*y)*f(a + y + x) + f(2*x)*f(2*y)*f(2*z)*f(b
+ 2*x)*f(b +
>      2*y) + 3*f(2*x)*f(2*y)*f(2*z)*f(a + 2*y)*f(b + y + x) +
f(2*x)*f(2*y)
>      *f(2*z)*f(a + 2*y)^2 + 3*f(2*x)*f(2*y)*f(y + x)*f(c + 2*
y)*f(c + y +
>      x) + 2*f(2*x)*f(2*y)*f(y + x)*f(b + z + y)*f(c + y + x)
+ f(2*x)*f(2*
>      y)*f(y + x)*f(b + 2*z)*f(b + y + x) - 4*f(2*x)*f(2*y)*f
(y + x)*f(b +

```

```

>      y + x)*f(c + z + y) - 2*f(2*x)*f(2*y)*f(y + x)*f(b + 2*
>      y)*f(c + z + x
>      ) - 1/2*f(2*x)*f(2*y)*f(y + x)*f(a + 2*z)*f(b + 2*y) -
>      2*f(2*x)*f(2*y
>      )*f(y + x)*f(a + 2*y)*f(c + z + y) + 1/2*f(2*x)*f(2*y)*f
>      (y + x)*f(a
>      + 2*y)*f(b + 2*z) - 2*f(2*x)*f(2*y)^2*f(c + y + x)^2 -
>      f(2*x)*f(2*y)
>      ^2*f(c + 2*y)*f(a + z + x) - f(2*x)*f(2*y)^2*f(c + 2*x)*
>      f(b + z + y)
>      + 2*f(2*x)*f(2*y)^2*f(b + y + x)*f(c + z + x) + f(2*x)*
>      f(2*y)^2*f(b
>      + 2*x)*f(c + z + y) + 2*f(2*x)*f(2*y)^2*f(a + y + x)*f
>      (c + z + y) +
>      f(2*x)*f(2*y)^2*f(a + 2*y)*f(c + z + x) + f(2*x)^2*f(2*
>      y)*f(c + 2*y)*
>      f(b + z + y) - f(2*x)^2*f(2*y)*f(b + 2*y)*f(c + z + y) )
>
>      - f(b + 2*x)*f(b + 2*y) - 2*f(a + 2*y)*f(b + y + x) - f(a
>      + 2*y)^2 + 2*
>      f(y + x)*f(b + a + 2*y) - 2*f(2*y)*f(b + a + y + x):
>
> eq[27] :=
> (1/HessUniv) * ( 2*f(y + x)*f(z + y)^2*f(a + 2*x)*f(a + 2*y) - 2*
> f(y
>      + x)*f(z + x)*f(z + y)*f(a + 2*y)*f(b + 2*x) + 4*f(y +
>      x)*f(z + x)*
>      f(z + y)*f(a + 2*y)*f(a + y + x) + 2*f(y + x)*f(z + x)*f
>      (z + y)*f(a
>      + 2*x)*f(b + 2*y) + 4*f(y + x)*f(z + x)^2*f(b + 2*y)*f
>      (a + y + x) -
>      2*f(y + x)*f(z + x)^2*f(b + 2*x)*f(b + 2*y) + 2*f(y + x)
>      ^2*f(z + y)*
>      f(a + 2*y)*f(c + 2*x) - 4*f(y + x)^2*f(z + y)*f(a + 2*y)
>      *f(a + z + x)
>      - 2*f(y + x)^2*f(z + y)*f(a + 2*x)*f(c + 2*y) - 4*f(y +
>      x)^2*f(z + x
>      )*f(c + 2*y)*f(a + y + x) + 2*f(y + x)^2*f(z + x)*f(b +
>      2*y)*f(c + 2*
>      x) - 4*f(y + x)^2*f(z + x)*f(b + 2*y)*f(a + z + x) + 2*f
>      (y + x)^2*f(z
>      + x)*f(b + 2*x)*f(c + 2*y) + 4*f(y + x)^3*f(c + 2*y)*f
>      (a + z + x) -
>      2*f(y + x)^3*f(c + 2*x)*f(c + 2*y) - 2*f(2*y)*f(z + y)
>      ^2*f(a + 2*x)*
>      f(a + y + x) + 2*f(2*y)*f(z + x)*f(z + y)*f(b + 2*x)*f(a
>      + y + x) + 4
>      *f(2*y)*f(z + x)*f(z + y)*f(a + y + x)^2 - 2*f(2*y)*f(z
>      + x)*f(z + y)
>      *f(a + 2*x)*f(b + y + x) + 2*f(2*y)*f(z + x)^2*f(b + 2*
>      x)*f(b + y + x
>      ) - 4*f(2*y)*f(z + x)^2*f(a + y + x)*f(b + y + x) + 2*f
>      (2*y)*f(z + x)
>      ^2*f(a + 2*y)*f(b + 2*x) - 4*f(2*y)*f(z + x)^2*f(a + 2*
>      y)*f(a + y + x
>      ) - 2*f(2*y)*f(z + x)^2*f(a + 2*x)*f(b + 2*y) - 4*f(2*y)
>      *f(2*z)*f(y

```

```

> + x)*f(a + y + x)^2 - 2*f(2*y)*f(2*z)*f(y + x)*f(a + 2*
x)*f(a + 2*y)
> - 2*f(2*y)*f(y + x)*f(z + y)*f(c + 2*x)*f(a + y + x) +
4*f(2*y)*f(y
> + x)*f(z + y)*f(a + y + x)*f(a + z + x) + 2*f(2*y)*f(y
+ x)*f(z + y)
> *f(a + 2*x)*f(c + y + x) - 2*f(2*y)*f(y + x)*f(z + x)*f
(c + 2*x)*f(b
> + y + x) - 2*f(2*y)*f(y + x)*f(z + x)*f(b + 2*x)*f(c +
y + x) + 4*f(
> 2*y)*f(y + x)*f(z + x)*f(a + z + x)*f(b + y + x) + 4*f
(2*y)*f(y + x)*
> f(z + x)*f(a + y + x)*f(c + y + x) - 2*f(2*y)*f(y + x)*f
(z + x)*f(a
> + 2*y)*f(c + 2*x) + 4*f(2*y)*f(y + x)*f(z + x)*f(a + 2*
y)*f(a + z +
> x) + 2*f(2*y)*f(y + x)*f(z + x)*f(a + 2*x)*f(c + 2*y) +
2*f(2*y)*f(y
> + x)^2*f(c + 2*x)*f(c + y + x) - 4*f(2*y)*f(y + x)^2*f
(a + z + x)*f(
> c + y + x) - 2*f(2*y)^2*f(z + x)*f(b + 2*x)*f(a + z + x)
- 4*f(2*y)^2
> *f(z + x)*f(a + y + x)*f(a + z + x) + 2*f(2*y)^2*f(z +
x)*f(a + 2*x)*
> f(b + z + x) + 2*f(2*y)^2*f(2*z)*f(a + 2*x)*f(a + y + x)
+ 2*f(2*y)^2
> *f(y + x)*f(c + 2*x)*f(a + z + x) - 2*f(2*y)^2*f(y + x)*
f(a + 2*x)*f(
> c + z + x) - 4*f(2*x)*f(z + y)^2*f(a + 2*y)*f(a + y + x)
- 2*f(2*x)*
> f(2*z)*f(y + x)*f(b + 2*y)*f(a + y + x) + f(2*x)*f(2*z)*
f(y + x)*f(b
> + 2*x)*f(b + 2*y) - f(2*x)*f(2*z)*f(y + x)*f(a + 2*y)^2
+ 4*f(2*x)*
> f(y + x)*f(z + y)*f(c + 2*y)*f(a + y + x) - 2*f(2*x)*f(y
+ x)*f(z + y
> )*f(b + 2*y)*f(c + 2*x) - 2*f(2*x)*f(y + x)*f(z + y)*f(a
+ 2*y)*f(c
> + y + x) + 2*f(2*x)*f(y + x)*f(z + y)*f(a + 2*y)*f(b +
z + x) + 2*f(
> 2*x)*f(y + x)*f(z + y)*f(a + 2*y)*f(a + z + y) - 2*f(2*
x)*f(y + x)*f(
> z + x)*f(b + 2*y)*f(c + y + x) + 2*f(2*x)*f(y + x)*f(z +
x)*f(b + 2*y
> )*f(b + z + x) - 2*f(2*x)*f(y + x)*f(z + x)*f(b + 2*y)*f
(a + z + y)
> + 2*f(2*x)*f(y + x)*f(z + x)*f(a + 2*y)*f(c + 2*y) + 2*
f(2*x)*f(y +
> x)^2*f(c + 2*y)*f(c + y + x) - 2*f(2*x)*f(y + x)^2*f(c +
2*y)*f(b + z
> + x) - 2*f(2*x)*f(y + x)^2*f(c + 2*y)*f(a + z + y) + 2*
f(2*x)*f(y +
> x)^2*f(a + 2*z)*f(b + 2*y) + 2*f(2*x)*f(2*y)*f(z + y)*f
(c + 2*x)*f(b
> + y + x) - 2*f(2*x)*f(2*y)*f(z + y)*f(a + y + x)*f(c +
y + x) - 2*f(
> 2*x)*f(2*y)*f(z + y)*f(a + y + x)*f(b + z + x) - 2*f(2*

```

```

x)*f(2*y)*f(z
> + y)*f(a + y + x)*f(a + z + y) + f(2*x)*f(2*y)*f(z + y)
> *f(a + 2*y)*
> f(c + 2*x) - f(2*x)*f(2*y)*f(z + y)*f(a + 2*x)*f(c + 2*
> y) - 2*f(2*x)*
> f(2*y)*f(z + x)*f(c + 2*y)*f(a + y + x) + 2*f(2*x)*f(2*
> y)*f(z + x)*f(
> b + y + x)*f(c + y + x) - 2*f(2*x)*f(2*y)*f(z + x)*f(b +
> y + x)*f(b
> + z + x) + f(2*x)*f(2*y)*f(z + x)*f(b + 2*y)*f(c + 2*x)
> + 2*f(2*x)*
> f(2*y)*f(z + x)*f(b + 2*y)*f(a + z + x) - f(2*x)*f(2*y)*
> f(z + x)*f(b
> + 2*x)*f(c + 2*y) + 2*f(2*x)*f(2*y)*f(z + x)*f(a + z +
> y)*f(b + y +
> x) - 2*f(2*x)*f(2*y)*f(z + x)*f(a + 2*y)*f(b + z + x) -
> f(2*x)*f(2*y)
> *f(2*z)*f(b + 2*x)*f(b + y + x) + 2*f(2*x)*f(2*y)*f(2*z)
> *f(a + y + x)
> *f(b + y + x) - 1/2*f(2*x)*f(2*y)*f(2*z)*f(a + 2*y)*f(b
> + 2*x) + 5*f(
> 2*x)*f(2*y)*f(2*z)*f(a + 2*y)*f(a + y + x) + 1/2*f(2*x)*
> f(2*y)*f(2*z)
> *f(a + 2*x)*f(b + 2*y) - 2*f(2*x)*f(2*y)*f(y + x)*f(c +
> y + x)^2 - 2*
> f(2*x)*f(2*y)*f(y + x)*f(c + 2*y)*f(a + z + x) + f(2*x)*
> f(2*y)*f(y +
> x)*f(c + 2*x)*f(c + 2*y) + 2*f(2*x)*f(2*y)*f(y + x)*f(b
> + z + x)*f(c
> + y + x) + 2*f(2*x)*f(2*y)*f(y + x)*f(a + z + y)*f(c +
> y + x) - 2*f(
> 2*x)*f(2*y)*f(y + x)*f(a + 2*z)*f(b + y + x) - f(2*x)*f
> (2*y)*f(y + x)
> *f(a + 2*y)*f(a + 2*z) - f(2*x)*f(2*y)^2*f(c + 2*x)*f(c
> + y + x) - f(
> 2*x)*f(2*y)^2*f(c + 2*x)*f(b + z + x) - f(2*x)*f(2*y)^2*
> f(c + 2*x)*f(
> a + z + y) + f(2*x)*f(2*y)^2*f(b + 2*x)*f(c + z + x) +
> 1/2*f(2*x)*f(2
> y)^2*f(a + 2*z)*f(b + 2*x) + f(2*x)*f(2*y)^2*f(a + 2*z)
> *f(a + y + x)
> + 2*f(2*x)*f(2*y)^2*f(a + y + x)*f(c + z + x) + f(2*x)*
> f(2*y)^2*f(a
> + 2*x)*f(c + z + y) - 1/2*f(2*x)*f(2*y)^2*f(a + 2*x)*f
> (b + 2*z) - f(
> 2*x)^2*f(y + x)*f(c + 2*y)^2 + 2*f(2*x)^2*f(y + x)*f(b +
> 2*y)*f(c + z
> + y) - f(2*x)^2*f(y + x)*f(b + 2*y)*f(b + 2*z) + f(2*x)
> ^2*f(2*y)*f(c
> + 2*y)*f(c + y + x) + f(2*x)^2*f(2*y)*f(c + 2*y)*f(b +
> z + x) + f(2*
> x)^2*f(2*y)*f(c + 2*y)*f(a + z + y) + f(2*x)^2*f(2*y)*f
> (b + 2*z)*f(b
> + y + x) - 2*f(2*x)^2*f(2*y)*f(b + y + x)*f(c + z + y)
> - f(2*x)^2*f(
> 2*y)*f(b + 2*y)*f(c + z + x) - 1/2*f(2*x)^2*f(2*y)*f(a +
> 2*z)*f(b + 2

```

```

>      *y) - f(2*x)^2*f(2*y)*f(a + 2*y)*f(c + z + y) + 1/2*f(2*
x)^2*f(2*y)*
>      f(a + 2*y)*f(b + 2*z) )
>
>      - 4*f(a + 2*y)*f(a + y + x) + 2*f(y + x)*f(2*a + 2*y) - 2*
f(2*y)*f(2*a
>      + y + x):
>
> eq[28] :=
> (1/HessUniv) * ( - 2*f(2*y)*f(z + y)^2*f(a + 2*x)*f(b + y + x) +
f(2
>      *y)*f(z + y)^2*f(a + 2*x)*f(a + 2*y) + 2*f(2*y)*f(z + x)
*f(z + y)*f(b
>      + 2*x)*f(b + y + x) + f(2*y)*f(z + x)*f(z + y)*f(a + 2*
y)*f(b + 2*x)
>      - f(2*y)*f(z + x)*f(z + y)*f(a + 2*x)*f(b + 2*y) - f(2*
y)*f(z + x)^2
>      *f(b + 2*x)*f(b + 2*y) - 2*f(2*y)*f(2*z)*f(y + x)*f(b +
2*x)*f(b + y
>      + x) + 2*f(2*y)*f(y + x)*f(z + y)*f(c + 2*x)*f(b + y +
x) - f(2*y)*
>      f(y + x)*f(z + y)*f(a + 2*y)*f(c + 2*x) - f(2*y)*f(y +
x)*f(z + y)*f(
>      a + 2*x)*f(c + 2*y) + 2*f(2*y)*f(y + x)*f(z + y)*f(a +
2*x)*f(b + z
>      + y) + f(2*y)*f(y + x)*f(z + x)*f(b + 2*y)*f(c + 2*x) -
f(2*y)*f(y
>      + x)*f(z + x)*f(b + 2*x)*f(c + 2*y) + 2*f(2*y)*f(y + x)
*f(z + x)*f(b
>      + 2*x)*f(b + z + y) + f(2*y)*f(y + x)^2*f(c + 2*x)*f(c
+ 2*y) - 2*f(
>      2*y)*f(y + x)^2*f(c + 2*x)*f(b + z + y) - f(2*y)^2*f(z +
y)*f(b + 2*x
>      )*f(c + 2*x) + f(2*y)^2*f(z + y)*f(a + 2*x)*f(c + y + x)
+ f(2*y)^2*
>      f(z + y)*f(a + 2*x)*f(b + z + x) - f(2*y)^2*f(z + y)*f(a
+ 2*x)*f(a
>      + z + y) - 2*f(2*y)^2*f(z + x)*f(c + 2*x)*f(b + y + x)
+ f(2*y)^2*f(
>      z + x)*f(b + 2*x)*f(c + y + x) - f(2*y)^2*f(z + x)*f(b +
2*x)*f(b + z
>      + x) - f(2*y)^2*f(z + x)*f(b + 2*x)*f(a + z + y) + f(2*
y)^2*f(z + x)
>      *f(a + 2*x)*f(c + 2*y) + 1/2*f(2*y)^2*f(2*z)*f(b + 2*x)
^2 + f(2*y)^2*
>      f(2*z)*f(a + 2*x)*f(b + y + x) - 1/2*f(2*y)^2*f(2*z)*f(a
+ 2*x)*f(a
>      + 2*y) - f(2*y)^2*f(y + x)*f(c + 2*x)*f(c + y + x) + f
(2*y)^2*f(y +
>      x)*f(c + 2*x)*f(b + z + x) + f(2*y)^2*f(y + x)*f(c + 2*
x)*f(a + z + y
>      ) - f(2*y)^2*f(y + x)*f(a + 2*x)*f(b + 2*z) + 1/2*f(2*y)
^3*f(c + 2*x)
>      ^2 - f(2*y)^3*f(a + 2*x)*f(c + z + x) + 1/2*f(2*y)^3*f(a
+ 2*x)*f(a
>      + 2*z) + 4*f(2*x)*f(z + y)^2*f(b + 2*y)*f(a + y + x) -
2*f(2*x)*f(z

```

```

> + y)^2*f(a + 2*y)*f(b + y + x) - f(2*x)*f(z + y)^2*f(a
> + 2*y)^2 - 2*
> f(2*x)*f(z + x)*f(z + y)*f(b + 2*y)*f(b + y + x) + f(2*
> x)*f(z + x)^2*
> f(b + 2*y)^2 + 2*f(2*x)*f(2*z)*f(y + x)*f(b + 2*y)*f(b +
> y + x) + 2*
> f(2*x)*f(y + x)*f(z + y)*f(c + 2*y)*f(b + y + x) - 4*f
> (2*x)*f(y + x)*
> f(z + y)*f(b + 2*y)*f(c + y + x) - 4*f(2*x)*f(y + x)*f(z
> + y)*f(b + 2
> *y)*f(a + z + y) + 2*f(2*x)*f(y + x)*f(z + y)*f(a + 2*y)
> *f(c + 2*y)
> + 2*f(2*x)*f(y + x)*f(z + y)*f(a + 2*y)*f(b + z + y) -
> 2*f(2*x)*f(y
> + x)*f(z + x)*f(b + 2*y)*f(b + z + y) - f(2*x)*f(y + x)
> ^2*f(c + 2*y)
> ^2 - 2*f(2*x)*f(y + x)^2*f(c + 2*y)*f(b + z + y) + 4*f
> (2*x)*f(y + x)^
> 2*f(b + 2*y)*f(c + z + y) - 2*f(2*x)*f(2*y)*f(z + y)*f(c
> + 2*y)*f(a
> + y + x) + f(2*x)*f(2*y)*f(z + y)*f(b + 2*y)*f(c + 2*x)
> - 2*f(2*x)*
> f(2*y)*f(z + y)*f(b + 2*x)*f(b + z + y) + 4*f(2*x)*f(2*
> y)*f(z + y)*f(
> a + z + y)*f(b + y + x) - 4*f(2*x)*f(2*y)*f(z + y)*f(a +
> y + x)*f(b
> + z + y) + f(2*x)*f(2*y)*f(z + y)*f(a + 2*y)*f(c + y +
> x) - f(2*x)*
> f(2*y)*f(z + y)*f(a + 2*y)*f(b + z + x) + f(2*x)*f(2*y)*
> f(z + y)*f(a
> + 2*y)*f(a + z + y) + f(2*x)*f(2*y)*f(z + x)*f(b + 2*y)
> *f(c + y + x)
> + f(2*x)*f(2*y)*f(z + x)*f(b + 2*y)*f(b + z + x) + f(2*
> x)*f(2*y)*f(z
> + x)*f(b + 2*y)*f(a + z + y) - f(2*x)*f(2*y)*f(z + x)*f
> (a + 2*y)*f(c
> + 2*y) - f(2*x)*f(2*y)*f(2*z)*f(b + 2*y)*f(a + y + x) +
> 1/2*f(2*x)*
> f(2*y)*f(2*z)*f(b + 2*x)*f(b + 2*y) + 1/2*f(2*x)*f(2*y)*
> f(2*z)*f(a +
> 2*y)^2 + f(2*x)*f(2*y)*f(y + x)*f(c + 2*y)*f(c + y + x)
> + f(2*x)*f(2*
> y)*f(y + x)*f(c + 2*y)*f(b + z + x) + f(2*x)*f(2*y)*f(y
> + x)*f(c + 2*
> y)*f(a + z + y) + 4*f(2*x)*f(2*y)*f(y + x)*f(b + z + y)*
> f(c + y + x)
> - 4*f(2*x)*f(2*y)*f(y + x)*f(b + y + x)*f(c + z + y) -
> 2*f(2*x)*f(2*
> y)*f(y + x)*f(b + 2*y)*f(c + z + x) + f(2*x)*f(2*y)*f(y
> + x)*f(a + 2*
> z)*f(b + 2*y) - 2*f(2*x)*f(2*y)*f(y + x)*f(a + 2*y)*f(c
> + z + y) - f(
> 2*x)*f(2*y)^2*f(c + 2*x)*f(c + 2*y) - 2*f(2*x)*f(2*y)^2*
> f(b + z + x)*
> f(c + y + x) + f(2*x)*f(2*y)^2*f(b + 2*z)*f(a + y + x) +
> 2*f(2*x)*f(2
> *y)^2*f(b + y + x)*f(c + z + x) + f(2*x)*f(2*y)^2*f(b +

```

```

2*x)*f(c + z
> + y) + 1/2*f(2*x)*f(2*y)^2*f(b + 2*x)*f(b + 2*z) - 2*f
(2*x)*f(2*y)^2
> *f(a + z + y)*f(c + y + x) - f(2*x)*f(2*y)^2*f(a + 2*z)*
f(b + y + x)
> + 2*f(2*x)*f(2*y)^2*f(a + y + x)*f(c + z + y) + f(2*x)*
f(2*y)^2*f(a
> + 2*y)*f(c + z + x) - 1/2*f(2*x)*f(2*y)^2*f(a + 2*y)*f
(a + 2*z) + 2*
> f(2*x)^2*f(z + y)*f(b + 2*y)*f(b + z + y) - f(2*x)^2*f
(2*z)*f(b + 2*y
> )^2 + 1/2*f(2*x)^2*f(2*y)*f(c + 2*y)^2 - f(2*x)^2*f(2*y)
*f(b + 2*y)*
> f(c + z + y) - 1/2*f(2*x)^2*f(2*y)*f(b + 2*y)*f(b + 2*z)
)
>
> - f(2*y)*f(2*b + 2*x) + f(2*x)*f(2*b + 2*y):
> eq[29] :=
> (1/HessUniv) * ( - f(2*y)*f(z + y)^2*f(a + 2*x)*f(b + 2*x) + f
(2*y)*
> f(z + x)*f(z + y)*f(b + 2*x)^2 + 2*f(2*y)*f(z + x)*f(z +
y)*f(b + 2*x
> )*f(a + y + x) - 2*f(2*y)*f(z + x)*f(z + y)*f(a + 2*x)*f
(b + y + x)
> + f(2*y)*f(z + x)*f(z + y)*f(a + 2*x)*f(a + 2*y) - f(2*
y)*f(z + x)^2
> *f(a + 2*x)*f(b + 2*y) - 1/2*f(2*y)*f(2*z)*f(y + x)*f(b
+ 2*x)^2 - f(
> 2*y)*f(2*z)*f(y + x)*f(b + 2*x)*f(a + y + x) - 1/2*f(2*
y)*f(2*z)*f(y
> + x)*f(a + 2*x)*f(a + 2*y) + 2*f(2*y)*f(y + x)*f(z + y)
*f(a + 2*x)*
> f(b + z + x) + 2*f(2*y)*f(y + x)*f(z + x)*f(a + 2*x)*f(b
+ z + y) -
> f(2*y)*f(y + x)^2*f(a + 2*x)*f(b + 2*z) - f(2*y)^2*f(z +
x)*f(c + 2*x
> )*f(a + y + x) - f(2*y)^2*f(z + x)*f(b + 2*x)*f(c + 2*x)
- f(2*y)^2*
> f(z + x)*f(b + 2*x)*f(a + z + x) + 2*f(2*y)^2*f(z + x)*f
(a + 2*x)*f(c
> + y + x) - f(2*y)^2*f(z + x)*f(a + 2*x)*f(a + z + y) +
f(2*y)^2*f(2*
> z)*f(a + 2*x)*f(b + 2*x) + 1/2*f(2*y)^2*f(y + x)*f(c +
2*x)^2 + f(2*y
> )^2*f(y + x)*f(c + 2*x)*f(a + z + x) - 2*f(2*y)^2*f(y +
x)*f(a + 2*x)
> *f(c + z + x) + 1/2*f(2*y)^2*f(y + x)*f(a + 2*x)*f(a +
2*z) + f(2*x)*
> f(z + y)^2*f(a + 2*x)*f(b + 2*y) + 2*f(2*x)*f(z + x)*f(z
+ y)*f(b + 2
> *y)*f(a + y + x) - f(2*x)*f(z + x)*f(z + y)*f(b + 2*x)*f
(b + 2*y) - 2
> *f(2*x)*f(z + x)*f(z + y)*f(a + 2*y)*f(b + y + x) - f(2*
x)*f(z + x)*
> f(z + y)*f(a + 2*y)^2 + f(2*x)*f(z + x)^2*f(a + 2*y)*f(b
+ 2*y) + 1/2

```



```

>      *f(2*x)*f(2*z)*f(y + x)*f(b + 2*x)*f(b + 2*y) + f(2*x)*f
(2*z)*f(y + x
>      )*f(a + 2*y)*f(b + y + x) + 1/2*f(2*x)*f(2*z)*f(y + x)*f
(a + 2*y)^2
>      - 2*f(2*x)*f(y + x)*f(z + y)*f(b + 2*y)*f(a + z + x) -
2*f(2*x)*f(y
>      + x)*f(z + x)*f(b + 2*y)*f(a + z + y) + f(2*x)*f(y + x)
^2*f(a + 2*z)
>      *f(b + 2*y) + f(2*x)*f(2*y)*f(z + y)*f(c + 2*x)*f(b + y
+ x) - f(2*x)
>      *f(2*y)*f(z + y)*f(b + 2*x)*f(b + z + x) + 2*f(2*x)*f(2*
y)*f(z + y)*
>      f(a + z + x)*f(b + y + x) - 2*f(2*x)*f(2*y)*f(z + y)*f(a
+ y + x)*f(b
>      + z + x) - f(2*x)*f(2*y)*f(z + y)*f(a + 2*x)*f(c + 2*y)
- f(2*x)*f(2
>      *y)*f(z + y)*f(a + 2*x)*f(b + z + y) - f(2*x)*f(2*y)*f(z
+ x)*f(c + 2
>      *y)*f(a + y + x) + f(2*x)*f(2*y)*f(z + x)*f(b + 2*y)*f(c
+ 2*x) + f(2
>      *x)*f(2*y)*f(z + x)*f(b + 2*y)*f(a + z + x) + 2*f(2*x)*f
(2*y)*f(z + x
>      )*f(a + z + y)*f(b + y + x) - 2*f(2*x)*f(2*y)*f(z + x)*f
(a + y + x)*
>      f(b + z + y) + f(2*x)*f(2*y)*f(z + x)*f(a + 2*y)*f(a + z
+ y) + f(2*x
>      )*f(2*y)*f(y + x)*f(c + 2*y)*f(a + z + x) - f(2*x)*f(2*
y)*f(y + x)*f(
>      c + 2*x)*f(b + z + y) + f(2*x)*f(2*y)*f(y + x)*f(b + 2*
z)*f(a + y + x
>      ) + 1/2*f(2*x)*f(2*y)*f(y + x)*f(b + 2*x)*f(b + 2*z) - f
(2*x)*f(2*y)*
>      f(y + x)*f(a + 2*z)*f(b + y + x) - 1/2*f(2*x)*f(2*y)*f(y
+ x)*f(a + 2
>      *y)*f(a + 2*z) - f(2*x)*f(2*y)^2*f(c + 2*x)*f(c + y + x)
+ f(2*x)*f(2
>      *y)^2*f(b + 2*x)*f(c + z + x) - 2*f(2*x)*f(2*y)^2*f(a +
z + x)*f(c +
>      y + x) + 2*f(2*x)*f(2*y)^2*f(a + y + x)*f(c + z + x) + f
(2*x)*f(2*y)^
>      2*f(a + 2*x)*f(c + z + y) + f(2*x)^2*f(z + y)*f(c + 2*y)
*f(b + y + x)
>      - 2*f(2*x)^2*f(z + y)*f(b + 2*y)*f(c + y + x) + f(2*x)
^2*f(z + y)*f(
>      b + 2*y)*f(b + z + x) + f(2*x)^2*f(z + y)*f(a + 2*y)*f(c
+ 2*y) + f(2
>      *x)^2*f(z + y)*f(a + 2*y)*f(b + z + y) - f(2*x)^2*f(2*z)
*f(a + 2*y)*
>      f(b + 2*y) - 1/2*f(2*x)^2*f(y + x)*f(c + 2*y)^2 - f(2*x)
^2*f(y + x)*
>      f(c + 2*y)*f(b + z + y) + 2*f(2*x)^2*f(y + x)*f(b + 2*y)
*f(c + z + y)
>      - 1/2*f(2*x)^2*f(y + x)*f(b + 2*y)*f(b + 2*z) + f(2*x)
^2*f(2*y)*f(c
>      + 2*y)*f(c + y + x) + 2*f(2*x)^2*f(2*y)*f(b + z + y)*f
(c + y + x) -
>      2*f(2*x)^2*f(2*y)*f(b + y + x)*f(c + z + y) - f(2*x)^2*f

```

```

(2*y)*f(b + 2
>      *y)*f(c + z + x) - f(2*x)^2*f(2*y)*f(a + 2*y)*f(c + z +
y) )
>      - f(2*y)*f(b + a + 2*x) + f(2*x)*f(b + a + 2*y):
> eq[30] :=
> (1/HessUniv) * ( - f(2*y)*f(z + y)^2*f(a + 2*x)^2 + 2*f(2*y)*f
(z + x
>      )*f(z + y)*f(a + 2*x)*f(a + y + x) + f(2*y)*f(z + x)^2*f
(b + 2*x)^2
>      + 2*f(2*y)*f(z + x)^2*f(b + 2*x)*f(a + y + x) - 4*f(2*
y)*f(z + x)^2*
>      f(a + 2*x)*f(b + y + x) - 2*f(2*y)*f(2*z)*f(y + x)*f(a +
2*x)*f(a + y
>      + x) + 2*f(2*y)*f(y + x)*f(z + y)*f(a + 2*x)*f(a + z +
x) - 2*f(2*y)
>      *f(y + x)*f(z + x)*f(c + 2*x)*f(a + y + x) - 2*f(2*y)*f
(y + x)*f(z +
>      x)*f(b + 2*x)*f(c + 2*x) - 2*f(2*y)*f(y + x)*f(z + x)*f
(b + 2*x)*f(a
>      + z + x) + 4*f(2*y)*f(y + x)*f(z + x)*f(a + 2*x)*f(c +
y + x) + 4*f(
>      2*y)*f(y + x)*f(z + x)*f(a + 2*x)*f(b + z + x) + f(2*y)*
f(y + x)^2*f(
>      c + 2*x)^2 + 2*f(2*y)*f(y + x)^2*f(c + 2*x)*f(a + z + x)
- 4*f(2*y)*
>      f(y + x)^2*f(a + 2*x)*f(c + z + x) - 2*f(2*y)^2*f(z + x)
*f(a + 2*x)*
>      f(a + z + x) + f(2*y)^2*f(2*z)*f(a + 2*x)^2 + f(2*x)*f(z
+ y)^2*f(a
>      + 2*x)*f(a + 2*y) - f(2*x)*f(z + x)*f(z + y)*f(a + 2*y)
*f(b + 2*x)
>      - 2*f(2*x)*f(z + x)*f(z + y)*f(a + 2*y)*f(a + y + x) +
f(2*x)*f(z +
>      x)*f(z + y)*f(a + 2*x)*f(b + 2*y) + 2*f(2*x)*f(z + x)^2*
f(b + 2*y)*f(
>      a + y + x) - f(2*x)*f(z + x)^2*f(b + 2*x)*f(b + 2*y) +
2*f(2*x)*f(2*z
>      )*f(y + x)*f(a + 2*y)*f(a + y + x) + f(2*x)*f(y + x)*f(z
+ y)*f(a + 2
>      *y)*f(c + 2*x) - 2*f(2*x)*f(y + x)*f(z + y)*f(a + 2*y)*f
(a + z + x)
>      - f(2*x)*f(y + x)*f(z + y)*f(a + 2*x)*f(c + 2*y) - 2*f
(2*x)*f(y + x)
>      *f(z + x)*f(c + 2*y)*f(a + y + x) + f(2*x)*f(y + x)*f(z
+ x)*f(b + 2*
>      y)*f(c + 2*x) - 2*f(2*x)*f(y + x)*f(z + x)*f(b + 2*y)*f
(a + z + x) +
>      f(2*x)*f(y + x)*f(z + x)*f(b + 2*x)*f(c + 2*y) + 2*f(2*
x)*f(y + x)^2*
>      f(c + 2*y)*f(a + z + x) - f(2*x)*f(y + x)^2*f(c + 2*x)*f
(c + 2*y) +
>      f(2*x)*f(2*y)*f(z + y)*f(b + 2*x)*f(c + 2*x) - f(2*x)*f
(2*y)*f(z + y)
>      *f(a + 2*x)*f(c + y + x) - f(2*x)*f(2*y)*f(z + y)*f(a +
2*x)*f(b + z

```

```

> + x) - f(2*x)*f(2*y)*f(z + y)*f(a + 2*x)*f(a + z + y) +
2*f(2*x)*f(2
> *y)*f(z + x)*f(c + 2*x)*f(b + y + x) - f(2*x)*f(2*y)*f(z
+ x)*f(b + 2
> *x)*f(c + y + x) - f(2*x)*f(2*y)*f(z + x)*f(b + 2*x)*f(b
+ z + x) +
> f(2*x)*f(2*y)*f(z + x)*f(b + 2*x)*f(a + z + y) + 4*f(2*
x)*f(2*y)*f(z
> + x)*f(a + z + x)*f(b + y + x) - 4*f(2*x)*f(2*y)*f(z +
x)*f(a + y +
> x)*f(b + z + x) + 2*f(2*x)*f(2*y)*f(z + x)*f(a + 2*y)*f
(a + z + x) -
> f(2*x)*f(2*y)*f(z + x)*f(a + 2*x)*f(c + 2*y) - 1/2*f(2*
x)*f(2*y)*f(2*
> z)*f(b + 2*x)^2 + f(2*x)*f(2*y)*f(2*z)*f(a + 2*x)*f(b +
y + x) - 1/2*
> f(2*x)*f(2*y)*f(2*z)*f(a + 2*x)*f(a + 2*y) - f(2*x)*f(2*
y)*f(y + x)*
> f(c + 2*x)*f(c + y + x) - f(2*x)*f(2*y)*f(y + x)*f(c +
2*x)*f(b + z
> + x) - f(2*x)*f(2*y)*f(y + x)*f(c + 2*x)*f(a + z + y) +
2*f(2*x)*f(2
> *y)*f(y + x)*f(b + 2*x)*f(c + z + x) - 4*f(2*x)*f(2*y)*f
(y + x)*f(a
> + z + x)*f(c + y + x) + 4*f(2*x)*f(2*y)*f(y + x)*f(a +
y + x)*f(c +
> z + x) + 2*f(2*x)*f(2*y)*f(y + x)*f(a + 2*x)*f(c + z +
y) - f(2*x)*f(
> 2*y)*f(y + x)*f(a + 2*x)*f(b + 2*z) - 1/2*f(2*x)*f(2*y)
^2*f(c + 2*x)^
> 2 + f(2*x)*f(2*y)^2*f(a + 2*x)*f(c + z + x) + 1/2*f(2*x)
*f(2*y)^2*f(a
> + 2*x)*f(a + 2*z) + 2*f(2*x)^2*f(z + y)*f(c + 2*y)*f(a
+ y + x) - f(
> 2*x)^2*f(z + y)*f(b + 2*y)*f(c + 2*x) - f(2*x)^2*f(z +
y)*f(a + 2*y)*
> f(c + y + x) + f(2*x)^2*f(z + y)*f(a + 2*y)*f(b + z + x)
+ f(2*x)^2*
> f(z + y)*f(a + 2*y)*f(a + z + y) - f(2*x)^2*f(z + x)*f(b
+ 2*y)*f(c
> + y + x) + f(2*x)^2*f(z + x)*f(b + 2*y)*f(b + z + x) -
f(2*x)^2*f(z
> + x)*f(b + 2*y)*f(a + z + y) + f(2*x)^2*f(z + x)*f(a +
2*y)*f(c + 2*
> y) - f(2*x)^2*f(2*z)*f(b + 2*y)*f(a + y + x) + 1/2*f(2*
x)^2*f(2*z)*f(
> b + 2*x)*f(b + 2*y) - 1/2*f(2*x)^2*f(2*z)*f(a + 2*y)^2 +
f(2*x)^2*f(y
> + x)*f(c + 2*y)*f(c + y + x) - f(2*x)^2*f(y + x)*f(c +
2*y)*f(b + z
> + x) - f(2*x)^2*f(y + x)*f(c + 2*y)*f(a + z + y) + f(2*
x)^2*f(y + x)
> *f(a + 2*z)*f(b + 2*y) + f(2*x)^2*f(2*y)*f(c + 2*x)*f(c
+ 2*y) + 2*f(
> 2*x)^2*f(2*y)*f(b + z + x)*f(c + y + x) + f(2*x)^2*f(2*
y)*f(b + 2*z)*
> f(a + y + x) - 2*f(2*x)^2*f(2*y)*f(b + y + x)*f(c + z +

```

```

x) - f(2*x)^2
>      *f(2*y)*f(b + 2*x)*f(c + z + y) + 1/2*f(2*x)^2*f(2*y)*f
(b + 2*x)*f(b
>      + 2*z) + 2*f(2*x)^2*f(2*y)*f(a + z + y)*f(c + y + x) -
f(2*x)^2*f(2*
>      y)*f(a + 2*z)*f(b + y + x) - 2*f(2*x)^2*f(2*y)*f(a + y +
x)*f(c + z
>      + y) - f(2*x)^2*f(2*y)*f(a + 2*y)*f(c + z + x) - 1/2*f
(2*x)^2*f(2*y)
>      *f(a + 2*y)*f(a + 2*z) - 1/2*f(2*x)^3*f(c + 2*y)^2 + f
(2*x)^3*f(b + 2
>      *y)*f(c + z + y) - 1/2*f(2*x)^3*f(b + 2*y)*f(b + 2*z) )
>
>      - f(2*y)*f(2*a + 2*x) + f(2*x)*f(2*a + 2*y):
> #
> # Result
> l := 0:
>
> for i from 1 to 30 do
>   if simplify(eq[i]) = 0 then
>     l := l+1; eqn[i] := 0;
>   else
>     eqn[i] := collect(simplify(eq[i])*denom(eq[i]), [a, b, c],
distributed);
>     print(i, eqn[i] = 0);
>   end if;
> end do;
>
> if l = 30 then
>   print(No*conditions);
> end if;
> #
> #

```

$$u_{xx} := 1$$

$$u_{yy} := 1$$

$$u_{zz} := -2a$$

$$u_{xy} := \lambda c$$

$$u_{xz} := c - \lambda b$$

$$u_{yz} := 0$$

$$HessUniv := 2a\lambda^2 c^2 - (c - \lambda b)^2 - 2a$$

$$1, -4a\lambda^2 c = 0$$

$$2, 4\lambda = 0$$

$$4, 4\lambda^3 b - 4\lambda^2 c = 0$$

$$5, 4a = 0$$

$$7, -2\lambda = 0$$

$$8, 2\lambda^2 c = 0$$

$$9, 2\lambda^2 c = 0$$

$$10, -2\lambda + 4\lambda^3 c^2 = 0$$

$$11, 2\lambda = 0$$

$$12, 2\lambda^2 c = 0$$

$$13, 4\lambda^2 b - 4\lambda c = 0$$

$$14, 2 = 0$$

$$15, 2\lambda^2 b = 0$$

$$16, 2 = 0$$

$$18, -4c + 4\lambda b = 0$$

$$19, -4\lambda^2 c = 0$$

$$20, -4a\lambda^2 = 0$$

$$21, -2 = 0$$

$$22, -2\lambda^2 b = 0$$

$$23, -2\lambda^2 b = 0$$

$$24, -2 + 4\lambda^2 c^2 - 4\lambda^3 c b + 4a\lambda^2 = 0$$

$$26, -2\lambda^2 = 0$$

$$27, -4\lambda^3 c = 0$$

$$28, 2\lambda^2 = 0$$

$$30, -2\lambda^2 = 0$$

(1)
