# Supplementary material for: Dispersionless integrable systems in 3D and Einstein-Weyl geometry
Source: arXiv:1208.2728 ancillary file (2013-05-09)
Supplement: Supplementary file 16 [file Integrability_conditions-type_II_n.pdf]

```

> # NB1: the coefficient Cyy at u_{yy} is normalized to 1
> # NB2: the coefficients of the mixed derivatives, like Cxy,
    should be divided by 2
> HessUniv := -f(2*z)*f(y+x)^2 + 2*f(y+x)*f(z+x)*f(z+y) - f(2*y)*f(z+x)
    ^2 - f(2*x)*f(z+y)^2 + f(2*x)*f(2*y)*f(2*z);
> eq[1] :=
> (1/HessUniv) * ( f(2*z)*f(z+y)^2*f(a+2*y)*f(c+2*x) - 2*f(2*
    z)*
>      f(z+x)*f(z+y)*f(a+2*y)*f(c+y+x) + f(2*z)*f(z+x)
    ^2*f(a+2
>      *y)*f(c+2*y) - 1/2*f(2*z)^2*f(z+y)*f(a+2*y)*f(b+
    2*x) + 1/2*f(
>      2*z)^2*f(z+y)*f(a+2*x)*f(b+2*y) + f(2*z)^2*f(z+
    x)*f(b+2*y)*
>      f(a+y+x) - 1/2*f(2*z)^2*f(z+x)*f(b+2*x)*f(b+2*
    y) - 1/2*f(2*
>      z)^2*f(z+x)*f(a+2*y)^2 + 1/2*f(2*z)^2*f(y+x)*f(b+
    2*y)*f(c+2
>      *x) - f(2*z)^2*f(y+x)*f(b+2*y)*f(a+z+x) + 1/2*f
    (2*z)^2*f(y+
>      x)*f(b+2*x)*f(c+2*y) + f(2*z)^2*f(y+x)*f(a+2*y)*
    f(c+y+x)
>      + f(2*z)^2*f(y+x)*f(a+2*y)*f(a+z+y) - f(2*z)*f
    (y+x)*f(z+
>      y)*f(c+2*x)*f(c+2*y) - f(2*z)*f(y+x)*f(z+y)*f(a
    +2*y)*f(a+
>      2*z) - 2*f(2*z)*f(y+x)*f(z+x)*f(c+2*y)*f(a+z+
    y) + 2*f(y+x
>      )*f(z+x)*f(z+y)*f(a+2*z)*f(c+2*y) - f(2*y)*f(z+
    y)^2*f(a+2
>      *x)*f(c+2*z) + 2*f(2*y)*f(z+x)*f(z+y)*f(c+2*z)*f
    (a+y+x)
>      - f(2*y)*f(z+x)^2*f(a+2*z)*f(c+2*y) - f(2*y)*f(z
    +x)^2*f(a+
>      2*y)*f(c+2*z) - f(2*y)*f(2*z)*f(z+y)*f(c+2*x)*f(a
    +z+y) - 1/
>      2*f(2*y)*f(2*z)*f(z+y)*f(a+2*z)*f(b+2*x) + f(2*y)*
    f(2*z)*f(z+
>      y)*f(a+2*x)*f(c+z+y) + 1/2*f(2*y)*f(2*z)*f(z+y)*
    f(a+2*x)*f(
>      b+2*z) + 1/2*f(2*y)*f(2*z)*f(z+x)*f(c+2*x)*f(c+
    2*y) - f(2*y)*
>      f(2*z)*f(z+x)*f(b+2*z)*f(a+y+x) + 1/2*f(2*y)*f
    (2*z)*f(z+x)*
>      f(b+2*x)*f(b+2*z) + 2*f(2*y)*f(2*z)*f(z+x)*f(a+z
    +y)*f(c+y
>      +x) - 2*f(2*y)*f(2*z)*f(z+x)*f(a+y+x)*f(c+z+
    y) + f(2*y)*
>      f(2*z)*f(z+x)*f(a+2*y)*f(c+z+x) + f(2*y)*f(2*z)*
    f(z+x)*f(a
>      +2*y)*f(a+2*z) + f(2*y)*f(2*z)^2*f(b+2*x)*f(a+z
    +y) - 1/2*f(
>      2*y)*f(2*z)^2*f(a+2*y)*f(c+2*x) - 1/2*f(2*y)*f(2*z)
    ^2*f(a+2*x)*
>      f(c+2*y) - f(2*y)*f(2*z)^2*f(a+2*x)*f(b+z+y) -
    1/2*f(2*y)*f(2

```

```

> *z)*f(y + x)*f(b + 2*z)*f(c + 2*x) + f(2*y)*f(2*z)*f(y +
x)*f(b + 2*z
> )*f(a + z + x) - 1/2*f(2*y)*f(2*z)*f(y + x)*f(b + 2*x)*f
(c + 2*z) - 2
> *f(2*y)*f(2*z)*f(y + x)*f(a + z + y)*f(c + z + x) + 2*f
(2*y)*f(2*z)*
> f(y + x)*f(a + z + x)*f(c + z + y) - f(2*y)*f(2*z)*f(y +
x)*f(a + 2*z
> )*f(c + y + x) - f(2*y)*f(2*z)*f(y + x)*f(a + 2*z)*f(a +
z + y) - 2*
> f(2*y)*f(y + x)*f(z + y)*f(c + 2*z)*f(a + z + x) + f(2*
y)*f(y + x)*f(
> z + y)*f(c + 2*x)*f(c + 2*z) + 2*f(2*y)*f(y + x)*f(z +
y)*f(a + 2*z)*
> f(c + z + x) + f(2*y)*f(y + x)*f(z + y)*f(a + 2*z)^2 +
2*f(2*y)*f(y
> + x)*f(z + x)*f(c + 2*z)*f(a + z + y) - f(2*y)*f(y + x)
^2*f(a + 2*z)
> *f(c + 2*z) - 1/2*f(2*y)^2*f(z + x)*f(c + 2*x)*f(c + 2*
z) - f(2*y)^2*
> f(z + x)*f(a + 2*z)*f(c + z + x) - 1/2*f(2*y)^2*f(z + x)
*f(a + 2*z)^2
> + 1/2*f(2*y)^2*f(2*z)*f(a + 2*z)*f(c + 2*x) + 1/2*f(2*
y)^2*f(2*z)*f(
> a + 2*x)*f(c + 2*z) - f(2*x)*f(z + y)^2*f(a + 2*z)*f(c +
2*y) + f(2*x
> )*f(2*z)*f(z + y)*f(c + 2*y)*f(c + y + x) + f(2*x)*f(2*
z)*f(z + y)*f(
> c + 2*y)*f(a + z + y) - f(2*x)*f(2*z)*f(z + y)*f(b + 2*
y)*f(c + z + x
> ) + 1/2*f(2*x)*f(2*z)*f(z + y)*f(a + 2*z)*f(b + 2*y) +
1/2*f(2*x)*f(2
> *z)*f(z + y)*f(a + 2*y)*f(b + 2*z) - 1/2*f(2*x)*f(2*z)*f
(z + x)*f(c
> + 2*y)^2 + f(2*x)*f(2*z)*f(z + x)*f(b + 2*y)*f(c + z +
y) - 1/2*f(2*
> x)*f(2*z)*f(z + x)*f(b + 2*y)*f(b + 2*z) - f(2*x)*f(2*z)
^2*f(b + 2*y)
> *f(c + y + x) + f(2*x)*f(2*z)^2*f(b + 2*y)*f(b + z + x)
- f(2*x)*f(2*
> z)^2*f(b + 2*y)*f(a + z + y) - 1/2*f(2*x)*f(2*z)*f(y +
x)*f(b + 2*z)*
> f(c + 2*y) + 1/2*f(2*x)*f(2*z)*f(y + x)*f(b + 2*y)*f(c +
2*z) - f(2*x
> )*f(2*y)*f(z + y)*f(c + 2*z)*f(c + y + x) + 2*f(2*x)*f
(2*y)*f(z + y)*
> f(c + 2*z)*f(b + z + x) - f(2*x)*f(2*y)*f(z + y)*f(b +
2*z)*f(c + z
> + x) - f(2*x)*f(2*y)*f(z + y)*f(a + 2*z)*f(c + z + y) -
f(2*x)*f(2*y
> )*f(z + y)*f(a + 2*z)*f(b + 2*z) - 2*f(2*x)*f(2*y)*f(z +
x)*f(c + 2*z
> )*f(b + z + y) + 1/2*f(2*x)*f(2*y)*f(z + x)*f(c + 2*y)*f
(c + 2*z) +
> f(2*x)*f(2*y)*f(z + x)*f(b + 2*z)*f(c + z + y) + 1/2*f
(2*x)*f(2*y)*f(
> z + x)*f(b + 2*z)^2 + 2*f(2*x)*f(2*y)*f(2*z)*f(b + z +

```

```

y)*f(c + z + x
>      ) - 2*f(2*x)*f(2*y)*f(2*z)*f(b + z + x)*f(c + z + y) + f
(2*x)*f(2*y)*
>      f(2*z)*f(b + 2*z)*f(c + y + x) - f(2*x)*f(2*y)*f(2*z)*f
(b + 2*z)*f(b
>      + z + x) + 1/2*f(2*x)*f(2*y)*f(2*z)*f(a + 2*z)*f(c + 2*
y) + f(2*x)*
>      f(2*y)*f(2*z)*f(a + 2*z)*f(b + z + y) - 1/2*f(2*x)*f(2*
y)*f(2*z)*f(a
>      + 2*y)*f(c + 2*z) + f(2*x)*f(2*y)^2*f(a + 2*z)*f(c + 2*
z) )
>
>      - f(a + 2*z)*f(c + 2*y) + f(2*z)*f(c + a + 2*y) - f(2*y)*f
(c + a + 2*z)
>      :
>
> eq[2] :=
> (1/HessUniv) * ( 2*f(z + y)^3*f(a + 2*x)*f(a + 2*y) - 2*f(z + x)
*f(z
>      + y)^2*f(a + 2*y)*f(b + 2*x) - 4*f(z + x)*f(z + y)^2*f
(a + 2*y)*f(a
>      + y + x) + 2*f(z + x)*f(z + y)^2*f(a + 2*x)*f(b + 2*y)
+ 4*f(z + x)^
>      2*f(z + y)*f(b + 2*y)*f(a + y + x) - 2*f(z + x)^2*f(z +
y)*f(b + 2*x)
>      *f(b + 2*y) + 4*f(2*z)*f(y + x)*f(z + y)*f(a + 2*y)*f(a
+ y + x) + 2*
>      f(y + x)*f(z + y)^2*f(a + 2*y)*f(c + 2*x) - 4*f(y + x)*f
(z + y)^2*f(a
>      + 2*y)*f(a + z + x) - 2*f(y + x)*f(z + y)^2*f(a + 2*x)*
f(c + 2*y) -
>      4*f(y + x)*f(z + x)*f(z + y)*f(c + 2*y)*f(a + y + x) +
2*f(y + x)*f(z
>      + x)*f(z + y)*f(b + 2*y)*f(c + 2*x) - 4*f(y + x)*f(z +
x)*f(z + y)*
>      f(b + 2*y)*f(a + z + x) + 2*f(y + x)*f(z + x)*f(z + y)*f
(b + 2*x)*f(c
>      + 2*y) + 4*f(y + x)^2*f(z + y)*f(c + 2*y)*f(a + z + x)
- 2*f(y + x)^
>      2*f(z + y)*f(c + 2*x)*f(c + 2*y) - 2*f(2*y)*f(z + y)^2*f
(a + 2*x)*f(a
>      + z + y) + 2*f(2*y)*f(z + x)*f(z + y)*f(b + 2*x)*f(a +
z + y) + 4*f(
>      2*y)*f(z + x)*f(z + y)*f(a + y + x)*f(a + z + y) + 4*f
(2*y)*f(z + x)*
>      f(z + y)*f(a + 2*y)*f(a + z + x) - 2*f(2*y)*f(z + x)*f(z
+ y)*f(a + 2
>      *x)*f(b + z + y) + 2*f(2*y)*f(z + x)^2*f(b + 2*x)*f(b +
z + y) - 4*f(
>      2*y)*f(z + x)^2*f(a + y + x)*f(b + z + y) - 2*f(2*y)*f
(2*z)*f(z + y)*
>      f(a + 2*x)*f(a + 2*y) + f(2*y)*f(2*z)*f(z + x)*f(a + 2*
y)*f(b + 2*x)
>      - f(2*y)*f(2*z)*f(z + x)*f(a + 2*x)*f(b + 2*y) - 4*f(2*
y)*f(2*z)*f(y
>      + x)*f(a + y + x)*f(a + z + y) - f(2*y)*f(2*z)*f(y + x)
*f(a + 2*y)*

```

```

>      f(c + 2*x) + f(2*y)*f(2*z)*f(y + x)*f(a + 2*x)*f(c + 2*
> y) - 2*f(2*y)*
>      f(y + x)*f(z + y)*f(c + 2*x)*f(a + z + y) + 4*f(2*y)*f(y
> + x)*f(z + y
>      )*f(a + z + x)*f(a + z + y) + 2*f(2*y)*f(y + x)*f(z + y)
> *f(a + 2*x)*
>      f(c + z + y) - 2*f(2*y)*f(y + x)*f(z + x)*f(c + 2*x)*f(b
> + z + y) - 2
>      *f(2*y)*f(y + x)*f(z + x)*f(b + 2*x)*f(c + z + y) + 4*f
> (2*y)*f(y + x)
>      *f(z + x)*f(a + z + x)*f(b + z + y) + 4*f(2*y)*f(y + x)*
> f(z + x)*f(a
>      + y + x)*f(c + z + y) + 2*f(2*y)*f(y + x)^2*f(c + 2*x)*
> f(c + z + y)
>      - 4*f(2*y)*f(y + x)^2*f(a + z + x)*f(c + z + y) - 4*f
> (2*y)^2*f(z + x
>      )*f(a + z + x)*f(a + z + y) - f(2*y)^2*f(z + x)*f(a + 2*
> z)*f(b + 2*x)
>      + f(2*y)^2*f(z + x)*f(a + 2*x)*f(b + 2*z) + 2*f(2*y)^2*
> f(2*z)*f(a +
>      2*x)*f(a + z + y) + f(2*y)^2*f(y + x)*f(a + 2*z)*f(c +
> 2*x) - f(2*y)^
>      2*f(y + x)*f(a + 2*x)*f(c + 2*z) + 4*f(2*x)*f(z + y)^2*f
> (c + 2*y)*f(a
>      + y + x) - 2*f(2*x)*f(z + y)^2*f(b + 2*y)*f(c + 2*x) -
> 2*f(2*x)*f(z
>      + y)^2*f(a + 2*y)*f(c + y + x) + 2*f(2*x)*f(z + y)^2*f
> (a + 2*y)*f(b
>      + z + x) + 2*f(2*x)*f(z + y)^2*f(a + 2*y)*f(a + z + y)
> - 2*f(2*x)*f(
>      z + x)*f(z + y)*f(b + 2*y)*f(c + y + x) + 2*f(2*x)*f(z +
> x)*f(z + y)*
>      f(b + 2*y)*f(b + z + x) - 2*f(2*x)*f(z + x)*f(z + y)*f(b
> + 2*y)*f(a
>      + z + y) + 2*f(2*x)*f(z + x)*f(z + y)*f(a + 2*y)*f(c +
> 2*y) - 2*f(2*
>      x)*f(2*z)*f(z + y)*f(b + 2*y)*f(a + y + x) + f(2*x)*f(2*
> z)*f(z + y)*
>      f(b + 2*x)*f(b + 2*y) - f(2*x)*f(2*z)*f(z + y)*f(a + 2*
> y)^2 + 2*f(2*x
>      )*f(y + x)*f(z + y)*f(c + 2*y)*f(c + y + x) - 2*f(2*x)*f
> (y + x)*f(z
>      + y)*f(c + 2*y)*f(b + z + x) - 2*f(2*x)*f(y + x)*f(z +
> y)*f(c + 2*y)
>      *f(a + z + y) + 2*f(2*x)*f(y + x)*f(z + y)*f(a + 2*z)*f
> (b + 2*y) - 2*
>      f(2*x)*f(2*y)*f(z + y)*f(c + 2*y)*f(a + z + x) + f(2*x)*
> f(2*y)*f(z +
>      y)*f(c + 2*x)*f(c + 2*y) + 2*f(2*x)*f(2*y)*f(z + y)*f(c
> + 2*x)*f(b +
>      z + y) + 2*f(2*x)*f(2*y)*f(z + y)*f(a + z + y)*f(c + y +
> x) - 2*f(2*x
>      )*f(2*y)*f(z + y)*f(a + z + y)*f(b + z + x) - 2*f(2*x)*f
> (2*y)*f(z + y
>      )*f(a + z + y)^2 - 4*f(2*x)*f(2*y)*f(z + y)*f(a + y + x)
> *f(c + z + y)
>      - f(2*x)*f(2*y)*f(z + y)*f(a + 2*y)*f(a + 2*z) + 2*f(2*

```

```

x)*f(2*y)*f(z
> + x)*f(b + z + y)*f(c + y + x) - 2*f(2*x)*f(2*y)*f(z +
x)*f(b + z +
> x)*f(b + z + y) + 2*f(2*x)*f(2*y)*f(z + x)*f(a + z + y)*
f(b + z + y)
> - 2*f(2*x)*f(2*y)*f(z + x)*f(a + 2*y)*f(c + z + y) - f
(2*x)*f(2*y)*
> f(2*z)*f(c + 2*y)*f(a + y + x) + 1/2*f(2*x)*f(2*y)*f(2*
z)*f(b + 2*y)*
> f(c + 2*x) + f(2*x)*f(2*y)*f(2*z)*f(b + 2*y)*f(a + z +
x) - 1/2*f(2*x
> )*f(2*y)*f(2*z)*f(b + 2*x)*f(c + 2*y) - f(2*x)*f(2*y)*f
(2*z)*f(b + 2*
> x)*f(b + z + y) + 2*f(2*x)*f(2*y)*f(2*z)*f(a + y + x)*f
(b + z + y) +
> f(2*x)*f(2*y)*f(2*z)*f(a + 2*y)*f(c + y + x) - f(2*x)*f
(2*y)*f(2*z)*
> f(a + 2*y)*f(b + z + x) + f(2*x)*f(2*y)*f(2*z)*f(a + 2*
y)*f(a + z + y
> ) - 2*f(2*x)*f(2*y)*f(y + x)*f(c + y + x)*f(c + z + y) +
2*f(2*x)*f(2
> *y)*f(y + x)*f(b + z + x)*f(c + z + y) + 2*f(2*x)*f(2*y)
*f(y + x)*f(a
> + z + y)*f(c + z + y) - 2*f(2*x)*f(2*y)*f(y + x)*f(a +
2*z)*f(b + z
> + y) + f(2*x)*f(2*y)^2*f(c + 2*z)*f(a + y + x) - f(2*x)
*f(2*y)^2*f(c
> + 2*x)*f(c + z + y) - 1/2*f(2*x)*f(2*y)^2*f(b + 2*z)*f
(c + 2*x) - f(
> 2*x)*f(2*y)^2*f(b + 2*z)*f(a + z + x) + 1/2*f(2*x)*f(2*
y)^2*f(b + 2*x
> )*f(c + 2*z) + 2*f(2*x)*f(2*y)^2*f(a + z + x)*f(c + z +
y) - f(2*x)*
> f(2*y)^2*f(a + 2*z)*f(c + y + x) + f(2*x)*f(2*y)^2*f(a +
2*z)*f(b + z
> + x) + f(2*x)*f(2*y)^2*f(a + 2*z)*f(a + z + y) - f(2*x)
^2*f(z + y)*
> f(c + 2*y)^2 + 2*f(2*x)^2*f(z + y)*f(b + 2*y)*f(c + z +
y) - f(2*x)^2
> *f(z + y)*f(b + 2*y)*f(b + 2*z) + f(2*x)^2*f(2*y)*f(c +
2*y)*f(c + z
> + y) - 2*f(2*x)^2*f(2*y)*f(b + z + y)*f(c + z + y) +
1/2*f(2*x)^2*f(
> 2*y)*f(b + 2*z)*f(c + 2*y) + f(2*x)^2*f(2*y)*f(b + 2*z)*
f(b + z + y)
> - 1/2*f(2*x)^2*f(2*y)*f(b + 2*y)*f(c + 2*z) )
>
> + 2*f(z + y)*f(2*a + 2*y) - 2*f(2*y)*f(2*a + z + y):
>
> eq[3] :=
> (1/HessUniv) * ( f(2*z)*f(z + y)^2*f(b + 2*y)*f(c + 2*x) - 2*f(2*
z)*
> f(z + x)*f(z + y)*f(b + 2*y)*f(c + y + x) + f(2*z)*f(z +
x)^2*f(b + 2
> *y)*f(c + 2*y) + 2*f(2*z)^2*f(z + y)*f(b + 2*y)*f(a + y
+ x) - 1/2*f(
> 2*z)^2*f(z + y)*f(b + 2*x)*f(b + 2*y) - f(2*z)^2*f(z +

```

```

y)*f(a + 2*y)*
> f(b + y + x) - 1/2*f(2*z)^2*f(z + y)*f(a + 2*y)^2 + f(2*
z)^2*f(y + x)
> *f(c + 2*y)*f(b + y + x) + f(2*z)^2*f(y + x)*f(b + 2*y)*
f(b + z + x)
> - 2*f(2*z)^2*f(y + x)*f(b + 2*y)*f(a + z + y) + f(2*z)
^2*f(y + x)*f(
> a + 2*y)*f(c + 2*y) + f(2*z)^2*f(y + x)*f(a + 2*y)*f(b +
z + y) - 2*
> f(2*z)*f(y + x)*f(z + y)*f(b + 2*y)*f(c + z + x) - f(2*
z)*f(y + x)*f(
> z + x)*f(c + 2*y)^2 - 2*f(2*z)*f(y + x)*f(z + x)*f(c +
2*y)*f(b + z
> + y) + 2*f(2*z)*f(y + x)*f(z + x)*f(b + 2*y)*f(c + z +
y) - f(2*z)*
> f(y + x)*f(z + x)*f(b + 2*y)*f(b + 2*z) + 2*f(y + x)*f(z
+ x)*f(z + y
> )*f(b + 2*y)*f(c + 2*z) - f(2*y)*f(z + y)^2*f(b + 2*x)*f
(c + 2*z) + 2
> *f(2*y)*f(z + x)*f(z + y)*f(c + 2*z)*f(b + y + x) - 2*f
(2*y)*f(z + x)
> ^2*f(b + 2*y)*f(c + 2*z) - 1/2*f(2*y)*f(2*z)*f(z + y)*f
(c + 2*x)*f(c
> + 2*y) - f(2*y)*f(2*z)*f(z + y)*f(c + 2*x)*f(b + z + y)
+ f(2*y)*f(2
> *z)*f(z + y)*f(b + 2*x)*f(c + z + y) + 1/2*f(2*y)*f(2*z)
*f(z + y)*f(b
> + 2*x)*f(b + 2*z) - f(2*y)*f(2*z)*f(z + y)*f(a + 2*z)*f
(b + y + x)
> + f(2*y)*f(2*z)*f(z + y)*f(a + 2*y)*f(c + z + x) + f(2*
y)*f(2*z)*f(z
> + x)*f(c + 2*y)*f(c + y + x) + 2*f(2*y)*f(2*z)*f(z + x)
*f(b + z + y)
> *f(c + y + x) - 2*f(2*y)*f(2*z)*f(z + x)*f(b + y + x)*f
(c + z + y) +
> f(2*y)*f(2*z)*f(z + x)*f(b + 2*y)*f(c + z + x) + f(2*y)*
f(2*z)*f(z +
> x)*f(a + 2*z)*f(b + 2*y) - f(2*y)*f(2*z)*f(z + x)*f(a +
2*y)*f(c + z
> + y) - f(2*y)*f(2*z)^2*f(c + 2*y)*f(a + y + x) - f(2*y)
*f(2*z)^2*f(b
> + 2*y)*f(a + z + x) + 2*f(2*y)*f(2*z)^2*f(a + z + y)*f
(b + y + x) -
> 2*f(2*y)*f(2*z)^2*f(a + y + x)*f(b + z + y) + f(2*y)*f
(2*z)^2*f(a + 2
> *y)*f(a + z + y) - f(2*y)*f(2*z)*f(y + x)*f(c + 2*z)*f(b
+ y + x) + 2
> *f(2*y)*f(2*z)*f(y + x)*f(b + z + y)*f(c + z + x) - 2*f
(2*y)*f(2*z)*
> f(y + x)*f(b + z + x)*f(c + z + y) - f(2*y)*f(2*z)*f(y +
x)*f(b + 2*z
> )*f(b + z + x) + f(2*y)*f(2*z)*f(y + x)*f(a + 2*z)*f(b +
z + y) - f(2
> *y)*f(2*z)*f(y + x)*f(a + 2*y)*f(c + 2*z) + 2*f(2*y)*f(y
+ x)*f(z + y
> )*f(c + 2*z)*f(b + z + x) - 2*f(2*y)*f(y + x)*f(z + x)*f
(c + 2*z)*f(b

```

```

> + z + y) + f(2*y)*f(y + x)*f(z + x)*f(c + 2*y)*f(c + 2*
> z) + 2*f(2*y)
> *f(y + x)*f(z + x)*f(b + 2*z)*f(c + z + y) + f(2*y)*f(y
> + x)*f(z + x)
> *f(b + 2*z)^2 - f(2*y)*f(y + x)^2*f(b + 2*z)*f(c + 2*z)
> - 2*f(2*y)^2*
> f(z + y)*f(c + 2*z)*f(a + z + x) + 1/2*f(2*y)^2*f(z + y)
> *f(c + 2*x)*
> f(c + 2*z) + f(2*y)^2*f(z + y)*f(a + 2*z)*f(c + z + x) +
> 1/2*f(2*y)^2
> *f(z + y)*f(a + 2*z)^2 - f(2*y)^2*f(z + x)*f(c + 2*z)*f
> (c + y + x) +
> 2*f(2*y)^2*f(z + x)*f(c + 2*z)*f(a + z + y) - f(2*y)^2*f
> (z + x)*f(b
> + 2*z)*f(c + z + x) - f(2*y)^2*f(z + x)*f(a + 2*z)*f(c
> + z + y) - f(
> 2*y)^2*f(z + x)*f(a + 2*z)*f(b + 2*z) + f(2*y)^2*f(2*z)*
> f(c + 2*z)*f(
> a + y + x) + f(2*y)^2*f(2*z)*f(b + 2*z)*f(a + z + x) -
> 2*f(2*y)^2*f(2
> *z)*f(a + z + y)*f(c + z + x) + 2*f(2*y)^2*f(2*z)*f(a +
> z + x)*f(c +
> z + y) - f(2*y)^2*f(2*z)*f(a + 2*z)*f(a + z + y) - f(2*
> x)*f(z + y)^2*
> f(b + 2*y)*f(c + 2*z) + 1/2*f(2*x)*f(2*z)*f(z + y)*f(c +
> 2*y)^2 + f(2
> *x)*f(2*z)*f(z + y)*f(c + 2*y)*f(b + z + y) + 1/2*f(2*x)
> *f(2*z)*f(z
> + y)*f(b + 2*y)*f(b + 2*z) - f(2*x)*f(2*z)^2*f(b + 2*y)
> *f(c + 2*y)
> - 1/2*f(2*x)*f(2*y)*f(z + y)*f(c + 2*y)*f(c + 2*z) - f
> (2*x)*f(2*y)*
> f(z + y)*f(b + 2*z)*f(c + z + y) - 1/2*f(2*x)*f(2*y)*f(z
> + y)*f(b + 2
> *z)^2 + f(2*x)*f(2*y)*f(2*z)*f(b + 2*y)*f(c + 2*z) + f
> (2*x)*f(2*y)^2*
> f(b + 2*z)*f(c + 2*z) )

> - f(b + 2*y)*f(c + 2*z) + f(2*z)*f(c + b + 2*y) - f(2*y)*f
> (c + b + 2*z)
> :

> eq[4] :=
> (1/HessUniv) * ( 2*f(z + x)*f(z + y)^2*f(a + 2*x)*f(a + 2*y) -
> 2*f(z
> + x)^2*f(z + y)*f(a + 2*y)*f(b + 2*x) - 4*f(z + x)^2*f
> (z + y)*f(a +
> 2*y)*f(a + y + x) + 2*f(z + x)^2*f(z + y)*f(a + 2*x)*f(b
> + 2*y) + 4*
> f(z + x)^3*f(b + 2*y)*f(a + y + x) - 2*f(z + x)^3*f(b +
> 2*x)*f(b + 2*
> y) + 4*f(2*z)*f(y + x)*f(z + x)*f(a + 2*y)*f(a + y + x)
> + 2*f(y + x)*
> f(z + x)*f(z + y)*f(a + 2*y)*f(c + 2*x) - 4*f(y + x)*f(z
> + x)*f(z + y
> )*f(a + 2*y)*f(a + z + x) - 2*f(y + x)*f(z + x)*f(z + y)
> *f(a + 2*x)*

```

```

>      f(c + 2*y) - 4*f(y + x)*f(z + x)^2*f(c + 2*y)*f(a + y +
>      x) + 2*f(y +
>      x)*f(z + x)^2*f(b + 2*y)*f(c + 2*x) - 4*f(y + x)*f(z +
>      x)^2*f(b + 2*y
>      )*f(a + z + x) + 2*f(y + x)*f(z + x)^2*f(b + 2*x)*f(c +
>      2*y) + 4*f(y
>      + x)^2*f(z + x)*f(c + 2*y)*f(a + z + x) - 2*f(y + x)^2*
>      f(z + x)*f(c
>      + 2*x)*f(c + 2*y) - 2*f(2*y)*f(z + y)^2*f(a + 2*x)*f(a
>      + z + x) - 2*
>      f(2*y)*f(z + x)*f(z + y)*f(b + 2*x)*f(a + z + x) + 4*f
>      (2*y)*f(z + x)*
>      f(z + y)*f(a + y + x)*f(a + z + x) + 2*f(2*y)*f(z + x)*f
>      (z + y)*f(a
>      + 2*x)*f(b + z + x) + 2*f(2*y)*f(z + x)^2*f(b + 2*x)*f
>      (b + z + x) +
>      4*f(2*y)*f(z + x)^2*f(b + 2*x)*f(a + z + y) - 4*f(2*y)*f
>      (z + x)^2*f(a
>      + y + x)*f(b + z + x) + 4*f(2*y)*f(z + x)^2*f(a + 2*y)*
>      f(a + z + x)
>      - 4*f(2*y)*f(z + x)^2*f(a + 2*x)*f(b + z + y) + 2*f(2*
>      y)*f(2*z)*f(z
>      + x)*f(b + 2*x)*f(a + y + x) - 2*f(2*y)*f(2*z)*f(z + x)
>      *f(a + 2*x)*
>      f(b + y + x) - 2*f(2*y)*f(2*z)*f(z + x)*f(a + 2*x)*f(a +
>      2*y) - 2*f(2
>      *y)*f(2*z)*f(y + x)*f(c + 2*x)*f(a + y + x) - 4*f(2*y)*f
>      (2*z)*f(y + x
>      )*f(a + y + x)*f(a + z + x) + 2*f(2*y)*f(2*z)*f(y + x)*f
>      (a + 2*x)*f(c
>      + y + x) + 2*f(2*y)*f(y + x)*f(z + y)*f(c + 2*x)*f(a +
>      z + x) + 4*f(
>      2*y)*f(y + x)*f(z + y)*f(a + z + x)^2 - 2*f(2*y)*f(y +
>      x)*f(z + y)*f(
>      a + 2*x)*f(c + z + x) - 2*f(2*y)*f(y + x)*f(z + x)*f(c +
>      2*x)*f(b + z
>      + x) - 4*f(2*y)*f(y + x)*f(z + x)*f(c + 2*x)*f(a + z +
>      y) - 2*f(2*y)
>      *f(y + x)*f(z + x)*f(b + 2*x)*f(c + z + x) + 4*f(2*y)*f
>      (y + x)*f(z +
>      x)*f(a + z + x)*f(b + z + x) - 2*f(2*y)*f(y + x)*f(z +
>      x)*f(a + 2*z)*
>      f(b + 2*x) + 4*f(2*y)*f(y + x)*f(z + x)*f(a + y + x)*f(c
>      + z + x) + 4
>      *f(2*y)*f(y + x)*f(z + x)*f(a + 2*x)*f(c + z + y) + 2*f
>      (2*y)*f(y + x)
>      *f(z + x)*f(a + 2*x)*f(b + 2*z) + 2*f(2*y)*f(y + x)^2*f
>      (c + 2*x)*f(c
>      + z + x) - 4*f(2*y)*f(y + x)^2*f(a + z + x)*f(c + z +
>      x) + 2*f(2*y)*
>      f(y + x)^2*f(a + 2*z)*f(c + 2*x) - 2*f(2*y)*f(y + x)^2*f
>      (a + 2*x)*f(c
>      + 2*z) - 4*f(2*y)^2*f(z + x)*f(a + z + x)^2 + 2*f(2*y)
>      ^2*f(2*z)*f(a
>      + 2*x)*f(a + z + x) + 4*f(2*x)*f(z + x)*f(z + y)*f(c +
>      2*y)*f(a + y
>      + x) - 2*f(2*x)*f(z + x)*f(z + y)*f(b + 2*y)*f(c + 2*x)

```



```

- 2*f(2*x)*
> f(z + x)*f(z + y)*f(a + 2*y)*f(c + y + x) + 2*f(2*x)*f(z
+ x)*f(z + y
> )*f(a + 2*y)*f(b + z + x) + 2*f(2*x)*f(z + x)*f(z + y)*f
(a + 2*y)*f(a
> + z + y) - 2*f(2*x)*f(z + x)^2*f(b + 2*y)*f(c + y + x)
+ 2*f(2*x)*f(
> z + x)^2*f(b + 2*y)*f(b + z + x) - 2*f(2*x)*f(z + x)^2*f
(b + 2*y)*f(a
> + z + y) + 2*f(2*x)*f(z + x)^2*f(a + 2*y)*f(c + 2*y) -
2*f(2*x)*f(2*
> z)*f(z + x)*f(b + 2*y)*f(a + y + x) + f(2*x)*f(2*z)*f(z
+ x)*f(b + 2*
> x)*f(b + 2*y) - f(2*x)*f(2*z)*f(z + x)*f(a + 2*y)^2 + 2*
f(2*x)*f(y +
> x)*f(z + x)*f(c + 2*y)*f(c + y + x) - 2*f(2*x)*f(y + x)*
f(z + x)*f(c
> + 2*y)*f(b + z + x) - 2*f(2*x)*f(y + x)*f(z + x)*f(c +
2*y)*f(a + z
> + y) + 2*f(2*x)*f(y + x)*f(z + x)*f(a + 2*z)*f(b + 2*y)
+ 2*f(2*x)*
> f(2*y)*f(z + y)*f(b + 2*x)*f(c + z + x) - 2*f(2*x)*f(2*
y)*f(z + y)*f(
> a + z + x)*f(c + y + x) - 2*f(2*x)*f(2*y)*f(z + y)*f(a +
z + x)*f(b
> + z + x) - 2*f(2*x)*f(2*y)*f(z + y)*f(a + z + x)*f(a +
z + y) + f(2*
> x)*f(2*y)*f(z + y)*f(a + 2*z)*f(b + 2*x) - f(2*x)*f(2*y)
*f(z + y)*f(a
> + 2*x)*f(b + 2*z) - 2*f(2*x)*f(2*y)*f(z + x)*f(c + 2*y)
*f(a + z + x)
> + f(2*x)*f(2*y)*f(z + x)*f(c + 2*x)*f(c + 2*y) + 2*f(2*
x)*f(2*y)*f(z
> + x)*f(c + 2*x)*f(b + z + y) + 2*f(2*x)*f(2*y)*f(z + x)
*f(b + z + x)
> *f(c + y + x) - 2*f(2*x)*f(2*y)*f(z + x)*f(b + z + x)^2
- 2*f(2*x)*f(
> 2*y)*f(z + x)*f(b + 2*x)*f(c + z + y) + 4*f(2*x)*f(2*y)*
f(z + x)*f(a
> + z + y)*f(c + y + x) - 2*f(2*x)*f(2*y)*f(z + x)*f(a +
z + y)*f(b +
> z + x) + 4*f(2*x)*f(2*y)*f(z + x)*f(a + z + x)*f(b + z +
y) - 4*f(2*x
> )*f(2*y)*f(z + x)*f(a + y + x)*f(c + z + y) - 2*f(2*x)*f
(2*y)*f(z + x
> )*f(a + 2*y)*f(c + z + x) - f(2*x)*f(2*y)*f(z + x)*f(a +
2*y)*f(a + 2
> *z) + f(2*x)*f(2*y)*f(2*z)*f(c + 2*x)*f(b + y + x) - f
(2*x)*f(2*y)*f(
> 2*z)*f(b + 2*x)*f(c + y + x) - f(2*x)*f(2*y)*f(2*z)*f(b
+ 2*x)*f(b +
> z + x) - f(2*x)*f(2*y)*f(2*z)*f(b + 2*x)*f(a + z + y) +
2*f(2*x)*f(2*
> y)*f(2*z)*f(a + z + x)*f(b + y + x) + 1/2*f(2*x)*f(2*y)*
f(2*z)*f(a +
> 2*y)*f(c + 2*x) + f(2*x)*f(2*y)*f(2*z)*f(a + 2*y)*f(a +
z + x) - 1/2*

```

```

>      f(2*x)*f(2*y)*f(2*z)*f(a + 2*x)*f(c + 2*y) + f(2*x)*f(2*
> y)*f(2*z)*f(a
>      + 2*x)*f(b + z + y) + 2*f(2*x)*f(2*y)*f(y + x)*f(c + 2*
> z)*f(a + y +
>      x) - 2*f(2*x)*f(2*y)*f(y + x)*f(c + y + x)*f(c + z + x)
> + 2*f(2*x)*f(
>      2*y)*f(y + x)*f(b + z + x)*f(c + z + x) - f(2*x)*f(2*y)*
> f(y + x)*f(b
>      + 2*z)*f(c + 2*x) - 2*f(2*x)*f(2*y)*f(y + x)*f(b + 2*z)
> *f(a + z + x)
>      + f(2*x)*f(2*y)*f(y + x)*f(b + 2*x)*f(c + 2*z) + 2*f(2*
> x)*f(2*y)*f(y
>      + x)*f(a + z + y)*f(c + z + x) - 2*f(2*x)*f(2*y)*f(y +
> x)*f(a + 2*z)
>      *f(c + y + x) - f(2*x)*f(2*y)^2*f(c + 2*x)*f(c + z + x)
> + 2*f(2*x)*f(
>      2*y)^2*f(a + z + x)*f(c + z + x) - 1/2*f(2*x)*f(2*y)^2*f
> (a + 2*z)*f(c
>      + 2*x) + f(2*x)*f(2*y)^2*f(a + 2*z)*f(a + z + x) + 1/2*
> f(2*x)*f(2*y)
>      ^2*f(a + 2*x)*f(c + 2*z) - f(2*x)^2*f(z + x)*f(c + 2*y)
> ^2 + 2*f(2*x)^
>      2*f(z + x)*f(b + 2*y)*f(c + z + y) - f(2*x)^2*f(z + x)*f
> (b + 2*y)*f(b
>      + 2*z) - f(2*x)^2*f(2*y)*f(c + 2*z)*f(b + y + x) + f(2*
> x)^2*f(2*y)*
>      f(c + 2*y)*f(c + z + x) - 2*f(2*x)^2*f(2*y)*f(b + z + y)
> *f(c + z + x)
>      + f(2*x)^2*f(2*y)*f(b + 2*z)*f(c + y + x) + f(2*x)^2*f
> (2*y)*f(b + 2*
>      z)*f(b + z + x) + f(2*x)^2*f(2*y)*f(b + 2*z)*f(a + z +
> y) + 1/2*f(2*x
>      )^2*f(2*y)*f(a + 2*z)*f(c + 2*y) - f(2*x)^2*f(2*y)*f(a +
> 2*z)*f(b + z
>      + y) - 1/2*f(2*x)^2*f(2*y)*f(a + 2*y)*f(c + 2*z) )
>
>      + 2*f(z + x)*f(2*a + 2*y) - 2*f(2*y)*f(2*a + z + x):
>
> eq[5] :=
> (1/HessUniv) * ( 2*f(2*z)*f(z + y)^2*f(a + 2*y)*f(c + z + x) - f
> (2*z)
>      *f(z + y)^2*f(a + 2*y)*f(a + 2*z) - 2*f(2*z)*f(z + x)*f
> (z + y)*f(b +
>      2*y)*f(c + z + x) + f(2*z)*f(z + x)*f(z + y)*f(a + 2*z)*
> f(b + 2*y) -
>      2*f(2*z)*f(z + x)*f(z + y)*f(a + 2*y)*f(c + z + y) + f
> (2*z)*f(z + x)*
>      f(z + y)*f(a + 2*y)*f(b + 2*z) + 2*f(2*z)*f(z + x)^2*f(b
> + 2*y)*f(c
>      + z + y) - f(2*z)*f(z + x)^2*f(b + 2*y)*f(b + 2*z) + f
> (2*z)^2*f(z +
>      y)*f(b + 2*y)*f(c + 2*x) - f(2*z)^2*f(z + y)*f(a + 2*y)*
> f(c + y + x)
>      - f(2*z)^2*f(z + y)*f(a + 2*y)*f(b + z + x) + f(2*z)^2*
> f(z + y)*f(a
>      + 2*y)*f(a + z + y) - f(2*z)^2*f(z + x)*f(b + 2*y)*f(c
> + y + x) + f(

```

```

>      2*z)^2*f(z + x)*f(b + 2*y)*f(b + z + x) - f(2*z)^2*f(z +
x)*f(b + 2*y
>      )*f(a + z + y) + f(2*z)^2*f(z + x)*f(a + 2*y)*f(c + 2*y)
+ f(2*z)^3*
>      f(b + 2*y)*f(a + y + x) - 1/2*f(2*z)^3*f(b + 2*x)*f(b +
2*y) - 1/2*f(
>      2*z)^3*f(a + 2*y)^2 + f(2*z)^2*f(y + x)*f(c + 2*y)*f(c +
y + x) + f(2
>      *z)^2*f(y + x)*f(c + 2*y)*f(b + z + x) - f(2*z)^2*f(y +
x)*f(c + 2*y)
>      *f(a + z + y) - f(2*z)^2*f(y + x)*f(a + 2*z)*f(b + 2*y)
+ 2*f(2*z)^2*
>      f(y + x)*f(a + 2*y)*f(c + z + y) - 2*f(2*z)*f(y + x)*f(z
+ y)*f(c + 2
>      *y)*f(c + z + x) + f(2*z)*f(y + x)*f(z + y)*f(a + 2*z)*f
(c + 2*y) -
>      f(2*z)*f(y + x)*f(z + y)*f(a + 2*y)*f(c + 2*z) - 2*f(2*
z)*f(y + x)*f(
>      z + x)*f(c + 2*y)*f(c + z + y) - f(2*z)*f(y + x)*f(z +
x)*f(b + 2*z)*
>      f(c + 2*y) + f(2*z)*f(y + x)*f(z + x)*f(b + 2*y)*f(c +
2*z) + 2*f(y
>      + x)*f(z + x)*f(z + y)*f(c + 2*y)*f(c + 2*z) - 4*f(2*y)
*f(z + y)^2*
>      f(c + 2*z)*f(a + z + x) + 2*f(2*y)*f(z + y)^2*f(a + 2*z)
*f(c + z + x)
>      + f(2*y)*f(z + y)^2*f(a + 2*z)^2 + 4*f(2*y)*f(z + x)*f
(z + y)*f(c +
>      2*z)*f(b + z + x) + 4*f(2*y)*f(z + x)*f(z + y)*f(c + 2*
z)*f(a + z + y
>      ) - 2*f(2*y)*f(z + x)*f(z + y)*f(b + 2*z)*f(c + z + x) -
2*f(2*y)*f(z
>      + x)*f(z + y)*f(a + 2*z)*f(c + z + y) - 2*f(2*y)*f(z +
x)*f(z + y)*
>      f(a + 2*z)*f(b + 2*z) - 4*f(2*y)*f(z + x)^2*f(c + 2*z)*f
(b + z + y)
>      - f(2*y)*f(z + x)^2*f(c + 2*y)*f(c + 2*z) + 2*f(2*y)*f
(z + x)^2*f(b
>      + 2*z)*f(c + z + y) + f(2*y)*f(z + x)^2*f(b + 2*z)^2 +
2*f(2*y)*f(2*
>      z)*f(z + y)*f(c + 2*z)*f(a + y + x) + 2*f(2*y)*f(2*z)*f
(z + y)*f(b +
>      2*z)*f(a + z + x) - f(2*y)*f(2*z)*f(z + y)*f(b + 2*x)*f
(c + 2*z) - 4*
>      f(2*y)*f(2*z)*f(z + y)*f(a + z + y)*f(c + z + x) + 4*f
(2*y)*f(2*z)*f(
>      z + y)*f(a + z + x)*f(c + z + y) - f(2*y)*f(2*z)*f(z +
y)*f(a + 2*z)*
>      f(c + y + x) - f(2*y)*f(2*z)*f(z + y)*f(a + 2*z)*f(b + z
+ x) - f(2*y
>      )*f(2*z)*f(z + y)*f(a + 2*z)*f(a + z + y) + 2*f(2*y)*f
(2*z)*f(z + x)*
>      f(c + 2*y)*f(c + z + x) + 4*f(2*y)*f(2*z)*f(z + x)*f(b +
z + y)*f(c
>      + z + x) - 4*f(2*y)*f(2*z)*f(z + x)*f(b + z + x)*f(c +
z + y) + f(2*
>      y)*f(2*z)*f(z + x)*f(b + 2*z)*f(c + y + x) - f(2*y)*f(2*

```

```

z)*f(z + x)*
>      f(b + 2*z)*f(b + z + x) - f(2*y)*f(2*z)*f(z + x)*f(b +
2*z)*f(a + z
>      + y) + 2*f(2*y)*f(2*z)*f(z + x)*f(a + 2*z)*f(b + z + y)
- f(2*y)*f(2
>      *z)*f(z + x)*f(a + 2*y)*f(c + 2*z) - f(2*y)*f(2*z)^2*f(c
+ 2*y)*f(a
>      + z + x) - 1/2*f(2*y)*f(2*z)^2*f(c + 2*x)*f(c + 2*y) -
f(2*y)*f(2*z)
>      ^2*f(c + 2*x)*f(b + z + y) - f(2*y)*f(2*z)^2*f(b + 2*z)*
f(a + y + x)
>      + f(2*y)*f(2*z)^2*f(b + 2*x)*f(c + z + y) + 1/2*f(2*y)*
f(2*z)^2*f(b
>      + 2*x)*f(b + 2*z) + 2*f(2*y)*f(2*z)^2*f(a + z + y)*f(c
+ y + x) + 2*
>      f(2*y)*f(2*z)^2*f(a + z + y)*f(b + z + x) - 2*f(2*y)*f
(2*z)^2*f(a + z
>      + x)*f(b + z + y) - 2*f(2*y)*f(2*z)^2*f(a + y + x)*f(c
+ z + y) + f(
>      2*y)*f(2*z)^2*f(a + 2*y)*f(a + 2*z) - f(2*y)*f(2*z)*f(y
+ x)*f(c + 2*
>      z)*f(c + y + x) - f(2*y)*f(2*z)*f(y + x)*f(c + 2*z)*f(b
+ z + x) - f(
>      2*y)*f(2*z)*f(y + x)*f(c + 2*z)*f(a + z + y) + f(2*y)*f
(2*z)*f(y + x)
>      *f(a + 2*z)*f(b + 2*z) + 2*f(2*y)*f(y + x)*f(z + y)*f(c
+ 2*z)*f(c +
>      z + x) + 2*f(2*y)*f(y + x)*f(z + x)*f(c + 2*z)*f(c + z +
y) - f(2*y)*
>      f(y + x)^2*f(c + 2*z)^2 - 2*f(2*y)^2*f(z + x)*f(c + 2*z)
*f(c + z + x)
>      + f(2*y)^2*f(2*z)*f(c + 2*z)*f(a + z + x) + 1/2*f(2*y)
^2*f(2*z)*f(c
>      + 2*x)*f(c + 2*z) - 1/2*f(2*y)^2*f(2*z)*f(a + 2*z)^2 -
f(2*x)*f(z +
>      y)^2*f(c + 2*y)*f(c + 2*z) + 2*f(2*x)*f(2*z)*f(z + y)*f
(c + 2*y)*f(c
>      + z + y) - 1/2*f(2*x)*f(2*z)^2*f(c + 2*y)^2 - f(2*x)*f
(2*z)^2*f(b +
>      2*y)*f(c + z + y) + 1/2*f(2*x)*f(2*z)^2*f(b + 2*y)*f(b +
2*z) - 2*f(2
>      *x)*f(2*y)*f(z + y)*f(c + 2*z)*f(c + z + y) + f(2*x)*f
(2*y)*f(2*z)*f(
>      c + 2*z)*f(b + z + y) + 1/2*f(2*x)*f(2*y)*f(2*z)*f(c +
2*y)*f(c + 2*z
>      ) - 1/2*f(2*x)*f(2*y)*f(2*z)*f(b + 2*z)^2 + f(2*x)*f(2*
y)^2*f(c + 2*z
>      )^2 )

>      - f(c + 2*y)*f(c + 2*z) + f(2*z)*f(2*c + 2*y) - f(2*y)*f
(2*c + 2*z):

> eq[6] :=
> (1/HessUniv) * ( 8*f(z + y)^3*f(b + 2*y)*f(a + y + x) - 4*f(z +
y)^3*
>      f(a + 2*y)*f(b + y + x) - 2*f(z + y)^3*f(a + 2*y)^2 - 4*
f(z + x)*f(z

```

```

> + y)^2*f(b + 2*y)*f(b + y + x) + 2*f(z + x)^2*f(z + y)*
f(b + 2*y)^2
> + 4*f(2*z)*f(y + x)*f(z + y)*f(b + 2*y)*f(b + y + x) +
4*f(y + x)*f(
> z + y)^2*f(c + 2*y)*f(b + y + x) - 8*f(y + x)*f(z + y)
^2*f(b + 2*y)*
> f(c + y + x) - 8*f(y + x)*f(z + y)^2*f(b + 2*y)*f(a + z
+ y) + 4*f(y
> + x)*f(z + y)^2*f(a + 2*y)*f(c + 2*y) + 4*f(y + x)*f(z
+ y)^2*f(a +
> 2*y)*f(b + z + y) - 4*f(y + x)*f(z + x)*f(z + y)*f(b +
2*y)*f(b + z
> + y) - 2*f(y + x)^2*f(z + y)*f(c + 2*y)^2 - 4*f(y + x)
^2*f(z + y)*f(
> c + 2*y)*f(b + z + y) + 8*f(y + x)^2*f(z + y)*f(b + 2*y)
*f(c + z + y)
> - 4*f(2*y)*f(z + y)^2*f(c + 2*y)*f(a + y + x) + 2*f(2*
y)*f(z + y)^2*
> f(b + 2*y)*f(c + 2*x) - 4*f(2*y)*f(z + y)^2*f(b + 2*y)*f
(a + z + x)
> + 4*f(2*y)*f(z + y)^2*f(a + z + y)*f(b + y + x) - 8*f
(2*y)*f(z + y)^
> 2*f(a + y + x)*f(b + z + y) + 2*f(2*y)*f(z + y)^2*f(a +
2*y)*f(c + y
> + x) + 2*f(2*y)*f(z + y)^2*f(a + 2*y)*f(b + z + x) + 4*
f(2*y)*f(z +
> y)^2*f(a + 2*y)*f(a + z + y) + 4*f(2*y)*f(z + x)*f(z +
y)*f(b + y + x
> )*f(b + z + y) + 2*f(2*y)*f(z + x)*f(z + y)*f(b + 2*y)*f
(c + y + x)
> + 2*f(2*y)*f(z + x)*f(z + y)*f(b + 2*y)*f(b + z + x) +
4*f(2*y)*f(z
> + x)*f(z + y)*f(b + 2*y)*f(a + z + y) - 2*f(2*y)*f(z +
x)*f(z + y)*
> f(a + 2*y)*f(c + 2*y) - 2*f(2*y)*f(z + x)*f(z + y)*f(a +
2*y)*f(b + z
> + y) - 2*f(2*y)*f(z + x)^2*f(b + 2*y)*f(b + z + y) - 4*
f(2*y)*f(2*z)
> *f(z + y)*f(b + 2*y)*f(a + y + x) - f(2*y)*f(2*z)*f(z +
y)*f(b + 2*x)
> *f(b + 2*y) + 2*f(2*y)*f(2*z)*f(z + y)*f(a + 2*y)*f(b +
y + x) + f(2*
> y)*f(2*z)*f(z + y)*f(a + 2*y)^2 - 2*f(2*y)*f(2*z)*f(y +
x)*f(c + 2*y)
> *f(b + y + x) - 4*f(2*y)*f(2*z)*f(y + x)*f(b + y + x)*f
(b + z + y) +
> 2*f(2*y)*f(2*z)*f(y + x)*f(b + 2*y)*f(c + y + x) + 2*f
(2*y)*f(y + x)*
> f(z + y)*f(c + 2*y)*f(c + y + x) - 2*f(2*y)*f(y + x)*f(z
+ y)*f(c + 2
> *y)*f(b + z + x) + 8*f(2*y)*f(y + x)*f(z + y)*f(b + z +
y)*f(c + y +
> x) - 4*f(2*y)*f(y + x)*f(z + y)*f(b + y + x)*f(c + z +
y) + 4*f(2*y)*
> f(y + x)*f(z + y)*f(a + z + y)*f(b + z + y) + 4*f(2*y)*f
(y + x)*f(z
> + y)*f(a + 2*z)*f(b + 2*y) - 6*f(2*y)*f(y + x)*f(z + y)

```

```

*f(a + 2*y)*
> f(c + z + y) - 2*f(2*y)*f(y + x)*f(z + y)*f(a + 2*y)*f(b
+ 2*z) + 2*
> f(2*y)*f(y + x)*f(z + x)*f(c + 2*y)*f(b + z + y) + 4*f
(2*y)*f(y + x)*
> f(z + x)*f(b + z + y)^2 - 2*f(2*y)*f(y + x)*f(z + x)*f(b
+ 2*y)*f(c
> + z + y) + 2*f(2*y)*f(y + x)^2*f(c + 2*y)*f(c + z + y)
- 4*f(2*y)*f(
> y + x)^2*f(b + z + y)*f(c + z + y) + 2*f(2*y)*f(y + x)
^2*f(b + 2*z)*
> f(c + 2*y) - 2*f(2*y)*f(y + x)^2*f(b + 2*y)*f(c + 2*z) +
2*f(2*y)^2*
> f(z + y)*f(c + 2*y)*f(a + z + x) - f(2*y)^2*f(z + y)*f(c
+ 2*x)*f(c
> + 2*y) - 2*f(2*y)^2*f(z + y)*f(c + 2*x)*f(b + z + y) +
2*f(2*y)^2*f(
> z + y)*f(b + 2*z)*f(a + y + x) - 2*f(2*y)^2*f(z + y)*f(a
+ z + y)*f(c
> + y + x) - 2*f(2*y)^2*f(z + y)*f(a + z + y)*f(b + z +
x) - 2*f(2*y)^
> 2*f(z + y)*f(a + z + y)^2 + 4*f(2*y)^2*f(z + y)*f(a + z
+ x)*f(b + z
> + y) - 2*f(2*y)^2*f(z + y)*f(a + 2*z)*f(b + y + x) + 4*
f(2*y)^2*f(z
> + y)*f(a + y + x)*f(c + z + y) - f(2*y)^2*f(z + y)*f(a
+ 2*y)*f(a +
> 2*z) - 2*f(2*y)^2*f(z + x)*f(b + z + y)*f(c + y + x) -
2*f(2*y)^2*f(z
> + x)*f(b + z + x)*f(b + z + y) - 2*f(2*y)^2*f(z + x)*f
(a + z + y)*f(
> b + z + y) - f(2*y)^2*f(z + x)*f(a + 2*z)*f(b + 2*y) +
2*f(2*y)^2*f(z
> + x)*f(a + 2*y)*f(c + z + y) + f(2*y)^2*f(z + x)*f(a +
2*y)*f(b + 2*
> z) + f(2*y)^2*f(2*z)*f(c + 2*y)*f(a + y + x) - 1/2*f(2*
y)^2*f(2*z)*f(
> b + 2*y)*f(c + 2*x) + f(2*y)^2*f(2*z)*f(b + 2*y)*f(a + z
+ x) + 1/2*
> f(2*y)^2*f(2*z)*f(b + 2*x)*f(c + 2*y) + f(2*y)^2*f(2*z)*
f(b + 2*x)*f(
> b + z + y) + 2*f(2*y)^2*f(2*z)*f(a + y + x)*f(b + z + y)
- f(2*y)^2*
> f(2*z)*f(a + 2*y)*f(c + y + x) - f(2*y)^2*f(2*z)*f(a +
2*y)*f(b + z
> + x) - f(2*y)^2*f(2*z)*f(a + 2*y)*f(a + z + y) + 2*f(2*
y)^2*f(y + x)
> *f(c + 2*z)*f(b + y + x) - 2*f(2*y)^2*f(y + x)*f(c + y +
x)*f(c + z
> + y) + 2*f(2*y)^2*f(y + x)*f(b + z + x)*f(c + z + y) -
2*f(2*y)^2*f(
> y + x)*f(b + 2*z)*f(c + y + x) + 2*f(2*y)^2*f(y + x)*f(a
+ z + y)*f(c
> + z + y) - f(2*y)^2*f(y + x)*f(a + 2*z)*f(c + 2*y) - 2*
f(2*y)^2*f(y
> + x)*f(a + 2*z)*f(b + z + y) + f(2*y)^2*f(y + x)*f(a +
2*y)*f(c + 2*

```

```

>      z) - f(2*y)^3*f(c + 2*z)*f(a + y + x) + f(2*y)^3*f(c +
2*x)*f(c + z
>      + y) + 1/2*f(2*y)^3*f(b + 2*z)*f(c + 2*x) - f(2*y)^3*f
(b + 2*z)*f(a
>      + z + x) - 1/2*f(2*y)^3*f(b + 2*x)*f(c + 2*z) - 2*f(2*
y)^3*f(a + z
>      + x)*f(c + z + y) + f(2*y)^3*f(a + 2*z)*f(c + y + x) +
f(2*y)^3*f(a
>      + 2*z)*f(b + z + x) + f(2*y)^3*f(a + 2*z)*f(a + z + y)
+ 4*f(2*x)*f(
>      z + y)^2*f(b + 2*y)*f(b + z + y) - 2*f(2*x)*f(2*z)*f(z +
y)*f(b + 2*y
>      )^2 + f(2*x)*f(2*y)*f(z + y)*f(c + 2*y)^2 - 4*f(2*x)*f
(2*y)*f(z + y)*
>      f(b + z + y)^2 - 2*f(2*x)*f(2*y)*f(z + y)*f(b + 2*y)*f(c
+ z + y) -
>      f(2*x)*f(2*y)*f(z + y)*f(b + 2*y)*f(b + 2*z) + 2*f(2*x)*
f(2*y)*f(2*z)
>      *f(b + 2*y)*f(b + z + y) - f(2*x)*f(2*y)^2*f(c + 2*y)*f
(c + z + y) +
>      2*f(2*x)*f(2*y)^2*f(b + z + y)*f(c + z + y) - 1/2*f(2*x)
*f(2*y)^2*f(b
>      + 2*z)*f(c + 2*y) + f(2*x)*f(2*y)^2*f(b + 2*z)*f(b + z
+ y) + 1/2*f(
>      2*x)*f(2*y)^2*f(b + 2*y)*f(c + 2*z) )
>
>      + 2*f(z + y)*f(2*b + 2*y) - 2*f(2*y)*f(2*b + z + y):
> eq[7] :=
> (1/HessUniv) * ( 2*f(z + x)*f(z + y)^2*f(a + 2*x)*f(b + 2*y) + 4*
f(z
>      + x)^2*f(z + y)*f(b + 2*y)*f(a + y + x) - 2*f(z + x)^2*
f(z + y)*f(b
>      + 2*x)*f(b + 2*y) - 4*f(z + x)^2*f(z + y)*f(a + 2*y)*f
(b + y + x) -
>      2*f(z + x)^2*f(z + y)*f(a + 2*y)^2 + 2*f(z + x)^3*f(a +
2*y)*f(b + 2*
>      y) + f(2*z)*f(y + x)*f(z + x)*f(b + 2*x)*f(b + 2*y) + 2*
f(2*z)*f(y +
>      x)*f(z + x)*f(a + 2*y)*f(b + y + x) + f(2*z)*f(y + x)*f
(z + x)*f(a +
>      2*y)^2 - 4*f(y + x)*f(z + x)*f(z + y)*f(b + 2*y)*f(a + z
+ x) - 4*f(y
>      + x)*f(z + x)^2*f(b + 2*y)*f(a + z + y) + 2*f(y + x)^2*
f(z + x)*f(a
>      + 2*z)*f(b + 2*y) - 2*f(2*y)*f(z + y)^2*f(b + 2*x)*f(a
+ z + x) + 2*
>      f(2*y)*f(z + x)*f(z + y)*f(b + 2*x)*f(b + z + x) + 2*f
(2*y)*f(z + x)*
>      f(z + y)*f(b + 2*x)*f(a + z + y) + f(2*y)*f(z + x)*f(z +
y)*f(a + 2*y
>      )*f(c + 2*x) + 2*f(2*y)*f(z + x)*f(z + y)*f(a + 2*y)*f(a
+ z + x) -
>      f(2*y)*f(z + x)*f(z + y)*f(a + 2*x)*f(c + 2*y) - 2*f(2*
y)*f(z + x)*f(
>      z + y)*f(a + 2*x)*f(b + z + y) - 2*f(2*y)*f(z + x)^2*f(c
+ 2*y)*f(a

```

```

>      + y + x) + f(2*y)*f(z + x)^2*f(b + 2*y)*f(c + 2*x) + f
>      (2*y)*f(z + x)
>      ^2*f(b + 2*x)*f(c + 2*y) + 4*f(2*y)*f(z + x)^2*f(a + z +
>      y)*f(b + y
>      + x) - 4*f(2*y)*f(z + x)^2*f(a + y + x)*f(b + z + y) +
>      2*f(2*y)*f(z
>      + x)^2*f(a + 2*y)*f(a + z + y) + f(2*y)*f(2*z)*f(z + y)
>      *f(b + 2*x)*
>      f(a + y + x) - f(2*y)*f(2*z)*f(z + y)*f(a + 2*x)*f(b + y
>      + x) - 1/2*
>      f(2*y)*f(2*z)*f(z + x)*f(a + 2*y)*f(b + 2*x) - 3/2*f(2*
>      y)*f(2*z)*f(z
>      + x)*f(a + 2*x)*f(b + 2*y) - f(2*y)*f(2*z)*f(y + x)*f(b
>      + 2*x)*f(b
>      + z + x) - f(2*y)*f(2*z)*f(y + x)*f(b + 2*x)*f(a + z +
>      y) - 2*f(2*y)
>      *f(2*z)*f(y + x)*f(a + y + x)*f(b + z + x) - f(2*y)*f(2*
>      z)*f(y + x)*
>      f(a + 2*y)*f(a + z + x) + f(2*y)*f(2*z)*f(y + x)*f(a +
>      2*x)*f(b + z
>      + y) + 4*f(2*y)*f(y + x)*f(z + y)*f(a + z + x)*f(b + z
>      + x) + 2*f(2*
>      y)*f(y + x)*f(z + x)*f(c + 2*y)*f(a + z + x) - f(2*y)*f
>      (y + x)*f(z +
>      x)*f(c + 2*x)*f(c + 2*y) + 2*f(2*y)*f(y + x)*f(z + x)*f
>      (b + 2*z)*f(a
>      + y + x) + 4*f(2*y)*f(y + x)*f(z + x)*f(a + z + x)*f(b
>      + z + y) - 2*
>      f(2*y)*f(y + x)*f(z + x)*f(a + 2*z)*f(b + y + x) - f(2*
>      y)*f(y + x)*f(
>      z + x)*f(a + 2*y)*f(a + 2*z) - 2*f(2*y)*f(y + x)^2*f(b +
>      2*z)*f(a + z
>      + x) + f(2*y)^2*f(z + y)*f(c + 2*x)*f(a + z + x) - f(2*
>      y)^2*f(z + y)
>      *f(a + 2*x)*f(c + z + x) - f(2*y)^2*f(z + x)*f(c + 2*x)*
>      f(b + z + x)
>      - 2*f(2*y)^2*f(z + x)*f(c + 2*x)*f(a + z + y) - f(2*y)
>      ^2*f(z + x)*f(
>      b + 2*x)*f(c + z + x) - 2*f(2*y)^2*f(z + x)*f(a + z + x)
>      *f(b + z + x)
>      - 2*f(2*y)^2*f(z + x)*f(a + z + x)*f(a + z + y) - 1/2*f
>      (2*y)^2*f(z
>      + x)*f(a + 2*z)*f(b + 2*x) + 2*f(2*y)^2*f(z + x)*f(a +
>      y + x)*f(c +
>      z + x) + 2*f(2*y)^2*f(z + x)*f(a + 2*x)*f(c + z + y) +
>      1/2*f(2*y)^2*
>      f(z + x)*f(a + 2*x)*f(b + 2*z) - f(2*y)^2*f(2*z)*f(c +
>      2*x)*f(a + y
>      + x) + f(2*y)^2*f(2*z)*f(b + 2*x)*f(a + z + x) + f(2*y)
>      ^2*f(2*z)*f(a
>      + 2*x)*f(c + y + x) + f(2*y)^2*f(2*z)*f(a + 2*x)*f(b +
>      z + x) + f(2*
>      y)^2*f(y + x)*f(c + 2*x)*f(c + z + x) - 2*f(2*y)^2*f(y +
>      x)*f(a + z
>      + x)*f(c + z + x) + f(2*y)^2*f(y + x)*f(a + 2*z)*f(c +
>      2*x) + f(2*y)
>      ^2*f(y + x)*f(a + 2*z)*f(a + z + x) - f(2*y)^2*f(y + x)*

```



```

f(a + 2*x)*f(
>      c + 2*z) + 2*f(2*x)*f(z + x)*f(z + y)*f(c + 2*y)*f(b + y
+ x) - 4*f(2
>      *x)*f(z + x)*f(z + y)*f(b + 2*y)*f(c + y + x) + 2*f(2*x)
*f(z + x)*f(z
>      + y)*f(b + 2*y)*f(b + z + x) + 2*f(2*x)*f(z + x)*f(z +
y)*f(a + 2*y)
>      *f(c + 2*y) + 2*f(2*x)*f(z + x)*f(z + y)*f(a + 2*y)*f(b
+ z + y) - 2*
>      f(2*x)*f(2*z)*f(z + x)*f(a + 2*y)*f(b + 2*y) - f(2*x)*f
(y + x)*f(z +
>      x)*f(c + 2*y)^2 - 2*f(2*x)*f(y + x)*f(z + x)*f(c + 2*y)*
f(b + z + y)
>      + 4*f(2*x)*f(y + x)*f(z + x)*f(b + 2*y)*f(c + z + y) -
f(2*x)*f(y +
>      x)*f(z + x)*f(b + 2*y)*f(b + 2*z) - f(2*x)*f(2*y)*f(z +
y)*f(c + 2*y)
>      *f(a + z + x) - 2*f(2*x)*f(2*y)*f(z + y)*f(b + z + x)^2
- f(2*x)*f(2*
>      y)*f(z + y)*f(b + 2*z)*f(a + y + x) + 2*f(2*x)*f(2*y)*f
(z + y)*f(b +
>      y + x)*f(c + z + x) - 2*f(2*x)*f(2*y)*f(z + y)*f(a + z +
y)*f(b + z
>      + x) + f(2*x)*f(2*y)*f(z + y)*f(a + 2*z)*f(b + y + x) -
f(2*x)*f(2*y
>      )*f(z + y)*f(a + 2*y)*f(c + z + x) + 2*f(2*x)*f(2*y)*f(z
+ x)*f(c + 2
>      *y)*f(c + y + x) - f(2*x)*f(2*y)*f(z + x)*f(c + 2*y)*f(b
+ z + x) + 4
>      *f(2*x)*f(2*y)*f(z + x)*f(b + z + y)*f(c + y + x) - 4*f
(2*x)*f(2*y)*
>      f(z + x)*f(b + y + x)*f(c + z + y) - f(2*x)*f(2*y)*f(z +
x)*f(b + 2*y
>      )*f(c + z + x) + 1/2*f(2*x)*f(2*y)*f(z + x)*f(a + 2*z)*f
(b + 2*y) - 2
>      *f(2*x)*f(2*y)*f(z + x)*f(a + 2*y)*f(c + z + y) - 1/2*f
(2*x)*f(2*y)*
>      f(z + x)*f(a + 2*y)*f(b + 2*z) + 1/2*f(2*x)*f(2*y)*f(2*
z)*f(b + 2*y)*
>      f(c + 2*x) + f(2*x)*f(2*y)*f(2*z)*f(b + 2*y)*f(a + z +
x) - 1/2*f(2*x
>      )*f(2*y)*f(2*z)*f(b + 2*x)*f(c + 2*y) + f(2*x)*f(2*y)*f
(2*z)*f(a + 2*
>      y)*f(b + z + x) + f(2*x)*f(2*y)*f(y + x)*f(c + 2*y)*f(c
+ z + x) - 2*
>      f(2*x)*f(2*y)*f(y + x)*f(b + z + y)*f(c + z + x) + f(2*
x)*f(2*y)*f(y
>      + x)*f(b + 2*z)*f(b + z + x) + f(2*x)*f(2*y)*f(y + x)*f
(b + 2*z)*f(a
>      + z + y) - f(2*x)*f(2*y)*f(y + x)*f(a + 2*z)*f(b + z +
y) + f(2*x)*
>      f(2*y)^2*f(c + 2*z)*f(a + y + x) - 2*f(2*x)*f(2*y)^2*f(c
+ y + x)*f(c
>      + z + x) + 2*f(2*x)*f(2*y)^2*f(b + z + x)*f(c + z + x)
- 1/2*f(2*x)*
>      f(2*y)^2*f(b + 2*z)*f(c + 2*x) + 1/2*f(2*x)*f(2*y)^2*f(b
+ 2*x)*f(c

```

```

>      + 2*z) + 2*f(2*x)*f(2*y)^2*f(a + z + y)*f(c + z + x) -
f(2*x)*f(2*y)
>      ^2*f(a + 2*z)*f(c + y + x) + 1/2*f(2*x)^2*f(2*y)*f(b +
2*z)*f(c + 2*y
>      ) - 1/2*f(2*x)^2*f(2*y)*f(b + 2*y)*f(c + 2*z) )
>
>      + 2*f(z + x)*f(b + a + 2*y) - 2*f(2*y)*f(b + a + z + x):
>
> eq[8] :=
> (1/HessUniv) * ( 2*f(z + y)^3*f(a + 2*x)*f(b + 2*y) + 4*f(z + x)*
f(z
>      + y)^2*f(b + 2*y)*f(a + y + x) - 2*f(z + x)*f(z + y)^2*
f(b + 2*x)*f(
>      b + 2*y) - 4*f(z + x)*f(z + y)^2*f(a + 2*y)*f(b + y + x)
- 2*f(z + x)
>      *f(z + y)^2*f(a + 2*y)^2 + 2*f(z + x)^2*f(z + y)*f(a +
2*y)*f(b + 2*y
>      ) + f(2*z)*f(y + x)*f(z + y)*f(b + 2*x)*f(b + 2*y) + 2*f
(2*z)*f(y + x
>      )*f(z + y)*f(a + 2*y)*f(b + y + x) + f(2*z)*f(y + x)*f(z
+ y)*f(a + 2
>      *y)^2 - 4*f(y + x)*f(z + y)^2*f(b + 2*y)*f(a + z + x) -
4*f(y + x)*f(
>      z + x)*f(z + y)*f(b + 2*y)*f(a + z + y) + 2*f(y + x)^2*f
(z + y)*f(a
>      + 2*z)*f(b + 2*y) + f(2*y)*f(z + y)^2*f(a + 2*y)*f(c +
2*x) - f(2*y)
>      *f(z + y)^2*f(a + 2*x)*f(c + 2*y) - 2*f(2*y)*f(z + y)^2*
f(a + 2*x)*f(
>      b + z + y) - 2*f(2*y)*f(z + x)*f(z + y)*f(c + 2*y)*f(a +
y + x) + f(2
>      *y)*f(z + x)*f(z + y)*f(b + 2*y)*f(c + 2*x) + f(2*y)*f(z
+ x)*f(z + y
>      )*f(b + 2*x)*f(c + 2*y) + 2*f(2*y)*f(z + x)*f(z + y)*f(b
+ 2*x)*f(b
>      + z + y) + 4*f(2*y)*f(z + x)*f(z + y)*f(a + z + y)*f(b
+ y + x) - 4*
>      f(2*y)*f(z + x)*f(z + y)*f(a + y + x)*f(b + z + y) + 2*f
(2*y)*f(z + x
>      )*f(z + y)*f(a + 2*y)*f(b + z + x) + 4*f(2*y)*f(z + x)*f
(z + y)*f(a
>      + 2*y)*f(a + z + y) - 2*f(2*y)*f(z + x)^2*f(a + 2*y)*f
(b + z + y) -
>      1/2*f(2*y)*f(2*z)*f(z + y)*f(a + 2*y)*f(b + 2*x) - 3/2*f
(2*y)*f(2*z)*
>      f(z + y)*f(a + 2*x)*f(b + 2*y) - f(2*y)*f(2*z)*f(z + x)*
f(b + 2*y)*f(
>      a + y + x) + f(2*y)*f(2*z)*f(z + x)*f(a + 2*y)*f(b + y +
x) + f(2*y)*
>      f(2*z)*f(y + x)*f(b + 2*y)*f(a + z + x) - f(2*y)*f(2*z)*
f(y + x)*f(b
>      + 2*x)*f(b + z + y) - 2*f(2*y)*f(2*z)*f(y + x)*f(a + z
+ y)*f(b + y
>      + x) - f(2*y)*f(2*z)*f(y + x)*f(a + 2*y)*f(b + z + x) -
f(2*y)*f(2*z
>      )*f(y + x)*f(a + 2*y)*f(a + z + y) + 2*f(2*y)*f(y + x)*f
(z + y)*f(c

```

```

> + 2*y)*f(a + z + x) - f(2*y)*f(y + x)*f(z + y)*f(c + 2*
x)*f(c + 2*y)
> + 4*f(2*y)*f(y + x)*f(z + y)*f(a + z + x)*f(b + z + y)
> - f(2*y)*f(y
> + x)*f(z + y)*f(a + 2*y)*f(a + 2*z) + 4*f(2*y)*f(y + x)
> *f(z + x)*f(a
> + z + y)*f(b + z + y) - 2*f(2*y)*f(y + x)^2*f(a + 2*z)*
f(b + z + y)
> - f(2*y)^2*f(z + y)*f(c + 2*x)*f(a + z + y) - 1/2*f(2*
y)^2*f(z + y)*
> f(a + 2*z)*f(b + 2*x) + f(2*y)^2*f(z + y)*f(a + 2*x)*f(c
+ z + y) + 1/
> 2*f(2*y)^2*f(z + y)*f(a + 2*x)*f(b + 2*z) - f(2*y)^2*f(z
+ x)*f(c + 2
> *x)*f(b + z + y) + f(2*y)^2*f(z + x)*f(b + 2*z)*f(a + y
+ x) - f(2*y)
> ^2*f(z + x)*f(b + 2*x)*f(c + z + y) - 2*f(2*y)^2*f(z +
x)*f(a + z + y
> )*f(b + z + x) - 2*f(2*y)^2*f(z + x)*f(a + z + y)^2 - f
(2*y)^2*f(z +
> x)*f(a + 2*z)*f(b + y + x) + 2*f(2*y)^2*f(z + x)*f(a + y
+ x)*f(c + z
> + y) + f(2*y)^2*f(2*z)*f(b + 2*x)*f(a + z + y) - 1/2*f
(2*y)^2*f(2*z)
> *f(a + 2*y)*f(c + 2*x) + 1/2*f(2*y)^2*f(2*z)*f(a + 2*x)*
f(c + 2*y) +
> f(2*y)^2*f(2*z)*f(a + 2*x)*f(b + z + y) + f(2*y)^2*f(y +
x)*f(c + 2*x
> )*f(c + z + y) - f(2*y)^2*f(y + x)*f(b + 2*z)*f(a + z +
x) - 2*f(2*y)
> ^2*f(y + x)*f(a + z + x)*f(c + z + y) + f(2*y)^2*f(y +
x)*f(a + 2*z)*
> f(b + z + x) + f(2*y)^2*f(y + x)*f(a + 2*z)*f(a + z + y)
+ 1/2*f(2*y)
> ^3*f(a + 2*z)*f(c + 2*x) - 1/2*f(2*y)^3*f(a + 2*x)*f(c +
2*z) + 2*f(2
> *x)*f(z + y)^2*f(c + 2*y)*f(b + y + x) - 4*f(2*x)*f(z +
y)^2*f(b + 2*
> y)*f(c + y + x) + 2*f(2*x)*f(z + y)^2*f(b + 2*y)*f(b + z
+ x) + 2*f(2
> *x)*f(z + y)^2*f(a + 2*y)*f(c + 2*y) + 2*f(2*x)*f(z + y)
^2*f(a + 2*y)
> *f(b + z + y) - 2*f(2*x)*f(2*z)*f(z + y)*f(a + 2*y)*f(b
+ 2*y) - f(2*
> x)*f(y + x)*f(z + y)*f(c + 2*y)^2 - 2*f(2*x)*f(y + x)*f
(z + y)*f(c +
> 2*y)*f(b + z + y) + 4*f(2*x)*f(y + x)*f(z + y)*f(b + 2*
y)*f(c + z + y
> ) - f(2*x)*f(y + x)*f(z + y)*f(b + 2*y)*f(b + 2*z) + 2*f
(2*x)*f(2*y)*
> f(z + y)*f(c + 2*y)*f(c + y + x) - 2*f(2*x)*f(2*y)*f(z +
y)*f(c + 2*y
> )*f(b + z + x) - f(2*x)*f(2*y)*f(z + y)*f(c + 2*y)*f(a +
z + y) + 4*
> f(2*x)*f(2*y)*f(z + y)*f(b + z + y)*f(c + y + x) - 2*f
(2*x)*f(2*y)*f(
> z + y)*f(b + z + x)*f(b + z + y) - 2*f(2*x)*f(2*y)*f(z +

```

```

y)*f(b + y
> + x)*f(c + z + y) - 2*f(2*x)*f(2*y)*f(z + y)*f(a + z +
y)*f(b + z +
> y) + 1/2*f(2*x)*f(2*y)*f(z + y)*f(a + 2*z)*f(b + 2*y) -
3*f(2*x)*f(2*
> y)*f(z + y)*f(a + 2*y)*f(c + z + y) - 1/2*f(2*x)*f(2*y)*
f(z + y)*f(a
> + 2*y)*f(b + 2*z) + f(2*x)*f(2*y)*f(z + x)*f(c + 2*y)*f
(b + z + y)
> - f(2*x)*f(2*y)*f(z + x)*f(b + 2*y)*f(c + z + y) - f(2*
x)*f(2*y)*f(2
> *z)*f(c + 2*y)*f(b + y + x) + f(2*x)*f(2*y)*f(2*z)*f(b +
2*y)*f(c + y
> + x) + f(2*x)*f(2*y)*f(2*z)*f(b + 2*y)*f(a + z + y) + f
(2*x)*f(2*y)*
> f(2*z)*f(a + 2*y)*f(b + z + y) + f(2*x)*f(2*y)*f(y + x)*
f(c + 2*y)*f(
> c + z + y) - 2*f(2*x)*f(2*y)*f(y + x)*f(b + z + y)*f(c +
z + y) + f(2
> *x)*f(2*y)*f(y + x)*f(b + 2*z)*f(c + 2*y) + f(2*x)*f(2*
y)*f(y + x)*f(
> b + 2*z)*f(b + z + y) - f(2*x)*f(2*y)*f(y + x)*f(b + 2*
y)*f(c + 2*z)
> + f(2*x)*f(2*y)^2*f(c + 2*z)*f(b + y + x) - 2*f(2*x)*f
(2*y)^2*f(c +
> y + x)*f(c + z + y) + 2*f(2*x)*f(2*y)^2*f(b + z + x)*f(c
+ z + y) -
> f(2*x)*f(2*y)^2*f(b + 2*z)*f(c + y + x) + 2*f(2*x)*f(2*
y)^2*f(a + z
> + y)*f(c + z + y) - 1/2*f(2*x)*f(2*y)^2*f(a + 2*z)*f(c
+ 2*y) + 1/2*
> f(2*x)*f(2*y)^2*f(a + 2*y)*f(c + 2*z) )
>
> + 2*f(z + y)*f(b + a + 2*y) - 2*f(2*y)*f(b + a + z + y):
> eq[9] :=
> (1/HessUniv) * ( 4*f(2*z)*f(y + x)*f(z + y)*f(b + 2*y)*f(a + y +
x)
> - f(2*z)*f(y + x)*f(z + y)*f(b + 2*x)*f(b + 2*y) - 2*f
(2*z)*f(y + x)
> *f(z + y)*f(a + 2*y)*f(b + y + x) - f(2*z)*f(y + x)*f(z
+ y)*f(a + 2*
> y)^2 + 2*f(y + x)*f(z + y)^2*f(b + 2*y)*f(c + 2*x) + 4*f
(y + x)*f(z
> + x)*f(z + y)*f(c + 2*y)*f(b + y + x) - 4*f(y + x)*f(z
+ x)*f(z + y)
> *f(b + 2*y)*f(c + y + x) + 4*f(y + x)*f(z + x)*f(z + y)*
f(b + 2*y)*f(
> b + z + x) - 8*f(y + x)*f(z + x)*f(z + y)*f(b + 2*y)*f(a
+ z + y) + 4
> *f(y + x)*f(z + x)*f(z + y)*f(a + 2*y)*f(c + 2*y) + 4*f
(y + x)*f(z +
> x)*f(z + y)*f(a + 2*y)*f(b + z + y) + 2*f(y + x)*f(z +
x)^2*f(b + 2*y
> )*f(c + 2*y) - 4*f(y + x)^2*f(z + y)*f(b + 2*y)*f(c + z
+ x) - 2*f(y
> + x)^2*f(z + x)*f(c + 2*y)^2 - 4*f(y + x)^2*f(z + x)*f

```

```

(c + 2*y)*f(b
> + z + y) + 4*f(y + x)^2*f(z + x)*f(b + 2*y)*f(c + z +
> y) - 2*f(y + x
> )^2*f(z + x)*f(b + 2*y)*f(b + 2*z) + 2*f(y + x)^3*f(b +
> 2*y)*f(c + 2*
> z) - 2*f(2*y)*f(z + y)^2*f(c + 2*x)*f(b + y + x) + 4*f
> (2*y)*f(z + x)*
> f(z + y)*f(b + y + x)*f(c + y + x) - 4*f(2*y)*f(z + x)
> ^2*f(c + 2*y)*
> f(b + y + x) - 2*f(2*y)*f(z + x)^2*f(b + 2*y)*f(b + z +
> x) + 4*f(2*y)
> *f(z + x)^2*f(b + 2*y)*f(a + z + y) - 2*f(2*y)*f(z + x)
> ^2*f(a + 2*y)*
> f(c + 2*y) - 2*f(2*y)*f(z + x)^2*f(a + 2*y)*f(b + z + y)
> + f(2*y)*f(2
> *z)*f(z + y)*f(b + 2*x)*f(b + y + x) - 2*f(2*y)*f(2*z)*f
> (z + y)*f(a
> + y + x)*f(b + y + x) + f(2*y)*f(2*z)*f(z + y)*f(a + 2*
> y)*f(b + 2*x)
> + f(2*y)*f(2*z)*f(z + y)*f(a + 2*y)*f(a + y + x) - f(2*
> y)*f(2*z)*f(z
> + y)*f(a + 2*x)*f(b + 2*y) - f(2*y)*f(2*z)*f(z + x)*f(b
> + 2*y)*f(a
> + y + x) + f(2*y)*f(2*z)*f(z + x)*f(a + 2*y)*f(b + y +
> x) - 3*f(2*y)
> *f(2*z)*f(y + x)*f(c + 2*y)*f(a + y + x) - 2*f(2*y)*f(2*
> z)*f(y + x)*
> f(b + y + x)*f(c + y + x) - 2*f(2*y)*f(2*z)*f(y + x)*f(b
> + y + x)*f(b
> + z + x) + 1/2*f(2*y)*f(2*z)*f(y + x)*f(b + 2*y)*f(c +
> 2*x) - 1/2*f(
> 2*y)*f(2*z)*f(y + x)*f(b + 2*x)*f(c + 2*y) + 4*f(2*y)*f
> (2*z)*f(y + x)
> *f(a + z + y)*f(b + y + x) - 2*f(2*y)*f(2*z)*f(y + x)*f
> (a + y + x)*f(
> b + z + y) - f(2*y)*f(2*z)*f(y + x)*f(a + 2*y)*f(c + y +
> x) - 2*f(2*y)
> )*f(2*z)*f(y + x)*f(a + 2*y)*f(b + z + x) + 2*f(2*y)*f
> (2*z)*f(y + x)*
> f(a + 2*y)*f(a + z + y) - f(2*y)*f(y + x)*f(z + y)*f(c +
> 2*x)*f(c + 2
> *y) + 4*f(2*y)*f(y + x)*f(z + y)*f(b + y + x)*f(c + z +
> x) + 2*f(2*y)
> *f(y + x)*f(z + y)*f(a + 2*y)*f(c + z + x) - f(2*y)*f(y
> + x)*f(z + y)
> *f(a + 2*y)*f(a + 2*z) + 4*f(2*y)*f(y + x)*f(z + x)*f(c
> + 2*y)*f(c +
> y + x) + 2*f(2*y)*f(y + x)*f(z + x)*f(c + 2*y)*f(b + z +
> x) + 4*f(2*y)
> )*f(y + x)*f(z + x)*f(b + z + y)*f(c + y + x) + 2*f(2*y)
> *f(y + x)*f(z
> + x)*f(b + 2*z)*f(b + y + x) - 4*f(2*y)*f(y + x)*f(z +
> x)*f(b + y +
> x)*f(c + z + y) + f(2*y)*f(y + x)*f(z + x)*f(a + 2*z)*f
> (b + 2*y) - 2*
> f(2*y)*f(y + x)*f(z + x)*f(a + 2*y)*f(c + z + y) + f(2*
> y)*f(y + x)*f(

```

```

> z + x)*f(a + 2*y)*f(b + 2*z) - 2*f(2*y)*f(y + x)^2*f(c +
2*z)*f(b + y
> + x) + f(2*y)*f(y + x)^2*f(a + 2*z)*f(c + 2*y) - f(2*y)
*f(y + x)^2*
> f(a + 2*y)*f(c + 2*z) + f(2*y)^2*f(z + y)*f(c + 2*x)*f(c
+ y + x) +
> f(2*y)^2*f(z + y)*f(c + 2*x)*f(b + z + x) - f(2*y)^2*f(z
+ y)*f(b + 2
> *x)*f(c + z + x) + f(2*y)^2*f(z + y)*f(a + 2*z)*f(a + y
+ x) - 2*f(2*
> y)^2*f(z + y)*f(a + y + x)*f(c + z + x) - 2*f(2*y)^2*f(z
+ x)*f(c + y
> + x)^2 - f(2*y)^2*f(z + x)*f(c + 2*x)*f(b + z + y) - 2*
f(2*y)^2*f(z
> + x)*f(b + z + x)*f(c + y + x) - f(2*y)^2*f(z + x)*f(b
+ 2*z)*f(a +
> y + x) + f(2*y)^2*f(z + x)*f(b + 2*x)*f(c + z + y) - f
(2*y)^2*f(z + x
> )*f(a + 2*z)*f(b + y + x) + 2*f(2*y)^2*f(z + x)*f(a + y
+ x)*f(c + z
> + y) - f(2*y)^2*f(2*z)*f(b + 2*x)*f(a + z + y) + 2*f(2*
y)^2*f(2*z)*
> f(a + y + x)*f(c + y + x) + 2*f(2*y)^2*f(2*z)*f(a + y +
x)*f(b + z +
> x) - 2*f(2*y)^2*f(2*z)*f(a + y + x)*f(a + z + y) - 1/2*f
(2*y)^2*f(2*z
> )*f(a + 2*y)*f(c + 2*x) + 1/2*f(2*y)^2*f(2*z)*f(a + 2*x)
*f(c + 2*y)
> + f(2*y)^2*f(2*z)*f(a + 2*x)*f(b + z + y) + f(2*y)^2*f
(y + x)*f(c +
> 2*z)*f(a + y + x) - 1/2*f(2*y)^2*f(y + x)*f(b + 2*z)*f(c
+ 2*x) + 1/2
> *f(2*y)^2*f(y + x)*f(b + 2*x)*f(c + 2*z) - f(2*y)^2*f(y
+ x)*f(a + 2*
> z)*f(c + y + x) + 1/2*f(2*y)^3*f(a + 2*z)*f(c + 2*x) -
1/2*f(2*y)^3*
> f(a + 2*x)*f(c + 2*z) - 2*f(2*x)*f(z + y)^2*f(c + 2*y)*f
(b + y + x)
> - 2*f(2*x)*f(z + y)^2*f(b + 2*y)*f(b + z + x) + 4*f(2*
x)*f(z + y)^2*
> f(b + 2*y)*f(a + z + y) - 2*f(2*x)*f(z + y)^2*f(a + 2*y)
*f(c + 2*y)
> - 2*f(2*x)*f(z + y)^2*f(a + 2*y)*f(b + z + y) - 2*f(2*
x)*f(2*z)*f(y
> + x)*f(b + 2*y)*f(c + 2*y) + f(2*x)*f(y + x)*f(z + y)*f
(c + 2*y)^2
> + 2*f(2*x)*f(y + x)*f(z + y)*f(c + 2*y)*f(b + z + y) +
f(2*x)*f(y +
> x)*f(z + y)*f(b + 2*y)*f(b + 2*z) - f(2*x)*f(2*y)*f(z +
y)*f(c + 2*y)
> *f(c + y + x) - f(2*x)*f(2*y)*f(z + y)*f(c + 2*y)*f(b +
z + x) - 2*f(
> 2*x)*f(2*y)*f(z + y)*f(b + z + y)*f(c + y + x) - f(2*x)*
f(2*y)*f(z +
> y)*f(b + 2*z)*f(b + y + x) + f(2*x)*f(2*y)*f(z + y)*f(b
+ 2*y)*f(c +
> z + x) + f(2*x)*f(2*y)*f(z + x)*f(c + 2*y)*f(b + z + y)

```

```

- f(2*x)*f(2*
> y)*f(z + x)*f(b + 2*y)*f(c + z + y) + 3*f(2*x)*f(2*y)*f
(2*z)*f(c + 2*
> y)*f(b + y + x) + f(2*x)*f(2*y)*f(2*z)*f(b + 2*y)*f(c +
y + x) + 2*f(
> 2*x)*f(2*y)*f(2*z)*f(b + 2*y)*f(b + z + x) - 3*f(2*x)*f
(2*y)*f(2*z)*
> f(b + 2*y)*f(a + z + y) + 2*f(2*x)*f(2*y)*f(2*z)*f(a +
2*y)*f(c + 2*y
> ) + f(2*x)*f(2*y)*f(2*z)*f(a + 2*y)*f(b + z + y) - 1/2*f
(2*x)*f(2*y)*
> f(y + x)*f(b + 2*z)*f(c + 2*y) - 3/2*f(2*x)*f(2*y)*f(y +
x)*f(b + 2*y
> )*f(c + 2*z) + f(2*x)*f(2*y)^2*f(c + 2*z)*f(b + y + x) +
f(2*x)*f(2*y
> )^2*f(b + 2*z)*f(c + y + x) - 1/2*f(2*x)*f(2*y)^2*f(a +
2*z)*f(c + 2*
> y) + 1/2*f(2*x)*f(2*y)^2*f(a + 2*y)*f(c + 2*z) )

> - 2*f(c + 2*y)*f(b + y + x) - 2*f(b + 2*y)*f(b + z + x) +
4*f(b + 2*y)*
> f(a + z + y) - 2*f(a + 2*y)*f(c + 2*y) - 2*f(a + 2*y)*f
(b + z + y) +
> 2*f(y + x)*f(c + b + 2*y) - 2*f(2*y)*f(c + b + y + x):

> eq[10] :=
> (1/HessUniv) * ( - f(2*z)*f(y + x)*f(z + y)*f(a + 2*y)*f(b + 2*
x) +
> f(2*z)*f(y + x)*f(z + y)*f(a + 2*x)*f(b + 2*y) + 2*f(2*
z)*f(y + x)*f(
> z + x)*f(b + 2*y)*f(a + y + x) - f(2*z)*f(y + x)*f(z +
x)*f(b + 2*x)*
> f(b + 2*y) - f(2*z)*f(y + x)*f(z + x)*f(a + 2*y)^2 + 2*f
(y + x)*f(z
> + y)^2*f(a + 2*y)*f(c + 2*x) + 2*f(y + x)*f(z + x)*f(z
+ y)*f(b + 2*
> y)*f(c + 2*x) - 4*f(y + x)*f(z + x)*f(z + y)*f(b + 2*y)*
f(a + z + x)
> + 2*f(y + x)*f(z + x)*f(z + y)*f(b + 2*x)*f(c + 2*y) +
4*f(y + x)*f(
> z + x)*f(z + y)*f(a + 2*y)*f(a + z + y) + 2*f(y + x)*f(z
+ x)^2*f(a
> + 2*y)*f(c + 2*y) - 2*f(y + x)^2*f(z + y)*f(c + 2*x)*f
(c + 2*y) - 2*
> f(y + x)^2*f(z + y)*f(a + 2*y)*f(a + 2*z) - 4*f(y + x)
^2*f(z + x)*f(c
> + 2*y)*f(a + z + y) + 2*f(y + x)^3*f(a + 2*z)*f(c + 2*
y) - 2*f(2*y)*
> f(z + y)^2*f(c + 2*x)*f(a + y + x) + 4*f(2*y)*f(z + x)*f
(z + y)*f(a
> + y + x)*f(c + y + x) - 2*f(2*y)*f(z + x)^2*f(c + 2*y)*
f(a + y + x)
> - f(2*y)*f(z + x)^2*f(b + 2*y)*f(c + 2*x) + 2*f(2*y)*f
(z + x)^2*f(b
> + 2*y)*f(a + z + x) - f(2*y)*f(z + x)^2*f(b + 2*x)*f(c
+ 2*y) - 2*f(
> 2*y)*f(z + x)^2*f(a + 2*y)*f(c + y + x) - 2*f(2*y)*f(z +

```

```

x)^2*f(a + 2
> *y)*f(a + z + y) + f(2*y)*f(2*z)*f(z + y)*f(b + 2*x)*f(a
+ y + x) -
> f(2*y)*f(2*z)*f(z + y)*f(a + 2*x)*f(b + y + x) + f(2*y)*
f(2*z)*f(z +
> x)*f(b + 2*x)*f(b + y + x) - 2*f(2*y)*f(2*z)*f(z + x)*f
(a + y + x)*f(
> b + y + x) + f(2*y)*f(2*z)*f(z + x)*f(a + 2*y)*f(b + 2*
x) + f(2*y)*f(
> 2*z)*f(z + x)*f(a + 2*y)*f(a + y + x) - f(2*y)*f(2*z)*f
(z + x)*f(a +
> 2*x)*f(b + 2*y) - f(2*y)*f(2*z)*f(y + x)*f(c + 2*x)*f(b
+ y + x) - f(
> 2*y)*f(2*z)*f(y + x)*f(b + 2*x)*f(c + y + x) + 2*f(2*y)*
f(2*z)*f(y +
> x)*f(a + z + x)*f(b + y + x) - 2*f(2*y)*f(2*z)*f(y + x)*
f(a + y + x)*
> f(c + y + x) - 2*f(2*y)*f(2*z)*f(y + x)*f(a + y + x)*f(a
+ z + y) - 3/
> 2*f(2*y)*f(2*z)*f(y + x)*f(a + 2*y)*f(c + 2*x) - 1/2*f
(2*y)*f(2*z)*f(
> y + x)*f(a + 2*x)*f(c + 2*y) + 2*f(2*y)*f(y + x)*f(z +
y)*f(c + 2*x)*
> f(c + y + x) + 2*f(2*y)*f(y + x)*f(z + y)*f(a + 2*z)*f(a
+ y + x) + 2
> *f(2*y)*f(y + x)*f(z + x)*f(c + 2*y)*f(a + z + x) + f(2*
y)*f(y + x)*
> f(z + x)*f(c + 2*x)*f(c + 2*y) + 4*f(2*y)*f(y + x)*f(z +
x)*f(a + z
> + y)*f(c + y + x) + f(2*y)*f(y + x)*f(z + x)*f(a + 2*y)
*f(a + 2*z)
> - 2*f(2*y)*f(y + x)^2*f(a + 2*z)*f(c + y + x) + f(2*y)
^2*f(z + y)*f(
> c + 2*x)*f(a + z + x) - f(2*y)^2*f(z + y)*f(a + 2*x)*f(c
+ z + x) -
> f(2*y)^2*f(z + x)*f(c + 2*x)*f(c + y + x) - f(2*y)^2*f(z
+ x)*f(c + 2
> *x)*f(a + z + y) - 2*f(2*y)^2*f(z + x)*f(a + z + x)*f(c
+ y + x) - f(
> 2*y)^2*f(z + x)*f(a + 2*z)*f(a + y + x) + f(2*y)^2*f(z +
x)*f(a + 2*x
> )*f(c + z + y) + f(2*y)^2*f(2*z)*f(c + 2*x)*f(a + y + x)
- f(2*y)^2*
> f(2*z)*f(b + 2*x)*f(a + z + x) + f(2*y)^2*f(2*z)*f(a +
2*x)*f(c + y
> + x) + f(2*y)^2*f(2*z)*f(a + 2*x)*f(b + z + x) + 1/2*f
(2*y)^2*f(y +
> x)*f(a + 2*z)*f(c + 2*x) - 1/2*f(2*y)^2*f(y + x)*f(a +
2*x)*f(c + 2*z
> ) - f(2*x)*f(z + y)^2*f(b + 2*y)*f(c + 2*x) + 2*f(2*x)*f
(z + y)^2*f(b
> + 2*y)*f(a + z + x) - f(2*x)*f(z + y)^2*f(b + 2*x)*f(c
+ 2*y) - 2*f(
> 2*x)*f(z + y)^2*f(a + 2*y)*f(c + y + x) - 2*f(2*x)*f(z +
y)^2*f(a + 2
> *y)*f(a + z + y) - 2*f(2*x)*f(2*z)*f(y + x)*f(b + 2*y)*f
(c + y + x)

```



```

> + 2*f(2*x)*f(2*z)*f(y + x)*f(b + 2*y)*f(b + z + x) - 2*
f(2*x)*f(2*z)
> *f(y + x)*f(b + 2*y)*f(a + z + y) + 2*f(2*x)*f(y + x)*f
(z + y)*f(c +
> 2*y)*f(c + y + x) + 2*f(2*x)*f(y + x)*f(z + y)*f(c + 2*
y)*f(a + z + y
> ) - 2*f(2*x)*f(y + x)*f(z + y)*f(b + 2*y)*f(c + z + x) +
f(2*x)*f(y
> + x)*f(z + y)*f(a + 2*z)*f(b + 2*y) + f(2*x)*f(y + x)*f
(z + y)*f(a
> + 2*y)*f(b + 2*z) - f(2*x)*f(y + x)*f(z + x)*f(c + 2*y)
^2 + 2*f(2*x)
> *f(y + x)*f(z + x)*f(b + 2*y)*f(c + z + y) - f(2*x)*f(y
+ x)*f(z + x)
> *f(b + 2*y)*f(b + 2*z) - f(2*x)*f(y + x)^2*f(b + 2*z)*f
(c + 2*y) + f(
> 2*x)*f(y + x)^2*f(b + 2*y)*f(c + 2*z) - 2*f(2*x)*f(2*y)*
f(z + y)*f(c
> + y + x)^2 - f(2*x)*f(2*y)*f(z + y)*f(c + 2*y)*f(a + z
+ x) - f(2*x)
> *f(2*y)*f(z + y)*f(b + 2*z)*f(a + y + x) + 2*f(2*x)*f(2*
y)*f(z + y)*
> f(b + y + x)*f(c + z + x) - 2*f(2*x)*f(2*y)*f(z + y)*f(a
+ z + y)*f(c
> + y + x) - f(2*x)*f(2*y)*f(z + y)*f(a + 2*z)*f(b + y +
x) + f(2*x)*
> f(2*y)*f(z + y)*f(a + 2*y)*f(c + z + x) + f(2*x)*f(2*y)*
f(z + x)*f(c
> + 2*y)*f(c + y + x) + f(2*x)*f(2*y)*f(z + x)*f(c + 2*y)
*f(a + z + y)
> + f(2*x)*f(2*y)*f(z + x)*f(b + 2*z)*f(b + y + x) - 2*f
(2*x)*f(2*y)*
> f(z + x)*f(b + y + x)*f(c + z + y) - f(2*x)*f(2*y)*f(z +
x)*f(a + 2*y
> )*f(c + z + y) + 2*f(2*x)*f(2*y)*f(2*z)*f(b + y + x)*f(c
+ y + x) - 2
> *f(2*x)*f(2*y)*f(2*z)*f(b + y + x)*f(b + z + x) + 3/2*f
(2*x)*f(2*y)*
> f(2*z)*f(b + 2*y)*f(c + 2*x) - f(2*x)*f(2*y)*f(2*z)*f(b
+ 2*y)*f(a +
> z + x) + 1/2*f(2*x)*f(2*y)*f(2*z)*f(b + 2*x)*f(c + 2*y)
+ 2*f(2*x)*f(
> 2*y)*f(2*z)*f(a + z + y)*f(b + y + x) + 2*f(2*x)*f(2*y)*
f(2*z)*f(a +
> 2*y)*f(c + y + x) - f(2*x)*f(2*y)*f(2*z)*f(a + 2*y)*f(b
+ z + x) + 2*
> f(2*x)*f(2*y)*f(2*z)*f(a + 2*y)*f(a + z + y) - f(2*x)*f
(2*y)*f(y + x)
> *f(c + 2*z)*f(b + y + x) + f(2*x)*f(2*y)*f(y + x)*f(b +
2*z)*f(c + y
> + x) - 3/2*f(2*x)*f(2*y)*f(y + x)*f(a + 2*z)*f(c + 2*y)
- 1/2*f(2*x)
> *f(2*y)*f(y + x)*f(a + 2*y)*f(c + 2*z) + f(2*x)*f(2*y)
^2*f(c + 2*z)*
> f(a + y + x) - 1/2*f(2*x)*f(2*y)^2*f(b + 2*z)*f(c + 2*x)
+ 1/2*f(2*x)
> *f(2*y)^2*f(b + 2*x)*f(c + 2*z) + f(2*x)*f(2*y)^2*f(a +

```

```

2*z)*f(c + y
> + x) + 1/2*f(2*x)^2*f(2*y)*f(b + 2*z)*f(c + 2*y) - 1/2*
f(2*x)^2*f(2*
> y)*f(b + 2*y)*f(c + 2*z) )
>
> - f(b + 2*y)*f(c + 2*x) + 2*f(b + 2*y)*f(a + z + x) - f(b
+ 2*x)*f(c +
> 2*y) - 2*f(a + 2*y)*f(c + y + x) - 2*f(a + 2*y)*f(a + z
+ y) + 2*f(y
> + x)*f(c + a + 2*y) - 2*f(2*y)*f(c + a + y + x):
> eq[11] :=
> (1/HessUniv) * ( - f(2*y)*f(z + y)^2*f(b + 2*x)*f(c + 2*x) + 2*f
(2*y
> )*f(z + x)*f(z + y)*f(b + 2*x)*f(c + y + x) - f(2*y)*f(z
+ x)^2*f(b
> + 2*x)*f(c + 2*y) + 1/2*f(2*y)*f(2*z)*f(z + y)*f(b + 2*
x)^2 - f(2*y)
> *f(2*z)*f(z + y)*f(a + 2*x)*f(b + y + x) + 1/2*f(2*y)*f
(2*z)*f(z + y)
> *f(a + 2*x)*f(a + 2*y) + 1/2*f(2*y)*f(2*z)*f(z + x)*f(a
+ 2*y)*f(b +
> 2*x) - 1/2*f(2*y)*f(2*z)*f(z + x)*f(a + 2*x)*f(b + 2*y)
- f(2*y)*f(2*
> z)*f(y + x)*f(b + 2*x)*f(c + y + x) - f(2*y)*f(2*z)*f(y
+ x)*f(b + 2*
> x)*f(b + z + x) - 1/2*f(2*y)*f(2*z)*f(y + x)*f(a + 2*y)*
f(c + 2*x) -
> 1/2*f(2*y)*f(2*z)*f(y + x)*f(a + 2*x)*f(c + 2*y) + f(2*
y)*f(2*z)*f(y
> + x)*f(a + 2*x)*f(b + z + y) + 2*f(2*y)*f(y + x)*f(z +
y)*f(c + 2*x)
> *f(b + z + x) + f(2*y)*f(y + x)*f(z + x)*f(c + 2*x)*f(c
+ 2*y) + f(2*
> y)*f(y + x)*f(z + x)*f(b + 2*x)*f(b + 2*z) - f(2*y)*f(y
+ x)^2*f(b +
> 2*z)*f(c + 2*x) + 1/2*f(2*y)^2*f(z + y)*f(c + 2*x)^2 - f
(2*y)^2*f(z
> + y)*f(a + 2*x)*f(c + z + x) + 1/2*f(2*y)^2*f(z + y)*f
(a + 2*x)*f(a
> + 2*z) - f(2*y)^2*f(z + x)*f(c + 2*x)*f(c + y + x) - f
(2*y)^2*f(z +
> x)*f(c + 2*x)*f(b + z + x) - 1/2*f(2*y)^2*f(z + x)*f(a +
2*z)*f(b + 2
> *x) + f(2*y)^2*f(z + x)*f(a + 2*x)*f(c + z + y) - 1/2*f
(2*y)^2*f(z +
> x)*f(a + 2*x)*f(b + 2*z) + f(2*y)^2*f(2*z)*f(a + 2*x)*f
(c + y + x) +
> f(2*y)^2*f(2*z)*f(a + 2*x)*f(b + z + x) - f(2*y)^2*f(2*
z)*f(a + 2*x)*
> f(a + z + y) + 1/2*f(2*y)^2*f(y + x)*f(a + 2*z)*f(c + 2*
x) - 1/2*f(2*
> y)^2*f(y + x)*f(a + 2*x)*f(c + 2*z) + f(2*x)*f(z + y)^2*
f(b + 2*y)*f(
> c + 2*x) - 2*f(2*x)*f(z + x)*f(z + y)*f(b + 2*y)*f(c + y
+ x) + f(2*x
> )*f(z + x)^2*f(b + 2*y)*f(c + 2*y) + 2*f(2*x)*f(2*z)*f(z
+ y)*f(b + 2

```

```

>      *y)*f(a + y + x) - 1/2*f(2*x)*f(2*z)*f(z + y)*f(b + 2*x)
>      *f(b + 2*y)
>      - f(2*x)*f(2*z)*f(z + y)*f(a + 2*y)*f(b + y + x) - 1/2*
>      f(2*x)*f(2*z)
>      *f(z + y)*f(a + 2*y)^2 + f(2*x)*f(2*z)*f(y + x)*f(c + 2*
>      y)*f(b + y +
>      x) + f(2*x)*f(2*z)*f(y + x)*f(b + 2*y)*f(b + z + x) - 2*
>      f(2*x)*f(2*z)
>      *f(y + x)*f(b + 2*y)*f(a + z + y) + f(2*x)*f(2*z)*f(y +
>      x)*f(a + 2*y)
>      *f(c + 2*y) + f(2*x)*f(2*z)*f(y + x)*f(a + 2*y)*f(b + z
>      + y) - 2*f(2*
>      x)*f(y + x)*f(z + y)*f(b + 2*y)*f(c + z + x) - f(2*x)*f
>      (y + x)*f(z +
>      x)*f(c + 2*y)^2 - 2*f(2*x)*f(y + x)*f(z + x)*f(c + 2*y)*
>      f(b + z + y)
>      + 2*f(2*x)*f(y + x)*f(z + x)*f(b + 2*y)*f(c + z + y) -
>      f(2*x)*f(y +
>      x)*f(z + x)*f(b + 2*y)*f(b + 2*z) + f(2*x)*f(y + x)^2*f
>      (b + 2*y)*f(c
>      + 2*z) - f(2*x)*f(2*y)*f(z + y)*f(c + 2*x)*f(c + 2*y) -
>      f(2*x)*f(2*y
>      )*f(z + y)*f(c + 2*x)*f(b + z + y) - 2*f(2*x)*f(2*y)*f(z
>      + y)*f(b + z
>      + x)*f(c + y + x) + 2*f(2*x)*f(2*y)*f(z + y)*f(b + y +
>      x)*f(c + z +
>      x) - 1/2*f(2*x)*f(2*y)*f(z + y)*f(b + 2*x)*f(b + 2*z) +
>      f(2*x)*f(2*y)
>      *f(z + y)*f(a + 2*y)*f(c + z + x) - 1/2*f(2*x)*f(2*y)*f
>      (z + y)*f(a +
>      2*y)*f(a + 2*z) + f(2*x)*f(2*y)*f(z + x)*f(c + 2*y)*f(c
>      + y + x) + f(
>      2*x)*f(2*y)*f(z + x)*f(c + 2*y)*f(b + z + x) + 2*f(2*x)*
>      f(2*y)*f(z +
>      x)*f(b + z + y)*f(c + y + x) - 2*f(2*x)*f(2*y)*f(z + x)*
>      f(b + y + x)*
>      f(c + z + y) + 1/2*f(2*x)*f(2*y)*f(z + x)*f(a + 2*z)*f(b
>      + 2*y) - f(2
>      *x)*f(2*y)*f(z + x)*f(a + 2*y)*f(c + z + y) + 1/2*f(2*x)
>      *f(2*y)*f(z
>      + x)*f(a + 2*y)*f(b + 2*z) - f(2*x)*f(2*y)*f(2*z)*f(c +
>      2*y)*f(a + y
>      + x) + 1/2*f(2*x)*f(2*y)*f(2*z)*f(b + 2*y)*f(c + 2*x) +
>      1/2*f(2*x)*
>      f(2*y)*f(2*z)*f(b + 2*x)*f(c + 2*y) + 2*f(2*x)*f(2*y)*f
>      (2*z)*f(a + z
>      + y)*f(b + y + x) - 2*f(2*x)*f(2*y)*f(2*z)*f(a + y + x)
>      *f(b + z + y)
>      - f(2*x)*f(2*y)*f(2*z)*f(a + 2*y)*f(b + z + x) + f(2*x)
>      *f(2*y)*f(2*z
>      )*f(a + 2*y)*f(a + z + y) - f(2*x)*f(2*y)*f(y + x)*f(c +
>      2*z)*f(b + y
>      + x) + f(2*x)*f(2*y)*f(y + x)*f(b + 2*z)*f(c + y + x) +
>      1/2*f(2*x)*
>      f(2*y)*f(y + x)*f(a + 2*z)*f(c + 2*y) - 1/2*f(2*x)*f(2*
>      y)*f(y + x)*f(
>      a + 2*y)*f(c + 2*z) + f(2*x)*f(2*y)^2*f(c + 2*z)*f(a + y

```

```

+ x) + 1/2*
>      f(2*x)*f(2*y)^2*f(b + 2*z)*f(c + 2*x) + 1/2*f(2*x)*f(2*
y)^2*f(b + 2*x
>      )*f(c + 2*z) - f(2*x)*f(2*y)^2*f(a + 2*z)*f(c + y + x) +
1/2*f(2*x)^2
>      *f(z + y)*f(c + 2*y)^2 + f(2*x)^2*f(z + y)*f(c + 2*y)*f
(b + z + y) +
>      1/2*f(2*x)^2*f(z + y)*f(b + 2*y)*f(b + 2*z) - f(2*x)^2*f
(2*z)*f(b + 2
>      *y)*f(c + 2*y) - 1/2*f(2*x)^2*f(2*y)*f(b + 2*z)*f(c + 2*
y) - 1/2*f(2*
>      x)^2*f(2*y)*f(b + 2*y)*f(c + 2*z) )
>
>      - f(2*y)*f(c + b + 2*x) + f(2*x)*f(c + b + 2*y):
>
> eq[12] :=
> (1/HessUniv) * ( - f(2*y)*f(z + y)^2*f(a + 2*x)*f(c + 2*x) + 2*f
(2*y
>      )*f(z + x)*f(z + y)*f(a + 2*x)*f(c + y + x) - f(2*y)*f(z
+ x)^2*f(a
>      + 2*x)*f(c + 2*y) + 1/2*f(2*y)*f(2*z)*f(z + x)*f(b + 2*
x)^2 + f(2*y)
>      *f(2*z)*f(z + x)*f(b + 2*x)*f(a + y + x) - 2*f(2*y)*f(2*
z)*f(z + x)*
>      f(a + 2*x)*f(b + y + x) + 1/2*f(2*y)*f(2*z)*f(z + x)*f(a
+ 2*x)*f(a
>      + 2*y) - f(2*y)*f(2*z)*f(y + x)*f(c + 2*x)*f(a + y + x)
- f(2*y)*f(2
>      *z)*f(y + x)*f(b + 2*x)*f(c + 2*x) - f(2*y)*f(2*z)*f(y +
x)*f(b + 2*x
>      )*f(a + z + x) + 2*f(2*y)*f(2*z)*f(y + x)*f(a + 2*x)*f(b
+ z + x) -
>      f(2*y)*f(2*z)*f(y + x)*f(a + 2*x)*f(a + z + y) + f(2*y)*
f(y + x)*f(z
>      + y)*f(c + 2*x)^2 + 2*f(2*y)*f(y + x)*f(z + y)*f(c + 2*
x)*f(a + z +
>      x) - 2*f(2*y)*f(y + x)*f(z + y)*f(a + 2*x)*f(c + z + x)
+ f(2*y)*f(y
>      + x)*f(z + y)*f(a + 2*x)*f(a + 2*z) + 2*f(2*y)*f(y + x)
*f(z + x)*f(a
>      + 2*x)*f(c + z + y) - f(2*y)*f(y + x)^2*f(a + 2*x)*f(c
+ 2*z) - 1/2*
>      f(2*y)^2*f(z + x)*f(c + 2*x)^2 - f(2*y)^2*f(z + x)*f(c +
2*x)*f(a + z
>      + x) - 1/2*f(2*y)^2*f(z + x)*f(a + 2*x)*f(a + 2*z) + f
(2*y)^2*f(2*z)
>      *f(a + 2*x)*f(c + 2*x) + f(2*x)*f(z + y)^2*f(a + 2*y)*f
(c + 2*x) - 2*
>      f(2*x)*f(z + x)*f(z + y)*f(a + 2*y)*f(c + y + x) + f(2*
x)*f(z + x)^2*
>      f(a + 2*y)*f(c + 2*y) - 1/2*f(2*x)*f(2*z)*f(z + y)*f(a +
2*y)*f(b + 2
>      *x) + 1/2*f(2*x)*f(2*z)*f(z + y)*f(a + 2*x)*f(b + 2*y) +
f(2*x)*f(2*z
>      )*f(z + x)*f(b + 2*y)*f(a + y + x) - 1/2*f(2*x)*f(2*z)*f
(z + x)*f(b
>      + 2*x)*f(b + 2*y) - 1/2*f(2*x)*f(2*z)*f(z + x)*f(a + 2*

```

```

y)^2 + 1/2*f(
>      2*x)*f(2*z)*f(y + x)*f(b + 2*y)*f(c + 2*x) - f(2*x)*f(2*
>      z)*f(y + x)*
>      f(b + 2*y)*f(a + z + x) + 1/2*f(2*x)*f(2*z)*f(y + x)*f(b
>      + 2*x)*f(c
>      + 2*y) + f(2*x)*f(2*z)*f(y + x)*f(a + 2*y)*f(c + y + x)
>      + f(2*x)*f(2
>      *z)*f(y + x)*f(a + 2*y)*f(a + z + y) - f(2*x)*f(y + x)*f
>      (z + y)*f(c
>      + 2*x)*f(c + 2*y) - f(2*x)*f(y + x)*f(z + y)*f(a + 2*y)
>      *f(a + 2*z)
>      - 2*f(2*x)*f(y + x)*f(z + x)*f(c + 2*y)*f(a + z + y) +
>      f(2*x)*f(y +
>      x)^2*f(a + 2*z)*f(c + 2*y) - f(2*x)*f(2*y)*f(z + y)*f(c
>      + 2*x)*f(c +
>      y + x) - f(2*x)*f(2*y)*f(z + y)*f(c + 2*x)*f(a + z + y)
>      + f(2*x)*f(2*
>      y)*f(z + y)*f(b + 2*x)*f(c + z + x) - 2*f(2*x)*f(2*y)*f
>      (z + y)*f(a +
>      z + x)*f(c + y + x) - 1/2*f(2*x)*f(2*y)*f(z + y)*f(a +
>      2*z)*f(b + 2*x
>      ) + 2*f(2*x)*f(2*y)*f(z + y)*f(a + y + x)*f(c + z + x) -
>      1/2*f(2*x)*
>      f(2*y)*f(z + y)*f(a + 2*x)*f(b + 2*z) + f(2*x)*f(2*y)*f
>      (z + x)*f(c +
>      2*y)*f(a + z + x) + f(2*x)*f(2*y)*f(z + x)*f(c + 2*x)*f
>      (c + 2*y) - f(
>      2*x)*f(2*y)*f(z + x)*f(b + 2*x)*f(c + z + y) + 1/2*f(2*
>      x)*f(2*y)*f(z
>      + x)*f(b + 2*x)*f(b + 2*z) + 2*f(2*x)*f(2*y)*f(z + x)*f
>      (a + z + y)*
>      f(c + y + x) - 2*f(2*x)*f(2*y)*f(z + x)*f(a + y + x)*f(c
>      + z + y) + 1/
>      2*f(2*x)*f(2*y)*f(z + x)*f(a + 2*y)*f(a + 2*z) + f(2*x)*
>      f(2*y)*f(2*z)
>      *f(c + 2*x)*f(b + y + x) - f(2*x)*f(2*y)*f(2*z)*f(b + 2*
>      x)*f(b + z +
>      x) + f(2*x)*f(2*y)*f(2*z)*f(b + 2*x)*f(a + z + y) + 2*f
>      (2*x)*f(2*y)*
>      f(2*z)*f(a + z + x)*f(b + y + x) - 2*f(2*x)*f(2*y)*f(2*
>      z)*f(a + y + x
>      )*f(b + z + x) - 1/2*f(2*x)*f(2*y)*f(2*z)*f(a + 2*y)*f(c
>      + 2*x) - 1/2
>      *f(2*x)*f(2*y)*f(2*z)*f(a + 2*x)*f(c + 2*y) + f(2*x)*f
>      (2*y)*f(y + x)*
>      f(c + 2*z)*f(a + y + x) - 1/2*f(2*x)*f(2*y)*f(y + x)*f(b
>      + 2*z)*f(c
>      + 2*x) + 1/2*f(2*x)*f(2*y)*f(y + x)*f(b + 2*x)*f(c + 2*
>      z) - f(2*x)*
>      f(2*y)*f(y + x)*f(a + 2*z)*f(c + y + x) + 1/2*f(2*x)*f
>      (2*y)^2*f(a + 2
>      *z)*f(c + 2*x) + 1/2*f(2*x)*f(2*y)^2*f(a + 2*x)*f(c + 2*
>      z) + f(2*x)^2
>      *f(z + y)*f(c + 2*y)*f(c + y + x) + f(2*x)^2*f(z + y)*f
>      (c + 2*y)*f(a
>      + z + y) - f(2*x)^2*f(z + y)*f(b + 2*y)*f(c + z + x) +
>      1/2*f(2*x)^2*

```

```

>      f(z + y)*f(a + 2*z)*f(b + 2*y) + 1/2*f(2*x)^2*f(z + y)*f
(a + 2*y)*f(b
>      + 2*z) - 1/2*f(2*x)^2*f(z + x)*f(c + 2*y)^2 + f(2*x)^2*
f(z + x)*f(b
>      + 2*y)*f(c + z + y) - 1/2*f(2*x)^2*f(z + x)*f(b + 2*y)*
f(b + 2*z) -
>      f(2*x)^2*f(2*z)*f(b + 2*y)*f(c + y + x) + f(2*x)^2*f(2*
z)*f(b + 2*y)*
>      f(b + z + x) - f(2*x)^2*f(2*z)*f(b + 2*y)*f(a + z + y) -
1/2*f(2*x)^2
>      *f(y + x)*f(b + 2*z)*f(c + 2*y) + 1/2*f(2*x)^2*f(y + x)*
f(b + 2*y)*f(
>      c + 2*z) - f(2*x)^2*f(2*y)*f(c + 2*z)*f(b + y + x) + f
(2*x)^2*f(2*y)*
>      f(b + 2*z)*f(c + y + x) - 1/2*f(2*x)^2*f(2*y)*f(a + 2*z)
*f(c + 2*y)
>      - 1/2*f(2*x)^2*f(2*y)*f(a + 2*y)*f(c + 2*z) )
>
>      - f(2*y)*f(c + a + 2*x) + f(2*x)*f(c + a + 2*y):
>
> eq[13] :=
> (1/HessUniv) * ( 2*f(2*z)^2*f(y + x)*f(b + 2*y)*f(a + y + x) - f
(2*z)
>      ^2*f(y + x)*f(b + 2*x)*f(b + 2*y) - f(2*z)^2*f(y + x)*f
(a + 2*y)^2 +
>      2*f(2*z)*f(y + x)*f(z + y)*f(b + 2*y)*f(c + 2*x) - 2*f
(2*z)*f(y + x)*
>      f(z + y)*f(a + 2*y)*f(c + y + x) - 2*f(2*z)*f(y + x)*f(z
+ y)*f(a + 2
>      *y)*f(b + z + x) + 2*f(2*z)*f(y + x)*f(z + y)*f(a + 2*y)
*f(a + z + y)
>      - 2*f(2*z)*f(y + x)*f(z + x)*f(b + 2*y)*f(c + y + x) +
2*f(2*z)*f(y
>      + x)*f(z + x)*f(b + 2*y)*f(b + z + x) - 2*f(2*z)*f(y +
x)*f(z + x)*
>      f(b + 2*y)*f(a + z + y) + 2*f(2*z)*f(y + x)*f(z + x)*f(a
+ 2*y)*f(c
>      + 2*y) + 4*f(y + x)*f(z + y)^2*f(a + 2*y)*f(c + z + x)
- 2*f(y + x)*
>      f(z + y)^2*f(a + 2*y)*f(a + 2*z) + 4*f(y + x)*f(z + x)*f
(z + y)*f(c
>      + 2*y)*f(c + y + x) + 4*f(y + x)*f(z + x)*f(z + y)*f(c
+ 2*y)*f(b +
>      z + x) - 4*f(y + x)*f(z + x)*f(z + y)*f(c + 2*y)*f(a + z
+ y) - 4*f(y
>      + x)*f(z + x)*f(z + y)*f(b + 2*y)*f(c + z + x) - 2*f(y
+ x)*f(z + x)
>      *f(z + y)*f(a + 2*z)*f(b + 2*y) + 4*f(y + x)*f(z + x)*f
(z + y)*f(a +
>      2*y)*f(c + z + y) + 2*f(y + x)*f(z + x)*f(z + y)*f(a +
2*y)*f(b + 2*z
>      ) + 4*f(y + x)*f(z + x)^2*f(b + 2*y)*f(c + z + y) - 2*f
(y + x)*f(z +
>      x)^2*f(b + 2*y)*f(b + 2*z) - 4*f(y + x)^2*f(z + y)*f(c +
2*y)*f(c + z
>      + x) + 2*f(y + x)^2*f(z + y)*f(a + 2*z)*f(c + 2*y) - 2*
f(y + x)^2*f(

```

```

>      z + y)*f(a + 2*y)*f(c + 2*z) - 4*f(y + x)^2*f(z + x)*f(c
+ 2*y)*f(c
>      + z + y) - 2*f(y + x)^2*f(z + x)*f(b + 2*z)*f(c + 2*y)
+ 2*f(y + x)^
>      2*f(z + x)*f(b + 2*y)*f(c + 2*z) + 2*f(y + x)^3*f(c + 2*
y)*f(c + 2*z)
>      + 2*f(2*y)*f(z + y)^2*f(a + 2*z)*f(a + y + x) - 4*f(2*
y)*f(z + y)^2*
>      f(a + y + x)*f(c + z + x) - 2*f(2*y)*f(z + x)*f(z + y)*f
(b + 2*z)*f(a
>      + y + x) + 4*f(2*y)*f(z + x)*f(z + y)*f(b + y + x)*f(c
+ z + x) - 2*
>      f(2*y)*f(z + x)*f(z + y)*f(a + 2*z)*f(b + y + x) + 4*f
(2*y)*f(z + x)*
>      f(z + y)*f(a + y + x)*f(c + z + y) - 2*f(2*y)*f(z + x)
^2*f(c + 2*y)*
>      f(c + y + x) - 2*f(2*y)*f(z + x)^2*f(c + 2*y)*f(b + z +
x) + 2*f(2*y)
>      *f(z + x)^2*f(c + 2*y)*f(a + z + y) + 2*f(2*y)*f(z + x)
^2*f(b + 2*z)*
>      f(b + y + x) - 4*f(2*y)*f(z + x)^2*f(b + y + x)*f(c + z
+ y) + 2*f(2*
>      y)*f(z + x)^2*f(a + 2*z)*f(b + 2*y) - 4*f(2*y)*f(z + x)
^2*f(a + 2*y)*
>      f(c + z + y) - 2*f(2*y)*f(2*z)*f(z + y)*f(c + 2*x)*f(b +
y + x) + 2*
>      f(2*y)*f(2*z)*f(z + y)*f(a + y + x)*f(c + y + x) + 2*f
(2*y)*f(2*z)*f(
>      z + y)*f(a + y + x)*f(b + z + x) - 2*f(2*y)*f(2*z)*f(z +
y)*f(a + y
>      + x)*f(a + z + y) - 2*f(2*y)*f(2*z)*f(z + x)*f(c + 2*y)
*f(a + y + x)
>      + 2*f(2*y)*f(2*z)*f(z + x)*f(b + y + x)*f(c + y + x) -
2*f(2*y)*f(2*
>      z)*f(z + x)*f(b + y + x)*f(b + z + x) + 2*f(2*y)*f(2*z)*
f(z + x)*f(a
>      + z + y)*f(b + y + x) + f(2*y)*f(2*z)^2*f(b + 2*x)*f(b
+ y + x) - 2*
>      f(2*y)*f(2*z)^2*f(a + y + x)*f(b + y + x) + 1/2*f(2*y)*f
(2*z)^2*f(a
>      + 2*y)*f(b + 2*x) + f(2*y)*f(2*z)^2*f(a + 2*y)*f(a + y
+ x) - 1/2*f(
>      2*y)*f(2*z)^2*f(a + 2*x)*f(b + 2*y) - 2*f(2*y)*f(2*z)*f
(y + x)*f(c +
>      y + x)^2 - f(2*y)*f(2*z)*f(y + x)*f(c + 2*x)*f(c + 2*y)
- 2*f(2*y)*f(
>      2*z)*f(y + x)*f(b + z + x)*f(c + y + x) + 2*f(2*y)*f(2*
z)*f(y + x)*f(
>      a + z + y)*f(c + y + x) + 2*f(2*y)*f(2*z)*f(y + x)*f(a +
2*z)*f(b + y
>      + x) - 4*f(2*y)*f(2*z)*f(y + x)*f(a + y + x)*f(c + z +
y) - 2*f(2*y)
>      *f(2*z)*f(y + x)*f(a + 2*y)*f(c + z + x) + f(2*y)*f(2*z)
*f(y + x)*f(a
>      + 2*y)*f(a + 2*z) + 2*f(2*y)*f(y + x)*f(z + y)*f(c + 2*
z)*f(a + y +
>      x) + 4*f(2*y)*f(y + x)*f(z + y)*f(c + y + x)*f(c + z +

```

```

x) - 2*f(2*y)*
>      f(y + x)*f(z + y)*f(a + 2*z)*f(c + y + x) - 2*f(2*y)*f(y
+ x)*f(z + x
>      )*f(c + 2*z)*f(b + y + x) + 4*f(2*y)*f(y + x)*f(z + x)*f
(c + y + x)*
>      f(c + z + y) + 4*f(2*y)*f(y + x)*f(z + x)*f(c + 2*y)*f(c
+ z + x) + 2
>      *f(2*y)*f(y + x)*f(z + x)*f(b + 2*z)*f(c + y + x) - 2*f
(2*y)*f(y + x)
>      ^2*f(c + 2*z)*f(c + y + x) + f(2*y)^2*f(z + y)*f(a + 2*
z)*f(c + 2*x)
>      - f(2*y)^2*f(z + y)*f(a + 2*x)*f(c + 2*z) - 4*f(2*y)^2*
f(z + x)*f(c
>      + y + x)*f(c + z + x) - f(2*y)^2*f(z + x)*f(b + 2*z)*f
(c + 2*x) + f(
>      2*y)^2*f(z + x)*f(b + 2*x)*f(c + 2*z) + f(2*y)^2*f(2*z)*
f(c + 2*x)*f(
>      c + y + x) + f(2*y)^2*f(2*z)*f(c + 2*x)*f(b + z + x) - f
(2*y)^2*f(2*z
>      )*f(c + 2*x)*f(a + z + y) - f(2*y)^2*f(2*z)*f(b + 2*x)*f
(c + z + x)
>      - 1/2*f(2*y)^2*f(2*z)*f(a + 2*z)*f(b + 2*x) - f(2*y)^2*
f(2*z)*f(a +
>      2*z)*f(a + y + x) + 2*f(2*y)^2*f(2*z)*f(a + y + x)*f(c +
z + x) + f(2
>      *y)^2*f(2*z)*f(a + 2*x)*f(c + z + y) + 1/2*f(2*y)^2*f(2*
z)*f(a + 2*x)
>      *f(b + 2*z) - 2*f(2*x)*f(z + y)^2*f(c + 2*y)*f(c + y +
x) - 2*f(2*x)*
>      f(z + y)^2*f(c + 2*y)*f(b + z + x) + 2*f(2*x)*f(z + y)
^2*f(c + 2*y)*
>      f(a + z + y) + 2*f(2*x)*f(z + y)^2*f(a + 2*z)*f(b + 2*y)
- 4*f(2*x)*
>      f(z + y)^2*f(a + 2*y)*f(c + z + y) - f(2*x)*f(2*z)*f(y +
x)*f(c + 2*y
>      )^2 - 2*f(2*x)*f(2*z)*f(y + x)*f(b + 2*y)*f(c + z + y) +
f(2*x)*f(2*z
>      )*f(y + x)*f(b + 2*y)*f(b + 2*z) + 4*f(2*x)*f(y + x)*f(z
+ y)*f(c + 2
>      *y)*f(c + z + y) - 4*f(2*x)*f(2*y)*f(z + y)*f(c + y + x)
*f(c + z + y)
>      - f(2*x)*f(2*y)*f(z + y)*f(a + 2*z)*f(c + 2*y) + f(2*x)
*f(2*y)*f(z
>      + y)*f(a + 2*y)*f(c + 2*z) + f(2*x)*f(2*y)*f(z + x)*f(b
+ 2*z)*f(c
>      + 2*y) - f(2*x)*f(2*y)*f(z + x)*f(b + 2*y)*f(c + 2*z) +
3*f(2*x)*f(2
>      *y)*f(2*z)*f(c + 2*y)*f(c + y + x) + f(2*x)*f(2*y)*f(2*
z)*f(c + 2*y)*
>      f(b + z + x) - f(2*x)*f(2*y)*f(2*z)*f(c + 2*y)*f(a + z +
y) - f(2*x)*
>      f(2*y)*f(2*z)*f(b + 2*z)*f(b + y + x) + 2*f(2*x)*f(2*y)*
f(2*z)*f(b +
>      y + x)*f(c + z + y) + f(2*x)*f(2*y)*f(2*z)*f(b + 2*y)*f
(c + z + x) -
>      3/2*f(2*x)*f(2*y)*f(2*z)*f(a + 2*z)*f(b + 2*y) + 3*f(2*
x)*f(2*y)*f(2*

```



```

>      z)*f(a + 2*y)*f(c + z + y) - 1/2*f(2*x)*f(2*y)*f(2*z)*f
(a + 2*y)*f(b
>      + 2*z) - 2*f(2*x)*f(2*y)*f(y + x)*f(c + 2*y)*f(c + 2*z)
+ 2*f(2*x)*
>      f(2*y)^2*f(c + 2*z)*f(c + y + x) )
>
>      - 2*f(c + 2*y)*f(c + y + x) - 2*f(c + 2*y)*f(b + z + x) +
2*f(c + 2*y)*
>      f(a + z + y) + 2*f(a + 2*z)*f(b + 2*y) - 4*f(a + 2*y)*f
(c + z + y) +
>      2*f(y + x)*f(2*c + 2*y) - 2*f(2*y)*f(2*c + y + x):
> eq[14] :=
> (1/HessUniv) * ( 4*f(2*z)*f(z + y)^2*f(b + 2*y)*f(a + y + x) - 2*
f(2*
>      z)*f(z + y)^2*f(a + 2*y)*f(b + y + x) - f(2*z)*f(z + y)
^2*f(a + 2*y)^
>      2 - 2*f(2*z)*f(z + x)*f(z + y)*f(b + 2*y)*f(b + y + x) +
f(2*z)*f(z
>      + x)^2*f(b + 2*y)^2 + 2*f(2*z)^2*f(y + x)*f(b + 2*y)*f
(b + y + x) +
>      2*f(2*z)*f(y + x)*f(z + y)*f(c + 2*y)*f(b + y + x) - 4*f
(2*z)*f(y + x
>      )*f(z + y)*f(b + 2*y)*f(c + y + x) - 4*f(2*z)*f(y + x)*f
(z + y)*f(b
>      + 2*y)*f(a + z + y) + 2*f(2*z)*f(y + x)*f(z + y)*f(a +
2*y)*f(c + 2*
>      y) + 2*f(2*z)*f(y + x)*f(z + y)*f(a + 2*y)*f(b + z + y)
- 2*f(2*z)*f(
>      y + x)*f(z + x)*f(b + 2*y)*f(b + z + y) - 2*f(y + x)*f(z
+ x)*f(z + y
>      )*f(c + 2*y)^2 - 4*f(y + x)*f(z + x)*f(z + y)*f(c + 2*y)
*f(b + z + y)
>      + 8*f(y + x)*f(z + x)*f(z + y)*f(b + 2*y)*f(c + z + y)
- 2*f(2*y)*f(
>      z + y)^2*f(a + 2*z)*f(b + y + x) + f(2*y)*f(z + y)^2*f(a
+ 2*y)*f(a
>      + 2*z) + 2*f(2*y)*f(z + x)*f(z + y)*f(b + 2*z)*f(b + y
+ x) + f(2*y)
>      *f(z + x)*f(z + y)*f(a + 2*z)*f(b + 2*y) - f(2*y)*f(z +
x)*f(z + y)*
>      f(a + 2*y)*f(b + 2*z) + f(2*y)*f(z + x)^2*f(c + 2*y)^2 +
2*f(2*y)*f(z
>      + x)^2*f(c + 2*y)*f(b + z + y) - 4*f(2*y)*f(z + x)^2*f
(b + 2*y)*f(c
>      + z + y) - f(2*y)*f(z + x)^2*f(b + 2*y)*f(b + 2*z) - 2*
f(2*y)*f(2*z)
>      *f(z + y)*f(c + 2*y)*f(a + y + x) + f(2*y)*f(2*z)*f(z +
y)*f(b + 2*y)
>      *f(c + 2*x) - 2*f(2*y)*f(2*z)*f(z + y)*f(b + 2*y)*f(a +
z + x) + 4*f(
>      2*y)*f(2*z)*f(z + y)*f(a + z + y)*f(b + y + x) - 4*f(2*
y)*f(2*z)*f(z
>      + y)*f(a + y + x)*f(b + z + y) + f(2*y)*f(2*z)*f(z + y)
*f(a + 2*y)*
>      f(c + y + x) + f(2*y)*f(2*z)*f(z + y)*f(a + 2*y)*f(b + z
+ x) + f(2*y

```

```

> )*f(2*z)*f(z + y)*f(a + 2*y)*f(a + z + y) + f(2*y)*f(2*
z)*f(z + x)*f(
> b + 2*y)*f(c + y + x) + f(2*y)*f(2*z)*f(z + x)*f(b + 2*
y)*f(b + z + x
> ) + f(2*y)*f(2*z)*f(z + x)*f(b + 2*y)*f(a + z + y) - f
(2*y)*f(2*z)*f(
> z + x)*f(a + 2*y)*f(c + 2*y) - f(2*y)*f(2*z)^2*f(b + 2*
y)*f(a + y + x
> ) - 1/2*f(2*y)*f(2*z)^2*f(b + 2*x)*f(b + 2*y) + 1/2*f(2*
y)*f(2*z)^2*
> f(a + 2*y)^2 + f(2*y)*f(2*z)*f(y + x)*f(c + 2*y)*f(c + y
+ x) - f(2*y
> )*f(2*z)*f(y + x)*f(c + 2*y)*f(b + z + x) + f(2*y)*f(2*
z)*f(y + x)*f(
> c + 2*y)*f(a + z + y) + 4*f(2*y)*f(2*z)*f(y + x)*f(b + z
+ y)*f(c + y
> + x) - 2*f(2*y)*f(2*z)*f(y + x)*f(b + 2*z)*f(b + y + x)
- 4*f(2*y)*
> f(2*z)*f(y + x)*f(b + y + x)*f(c + z + y) + f(2*y)*f(2*
z)*f(y + x)*f(
> a + 2*z)*f(b + 2*y) - 2*f(2*y)*f(2*z)*f(y + x)*f(a + 2*
y)*f(c + z + y
> ) + 2*f(2*y)*f(y + x)*f(z + y)*f(c + 2*z)*f(b + y + x) -
f(2*y)*f(y
> + x)*f(z + y)*f(a + 2*z)*f(c + 2*y) + 2*f(2*y)*f(y + x)
*f(z + y)*f(a
> + 2*z)*f(b + z + y) - f(2*y)*f(y + x)*f(z + y)*f(a + 2*
y)*f(c + 2*z)
> + f(2*y)*f(y + x)*f(z + x)*f(b + 2*z)*f(c + 2*y) + 2*f
(2*y)*f(y + x)
> *f(z + x)*f(b + 2*z)*f(b + z + y) - f(2*y)*f(y + x)*f(z
+ x)*f(b + 2*
> y)*f(c + 2*z) - 2*f(2*y)*f(y + x)^2*f(c + 2*z)*f(b + z +
y) + f(2*y)*
> f(y + x)^2*f(c + 2*y)*f(c + 2*z) - f(2*y)^2*f(z + y)*f(b
+ 2*x)*f(c
> + 2*z) + f(2*y)^2*f(z + y)*f(a + 2*z)*f(c + y + x) + f
(2*y)^2*f(z +
> y)*f(a + 2*z)*f(b + z + x) - f(2*y)^2*f(z + y)*f(a + 2*
z)*f(a + z + y
> ) - f(2*y)^2*f(z + x)*f(b + 2*z)*f(c + y + x) - f(2*y)
^2*f(z + x)*f(b
> + 2*z)*f(b + z + x) + f(2*y)^2*f(z + x)*f(b + 2*z)*f(a
+ z + y) - 2*
> f(2*y)^2*f(z + x)*f(a + 2*z)*f(b + z + y) + f(2*y)^2*f(z
+ x)*f(a + 2
> *y)*f(c + 2*z) + f(2*y)^2*f(2*z)*f(c + 2*y)*f(a + z + x)
- 1/2*f(2*y)
> ^2*f(2*z)*f(c + 2*x)*f(c + 2*y) - f(2*y)^2*f(2*z)*f(c +
2*x)*f(b + z
> + y) + f(2*y)^2*f(2*z)*f(b + 2*z)*f(a + y + x) + f(2*y)
^2*f(2*z)*f(b
> + 2*x)*f(c + z + y) + 1/2*f(2*y)^2*f(2*z)*f(b + 2*x)*f
(b + 2*z) - 2*
> f(2*y)^2*f(2*z)*f(a + z + y)*f(c + y + x) - 2*f(2*y)^2*f
(2*z)*f(a + z
> + y)*f(b + z + x) + 2*f(2*y)^2*f(2*z)*f(a + z + x)*f(b

```

```

+ z + y) + 2*
>      f(2*y)^2*f(2*z)*f(a + y + x)*f(c + z + y) - f(2*y)^2*f
(2*z)*f(a + 2*y
>      )*f(a + 2*z) - f(2*y)^2*f(y + x)*f(c + 2*z)*f(c + y + x)
+ f(2*y)^2*
>      f(y + x)*f(c + 2*z)*f(b + z + x) + f(2*y)^2*f(y + x)*f(c
+ 2*z)*f(a
>      + z + y) - f(2*y)^2*f(y + x)*f(a + 2*z)*f(b + 2*z) - f
(2*y)^3*f(c +
>      2*z)*f(a + z + x) + 1/2*f(2*y)^3*f(c + 2*x)*f(c + 2*z) +
1/2*f(2*y)^3
>      *f(a + 2*z)^2 + f(2*x)*f(z + y)^2*f(c + 2*y)^2 + 2*f(2*
x)*f(z + y)^2*
>      f(c + 2*y)*f(b + z + y) - 4*f(2*x)*f(z + y)^2*f(b + 2*y)
*f(c + z + y)
>      + 2*f(2*x)*f(2*z)*f(z + y)*f(b + 2*y)*f(b + z + y) - f
(2*x)*f(2*z)^2
>      *f(b + 2*y)^2 - 2*f(2*x)*f(2*y)*f(z + y)*f(b + 2*z)*f(b
+ z + y) - 1/
>      2*f(2*x)*f(2*y)*f(2*z)*f(c + 2*y)^2 - 2*f(2*x)*f(2*y)*f
(2*z)*f(c + 2*
>      y)*f(b + z + y) + 3*f(2*x)*f(2*y)*f(2*z)*f(b + 2*y)*f(c
+ z + y) + 1/
>      2*f(2*x)*f(2*y)*f(2*z)*f(b + 2*y)*f(b + 2*z) + f(2*x)*f
(2*y)^2*f(c +
>      2*z)*f(b + z + y) - 1/2*f(2*x)*f(2*y)^2*f(c + 2*y)*f(c +
2*z) + 1/2*
>      f(2*x)*f(2*y)^2*f(b + 2*z)^2 )
>
>      + f(c + 2*y)^2 + 2*f(c + 2*y)*f(b + z + y) - 4*f(b + 2*y)*
f(c + z + y)
>      + f(2*z)*f(2*b + 2*y) - f(2*y)*f(2*b + 2*z):

> eq[15] :=
> (1/HessUniv) * ( f(2*z)*f(z + y)^2*f(a + 2*x)*f(b + 2*y) + 2*f(2*
z)*
>      f(z + x)*f(z + y)*f(b + 2*y)*f(a + y + x) - f(2*z)*f(z +
x)*f(z + y)*
>      f(b + 2*x)*f(b + 2*y) - 2*f(2*z)*f(z + x)*f(z + y)*f(a +
2*y)*f(b + y
>      + x) - f(2*z)*f(z + x)*f(z + y)*f(a + 2*y)^2 + f(2*z)*f
(z + x)^2*f(a
>      + 2*y)*f(b + 2*y) + 1/2*f(2*z)^2*f(y + x)*f(b + 2*x)*f
(b + 2*y) + f(
>      2*z)^2*f(y + x)*f(a + 2*y)*f(b + y + x) + 1/2*f(2*z)^2*f
(y + x)*f(a
>      + 2*y)^2 - 2*f(2*z)*f(y + x)*f(z + y)*f(b + 2*y)*f(a +
z + x) - 2*f(
>      2*z)*f(y + x)*f(z + x)*f(b + 2*y)*f(a + z + y) + 2*f(y +
x)*f(z + x)*
>      f(z + y)*f(a + 2*z)*f(b + 2*y) - f(2*y)*f(z + y)^2*f(a +
2*z)*f(b + 2
>      *x) + f(2*y)*f(z + x)*f(z + y)*f(b + 2*x)*f(b + 2*z) + f
(2*y)*f(z + x
>      )*f(z + y)*f(a + 2*y)*f(a + 2*z) - f(2*y)*f(z + x)^2*f(a
+ 2*z)*f(b

```

```

> + 2*y) - f(2*y)*f(z + x)^2*f(a + 2*y)*f(b + 2*z) + f(2*
y)*f(2*z)*f(z
> + y)*f(b + 2*x)*f(a + z + y) + 1/2*f(2*y)*f(2*z)*f(z +
y)*f(a + 2*y)
> *f(c + 2*x) - 1/2*f(2*y)*f(2*z)*f(z + y)*f(a + 2*x)*f(c
+ 2*y) - f(2*
> y)*f(2*z)*f(z + y)*f(a + 2*x)*f(b + z + y) - f(2*y)*f(2*
z)*f(z + x)*
> f(c + 2*y)*f(a + y + x) + 1/2*f(2*y)*f(2*z)*f(z + x)*f(b
+ 2*y)*f(c
> + 2*x) + 1/2*f(2*y)*f(2*z)*f(z + x)*f(b + 2*x)*f(c + 2*
y) + 2*f(2*y)
> *f(2*z)*f(z + x)*f(a + z + y)*f(b + y + x) - 2*f(2*y)*f
(2*z)*f(z + x)
> *f(a + y + x)*f(b + z + y) + f(2*y)*f(2*z)*f(z + x)*f(a
+ 2*y)*f(b +
> z + x) + f(2*y)*f(2*z)*f(z + x)*f(a + 2*y)*f(a + z + y)
- 1/2*f(2*y)*
> f(2*z)^2*f(a + 2*y)*f(b + 2*x) - 1/2*f(2*y)*f(2*z)^2*f(a
+ 2*x)*f(b
> + 2*y) + f(2*y)*f(2*z)*f(y + x)*f(c + 2*y)*f(a + z + x)
- 1/2*f(2*y)
> *f(2*z)*f(y + x)*f(c + 2*x)*f(c + 2*y) - 1/2*f(2*y)*f(2*
z)*f(y + x)*
> f(b + 2*x)*f(b + 2*z) - 2*f(2*y)*f(2*z)*f(y + x)*f(a + z
+ y)*f(b + z
> + x) + 2*f(2*y)*f(2*z)*f(y + x)*f(a + z + x)*f(b + z +
y) - f(2*y)*
> f(2*z)*f(y + x)*f(a + 2*z)*f(b + y + x) - f(2*y)*f(2*z)*
f(y + x)*f(a
> + 2*y)*f(a + 2*z) + 2*f(2*y)*f(y + x)*f(z + y)*f(a + 2*
z)*f(b + z +
> x) + 2*f(2*y)*f(y + x)*f(z + x)*f(b + 2*z)*f(a + z + y)
- f(2*y)*f(y
> + x)^2*f(a + 2*z)*f(b + 2*z) + 1/2*f(2*y)^2*f(z + y)*f
(a + 2*z)*f(c
> + 2*x) - 1/2*f(2*y)^2*f(z + y)*f(a + 2*x)*f(c + 2*z) +
f(2*y)^2*f(z
> + x)*f(c + 2*z)*f(a + y + x) - 1/2*f(2*y)^2*f(z + x)*f
(b + 2*z)*f(c
> + 2*x) - 1/2*f(2*y)^2*f(z + x)*f(b + 2*x)*f(c + 2*z) -
f(2*y)^2*f(z
> + x)*f(a + 2*z)*f(b + z + x) - f(2*y)^2*f(z + x)*f(a +
2*z)*f(a + z
> + y) - f(2*y)^2*f(2*z)*f(c + 2*x)*f(a + z + y) + 1/2*f
(2*y)^2*f(2*z)
> *f(a + 2*z)*f(b + 2*x) + f(2*y)^2*f(2*z)*f(a + 2*x)*f(c
+ z + y) + 1/
> 2*f(2*y)^2*f(2*z)*f(a + 2*x)*f(b + 2*z) - f(2*y)^2*f(y +
x)*f(c + 2*z
> )*f(a + z + x) + 1/2*f(2*y)^2*f(y + x)*f(c + 2*x)*f(c +
2*z) + 1/2*f(
> 2*y)^2*f(y + x)*f(a + 2*z)^2 - f(2*x)*f(z + y)^2*f(a +
2*z)*f(b + 2*y
> ) + f(2*x)*f(2*z)*f(z + y)*f(c + 2*y)*f(b + y + x) - 2*f
(2*x)*f(2*z)*
> f(z + y)*f(b + 2*y)*f(c + y + x) + f(2*x)*f(2*z)*f(z +

```

```

y)*f(b + 2*y)*
> f(b + z + x) + f(2*x)*f(2*z)*f(z + y)*f(a + 2*y)*f(c +
2*y) + f(2*x)*
> f(2*z)*f(z + y)*f(a + 2*y)*f(b + z + y) - f(2*x)*f(2*z)
^2*f(a + 2*y)*
> f(b + 2*y) - 1/2*f(2*x)*f(2*z)*f(y + x)*f(c + 2*y)^2 - f
(2*x)*f(2*z)*
> f(y + x)*f(c + 2*y)*f(b + z + y) + 2*f(2*x)*f(2*z)*f(y +
x)*f(b + 2*y
> )*f(c + z + y) - 1/2*f(2*x)*f(2*z)*f(y + x)*f(b + 2*y)*f
(b + 2*z) +
> f(2*x)*f(2*y)*f(z + y)*f(c + 2*z)*f(b + y + x) - f(2*x)*
f(2*y)*f(z +
> y)*f(b + 2*z)*f(b + z + x) - f(2*x)*f(2*y)*f(z + y)*f(b
+ 2*z)*f(a +
> z + y) - 1/2*f(2*x)*f(2*y)*f(z + y)*f(a + 2*z)*f(c + 2*
y) - 1/2*f(2*x
> )*f(2*y)*f(z + y)*f(a + 2*y)*f(c + 2*z) + 1/2*f(2*x)*f
(2*y)*f(z + x)*
> f(b + 2*z)*f(c + 2*y) - 1/2*f(2*x)*f(2*y)*f(z + x)*f(b +
2*y)*f(c + 2
> *z) + f(2*x)*f(2*y)*f(2*z)*f(c + 2*y)*f(c + y + x) - f
(2*x)*f(2*y)*f(
> 2*z)*f(c + 2*y)*f(b + z + x) + 2*f(2*x)*f(2*y)*f(2*z)*f
(b + z + y)*f(
> c + y + x) - 2*f(2*x)*f(2*y)*f(2*z)*f(b + y + x)*f(c + z
+ y) + 3/2*
> f(2*x)*f(2*y)*f(2*z)*f(a + 2*z)*f(b + 2*y) - f(2*x)*f(2*
y)*f(2*z)*f(a
> + 2*y)*f(c + z + y) + 1/2*f(2*x)*f(2*y)*f(2*z)*f(a + 2*
y)*f(b + 2*z)
> - f(2*x)*f(2*y)*f(y + x)*f(c + 2*z)*f(b + z + y) + 1/2*
f(2*x)*f(2*y)
> *f(y + x)*f(c + 2*y)*f(c + 2*z) + 1/2*f(2*x)*f(2*y)*f(y
+ x)*f(b + 2*
> z)^2 - f(2*x)*f(2*y)^2*f(c + 2*z)*f(c + y + x) + f(2*x)*
f(2*y)^2*f(c
> + 2*z)*f(b + z + x) + f(2*x)*f(2*y)^2*f(c + 2*z)*f(a +
z + y) )
> - f(a + 2*z)*f(b + 2*y) + f(2*z)*f(b + a + 2*y) - f(2*y)*f
(b + a + 2*z)
> :
> eq[16] :=
> (1/HessUniv) * ( f(2*z)*f(z + y)^2*f(a + 2*x)*f(a + 2*y) - f(2*z)
*f(z
> + x)*f(z + y)*f(a + 2*y)*f(b + 2*x) - 2*f(2*z)*f(z + x)
*f(z + y)*f(a
> + 2*y)*f(a + y + x) + f(2*z)*f(z + x)*f(z + y)*f(a + 2*
x)*f(b + 2*y)
> + 2*f(2*z)*f(z + x)^2*f(b + 2*y)*f(a + y + x) - f(2*z)*
f(z + x)^2*f(
> b + 2*x)*f(b + 2*y) + 2*f(2*z)^2*f(y + x)*f(a + 2*y)*f(a
+ y + x) +
> f(2*z)*f(y + x)*f(z + y)*f(a + 2*y)*f(c + 2*x) - 2*f(2*
z)*f(y + x)*f(

```

```

>      z + y)*f(a + 2*y)*f(a + z + x) - f(2*z)*f(y + x)*f(z +
> y)*f(a + 2*x)*
>      f(c + 2*y) - 2*f(2*z)*f(y + x)*f(z + x)*f(c + 2*y)*f(a +
> y + x) + f(2
>      *z)*f(y + x)*f(z + x)*f(b + 2*y)*f(c + 2*x) - 2*f(2*z)*f
> (y + x)*f(z
>      + x)*f(b + 2*y)*f(a + z + x) + f(2*z)*f(y + x)*f(z + x)
> *f(b + 2*x)*
>      f(c + 2*y) + 4*f(y + x)*f(z + x)*f(z + y)*f(c + 2*y)*f(a
> + z + x) - 2
>      *f(y + x)*f(z + x)*f(z + y)*f(c + 2*x)*f(c + 2*y) - f(2*
> y)*f(z + y)^2
>      *f(a + 2*x)*f(a + 2*z) - f(2*y)*f(z + x)*f(z + y)*f(a +
> 2*z)*f(b + 2*
>      x) + 2*f(2*y)*f(z + x)*f(z + y)*f(a + 2*z)*f(a + y + x)
> + f(2*y)*f(z
>      + x)*f(z + y)*f(a + 2*x)*f(b + 2*z) - 2*f(2*y)*f(z + x)
> ^2*f(c + 2*y)
>      *f(a + z + x) + f(2*y)*f(z + x)^2*f(c + 2*x)*f(c + 2*y)
> - 2*f(2*y)*f(
>      z + x)^2*f(b + 2*z)*f(a + y + x) + f(2*y)*f(z + x)^2*f(b
> + 2*x)*f(b
>      + 2*z) + 2*f(2*y)*f(2*z)*f(z + x)*f(b + 2*x)*f(a + z +
> y) + 2*f(2*y)
>      *f(2*z)*f(z + x)*f(a + 2*y)*f(a + z + x) - 2*f(2*y)*f(2*
> z)*f(z + x)*
>      f(a + 2*x)*f(b + z + y) - f(2*y)*f(2*z)^2*f(a + 2*x)*f(a
> + 2*y) - 2*
>      f(2*y)*f(2*z)*f(y + x)*f(c + 2*x)*f(a + z + y) - 2*f(2*
> y)*f(2*z)*f(y
>      + x)*f(a + 2*z)*f(a + y + x) + 2*f(2*y)*f(2*z)*f(y + x)
> *f(a + 2*x)*
>      f(c + z + y) + f(2*y)*f(y + x)*f(z + y)*f(a + 2*z)*f(c +
> 2*x) + 2*f(2
>      *y)*f(y + x)*f(z + y)*f(a + 2*z)*f(a + z + x) - f(2*y)*f
> (y + x)*f(z
>      + y)*f(a + 2*x)*f(c + 2*z) + 2*f(2*y)*f(y + x)*f(z + x)
> *f(c + 2*z)*
>      f(a + y + x) - f(2*y)*f(y + x)*f(z + x)*f(b + 2*z)*f(c +
> 2*x) + 2*f(2
>      *y)*f(y + x)*f(z + x)*f(b + 2*z)*f(a + z + x) - f(2*y)*f
> (y + x)*f(z
>      + x)*f(b + 2*x)*f(c + 2*z) - 2*f(2*y)*f(y + x)^2*f(c +
> 2*z)*f(a + z
>      + x) + f(2*y)*f(y + x)^2*f(c + 2*x)*f(c + 2*z) - 2*f(2*
> y)^2*f(z + x)
>      *f(a + 2*z)*f(a + z + x) + f(2*y)^2*f(2*z)*f(a + 2*x)*f
> (a + 2*z) - 2*
>      f(2*x)*f(z + y)^2*f(c + 2*y)*f(a + z + x) + f(2*x)*f(z +
> y)^2*f(c + 2
>      *x)*f(c + 2*y) + 2*f(2*x)*f(2*z)*f(z + y)*f(c + 2*y)*f(a
> + y + x) -
>      f(2*x)*f(2*z)*f(z + y)*f(b + 2*y)*f(c + 2*x) - f(2*x)*f
> (2*z)*f(z + y)
>      *f(a + 2*y)*f(c + y + x) + f(2*x)*f(2*z)*f(z + y)*f(a +
> 2*y)*f(b + z
>      + x) + f(2*x)*f(2*z)*f(z + y)*f(a + 2*y)*f(a + z + y) -

```

```

f(2*x)*f(2*z
> )*f(z + x)*f(b + 2*y)*f(c + y + x) + f(2*x)*f(2*z)*f(z +
x)*f(b + 2*y
> )*f(b + z + x) - f(2*x)*f(2*z)*f(z + x)*f(b + 2*y)*f(a +
z + y) + f(2
> *x)*f(2*z)*f(z + x)*f(a + 2*y)*f(c + 2*y) - f(2*x)*f(2*
z)^2*f(b + 2*y
> )*f(a + y + x) + 1/2*f(2*x)*f(2*z)^2*f(b + 2*x)*f(b + 2*
y) - 1/2*f(2*
> x)*f(2*z)^2*f(a + 2*y)^2 + f(2*x)*f(2*z)*f(y + x)*f(c +
2*y)*f(c + y
> + x) - f(2*x)*f(2*z)*f(y + x)*f(c + 2*y)*f(b + z + x) -
f(2*x)*f(2*z
> )*f(y + x)*f(c + 2*y)*f(a + z + y) + f(2*x)*f(2*z)*f(y +
x)*f(a + 2*z
> )*f(b + 2*y) - 2*f(2*x)*f(2*y)*f(z + y)*f(b + 2*z)*f(a +
z + x) + f(2
> *x)*f(2*y)*f(z + y)*f(b + 2*x)*f(c + 2*z) - f(2*x)*f(2*
y)*f(z + y)*f(
> a + 2*z)*f(c + y + x) + f(2*x)*f(2*y)*f(z + y)*f(a + 2*
z)*f(b + z + x
> ) - f(2*x)*f(2*y)*f(z + y)*f(a + 2*z)*f(a + z + y) + f
(2*x)*f(2*y)*f(
> z + x)*f(b + 2*z)*f(c + y + x) - f(2*x)*f(2*y)*f(z + x)*
f(b + 2*z)*f(
> b + z + x) + f(2*x)*f(2*y)*f(z + x)*f(b + 2*z)*f(a + z +
y) - f(2*x)*
> f(2*y)*f(z + x)*f(a + 2*y)*f(c + 2*z) + f(2*x)*f(2*y)*f
(2*z)*f(c + 2*
> y)*f(a + z + x) - 1/2*f(2*x)*f(2*y)*f(2*z)*f(c + 2*x)*f
(c + 2*y) + f(
> 2*x)*f(2*y)*f(2*z)*f(c + 2*x)*f(b + z + y) + f(2*x)*f(2*
y)*f(2*z)*f(b
> + 2*z)*f(a + y + x) - f(2*x)*f(2*y)*f(2*z)*f(b + 2*x)*f
(c + z + y)
> - 1/2*f(2*x)*f(2*y)*f(2*z)*f(b + 2*x)*f(b + 2*z) + 2*f
(2*x)*f(2*y)*
> f(2*z)*f(a + z + y)*f(c + y + x) - 2*f(2*x)*f(2*y)*f(2*
z)*f(a + z + y
> )*f(b + z + x) + 2*f(2*x)*f(2*y)*f(2*z)*f(a + z + x)*f(b
+ z + y) - 2
> *f(2*x)*f(2*y)*f(2*z)*f(a + y + x)*f(c + z + y) - f(2*x)
*f(2*y)*f(y
> + x)*f(c + 2*z)*f(c + y + x) + f(2*x)*f(2*y)*f(y + x)*f
(c + 2*z)*f(b
> + z + x) + f(2*x)*f(2*y)*f(y + x)*f(c + 2*z)*f(a + z +
y) - f(2*x)*
> f(2*y)*f(y + x)*f(a + 2*z)*f(b + 2*z) + f(2*x)*f(2*y)^2*
f(c + 2*z)*f(
> a + z + x) - 1/2*f(2*x)*f(2*y)^2*f(c + 2*x)*f(c + 2*z) +
1/2*f(2*x)*
> f(2*y)^2*f(a + 2*z)^2 - 1/2*f(2*x)^2*f(2*z)*f(c + 2*y)^2
+ f(2*x)^2*
> f(2*z)*f(b + 2*y)*f(c + z + y) - 1/2*f(2*x)^2*f(2*z)*f(b
+ 2*y)*f(b
> + 2*z) - f(2*x)^2*f(2*y)*f(c + 2*z)*f(b + z + y) + 1/2*
f(2*x)^2*f(2*

```

```

> y)*f(c + 2*y)*f(c + 2*z) + 1/2*f(2*x)^2*f(2*y)*f(b + 2*
z)^2 )
> - 2*f(c + 2*y)*f(a + z + x) + f(c + 2*x)*f(c + 2*y) + f(2*
z)*f(2*a + 2*
> y) - f(2*y)*f(2*a + 2*z):
> eq[17] :=
> (1/HessUniv) * ( 4*f(z + y)^3*f(a + 2*y)*f(c + z + x) - 2*f(z +
y)^3*
> f(a + 2*y)*f(a + 2*z) - 4*f(z + x)*f(z + y)^2*f(b + 2*y)
*f(c + z + x)
> + 2*f(z + x)*f(z + y)^2*f(a + 2*z)*f(b + 2*y) - 4*f(z +
x)*f(z + y)^
> 2*f(a + 2*y)*f(c + z + y) + 2*f(z + x)*f(z + y)^2*f(a +
2*y)*f(b + 2*
> z) + 4*f(z + x)^2*f(z + y)*f(b + 2*y)*f(c + z + y) - 2*f
(z + x)^2*f(z
> + y)*f(b + 2*y)*f(b + 2*z) + 2*f(2*z)*f(z + y)^2*f(b +
2*y)*f(c + 2*
> x) - 2*f(2*z)*f(z + y)^2*f(a + 2*y)*f(c + y + x) - 2*f
(2*z)*f(z + y)^
> 2*f(a + 2*y)*f(b + z + x) + 2*f(2*z)*f(z + y)^2*f(a + 2*
y)*f(a + z +
> y) - 2*f(2*z)*f(z + x)*f(z + y)*f(b + 2*y)*f(c + y + x)
+ 2*f(2*z)*f(
> z + x)*f(z + y)*f(b + 2*y)*f(b + z + x) - 2*f(2*z)*f(z +
x)*f(z + y)*
> f(b + 2*y)*f(a + z + y) + 2*f(2*z)*f(z + x)*f(z + y)*f(a
+ 2*y)*f(c
> + 2*y) + 2*f(2*z)^2*f(z + y)*f(b + 2*y)*f(a + y + x) -
f(2*z)^2*f(z
> + y)*f(b + 2*x)*f(b + 2*y) - f(2*z)^2*f(z + y)*f(a + 2*
y)^2 + 2*f(2*
> z)*f(y + x)*f(z + y)*f(c + 2*y)*f(c + y + x) + 2*f(2*z)*
f(y + x)*f(z
> + y)*f(c + 2*y)*f(b + z + x) - 2*f(2*z)*f(y + x)*f(z +
y)*f(c + 2*y)
> *f(a + z + y) - 2*f(2*z)*f(y + x)*f(z + y)*f(a + 2*z)*f
(b + 2*y) + 4*
> f(2*z)*f(y + x)*f(z + y)*f(a + 2*y)*f(c + z + y) - 4*f(y
+ x)*f(z + y
> )^2*f(c + 2*y)*f(c + z + x) + 2*f(y + x)*f(z + y)^2*f(a
+ 2*z)*f(c +
> 2*y) - 2*f(y + x)*f(z + y)^2*f(a + 2*y)*f(c + 2*z) - 4*f
(y + x)*f(z
> + x)*f(z + y)*f(c + 2*y)*f(c + z + y) - 2*f(y + x)*f(z
+ x)*f(z + y)
> *f(b + 2*z)*f(c + 2*y) + 2*f(y + x)*f(z + x)*f(z + y)*f
(b + 2*y)*f(c
> + 2*z) + 2*f(y + x)^2*f(z + y)*f(c + 2*y)*f(c + 2*z) -
4*f(2*y)*f(z
> + y)^2*f(a + z + y)*f(c + z + x) + 2*f(2*y)*f(z + y)^2*
f(a + 2*z)*f(
> a + z + y) + 4*f(2*y)*f(z + x)*f(z + y)*f(c + 2*y)*f(c +
z + x) + 4*
> f(2*y)*f(z + x)*f(z + y)*f(b + z + y)*f(c + z + x) - 2*f

```



```

(2*y)*f(z + x
> )*f(z + y)*f(b + 2*z)*f(a + z + y) + 4*f(2*y)*f(z + x)*f
(z + y)*f(a
> + z + y)*f(c + z + y) - 2*f(2*y)*f(z + x)*f(z + y)*f(a
+ 2*z)*f(c +
> 2*y) - 2*f(2*y)*f(z + x)*f(z + y)*f(a + 2*z)*f(b + z +
y) + 2*f(2*y)*
> f(z + x)*f(z + y)*f(a + 2*y)*f(c + 2*z) - 4*f(2*y)*f(z +
x)^2*f(b + z
> + y)*f(c + z + y) + 2*f(2*y)*f(z + x)^2*f(b + 2*z)*f(c
+ 2*y) + 2*f(
> 2*y)*f(z + x)^2*f(b + 2*z)*f(b + z + y) - 2*f(2*y)*f(z +
x)^2*f(b + 2
> *y)*f(c + 2*z) - f(2*y)*f(2*z)*f(z + y)*f(c + 2*x)*f(c +
2*y) - 2*f(2
> *y)*f(2*z)*f(z + y)*f(c + 2*x)*f(b + z + y) + 2*f(2*y)*f
(2*z)*f(z + y
> )*f(a + z + y)*f(c + y + x) + 2*f(2*y)*f(2*z)*f(z + y)*f
(a + z + y)*
> f(b + z + x) - 2*f(2*y)*f(2*z)*f(z + y)*f(a + z + y)^2 -
2*f(2*y)*f(2
> *z)*f(z + y)*f(a + 2*y)*f(c + z + x) + f(2*y)*f(2*z)*f(z
+ y)*f(a + 2
> *y)*f(a + 2*z) - 2*f(2*y)*f(2*z)*f(z + x)*f(c + 2*y)*f(b
+ z + x) + 2
> *f(2*y)*f(2*z)*f(z + x)*f(b + z + y)*f(c + y + x) - 2*f
(2*y)*f(2*z)*
> f(z + x)*f(b + z + x)*f(b + z + y) + 2*f(2*y)*f(2*z)*f(z
+ x)*f(b + 2
> *y)*f(c + z + x) + 2*f(2*y)*f(2*z)*f(z + x)*f(a + z + y)
*f(b + z + y)
> + f(2*y)*f(2*z)*f(z + x)*f(a + 2*z)*f(b + 2*y) - 2*f(2*
y)*f(2*z)*f(z
> + x)*f(a + 2*y)*f(c + z + y) - f(2*y)*f(2*z)*f(z + x)*f
(a + 2*y)*f(b
> + 2*z) - f(2*y)*f(2*z)^2*f(c + 2*y)*f(a + y + x) - 1/2*
f(2*y)*f(2*z)
> ^2*f(b + 2*y)*f(c + 2*x) - f(2*y)*f(2*z)^2*f(b + 2*y)*f
(a + z + x) +
> 1/2*f(2*y)*f(2*z)^2*f(b + 2*x)*f(c + 2*y) + f(2*y)*f(2*
z)^2*f(b + 2*x
> )*f(b + z + y) - 2*f(2*y)*f(2*z)^2*f(a + y + x)*f(b + z
+ y) + f(2*y)
> *f(2*z)^2*f(a + 2*y)*f(c + y + x) + f(2*y)*f(2*z)^2*f(a
+ 2*y)*f(b +
> z + x) + f(2*y)*f(2*z)^2*f(a + 2*y)*f(a + z + y) - 2*f
(2*y)*f(2*z)*f(
> y + x)*f(c + y + x)*f(c + z + y) - 2*f(2*y)*f(2*z)*f(y +
x)*f(b + z
> + x)*f(c + z + y) - 2*f(2*y)*f(2*z)*f(y + x)*f(a + z +
y)*f(c + z +
> y) + f(2*y)*f(2*z)*f(y + x)*f(a + 2*z)*f(c + 2*y) + 2*f
(2*y)*f(2*z)*
> f(y + x)*f(a + 2*z)*f(b + z + y) - f(2*y)*f(2*z)*f(y +
x)*f(a + 2*y)*
> f(c + 2*z) + 4*f(2*y)*f(y + x)*f(z + y)*f(c + z + x)*f(c
+ z + y) + 2

```

```

>      *f(2*y)*f(y + x)*f(z + y)*f(c + 2*z)*f(a + z + y) - 2*f
> (2*y)*f(y + x)
>      *f(z + y)*f(a + 2*z)*f(c + z + y) + 4*f(2*y)*f(y + x)*f
> (z + x)*f(c +
>      z + y)^2 - 2*f(2*y)*f(y + x)*f(z + x)*f(c + 2*z)*f(b + z
> + y) + 2*f(2
>      *y)*f(y + x)*f(z + x)*f(b + 2*z)*f(c + z + y) - 2*f(2*y)
> *f(y + x)^2*
>      f(c + 2*z)*f(c + z + y) - 2*f(2*y)^2*f(z + y)*f(c + 2*z)
> *f(a + z + x)
>      + 2*f(2*y)^2*f(z + y)*f(a + 2*z)*f(c + z + x) - 4*f(2*
> y)^2*f(z + x)*
>      f(c + z + x)*f(c + z + y) + 2*f(2*y)^2*f(z + x)*f(c + 2*
> z)*f(b + z +
>      x) - 2*f(2*y)^2*f(z + x)*f(b + 2*z)*f(c + z + x) + f(2*
> y)^2*f(2*z)*f(
>      c + 2*z)*f(a + y + x) + f(2*y)^2*f(2*z)*f(c + 2*x)*f(c +
> z + y) + 1/2
>      *f(2*y)^2*f(2*z)*f(b + 2*z)*f(c + 2*x) + f(2*y)^2*f(2*z)
> *f(b + 2*z)*
>      f(a + z + x) - 1/2*f(2*y)^2*f(2*z)*f(b + 2*x)*f(c + 2*z)
> + 2*f(2*y)^2
>      *f(2*z)*f(a + z + x)*f(c + z + y) - f(2*y)^2*f(2*z)*f(a
> + 2*z)*f(c +
>      y + x) - f(2*y)^2*f(2*z)*f(a + 2*z)*f(b + z + x) - f(2*
> y)^2*f(2*z)*f(
>      a + 2*z)*f(a + z + y) + 4*f(2*x)*f(z + y)^2*f(c + 2*y)*f
> (c + z + y)
>      - f(2*x)*f(2*z)*f(z + y)*f(c + 2*y)^2 - 2*f(2*x)*f(2*z)
> *f(z + y)*f(b
>      + 2*y)*f(c + z + y) + f(2*x)*f(2*z)*f(z + y)*f(b + 2*y)
> *f(b + 2*z)
>      - 4*f(2*x)*f(2*y)*f(z + y)*f(c + z + y)^2 - 2*f(2*x)*f
> (2*y)*f(z + y)
>      *f(c + 2*y)*f(c + 2*z) + f(2*x)*f(2*y)*f(2*z)*f(c + 2*y)
> *f(c + z + y)
>      + 2*f(2*x)*f(2*y)*f(2*z)*f(b + z + y)*f(c + z + y) -
> 1/2*f(2*x)*f(2*
>      y)*f(2*z)*f(b + 2*z)*f(c + 2*y) - f(2*x)*f(2*y)*f(2*z)*f
> (b + 2*z)*f(b
>      + z + y) + 1/2*f(2*x)*f(2*y)*f(2*z)*f(b + 2*y)*f(c + 2*
> z) + 2*f(2*x)
>      *f(2*y)^2*f(c + 2*z)*f(c + z + y) )
>
>      + 2*f(z + y)*f(2*c + 2*y) - 2*f(2*y)*f(2*c + z + y):
>
> eq[18] :=
> (1/HessUniv) * ( 4*f(z + x)*f(z + y)^2*f(a + 2*y)*f(c + z + x) -
> 2*f(
>      z + x)*f(z + y)^2*f(a + 2*y)*f(a + 2*z) - 4*f(z + x)^2*f
> (z + y)*f(b
>      + 2*y)*f(c + z + x) + 2*f(z + x)^2*f(z + y)*f(a + 2*z)*
> f(b + 2*y) -
>      4*f(z + x)^2*f(z + y)*f(a + 2*y)*f(c + z + y) + 2*f(z +
> x)^2*f(z + y)
>      *f(a + 2*y)*f(b + 2*z) + 4*f(z + x)^3*f(b + 2*y)*f(c + z
> + y) - 2*f(z

```

```

> + x)^3*f(b + 2*y)*f(b + 2*z) + 2*f(2*z)*f(z + x)*f(z +
> y)*f(b + 2*y)
> *f(c + 2*x) - 2*f(2*z)*f(z + x)*f(z + y)*f(a + 2*y)*f(c
> + y + x) - 2*
> f(2*z)*f(z + x)*f(z + y)*f(a + 2*y)*f(b + z + x) + 2*f
> (2*z)*f(z + x)*
> f(z + y)*f(a + 2*y)*f(a + z + y) - 2*f(2*z)*f(z + x)^2*f
> (b + 2*y)*f(c
> + y + x) + 2*f(2*z)*f(z + x)^2*f(b + 2*y)*f(b + z + x)
> - 2*f(2*z)*f(
> z + x)^2*f(b + 2*y)*f(a + z + y) + 2*f(2*z)*f(z + x)^2*f
> (a + 2*y)*f(c
> + 2*y) + 2*f(2*z)^2*f(z + x)*f(b + 2*y)*f(a + y + x) -
> f(2*z)^2*f(z
> + x)*f(b + 2*x)*f(b + 2*y) - f(2*z)^2*f(z + x)*f(a + 2*
> y)^2 + 2*f(2*
> z)*f(y + x)*f(z + x)*f(c + 2*y)*f(c + y + x) + 2*f(2*z)*
> f(y + x)*f(z
> + x)*f(c + 2*y)*f(b + z + x) - 2*f(2*z)*f(y + x)*f(z +
> x)*f(c + 2*y)
> *f(a + z + y) - 2*f(2*z)*f(y + x)*f(z + x)*f(a + 2*z)*f
> (b + 2*y) + 4*
> f(2*z)*f(y + x)*f(z + x)*f(a + 2*y)*f(c + z + y) - 4*f(y
> + x)*f(z + x
> )*f(z + y)*f(c + 2*y)*f(c + z + x) + 2*f(y + x)*f(z + x)
> *f(z + y)*f(a
> + 2*z)*f(c + 2*y) - 2*f(y + x)*f(z + x)*f(z + y)*f(a +
> 2*y)*f(c + 2*
> z) - 4*f(y + x)*f(z + x)^2*f(c + 2*y)*f(c + z + y) - 2*f
> (y + x)*f(z
> + x)^2*f(b + 2*z)*f(c + 2*y) + 2*f(y + x)*f(z + x)^2*f
> (b + 2*y)*f(c
> + 2*z) + 2*f(y + x)^2*f(z + x)*f(c + 2*y)*f(c + 2*z) -
> 4*f(2*y)*f(z
> + y)^2*f(a + z + x)*f(c + z + x) + 2*f(2*y)*f(z + y)^2*
> f(a + 2*z)*f(
> c + 2*x) + 2*f(2*y)*f(z + y)^2*f(a + 2*z)*f(a + z + x) -
> 2*f(2*y)*f(z
> + y)^2*f(a + 2*x)*f(c + 2*z) + 4*f(2*y)*f(z + x)*f(z +
> y)*f(c + 2*z)
> *f(a + y + x) + 4*f(2*y)*f(z + x)*f(z + y)*f(b + z + x)*
> f(c + z + x)
> - 2*f(2*y)*f(z + x)*f(z + y)*f(b + 2*z)*f(c + 2*x) - 2*
> f(2*y)*f(z +
> x)*f(z + y)*f(b + 2*z)*f(a + z + x) + 2*f(2*y)*f(z + x)*
> f(z + y)*f(b
> + 2*x)*f(c + 2*z) + 4*f(2*y)*f(z + x)*f(z + y)*f(a + z
> + x)*f(c + z
> + y) - 4*f(2*y)*f(z + x)*f(z + y)*f(a + 2*z)*f(c + y +
> x) - 2*f(2*y)
> *f(z + x)*f(z + y)*f(a + 2*z)*f(b + z + x) - 4*f(2*y)*f
> (z + x)^2*f(c
> + 2*z)*f(b + y + x) + 4*f(2*y)*f(z + x)^2*f(c + 2*y)*f
> (c + z + x) -
> 4*f(2*y)*f(z + x)^2*f(b + z + x)*f(c + z + y) + 4*f(2*y)
> *f(z + x)^2*
> f(b + 2*z)*f(c + y + x) + 2*f(2*y)*f(z + x)^2*f(b + 2*z)

```

```

*f(b + z + x)
> - 2*f(2*y)*f(2*z)*f(z + y)*f(c + 2*x)*f(a + z + y) - 2*
f(2*y)*f(2*z)
> *f(z + y)*f(b + 2*x)*f(c + z + x) + 2*f(2*y)*f(2*z)*f(z
+ y)*f(a + z
> + x)*f(c + y + x) + 2*f(2*y)*f(2*z)*f(z + y)*f(a + z +
x)*f(b + z +
> x) - 2*f(2*y)*f(2*z)*f(z + y)*f(a + z + x)*f(a + z + y)
- f(2*y)*f(2*
> z)*f(z + y)*f(a + 2*z)*f(b + 2*x) + 2*f(2*y)*f(2*z)*f(z
+ y)*f(a + 2*
> x)*f(c + z + y) + f(2*y)*f(2*z)*f(z + y)*f(a + 2*x)*f(b
+ 2*z) - 2*f(
> 2*y)*f(2*z)*f(z + x)*f(c + 2*y)*f(a + z + x) - f(2*y)*f
(2*z)*f(z + x)
> *f(c + 2*x)*f(c + 2*y) - 2*f(2*y)*f(2*z)*f(z + x)*f(b +
z + x)*f(c +
> y + x) - 2*f(2*y)*f(2*z)*f(z + x)*f(b + z + x)^2 - 2*f
(2*y)*f(2*z)*f(
> z + x)*f(b + 2*z)*f(a + y + x) + 4*f(2*y)*f(2*z)*f(z +
x)*f(b + y + x
> )*f(c + z + x) + 4*f(2*y)*f(2*z)*f(z + x)*f(a + z + y)*f
(c + y + x)
> + 2*f(2*y)*f(2*z)*f(z + x)*f(a + z + y)*f(b + z + x) +
2*f(2*y)*f(2*
> z)*f(z + x)*f(a + 2*z)*f(b + y + x) - 4*f(2*y)*f(2*z)*f
(z + x)*f(a +
> y + x)*f(c + z + y) - 2*f(2*y)*f(2*z)*f(z + x)*f(a + 2*
y)*f(c + z + x
> ) + f(2*y)*f(2*z)*f(z + x)*f(a + 2*y)*f(a + 2*z) - f(2*
y)*f(2*z)^2*f(
> c + 2*x)*f(b + y + x) + f(2*y)*f(2*z)^2*f(b + 2*x)*f(c +
y + x) + f(2
> *y)*f(2*z)^2*f(b + 2*x)*f(b + z + x) + f(2*y)*f(2*z)^2*f
(b + 2*x)*f(a
> + z + y) - 2*f(2*y)*f(2*z)^2*f(a + z + x)*f(b + y + x)
+ 1/2*f(2*y)*
> f(2*z)^2*f(a + 2*y)*f(c + 2*x) + f(2*y)*f(2*z)^2*f(a +
2*y)*f(a + z
> + x) - 1/2*f(2*y)*f(2*z)^2*f(a + 2*x)*f(c + 2*y) - f(2*
y)*f(2*z)^2*
> f(a + 2*x)*f(b + z + y) - 2*f(2*y)*f(2*z)*f(y + x)*f(c +
y + x)*f(c
> + z + x) - 2*f(2*y)*f(2*z)*f(y + x)*f(b + z + x)*f(c +
z + x) + f(2*
> y)*f(2*z)*f(y + x)*f(b + 2*z)*f(c + 2*x) + 2*f(2*y)*f(2*
z)*f(y + x)*
> f(b + 2*z)*f(a + z + x) - f(2*y)*f(2*z)*f(y + x)*f(b +
2*x)*f(c + 2*z
> ) - 2*f(2*y)*f(2*z)*f(y + x)*f(a + z + y)*f(c + z + x) +
4*f(2*y)*f(y
> + x)*f(z + y)*f(c + z + x)^2 - 2*f(2*y)*f(y + x)*f(z +
y)*f(c + 2*z)
> *f(a + z + x) + 2*f(2*y)*f(y + x)*f(z + y)*f(a + 2*z)*f
(c + z + x) +
> 4*f(2*y)*f(y + x)*f(z + x)*f(c + z + x)*f(c + z + y) +
2*f(2*y)*f(y

```

```

> + x)*f(z + x)*f(c + 2*z)*f(b + z + x) - 2*f(2*y)*f(y +
> x)*f(z + x)*
> f(b + 2*z)*f(c + z + x) - 2*f(2*y)*f(y + x)^2*f(c + 2*z)
> *f(c + z + x)
> - 4*f(2*y)^2*f(z + x)*f(c + z + x)^2 + f(2*y)^2*f(2*z)*
> f(c + 2*x)*f(
> c + z + x) + 2*f(2*y)^2*f(2*z)*f(a + z + x)*f(c + z + x)
> - 1/2*f(2*y)
> ^2*f(2*z)*f(a + 2*z)*f(c + 2*x) - f(2*y)^2*f(2*z)*f(a +
> 2*z)*f(a + z
> + x) + 1/2*f(2*y)^2*f(2*z)*f(a + 2*x)*f(c + 2*z) + 4*f
> (2*x)*f(z + x)
> *f(z + y)*f(c + 2*y)*f(c + z + y) - f(2*x)*f(2*z)*f(z +
> x)*f(c + 2*y)
> ^2 - 2*f(2*x)*f(2*z)*f(z + x)*f(b + 2*y)*f(c + z + y) +
> f(2*x)*f(2*z)
> *f(z + x)*f(b + 2*y)*f(b + 2*z) - 4*f(2*x)*f(2*y)*f(z +
> y)*f(c + z +
> x)*f(c + z + y) + 2*f(2*x)*f(2*y)*f(z + y)*f(c + 2*z)*f
> (a + z + y) -
> 2*f(2*x)*f(2*y)*f(z + y)*f(a + 2*z)*f(c + z + y) - 2*f
> (2*x)*f(2*y)*f(
> z + x)*f(c + 2*z)*f(b + z + y) - 2*f(2*x)*f(2*y)*f(z +
> x)*f(c + 2*y)*
> f(c + 2*z) + 2*f(2*x)*f(2*y)*f(z + x)*f(b + 2*z)*f(c + z
> + y) + f(2*x)
> )*f(2*y)*f(2*z)*f(c + 2*z)*f(b + y + x) + f(2*x)*f(2*y)*
> f(2*z)*f(c +
> 2*y)*f(c + z + x) + 2*f(2*x)*f(2*y)*f(2*z)*f(b + z + y)*
> f(c + z + x)
> - f(2*x)*f(2*y)*f(2*z)*f(b + 2*z)*f(c + y + x) - f(2*x)
> *f(2*y)*f(2*z)
> )*f(b + 2*z)*f(b + z + x) - f(2*x)*f(2*y)*f(2*z)*f(b +
> 2*z)*f(a + z
> + y) + 1/2*f(2*x)*f(2*y)*f(2*z)*f(a + 2*z)*f(c + 2*y) +
> f(2*x)*f(2*y)
> )*f(2*z)*f(a + 2*z)*f(b + z + y) - 1/2*f(2*x)*f(2*y)*f
> (2*z)*f(a + 2*y
> )*f(c + 2*z) + 2*f(2*x)*f(2*y)^2*f(c + 2*z)*f(c + z + x)
> )
>
> + 2*f(z + x)*f(2*c + 2*y) - 2*f(2*y)*f(2*c + z + x):
>
> eq[19] :=
> (1/HessUniv) * ( 8*f(z + x)*f(z + y)^2*f(b + 2*y)*f(a + y + x) -
> 4*f(
> z + x)*f(z + y)^2*f(a + 2*y)*f(b + y + x) - 2*f(z + x)*f
> (z + y)^2*f(a
> + 2*y)^2 - 4*f(z + x)^2*f(z + y)*f(b + 2*y)*f(b + y +
> x) + 2*f(z + x
> )^3*f(b + 2*y)^2 + 4*f(2*z)*f(y + x)*f(z + x)*f(b + 2*y)
> *f(b + y + x)
> + 4*f(y + x)*f(z + x)*f(z + y)*f(c + 2*y)*f(b + y + x)
> - 8*f(y + x)*
> f(z + x)*f(z + y)*f(b + 2*y)*f(c + y + x) - 8*f(y + x)*f
> (z + x)*f(z

```

```

> + y)*f(b + 2*y)*f(a + z + y) + 4*f(y + x)*f(z + x)*f(z
> + y)*f(a + 2*
> y)*f(c + 2*y) + 4*f(y + x)*f(z + x)*f(z + y)*f(a + 2*y)*
f(b + z + y)
> - 4*f(y + x)*f(z + x)^2*f(b + 2*y)*f(b + z + y) - 2*f(y
+ x)^2*f(z
> + x)*f(c + 2*y)^2 - 4*f(y + x)^2*f(z + x)*f(c + 2*y)*f
(b + z + y) +
> 8*f(y + x)^2*f(z + x)*f(b + 2*y)*f(c + z + y) - 4*f(2*y)
*f(z + y)^2*
> f(a + z + x)*f(b + y + x) + 2*f(2*y)*f(z + y)^2*f(a + 2*
y)*f(a + z +
> x) - 4*f(2*y)*f(z + x)*f(z + y)*f(c + 2*y)*f(a + y + x)
+ 4*f(2*y)*f(
> z + x)*f(z + y)*f(b + y + x)*f(b + z + x) + 2*f(2*y)*f(z
+ x)*f(z + y
> )*f(b + 2*y)*f(c + 2*x) - 2*f(2*y)*f(z + x)*f(z + y)*f(b
+ 2*y)*f(a
> + z + x) + 8*f(2*y)*f(z + x)*f(z + y)*f(a + z + y)*f(b
+ y + x) - 8*
> f(2*y)*f(z + x)*f(z + y)*f(a + y + x)*f(b + z + y) + 2*f
(2*y)*f(z + x
> )*f(z + y)*f(a + 2*y)*f(c + y + x) + 2*f(2*y)*f(z + x)*f
(z + y)*f(a
> + 2*y)*f(a + z + y) + 2*f(2*y)*f(z + x)^2*f(b + 2*y)*f
(c + y + x) +
> 2*f(2*y)*f(z + x)^2*f(b + 2*y)*f(a + z + y) - 2*f(2*y)*f
(z + x)^2*f(a
> + 2*y)*f(c + 2*y) + f(2*y)*f(2*z)*f(z + y)*f(a + 2*y)*f
(b + 2*x) -
> f(2*y)*f(2*z)*f(z + y)*f(a + 2*x)*f(b + 2*y) - 2*f(2*y)*
f(2*z)*f(z +
> x)*f(b + 2*y)*f(a + y + x) - f(2*y)*f(2*z)*f(z + x)*f(b
+ 2*x)*f(b +
> 2*y) + f(2*y)*f(2*z)*f(z + x)*f(a + 2*y)^2 - 4*f(2*y)*f
(2*z)*f(y + x)
> *f(b + y + x)*f(b + z + x) + f(2*y)*f(2*z)*f(y + x)*f(b
+ 2*y)*f(c +
> 2*x) - f(2*y)*f(2*z)*f(y + x)*f(b + 2*x)*f(c + 2*y) - 2*
f(2*y)*f(y +
> x)*f(z + y)*f(c + 2*y)*f(a + z + x) + 4*f(2*y)*f(y + x)*
f(z + y)*f(b
> + y + x)*f(c + z + x) + 4*f(2*y)*f(y + x)*f(z + y)*f(a
+ z + x)*f(b
> + z + y) - 2*f(2*y)*f(y + x)*f(z + y)*f(a + 2*y)*f(c +
z + x) + 2*f(
> 2*y)*f(y + x)*f(z + x)*f(c + 2*y)*f(c + y + x) + 2*f(2*
y)*f(y + x)*f(
> z + x)*f(c + 2*y)*f(a + z + y) + 8*f(2*y)*f(y + x)*f(z +
x)*f(b + z
> + y)*f(c + y + x) + 4*f(2*y)*f(y + x)*f(z + x)*f(b + z
+ x)*f(b + z
> + y) - 8*f(2*y)*f(y + x)*f(z + x)*f(b + y + x)*f(c + z
+ y) - 2*f(2*
> y)*f(y + x)*f(z + x)*f(b + 2*y)*f(c + z + x) + 2*f(2*y)*
f(y + x)*f(z
> + x)*f(a + 2*z)*f(b + 2*y) - 4*f(2*y)*f(y + x)*f(z + x)

```

```

*f(a + 2*y)*
> f(c + z + y) + 2*f(2*y)*f(y + x)^2*f(c + 2*y)*f(c + z +
> x) - 4*f(2*y)
> *f(y + x)^2*f(b + z + y)*f(c + z + x) - 2*f(2*y)^2*f(z +
> y)*f(b + 2*x
> )*f(c + z + x) + 2*f(2*y)^2*f(z + y)*f(a + z + x)*f(c +
> y + x) + 2*f(
> 2*y)^2*f(z + y)*f(a + z + x)*f(b + z + x) - 2*f(2*y)^2*f
> (z + y)*f(a
> + z + x)*f(a + z + y) + 2*f(2*y)^2*f(z + x)*f(c + 2*y)*
> f(a + z + x)
> - f(2*y)^2*f(z + x)*f(c + 2*x)*f(c + 2*y) - 2*f(2*y)^2*
> f(z + x)*f(c
> + 2*x)*f(b + z + y) - 2*f(2*y)^2*f(z + x)*f(b + z + x)*
> f(c + y + x)
> - 2*f(2*y)^2*f(z + x)*f(b + z + x)^2 + 2*f(2*y)^2*f(z +
> x)*f(b + 2*z
> )*f(a + y + x) + 2*f(2*y)^2*f(z + x)*f(b + 2*x)*f(c + z
> + y) - 4*f(2*
> y)^2*f(z + x)*f(a + z + y)*f(c + y + x) - 2*f(2*y)^2*f(z
> + x)*f(a + z
> + y)*f(b + z + x) - 2*f(2*y)^2*f(z + x)*f(a + 2*z)*f(b
> + y + x) + 4*
> f(2*y)^2*f(z + x)*f(a + y + x)*f(c + z + y) + 2*f(2*y)
> ^2*f(z + x)*f(a
> + 2*y)*f(c + z + x) - f(2*y)^2*f(z + x)*f(a + 2*y)*f(a
> + 2*z) - f(2*
> y)^2*f(2*z)*f(c + 2*x)*f(b + y + x) + f(2*y)^2*f(2*z)*f
> (b + 2*x)*f(c
> + y + x) + f(2*y)^2*f(2*z)*f(b + 2*x)*f(b + z + x) - f
> (2*y)^2*f(2*z)
> *f(b + 2*x)*f(a + z + y) + 2*f(2*y)^2*f(2*z)*f(a + z +
> x)*f(b + y + x
> ) - 1/2*f(2*y)^2*f(2*z)*f(a + 2*y)*f(c + 2*x) - f(2*y)
> ^2*f(2*z)*f(a
> + 2*y)*f(a + z + x) + 1/2*f(2*y)^2*f(2*z)*f(a + 2*x)*f
> (c + 2*y) + f(
> 2*y)^2*f(2*z)*f(a + 2*x)*f(b + z + y) - 2*f(2*y)^2*f(y +
> x)*f(c + y
> + x)*f(c + z + x) + 2*f(2*y)^2*f(y + x)*f(b + z + x)*f
> (c + z + x) -
> 2*f(2*y)^2*f(y + x)*f(b + 2*z)*f(a + z + x) + 2*f(2*y)
> ^2*f(y + x)*f(a
> + z + y)*f(c + z + x) + f(2*y)^3*f(c + 2*x)*f(c + z +
> x) - 2*f(2*y)^
> 3*f(a + z + x)*f(c + z + x) + 1/2*f(2*y)^3*f(a + 2*z)*f
> (c + 2*x) + f(
> 2*y)^3*f(a + 2*z)*f(a + z + x) - 1/2*f(2*y)^3*f(a + 2*x)
> *f(c + 2*z)
> + 4*f(2*x)*f(z + x)*f(z + y)*f(b + 2*y)*f(b + z + y) -
> 2*f(2*x)*f(2*
> z)*f(z + x)*f(b + 2*y)^2 - 4*f(2*x)*f(2*y)*f(z + y)*f(b
> + z + x)*f(b
> + z + y) + f(2*x)*f(2*y)*f(z + y)*f(a + 2*z)*f(b + 2*y)
> - f(2*x)*f(2
> y)*f(z + y)*f(a + 2*y)*f(b + 2*z) + f(2*x)*f(2*y)*f(z +
> x)*f(c + 2*y

```

```

> )^2 - 2*f(2*x)*f(2*y)*f(z + x)*f(b + 2*y)*f(c + z + y) -
f(2*x)*f(2*y
> )*f(z + x)*f(b + 2*y)*f(b + 2*z) + 2*f(2*x)*f(2*y)*f(2*
z)*f(b + 2*y)*
> f(b + z + x) + f(2*x)*f(2*y)*f(y + x)*f(b + 2*z)*f(c +
2*y) - f(2*x)*
> f(2*y)*f(y + x)*f(b + 2*y)*f(c + 2*z) + f(2*x)*f(2*y)^2*
f(c + 2*z)*f(
> b + y + x) - f(2*x)*f(2*y)^2*f(c + 2*y)*f(c + z + x) +
2*f(2*x)*f(2*y
> )^2*f(b + z + y)*f(c + z + x) - f(2*x)*f(2*y)^2*f(b + 2*
z)*f(c + y +
> x) + f(2*x)*f(2*y)^2*f(b + 2*z)*f(b + z + x) + f(2*x)*f
(2*y)^2*f(b +
> 2*z)*f(a + z + y) - 1/2*f(2*x)*f(2*y)^2*f(a + 2*z)*f(c +
2*y) - f(2*x
> )*f(2*y)^2*f(a + 2*z)*f(b + z + y) + 1/2*f(2*x)*f(2*y)
^2*f(a + 2*y)*
> f(c + 2*z) )

> + 2*f(z + x)*f(2*b + 2*y) - 2*f(2*y)*f(2*b + z + x):

> eq[20] :=
> (1/HessUniv) * ( - 2*f(2*y)*f(z + y)^2*f(a + 2*x)*f(c + z + x) +
f(2
> *y)*f(z + y)^2*f(a + 2*x)*f(a + 2*z) + 2*f(2*y)*f(z + x)
*f(z + y)*f(b
> + 2*x)*f(c + z + x) - f(2*y)*f(z + x)*f(z + y)*f(a + 2*
z)*f(b + 2*x)
> + 2*f(2*y)*f(z + x)*f(z + y)*f(a + 2*x)*f(c + z + y) -
f(2*y)*f(z +
> x)*f(z + y)*f(a + 2*x)*f(b + 2*z) - 2*f(2*y)*f(z + x)^2*
f(b + 2*x)*f(
> c + z + y) + f(2*y)*f(z + x)^2*f(b + 2*x)*f(b + 2*z) - f
(2*y)*f(2*z)*
> f(z + y)*f(b + 2*x)*f(c + 2*x) + f(2*y)*f(2*z)*f(z + y)*
f(a + 2*x)*f(
> c + y + x) + f(2*y)*f(2*z)*f(z + y)*f(a + 2*x)*f(b + z +
x) - f(2*y)*
> f(2*z)*f(z + y)*f(a + 2*x)*f(a + z + y) + f(2*y)*f(2*z)*
f(z + x)*f(b
> + 2*x)*f(c + y + x) - f(2*y)*f(2*z)*f(z + x)*f(b + 2*x)
*f(b + z + x)
> + f(2*y)*f(2*z)*f(z + x)*f(b + 2*x)*f(a + z + y) - f(2*
y)*f(2*z)*f(z
> + x)*f(a + 2*x)*f(c + 2*y) + 1/2*f(2*y)*f(2*z)^2*f(b +
2*x)^2 - f(2*
> y)*f(2*z)^2*f(a + 2*x)*f(b + y + x) + 1/2*f(2*y)*f(2*z)
^2*f(a + 2*x)*
> f(a + 2*y) - f(2*y)*f(2*z)*f(y + x)*f(c + 2*x)*f(c + y +
x) + f(2*y)*
> f(2*z)*f(y + x)*f(c + 2*x)*f(b + z + x) - f(2*y)*f(2*z)*
f(y + x)*f(c
> + 2*x)*f(a + z + y) - 2*f(2*y)*f(2*z)*f(y + x)*f(b + 2*
x)*f(c + z +
> x) + f(2*y)*f(2*z)*f(y + x)*f(a + 2*x)*f(b + 2*z) + 2*f
(2*y)*f(y + x)

```



```

>      *f(z + y)*f(c + 2*x)*f(c + z + x) + f(2*y)*f(y + x)*f(z
+ y)*f(a + 2*
>      z)*f(c + 2*x) - f(2*y)*f(y + x)*f(z + y)*f(a + 2*x)*f(c
+ 2*z) + 2*f(
>      2*y)*f(y + x)*f(z + x)*f(c + 2*x)*f(c + z + y) - f(2*y)*
f(y + x)*f(z
>      + x)*f(b + 2*z)*f(c + 2*x) + f(2*y)*f(y + x)*f(z + x)*f
(b + 2*x)*f(c
>      + 2*z) - f(2*y)*f(y + x)^2*f(c + 2*x)*f(c + 2*z) - 2*f
(2*y)^2*f(z +
>      x)*f(c + 2*x)*f(c + z + x) + 1/2*f(2*y)^2*f(2*z)*f(c +
2*x)^2 + f(2*y
>      )^2*f(2*z)*f(a + 2*x)*f(c + z + x) - 1/2*f(2*y)^2*f(2*z)
*f(a + 2*x)*
>      f(a + 2*z) + 2*f(2*x)*f(z + y)^2*f(a + 2*y)*f(c + z + x)
- f(2*x)*f(z
>      + y)^2*f(a + 2*y)*f(a + 2*z) - 2*f(2*x)*f(z + x)*f(z +
y)*f(b + 2*y)
>      *f(c + z + x) + f(2*x)*f(z + x)*f(z + y)*f(a + 2*z)*f(b
+ 2*y) - 2*f(
>      2*x)*f(z + x)*f(z + y)*f(a + 2*y)*f(c + z + y) + f(2*x)*
f(z + x)*f(z
>      + y)*f(a + 2*y)*f(b + 2*z) + 2*f(2*x)*f(z + x)^2*f(b +
2*y)*f(c + z
>      + y) - f(2*x)*f(z + x)^2*f(b + 2*y)*f(b + 2*z) + f(2*x)
*f(2*z)*f(z
>      + y)*f(b + 2*y)*f(c + 2*x) - f(2*x)*f(2*z)*f(z + y)*f(a
+ 2*y)*f(c
>      + y + x) - f(2*x)*f(2*z)*f(z + y)*f(a + 2*y)*f(b + z +
x) + f(2*x)*
>      f(2*z)*f(z + y)*f(a + 2*y)*f(a + z + y) - f(2*x)*f(2*z)*
f(z + x)*f(b
>      + 2*y)*f(c + y + x) + f(2*x)*f(2*z)*f(z + x)*f(b + 2*y)
*f(b + z + x)
>      - f(2*x)*f(2*z)*f(z + x)*f(b + 2*y)*f(a + z + y) + f(2*
x)*f(2*z)*f(z
>      + x)*f(a + 2*y)*f(c + 2*y) + f(2*x)*f(2*z)^2*f(b + 2*y)
*f(a + y + x)
>      - 1/2*f(2*x)*f(2*z)^2*f(b + 2*x)*f(b + 2*y) - 1/2*f(2*
x)*f(2*z)^2*f(
>      a + 2*y)^2 + f(2*x)*f(2*z)*f(y + x)*f(c + 2*y)*f(c + y +
x) + f(2*x)*
>      f(2*z)*f(y + x)*f(c + 2*y)*f(b + z + x) - f(2*x)*f(2*z)*
f(y + x)*f(c
>      + 2*y)*f(a + z + y) - f(2*x)*f(2*z)*f(y + x)*f(a + 2*z)
*f(b + 2*y)
>      + 2*f(2*x)*f(2*z)*f(y + x)*f(a + 2*y)*f(c + z + y) - 2*
f(2*x)*f(y +
>      x)*f(z + y)*f(c + 2*y)*f(c + z + x) + f(2*x)*f(y + x)*f
(z + y)*f(a +
>      2*z)*f(c + 2*y) - f(2*x)*f(y + x)*f(z + y)*f(a + 2*y)*f
(c + 2*z) - 2*
>      f(2*x)*f(y + x)*f(z + x)*f(c + 2*y)*f(c + z + y) - f(2*
x)*f(y + x)*f(
>      z + x)*f(b + 2*z)*f(c + 2*y) + f(2*x)*f(y + x)*f(z + x)*
f(b + 2*y)*f(
>      c + 2*z) + f(2*x)*f(y + x)^2*f(c + 2*y)*f(c + 2*z) + 2*f

```

```

(2*x)*f(2*y)*
> f(z + y)*f(c + 2*z)*f(a + y + x) - 2*f(2*x)*f(2*y)*f(z +
y)*f(c + 2*x
> )*f(c + z + y) - 2*f(2*x)*f(2*y)*f(z + y)*f(a + 2*z)*f(c
+ y + x) - 2
> *f(2*x)*f(2*y)*f(z + x)*f(c + 2*z)*f(b + y + x) + 2*f(2*
x)*f(2*y)*f(z
> + x)*f(c + 2*y)*f(c + z + x) + 2*f(2*x)*f(2*y)*f(z + x)
*f(b + 2*z)*
> f(c + y + x) - 2*f(2*x)*f(2*y)*f(2*z)*f(b + z + x)*f(c +
y + x) - f(2
> *x)*f(2*y)*f(2*z)*f(b + 2*z)*f(a + y + x) + 2*f(2*x)*f
(2*y)*f(2*z)*f(
> b + y + x)*f(c + z + x) + f(2*x)*f(2*y)*f(2*z)*f(b + 2*
x)*f(c + z + y
> ) - 1/2*f(2*x)*f(2*y)*f(2*z)*f(b + 2*x)*f(b + 2*z) + 2*f
(2*x)*f(2*y)*
> f(2*z)*f(a + z + y)*f(c + y + x) + f(2*x)*f(2*y)*f(2*z)*
f(a + 2*z)*f(
> b + y + x) - 2*f(2*x)*f(2*y)*f(2*z)*f(a + y + x)*f(c + z
+ y) - f(2*x
> )*f(2*y)*f(2*z)*f(a + 2*y)*f(c + z + x) + 1/2*f(2*x)*f
(2*y)*f(2*z)*f(
> a + 2*y)*f(a + 2*z) + f(2*x)*f(2*y)^2*f(c + 2*x)*f(c +
2*z) + 2*f(2*x
> )^2*f(z + y)*f(c + 2*y)*f(c + z + y) - 1/2*f(2*x)^2*f(2*
z)*f(c + 2*y)
> ^2 - f(2*x)^2*f(2*z)*f(b + 2*y)*f(c + z + y) + 1/2*f(2*
x)^2*f(2*z)*f(
> b + 2*y)*f(b + 2*z) - f(2*x)^2*f(2*y)*f(c + 2*y)*f(c +
2*z) )
> - f(2*y)*f(2*c + 2*x) + f(2*x)*f(2*c + 2*y):

> eq[21] :=
> (1/HessUniv) * ( 2*f(z + y)^3*f(b + 2*y)*f(c + 2*x) - 4*f(z + x)*
f(z
> + y)^2*f(b + 2*y)*f(c + y + x) + 2*f(z + x)^2*f(z + y)*
f(b + 2*y)*f(
> c + 2*y) + 4*f(2*z)*f(z + y)^2*f(b + 2*y)*f(a + y + x) -
f(2*z)*f(z
> + y)^2*f(b + 2*x)*f(b + 2*y) - 2*f(2*z)*f(z + y)^2*f(a
+ 2*y)*f(b +
> y + x) - f(2*z)*f(z + y)^2*f(a + 2*y)^2 + 2*f(2*z)*f(y +
x)*f(z + y)*
> f(c + 2*y)*f(b + y + x) + 2*f(2*z)*f(y + x)*f(z + y)*f(b
+ 2*y)*f(b
> + z + x) - 4*f(2*z)*f(y + x)*f(z + y)*f(b + 2*y)*f(a +
z + y) + 2*f(
> 2*z)*f(y + x)*f(z + y)*f(a + 2*y)*f(c + 2*y) + 2*f(2*z)*
f(y + x)*f(z
> + y)*f(a + 2*y)*f(b + z + y) - 4*f(y + x)*f(z + y)^2*f
(b + 2*y)*f(c
> + z + x) - 2*f(y + x)*f(z + x)*f(z + y)*f(c + 2*y)^2 -
4*f(y + x)*f(
> z + x)*f(z + y)*f(c + 2*y)*f(b + z + y) + 4*f(y + x)*f(z
+ x)*f(z + y

```

```

> )*f(b + 2*y)*f(c + z + y) - 2*f(y + x)*f(z + x)*f(z + y)
> *f(b + 2*y)*
> f(b + 2*z) + 2*f(y + x)^2*f(z + y)*f(b + 2*y)*f(c + 2*z)
> - f(2*y)*f(z
> + y)^2*f(c + 2*x)*f(c + 2*y) - 2*f(2*y)*f(z + y)^2*f(c
> + 2*x)*f(b +
> z + y) + 2*f(2*y)*f(z + y)^2*f(a + 2*y)*f(c + z + x) - f
> (2*y)*f(z + y
> )^2*f(a + 2*y)*f(a + 2*z) + 2*f(2*y)*f(z + x)*f(z + y)*f
> (c + 2*y)*f(c
> + y + x) + 4*f(2*y)*f(z + x)*f(z + y)*f(b + z + y)*f(c
> + y + x) + 2*
> f(2*y)*f(z + x)*f(z + y)*f(b + 2*y)*f(c + z + x) + f(2*
> y)*f(z + x)*f(
> z + y)*f(a + 2*z)*f(b + 2*y) - 2*f(2*y)*f(z + x)*f(z +
> y)*f(a + 2*y)*
> f(c + z + y) + f(2*y)*f(z + x)*f(z + y)*f(a + 2*y)*f(b +
> 2*z) - 2*f(2
> *y)*f(z + x)^2*f(b + 2*y)*f(c + z + y) - 2*f(2*y)*f(2*z)
> *f(z + y)*f(c
> + 2*y)*f(a + y + x) - 1/2*f(2*y)*f(2*z)*f(z + y)*f(b +
> 2*y)*f(c + 2*
> x) - 2*f(2*y)*f(2*z)*f(z + y)*f(b + 2*y)*f(a + z + x) +
> 1/2*f(2*y)*f(
> 2*z)*f(z + y)*f(b + 2*x)*f(c + 2*y) + f(2*y)*f(2*z)*f(z
> + y)*f(b + 2*
> x)*f(b + z + y) + 2*f(2*y)*f(2*z)*f(z + y)*f(a + z + y)*
> f(b + y + x)
> - 4*f(2*y)*f(2*z)*f(z + y)*f(a + y + x)*f(b + z + y) +
> 3*f(2*y)*f(2*
> z)*f(z + y)*f(a + 2*y)*f(a + z + y) - f(2*y)*f(2*z)*f(z
> + x)*f(c + 2*
> y)*f(b + y + x) + f(2*y)*f(2*z)*f(z + x)*f(b + 2*y)*f(c
> + y + x) + f(
> 2*y)*f(2*z)*f(z + x)*f(b + 2*y)*f(a + z + y) - f(2*y)*f
> (2*z)*f(z + x)
> *f(a + 2*y)*f(b + z + y) - f(2*y)*f(2*z)^2*f(b + 2*y)*f
> (a + y + x) +
> f(2*y)*f(2*z)^2*f(a + 2*y)*f(b + y + x) - f(2*y)*f(2*z)*
> f(y + x)*f(c
> + 2*y)*f(b + z + x) - f(2*y)*f(2*z)*f(y + x)*f(c + 2*y)
> *f(a + z + y)
> - 2*f(2*y)*f(2*z)*f(y + x)*f(b + z + x)*f(b + z + y) -
> 2*f(2*y)*f(2*
> z)*f(y + x)*f(b + y + x)*f(c + z + y) + f(2*y)*f(2*z)*f
> (y + x)*f(b +
> 2*y)*f(c + z + x) + 2*f(2*y)*f(2*z)*f(y + x)*f(a + z +
> y)*f(b + z + y
> ) + f(2*y)*f(2*z)*f(y + x)*f(a + 2*z)*f(b + 2*y) - f(2*
> y)*f(2*z)*f(y
> + x)*f(a + 2*y)*f(c + z + y) - f(2*y)*f(2*z)*f(y + x)*f
> (a + 2*y)*f(b
> + 2*z) + 4*f(2*y)*f(y + x)*f(z + y)*f(b + z + y)*f(c +
> z + x) + f(2*
> y)*f(y + x)*f(z + y)*f(a + 2*z)*f(c + 2*y) - f(2*y)*f(y
> + x)*f(z + y)
> *f(a + 2*y)*f(c + 2*z) + 2*f(2*y)*f(y + x)*f(z + x)*f(c

```

```

+ 2*y)*f(c +
>      z + y) + 2*f(2*y)*f(y + x)*f(z + x)*f(b + 2*z)*f(c + 2*
y) + 2*f(2*y)*
>      f(y + x)*f(z + x)*f(b + 2*z)*f(b + z + y) - 2*f(2*y)*f(y
+ x)*f(z + x
>      )*f(b + 2*y)*f(c + 2*z) - 2*f(2*y)*f(y + x)^2*f(c + 2*z)
*f(b + z + y)
>      + f(2*y)^2*f(z + y)*f(c + 2*x)*f(c + z + y) + 1/2*f(2*
y)^2*f(z + y)*
>      f(b + 2*z)*f(c + 2*x) - 1/2*f(2*y)^2*f(z + y)*f(b + 2*x)
*f(c + 2*z)
>      - 2*f(2*y)^2*f(z + y)*f(a + z + y)*f(c + z + x) + f(2*
y)^2*f(z + y)*
>      f(a + 2*z)*f(a + z + y) + f(2*y)^2*f(z + x)*f(c + 2*z)*f
(b + y + x)
>      - 2*f(2*y)^2*f(z + x)*f(c + y + x)*f(c + z + y) - 2*f
(2*y)^2*f(z + x
>      )*f(b + z + y)*f(c + z + x) - f(2*y)^2*f(z + x)*f(b + 2*
z)*f(c + y +
>      x) - f(2*y)^2*f(z + x)*f(b + 2*z)*f(a + z + y) + 2*f(2*
y)^2*f(z + x)*
>      f(a + z + y)*f(c + z + y) - f(2*y)^2*f(z + x)*f(a + 2*z)
*f(c + 2*y)
>      - f(2*y)^2*f(z + x)*f(a + 2*z)*f(b + z + y) + f(2*y)^2*
f(z + x)*f(a
>      + 2*y)*f(c + 2*z) + f(2*y)^2*f(2*z)*f(c + 2*y)*f(a + z
+ x) + f(2*y)
>      ^2*f(2*z)*f(b + 2*z)*f(a + y + x) - 2*f(2*y)^2*f(2*z)*f
(a + z + y)^2
>      + 2*f(2*y)^2*f(2*z)*f(a + z + x)*f(b + z + y) - f(2*y)
^2*f(2*z)*f(a
>      + 2*z)*f(b + y + x) + 2*f(2*y)^2*f(2*z)*f(a + y + x)*f
(c + z + y) -
>      f(2*y)^2*f(2*z)*f(a + 2*y)*f(c + z + x) + f(2*y)^2*f(y +
x)*f(c + 2*z
>      )*f(b + z + x) + f(2*y)^2*f(y + x)*f(c + 2*z)*f(a + z +
y) - f(2*y)^2
>      *f(y + x)*f(b + 2*z)*f(c + z + x) - f(2*y)^2*f(y + x)*f
(a + 2*z)*f(c
>      + z + y) - f(2*y)^3*f(c + 2*z)*f(a + z + x) + f(2*y)^3*
f(a + 2*z)*f(c
>      + z + x) + f(2*x)*f(z + y)^2*f(c + 2*y)^2 + 2*f(2*x)*f
(z + y)^2*f(c
>      + 2*y)*f(b + z + y) + f(2*x)*f(z + y)^2*f(b + 2*y)*f(b
+ 2*z) - 2*f(
>      2*x)*f(2*z)*f(z + y)*f(b + 2*y)*f(c + 2*y) - f(2*x)*f(2*
y)*f(z + y)*
>      f(c + 2*y)*f(c + z + y) - 2*f(2*x)*f(2*y)*f(z + y)*f(b +
z + y)*f(c
>      + z + y) - 3/2*f(2*x)*f(2*y)*f(z + y)*f(b + 2*z)*f(c +
2*y) - f(2*x)
>      *f(2*y)*f(z + y)*f(b + 2*z)*f(b + z + y) - 1/2*f(2*x)*f
(2*y)*f(z + y)
>      *f(b + 2*y)*f(c + 2*z) + f(2*x)*f(2*y)*f(2*z)*f(c + 2*y)
*f(b + z + y)
>      + f(2*x)*f(2*y)*f(2*z)*f(b + 2*y)*f(c + z + y) + f(2*x)
*f(2*y)^2*f(c

```

```

>      + 2*z)*f(b + z + y) + f(2*x)*f(2*y)^2*f(b + 2*z)*f(c +
>      z + y) )
>      + 2*f(z + y)*f(c + b + 2*y) - 2*f(2*y)*f(c + b + z + y):
> eq[22] :=
> (1/HessUniv) * ( 2*f(z + y)^3*f(a + 2*y)*f(c + 2*x) - 4*f(z + x)*
> f(z
>      + y)^2*f(a + 2*y)*f(c + y + x) + 2*f(z + x)^2*f(z + y)*
> f(a + 2*y)*f(
>      c + 2*y) - f(2*z)*f(z + y)^2*f(a + 2*y)*f(b + 2*x) + f
> (2*z)*f(z + y)^
>      2*f(a + 2*x)*f(b + 2*y) + 2*f(2*z)*f(z + x)*f(z + y)*f(b
> + 2*y)*f(a
>      + y + x) - f(2*z)*f(z + x)*f(z + y)*f(b + 2*x)*f(b + 2*
> y) - f(2*z)*
>      f(z + x)*f(z + y)*f(a + 2*y)^2 + f(2*z)*f(y + x)*f(z +
> y)*f(b + 2*y)*
>      f(c + 2*x) - 2*f(2*z)*f(y + x)*f(z + y)*f(b + 2*y)*f(a +
> z + x) + f(2
>      *z)*f(y + x)*f(z + y)*f(b + 2*x)*f(c + 2*y) + 2*f(2*z)*f
> (y + x)*f(z
>      + y)*f(a + 2*y)*f(c + y + x) + 2*f(2*z)*f(y + x)*f(z +
> y)*f(a + 2*y)
>      *f(a + z + y) - 2*f(y + x)*f(z + y)^2*f(c + 2*x)*f(c +
> 2*y) - 2*f(y
>      + x)*f(z + y)^2*f(a + 2*y)*f(a + 2*z) - 4*f(y + x)*f(z
> + x)*f(z + y)
>      *f(c + 2*y)*f(a + z + y) + 2*f(y + x)^2*f(z + y)*f(a +
> 2*z)*f(c + 2*y
>      ) - 2*f(2*y)*f(z + y)^2*f(c + 2*x)*f(a + z + y) + f(2*y)
> *f(z + x)*f(z
>      + y)*f(c + 2*x)*f(c + 2*y) + 4*f(2*y)*f(z + x)*f(z + y)
> *f(a + z + y)
>      *f(c + y + x) + 2*f(2*y)*f(z + x)*f(z + y)*f(a + 2*y)*f
> (c + z + x) +
>      f(2*y)*f(z + x)*f(z + y)*f(a + 2*y)*f(a + 2*z) - 2*f(2*
> y)*f(z + x)^2*
>      f(a + 2*y)*f(c + z + y) + f(2*y)*f(2*z)*f(z + y)*f(b +
> 2*x)*f(a + z
>      + y) - 3/2*f(2*y)*f(2*z)*f(z + y)*f(a + 2*y)*f(c + 2*x)
> - 1/2*f(2*y)
>      *f(2*z)*f(z + y)*f(a + 2*x)*f(c + 2*y) - f(2*y)*f(2*z)*f
> (z + y)*f(a
>      + 2*x)*f(b + z + y) - f(2*y)*f(2*z)*f(z + x)*f(c + 2*y)
> *f(a + y + x)
>      + f(2*y)*f(2*z)*f(z + x)*f(b + 2*x)*f(b + z + y) - 2*f
> (2*y)*f(2*z)*
>      f(z + x)*f(a + y + x)*f(b + z + y) + f(2*y)*f(2*z)*f(z +
> x)*f(a + 2*y
>      )*f(c + y + x) + f(2*y)*f(2*z)*f(z + x)*f(a + 2*y)*f(a +
> z + y) + 1/2
>      *f(2*y)*f(2*z)^2*f(a + 2*y)*f(b + 2*x) - 1/2*f(2*y)*f(2*
> z)^2*f(a + 2*
>      x)*f(b + 2*y) + f(2*y)*f(2*z)*f(y + x)*f(c + 2*y)*f(a +
> z + x) - f(2*
>      y)*f(2*z)*f(y + x)*f(c + 2*x)*f(b + z + y) - f(2*y)*f(2*

```

```

z)*f(y + x)*
> f(b + 2*x)*f(c + z + y) - 2*f(2*y)*f(2*z)*f(y + x)*f(a +
z + y)*f(c
> + y + x) - 2*f(2*y)*f(2*z)*f(y + x)*f(a + z + y)^2 + 2*
f(2*y)*f(2*z)
> *f(y + x)*f(a + z + x)*f(b + z + y) - f(2*y)*f(2*z)*f(y
+ x)*f(a + 2*
> y)*f(c + z + x) + 2*f(2*y)*f(y + x)*f(z + y)*f(c + 2*x)*
f(c + z + y)
> + 2*f(2*y)*f(y + x)*f(z + y)*f(a + 2*z)*f(a + z + y) +
4*f(2*y)*f(y
> + x)*f(z + x)*f(a + z + y)*f(c + z + y) - 2*f(2*y)*f(y
+ x)^2*f(a +
> 2*z)*f(c + z + y) + 1/2*f(2*y)^2*f(z + y)*f(a + 2*z)*f(c
+ 2*x) - 1/2
> *f(2*y)^2*f(z + y)*f(a + 2*x)*f(c + 2*z) + f(2*y)^2*f(z
+ x)*f(c + 2*
> z)*f(a + y + x) - f(2*y)^2*f(z + x)*f(c + 2*x)*f(c + z +
y) - 2*f(2*y
> )^2*f(z + x)*f(a + z + y)*f(c + z + x) - f(2*y)^2*f(z +
x)*f(a + 2*z)
> *f(c + y + x) - f(2*y)^2*f(z + x)*f(a + 2*z)*f(a + z +
y) + f(2*y)^2*
> f(2*z)*f(c + 2*x)*f(a + z + y) - 1/2*f(2*y)^2*f(2*z)*f(a
+ 2*z)*f(b
> + 2*x) + f(2*y)^2*f(2*z)*f(a + 2*x)*f(c + z + y) + 1/2*
f(2*y)^2*f(2*
> z)*f(a + 2*x)*f(b + 2*z) - f(2*y)^2*f(y + x)*f(c + 2*z)*
f(a + z + x)
> + f(2*y)^2*f(y + x)*f(a + 2*z)*f(c + z + x) + 2*f(2*x)*
f(z + y)^2*f(
> c + 2*y)*f(c + y + x) + 2*f(2*x)*f(z + y)^2*f(c + 2*y)*f
(a + z + y)
> - 2*f(2*x)*f(z + y)^2*f(b + 2*y)*f(c + z + x) + f(2*x)*
f(z + y)^2*f(
> a + 2*z)*f(b + 2*y) + f(2*x)*f(z + y)^2*f(a + 2*y)*f(b +
2*z) - f(2*x
> )*f(z + x)*f(z + y)*f(c + 2*y)^2 + 2*f(2*x)*f(z + x)*f(z
+ y)*f(b + 2
> *y)*f(c + z + y) - f(2*x)*f(z + x)*f(z + y)*f(b + 2*y)*f
(b + 2*z) - 2
> *f(2*x)*f(2*z)*f(z + y)*f(b + 2*y)*f(c + y + x) + 2*f(2*
x)*f(2*z)*f(z
> + y)*f(b + 2*y)*f(b + z + x) - 2*f(2*x)*f(2*z)*f(z + y)
*f(b + 2*y)*
> f(a + z + y) - f(2*x)*f(y + x)*f(z + y)*f(b + 2*z)*f(c +
2*y) + f(2*x
> )*f(y + x)*f(z + y)*f(b + 2*y)*f(c + 2*z) - 2*f(2*x)*f
(2*y)*f(z + y)*
> f(c + y + x)*f(c + z + y) + 2*f(2*x)*f(2*y)*f(z + y)*f(b
+ z + y)*f(c
> + z + x) - f(2*x)*f(2*y)*f(z + y)*f(b + 2*z)*f(a + z +
y) - 2*f(2*x)
> *f(2*y)*f(z + y)*f(a + z + y)*f(c + z + y) - 3/2*f(2*x)*
f(2*y)*f(z +
> y)*f(a + 2*z)*f(c + 2*y) - f(2*x)*f(2*y)*f(z + y)*f(a +
2*z)*f(b + z

```

```

> + y) - 1/2*f(2*x)*f(2*y)*f(z + y)*f(a + 2*y)*f(c + 2*z)
> + f(2*x)*f(2
> *y)*f(z + x)*f(c + 2*y)*f(c + z + y) - 2*f(2*x)*f(2*y)*f
> (z + x)*f(b
> + z + y)*f(c + z + y) + f(2*x)*f(2*y)*f(z + x)*f(b + 2*
> z)*f(c + 2*y)
> + f(2*x)*f(2*y)*f(z + x)*f(b + 2*z)*f(b + z + y) - f(2*
> x)*f(2*y)*f(z
> + x)*f(b + 2*y)*f(c + 2*z) - f(2*x)*f(2*y)*f(2*z)*f(c +
> 2*y)*f(b + z
> + x) + 2*f(2*x)*f(2*y)*f(2*z)*f(b + z + y)*f(c + y + x)
> - 2*f(2*x)*
> f(2*y)*f(2*z)*f(b + z + x)*f(b + z + y) + f(2*x)*f(2*y)*
> f(2*z)*f(b +
> 2*y)*f(c + z + x) + 2*f(2*x)*f(2*y)*f(2*z)*f(a + z + y)*
> f(b + z + y)
> + 1/2*f(2*x)*f(2*y)*f(2*z)*f(a + 2*z)*f(b + 2*y) - 1/2*
> f(2*x)*f(2*y)
> *f(2*z)*f(a + 2*y)*f(b + 2*z) - f(2*x)*f(2*y)*f(y + x)*f
> (c + 2*z)*f(b
> + z + y) + f(2*x)*f(2*y)*f(y + x)*f(b + 2*z)*f(c + z +
> y) + f(2*x)*
> f(2*y)^2*f(c + 2*z)*f(b + z + x) + f(2*x)*f(2*y)^2*f(c +
> 2*z)*f(a + z
> + y) - f(2*x)*f(2*y)^2*f(b + 2*z)*f(c + z + x) + f(2*x)
> *f(2*y)^2*f(a
> + 2*z)*f(c + z + y) )
>
> + 2*f(z + y)*f(c + a + 2*y) - 2*f(2*y)*f(c + a + z + y):
>
> eq[23] :=
> (1/HessUniv) * ( 2*f(z + x)*f(z + y)^2*f(b + 2*y)*f(c + 2*x) - 4*
> f(z
> + x)^2*f(z + y)*f(b + 2*y)*f(c + y + x) + 2*f(z + x)^3*
> f(b + 2*y)*f(
> c + 2*y) + 4*f(2*z)*f(z + x)*f(z + y)*f(b + 2*y)*f(a + y
> + x) - f(2*z
> )*f(z + x)*f(z + y)*f(b + 2*x)*f(b + 2*y) - 2*f(2*z)*f(z
> + x)*f(z + y
> )*f(a + 2*y)*f(b + y + x) - f(2*z)*f(z + x)*f(z + y)*f(a
> + 2*y)^2 + 2
> *f(2*z)*f(y + x)*f(z + x)*f(c + 2*y)*f(b + y + x) + 2*f
> (2*z)*f(y + x)
> *f(z + x)*f(b + 2*y)*f(b + z + x) - 4*f(2*z)*f(y + x)*f
> (z + x)*f(b +
> 2*y)*f(a + z + y) + 2*f(2*z)*f(y + x)*f(z + x)*f(a + 2*
> y)*f(c + 2*y)
> + 2*f(2*z)*f(y + x)*f(z + x)*f(a + 2*y)*f(b + z + y) -
> 4*f(y + x)*f(
> z + x)*f(z + y)*f(b + 2*y)*f(c + z + x) - 2*f(y + x)*f(z
> + x)^2*f(c
> + 2*y)^2 - 4*f(y + x)*f(z + x)^2*f(c + 2*y)*f(b + z +
> y) + 4*f(y + x
> )*f(z + x)^2*f(b + 2*y)*f(c + z + y) - 2*f(y + x)*f(z +
> x)^2*f(b + 2*
> y)*f(b + 2*z) + 2*f(y + x)^2*f(z + x)*f(b + 2*y)*f(c +
> 2*z) - 2*f(2*y

```

```

> )*f(z + y)^2*f(b + 2*x)*f(c + z + x) - f(2*y)*f(z + x)*f
(z + y)*f(c
> + 2*x)*f(c + 2*y) - 2*f(2*y)*f(z + x)*f(z + y)*f(c + 2*
x)*f(b + z +
> y) + 4*f(2*y)*f(z + x)*f(z + y)*f(b + y + x)*f(c + z +
x) + 2*f(2*y)*
> f(z + x)*f(z + y)*f(b + 2*x)*f(c + z + y) + 2*f(2*y)*f(z
+ x)*f(z + y
> )*f(a + 2*y)*f(c + z + x) - f(2*y)*f(z + x)*f(z + y)*f(a
+ 2*y)*f(a
> + 2*z) + 2*f(2*y)*f(z + x)^2*f(c + 2*y)*f(c + y + x) +
4*f(2*y)*f(z
> + x)^2*f(b + z + y)*f(c + y + x) - 4*f(2*y)*f(z + x)^2*
f(b + y + x)*
> f(c + z + y) + f(2*y)*f(z + x)^2*f(a + 2*z)*f(b + 2*y) -
2*f(2*y)*f(z
> + x)^2*f(a + 2*y)*f(c + z + y) + f(2*y)*f(z + x)^2*f(a
+ 2*y)*f(b +
> 2*z) - f(2*y)*f(2*z)*f(z + y)*f(c + 2*x)*f(b + y + x) +
f(2*y)*f(2*z)
> *f(z + y)*f(b + 2*x)*f(c + y + x) + f(2*y)*f(2*z)*f(z +
y)*f(b + 2*x)
> *f(b + z + x) - 2*f(2*y)*f(2*z)*f(z + y)*f(a + z + x)*f
(b + y + x) +
> f(2*y)*f(2*z)*f(z + y)*f(a + 2*y)*f(a + z + x) - 2*f(2*
y)*f(2*z)*f(z
> + x)*f(c + 2*y)*f(a + y + x) + 1/2*f(2*y)*f(2*z)*f(z +
x)*f(b + 2*y)
> *f(c + 2*x) - f(2*y)*f(2*z)*f(z + x)*f(b + 2*y)*f(a + z
+ x) - 1/2*f(
> 2*y)*f(2*z)*f(z + x)*f(b + 2*x)*f(c + 2*y) + 4*f(2*y)*f
(2*z)*f(z + x)
> *f(a + z + y)*f(b + y + x) - 4*f(2*y)*f(2*z)*f(z + x)*f
(a + y + x)*f(
> b + z + y) - f(2*y)*f(2*z)*f(z + x)*f(a + 2*y)*f(b + z +
x) + 2*f(2*y
> )*f(2*z)*f(z + x)*f(a + 2*y)*f(a + z + y) + 1/2*f(2*y)*f
(2*z)^2*f(a
> + 2*y)*f(b + 2*x) - 1/2*f(2*y)*f(2*z)^2*f(a + 2*x)*f(b
+ 2*y) - f(2*
> y)*f(2*z)*f(y + x)*f(c + 2*y)*f(a + z + x) + f(2*y)*f(2*
z)*f(y + x)*
> f(c + 2*x)*f(b + z + y) - 2*f(2*y)*f(2*z)*f(y + x)*f(b +
z + x)*f(c
> + y + x) - 2*f(2*y)*f(2*z)*f(y + x)*f(b + z + x)^2 - f
(2*y)*f(2*z)*
> f(y + x)*f(b + 2*x)*f(c + z + y) + 2*f(2*y)*f(2*z)*f(y +
x)*f(a + z
> + x)*f(b + z + y) - f(2*y)*f(2*z)*f(y + x)*f(a + 2*y)*f
(c + z + x)
> + 4*f(2*y)*f(y + x)*f(z + y)*f(b + z + x)*f(c + z + x)
- 2*f(2*y)*f(
> y + x)*f(z + x)*f(c + 2*z)*f(b + y + x) + 2*f(2*y)*f(y +
x)*f(z + x)*
> f(c + 2*y)*f(c + z + x) + 2*f(2*y)*f(y + x)*f(z + x)*f(b
+ 2*z)*f(c
> + y + x) + 2*f(2*y)*f(y + x)*f(z + x)*f(b + 2*z)*f(b +

```



```

z + x) + f(2*
>      y)*f(y + x)*f(z + x)*f(a + 2*z)*f(c + 2*y) - f(2*y)*f(y
+ x)*f(z + x)
>      *f(a + 2*y)*f(c + 2*z) - 2*f(2*y)*f(y + x)^2*f(b + 2*z)*
f(c + z + x)
>      + f(2*y)^2*f(z + y)*f(c + 2*x)*f(c + z + x) - 2*f(2*y)
^2*f(z + y)*f(
>      a + z + x)*f(c + z + x) + f(2*y)^2*f(z + y)*f(a + 2*z)*f
(c + 2*x) +
>      f(2*y)^2*f(z + y)*f(a + 2*z)*f(a + z + x) - f(2*y)^2*f(z
+ y)*f(a + 2
>      *x)*f(c + 2*z) + 2*f(2*y)^2*f(z + x)*f(c + 2*z)*f(a + y
+ x) - 2*f(2*
>      y)^2*f(z + x)*f(c + y + x)*f(c + z + x) - 2*f(2*y)^2*f(z
+ x)*f(b + z
>      + x)*f(c + z + x) - 1/2*f(2*y)^2*f(z + x)*f(b + 2*z)*f
(c + 2*x) - f(
>      2*y)^2*f(z + x)*f(b + 2*z)*f(a + z + x) + 1/2*f(2*y)^2*f
(z + x)*f(b
>      + 2*x)*f(c + 2*z) + 2*f(2*y)^2*f(z + x)*f(a + z + x)*f
(c + z + y) -
>      2*f(2*y)^2*f(z + x)*f(a + 2*z)*f(c + y + x) - f(2*y)^2*f
(z + x)*f(a
>      + 2*z)*f(b + z + x) - f(2*y)^2*f(2*z)*f(c + 2*x)*f(a +
z + y) + 2*f(
>      2*y)^2*f(2*z)*f(a + z + x)*f(c + y + x) + 2*f(2*y)^2*f
(2*z)*f(a + z
>      + x)*f(b + z + x) - 2*f(2*y)^2*f(2*z)*f(a + z + x)*f(a
+ z + y) - 1/
>      2*f(2*y)^2*f(2*z)*f(a + 2*z)*f(b + 2*x) + f(2*y)^2*f(2*
z)*f(a + 2*x)*
>      f(c + z + y) + 1/2*f(2*y)^2*f(2*z)*f(a + 2*x)*f(b + 2*z)
- f(2*y)^2*
>      f(y + x)*f(c + 2*z)*f(a + z + x) + f(2*y)^2*f(y + x)*f(a
+ 2*z)*f(c
>      + z + x) + f(2*x)*f(z + x)*f(z + y)*f(c + 2*y)^2 + 2*f
(2*x)*f(z + x)
>      *f(z + y)*f(c + 2*y)*f(b + z + y) + f(2*x)*f(z + x)*f(z
+ y)*f(b + 2*
>      y)*f(b + 2*z) - 2*f(2*x)*f(2*z)*f(z + x)*f(b + 2*y)*f(c
+ 2*y) + f(2*
>      x)*f(2*y)*f(z + y)*f(c + 2*z)*f(b + y + x) - f(2*x)*f(2*
y)*f(z + y)*
>      f(c + 2*y)*f(c + z + x) - 2*f(2*x)*f(2*y)*f(z + y)*f(b +
z + x)*f(c
>      + z + y) - f(2*x)*f(2*y)*f(z + y)*f(b + 2*z)*f(c + y +
x) - f(2*x)*
>      f(2*y)*f(z + y)*f(b + 2*z)*f(b + z + x) - 1/2*f(2*x)*f
(2*y)*f(z + x)*
>      f(b + 2*z)*f(c + 2*y) - 3/2*f(2*x)*f(2*y)*f(z + x)*f(b +
2*y)*f(c + 2
>      *z) + f(2*x)*f(2*y)*f(2*z)*f(c + 2*y)*f(b + z + x) + f
(2*x)*f(2*y)*f(
>      2*z)*f(b + 2*y)*f(c + z + x) + 1/2*f(2*x)*f(2*y)*f(2*z)*
f(a + 2*z)*f(
>      b + 2*y) - 1/2*f(2*x)*f(2*y)*f(2*z)*f(a + 2*y)*f(b + 2*
z) - f(2*x)*f(

```

```

>      2*y)*f(y + x)*f(c + 2*z)*f(b + z + y) + f(2*x)*f(2*y)*f
(y + x)*f(b +
>      2*z)*f(c + z + y) + f(2*x)*f(2*y)^2*f(c + 2*z)*f(b + z +
x) + f(2*x)*
>      f(2*y)^2*f(c + 2*z)*f(a + z + y) + f(2*x)*f(2*y)^2*f(b +
2*z)*f(c + z
>      + x) - f(2*x)*f(2*y)^2*f(a + 2*z)*f(c + z + y) )
>
>      + 2*f(z + x)*f(c + b + 2*y) - 2*f(2*y)*f(c + b + z + x):
>
> eq[24] :=
> (1/HessUniv) * ( 2*f(z + x)*f(z + y)^2*f(a + 2*y)*f(c + 2*x) - 4*
f(z
>      + x)^2*f(z + y)*f(a + 2*y)*f(c + y + x) + 2*f(z + x)^3*
f(a + 2*y)*f(
>      c + 2*y) - f(2*z)*f(z + x)*f(z + y)*f(a + 2*y)*f(b + 2*
x) + f(2*z)*f(
>      z + x)*f(z + y)*f(a + 2*x)*f(b + 2*y) + 2*f(2*z)*f(z +
x)^2*f(b + 2*y
>      )*f(a + y + x) - f(2*z)*f(z + x)^2*f(b + 2*x)*f(b + 2*y)
- f(2*z)*f(z
>      + x)^2*f(a + 2*y)^2 + f(2*z)*f(y + x)*f(z + x)*f(b + 2*
y)*f(c + 2*x)
>      - 2*f(2*z)*f(y + x)*f(z + x)*f(b + 2*y)*f(a + z + x) +
f(2*z)*f(y +
>      x)*f(z + x)*f(b + 2*x)*f(c + 2*y) + 2*f(2*z)*f(y + x)*f
(z + x)*f(a +
>      2*y)*f(c + y + x) + 2*f(2*z)*f(y + x)*f(z + x)*f(a + 2*
y)*f(a + z + y
>      ) - 2*f(y + x)*f(z + x)*f(z + y)*f(c + 2*x)*f(c + 2*y) -
2*f(y + x)*
>      f(z + x)*f(z + y)*f(a + 2*y)*f(a + 2*z) - 4*f(y + x)*f(z
+ x)^2*f(c
>      + 2*y)*f(a + z + y) + 2*f(y + x)^2*f(z + x)*f(a + 2*z)*
f(c + 2*y) -
>      2*f(2*y)*f(z + y)^2*f(a + 2*x)*f(c + z + x) - 2*f(2*y)*f
(z + x)*f(z
>      + y)*f(c + 2*x)*f(a + z + y) + 4*f(2*y)*f(z + x)*f(z +
y)*f(a + y +
>      x)*f(c + z + x) + 2*f(2*y)*f(z + x)*f(z + y)*f(a + 2*x)*
f(c + z + y)
>      + f(2*y)*f(z + x)^2*f(c + 2*x)*f(c + 2*y) + 4*f(2*y)*f
(z + x)^2*f(a
>      + z + y)*f(c + y + x) - 4*f(2*y)*f(z + x)^2*f(a + y +
x)*f(c + z + y
>      ) + f(2*y)*f(z + x)^2*f(a + 2*y)*f(a + 2*z) - f(2*y)*f
(2*z)*f(z + y)*
>      f(c + 2*x)*f(a + y + x) - f(2*y)*f(2*z)*f(z + y)*f(b +
2*x)*f(a + z
>      + x) + f(2*y)*f(2*z)*f(z + y)*f(a + 2*x)*f(c + y + x) +
f(2*y)*f(2*z
>      )*f(z + y)*f(a + 2*x)*f(b + z + x) + f(2*y)*f(2*z)*f(z +
x)*f(b + 2*x
>      )*f(b + z + x) + 2*f(2*y)*f(2*z)*f(z + x)*f(b + 2*x)*f(a
+ z + y) - 2
>      *f(2*y)*f(2*z)*f(z + x)*f(a + y + x)*f(b + z + x) - 1/2*
f(2*y)*f(2*z)

```

```

>      *f(z + x)*f(a + 2*y)*f(c + 2*x) + f(2*y)*f(2*z)*f(z + x)
>      *f(a + 2*y)*
>      f(a + z + x) - 3/2*f(2*y)*f(2*z)*f(z + x)*f(a + 2*x)*f(c
>      + 2*y) - 2*
>      f(2*y)*f(2*z)*f(z + x)*f(a + 2*x)*f(b + z + y) + f(2*y)*
>      f(2*z)^2*f(b
>      + 2*x)*f(a + y + x) - f(2*y)*f(2*z)^2*f(a + 2*x)*f(b +
>      y + x) - f(2*
>      y)*f(2*z)*f(y + x)*f(c + 2*x)*f(b + z + x) - f(2*y)*f(2*
>      z)*f(y + x)*
>      f(c + 2*x)*f(a + z + y) - f(2*y)*f(2*z)*f(y + x)*f(b +
>      2*x)*f(c + z
>      + x) + 2*f(2*y)*f(2*z)*f(y + x)*f(a + z + x)*f(b + z +
>      x) - 2*f(2*y)
>      *f(2*z)*f(y + x)*f(a + z + x)*f(a + z + y) - f(2*y)*f(2*
>      z)*f(y + x)*
>      f(a + 2*z)*f(b + 2*x) - 2*f(2*y)*f(2*z)*f(y + x)*f(a + y
>      + x)*f(c + z
>      + x) + f(2*y)*f(2*z)*f(y + x)*f(a + 2*x)*f(c + z + y) +
>      f(2*y)*f(2*z
>      )*f(y + x)*f(a + 2*x)*f(b + 2*z) + 2*f(2*y)*f(y + x)*f(z
>      + y)*f(c + 2
>      *x)*f(c + z + x) + 2*f(2*y)*f(y + x)*f(z + y)*f(a + 2*z)
>      *f(c + 2*x)
>      + 2*f(2*y)*f(y + x)*f(z + y)*f(a + 2*z)*f(a + z + x) -
>      2*f(2*y)*f(y
>      + x)*f(z + y)*f(a + 2*x)*f(c + 2*z) + 2*f(2*y)*f(y + x)
>      *f(z + x)*f(c
>      + 2*z)*f(a + y + x) + 4*f(2*y)*f(y + x)*f(z + x)*f(a +
>      z + x)*f(c +
>      z + y) - 2*f(2*y)*f(y + x)*f(z + x)*f(a + 2*z)*f(c + y +
>      x) - 2*f(2*y
>      )*f(y + x)^2*f(c + 2*z)*f(a + z + x) - f(2*y)^2*f(z + x)
>      *f(c + 2*x)*
>      f(c + z + x) - 2*f(2*y)^2*f(z + x)*f(a + z + x)*f(c + z
>      + x) - 1/2*f(
>      2*y)^2*f(z + x)*f(a + 2*z)*f(c + 2*x) - f(2*y)^2*f(z +
>      x)*f(a + 2*z)*
>      f(a + z + x) + 1/2*f(2*y)^2*f(z + x)*f(a + 2*x)*f(c + 2*
>      z) + f(2*y)^2
>      *f(2*z)*f(c + 2*x)*f(a + z + x) + f(2*y)^2*f(2*z)*f(a +
>      2*x)*f(c + z
>      + x) + 2*f(2*x)*f(z + x)*f(z + y)*f(c + 2*y)*f(c + y +
>      x) + 2*f(2*x)
>      *f(z + x)*f(z + y)*f(c + 2*y)*f(a + z + y) - 2*f(2*x)*f
>      (z + x)*f(z +
>      y)*f(b + 2*y)*f(c + z + x) + f(2*x)*f(z + x)*f(z + y)*f
>      (a + 2*z)*f(b
>      + 2*y) + f(2*x)*f(z + x)*f(z + y)*f(a + 2*y)*f(b + 2*z)
>      - f(2*x)*f(z
>      + x)^2*f(c + 2*y)^2 + 2*f(2*x)*f(z + x)^2*f(b + 2*y)*f
>      (c + z + y) -
>      f(2*x)*f(z + x)^2*f(b + 2*y)*f(b + 2*z) - 2*f(2*x)*f(2*
>      z)*f(z + x)*f(
>      b + 2*y)*f(c + y + x) + 2*f(2*x)*f(2*z)*f(z + x)*f(b +
>      2*y)*f(b + z
>      + x) - 2*f(2*x)*f(2*z)*f(z + x)*f(b + 2*y)*f(a + z + y)

```

```

- f(2*x)*f(y
> + x)*f(z + x)*f(b + 2*z)*f(c + 2*y) + f(2*x)*f(y + x)*f
(z + x)*f(b
> + 2*y)*f(c + 2*z) + f(2*x)*f(2*y)*f(z + y)*f(c + 2*z)*f
(a + y + x)
> - 2*f(2*x)*f(2*y)*f(z + y)*f(c + y + x)*f(c + z + x) +
2*f(2*x)*f(2*
> y)*f(z + y)*f(b + z + x)*f(c + z + x) - f(2*x)*f(2*y)*f
(z + y)*f(b +
> 2*z)*f(c + 2*x) - f(2*x)*f(2*y)*f(z + y)*f(b + 2*z)*f(a
+ z + x) + f(
> 2*x)*f(2*y)*f(z + y)*f(b + 2*x)*f(c + 2*z) - 2*f(2*x)*f
(2*y)*f(z + y)
> *f(a + z + x)*f(c + z + y) - f(2*x)*f(2*y)*f(z + y)*f(a
+ 2*z)*f(c +
> y + x) - f(2*x)*f(2*y)*f(z + y)*f(a + 2*z)*f(b + z + x)
- 2*f(2*x)*f(
> 2*y)*f(z + x)*f(c + 2*z)*f(b + y + x) + f(2*x)*f(2*y)*f
(z + x)*f(c +
> 2*y)*f(c + z + x) - 2*f(2*x)*f(2*y)*f(z + x)*f(b + z +
x)*f(c + z + y
> ) + 2*f(2*x)*f(2*y)*f(z + x)*f(b + 2*z)*f(c + y + x) + f
(2*x)*f(2*y)*
> f(z + x)*f(b + 2*z)*f(b + z + x) - 1/2*f(2*x)*f(2*y)*f(z
+ x)*f(a + 2
> *z)*f(c + 2*y) - 3/2*f(2*x)*f(2*y)*f(z + x)*f(a + 2*y)*f
(c + 2*z) +
> f(2*x)*f(2*y)*f(2*z)*f(c + 2*x)*f(b + z + y) - 2*f(2*x)*
f(2*y)*f(2*z)
> *f(b + z + x)^2 - f(2*x)*f(2*y)*f(2*z)*f(b + 2*z)*f(a +
y + x) + 2*f(
> 2*x)*f(2*y)*f(2*z)*f(b + y + x)*f(c + z + x) - f(2*x)*f
(2*y)*f(2*z)*
> f(b + 2*x)*f(c + z + y) + 2*f(2*x)*f(2*y)*f(2*z)*f(a + z
+ x)*f(b + z
> + y) + f(2*x)*f(2*y)*f(2*z)*f(a + 2*z)*f(b + y + x) + f
(2*x)*f(2*y)*
> f(y + x)*f(c + 2*z)*f(b + z + x) + f(2*x)*f(2*y)*f(y +
x)*f(c + 2*z)*
> f(a + z + y) - f(2*x)*f(2*y)*f(y + x)*f(b + 2*z)*f(c + z
+ x) - f(2*x
> )*f(2*y)*f(y + x)*f(a + 2*z)*f(c + z + y) + f(2*x)*f(2*
y)^2*f(c + 2*z
> )*f(a + z + x) + f(2*x)*f(2*y)^2*f(a + 2*z)*f(c + z + x)
- f(2*x)^2*
> f(2*y)*f(c + 2*z)*f(b + z + y) + f(2*x)^2*f(2*y)*f(b +
2*z)*f(c + z
> + y) )
>
> + 2*f(z + x)*f(c + a + 2*y) - 2*f(2*y)*f(c + a + z + x):
>
> eq[25] :=
> (1/HessUniv) * ( 8*f(y + x)*f(z + y)^2*f(b + 2*y)*f(a + y + x) -
4*f(
> y + x)*f(z + y)^2*f(a + 2*y)*f(b + y + x) - 2*f(y + x)*f
(z + y)^2*f(a
> + 2*y)^2 + 4*f(y + x)*f(z + x)*f(z + y)*f(b + 2*y)*f(b

```

```

+ y + x) + 2*
> f(y + x)*f(z + x)^2*f(b + 2*y)^2 + 4*f(y + x)^2*f(z + y)
*f(c + 2*y)*
> f(b + y + x) - 8*f(y + x)^2*f(z + y)*f(b + 2*y)*f(c + y
+ x) - 8*f(y
> + x)^2*f(z + y)*f(b + 2*y)*f(a + z + y) + 4*f(y + x)^2*
f(z + y)*f(a
> + 2*y)*f(c + 2*y) + 4*f(y + x)^2*f(z + y)*f(a + 2*y)*f
(b + z + y) -
> 4*f(y + x)^2*f(z + x)*f(b + 2*y)*f(b + z + y) - 2*f(y +
x)^3*f(c + 2*
> y)^2 - 4*f(y + x)^3*f(c + 2*y)*f(b + z + y) + 8*f(y + x)
^3*f(b + 2*y)
> *f(c + z + y) - 4*f(2*y)*f(z + y)^2*f(a + y + x)*f(b + y
+ x) + 2*f(2
> *y)*f(z + y)^2*f(a + 2*y)*f(b + 2*x) + 2*f(2*y)*f(z + y)
^2*f(a + 2*y)
> *f(a + y + x) - 2*f(2*y)*f(z + y)^2*f(a + 2*x)*f(b + 2*
y) + 4*f(2*y)*
> f(z + x)*f(z + y)*f(b + y + x)^2 - 2*f(2*y)*f(z + x)*f(z
+ y)*f(b + 2
> *y)*f(a + y + x) + 2*f(2*y)*f(z + x)*f(z + y)*f(a + 2*y)
*f(b + y + x)
> - 6*f(2*y)*f(z + x)^2*f(b + 2*y)*f(b + y + x) - 4*f(2*
y)*f(2*z)*f(y
> + x)*f(b + y + x)^2 - 2*f(2*y)*f(2*z)*f(y + x)*f(b + 2*
y)*f(a + y +
> x) - f(2*y)*f(2*z)*f(y + x)*f(b + 2*x)*f(b + 2*y) + f(2*
y)*f(2*z)*f(y
> + x)*f(a + 2*y)^2 - 6*f(2*y)*f(y + x)*f(z + y)*f(c + 2*
y)*f(a + y +
> x) + 4*f(2*y)*f(y + x)*f(z + y)*f(b + y + x)*f(c + y +
x) + 4*f(2*y)*
> f(y + x)*f(z + y)*f(b + 2*y)*f(c + 2*x) - 2*f(2*y)*f(y +
x)*f(z + y)*
> f(b + 2*x)*f(c + 2*y) + 8*f(2*y)*f(y + x)*f(z + y)*f(a +
z + y)*f(b
> + y + x) - 4*f(2*y)*f(y + x)*f(z + y)*f(a + y + x)*f(b
+ z + y) - 2*
> f(2*y)*f(y + x)*f(z + y)*f(a + 2*y)*f(b + z + x) + 2*f
(2*y)*f(y + x)*
> f(z + y)*f(a + 2*y)*f(a + z + y) - 2*f(2*y)*f(y + x)*f(z
+ x)*f(c + 2
> *y)*f(b + y + x) + 4*f(2*y)*f(y + x)*f(z + x)*f(b + y +
x)*f(b + z +
> y) + 4*f(2*y)*f(y + x)*f(z + x)*f(b + 2*y)*f(c + y + x)
+ 2*f(2*y)*f(
> y + x)*f(z + x)*f(b + 2*y)*f(b + z + x) + 2*f(2*y)*f(y +
x)*f(z + x)*
> f(b + 2*y)*f(a + z + y) - 2*f(2*y)*f(y + x)*f(z + x)*f(a
+ 2*y)*f(c
> + 2*y) + 4*f(2*y)*f(y + x)^2*f(c + 2*y)*f(c + y + x) +
2*f(2*y)*f(y
> + x)^2*f(c + 2*y)*f(b + z + x) + 2*f(2*y)*f(y + x)^2*f
(c + 2*y)*f(a
> + z + y) + 4*f(2*y)*f(y + x)^2*f(b + z + y)*f(c + y +
x) - 8*f(2*y)*

```

```

>      f(y + x)^2*f(b + y + x)*f(c + z + y) - 4*f(2*y)*f(y + x)
>      ^2*f(b + 2*y)
>      *f(c + z + x) + 2*f(2*y)*f(y + x)^2*f(a + 2*z)*f(b + 2*
>      y) - 4*f(2*y)*
>      f(y + x)^2*f(a + 2*y)*f(c + z + y) - 2*f(2*y)^2*f(z + y)
>      *f(c + 2*x)*
>      f(b + y + x) - 2*f(2*y)^2*f(z + y)*f(b + 2*x)*f(a + z +
>      y) + 2*f(2*y)
>      ^2*f(z + y)*f(a + y + x)*f(c + y + x) + 2*f(2*y)^2*f(z +
>      y)*f(a + y
>      + x)*f(b + z + x) - 2*f(2*y)^2*f(z + y)*f(a + y + x)*f
>      (a + z + y) -
>      f(2*y)^2*f(z + y)*f(a + 2*y)*f(c + 2*x) + f(2*y)^2*f(z +
>      y)*f(a + 2*x
>      )*f(c + 2*y) + 2*f(2*y)^2*f(z + y)*f(a + 2*x)*f(b + z +
>      y) + 2*f(2*y)
>      ^2*f(z + x)*f(c + 2*y)*f(a + y + x) - 2*f(2*y)^2*f(z +
>      x)*f(b + y + x
>      )*f(c + y + x) - 2*f(2*y)^2*f(z + x)*f(b + y + x)*f(b +
>      z + x) - f(2*
>      y)^2*f(z + x)*f(b + 2*y)*f(c + 2*x) + f(2*y)^2*f(z + x)*
>      f(b + 2*x)*f(
>      c + 2*y) - 2*f(2*y)^2*f(z + x)*f(a + z + y)*f(b + y + x)
>      + f(2*y)^2*
>      f(2*z)*f(b + 2*x)*f(b + y + x) + 2*f(2*y)^2*f(2*z)*f(a +
>      y + x)*f(b
>      + y + x) - 1/2*f(2*y)^2*f(2*z)*f(a + 2*y)*f(b + 2*x) -
>      f(2*y)^2*f(2*
>      z)*f(a + 2*y)*f(a + y + x) + 1/2*f(2*y)^2*f(2*z)*f(a +
>      2*x)*f(b + 2*y
>      ) - 2*f(2*y)^2*f(y + x)*f(c + y + x)^2 - f(2*y)^2*f(y +
>      x)*f(c + 2*x)
>      *f(c + 2*y) - 2*f(2*y)^2*f(y + x)*f(c + 2*x)*f(b + z +
>      y) - 2*f(2*y)^
>      2*f(y + x)*f(b + z + x)*f(c + y + x) + 4*f(2*y)^2*f(y +
>      x)*f(b + y +
>      x)*f(c + z + x) + 2*f(2*y)^2*f(y + x)*f(b + 2*x)*f(c + z
>      + y) - 2*f(2
>      *y)^2*f(y + x)*f(a + z + y)*f(c + y + x) - 2*f(2*y)^2*f
>      (y + x)*f(a +
>      2*z)*f(b + y + x) + 4*f(2*y)^2*f(y + x)*f(a + y + x)*f(c
>      + z + y) + 2
>      *f(2*y)^2*f(y + x)*f(a + 2*y)*f(c + z + x) - f(2*y)^2*f
>      (y + x)*f(a +
>      2*y)*f(a + 2*z) + f(2*y)^3*f(c + 2*x)*f(c + y + x) + f
>      (2*y)^3*f(c + 2
>      *x)*f(b + z + x) + f(2*y)^3*f(c + 2*x)*f(a + z + y) - f
>      (2*y)^3*f(b +
>      2*x)*f(c + z + x) + 1/2*f(2*y)^3*f(a + 2*z)*f(b + 2*x) +
>      f(2*y)^3*f(a
>      + 2*z)*f(a + y + x) - 2*f(2*y)^3*f(a + y + x)*f(c + z +
>      x) - f(2*y)^
>      3*f(a + 2*x)*f(c + z + y) - 1/2*f(2*y)^3*f(a + 2*x)*f(b
>      + 2*z) - 4*f(
>      2*x)*f(z + y)^2*f(b + 2*y)*f(b + y + x) - 2*f(2*x)*f(2*
>      z)*f(y + x)*f(
>      b + 2*y)^2 + 4*f(2*x)*f(y + x)*f(z + y)*f(b + 2*y)*f(b +

```

```

z + y) - 4*
>      f(2*x)*f(2*y)*f(z + y)*f(b + y + x)*f(b + z + y) + 2*f
(2*x)*f(2*y)*f(
>      z + y)*f(b + 2*y)*f(a + z + y) - 2*f(2*x)*f(2*y)*f(z +
y)*f(a + 2*y)*
>      f(b + z + y) + 6*f(2*x)*f(2*y)*f(2*z)*f(b + 2*y)*f(b + y
+ x) + f(2*x
>      )*f(2*y)*f(y + x)*f(c + 2*y)^2 + 2*f(2*x)*f(2*y)*f(y +
x)*f(c + 2*y)*
>      f(b + z + y) - 4*f(2*x)*f(2*y)*f(y + x)*f(b + 2*y)*f(c +
z + y) - f(2
>      *x)*f(2*y)*f(y + x)*f(b + 2*y)*f(b + 2*z) - f(2*x)*f(2*
y)^2*f(c + 2*y
>      )*f(c + y + x) - f(2*x)*f(2*y)^2*f(c + 2*y)*f(b + z + x)
- f(2*x)*f(2
>      *y)^2*f(c + 2*y)*f(a + z + y) + f(2*x)*f(2*y)^2*f(b + 2*
z)*f(b + y +
>      x) + 2*f(2*x)*f(2*y)^2*f(b + y + x)*f(c + z + y) + f(2*
x)*f(2*y)^2*f(
>      b + 2*y)*f(c + z + x) - 1/2*f(2*x)*f(2*y)^2*f(a + 2*z)*f
(b + 2*y) +
>      f(2*x)*f(2*y)^2*f(a + 2*y)*f(c + z + y) + 1/2*f(2*x)*f
(2*y)^2*f(a + 2
>      *y)*f(b + 2*z) )

>      - 4*f(b + 2*y)*f(b + y + x) + 2*f(y + x)*f(2*b + 2*y) - 2*
f(2*y)*f(2*b
>      + y + x):

> eq[26] :=
> (1/HessUniv) * ( 2*f(y + x)*f(z + y)^2*f(a + 2*x)*f(b + 2*y) + 4*
f(y
>      + x)*f(z + x)*f(z + y)*f(b + 2*y)*f(a + y + x) + 2*f(y
+ x)*f(z + x)
>      ^2*f(a + 2*y)*f(b + 2*y) - 4*f(y + x)^2*f(z + y)*f(b +
2*y)*f(a + z
>      + x) - 4*f(y + x)^2*f(z + x)*f(b + 2*y)*f(a + z + y) +
2*f(y + x)^3*
>      f(a + 2*z)*f(b + 2*y) - 2*f(2*y)*f(z + y)^2*f(a + 2*x)*f
(b + y + x)
>      + 2*f(2*y)*f(z + x)*f(z + y)*f(b + 2*x)*f(b + y + x) +
2*f(2*y)*f(z
>      + x)*f(z + y)*f(a + 2*y)*f(b + 2*x) + 2*f(2*y)*f(z + x)
*f(z + y)*f(a
>      + 2*y)*f(a + y + x) - 2*f(2*y)*f(z + x)*f(z + y)*f(a +
2*x)*f(b + 2*
>      y) - 2*f(2*y)*f(z + x)^2*f(b + 2*y)*f(a + y + x) - f(2*
y)*f(z + x)^2*
>      f(b + 2*x)*f(b + 2*y) - 2*f(2*y)*f(z + x)^2*f(a + 2*y)*f
(b + y + x)
>      - f(2*y)*f(z + x)^2*f(a + 2*y)^2 - f(2*y)*f(2*z)*f(y +
x)*f(b + 2*x)
>      *f(b + y + x) - 2*f(2*y)*f(2*z)*f(y + x)*f(a + y + x)*f
(b + y + x) -
>      3/2*f(2*y)*f(2*z)*f(y + x)*f(a + 2*y)*f(b + 2*x) - f(2*
y)*f(2*z)*f(y
>      + x)*f(a + 2*y)*f(a + y + x) - 1/2*f(2*y)*f(2*z)*f(y +

```

```

x)*f(a + 2*x)
>      *f(b + 2*y) + 4*f(2*y)*f(y + x)*f(z + y)*f(a + z + x)*f
(b + y + x) +
>      f(2*y)*f(y + x)*f(z + y)*f(a + 2*y)*f(c + 2*x) - f(2*y)*
f(y + x)*f(z
>      + y)*f(a + 2*x)*f(c + 2*y) - 2*f(2*y)*f(y + x)*f(z + x)
*f(c + 2*y)*
>      f(a + y + x) + f(2*y)*f(y + x)*f(z + x)*f(b + 2*y)*f(c +
2*x) + 2*f(2
>      *y)*f(y + x)*f(z + x)*f(b + 2*y)*f(a + z + x) + f(2*y)*f
(y + x)*f(z
>      + x)*f(b + 2*x)*f(c + 2*y) + 4*f(2*y)*f(y + x)*f(z + x)
*f(a + z + y)
>      *f(b + y + x) + 2*f(2*y)*f(y + x)*f(z + x)*f(a + 2*y)*f
(a + z + y) +
>      2*f(2*y)*f(y + x)^2*f(c + 2*y)*f(a + z + x) - f(2*y)*f(y
+ x)^2*f(c
>      + 2*x)*f(c + 2*y) - 2*f(2*y)*f(y + x)^2*f(a + 2*z)*f(b
+ y + x) - f(
>      2*y)*f(y + x)^2*f(a + 2*y)*f(a + 2*z) - f(2*y)^2*f(z +
y)*f(c + 2*x)*
>      f(a + y + x) - f(2*y)^2*f(z + y)*f(b + 2*x)*f(a + z + x)
+ f(2*y)^2*
>      f(z + y)*f(a + 2*x)*f(c + y + x) + f(2*y)^2*f(z + y)*f(a
+ 2*x)*f(b
>      + z + x) - f(2*y)^2*f(z + x)*f(c + 2*x)*f(b + y + x) -
f(2*y)^2*f(z
>      + x)*f(b + 2*x)*f(c + y + x) - f(2*y)^2*f(z + x)*f(b +
2*x)*f(a + z
>      + y) - 2*f(2*y)^2*f(z + x)*f(a + z + x)*f(b + y + x) +
2*f(2*y)^2*f(
>      z + x)*f(a + y + x)*f(c + y + x) - 2*f(2*y)^2*f(z + x)*f
(a + y + x)*
>      f(a + z + y) - f(2*y)^2*f(z + x)*f(a + 2*y)*f(c + 2*x) +
f(2*y)^2*f(z
>      + x)*f(a + 2*x)*f(c + 2*y) + f(2*y)^2*f(z + x)*f(a + 2*
x)*f(b + z +
>      y) + f(2*y)^2*f(2*z)*f(b + 2*x)*f(a + y + x) + f(2*y)^2*
f(2*z)*f(a +
>      2*x)*f(b + y + x) + f(2*y)^2*f(y + x)*f(c + 2*x)*f(c + y
+ x) - 2*f(2
>      *y)^2*f(y + x)*f(a + z + x)*f(c + y + x) + 1/2*f(2*y)^2*
f(y + x)*f(a
>      + 2*z)*f(b + 2*x) + f(2*y)^2*f(y + x)*f(a + 2*z)*f(a +
y + x) - 1/2*
>      f(2*y)^2*f(y + x)*f(a + 2*x)*f(b + 2*z) + f(2*y)^3*f(c +
2*x)*f(a + z
>      + x) - f(2*y)^3*f(a + 2*x)*f(c + z + x) - f(2*x)*f(z +
y)^2*f(b + 2*
>      x)*f(b + 2*y) - 2*f(2*x)*f(z + y)^2*f(a + 2*y)*f(b + y +
x) - f(2*x)*
>      f(z + y)^2*f(a + 2*y)^2 - 2*f(2*x)*f(2*z)*f(y + x)*f(a +
2*y)*f(b + 2
>      *y) + 2*f(2*x)*f(y + x)*f(z + y)*f(c + 2*y)*f(b + y + x)
- 4*f(2*x)*
>      f(y + x)*f(z + y)*f(b + 2*y)*f(c + y + x) + 2*f(2*x)*f(y
+ x)*f(z + y

```



```

> )*f(b + 2*y)*f(b + z + x) + 2*f(2*x)*f(y + x)*f(z + y)*f
(a + 2*y)*f(c
> + 2*y) + 2*f(2*x)*f(y + x)*f(z + y)*f(a + 2*y)*f(b + z
+ y) - f(2*x)
> *f(y + x)^2*f(c + 2*y)^2 - 2*f(2*x)*f(y + x)^2*f(c + 2*
y)*f(b + z + y
> ) + 4*f(2*x)*f(y + x)^2*f(b + 2*y)*f(c + z + y) - f(2*x)
*f(y + x)^2*
> f(b + 2*y)*f(b + 2*z) - f(2*x)*f(2*y)*f(z + y)*f(c + 2*
y)*f(a + y + x
> ) + 2*f(2*x)*f(2*y)*f(z + y)*f(b + y + x)*f(c + y + x) -
2*f(2*x)*f(2
> *y)*f(z + y)*f(b + y + x)*f(b + z + x) + f(2*x)*f(2*y)*f
(z + y)*f(b
> + 2*y)*f(c + 2*x) + f(2*x)*f(2*y)*f(z + y)*f(b + 2*y)*f
(a + z + x)
> - f(2*x)*f(2*y)*f(z + y)*f(b + 2*x)*f(c + 2*y) - 2*f(2*
x)*f(2*y)*f(z
> + y)*f(a + y + x)*f(b + z + y) - f(2*x)*f(2*y)*f(z + y)
*f(a + 2*y)*
> f(c + y + x) - f(2*x)*f(2*y)*f(z + y)*f(a + 2*y)*f(b + z
+ x) - f(2*x
> )*f(2*y)*f(z + x)*f(c + 2*y)*f(b + y + x) + f(2*x)*f(2*
y)*f(z + x)*f(
> b + 2*y)*f(c + y + x) + f(2*x)*f(2*y)*f(z + x)*f(b + 2*
y)*f(a + z + y
> ) - f(2*x)*f(2*y)*f(z + x)*f(a + 2*y)*f(b + z + y) + f
(2*x)*f(2*y)*f(
> 2*x)*f(b + 2*y)*f(a + y + x) + f(2*x)*f(2*y)*f(2*z)*f(b
+ 2*x)*f(b +
> 2*y) + 3*f(2*x)*f(2*y)*f(2*z)*f(a + 2*y)*f(b + y + x) +
f(2*x)*f(2*y)
> *f(2*z)*f(a + 2*y)^2 + 3*f(2*x)*f(2*y)*f(y + x)*f(c + 2*
y)*f(c + y +
> x) + 2*f(2*x)*f(2*y)*f(y + x)*f(b + z + y)*f(c + y + x)
+ f(2*x)*f(2*
> y)*f(y + x)*f(b + 2*z)*f(b + y + x) - 4*f(2*x)*f(2*y)*f
(y + x)*f(b +
> y + x)*f(c + z + y) - 2*f(2*x)*f(2*y)*f(y + x)*f(b + 2*
y)*f(c + z + x
> ) - 1/2*f(2*x)*f(2*y)*f(y + x)*f(a + 2*z)*f(b + 2*y) -
2*f(2*x)*f(2*y
> )*f(y + x)*f(a + 2*y)*f(c + z + y) + 1/2*f(2*x)*f(2*y)*f
(y + x)*f(a
> + 2*y)*f(b + 2*z) - 2*f(2*x)*f(2*y)^2*f(c + y + x)^2 -
f(2*x)*f(2*y)
> ^2*f(c + 2*y)*f(a + z + x) - f(2*x)*f(2*y)^2*f(c + 2*x)*
f(b + z + y)
> + 2*f(2*x)*f(2*y)^2*f(b + y + x)*f(c + z + x) + f(2*x)*
f(2*y)^2*f(b
> + 2*x)*f(c + z + y) + 2*f(2*x)*f(2*y)^2*f(a + y + x)*f
(c + z + y) +
> f(2*x)*f(2*y)^2*f(a + 2*y)*f(c + z + x) + f(2*x)^2*f(2*
y)*f(c + 2*y)*
> f(b + z + y) - f(2*x)^2*f(2*y)*f(b + 2*y)*f(c + z + y) )
>
> - f(b + 2*x)*f(b + 2*y) - 2*f(a + 2*y)*f(b + y + x) - f(a

```

```

+ 2*y)^2 + 2*
> f(y + x)*f(b + a + 2*y) - 2*f(2*y)*f(b + a + y + x):
> eq[27] :=
> (1/HessUniv) * ( 2*f(y + x)*f(z + y)^2*f(a + 2*x)*f(a + 2*y) - 2*
f(y
> + x)*f(z + x)*f(z + y)*f(a + 2*y)*f(b + 2*x) + 4*f(y +
x)*f(z + x)*
> f(z + y)*f(a + 2*y)*f(a + y + x) + 2*f(y + x)*f(z + x)*f
(z + y)*f(a
> + 2*x)*f(b + 2*y) + 4*f(y + x)*f(z + x)^2*f(b + 2*y)*f
(a + y + x) -
> 2*f(y + x)*f(z + x)^2*f(b + 2*x)*f(b + 2*y) + 2*f(y + x)
^2*f(z + y)*
> f(a + 2*y)*f(c + 2*x) - 4*f(y + x)^2*f(z + y)*f(a + 2*y)
*f(a + z + x)
> - 2*f(y + x)^2*f(z + y)*f(a + 2*x)*f(c + 2*y) - 4*f(y +
x)^2*f(z + x
> )*f(c + 2*y)*f(a + y + x) + 2*f(y + x)^2*f(z + x)*f(b +
2*y)*f(c + 2*
> x) - 4*f(y + x)^2*f(z + x)*f(b + 2*y)*f(a + z + x) + 2*f
(y + x)^2*f(z
> + x)*f(b + 2*x)*f(c + 2*y) + 4*f(y + x)^3*f(c + 2*y)*f
(a + z + x) -
> 2*f(y + x)^3*f(c + 2*x)*f(c + 2*y) - 2*f(2*y)*f(z + y)
^2*f(a + 2*x)*
> f(a + y + x) + 2*f(2*y)*f(z + x)*f(z + y)*f(b + 2*x)*f(a
+ y + x) + 4
> *f(2*y)*f(z + x)*f(z + y)*f(a + y + x)^2 - 2*f(2*y)*f(z
+ x)*f(z + y)
> *f(a + 2*x)*f(b + y + x) + 2*f(2*y)*f(z + x)^2*f(b + 2*
x)*f(b + y + x
> ) - 4*f(2*y)*f(z + x)^2*f(a + y + x)*f(b + y + x) + 2*f
(2*y)*f(z + x)
> ^2*f(a + 2*y)*f(b + 2*x) - 4*f(2*y)*f(z + x)^2*f(a + 2*
y)*f(a + y + x
> ) - 2*f(2*y)*f(z + x)^2*f(a + 2*x)*f(b + 2*y) - 4*f(2*y)
*f(2*z)*f(y
> + x)*f(a + y + x)^2 - 2*f(2*y)*f(2*z)*f(y + x)*f(a + 2*
x)*f(a + 2*y)
> - 2*f(2*y)*f(y + x)*f(z + y)*f(c + 2*x)*f(a + y + x) +
4*f(2*y)*f(y
> + x)*f(z + y)*f(a + y + x)*f(a + z + x) + 2*f(2*y)*f(y
+ x)*f(z + y)
> *f(a + 2*x)*f(c + y + x) - 2*f(2*y)*f(y + x)*f(z + x)*f
(c + 2*x)*f(b
> + y + x) - 2*f(2*y)*f(y + x)*f(z + x)*f(b + 2*x)*f(c +
y + x) + 4*f(
> 2*y)*f(y + x)*f(z + x)*f(a + z + x)*f(b + y + x) + 4*f
(2*y)*f(y + x)*
> f(z + x)*f(a + y + x)*f(c + y + x) - 2*f(2*y)*f(y + x)*f
(z + x)*f(a
> + 2*y)*f(c + 2*x) + 4*f(2*y)*f(y + x)*f(z + x)*f(a + 2*
y)*f(a + z +
> x) + 2*f(2*y)*f(y + x)*f(z + x)*f(a + 2*x)*f(c + 2*y) +
2*f(2*y)*f(y
> + x)^2*f(c + 2*x)*f(c + y + x) - 4*f(2*y)*f(y + x)^2*f

```

```

(a + z + x)*f(
>      c + y + x) - 2*f(2*y)^2*f(z + x)*f(b + 2*x)*f(a + z + x)
- 4*f(2*y)^2
>      *f(z + x)*f(a + y + x)*f(a + z + x) + 2*f(2*y)^2*f(z +
x)*f(a + 2*x)*
>      f(b + z + x) + 2*f(2*y)^2*f(2*z)*f(a + 2*x)*f(a + y + x)
+ 2*f(2*y)^2
>      *f(y + x)*f(c + 2*x)*f(a + z + x) - 2*f(2*y)^2*f(y + x)*
f(a + 2*x)*f(
>      c + z + x) - 4*f(2*x)*f(z + y)^2*f(a + 2*y)*f(a + y + x)
- 2*f(2*x)*
>      f(2*z)*f(y + x)*f(b + 2*y)*f(a + y + x) + f(2*x)*f(2*z)*
f(y + x)*f(b
>      + 2*x)*f(b + 2*y) - f(2*x)*f(2*z)*f(y + x)*f(a + 2*y)^2
+ 4*f(2*x)*
>      f(y + x)*f(z + y)*f(c + 2*y)*f(a + y + x) - 2*f(2*x)*f(y
+ x)*f(z + y
>      )*f(b + 2*y)*f(c + 2*x) - 2*f(2*x)*f(y + x)*f(z + y)*f(a
+ 2*y)*f(c
>      + y + x) + 2*f(2*x)*f(y + x)*f(z + y)*f(a + 2*y)*f(b +
z + x) + 2*f(
>      2*x)*f(y + x)*f(z + y)*f(a + 2*y)*f(a + z + y) - 2*f(2*
x)*f(y + x)*f(
>      z + x)*f(b + 2*y)*f(c + y + x) + 2*f(2*x)*f(y + x)*f(z +
x)*f(b + 2*y
>      )*f(b + z + x) - 2*f(2*x)*f(y + x)*f(z + x)*f(b + 2*y)*f
(a + z + y)
>      + 2*f(2*x)*f(y + x)*f(z + x)*f(a + 2*y)*f(c + 2*y) + 2*
f(2*x)*f(y +
>      x)^2*f(c + 2*y)*f(c + y + x) - 2*f(2*x)*f(y + x)^2*f(c +
2*y)*f(b + z
>      + x) - 2*f(2*x)*f(y + x)^2*f(c + 2*y)*f(a + z + y) + 2*
f(2*x)*f(y +
>      x)^2*f(a + 2*z)*f(b + 2*y) + 2*f(2*x)*f(2*y)*f(z + y)*f
(c + 2*x)*f(b
>      + y + x) - 2*f(2*x)*f(2*y)*f(z + y)*f(a + y + x)*f(c +
y + x) - 2*f(
>      2*x)*f(2*y)*f(z + y)*f(a + y + x)*f(b + z + x) - 2*f(2*
x)*f(2*y)*f(z
>      + y)*f(a + y + x)*f(a + z + y) + f(2*x)*f(2*y)*f(z + y)
*f(a + 2*y)*
>      f(c + 2*x) - f(2*x)*f(2*y)*f(z + y)*f(a + 2*x)*f(c + 2*
y) - 2*f(2*x)*
>      f(2*y)*f(z + x)*f(c + 2*y)*f(a + y + x) + 2*f(2*x)*f(2*
y)*f(z + x)*f(
>      b + y + x)*f(c + y + x) - 2*f(2*x)*f(2*y)*f(z + x)*f(b +
y + x)*f(b
>      + z + x) + f(2*x)*f(2*y)*f(z + x)*f(b + 2*y)*f(c + 2*x)
+ 2*f(2*x)*
>      f(2*y)*f(z + x)*f(b + 2*y)*f(a + z + x) - f(2*x)*f(2*y)*
f(z + x)*f(b
>      + 2*x)*f(c + 2*y) + 2*f(2*x)*f(2*y)*f(z + x)*f(a + z +
y)*f(b + y +
>      x) - 2*f(2*x)*f(2*y)*f(z + x)*f(a + 2*y)*f(b + z + x) -
f(2*x)*f(2*y)
>      *f(2*z)*f(b + 2*x)*f(b + y + x) + 2*f(2*x)*f(2*y)*f(2*z)
*f(a + y + x)

```

```

>      *f(b + y + x) - 1/2*f(2*x)*f(2*y)*f(2*z)*f(a + 2*y)*f(b
+ 2*x) + 5*f(
>      2*x)*f(2*y)*f(2*z)*f(a + 2*y)*f(a + y + x) + 1/2*f(2*x)*
f(2*y)*f(2*z)
>      *f(a + 2*x)*f(b + 2*y) - 2*f(2*x)*f(2*y)*f(y + x)*f(c +
y + x)^2 - 2*
>      f(2*x)*f(2*y)*f(y + x)*f(c + 2*y)*f(a + z + x) + f(2*x)*
f(2*y)*f(y +
>      x)*f(c + 2*x)*f(c + 2*y) + 2*f(2*x)*f(2*y)*f(y + x)*f(b
+ z + x)*f(c
>      + y + x) + 2*f(2*x)*f(2*y)*f(y + x)*f(a + z + y)*f(c +
y + x) - 2*f(
>      2*x)*f(2*y)*f(y + x)*f(a + 2*z)*f(b + y + x) - f(2*x)*f
(2*y)*f(y + x)
>      *f(a + 2*y)*f(a + 2*z) - f(2*x)*f(2*y)^2*f(c + 2*x)*f(c
+ y + x) - f(
>      2*x)*f(2*y)^2*f(c + 2*x)*f(b + z + x) - f(2*x)*f(2*y)^2*
f(c + 2*x)*f(
>      a + z + y) + f(2*x)*f(2*y)^2*f(b + 2*x)*f(c + z + x) +
1/2*f(2*x)*f(2
>      *y)^2*f(a + 2*z)*f(b + 2*x) + f(2*x)*f(2*y)^2*f(a + 2*z)
*f(a + y + x)
>      + 2*f(2*x)*f(2*y)^2*f(a + y + x)*f(c + z + x) + f(2*x)*
f(2*y)^2*f(a
>      + 2*x)*f(c + z + y) - 1/2*f(2*x)*f(2*y)^2*f(a + 2*x)*f
(b + 2*z) - f(
>      2*x)^2*f(y + x)*f(c + 2*y)^2 + 2*f(2*x)^2*f(y + x)*f(b +
2*y)*f(c + z
>      + y) - f(2*x)^2*f(y + x)*f(b + 2*y)*f(b + 2*z) + f(2*x)
^2*f(2*y)*f(c
>      + 2*y)*f(c + y + x) + f(2*x)^2*f(2*y)*f(c + 2*y)*f(b +
z + x) + f(2*
>      x)^2*f(2*y)*f(c + 2*y)*f(a + z + y) + f(2*x)^2*f(2*y)*f
(b + 2*z)*f(b
>      + y + x) - 2*f(2*x)^2*f(2*y)*f(b + y + x)*f(c + z + y)
- f(2*x)^2*f(
>      2*y)*f(b + 2*y)*f(c + z + x) - 1/2*f(2*x)^2*f(2*y)*f(a +
2*z)*f(b + 2
>      *y) - f(2*x)^2*f(2*y)*f(a + 2*y)*f(c + z + y) + 1/2*f(2*
x)^2*f(2*y)*
>      f(a + 2*y)*f(b + 2*z) )

>      - 4*f(a + 2*y)*f(a + y + x) + 2*f(y + x)*f(2*a + 2*y) - 2*
f(2*y)*f(2*a
>      + y + x):

> eq[28] :=
> (1/HessUniv) * ( - 2*f(2*y)*f(z + y)^2*f(a + 2*x)*f(b + y + x) +
f(2
>      *y)*f(z + y)^2*f(a + 2*x)*f(a + 2*y) + 2*f(2*y)*f(z + x)
*f(z + y)*f(b
>      + 2*x)*f(b + y + x) + f(2*y)*f(z + x)*f(z + y)*f(a + 2*
y)*f(b + 2*x)
>      - f(2*y)*f(z + x)*f(z + y)*f(a + 2*x)*f(b + 2*y) - f(2*
y)*f(z + x)^2
>      *f(b + 2*x)*f(b + 2*y) - 2*f(2*y)*f(2*z)*f(y + x)*f(b +
2*x)*f(b + y

```

```

> + x) + 2*f(2*y)*f(y + x)*f(z + y)*f(c + 2*x)*f(b + y +
> x) - f(2*y)*
> f(y + x)*f(z + y)*f(a + 2*y)*f(c + 2*x) - f(2*y)*f(y +
> x)*f(z + y)*f(
> a + 2*x)*f(c + 2*y) + 2*f(2*y)*f(y + x)*f(z + y)*f(a +
> 2*x)*f(b + z
> + y) + f(2*y)*f(y + x)*f(z + x)*f(b + 2*y)*f(c + 2*x) -
> f(2*y)*f(y
> + x)*f(z + x)*f(b + 2*x)*f(c + 2*y) + 2*f(2*y)*f(y + x)
> *f(z + x)*f(b
> + 2*x)*f(b + z + y) + f(2*y)*f(y + x)^2*f(c + 2*x)*f(c
> + 2*y) - 2*f(
> 2*y)*f(y + x)^2*f(c + 2*x)*f(b + z + y) - f(2*y)^2*f(z +
> y)*f(b + 2*x
> )*f(c + 2*x) + f(2*y)^2*f(z + y)*f(a + 2*x)*f(c + y + x)
> + f(2*y)^2*
> f(z + y)*f(a + 2*x)*f(b + z + x) - f(2*y)^2*f(z + y)*f(a
> + 2*x)*f(a
> + z + y) - 2*f(2*y)^2*f(z + x)*f(c + 2*x)*f(b + y + x)
> + f(2*y)^2*f(
> z + x)*f(b + 2*x)*f(c + y + x) - f(2*y)^2*f(z + x)*f(b +
> 2*x)*f(b + z
> + x) - f(2*y)^2*f(z + x)*f(b + 2*x)*f(a + z + y) + f(2*
> y)^2*f(z + x)
> *f(a + 2*x)*f(c + 2*y) + 1/2*f(2*y)^2*f(2*z)*f(b + 2*x)
> ^2 + f(2*y)^2*
> f(2*z)*f(a + 2*x)*f(b + y + x) - 1/2*f(2*y)^2*f(2*z)*f(a
> + 2*x)*f(a
> + 2*y) - f(2*y)^2*f(y + x)*f(c + 2*x)*f(c + y + x) + f
> (2*y)^2*f(y +
> x)*f(c + 2*x)*f(b + z + x) + f(2*y)^2*f(y + x)*f(c + 2*
> x)*f(a + z + y
> ) - f(2*y)^2*f(y + x)*f(a + 2*x)*f(b + 2*z) + 1/2*f(2*y)
> ^3*f(c + 2*x)
> ^2 - f(2*y)^3*f(a + 2*x)*f(c + z + x) + 1/2*f(2*y)^3*f(a
> + 2*x)*f(a
> + 2*z) + 4*f(2*x)*f(z + y)^2*f(b + 2*y)*f(a + y + x) -
> 2*f(2*x)*f(z
> + y)^2*f(a + 2*y)*f(b + y + x) - f(2*x)*f(z + y)^2*f(a
> + 2*y)^2 - 2*
> f(2*x)*f(z + x)*f(z + y)*f(b + 2*y)*f(b + y + x) + f(2*
> x)*f(z + x)^2*
> f(b + 2*y)^2 + 2*f(2*x)*f(2*z)*f(y + x)*f(b + 2*y)*f(b +
> y + x) + 2*
> f(2*x)*f(y + x)*f(z + y)*f(c + 2*y)*f(b + y + x) - 4*f
> (2*x)*f(y + x)*
> f(z + y)*f(b + 2*y)*f(c + y + x) - 4*f(2*x)*f(y + x)*f(z
> + y)*f(b + 2
> *y)*f(a + z + y) + 2*f(2*x)*f(y + x)*f(z + y)*f(a + 2*y)
> *f(c + 2*y)
> + 2*f(2*x)*f(y + x)*f(z + y)*f(a + 2*y)*f(b + z + y) -
> 2*f(2*x)*f(y
> + x)*f(z + x)*f(b + 2*y)*f(b + z + y) - f(2*x)*f(y + x)
> ^2*f(c + 2*y)
> ^2 - 2*f(2*x)*f(y + x)^2*f(c + 2*y)*f(b + z + y) + 4*f
> (2*x)*f(y + x)^
> 2*f(b + 2*y)*f(c + z + y) - 2*f(2*x)*f(2*y)*f(z + y)*f(c

```

```

+ 2*y)*f(a
> + y + x) + f(2*x)*f(2*y)*f(z + y)*f(b + 2*y)*f(c + 2*x)
- 2*f(2*x)*
> f(2*y)*f(z + y)*f(b + 2*x)*f(b + z + y) + 4*f(2*x)*f(2*
y)*f(z + y)*f(
> a + z + y)*f(b + y + x) - 4*f(2*x)*f(2*y)*f(z + y)*f(a +
y + x)*f(b
> + z + y) + f(2*x)*f(2*y)*f(z + y)*f(a + 2*y)*f(c + y +
x) - f(2*x)*
> f(2*y)*f(z + y)*f(a + 2*y)*f(b + z + x) + f(2*x)*f(2*y)*
f(z + y)*f(a
> + 2*y)*f(a + z + y) + f(2*x)*f(2*y)*f(z + x)*f(b + 2*y)
*f(c + y + x)
> + f(2*x)*f(2*y)*f(z + x)*f(b + 2*y)*f(b + z + x) + f(2*
x)*f(2*y)*f(z
> + x)*f(b + 2*y)*f(a + z + y) - f(2*x)*f(2*y)*f(z + x)*f
(a + 2*y)*f(c
> + 2*y) - f(2*x)*f(2*y)*f(2*z)*f(b + 2*y)*f(a + y + x) +
1/2*f(2*x)*
> f(2*y)*f(2*z)*f(b + 2*x)*f(b + 2*y) + 1/2*f(2*x)*f(2*y)*
f(2*z)*f(a +
> 2*y)^2 + f(2*x)*f(2*y)*f(y + x)*f(c + 2*y)*f(c + y + x)
+ f(2*x)*f(2*
> y)*f(y + x)*f(c + 2*y)*f(b + z + x) + f(2*x)*f(2*y)*f(y
+ x)*f(c + 2*
> y)*f(a + z + y) + 4*f(2*x)*f(2*y)*f(y + x)*f(b + z + y)*
f(c + y + x)
> - 4*f(2*x)*f(2*y)*f(y + x)*f(b + y + x)*f(c + z + y) -
2*f(2*x)*f(2*
> y)*f(y + x)*f(b + 2*y)*f(c + z + x) + f(2*x)*f(2*y)*f(y
+ x)*f(a + 2*
> z)*f(b + 2*y) - 2*f(2*x)*f(2*y)*f(y + x)*f(a + 2*y)*f(c
+ z + y) - f(
> 2*x)*f(2*y)^2*f(c + 2*x)*f(c + 2*y) - 2*f(2*x)*f(2*y)^2*
f(b + z + x)*
> f(c + y + x) + f(2*x)*f(2*y)^2*f(b + 2*z)*f(a + y + x) +
2*f(2*x)*f(2
> y)^2*f(b + y + x)*f(c + z + x) + f(2*x)*f(2*y)^2*f(b +
2*x)*f(c + z
> + y) + 1/2*f(2*x)*f(2*y)^2*f(b + 2*x)*f(b + 2*z) - 2*f
(2*x)*f(2*y)^2
> *f(a + z + y)*f(c + y + x) - f(2*x)*f(2*y)^2*f(a + 2*z)*
f(b + y + x)
> + 2*f(2*x)*f(2*y)^2*f(a + y + x)*f(c + z + y) + f(2*x)*
f(2*y)^2*f(a
> + 2*y)*f(c + z + x) - 1/2*f(2*x)*f(2*y)^2*f(a + 2*y)*f
(a + 2*z) + 2*
> f(2*x)^2*f(z + y)*f(b + 2*y)*f(b + z + y) - f(2*x)^2*f
(2*z)*f(b + 2*y
> )^2 + 1/2*f(2*x)^2*f(2*y)*f(c + 2*y)^2 - f(2*x)^2*f(2*y)
*f(b + 2*y)*
> f(c + z + y) - 1/2*f(2*x)^2*f(2*y)*f(b + 2*y)*f(b + 2*z)
)
>
> - f(2*y)*f(2*b + 2*x) + f(2*x)*f(2*b + 2*y):
> eq[29] :=

```

```

> (1/HessUniv) * ( - f(2*y)*f(z + y)^2*f(a + 2*x)*f(b + 2*x) + f
(2*y)*
> f(z + x)*f(z + y)*f(b + 2*x)^2 + 2*f(2*y)*f(z + x)*f(z +
y)*f(b + 2*x
> )*f(a + y + x) - 2*f(2*y)*f(z + x)*f(z + y)*f(a + 2*x)*f
(b + y + x)
> + f(2*y)*f(z + x)*f(z + y)*f(a + 2*x)*f(a + 2*y) - f(2*
y)*f(z + x)^2
> *f(a + 2*x)*f(b + 2*y) - 1/2*f(2*y)*f(2*z)*f(y + x)*f(b
+ 2*x)^2 - f(
> 2*y)*f(2*z)*f(y + x)*f(b + 2*x)*f(a + y + x) - 1/2*f(2*
y)*f(2*z)*f(y
> + x)*f(a + 2*x)*f(a + 2*y) + 2*f(2*y)*f(y + x)*f(z + y)
*f(a + 2*x)*
> f(b + z + x) + 2*f(2*y)*f(y + x)*f(z + x)*f(a + 2*x)*f(b
+ z + y) -
> f(2*y)*f(y + x)^2*f(a + 2*x)*f(b + 2*z) - f(2*y)^2*f(z +
x)*f(c + 2*x
> )*f(a + y + x) - f(2*y)^2*f(z + x)*f(b + 2*x)*f(c + 2*x)
- f(2*y)^2*
> f(z + x)*f(b + 2*x)*f(a + z + x) + 2*f(2*y)^2*f(z + x)*f
(a + 2*x)*f(c
> + y + x) - f(2*y)^2*f(z + x)*f(a + 2*x)*f(a + z + y) +
f(2*y)^2*f(2*
> z)*f(a + 2*x)*f(b + 2*x) + 1/2*f(2*y)^2*f(y + x)*f(c +
2*x)^2 + f(2*y
> )^2*f(y + x)*f(c + 2*x)*f(a + z + x) - 2*f(2*y)^2*f(y +
x)*f(a + 2*x)
> *f(c + z + x) + 1/2*f(2*y)^2*f(y + x)*f(a + 2*x)*f(a +
2*z) + f(2*x)*
> f(z + y)^2*f(a + 2*x)*f(b + 2*y) + 2*f(2*x)*f(z + x)*f(z
+ y)*f(b + 2
> *y)*f(a + y + x) - f(2*x)*f(z + x)*f(z + y)*f(b + 2*x)*f
(b + 2*y) - 2
> *f(2*x)*f(z + x)*f(z + y)*f(a + 2*y)*f(b + y + x) - f(2*
x)*f(z + x)*
> f(z + y)*f(a + 2*y)^2 + f(2*x)*f(z + x)^2*f(a + 2*y)*f(b
+ 2*y) + 1/2
> *f(2*x)*f(2*z)*f(y + x)*f(b + 2*x)*f(b + 2*y) + f(2*x)*f
(2*z)*f(y + x
> )*f(a + 2*y)*f(b + y + x) + 1/2*f(2*x)*f(2*z)*f(y + x)*f
(a + 2*y)^2
> - 2*f(2*x)*f(y + x)*f(z + y)*f(b + 2*y)*f(a + z + x) -
2*f(2*x)*f(y
> + x)*f(z + x)*f(b + 2*y)*f(a + z + y) + f(2*x)*f(y + x)
^2*f(a + 2*z)
> *f(b + 2*y) + f(2*x)*f(2*y)*f(z + y)*f(c + 2*x)*f(b + y
+ x) - f(2*x)
> *f(2*y)*f(z + y)*f(b + 2*x)*f(b + z + x) + 2*f(2*x)*f(2*
y)*f(z + y)*
> f(a + z + x)*f(b + y + x) - 2*f(2*x)*f(2*y)*f(z + y)*f(a
+ y + x)*f(b
> + z + x) - f(2*x)*f(2*y)*f(z + y)*f(a + 2*x)*f(c + 2*y)
- f(2*x)*f(2
> *y)*f(z + y)*f(a + 2*x)*f(b + z + y) - f(2*x)*f(2*y)*f(z
+ x)*f(c + 2
> *y)*f(a + y + x) + f(2*x)*f(2*y)*f(z + x)*f(b + 2*y)*f(c

```

```

+ 2*x) + f(2
>      *x)*f(2*y)*f(z + x)*f(b + 2*y)*f(a + z + x) + 2*f(2*x)*f
(2*y)*f(z + x
>      )*f(a + z + y)*f(b + y + x) - 2*f(2*x)*f(2*y)*f(z + x)*f
(a + y + x)*
>      f(b + z + y) + f(2*x)*f(2*y)*f(z + x)*f(a + 2*y)*f(a + z
+ y) + f(2*x
>      )*f(2*y)*f(y + x)*f(c + 2*y)*f(a + z + x) - f(2*x)*f(2*
y)*f(y + x)*f(
>      c + 2*x)*f(b + z + y) + f(2*x)*f(2*y)*f(y + x)*f(b + 2*
z)*f(a + y + x
>      ) + 1/2*f(2*x)*f(2*y)*f(y + x)*f(b + 2*x)*f(b + 2*z) - f
(2*x)*f(2*y)*
>      f(y + x)*f(a + 2*z)*f(b + y + x) - 1/2*f(2*x)*f(2*y)*f(y
+ x)*f(a + 2
>      *y)*f(a + 2*z) - f(2*x)*f(2*y)^2*f(c + 2*x)*f(c + y + x)
+ f(2*x)*f(2
>      *y)^2*f(b + 2*x)*f(c + z + x) - 2*f(2*x)*f(2*y)^2*f(a +
z + x)*f(c +
>      y + x) + 2*f(2*x)*f(2*y)^2*f(a + y + x)*f(c + z + x) + f
(2*x)*f(2*y)^
>      2*f(a + 2*x)*f(c + z + y) + f(2*x)^2*f(z + y)*f(c + 2*y)
*f(b + y + x)
>      - 2*f(2*x)^2*f(z + y)*f(b + 2*y)*f(c + y + x) + f(2*x)
^2*f(z + y)*f(
>      b + 2*y)*f(b + z + x) + f(2*x)^2*f(z + y)*f(a + 2*y)*f(c
+ 2*y) + f(2
>      *x)^2*f(z + y)*f(a + 2*y)*f(b + z + y) - f(2*x)^2*f(2*z)
*f(a + 2*y)*
>      f(b + 2*y) - 1/2*f(2*x)^2*f(y + x)*f(c + 2*y)^2 - f(2*x)
^2*f(y + x)*
>      f(c + 2*y)*f(b + z + y) + 2*f(2*x)^2*f(y + x)*f(b + 2*y)
*f(c + z + y)
>      - 1/2*f(2*x)^2*f(y + x)*f(b + 2*y)*f(b + 2*z) + f(2*x)
^2*f(2*y)*f(c
>      + 2*y)*f(c + y + x) + 2*f(2*x)^2*f(2*y)*f(b + z + y)*f
(c + y + x) -
>      2*f(2*x)^2*f(2*y)*f(b + y + x)*f(c + z + y) - f(2*x)^2*f
(2*y)*f(b + 2
>      *y)*f(c + z + x) - f(2*x)^2*f(2*y)*f(a + 2*y)*f(c + z +
y) )
>
>      - f(2*y)*f(b + a + 2*x) + f(2*x)*f(b + a + 2*y):
>
> eq[30] :=
> (1/HessUniv) * ( - f(2*y)*f(z + y)^2*f(a + 2*x)^2 + 2*f(2*y)*f
(z + x
>      )*f(z + y)*f(a + 2*x)*f(a + y + x) + f(2*y)*f(z + x)^2*f
(b + 2*x)^2
>      + 2*f(2*y)*f(z + x)^2*f(b + 2*x)*f(a + y + x) - 4*f(2*
y)*f(z + x)^2*
>      f(a + 2*x)*f(b + y + x) - 2*f(2*y)*f(2*z)*f(y + x)*f(a +
2*x)*f(a + y
>      + x) + 2*f(2*y)*f(y + x)*f(z + y)*f(a + 2*x)*f(a + z +
x) - 2*f(2*y)
>      *f(y + x)*f(z + x)*f(c + 2*x)*f(a + y + x) - 2*f(2*y)*f
(y + x)*f(z +

```



```

>      x)*f(b + 2*x)*f(c + 2*x) - 2*f(2*y)*f(y + x)*f(z + x)*f
> (b + 2*x)*f(a
>      + z + x) + 4*f(2*y)*f(y + x)*f(z + x)*f(a + 2*x)*f(c +
> y + x) + 4*f(
>      2*y)*f(y + x)*f(z + x)*f(a + 2*x)*f(b + z + x) + f(2*y)*
> f(y + x)^2*f(
>      c + 2*x)^2 + 2*f(2*y)*f(y + x)^2*f(c + 2*x)*f(a + z + x)
> - 4*f(2*y)*
>      f(y + x)^2*f(a + 2*x)*f(c + z + x) - 2*f(2*y)^2*f(z + x)
> *f(a + 2*x)*
>      f(a + z + x) + f(2*y)^2*f(2*z)*f(a + 2*x)^2 + f(2*x)*f(z
> + y)^2*f(a
>      + 2*x)*f(a + 2*y) - f(2*x)*f(z + x)*f(z + y)*f(a + 2*y)
> *f(b + 2*x)
>      - 2*f(2*x)*f(z + x)*f(z + y)*f(a + 2*y)*f(a + y + x) +
> f(2*x)*f(z +
>      x)*f(z + y)*f(a + 2*x)*f(b + 2*y) + 2*f(2*x)*f(z + x)^2*
> f(b + 2*y)*f(
>      a + y + x) - f(2*x)*f(z + x)^2*f(b + 2*x)*f(b + 2*y) +
> 2*f(2*x)*f(2*z
>      )*f(y + x)*f(a + 2*y)*f(a + y + x) + f(2*x)*f(y + x)*f(z
> + y)*f(a + 2
>      *y)*f(c + 2*x) - 2*f(2*x)*f(y + x)*f(z + y)*f(a + 2*y)*f
> (a + z + x)
>      - f(2*x)*f(y + x)*f(z + y)*f(a + 2*x)*f(c + 2*y) - 2*f
> (2*x)*f(y + x)
>      *f(z + x)*f(c + 2*y)*f(a + y + x) + f(2*x)*f(y + x)*f(z
> + x)*f(b + 2*
>      y)*f(c + 2*x) - 2*f(2*x)*f(y + x)*f(z + x)*f(b + 2*y)*f
> (a + z + x) +
>      f(2*x)*f(y + x)*f(z + x)*f(b + 2*x)*f(c + 2*y) + 2*f(2*
> x)*f(y + x)^2*
>      f(c + 2*y)*f(a + z + x) - f(2*x)*f(y + x)^2*f(c + 2*x)*f
> (c + 2*y) +
>      f(2*x)*f(2*y)*f(z + y)*f(b + 2*x)*f(c + 2*x) - f(2*x)*f
> (2*y)*f(z + y)
>      *f(a + 2*x)*f(c + y + x) - f(2*x)*f(2*y)*f(z + y)*f(a +
> 2*x)*f(b + z
>      + x) - f(2*x)*f(2*y)*f(z + y)*f(a + 2*x)*f(a + z + y) +
> 2*f(2*x)*f(2
>      *y)*f(z + x)*f(c + 2*x)*f(b + y + x) - f(2*x)*f(2*y)*f(z
> + x)*f(b + 2
>      *x)*f(c + y + x) - f(2*x)*f(2*y)*f(z + x)*f(b + 2*x)*f(b
> + z + x) +
>      f(2*x)*f(2*y)*f(z + x)*f(b + 2*x)*f(a + z + y) + 4*f(2*
> x)*f(2*y)*f(z
>      + x)*f(a + z + x)*f(b + y + x) - 4*f(2*x)*f(2*y)*f(z +
> x)*f(a + y +
>      x)*f(b + z + x) + 2*f(2*x)*f(2*y)*f(z + x)*f(a + 2*y)*f
> (a + z + x) -
>      f(2*x)*f(2*y)*f(z + x)*f(a + 2*x)*f(c + 2*y) - 1/2*f(2*
> x)*f(2*y)*f(2*
>      z)*f(b + 2*x)^2 + f(2*x)*f(2*y)*f(2*z)*f(a + 2*x)*f(b +
> y + x) - 1/2*
>      f(2*x)*f(2*y)*f(2*z)*f(a + 2*x)*f(a + 2*y) - f(2*x)*f(2*
> y)*f(y + x)*
>      f(c + 2*x)*f(c + y + x) - f(2*x)*f(2*y)*f(y + x)*f(c +

```

```

2*x)*f(b + z
> + x) - f(2*x)*f(2*y)*f(y + x)*f(c + 2*x)*f(a + z + y) +
2*f(2*x)*f(2
> *y)*f(y + x)*f(b + 2*x)*f(c + z + x) - 4*f(2*x)*f(2*y)*f
(y + x)*f(a
> + z + x)*f(c + y + x) + 4*f(2*x)*f(2*y)*f(y + x)*f(a +
y + x)*f(c +
> z + x) + 2*f(2*x)*f(2*y)*f(y + x)*f(a + 2*x)*f(c + z +
y) - f(2*x)*f(
> 2*y)*f(y + x)*f(a + 2*x)*f(b + 2*z) - 1/2*f(2*x)*f(2*y)
^2*f(c + 2*x)^
> 2 + f(2*x)*f(2*y)^2*f(a + 2*x)*f(c + z + x) + 1/2*f(2*x)
*f(2*y)^2*f(a
> + 2*x)*f(a + 2*z) + 2*f(2*x)^2*f(z + y)*f(c + 2*y)*f(a
+ y + x) - f(
> 2*x)^2*f(z + y)*f(b + 2*y)*f(c + 2*x) - f(2*x)^2*f(z +
y)*f(a + 2*y)*
> f(c + y + x) + f(2*x)^2*f(z + y)*f(a + 2*y)*f(b + z + x)
+ f(2*x)^2*
> f(z + y)*f(a + 2*y)*f(a + z + y) - f(2*x)^2*f(z + x)*f(b
+ 2*y)*f(c
> + y + x) + f(2*x)^2*f(z + x)*f(b + 2*y)*f(b + z + x) -
f(2*x)^2*f(z
> + x)*f(b + 2*y)*f(a + z + y) + f(2*x)^2*f(z + x)*f(a +
2*y)*f(c + 2*
> y) - f(2*x)^2*f(2*z)*f(b + 2*y)*f(a + y + x) + 1/2*f(2*
x)^2*f(2*z)*f(
> b + 2*x)*f(b + 2*y) - 1/2*f(2*x)^2*f(2*z)*f(a + 2*y)^2 +
f(2*x)^2*f(y
> + x)*f(c + 2*y)*f(c + y + x) - f(2*x)^2*f(y + x)*f(c +
2*y)*f(b + z
> + x) - f(2*x)^2*f(y + x)*f(c + 2*y)*f(a + z + y) + f(2*
x)^2*f(y + x)
> *f(a + 2*z)*f(b + 2*y) + f(2*x)^2*f(2*y)*f(c + 2*x)*f(c
+ 2*y) + 2*f(
> 2*x)^2*f(2*y)*f(b + z + x)*f(c + y + x) + f(2*x)^2*f(2*
y)*f(b + 2*z)*
> f(a + y + x) - 2*f(2*x)^2*f(2*y)*f(b + y + x)*f(c + z +
x) - f(2*x)^2
> *f(2*y)*f(b + 2*x)*f(c + z + y) + 1/2*f(2*x)^2*f(2*y)*f
(b + 2*x)*f(b
> + 2*z) + 2*f(2*x)^2*f(2*y)*f(a + z + y)*f(c + y + x) -
f(2*x)^2*f(2*
> y)*f(a + 2*z)*f(b + y + x) - 2*f(2*x)^2*f(2*y)*f(a + y +
x)*f(c + z
> + y) - f(2*x)^2*f(2*y)*f(a + 2*y)*f(c + z + x) - 1/2*f
(2*x)^2*f(2*y)
> *f(a + 2*y)*f(a + 2*z) - 1/2*f(2*x)^3*f(c + 2*y)^2 + f
(2*x)^3*f(b + 2
> *y)*f(c + z + y) - 1/2*f(2*x)^3*f(b + 2*y)*f(b + 2*z) )
>
> - f(2*y)*f(2*a + 2*x) + f(2*x)*f(2*a + 2*y):
>
>
>

```

```

> SubSt := [f(2 z) = Ctt(r, p, q), f(a + 2 z) = D[2](Ctt)(r, p, q), f(b + 2 z) = D[3](Ctt)(r, p,
q), f(c + 2 z) = D[1](Ctt)(r, p, q), f(2 a + 2 z) = D[2, 2](Ctt)(r, p, q), f(2 b + 2 z)

```

$=D[3, 3](Ctt)(r, p, q), f(2c + 2z) = D[1, 1](Ctt)(r, p, q), f(c + a + 2z) = D[1, 2](Ctt)(r, p, q), f(c + b + 2z) = D[1, 3](Ctt)(r, p, q), f(b + a + 2z) = D[2, 3](Ctt)(r, p, q), f(2x) = Cxx(r, p, q), f(a + 2x) = D[2](Cxx)(r, p, q), f(b + 2x) = D[3](Cxx)(r, p, q), f(c + 2x) = D[1](Cxx)(r, p, q), f(2a + 2x) = D[2, 2](Cxx)(r, p, q), f(2b + 2x) = D[3, 3](Cxx)(r, p, q), f(2c + 2x) = D[1, 1](Cxx)(r, p, q), f(c + a + 2x) = D[1, 2](Cxx)(r, p, q), f(c + b + 2x) = D[1, 3](Cxx)(r, p, q), f(b + a + 2x) = D[2, 3](Cxx)(r, p, q), f(2y) = 1, f(a + 2y) = 0, f(b + 2y) = 0, f(c + 2y) = 0, f(2a + 2y) = 0, f(2b + 2y) = 0, f(2c + 2y) = 0, f(c + a + 2y) = 0, f(c + b + 2y) = 0, f(b + a + 2y) = 0, f(z + x) = Ctx(r, p, q), f(a + z + x) = D[2](Ctx)(r, p, q), f(b + z + x) = D[3](Ctx)(r, p, q), f(c + z + x) = D[1](Ctx)(r, p, q), f(2a + z + x) = D[2, 2](Ctx)(r, p, q), f(2b + z + x) = D[3, 3](Ctx)(r, p, q), f(2c + z + x) = D[1, 1](Ctx)(r, p, q), f(c + a + z + x) = D[1, 2](Ctx)(r, p, q), f(c + b + z + x) = D[1, 3](Ctx)(r, p, q), f(b + a + z + x) = D[2, 3](Ctx)(r, p, q), f(z + y) = Cty(r, p, q), f(a + z + y) = D[2](Cty)(r, p, q), f(b + z + y) = D[3](Cty)(r, p, q), f(c + z + y) = D[1](Cty)(r, p, q), f(2a + z + y) = D[2, 2](Cty)(r, p, q), f(2b + z + y) = D[3, 3](Cty)(r, p, q), f(2c + z + y) = D[1, 1](Cty)(r, p, q), f(c + a + z + y) = D[1, 2](Cty)(r, p, q), f(c + b + z + y) = D[1, 3](Cty)(r, p, q), f(b + a + z + y) = D[2, 3](Cty)(r, p, q), f(y + x) = Cxy(r, p, q), f(a + y + x) = D[2](Cxy)(r, p, q), f(b + y + x) = D[3](Cxy)(r, p, q), f(c + y + x) = D[1](Cxy)(r, p, q), f(2a + y + x) = D[2, 2](Cxy)(r, p, q), f(2b + y + x) = D[3, 3](Cxy)(r, p, q), f(2c + y + x) = D[1, 1](Cxy)(r, p, q), f(c + a + y + x) = D[1, 2](Cxy)(r, p, q), f(c + b + y + x) = D[1, 3](Cxy)(r, p, q), f(b + a + y + x) = D[2, 3](Cxy)(r, p, q) ] :$

> Eeq := subs(SubSt, [seq(eq[j], j = 1..30)]) :

> SubsVars := [D<sub>1,1</sub>(Ctt)(r, p, q), D<sub>1,2</sub>(Ctt)(r, p, q), D<sub>1,3</sub>(Ctt)(r, p, q), D<sub>2,2</sub>(Ctt)(r, p, q), D<sub>2,3</sub>(Ctt)(r, p, q), D<sub>3,3</sub>(Ctt)(r, p, q), D<sub>1,1</sub>(Cxx)(r, p, q), D<sub>1,2</sub>(Cxx)(r, p, q), D<sub>1,3</sub>(Cxx)(r, p, q), D<sub>2,2</sub>(Cxx)(r, p, q), D<sub>2,3</sub>(Cxx)(r, p, q), D<sub>3,3</sub>(Cxx)(r, p, q), D<sub>1,1</sub>(Ctx)(r, p, q), D<sub>1,2</sub>(Ctx)(r, p, q), D<sub>1,3</sub>(Ctx)(r, p, q), D<sub>2,2</sub>(Ctx)(r, p, q), D<sub>2,3</sub>(Ctx)(r, p, q), D<sub>3,3</sub>(Ctx)(r, p, q), D<sub>1,1</sub>(Cty)(r, p, q), D<sub>1,2</sub>(Cty)(r, p, q), D<sub>1,3</sub>(Cty)(r, p, q), D<sub>2,2</sub>(Cty)(r, p, q), D<sub>2,3</sub>(Cty)(r, p, q), D<sub>3,3</sub>(Cty)(r, p, q), D<sub>1,1</sub>(Cxy)(r, p, q), D<sub>1,2</sub>(Cxy)(r, p, q), D<sub>1,3</sub>(Cxy)(r, p, q), D<sub>2,2</sub>(Cxy)(r, p, q), D<sub>2,3</sub>(Cxy)(r, p, q), D<sub>3,3</sub>(Cxy)(r, p, q), ] :

> ICsubs := solve(Eeq, SubsVars)[1]

$$ICsubs := \left[ D_{1,1}(Ctt)(r, p, q) = -\frac{1}{2} \frac{1}{HessUniv} \left( -2 Ctt(r, p, q) Cxy(r, p, q) D_2(Ctt)(r, p, q) \right. \right. \quad (1)$$

$$q) D_3(Ctt)(r, p, q) - 2 Cxx(r, p, q) Ctt(r, p, q) D_1(Ctt)(r, p, q) D_3(Cty)(r, p, q)$$

$$+ 4 Cxx(r, p, q) Cty(r, p, q) D_1(Ctt)(r, p, q) D_1(Cty)(r, p, q) + 2 Ctt(r, p, q) Cty(r, p,$$

$$q) D_3(Cxx)(r, p, q) D_1(Ctt)(r, p, q) + 2 Ctt(r, p, q) Cty(r, p, q) D_2(Ctt)(r, p,$$

$$q) D_1(Cxy)(r, p, q) + 2 Ctt(r, p, q) Cty(r, p, q) D_2(Ctt)(r, p, q) D_3(Ctx)(r, p, q)$$

$$+ 2 Ctt(r, p, q) Cty(r, p, q) D_2(Ctt)(r, p, q) D_2(Cty)(r, p, q) - 2 Ctt(r, p, q) Ctx(r, p,$$

$$\begin{aligned}
& q) D_3(Ctt)(r, p, q) D_1(Cxy)(r, p, q) + 2 Ctt(r, p, q) Ctx(r, p, q) D_3(Ctt)(r, p, \\
& q) D_3(Ctx)(r, p, q) + 2 Ctt(r, p, q) Ctx(r, p, q) D_3(Ctt)(r, p, q) D_2(Cty)(r, p, q) \\
& + 2 Ctt(r, p, q) Cxy(r, p, q) D_1(Ctt)(r, p, q) D_1(Cxy)(r, p, q) + 2 Ctt(r, p, q) Cxy(r, p, \\
& q) D_1(Ctt)(r, p, q) D_3(Ctx)(r, p, q) + 2 Ctt(r, p, q) Cxy(r, p, q) D_1(Ctt)(r, p, \\
& q) D_2(Cty)(r, p, q) - 8 Ctx(r, p, q) Cty(r, p, q) D_1(Ctt)(r, p, q) D_3(Ctx)(r, p, q) \\
& - 8 Ctx(r, p, q) Cty(r, p, q) D_1(Ctt)(r, p, q) D_2(Cty)(r, p, q) + 4 Ctx(r, p, q) Cty(r, p, \\
& q) D_3(Ctt)(r, p, q) D_1(Ctx)(r, p, q) + 4 Ctx(r, p, q) Cty(r, p, q) D_2(Ctt)(r, p, \\
& q) D_1(Cty)(r, p, q) + 4 Ctx(r, p, q) Cty(r, p, q) D_2(Ctt)(r, p, q) D_3(Ctt)(r, p, q) \\
& - 4 Ctt(r, p, q) Cty(r, p, q) D_1(Ctt)(r, p, q) D_2(Cxy)(r, p, q) - 4 Ctt(r, p, q) Cty(r, p, \\
& q) D_3(Ctt)(r, p, q) D_2(Ctx)(r, p, q) + 8 Ctt(r, p, q) Cty(r, p, q) D_2(Cty)(r, p, \\
& q) D_1(Ctx)(r, p, q) - 8 Ctt(r, p, q) Cty(r, p, q) D_2(Ctx)(r, p, q) D_1(Cty)(r, p, q) \\
& - 8 Ctt(r, p, q) Ctx(r, p, q) D_3(Cty)(r, p, q) D_1(Ctx)(r, p, q) + 8 Ctt(r, p, q) Ctx(r, p, \\
& q) D_3(Ctx)(r, p, q) D_1(Cty)(r, p, q) - 4 Ctt(r, p, q) Ctx(r, p, q) D_2(Ctt)(r, p, \\
& q) D_3(Cty)(r, p, q) - 4 Cxy(r, p, q) Cty(r, p, q) D_1(Ctt)(r, p, q) D_1(Ctx)(r, p, q) \\
& - 4 Cxy(r, p, q) Ctx(r, p, q) D_1(Ctt)(r, p, q) D_1(Cty)(r, p, q) + 2 Ctt(r, p, \\
& q)^2 D_1(Cxx)(r, p, q) D_3(Cty)(r, p, q) + 2 Ctt(r, p, q)^2 D_3(Ctt)(r, p, q) D_2(Cxy)(r, p, q) \\
& - 2 Ctt(r, p, q)^2 D_3(Cxx)(r, p, q) D_1(Cty)(r, p, q) - 2 Ctt(r, p, q) D_1(Ctt)(r, p, \\
& q) D_2(Ctx)(r, p, q) + 8 Cty(r, p, q)^2 D_1(Ctt)(r, p, q) D_2(Ctx)(r, p, q) - 4 Cty(r, p,
\end{aligned}$$

$$\begin{aligned}
& q)^2 D_2(Ctt)(r, p, q) D_1(Ctx)(r, p, q) + 8 Ctx(r, p, q)^2 D_1(Ctt)(r, p, q) D_3(Cty)(r, p, q) \\
& - 4 Ctx(r, p, q)^2 D_3(Ctt)(r, p, q) D_1(Cty)(r, p, q) - Ctt(r, p, q)^2 D_3(Cxx)(r, p, \\
& q) D_3(Ctt)(r, p, q) - 4 Ctt(r, p, q)^2 D_2(Cty)(r, p, q) D_1(Cxy)(r, p, q) - 4 Ctt(r, p, \\
& q)^2 D_2(Cty)(r, p, q) D_3(Ctx)(r, p, q) + 4 Ctt(r, p, q)^2 D_2(Ctx)(r, p, q) D_3(Cty)(r, p, q) \\
& + 4 Ctt(r, p, q)^2 D_2(Cxy)(r, p, q) D_1(Cty)(r, p, q) + 4 Ctx(r, p, q) D_1(Ctt)(r, p, \\
& q) D_1(Ctx)(r, p, q) - Ctt(r, p, q) D_1(Cxx)(r, p, q) D_1(Ctt)(r, p, q) + Cxx(r, p, q) Ctt(r, \\
& p, q) D_3(Ctt)(r, p, q)^2 - 2 Ctx(r, p, q)^2 D_3(Ctt)(r, p, q)^2 - 2 Cty(r, p, q)^2 D_2(Ctt)(r, \\
& p, q)^2 + Ctt(r, p, q) D_2(Ctt)(r, p, q)^2 + 2 Cxy(r, p, q)^2 D_1(Ctt)(r, p, q)^2 - 2 Cxx(r, p, \\
& q) D_1(Ctt)(r, p, q)^2), D_{1,2}(Ctt)(r, p, q) = \frac{1}{2} \frac{1}{HessUniv} \left( 4 Cxx(r, p, q) Ctt(r, p, \right. \\
& q) D_3(Cty)(r, p, q) D_1(Ctx)(r, p, q) - 4 Cxx(r, p, q) Ctt(r, p, q) D_3(Ctx)(r, p, \\
& q) D_1(Cty)(r, p, q) - 2 Cxx(r, p, q) Cty(r, p, q) D_1(Ctt)(r, p, q) D_1(Cxy)(r, p, q) \\
& - 2 Cxx(r, p, q) Cty(r, p, q) D_3(Ctt)(r, p, q) D_1(Ctx)(r, p, q) - 2 Cxx(r, p, q) Cty(r, p, \\
& q) D_2(Ctt)(r, p, q) D_1(Cty)(r, p, q) - 2 Cxx(r, p, q) Cty(r, p, q) D_2(Ctt)(r, p, \\
& q) D_3(Ctt)(r, p, q) + 2 Cxx(r, p, q) Ctx(r, p, q) D_3(Ctt)(r, p, q) D_1(Cty)(r, p, q) \\
& + 2 Cxx(r, p, q) Ctt(r, p, q) D_3(Ctt)(r, p, q) D_1(Cxy)(r, p, q) - 2 Cxx(r, p, q) Ctt(r, p, \\
& q) D_3(Ctt)(r, p, q) D_3(Ctx)(r, p, q) + 2 Cxx(r, p, q) Ctt(r, p, q) D_2(Ctt)(r, p, \\
& q) D_3(Cty)(r, p, q) + 4 Cxy(r, p, q) Ctx(r, p, q) D_1(Ctt)(r, p, q) D_2(Cty)(r, p, q) \\
& + 4 Cxx(r, p, q) Cty(r, p, q) D_1(Ctt)(r, p, q) D_3(Ctx)(r, p, q) - 4 Cxx(r, p, q) Ctx(r, p,
\end{aligned}$$

$$\begin{aligned}
& q) D_1(Ctt)(r, p, q) D_3(Cty)(r, p, q) - 2 Ctt(r, p, q) Cty(r, p, q) D_1(Cxx)(r, p, \\
& q) D_2(Cty)(r, p, q) + 2 Ctt(r, p, q) Cty(r, p, q) D_2(Cxx)(r, p, q) D_1(Cty)(r, p, q) \\
& - 2 Ctt(r, p, q) Ctx(r, p, q) D_3(Ctt)(r, p, q) D_2(Cxy)(r, p, q) + 2 Ctt(r, p, q) Cxy(r, p, \\
& q) D_3(Ctt)(r, p, q) D_2(Ctx)(r, p, q) - 2 Ctt(r, p, q) Cxy(r, p, q) D_2(Ctt)(r, p, \\
& q) D_1(Cxy)(r, p, q) - 2 Ctt(r, p, q) Cxy(r, p, q) D_2(Ctt)(r, p, q) D_2(Cty)(r, p, q) \\
& + 2 Cxy(r, p, q) Cty(r, p, q) D_1(Cxx)(r, p, q) D_1(Ctt)(r, p, q) + 4 Ctx(r, p, q) Cty(r, p, \\
& q) D_1(Ctt)(r, p, q) D_2(Cxy)(r, p, q) - Ctt(r, p, q) Cty(r, p, q) D_2(Ctt)(r, p, \\
& q) D_3(Cxx)(r, p, q) + Ctt(r, p, q) Cty(r, p, q) D_2(Cxx)(r, p, q) D_3(Ctt)(r, p, q) + Ctt(r, \\
& p, q) Ctx(r, p, q) D_3(Cxx)(r, p, q) D_3(Ctt)(r, p, q) + 4 Ctt(r, p, q) Ctx(r, p, q) D_2(Cty)(r, \\
& p, q) D_1(Cxy)(r, p, q) - 4 Ctt(r, p, q) Ctx(r, p, q) D_2(Cxy)(r, p, q) D_1(Cty)(r, p, q) \\
& - Ctt(r, p, q) Cxy(r, p, q) D_3(Ctt)(r, p, q) D_1(Cxx)(r, p, q) - Ctt(r, p, q) Cxy(r, p, \\
& q) D_3(Cxx)(r, p, q) D_1(Ctt)(r, p, q) - 4 Ctt(r, p, q) Cxy(r, p, q) D_2(Cty)(r, p, \\
& q) D_1(Ctx)(r, p, q) + 4 Ctt(r, p, q) Cxy(r, p, q) D_2(Ctx)(r, p, q) D_1(Cty)(r, p, q) \\
& - 4 Cxy(r, p, q) Cty(r, p, q) D_1(Ctt)(r, p, q) D_2(Ctx)(r, p, q) + 4 Cxy(r, p, q) Cty(r, p, \\
& q) D_2(Ctt)(r, p, q) D_1(Ctx)(r, p, q) - 2 Cty(r, p, q)^2 D_2(Cxx)(r, p, q) D_1(Ctt)(r, p, q) \\
& + 2 Ctt(r, p, q)^2 D_3(Cxx)(r, p, q) D_2(Cty)(r, p, q) - 2 Ctt(r, p, q)^2 D_2(Cxx)(r, p, \\
& q) D_3(Cty)(r, p, q) + 2 Cxy(r, p, q) Cty(r, p, q) D_2(Ctt)(r, p, q)^2 - 2 Cxy(r, p, \\
& q)^2 D_2(Ctt)(r, p, q) D_1(Ctt)(r, p, q) - 2 Ctx(r, p, q) D_2(Ctt)(r, p, q) D_1(Ctx)(r, p, q)
\end{aligned}$$

$$\begin{aligned}
& + 2 C_{xx}(r, p, q) D_2(C_{tt})(r, p, q) D_1(C_{tt})(r, p, q) - C_{tx}(r, p, q) D_1(C_{xx})(r, p, \\
& q) D_1(C_{tt})(r, p, q) + C_{tt}(r, p, q) D_2(C_{tt})(r, p, q) D_1(C_{xx})(r, p, q) + C_{tt}(r, p, \\
& q) D_2(C_{xx})(r, p, q) D_1(C_{tt})(r, p, q) + C_{xx}(r, p, q) C_{tx}(r, p, q) D_3(C_{tt})(r, p, q)^2 - C_{tx}(r, \\
& p, q) D_2(C_{tt})(r, p, q)^2 \Big), D_{1,3}(C_{tt})(r, p, q) = -\frac{1}{2} \frac{1}{HessUniv} \Big( -4 C_{tx}(r, p, q) C_{ty}(r, \\
& p, q) D_1(C_{tt})(r, p, q) D_3(C_{xy})(r, p, q) - C_{tt}(r, p, q) C_{ty}(r, p, q) D_3(C_{xx})(r, p, \\
& q) D_3(C_{tt})(r, p, q) - 4 C_{tt}(r, p, q) C_{tx}(r, p, q) D_3(C_{ty})(r, p, q) D_1(C_{xy})(r, p, q) \\
& + 4 C_{tt}(r, p, q) C_{tx}(r, p, q) D_3(C_{xy})(r, p, q) D_1(C_{ty})(r, p, q) - 4 C_{tt}(r, p, q) C_{xy}(r, p, \\
& q) D_3(C_{ty})(r, p, q) D_1(C_{tx})(r, p, q) + 4 C_{tt}(r, p, q) C_{xy}(r, p, q) D_3(C_{tx})(r, p, \\
& q) D_1(C_{ty})(r, p, q) - 4 C_{xy}(r, p, q) C_{ty}(r, p, q) D_1(C_{tt})(r, p, q) D_3(C_{tx})(r, p, q) \\
& + 4 C_{xy}(r, p, q) C_{tx}(r, p, q) D_1(C_{tt})(r, p, q) D_3(C_{ty})(r, p, q) - 4 C_{xy}(r, p, q) C_{tx}(r, p, \\
& q) D_3(C_{tt})(r, p, q) D_1(C_{ty})(r, p, q) + 2 C_{tt}(r, p, q) C_{ty}(r, p, q) D_1(C_{xx})(r, p, \\
& q) D_3(C_{ty})(r, p, q) - 2 C_{tt}(r, p, q) C_{ty}(r, p, q) D_3(C_{xx})(r, p, q) D_1(C_{ty})(r, p, q) \\
& + 2 C_{tt}(r, p, q) C_{ty}(r, p, q) D_2(C_{tt})(r, p, q) D_3(C_{xy})(r, p, q) + 2 C_{tt}(r, p, q) C_{xy}(r, p, \\
& q) D_1(C_{tt})(r, p, q) D_3(C_{xy})(r, p, q) + 2 C_{tt}(r, p, q) C_{xy}(r, p, q) D_3(C_{tt})(r, p, \\
& q) D_3(C_{tx})(r, p, q) - 2 C_{tt}(r, p, q) C_{xy}(r, p, q) D_2(C_{tt})(r, p, q) D_3(C_{ty})(r, p, q) \\
& + 2 C_{xx}(r, p, q) C_{ty}(r, p, q) D_3(C_{tt})(r, p, q) D_1(C_{ty})(r, p, q) + 2 C_{ty}(r, p, \\
& q)^2 D_3(C_{xx})(r, p, q) D_1(C_{tt})(r, p, q) - 2 C_{xy}(r, p, q) C_{tx}(r, p, q) D_3(C_{tt})(r, p, q)^2 \\
& + 2 C_{xy}(r, p, q)^2 D_3(C_{tt})(r, p, q) D_1(C_{tt})(r, p, q) - 2 C_{ty}(r, p, q) D_2(C_{tt})(r, p,
\end{aligned}$$

$$\begin{aligned}
& q) D_1(Ctx)(r, p, q) + 2 Ctx(r, p, q) D_1(Ctt)(r, p, q) D_1(Cxy)(r, p, q) + 2 Ctx(r, p, \\
& q) D_3(Ctt)(r, p, q) D_1(Ctx)(r, p, q) + 2 Ctx(r, p, q) D_2(Ctt)(r, p, q) D_1(Cty)(r, p, q) \\
& + 2 Ctx(r, p, q) D_2(Ctt)(r, p, q) D_3(Ctt)(r, p, q) - 2 Ctt(r, p, q) D_1(Ctt)(r, p, \\
& q) D_2(Cxy)(r, p, q) - 2 Ctt(r, p, q) D_3(Ctt)(r, p, q) D_2(Ctx)(r, p, q) + 2 Ctt(r, p, \\
& q) D_2(Ctt)(r, p, q) D_2(Cty)(r, p, q) - 2 Cxx(r, p, q) D_3(Ctt)(r, p, q) D_1(Ctt)(r, p, q) \\
& - 4 Ctt(r, p, q)^2 D_2(Cty)(r, p, q) D_3(Cxy)(r, p, q) + 4 Ctt(r, p, q)^2 D_2(Cxy)(r, p, \\
& q) D_3(Cty)(r, p, q) + 4 Cty(r, p, q) D_1(Ctt)(r, p, q) D_2(Ctx)(r, p, q) - Cty(r, p, \\
& q) D_1(Cxx)(r, p, q) D_1(Ctt)(r, p, q) - 4 Ctx(r, p, q) D_1(Ctt)(r, p, q) D_2(Cty)(r, p, q) \\
& + 4 Ctt(r, p, q) D_2(Cty)(r, p, q) D_1(Ctx)(r, p, q) - 4 Ctt(r, p, q) D_2(Ctx)(r, p, \\
& q) D_1(Cty)(r, p, q) + Cxx(r, p, q) Cty(r, p, q) D_3(Ctt)(r, p, q)^2 - Cty(r, p, \\
& q) D_2(Ctt)(r, p, q)^2, D_{2,2}(Ctt)(r, p, q) = \frac{1}{2} \frac{1}{HessUniv} \left( 2 Cxx(r, p, q) D_1(Ctt)(r, p, \\
& q) D_2(Ctx)(r, p, q) - 2 Cxx(r, p, q)^2 D_1(Ctt)(r, p, q) D_3(Cty)(r, p, q) - 4 Ctx(r, p, \\
& q)^2 D_3(Ctt)(r, p, q) D_2(Cxy)(r, p, q) - 4 Cxy(r, p, q)^2 D_1(Ctt)(r, p, q) D_2(Ctx)(r, p, q) \right. \\
& \left. - 4 Ctx(r, p, q) D_2(Ctt)(r, p, q) D_2(Ctx)(r, p, q) - Cxx(r, p, q) D_1(Cxx)(r, p, \\
& q) D_1(Ctt)(r, p, q) - 2 Cty(r, p, q)^2 D_2(Cxx)(r, p, q) D_2(Ctt)(r, p, q) + 2 Ctx(r, p, \\
& q)^2 D_3(Cxx)(r, p, q) D_3(Ctt)(r, p, q) + 2 Cxy(r, p, q)^2 D_1(Cxx)(r, p, q) D_1(Ctt)(r, p, q) \right. \\
& \left. + 2 Ctt(r, p, q) D_2(Cxx)(r, p, q) D_2(Ctt)(r, p, q) + Cxx(r, p, q) D_2(Ctt)(r, p, q)^2 \right. \\
& \left. + Cxx(r, p, q)^2 D_3(Ctt)(r, p, q)^2 - 2 Ctx(r, p, q) Cty(r, p, q) D_2(Ctt)(r, p, q) D_3(Cxx)(r, \right.
\end{aligned}$$



$$\begin{aligned}
& p, q) + 2 Ctx(r, p, q) Cty(r, p, q) D_2(Cxx)(r, p, q) D_3(Ctt)(r, p, q) + 2 Cxy(r, p, \\
& q) Cty(r, p, q) D_2(Ctt)(r, p, q) D_1(Cxx)(r, p, q) - 2 Cxy(r, p, q) Cty(r, p, q) D_2(Cxx)(r, \\
& p, q) D_1(Ctt)(r, p, q) - 2 Cxy(r, p, q) Ctx(r, p, q) D_3(Ctt)(r, p, q) D_1(Cxx)(r, p, q) \\
& - 2 Cxy(r, p, q) Ctx(r, p, q) D_3(Cxx)(r, p, q) D_1(Ctt)(r, p, q) + 2 Cxx(r, p, q) Cty(r, p, \\
& q) D_3(Cxx)(r, p, q) D_1(Ctt)(r, p, q) - 2 Cxx(r, p, q) Cty(r, p, q) D_2(Ctt)(r, p, \\
& q) D_1(Cxy)(r, p, q) + 2 Cxx(r, p, q) Cty(r, p, q) D_2(Ctt)(r, p, q) D_3(Ctx)(r, p, q) \\
& - 2 Cxx(r, p, q) Cty(r, p, q) D_2(Ctt)(r, p, q) D_2(Cty)(r, p, q) + 2 Cxx(r, p, q) Ctx(r, p, \\
& q) D_3(Ctt)(r, p, q) D_1(Cxy)(r, p, q) - 2 Cxx(r, p, q) Ctx(r, p, q) D_3(Ctt)(r, p, \\
& q) D_3(Ctx)(r, p, q) + 2 Cxx(r, p, q) Ctx(r, p, q) D_3(Ctt)(r, p, q) D_2(Cty)(r, p, q) \\
& + 2 Cxx(r, p, q) Ctt(r, p, q) D_1(Cxx)(r, p, q) D_3(Cty)(r, p, q) + 2 Cxx(r, p, q) Ctt(r, p, \\
& q) D_3(Ctt)(r, p, q) D_2(Cxy)(r, p, q) - 2 Cxx(r, p, q) Ctt(r, p, q) D_3(Cxx)(r, p, \\
& q) D_1(Cty)(r, p, q) - 2 Cxx(r, p, q) Cxy(r, p, q) D_1(Ctt)(r, p, q) D_1(Cxy)(r, p, q) \\
& + 2 Cxx(r, p, q) Cxy(r, p, q) D_1(Ctt)(r, p, q) D_3(Ctx)(r, p, q) + 2 Cxx(r, p, q) Cxy(r, p, \\
& q) D_1(Ctt)(r, p, q) D_2(Cty)(r, p, q) - 2 Cxx(r, p, q) Cxy(r, p, q) D_2(Ctt)(r, p, \\
& q) D_3(Ctt)(r, p, q) + 4 Ctx(r, p, q) Cty(r, p, q) D_2(Ctt)(r, p, q) D_2(Cxy)(r, p, q) \\
& + 4 Ctt(r, p, q) Ctx(r, p, q) D_3(Cxx)(r, p, q) D_2(Cty)(r, p, q) - 4 Ctt(r, p, q) Ctx(r, p, \\
& q) D_2(Cxx)(r, p, q) D_3(Cty)(r, p, q) - 4 Ctt(r, p, q) Cxy(r, p, q) D_1(Cxx)(r, p, \\
& q) D_2(Cty)(r, p, q) - 4 Ctt(r, p, q) Cxy(r, p, q) D_2(Ctt)(r, p, q) D_2(Cxy)(r, p, q)
\end{aligned}$$

$$\begin{aligned}
& + 4 Ctt(r, p, q) Cxy(r, p, q) D_2(Cxx)(r, p, q) D_1(Cty)(r, p, q) + 4 Cxy(r, p, q) Cty(r, p, \\
& q) D_2(Ctt)(r, p, q) D_2(Ctx)(r, p, q) + 4 Cxy(r, p, q) Ctx(r, p, q) D_1(Ctt)(r, p, \\
& q) D_2(Cxy)(r, p, q) + 4 Cxy(r, p, q) Ctx(r, p, q) D_3(Ctt)(r, p, q) D_2(Ctx)(r, p, q) \\
& - 4 Cxx(r, p, q) Cty(r, p, q) D_3(Ctt)(r, p, q) D_2(Ctx)(r, p, q) - Cxx(r, p, q) Ctt(r, p, \\
& q) D_3(Cxx)(r, p, q) D_3(Ctt)(r, p, q) + 4 Cxx(r, p, q) Ctt(r, p, q) D_2(Cty)(r, p, \\
& q) D_1(Cxy)(r, p, q) - 4 Cxx(r, p, q) Ctt(r, p, q) D_2(Cty)(r, p, q) D_3(Ctx)(r, p, q) \\
& + 4 Cxx(r, p, q) Ctt(r, p, q) D_2(Ctx)(r, p, q) D_3(Cty)(r, p, q) - 4 Cxx(r, p, q) Ctt(r, p, \\
& q) D_2(Cxy)(r, p, q) D_1(Cty)(r, p, q) \Big), D_{2,3}(Ctt)(r, p, q) = \frac{1}{2} \frac{1}{HessUniv} \Big( 2 Cxx(r, p, \\
& q) D_1(Ctt)(r, p, q) D_3(Ctx)(r, p, q) + 2 Cxx(r, p, q) D_1(Ctt)(r, p, q) D_2(Cty)(r, p, q) \\
& + Cxy(r, p, q) D_1(Cxx)(r, p, q) D_1(Ctt)(r, p, q) + Cxx(r, p, q) Cxy(r, p, \\
& q) D_3(Ctt)(r, p, q)^2 - 2 Cxy(r, p, q)^2 D_2(Ctt)(r, p, q) D_3(Ctt)(r, p, q) + 2 Ctx(r, p, \\
& q) D_1(Ctt)(r, p, q) D_2(Cxy)(r, p, q) - 2 Ctx(r, p, q) D_2(Ctt)(r, p, q) D_3(Ctx)(r, p, q) \\
& - 2 Ctx(r, p, q) D_2(Ctt)(r, p, q) D_2(Cty)(r, p, q) - 2 Cxy(r, p, q) D_1(Ctt)(r, p, \\
& q) D_2(Ctx)(r, p, q) - 2 Cty(r, p, q)^2 D_2(Ctt)(r, p, q) D_3(Cxx)(r, p, q) + Ctt(r, p, \\
& q) D_2(Ctt)(r, p, q) D_3(Cxx)(r, p, q) + Ctt(r, p, q) D_2(Cxx)(r, p, q) D_3(Ctt)(r, p, q) \\
& - 2 Cxx(r, p, q) D_1(Ctt)(r, p, q) D_1(Cxy)(r, p, q) + Cty(r, p, q) D_2(Ctt)(r, p, \\
& q) D_1(Cxx)(r, p, q) - Cty(r, p, q) D_2(Cxx)(r, p, q) D_1(Ctt)(r, p, q) - Ctx(r, p, \\
& q) D_3(Ctt)(r, p, q) D_1(Cxx)(r, p, q) - Ctx(r, p, q) D_3(Cxx)(r, p, q) D_1(Ctt)(r, p, q)
\end{aligned}$$

$$\begin{aligned}
& -2 Ctt(r, p, q) D_1(Cxx)(r, p, q) D_2(Cty)(r, p, q) + 2 Ctt(r, p, q) D_2(Cxx)(r, p, \\
& q) D_1(Cty)(r, p, q) + Cxy(r, p, q) D_2(Ctt)(r, p, q)^2 + 4 Cxy(r, p, q) Cty(r, p, \\
& q) D_2(Ctt)(r, p, q) D_3(Ctx)(r, p, q) + 4 Cxy(r, p, q) Ctx(r, p, q) D_3(Ctt)(r, p, \\
& q) D_2(Cty)(r, p, q) + 4 Cxx(r, p, q) Ctt(r, p, q) D_3(Cty)(r, p, q) D_1(Cxy)(r, p, q) \\
& + 2 Ctx(r, p, q) Cty(r, p, q) D_3(Cxx)(r, p, q) D_3(Ctt)(r, p, q) + 2 Ctt(r, p, q) Cty(r, p, \\
& q) D_3(Cxx)(r, p, q) D_2(Cty)(r, p, q) - 2 Ctt(r, p, q) Cty(r, p, q) D_2(Cxx)(r, p, \\
& q) D_3(Cty)(r, p, q) + 2 Cxx(r, p, q) Cty(r, p, q) D_1(Ctt)(r, p, q) D_3(Cxy)(r, p, q) \\
& - 2 Cxx(r, p, q) Cty(r, p, q) D_3(Ctt)(r, p, q) D_3(Ctx)(r, p, q) - 2 Cxx(r, p, q) Cty(r, p, \\
& q) D_3(Ctt)(r, p, q) D_2(Cty)(r, p, q) - 2 Cxx(r, p, q) Cxy(r, p, q) D_1(Ctt)(r, p, \\
& q) D_3(Cty)(r, p, q) - 4 Ctt(r, p, q) Ctx(r, p, q) D_2(Cxy)(r, p, q) D_3(Cty)(r, p, q) - Ctt(r, \\
& p, q) Cxy(r, p, q) D_3(Cxx)(r, p, q) D_3(Ctt)(r, p, q) - 4 Ctt(r, p, q) Cxy(r, p, \\
& q) D_2(Cty)(r, p, q) D_3(Ctx)(r, p, q) + 4 Ctt(r, p, q) Cxy(r, p, q) D_2(Ctx)(r, p, \\
& q) D_3(Cty)(r, p, q) + 4 Ctt(r, p, q) Ctx(r, p, q) D_2(Cty)(r, p, q) D_3(Cxy)(r, p, q) \\
& - 2 Ctt(r, p, q) Cxy(r, p, q) D_2(Ctt)(r, p, q) D_3(Cxy)(r, p, q) - 4 Cxx(r, p, q) Ctt(r, p, \\
& q) D_3(Cxy)(r, p, q) D_1(Cty)(r, p, q) \big), D_{3,3}(Ctt)(r, p, q) = -\frac{1}{2} \frac{1}{HessUniv} \big( \\
& -D_2(Ctt)(r, p, q)^2 + 2 Cty(r, p, q) D_3(Cxx)(r, p, q) D_1(Ctt)(r, p, q) - 2 Cty(r, p, \\
& q) D_2(Ctt)(r, p, q) D_1(Cxy)(r, p, q) - 2 Cty(r, p, q) D_2(Ctt)(r, p, q) D_3(Ctx)(r, p, q) \\
& + 2 Cty(r, p, q) D_2(Ctt)(r, p, q) D_2(Cty)(r, p, q) + 2 Ctx(r, p, q) D_3(Ctt)(r, p,
\end{aligned}$$

$$\begin{aligned}
& q) D_1(Cxy)(r, p, q) + 2 Ctx(r, p, q) D_3(Ctt)(r, p, q) D_3(Ctx)(r, p, q) - 2 Ctx(r, p, \\
& q) D_3(Ctt)(r, p, q) D_2(Cty)(r, p, q) + 2 Ctt(r, p, q) D_1(Cxx)(r, p, q) D_3(Cty)(r, p, q) \\
& - 2 Ctt(r, p, q) D_3(Ctt)(r, p, q) D_2(Cxy)(r, p, q) - 2 Ctt(r, p, q) D_3(Cxx)(r, p, \\
& q) D_1(Cty)(r, p, q) + 4 Ctt(r, p, q) D_2(Cty)(r, p, q) D_3(Ctx)(r, p, q) - 4 Ctt(r, p, \\
& q) D_2(Ctx)(r, p, q) D_3(Cty)(r, p, q) - 4 Ctt(r, p, q) D_2(Cxy)(r, p, q) D_1(Cty)(r, p, q) \\
& + 2 Cxy(r, p, q) D_1(Ctt)(r, p, q) D_1(Cxy)(r, p, q) - 2 Cxy(r, p, q) D_1(Ctt)(r, p, \\
& q) D_3(Ctx)(r, p, q) - 2 Cxy(r, p, q) D_1(Ctt)(r, p, q) D_2(Cty)(r, p, q) + 2 Cxy(r, p, \\
& q) D_2(Ctt)(r, p, q) D_3(Ctt)(r, p, q) - 2 Cxx(r, p, q) D_1(Ctt)(r, p, q) D_3(Cty)(r, p, q) \\
& + 4 Cty(r, p, q)^2 D_2(Ctt)(r, p, q) D_3(Cxy)(r, p, q) + 4 Cxy(r, p, q)^2 D_1(Ctt)(r, p, \\
& q) D_3(Cty)(r, p, q) + 4 Ctx(r, p, q) D_2(Ctt)(r, p, q) D_3(Cty)(r, p, q) - Ctt(r, p, \\
& q) D_3(Cxx)(r, p, q) D_3(Ctt)(r, p, q) + 4 Ctt(r, p, q) D_2(Cty)(r, p, q) D_1(Cxy)(r, p, q) \\
& + 2 D_1(Ctt)(r, p, q) D_2(Ctx)(r, p, q) - D_1(Cxx)(r, p, q) D_1(Ctt)(r, p, q) - Cxx(r, p, \\
& q) D_3(Ctt)(r, p, q)^2 - 8 Ctt(r, p, q) Cty(r, p, q) D_2(Cty)(r, p, q) D_3(Cxy)(r, p, q) \\
& + 8 Ctt(r, p, q) Cty(r, p, q) D_2(Cxy)(r, p, q) D_3(Cty)(r, p, q) - 8 Ctt(r, p, q) Cxy(r, p, \\
& q) D_3(Cty)(r, p, q) D_1(Cxy)(r, p, q) + 4 Ctt(r, p, q) Cxy(r, p, q) D_3(Ctt)(r, p, \\
& q) D_3(Cxy)(r, p, q) + 8 Ctt(r, p, q) Cxy(r, p, q) D_3(Cxy)(r, p, q) D_1(Cty)(r, p, q) \\
& - 4 Cxy(r, p, q) Cty(r, p, q) D_1(Ctt)(r, p, q) D_3(Cxy)(r, p, q) - 4 Cxy(r, p, q) Cty(r, p, \\
& q) D_2(Ctt)(r, p, q) D_3(Cty)(r, p, q) - 4 Cxy(r, p, q) Ctx(r, p, q) D_3(Ctt)(r, p,
\end{aligned}$$

$$\begin{aligned}
& q) D_3(Cty)(r, p, q) + 4 Cxx(r, p, q) Cty(r, p, q) D_3(Ctt)(r, p, q) D_3(Cty)(r, p, q) \\
& - 4 Ctx(r, p, q) Cty(r, p, q) D_3(Ctt)(r, p, q) D_3(Cxy)(r, p, q) \big), D_{1,1}(Cxx)(r, p, q) \\
& = \frac{1}{2} \frac{1}{HessUniv} \big( -4 Cty(r, p, q)^2 D_2(Cxx)(r, p, q) D_1(Ctx)(r, p, q) - 4 Ctx(r, p, \\
& q)^2 D_3(Cxx)(r, p, q) D_1(Cty)(r, p, q) - 4 Ctx(r, p, q) D_1(Cxx)(r, p, q) D_1(Ctx)(r, p, q) \\
& + 2 Ctt(r, p, q) D_2(Cxx)(r, p, q) D_1(Ctx)(r, p, q) - 2 Ctt(r, p, q)^2 D_2(Cxx)(r, p, \\
& q) D_3(Cxy)(r, p, q) + 2 Cxx(r, p, q) D_1(Cxx)(r, p, q) D_1(Ctt)(r, p, q) + 2 Cty(r, p, \\
& q)^2 D_2(Cxx)(r, p, q) D_2(Ctt)(r, p, q) + 2 Ctx(r, p, q)^2 D_3(Cxx)(r, p, q) D_3(Ctt)(r, p, q) \\
& - 2 Cxy(r, p, q)^2 D_1(Cxx)(r, p, q) D_1(Ctt)(r, p, q) - Ctt(r, p, q) D_2(Cxx)(r, p, \\
& q) D_2(Ctt)(r, p, q) + Ctt(r, p, q)^2 D_3(Cxx)(r, p, q)^2 + Ctt(r, p, q) D_1(Cxx)(r, p, q)^2 \\
& + 2 Cxx(r, p, q) Ctt(r, p, q) D_2(Ctt)(r, p, q) D_3(Cxy)(r, p, q) - 2 Ctt(r, p, q) Cty(r, p, \\
& q) D_3(Cxx)(r, p, q) D_1(Cxx)(r, p, q) + 2 Ctt(r, p, q) Cty(r, p, q) D_2(Cxx)(r, p, \\
& q) D_1(Cxy)(r, p, q) + 2 Ctt(r, p, q) Cty(r, p, q) D_2(Cxx)(r, p, q) D_3(Ctx)(r, p, q) \\
& - 2 Ctt(r, p, q) Cty(r, p, q) D_2(Cxx)(r, p, q) D_2(Cty)(r, p, q) + 2 Ctt(r, p, q) Ctx(r, p, \\
& q) D_3(Cxx)(r, p, q) D_1(Cxy)(r, p, q) - 2 Ctt(r, p, q) Ctx(r, p, q) D_3(Cxx)(r, p, \\
& q) D_3(Ctx)(r, p, q) - 2 Ctt(r, p, q) Cxy(r, p, q) D_1(Cxx)(r, p, q) D_1(Cxy)(r, p, q) \\
& + 2 Ctt(r, p, q) Cxy(r, p, q) D_1(Cxx)(r, p, q) D_3(Ctx)(r, p, q) + 2 Ctt(r, p, q) Cxy(r, p, \\
& q) D_2(Cxx)(r, p, q) D_3(Ctt)(r, p, q) + 4 Cxy(r, p, q) Cty(r, p, q) D_1(Cxx)(r, p, \\
& q) D_1(Ctx)(r, p, q) + 4 Cxy(r, p, q) Ctx(r, p, q) D_1(Cxx)(r, p, q) D_1(Cty)(r, p, q)
\end{aligned}$$

$$\begin{aligned}
& + 4 C_{xx}(r, p, q) C_{ty}(r, p, q) D_1(C_{tt})(r, p, q) D_2(C_{xy})(r, p, q) - 4 C_{xx}(r, p, q) C_{ty}(r, p, \\
& q) D_1(C_{xx})(r, p, q) D_1(C_{ty})(r, p, q) - 4 C_{xx}(r, p, q) C_{tx}(r, p, q) D_1(C_{tt})(r, p, \\
& q) D_3(C_{xy})(r, p, q) - 4 C_{xx}(r, p, q) C_{tt}(r, p, q) D_3(C_{tx})(r, p, q) D_1(C_{xy})(r, p, q) \\
& + 4 C_{xx}(r, p, q) C_{tt}(r, p, q) D_3(C_{xy})(r, p, q) D_1(C_{tx})(r, p, q) + 4 C_{tx}(r, p, q) C_{ty}(r, p, \\
& q) D_3(C_{xx})(r, p, q) D_1(C_{tx})(r, p, q) + 4 C_{tx}(r, p, q) C_{ty}(r, p, q) D_2(C_{xx})(r, p, \\
& q) D_1(C_{ty})(r, p, q) - 4 C_{tt}(r, p, q) C_{xy}(r, p, q) D_3(C_{xx})(r, p, q) D_1(C_{tx})(r, p, q) \\
& - 2 C_{tx}(r, p, q) C_{ty}(r, p, q) D_2(C_{tt})(r, p, q) D_3(C_{xx})(r, p, q) - 2 C_{tx}(r, p, q) C_{ty}(r, p, \\
& q) D_2(C_{xx})(r, p, q) D_3(C_{tt})(r, p, q) + 2 C_{xy}(r, p, q) C_{ty}(r, p, q) D_2(C_{tt})(r, p, \\
& q) D_1(C_{xx})(r, p, q) - 2 C_{xy}(r, p, q) C_{ty}(r, p, q) D_2(C_{xx})(r, p, q) D_1(C_{tt})(r, p, q) \\
& - 2 C_{xy}(r, p, q) C_{tx}(r, p, q) D_3(C_{tt})(r, p, q) D_1(C_{xx})(r, p, q) + 2 C_{xy}(r, p, q) C_{tx}(r, p, \\
& q) D_3(C_{xx})(r, p, q) D_1(C_{tt})(r, p, q) - 4 C_{xx}(r, p, q) C_{ty}(r, p, q) D_2(C_{tt})(r, p, \\
& q) D_1(C_{xy})(r, p, q) + 4 C_{xx}(r, p, q) C_{tx}(r, p, q) D_3(C_{tt})(r, p, q) D_1(C_{xy})(r, p, q) \\
& - 2 C_{xx}(r, p, q) C_{tt}(r, p, q) D_3(C_{tt})(r, p, q) D_2(C_{xy})(r, p, q) + 2 C_{xx}(r, p, q) C_{tt}(r, p, \\
& q) D_3(C_{xx})(r, p, q) D_1(C_{ty})(r, p, q) + 2 C_{tt}(r, p, q) C_{tx}(r, p, q) D_3(C_{xx})(r, p, \\
& q) D_2(C_{ty})(r, p, q) - 2 C_{tt}(r, p, q) C_{xy}(r, p, q) D_1(C_{xx})(r, p, q) D_2(C_{ty})(r, p, q) \\
& - C_{xx}(r, p, q) C_{tt}(r, p, q) D_3(C_{xx})(r, p, q) D_3(C_{tt})(r, p, q) + 4 C_{xx}(r, p, q) C_{tt}(r, p, \\
& q) D_2(C_{ty})(r, p, q) D_1(C_{xy})(r, p, q) - 4 C_{xx}(r, p, q) C_{tt}(r, p, q) D_2(C_{xy})(r, p, \\
& q) D_1(C_{ty})(r, p, q) \Big), D_{1,2}(C_{xx})(r, p, q) = \frac{1}{2} \frac{1}{HessUniv} \Big( 4 C_{xx}(r, p, q) C_{tt}(r, p,
\end{aligned}$$

$$\begin{aligned}
& q) D_2(Ctx)(r, p, q) D_3(Cxy)(r, p, q) + 2 Cxx(r, p, q) Cxy(r, p, q) D_1(Ctt)(r, p, \\
& q) D_2(Cxy)(r, p, q) - 2 Cxx(r, p, q) Cxy(r, p, q) D_2(Ctt)(r, p, q) D_1(Cxy)(r, p, q) \\
& - Cxx(r, p, q) Cty(r, p, q) D_2(Ctt)(r, p, q) D_3(Cxx)(r, p, q) - Cxx(r, p, q) Cty(r, p, \\
& q) D_2(Cxx)(r, p, q) D_3(Ctt)(r, p, q) + 2 Cxx(r, p, q) Ctt(r, p, q) D_1(Cxx)(r, p, \\
& q) D_3(Cxy)(r, p, q) - 2 Cxx(r, p, q) Ctt(r, p, q) D_3(Cxx)(r, p, q) D_3(Ctx)(r, p, q) \\
& + 2 Cxx(r, p, q) Ctt(r, p, q) D_3(Cxx)(r, p, q) D_2(Cty)(r, p, q) - Cxx(r, p, q) Cxy(r, p, \\
& q) D_3(Ctt)(r, p, q) D_1(Cxx)(r, p, q) + Cxx(r, p, q) Cxy(r, p, q) D_3(Cxx)(r, p, \\
& q) D_1(Ctt)(r, p, q) + 2 Ctt(r, p, q) Ctx(r, p, q) D_3(Cxx)(r, p, q) D_2(Cxy)(r, p, q) \\
& - 4 Ctt(r, p, q) Ctx(r, p, q) D_2(Cxx)(r, p, q) D_3(Cxy)(r, p, q) - 2 Ctt(r, p, q) Cxy(r, p, \\
& q) D_1(Cxx)(r, p, q) D_2(Cxy)(r, p, q) + 4 Cxy(r, p, q) Cty(r, p, q) D_1(Cxx)(r, p, \\
& q) D_2(Ctx)(r, p, q) - 4 Cxy(r, p, q) Cty(r, p, q) D_2(Cxx)(r, p, q) D_1(Ctx)(r, p, q) \\
& + 4 Cxy(r, p, q) Ctx(r, p, q) D_2(Cxx)(r, p, q) D_1(Cty)(r, p, q) + 2 Cxx(r, p, q) Cty(r, p, \\
& q) D_3(Cxx)(r, p, q) D_1(Ctx)(r, p, q) - 4 Cxx(r, p, q) Cty(r, p, q) D_2(Ctx)(r, p, \\
& q) D_1(Cxy)(r, p, q) - 2 Cxx(r, p, q) Ctx(r, p, q) D_3(Cxx)(r, p, q) D_1(Cty)(r, p, q) \\
& + 4 Cxx(r, p, q) Ctx(r, p, q) D_2(Cty)(r, p, q) D_1(Cxy)(r, p, q) - 4 Cxx(r, p, q) Ctx(r, p, \\
& q) D_2(Cxy)(r, p, q) D_1(Cty)(r, p, q) - 2 Cty(r, p, q)^2 D_2(Cxx)(r, p, q) D_1(Cxx)(r, p, q) \\
& + 2 Cxy(r, p, q) Cty(r, p, q) D_1(Cxx)(r, p, q)^2 - 2 Ctx(r, p, q) D_1(Cxx)(r, p, \\
& q) D_2(Ctx)(r, p, q) + 2 Ctt(r, p, q) D_2(Cxx)(r, p, q) D_1(Cxx)(r, p, q) + Ctt(r, p,
\end{aligned}$$

$$\begin{aligned}
& q) \text{ Ctx}(r, p, q) \text{ D}_3(\text{Cxx})(r, p, q)^2 - \text{Ctx}(r, p, q) \text{ D}_2(\text{Cxx})(r, p, q) \text{ D}_2(\text{Ctt})(r, p, q) \\
& - 2 \text{Cxx}(r, p, q)^2 \text{ D}_1(\text{Ctt})(r, p, q) \text{ D}_3(\text{Cxy})(r, p, q) + 2 \text{Cxx}(r, p, q)^2 \text{ D}_3(\text{Ctt})(r, p, \\
& q) \text{ D}_1(\text{Cxy})(r, p, q) - 2 \text{Cxy}(r, p, q)^2 \text{ D}_2(\text{Cxx})(r, p, q) \text{ D}_1(\text{Ctt})(r, p, q) + \text{Cxx}(r, p, \\
& q) \text{ D}_2(\text{Ctt})(r, p, q) \text{ D}_1(\text{Cxx})(r, p, q) + \text{Cxx}(r, p, q) \text{ D}_2(\text{Cxx})(r, p, q) \text{ D}_1(\text{Ctt})(r, p, q) \\
& + 4 \text{Ctx}(r, p, q) \text{ Cty}(r, p, q) \text{ D}_2(\text{Cxx})(r, p, q) \text{ D}_1(\text{Cxy})(r, p, q) + 4 \text{Ctt}(r, p, q) \text{ Cxy}(r, p, \\
& q) \text{ D}_2(\text{Cxx})(r, p, q) \text{ D}_3(\text{Ctx})(r, p, q) + 4 \text{Cxx}(r, p, q) \text{ Cty}(r, p, q) \text{ D}_2(\text{Cxy})(r, p, \\
& q) \text{ D}_1(\text{Ctx})(r, p, q) + \text{Cxx}(r, p, q) \text{ Ctx}(r, p, q) \text{ D}_3(\text{Cxx})(r, p, q) \text{ D}_3(\text{Ctt})(r, p, q) \\
& - 4 \text{Cxx}(r, p, q) \text{ Ctt}(r, p, q) \text{ D}_2(\text{Cxy})(r, p, q) \text{ D}_3(\text{Ctx})(r, p, q) - 2 \text{Ctt}(r, p, q) \text{ Cxy}(r, p, \\
& q) \text{ D}_3(\text{Cxx})(r, p, q) \text{ D}_1(\text{Cxx})(r, p, q) - 2 \text{Ctt}(r, p, q) \text{ Cxy}(r, p, q) \text{ D}_3(\text{Cxx})(r, p, \\
& q) \text{ D}_2(\text{Ctx})(r, p, q) - 2 \text{Ctt}(r, p, q) \text{ Cxy}(r, p, q) \text{ D}_2(\text{Cxx})(r, p, q) \text{ D}_2(\text{Cty})(r, p, q) \\
& + 2 \text{Cxy}(r, p, q) \text{ Cty}(r, p, q) \text{ D}_2(\text{Cxx})(r, p, q) \text{ D}_2(\text{Ctt})(r, p, q) - \text{Ctx}(r, p, \\
& q) \text{ D}_1(\text{Cxx})(r, p, q)^2 - 2 \text{Cxx}(r, p, q) \text{ Cty}(r, p, q) \text{ D}_1(\text{Cxx})(r, p, q) \text{ D}_1(\text{Cxy})(r, p, q) \\
& - 2 \text{Cxx}(r, p, q) \text{ Cty}(r, p, q) \text{ D}_1(\text{Cxx})(r, p, q) \text{ D}_2(\text{Cty})(r, p, q) \Big), \text{D}_{1,3}(\text{Cxx})(r, p, q) \\
& = \frac{1}{2} \frac{1}{\text{HessUniv}} \Big( -2 \text{Cxx}(r, p, q) \text{ Cty}(r, p, q) \text{ D}_1(\text{Cxx})(r, p, q) \text{ D}_3(\text{Cty})(r, p, q) \\
& + 4 \text{Cxx}(r, p, q) \text{ Ctx}(r, p, q) \text{ D}_3(\text{Cty})(r, p, q) \text{ D}_1(\text{Cxy})(r, p, q) - 4 \text{Cxx}(r, p, q) \text{ Ctt}(r, p, \\
& q) \text{ D}_2(\text{Cxy})(r, p, q) \text{ D}_3(\text{Cty})(r, p, q) + 4 \text{Cxx}(r, p, q) \text{ Cty}(r, p, q) \text{ D}_3(\text{Cxy})(r, p, \\
& q) \text{ D}_1(\text{Ctx})(r, p, q) - 4 \text{Cxx}(r, p, q) \text{ Ctx}(r, p, q) \text{ D}_3(\text{Cxy})(r, p, q) \text{ D}_1(\text{Cty})(r, p, q) \\
& - 2 \text{Ctt}(r, p, q) \text{ Cty}(r, p, q) \text{ D}_2(\text{Cxx})(r, p, q) \text{ D}_3(\text{Cxy})(r, p, q) - 2 \text{Ctt}(r, p, q) \text{ Cxy}(r, p,
\end{aligned}$$



$$\begin{aligned}
& q) D_3(Cxx)(r, p, q) D_3(Ctx)(r, p, q) + 2 Ctt(r, p, q) Cxy(r, p, q) D_2(Cxx)(r, p, \\
& q) D_3(Cty)(r, p, q) - 2 Cty(r, p, q)^2 D_3(Cxx)(r, p, q) D_1(Cxx)(r, p, q) - 2 Cxy(r, p, \\
& q)^2 D_3(Ctt)(r, p, q) D_1(Cxx)(r, p, q) + Ctt(r, p, q) Cty(r, p, q) D_3(Cxx)(r, p, q)^2 \\
& + Cty(r, p, q) D_2(Cxx)(r, p, q) D_2(Ctt)(r, p, q) - 2 Ctx(r, p, q) D_1(Cxx)(r, p, \\
& q) D_1(Cxy)(r, p, q) + 2 Ctx(r, p, q) D_2(Cxx)(r, p, q) D_1(Cty)(r, p, q) - 2 Cty(r, p, \\
& q) D_2(Cxx)(r, p, q) D_1(Ctx)(r, p, q) - 2 Ctx(r, p, q) D_1(Cxx)(r, p, q) D_3(Ctx)(r, p, q) \\
& + 2 Ctt(r, p, q) D_2(Cxx)(r, p, q) D_1(Cxy)(r, p, q) + 2 Ctt(r, p, q) D_2(Cxx)(r, p, \\
& q) D_3(Ctx)(r, p, q) - 2 Ctt(r, p, q) D_2(Cxx)(r, p, q) D_2(Cty)(r, p, q) + Cxx(r, p, \\
& q) D_3(Ctt)(r, p, q) D_1(Cxx)(r, p, q) + Cxx(r, p, q) D_3(Cxx)(r, p, q) D_1(Ctt)(r, p, q) \\
& - Ctx(r, p, q) D_2(Ctt)(r, p, q) D_3(Cxx)(r, p, q) - Ctx(r, p, q) D_2(Cxx)(r, p, \\
& q) D_3(Ctt)(r, p, q) + Cxy(r, p, q) D_2(Ctt)(r, p, q) D_1(Cxx)(r, p, q) - Cxy(r, p, \\
& q) D_2(Cxx)(r, p, q) D_1(Ctt)(r, p, q) + 2 Cxx(r, p, q) D_1(Ctt)(r, p, q) D_2(Cxy)(r, p, q) \\
& - 2 Cxx(r, p, q) D_2(Ctt)(r, p, q) D_1(Cxy)(r, p, q) + 4 Cxx(r, p, q) Ctt(r, p, \\
& q) D_2(Cty)(r, p, q) D_3(Cxy)(r, p, q) - 2 Ctt(r, p, q) Cxy(r, p, q) D_3(Cxx)(r, p, \\
& q) D_1(Cxy)(r, p, q) - 2 Cxx(r, p, q) Cxy(r, p, q) D_1(Ctt)(r, p, q) D_3(Cxy)(r, p, q) \\
& + 2 Cxx(r, p, q) Cxy(r, p, q) D_3(Ctt)(r, p, q) D_1(Cxy)(r, p, q) + 4 Ctx(r, p, q) Cty(r, p, \\
& q) D_3(Cxx)(r, p, q) D_1(Cxy)(r, p, q) + 4 Cxy(r, p, q) Cty(r, p, q) D_1(Cxx)(r, p, \\
& q) D_3(Ctx)(r, p, q) - 4 Cxx(r, p, q) Cty(r, p, q) D_3(Ctx)(r, p, q) D_1(Cxy)(r, p, q)
\end{aligned}$$

$$\begin{aligned}
& - C_{xx}(r, p, q) C_{ty}(r, p, q) D_3(C_{xx})(r, p, q) D_3(C_{tt})(r, p, q) + 2 C_{xy}(r, p, q) C_{tx}(r, p, \\
& q) D_3(C_{xx})(r, p, q) D_3(C_{tt})(r, p, q) + C_{ty}(r, p, q) D_1(C_{xx})(r, p, q)^2, D_{2,2}(C_{xx})(r, p, q) \\
& = -\frac{1}{2} \frac{1}{HessUniv} \left( -4 C_{xx}(r, p, q)^2 D_3(C_{tx})(r, p, q) D_1(C_{xy})(r, p, q) + 4 C_{xx}(r, \\
& p, q)^2 D_3(C_{xy})(r, p, q) D_1(C_{tx})(r, p, q) - C_{xx}(r, p, q)^2 D_3(C_{xx})(r, p, q) D_3(C_{tt})(r, p, q) \right. \\
& \quad - 4 C_{xx}(r, p, q)^2 D_2(C_{ty})(r, p, q) D_1(C_{xy})(r, p, q) + 4 C_{xx}(r, p, q)^2 D_2(C_{xy})(r, p, \\
& q) D_1(C_{ty})(r, p, q) - 2 C_{xx}(r, p, q)^2 D_3(C_{tt})(r, p, q) D_2(C_{xy})(r, p, q) + 2 C_{xx}(r, p, \\
& q)^2 D_3(C_{xx})(r, p, q) D_1(C_{ty})(r, p, q) + 2 C_{xx}(r, p, q)^2 D_2(C_{tt})(r, p, q) D_3(C_{xy})(r, p, q) \\
& \quad - 4 C_{tx}(r, p, q)^2 D_3(C_{xx})(r, p, q) D_2(C_{xy})(r, p, q) + 8 C_{tx}(r, p, q)^2 D_2(C_{xx})(r, p, \\
& q) D_3(C_{xy})(r, p, q) - 4 C_{xy}(r, p, q)^2 D_1(C_{xx})(r, p, q) D_2(C_{tx})(r, p, q) + 8 C_{xy}(r, p, \\
& q)^2 D_2(C_{xx})(r, p, q) D_1(C_{tx})(r, p, q) + 4 C_{tx}(r, p, q) D_2(C_{xx})(r, p, q) D_2(C_{tx})(r, p, q) \\
& \quad + C_{xx}(r, p, q) C_{tt}(r, p, q) D_3(C_{xx})(r, p, q)^2 - C_{xx}(r, p, q) D_2(C_{xx})(r, p, q) D_2(C_{tt})(r, \\
& p, q) - 2 C_{xx}(r, p, q) D_2(C_{xx})(r, p, q) D_1(C_{tx})(r, p, q) + C_{xx}(r, p, q) D_1(C_{xx})(r, p, q)^2 \\
& \quad + 2 C_{ty}(r, p, q)^2 D_2(C_{xx})(r, p, q)^2 - 2 C_{tx}(r, p, q)^2 D_3(C_{xx})(r, p, q)^2 - 2 C_{xy}(r, p, \\
& q)^2 D_1(C_{xx})(r, p, q)^2 - 2 C_{tt}(r, p, q) D_2(C_{xx})(r, p, q)^2 - 4 C_{xx}(r, p, q) C_{xy}(r, p, \\
& q) D_3(C_{xx})(r, p, q) D_1(C_{tx})(r, p, q) + 8 C_{xx}(r, p, q) C_{xy}(r, p, q) D_2(C_{tx})(r, p, \\
& q) D_1(C_{xy})(r, p, q) - 8 C_{xx}(r, p, q) C_{xy}(r, p, q) D_2(C_{xy})(r, p, q) D_1(C_{tx})(r, p, q) \\
& \quad - 4 C_{xx}(r, p, q) C_{xy}(r, p, q) D_2(C_{xx})(r, p, q) D_1(C_{ty})(r, p, q) + 2 C_{xx}(r, p, q) C_{tx}(r, p, \\
& q) D_3(C_{xx})(r, p, q) D_1(C_{xy})(r, p, q) + 2 C_{xx}(r, p, q) C_{tx}(r, p, q) D_3(C_{xx})(r, p,
\end{aligned}$$

$$\begin{aligned}
& q) D_3(Ctx)(r, p, q) - 2 Cxx(r, p, q) Ctx(r, p, q) D_3(Cxx)(r, p, q) D_2(Cty)(r, p, q) \\
& - 2 Cxx(r, p, q) Ctt(r, p, q) D_2(Cxx)(r, p, q) D_3(Cxy)(r, p, q) + 2 Cxx(r, p, q) Cxy(r, p, \\
& q) D_1(Cxx)(r, p, q) D_1(Cxy)(r, p, q) + 2 Cxx(r, p, q) Cxy(r, p, q) D_1(Cxx)(r, p, \\
& q) D_3(Ctx)(r, p, q) + 2 Cxx(r, p, q) Cxy(r, p, q) D_1(Cxx)(r, p, q) D_2(Cty)(r, p, q) \\
& + 2 Cxx(r, p, q) Cxy(r, p, q) D_2(Cxx)(r, p, q) D_3(Ctt)(r, p, q) - 2 Cxx(r, p, q) Cty(r, p, \\
& q) D_3(Cxx)(r, p, q) D_1(Cxx)(r, p, q) + 2 Cxx(r, p, q) Cty(r, p, q) D_2(Cxx)(r, p, \\
& q) D_1(Cxy)(r, p, q) + 2 Cxx(r, p, q) Cty(r, p, q) D_2(Cxx)(r, p, q) D_3(Ctx)(r, p, q) \\
& + 2 Cxx(r, p, q) Cty(r, p, q) D_2(Cxx)(r, p, q) D_2(Cty)(r, p, q) - 4 Ctx(r, p, q) Cty(r, p, \\
& q) D_2(Cxx)(r, p, q) D_2(Cxy)(r, p, q) + 4 Ctt(r, p, q) Cxy(r, p, q) D_2(Cxx)(r, p, \\
& q) D_2(Cxy)(r, p, q) - 4 Cxy(r, p, q) Cty(r, p, q) D_2(Cxx)(r, p, q) D_2(Ctx)(r, p, q) \\
& + 4 Cxy(r, p, q) Ctx(r, p, q) D_1(Cxx)(r, p, q) D_2(Cxy)(r, p, q) + 4 Cxy(r, p, q) Ctx(r, p, \\
& q) D_3(Cxx)(r, p, q) D_1(Cxx)(r, p, q) + 4 Cxy(r, p, q) Ctx(r, p, q) D_3(Cxx)(r, p, \\
& q) D_2(Ctx)(r, p, q) - 8 Cxy(r, p, q) Ctx(r, p, q) D_2(Cxx)(r, p, q) D_1(Cxy)(r, p, q) \\
& - 8 Cxy(r, p, q) Ctx(r, p, q) D_2(Cxx)(r, p, q) D_3(Ctx)(r, p, q) - 4 Cxx(r, p, q) Ctx(r, p, \\
& q) D_1(Cxx)(r, p, q) D_3(Cxy)(r, p, q) - 8 Cxx(r, p, q) Ctx(r, p, q) D_2(Ctx)(r, p, \\
& q) D_3(Cxy)(r, p, q) + 8 Cxx(r, p, q) Ctx(r, p, q) D_2(Cxy)(r, p, q) D_3(Ctx)(r, p, q) ), \\
& D_{2,3}(Cxx)(r, p, q) = \frac{1}{2} \frac{1}{HessUniv} \left( 2 Cxy(r, p, q) D_1(Cxx)(r, p, q) D_2(Ctx)(r, p, q) \right. \\
& \left. - 4 Cxy(r, p, q) D_2(Cxx)(r, p, q) D_1(Ctx)(r, p, q) + 4 Cxx(r, p, q) D_2(Cxy)(r, p, \right.
\end{aligned}$$

$$\begin{aligned}
& q) D_1(Ctx)(r, p, q) - 4 Cxx(r, p, q)^2 D_3(Cxy)(r, p, q) D_1(Cty)(r, p, q) + 2 Cxx(r, p, \\
& q) D_2(Cxx)(r, p, q) D_1(Cty)(r, p, q) - 2 Ctx(r, p, q) D_3(Cxx)(r, p, q) D_2(Ctx)(r, p, q) \\
& - 2 Cxx(r, p, q) D_1(Cxx)(r, p, q) D_1(Cxy)(r, p, q) + 2 Cxx(r, p, q) D_3(Cxx)(r, p, \\
& q) D_1(Ctx)(r, p, q) - Ctt(r, p, q) Cxy(r, p, q) D_3(Cxx)(r, p, q)^2 + 4 Ctx(r, p, \\
& q) D_2(Cxx)(r, p, q) D_1(Cxy)(r, p, q) + Cxy(r, p, q) D_2(Cxx)(r, p, q) D_2(Ctt)(r, p, q) \\
& - 4 Cxx(r, p, q) D_2(Ctx)(r, p, q) D_1(Cxy)(r, p, q) + 4 Cxx(r, p, q)^2 D_3(Cty)(r, p, \\
& q) D_1(Cxy)(r, p, q) - 2 Cty(r, p, q)^2 D_2(Cxx)(r, p, q) D_3(Cxx)(r, p, q) + 2 Ctx(r, p, \\
& q) Cty(r, p, q) D_3(Cxx)(r, p, q)^2 - 2 Cxy(r, p, q)^2 D_2(Cxx)(r, p, q) D_3(Ctt)(r, p, q) \\
& - 2 Ctx(r, p, q) D_1(Cxx)(r, p, q) D_2(Cxy)(r, p, q) - 2 Ctx(r, p, q) D_3(Cxx)(r, p, \\
& q) D_1(Cxx)(r, p, q) - 2 Ctx(r, p, q) D_2(Cxx)(r, p, q) D_2(Cty)(r, p, q) + 2 Ctt(r, p, \\
& q) D_2(Cxx)(r, p, q) D_3(Cxx)(r, p, q) + Cxy(r, p, q) D_1(Cxx)(r, p, q)^2 + 4 Cxy(r, p, \\
& q) Cty(r, p, q) D_2(Cxx)(r, p, q) D_3(Ctx)(r, p, q) + 4 Cxy(r, p, q) Ctx(r, p, q) D_2(Cxx)(r, \\
& p, q) D_3(Cty)(r, p, q) + 4 Cxx(r, p, q) Cty(r, p, q) D_2(Ctx)(r, p, q) D_3(Cxy)(r, p, q) \\
& - 4 Cxx(r, p, q) Ctx(r, p, q) D_2(Cxy)(r, p, q) D_3(Cty)(r, p, q) + Cxx(r, p, q) Cxy(r, p, \\
& q) D_3(Cxx)(r, p, q) D_3(Ctt)(r, p, q) - 2 Ctt(r, p, q) Cxy(r, p, q) D_3(Cxx)(r, p, \\
& q) D_2(Cxy)(r, p, q) - 2 Cxx(r, p, q) Cty(r, p, q) D_3(Cxx)(r, p, q) D_3(Ctx)(r, p, q) \\
& - 2 Cxx(r, p, q) Cty(r, p, q) D_2(Cxx)(r, p, q) D_3(Cty)(r, p, q) - 2 Cxx(r, p, q) Cxy(r, p, \\
& q) D_1(Cxx)(r, p, q) D_3(Cty)(r, p, q) + 2 Cxx(r, p, q) Cxy(r, p, q) D_3(Ctt)(r, p,
\end{aligned}$$

$$\begin{aligned}
& q) D_2(Cxy)(r, p, q) + 4 Cxx(r, p, q) Ctx(r, p, q) D_2(Cty)(r, p, q) D_3(Cxy)(r, p, q) \\
& - 2 Cxx(r, p, q) Cxy(r, p, q) D_2(Ctt)(r, p, q) D_3(Cxy)(r, p, q) + 4 Ctx(r, p, q) Cty(r, p, \\
& q) D_3(Cxx)(r, p, q) D_2(Cxy)(r, p, q) - 4 Ctx(r, p, q) Cty(r, p, q) D_2(Cxx)(r, p, \\
& q) D_3(Cxy)(r, p, q) + 2 Cxx(r, p, q) Cty(r, p, q) D_1(Cxx)(r, p, q) D_3(Cxy)(r, p, q) \\
& - 4 Cxx(r, p, q) Cty(r, p, q) D_2(Cxy)(r, p, q) D_3(Ctx)(r, p, q) \big), D_{3,3}(Cxx)(r, p, q) \\
& = \frac{1}{2} \frac{1}{HessUniv} \left( D_1(Cxx)(r, p, q)^2 + 2 Cxx(r, p, q) D_3(Cxx)(r, p, q) D_1(Cty)(r, p, q) \right. \\
& - 4 Cty(r, p, q)^2 D_2(Cxx)(r, p, q) D_3(Cxy)(r, p, q) - 2 Cxy(r, p, q) D_2(Cxx)(r, p, \\
& q) D_3(Ctt)(r, p, q) + 4 Cxx(r, p, q) D_3(Cxy)(r, p, q) D_1(Ctx)(r, p, q) + 4 Cxx(r, p, \\
& q) D_2(Cxy)(r, p, q) D_1(Cty)(r, p, q) + 2 Cty(r, p, q) D_2(Cxx)(r, p, q) D_1(Cxy)(r, p, q) \\
& + 2 Cty(r, p, q) D_2(Cxx)(r, p, q) D_3(Ctx)(r, p, q) - 4 Ctx(r, p, q) D_1(Cxx)(r, p, \\
& q) D_3(Cxy)(r, p, q) + 2 Ctx(r, p, q) D_3(Cxx)(r, p, q) D_1(Cxy)(r, p, q) - 2 Ctx(r, p, \\
& q) D_3(Cxx)(r, p, q) D_2(Cty)(r, p, q) + 2 Ctt(r, p, q) D_2(Cxx)(r, p, q) D_3(Cxy)(r, p, q) \\
& - 2 Cxy(r, p, q) D_1(Cxx)(r, p, q) D_1(Cxy)(r, p, q) - 4 Cxy(r, p, q)^2 D_1(Cxx)(r, p, \\
& q) D_3(Cty)(r, p, q) - 4 Cxx(r, p, q) D_3(Ctx)(r, p, q) D_1(Cxy)(r, p, q) + Cxx(r, p, \\
& q) D_3(Cxx)(r, p, q) D_3(Ctt)(r, p, q) - 4 Cxx(r, p, q) D_2(Cty)(r, p, q) D_1(Cxy)(r, p, q) \\
& + 2 Cxx(r, p, q) D_3(Ctt)(r, p, q) D_2(Cxy)(r, p, q) - 2 Cxx(r, p, q) D_2(Ctt)(r, p, \\
& q) D_3(Cxy)(r, p, q) + 2 Cxy(r, p, q) D_1(Cxx)(r, p, q) D_3(Ctx)(r, p, q) + 2 Cxy(r, p, \\
& q) D_1(Cxx)(r, p, q) D_2(Cty)(r, p, q) - 2 Cty(r, p, q) D_3(Cxx)(r, p, q) D_1(Cxx)(r, p, q) \big)
\end{aligned}$$

$$\begin{aligned}
& -2 Cty(r, p, q) D_2(Cxx)(r, p, q) D_2(Cty)(r, p, q) - 2 Ctx(r, p, q) D_3(Cxx)(r, p, \\
& q) D_3(Ctx)(r, p, q) - 2 D_2(Cxx)(r, p, q) D_1(Ctx)(r, p, q) + Ctt(r, p, q) D_3(Cxx)(r, p, q)^2 \\
& + D_2(Cxx)(r, p, q) D_2(Ctt)(r, p, q) - 4 Cxx(r, p, q) Cty(r, p, q) D_3(Cxx)(r, p, \\
& q) D_3(Cty)(r, p, q) + 8 Cxx(r, p, q) Cty(r, p, q) D_2(Cty)(r, p, q) D_3(Cxy)(r, p, q) \\
& + 4 Cxy(r, p, q) Cty(r, p, q) D_1(Cxx)(r, p, q) D_3(Cxy)(r, p, q) + 4 Cxy(r, p, q) Cty(r, p, \\
& q) D_2(Cxx)(r, p, q) D_3(Cty)(r, p, q) + 4 Cxy(r, p, q) Ctx(r, p, q) D_3(Cxx)(r, p, \\
& q) D_3(Cty)(r, p, q) - 8 Cxx(r, p, q) Cty(r, p, q) D_2(Cxy)(r, p, q) D_3(Cty)(r, p, q) \\
& + 8 Cxx(r, p, q) Cxy(r, p, q) D_3(Cty)(r, p, q) D_1(Cxy)(r, p, q) - 8 Cxx(r, p, q) Cxy(r, p, \\
& q) D_3(Cxy)(r, p, q) D_1(Cty)(r, p, q) + 4 Ctx(r, p, q) Cty(r, p, q) D_3(Cxx)(r, p, \\
& q) D_3(Cxy)(r, p, q) - 4 Ctt(r, p, q) Cxy(r, p, q) D_3(Cxx)(r, p, q) D_3(Cxy)(r, p, q) \Big), \\
& D_{1,1}(Ctx)(r, p, q) = \frac{1}{4} \frac{1}{HessUniv} \Big( -8 Cty(r, p, q)^2 D_2(Ctx)(r, p, q) D_1(Ctx)(r, p, q) \\
& + 4 Cty(r, p, q)^2 D_2(Ctt)(r, p, q) D_1(Cxx)(r, p, q) + 4 Cty(r, p, q)^2 D_2(Ctt)(r, p, \\
& q) D_2(Ctx)(r, p, q) - 8 Ctx(r, p, q)^2 D_1(Ctt)(r, p, q) D_3(Cxy)(r, p, q) - 8 Ctx(r, p, \\
& q)^2 D_3(Ctx)(r, p, q) D_1(Cty)(r, p, q) + 8 Ctx(r, p, q)^2 D_3(Ctt)(r, p, q) D_1(Cxy)(r, p, q) \\
& + 4 Ctx(r, p, q)^2 D_3(Ctt)(r, p, q) D_3(Ctx)(r, p, q) - 4 Ctt(r, p, q) Ctx(r, p, \\
& q) D_3(Ctx)(r, p, q)^2 - 4 Ctt(r, p, q)^2 D_2(Ctx)(r, p, q) D_3(Cxy)(r, p, q) + 8 Cxy(r, p, \\
& q) Cty(r, p, q) D_1(Ctx)(r, p, q)^2 - 4 Cxy(r, p, q)^2 D_1(Ctt)(r, p, q) D_1(Ctx)(r, p, q) \\
& + 4 Ctt(r, p, q) D_2(Ctx)(r, p, q) D_1(Ctx)(r, p, q) + 4 Cxx(r, p, q) D_1(Ctt)(r, p,
\end{aligned}$$

$$\begin{aligned}
& q) D_1(Ctx)(r, p, q) + 2 Ctt(r, p, q) D_1(Cxx)(r, p, q) D_1(Ctx)(r, p, q) - 2 Ctt(r, p, \\
& q) D_2(Ctt)(r, p, q) D_2(Ctx)(r, p, q) - 2 Ctt(r, p, q)^2 D_1(Cxx)(r, p, q) D_3(Cxy)(r, p, q) \\
& + 2 Ctt(r, p, q)^2 D_3(Cxx)(r, p, q) D_1(Cxy)(r, p, q) + 2 Ctt(r, p, q)^2 D_3(Cxx)(r, p, \\
& q) D_3(Ctx)(r, p, q) + 4 Cxx(r, p, q) Ctt(r, p, q) D_3(Cty)(r, p, q) D_1(Ctx)(r, p, q) \\
& - 4 Cxx(r, p, q) Cty(r, p, q) D_2(Ctt)(r, p, q) D_1(Cty)(r, p, q) + 4 Cxx(r, p, q) Ctx(r, p, \\
& q) D_3(Ctt)(r, p, q) D_1(Cty)(r, p, q) - 2 Cxx(r, p, q) Ctt(r, p, q) D_3(Ctt)(r, p, \\
& q) D_1(Cxy)(r, p, q) - 2 Cxx(r, p, q) Ctt(r, p, q) D_3(Ctt)(r, p, q) D_3(Ctx)(r, p, q) \\
& + 2 Cxx(r, p, q) Ctt(r, p, q) D_2(Ctt)(r, p, q) D_3(Cty)(r, p, q) - 4 Cxx(r, p, q) Ctx(r, p, \\
& q) D_1(Ctt)(r, p, q) D_3(Cty)(r, p, q) - 4 Ctt(r, p, q) Cty(r, p, q) D_1(Cxx)(r, p, \\
& q) D_2(Cty)(r, p, q) + 4 Ctt(r, p, q) Cty(r, p, q) D_2(Cxx)(r, p, q) D_1(Cty)(r, p, q) \\
& - 4 Ctt(r, p, q) Ctx(r, p, q) D_3(Ctt)(r, p, q) D_2(Cxy)(r, p, q) + 4 Ctt(r, p, q) Cxy(r, p, \\
& q) D_3(Ctt)(r, p, q) D_2(Ctx)(r, p, q) + 8 Ctx(r, p, q) Cty(r, p, q) D_1(Ctt)(r, p, \\
& q) D_2(Cxy)(r, p, q) - 2 Ctt(r, p, q) Cty(r, p, q) D_2(Ctt)(r, p, q) D_3(Cxx)(r, p, q) \\
& + 2 Ctt(r, p, q) Cty(r, p, q) D_2(Cxx)(r, p, q) D_3(Ctt)(r, p, q) + 8 Ctt(r, p, q) Ctx(r, p, \\
& q) D_2(Cty)(r, p, q) D_1(Cxy)(r, p, q) - 8 Ctt(r, p, q) Ctx(r, p, q) D_2(Cxy)(r, p, \\
& q) D_1(Cty)(r, p, q) + 2 Ctt(r, p, q) Cxy(r, p, q) D_3(Ctt)(r, p, q) D_1(Cxx)(r, p, q) \\
& - 2 Ctt(r, p, q) Cxy(r, p, q) D_3(Cxx)(r, p, q) D_1(Ctt)(r, p, q) - 4 Ctt(r, p, q) Cxy(r, p, \\
& q) D_2(Cty)(r, p, q) D_1(Ctx)(r, p, q) - 4 Cxy(r, p, q) Cty(r, p, q) D_1(Ctt)(r, p,
\end{aligned}$$

$$\begin{aligned}
& q) D_2(Ctx)(r, p, q) + 4 Cxy(r, p, q) Cty(r, p, q) D_2(Ctt)(r, p, q) D_1(Ctx)(r, p, q) \\
& - 4 Cty(r, p, q)^2 D_2(Cxx)(r, p, q) D_1(Ctt)(r, p, q) + 2 Ctt(r, p, q)^2 D_3(Cxx)(r, p, \\
& q) D_2(Cty)(r, p, q) - 2 Ctt(r, p, q)^2 D_2(Cxx)(r, p, q) D_3(Cty)(r, p, q) - Ctt(r, p, \\
& q) D_2(Ctt)(r, p, q) D_1(Cxx)(r, p, q) + Ctt(r, p, q) D_2(Cxx)(r, p, q) D_1(Ctt)(r, p, q) \\
& - 8 Ctx(r, p, q) D_1(Ctx)(r, p, q)^2 + 2 Cxx(r, p, q) Ctt(r, p, q) D_1(Ctt)(r, p, \\
& q) D_3(Cxy)(r, p, q) - 2 Cxx(r, p, q) Ctt(r, p, q) D_3(Ctt)(r, p, q) D_2(Cty)(r, p, q) \\
& - 8 Cxx(r, p, q) Cty(r, p, q) D_1(Ctx)(r, p, q) D_1(Cty)(r, p, q) + 4 Cxx(r, p, q) Cty(r, p, \\
& q) D_1(Ctt)(r, p, q) D_2(Cty)(r, p, q) + 8 Ctx(r, p, q) Cty(r, p, q) D_3(Ctx)(r, p, \\
& q) D_1(Ctx)(r, p, q) - 4 Ctx(r, p, q) Cty(r, p, q) D_3(Ctt)(r, p, q) D_1(Cxx)(r, p, q) \\
& - 4 Ctx(r, p, q) Cty(r, p, q) D_3(Ctt)(r, p, q) D_2(Ctx)(r, p, q) + 4 Ctx(r, p, q) Cty(r, p, \\
& q) D_3(Cxx)(r, p, q) D_1(Ctt)(r, p, q) + 8 Ctx(r, p, q) Cty(r, p, q) D_2(Ctx)(r, p, \\
& q) D_1(Cty)(r, p, q) - 8 Ctx(r, p, q) Cty(r, p, q) D_2(Ctt)(r, p, q) D_1(Cxy)(r, p, q) \\
& - 4 Ctx(r, p, q) Cty(r, p, q) D_2(Ctt)(r, p, q) D_3(Ctx)(r, p, q) - 4 Ctt(r, p, q) Cty(r, p, \\
& q) D_3(Cxx)(r, p, q) D_1(Ctx)(r, p, q) + 4 Ctt(r, p, q) Cty(r, p, q) D_2(Ctx)(r, p, \\
& q) D_1(Cxy)(r, p, q) + 4 Ctt(r, p, q) Cty(r, p, q) D_2(Ctx)(r, p, q) D_3(Ctx)(r, p, q) \\
& - 4 Ctt(r, p, q) Cty(r, p, q) D_2(Ctx)(r, p, q) D_2(Cty)(r, p, q) - 4 Ctt(r, p, q) Ctx(r, p, \\
& q) D_3(Ctx)(r, p, q) D_1(Cxy)(r, p, q) + 8 Ctt(r, p, q) Ctx(r, p, q) D_3(Cxy)(r, p, \\
& q) D_1(Ctx)(r, p, q) + 4 Ctt(r, p, q) Ctx(r, p, q) D_2(Cty)(r, p, q) D_3(Ctx)(r, p, q)
\end{aligned}$$



$$\begin{aligned}
& + 4 \, Ctt(r, p, q) \, Ctx(r, p, q) \, D_2(Ctt)(r, p, q) \, D_3(Cxy)(r, p, q) - 4 \, Ctt(r, p, q) \, Cxy(r, p, \\
& q) \, D_1(Cxy)(r, p, q) \, D_1(Ctx)(r, p, q) - 4 \, Ctt(r, p, q) \, Cxy(r, p, q) \, D_3(Ctx)(r, p, \\
& q) \, D_1(Ctx)(r, p, q) + 8 \, Cxy(r, p, q) \, Ctx(r, p, q) \, D_1(Ctx)(r, p, q) \, D_1(Cty)(r, p, q) \\
& + 4 \, Cxy(r, p, q) \, Ctx(r, p, q) \, D_1(Ctt)(r, p, q) \, D_3(Ctx)(r, p, q) - 4 \, Cxy(r, p, q) \, Ctx(r, p, \\
& q) \, D_3(Ctt)(r, p, q) \, D_1(Ctx)(r, p, q) \, D_{1,2}(Ctx)(r, p, q) = \\
& - \frac{1}{4} \frac{1}{HessUniv} \left( 4 \, Cty(r, p, q)^2 \, D_2(Cxx)(r, p, q) \, D_1(Ctx)(r, p, q) + 2 \, Ctx(r, p, \\
& q) \, D_1(Cxx)(r, p, q) \, D_1(Ctx)(r, p, q) - 2 \, Ctt(r, p, q) \, D_2(Cxx)(r, p, q) \, D_1(Ctx)(r, p, q) \right. \\
& + 2 \, Ctt(r, p, q)^2 \, D_2(Cxx)(r, p, q) \, D_3(Cxy)(r, p, q) - 8 \, Ctx(r, p, q)^2 \, D_2(Cty)(r, p, \\
& q) \, D_1(Cxy)(r, p, q) + 8 \, Ctx(r, p, q)^2 \, D_2(Cxy)(r, p, q) \, D_1(Cty)(r, p, q) + 4 \, Ctx(r, p, \\
& q) \, D_2(Ctx)(r, p, q) \, D_1(Ctx)(r, p, q) + Ctx(r, p, q) \, D_2(Ctt)(r, p, q) \, D_1(Cxx)(r, p, q) \\
& - Ctx(r, p, q) \, D_2(Cxx)(r, p, q) \, D_1(Ctt)(r, p, q) + 4 \, Cxx(r, p, q) \, Ctt(r, p, \\
& q) \, D_3(Ctx)(r, p, q)^2 - 2 \, Cxx(r, p, q) \, D_2(Ctt)(r, p, q) \, D_1(Ctx)(r, p, q) - 2 \, Cxx(r, p, \\
& q)^2 \, D_3(Ctt)(r, p, q) \, D_1(Cty)(r, p, q) - 2 \, Ctt(r, p, q) \, D_1(Cxx)(r, p, q) \, D_2(Ctx)(r, p, q) \\
& - 2 \, Ctt(r, p, q)^2 \, D_3(Cxx)(r, p, q) \, D_2(Cxy)(r, p, q) - 2 \, Cxx(r, p, q) \, D_1(Ctt)(r, p, \\
& q) \, D_2(Ctx)(r, p, q) + 2 \, Cxx(r, p, q)^2 \, D_1(Ctt)(r, p, q) \, D_3(Cty)(r, p, q) + 4 \, Cxy(r, p, \\
& q)^2 \, D_1(Ctt)(r, p, q) \, D_2(Ctx)(r, p, q) + 2 \, Ctx(r, p, q) \, D_2(Ctt)(r, p, q) \, D_2(Ctx)(r, p, q) \\
& + 2 \, Cxx(r, p, q) \, Cxy(r, p, q) \, D_3(Ctt)(r, p, q) \, D_1(Ctx)(r, p, q) + 2 \, Cxx(r, p, q) \, Cxy(r, p, \\
& q) \, D_2(Ctt)(r, p, q) \, D_1(Cty)(r, p, q) + 4 \, Cxx(r, p, q) \, Cty(r, p, q) \, D_1(Cxy)(r, p,
\end{aligned}$$

$$\begin{aligned}
& q) D_1(Ctx)(r, p, q) - 4 Cxx(r, p, q) Cty(r, p, q) D_3(Ctx)(r, p, q) D_1(Ctx)(r, p, q) \\
& + 4 Cxx(r, p, q) Cty(r, p, q) D_2(Ctx)(r, p, q) D_1(Cty)(r, p, q) + 4 Cxx(r, p, q) Ctx(r, p, \\
& q) D_3(Ctx)(r, p, q) D_1(Cty)(r, p, q) + 4 Ctx(r, p, q) Cty(r, p, q) D_1(Cxx)(r, p, \\
& q) D_2(Cty)(r, p, q) - 8 Ctx(r, p, q) Cty(r, p, q) D_2(Cxy)(r, p, q) D_1(Ctx)(r, p, q) \\
& + 4 Ctt(r, p, q) Ctx(r, p, q) D_2(Cxy)(r, p, q) D_3(Ctx)(r, p, q) - 4 Ctt(r, p, q) Cxy(r, p, \\
& q) D_2(Ctx)(r, p, q) D_3(Ctx)(r, p, q) + 4 Ctt(r, p, q) Cxy(r, p, q) D_2(Ctx)(r, p, \\
& q) D_2(Cty)(r, p, q) + 4 Ctt(r, p, q) Cxy(r, p, q) D_2(Cxy)(r, p, q) D_1(Ctx)(r, p, q) \\
& - 8 Cxy(r, p, q) Ctx(r, p, q) D_2(Ctx)(r, p, q) D_1(Cty)(r, p, q) + 4 Cxy(r, p, q) Ctx(r, p, \\
& q) D_2(Ctt)(r, p, q) D_1(Cxy)(r, p, q) + 2 Cxx(r, p, q) Cty(r, p, q) D_3(Ctt)(r, p, \\
& q) D_1(Cxx)(r, p, q) + 2 Ctt(r, p, q) Cty(r, p, q) D_1(Cxx)(r, p, q) D_2(Cxy)(r, p, q) \\
& + 2 Ctt(r, p, q) Cty(r, p, q) D_3(Cxx)(r, p, q) D_2(Ctx)(r, p, q) + 2 Ctt(r, p, q) Cxy(r, p, \\
& q) D_2(Ctt)(r, p, q) D_3(Cxx)(r, p, q) - 2 Cxx(r, p, q) Ctt(r, p, q) D_2(Ctt)(r, p, \\
& q) D_3(Cxy)(r, p, q) - 2 Ctt(r, p, q) Cty(r, p, q) D_2(Cxx)(r, p, q) D_1(Cxy)(r, p, q) \\
& - 2 Ctt(r, p, q) Cty(r, p, q) D_2(Cxx)(r, p, q) D_3(Ctx)(r, p, q) - 2 Ctt(r, p, q) Ctx(r, p, \\
& q) D_3(Cxx)(r, p, q) D_3(Ctx)(r, p, q) + 2 Ctt(r, p, q) Cxy(r, p, q) D_1(Cxx)(r, p, \\
& q) D_3(Ctx)(r, p, q) - 2 Ctt(r, p, q) Cxy(r, p, q) D_2(Cxx)(r, p, q) D_3(Ctt)(r, p, q) \\
& - 4 Cxy(r, p, q) Cty(r, p, q) D_1(Cxx)(r, p, q) D_1(Ctx)(r, p, q) - 2 Cxx(r, p, q) Cty(r, p, \\
& q) D_1(Ctt)(r, p, q) D_2(Cxy)(r, p, q) + 4 Cxx(r, p, q) Ctx(r, p, q) D_1(Ctt)(r, p,
\end{aligned}$$

$$\begin{aligned}
& q) D_3(Cxy)(r, p, q) - 4 Cxx(r, p, q) Ctt(r, p, q) D_3(Cxy)(r, p, q) D_1(Ctx)(r, p, q) \\
& - 4 Ctx(r, p, q) Cty(r, p, q) D_2(Cxx)(r, p, q) D_1(Cty)(r, p, q) + 2 Ctt(r, p, q) Cxy(r, p, \\
& q) D_3(Cxx)(r, p, q) D_1(Ctx)(r, p, q) - 4 Cxy(r, p, q) Cty(r, p, q) D_2(Ctt)(r, p, \\
& q) D_1(Cxx)(r, p, q) + 4 Cxy(r, p, q) Cty(r, p, q) D_2(Cxx)(r, p, q) D_1(Ctt)(r, p, q) \\
& - 2 Cxx(r, p, q) Cty(r, p, q) D_3(Cxx)(r, p, q) D_1(Ctt)(r, p, q) + 2 Cxx(r, p, q) Cty(r, p, \\
& q) D_2(Ctt)(r, p, q) D_1(Cxy)(r, p, q) + 2 Cxx(r, p, q) Cty(r, p, q) D_2(Ctt)(r, p, \\
& q) D_3(Ctx)(r, p, q) - 4 Cxx(r, p, q) Ctx(r, p, q) D_3(Ctt)(r, p, q) D_1(Cxy)(r, p, q) \\
& - 2 Cxx(r, p, q) Ctx(r, p, q) D_3(Ctt)(r, p, q) D_3(Ctx)(r, p, q) - 2 Cxx(r, p, q) Ctt(r, p, \\
& q) D_1(Cxx)(r, p, q) D_3(Cty)(r, p, q) + 2 Cxx(r, p, q) Ctt(r, p, q) D_3(Ctt)(r, p, \\
& q) D_2(Cxy)(r, p, q) + 2 Cxx(r, p, q) Ctt(r, p, q) D_3(Cxx)(r, p, q) D_1(Cty)(r, p, q) \\
& - 2 Cxx(r, p, q) Cxy(r, p, q) D_1(Ctt)(r, p, q) D_3(Ctx)(r, p, q) - 2 Cxx(r, p, q) Cxy(r, p, \\
& q) D_1(Ctt)(r, p, q) D_2(Cty)(r, p, q) - 4 Ctt(r, p, q) Ctx(r, p, q) D_3(Cxx)(r, p, \\
& q) D_2(Cty)(r, p, q) + 4 Ctt(r, p, q) Ctx(r, p, q) D_2(Cxx)(r, p, q) D_3(Cty)(r, p, q) \\
& + 2 Ctt(r, p, q) Cxy(r, p, q) D_1(Cxx)(r, p, q) D_2(Cty)(r, p, q) - 2 Ctt(r, p, q) Cxy(r, p, \\
& q) D_2(Cxx)(r, p, q) D_1(Cty)(r, p, q) - 4 Cxy(r, p, q) Cty(r, p, q) D_2(Ctt)(r, p, \\
& q) D_2(Ctx)(r, p, q) - 4 Cxy(r, p, q) Ctx(r, p, q) D_1(Ctt)(r, p, q) D_2(Cxy)(r, p, q) \\
& + 2 Cxx(r, p, q) Cty(r, p, q) D_3(Ctt)(r, p, q) D_2(Ctx)(r, p, q) - 4 Cxx(r, p, q) Ctt(r, p, \\
& q) D_2(Ctx)(r, p, q) D_3(Cty)(r, p, q) \big), D_{1,3}(Ctx)(r, p, q) = -\frac{1}{4} \frac{1}{HessUniv} \big(
\end{aligned}$$

$$\begin{aligned}
& -2 C_{xx}(r, p, q) D_3(C_{tt})(r, p, q) D_1(C_{tx})(r, p, q) + 2 C_{xx}(r, p, q) D_2(C_{tt})(r, p, \\
& q) D_1(C_{ty})(r, p, q) + 4 C_{tx}(r, p, q) D_2(C_{tt})(r, p, q) D_1(C_{xy})(r, p, q) - 2 C_{xy}(r, p, \\
& q) D_2(C_{tt})(r, p, q) D_1(C_{tx})(r, p, q) + 4 C_{ty}(r, p, q)^2 D_3(C_{xx})(r, p, q) D_1(C_{tx})(r, p, q) \\
& - 8 C_{tx}(r, p, q)^2 D_3(C_{ty})(r, p, q) D_1(C_{xy})(r, p, q) + 4 C_{tt}(r, p, q) C_{xy}(r, p, \\
& q) D_3(C_{tx})(r, p, q)^2 + 4 C_{xy}(r, p, q)^2 D_3(C_{tt})(r, p, q) D_1(C_{tx})(r, p, q) + 4 C_{ty}(r, p, \\
& q) D_2(C_{tx})(r, p, q) D_1(C_{tx})(r, p, q) + 4 C_{tx}(r, p, q) D_3(C_{tx})(r, p, q) D_1(C_{tx})(r, p, q) \\
& - 4 C_{tx}(r, p, q) D_2(C_{tx})(r, p, q) D_1(C_{ty})(r, p, q) - 4 C_{tt}(r, p, q) D_2(C_{tx})(r, p, \\
& q) D_1(C_{xy})(r, p, q) - 4 C_{tt}(r, p, q) D_2(C_{tx})(r, p, q) D_3(C_{tx})(r, p, q) + 4 C_{tt}(r, p, \\
& q) D_2(C_{tx})(r, p, q) D_2(C_{ty})(r, p, q) - 2 C_{ty}(r, p, q) D_1(C_{xx})(r, p, q) D_1(C_{tx})(r, p, q) \\
& - 2 C_{ty}(r, p, q) D_2(C_{tt})(r, p, q) D_2(C_{tx})(r, p, q) + 2 C_{tx}(r, p, q) D_3(C_{tt})(r, p, \\
& q) D_2(C_{tx})(r, p, q) - 2 C_{xx}(r, p, q) D_1(C_{tt})(r, p, q) D_3(C_{tx})(r, p, q) - 2 C_{xx}(r, p, \\
& q) D_1(C_{tt})(r, p, q) D_2(C_{ty})(r, p, q) - 4 C_{tx}(r, p, q) D_1(C_{tt})(r, p, q) D_2(C_{xy})(r, p, q) \\
& + 2 C_{tx}(r, p, q) D_2(C_{tt})(r, p, q) D_3(C_{tx})(r, p, q) + 2 C_{xy}(r, p, q) D_1(C_{tt})(r, p, \\
& q) D_2(C_{tx})(r, p, q) + 8 C_{tx}(r, p, q)^2 D_3(C_{xy})(r, p, q) D_1(C_{ty})(r, p, q) + 4 C_{tx}(r, p, \\
& q) D_1(C_{xy})(r, p, q) D_1(C_{tx})(r, p, q) + C_{tt}(r, p, q) D_2(C_{tt})(r, p, q) D_3(C_{xx})(r, p, q) \\
& - C_{tt}(r, p, q) D_2(C_{xx})(r, p, q) D_3(C_{tt})(r, p, q) - 2 C_{ty}(r, p, q) D_2(C_{tt})(r, p, \\
& q) D_1(C_{xx})(r, p, q) + 2 C_{ty}(r, p, q) D_2(C_{xx})(r, p, q) D_1(C_{tt})(r, p, q) + C_{tx}(r, p, \\
& q) D_3(C_{tt})(r, p, q) D_1(C_{xx})(r, p, q) - C_{tx}(r, p, q) D_3(C_{xx})(r, p, q) D_1(C_{tt})(r, p, q)
\end{aligned}$$

$$\begin{aligned}
& + 2 Ctt(r, p, q) D_1(Cxx)(r, p, q) D_2(Cty)(r, p, q) - 2 Ctt(r, p, q) D_2(Cxx)(r, p, \\
& q) D_1(Cty)(r, p, q) - 8 Ctx(r, p, q) Cty(r, p, q) D_3(Cxy)(r, p, q) D_1(Ctx)(r, p, q) \\
& + 2 Ctt(r, p, q) Cty(r, p, q) D_1(Cxx)(r, p, q) D_3(Cxy)(r, p, q) + 4 Ctx(r, p, q) Cty(r, p, \\
& q) D_1(Cxx)(r, p, q) D_3(Cty)(r, p, q) - 4 Ctx(r, p, q) Cty(r, p, q) D_3(Cxx)(r, p, \\
& q) D_1(Cty)(r, p, q) + 2 Cxx(r, p, q) Cty(r, p, q) D_3(Ctt)(r, p, q) D_1(Cxy)(r, p, q) \\
& - 2 Ctt(r, p, q) Cty(r, p, q) D_3(Cxx)(r, p, q) D_1(Cxy)(r, p, q) - 2 Ctt(r, p, q) Cty(r, p, \\
& q) D_3(Cxx)(r, p, q) D_3(Ctx)(r, p, q) - 2 Cxx(r, p, q) Cxy(r, p, q) D_3(Ctt)(r, p, \\
& q) D_1(Cty)(r, p, q) - 2 Ctt(r, p, q) Cxy(r, p, q) D_1(Cxx)(r, p, q) D_3(Cty)(r, p, q) \\
& + 2 Ctt(r, p, q) Cxy(r, p, q) D_3(Cxx)(r, p, q) D_1(Cty)(r, p, q) + 4 Ctt(r, p, q) Cty(r, p, \\
& q) D_2(Ctx)(r, p, q) D_3(Cxy)(r, p, q) - 8 Cxy(r, p, q) Cty(r, p, q) D_3(Ctx)(r, p, \\
& q) D_1(Ctx)(r, p, q) - 4 Cxy(r, p, q) Ctx(r, p, q) D_3(Ctt)(r, p, q) D_3(Ctx)(r, p, q) \\
& + 4 Cxx(r, p, q) Cty(r, p, q) D_3(Ctx)(r, p, q) D_1(Cty)(r, p, q) - 2 Cxx(r, p, q) Cty(r, p, \\
& q) D_1(Ctt)(r, p, q) D_3(Cxy)(r, p, q) + 2 Cxx(r, p, q) Cty(r, p, q) D_3(Ctt)(r, p, \\
& q) D_3(Ctx)(r, p, q) + 2 Cxx(r, p, q) Cxy(r, p, q) D_1(Ctt)(r, p, q) D_3(Cty)(r, p, q) \\
& + 8 Ctt(r, p, q) Ctx(r, p, q) D_2(Cxy)(r, p, q) D_3(Cty)(r, p, q) - 4 Ctt(r, p, q) Cxy(r, p, \\
& q) D_2(Ctx)(r, p, q) D_3(Cty)(r, p, q) - 8 Ctt(r, p, q) Ctx(r, p, q) D_2(Cty)(r, p, \\
& q) D_3(Cxy)(r, p, q) + 4 Ctt(r, p, q) Cxy(r, p, q) D_3(Ctx)(r, p, q) D_1(Cxy)(r, p, q) \\
& + 4 Cxy(r, p, q) Ctx(r, p, q) D_1(Ctt)(r, p, q) D_3(Cxy)(r, p, q) - 4 Cxy(r, p, q) Ctx(r, p,
\end{aligned}$$

$$\begin{aligned}
& q) D_3(Ctt)(r, p, q) D_1(Cxy)(r, p, q) \Big), D_{2,2}(Ctx)(r, p, q) = \frac{1}{4} \frac{1}{HessUniv} \Big( 4 Cxx(r, p, \\
& q) Ctt(r, p, q) D_2(Ctx)(r, p, q) D_3(Cxy)(r, p, q) + 4 Cxx(r, p, q) Cxy(r, p, q) D_1(Ctt)(r, \\
& p, q) D_2(Cxy)(r, p, q) - 4 Cxx(r, p, q) Cxy(r, p, q) D_1(Cxy)(r, p, q) D_1(Ctx)(r, p, q) \\
& + 4 Cxx(r, p, q) Cxy(r, p, q) D_3(Ctx)(r, p, q) D_1(Ctx)(r, p, q) - 4 Cxx(r, p, q) Cxy(r, p, \\
& q) D_3(Ctt)(r, p, q) D_2(Ctx)(r, p, q) + 4 Cxx(r, p, q) Cxy(r, p, q) D_2(Cty)(r, p, \\
& q) D_1(Ctx)(r, p, q) - 4 Cxx(r, p, q) Cxy(r, p, q) D_2(Ctt)(r, p, q) D_1(Cxy)(r, p, q) \\
& + 2 Cxx(r, p, q) Cty(r, p, q) D_2(Ctt)(r, p, q) D_3(Cxx)(r, p, q) - 2 Cxx(r, p, q) Cty(r, p, \\
& q) D_2(Cxx)(r, p, q) D_3(Ctt)(r, p, q) + 2 Cxx(r, p, q) Ctt(r, p, q) D_1(Cxx)(r, p, \\
& q) D_3(Cxy)(r, p, q) - 2 Cxx(r, p, q) Ctt(r, p, q) D_3(Cxx)(r, p, q) D_1(Cxy)(r, p, q) \\
& - 2 Cxx(r, p, q) Ctt(r, p, q) D_3(Cxx)(r, p, q) D_3(Ctx)(r, p, q) - 2 Cxx(r, p, q) Ctt(r, p, \\
& q) D_3(Cxx)(r, p, q) D_2(Cty)(r, p, q) + 2 Cxx(r, p, q) Ctt(r, p, q) D_2(Cxx)(r, p, \\
& q) D_3(Cty)(r, p, q) - 2 Cxx(r, p, q) Cxy(r, p, q) D_3(Ctt)(r, p, q) D_1(Cxx)(r, p, q) \\
& + 2 Cxx(r, p, q) Cxy(r, p, q) D_3(Cxx)(r, p, q) D_1(Ctt)(r, p, q) - 4 Ctx(r, p, q) Cty(r, p, \\
& q) D_3(Cxx)(r, p, q) D_2(Ctx)(r, p, q) + 8 Ctx(r, p, q) Cty(r, p, q) D_2(Cxy)(r, p, \\
& q) D_2(Ctx)(r, p, q) + 4 Ctx(r, p, q) Cty(r, p, q) D_2(Cxx)(r, p, q) D_3(Ctx)(r, p, q) \\
& + 4 Ctt(r, p, q) Ctx(r, p, q) D_3(Cxx)(r, p, q) D_2(Cxy)(r, p, q) - 4 Ctt(r, p, q) Ctx(r, p, \\
& q) D_2(Cxx)(r, p, q) D_3(Cxy)(r, p, q) - 4 Ctt(r, p, q) Cxy(r, p, q) D_1(Cxx)(r, p, \\
& q) D_2(Cxy)(r, p, q) - 8 Ctt(r, p, q) Cxy(r, p, q) D_2(Cxy)(r, p, q) D_2(Ctx)(r, p, q)
\end{aligned}$$

$$\begin{aligned}
& + 4 Ctt(r, p, q) Cxy(r, p, q) D_2(Cxx)(r, p, q) D_1(Cxy)(r, p, q) + 4 Cxy(r, p, q) Cty(r, p, \\
& q) D_1(Cxx)(r, p, q) D_2(Ctx)(r, p, q) - 4 Cxy(r, p, q) Cty(r, p, q) D_2(Cxx)(r, p, \\
& q) D_1(Ctx)(r, p, q) - 4 Cxy(r, p, q) Ctx(r, p, q) D_1(Cxx)(r, p, q) D_3(Ctx)(r, p, q) \\
& - 8 Cxy(r, p, q) Ctx(r, p, q) D_1(Cxx)(r, p, q) D_2(Cty)(r, p, q) - 4 Cxy(r, p, q) Ctx(r, p, \\
& q) D_3(Cxx)(r, p, q) D_1(Ctx)(r, p, q) + 8 Cxy(r, p, q) Ctx(r, p, q) D_2(Ctx)(r, p, \\
& q) D_3(Ctx)(r, p, q) - 4 Cxy(r, p, q) Ctx(r, p, q) D_2(Ctt)(r, p, q) D_3(Cxx)(r, p, q) \\
& + 8 Cxy(r, p, q) Ctx(r, p, q) D_2(Cxy)(r, p, q) D_1(Ctx)(r, p, q) + 8 Cxy(r, p, q) Ctx(r, p, \\
& q) D_2(Cxx)(r, p, q) D_1(Cty)(r, p, q) + 4 Cxy(r, p, q) Ctx(r, p, q) D_2(Cxx)(r, p, \\
& q) D_3(Ctt)(r, p, q) + 4 Cxx(r, p, q) Cty(r, p, q) D_3(Cxx)(r, p, q) D_1(Ctx)(r, p, q) \\
& - 4 Cxx(r, p, q) Cty(r, p, q) D_2(Ctx)(r, p, q) D_1(Cxy)(r, p, q) - 4 Cxx(r, p, q) Cty(r, p, \\
& q) D_2(Ctx)(r, p, q) D_3(Ctx)(r, p, q) - 4 Cxx(r, p, q) Cty(r, p, q) D_2(Ctx)(r, p, \\
& q) D_2(Cty)(r, p, q) + 4 Cxx(r, p, q) Ctx(r, p, q) D_1(Cxx)(r, p, q) D_3(Cty)(r, p, q) \\
& + 4 Cxx(r, p, q) Ctx(r, p, q) D_3(Ctx)(r, p, q) D_1(Cxy)(r, p, q) - 4 Cxx(r, p, q) Ctx(r, p, \\
& q) D_3(Cxx)(r, p, q) D_1(Cty)(r, p, q) + 8 Cxx(r, p, q) Ctx(r, p, q) D_2(Cty)(r, p, \\
& q) D_1(Cxy)(r, p, q) - 4 Cxx(r, p, q) Ctx(r, p, q) D_2(Cty)(r, p, q) D_3(Ctx)(r, p, q) \\
& + 8 Cxx(r, p, q) Ctx(r, p, q) D_2(Ctx)(r, p, q) D_3(Cty)(r, p, q) - 8 Cxx(r, p, q) Ctx(r, p, \\
& q) D_2(Cxy)(r, p, q) D_1(Cty)(r, p, q) + 2 Cxx(r, p, q) D_2(Ctt)(r, p, q) D_2(Ctx)(r, p, q) \\
& - 2 Cxx(r, p, q)^2 D_1(Ctt)(r, p, q) D_3(Cxy)(r, p, q) + 2 Cxx(r, p, q)^2 D_3(Ctt)(r, p,
\end{aligned}$$

$$\begin{aligned}
& q) D_1(Cxy)(r, p, q) + 2 Cxx(r, p, q)^2 D_3(Ctt)(r, p, q) D_3(Ctx)(r, p, q) + 2 Cxx(r, p, \\
& q)^2 D_3(Ctt)(r, p, q) D_2(Cty)(r, p, q) - 2 Cxx(r, p, q)^2 D_2(Ctt)(r, p, q) D_3(Cty)(r, p, q) \\
& - 4 Cty(r, p, q)^2 D_2(Cxx)(r, p, q) D_2(Ctx)(r, p, q) + 4 Ctx(r, p, q)^2 D_3(Cxx)(r, p, \\
& q) D_3(Ctx)(r, p, q) + 8 Ctx(r, p, q)^2 D_3(Cxx)(r, p, q) D_2(Cty)(r, p, q) - 8 Ctx(r, p, \\
& q)^2 D_2(Cxy)(r, p, q) D_3(Ctx)(r, p, q) - 8 Ctx(r, p, q)^2 D_2(Cxx)(r, p, q) D_3(Cty)(r, p, q) \\
& + 8 Cxy(r, p, q) Cty(r, p, q) D_2(Ctx)(r, p, q)^2 + 4 Cxy(r, p, q)^2 D_1(Cxx)(r, p, \\
& q) D_1(Ctx)(r, p, q) - 8 Cxy(r, p, q)^2 D_2(Ctx)(r, p, q) D_1(Ctx)(r, p, q) + 4 Cxy(r, p, \\
& q)^2 D_2(Ctt)(r, p, q) D_1(Cxx)(r, p, q) - 4 Cxy(r, p, q)^2 D_2(Cxx)(r, p, q) D_1(Ctt)(r, p, q) \\
& + 4 Ctt(r, p, q) D_2(Cxx)(r, p, q) D_2(Ctx)(r, p, q) - 4 Cxx(r, p, q) Ctx(r, p, \\
& q) D_3(Ctx)(r, p, q)^2 + 4 Cxx(r, p, q) D_2(Ctx)(r, p, q) D_1(Ctx)(r, p, q) - Cxx(r, p, \\
& q) D_2(Ctt)(r, p, q) D_1(Cxx)(r, p, q) + Cxx(r, p, q) D_2(Cxx)(r, p, q) D_1(Ctt)(r, p, q) \\
& - 4 Cxx(r, p, q)^2 D_3(Cty)(r, p, q) D_1(Ctx)(r, p, q) - 2 Cxx(r, p, q) D_1(Cxx)(r, p, \\
& q) D_1(Ctx)(r, p, q) - 8 Ctx(r, p, q) D_2(Ctx)(r, p, q)^2), D_{2,3}(Ctx)(r, p, q) = \\
& - \frac{1}{4} \frac{1}{HessUniv} \left( -4 Ctx(r, p, q) Cty(r, p, q) D_3(Cxx)(r, p, q) D_2(Cty)(r, p, q) + 4 Ctx(r, \\
& p, q) Cty(r, p, q) D_2(Cxx)(r, p, q) D_3(Cty)(r, p, q) - 8 Cxy(r, p, q) Ctx(r, p, \\
& q) D_2(Ctx)(r, p, q) D_3(Cty)(r, p, q) + 4 Cxx(r, p, q) Cty(r, p, q) D_2(Cty)(r, p, \\
& q) D_3(Ctx)(r, p, q) - 8 Cxx(r, p, q) Ctx(r, p, q) D_3(Cty)(r, p, q) D_1(Cxy)(r, p, q) \right. \\
& \left. + 2 Cxx(r, p, q) Cxy(r, p, q) D_2(Ctt)(r, p, q) D_3(Cty)(r, p, q) - 4 Cxx(r, p, q) Cty(r, p, \right.
\end{aligned}$$



$$\begin{aligned}
& q) D_3(Cxy)(r, p, q) D_1(Ctx)(r, p, q) + 8 Cxx(r, p, q) Ctx(r, p, q) D_3(Cxy)(r, p, \\
& q) D_1(Cty)(r, p, q) + 4 Cxx(r, p, q) Cxy(r, p, q) D_3(Cty)(r, p, q) D_1(Ctx)(r, p, q) \\
& - 2 Ctt(r, p, q) Cty(r, p, q) D_3(Cxx)(r, p, q) D_2(Cxy)(r, p, q) + 2 Ctt(r, p, q) Cty(r, p, \\
& q) D_2(Cxx)(r, p, q) D_3(Cxy)(r, p, q) + 2 Ctt(r, p, q) Cxy(r, p, q) D_3(Cxx)(r, p, \\
& q) D_3(Ctx)(r, p, q) + 2 Ctt(r, p, q) Cxy(r, p, q) D_3(Cxx)(r, p, q) D_2(Cty)(r, p, q) \\
& - 2 Ctt(r, p, q) Cxy(r, p, q) D_2(Cxx)(r, p, q) D_3(Cty)(r, p, q) + 2 Cxx(r, p, q) Cty(r, p, \\
& q) D_3(Ctt)(r, p, q) D_2(Cxy)(r, p, q) - 2 Cxx(r, p, q) Cty(r, p, q) D_2(Ctt)(r, p, \\
& q) D_3(Cxy)(r, p, q) - 2 Cxx(r, p, q) Cxy(r, p, q) D_3(Ctt)(r, p, q) D_3(Ctx)(r, p, q) \\
& - 2 Cxx(r, p, q) Cxy(r, p, q) D_3(Ctt)(r, p, q) D_2(Cty)(r, p, q) - 4 Ctx(r, p, q) Cty(r, p, \\
& q) D_3(Cxx)(r, p, q) D_3(Ctx)(r, p, q) + 4 Ctt(r, p, q) Cxy(r, p, q) D_2(Cxy)(r, p, \\
& q) D_3(Ctx)(r, p, q) - 8 Cxy(r, p, q) Cty(r, p, q) D_2(Ctx)(r, p, q) D_3(Ctx)(r, p, q) \\
& - 4 Cxy(r, p, q) Ctx(r, p, q) D_3(Ctt)(r, p, q) D_2(Cxy)(r, p, q) + 4 Cxy(r, p, q) Ctx(r, p, \\
& q) D_2(Ctt)(r, p, q) D_3(Cxy)(r, p, q) + 4 Cty(r, p, q)^2 D_3(Cxx)(r, p, q) D_2(Ctx)(r, p, q) \\
& - 8 Ctx(r, p, q)^2 D_2(Cty)(r, p, q) D_3(Cxy)(r, p, q) + 4 Cxy(r, p, q)^2 D_3(Ctt)(r, p, \\
& q) D_2(Ctx)(r, p, q) + 4 Ctx(r, p, q) D_1(Cxx)(r, p, q) D_2(Cty)(r, p, q) + 4 Ctx(r, p, \\
& q) D_2(Ctx)(r, p, q) D_3(Ctx)(r, p, q) - 4 Ctx(r, p, q) D_2(Cxy)(r, p, q) D_1(Ctx)(r, p, q) \\
& - 4 Ctx(r, p, q) D_2(Cxx)(r, p, q) D_1(Cty)(r, p, q) + 4 Cxy(r, p, q) D_2(Ctx)(r, p, \\
& q) D_1(Ctx)(r, p, q) + 4 Cxx(r, p, q) Cty(r, p, q) D_3(Ctx)(r, p, q)^2 + 4 Cxx(r, p,
\end{aligned}$$

$$\begin{aligned}
& q) D_1(Cxy)(r, p, q) D_1(Ctx)(r, p, q) - 4 Cxx(r, p, q) D_3(Ctx)(r, p, q) D_1(Ctx)(r, p, q) \\
& - 4 Cxx(r, p, q) D_2(Cty)(r, p, q) D_1(Ctx)(r, p, q) - 2 Cty(r, p, q) D_1(Cxx)(r, p, \\
& q) D_2(Ctx)(r, p, q) + 2 Cty(r, p, q) D_2(Cxx)(r, p, q) D_1(Ctx)(r, p, q) + 2 Ctx(r, p, \\
& q) D_1(Cxx)(r, p, q) D_3(Ctx)(r, p, q) + 2 Ctx(r, p, q) D_3(Cxx)(r, p, q) D_1(Ctx)(r, p, q) \\
& + 2 Ctt(r, p, q) D_1(Cxx)(r, p, q) D_2(Cxy)(r, p, q) - 2 Ctt(r, p, q) D_3(Cxx)(r, p, \\
& q) D_2(Ctx)(r, p, q) - 2 Ctt(r, p, q) D_2(Cxx)(r, p, q) D_1(Cxy)(r, p, q) - 2 Ctt(r, p, \\
& q) D_2(Cxx)(r, p, q) D_3(Ctx)(r, p, q) - 2 Cxy(r, p, q) D_1(Cxx)(r, p, q) D_1(Ctx)(r, p, q) \\
& - 2 Cxy(r, p, q) D_2(Ctt)(r, p, q) D_2(Ctx)(r, p, q) + 4 Ctx(r, p, q) D_2(Ctx)(r, p, \\
& q) D_2(Cty)(r, p, q) + Cxx(r, p, q) D_3(Ctt)(r, p, q) D_1(Cxx)(r, p, q) - Cxx(r, p, \\
& q) D_3(Cxx)(r, p, q) D_1(Ctt)(r, p, q) + Ctx(r, p, q) D_2(Ctt)(r, p, q) D_3(Cxx)(r, p, q) \\
& - Ctx(r, p, q) D_2(Cxx)(r, p, q) D_3(Ctt)(r, p, q) - 2 Cxy(r, p, q) D_2(Ctt)(r, p, \\
& q) D_1(Cxx)(r, p, q) + 2 Cxy(r, p, q) D_2(Cxx)(r, p, q) D_1(Ctt)(r, p, q) - 2 Cxx(r, p, \\
& q) D_1(Ctt)(r, p, q) D_2(Cxy)(r, p, q) + 2 Cxx(r, p, q) D_2(Ctt)(r, p, q) D_1(Cxy)(r, p, q) \\
& + 8 Ctx(r, p, q)^2 D_2(Cxy)(r, p, q) D_3(Cty)(r, p, q) \Big), D_{3,3}(Ctx)(r, p, q) = \\
& - \frac{1}{4} \frac{1}{HessUniv} \Big( -4 Ctt(r, p, q) D_2(Ctx)(r, p, q) D_3(Cxy)(r, p, q) + 4 Cxy(r, p, \\
& q) D_1(Cxy)(r, p, q) D_1(Ctx)(r, p, q) - 4 Cxy(r, p, q) D_3(Ctx)(r, p, q) D_1(Ctx)(r, p, q) \\
& - 4 Cxy(r, p, q) D_2(Cty)(r, p, q) D_1(Ctx)(r, p, q) - 4 Cxx(r, p, q) D_3(Cty)(r, p, \\
& q) D_1(Ctx)(r, p, q) - 2 Cxx(r, p, q) D_3(Ctt)(r, p, q) D_3(Ctx)(r, p, q) - 2 Cxx(r, p,
\end{aligned}$$

$$\begin{aligned}
& q) D_3(Ctt)(r, p, q) D_2(Cty)(r, p, q) + 2 Cxx(r, p, q) D_2(Ctt)(r, p, q) D_3(Cty)(r, p, q) \\
& + 8 Cty(r, p, q)^2 D_2(Ctx)(r, p, q) D_3(Cxy)(r, p, q) + 8 Cxy(r, p, q)^2 D_3(Cty)(r, p, \\
& q) D_1(Ctx)(r, p, q) - 4 Cty(r, p, q) D_2(Ctx)(r, p, q) D_1(Cxy)(r, p, q) - 4 Cty(r, p, \\
& q) D_2(Ctx)(r, p, q) D_3(Ctx)(r, p, q) + 4 Cty(r, p, q) D_2(Ctx)(r, p, q) D_2(Cty)(r, p, q) \\
& + 8 Ctx(r, p, q) D_2(Cty)(r, p, q) D_1(Cxy)(r, p, q) + 2 Ctt(r, p, q) D_1(Cxx)(r, p, \\
& q) D_3(Cxy)(r, p, q) - 2 Ctt(r, p, q) D_3(Cxx)(r, p, q) D_1(Cxy)(r, p, q) - 2 Ctt(r, p, \\
& q) D_3(Cxx)(r, p, q) D_3(Ctx)(r, p, q) + 8 Cxx(r, p, q) Cty(r, p, q) D_3(Ctx)(r, p, \\
& q) D_3(Cty)(r, p, q) - 16 Ctx(r, p, q) Cty(r, p, q) D_2(Cty)(r, p, q) D_3(Cxy)(r, p, q) \\
& + 16 Ctx(r, p, q) Cty(r, p, q) D_2(Cxy)(r, p, q) D_3(Cty)(r, p, q) - 8 Cxy(r, p, q) Cty(r, p, \\
& q) D_2(Ctx)(r, p, q) D_3(Cty)(r, p, q) + 4 Cty(r, p, q) D_3(Cxx)(r, p, q) D_1(Ctx)(r, p, q) \\
& + 4 Ctx(r, p, q) D_3(Ctx)(r, p, q) D_1(Cxy)(r, p, q) + 4 Ctx(r, p, q) D_1(Cxx)(r, p, \\
& q) D_3(Cty)(r, p, q) - 4 Ctx(r, p, q) D_3(Ctt)(r, p, q) D_2(Cxy)(r, p, q) - 4 Ctx(r, p, \\
& q) D_3(Cxx)(r, p, q) D_1(Cty)(r, p, q) + 4 Ctx(r, p, q) D_2(Ctt)(r, p, q) D_3(Cxy)(r, p, q) \\
& + 2 Ctt(r, p, q) D_3(Cxx)(r, p, q) D_2(Cty)(r, p, q) - 2 Ctt(r, p, q) D_2(Cxx)(r, p, \\
& q) D_3(Cty)(r, p, q) + 4 Cxy(r, p, q) D_3(Ctt)(r, p, q) D_2(Ctx)(r, p, q) - 2 Cxx(r, p, \\
& q) D_1(Ctt)(r, p, q) D_3(Cxy)(r, p, q) + 2 Cxx(r, p, q) D_3(Ctt)(r, p, q) D_1(Cxy)(r, p, q) \\
& + 4 Ctx(r, p, q) D_2(Cty)(r, p, q) D_3(Ctx)(r, p, q) - 8 Ctx(r, p, q) D_2(Cxy)(r, p, \\
& q) D_1(Cty)(r, p, q) + 8 Ctt(r, p, q) Cxy(r, p, q) D_3(Cxy)(r, p, q) D_3(Ctx)(r, p, q)
\end{aligned}$$

$$\begin{aligned}
& -8 Cxy(r, p, q) Cty(r, p, q) D_3(Cxy)(r, p, q) D_1(Ctx)(r, p, q) - 16 Cxy(r, p, q) Ctx(r, p, \\
& q) D_3(Cty)(r, p, q) D_1(Cxy)(r, p, q) + 16 Cxy(r, p, q) Ctx(r, p, q) D_3(Cxy)(r, p, \\
& q) D_1(Cty)(r, p, q) + 4 Ctx(r, p, q) D_3(Ctx)(r, p, q)^2 + 4 D_2(Ctx)(r, p, q) D_1(Ctx)(r, p, \\
& q) - 2 D_1(Cxx)(r, p, q) D_1(Ctx)(r, p, q) - 2 D_2(Ctt)(r, p, q) D_2(Ctx)(r, p, q) \\
& - D_2(Ctt)(r, p, q) D_1(Cxx)(r, p, q) + D_2(Cxx)(r, p, q) D_1(Ctt)(r, p, q) - 8 Ctx(r, p, \\
& q) Cty(r, p, q) D_3(Cxy)(r, p, q) D_3(Ctx)(r, p, q) - 8 Cxy(r, p, q) Ctx(r, p, q) D_3(Ctx)(r, \\
& p, q) D_3(Cty)(r, p, q) \Big), D_{1,1}(Cty)(r, p, q) = \frac{1}{4} \frac{1}{HessUniv} \Big( -Ctt(r, p, q) D_3(Cxx)(r, \\
& p, q) D_1(Ctt)(r, p, q) - 8 Cxx(r, p, q) Cty(r, p, q) D_1(Cty)(r, p, q)^2 + 4 Cxx(r, p, \\
& q) D_1(Ctt)(r, p, q) D_1(Cty)(r, p, q) - 8 Cty(r, p, q)^2 D_2(Cty)(r, p, q) D_1(Ctx)(r, p, q) \\
& + 4 Cty(r, p, q)^2 D_2(Ctt)(r, p, q) D_2(Cty)(r, p, q) - 8 Ctx(r, p, q)^2 D_3(Cty)(r, p, \\
& q) D_1(Cty)(r, p, q) + 4 Ctx(r, p, q)^2 D_3(Ctt)(r, p, q) D_3(Cty)(r, p, q) - 4 Ctt(r, p, \\
& q) Cty(r, p, q) D_2(Cty)(r, p, q)^2 + 8 Cxy(r, p, q) Ctx(r, p, q) D_1(Cty)(r, p, q)^2 \\
& - 4 Cxy(r, p, q)^2 D_1(Ctt)(r, p, q) D_1(Cty)(r, p, q) - 8 Ctx(r, p, q) D_1(Ctx)(r, p, \\
& q) D_1(Cty)(r, p, q) + 4 Ctx(r, p, q) D_1(Ctt)(r, p, q) D_3(Ctx)(r, p, q) + Ctt(r, p, \\
& q) D_3(Ctt)(r, p, q) D_1(Cxx)(r, p, q) + 2 Ctt(r, p, q) D_1(Cxx)(r, p, q) D_1(Cty)(r, p, q) \\
& - 2 Ctt(r, p, q) D_2(Ctt)(r, p, q) D_1(Cxy)(r, p, q) - 2 Ctt(r, p, q) D_2(Ctt)(r, p, \\
& q) D_3(Ctx)(r, p, q) + 2 Ctt(r, p, q)^2 D_3(Cxx)(r, p, q) D_3(Cty)(r, p, q) + 4 Ctt(r, p, \\
& q) Ctx(r, p, q) D_3(Cty)(r, p, q) D_1(Cxy)(r, p, q) - 4 Ctt(r, p, q) Cxy(r, p, q) D_3(Ctx)(r,
\end{aligned}$$

$$\begin{aligned}
& p, q) D_1(Cty)(r, p, q) - 4 Cxy(r, p, q) Ctx(r, p, q) D_1(Ctt)(r, p, q) D_3(Cty)(r, p, q) \\
& + 4 Cxy(r, p, q) Ctx(r, p, q) D_3(Ctt)(r, p, q) D_1(Cty)(r, p, q) - 4 Ctt(r, p, q) Cty(r, p, \\
& q) D_1(Cxx)(r, p, q) D_3(Cty)(r, p, q) + 4 Ctt(r, p, q) Cxy(r, p, q) D_2(Ctt)(r, p, \\
& q) D_3(Cty)(r, p, q) + 4 Cty(r, p, q) D_2(Ctt)(r, p, q) D_1(Ctx)(r, p, q) - 4 Ctx(r, p, \\
& q) D_3(Ctt)(r, p, q) D_1(Ctx)(r, p, q) + 2 Ctt(r, p, q) D_1(Ctt)(r, p, q) D_2(Cxy)(r, p, q) \\
& + 2 Ctt(r, p, q) D_3(Ctt)(r, p, q) D_2(Ctx)(r, p, q) - 2 Ctt(r, p, q) D_2(Ctt)(r, p, \\
& q) D_2(Cty)(r, p, q) - 4 Ctt(r, p, q)^2 D_2(Cxy)(r, p, q) D_3(Cty)(r, p, q) - 4 Cty(r, p, \\
& q) D_1(Ctt)(r, p, q) D_2(Ctx)(r, p, q) + 4 Ctt(r, p, q) D_2(Ctx)(r, p, q) D_1(Cty)(r, p, q) \\
& + 8 Ctx(r, p, q) Cty(r, p, q) D_3(Cty)(r, p, q) D_1(Ctx)(r, p, q) - 4 Ctx(r, p, q) Cty(r, p, \\
& q) D_3(Ctt)(r, p, q) D_2(Cty)(r, p, q) + 8 Ctx(r, p, q) Cty(r, p, q) D_2(Cty)(r, p, \\
& q) D_1(Cty)(r, p, q) - 4 Ctx(r, p, q) Cty(r, p, q) D_2(Ctt)(r, p, q) D_3(Cty)(r, p, q) \\
& + 4 Ctt(r, p, q) Cty(r, p, q) D_2(Cty)(r, p, q) D_1(Cxy)(r, p, q) + 4 Ctt(r, p, q) Cty(r, p, \\
& q) D_2(Cty)(r, p, q) D_3(Ctx)(r, p, q) - 4 Ctt(r, p, q) Ctx(r, p, q) D_3(Ctx)(r, p, \\
& q) D_3(Cty)(r, p, q) + 4 Ctt(r, p, q) Ctx(r, p, q) D_2(Cty)(r, p, q) D_3(Cty)(r, p, q) \\
& - 4 Ctt(r, p, q) Cxy(r, p, q) D_1(Cxy)(r, p, q) D_1(Cty)(r, p, q) - 4 Ctt(r, p, q) Cxy(r, p, \\
& q) D_2(Cty)(r, p, q) D_1(Cty)(r, p, q) + 8 Cxy(r, p, q) Cty(r, p, q) D_1(Ctx)(r, p, \\
& q) D_1(Cty)(r, p, q) + 4 Cxy(r, p, q) Cty(r, p, q) D_1(Ctt)(r, p, q) D_2(Cty)(r, p, q) \\
& - 4 Cxy(r, p, q) Cty(r, p, q) D_2(Ctt)(r, p, q) D_1(Cty)(r, p, q) + 4 Cxx(r, p, q) Ctt(r, p,
\end{aligned}$$

$$\begin{aligned}
& q) D_3(Cty)(r, p, q) D_1(Cty)(r, p, q) - 2 Cxx(r, p, q) Ctt(r, p, q) D_3(Ctt)(r, p, \\
& q) D_3(Cty)(r, p, q) \Big), D_{1,2}(Cty)(r, p, q) = \frac{1}{4} \frac{1}{HessUniv} \Big( -4 Cty(r, p, q)^2 D_1(Cxx)(r, \\
& p, q) D_2(Cty)(r, p, q) - 4 Ctt(r, p, q) Cxy(r, p, q) D_2(Cty)(r, p, q)^2 - 4 Cxy(r, p, \\
& q)^2 D_2(Ctt)(r, p, q) D_1(Cty)(r, p, q) - 4 Ctx(r, p, q) D_2(Cty)(r, p, q) D_1(Ctx)(r, p, q) \\
& - 2 Cxx(r, p, q) D_3(Ctt)(r, p, q) D_1(Ctx)(r, p, q) + 2 Cxx(r, p, q) D_2(Ctt)(r, p, \\
& q) D_1(Cty)(r, p, q) - 2 Ctx(r, p, q) D_1(Cxx)(r, p, q) D_1(Cty)(r, p, q) - 2 Ctx(r, p, \\
& q) D_2(Ctt)(r, p, q) D_1(Cxy)(r, p, q) + 2 Cxy(r, p, q) D_2(Ctt)(r, p, q) D_1(Ctx)(r, p, q) \\
& + 2 Cxx(r, p, q) D_1(Ctt)(r, p, q) D_3(Ctx)(r, p, q) + 2 Cxx(r, p, q) D_1(Ctt)(r, p, \\
& q) D_2(Cty)(r, p, q) + 2 Ctx(r, p, q) D_1(Ctt)(r, p, q) D_2(Cxy)(r, p, q) - 2 Ctx(r, p, \\
& q) D_2(Ctt)(r, p, q) D_2(Cty)(r, p, q) - 2 Cxy(r, p, q) D_1(Ctt)(r, p, q) D_2(Ctx)(r, p, q) \\
& - Ctt(r, p, q) D_2(Ctt)(r, p, q) D_3(Cxx)(r, p, q) + Ctt(r, p, q) D_2(Cxx)(r, p, \\
& q) D_3(Ctt)(r, p, q) + Cty(r, p, q) D_2(Ctt)(r, p, q) D_1(Cxx)(r, p, q) - Cty(r, p, \\
& q) D_2(Cxx)(r, p, q) D_1(Ctt)(r, p, q) + 2 Ctt(r, p, q) D_1(Cxx)(r, p, q) D_2(Cty)(r, p, q) \\
& + 2 Ctt(r, p, q) D_2(Cxx)(r, p, q) D_1(Cty)(r, p, q) + 8 Ctx(r, p, q) Cty(r, p, q) D_2(Cty)(r, \\
& p, q) D_1(Cxy)(r, p, q) + 4 Cxy(r, p, q) Cty(r, p, q) D_1(Cxx)(r, p, q) D_1(Cty)(r, p, q) \\
& + 4 Cxy(r, p, q) Cty(r, p, q) D_2(Ctt)(r, p, q) D_2(Cty)(r, p, q) + 8 Cxy(r, p, q) Ctx(r, p, \\
& q) D_2(Cty)(r, p, q) D_1(Cty)(r, p, q) + 4 Cxx(r, p, q) Cty(r, p, q) D_3(Cty)(r, p, \\
& q) D_1(Ctx)(r, p, q) - 4 Cxx(r, p, q) Cty(r, p, q) D_2(Cty)(r, p, q) D_1(Cty)(r, p, q)
\end{aligned}$$

$$\begin{aligned}
& -4 C_{xx}(r, p, q) C_{tx}(r, p, q) D_3(C_{ty})(r, p, q) D_1(C_{ty})(r, p, q) -4 C_{xx}(r, p, q) C_{tt}(r, p, \\
& q) D_3(C_{tx})(r, p, q) D_3(C_{ty})(r, p, q) +4 C_{xx}(r, p, q) C_{tt}(r, p, q) D_2(C_{ty})(r, p, \\
& q) D_3(C_{ty})(r, p, q) -2 C_{xx}(r, p, q) C_{ty}(r, p, q) D_2(C_{tt})(r, p, q) D_3(C_{ty})(r, p, q) \\
& +2 C_{xx}(r, p, q) C_{tx}(r, p, q) D_3(C_{tt})(r, p, q) D_3(C_{ty})(r, p, q) +2 C_{xx}(r, p, q) C_{xy}(r, p, \\
& q) D_3(C_{tt})(r, p, q) D_1(C_{ty})(r, p, q) +2 C_{tt}(r, p, q) C_{tx}(r, p, q) D_3(C_{xx})(r, p, \\
& q) D_3(C_{ty})(r, p, q) -2 C_{tt}(r, p, q) C_{xy}(r, p, q) D_1(C_{xx})(r, p, q) D_3(C_{ty})(r, p, q) \\
& -2 C_{tt}(r, p, q) C_{xy}(r, p, q) D_3(C_{xx})(r, p, q) D_1(C_{ty})(r, p, q) +4 C_{xx}(r, p, q) C_{tt}(r, p, \\
& q) D_3(C_{ty})(r, p, q) D_1(C_{xy})(r, p, q) +2 C_{tt}(r, p, q) C_{ty}(r, p, q) D_3(C_{xx})(r, p, \\
& q) D_2(C_{ty})(r, p, q) -2 C_{tt}(r, p, q) C_{ty}(r, p, q) D_2(C_{xx})(r, p, q) D_3(C_{ty})(r, p, q) \\
& -2 C_{xx}(r, p, q) C_{ty}(r, p, q) D_3(C_{tt})(r, p, q) D_2(C_{ty})(r, p, q) -2 C_{xx}(r, p, q) C_{xy}(r, p, \\
& q) D_1(C_{tt})(r, p, q) D_3(C_{ty})(r, p, q) -4 C_{tt}(r, p, q) C_{tx}(r, p, q) D_2(C_{xy})(r, p, \\
& q) D_3(C_{ty})(r, p, q) +4 C_{tt}(r, p, q) C_{xy}(r, p, q) D_2(C_{tx})(r, p, q) D_3(C_{ty})(r, p, q) \\
& -4 C_{tt}(r, p, q) C_{xy}(r, p, q) D_2(C_{ty})(r, p, q) D_1(C_{xy})(r, p, q) -4 C_{xx}(r, p, q) C_{ty}(r, p, \\
& q) D_1(C_{xy})(r, p, q) D_1(C_{ty})(r, p, q) \Big), D_{1,3}(C_{ty})(r, p, q) = \frac{1}{4} \frac{1}{HessUniv} \Big( 2 C_{xx}(r, \\
& p, q) D_3(C_{tt})(r, p, q) D_1(C_{ty})(r, p, q) -4 C_{ty}(r, p, q)^2 D_1(C_{xx})(r, p, q) D_3(C_{ty})(r, p, q) \\
& + C_{ty}(r, p, q) D_3(C_{tt})(r, p, q) D_1(C_{xx})(r, p, q) -4 C_{ty}(r, p, q) D_2(C_{ty})(r, p, \\
& q) D_1(C_{tx})(r, p, q) -4 C_{tx}(r, p, q) D_1(C_{xy})(r, p, q) D_1(C_{ty})(r, p, q) -4 C_{tx}(r, p, \\
& q) D_3(C_{ty})(r, p, q) D_1(C_{tx})(r, p, q) +4 C_{tx}(r, p, q) D_2(C_{ty})(r, p, q) D_1(C_{ty})(r, p, q)
\end{aligned}$$

$$\begin{aligned}
& + 2 Ctx(r, p, q) D_1(Ctt)(r, p, q) D_3(Cxy)(r, p, q) - 2 Ctt(r, p, q) D_2(Ctt)(r, p, \\
& q) D_3(Cxy)(r, p, q) - 2 Cxy(r, p, q) D_3(Ctt)(r, p, q) D_1(Ctx)(r, p, q) - 2 Cxy(r, p, \\
& q) D_2(Ctt)(r, p, q) D_1(Cty)(r, p, q) + 2 Cty(r, p, q) D_1(Cxx)(r, p, q) D_1(Cty)(r, p, q) \\
& - Cty(r, p, q) D_3(Cxx)(r, p, q) D_1(Ctt)(r, p, q) + 2 Cty(r, p, q) D_2(Ctt)(r, p, \\
& q) D_2(Cty)(r, p, q) - 2 Ctx(r, p, q) D_3(Ctt)(r, p, q) D_1(Cxy)(r, p, q) - 2 Ctx(r, p, \\
& q) D_3(Ctt)(r, p, q) D_2(Cty)(r, p, q) + 2 Ctt(r, p, q) D_3(Ctt)(r, p, q) D_2(Cxy)(r, p, q) \\
& + 4 Ctt(r, p, q) D_2(Ctx)(r, p, q) D_3(Cty)(r, p, q) + 4 Ctt(r, p, q) D_2(Cxy)(r, p, \\
& q) D_1(Cty)(r, p, q) + 2 Cxy(r, p, q) D_1(Ctt)(r, p, q) D_3(Ctx)(r, p, q) + 2 Cxy(r, p, \\
& q) D_1(Ctt)(r, p, q) D_2(Cty)(r, p, q) + 2 Cxx(r, p, q) D_1(Ctt)(r, p, q) D_3(Cty)(r, p, q) \\
& - 4 Cxy(r, p, q)^2 D_1(Ctt)(r, p, q) D_3(Cty)(r, p, q) - 2 Ctx(r, p, q) D_2(Ctt)(r, p, \\
& q) D_3(Cty)(r, p, q) - 2 D_1(Ctt)(r, p, q) D_2(Ctx)(r, p, q) - 4 Ctt(r, p, q) D_2(Cty)(r, p, q)^2 \\
& + 2 D_2(Ctt)(r, p, q) D_1(Ctx)(r, p, q) - 4 Cxx(r, p, q) Cty(r, p, q) D_3(Cty)(r, p, \\
& q) D_1(Cty)(r, p, q) + 8 Ctx(r, p, q) Cty(r, p, q) D_3(Cty)(r, p, q) D_1(Cxy)(r, p, q) \\
& - 4 Ctt(r, p, q) Cxy(r, p, q) D_3(Ctx)(r, p, q) D_3(Cty)(r, p, q) + 4 Ctt(r, p, q) Cxy(r, p, \\
& q) D_2(Cty)(r, p, q) D_3(Cty)(r, p, q) + 8 Cxy(r, p, q) Cty(r, p, q) D_3(Cty)(r, p, \\
& q) D_1(Ctx)(r, p, q) + 2 Ctt(r, p, q) Cty(r, p, q) D_3(Cxx)(r, p, q) D_3(Cty)(r, p, q) \\
& + 4 Ctt(r, p, q) Cty(r, p, q) D_2(Cty)(r, p, q) D_3(Cxy)(r, p, q) - 8 Ctt(r, p, q) Cty(r, p, \\
& q) D_2(Cxy)(r, p, q) D_3(Cty)(r, p, q) - 4 Ctt(r, p, q) Cxy(r, p, q) D_3(Cxy)(r, p,
\end{aligned}$$



$$\begin{aligned}
& q) D_1(Cty)(r, p, q) + 4 Cxy(r, p, q) Ctx(r, p, q) D_3(Ctt)(r, p, q) D_3(Cty)(r, p, q) \\
& - 2 Cxx(r, p, q) Cty(r, p, q) D_3(Ctt)(r, p, q) D_3(Cty)(r, p, q) \Big), D_{2,2}(Cty)(r, p, q) = \\
& - \frac{1}{4} \frac{1}{HessUniv} \Big( -4 Ctx(r, p, q) Cty(r, p, q) D_3(Cxx)(r, p, q) D_2(Cty)(r, p, q) - 8 Ctx(r, \\
& p, q) Cty(r, p, q) D_2(Cxy)(r, p, q) D_2(Cty)(r, p, q) + 4 Ctx(r, p, q) Cty(r, p, \\
& q) D_2(Cxx)(r, p, q) D_3(Cty)(r, p, q) + 8 Ctt(r, p, q) Cxy(r, p, q) D_2(Cxy)(r, p, \\
& q) D_2(Cty)(r, p, q) + 4 Cxy(r, p, q) Cty(r, p, q) D_1(Cxx)(r, p, q) D_2(Cty)(r, p, q) \\
& - 8 Cxy(r, p, q) Cty(r, p, q) D_2(Ctx)(r, p, q) D_2(Cty)(r, p, q) - 4 Cxy(r, p, q) Cty(r, p, \\
& q) D_2(Cxx)(r, p, q) D_1(Cty)(r, p, q) + 4 Cxy(r, p, q) Ctx(r, p, q) D_1(Cxx)(r, p, \\
& q) D_3(Cty)(r, p, q) + 4 Cxy(r, p, q) Ctx(r, p, q) D_3(Cxx)(r, p, q) D_1(Cty)(r, p, q) \\
& - 8 Cxy(r, p, q) Ctx(r, p, q) D_2(Ctx)(r, p, q) D_3(Cty)(r, p, q) - 8 Cxy(r, p, q) Ctx(r, p, \\
& q) D_2(Cxy)(r, p, q) D_1(Cty)(r, p, q) - 4 Cxx(r, p, q) Cty(r, p, q) D_1(Cxx)(r, p, \\
& q) D_3(Cty)(r, p, q) - 4 Cxx(r, p, q) Cty(r, p, q) D_2(Cty)(r, p, q) D_1(Cxy)(r, p, q) \\
& + 4 Cxx(r, p, q) Cty(r, p, q) D_2(Cty)(r, p, q) D_3(Ctx)(r, p, q) + 8 Cxx(r, p, q) Cty(r, p, \\
& q) D_2(Cxy)(r, p, q) D_1(Cty)(r, p, q) - 4 Cxx(r, p, q) Ctx(r, p, q) D_3(Cty)(r, p, \\
& q) D_1(Cxy)(r, p, q) + 4 Cxx(r, p, q) Ctx(r, p, q) D_3(Ctx)(r, p, q) D_3(Cty)(r, p, q) \\
& - 4 Cxx(r, p, q) Ctx(r, p, q) D_2(Cty)(r, p, q) D_3(Cty)(r, p, q) - 4 Cxx(r, p, q) Ctt(r, p, \\
& q) D_2(Cxy)(r, p, q) D_3(Cty)(r, p, q) + 4 Cxx(r, p, q) Cxy(r, p, q) D_1(Cxy)(r, p, \\
& q) D_1(Cty)(r, p, q) - 4 Cxx(r, p, q) Cxy(r, p, q) D_3(Ctx)(r, p, q) D_1(Cty)(r, p, q)
\end{aligned}$$

$$\begin{aligned}
& -4 C_{xx}(r, p, q) C_{xy}(r, p, q) D_2(Cty)(r, p, q) D_1(Cty)(r, p, q) + 4 C_{xx}(r, p, q) C_{xy}(r, p, \\
& q) D_2(Ctt)(r, p, q) D_3(Cty)(r, p, q) + 2 C_{xx}(r, p, q) C_{tt}(r, p, q) D_3(C_{xx})(r, p, \\
& q) D_3(Cty)(r, p, q) + 8 C_{tx}(r, p, q) D_2(Ctx)(r, p, q) D_2(Cty)(r, p, q) - 4 C_{tt}(r, p, \\
& q) D_2(C_{xx})(r, p, q) D_2(Cty)(r, p, q) + 4 C_{xx}(r, p, q) C_{ty}(r, p, q) D_2(Cty)(r, p, q)^2 \\
& + C_{xx}(r, p, q) D_3(Ctt)(r, p, q) D_1(C_{xx})(r, p, q) - C_{xx}(r, p, q) D_3(C_{xx})(r, p, \\
& q) D_1(Ctt)(r, p, q) - 4 C_{xx}(r, p, q) D_2(Ctx)(r, p, q) D_1(Cty)(r, p, q) + 4 C_{xx}(r, p, \\
& q)^2 D_3(Cty)(r, p, q) D_1(Cty)(r, p, q) + 2 C_{tx}(r, p, q) D_2(Ctt)(r, p, q) D_3(C_{xx})(r, p, q) \\
& - 2 C_{tx}(r, p, q) D_2(C_{xx})(r, p, q) D_3(Ctt)(r, p, q) - 2 C_{xy}(r, p, q) D_2(Ctt)(r, p, \\
& q) D_1(C_{xx})(r, p, q) + 2 C_{xy}(r, p, q) D_2(C_{xx})(r, p, q) D_1(Ctt)(r, p, q) - 2 C_{xx}(r, p, \\
& q) D_1(Ctt)(r, p, q) D_2(C_{xy})(r, p, q) + 2 C_{xx}(r, p, q) D_1(C_{xx})(r, p, q) D_1(Cty)(r, p, q) \\
& + 2 C_{xx}(r, p, q) D_3(Ctt)(r, p, q) D_2(Ctx)(r, p, q) + 2 C_{xx}(r, p, q) D_2(Ctt)(r, p, \\
& q) D_1(C_{xy})(r, p, q) - 2 C_{xx}(r, p, q) D_2(Ctt)(r, p, q) D_3(Ctx)(r, p, q) - 2 C_{xx}(r, p, \\
& q) D_2(Ctt)(r, p, q) D_2(Cty)(r, p, q) - 2 C_{xx}(r, p, q)^2 D_3(Ctt)(r, p, q) D_3(Cty)(r, p, q) \\
& + 4 C_{ty}(r, p, q)^2 D_2(C_{xx})(r, p, q) D_2(Cty)(r, p, q) - 4 C_{tx}(r, p, q)^2 D_3(C_{xx})(r, p, \\
& q) D_3(Cty)(r, p, q) + 8 C_{tx}(r, p, q)^2 D_2(C_{xy})(r, p, q) D_3(Cty)(r, p, q) - 4 C_{xy}(r, p, \\
& q)^2 D_1(C_{xx})(r, p, q) D_1(Cty)(r, p, q) + 8 C_{xy}(r, p, q)^2 D_2(Ctx)(r, p, q) D_1(Cty)(r, p, q) \Big) \\
& , D_{2,3}(Cty)(r, p, q) = \frac{1}{4} \frac{1}{HessUniv} \Big( 8 C_{xx}(r, p, q) C_{ty}(r, p, q) D_3(Cty)(r, p, \\
& q) D_1(C_{xy})(r, p, q) - 4 C_{xx}(r, p, q) C_{ty}(r, p, q) D_3(Ctx)(r, p, q) D_3(Cty)(r, p, q)
\end{aligned}$$

$$\begin{aligned}
& -4 C_{xx}(r, p, q) C_{ty}(r, p, q) D_3(C_{xy})(r, p, q) D_1(C_{ty})(r, p, q) -4 C_{xx}(r, p, q) C_{ty}(r, p, \\
& q) D_2(C_{ty})(r, p, q) D_3(C_{ty})(r, p, q) -4 C_{xx}(r, p, q) C_{xy}(r, p, q) D_3(C_{ty})(r, p, \\
& q) D_1(C_{ty})(r, p, q) -2 C_{tt}(r, p, q) C_{xy}(r, p, q) D_3(C_{xx})(r, p, q) D_3(C_{ty})(r, p, q) \\
& +4 C_{tx}(r, p, q) C_{ty}(r, p, q) D_3(C_{xx})(r, p, q) D_3(C_{ty})(r, p, q) +8 C_{tx}(r, p, q) C_{ty}(r, p, \\
& q) D_2(C_{ty})(r, p, q) D_3(C_{xy})(r, p, q) -8 C_{tx}(r, p, q) C_{ty}(r, p, q) D_2(C_{xy})(r, p, \\
& q) D_3(C_{ty})(r, p, q) -4 C_{tt}(r, p, q) C_{xy}(r, p, q) D_2(C_{ty})(r, p, q) D_3(C_{xy})(r, p, q) \\
& +8 C_{xy}(r, p, q) C_{ty}(r, p, q) D_2(C_{tx})(r, p, q) D_3(C_{ty})(r, p, q) +8 C_{xy}(r, p, q) C_{tx}(r, p, \\
& q) D_2(C_{ty})(r, p, q) D_3(C_{ty})(r, p, q) -4 C_{xx}(r, p, q) D_1(C_{xy})(r, p, q) D_1(C_{ty})(r, p, q) \\
& +4 C_{xx}(r, p, q) D_3(C_{tx})(r, p, q) D_1(C_{ty})(r, p, q) +4 C_{xx}(r, p, q) D_2(C_{ty})(r, p, \\
& q) D_1(C_{ty})(r, p, q) -2 C_{ty}(r, p, q) D_1(C_{xx})(r, p, q) D_2(C_{ty})(r, p, q) +2 C_{ty}(r, p, \\
& q) D_2(C_{xx})(r, p, q) D_1(C_{ty})(r, p, q) -2 C_{tx}(r, p, q) D_1(C_{xx})(r, p, q) D_3(C_{ty})(r, p, q) \\
& +2 C_{tx}(r, p, q) D_3(C_{tt})(r, p, q) D_2(C_{xy})(r, p, q) -2 C_{tx}(r, p, q) D_3(C_{xx})(r, p, \\
& q) D_1(C_{ty})(r, p, q) -2 C_{tx}(r, p, q) D_2(C_{tt})(r, p, q) D_3(C_{xy})(r, p, q) +2 C_{tt}(r, p, \\
& q) D_3(C_{xx})(r, p, q) D_2(C_{ty})(r, p, q) +2 C_{tt}(r, p, q) D_2(C_{xx})(r, p, q) D_3(C_{ty})(r, p, q) \\
& +2 C_{xy}(r, p, q) D_1(C_{xx})(r, p, q) D_1(C_{ty})(r, p, q) -2 C_{xy}(r, p, q) D_3(C_{tt})(r, p, \\
& q) D_2(C_{tx})(r, p, q) +2 C_{xy}(r, p, q) D_2(C_{tt})(r, p, q) D_3(C_{tx})(r, p, q) +2 C_{xy}(r, p, \\
& q) D_2(C_{tt})(r, p, q) D_2(C_{ty})(r, p, q) +2 C_{xx}(r, p, q) D_1(C_{tt})(r, p, q) D_3(C_{xy})(r, p, q) \\
& -2 C_{xx}(r, p, q) D_3(C_{tt})(r, p, q) D_1(C_{xy})(r, p, q) -4 C_{ty}(r, p, q)^2 D_2(C_{xx})(r, p,
\end{aligned}$$

$$\begin{aligned}
& q) D_3(Cty)(r, p, q) - 4 Cxy(r, p, q)^2 D_2(Ctt)(r, p, q) D_3(Cty)(r, p, q) - Cty(r, p, \\
& q) D_2(Ctt)(r, p, q) D_3(Cxx)(r, p, q) + Cty(r, p, q) D_2(Cxx)(r, p, q) D_3(Ctt)(r, p, q) \\
& - 4 Ctx(r, p, q) D_2(Cty)(r, p, q) D_3(Ctx)(r, p, q) + 4 Ctx(r, p, q) D_2(Cxy)(r, p, \\
& q) D_1(Cty)(r, p, q) - 4 Cxy(r, p, q) D_2(Ctx)(r, p, q) D_1(Cty)(r, p, q) + 2 Cxx(r, p, \\
& q) Cxy(r, p, q) D_3(Ctt)(r, p, q) D_3(Cty)(r, p, q) + D_2(Ctt)(r, p, q) D_1(Cxx)(r, p, q) \\
& - 4 Ctx(r, p, q) D_2(Cty)(r, p, q)^2 - D_2(Cxx)(r, p, q) D_1(Ctt)(r, p, q) \Big), D_{3,3}(Cty)(r, p, \\
& q) = \frac{1}{4} \frac{1}{HessUniv} \Big( 8 Ctx(r, p, q) Cty(r, p, q) D_3(Cxy)(r, p, q) D_3(Cty)(r, p, q) \\
& - 8 Ctt(r, p, q) Cxy(r, p, q) D_3(Cxy)(r, p, q) D_3(Cty)(r, p, q) + 16 Cxy(r, p, q) Cty(r, p, \\
& q) D_3(Cty)(r, p, q) D_1(Cxy)(r, p, q) - 8 Cxy(r, p, q) Cty(r, p, q) D_3(Cxy)(r, p, \\
& q) D_1(Cty)(r, p, q) + 8 Cxy(r, p, q) Cty(r, p, q) D_2(Cty)(r, p, q) D_3(Cty)(r, p, q) \\
& + 8 Cxy(r, p, q) Ctx(r, p, q) D_3(Cty)(r, p, q)^2 - 8 Cxy(r, p, q)^2 D_3(Cty)(r, p, \\
& q) D_1(Cty)(r, p, q) - 4 Cty(r, p, q) D_1(Cxx)(r, p, q) D_3(Cty)(r, p, q) + 4 Cty(r, p, \\
& q) D_3(Ctt)(r, p, q) D_2(Cxy)(r, p, q) - 4 Cty(r, p, q) D_2(Cty)(r, p, q) D_1(Cxy)(r, p, q) \\
& - 4 Cty(r, p, q) D_2(Cty)(r, p, q) D_3(Ctx)(r, p, q) + 8 Cty(r, p, q) D_2(Ctx)(r, p, \\
& q) D_3(Cty)(r, p, q) - 4 Cty(r, p, q) D_2(Ctt)(r, p, q) D_3(Cxy)(r, p, q) + 8 Cty(r, p, \\
& q) D_2(Cxy)(r, p, q) D_1(Cty)(r, p, q) - 4 Ctx(r, p, q) D_3(Cty)(r, p, q) D_1(Cxy)(r, p, q) \\
& - 4 Ctx(r, p, q) D_3(Ctx)(r, p, q) D_3(Cty)(r, p, q) - 4 Ctx(r, p, q) D_2(Cty)(r, p, \\
& q) D_3(Cty)(r, p, q) + 4 Ctt(r, p, q) D_2(Cxy)(r, p, q) D_3(Cty)(r, p, q) + 4 Cxy(r, p,
\end{aligned}$$

$$\begin{aligned}
& q) D_1(Ctt)(r, p, q) D_3(Cxy)(r, p, q) - 4 Cxy(r, p, q) D_1(Cxy)(r, p, q) D_1(Cty)(r, p, q) \\
& + 4 Cxy(r, p, q) D_3(Ctx)(r, p, q) D_1(Cty)(r, p, q) - 4 Cxy(r, p, q) D_3(Ctt)(r, p, \\
& q) D_1(Cxy)(r, p, q) + 4 Cxy(r, p, q) D_2(Cty)(r, p, q) D_1(Cty)(r, p, q) - 4 Cxy(r, p, \\
& q) D_2(Ctt)(r, p, q) D_3(Cty)(r, p, q) - 8 Cxx(r, p, q) Cty(r, p, q) D_3(Cty)(r, p, q)^2 \\
& + 4 Cxx(r, p, q) D_3(Cty)(r, p, q) D_1(Cty)(r, p, q) + 2 Ctt(r, p, q) D_3(Cxx)(r, p, \\
& q) D_3(Cty)(r, p, q) + 2 Cxx(r, p, q) D_3(Ctt)(r, p, q) D_3(Cty)(r, p, q) + 8 Cty(r, p, \\
& q)^2 D_2(Cty)(r, p, q) D_3(Cxy)(r, p, q) - 16 Cty(r, p, q)^2 D_2(Cxy)(r, p, q) D_3(Cty)(r, p, q) \\
& + 2 D_2(Ctt)(r, p, q) D_1(Cxy)(r, p, q) + 2 D_2(Ctt)(r, p, q) D_3(Ctx)(r, p, q) \\
& + 2 D_2(Ctt)(r, p, q) D_2(Cty)(r, p, q) - 2 D_3(Ctt)(r, p, q) D_2(Ctx)(r, p, q) - D_3(Cxx)(r, \\
& p, q) D_1(Ctt)(r, p, q) - 4 D_2(Ctx)(r, p, q) D_1(Cty)(r, p, q) + 2 D_1(Cxx)(r, p, \\
& q) D_1(Cty)(r, p, q) - 4 Cty(r, p, q) D_2(Cty)(r, p, q)^2 - 2 D_1(Ctt)(r, p, q) D_2(Cxy)(r, p, \\
& q) + D_3(Ctt)(r, p, q) D_1(Cxx)(r, p, q) \Big), D_{1,1}(Cxy)(r, p, q) = -\frac{1}{4} \frac{1}{HessUniv} \Big( \\
& -4 Cty(r, p, q)^2 D_2(Ctt)(r, p, q) D_2(Cxy)(r, p, q) + 8 Cty(r, p, q)^2 D_2(Cxy)(r, p, \\
& q) D_1(Ctx)(r, p, q) - 4 Ctx(r, p, q)^2 D_3(Ctt)(r, p, q) D_3(Cxy)(r, p, q) + 8 Ctx(r, p, \\
& q)^2 D_3(Cxy)(r, p, q) D_1(Cty)(r, p, q) + 4 Ctt(r, p, q)^2 D_2(Cxy)(r, p, q) D_3(Cxy)(r, p, q) \\
& + 4 Ctt(r, p, q) Cxy(r, p, q) D_1(Cxy)(r, p, q)^2 + 4 Cxy(r, p, q)^2 D_1(Ctt)(r, p, \\
& q) D_1(Cxy)(r, p, q) + 8 Ctx(r, p, q) D_1(Cxy)(r, p, q) D_1(Ctx)(r, p, q) + Ctt(r, p, \\
& q) D_2(Ctt)(r, p, q) D_3(Cxx)(r, p, q) - 4 Ctt(r, p, q) D_2(Cxy)(r, p, q) D_1(Ctx)(r, p, q)
\end{aligned}$$

$$\begin{aligned}
& - Ctt(r, p, q) D_2(Cxx)(r, p, q) D_3(Ctt)(r, p, q) - 4 Cxx(r, p, q) D_1(Ctt)(r, p, \\
& q) D_1(Cxy)(r, p, q) - 2 Ctt(r, p, q)^2 D_3(Cxx)(r, p, q) D_3(Cxy)(r, p, q) - 2 Cty(r, p, \\
& q) D_2(Ctt)(r, p, q) D_1(Cxx)(r, p, q) + 2 Cty(r, p, q) D_2(Cxx)(r, p, q) D_1(Ctt)(r, p, q) \\
& + 2 Ctx(r, p, q) D_3(Ctt)(r, p, q) D_1(Cxx)(r, p, q) - 2 Ctx(r, p, q) D_3(Cxx)(r, p, \\
& q) D_1(Ctt)(r, p, q) - 2 Ctt(r, p, q) D_1(Cxx)(r, p, q) D_1(Cxy)(r, p, q) - 2 Ctt(r, p, \\
& q) D_1(Cxx)(r, p, q) D_3(Ctx)(r, p, q) + 2 Ctt(r, p, q) D_1(Cxx)(r, p, q) D_2(Cty)(r, p, q) \\
& + 2 Ctt(r, p, q) D_3(Cxx)(r, p, q) D_1(Ctx)(r, p, q) + 2 Ctt(r, p, q) D_2(Ctt)(r, p, \\
& q) D_2(Cxy)(r, p, q) - 2 Ctt(r, p, q) D_2(Cxx)(r, p, q) D_1(Cty)(r, p, q) - 8 Ctx(r, p, \\
& q) Cty(r, p, q) D_3(Cxy)(r, p, q) D_1(Ctx)(r, p, q) + 4 Ctx(r, p, q) Cty(r, p, q) D_2(Ctt)(r, \\
& p, q) D_3(Cxy)(r, p, q) - 8 Ctx(r, p, q) Cty(r, p, q) D_2(Cxy)(r, p, q) D_1(Cty)(r, p, q) \\
& + 4 Ctt(r, p, q) Cty(r, p, q) D_1(Cxx)(r, p, q) D_3(Cxy)(r, p, q) - 4 Ctt(r, p, q) Cty(r, p, \\
& q) D_2(Cxy)(r, p, q) D_1(Cxy)(r, p, q) - 4 Ctt(r, p, q) Cty(r, p, q) D_2(Cxy)(r, p, \\
& q) D_3(Ctx)(r, p, q) + 4 Ctt(r, p, q) Cty(r, p, q) D_2(Cxy)(r, p, q) D_2(Cty)(r, p, q) \\
& + 4 Ctx(r, p, q) Cty(r, p, q) D_3(Ctt)(r, p, q) D_2(Cxy)(r, p, q) - 4 Ctt(r, p, q) Ctx(r, p, \\
& q) D_3(Cxy)(r, p, q) D_1(Cxy)(r, p, q) + 4 Ctt(r, p, q) Ctx(r, p, q) D_3(Cxy)(r, p, \\
& q) D_3(Ctx)(r, p, q) - 4 Ctt(r, p, q) Ctx(r, p, q) D_2(Cty)(r, p, q) D_3(Cxy)(r, p, q) \\
& + 4 Ctt(r, p, q) Cxy(r, p, q) D_3(Ctx)(r, p, q) D_1(Cxy)(r, p, q) - 4 Ctt(r, p, q) Cxy(r, p, \\
& q) D_2(Cty)(r, p, q) D_1(Cxy)(r, p, q) - 4 Ctt(r, p, q) Cxy(r, p, q) D_2(Ctt)(r, p,
\end{aligned}$$

$$\begin{aligned}
& q) D_3(Cxy)(r, p, q) + 8 Ctt(r, p, q) Cxy(r, p, q) D_2(Cxy)(r, p, q) D_1(Cty)(r, p, q) \\
& - 4 Cxy(r, p, q) Cty(r, p, q) D_1(Ctt)(r, p, q) D_2(Cxy)(r, p, q) - 8 Cxy(r, p, q) Cty(r, p, \\
& q) D_1(Cxy)(r, p, q) D_1(Ctx)(r, p, q) + 4 Cxy(r, p, q) Cty(r, p, q) D_2(Ctt)(r, p, \\
& q) D_1(Cxy)(r, p, q) + 4 Cxy(r, p, q) Ctx(r, p, q) D_1(Ctt)(r, p, q) D_3(Cxy)(r, p, q) \\
& - 8 Cxy(r, p, q) Ctx(r, p, q) D_1(Cxy)(r, p, q) D_1(Cty)(r, p, q) - 4 Cxy(r, p, q) Ctx(r, p, \\
& q) D_3(Ctt)(r, p, q) D_1(Cxy)(r, p, q) + 8 Cxx(r, p, q) Cty(r, p, q) D_1(Cxy)(r, p, \\
& q) D_1(Cty)(r, p, q) - 4 Cxx(r, p, q) Ctt(r, p, q) D_3(Cxy)(r, p, q) D_1(Cty)(r, p, q) \\
& + 2 Cxx(r, p, q) Ctt(r, p, q) D_3(Ctt)(r, p, q) D_3(Cxy)(r, p, q) \Big), D_{1,2}(Cxy)(r, p, q) = \\
& - \frac{1}{4} \frac{1}{HessUniv} \Big( 4 Ctt(r, p, q) Cxy(r, p, q) D_2(Cxy)(r, p, q) D_2(Cty)(r, p, q) + 4 Cxx(r, \\
& p, q) Cty(r, p, q) D_2(Cty)(r, p, q) D_1(Cxy)(r, p, q) - 4 Cxx(r, p, q) Cty(r, p, \\
& q) D_3(Cxy)(r, p, q) D_1(Ctx)(r, p, q) + 4 Cxx(r, p, q) Ctx(r, p, q) D_3(Cxy)(r, p, \\
& q) D_1(Cty)(r, p, q) - 2 Ctt(r, p, q) Cty(r, p, q) D_3(Cxx)(r, p, q) D_2(Cxy)(r, p, q) \\
& + 2 Ctt(r, p, q) Cty(r, p, q) D_2(Cxx)(r, p, q) D_3(Cxy)(r, p, q) + 2 Cxx(r, p, q) Cty(r, p, \\
& q) D_3(Ctt)(r, p, q) D_2(Cxy)(r, p, q) + 2 Cxx(r, p, q) Cty(r, p, q) D_2(Ctt)(r, p, \\
& q) D_3(Cxy)(r, p, q) + 2 Ctx(r, p, q) D_1(Cxx)(r, p, q) D_1(Cxy)(r, p, q) + 2 Ctx(r, p, \\
& q) D_2(Ctt)(r, p, q) D_2(Cxy)(r, p, q) + 4 Cty(r, p, q)^2 D_1(Cxx)(r, p, q) D_2(Cxy)(r, p, q) \\
& + 4 Cxy(r, p, q)^2 D_2(Ctt)(r, p, q) D_1(Cxy)(r, p, q) + 4 Ctx(r, p, q) D_2(Ctx)(r, p, \\
& q) D_1(Cxy)(r, p, q) + 4 Cxx(r, p, q) Cty(r, p, q) D_1(Cxy)(r, p, q)^2 + 2 Ctx(r, p,
\end{aligned}$$

$$\begin{aligned}
& q) D_1(Cxx)(r, p, q) D_2(Cty)(r, p, q) - 2 Ctx(r, p, q) D_2(Cxx)(r, p, q) D_1(Cty)(r, p, q) \\
& - 2 Cty(r, p, q) D_1(Cxx)(r, p, q) D_2(Ctx)(r, p, q) + 2 Cty(r, p, q) D_2(Cxx)(r, p, \\
& q) D_1(Ctx)(r, p, q) - 2 Ctt(r, p, q) D_1(Cxx)(r, p, q) D_2(Cxy)(r, p, q) + 2 Ctt(r, p, \\
& q) D_3(Cxx)(r, p, q) D_2(Ctx)(r, p, q) - 2 Ctt(r, p, q) D_2(Cxx)(r, p, q) D_1(Cxy)(r, p, q) \\
& - 2 Ctt(r, p, q) D_2(Cxx)(r, p, q) D_3(Ctx)(r, p, q) + Cxx(r, p, q) D_3(Ctt)(r, p, \\
& q) D_1(Cxx)(r, p, q) - Cxx(r, p, q) D_3(Cxx)(r, p, q) D_1(Ctt)(r, p, q) - Cxy(r, p, \\
& q) D_2(Ctt)(r, p, q) D_1(Cxx)(r, p, q) + Cxy(r, p, q) D_2(Cxx)(r, p, q) D_1(Ctt)(r, p, q) \\
& - 2 Cxx(r, p, q) D_1(Ctt)(r, p, q) D_2(Cxy)(r, p, q) - 2 Cxx(r, p, q) D_2(Ctt)(r, p, \\
& q) D_1(Cxy)(r, p, q) - 8 Ctx(r, p, q) Cty(r, p, q) D_2(Cxy)(r, p, q) D_1(Cxy)(r, p, q) \\
& + 4 Ctt(r, p, q) Ctx(r, p, q) D_2(Cxy)(r, p, q) D_3(Cxy)(r, p, q) - 4 Ctt(r, p, q) Cxy(r, p, \\
& q) D_2(Ctx)(r, p, q) D_3(Cxy)(r, p, q) + 4 Ctt(r, p, q) Cxy(r, p, q) D_2(Cxy)(r, p, \\
& q) D_1(Cxy)(r, p, q) - 4 Cxy(r, p, q) Cty(r, p, q) D_1(Cxx)(r, p, q) D_1(Cxy)(r, p, q) \\
& - 4 Cxy(r, p, q) Cty(r, p, q) D_2(Ctt)(r, p, q) D_2(Cxy)(r, p, q) - 8 Cxy(r, p, q) Ctx(r, p, \\
& q) D_2(Cty)(r, p, q) D_1(Cxy)(r, p, q) - 4 Cxx(r, p, q) Ctt(r, p, q) D_3(Cxy)(r, p, \\
& q) D_1(Cxy)(r, p, q) + 4 Cxx(r, p, q) Ctt(r, p, q) D_3(Cxy)(r, p, q) D_3(Ctx)(r, p, q) \\
& - 4 Cxx(r, p, q) Ctt(r, p, q) D_2(Cty)(r, p, q) D_3(Cxy)(r, p, q) - 2 Ctt(r, p, q) Ctx(r, p, \\
& q) D_3(Cxx)(r, p, q) D_3(Cxy)(r, p, q) + 2 Ctt(r, p, q) Cxy(r, p, q) D_1(Cxx)(r, p, \\
& q) D_3(Cxy)(r, p, q) + 2 Ctt(r, p, q) Cxy(r, p, q) D_3(Cxx)(r, p, q) D_1(Cxy)(r, p, q)
\end{aligned}$$



$$\begin{aligned}
& -2 C_{xx}(r, p, q) C_{tx}(r, p, q) D_3(C_{tt})(r, p, q) D_3(C_{xy})(r, p, q) + 2 C_{xx}(r, p, q) C_{xy}(r, p, \\
& q) D_1(C_{tt})(r, p, q) D_3(C_{xy})(r, p, q) - 2 C_{xx}(r, p, q) C_{xy}(r, p, q) D_3(C_{tt})(r, p, \\
& q) D_1(C_{xy})(r, p, q) \Big), D_{1,3}(C_{xy})(r, p, q) = -\frac{1}{4} \frac{1}{HessUniv} \Big( 4 C_{xx}(r, p, q) C_{ty}(r, p, \\
& q) D_3(C_{ty})(r, p, q) D_1(C_{xy})(r, p, q) - 8 C_{tt}(r, p, q) C_{xy}(r, p, q) D_2(C_{ty})(r, p, \\
& q) D_3(C_{xy})(r, p, q) - 2 C_{ty}(r, p, q) D_1(C_{xx})(r, p, q) D_1(C_{xy})(r, p, q) - 2 C_{ty}(r, p, \\
& q) D_1(C_{xx})(r, p, q) D_3(C_{tx})(r, p, q) + 2 C_{ty}(r, p, q) D_3(C_{xx})(r, p, q) D_1(C_{tx})(r, p, q) \\
& - 2 C_{ty}(r, p, q) D_2(C_{tt})(r, p, q) D_2(C_{xy})(r, p, q) - 2 C_{xy}(r, p, q) D_1(C_{tt})(r, p, \\
& q) D_2(C_{xy})(r, p, q) + 2 C_{xy}(r, p, q) D_2(C_{tt})(r, p, q) D_1(C_{xy})(r, p, q) + 4 C_{ty}(r, p, \\
& q)^2 D_1(C_{xx})(r, p, q) D_3(C_{xy})(r, p, q) + 4 C_{xy}(r, p, q)^2 D_1(C_{tt})(r, p, q) D_3(C_{xy})(r, p, q) \\
& + 4 C_{ty}(r, p, q) D_2(C_{xy})(r, p, q) D_1(C_{tx})(r, p, q) + 4 C_{tx}(r, p, q) D_3(C_{tx})(r, p, \\
& q) D_1(C_{xy})(r, p, q) - 4 C_{tt}(r, p, q) D_2(C_{xy})(r, p, q) D_1(C_{xy})(r, p, q) - 4 C_{tt}(r, p, \\
& q) D_2(C_{xy})(r, p, q) D_3(C_{tx})(r, p, q) + 4 C_{tt}(r, p, q) D_2(C_{xy})(r, p, q) D_2(C_{ty})(r, p, q) \\
& + C_{xy}(r, p, q) D_3(C_{tt})(r, p, q) D_1(C_{xx})(r, p, q) - C_{xy}(r, p, q) D_3(C_{xx})(r, p, \\
& q) D_1(C_{tt})(r, p, q) + 2 C_{tx}(r, p, q) D_1(C_{xx})(r, p, q) D_3(C_{ty})(r, p, q) + 2 C_{tx}(r, p, \\
& q) D_3(C_{tt})(r, p, q) D_2(C_{xy})(r, p, q) - 2 C_{tx}(r, p, q) D_3(C_{xx})(r, p, q) D_1(C_{ty})(r, p, q) \\
& + 2 C_{tx}(r, p, q) D_2(C_{tt})(r, p, q) D_3(C_{xy})(r, p, q) + 2 C_{tt}(r, p, q) D_3(C_{xx})(r, p, \\
& q) D_2(C_{ty})(r, p, q) - 2 C_{tt}(r, p, q) D_2(C_{xx})(r, p, q) D_3(C_{ty})(r, p, q) - 2 C_{xx}(r, p, \\
& q) D_1(C_{tt})(r, p, q) D_3(C_{xy})(r, p, q) - 2 C_{xx}(r, p, q) D_3(C_{tt})(r, p, q) D_1(C_{xy})(r, p, q)
\end{aligned}$$

$$\begin{aligned}
& -4 Ctx(r, p, q) D_2(Cxy)(r, p, q) D_1(Cty)(r, p, q) - 2 Ctt(r, p, q) Cty(r, p, \\
& q) D_3(Cxx)(r, p, q) D_3(Cxy)(r, p, q) + 2 Cxx(r, p, q) Cty(r, p, q) D_3(Ctt)(r, p, \\
& q) D_3(Cxy)(r, p, q) - 8 Ctx(r, p, q) Cty(r, p, q) D_3(Cxy)(r, p, q) D_1(Cxy)(r, p, q) \\
& + 4 Ctt(r, p, q) Cty(r, p, q) D_2(Cxy)(r, p, q) D_3(Cxy)(r, p, q) + 4 Ctt(r, p, q) Cxy(r, p, \\
& q) D_3(Cxy)(r, p, q) D_1(Cxy)(r, p, q) + 4 Ctt(r, p, q) Cxy(r, p, q) D_3(Cxy)(r, p, \\
& q) D_3(Ctx)(r, p, q) + 4 Ctt(r, p, q) Cxy(r, p, q) D_2(Cxy)(r, p, q) D_3(Cty)(r, p, q) \\
& - 8 Cxy(r, p, q) Cty(r, p, q) D_3(Cxy)(r, p, q) D_1(Ctx)(r, p, q) - 8 Cxy(r, p, q) Ctx(r, p, \\
& q) D_3(Cty)(r, p, q) D_1(Cxy)(r, p, q) - 4 Cxy(r, p, q) Ctx(r, p, q) D_3(Ctt)(r, p, \\
& q) D_3(Cxy)(r, p, q) + 8 Cxy(r, p, q) Ctx(r, p, q) D_3(Cxy)(r, p, q) D_1(Cty)(r, p, q) \\
& - D_2(Ctt)(r, p, q) D_1(Cxx)(r, p, q) + 4 Ctx(r, p, q) D_1(Cxy)(r, p, q)^2 + D_2(Cxx)(r, p, \\
& q) D_1(Ctt)(r, p, q) \Big), D_{2,2}(Cxy)(r, p, q) = \frac{1}{4} \frac{1}{HessUniv} \Big( -8 Ctx(r, p, q) D_2(Cxy)(r, \\
& p, q) D_2(Ctx)(r, p, q) + 4 Ctx(r, p, q) D_2(Cxx)(r, p, q) D_3(Ctx)(r, p, q) + 4 Ctt(r, p, \\
& q) D_2(Cxx)(r, p, q) D_2(Cxy)(r, p, q) + 4 Cxy(r, p, q) D_1(Cxx)(r, p, q) D_2(Ctx)(r, p, q) \\
& - 4 Cxy(r, p, q) D_2(Cxx)(r, p, q) D_1(Ctx)(r, p, q) - 4 Cxx(r, p, q) Cxy(r, p, \\
& q) D_1(Cxy)(r, p, q)^2 + Cxx(r, p, q) D_2(Ctt)(r, p, q) D_3(Cxx)(r, p, q) + 4 Cxx(r, p, \\
& q) D_2(Cxy)(r, p, q) D_1(Ctx)(r, p, q) - Cxx(r, p, q) D_2(Cxx)(r, p, q) D_3(Ctt)(r, p, q) \\
& - 4 Cxx(r, p, q)^2 D_3(Cxy)(r, p, q) D_1(Cty)(r, p, q) + 2 Cxx(r, p, q) D_2(Cxx)(r, p, \\
& q) D_1(Cty)(r, p, q) + 2 Cxx(r, p, q)^2 D_3(Ctt)(r, p, q) D_3(Cxy)(r, p, q) - 4 Cty(r, p,
\end{aligned}$$

$$\begin{aligned}
& q)^2 D_2(Cxx)(r, p, q) D_2(Cxy)(r, p, q) + 8 Ctx(r, p, q) Cty(r, p, q) D_2(Cxy)(r, p, q)^2 \\
& + 4 Ctx(r, p, q)^2 D_3(Cxx)(r, p, q) D_3(Cxy)(r, p, q) - 8 Ctx(r, p, q)^2 D_2(Cxy)(r, p, \\
& q) D_3(Cxy)(r, p, q) - 8 Ctt(r, p, q) Cxy(r, p, q) D_2(Cxy)(r, p, q)^2 + 4 Cxy(r, p, \\
& q)^2 D_1(Cxx)(r, p, q) D_1(Cxy)(r, p, q) - 8 Cxy(r, p, q)^2 D_2(Ctx)(r, p, q) D_1(Cxy)(r, p, q) \\
& - 4 Ctx(r, p, q) D_3(Cxx)(r, p, q) D_2(Ctx)(r, p, q) - 2 Cxx(r, p, q) D_1(Cxx)(r, p, \\
& q) D_1(Cxy)(r, p, q) - 2 Cxx(r, p, q) D_1(Cxx)(r, p, q) D_3(Ctx)(r, p, q) - 2 Cxx(r, p, \\
& q) D_1(Cxx)(r, p, q) D_2(Cty)(r, p, q) + 2 Cxx(r, p, q) D_3(Cxx)(r, p, q) D_1(Ctx)(r, p, q) \\
& + 2 Cxx(r, p, q) D_2(Ctt)(r, p, q) D_2(Cxy)(r, p, q) + 4 Cxx(r, p, q) Ctx(r, p, \\
& q) D_2(Cty)(r, p, q) D_3(Cxy)(r, p, q) + 4 Cxx(r, p, q) Ctt(r, p, q) D_2(Cxy)(r, p, \\
& q) D_3(Cxy)(r, p, q) + 4 Cxx(r, p, q) Cxy(r, p, q) D_3(Ctx)(r, p, q) D_1(Cxy)(r, p, q) \\
& + 4 Cxx(r, p, q) Cxy(r, p, q) D_2(Cty)(r, p, q) D_1(Cxy)(r, p, q) - 4 Cxx(r, p, q) Cxy(r, p, \\
& q) D_2(Ctt)(r, p, q) D_3(Cxy)(r, p, q) + 4 Ctx(r, p, q) Cty(r, p, q) D_3(Cxx)(r, p, \\
& q) D_2(Cxy)(r, p, q) - 4 Ctx(r, p, q) Cty(r, p, q) D_2(Cxx)(r, p, q) D_3(Cxy)(r, p, q) \\
& - 4 Cxy(r, p, q) Cty(r, p, q) D_1(Cxx)(r, p, q) D_2(Cxy)(r, p, q) + 8 Cxy(r, p, q) Cty(r, p, \\
& q) D_2(Cxy)(r, p, q) D_2(Ctx)(r, p, q) + 4 Cxy(r, p, q) Cty(r, p, q) D_2(Cxx)(r, p, \\
& q) D_1(Cxy)(r, p, q) - 4 Cxy(r, p, q) Ctx(r, p, q) D_1(Cxx)(r, p, q) D_3(Cxy)(r, p, q) \\
& - 4 Cxy(r, p, q) Ctx(r, p, q) D_3(Cxx)(r, p, q) D_1(Cxy)(r, p, q) + 8 Cxy(r, p, q) Ctx(r, p, \\
& q) D_2(Ctx)(r, p, q) D_3(Cxy)(r, p, q) + 8 Cxy(r, p, q) Ctx(r, p, q) D_2(Cxy)(r, p,
\end{aligned}$$

$$\begin{aligned}
& q) D_1(Cxy)(r, p, q) - 2 Cxx(r, p, q) Ctt(r, p, q) D_3(Cxx)(r, p, q) D_3(Cxy)(r, p, q) \\
& + 4 Cxx(r, p, q) Cty(r, p, q) D_1(Cxx)(r, p, q) D_3(Cxy)(r, p, q) - 4 Cxx(r, p, q) Cty(r, p, \\
& q) D_2(Cxy)(r, p, q) D_1(Cxy)(r, p, q) - 4 Cxx(r, p, q) Cty(r, p, q) D_2(Cxy)(r, p, \\
& q) D_3(Ctx)(r, p, q) - 4 Cxx(r, p, q) Cty(r, p, q) D_2(Cxy)(r, p, q) D_2(Cty)(r, p, q) \\
& + 4 Cxx(r, p, q) Ctx(r, p, q) D_3(Cxy)(r, p, q) D_1(Cxy)(r, p, q) - 4 Cxx(r, p, q) Ctx(r, p, \\
& q) D_3(Cxy)(r, p, q) D_3(Ctx)(r, p, q) \Big), D_{2,3}(Cxy)(r, p, q) = -\frac{1}{4} \frac{1}{HessUniv} \Big( 2 Cxx(r, \\
& p, q) D_1(Cxx)(r, p, q) D_3(Cty)(r, p, q) - 2 Cxx(r, p, q) D_3(Cxx)(r, p, q) D_1(Cty)(r, p, q) \\
& + 4 Cty(r, p, q)^2 D_2(Cxx)(r, p, q) D_3(Cxy)(r, p, q) + 4 Cxy(r, p, q)^2 D_2(Ctt)(r, p, \\
& q) D_3(Cxy)(r, p, q) + 4 Ctx(r, p, q) D_2(Ctx)(r, p, q) D_3(Cxy)(r, p, q) - 4 Ctx(r, p, \\
& q) D_2(Cxy)(r, p, q) D_1(Cxy)(r, p, q) + 4 Ctx(r, p, q) D_2(Cxy)(r, p, q) D_2(Cty)(r, p, q) \\
& + 4 Cxy(r, p, q) D_2(Ctx)(r, p, q) D_1(Cxy)(r, p, q) - Cxy(r, p, q) D_2(Ctt)(r, p, \\
& q) D_3(Cxx)(r, p, q) + Cxy(r, p, q) D_2(Cxx)(r, p, q) D_3(Ctt)(r, p, q) - 4 Cxx(r, p, \\
& q) D_3(Cxy)(r, p, q) D_1(Ctx)(r, p, q) - 4 Cxx(r, p, q) D_2(Cxy)(r, p, q) D_1(Cty)(r, p, q) \\
& + 2 Cty(r, p, q) D_1(Cxx)(r, p, q) D_2(Cxy)(r, p, q) + 2 Cty(r, p, q) D_3(Cxx)(r, p, \\
& q) D_2(Ctx)(r, p, q) - 2 Cty(r, p, q) D_2(Cxx)(r, p, q) D_1(Cxy)(r, p, q) - 2 Cty(r, p, \\
& q) D_2(Cxx)(r, p, q) D_3(Ctx)(r, p, q) + 2 Ctx(r, p, q) D_1(Cxx)(r, p, q) D_3(Cxy)(r, p, q) \\
& + 2 Ctx(r, p, q) D_3(Cxx)(r, p, q) D_1(Cxy)(r, p, q) + 2 Ctx(r, p, q) D_3(Cxx)(r, p, \\
& q) D_2(Cty)(r, p, q) - 2 Ctx(r, p, q) D_2(Cxx)(r, p, q) D_3(Cty)(r, p, q) - 2 Ctt(r, p,
\end{aligned}$$

$$\begin{aligned}
& q) D_3(Cxx)(r, p, q) D_2(Cxy)(r, p, q) - 2 Ctt(r, p, q) D_2(Cxx)(r, p, q) D_3(Cxy)(r, p, q) \\
& - 2 Cxy(r, p, q) D_1(Cxx)(r, p, q) D_1(Cxy)(r, p, q) - 2 Cxy(r, p, q) D_2(Ctt)(r, p, \\
& q) D_2(Cxy)(r, p, q) - 2 D_1(Cxx)(r, p, q) D_2(Ctx)(r, p, q) + 2 D_2(Cxx)(r, p, \\
& q) D_1(Ctx)(r, p, q) + 4 Cxx(r, p, q) D_1(Cxy)(r, p, q)^2 + 4 Cxx(r, p, q) Cty(r, p, \\
& q) D_3(Cxy)(r, p, q) D_3(Ctx)(r, p, q) + 4 Cxx(r, p, q) Cty(r, p, q) D_2(Cxy)(r, p, \\
& q) D_3(Cty)(r, p, q) - 4 Cxx(r, p, q) Cxy(r, p, q) D_3(Cty)(r, p, q) D_1(Cxy)(r, p, q) \\
& + 8 Cxx(r, p, q) Cxy(r, p, q) D_3(Cxy)(r, p, q) D_1(Cty)(r, p, q) - 4 Ctx(r, p, q) Cty(r, p, \\
& q) D_3(Cxx)(r, p, q) D_3(Cxy)(r, p, q) + 4 Ctt(r, p, q) Cxy(r, p, q) D_2(Cxy)(r, p, \\
& q) D_3(Cxy)(r, p, q) - 2 Cxx(r, p, q) Cxy(r, p, q) D_3(Ctt)(r, p, q) D_3(Cxy)(r, p, q) \\
& + 2 Ctt(r, p, q) Cxy(r, p, q) D_3(Cxx)(r, p, q) D_3(Cxy)(r, p, q) - 8 Cxy(r, p, q) Cty(r, p, \\
& q) D_2(Ctx)(r, p, q) D_3(Cxy)(r, p, q) - 8 Cxy(r, p, q) Ctx(r, p, q) D_2(Cty)(r, p, \\
& q) D_3(Cxy)(r, p, q) - 4 Cxx(r, p, q) Cty(r, p, q) D_3(Cxy)(r, p, q) D_1(Cxy)(r, p, q) ), \\
& D_{3,3}(Cxy)(r, p, q) = -\frac{1}{4} \frac{1}{HessUniv} \left( -4 Cxx(r, p, q) D_3(Cxy)(r, p, q) D_1(Cty)(r, p, \right. \\
& q) + 8 Cty(r, p, q)^2 D_2(Cxy)(r, p, q) D_3(Cxy)(r, p, q) - 8 Ctx(r, p, q) Cty(r, p, \\
& q) D_3(Cxy)(r, p, q)^2 + 8 Ctt(r, p, q) Cxy(r, p, q) D_3(Cxy)(r, p, q)^2 - 8 Cxy(r, p, \\
& q)^2 D_3(Cty)(r, p, q) D_1(Cxy)(r, p, q) + 16 Cxy(r, p, q)^2 D_3(Cxy)(r, p, q) D_1(Cty)(r, p, q) \\
& + 4 Cty(r, p, q) D_1(Cxx)(r, p, q) D_3(Cxy)(r, p, q) + 4 Cty(r, p, q) D_3(Cxx)(r, p, \\
& q) D_2(Cty)(r, p, q) - 4 Cty(r, p, q) D_2(Cxy)(r, p, q) D_1(Cxy)(r, p, q) - 4 Cty(r, p, \\
& q) D_2(Cxy)(r, p, q) D_3(Ctx)(r, p, q) + 4 Cty(r, p, q) D_2(Cxy)(r, p, q) D_2(Cty)(r, p, q) \\
& - 4 Cty(r, p, q) D_2(Cxx)(r, p, q) D_3(Cty)(r, p, q) + 4 Ctx(r, p, q) D_3(Cxy)(r, p, \\
& q) D_1(Cxy)(r, p, q) + 4 Ctx(r, p, q) D_3(Cxy)(r, p, q) D_3(Ctx)(r, p, q) + 4 Ctx(r, p,
\end{aligned}$$

$$\begin{aligned}
& q) D_2(Cty)(r, p, q) D_3(Cxy)(r, p, q) - 4 Ctt(r, p, q) D_2(Cxy)(r, p, q) D_3(Cxy)(r, p, q) \\
& + 4 Cxy(r, p, q) D_1(Cxx)(r, p, q) D_3(Cty)(r, p, q) + 4 Cxy(r, p, q) D_3(Ctx)(r, p, \\
& q) D_1(Cxy)(r, p, q) - 8 Cxy(r, p, q) D_3(Cxy)(r, p, q) D_1(Ctx)(r, p, q) - 4 Cxy(r, p, \\
& q) D_3(Cxx)(r, p, q) D_1(Cty)(r, p, q) + 4 Cxy(r, p, q) D_2(Cty)(r, p, q) D_1(Cxy)(r, p, q) \\
& + 4 Cxy(r, p, q) D_2(Ctt)(r, p, q) D_3(Cxy)(r, p, q) - 8 Cxy(r, p, q) D_2(Cxy)(r, p, \\
& q) D_1(Cty)(r, p, q) - 2 Cxx(r, p, q) D_3(Ctt)(r, p, q) D_3(Cxy)(r, p, q) - 2 Ctt(r, p, \\
& q) D_3(Cxx)(r, p, q) D_3(Cxy)(r, p, q) + 4 Cxy(r, p, q) D_1(Cxy)(r, p, q)^2 - D_2(Ctt)(r, p, \\
& q) D_3(Cxx)(r, p, q) + 4 D_2(Cxy)(r, p, q) D_1(Ctx)(r, p, q) + D_2(Cxx)(r, p, q) D_3(Ctt)(r, \\
& p, q) - 2 D_1(Cxx)(r, p, q) D_1(Cxy)(r, p, q) - 2 D_1(Cxx)(r, p, q) D_3(Ctx)(r, p, q) \\
& - 2 D_1(Cxx)(r, p, q) D_2(Cty)(r, p, q) + 2 D_3(Cxx)(r, p, q) D_1(Ctx)(r, p, q) \\
& - 2 D_2(Ctt)(r, p, q) D_2(Cxy)(r, p, q) + 2 D_2(Cxx)(r, p, q) D_1(Cty)(r, p, q) - 8 Cxy(r, \\
& p, q) Cty(r, p, q) D_3(Cxy)(r, p, q) D_1(Cxy)(r, p, q) - 16 Cxy(r, p, q) Cty(r, p, \\
& q) D_2(Cty)(r, p, q) D_3(Cxy)(r, p, q) + 8 Cxy(r, p, q) Cty(r, p, q) D_2(Cxy)(r, p, \\
& q) D_3(Cty)(r, p, q) - 8 Cxy(r, p, q) Ctx(r, p, q) D_3(Cxy)(r, p, q) D_3(Cty)(r, p, q) \\
& + 8 Cxx(r, p, q) Cty(r, p, q) D_3(Cxy)(r, p, q) D_3(Cty)(r, p, q) ) ]
\end{aligned}$$

>  
>  
> ICsubs[30]

$$\begin{aligned}
D_{3,3}(Cxy)(r, p, q) = & -\frac{1}{4} \frac{1}{HessUniv} \left( -4 Cxx(r, p, q) D_3(Cxy)(r, p, q) D_1(Cty)(r, p, q) \right. \\
& + 8 Cty(r, p, q)^2 D_2(Cxy)(r, p, q) D_3(Cxy)(r, p, q) - 8 Ctx(r, p, q) Cty(r, p, \\
& q) D_3(Cxy)(r, p, q)^2 + 8 Ctt(r, p, q) Cxy(r, p, q) D_3(Cxy)(r, p, q)^2 - 8 Cxy(r, p, \\
& q)^2 D_3(Cty)(r, p, q) D_1(Cxy)(r, p, q) + 16 Cxy(r, p, q)^2 D_3(Cxy)(r, p, q) D_1(Cty)(r, p, q) \\
& + 4 Cty(r, p, q) D_1(Cxx)(r, p, q) D_3(Cxy)(r, p, q) + 4 Cty(r, p, q) D_3(Cxx)(r, p, \\
& q) D_2(Cty)(r, p, q) - 4 Cty(r, p, q) D_2(Cxy)(r, p, q) D_1(Cxy)(r, p, q) - 4 Cty(r, p, \\
& q) D_2(Cxy)(r, p, q) D_3(Ctx)(r, p, q) + 4 Cty(r, p, q) D_2(Cxy)(r, p, q) D_2(Cty)(r, p, q) \\
& - 4 Cty(r, p, q) D_2(Cxx)(r, p, q) D_3(Cty)(r, p, q) + 4 Ctx(r, p, q) D_3(Cxy)(r, p, \\
& q) D_1(Cxy)(r, p, q) + 4 Ctx(r, p, q) D_3(Cxy)(r, p, q) D_3(Ctx)(r, p, q) + 4 Ctx(r, p, \\
& q) D_2(Cty)(r, p, q) D_3(Cxy)(r, p, q) - 4 Ctt(r, p, q) D_2(Cxy)(r, p, q) D_3(Cxy)(r, p, q) \\
& + 4 Cxy(r, p, q) D_1(Cxx)(r, p, q) D_3(Cty)(r, p, q) + 4 Cxy(r, p, q) D_3(Ctx)(r, p, \\
& q) D_1(Cxy)(r, p, q) - 8 Cxy(r, p, q) D_3(Cxy)(r, p, q) D_1(Ctx)(r, p, q) - 4 Cxy(r, p, \\
& q) D_3(Cxx)(r, p, q) D_1(Cty)(r, p, q) + 4 Cxy(r, p, q) D_2(Cty)(r, p, q) D_1(Cxy)(r, p, q)
\end{aligned} \tag{2}$$
